# Supplementary material for: Hochschild cohomology rings for self-injective algebras of tree classes $E_7$ and $E_8$
Source: arXiv:1910.03043 ancillary file (2021-02-14)
Supplement: Supplementary file 1 [file e7-differentials.pdf]

## TREE CLASS $E_7$ : DIFFERENTIALS OF THE BIMODULE RESOLUTION

Since  $Q_i$  are direct sums, their elements can be concerned as column vectors, hence differentials can be described as matrixes (which are being multiplied by column vectors from the right). Now let us describe the matrixes of differentials componentwisely.

*Remark 1.* Numeration of lines and columns always starts with zero.

### Notation.

- (1) Denote by  $w_{i \rightarrow j}$  the way that starts in  $i$ th vertex and ends in  $j$ th.
- (2) For  $j$ th column of differential matrix let  $j_2$  be the aliquot of division of  $j$  by  $s$ .

### Description of the $d_0$

$d_0 : Q_1 \rightarrow Q_0$  – is an  $(7s \times 8s)$  matrix.

If  $0 \leq j < 2s$ , then

$$(d_0)_{ij} = \begin{cases} w_{7(j+m) \rightarrow 7(j+m)+1+3f(j_2,1)} \otimes e_{7j}, & i = j_s; \\ -e_{7(j+m)+1+3f(j_2,1)} \otimes w_{7j \rightarrow 7j+1+3f(j_2,1)}, & i = j + s + 2sf(j_2, 1); \\ 0, & \text{otherwise.} \end{cases}$$

If  $2s \leq j < 5s$ , then

$$(d_0)_{ij} = \begin{cases} w_{7(j+m)+j_2-1 \rightarrow 7(j+m)+j_2+2f(j_2,4)} \otimes e_{7j+j_2-1}, & i = j - s; \\ -e_{7(j+m)+j_2+2f(j_2,4)} \otimes w_{7j+j_2-1 \rightarrow 7j+j_2+2f(j_2,4)}, & i = j + 2sf(j_2, 4); \\ 0, & \text{otherwise.} \end{cases}$$

If  $5s \leq j < 7s$ , then

$$(d_0)_{ij} = \begin{cases} w_{7(j+m)+j_2-1 \rightarrow 7(j+m)+j_2} \otimes e_{7j+j_2-1}, & i = j - s; \\ -e_{7(j+m)+j_2} \otimes w_{7j+j_2-1 \rightarrow 7j+j_2}, & i = j; \\ 0, & \text{otherwise.} \end{cases}$$

If  $7s \leq j < 8s$ , then

$$(d_0)_{ij} = \begin{cases} -e_{7(j+m+1)} \otimes w_{7j+6 \rightarrow 7(j+1)}, & i = (j+1)_s; \\ w_{7(j+m)+6 \rightarrow 7(j+m+1)} \otimes e_{7j+6}, & i = j - s; \\ 0, & \text{otherwise.} \end{cases}$$

### Description of the $d_1$

$d_1 : Q_2 \rightarrow Q_1$  – is an  $(8s \times 7s)$  matrix.

If  $0 \leq j < s$ , then

$$(d_1)_{ij} = \begin{cases} w_{7(j+m)+1+j_1+2f(j_1,3) \rightarrow 7(j+m+1)-1} \otimes w_{7j \rightarrow 7j+j_1}, & \\ i = j + s(j_1 + 1 - f(j_1, 0)), & 0 \leq j_1 < 4; \\ -w_{7(j+m+1)-3+j_1 \rightarrow 7(j+m+1)-1} \otimes w_{7j \rightarrow 7j+j_1+3(1-f(j_1,0))}, & \\ i = j + s(j_1 + 4 - 3f(j_1, 0)), & 0 \leq j_1 < 3; \\ 0, & \text{otherwise.} \end{cases}$$

If  $s \leq j < 2s$ , then

$$(d_1)_{ij} = \begin{cases} w_{7(j+m+1)+1+j_1 \rightarrow 7(j+m+1)+2} \otimes w_{7j+1 \rightarrow 7(j+1)+j_1}, \\ \quad i = (j+1)_s + 2sf(j_1, 1), \quad 0 \leq j_1 < 2; \\ w_{7(j+m)+2+j_1+2f(j_1, 2, 3) \rightarrow 7(j+m+1)+2} \otimes w_{7j+1 \rightarrow 7j+1+j_1+2f(j_1, 3)}, \\ \quad i = j + s(1 + j_1 + 2f(j_1, 3)), \quad 0 \leq j_1 < 4; \\ 0, \quad \text{otherwise.} \end{cases}$$

If  $2s \leq j < 3s$ , then

$$(d_1)_{ij} = \begin{cases} w_{7(j+m+1)+1+j_1 \rightarrow 7(j+m+1)+3} \otimes w_{7j+2 \rightarrow 7(j+1)+j_1}, \\ \quad i = (j+1)_s + s(j_1 + 1 - f(j_1, 0)), \quad 0 \leq j_1 < 3; \\ w_{7(j+m)+3+j_1+2f(j_1, 1, 2) \rightarrow 7(j+m+1)+3} \otimes w_{7j+2 \rightarrow 7j+2+j_1+2f(j_1, 2)}, \\ \quad i = j + s(1 + j_1 + 2f(j_1, 2)), \quad 0 \leq j_1 < 3; \\ 0, \quad \text{otherwise.} \end{cases}$$

If  $3s \leq j < 4s$ , then

$$(d_1)_{ij} = \begin{cases} e_{7(j+m+1)+4} \otimes w_{7j+3 \rightarrow 7(j+1)}, \quad i = s + (j+1)_s; \\ w_{7(j+m)+6 \rightarrow 7(j+m+1)+4} \otimes e_{7j+3}, \quad i = j + s; \\ w_{7(j+m+1) \rightarrow 7(j+m+1)+4} \otimes w_{7j+3 \rightarrow 7j+6}, \quad i = j + 4s; \\ 0, \quad \text{otherwise.} \end{cases}$$

If  $4s \leq j < 5s$ , then

$$(d_1)_{ij} = \begin{cases} w_{7(j+m+1)+4+j_1 \rightarrow 7(j+m+1)+5} \otimes w_{7j+4 \rightarrow 7(j+1)+4f(j_1, 1)}, \\ \quad i = (j+1)_s + s(1 + 4f(j_1, 1)), \quad 0 \leq j_1 < 2; \\ w_{7(j+m)+5+j_1 \rightarrow 7(j+m+1)+5} \otimes w_{7j+4 \rightarrow 7j+4+j_1}, \quad i = j + s(j_1 + 1), \quad 0 \leq j_1 < 3; \\ 0, \quad \text{otherwise.} \end{cases}$$

If  $5s \leq j < 6s$ , then

$$(d_1)_{ij} = \begin{cases} e_{7(j+m+1)+1} \otimes w_{7j+5 \rightarrow 7(j+1)}, \quad i = (j+1)_s; \\ w_{7(j+m)+6 \rightarrow 7(j+m+1)+1} \otimes e_{7j+5}, \quad i = j + s; \\ w_{7(j+m+1) \rightarrow 7(j+m+1)+1} \otimes w_{7j+5 \rightarrow 7j+6}, \quad i = j + 2s; \\ 0, \quad \text{otherwise.} \end{cases}$$

If  $6s \leq j < 7s$ , then

$$(d_1)_{ij} = \begin{cases} w_{7(j+m+1)+1+j_1+2f(j_1, 3, 4) \rightarrow 7(j+m+2)} \otimes w_{7j+6 \rightarrow 7(j+1)+j_1+2f(j_1, 4)}, \\ \quad i = (j+1)_s + s(j_1 + f(j_1, 1, 4) + 2f(j_1, 4)), \quad 0 \leq j_1 < 5; \\ w_{7(j+m+1) \rightarrow 7(j+m+2)} \otimes e_{7j+6}, \quad i = j + s; \\ 0, \quad \text{otherwise.} \end{cases}$$

### Description of the $d_2$

$d_2 : Q_3 \rightarrow Q_2$  – is an  $(7s \times 9s)$  matrix.

If  $0 \leq j < s$ , then

$$(d_2)_{ij} = \begin{cases} w_{7(j+m-1)+6 \rightarrow 7(j+m)+2} \otimes e_{7j}, & i = j; \\ -e_{7(j+m)+2} \otimes w_{7j \rightarrow 7j+1}, & i = j + s; \\ w_{7(j+m)+1 \rightarrow 7(j+m)+2} \otimes w_{7j \rightarrow 7j+5}, & i = j + 5s; \\ 0, & \text{otherwise.} \end{cases}$$

If  $s \leq j < 2s$ , then

$$(d_2)_{ij} = \begin{cases} w_{7(j+m-1)+6 \rightarrow 7(j+m)+5} \otimes e_{7j}, & i = j_s; \\ -w_{7(j+m)+4 \rightarrow 7(j+m)+5} \otimes w_{7j \rightarrow 7j+3}, & i = j + 2s; \\ e_{7(j+m)+5} \otimes w_{7j \rightarrow 7j+4}, & i = j + 3s; \\ 0, & \text{otherwise.} \end{cases}$$

If  $2s \leq j < 3s$ , then

$$(d_2)_{ij} = \begin{cases} w_{7(j+m)+2 \rightarrow 7(j+m)+3} \otimes e_{7j+1}, & i = j - s; \\ -e_{7(j+m)+3} \otimes w_{7j+1 \rightarrow 7j+2}, & i = j; \\ 0, & \text{otherwise.} \end{cases}$$

If  $3s \leq j < 4s$ , then

$$(d_2)_{ij} = \begin{cases} -e_{7(j+m)+6} \otimes w_{7j+2 \rightarrow 7(j+1)}, & i = (j+1)_s; \\ w_{7(j+m)+3 \rightarrow 7(j+m)+6} \otimes e_{7j+2}, & i = j - s; \\ -w_{7(j+m)+4 \rightarrow 7(j+m)+6} \otimes w_{7j+2 \rightarrow 7j+3}, & i = j; \\ 0, & \text{otherwise.} \end{cases}$$

If  $4s \leq j < 6s$ , then

$$(d_2)_{ij} = \begin{cases} w_{7(j+m)+6 \rightarrow 7(j+m+1)-f(j_2,5)} \otimes w_{7j+j_2-1 \rightarrow 7(j+1)}, & i = (j+1)_s; \\ w_{7(j+m)+j_2 \rightarrow 7(j+m+1)-f(j_2,5)} \otimes e_{7j+j_2-1}, & i = j - s; \\ -w_{7(j+m+1)-6f(j_2,5) \rightarrow 7(j+m+1)-f(j_2,5)} \otimes w_{7j+j_2-1 \rightarrow 7j+10-j_2}, & i = j + 2sf(j_2,4); \\ 0, & \text{otherwise.} \end{cases}$$

If  $6s \leq j < 7s$ , then

$$(d_2)_{ij} = \begin{cases} w_{7(j+m)+1 \rightarrow 7(j+m+1)} \otimes e_{7j+5}, & i = j - s; \\ -e_{7(j+m+1)} \otimes w_{7j+5 \rightarrow 7j+6}, & i = j; \\ 0, & \text{otherwise.} \end{cases}$$

If  $7s \leq j < 8s$ , then

$$(d_2)_{ij} = \begin{cases} -w_{7(j+m)+6 \rightarrow 7(j+m+1)+1} \otimes w_{7j+6 \rightarrow 7(j+1)}, & i = (j+1)_s; \\ -e_{7(j+m+1)+1} \otimes w_{7j+6 \rightarrow 7(j+1)+5}, & i = 5s + (j+1)_s; \\ w_{7(j+m+1) \rightarrow 7(j+m+1)+1} \otimes e_{7j+6}, & i = j - s; \\ 0, & \text{otherwise.} \end{cases}$$

If  $8s \leq j < 9s$ , then

$$(d_2)_{ij} = \begin{cases} -e_{7(j+m+1)+4} \otimes w_{7j+6 \rightarrow 7(j+1)+3}, & i = 3s + (j+1)s; \\ w_{7(j+m+1) \rightarrow 7(j+m+1)+4} \otimes e_{7j+6}, & i = j - 2s; \\ 0, & \text{otherwise.} \end{cases}$$

### Description of the $d_3$

$d_3 : Q_4 \rightarrow Q_3$  - is an  $(9s \times 10s)$  matrix.

If  $0 \leq j < s$ , then

$$(d_3)_{ij} = \begin{cases} (1 - 2f(j_1, 1))w_{7(j+m)+2+3f(j_1,1)+f(j_1,2)+4f(j_1,3,4) \rightarrow 7(j+m)+6} \otimes w_{7j \rightarrow 7j+j_1-1+f(j_1,0)+f(j_1,4)}, \\ \quad i = j + s(j_1 + f(j_1, 4)), \quad 0 \leq j_1 < 5; \\ 0, & \text{otherwise.} \end{cases}$$

If  $s \leq j < 2s$ , then

$$(d_3)_{ij} = \begin{cases} (1 - 2f(j_1, 2, 3))w_{7(j+m+1)-2f(j_1,0)-f(j_1,2) \rightarrow 7(j+m+1)} \otimes w_{7j \rightarrow 7j+j_1+2-2f(j_1,0)}, \\ \quad i = j + s(j_1 + 2 - 2f(j_1, 0)), \quad 0 \leq j_1 < 4; \\ 0, & \text{otherwise.} \end{cases}$$

If  $2s \leq j < 3s$ , then

$$(d_3)_{ij} = \begin{cases} w_{7(j+m+1)+2+j_1 \rightarrow 7(j+m+1)+3} \otimes w_{7j+1 \rightarrow 7(j+1)+j_1}, & i = (j+1)s + 2sj_1, \quad 0 \leq j_1 < 2; \\ w_{7(j+m)+3+3j_1 \rightarrow 7(j+m+1)+3} \otimes w_{7j+1 \rightarrow 7j+1+j_1}, & i = j + sj_1, \quad 0 \leq j_1 < 2; \\ 0, & \text{otherwise.} \end{cases}$$

If  $3s \leq j < 4s$ , then

$$(d_3)_{ij} = \begin{cases} w_{7(j+m)+6+j_1 \rightarrow 7(j+m+1)+4} \otimes w_{7j+2 \rightarrow 7j+2+j_1}, & i = j + sj_1, \quad 0 \leq j_1 < 2; \\ e_{7(j+m+1)+4} \otimes w_{7j+2 \rightarrow 7j+6}, & i = j + 5s; \\ 0, & \text{otherwise.} \end{cases}$$

If  $4s \leq j < 5s$ , then

$$(d_3)_{ij} = \begin{cases} w_{7(j+m+1)+j_1 \rightarrow 7(j+m+1)+1} \otimes w_{7j+3 \rightarrow 7j+3+3j_1}, & i = j + 3j_1s, \quad 0 \leq j_1 < 2; \\ 0, & \text{otherwise.} \end{cases}$$

If  $5s \leq j < 6s$ , then

$$(d_3)_{ij} = \begin{cases} -e_{7(j+m+1)+5} \otimes w_{7j+3 \rightarrow 7(j+1)}, & i = s + (j+1)s; \\ w_{7(j+m+1) \rightarrow 7(j+m+1)+5} \otimes e_{7j+3}, & i = j - s; \\ w_{7(j+m+1)+4 \rightarrow 7(j+m+1)+5} \otimes w_{7j+3 \rightarrow 7j+6}, & i = j + 3s; \\ 0, & \text{otherwise.} \end{cases}$$

If  $6s \leq j < 7s$ , then

$$(d_3)_{ij} = \begin{cases} w_{7(j+m)+6+j_1 \rightarrow 7(j+m+1)+1} \otimes w_{7j+4 \rightarrow 7j+4+j_1}, & i = j + s(j_1 - 1), \quad 0 \leq j_1 < 3; \\ 0, & \text{otherwise.} \end{cases}$$

If  $7s \leq j < 8s$ , then

$$(d_3)_{ij} = \begin{cases} e_{7(j+m+1)+2} \otimes w_{7j+5 \rightarrow 7(j+1)}, & i = (j+1)_s; \\ w_{7(j+m+1) \rightarrow 7(j+m+1)+2} \otimes e_{7j+5}, & i = j - s; \\ w_{7(j+m+1)+1 \rightarrow 7(j+m+1)+2} \otimes w_{7j+5 \rightarrow 7j+6}, & i = j; \\ 0, & \text{otherwise.} \end{cases}$$

If  $8s \leq j < 9s$ , then

$$(d_3)_{ij} = \begin{cases} w_{7(j+m+1) \rightarrow 7(j+m+1)+4} \otimes e_{7j+5}, & i = j - 2s; \\ e_{7(j+m+1)+4} \otimes w_{7j+5 \rightarrow 7j+6}, & i = j; \\ 0, & \text{otherwise.} \end{cases}$$

If  $9s \leq j < 10s$ , then

$$(d_3)_{ij} = \begin{cases} w_{7(j+m+1)+2+j_1+2f(j_1,2) \rightarrow 7(j+m+1)+6} \otimes w_{7j+6 \rightarrow 7(j+1)+j_1}, & i = (j+1)_s + s(j_1 + f(j_1, 1, 2)), \ 0 \leq j_1 < 3; \\ w_{7(j+m+1)+1 \rightarrow 7(j+m+1)+6} \otimes e_{7j+6}, & i = j - 2s; \\ -w_{7(j+m+1)+4 \rightarrow 7(j+m+1)+6} \otimes e_{7j+6}, & i = j - s; \\ 0, & \text{otherwise.} \end{cases}$$

#### Description of the $d_4$

$d_4 : Q_5 \rightarrow Q_4$  - is an  $(10s \times 10s)$  matrix.

If  $0 \leq j < s$ , then

$$(d_4)_{ij} = \begin{cases} w_{7(j+m-1)+6+j_1 \rightarrow 7(j+m)+4} \otimes e_{7j}, & i = j + sj_1, \ 0 \leq j_1 < 2; \\ -e_{7(j+m)+4} \otimes w_{7j \rightarrow 7j+2}, & i = j + 3s; \\ e_{7(j+m)+4} \otimes w_{7j \rightarrow 7j+5}, & i = j + 8s; \\ 0, & \text{otherwise.} \end{cases}$$

If  $s \leq j < 2s$ , then

$$(d_4)_{ij} = \begin{cases} w_{7(j+m-1)+6 \rightarrow 7(j+m)+3} \otimes e_{7j}, & i = j_s; \\ -e_{7(j+m)+3} \otimes w_{7j \rightarrow 7j+1}, & i = j + s; \\ (-1)^{j_1+1} w_{7(j+m)+1+j_1 \rightarrow 7(j+m)+3} \otimes w_{7j \rightarrow 7j+4+j_1}, & i = j + (5+j_1)s, \ 0 \leq j_1 < 2; \\ 0, & \text{otherwise.} \end{cases}$$

If  $2s \leq j < 3s$ , then

$$(d_4)_{ij} = \begin{cases} (-1)^{j_1} w_{7(j+m)+f(j_1,1,2) \rightarrow 7(j+m)+1} \otimes w_{7j \rightarrow 7j+2+j_1-2f(j_1,0)}, & i = j + s(2j_1 - f(j_1, 0)), \ 0 \leq j_1 < 3; \\ 0, & \text{otherwise.} \end{cases}$$

If  $3s \leq j < 4s$ , then

$$(d_4)_{ij} = \begin{cases} -e_{7(j+m)+6} \otimes w_{7j+1 \rightarrow 7(j+1)}, & i = (j+1)_s; \\ (-1)^{j_1} w_{7(j+m)+3+j_1 \rightarrow 7(j+m)+6} \otimes w_{7j+1 \rightarrow 7j+1+j_1}, & i = j + s(j_1 - 1 + f(j_1, 2)), \ 0 \leq j_1 < 3; \\ 0, & \text{otherwise.} \end{cases}$$

If  $4s \leq j < 5s$ , then

$$(d_4)_{ij} = \begin{cases} -e_{7(j+m+1)} \otimes w_{7j+2 \rightarrow 7(j+1)}, & i = s + (j+1)_s; \\ (-1)^{j_1} w_{7(j+m)+4+j_1 \rightarrow 7(j+m+1)} \otimes w_{7j+2 \rightarrow 7j+2+j_1}, & i = j + s(2j_1 - 1), \ 0 \leq j_1 < 2; \\ 0, & \text{otherwise.} \end{cases}$$

If  $5s \leq j < 6s$ , then

$$(d_4)_{ij} = \begin{cases} e_{7(j+m)+6} \otimes w_{7j+3 \rightarrow 7(j+1)}, & i = (j+1)_s; \\ (2f(j_1, 0) - 1) w_{7(j+m)+4+j_1-3f(j_1, 0) \rightarrow 7(j+m)+6} \otimes w_{7j+3 \rightarrow 7j+3+3f(j_1, 2)}, \\ \quad i = j + s(j_1 - 1 + 3f(j_1, 2)), \ 0 \leq j_1 < 3; \\ 0, & \text{otherwise.} \end{cases}$$

If  $6s \leq j < 7s$ , then

$$(d_4)_{ij} = \begin{cases} w_{7(j+m)+6+j_1 \rightarrow 7(j+m+1)} \otimes w_{7j+4 \rightarrow 7(j+1)}, & i = (j+1)_s + sj_1, \ 0 \leq j_1 < 2; \\ (1 - 2f(j_1, 1)) w_{7(j+m)+1+j_1 \rightarrow 7(j+m+1)} \otimes w_{7j+4 \rightarrow 7j+4+j_1}, & i = j + sj_1, \ 0 \leq j_1 < 2; \\ 0, & \text{otherwise.} \end{cases}$$

If  $7s \leq j < 8s$ , then

$$(d_4)_{ij} = \begin{cases} w_{7(j+m)+2 \rightarrow 7(j+m)+6} \otimes e_{7j+5}, & i = j; \\ -w_{7(j+m)+4+2j_1 \rightarrow 7(j+m)+6} \otimes w_{7j+5 \rightarrow 7j+5+j_1}, & i = j + s(j_1 + 1), \ 0 \leq j_1 < 2; \\ 0, & \text{otherwise.} \end{cases}$$

If  $8s \leq j < 9s$ , then

$$(d_4)_{ij} = \begin{cases} (2f(j_1, 2) - 1) w_{7(j+m)+6+j_1 \rightarrow 7(j+m+1)+2} \otimes w_{7j+6 \rightarrow 7(j+1)+3f(j_1, 2)+5f(j_1, 3)}, \\ \quad i = (j+1)_s + s(j_1 + 2f(j_1, 2) + 4f(j_1, 3)), \ 0 \leq j_1 < 4; \\ w_{7(j+m)+6 \rightarrow 7(j+m+1)+2} \otimes e_{7j+6}, & i = j + s; \\ 0, & \text{otherwise.} \end{cases}$$

If  $9s \leq j < 10s$ , then

$$(d_4)_{ij} = \begin{cases} (-1)^{j_1+1} w_{7(j+m+1)+4+j_1 \rightarrow 7(j+m+1)+5} \otimes w_{7j+6 \rightarrow 7(j+1)+2+j_1}, \\ \quad i = (3 + 2j_1)s + (j+1)_s, \ 0 \leq j_1 < 2; \\ w_{7(j+m)+6 \rightarrow 7(j+m+1)+5} \otimes e_{7j+6}, & i = j; \\ 0, & \text{otherwise.} \end{cases}$$

### Description of the $d_5$

$d_5 : Q_6 \rightarrow Q_5$  - is an  $(10s \times 12s)$  matrix.

If  $0 \leq j < s$ , then

$$(d_5)_{ij} = \begin{cases} (2f(j_1, 0) - 1) w_{7(j+m)+4-j_1-f(j_1, 2) \rightarrow 7(j+m)+6} \otimes e_{7j}, & i = j + j_1s, \ 0 \leq j_1 < 3; \\ (2f(j_1, 2) - 1) e_{7(j+m)+6} \otimes w_{7j \rightarrow 7j+1+2j_1}, & i = j + (3 + 2j_1)s, \ 0 \leq j_1 < 3; \\ 0, & \text{otherwise.} \end{cases}$$

If  $s \leq j < 2s$ , then

$$(d_5)_{ij} = \begin{cases} w_{7(j+m)+3 \rightarrow 7(j+m+1)} \otimes e_{7j}, & i = j; \\ w_{7(j+m)+6+f(j_1,1,2) \rightarrow 7(j+m+1)} \otimes w_{7j \rightarrow 7j+1+j_1+f(j_1,2)}, \\ \quad i = j + (2 + j_1 + f(j_1,2))s, & 0 \leq j_1 < 3; \\ 0, & \text{otherwise.} \end{cases}$$

If  $2s \leq j < 3s$ , then

$$(d_5)_{ij} = \begin{cases} e_{7(j+m+1)+4} \otimes w_{7j+1 \rightarrow 7(j+1)}, & i = (j+1)s; \\ w_{7(j+m)+6+j_1 \rightarrow 7(j+m+1)+4} \otimes w_{7j+1 \rightarrow 7j+1+j_1}, & i = j + s(j_1+1), \ 0 \leq j_1 < 2; \\ 0, & \text{otherwise.} \end{cases}$$

If  $3s \leq j < 4s$ , then

$$(d_5)_{ij} = \begin{cases} e_{7(j+m+1)+1} \otimes w_{7j+2 \rightarrow 7(j+1)}, & i = 2s + (j+1)s; \\ w_{7(j+m+1) \rightarrow 7(j+m+1)+1} \otimes e_{7j+2}, & i = j + s; \\ 0, & \text{otherwise.} \end{cases}$$

If  $4s \leq j < 5s$ , then

$$(d_5)_{ij} = \begin{cases} w_{7(j+m+1)+4 \rightarrow 7(j+m+1)+5} \otimes w_{7j+2 \rightarrow 7(j+1)}, & i = (j+1)s; \\ (2f(j_1,0) - 1)w_{7(j+m+1)+f(j_1,2)-j_1 \rightarrow 7(j+m+1)+5} \otimes w_{7j+2 \rightarrow 7j+2+j_1+2f(j_1,2)}, \\ \quad i = j + s(j_1 + 3f(j_1,2)), & 0 \leq j_1 < 3; \\ 0, & \text{otherwise.} \end{cases}$$

If  $5s \leq j < 6s$ , then

$$(d_5)_{ij} = \begin{cases} w_{7(j+m+1)+1 \rightarrow 7(j+m+1)+2} \otimes w_{7j+3 \rightarrow 7(j+1)}, & i = 2s + (j+1)s; \\ w_{7(j+m)+6+3j_1 \rightarrow 7(j+m+1)+2} \otimes w_{7j+3 \rightarrow 7j+3+3j_1}, & i = j + 3sj_1, \ 0 \leq j_1 < 2; \\ 0, & \text{otherwise.} \end{cases}$$

If  $6s \leq j < 7s$ , then

$$(d_5)_{ij} = \begin{cases} w_{7(j+m+1)-j_1+4f(j_1,2) \rightarrow 7(j+m+1)+2} \otimes w_{7j+4 \rightarrow 7j+4+j_1}, & i = j + sj_1, \ 0 \leq j_1 < 3; \\ 0, & \text{otherwise.} \end{cases}$$

If  $7s \leq j < 8s$ , then

$$(d_5)_{ij} = \begin{cases} -e_{7(j+m+1)+4} \otimes w_{7j+4 \rightarrow 7(j+1)}, & i = (j+1)s; \\ w_{7(j+m+1) \rightarrow 7(j+m+1)+4} \otimes e_{7j+4}, & i = j - s; \\ 0, & \text{otherwise.} \end{cases}$$

If  $8s \leq j < 9s$ , then

$$(d_5)_{ij} = \begin{cases} w_{7(j+m+1)+3-2j_1 \rightarrow 7(j+m+1)+3} \otimes w_{7j+5 \rightarrow 7(j+1)}, & i = s(j_1+1) + (j+1)s, \ 0 \leq j_1 < 2; \\ w_{7(j+m)+6+3j_1 \rightarrow 7(j+m+1)+3} \otimes w_{7j+5 \rightarrow 7j+5+j_1}, & i = j + (j_1-1)s, \ 0 \leq j_1 < 2; \\ 0, & \text{otherwise.} \end{cases}$$

If  $9s \leq j < 10s$ , then

$$(d_5)_{ij} = \begin{cases} w_{7(j+m)+6 \rightarrow 7(j+m+1)+5} \otimes e_{7j+5}, & i = j - 2s; \\ e_{7(j+m+1)+5} \otimes w_{7j+5 \rightarrow 7j+6}, & i = j; \\ 0, & \text{otherwise.} \end{cases}$$

If  $10s \leq j < 11s$ , then

$$(d_5)_{ij} = \begin{cases} w_{7(j+m+1+f(j_1,2))+3-2j_1 \rightarrow 7(j+m+1)+6} \otimes w_{7j+6 \rightarrow 7(j+1)+f(j_1,2)}, \\ \quad i = s(j_1 + 1) + (j + 1)_s, \quad 0 \leq j_1 < 3; \\ (-1)^{j_1} w_{7(j+m+1)+2+3j_1 \rightarrow 7(j+m+1)+6} \otimes e_{7j+6}, & i = j + s(j_1 - 2), \quad 0 \leq j_1 < 2; \\ 0, & \text{otherwise.} \end{cases}$$

If  $11s \leq j < 12s$ , then

$$(d_5)_{ij} = \begin{cases} e_{7(j+m+2)} \otimes w_{7j+6 \rightarrow 7(j+1)+2}, & i = 4s + (j + 1)_s; \\ w_{7(j+m+1)+5 \rightarrow 7(j+m+2)} \otimes e_{7j+6}, & i = j - 2s; \\ 0, & \text{otherwise.} \end{cases}$$

### Description of the $d_6$

$d_6 : Q_7 \rightarrow Q_6$  - is an  $(12s \times 12s)$  matrix.

If  $0 \leq j < s$ , then

$$(d_6)_{ij} = \begin{cases} w_{7(j+m-1)+6 \rightarrow 7(j+m)+2} \otimes e_{7j}, & i = j; \\ w_{7(j+m) \rightarrow 7(j+m)+2} \otimes e_{7j}, & i = j + s; \\ (-1)^{j_1+1} w_{7(j+m)+2-f(j_1,0) \rightarrow 7(j+m)+2} \otimes w_{7j \rightarrow 7j+2+j_1}, \\ \quad i = j + s(j_1 + 4 - f(j_1, 0)), \quad 0 \leq j_1 < 3; \\ 0, & \text{otherwise.} \end{cases}$$

If  $s \leq j < 2s$ , then

$$(d_6)_{ij} = \begin{cases} w_{7(j+m-1)+6 \rightarrow 7(j+m)+5} \otimes e_{7j}, & i = j_s; \\ (2f(j_1, 0) - 1) w_{7(j+m)+5-f(j_1,0) \rightarrow 7(j+m)+5} \otimes w_{7j \rightarrow 7j+1+j_1+2f(j_1,2)}, \\ \quad i = j + s(1 + 2j_1 + 3f(j_1, 2)), \quad 0 \leq j_1 < 3; \\ 0, & \text{otherwise.} \end{cases}$$

If  $2s \leq j < 3s$ , then

$$(d_6)_{ij} = \begin{cases} (2f(j_1, 0) - 1) w_{7(j+m)+4(1-f(j_1,0)) \rightarrow 7(j+m)+4} \otimes w_{7j \rightarrow 7j+j_1+2f(j_1,2)}, \\ \quad i = j + s(j_1 - 1 + 4f(j_1, 2)), \quad 0 \leq j_1 < 3; \\ 0, & \text{otherwise.} \end{cases}$$

If  $3s \leq j < 4s$ , then

$$(d_6)_{ij} = \begin{cases} -w_{7(j+m)+6+j_1 \rightarrow 7(j+m+1)} \otimes w_{7j+1 \rightarrow 7(j+1)}, & i = (j + 1)_s + sj_1, \quad 0 \leq j_1 < 2; \\ (-1)^{j_1} w_{7(j+m)+4-3j_1 \rightarrow 7(j+m+1)} \otimes w_{7j+1 \rightarrow 7j+1+j_1}, & i = j + s(j_1 - 1), \quad 0 \leq j_1 < 2; \\ 0, & \text{otherwise.} \end{cases}$$



If  $4s \leq j < 5s$ , then

$$(d_6)_{ij} = \begin{cases} e_{7(j+m)+6} \otimes w_{7j+2 \rightarrow 7(j+1)}, & i = (j+1)_s; \\ w_{7(j+m)+1 \rightarrow 7(j+m)+6} \otimes e_{7j+2}, & i = j-s; \\ (2f(j_1, 2) - 1)w_{7(j+m)+5-3f(j_1, 1)+f(j_1, 2) \rightarrow 7(j+m)+6} \otimes w_{7j+2 \rightarrow 7j+2+j_1+2f(j_1, 2)}, \\ \quad i = j + s(j_1 + 4f(j_1, 2)), & 0 \leq j_1 < 3; \\ 0, & \text{otherwise.} \end{cases}$$

If  $5s \leq j < 6s$ , then

$$(d_6)_{ij} = \begin{cases} e_{7(j+m+1)} \otimes w_{7j+3 \rightarrow 7(j+1)}, & i = s + (j+1)_s; \\ (2f(j_1, 0) - 1)w_{7(j+m)+5+j_1-3f(j_1, 0) \rightarrow 7(j+m+1)} \otimes w_{7j+3 \rightarrow 7j+6-3f(j_1, 0)}, \\ \quad i = j + s(j_1 + 4 - 4f(j_1, 0)), & 0 \leq j_1 < 3; \\ 0, & \text{otherwise.} \end{cases}$$

If  $6s \leq j < 7s$ , then

$$(d_6)_{ij} = \begin{cases} -e_{7(j+m)+6} \otimes w_{7j+4 \rightarrow 7(j+1)}, & i = (j+1)_s; \\ (2f(j_1, 0) - 1)w_{7(j+m)+2+2j_1-3f(j_1, 2) \rightarrow 7(j+m)+6} \otimes w_{7j+4 \rightarrow 7j+4+f(j_1, 2)}, \\ \quad i = j + sj_1, & 0 \leq j_1 < 3; \\ 0, & \text{otherwise.} \end{cases}$$

If  $7s \leq j < 8s$ , then

$$(d_6)_{ij} = \begin{cases} (2f(j_1, 0) - 1)w_{7(j+m)+4+j_1-f(j_1, 0) \rightarrow 7(j+m)+6} \otimes w_{7j+5 \rightarrow 7j+5+f(j_1, 2)}, \\ \quad i = j + s(j_1 + 1), & 0 \leq j_1 < 3; \\ 0, & \text{otherwise.} \end{cases}$$

If  $8s \leq j < 9s$ , then

$$(d_6)_{ij} = \begin{cases} (-1)^{j_1} w_{7(j+m)+5+2j_1 \rightarrow 7(j+m+1)} \otimes w_{7j+5 \rightarrow 7j+5+j_1}, & i = j + s(2j_1 + 1), & 0 \leq j_1 < 2; \\ 0, & \text{otherwise.} \end{cases}$$

If  $9s \leq j < 10s$ , then

$$(d_6)_{ij} = \begin{cases} -e_{7(j+m+1)+4} \otimes w_{7j+6 \rightarrow 7(j+1)+1}, & i = 2s + (j+1)_s; \\ w_{7(j+m)+6+j_1 \rightarrow 7(j+m+1)+4} \otimes e_{7j+6}, & i = j + s(j_1 + 1), & 0 \leq j_1 < 2; \\ 0, & \text{otherwise.} \end{cases}$$

If  $10s \leq j < 11s$ , then

$$(d_6)_{ij} = \begin{cases} (1 - 2f(j_1, 2))w_{7(j+m)+6+3j_1-2f(j_1, 2) \rightarrow 7(j+m+1)+3} \otimes w_{7j+6 \rightarrow 7(j+1)+3j_1-f(j_1, 2)}, \\ \quad i = (j+1)_s + s(5j_1 - 2f(j_1, 2)), & 0 \leq j_1 < 3; \\ w_{7(j+m)+6 \rightarrow 7(j+m+1)+3} \otimes e_{7j+6}, & i = j; \\ 0, & \text{otherwise.} \end{cases}$$

If  $11s \leq j < 12s$ , then

$$(d_6)_{ij} = \begin{cases} -e_{7(j+m+1)+1} \otimes w_{7j+6 \rightarrow 7(j+1)+2}, & i = 3s + (j+1)_s; \\ w_{7(j+m+1) \rightarrow 7(j+m+1)+1} \otimes e_{7j+6}, & i = j; \\ 0, & \text{otherwise.} \end{cases}$$

### Description of the $d_7$

$d_7 : Q_8 \rightarrow Q_7$  – is an  $(12s \times 13s)$  matrix.

If  $0 \leq j < s$ , then

$$(d_7)_{ij} = \begin{cases} (1 - 2f(j_1, 1, 2))w_{7(j+m)+2+j_1+2f(j_1,1)+f(j_1,3)-f(j_1,5) \rightarrow 7(j+m)+6} \otimes \\ \quad w_{7j \rightarrow 7j+2f(j_1,3)+4f(j_1,4)+5f(j_1,5)}, \\ \quad i = j + s(j_1 + f(j_1, 3) + 2f(j_1, 4, 5)), \quad 0 \leq j_1 < 6; \\ 0, \quad \text{otherwise.} \end{cases}$$

If  $s \leq j < 2s$ , then

$$(d_7)_{ij} = \begin{cases} (1 - 2f(j_1, 1, 3))w_{7(j+m+1)-2f(j_1,0)-f(j_1,2) \rightarrow 7(j+m+1)} \otimes w_{7j \rightarrow 7j+j_1+f(j_1,4)}, \\ \quad i = j + s(1 + j_1 - f(j_1, 0) + 2f(j_1, 4)), \quad 0 \leq j_1 < 5; \\ 0, \quad \text{otherwise.} \end{cases}$$

If  $2s \leq j < 3s$ , then

$$(d_7)_{ij} = \begin{cases} w_{7(j+m+1)-f(j_1,1)+f(j_1,3) \rightarrow 7(j+m+1)+1} \otimes w_{7j+1 \rightarrow 7j+1+j_1+2f(j_1,3)}, \\ \quad i = j + s(1 + j_1 + 5f(j_1, 3)), \quad 0 \leq j_1 < 4; \\ 0, \quad \text{otherwise.} \end{cases}$$

If  $3s \leq j < 4s$ , then

$$(d_7)_{ij} = \begin{cases} w_{7(j+m+1)+5-j_1 \rightarrow 7(j+m+1)+5} \otimes w_{7j+1 \rightarrow 7(j+1)}, & i = s(j_1 + 1) + (j + 1)_s, \quad 0 \leq j_1 < 2; \\ w_{7(j+m+1) \rightarrow 7(j+m+1)+5} \otimes e_{7j+1}, & i = j; \\ 0, & \text{otherwise.} \end{cases}$$

If  $4s \leq j < 5s$ , then

$$(d_7)_{ij} = \begin{cases} -e_{7(j+m+1)+2} \otimes w_{7j+2 \rightarrow 7(j+1)}, & i = (j + 1)_s; \\ w_{7(j+m)+6+j_1 \rightarrow 7(j+m+1)+2} \otimes w_{7j+2 \rightarrow 7j+2+j_1+2f(j_1,2)}, \\ \quad i = j + s(j_1 + 5f(j_1, 2)), \quad 0 \leq j_1 < 3; \\ 0, & \text{otherwise.} \end{cases}$$

If  $5s \leq j < 6s$ , then

$$(d_7)_{ij} = \begin{cases} -w_{7(j+m+1)+2 \rightarrow 7(j+m+1)+3} \otimes w_{7j+3 \rightarrow 7(j+1)}, & i = (j + 1)_s; \\ w_{7(j+m+1)+3j_1-5f(j_1,2) \rightarrow 7(j+m+1)+3} \otimes w_{7j+3 \rightarrow 7j+6-3f(j_1,0)}, \\ \quad i = j + s(4 + j_1 - 4f(j_1, 0)), \quad 0 \leq j_1 < 3; \\ 0, & \text{otherwise.} \end{cases}$$

If  $6s \leq j < 7s$ , then

$$(d_7)_{ij} = \begin{cases} -e_{7(j+m+1)+4} \otimes w_{7j+3 \rightarrow 7(j+1)}, & i = 2s + (j + 1)_s; \\ w_{7(j+m+1)+4j_1 \rightarrow 7(j+m+1)+4} \otimes w_{7j+3 \rightarrow 7j+3+3j_1}, & i = j + s(4j_1 - 1), \quad 0 \leq j_1 < 2; \\ 0, & \text{otherwise.} \end{cases}$$

If  $7s \leq j < 8s$ , then

$$(d_7)_{ij} = \begin{cases} w_{7(j+m)+6+4f(j_1,2) \rightarrow 7(j+m+1)+3} \otimes w_{7j+4 \rightarrow 7j+4+j_1}, \\ \quad i = j + s(j_1 - 1 + 2f(j_1, 2)), \quad 0 \leq j_1 < 3; \\ 0, \quad \text{otherwise.} \end{cases}$$

If  $8s \leq j < 9s$ , then

$$(d_7)_{ij} = \begin{cases} e_{7(j+m+1)+5} \otimes w_{7j+4 \rightarrow 7(j+1)}, \quad i = s + (j + 1)_s; \\ w_{7(j+m)+6 \rightarrow 7(j+m+1)+5} \otimes e_{7j+4}, \quad i = j - 2s; \\ 0, \quad \text{otherwise.} \end{cases}$$

If  $9s \leq j < 10s$ , then

$$(d_7)_{ij} = \begin{cases} w_{7(j+m)+6+j_1+3f(j_1,2) \rightarrow 7(j+m+1)+4} \otimes w_{7j+5 \rightarrow 7j+5+f(j_1,2)}, \\ \quad i = j + s(j_1 - 2), \quad 0 \leq j_1 < 3; \\ 0, \quad \text{otherwise.} \end{cases}$$

If  $10s \leq j < 11s$ , then

$$(d_7)_{ij} = \begin{cases} w_{7(j+m+1)+j_1 \rightarrow 7(j+m+1)+1} \otimes w_{7j+5 \rightarrow 7j+5+j_1}, \quad i = j + s(3j_1 - 2), \quad 0 \leq j_1 < 2; \\ 0, \quad \text{otherwise.} \end{cases}$$

If  $11s \leq j < 12s$ , then

$$(d_7)_{ij} = \begin{cases} (-1)^{j_1} w_{7(j+m+1)+2+2j_1 \rightarrow 7(j+m+1)+6} \otimes w_{7j+6 \rightarrow 7(j+1)+4f(j_1,2)}, \\ \quad i = (j + 1)_s + 2s(j_1 + f(j_1, 2)), \quad 0 \leq j_1 < 3; \\ (2f(j_1, 0) - 1) w_{7(j+m+1)+4-j_1-f(j_1,2) \rightarrow 7(j+m+1)+6} \otimes e_{7j+6}, \\ \quad i = j + s(j_1 - 2), \quad 0 \leq j_1 < 3; \\ 0, \quad \text{otherwise.} \end{cases}$$

If  $12s \leq j < 13s$ , then

$$(d_7)_{ij} = \begin{cases} (2f(j_1, 1, 2) - 1) w_{7(j+m+1)+2+2j_1+f(j_1,2)-2f(j_1,3) \rightarrow 7(j+m+2)} \otimes w_{7j+6 \rightarrow 7(j+1)+f(j_1,2)+4f(j_1,3)}, \\ \quad i = (j + 1)_s + s(1 + j_1 - f(j_1, 0) + 2f(j_1, 3)), \quad 0 \leq j_1 < 4; \\ w_{7(j+m+1)+3 \rightarrow 7(j+m+2)} \otimes e_{7j+6}, \quad i = j - 2s; \\ 0, \quad \text{otherwise.} \end{cases}$$

### Description of the $d_8$

$d_8 : Q_9 \rightarrow Q_8$  - is an  $(13s \times 12s)$  matrix.

If  $0 \leq j < s$ , then

$$(d_8)_{ij} = \begin{cases} w_{7(j+m-1)+6+j_1 \rightarrow 7(j+m)+5} \otimes e_{7j}, \quad i = j + sj_1, \quad 0 \leq j_1 < 2; \\ (1 - 2f(j_1, 2, 3)) w_{7(j+m)+4+f(j_1,0)+f(j_1,2) \rightarrow 7(j+m)+5} \otimes w_{7j \rightarrow 7j+2+j_1-f(j_1,0)}, \\ \quad i = j + s(3 + 3j_1 - f(j_1, 2) - 3f(j_1, 3)), \quad 0 \leq j_1 < 4; \\ 0, \quad \text{otherwise.} \end{cases}$$

If  $s \leq j < 2s$ , then

$$(d_8)_{ij} = \begin{cases} w_{7(j+m-1)+6 \rightarrow 7(j+m)+3} \otimes e_{7j}, & i = js; \\ (-1)^{j_1+1} w_{7(j+m)+3-f(j_1,0) \rightarrow 7(j+m)+3} \otimes w_{7j \rightarrow 7j+2+j_1}, \\ \quad i = j + s(3 + j_1 + f(j_1, 2)), & 0 \leq j_1 < 3; \\ 0, & \text{otherwise.} \end{cases}$$

If  $2s \leq j < 3s$ , then

$$(d_8)_{ij} = \begin{cases} (1 - 2f(j_1, 2)) w_{7(j+m)+1-f(j_1,0) \rightarrow 7(j+m)+1} \otimes w_{7j \rightarrow 7j+j_1+3f(j_1,2)}, \\ \quad i = j + s(j_1 - 1 + 7f(j_1, 2)), & 0 \leq j_1 < 3; \\ 0, & \text{otherwise.} \end{cases}$$

If  $3s \leq j < 4s$ , then

$$(d_8)_{ij} = \begin{cases} -e_{7(j+m)+6} \otimes w_{7j+1 \rightarrow 7(j+1)}, & i = (j+1)_s; \\ (2f(j_1, 0) - 1) w_{7(j+m)+1+4f(j_1,1)+f(j_1,2) \rightarrow 7(j+m)+6} \otimes w_{7j+1 \rightarrow 7j+1+f(j_1,2)}, \\ \quad i = j + s(j_1 - 1), & 0 \leq j_1 < 3; \\ 0, & \text{otherwise.} \end{cases}$$

If  $4s \leq j < 5s$ , then

$$(d_8)_{ij} = \begin{cases} w_{7(j+m)+6+j_1 \rightarrow 7(j+m+1)} \otimes w_{7j+2 \rightarrow 7(j+1)}, & i = (j+1)_s + sj_1, \quad 0 \leq j_1 < 2; \\ (-1)^{j_1} w_{7(j+m)+2+j_1+3f(j_1,2) \rightarrow 7(j+m+1)} \otimes w_{7j+2 \rightarrow 7j+2+j_1+2f(j_1,2)}, \\ \quad i = j + s(j_1 + 6f(j_1, 2)), & 0 \leq j_1 < 3; \\ 0, & \text{otherwise.} \end{cases}$$

If  $5s \leq j < 6s$ , then

$$(d_8)_{ij} = \begin{cases} (-1)^{j_1} w_{7(j+m)+3+j_1+f(j_1,2) \rightarrow 7(j+m)+6} \otimes w_{7j+3 \rightarrow 7j+3+3f(j_1,2)}, \\ \quad i = j + s(j_1 + 4f(j_1, 2)), & 0 \leq j_1 < 3; \\ 0, & \text{otherwise.} \end{cases}$$

If  $6s \leq j < 7s$ , then

$$(d_8)_{ij} = \begin{cases} -e_{7(j+m)+6} \otimes w_{7j+4 \rightarrow 7(j+1)}, & i = (j+1)_s; \\ (1 - 2f(j_1, 1, 2)) w_{7(j+m)+2+j_1+f(j_1,0)+2f(j_1,1)-4f(j_1,3) \rightarrow 7(j+m)+6} \otimes \\ \quad w_{7j+4 \rightarrow 7j+4+f(j_1,2,3)+2f(j_1,4)}, & i = j + s(j_1 + 1), \quad 0 \leq j_1 < 5; \\ 0, & \text{otherwise.} \end{cases}$$

If  $7s \leq j < 8s$ , then

$$(d_8)_{ij} = \begin{cases} -e_{7(j+m+1)} \otimes w_{7j+4 \rightarrow 7(j+1)}, & i = s + (j+1)_s; \\ w_{7(j+m)+5 \rightarrow 7(j+m+1)} \otimes e_{7j+4}, & i = j + s; \\ 0, & \text{otherwise.} \end{cases}$$

If  $8s \leq j < 9s$ , then

$$(d_8)_{ij} = \begin{cases} (2f(j_1, 0) - 1) w_{7(j+m)+4+j_1-4f(j_1,1) \rightarrow 7(j+m+1)} \otimes w_{7j+5 \rightarrow 7j+5+f(j_1,2,3)}, \\ \quad i = j + s(j_1 + 1), & 0 \leq j_1 < 4; \\ 0, & \text{otherwise.} \end{cases}$$

If  $9s \leq j < 10s$ , then

$$(d_8)_{ij} = \begin{cases} (-1)^{j_1+1} w_{7(j+m+1)+1+j_1 \rightarrow 7(j+m+1)+2} \otimes w_{7j+6 \rightarrow 7(j+1)+1+j_1}, \\ \quad i = (j+1)_s + 2s(j_1+1), \quad 0 \leq j_1 < 2; \\ w_{7(j+m)+6+j_1 \rightarrow 7(j+m+1)+2} \otimes e_{7j+6}, \quad i = j + s(2+j_1), \quad 0 \leq j_1 < 2; \\ 0, \quad \text{otherwise.} \end{cases}$$

If  $10s \leq j < 11s$ , then

$$(d_8)_{ij} = \begin{cases} -e_{7(j+m+1)+5} \otimes w_{7j+6 \rightarrow 7(j+1)+4}, \quad i = 8s + (j+1)_s; \\ w_{7(j+m)+6 \rightarrow 7(j+m+1)+5} \otimes e_{7j+6}, \quad i = j + s; \\ 0, \quad \text{otherwise.} \end{cases}$$

If  $11s \leq j < 12s$ , then

$$(d_8)_{ij} = \begin{cases} (1 - 2f(j_1, 3)) w_{7(j+m)+6+j_1+3f(j_1,2)+2f(j_1,3) \rightarrow 7(j+m+1)+4} \otimes w_{7j+6 \rightarrow 7(j+1)+3f(j_1,2)+5f(j_1,3)}, \\ \quad i = (j+1)_s + s(j_1 + 4f(j_1, 2) + 6f(j_1, 3)), \quad 0 \leq j_1 < 4; \\ w_{7(j+m+1) \rightarrow 7(j+m+1)+4} \otimes e_{7j+6}, \quad i = j + s; \\ 0, \quad \text{otherwise.} \end{cases}$$

### Description of the $d_9$

$d_9 : Q_{10} \rightarrow Q_9$  – is an  $(12s \times 12s)$  matrix.

If  $0 \leq j < s$ , then

$$(d_9)_{ij} = \begin{cases} (2f(j_1, 0) - 1) w_{7(j+m)+5-2j_1 \rightarrow 7(j+m)+6} \otimes e_{7j}, \quad i = j + sj_1, \quad 0 \leq j_1 < 3; \\ (1 - 2f(j_1, 2)) e_{7(j+m)+6} \otimes w_{7j \rightarrow 7j+2+j_1-f(j_1,0)}, \quad i = j + s(4 + j_1 - f(j_1, 0)), \quad 0 \leq j_1 < 3; \\ 0, \quad \text{otherwise.} \end{cases}$$

If  $s \leq j < 2s$ , then

$$(d_9)_{ij} = \begin{cases} w_{7(j+m+1)-4f(j_1,0)-f(j_1,2) \rightarrow 7(j+m+1)} \otimes w_{7j \rightarrow 7j+2j_1-2f(j_1,3)-3f(j_1,4)}, \\ \quad i = j + s(3 + j_1 - 3f(j_1, 0) - f(j_1, 1)), \quad 0 \leq j_1 < 5; \\ 0, \quad \text{otherwise.} \end{cases}$$

If  $2s \leq j < 3s$ , then

$$(d_9)_{ij} = \begin{cases} -w_{7(j+m+1)+1 \rightarrow 7(j+m+1)+2} \otimes w_{7j+1 \rightarrow 7(j+1)}, \quad i = 2s + (j+1)_s; \\ w_{7(j+m)+6+f(j_1,1) \rightarrow 7(j+m+1)+2} \otimes w_{7j+1 \rightarrow 7j+1+j_1}, \quad i = j + s(j_1 + 1), \quad 0 \leq j_1 < 3; \\ -e_{7(j+m+1)+2} \otimes w_{7j+1 \rightarrow 7j+6}, \quad i = j + 7s; \\ 0, \quad \text{otherwise.} \end{cases}$$

If  $3s \leq j < 4s$ , then

$$(d_9)_{ij} = \begin{cases} -w_{7(j+m+1)+3-2j_1 \rightarrow 7(j+m+1)+3} \otimes w_{7j+2 \rightarrow 7(j+1)}, \quad i = (j+1)_s + s(j_1 + 1), \quad 0 \leq j_1 < 2; \\ w_{7(j+m+1)-j_1 \rightarrow 7(j+m+1)+3} \otimes w_{7j+2 \rightarrow 7j+2+j_1}, \quad i = j + s(j_1 + 1), \quad 0 \leq j_1 < 2; \\ -w_{7(j+m+1)+2 \rightarrow 7(j+m+1)+3} \otimes w_{7j+2 \rightarrow 7j+6}, \quad i = j + 6s; \\ 0, \quad \text{otherwise.} \end{cases}$$

If  $4s \leq j < 5s$ , then

$$(d_9)_{ij} = \begin{cases} w_{7(j+m+1) \rightarrow 7(j+m+1)+4} \otimes e_{7j+2}, & i = j; \\ -e_{7(j+m+1)+4} \otimes w_{7j+2 \rightarrow 7j+6}, & i = j + 7s; \\ 0, & \text{otherwise.} \end{cases}$$

If  $5s \leq j < 6s$ , then

$$(d_9)_{ij} = \begin{cases} w_{7(j+m)+6 \rightarrow 7(j+m+1)+5} \otimes e_{7j+3}, & i = j; \\ -e_{7(j+m+1)+5} \otimes w_{7j+3 \rightarrow 7j+6}, & i = j + 5s; \\ 0, & \text{otherwise.} \end{cases}$$

If  $6s \leq j < 7s$ , then

$$(d_9)_{ij} = \begin{cases} w_{7(j+m+1)-f(j_1,0)+4f(j_1,3) \rightarrow 7(j+m+1)+4} \otimes w_{7j+4 \rightarrow 7j+3+j_1+f(j_1,0)}, \\ i = j + s(j_1 + 2f(j_1,3)), \quad 0 \leq j_1 < 4; \\ 0, & \text{otherwise.} \end{cases}$$

If  $7s \leq j < 8s$ , then

$$(d_9)_{ij} = \begin{cases} e_{7(j+m+1)+1} \otimes w_{7j+4 \rightarrow 7(j+1)}, & i = 2s + (j+1)_s; \\ w_{7(j+m+1) \rightarrow 7(j+m+1)+1} \otimes e_{7j+4}, & i = j; \\ 0, & \text{otherwise.} \end{cases}$$

If  $8s \leq j < 9s$ , then

$$(d_9)_{ij} = \begin{cases} w_{7(j+m+1)+2j_1 \rightarrow 7(j+m+1)+2} \otimes w_{7j+5 \rightarrow 7j+5+j_1}, & i = j + sj_1, \quad 0 \leq j_1 < 2; \\ 0, & \text{otherwise.} \end{cases}$$

If  $9s \leq j < 10s$ , then

$$(d_9)_{ij} = \begin{cases} -e_{7(j+m+1)+5} \otimes w_{7j+5 \rightarrow 7(j+1)}, & i = (j+1)_s; \\ w_{7(j+m+1)+6-j_1-6f(j_1,0) \rightarrow 7(j+m+1)+5} \otimes w_{7j+5 \rightarrow 7j+6-f(j_1,0)}, \\ i = j + s(j_1 - f(j_1,0)), \quad 0 \leq j_1 < 3; \\ 0, & \text{otherwise.} \end{cases}$$

If  $10s \leq j < 11s$ , then

$$(d_9)_{ij} = \begin{cases} w_{7(j+m+1)+5+j_1 \rightarrow 7(j+m+1)+6} \otimes w_{7j+6 \rightarrow 7(j+1)+j_1}, & i = (j+1)_s + 3sj_1, \quad 0 \leq j_1 < 2; \\ (2f(j_1,0) - 1)w_{7(j+m+1)+6-j_1-4f(j_1,0) \rightarrow 7(j+m+1)+6} \otimes e_{7j+6}, \\ i = j + s(j_1 - 1), \quad 0 \leq j_1 < 3; \\ 0, & \text{otherwise.} \end{cases}$$

If  $11s \leq j < 12s$ , then

$$(d_9)_{ij} = \begin{cases} e_{7(j+m+2)} \otimes w_{7j+6 \rightarrow 7(j+1)+4}, & i = 7s + (j+1)_s; \\ w_{7(j+m+1)+5 \rightarrow 7(j+m+2)} \otimes e_{7j+6}, & i = j - s; \\ 0, & \text{otherwise.} \end{cases}$$

#### Description of the $d_{10}$

$d_{10} : Q_{11} \rightarrow Q_{10}$  - is an  $(12s \times 10s)$  matrix.

If  $0 \leq j < s$ , then

$$(d_{10})_{ij} = \begin{cases} w_{7(j+m-1)+6+j_1 \rightarrow 7(j+m)+2} \otimes e_{7j}, & i = j + sj_1, \ 0 \leq j_1 < 2; \\ -w_{7(j+m)+2-f(j_1,1) \rightarrow 7(j+m)+2} \otimes w_{7j \rightarrow 7j+3+j_1-2f(j_1,0)}, \\ \quad i = j + s(j_1 + 6 - 4f(j_1,0)), \ 0 \leq j_1 < 3; \\ 0, & \text{otherwise.} \end{cases}$$

If  $s \leq j < 2s$ , then

$$(d_{10})_{ij} = \begin{cases} (2f(j_1,0) - 1)w_{7(j+m)+4-4f(j_1,0) \rightarrow 7(j+m)+4} \otimes w_{7j \rightarrow 7j+2j_1}, \\ \quad i = j + s(2j_1 + 1 - f(j_1,0)), \ 0 \leq j_1 < 3; \\ 0, & \text{otherwise.} \end{cases}$$

If  $2s \leq j < 3s$ , then

$$(d_{10})_{ij} = \begin{cases} -e_{7(j+m+1)} \otimes w_{7j+1 \rightarrow 7(j+1)}, & i = s + (j+1)_s; \\ (-1)^{j_1} w_{7(j+m)+2+j_1 \rightarrow 7(j+m+1)} \otimes w_{7j+1 \rightarrow 7j+1+j_1}, & i = j + sj_1, \ 0 \leq j_1 < 2; \\ 0, & \text{otherwise.} \end{cases}$$

If  $3s \leq j < 4s$ , then

$$(d_{10})_{ij} = \begin{cases} -e_{7(j+m)+6} \otimes w_{7j+2 \rightarrow 7(j+1)}, & i = (j+1)_s; \\ (1 - 2f(j_1,1,2))w_{7(j+m)+3+j_1 \rightarrow 7(j+m)+6} \otimes w_{7j+2 \rightarrow 7j+2+f(j_1,2)+4f(j_1,3)}, \\ \quad i = j + s(j_1 + 4f(j_1,3)), \ 0 \leq j_1 < 4; \\ 0, & \text{otherwise.} \end{cases}$$

If  $4s \leq j < 5s$ , then

$$(d_{10})_{ij} = \begin{cases} w_{7(j+m)+5+2j_1 \rightarrow 7(j+m+1)} \otimes w_{7j+3 \rightarrow 7j+3+3j_1}, & i = j + s(1 + 6j_1), \ 0 \leq j_1 < 2; \\ 0, & \text{otherwise.} \end{cases}$$

If  $5s \leq j < 6s$ , then

$$(d_{10})_{ij} = \begin{cases} -w_{7(j+m)+6+j_1 \rightarrow 7(j+m+1)} \otimes w_{7j+4 \rightarrow 7(j+1)}, & i = (j+1)_s + sj_1, \ 0 \leq j_1 < 2; \\ (1 - 2f(j_1,1,2))w_{7(j+m)+2j_1+1+3f(j_1,0)-2f(j_1,1) \rightarrow 7(j+m+1)} \otimes w_{7j+4 \rightarrow 7j+3+j_1+f(j_1,0)}, \\ \quad i = j + s(2j_1 + f(j_1,0)), \ 0 \leq j_1 < 4; \\ 0, & \text{otherwise.} \end{cases}$$

If  $6s \leq j < 7s$ , then

$$(d_{10})_{ij} = \begin{cases} (2f(j_1,0) - 1)w_{7(j+m)+4+j_1-2f(j_1,0) \rightarrow 7(j+m)+6} \otimes w_{7j+5 \rightarrow 7j+5+f(j_1,2)}, \\ \quad i = j + s(j_1 + 2), \ 0 \leq j_1 < 3; \\ 0, & \text{otherwise.} \end{cases}$$

If  $7s \leq j < 8s$ , then

$$(d_{10})_{ij} = \begin{cases} (1 - 2f(j_1,0,1))w_{7(j+m)+6+j_1+3f(j_1,2,3)+2f(j_1,4) \rightarrow 7(j+m+1)+5} \otimes w_{7j+6 \rightarrow 7(j+1)+j_1-f(j_1,1)+f(j_1,4)}, \\ \quad i = (j+1)_s + s(j_1 + 2f(j_1,2,3) + 5f(j_1,4)), \ 0 \leq j_1 < 5; \\ w_{7(j+m)+6+j_1 \rightarrow 7(j+m+1)+5} \otimes e_{7j+6}, & i = j + s(3 + j_1), \ 0 \leq j_1 < 2; \\ 0, & \text{otherwise.} \end{cases}$$

If  $8s \leq j < 9s$ , then

$$(d_{10})_{ij} = \begin{cases} (-1)^{j_1+1} w_{7(j+m+1)+2+j_1 \rightarrow 7(j+m+1)+3} \otimes w_{7j+6 \rightarrow 7(j+1)+1+j_1}, \\ \quad i = (j+1)_s + s(j_1+2), \quad 0 \leq j_1 < 2; \\ w_{7(j+m)+6 \rightarrow 7(j+m+1)+3} \otimes e_{7j+6}, \quad i = j+2s; \\ 0, \quad \text{otherwise.} \end{cases}$$

If  $9s \leq j < 10s$ , then

$$(d_{10})_{ij} = \begin{cases} -e_{7(j+m+1)+1} \otimes w_{7j+6 \rightarrow 7(j+1)+4}, \quad i = 7s + (j+1)_s; \\ w_{7(j+m+1) \rightarrow 7(j+m+1)+1} \otimes e_{7j+6}, \quad i = j+2s; \\ 0, \quad \text{otherwise.} \end{cases}$$

### Description of the $d_{11}$

$d_{11} : Q_{12} \rightarrow Q_{11}$  - is an  $(10s \times 10s)$  matrix.

If  $0 \leq j < s$ , then

$$(d_{11})_{ij} = \begin{cases} (1 - 2f(j_1, 1) - 2f(j_1, 5)) w_{7(j+m)+3+j_1-f(j_1,0)+2f(j_1,2)-f(j_1,5)-3f(j_1,6) \rightarrow 7(j+m+1)} \otimes \\ \quad w_{7j \rightarrow 7j+j_1-1+f(j_1,0)}, \\ \quad i = j + sj_1, \quad 0 \leq j_1 < 7; \\ 0, \quad \text{otherwise.} \end{cases}$$

If  $s \leq j < 2s$ , then

$$(d_{11})_{ij} = \begin{cases} w_{7(j+m+1)+2 \rightarrow 7(j+m+1)+3} \otimes w_{7j+1 \rightarrow 7(j+1)}, \quad i = (j+1)_s; \\ (1 - 2f(j_1, 2)) w_{7(j+m+1)-j_1+5f(j_1,2) \rightarrow 7(j+m+1)+3} \otimes w_{7j+1 \rightarrow 7j+1+j_1+3f(j_1,2)}, \\ \quad i = j + s(j_1+1+4f(j_1,2)), \quad 0 \leq j_1 < 3; \\ 0, \quad \text{otherwise.} \end{cases}$$

If  $2s \leq j < 3s$ , then

$$(d_{11})_{ij} = \begin{cases} e_{7(j+m+1)+4} \otimes w_{7j+1 \rightarrow 7(j+1)}, \quad i = s + (j+1)_s; \\ w_{7(j+m+1) \rightarrow 7(j+m+1)+4} \otimes e_{7j+1}, \quad i = j; \\ 0, \quad \text{otherwise.} \end{cases}$$

If  $3s \leq j < 4s$ , then

$$(d_{11})_{ij} = \begin{cases} -w_{7(j+m+1)+4 \rightarrow 7(j+m+1)+5} \otimes w_{7j+2 \rightarrow 7(j+1)}, \quad i = s + (j+1)_s; \\ (1 - 2f(j_1, 2)) w_{7(j+m)+6+j_1+4f(j_1,2) \rightarrow 7(j+m+1)+5} \otimes w_{7j+2 \rightarrow 7j+2+j_1+2f(j_1,2)}, \\ \quad i = j + s(j_1+2f(j_1,2)), \quad 0 \leq j_1 < 3; \\ 0, \quad \text{otherwise.} \end{cases}$$

If  $4s \leq j < 5s$ , then

$$(d_{11})_{ij} = \begin{cases} (-1)^{j_1} w_{7(j+m+1)+j_1 \rightarrow 7(j+m+1)+1} \otimes w_{7j+3 \rightarrow 7j+3+3j_1}, \quad i = j + 5sj_1, \quad 0 \leq j_1 < 2; \\ 0, \quad \text{otherwise.} \end{cases}$$



If  $5s \leq j < 6s$ , then

$$(d_{11})_{ij} = \begin{cases} e_{7(j+m+1)+2} \otimes w_{7j+4 \rightarrow 7(j+1)}, & i = (j+1)_s; \\ (-1)^{j_1} w_{7(j+m+1)+j_1 \rightarrow 7(j+m+1)+2} \otimes w_{7j+4 \rightarrow 7j+4+2j_1}, & i = j + 4sj_1, \ 0 \leq j_1 < 2; \\ 0, & \text{otherwise.} \end{cases}$$

If  $6s \leq j < 7s$ , then

$$(d_{11})_{ij} = \begin{cases} (2f(j_1, 0) - 1) w_{7(j+m+1)-j_1+7f(j_1, 2) \rightarrow 7(j+m+1)+5} \otimes w_{7j+4 \rightarrow 7j+4+j_1}, \\ i = j + s(j_1 - 1), \ 0 \leq j_1 < 3; \\ 0, & \text{otherwise.} \end{cases}$$

If  $7s \leq j < 8s$ , then

$$(d_{11})_{ij} = \begin{cases} w_{7(j+m)+6+4j_1 \rightarrow 7(j+m+1)+3} \otimes w_{7j+5 \rightarrow 7j+5+j_1}, & i = j + s(2j_1 - 1), \ 0 \leq j_1 < 2; \\ 0, & \text{otherwise.} \end{cases}$$

If  $8s \leq j < 9s$ , then

$$(d_{11})_{ij} = \begin{cases} w_{7(j+m+1)+6-4f(j_1, 0) \rightarrow 7(j+m+1)+6} \otimes w_{7j+6 \rightarrow 7(j+1)+2j_1+f(j_1, 2)}, \\ i = (j+1)_s + 3sj_1, \ 0 \leq j_1 < 3; \\ (2f(j_1, 0) - 1) w_{7(j+m+1)+5-2j_1 \rightarrow 7(j+m+1)+6} \otimes e_{7j+6}, & i = j + s(j_1 - 1), \ 0 \leq j_1 < 3; \\ 0, & \text{otherwise.} \end{cases}$$

If  $9s \leq j < 10s$ , then

$$(d_{11})_{ij} = \begin{cases} e_{7(j+m+2)} \otimes w_{7j+6 \rightarrow 7(j+1)+1}, & i = 2s + (j+1)_s; \\ w_{7(j+m+1)+3 \rightarrow 7(j+m+2)} \otimes e_{7j+6}, & i = j - s; \\ 0, & \text{otherwise.} \end{cases}$$

### Description of the $d_{12}$

$d_{12} : Q_{13} \rightarrow Q_{12}$  - is an  $(10s \times 9s)$  matrix.

If  $0 \leq j < s$ , then

$$(d_{12})_{ij} = \begin{cases} (2f(j_1, 0) + 2f(j_1, 3) - 1) w_{7(j+m)+j_1-1+f(j_1, 0)+3f(j_1, 1) \rightarrow 7(j+m)+3} \otimes w_{7j \rightarrow 7j+j_1+1-f(j_1, 0, 1)}, \\ i = j + s(2j_1 - 1 + f(j_1, 0) + f(j_1, 2)), \ 0 \leq j_1 < 5; \\ 0, & \text{otherwise.} \end{cases}$$

If  $s \leq j < 2s$ , then

$$(d_{12})_{ij} = \begin{cases} w_{7(j+m) \rightarrow 7(j+m)+5} \otimes e_{7j}, & i = j_s; \\ (2f(j_1, 2) - 1) w_{7(j+m)+5-f(j_1, 0) \rightarrow 7(j+m)+5} \otimes w_{7j \rightarrow 7j+2j_1+f(j_1, 0)}, \\ i = j + s(j_1 + 1 + 2f(j_1, 2)), \ 0 \leq j_1 < 3; \\ 0, & \text{otherwise.} \end{cases}$$

If  $2s \leq j < 3s$ , then

$$(d_{12})_{ij} = \begin{cases} (2f(j_1, 0) + 2f(j_1, 3) - 1) w_{7(j+m)+3+j_1-5f(j_1, 3)-f(j_1, 4) \rightarrow 7(j+m)+6} \otimes \\ w_{7j+1 \rightarrow 7j+j_1+f(j_1, 0)+2f(j_1, 4)}, & i = j + s(j_1 - 1 + 3f(j_1, 4)), \ 0 \leq j_1 < 5; \\ 0, & \text{otherwise.} \end{cases}$$

If  $3s \leq j < 4s$ , then

$$(d_{12})_{ij} = \begin{cases} -e_{7(j+m+1)} \otimes w_{7j+2 \rightarrow 7(j+1)}, & i = (j+1)_s; \\ (1 - 2f(j_1, 1))w_{7(j+m)+4+j_1+f(j_1,0)-4f(j_1,1) \rightarrow 7(j+m+1)} \otimes w_{7j+2 \rightarrow 7j+6-4f(j_1,0)-3f(j_1,1)}, \\ \quad i = j + s(j_1 + 3f(j_1, 2, 3)), & 0 \leq j_1 < 4; \\ 0, & \text{otherwise.} \end{cases}$$

If  $4s \leq j < 5s$ , then

$$(d_{12})_{ij} = \begin{cases} (-1)^{j_1} w_{7(j+m+1)+j_1 \rightarrow 7(j+m+1)+1} \otimes w_{7j+3 \rightarrow 7(j+1)+3j_1}, \\ \quad i = (j+1)_s + 4sj_1, & 0 \leq j_1 < 2; \\ (2f(j_1, 0) - 1)w_{7(j+m)+5+j_1-4f(j_1,0) \rightarrow 7(j+m+1)+1} \otimes w_{7j+3 \rightarrow 7j+6-3f(j_1,0)}, \\ \quad i = j + s(3 + j_1 - 3f(j_1, 0)), & 0 \leq j_1 < 3; \\ 0, & \text{otherwise.} \end{cases}$$

If  $5s \leq j < 6s$ , then

$$(d_{12})_{ij} = \begin{cases} (2f(j_1, 0) - 1)w_{7(j+m)+2+3f(j_1,1)+f(j_1,2)+4f(j_1,3) \rightarrow 7(j+m)+6} \otimes w_{7j+4 \rightarrow 7j+3+j_1+f(j_1,0)}, \\ \quad i = j + sj_1, & 0 \leq j_1 < 4; \\ 0, & \text{otherwise.} \end{cases}$$

If  $6s \leq j < 7s$ , then

$$(d_{12})_{ij} = \begin{cases} (-1)^{j_1} w_{7(j+m)+3+4j_1 \rightarrow 7(j+m+1)} \otimes w_{7j+5 \rightarrow 7j+5+j_1}, & i = j + s(2j_1 + 1), & 0 \leq j_1 < 2; \\ 0, & \text{otherwise.} \end{cases}$$

If  $7s \leq j < 8s$ , then

$$(d_{12})_{ij} = \begin{cases} (2f(j_1, 1) - 1)w_{7(j+m+1)+j_1 \rightarrow 7(j+m+1)+2} \otimes w_{7j+6 \rightarrow 7(j+1)+2+j_1-2f(j_1,0)}, \\ \quad i = (j+1)_s + s(3 + j_1 - 3f(j_1, 0)), & 0 \leq j_1 < 3; \\ w_{7(j+m)+6+j_1 \rightarrow 7(j+m+1)+2} \otimes e_{7j+6}, & i = j + s(j_1 + 1), & 0 \leq j_1 < 2; \\ 0, & \text{otherwise.} \end{cases}$$

If  $8s \leq j < 9s$ , then

$$(d_{12})_{ij} = \begin{cases} -e_{7(j+m+1)+4} \otimes w_{7j+6 \rightarrow 7(j+1)+1}, & i = 2s + (j+1)_s; \\ w_{7(j+m+1) \rightarrow 7(j+m+1)+4} \otimes e_{7j+6}, & i = j + s; \\ 0, & \text{otherwise.} \end{cases}$$

### Description of the $d_{13}$

$d_{13} : Q_{14} \rightarrow Q_{13}$  - is an  $(9s \times 7s)$  matrix.

If  $0 \leq j < s$ , then

$$(d_{13})_{ij} = \begin{cases} (-1)^{j_1} w_{7(j+m)+6-3f(j_1,0)-f(j_1,1) \rightarrow 7(j+m)+6} \otimes w_{7j \rightarrow 7j+j_1-1+f(j_1,0)+2f(j_1,3)}, \\ \quad i = j + s(j_1 + 2f(j_1, 3)), & 0 \leq j_1 < 4; \\ 0, & \text{otherwise.} \end{cases}$$

If  $s \leq j < 2s$ , then

$$(d_{13})_{ij} = \begin{cases} e_{7(j+m+1)+5} \otimes w_{7j+1 \rightarrow 7(j+1)}, & i = s + (j+1)_s; \\ (1 - 2f(j_1, 2))w_{7(j+m)+6+j_1+3f(j_1, 2) \rightarrow 7(j+m+1)+5} \otimes w_{7j+1 \rightarrow 7j+1+j_1+3f(j_1, 2)}, \\ \quad i = j + s(j_1 + 1 + 4f(j_1, 2)), & 0 \leq j_1 < 3; \\ 0, & \text{otherwise.} \end{cases}$$

If  $2s \leq j < 3s$ , then

$$(d_{13})_{ij} = \begin{cases} w_{7(j+m+1)+j_1 \rightarrow 7(j+m+1)+1} \otimes w_{7j+2 \rightarrow 7j+2+j_1}, & i = j + s(j_1 + 1), \quad 0 \leq j_1 < 2; \\ 0, & \text{otherwise.} \end{cases}$$

If  $3s \leq j < 4s$ , then

$$(d_{13})_{ij} = \begin{cases} w_{7(j+m+1)+1+j_1 \rightarrow 7(j+m+1)+2} \otimes w_{7j+3 \rightarrow 7j+3+3j_1}, & i = j + s(3j_1 + 1), \quad 0 \leq j_1 < 2; \\ 0, & \text{otherwise.} \end{cases}$$

If  $4s \leq j < 5s$ , then

$$(d_{13})_{ij} = \begin{cases} e_{7(j+m+1)+3} \otimes w_{7j+4 \rightarrow 7(j+1)}, & i = (j+1)_s; \\ w_{7(j+m)+6+j_1+f(j_1, 2) \rightarrow 7(j+m+1)+3} \otimes w_{7j+4 \rightarrow 7j+4+j_1}, & i = j + s(j_1 + 1), \quad 0 \leq j_1 < 3; \\ 0, & \text{otherwise.} \end{cases}$$

If  $5s \leq j < 6s$ , then

$$(d_{13})_{ij} = \begin{cases} w_{7(j+m+1)+4j_1 \rightarrow 7(j+m+1)+4} \otimes w_{7j+5 \rightarrow 7j+5+j_1}, & i = j + s(2j_1 + 1), \quad 0 \leq j_1 < 2; \\ 0, & \text{otherwise.} \end{cases}$$

If  $6s \leq j < 7s$ , then

$$(d_{13})_{ij} = \begin{cases} w_{7(j+m+2)-4f(j_1, 0)-f(j_1, 1) \rightarrow 7(j+m+2)} \otimes w_{7j+6 \rightarrow 7(j+1)+j_1+2f(j_1, 3)}, \\ \quad i = (j+1)_s + s(j_1 + 1 - f(j_1, 0) + 2f(j_1, 3)), & 0 \leq j_1 < 4; \\ (-1)^{j_1} w_{7(j+m+1)+2+2j_1 \rightarrow 7(j+m+2)} \otimes e_{7j+6}, & i = j + s(j_1 + 1), \quad 0 \leq j_1 < 2; \\ 0, & \text{otherwise.} \end{cases}$$

#### Description of the $d_{14}$

$d_{14} : Q_{15} \rightarrow Q_{14}$  - is an  $(7s \times 8s)$  matrix.

If  $0 \leq j < s$ , then

$$(d_{14})_{ij} = \begin{cases} -e_{7(j+m)+6} \otimes w_{7j \rightarrow 7(j+1)}, & i = (j+1)_s; \\ (-1)^{j_1} w_{7(j+m-1)+6+j_1+5f(j_1, 1) \rightarrow 7(j+m)+6} \otimes w_{7j \rightarrow 7j+j_1}, \\ \quad i = j + sj_1, & 0 \leq j_1 < 6; \\ 0, & \text{otherwise.} \end{cases}$$

If  $s \leq j < 2s$ , then

$$(d_{14})_{ij} = \begin{cases} w_{7(j+m)+6 \rightarrow 7(j+m+1)} \otimes w_{7j+1 \rightarrow 7(j+1)}, & i = (j+1)_s; \\ (-1)^{j_1} w_{7(j+m)+j_1+5f(j_1, 0) \rightarrow 7(j+m+1)} \otimes w_{7j+1 \rightarrow 7j+1+j_1}, \\ \quad i = j + sj_1, & 0 \leq j_1 < 3; \\ -e_{7(j+m+1)} \otimes w_{7j+1 \rightarrow 7j+6}, & i = j + 5s; \\ 0, & \text{otherwise.} \end{cases}$$

If  $2s \leq j < 3s$ , then

$$(d_{14})_{ij} = \begin{cases} -w_{7(j+m)+6+2j_1 \rightarrow 7(j+m+1)+1} \otimes w_{7j+2 \rightarrow 7(j+1)+2j_1}, & i = (j+1)_s + 2sj_1, \ 0 \leq j_1 < 2; \\ (-1)^{j_1} w_{7(j+m)+1+j_1 \rightarrow 7(j+m+1)+1} \otimes w_{7j+2 \rightarrow 7j+2+j_1}, & i = j + sj_1, \ 0 \leq j_1 < 2; \\ w_{7(j+m+1) \rightarrow 7(j+m+1)+1} \otimes w_{7j+2 \rightarrow 7j+6}, & i = j + 4s; \\ 0, & \text{otherwise.} \end{cases}$$

If  $3s \leq j < 4s$ , then

$$(d_{14})_{ij} = \begin{cases} (-1)^{j_1} w_{7(j+m+1)+1+j_1 \rightarrow 7(j+m+1)+2} \otimes w_{7j+3 \rightarrow 7(j+1)+2+j_1}, & i = (j+1)_s + s(2+j_1), \ 0 \leq j_1 < 2; \\ w_{7(j+m)+6 \rightarrow 7(j+m+1)+2} \otimes w_{7j+3 \rightarrow 7(j+1)}, & i = (j+1)_s; \\ (-1)^{j_1} w_{7(j+m)+2+5j_1 \rightarrow 7(j+m+1)+2} \otimes w_{7j+3 \rightarrow 7j+3+3j_1}, & i = j + 3sj_1, \ 0 \leq j_1 < 2; \\ 0, & \text{otherwise.} \end{cases}$$

If  $4s \leq j < 5s$ , then

$$(d_{14})_{ij} = \begin{cases} (2f(j_1, 0) - 1) w_{7(j+m)+3+j_1 \rightarrow 7(j+m+1)} \otimes w_{7j+4 \rightarrow 7j+4+j_1}, & i = j + sj_1, \ 0 \leq j_1 < 3; \\ 0, & \text{otherwise.} \end{cases}$$

If  $5s \leq j < 6s$ , then

$$(d_{14})_{ij} = \begin{cases} -e_{7(j+m+1)+4} \otimes w_{7j+5 \rightarrow 7(j+1)+5}, & i = 5s + (j+1)_s; \\ w_{7(j+m)+4+3j_1 \rightarrow 7(j+m+1)+4} \otimes w_{7j+5 \rightarrow 7j+5+j_1}, & i = j + sj_1, \ 0 \leq j_1 < 2; \\ 0, & \text{otherwise.} \end{cases}$$

If  $6s \leq j < 7s$ , then

$$(d_{14})_{ij} = \begin{cases} -w_{7(j+m)+6 \rightarrow 7(j+m+1)+3} \otimes w_{7j+6 \rightarrow 7(j+1)}, & i = (j+1)_s; \\ (-1)^{j_1+1} w_{7(j+m+1)+1+j_1 \rightarrow 7(j+m+1)+3} \otimes w_{7j+6 \rightarrow 7(j+1)+2+j_1}, & i = (j+1)_s + s(2+j_1), \ 0 \leq j_1 < 3; \\ w_{7(j+m+1) \rightarrow 7(j+m+1)+3} \otimes e_{7j+6}, & i = j; \\ 0, & \text{otherwise.} \end{cases}$$

If  $7s \leq j < 8s$ , then

$$(d_{14})_{ij} = \begin{cases} -w_{7(j+m+1)+5-j_1 \rightarrow 7(j+m+1)+5} \otimes w_{7j+6 \rightarrow 7(j+1)+1+4j_1}, & i = (j+1)_s + s(1+4j_1), \ 0 \leq j_1 < 2; \\ w_{7(j+m+1) \rightarrow 7(j+m+1)+5} \otimes e_{7j+6}, & i = j - s; \\ 0, & \text{otherwise.} \end{cases}$$

### Description of the $d_{15}$

$d_{15} : Q_{16} \rightarrow Q_{15}$  - is an  $(8s \times 7s)$  matrix.

If  $0 \leq j < s$ , then

$$(d_{15})_{ij} = \begin{cases} w_{7(j+m)+6+j_1 \rightarrow 7(j+m+1)} \otimes w_{7j \rightarrow 7j+j_1}, & i = j + sj_1, \ 0 \leq j_1 < 2; \\ -e_{7(j+m+1)} \otimes w_{7j \rightarrow 7j+4}, & i = j + 4s; \\ 0, & \text{otherwise.} \end{cases}$$

If  $s \leq j < 2s$ , then

$$(d_{15})_{ij} = \begin{cases} w_{7(j+m+1)+j_1 \rightarrow 7(j+m+1)+1} \otimes w_{7j+1 \rightarrow 7j+1+j_1}, & i = j + sj_1, 0 \leq j_1 < 2; \\ 0, & \text{otherwise.} \end{cases}$$

If  $2s \leq j < 3s$ , then

$$(d_{15})_{ij} = \begin{cases} w_{7(j+m+1)+1+j_1 \rightarrow 7(j+m+1)+2} \otimes w_{7j+2 \rightarrow 7j+2+j_1}, & i = j + sj_1, 0 \leq j_1 < 2; \\ 0, & \text{otherwise.} \end{cases}$$

If  $3s \leq j < 4s$ , then

$$(d_{15})_{ij} = \begin{cases} w_{7(j+m+1)+2+j_1 \rightarrow 7(j+m+1)+3} \otimes w_{7j+3 \rightarrow 7j+3+j_1}, & i = j + 3sj_1, 0 \leq j_1 < 2; \\ 0, & \text{otherwise.} \end{cases}$$

If  $4s \leq j < 5s$ , then

$$(d_{15})_{ij} = \begin{cases} w_{7(j+m+1)+4+j_1 \rightarrow 7(j+m+1)+4} \otimes w_{7j+4 \rightarrow 7j+4+j_1}, & i = j + sj_1, 0 \leq j_1 < 2; \\ 0, & \text{otherwise.} \end{cases}$$

If  $5s \leq j < 6s$ , then

$$(d_{15})_{ij} = \begin{cases} (-1)^{j_1} w_{7(j+m+1)+4+j_1 \rightarrow 7(j+m+1)+5} \otimes w_{7j+5 \rightarrow 7j+5+j_1}, & i = j + 2sj_1, 0 \leq j_1 < 2; \\ 0, & \text{otherwise.} \end{cases}$$

If  $6s \leq j < 7s$ , then

$$(d_{15})_{ij} = \begin{cases} e_{7(j+m+1)+6} \otimes w_{7j+6 \rightarrow 7(j+1)}, & i = (j+1)_s; \\ (-1)^{j_1} w_{7(j+m+1)+3+2j_1 \rightarrow 7(j+m+1)+6} \otimes e_{7j+6}, & i = j + sj_1, 0 \leq j_1 < 2; \\ 0, & \text{otherwise.} \end{cases}$$

### Description of the $d_{16}$

$d_{16} : Q_{17} \rightarrow Q_{16}$  – is an  $(7s \times 7s)$  matrix.

If  $0 \leq j < s$ , then

$$(d_{16})_{ij} = \begin{cases} -e_{7(j+m+1)} \otimes w_{7j \rightarrow 7(j+1)}, & i = (j+1)_s; \\ (-1)^{j_1} w_{7(j+m)+j_1 \rightarrow 7(j+m+1)} \otimes w_{7j \rightarrow 7j+j_1}, & i = j + sj_1, 0 \leq j_1 < 7; \\ 0, & \text{otherwise.} \end{cases}$$

If  $s \leq j < 2s$ , then

$$(d_{16})_{ij} = \begin{cases} (-1)^{j_1} w_{7(j+m+1)+j_1 \rightarrow 7(j+m+1)+1} \otimes w_{7j+1 \rightarrow 7(j+1)+j_1}, \\ \quad i = (j+1)_s + sj_1, 0 \leq j_1 < 2; \\ (-1)^{j_1} w_{7(j+m)+1+j_1 \rightarrow 7(j+m+1)+1} \otimes w_{7j+1 \rightarrow 7j+1+j_1}, & i = j + sj_1, 0 \leq j_1 < 3; \\ -w_{7(j+m)+6 \rightarrow 7(j+m+1)+1} \otimes w_{7j+1 \rightarrow 7j+6}, & i = j + 5s; \\ 0, & \text{otherwise.} \end{cases}$$

If  $2s \leq j < 3s$ , then

$$(d_{16})_{ij} = \begin{cases} (-1)^{j_1+1} w_{7(j+m+1)+j_1 \rightarrow 7(j+m+1)+2} \otimes w_{7j+2 \rightarrow 7(j+1)+j_1}, \\ \quad i = (j+1)_s + sj_1, \quad 0 \leq j_1 < 3; \\ (-1)^{j_1} w_{7(j+m)+2+j_1 \rightarrow 7(j+m+1)+2} \otimes w_{7j+2 \rightarrow 7j+2+j_1}, & i = j + sj_1, \quad 0 \leq j_1 < 2; \\ w_{7(j+m)+6 \rightarrow 7(j+m+1)+2} \otimes w_{7j+2 \rightarrow 7j+6}, & i = j + 4s; \\ 0, & \text{otherwise.} \end{cases}$$

If  $3s \leq j < 4s$ , then

$$(d_{16})_{ij} = \begin{cases} (-1)^{j_1} w_{7(j+m+1)+j_1 \rightarrow 7(j+m+1)+3} \otimes w_{7j+3 \rightarrow 7(j+1)+j_1}, \\ \quad i = (j+1)_s + sj_1, \quad 0 \leq j_1 < 4; \\ (-1)^{j_1} w_{7(j+m)+3+3j_1 \rightarrow 7(j+m+1)+3} \otimes w_{7j+3 \rightarrow 7j+3+3j_1}, & i = j + 3sj_1, \quad 0 \leq j_1 < 2; \\ 0, & \text{otherwise.} \end{cases}$$

If  $4s \leq j < 5s$ , then

$$(d_{16})_{ij} = \begin{cases} -w_{7(j+m+1)+4j_1 \rightarrow 7(j+m+1)+4} \otimes w_{7j+4 \rightarrow 7(j+1)+4j_1}, & i = (j+1)_s + 4sj_1, \quad 0 \leq j_1 < 2; \\ (-1)^{j_1} w_{7(j+m)+4+j_1 \rightarrow 7(j+m+1)+4} \otimes w_{7j+4 \rightarrow 7j+4+j_1}, & i = j + sj_1, \quad 0 \leq j_1 < 3; \\ 0, & \text{otherwise.} \end{cases}$$

If  $5s \leq j < 6s$ , then

$$(d_{16})_{ij} = \begin{cases} w_{7(j+m+1) \rightarrow 7(j+m+1)+5} \otimes w_{7j+5 \rightarrow 7(j+1)}, & i = (j+1)_s; \\ (-1)^{j_1} w_{7(j+m+1)+4+j_1 \rightarrow 7(j+m+1)+5} \otimes w_{7j+5 \rightarrow 7(j+1)+4+j_1}, \\ \quad i = (j+1)_s + s(4+j_1), \quad 0 \leq j_1 < 2; \\ (-1)^{j_1} w_{7(j+m)+5+j_1 \rightarrow 7(j+m+1)+5} \otimes w_{7j+5 \rightarrow 7j+5+j_1}, & i = j + sj_1, \quad 0 \leq j_1 < 2; \\ 0, & \text{otherwise.} \end{cases}$$

If  $6s \leq j < 7s$ , then

$$(d_{16})_{ij} = \begin{cases} (-1)^{j_1+1} w_{7(j+m+1)+j_1 \rightarrow 7(j+m+1)+6} \otimes w_{7j+6 \rightarrow 7(j+1)+j_1}, \\ \quad i = (j+1)_s + sj_1, \quad 0 \leq j_1 < 7; \\ w_{7(j+m)+6 \rightarrow 7(j+m+1)+6} \otimes e_{7j+6}, & i = j; \\ 0, & \text{otherwise.} \end{cases}$$
