# Supplementary material for: Hochschild cohomology rings for self-injective algebras of tree classes $E_7$ and $E_8$
Source: arXiv:1910.03043 ancillary file (2021-02-14)
Supplement: Supplementary file 2 [file e7-omega-shifts.pdf]

TREE CLASS  $E_7$ :  $\Omega$ -SHIFTS OF GENERATORS OF THE ALGEBRA  $\mathrm{HH}^*(R)$

**Notation.**

- (1) For generator degree  $t$  represent it in the form  $t = 17\ell + r$  ( $0 \leq r \leq 16$ ).
- (2) For translate  $\Omega^{t_0}$  represent  $t_0$  in the form  $t_0 = 17\ell_0 + r_0$  ( $0 \leq r_0 \leq 16$ ).

**Proposition 1** (Translates for the case 1). (I) *Let  $r_0 \in \mathbb{N}$ ,  $r_0 < 17$ .  $r_0$ -translates of the elements  $Y_t^{(1)}$  are described by the following way.*

- (1) *If  $r_0 = 0$ , then  $\Omega^0(Y_t^{(1)})$  is described with  $(7s \times 7s)$ -matrix with the following elements  $b_{ij}$ :  
If  $0 \leq j < s$ , then*

$$b_{ij} = \begin{cases} e_{7(j+m)} \otimes e_{7j}, & i = j; \\ 0, & \text{otherwise.} \end{cases}$$

*If  $s \leq j < 2s$ , then*

$$b_{ij} = \begin{cases} e_{7(j+m)+1} \otimes e_{7j+1}, & i = j; \\ 0, & \text{otherwise.} \end{cases}$$

*If  $2s \leq j < 3s$ , then*

$$b_{ij} = \begin{cases} e_{7(j+m)+2} \otimes e_{7j+2}, & i = j; \\ 0, & \text{otherwise.} \end{cases}$$

*If  $3s \leq j < 4s$ , then*

$$b_{ij} = \begin{cases} e_{7(j+m)+3} \otimes e_{7j+3}, & i = j; \\ 0, & \text{otherwise.} \end{cases}$$

*If  $4s \leq j < 5s$ , then*

$$b_{ij} = \begin{cases} e_{7(j+m)+4} \otimes e_{7j+4}, & i = j; \\ 0, & \text{otherwise.} \end{cases}$$

*If  $5s \leq j < 6s$ , then*

$$b_{ij} = \begin{cases} e_{7(j+m)+5} \otimes e_{7j+5}, & i = j; \\ 0, & \text{otherwise.} \end{cases}$$

*If  $6s \leq j < 7s$ , then*

$$b_{ij} = \begin{cases} e_{7(j+m)+6} \otimes e_{7j+6}, & i = j; \\ 0, & \text{otherwise.} \end{cases}$$

- (2) *If  $r_0 = 1$ , then  $\Omega^1(Y_t^{(1)})$  is described with  $(8s \times 8s)$ -matrix with the following elements  $b_{ij}$ :  
If  $0 \leq j < s$ , then*

$$b_{ij} = \begin{cases} e_{7(j+m)+1} \otimes e_{7j}, & i = j; \\ 0, & \text{otherwise.} \end{cases}$$

*If  $s \leq j < 2s$ , then*

$$b_{ij} = \begin{cases} e_{7(j+m)+4} \otimes e_{7j}, & i = j; \\ 0, & \text{otherwise.} \end{cases}$$

*If  $2s \leq j < 3s$ , then*

$$b_{ij} = \begin{cases} e_{7(j+m)+2} \otimes e_{7j+1}, & i = j; \\ 0, & \text{otherwise.} \end{cases}$$

If  $3s \leq j < 4s$ , then

$$b_{ij} = \begin{cases} e_{7(j+m)+3} \otimes e_{7j+2}, & i = j; \\ 0, & \text{otherwise.} \end{cases}$$

If  $4s \leq j < 5s$ , then

$$b_{ij} = \begin{cases} e_{7(j+m)+6} \otimes e_{7j+3}, & i = j; \\ 0, & \text{otherwise.} \end{cases}$$

If  $5s \leq j < 6s$ , then

$$b_{ij} = \begin{cases} e_{7(j+m)+5} \otimes e_{7j+4}, & i = j; \\ 0, & \text{otherwise.} \end{cases}$$

If  $6s \leq j < 7s$ , then

$$b_{ij} = \begin{cases} e_{7(j+m)+6} \otimes e_{7j+5}, & i = j; \\ 0, & \text{otherwise.} \end{cases}$$

If  $7s \leq j < 8s$ , then

$$b_{ij} = \begin{cases} e_{7(j+m+1)} \otimes e_{7j+6}, & i = j; \\ 0, & \text{otherwise.} \end{cases}$$

(3) If  $r_0 = 2$ , then  $\Omega^2(Y_t^{(1)})$  is described with  $(7s \times 7s)$ -matrix with the following elements  $b_{ij}$ :  
If  $0 \leq j < s$ , then

$$b_{ij} = \begin{cases} e_{7(j+m-1)+6} \otimes e_{7j}, & i = j; \\ 0, & \text{otherwise.} \end{cases}$$

If  $s \leq j < 2s$ , then

$$b_{ij} = \begin{cases} e_{7(j+m)+2} \otimes e_{7j+1}, & i = j; \\ 0, & \text{otherwise.} \end{cases}$$

If  $2s \leq j < 3s$ , then

$$b_{ij} = \begin{cases} e_{7(j+m)+3} \otimes e_{7j+2}, & i = j; \\ 0, & \text{otherwise.} \end{cases}$$

If  $3s \leq j < 4s$ , then

$$b_{ij} = \begin{cases} e_{7(j+m)+4} \otimes e_{7j+3}, & i = j; \\ 0, & \text{otherwise.} \end{cases}$$

If  $4s \leq j < 5s$ , then

$$b_{ij} = \begin{cases} e_{7(j+m)+5} \otimes e_{7j+4}, & i = j; \\ 0, & \text{otherwise.} \end{cases}$$

If  $5s \leq j < 6s$ , then

$$b_{ij} = \begin{cases} e_{7(j+m)+1} \otimes e_{7j+5}, & i = j; \\ 0, & \text{otherwise.} \end{cases}$$

If  $6s \leq j < 7s$ , then

$$b_{ij} = \begin{cases} e_{7(j+m+1)} \otimes e_{7j+6}, & i = j; \\ 0, & \text{otherwise.} \end{cases}$$

(4) If  $r_0 = 3$ , then  $\Omega^3(Y_t^{(1)})$  is described with  $(9s \times 9s)$ -matrix with the following elements  $b_{ij}$ :

If  $0 \leq j < s$ , then

$$b_{ij} = \begin{cases} e_{7(j+m)+2} \otimes e_{7j}, & i = j; \\ 0, & \text{otherwise.} \end{cases}$$

If  $s \leq j < 2s$ , then

$$b_{ij} = \begin{cases} e_{7(j+m)+5} \otimes e_{7j}, & i = j; \\ 0, & \text{otherwise.} \end{cases}$$

If  $2s \leq j < 3s$ , then

$$b_{ij} = \begin{cases} e_{7(j+m)+3} \otimes e_{7j+1}, & i = j; \\ 0, & \text{otherwise.} \end{cases}$$

If  $3s \leq j < 4s$ , then

$$b_{ij} = \begin{cases} e_{7(j+m)+6} \otimes e_{7j+2}, & i = j; \\ 0, & \text{otherwise.} \end{cases}$$

If  $4s \leq j < 5s$ , then

$$b_{ij} = \begin{cases} e_{7(j+m+1)} \otimes e_{7j+3}, & i = j; \\ 0, & \text{otherwise.} \end{cases}$$

If  $5s \leq j < 6s$ , then

$$b_{ij} = \begin{cases} e_{7(j+m)+6} \otimes e_{7j+4}, & i = j; \\ 0, & \text{otherwise.} \end{cases}$$

If  $6s \leq j < 7s$ , then

$$b_{ij} = \begin{cases} e_{7(j+m+1)} \otimes e_{7j+5}, & i = j; \\ 0, & \text{otherwise.} \end{cases}$$

If  $7s \leq j < 8s$ , then

$$b_{ij} = \begin{cases} e_{7(j+m+1)+1} \otimes e_{7j+6}, & i = j; \\ 0, & \text{otherwise.} \end{cases}$$

If  $8s \leq j < 9s$ , then

$$b_{ij} = \begin{cases} e_{7(j+m+1)+4} \otimes e_{7j+6}, & i = j; \\ 0, & \text{otherwise.} \end{cases}$$

(5) If  $r_0 = 4$ , then  $\Omega^4(Y_t^{(1)})$  is described with  $(10s \times 10s)$ -matrix with the following elements  $b_{ij}$ :

If  $0 \leq j < s$ , then

$$b_{ij} = \begin{cases} e_{7(j+m-1)+6} \otimes e_{7j}, & i = j; \\ 0, & \text{otherwise.} \end{cases}$$

If  $s \leq j < 2s$ , then

$$b_{ij} = \begin{cases} e_{7(j+m)} \otimes e_{7j}, & i = j; \\ 0, & \text{otherwise.} \end{cases}$$

If  $2s \leq j < 3s$ , then

$$b_{ij} = \begin{cases} e_{7(j+m)+3} \otimes e_{7j+1}, & i = j; \\ 0, & \text{otherwise.} \end{cases}$$

If  $3s \leq j < 4s$ , then

$$b_{ij} = \begin{cases} e_{7(j+m)+4} \otimes e_{7j+2}, & i = j; \\ 0, & \text{otherwise.} \end{cases}$$

If  $4s \leq j < 5s$ , then

$$b_{ij} = \begin{cases} e_{7(j+m)+1} \otimes e_{7j+3}, & i = j; \\ 0, & \text{otherwise.} \end{cases}$$

If  $5s \leq j < 6s$ , then

$$b_{ij} = \begin{cases} e_{7(j+m)+5} \otimes e_{7j+3}, & i = j; \\ 0, & \text{otherwise.} \end{cases}$$

If  $6s \leq j < 7s$ , then

$$b_{ij} = \begin{cases} e_{7(j+m)+1} \otimes e_{7j+4}, & i = j; \\ 0, & \text{otherwise.} \end{cases}$$

If  $7s \leq j < 8s$ , then

$$b_{ij} = \begin{cases} e_{7(j+m)+2} \otimes e_{7j+5}, & i = j; \\ 0, & \text{otherwise.} \end{cases}$$

If  $8s \leq j < 9s$ , then

$$b_{ij} = \begin{cases} e_{7(j+m)+4} \otimes e_{7j+5}, & i = j; \\ 0, & \text{otherwise.} \end{cases}$$

If  $9s \leq j < 10s$ , then

$$b_{ij} = \begin{cases} e_{7(j+m)+6} \otimes e_{7j+6}, & i = j; \\ 0, & \text{otherwise.} \end{cases}$$

(6) If  $r_0 = 5$ , then  $\Omega^5(Y_t^{(1)})$  is described with  $(10s \times 10s)$ -matrix with the following elements  $b_{ij}$ :

If  $0 \leq j < s$ , then

$$b_{ij} = \begin{cases} e_{7(j+m)+4} \otimes e_{7j}, & i = j; \\ 0, & \text{otherwise.} \end{cases}$$

If  $s \leq j < 2s$ , then

$$b_{ij} = \begin{cases} e_{7(j+m)+3} \otimes e_{7j}, & i = j; \\ 0, & \text{otherwise.} \end{cases}$$

If  $2s \leq j < 3s$ , then

$$b_{ij} = \begin{cases} e_{7(j+m)+1} \otimes e_{7j}, & i = j; \\ 0, & \text{otherwise.} \end{cases}$$

If  $3s \leq j < 4s$ , then

$$b_{ij} = \begin{cases} e_{7(j+m)+6} \otimes e_{7j+1}, & i = j; \\ 0, & \text{otherwise.} \end{cases}$$

If  $4s \leq j < 5s$ , then

$$b_{ij} = \begin{cases} e_{7(j+m+1)} \otimes e_{7j+2}, & i = j; \\ 0, & \text{otherwise.} \end{cases}$$

If  $5s \leq j < 6s$ , then

$$b_{ij} = \begin{cases} e_{7(j+m)+6} \otimes e_{7j+3}, & i = j; \\ 0, & \text{otherwise.} \end{cases}$$

If  $6s \leq j < 7s$ , then

$$b_{ij} = \begin{cases} e_{7(j+m+1)} \otimes e_{7j+4}, & i = j; \\ 0, & \text{otherwise.} \end{cases}$$

If  $7s \leq j < 8s$ , then

$$b_{ij} = \begin{cases} e_{7(j+m)+6} \otimes e_{7j+5}, & i = j; \\ 0, & \text{otherwise.} \end{cases}$$

If  $8s \leq j < 9s$ , then

$$b_{ij} = \begin{cases} e_{7(j+m+1)+2} \otimes e_{7j+6}, & i = j; \\ 0, & \text{otherwise.} \end{cases}$$

If  $9s \leq j < 10s$ , then

$$b_{ij} = \begin{cases} e_{7(j+m+1)+5} \otimes e_{7j+6}, & i = j; \\ 0, & \text{otherwise.} \end{cases}$$

(7) If  $r_0 = 6$ , then  $\Omega^6(Y_t^{(1)})$  is described with  $(12s \times 12s)$ -matrix with the following elements  $b_{ij}$ :

If  $0 \leq j < s$ , then

$$b_{ij} = \begin{cases} e_{7(j+m-1)+6} \otimes e_{7j}, & i = j; \\ 0, & \text{otherwise.} \end{cases}$$

If  $s \leq j < 2s$ , then

$$b_{ij} = \begin{cases} e_{7(j+m)} \otimes e_{7j}, & i = j; \\ 0, & \text{otherwise.} \end{cases}$$

If  $2s \leq j < 3s$ , then

$$b_{ij} = \begin{cases} e_{7(j+m)+4} \otimes e_{7j+1}, & i = j; \\ 0, & \text{otherwise.} \end{cases}$$

If  $3s \leq j < 4s$ , then

$$b_{ij} = \begin{cases} e_{7(j+m)+1} \otimes e_{7j+2}, & i = j; \\ 0, & \text{otherwise.} \end{cases}$$

If  $4s \leq j < 5s$ , then

$$b_{ij} = \begin{cases} e_{7(j+m)+5} \otimes e_{7j+2}, & i = j; \\ 0, & \text{otherwise.} \end{cases}$$

If  $5s \leq j < 6s$ , then

$$b_{ij} = \begin{cases} e_{7(j+m)+2} \otimes e_{7j+3}, & i = j; \\ 0, & \text{otherwise.} \end{cases}$$

If  $6s \leq j < 7s$ , then

$$b_{ij} = \begin{cases} e_{7(j+m)+2} \otimes e_{7j+4}, & i = j; \\ 0, & \text{otherwise.} \end{cases}$$

If  $7s \leq j < 8s$ , then

$$b_{ij} = \begin{cases} e_{7(j+m)+4} \otimes e_{7j+4}, & i = j; \\ 0, & \text{otherwise.} \end{cases}$$

If  $8s \leq j < 9s$ , then

$$b_{ij} = \begin{cases} e_{7(j+m)+3} \otimes e_{7j+5}, & i = j; \\ 0, & \text{otherwise.} \end{cases}$$

If  $9s \leq j < 10s$ , then

$$b_{ij} = \begin{cases} e_{7(j+m)+5} \otimes e_{7j+5}, & i = j; \\ 0, & \text{otherwise.} \end{cases}$$

If  $10s \leq j < 11s$ , then

$$b_{ij} = \begin{cases} e_{7(j+m)+6} \otimes e_{7j+6}, & i = j; \\ 0, & \text{otherwise.} \end{cases}$$

If  $11s \leq j < 12s$ , then

$$b_{ij} = \begin{cases} e_{7(j+m+1)} \otimes e_{7j+6}, & i = j; \\ 0, & \text{otherwise.} \end{cases}$$

(8) If  $r_0 = 7$ , then  $\Omega^7(Y_t^{(1)})$  is described with  $(12s \times 12s)$ -matrix with the following elements  $b_{ij}$ :

If  $0 \leq j < s$ , then

$$b_{ij} = \begin{cases} e_{7(j+m)+2} \otimes e_{7j}, & i = j; \\ 0, & \text{otherwise.} \end{cases}$$

If  $s \leq j < 2s$ , then

$$b_{ij} = \begin{cases} e_{7(j+m)+5} \otimes e_{7j}, & i = j; \\ 0, & \text{otherwise.} \end{cases}$$

If  $2s \leq j < 3s$ , then

$$b_{ij} = \begin{cases} e_{7(j+m)+4} \otimes e_{7j}, & i = j; \\ 0, & \text{otherwise.} \end{cases}$$

If  $3s \leq j < 4s$ , then

$$b_{ij} = \begin{cases} e_{7(j+m+1)} \otimes e_{7j+1}, & i = j; \\ 0, & \text{otherwise.} \end{cases}$$

If  $4s \leq j < 5s$ , then

$$b_{ij} = \begin{cases} e_{7(j+m)+6} \otimes e_{7j+2}, & i = j; \\ 0, & \text{otherwise.} \end{cases}$$

If  $5s \leq j < 6s$ , then

$$b_{ij} = \begin{cases} e_{7(j+m+1)} \otimes e_{7j+3}, & i = j; \\ 0, & \text{otherwise.} \end{cases}$$

If  $6s \leq j < 7s$ , then

$$b_{ij} = \begin{cases} e_{7(j+m)+6} \otimes e_{7j+4}, & i = j; \\ 0, & \text{otherwise.} \end{cases}$$

If  $7s \leq j < 8s$ , then

$$b_{ij} = \begin{cases} e_{7(j+m)+6} \otimes e_{7j+5}, & i = j; \\ 0, & \text{otherwise.} \end{cases}$$

If  $8s \leq j < 9s$ , then

$$b_{ij} = \begin{cases} e_{7(j+m+1)} \otimes e_{7j+5}, & i = j; \\ 0, & \text{otherwise.} \end{cases}$$

If  $9s \leq j < 10s$ , then

$$b_{ij} = \begin{cases} e_{7(j+m+1)+4} \otimes e_{7j+6}, & i = j; \\ 0, & \text{otherwise.} \end{cases}$$

If  $10s \leq j < 11s$ , then

$$b_{ij} = \begin{cases} e_{7(j+m+1)+3} \otimes e_{7j+6}, & i = j; \\ 0, & \text{otherwise.} \end{cases}$$

If  $11s \leq j < 12s$ , then

$$b_{ij} = \begin{cases} e_{7(j+m+1)+1} \otimes e_{7j+6}, & i = j; \\ 0, & \text{otherwise.} \end{cases}$$

(9) If  $r_0 = 8$ , then  $\Omega^8(Y_t^{(1)})$  is described with  $(13s \times 13s)$ -matrix with the following elements  $b_{ij}$ :

If  $0 \leq j < s$ , then

$$b_{ij} = \begin{cases} e_{7(j+m-1)+6} \otimes e_{7j}, & i = j; \\ 0, & \text{otherwise.} \end{cases}$$

If  $s \leq j < 2s$ , then

$$b_{ij} = \begin{cases} e_{7(j+m)} \otimes e_{7j}, & i = j; \\ 0, & \text{otherwise.} \end{cases}$$

If  $2s \leq j < 3s$ , then

$$b_{ij} = \begin{cases} e_{7(j+m)+1} \otimes e_{7j+1}, & i = j; \\ 0, & \text{otherwise.} \end{cases}$$

If  $3s \leq j < 4s$ , then

$$b_{ij} = \begin{cases} e_{7(j+m)+5} \otimes e_{7j+1}, & i = j; \\ 0, & \text{otherwise.} \end{cases}$$

If  $4s \leq j < 5s$ , then

$$b_{ij} = \begin{cases} e_{7(j+m)+2} \otimes e_{7j+2}, & i = j; \\ 0, & \text{otherwise.} \end{cases}$$

If  $5s \leq j < 6s$ , then

$$b_{ij} = \begin{cases} e_{7(j+m)+3} \otimes e_{7j+3}, & i = j; \\ 0, & \text{otherwise.} \end{cases}$$

If  $6s \leq j < 7s$ , then

$$b_{ij} = \begin{cases} e_{7(j+m)+4} \otimes e_{7j+3}, & i = j; \\ 0, & \text{otherwise.} \end{cases}$$

If  $7s \leq j < 8s$ , then

$$b_{ij} = \begin{cases} e_{7(j+m)+3} \otimes e_{7j+4}, & i = j; \\ 0, & \text{otherwise.} \end{cases}$$

If  $8s \leq j < 9s$ , then

$$b_{ij} = \begin{cases} e_{7(j+m)+5} \otimes e_{7j+4}, & i = j; \\ 0, & \text{otherwise.} \end{cases}$$

If  $9s \leq j < 10s$ , then

$$b_{ij} = \begin{cases} e_{7(j+m)+4} \otimes e_{7j+5}, & i = j; \\ 0, & \text{otherwise.} \end{cases}$$

If  $10s \leq j < 11s$ , then

$$b_{ij} = \begin{cases} e_{7(j+m)+1} \otimes e_{7j+5}, & i = j; \\ 0, & \text{otherwise.} \end{cases}$$

If  $11s \leq j < 12s$ , then

$$b_{ij} = \begin{cases} e_{7(j+m)+6} \otimes e_{7j+6}, & i = j; \\ 0, & \text{otherwise.} \end{cases}$$

If  $12s \leq j < 13s$ , then

$$b_{ij} = \begin{cases} e_{7(j+m+1)} \otimes e_{7j+6}, & i = j; \\ 0, & \text{otherwise.} \end{cases}$$

(10) If  $r_0 = 9$ , then  $\Omega^9(Y_t^{(1)})$  is described with  $(12s \times 12s)$ -matrix with the following elements  $b_{ij}$ :

If  $0 \leq j < s$ , then

$$b_{ij} = \begin{cases} e_{7(j+m)+5} \otimes e_{7j}, & i = j; \\ 0, & \text{otherwise.} \end{cases}$$

If  $s \leq j < 2s$ , then

$$b_{ij} = \begin{cases} e_{7(j+m)+3} \otimes e_{7j}, & i = j; \\ 0, & \text{otherwise.} \end{cases}$$

If  $2s \leq j < 3s$ , then

$$b_{ij} = \begin{cases} e_{7(j+m)+1} \otimes e_{7j}, & i = j; \\ 0, & \text{otherwise.} \end{cases}$$

If  $3s \leq j < 4s$ , then

$$b_{ij} = \begin{cases} e_{7(j+m)+6} \otimes e_{7j+1}, & i = j; \\ 0, & \text{otherwise.} \end{cases}$$

If  $4s \leq j < 5s$ , then

$$b_{ij} = \begin{cases} e_{7(j+m+1)} \otimes e_{7j+2}, & i = j; \\ 0, & \text{otherwise.} \end{cases}$$



If  $5s \leq j < 6s$ , then

$$b_{ij} = \begin{cases} e_{7(j+m)+6} \otimes e_{7j+3}, & i = j; \\ 0, & \text{otherwise.} \end{cases}$$

If  $6s \leq j < 7s$ , then

$$b_{ij} = \begin{cases} e_{7(j+m)+6} \otimes e_{7j+4}, & i = j; \\ 0, & \text{otherwise.} \end{cases}$$

If  $7s \leq j < 8s$ , then

$$b_{ij} = \begin{cases} e_{7(j+m+1)} \otimes e_{7j+4}, & i = j; \\ 0, & \text{otherwise.} \end{cases}$$

If  $8s \leq j < 9s$ , then

$$b_{ij} = \begin{cases} e_{7(j+m+1)} \otimes e_{7j+5}, & i = j; \\ 0, & \text{otherwise.} \end{cases}$$

If  $9s \leq j < 10s$ , then

$$b_{ij} = \begin{cases} e_{7(j+m+1)+2} \otimes e_{7j+6}, & i = j; \\ 0, & \text{otherwise.} \end{cases}$$

If  $10s \leq j < 11s$ , then

$$b_{ij} = \begin{cases} e_{7(j+m+1)+5} \otimes e_{7j+6}, & i = j; \\ 0, & \text{otherwise.} \end{cases}$$

If  $11s \leq j < 12s$ , then

$$b_{ij} = \begin{cases} e_{7(j+m+1)+4} \otimes e_{7j+6}, & i = j; \\ 0, & \text{otherwise.} \end{cases}$$

(11) If  $r_0 = 10$ , then  $\Omega^{10}(Y_t^{(1)})$  is described with  $(12s \times 12s)$ -matrix with the following elements  $b_{ij}$ :

If  $0 \leq j < s$ , then

$$b_{ij} = \begin{cases} e_{7(j+m-1)+6} \otimes e_{7j}, & i = j; \\ 0, & \text{otherwise.} \end{cases}$$

If  $s \leq j < 2s$ , then

$$b_{ij} = \begin{cases} e_{7(j+m)} \otimes e_{7j}, & i = j; \\ 0, & \text{otherwise.} \end{cases}$$

If  $2s \leq j < 3s$ , then

$$b_{ij} = \begin{cases} e_{7(j+m)+2} \otimes e_{7j+1}, & i = j; \\ 0, & \text{otherwise.} \end{cases}$$

If  $3s \leq j < 4s$ , then

$$b_{ij} = \begin{cases} e_{7(j+m)+3} \otimes e_{7j+2}, & i = j; \\ 0, & \text{otherwise.} \end{cases}$$

If  $4s \leq j < 5s$ , then

$$b_{ij} = \begin{cases} e_{7(j+m)+4} \otimes e_{7j+2}, & i = j; \\ 0, & \text{otherwise.} \end{cases}$$

If  $5s \leq j < 6s$ , then

$$b_{ij} = \begin{cases} e_{7(j+m)+5} \otimes e_{7j+3}, & i = j; \\ 0, & \text{otherwise.} \end{cases}$$

If  $6s \leq j < 7s$ , then

$$b_{ij} = \begin{cases} e_{7(j+m)+4} \otimes e_{7j+4}, & i = j; \\ 0, & \text{otherwise.} \end{cases}$$

If  $7s \leq j < 8s$ , then

$$b_{ij} = \begin{cases} e_{7(j+m)+1} \otimes e_{7j+4}, & i = j; \\ 0, & \text{otherwise.} \end{cases}$$

If  $8s \leq j < 9s$ , then

$$b_{ij} = \begin{cases} e_{7(j+m)+2} \otimes e_{7j+5}, & i = j; \\ 0, & \text{otherwise.} \end{cases}$$

If  $9s \leq j < 10s$ , then

$$b_{ij} = \begin{cases} e_{7(j+m)+5} \otimes e_{7j+5}, & i = j; \\ 0, & \text{otherwise.} \end{cases}$$

If  $10s \leq j < 11s$ , then

$$b_{ij} = \begin{cases} e_{7(j+m)+6} \otimes e_{7j+6}, & i = j; \\ 0, & \text{otherwise.} \end{cases}$$

If  $11s \leq j < 12s$ , then

$$b_{ij} = \begin{cases} e_{7(j+m+1)} \otimes e_{7j+6}, & i = j; \\ 0, & \text{otherwise.} \end{cases}$$

(12) If  $r_0 = 11$ , then  $\Omega^{11}(Y_t^{(1)})$  is described with  $(10s \times 10s)$ -matrix with the following elements  $b_{ij}$ :

If  $0 \leq j < s$ , then

$$b_{ij} = \begin{cases} e_{7(j+m)+2} \otimes e_{7j}, & i = j; \\ 0, & \text{otherwise.} \end{cases}$$

If  $s \leq j < 2s$ , then

$$b_{ij} = \begin{cases} e_{7(j+m)+4} \otimes e_{7j}, & i = j; \\ 0, & \text{otherwise.} \end{cases}$$

If  $2s \leq j < 3s$ , then

$$b_{ij} = \begin{cases} e_{7(j+m+1)} \otimes e_{7j+1}, & i = j; \\ 0, & \text{otherwise.} \end{cases}$$

If  $3s \leq j < 4s$ , then

$$b_{ij} = \begin{cases} e_{7(j+m)+6} \otimes e_{7j+2}, & i = j; \\ 0, & \text{otherwise.} \end{cases}$$

If  $4s \leq j < 5s$ , then

$$b_{ij} = \begin{cases} e_{7(j+m+1)} \otimes e_{7j+3}, & i = j; \\ 0, & \text{otherwise.} \end{cases}$$

If  $5s \leq j < 6s$ , then

$$b_{ij} = \begin{cases} e_{7(j+m+1)} \otimes e_{7j+4}, & i = j; \\ 0, & \text{otherwise.} \end{cases}$$

If  $6s \leq j < 7s$ , then

$$b_{ij} = \begin{cases} e_{7(j+m)+6} \otimes e_{7j+5}, & i = j; \\ 0, & \text{otherwise.} \end{cases}$$

If  $7s \leq j < 8s$ , then

$$b_{ij} = \begin{cases} e_{7(j+m+1)+5} \otimes e_{7j+6}, & i = j; \\ 0, & \text{otherwise.} \end{cases}$$

If  $8s \leq j < 9s$ , then

$$b_{ij} = \begin{cases} e_{7(j+m+1)+3} \otimes e_{7j+6}, & i = j; \\ 0, & \text{otherwise.} \end{cases}$$

If  $9s \leq j < 10s$ , then

$$b_{ij} = \begin{cases} e_{7(j+m+1)+1} \otimes e_{7j+6}, & i = j; \\ 0, & \text{otherwise.} \end{cases}$$

(13) If  $r_0 = 12$ , then  $\Omega^{12}(Y_t^{(1)})$  is described with  $(10s \times 10s)$ -matrix with the following elements  $b_{ij}$ :

If  $0 \leq j < s$ , then

$$b_{ij} = \begin{cases} e_{7(j+m)} \otimes e_{7j}, & i = j; \\ 0, & \text{otherwise.} \end{cases}$$

If  $s \leq j < 2s$ , then

$$b_{ij} = \begin{cases} e_{7(j+m)+3} \otimes e_{7j+1}, & i = j; \\ 0, & \text{otherwise.} \end{cases}$$

If  $2s \leq j < 3s$ , then

$$b_{ij} = \begin{cases} e_{7(j+m)+4} \otimes e_{7j+1}, & i = j; \\ 0, & \text{otherwise.} \end{cases}$$

If  $3s \leq j < 4s$ , then

$$b_{ij} = \begin{cases} e_{7(j+m)+5} \otimes e_{7j+2}, & i = j; \\ 0, & \text{otherwise.} \end{cases}$$

If  $4s \leq j < 5s$ , then

$$b_{ij} = \begin{cases} e_{7(j+m)+1} \otimes e_{7j+3}, & i = j; \\ 0, & \text{otherwise.} \end{cases}$$

If  $5s \leq j < 6s$ , then

$$b_{ij} = \begin{cases} e_{7(j+m)+2} \otimes e_{7j+4}, & i = j; \\ 0, & \text{otherwise.} \end{cases}$$

If  $6s \leq j < 7s$ , then

$$b_{ij} = \begin{cases} e_{7(j+m)+5} \otimes e_{7j+4}, & i = j; \\ 0, & \text{otherwise.} \end{cases}$$

If  $7s \leq j < 8s$ , then

$$b_{ij} = \begin{cases} e_{7(j+m)+3} \otimes e_{7j+5}, & i = j; \\ 0, & \text{otherwise.} \end{cases}$$

If  $8s \leq j < 9s$ , then

$$b_{ij} = \begin{cases} e_{7(j+m)+6} \otimes e_{7j+6}, & i = j; \\ 0, & \text{otherwise.} \end{cases}$$

If  $9s \leq j < 10s$ , then

$$b_{ij} = \begin{cases} e_{7(j+m+1)} \otimes e_{7j+6}, & i = j; \\ 0, & \text{otherwise.} \end{cases}$$

(14) If  $r_0 = 13$ , then  $\Omega^{13}(Y_t^{(1)})$  is described with  $(9s \times 9s)$ -matrix with the following elements  $b_{ij}$ :

If  $0 \leq j < s$ , then

$$b_{ij} = \begin{cases} e_{7(j+m)+3} \otimes e_{7j}, & i = j; \\ 0, & \text{otherwise.} \end{cases}$$

If  $s \leq j < 2s$ , then

$$b_{ij} = \begin{cases} e_{7(j+m)+5} \otimes e_{7j}, & i = j; \\ 0, & \text{otherwise.} \end{cases}$$

If  $2s \leq j < 3s$ , then

$$b_{ij} = \begin{cases} e_{7(j+m)+6} \otimes e_{7j+1}, & i = j; \\ 0, & \text{otherwise.} \end{cases}$$

If  $3s \leq j < 4s$ , then

$$b_{ij} = \begin{cases} e_{7(j+m+1)} \otimes e_{7j+2}, & i = j; \\ 0, & \text{otherwise.} \end{cases}$$

If  $4s \leq j < 5s$ , then

$$b_{ij} = \begin{cases} e_{7(j+m+1)+1} \otimes e_{7j+3}, & i = j; \\ 0, & \text{otherwise.} \end{cases}$$

If  $5s \leq j < 6s$ , then

$$b_{ij} = \begin{cases} e_{7(j+m)+6} \otimes e_{7j+4}, & i = j; \\ 0, & \text{otherwise.} \end{cases}$$

If  $6s \leq j < 7s$ , then

$$b_{ij} = \begin{cases} e_{7(j+m+1)} \otimes e_{7j+5}, & i = j; \\ 0, & \text{otherwise.} \end{cases}$$

If  $7s \leq j < 8s$ , then

$$b_{ij} = \begin{cases} e_{7(j+m+1)+2} \otimes e_{7j+6}, & i = j; \\ 0, & \text{otherwise.} \end{cases}$$

If  $8s \leq j < 9s$ , then

$$b_{ij} = \begin{cases} e_{7(j+m+1)+4} \otimes e_{7j+6}, & i = j; \\ 0, & \text{otherwise.} \end{cases}$$

(15) If  $r_0 = 14$ , then  $\Omega^{14}(Y_t^{(1)})$  is described with  $(7s \times 7s)$ -matrix with the following elements  $b_{ij}$ :

If  $0 \leq j < s$ , then

$$b_{ij} = \begin{cases} e_{7(j+m-1)+6} \otimes e_{7j}, & i = j; \\ 0, & \text{otherwise.} \end{cases}$$

If  $s \leq j < 2s$ , then

$$b_{ij} = \begin{cases} e_{7(j+m)+5} \otimes e_{7j+1}, & i = j; \\ 0, & \text{otherwise.} \end{cases}$$

If  $2s \leq j < 3s$ , then

$$b_{ij} = \begin{cases} e_{7(j+m)+1} \otimes e_{7j+2}, & i = j; \\ 0, & \text{otherwise.} \end{cases}$$

If  $3s \leq j < 4s$ , then

$$b_{ij} = \begin{cases} e_{7(j+m)+2} \otimes e_{7j+3}, & i = j; \\ 0, & \text{otherwise.} \end{cases}$$

If  $4s \leq j < 5s$ , then

$$b_{ij} = \begin{cases} e_{7(j+m)+3} \otimes e_{7j+4}, & i = j; \\ 0, & \text{otherwise.} \end{cases}$$

If  $5s \leq j < 6s$ , then

$$b_{ij} = \begin{cases} e_{7(j+m)+4} \otimes e_{7j+5}, & i = j; \\ 0, & \text{otherwise.} \end{cases}$$

If  $6s \leq j < 7s$ , then

$$b_{ij} = \begin{cases} e_{7(j+m+1)} \otimes e_{7j+6}, & i = j; \\ 0, & \text{otherwise.} \end{cases}$$

(16) If  $r_0 = 15$ , then  $\Omega^{15}(Y_t^{(1)})$  is described with  $(8s \times 8s)$ -matrix with the following elements  $b_{ij}$ :

If  $0 \leq j < s$ , then

$$b_{ij} = \begin{cases} e_{7(j+m)+6} \otimes e_{7j}, & i = j; \\ 0, & \text{otherwise.} \end{cases}$$

If  $s \leq j < 2s$ , then

$$b_{ij} = \begin{cases} e_{7(j+m+1)} \otimes e_{7j+1}, & i = j; \\ 0, & \text{otherwise.} \end{cases}$$

If  $2s \leq j < 3s$ , then

$$b_{ij} = \begin{cases} e_{7(j+m+1)+1} \otimes e_{7j+2}, & i = j; \\ 0, & \text{otherwise.} \end{cases}$$

If  $3s \leq j < 4s$ , then

$$b_{ij} = \begin{cases} e_{7(j+m+1)+2} \otimes e_{7j+3}, & i = j; \\ 0, & \text{otherwise.} \end{cases}$$

If  $4s \leq j < 5s$ , then

$$b_{ij} = \begin{cases} e_{7(j+m+1)} \otimes e_{7j+4}, & i = j; \\ 0, & \text{otherwise.} \end{cases}$$

If  $5s \leq j < 6s$ , then

$$b_{ij} = \begin{cases} e_{7(j+m+1)+4} \otimes e_{7j+5}, & i = j; \\ 0, & \text{otherwise.} \end{cases}$$

If  $6s \leq j < 7s$ , then

$$b_{ij} = \begin{cases} e_{7(j+m+1)+3} \otimes e_{7j+6}, & i = j; \\ 0, & \text{otherwise.} \end{cases}$$

If  $7s \leq j < 8s$ , then

$$b_{ij} = \begin{cases} e_{7(j+m+1)+5} \otimes e_{7j+6}, & i = j; \\ 0, & \text{otherwise.} \end{cases}$$

(17) If  $r_0 = 16$ , then  $\Omega^{16}(Y_t^{(1)})$  is described with  $(7s \times 7s)$ -matrix with the following elements  $b_{ij}$ :

If  $0 \leq j < s$ , then

$$b_{ij} = \begin{cases} e_{7(j+m)} \otimes e_{7j}, & i = j; \\ 0, & \text{otherwise.} \end{cases}$$

If  $s \leq j < 2s$ , then

$$b_{ij} = \begin{cases} e_{7(j+m)+1} \otimes e_{7j+1}, & i = j; \\ 0, & \text{otherwise.} \end{cases}$$

If  $2s \leq j < 3s$ , then

$$b_{ij} = \begin{cases} e_{7(j+m)+2} \otimes e_{7j+2}, & i = j; \\ 0, & \text{otherwise.} \end{cases}$$

If  $3s \leq j < 4s$ , then

$$b_{ij} = \begin{cases} e_{7(j+m)+3} \otimes e_{7j+3}, & i = j; \\ 0, & \text{otherwise.} \end{cases}$$

If  $4s \leq j < 5s$ , then

$$b_{ij} = \begin{cases} e_{7(j+m)+4} \otimes e_{7j+4}, & i = j; \\ 0, & \text{otherwise.} \end{cases}$$

If  $5s \leq j < 6s$ , then

$$b_{ij} = \begin{cases} e_{7(j+m)+5} \otimes e_{7j+5}, & i = j; \\ 0, & \text{otherwise.} \end{cases}$$

If  $6s \leq j < 7s$ , then

$$b_{ij} = \begin{cases} e_{7(j+m)+6} \otimes e_{7j+6}, & i = j; \\ 0, & \text{otherwise.} \end{cases}$$

(II) Represent an arbitrary  $t_0 \in \mathbb{N}$  in the form  $t_0 = 17\ell_0 + r_0$ , where  $0 \leq r_0 \leq 16$ . Then  $\Omega^{t_0}(Y_t^{(1)})$  is a  $\Omega^{r_0}(Y_t^{(1)})$ , whose left components twisted by  $\sigma^{\ell_0}$ .

**Proposition 2** (Translates for the case 2). (I) Let  $r_0 \in \mathbb{N}$ ,  $r_0 < 17$ .  $r_0$ -translates of the elements  $Y_t^{(2)}$  are described by the following way.

(1) If  $r_0 = 0$ , then  $\Omega^0(Y_t^{(2)})$  is described with  $(7s \times 7s)$ -matrix with one nonzero element that is of the following form:

$$b_{j,(9)_s} = w_{7(j+m) \rightarrow 7(j+m+1)} \otimes e_{7j}.$$

(2) If  $r_0 = 1$ , then  $\Omega^1(Y_t^{(2)})$  is described with  $(8s \times 8s)$ -matrix with one nonzero element that is of the following form:

$$b_{j,7s+(8)_s} = w_{7(j+m+1) \rightarrow 7(j+m+2)} \otimes e_{7j+6}.$$

(3) If  $r_0 = 2$ , then  $\Omega^2(Y_t^{(2)})$  is described with  $(7s \times 7s)$ -matrix with one nonzero element that is of the following form:

$$b_{j,6s+(7)_s} = w_{7(j+m+1) \rightarrow 7(j+m+2)} \otimes e_{7j+6}.$$

(4) If  $r_0 = 3$ , then  $\Omega^3(Y_t^{(2)})$  is described with  $(9s \times 9s)$ -matrix with the following two nonzero elements:

$$b_{j,4s+(7)_s} = w_{7(j+m+1) \rightarrow 7(j+m+2)} \otimes e_{7j+3};$$

$$b_{j,6s+(7)_s} = w_{7(j+m+1) \rightarrow 7(j+m+2)} \otimes e_{7j+5}.$$

(5) If  $r_0 = 4$ , then  $\Omega^4(Y_t^{(2)})$  is described with  $(10s \times 10s)$ -matrix with one nonzero element that is of the following form:

$$b_{j,s+(7)_s} = w_{7(j+m) \rightarrow 7(j+m+1)} \otimes e_{7j}.$$

(6) If  $r_0 = 5$ , then  $\Omega^5(Y_t^{(2)})$  is described with  $(10s \times 10s)$ -matrix with the following two nonzero elements:

$$b_{j,4s+(6)_s} = w_{7(j+m+1) \rightarrow 7(j+m+2)} \otimes e_{7j+2};$$

$$b_{j,6s+(6)_s} = w_{7(j+m+1) \rightarrow 7(j+m+2)} \otimes e_{7j+4}.$$

(7) If  $r_0 = 6$ , then  $\Omega^6(Y_t^{(2)})$  is described with  $(12s \times 12s)$ -matrix with the following two nonzero elements:

$$b_{j,s+(6)_s} = w_{7(j+m) \rightarrow 7(j+m+1)} \otimes e_{7j};$$

$$b_{j,11s+(5)_s} = w_{7(j+m+1) \rightarrow 7(j+m+2)} \otimes e_{7j+6}.$$

(8) If  $r_0 = 7$ , then  $\Omega^7(Y_t^{(2)})$  is described with  $(12s \times 12s)$ -matrix with the following nonzero elements:

$$b_{j,3s+(5)_s} = w_{7(j+m+1) \rightarrow 7(j+m+2)} \otimes e_{7j+1};$$

$$b_{j,5s+(5)_s} = w_{7(j+m+1) \rightarrow 7(j+m+2)} \otimes e_{7j+3};$$

$$b_{j,8s+(5)_s} = w_{7(j+m+1) \rightarrow 7(j+m+2)} \otimes e_{7j+5}.$$

(9) If  $r_0 = 8$ , then  $\Omega^8(Y_t^{(2)})$  is described with  $(13s \times 13s)$ -matrix with the following two nonzero elements:

$$b_{j,s+(5)_s} = w_{7(j+m) \rightarrow 7(j+m+1)} \otimes e_{7j};$$

$$b_{j,12s+(4)_s} = w_{7(j+m+1) \rightarrow 7(j+m+2)} \otimes e_{7j+6}.$$

(10) If  $r_0 = 9$ , then  $\Omega^9(Y_t^{(2)})$  is described with  $(12s \times 12s)$ -matrix with the following nonzero elements:

$$b_{j,4s+(4)_s} = w_{7(j+m+1) \rightarrow 7(j+m+2)} \otimes e_{7j+2};$$

$$b_{j,7s+(4)_s} = w_{7(j+m+1) \rightarrow 7(j+m+2)} \otimes e_{7j+4};$$

$$b_{j,8s+(4)_s} = w_{7(j+m+1) \rightarrow 7(j+m+2)} \otimes e_{7j+5}.$$

(11) If  $r_0 = 10$ , then  $\Omega^{10}(Y_t^{(2)})$  is described with  $(12s \times 12s)$ -matrix with the following two nonzero elements:

$$\begin{aligned} b_{j,s+(4)_s} &= w_{7(j+m) \rightarrow 7(j+m+1)} \otimes e_{7j}; \\ b_{j,11s+(3)_s} &= w_{7(j+m+1) \rightarrow 7(j+m+2)} \otimes e_{7j+6}. \end{aligned}$$

(12) If  $r_0 = 11$ , then  $\Omega^{11}(Y_t^{(2)})$  is described with  $(10s \times 10s)$ -matrix with the following nonzero elements:

$$\begin{aligned} b_{j,2s+(3)_s} &= w_{7(j+m+1) \rightarrow 7(j+m+2)} \otimes e_{7j+1}; \\ b_{j,4s+(3)_s} &= w_{7(j+m+1) \rightarrow 7(j+m+2)} \otimes e_{7j+3}; \\ b_{j,5s+(3)_s} &= w_{7(j+m+1) \rightarrow 7(j+m+2)} \otimes e_{7j+4}. \end{aligned}$$

(13) If  $r_0 = 12$ , then  $\Omega^{12}(Y_t^{(2)})$  is described with  $(10s \times 10s)$ -matrix with the following two nonzero elements:

$$\begin{aligned} b_{j,(3)_s} &= w_{7(j+m) \rightarrow 7(j+m+1)} \otimes e_{7j}; \\ b_{j,9s+(2)_s} &= w_{7(j+m+1) \rightarrow 7(j+m+2)} \otimes e_{7j+6}. \end{aligned}$$

(14) If  $r_0 = 13$ , then  $\Omega^{13}(Y_t^{(2)})$  is described with  $(9s \times 9s)$ -matrix with the following two nonzero elements:

$$\begin{aligned} b_{j,3s+(2)_s} &= w_{7(j+m+1) \rightarrow 7(j+m+2)} \otimes e_{7j+2}; \\ b_{j,6s+(2)_s} &= w_{7(j+m+1) \rightarrow 7(j+m+2)} \otimes e_{7j+5}. \end{aligned}$$

(15) If  $r_0 = 14$ , then  $\Omega^{14}(Y_t^{(2)})$  is described with  $(7s \times 7s)$ -matrix with one nonzero element that is of the following form:

$$b_{j,6s+(1)_s} = w_{7(j+m+1) \rightarrow 7(j+m+2)} \otimes e_{7j+6}.$$

(16) If  $r_0 = 15$ , then  $\Omega^{15}(Y_t^{(2)})$  is described with  $(8s \times 8s)$ -matrix with the following two nonzero elements:

$$\begin{aligned} b_{j,s+(1)_s} &= w_{7(j+m+1) \rightarrow 7(j+m+2)} \otimes e_{7j+1}; \\ b_{j,4s+(1)_s} &= w_{7(j+m+1) \rightarrow 7(j+m+2)} \otimes e_{7j+4}. \end{aligned}$$

(17) If  $r_0 = 16$ , then  $\Omega^{16}(Y_t^{(2)})$  is described with  $(7s \times 7s)$ -matrix with one nonzero element that is of the following form:

$$b_{j,(1)_s} = w_{7(j+m) \rightarrow 7(j+m+1)} \otimes e_{7j}.$$

(II) Represent an arbitrary  $t_0 \in \mathbb{N}$  in the form  $t_0 = 17\ell_0 + r_0$ , where  $0 \leq r_0 \leq 16$ . Then  $\Omega^{t_0}(Y_t^{(2)})$  is a  $\Omega^{r_0}(Y_t^{(2)})$ , whose left components twisted by  $\sigma^{\ell_0}$ , and coefficients multiplied by  $(-1)^{\ell_0}$ .

**Proposition 3** (Translates for the case 3). (I) Let  $r_0 \in \mathbb{N}$ ,  $r_0 < 17$ .  $r_0$ -translates of the elements  $Y_t^{(3)}$  are described by the following way.

(1) If  $r_0 = 0$ , then  $\Omega^0(Y_t^{(3)})$  is described with  $(7s \times 8s)$ -matrix with the following two nonzero elements:

$$\begin{aligned} b_{j,(2)_s} &= w_{7(j+m) \rightarrow 7(j+m)+1} \otimes e_{7j}; \\ b_{j-s,s+(2)_s} &= w_{7(j+m) \rightarrow 7(j+m)+4} \otimes e_{7j}. \end{aligned}$$

(2) If  $r_0 = 1$ , then  $\Omega^1(Y_t^{(3)})$  is described with  $(8s \times 7s)$ -matrix with the following nonzero elements:

$$b_{(j+1)_s,s+(1)_s} = w_{7(j+m+1)+1 \rightarrow 7(j+m+1)+2} \otimes w_{7j+1 \rightarrow 7(j+1)};$$



$$\begin{aligned}
b_{2s+(j+1)s,s+(1)s} &= e_{7(j+m+1)+2} \otimes w_{7j+1 \rightarrow 7(j+1)+1}; \\
b_{(j+1)s,2s+(1)s} &= w_{7(j+m+1)+1 \rightarrow 7(j+m+1)+3} \otimes w_{7j+2 \rightarrow 7(j+1)}; \\
b_{2s+(j+1)s,2s+(1)s} &= w_{7(j+m+1)+2 \rightarrow 7(j+m+1)+3} \otimes w_{7j+2 \rightarrow 7(j+1)+1}; \\
b_{3s+(j+1)s,2s+(1)s} &= e_{7(j+m+1)+3} \otimes w_{7j+2 \rightarrow 7(j+1)+2}; \\
b_{s+(j+1)s,3s+(1)s} &= e_{7(j+m+1)+4} \otimes w_{7j+3 \rightarrow 7(j+1)}; \\
b_{s+(j+1)s,4s+(1)s} &= w_{7(j+m+1)+4 \rightarrow 7(j+m+1)+5} \otimes w_{7j+4 \rightarrow 7(j+1)}; \\
b_{5s+(j+1)s,4s+(1)s} &= e_{7(j+m+1)+5} \otimes w_{7j+4 \rightarrow 7(j+1)+4}; \\
b_{(j+1)s,5s+(1)s} &= e_{7(j+m+1)+1} \otimes w_{7j+5 \rightarrow 7(j+1)}; \\
b_{j+s,6s+(1)s} &= -w_{7(j+m+1) \rightarrow 7(j+m+2)} \otimes e_{7j+6}.
\end{aligned}$$

(3) If  $r_0 = 2$ , then  $\Omega^2(Y_t^{(3)})$  is described with  $(7s \times 9s)$ -matrix with the following nonzero elements:

$$\begin{aligned}
b_{(j+1)s,3s+(1)s} &= e_{7(j+m)+6} \otimes w_{7j+2 \rightarrow 7(j+1)}; \\
b_{j-s,4s+(1)s} &= w_{7(j+m)+4 \rightarrow 7(j+m+1)} \otimes e_{7j+3}; \\
b_{(j+1)s,5s+(1)s} &= -e_{7(j+m)+6} \otimes w_{7j+4 \rightarrow 7(j+1)}; \\
b_{j-s,6s+(1)s} &= w_{7(j+m)+1 \rightarrow 7(j+m+1)} \otimes e_{7j+5}.
\end{aligned}$$

(4) If  $r_0 = 3$ , then  $\Omega^3(Y_t^{(3)})$  is described with  $(9s \times 10s)$ -matrix with the following nonzero elements:

$$\begin{aligned}
b_{j-s,s+(1)s} &= -w_{7(j+m)+2 \rightarrow 7(j+m+1)} \otimes e_{7j}; \\
b_{j+s,s+(1)s} &= -w_{7(j+m)+3 \rightarrow 7(j+m+1)} \otimes w_{7j \rightarrow 7j+1}; \\
b_{j+2s,s+(1)s} &= -w_{7(j+m)+6 \rightarrow 7(j+m+1)} \otimes w_{7j \rightarrow 7j+2}; \\
b_{(j+1)s,2s+(1)s} &= w_{7(j+m+1)+2 \rightarrow 7(j+m+1)+3} \otimes w_{7j+1 \rightarrow 7(j+1)}; \\
b_{2s+(j+1)s,2s+(1)s} &= e_{7(j+m+1)+3} \otimes w_{7j+1 \rightarrow 7(j+1)+1}; \\
b_{j,3s+(1)s} &= -w_{7(j+m)+6 \rightarrow 7(j+m+1)+4} \otimes e_{7j+2}; \\
b_{j-s,6s+(1)s} &= -w_{7(j+m)+6 \rightarrow 7(j+m+1)+1} \otimes e_{7j+4}.
\end{aligned}$$

(5) If  $r_0 = 4$ , then  $\Omega^4(Y_t^{(3)})$  is described with  $(10s \times 10s)$ -matrix with the following nonzero elements:

$$\begin{aligned}
b_{j-s,s+(1)s} &= w_{7(j+m-1)+6 \rightarrow 7(j+m)+3} \otimes e_{7j}; \\
b_{j+s,s+(1)s} &= -e_{7(j+m)+3} \otimes w_{7j \rightarrow 7j+1}; \\
b_{j-2s,2s+(1)s} &= -w_{7(j+m-1)+6 \rightarrow 7(j+m)+1} \otimes e_{7j}; \\
b_{j-s,3s+(1)s} &= w_{7(j+m)+3 \rightarrow 7(j+m)+6} \otimes e_{7j+1}; \\
b_{(j+1)s,4s} &= w_{7(j+m)+6 \rightarrow 7(j+m+1)} \otimes w_{7j+2 \rightarrow 7(j+1)}; \\
b_{s+(j+1)s,4s} &= e_{7(j+m+1)} \otimes w_{7j+2 \rightarrow 7(j+1)}; \\
b_{(j+1)s,6s} &= -w_{7(j+m)+6 \rightarrow 7(j+m+1)} \otimes w_{7j+4 \rightarrow 7(j+1)}; \\
b_{s+(j+1)s,6s} &= -e_{7(j+m+1)} \otimes w_{7j+4 \rightarrow 7(j+1)}; \\
b_{(j+1)s,8s} &= w_{7(j+m)+6 \rightarrow 7(j+m+1)+2} \otimes w_{7j+6 \rightarrow 7(j+1)}; \\
b_{s+(j+1)s,8s} &= w_{7(j+m+1) \rightarrow 7(j+m+1)+2} \otimes w_{7j+6 \rightarrow 7(j+1)}; \\
b_{4s+(j+1)s,8s} &= -w_{7(j+m+1)+1 \rightarrow 7(j+m+1)+2} \otimes w_{7j+6 \rightarrow 7(j+1)+3}; \\
b_{7s+(j+1)s,8s} &= e_{7(j+m+1)+2} \otimes w_{7j+6 \rightarrow 7(j+1)+5}; \\
b_{3s+(j+1)s,9s} &= w_{7(j+m+1)+4 \rightarrow 7(j+m+1)+5} \otimes w_{7j+6 \rightarrow 7(j+1)+2}; \\
b_{5s+(j+1)s,9s} &= -e_{7(j+m+1)+5} \otimes w_{7j+6 \rightarrow 7(j+1)+3}.
\end{aligned}$$

(6) If  $r_0 = 5$ , then  $\Omega^5(Y_t^{(3)})$  is described with  $(10s \times 12s)$ -matrix with the following nonzero elements:

$$\begin{aligned}
b_{(j+1)s, 2s} &= e_{7(j+m+1)+4} \otimes w_{7j+1 \rightarrow 7(j+1)}; \\
b_{2s+(j+1)s, 3s} &= e_{7(j+m+1)+1} \otimes w_{7j+2 \rightarrow 7(j+1)}; \\
b_{(j+1)s, 4s} &= w_{7(j+m+1)+4 \rightarrow 7(j+m+1)+5} \otimes w_{7j+2 \rightarrow 7(j+1)}; \\
b_{2s+(j+1)s, 5s} &= w_{7(j+m+1)+1 \rightarrow 7(j+m+1)+2} \otimes w_{7j+3 \rightarrow 7(j+1)}; \\
b_{(j+1)s, 7s} &= -e_{7(j+m+1)+4} \otimes w_{7j+4 \rightarrow 7(j+1)}; \\
b_{s+(j+1)s, 8s} &= e_{7(j+m+1)+3} \otimes w_{7j+5 \rightarrow 7(j+1)}; \\
b_{2s+(j+1)s, 8s} &= w_{7(j+m+1)+1 \rightarrow 7(j+m+1)+3} \otimes w_{7j+5 \rightarrow 7(j+1)}; \\
b_{s+(j+1)s, 10s} &= w_{7(j+m+1)+3 \rightarrow 7(j+m+1)+6} \otimes w_{7j+6 \rightarrow 7(j+1)}; \\
b_{2s+(j+1)s, 10s} &= w_{7(j+m+1)+1 \rightarrow 7(j+m+1)+6} \otimes w_{7j+6 \rightarrow 7(j+1)}; \\
b_{3s+(j+1)s, 10s} &= e_{7(j+m+1)+6} \otimes w_{7j+6 \rightarrow 7(j+1)+1}; \\
b_{4s+(j+1)s, 11s} &= e_{7(j+m+2)} \otimes w_{7j+6 \rightarrow 7(j+1)+2}.
\end{aligned}$$

(7) If  $r_0 = 6$ , then  $\Omega^6(Y_t^{(3)})$  is described with  $(12s \times 12s)$ -matrix with the following nonzero elements:

$$\begin{aligned}
b_{(j+1)s, 3s} &= w_{7(j+m)+6 \rightarrow 7(j+m+1)} \otimes w_{7j+1 \rightarrow 7(j+1)}; \\
b_{s+(j+1)s, 3s} &= e_{7(j+m+1)} \otimes w_{7j+1 \rightarrow 7(j+1)}; \\
b_{(j+1)s, 4s} &= -e_{7(j+m)+6} \otimes w_{7j+2 \rightarrow 7(j+1)}; \\
b_{s+(j+1)s, 5s} &= -e_{7(j+m+1)} \otimes w_{7j+3 \rightarrow 7(j+1)}; \\
b_{(j+1)s, 6s} &= e_{7(j+m)+6} \otimes w_{7j+4 \rightarrow 7(j+1)}; \\
b_{2s+(j+1)s, 9s} &= e_{7(j+m+1)+4} \otimes w_{7j+6 \rightarrow 7(j+1)+1}; \\
b_{(j+1)s, 10s} &= -w_{7(j+m)+6 \rightarrow 7(j+m+1)+3} \otimes w_{7j+6 \rightarrow 7(j+1)}; \\
b_{5s+(j+1)s, 10s} &= -w_{7(j+m+1)+2 \rightarrow 7(j+m+1)+3} \otimes w_{7j+6 \rightarrow 7(j+1)+3}; \\
b_{8s+(j+1)s, 10s} &= e_{7(j+m+1)+3} \otimes w_{7j+6 \rightarrow 7(j+1)+5}; \\
b_{3s+(j+1)s, 11s} &= e_{7(j+m+1)+1} \otimes w_{7j+6 \rightarrow 7(j+1)+2}.
\end{aligned}$$

(8) If  $r_0 = 7$ , then  $\Omega^7(Y_t^{(3)})$  is described with  $(12s \times 13s)$ -matrix with the following nonzero elements:

$$\begin{aligned}
b_{s+(j+1)s, 3s} &= e_{7(j+m+1)+5} \otimes w_{7j+1 \rightarrow 7(j+1)}; \\
b_{2s+(j+1)s, 3s} &= w_{7(j+m+1)+4 \rightarrow 7(j+m+1)+5} \otimes w_{7j+1 \rightarrow 7(j+1)}; \\
b_{(j+1)s, 4s} &= -e_{7(j+m+1)+2} \otimes w_{7j+2 \rightarrow 7(j+1)}; \\
b_{(j+1)s, 5s} &= -w_{7(j+m+1)+2 \rightarrow 7(j+m+1)+3} \otimes w_{7j+3 \rightarrow 7(j+1)}; \\
b_{2s+(j+1)s, 6s} &= -e_{7(j+m+1)+4} \otimes w_{7j+3 \rightarrow 7(j+1)}; \\
b_{s+(j+1)s, 8s} &= e_{7(j+m+1)+5} \otimes w_{7j+4 \rightarrow 7(j+1)}; \\
b_{(j+1)s, 11s} &= w_{7(j+m+1)+2 \rightarrow 7(j+m+1)+6} \otimes w_{7j+6 \rightarrow 7(j+1)}; \\
b_{2s+(j+1)s, 11s} &= -w_{7(j+m+1)+4 \rightarrow 7(j+m+1)+6} \otimes w_{7j+6 \rightarrow 7(j+1)}; \\
b_{6s+(j+1)s, 11s} &= e_{7(j+m+1)+6} \otimes w_{7j+6 \rightarrow 7(j+1)+4}; \\
b_{(j+1)s, 12s} &= -w_{7(j+m+1)+2 \rightarrow 7(j+m+2)} \otimes w_{7j+6 \rightarrow 7(j+1)}; \\
b_{2s+(j+1)s, 12s} &= w_{7(j+m+1)+4 \rightarrow 7(j+m+2)} \otimes w_{7j+6 \rightarrow 7(j+1)}; \\
b_{3s+(j+1)s, 12s} &= e_{7(j+m+2)} \otimes w_{7j+6 \rightarrow 7(j+1)+1}; \\
b_{6s+(j+1)s, 12s} &= -w_{7(j+m+1)+6 \rightarrow 7(j+m+2)} \otimes w_{7j+6 \rightarrow 7(j+1)+4}.
\end{aligned}$$

(9) If  $r_0 = 8$ , then  $\Omega^8(Y_t^{(3)})$  is described with  $(13s \times 12s)$ -matrix with the following nonzero elements:

$$\begin{aligned}
b_{(j+1)s,3s} &= e_{7(j+m)+6} \otimes w_{7j+1 \rightarrow 7(j+1)}; \\
b_{(j+1)s,4s} &= -w_{7(j+m)+6 \rightarrow 7(j+m+1)} \otimes w_{7j+2 \rightarrow 7(j+1)}; \\
b_{s+(j+1)s,4s} &= -e_{7(j+m+1)} \otimes w_{7j+2 \rightarrow 7(j+1)}; \\
b_{(j+1)s,6s} &= e_{7(j+m)+6} \otimes w_{7j+4 \rightarrow 7(j+1)}; \\
b_{s+(j+1)s,7s} &= e_{7(j+m+1)} \otimes w_{7j+4 \rightarrow 7(j+1)}; \\
b_{2s+(j+1)s,9s} &= w_{7(j+m+1)+1 \rightarrow 7(j+m+1)+2} \otimes w_{7j+6 \rightarrow 7(j+1)+1}; \\
b_{4s+(j+1)s,9s} &= -e_{7(j+m+1)+2} \otimes w_{7j+6 \rightarrow 7(j+1)+2}; \\
b_{8s+(j+1)s,10s} &= e_{7(j+m+1)+5} \otimes w_{7j+6 \rightarrow 7(j+1)+4}; \\
b_{(j+1)s,11s} &= -w_{7(j+m)+6 \rightarrow 7(j+m+1)+4} \otimes w_{7j+6 \rightarrow 7(j+1)}; \\
b_{s+(j+1)s,11s} &= -w_{7(j+m+1) \rightarrow 7(j+m+1)+4} \otimes w_{7j+6 \rightarrow 7(j+1)}; \\
b_{6s+(j+1)s,11s} &= -e_{7(j+m+1)+4} \otimes w_{7j+6 \rightarrow 7(j+1)+3}; \\
b_{9s+(j+1)s,11s} &= e_{7(j+m+1)+4} \otimes w_{7j+6 \rightarrow 7(j+1)+5}.
\end{aligned}$$

(10) If  $r_0 = 9$ , then  $\Omega^9(Y_t^{(3)})$  is described with  $(12s \times 12s)$ -matrix with the following nonzero elements:

$$\begin{aligned}
b_{2s+(j+1)s,2s} &= -w_{7(j+m+1)+1 \rightarrow 7(j+m+1)+2} \otimes w_{7j+1 \rightarrow 7(j+1)}; \\
b_{s+(j+1)s,3s} &= -e_{7(j+m+1)+3} \otimes w_{7j+2 \rightarrow 7(j+1)}; \\
b_{2s+(j+1)s,3s} &= -w_{7(j+m+1)+1 \rightarrow 7(j+m+1)+3} \otimes w_{7j+2 \rightarrow 7(j+1)}; \\
b_{2s+(j+1)s,7s} &= e_{7(j+m+1)+1} \otimes w_{7j+4 \rightarrow 7(j+1)}; \\
b_{(j+1)s,9s} &= -e_{7(j+m+1)+5} \otimes w_{7j+5 \rightarrow 7(j+1)}; \\
b_{(j+1)s,10s} &= w_{7(j+m+1)+5 \rightarrow 7(j+m+1)+6} \otimes w_{7j+6 \rightarrow 7(j+1)}; \\
b_{3s+(j+1)s,10s} &= e_{7(j+m+1)+6} \otimes w_{7j+6 \rightarrow 7(j+1)+1}; \\
b_{7s+(j+1)s,11s} &= e_{7(j+m+2)} \otimes w_{7j+6 \rightarrow 7(j+1)+4}.
\end{aligned}$$

(11) If  $r_0 = 10$ , then  $\Omega^{10}(Y_t^{(3)})$  is described with  $(12s \times 10s)$ -matrix with the following nonzero elements:

$$\begin{aligned}
b_{s+(j+1)s,2s} &= e_{7(j+m+1)} \otimes w_{7j+1 \rightarrow 7(j+1)}; \\
b_{(j+1)s,3s} &= e_{7(j+m)+6} \otimes w_{7j+2 \rightarrow 7(j+1)}; \\
b_{(j+1)s,5s} &= w_{7(j+m)+6 \rightarrow 7(j+m+1)} \otimes w_{7j+4 \rightarrow 7(j+1)}; \\
b_{s+(j+1)s,5s} &= e_{7(j+m+1)} \otimes w_{7j+4 \rightarrow 7(j+1)}; \\
b_{(j+1)s,7s} &= w_{7(j+m)+6 \rightarrow 7(j+m+1)+5} \otimes w_{7j+6 \rightarrow 7(j+1)}; \\
b_{s+(j+1)s,7s} &= w_{7(j+m+1) \rightarrow 7(j+m+1)+5} \otimes w_{7j+6 \rightarrow 7(j+1)}; \\
b_{4s+(j+1)s,7s} &= -w_{7(j+m+1)+4 \rightarrow 7(j+m+1)+5} \otimes w_{7j+6 \rightarrow 7(j+1)+2}; \\
b_{5s+(j+1)s,7s} &= -e_{7(j+m+1)+5} \otimes w_{7j+6 \rightarrow 7(j+1)+3}; \\
b_{9s+(j+1)s,7s} &= -e_{7(j+m+1)+5} \otimes w_{7j+6 \rightarrow 7(j+1)+5}; \\
b_{2s+(j+1)s,8s} &= w_{7(j+m+1)+2 \rightarrow 7(j+m+1)+3} \otimes w_{7j+6 \rightarrow 7(j+1)+1}; \\
b_{3s+(j+1)s,8s} &= -e_{7(j+m+1)+3} \otimes w_{7j+6 \rightarrow 7(j+1)+2}; \\
b_{7s+(j+1)s,9s} &= e_{7(j+m+1)+1} \otimes w_{7j+6 \rightarrow 7(j+1)+4}.
\end{aligned}$$

(12) If  $r_0 = 11$ , then  $\Omega^{11}(Y_t^{(3)})$  is described with  $(10s \times 10s)$ -matrix with the following nonzero elements:

$$\begin{aligned}
b_{(j+1)s,s} &= w_{7(j+m+1)+2 \rightarrow 7(j+m+1)+3} \otimes w_{7j+1 \rightarrow 7(j+1)}; \\
b_{s+(j+1)s,2s} &= e_{7(j+m+1)+4} \otimes w_{7j+1 \rightarrow 7(j+1)}; \\
b_{s+(j+1)s,3s} &= -w_{7(j+m+1)+4 \rightarrow 7(j+m+1)+5} \otimes w_{7j+2 \rightarrow 7(j+1)}; \\
b_{(j+1)s,5s} &= e_{7(j+m+1)+2} \otimes w_{7j+4 \rightarrow 7(j+1)}; \\
b_{(j+1)s,8s} &= w_{7(j+m+1)+2 \rightarrow 7(j+m+1)+6} \otimes w_{7j+6 \rightarrow 7(j+1)}; \\
b_{3s+(j+1)s,8s} &= e_{7(j+m+1)+6} \otimes w_{7j+6 \rightarrow 7(j+1)+2}; \\
b_{6s+(j+1)s,8s} &= e_{7(j+m+1)+6} \otimes w_{7j+6 \rightarrow 7(j+1)+5}; \\
b_{2s+(j+1)s,9s} &= e_{7(j+m+2)} \otimes w_{7j+6 \rightarrow 7(j+1)+1}.
\end{aligned}$$

(13) If  $r_0 = 12$ , then  $\Omega^{12}(Y_t^{(3)})$  is described with  $(10s \times 9s)$ -matrix with the following nonzero elements:

$$\begin{aligned}
b_{(j+1)s,3s} &= e_{7(j+m+1)} \otimes w_{7j+2 \rightarrow 7(j+1)}; \\
b_{(j+1)s,4s} &= -w_{7(j+m+1) \rightarrow 7(j+m+1)+1} \otimes w_{7j+3 \rightarrow 7(j+1)}; \\
b_{4s+(j+1)s,4s} &= e_{7(j+m+1)+1} \otimes w_{7j+3 \rightarrow 7(j+1)+3}; \\
b_{(j+1)s,7s} &= w_{7(j+m+1) \rightarrow 7(j+m+1)+2} \otimes w_{7j+6 \rightarrow 7(j+1)}; \\
b_{4s+(j+1)s,7s} &= -w_{7(j+m+1)+1 \rightarrow 7(j+m+1)+2} \otimes w_{7j+6 \rightarrow 7(j+1)+3}; \\
b_{5s+(j+1)s,7s} &= e_{7(j+m+1)+2} \otimes w_{7j+6 \rightarrow 7(j+1)+4}; \\
b_{2s+(j+1)s,8s} &= e_{7(j+m+1)+4} \otimes w_{7j+6 \rightarrow 7(j+1)+1}.
\end{aligned}$$

(14) If  $r_0 = 13$ , then  $\Omega^{13}(Y_t^{(3)})$  is described with  $(9s \times 7s)$ -matrix with the following nonzero elements:

$$\begin{aligned}
b_{s+(j+1)s,s} &= e_{7(j+m+1)+5} \otimes w_{7j+1 \rightarrow 7(j+1)}; \\
b_{(j+1)s,4s} &= e_{7(j+m+1)+3} \otimes w_{7j+4 \rightarrow 7(j+1)}; \\
b_{(j+1)s,6s} &= w_{7(j+m+1)+3 \rightarrow 7(j+m+2)} \otimes w_{7j+6 \rightarrow 7(j+1)}; \\
b_{2s+(j+1)s,6s} &= w_{7(j+m+1)+6 \rightarrow 7(j+m+2)} \otimes w_{7j+6 \rightarrow 7(j+1)+1}; \\
b_{3s+(j+1)s,6s} &= e_{7(j+m+2)} \otimes w_{7j+6 \rightarrow 7(j+1)+2}; \\
b_{6s+(j+1)s,6s} &= e_{7(j+m+2)} \otimes w_{7j+6 \rightarrow 7(j+1)+5}.
\end{aligned}$$

(15) If  $r_0 = 14$ , then  $\Omega^{14}(Y_t^{(3)})$  is described with  $(7s \times 8s)$ -matrix with the following nonzero elements:

$$\begin{aligned}
b_{(j+1)s,0} &= e_{7(j+m)+6} \otimes w_{7j \rightarrow 7(j+1)}; \\
b_{(j+1)s,s} &= -w_{7(j+m)+6 \rightarrow 7(j+m+1)} \otimes w_{7j+1 \rightarrow 7(j+1)}; \\
b_{(j+1)s,2s} &= w_{7(j+m)+6 \rightarrow 7(j+m+1)+1} \otimes w_{7j+2 \rightarrow 7(j+1)}; \\
b_{2s+(j+1)s,2s} &= e_{7(j+m+1)+1} \otimes w_{7j+2 \rightarrow 7(j+1)+2}; \\
b_{(j+1)s,3s} &= -w_{7(j+m)+6 \rightarrow 7(j+m+1)+2} \otimes w_{7j+3 \rightarrow 7(j+1)}; \\
b_{2s+(j+1)s,3s} &= -w_{7(j+m+1)+1 \rightarrow 7(j+m+1)+2} \otimes w_{7j+3 \rightarrow 7(j+1)+2}; \\
b_{3s+(j+1)s,3s} &= e_{7(j+m+1)+2} \otimes w_{7j+3 \rightarrow 7(j+1)+3}; \\
b_{5s+(j+1)s,5s} &= e_{7(j+m+1)+4} \otimes w_{7j+5 \rightarrow 7(j+1)+5}; \\
b_{(j+1)s,6s} &= w_{7(j+m)+6 \rightarrow 7(j+m+1)+3} \otimes w_{7j+6 \rightarrow 7(j+1)}; \\
b_{2s+(j+1)s,6s} &= w_{7(j+m+1)+1 \rightarrow 7(j+m+1)+3} \otimes w_{7j+6 \rightarrow 7(j+1)+2}; \\
b_{3s+(j+1)s,6s} &= -w_{7(j+m+1)+2 \rightarrow 7(j+m+1)+3} \otimes w_{7j+6 \rightarrow 7(j+1)+3};
\end{aligned}$$

$$b_{4s+(j+1)s,6s} = e_{7(j+m+1)+3} \otimes w_{7j+6 \rightarrow 7(j+1)+4};$$

$$b_{s+(j+1)s,7s} = e_{7(j+m+1)+5} \otimes w_{7j+6 \rightarrow 7(j+1)+1};$$

$$b_{5s+(j+1)s,7s} = w_{7(j+m+1)+4 \rightarrow 7(j+m+1)+5} \otimes w_{7j+6 \rightarrow 7(j+1)+5}.$$

(16) If  $r_0 = 15$ , then  $\Omega^{15}(Y_t^{(3)})$  is described with  $(8s \times 7s)$ -matrix with the following two nonzero elements:

$$b_{j,6s} = -w_{7(j+m+1)+3 \rightarrow 7(j+m+1)+6} \otimes e_{7j+6};$$

$$b_{j+s,6s} = w_{7(j+m+1)+5 \rightarrow 7(j+m+1)+6} \otimes e_{7j+6}.$$

(17) If  $r_0 = 16$ , then  $\Omega^{16}(Y_t^{(3)})$  is described with  $(7s \times 7s)$ -matrix with the following nonzero elements:

$$b_{(j+1)s,0} = e_{7(j+m+1)} \otimes w_{7j \rightarrow 7(j+1)};$$

$$b_{j+6s,0} = -w_{7(j+m)+6 \rightarrow 7(j+m+1)} \otimes w_{7j \rightarrow 7j+6};$$

$$b_{j,s} = w_{7(j+m)+1 \rightarrow 7(j+m+1)+1} \otimes e_{7j+1};$$

$$b_{j+s,s} = -w_{7(j+m)+2 \rightarrow 7(j+m+1)+1} \otimes w_{7j+1 \rightarrow 7j+2};$$

$$b_{j+2s,s} = w_{7(j+m)+3 \rightarrow 7(j+m+1)+1} \otimes w_{7j+1 \rightarrow 7j+3};$$

$$b_{j,2s} = w_{7(j+m)+2 \rightarrow 7(j+m+1)+2} \otimes e_{7j+2};$$

$$b_{j+s,2s} = -w_{7(j+m)+3 \rightarrow 7(j+m+1)+2} \otimes w_{7j+2 \rightarrow 7j+3};$$

$$b_{j,3s} = w_{7(j+m)+3 \rightarrow 7(j+m+1)+3} \otimes e_{7j+3};$$

$$b_{j,4s} = w_{7(j+m)+4 \rightarrow 7(j+m+1)+4} \otimes e_{7j+4};$$

$$b_{j+s,4s} = -w_{7(j+m)+5 \rightarrow 7(j+m+1)+4} \otimes w_{7j+4 \rightarrow 7j+5};$$

$$b_{j,5s} = w_{7(j+m)+5 \rightarrow 7(j+m+1)+5} \otimes e_{7j+5};$$

$$b_{6s+(j+1)s,7s-1} = e_{7(j+m+1)+6} \otimes w_{7j+6 \rightarrow 7(j+1)+6}.$$

(II) Represent an arbitrary  $t_0 \in \mathbb{N}$  in the form  $t_0 = 17\ell_0 + r_0$ , where  $0 \leq r_0 \leq 16$ . Then  $\Omega^{t_0}(Y_t^{(3)})$  is a  $\Omega^{r_0}(Y_t^{(3)})$ , whose left components twisted by  $\sigma^{\ell_0}$ , and coefficients multiplied by  $(-1)^{\ell_0}$ .

**Proposition 4** (Translates for the case 4). (I) Let  $r_0 \in \mathbb{N}$ ,  $r_0 < 17$ .  $r_0$ -translates of the elements  $Y_t^{(4)}$  are described by the following way.

(1) If  $r_0 = 0$ , then  $\Omega^0(Y_t^{(4)})$  is described with  $(7s \times 9s)$ -matrix with the following elements  $b_{ij}$ :  
If  $0 \leq j < s$ , then

$$b_{ij} = \begin{cases} w_{7(j+m) \rightarrow 7(j+m)+2} \otimes e_{7j}, & i = j; \\ 0, & \text{otherwise.} \end{cases}$$

If  $s \leq j < 2s$ , then

$$b_{ij} = \begin{cases} -w_{7(j+m) \rightarrow 7(j+m)+5} \otimes e_{7j}, & i = j - s; \\ 0, & \text{otherwise.} \end{cases}$$

If  $2s \leq j < 4s$ , then  $b_{ij} = 0$ .

If  $4s \leq j < 5s$ , then

$$b_{ij} = \begin{cases} w_{7(j+m)+3 \rightarrow 7(j+m+1)} \otimes e_{7j+3}, & i = j - s; \\ 0, & \text{otherwise.} \end{cases}$$

If  $5s \leq j < 7s$ , then  $b_{ij} = 0$ .

If  $7s \leq j < 8s$ , then

$$b_{ij} = \begin{cases} w_{7(j+m)+6 \rightarrow 7(j+m+1)+1} \otimes e_{7j+6}, & i = j - s; \\ 0, & \text{otherwise.} \end{cases}$$

If  $8s \leq j < 9s$ , then  $b_{ij} = 0$ .

(2) If  $r_0 = 1$ , then  $\Omega^1(Y_t^{(4)})$  is described with  $(8s \times 10s)$ -matrix with the following elements  $b_{ij}$ :  
If  $s \leq j < 2s$ , then

$$b_{ij} = \begin{cases} -w_{7(j+m)+1 \rightarrow 7(j+m+1)} \otimes e_{7j}, & i = j - s; \\ -w_{7(j+m)+2 \rightarrow 7(j+m+1)} \otimes w_{7j \rightarrow 7j+1}, & i = j + s; \\ -w_{7(j+m)+3 \rightarrow 7(j+m+1)} \otimes w_{7j \rightarrow 7j+2}, & i = j + 2s; \\ 0, & \text{otherwise.} \end{cases}$$

If  $2s \leq j < 3s$ , then

$$b_{ij} = \begin{cases} -w_{7(j+m+1)+1 \rightarrow 7(j+m+1)+3} \otimes w_{7j+1 \rightarrow 7(j+1)}, & i = (j+1)_s; \\ -w_{7(j+m+1)+2 \rightarrow 7(j+m+1)+3} \otimes w_{7j+1 \rightarrow 7(j+1)+1}, & i = 2s + (j+1)_s; \\ 0, & \text{otherwise.} \end{cases}$$

If  $3s \leq j < 4s$ , then  $b_{ij} = 0$ .

If  $4s \leq j < 5s$ , then

$$b_{ij} = \begin{cases} -w_{7(j+m)+6 \rightarrow 7(j+m+1)+1} \otimes e_{7j+3}, & i = j; \\ 0, & \text{otherwise.} \end{cases}$$

If  $5s \leq j < 6s$ , then

$$b_{ij} = \begin{cases} w_{7(j+m+1)+4 \rightarrow 7(j+m+1)+5} \otimes w_{7j+3 \rightarrow 7(j+1)}, & i = s + (j+1)_s; \\ 0, & \text{otherwise.} \end{cases}$$

If  $6s \leq j < 7s$ , then

$$b_{ij} = \begin{cases} -w_{7(j+m)+6 \rightarrow 7(j+m+1)+1} \otimes w_{7j+4 \rightarrow 7j+5}, & i = j; \\ 0, & \text{otherwise.} \end{cases}$$

If  $7s \leq j < 8s$ , then

$$b_{ij} = \begin{cases} w_{7(j+m+1)+1 \rightarrow 7(j+m+1)+2} \otimes w_{7j+5 \rightarrow 7(j+1)}, & i = (j+1)_s; \\ w_{7(j+m)+6 \rightarrow 7(j+m+1)+2} \otimes e_{7j+5}, & i = j - s; \\ 0, & \text{otherwise.} \end{cases}$$

If  $8s \leq j < 9s$ , then  $b_{ij} = 0$ .

If  $9s \leq j < 10s$ , then

$$b_{ij} = \begin{cases} -w_{7(j+m+1) \rightarrow 7(j+m+1)+6} \otimes e_{7j+6}, & i = j - 2s; \\ 0, & \text{otherwise.} \end{cases}$$

(3) If  $r_0 = 2$ , then  $\Omega^2(Y_t^{(4)})$  is described with  $(7s \times 10s)$ -matrix with the following elements  $b_{ij}$ :

If  $2s \leq j < 3s$ , then

$$b_{ij} = \begin{cases} w_{7(j+m-1)+6 \rightarrow 7(j+m)+1} \otimes e_{7j}, & i = j - 2s; \\ 0, & \text{otherwise.} \end{cases}$$

If  $3s \leq j < 4s$ , then

$$b_{ij} = \begin{cases} e_{7(j+m)+6} \otimes w_{7j+1 \rightarrow 7(j+1)}, & i = (j+1)_s; \\ 0, & \text{otherwise.} \end{cases}$$

If  $4s \leq j < 5s$ , then

$$b_{ij} = \begin{cases} w_{7(j+m)+6 \rightarrow 7(j+m+1)} \otimes w_{7j+2 \rightarrow 7(j+1)}, & i = (j+1)_s; \\ 0, & \text{otherwise.} \end{cases}$$

If  $5s \leq j < 6s$ , then

$$b_{ij} = \begin{cases} w_{7(j+m)+4 \rightarrow 7(j+m)+6} \otimes e_{7j+3}, & i = j - 2s; \\ 0, & \text{otherwise.} \end{cases}$$

If  $6s \leq j < 7s$ , then  $b_{ij} = 0$ .

If  $7s \leq j < 8s$ , then

$$b_{ij} = \begin{cases} w_{7(j+m)+1 \rightarrow 7(j+m)+6} \otimes e_{7j+5}, & i = j - 2s; \\ 0, & \text{otherwise.} \end{cases}$$

If  $8s \leq j < 9s$ , then

$$b_{ij} = \begin{cases} w_{7(j+m)+6 \rightarrow 7(j+m+1)+2} \otimes w_{7j+6 \rightarrow 7(j+1)}, & i = (j+1)_s; \\ 0, & \text{otherwise.} \end{cases}$$

If  $9s \leq j < 10s$ , then  $b_{ij} = 0$ .

(4) If  $r_0 = 3$ , then  $\Omega^3(Y_t^{(4)})$  is described with  $(9s \times 12s)$ -matrix with the following elements  $b_{ij}$ :

If  $0 \leq j < s$ , then

$$b_{ij} = \begin{cases} w_{7(j+m)+2 \rightarrow 7(j+m)+6} \otimes e_{7j}, & i = j; \\ w_{7(j+m)+3 \rightarrow 7(j+m)+6} \otimes w_{7j \rightarrow 7j+1}, & i = j + 2s; \\ e_{7(j+m)+6} \otimes w_{7j \rightarrow 7j+2}, & i = j + 3s; \\ 0, & \text{otherwise.} \end{cases}$$

If  $s \leq j < 4s$ , then  $b_{ij} = 0$ .

If  $4s \leq j < 5s$ , then

$$b_{ij} = \begin{cases} -e_{7(j+m+1)+5} \otimes w_{7j+2 \rightarrow 7(j+1)}, & i = s + (j+1)_s; \\ 0, & \text{otherwise.} \end{cases}$$

If  $5s \leq j < 6s$ , then  $b_{ij} = 0$ .

If  $6s \leq j < 7s$ , then

$$b_{ij} = \begin{cases} e_{7(j+m+1)+2} \otimes w_{7j+4 \rightarrow 7(j+1)}, & i = (j+1)_s; \\ 0, & \text{otherwise.} \end{cases}$$

If  $7s \leq j < 12s$ , then  $b_{ij} = 0$ .

(5) If  $r_0 = 4$ , then  $\Omega^4(Y_t^{(4)})$  is described with  $(10s \times 12s)$ -matrix with the following elements  $b_{ij}$ :

If  $0 \leq j < s$ , then

$$b_{ij} = \begin{cases} -w_{7(j+m-1)+6 \rightarrow 7(j+m)+2} \otimes e_{7j}, & i = j; \\ -w_{7(j+m) \rightarrow 7(j+m)+2} \otimes e_{7j}, & i = j + s; \\ w_{7(j+m)+1 \rightarrow 7(j+m)+2} \otimes w_{7j \rightarrow 7j+3}, & i = j + 4s; \\ -e_{7(j+m)+2} \otimes w_{7j \rightarrow 7j+5}, & i = j + 7s; \\ 0, & \text{otherwise.} \end{cases}$$

If  $s \leq j < 2s$ , then

$$b_{ij} = \begin{cases} w_{7(j+m)+4 \rightarrow 7(j+m)+5} \otimes w_{7j \rightarrow 7j+2}, & i = j + 2s; \\ -e_{7(j+m)+5} \otimes w_{7j \rightarrow 7j+3}, & i = j + 4s; \\ 0, & \text{otherwise.} \end{cases}$$

If  $2s \leq j < 3s$ , then  $b_{ij} = 0$ .

If  $3s \leq j < 4s$ , then

$$b_{ij} = \begin{cases} w_{7(j+m)+6 \rightarrow 7(j+m+1)} \otimes w_{7j+1 \rightarrow 7(j+1)}, & i = (j+1)_s; \\ e_{7(j+m+1)} \otimes w_{7j+1 \rightarrow 7(j+1)}, & i = s + (j+1)_s; \\ 0, & \text{otherwise.} \end{cases}$$

If  $4s \leq j < 5s$ , then

$$b_{ij} = \begin{cases} e_{7(j+m)+6} \otimes w_{7j+2 \rightarrow 7(j+1)}, & i = (j+1)_s; \\ 0, & \text{otherwise.} \end{cases}$$

If  $5s \leq j < 10s$ , then  $b_{ij} = 0$ .

If  $10s \leq j < 11s$ , then

$$b_{ij} = \begin{cases} e_{7(j+m+1)+3} \otimes w_{7j+6 \rightarrow 7(j+1)+1}, & i = 2s + (j+1)_s; \\ 0, & \text{otherwise.} \end{cases}$$

If  $11s \leq j < 12s$ , then  $b_{ij} = 0$ .

(6) If  $r_0 = 5$ , then  $\Omega^5(Y_t^{(4)})$  is described with  $(10s \times 13s)$ -matrix with the following elements  $b_{ij}$ :

If  $0 \leq j < s$ , then

$$b_{ij} = \begin{cases} -w_{7(j+m)+3 \rightarrow 7(j+m)+6} \otimes e_{7j}, & i = j + s; \\ -w_{7(j+m)+1 \rightarrow 7(j+m)+6} \otimes e_{7j}, & i = j + 2s; \\ -e_{7(j+m)+6} \otimes w_{7j \rightarrow 7j+1}, & i = j + 3s; \\ 0, & \text{otherwise.} \end{cases}$$

If  $s \leq j < 2s$ , then

$$b_{ij} = \begin{cases} e_{7(j+m+1)} \otimes w_{7j \rightarrow 7j+2}, & i = j + 3s; \\ 0, & \text{otherwise.} \end{cases}$$



If  $2s \leq j < 3s$ , then

$$b_{ij} = \begin{cases} -e_{7(j+m+1)+1} \otimes w_{7j+1 \rightarrow 7(j+1)}, & i = 2s + (j+1)_s; \\ 0, & \text{otherwise.} \end{cases}$$

If  $3s \leq j < 4s$ , then

$$b_{ij} = \begin{cases} -w_{7(j+m+1)+4 \rightarrow 7(j+m+1)+5} \otimes w_{7j+1 \rightarrow 7(j+1)}, & i = (j+1)_s; \\ 0, & \text{otherwise.} \end{cases}$$

If  $4s \leq j < 5s$ , then

$$b_{ij} = \begin{cases} w_{7(j+m+1)+1 \rightarrow 7(j+m+1)+2} \otimes w_{7j+2 \rightarrow 7(j+1)}, & i = 2s + (j+1)_s; \\ 0, & \text{otherwise.} \end{cases}$$

If  $5s \leq j < 6s$ , then

$$b_{ij} = \begin{cases} -e_{7(j+m+1)+3} \otimes w_{7j+3 \rightarrow 7(j+1)}, & i = s + (j+1)_s; \\ -w_{7(j+m+1)+1 \rightarrow 7(j+m+1)+3} \otimes w_{7j+3 \rightarrow 7(j+1)}, & i = 2s + (j+1)_s; \\ 0, & \text{otherwise.} \end{cases}$$

If  $6s \leq j < 11s$ , then  $b_{ij} = 0$ .

If  $11s \leq j < 12s$ , then

$$b_{ij} = \begin{cases} -w_{7(j+m+1)+3 \rightarrow 7(j+m+1)+6} \otimes w_{7j+6 \rightarrow 7(j+1)}, & i = s + (j+1)_s; \\ -w_{7(j+m+1)+1 \rightarrow 7(j+m+1)+6} \otimes w_{7j+6 \rightarrow 7(j+1)}, & i = 2s + (j+1)_s; \\ 0, & \text{otherwise.} \end{cases}$$

If  $12s \leq j < 13s$ , then

$$b_{ij} = \begin{cases} -w_{7(j+m+1)+3 \rightarrow 7(j+m+2)} \otimes w_{7j+6 \rightarrow 7(j+1)}, & i = s + (j+1)_s; \\ -w_{7(j+m+1)+1 \rightarrow 7(j+m+2)} \otimes w_{7j+6 \rightarrow 7(j+1)}, & i = 2s + (j+1)_s; \\ 0, & \text{otherwise.} \end{cases}$$

(7) If  $r_0 = 6$ , then  $\Omega^6(Y_t^{(4)})$  is described with  $(12s \times 12s)$ -matrix with the following elements  $b_{ij}$ :

If  $0 \leq j < s$ , then

$$b_{ij} = \begin{cases} -w_{7(j+m)+4 \rightarrow 7(j+m)+5} \otimes w_{7j \rightarrow 7j+1}, & i = j + 2s; \\ 0, & \text{otherwise.} \end{cases}$$

If  $s \leq j < 2s$ , then

$$b_{ij} = \begin{cases} w_{7(j+m-1)+6 \rightarrow 7(j+m)+3} \otimes e_{7j}, & i = j - s; \\ w_{7(j+m)+2 \rightarrow 7(j+m)+3} \otimes w_{7j \rightarrow 7j+3}, & i = j + 4s; \\ -e_{7(j+m)+3} \otimes w_{7j \rightarrow 7j+5}, & i = j + 7s; \\ 0, & \text{otherwise.} \end{cases}$$

If  $2s \leq j < 3s$ , then

$$b_{ij} = \begin{cases} -e_{7(j+m)+1} \otimes w_{7j \rightarrow 7j+2}, & i = j + s; \\ 0, & \text{otherwise.} \end{cases}$$

If  $3s \leq j < 4s$ , then

$$b_{ij} = \begin{cases} -e_{7(j+m)+6} \otimes w_{7j+1 \rightarrow 7(j+1)}, & i = (j+1)_s; \\ 0, & \text{otherwise.} \end{cases}$$

If  $4s \leq j < 5s$ , then

$$b_{ij} = \begin{cases} e_{7(j+m+1)} \otimes w_{7j+2 \rightarrow 7(j+1)}, & i = s + (j+1)_s; \\ 0, & \text{otherwise.} \end{cases}$$

If  $5s \leq j < 11s$ , then  $b_{ij} = 0$ .

If  $11s \leq j < 12s$ , then

$$b_{ij} = \begin{cases} e_{7(j+m+1)+4} \otimes w_{7j+6 \rightarrow 7(j+1)+1}, & i = 2s + (j+1)_s; \\ 0, & \text{otherwise.} \end{cases}$$

(8) If  $r_0 = 7$ , then  $\Omega^7(Y_t^{(4)})$  is described with  $(12s \times 12s)$ -matrix with the following elements  $b_{ij}$ :

If  $0 \leq j < s$ , then

$$b_{ij} = \begin{cases} w_{7(j+m)+2 \rightarrow 7(j+m)+6} \otimes e_{7j}, & i = j; \\ -w_{7(j+m)+4 \rightarrow 7(j+m)+6} \otimes e_{7j}, & i = j + 2s; \\ e_{7(j+m)+6} \otimes w_{7j \rightarrow 7j+4}, & i = j + 6s; \\ 0, & \text{otherwise.} \end{cases}$$

If  $s \leq j < 2s$ , then

$$b_{ij} = \begin{cases} w_{7(j+m)+2 \rightarrow 7(j+m+1)} \otimes e_{7j}, & i = j - s; \\ -w_{7(j+m)+4 \rightarrow 7(j+m+1)} \otimes e_{7j}, & i = j + s; \\ -e_{7(j+m+1)} \otimes w_{7j \rightarrow 7j+1}, & i = j + 2s; \\ w_{7(j+m)+6 \rightarrow 7(j+m+1)} \otimes w_{7j \rightarrow 7j+4}, & i = j + 5s; \\ 0, & \text{otherwise.} \end{cases}$$

If  $2s \leq j < 3s$ , then

$$b_{ij} = \begin{cases} e_{7(j+m+1)+2} \otimes w_{7j+1 \rightarrow 7(j+1)}, & i = (j+1)_s; \\ 0, & \text{otherwise.} \end{cases}$$

If  $3s \leq j < 4s$ , then

$$b_{ij} = \begin{cases} -w_{7(j+m+1)+2 \rightarrow 7(j+m+1)+3} \otimes w_{7j+2 \rightarrow 7(j+1)}, & i = (j+1)_s; \\ 0, & \text{otherwise.} \end{cases}$$

If  $4s \leq j < 5s$ , then

$$b_{ij} = \begin{cases} e_{7(j+m+1)+4} \otimes w_{7j+2 \rightarrow 7(j+1)}, & i = 2s + (j+1)_s; \\ 0, & \text{otherwise.} \end{cases}$$

If  $5s \leq j < 12s$ , then  $b_{ij} = 0$ .

(9) If  $r_0 = 8$ , then  $\Omega^8(Y_t^{(4)})$  is described with  $(13s \times 10s)$ -matrix with the following elements  $b_{ij}$ :

If  $0 \leq j < s$ , then

$$b_{ij} = \begin{cases} -w_{7(j+m)+1 \rightarrow 7(j+m)+2} \otimes w_{7j \rightarrow 7j+1}, & i = j + 2s; \\ e_{7(j+m)+2} \otimes w_{7j \rightarrow 7j+2}, & i = j + 4s; \\ 0, & \text{otherwise.} \end{cases}$$

If  $s \leq j < 2s$ , then

$$b_{ij} = \begin{cases} w_{7(j+m-1)+6 \rightarrow 7(j+m)+4} \otimes e_{7j}, & i = j - s; \\ w_{7(j+m) \rightarrow 7(j+m)+4} \otimes e_{7j}, & i = j; \\ e_{7(j+m)+4} \otimes w_{7j \rightarrow 7j+3}, & i = j + 5s; \\ -e_{7(j+m)+4} \otimes w_{7j \rightarrow 7j+5}, & i = j + 8s; \\ 0, & \text{otherwise.} \end{cases}$$

If  $2s \leq j < 3s$ , then

$$b_{ij} = \begin{cases} -w_{7(j+m)+6 \rightarrow 7(j+m+1)} \otimes w_{7j+1 \rightarrow 7(j+1)}, & i = (j + 1)_s; \\ -e_{7(j+m+1)} \otimes w_{7j+1 \rightarrow 7(j+1)}, & i = s + (j + 1)_s; \\ 0, & \text{otherwise.} \end{cases}$$

If  $3s \leq j < 7s$ , then  $b_{ij} = 0$ .

If  $7s \leq j < 8s$ , then

$$b_{ij} = \begin{cases} -e_{7(j+m+1)+5} \otimes w_{7j+6 \rightarrow 7(j+1)+1}, & i = 3s + (j + 1)_s; \\ 0, & \text{otherwise.} \end{cases}$$

If  $8s \leq j < 10s$ , then  $b_{ij} = 0$ .

(10) If  $r_0 = 9$ , then  $\Omega^9(Y_t^{(4)})$  is described with  $(12s \times 10s)$ -matrix with the following elements  $b_{ij}$ :

If  $0 \leq j < s$ , then

$$b_{ij} = \begin{cases} w_{7(j+m)+5 \rightarrow 7(j+m+1)} \otimes e_{7j}, & i = j; \\ w_{7(j+m)+6 \rightarrow 7(j+m+1)} \otimes w_{7j \rightarrow 7j+1}, & i = j + 3s; \\ e_{7(j+m+1)} \otimes w_{7j \rightarrow 7j+4}, & i = j + 7s; \\ 0, & \text{otherwise.} \end{cases}$$

If  $s \leq j < 2s$ , then

$$b_{ij} = \begin{cases} e_{7(j+m+1)+3} \otimes w_{7j+1 \rightarrow 7(j+1)}, & i = s + (j + 1)_s; \\ w_{7(j+m+1)+1 \rightarrow 7(j+m+1)+3} \otimes w_{7j+1 \rightarrow 7(j+1)}, & i = 2s + (j + 1)_s; \\ 0, & \text{otherwise.} \end{cases}$$

If  $2s \leq j < 3s$ , then  $b_{ij} = 0$ .

If  $3s \leq j < 4s$ , then

$$b_{ij} = \begin{cases} e_{7(j+m+1)+5} \otimes w_{7j+2 \rightarrow 7(j+1)}, & i = (j + 1)_s; \\ 0, & \text{otherwise.} \end{cases}$$

If  $4s \leq j < 8s$ , then  $b_{ij} = 0$ .

If  $8s \leq j < 9s$ , then

$$b_{ij} = \begin{cases} -e_{7(j+m+1)+6} \otimes w_{7j+6 \rightarrow 7(j+1)+1}, & i = 3s + (j+1)_s; \\ 0, & \text{otherwise.} \end{cases}$$

If  $9s \leq j < 10s$ , then  $b_{ij} = 0$ .

(11) If  $r_0 = 10$ , then  $\Omega^{10}(Y_t^{(4)})$  is described with  $(12s \times 9s)$ -matrix with the following elements  $b_{ij}$ :

If  $0 \leq j < s$ , then

$$b_{ij} = \begin{cases} -w_{7(j+m)+2 \rightarrow 7(j+m)+3} \otimes w_{7j \rightarrow 7j+1}, & i = j + 2s; \\ e_{7(j+m)+3} \otimes w_{7j \rightarrow 7j+2}, & i = j + 3s; \\ -w_{7(j+m)+1 \rightarrow 7(j+m)+3} \otimes w_{7j \rightarrow 7j+4}, & i = j + 7s; \\ 0, & \text{otherwise.} \end{cases}$$

If  $s \leq j < 2s$ , then

$$b_{ij} = \begin{cases} -w_{7(j+m-1)+6 \rightarrow 7(j+m)+5} \otimes e_{7j}, & i = j - s; \\ -w_{7(j+m) \rightarrow 7(j+m)+5} \otimes e_{7j}, & i = j; \\ w_{7(j+m)+4 \rightarrow 7(j+m)+5} \otimes w_{7j \rightarrow 7j+2}, & i = j + 3s; \\ e_{7(j+m)+5} \otimes w_{7j \rightarrow 7j+3}, & i = j + 4s; \\ e_{7(j+m)+5} \otimes w_{7j \rightarrow 7j+5}, & i = j + 8s; \\ 0, & \text{otherwise.} \end{cases}$$

If  $2s \leq j < 3s$ , then

$$b_{ij} = \begin{cases} e_{7(j+m)+6} \otimes w_{7j+1 \rightarrow 7(j+1)}, & i = (j+1)_s; \\ 0, & \text{otherwise.} \end{cases}$$

If  $3s \leq j < 7s$ , then  $b_{ij} = 0$ .

If  $7s \leq j < 8s$ , then

$$b_{ij} = \begin{cases} -w_{7(j+m+1)+1 \rightarrow 7(j+m+1)+2} \otimes w_{7j+6 \rightarrow 7(j+1)+4}, & i = 7s + (j+1)_s; \\ 0, & \text{otherwise.} \end{cases}$$

If  $8s \leq j < 9s$ , then  $b_{ij} = 0$ .

(12) If  $r_0 = 11$ , then  $\Omega^{11}(Y_t^{(4)})$  is described with  $(10s \times 7s)$ -matrix with the following elements  $b_{ij}$ :

If  $0 \leq j < s$ , then

$$b_{ij} = \begin{cases} -w_{7(j+m)+2 \rightarrow 7(j+m)+6} \otimes e_{7j}, & i = j; \\ -e_{7(j+m)+6} \otimes w_{7j \rightarrow 7j+2}, & i = j + 3s; \\ -e_{7(j+m)+6} \otimes w_{7j \rightarrow 7j+5}, & i = j + 6s; \\ 0, & \text{otherwise.} \end{cases}$$

If  $s \leq j < 2s$ , then

$$b_{ij} = \begin{cases} -w_{7(j+m+1)+4 \rightarrow 7(j+m+1)+5} \otimes w_{7j+1 \rightarrow 7(j+1)}, & i = s + (j+1)_s; \\ 0, & \text{otherwise.} \end{cases}$$

If  $2s \leq j < 6s$ , then  $b_{ij} = 0$ .

If  $6s \leq j < 7s$ , then

$$b_{ij} = \begin{cases} -e_{7(j+m+2)} \otimes w_{7j+6 \rightarrow 7(j+1)+1}, & i = 2s + (j+1)_s; \\ 0, & \text{otherwise.} \end{cases}$$

(13) If  $r_0 = 12$ , then  $\Omega^{12}(Y_t^{(4)})$  is described with  $(10s \times 8s)$ -matrix with the following elements  $b_{ij}$ :

If  $0 \leq j < s$ , then

$$b_{ij} = \begin{cases} w_{7(j+m) \rightarrow 7(j+m)+6} \otimes e_{7j}, & i = j; \\ -w_{7(j+m)+4 \rightarrow 7(j+m)+6} \otimes w_{7j \rightarrow 7j+1}, & i = j + 2s; \\ -w_{7(j+m)+1 \rightarrow 7(j+m)+6} \otimes w_{7j \rightarrow 7j+3}, & i = j + 4s; \\ w_{7(j+m)+2 \rightarrow 7(j+m)+6} \otimes w_{7j \rightarrow 7j+4}, & i = j + 5s; \\ 0, & \text{otherwise.} \end{cases}$$

If  $s \leq j < 2s$ , then

$$b_{ij} = \begin{cases} e_{7(j+m+1)} \otimes w_{7j+1 \rightarrow 7(j+1)}, & i = (j+1)_s; \\ 0, & \text{otherwise.} \end{cases}$$

If  $2s \leq j < 3s$ , then

$$b_{ij} = \begin{cases} w_{7(j+m+1) \rightarrow 7(j+m+1)+1} \otimes w_{7j+2 \rightarrow 7(j+1)}, & i = (j+1)_s; \\ 0, & \text{otherwise.} \end{cases}$$

If  $3s \leq j < 4s$ , then

$$b_{ij} = \begin{cases} w_{7(j+m+1) \rightarrow 7(j+m+1)+2} \otimes w_{7j+3 \rightarrow 7(j+1)}, & i = (j+1)_s; \\ -w_{7(j+m+1)+1 \rightarrow 7(j+m+1)+2} \otimes w_{7j+3 \rightarrow 7(j+1)+3}, & i = 4s + (j+1)_s; \\ 0, & \text{otherwise.} \end{cases}$$

If  $4s \leq j < 6s$ , then  $b_{ij} = 0$ .

If  $6s \leq j < 7s$ , then

$$b_{ij} = \begin{cases} w_{7(j+m+1) \rightarrow 7(j+m+1)+3} \otimes w_{7j+6 \rightarrow 7(j+1)}, & i = (j+1)_s; \\ -w_{7(j+m+1)+1 \rightarrow 7(j+m+1)+3} \otimes w_{7j+6 \rightarrow 7(j+1)+3}, & i = 4s + (j+1)_s; \\ w_{7(j+m+1)+2 \rightarrow 7(j+m+1)+3} \otimes w_{7j+6 \rightarrow 7(j+1)+4}, & i = 5s + (j+1)_s; \\ 0, & \text{otherwise.} \end{cases}$$

If  $7s \leq j < 8s$ , then

$$b_{ij} = \begin{cases} w_{7(j+m+1)+4 \rightarrow 7(j+m+1)+5} \otimes w_{7j+6 \rightarrow 7(j+1)+1}, & i = 2s + (j+1)_s; \\ 0, & \text{otherwise.} \end{cases}$$

(14) If  $r_0 = 13$ , then  $\Omega^{13}(Y_t^{(4)})$  is described with  $(9s \times 7s)$ -matrix with the following elements  $b_{ij}$ :

If  $0 \leq j < s$ , then

$$b_{ij} = \begin{cases} -w_{7(j+m)+3 \rightarrow 7(j+m+1)} \otimes e_{7j}, & i = j; \\ -w_{7(j+m)+6 \rightarrow 7(j+m+1)} \otimes w_{7j \rightarrow 7j+1}, & i = j + 2s; \\ -e_{7(j+m+1)} \otimes w_{7j \rightarrow 7j+2}, & i = j + 3s; \\ -e_{7(j+m+1)} \otimes w_{7j \rightarrow 7j+5}, & i = j + 6s; \\ 0, & \text{otherwise.} \end{cases}$$

If  $s \leq j < 7s$ , then  $b_{ij} = 0$ .

(15) If  $r_0 = 14$ , then  $\Omega^{14}(Y_t^{(4)})$  is described with  $(7s \times 7s)$ -matrix with the following elements  $b_{ij}$ :

If  $0 \leq j < s$ , then

$$b_{ij} = \begin{cases} w_{7(j+m)+1 \rightarrow 7(j+m+1)} \otimes w_{7j \rightarrow 7j+2}, & i = j + 2s; \\ -w_{7(j+m)+2 \rightarrow 7(j+m+1)} \otimes w_{7j \rightarrow 7j+3}, & i = j + 3s; \\ w_{7(j+m)+3 \rightarrow 7(j+m+1)} \otimes w_{7j \rightarrow 7j+4}, & i = j + 4s; \\ 0, & \text{otherwise.} \end{cases}$$

If  $s \leq j < 2s$ , then

$$b_{ij} = \begin{cases} w_{7(j+m)+6 \rightarrow 7(j+m+1)+1} \otimes w_{7j+1 \rightarrow 7(j+1)}, & i = (j+1)_s; \\ 0, & \text{otherwise.} \end{cases}$$

If  $2s \leq j < 3s$ , then

$$b_{ij} = \begin{cases} w_{7(j+m)+6 \rightarrow 7(j+m+1)+2} \otimes w_{7j+2 \rightarrow 7(j+1)}, & i = (j+1)_s; \\ w_{7(j+m+1)+1 \rightarrow 7(j+m+1)+2} \otimes w_{7j+2 \rightarrow 7(j+1)+2}, & i = 2s + (j+1)_s; \\ 0, & \text{otherwise.} \end{cases}$$

If  $3s \leq j < 4s$ , then

$$b_{ij} = \begin{cases} w_{7(j+m)+6 \rightarrow 7(j+m+1)+3} \otimes w_{7j+3 \rightarrow 7(j+1)}, & i = (j+1)_s; \\ w_{7(j+m+1)+1 \rightarrow 7(j+m+1)+3} \otimes w_{7j+3 \rightarrow 7(j+1)+2}, & i = 2s + (j+1)_s; \\ -w_{7(j+m+1)+2 \rightarrow 7(j+m+1)+3} \otimes w_{7j+3 \rightarrow 7(j+1)+3}, & i = 3s + (j+1)_s; \\ 0, & \text{otherwise.} \end{cases}$$

If  $4s \leq j < 5s$ , then  $b_{ij} = 0$ .

If  $5s \leq j < 6s$ , then

$$b_{ij} = \begin{cases} w_{7(j+m+1)+4 \rightarrow 7(j+m+1)+5} \otimes w_{7j+5 \rightarrow 7(j+1)+5}, & i = 5s + (j+1)_s; \\ 0, & \text{otherwise.} \end{cases}$$

If  $6s \leq j < 7s$ , then

$$b_{ij} = \begin{cases} w_{7(j+m)+6 \rightarrow 7(j+m+1)+6} \otimes w_{7j+6 \rightarrow 7(j+1)}, & i = (j+1)_s; \\ w_{7(j+m+1)+1 \rightarrow 7(j+m+1)+6} \otimes w_{7j+6 \rightarrow 7(j+1)+2}, & i = 2s + (j+1)_s; \\ -w_{7(j+m+1)+2 \rightarrow 7(j+m+1)+6} \otimes w_{7j+6 \rightarrow 7(j+1)+3}, & i = 3s + (j+1)_s; \\ w_{7(j+m+1)+3 \rightarrow 7(j+m+1)+6} \otimes w_{7j+6 \rightarrow 7(j+1)+4}, & i = 4s + (j+1)_s; \\ 0, & \text{otherwise.} \end{cases}$$

(16) If  $r_0 = 15$ , then  $\Omega^{15}(Y_t^{(4)})$  is described with  $(8s \times 8s)$ -matrix with the following elements  $b_{ij}$ :

If  $0 \leq j < s$ , then

$$b_{ij} = \begin{cases} w_{7(j+m)+6 \rightarrow 7(j+m+1)+1} \otimes e_{7j}, & i = j; \\ 0, & \text{otherwise.} \end{cases}$$

If  $s \leq j < 6s$ , then  $b_{ij} = 0$ .

If  $6s \leq j < 7s$ , then

$$b_{ij} = \begin{cases} -e_{7(j+m+1)+6} \otimes w_{7j+5 \rightarrow 7(j+1)}, & i = (j+1)_s; \\ 0, & \text{otherwise.} \end{cases}$$

If  $7s \leq j < 8s$ , then  $b_{ij} = 0$ .

(17) If  $r_0 = 16$ , then  $\Omega^{16}(Y_t^{(4)})$  is described with  $(7s \times 7s)$ -matrix with the following elements  $b_{ij}$ :

If  $0 \leq j < s$ , then

$$b_{ij} = \begin{cases} w_{7(j+m) \rightarrow 7(j+m)+6} \otimes e_{7j}, & i = j; \\ -w_{7(j+m)+1 \rightarrow 7(j+m)+6} \otimes w_{7j \rightarrow 7j+1}, & i = j+s; \\ w_{7(j+m)+2 \rightarrow 7(j+m)+6} \otimes w_{7j \rightarrow 7j+2}, & i = j+2s; \\ -w_{7(j+m)+3 \rightarrow 7(j+m)+6} \otimes w_{7j \rightarrow 7j+3}, & i = j+3s; \\ w_{7(j+m)+4 \rightarrow 7(j+m)+6} \otimes w_{7j \rightarrow 7j+4}, & i = j+4s; \\ -w_{7(j+m)+5 \rightarrow 7(j+m)+6} \otimes w_{7j \rightarrow 7j+5}, & i = j+5s; \\ e_{7(j+m)+6} \otimes w_{7j \rightarrow 7j+6}, & i = j+6s; \\ 0, & \text{otherwise.} \end{cases}$$

If  $s \leq j < 2s$ , then

$$b_{ij} = \begin{cases} w_{7(j+m+1) \rightarrow 7(j+m+1)+2} \otimes w_{7j+1 \rightarrow 7(j+1)}, & i = (j+1)_s; \\ -w_{7(j+m+1)+1 \rightarrow 7(j+m+1)+2} \otimes w_{7j+1 \rightarrow 7(j+1)+1}, & i = s + (j+1)_s; \\ 0, & \text{otherwise.} \end{cases}$$

If  $2s \leq j < 3s$ , then

$$b_{ij} = \begin{cases} w_{7(j+m+1) \rightarrow 7(j+m+1)+3} \otimes w_{7j+2 \rightarrow 7(j+1)}, & i = (j+1)_s; \\ -w_{7(j+m+1)+1 \rightarrow 7(j+m+1)+3} \otimes w_{7j+2 \rightarrow 7(j+1)+1}, & i = s + (j+1)_s; \\ w_{7(j+m+1)+2 \rightarrow 7(j+m+1)+3} \otimes w_{7j+2 \rightarrow 7(j+1)+2}, & i = 2s + (j+1)_s; \\ 0, & \text{otherwise.} \end{cases}$$

If  $3s \leq j < 4s$ , then  $b_{ij} = 0$ .

If  $4s \leq j < 5s$ , then

$$b_{ij} = \begin{cases} -w_{7(j+m+1) \rightarrow 7(j+m+1)+5} \otimes w_{7j+4 \rightarrow 7(j+1)}, & i = (j+1)_s; \\ -w_{7(j+m+1)+4 \rightarrow 7(j+m+1)+5} \otimes w_{7j+4 \rightarrow 7(j+1)+4}, & i = 4s + (j+1)_s; \\ 0, & \text{otherwise.} \end{cases}$$

If  $5s \leq j < 7s$ , then  $b_{ij} = 0$ .

(II) Represent an arbitrary  $t_0 \in \mathbb{N}$  in the form  $t_0 = 17\ell_0 + r_0$ , where  $0 \leq r_0 \leq 16$ . Then  $\Omega^{t_0}(Y_t^{(4)})$  is a  $\Omega^{r_0}(Y_t^{(4)})$ , whose left components twisted by  $\sigma^{\ell_0}$ .

**Proposition 5** (Translates for the case 6). (I) Let  $r_0 \in \mathbb{N}$ ,  $r_0 < 17$ .  $r_0$ -translates of the elements  $Y_t^{(6)}$  are described by the following way.

(1) If  $r_0 = 0$ , then  $\Omega^0(Y_t^{(6)})$  is described with  $(7s \times 10s)$ -matrix with the following elements  $b_{ij}$ :  
If  $0 \leq j < s$ , then

$$b_{ij} = \begin{cases} w_{7(j+m) \rightarrow 7(j+m)+4} \otimes e_{7j}, & i = j; \\ 0, & \text{otherwise.} \end{cases}$$

If  $s \leq j < 2s$ , then

$$b_{ij} = \begin{cases} -w_{7(j+m) \rightarrow 7(j+m)+3} \otimes e_{7j}, & i = j - s; \\ 0, & \text{otherwise.} \end{cases}$$

If  $2s \leq j < 6s$ , then  $b_{ij} = 0$ .

If  $6s \leq j < 7s$ , then

$$b_{ij} = \begin{cases} w_{7(j+m)+4 \rightarrow 7(j+m+1)} \otimes e_{7j+4}, & i = j - 2s; \\ 0, & \text{otherwise.} \end{cases}$$

If  $7s \leq j < 8s$ , then

$$b_{ij} = \begin{cases} w_{7(j+m)+5 \rightarrow 7(j+m)+6} \otimes e_{7j+5}, & i = j - 2s; \\ 0, & \text{otherwise.} \end{cases}$$

If  $8s \leq j < 9s$ , then  $b_{ij} = 0$ .

If  $9s \leq j < 10s$ , then

$$b_{ij} = \begin{cases} -w_{7(j+m)+6 \rightarrow 7(j+m+1)+5} \otimes e_{7j+6}, & i = j - 3s; \\ 0, & \text{otherwise.} \end{cases}$$

(2) If  $r_0 = 1$ , then  $\Omega^1(Y_t^{(6)})$  is described with  $(8s \times 12s)$ -matrix with the following elements  $b_{ij}$ :  
If  $0 \leq j < s$ , then

$$b_{ij} = \begin{cases} -w_{7(j+m)+4 \rightarrow 7(j+m)+6} \otimes e_{7j}, & i = j + s; \\ -w_{7(j+m)+5 \rightarrow 7(j+m)+6} \otimes w_{7j \rightarrow 7j+4}, & i = j + 5s; \\ 0, & \text{otherwise.} \end{cases}$$

If  $s \leq j < 2s$ , then

$$b_{ij} = \begin{cases} -w_{7(j+m)+4 \rightarrow 7(j+m+1)} \otimes e_{7j}, & i = j; \\ 0, & \text{otherwise.} \end{cases}$$

If  $2s \leq j < 3s$ , then

$$b_{ij} = \begin{cases} e_{7(j+m+1)+4} \otimes w_{7j+1 \rightarrow 7(j+1)}, & i = s + (j+1)s; \\ 0, & \text{otherwise.} \end{cases}$$

If  $3s \leq j < 4s$ , then  $b_{ij} = 0$ .

If  $4s \leq j < 5s$ , then

$$b_{ij} = \begin{cases} w_{7(j+m+1)+4 \rightarrow 7(j+m+1)+5} \otimes w_{7j+2 \rightarrow 7(j+1)}, & i = s + (j+1)s; \\ -w_{7(j+m)+6 \rightarrow 7(j+m+1)+5} \otimes w_{7j+2 \rightarrow 7j+3}, & i = j; \\ 0, & \text{otherwise.} \end{cases}$$



If  $5s \leq j < 7s$ , then  $b_{ij} = 0$ .

If  $7s \leq j < 8s$ , then

$$b_{ij} = \begin{cases} w_{7(j+m)+5 \rightarrow 7(j+m+1)+4} \otimes e_{7j+4}, & i = j - 2s; \\ w_{7(j+m)+6 \rightarrow 7(j+m+1)+4} \otimes w_{7j+4 \rightarrow 7j+5}, & i = j - s; \\ w_{7(j+m+1) \rightarrow 7(j+m+1)+4} \otimes w_{7j+4 \rightarrow 7j+6}, & i = j; \\ 0, & \text{otherwise.} \end{cases}$$

If  $8s \leq j < 9s$ , then

$$b_{ij} = \begin{cases} -w_{7(j+m+1)+1 \rightarrow 7(j+m+1)+3} \otimes w_{7j+5 \rightarrow 7(j+1)}, & i = (j+1)_s; \\ 0, & \text{otherwise.} \end{cases}$$

If  $9s \leq j < 10s$ , then

$$b_{ij} = \begin{cases} w_{7(j+m)+6 \rightarrow 7(j+m+1)+5} \otimes e_{7j+5}, & i = j - 3s; \\ 0, & \text{otherwise.} \end{cases}$$

If  $10s \leq j < 11s$ , then

$$b_{ij} = \begin{cases} w_{7(j+m+1) \rightarrow 7(j+m+1)+6} \otimes e_{7j+6}, & i = j - 3s; \\ 0, & \text{otherwise.} \end{cases}$$

If  $11s \leq j < 12s$ , then  $b_{ij} = 0$ .

(3) If  $r_0 = 2$ , then  $\Omega^2(Y_t^{(6)})$  is described with  $(7s \times 12s)$ -matrix with the following elements  $b_{ij}$ :  
If  $s \leq j < 2s$ , then

$$b_{ij} = \begin{cases} w_{7(j+m-1)+6 \rightarrow 7(j+m)+5} \otimes e_{7j}, & i = j - s; \\ 0, & \text{otherwise.} \end{cases}$$

If  $2s \leq j < 3s$ , then

$$b_{ij} = \begin{cases} w_{7(j+m-1)+6 \rightarrow 7(j+m)+4} \otimes e_{7j}, & i = j - 2s; \\ -e_{7(j+m)+4} \otimes w_{7j \rightarrow 7j+3}, & i = j + s; \\ 0, & \text{otherwise.} \end{cases}$$

If  $3s \leq j < 4s$ , then  $b_{ij} = 0$ .

If  $4s \leq j < 5s$ , then

$$b_{ij} = \begin{cases} -e_{7(j+m)+6} \otimes w_{7j+2 \rightarrow 7(j+1)}, & i = (j+1)_s; \\ w_{7(j+m)+3 \rightarrow 7(j+m)+6} \otimes e_{7j+2}, & i = j - 2s; \\ 0, & \text{otherwise.} \end{cases}$$

If  $5s \leq j < 6s$ , then

$$b_{ij} = \begin{cases} -w_{7(j+m)+4 \rightarrow 7(j+m+1)} \otimes e_{7j+3}, & i = j - 2s; \\ 0, & \text{otherwise.} \end{cases}$$

If  $6s \leq j < 7s$ , then

$$b_{ij} = \begin{cases} e_{7(j+m)+6} \otimes w_{7j+4 \rightarrow 7(j+1)}, & i = (j+1)_s; \\ -w_{7(j+m)+5 \rightarrow 7(j+m)+6} \otimes e_{7j+4}, & i = j - 2s; \\ 0, & \text{otherwise.} \end{cases}$$

If  $7s \leq j < 8s$ , then

$$b_{ij} = \begin{cases} -w_{7(j+m)+1 \rightarrow 7(j+m)+6} \otimes e_{7j+5}, & i = j - 2s; \\ 0, & \text{otherwise.} \end{cases}$$

If  $8s \leq j < 12s$ , then  $b_{ij} = 0$ .

(4) If  $r_0 = 3$ , then  $\Omega^3(Y_t^{(6)})$  is described with  $(9s \times 13s)$ -matrix with the following elements  $b_{ij}$ :

If  $0 \leq j < s$ , then

$$b_{ij} = \begin{cases} -w_{7(j+m)+2 \rightarrow 7(j+m)+6} \otimes e_{7j}, & i = j; \\ -w_{7(j+m)+5 \rightarrow 7(j+m)+6} \otimes e_{7j}, & i = j + s; \\ -w_{7(j+m)+3 \rightarrow 7(j+m)+6} \otimes w_{7j \rightarrow 7j+1}, & i = j + 2s; \\ 0, & \text{otherwise.} \end{cases}$$

If  $s \leq j < 2s$ , then

$$b_{ij} = \begin{cases} -w_{7(j+m)+6 \rightarrow 7(j+m+1)} \otimes w_{7j \rightarrow 7j+2}, & i = j + 2s; \\ 0, & \text{otherwise.} \end{cases}$$

If  $2s \leq j < 3s$ , then

$$b_{ij} = \begin{cases} w_{7(j+m)+6 \rightarrow 7(j+m+1)+1} \otimes w_{7j+1 \rightarrow 7j+2}, & i = j + s; \\ 0, & \text{otherwise.} \end{cases}$$

If  $3s \leq j < 4s$ , then

$$b_{ij} = \begin{cases} -e_{7(j+m+1)+5} \otimes w_{7j+1 \rightarrow 7(j+1)}, & i = s + (j+1)_s; \\ 0, & \text{otherwise.} \end{cases}$$

If  $4s \leq j < 5s$ , then

$$b_{ij} = \begin{cases} w_{7(j+m)+6 \rightarrow 7(j+m+1)+2} \otimes e_{7j+2}, & i = j - s; \\ 0, & \text{otherwise.} \end{cases}$$

If  $5s \leq j < 6s$ , then  $b_{ij} = 0$ .

If  $6s \leq j < 7s$ , then

$$b_{ij} = \begin{cases} -w_{7(j+m+1) \rightarrow 7(j+m+1)+4} \otimes e_{7j+3}, & i = j - 2s; \\ -e_{7(j+m+1)+4} \otimes w_{7j+3 \rightarrow 7j+6}, & i = j + 2s; \\ 0, & \text{otherwise.} \end{cases}$$

If  $7s \leq j < 8s$ , then

$$b_{ij} = \begin{cases} w_{7(j+m+1)+2 \rightarrow 7(j+m+1)+3} \otimes w_{7j+4 \rightarrow 7(j+1)}, & i = (j+1)_s; \\ 0, & \text{otherwise.} \end{cases}$$

If  $8s \leq j < 9s$ , then

$$b_{ij} = \begin{cases} -w_{7(j+m)+6 \rightarrow 7(j+m+1)+5} \otimes e_{7j+4}, & i = j - 3s; \\ 0, & \text{otherwise.} \end{cases}$$

If  $9s \leq j < 11s$ , then  $b_{ij} = 0$ .

If  $11s \leq j < 12s$ , then

$$b_{ij} = \begin{cases} -w_{7(j+m+1)+5 \rightarrow 7(j+m+1)+6} \otimes w_{7j+6 \rightarrow 7(j+1)}, & i = s + (j+1)_s; \\ 0, & \text{otherwise.} \end{cases}$$

If  $12s \leq j < 13s$ , then

$$b_{ij} = \begin{cases} w_{7(j+m+1)+5 \rightarrow 7(j+m+2)} \otimes w_{7j+6 \rightarrow 7(j+1)}, & i = s + (j+1)_s; \\ 0, & \text{otherwise.} \end{cases}$$

(5) If  $r_0 = 4$ , then  $\Omega^4(Y_t^{(6)})$  is described with  $(10s \times 12s)$ -matrix with the following elements  $b_{ij}$ :

If  $0 \leq j < s$ , then

$$b_{ij} = \begin{cases} w_{7(j+m-1)+6 \rightarrow 7(j+m)+5} \otimes e_{7j}, & i = j; \\ w_{7(j+m)+4 \rightarrow 7(j+m)+5} \otimes w_{7j \rightarrow 7j+2}, & i = j + 3s; \\ e_{7(j+m)+5} \otimes w_{7j \rightarrow 7j+3}, & i = j + 5s; \\ 0, & \text{otherwise.} \end{cases}$$

If  $s \leq j < 2s$ , then

$$b_{ij} = \begin{cases} -e_{7(j+m)+3} \otimes w_{7j \rightarrow 7j+1}, & i = j + s; \\ 0, & \text{otherwise.} \end{cases}$$

If  $2s \leq j < 3s$ , then  $b_{ij} = 0$ .

If  $3s \leq j < 4s$ , then

$$b_{ij} = \begin{cases} e_{7(j+m)+6} \otimes w_{7j+1 \rightarrow 7(j+1)}, & i = (j+1)_s; \\ 0, & \text{otherwise.} \end{cases}$$

If  $4s \leq j < 5s$ , then

$$b_{ij} = \begin{cases} -w_{7(j+m)+6 \rightarrow 7(j+m+1)} \otimes w_{7j+2 \rightarrow 7(j+1)}, & i = (j+1)_s; \\ -e_{7(j+m+1)} \otimes w_{7j+2 \rightarrow 7(j+1)}, & i = s + (j+1)_s; \\ 0, & \text{otherwise.} \end{cases}$$

If  $5s \leq j < 6s$ , then

$$b_{ij} = \begin{cases} w_{7(j+m)+5 \rightarrow 7(j+m)+6} \otimes e_{7j+3}, & i = j; \\ 0, & \text{otherwise.} \end{cases}$$

If  $6s \leq j < 7s$ , then

$$b_{ij} = \begin{cases} w_{7(j+m)+1 \rightarrow 7(j+m)+6} \otimes e_{7j+4}, & i = j; \\ -w_{7(j+m)+2 \rightarrow 7(j+m)+6} \otimes w_{7j+4 \rightarrow 7j+5}, & i = j + s; \\ 0, & \text{otherwise.} \end{cases}$$

If  $7s \leq j < 10s$ , then  $b_{ij} = 0$ .

If  $10s \leq j < 11s$ , then

$$b_{ij} = \begin{cases} w_{7(j+m)+6 \rightarrow 7(j+m+1)+5} \otimes w_{7j+6 \rightarrow 7(j+1)}, & i = (j+1)_s; \\ -w_{7(j+m+1)+4 \rightarrow 7(j+m+1)+5} \otimes w_{7j+6 \rightarrow 7(j+1)+2}, & i = 3s + (j+1)_s; \\ e_{7(j+m+1)+5} \otimes w_{7j+6 \rightarrow 7(j+1)+3}, & i = 5s + (j+1)_s; \\ 0, & \text{otherwise.} \end{cases}$$

If  $11s \leq j < 12s$ , then

$$b_{ij} = \begin{cases} -e_{7(j+m+1)+4} \otimes w_{7j+6 \rightarrow 7(j+1)+2}, & i = 3s + (j+1)_s; \\ 0, & \text{otherwise.} \end{cases}$$

(6) If  $r_0 = 5$ , then  $\Omega^5(Y_t^{(6)})$  is described with  $(10s \times 12s)$ -matrix with the following elements  $b_{ij}$ :

If  $0 \leq j < s$ , then

$$b_{ij} = \begin{cases} w_{7(j+m)+3 \rightarrow 7(j+m)+6} \otimes e_{7j}, & i = j + s; \\ -e_{7(j+m)+6} \otimes w_{7j \rightarrow 7j+1}, & i = j + 3s; \\ 0, & \text{otherwise.} \end{cases}$$

If  $s \leq j < 2s$ , then

$$b_{ij} = \begin{cases} -w_{7(j+m)+3 \rightarrow 7(j+m+1)} \otimes e_{7j}, & i = j; \\ w_{7(j+m)+6 \rightarrow 7(j+m+1)} \otimes w_{7j \rightarrow 7j+1}, & i = j + 2s; \\ e_{7(j+m+1)} \otimes w_{7j \rightarrow 7j+2}, & i = j + 3s; \\ 0, & \text{otherwise.} \end{cases}$$

If  $2s \leq j < 3s$ , then

$$b_{ij} = \begin{cases} -w_{7(j+m+1)+1 \rightarrow 7(j+m+1)+2} \otimes w_{7j+1 \rightarrow 7(j+1)}, & i = 2s + (j+1)_s; \\ 0, & \text{otherwise.} \end{cases}$$

If  $3s \leq j < 4s$ , then

$$b_{ij} = \begin{cases} -e_{7(j+m+1)+3} \otimes w_{7j+2 \rightarrow 7(j+1)}, & i = s + (j+1)_s; \\ -w_{7(j+m+1)+1 \rightarrow 7(j+m+1)+3} \otimes w_{7j+2 \rightarrow 7(j+1)}, & i = 2s + (j+1)_s; \\ 0, & \text{otherwise.} \end{cases}$$

If  $4s \leq j < 5s$ , then

$$b_{ij} = \begin{cases} -e_{7(j+m+1)+4} \otimes w_{7j+2 \rightarrow 7(j+1)}, & i = (j+1)_s; \\ 0, & \text{otherwise.} \end{cases}$$

If  $5s \leq j < 6s$ , then

$$b_{ij} = \begin{cases} -w_{7(j+m)+6 \rightarrow 7(j+m+1)+5} \otimes e_{7j+3}, & i = j; \\ -e_{7(j+m+1)+5} \otimes w_{7j+3 \rightarrow 7j+6}, & i = j + 4s; \\ 0, & \text{otherwise.} \end{cases}$$

If  $6s \leq j < 11s$ , then  $b_{ij} = 0$ .

If  $11s \leq j < 12s$ , then

$$b_{ij} = \begin{cases} -e_{7(j+m+2)} \otimes w_{7j+6 \rightarrow 7(j+1)+2}, & i = 4s + (j+1)_s; \\ 0, & \text{otherwise.} \end{cases}$$

(7) If  $r_0 = 6$ , then  $\Omega^6(Y_t^{(6)})$  is described with  $(12s \times 10s)$ -matrix with the following elements  $b_{ij}$ :

If  $0 \leq j < s$ , then

$$b_{ij} = \begin{cases} w_{7(j+m)+1 \rightarrow 7(j+m)+2} \otimes w_{7j \rightarrow 7j+2}, & i = j + 3s; \\ 0, & \text{otherwise.} \end{cases}$$

If  $s \leq j < 2s$ , then

$$b_{ij} = \begin{cases} e_{7(j+m)+4} \otimes w_{7j \rightarrow 7j+1}, & i = j + s; \\ 0, & \text{otherwise.} \end{cases}$$

If  $2s \leq j < 3s$ , then

$$b_{ij} = \begin{cases} -e_{7(j+m+1)} \otimes w_{7j+1 \rightarrow 7(j+1)}, & i = s + (j+1)_s; \\ 0, & \text{otherwise.} \end{cases}$$

If  $3s \leq j < 4s$ , then

$$b_{ij} = \begin{cases} -e_{7(j+m)+6} \otimes w_{7j+2 \rightarrow 7(j+1)}, & i = (j+1)_s; \\ w_{7(j+m)+1 \rightarrow 7(j+m)+6} \otimes e_{7j+2}, & i = j; \\ -w_{7(j+m)+5 \rightarrow 7(j+m)+6} \otimes e_{7j+2}, & i = j + s; \\ 0, & \text{otherwise.} \end{cases}$$

If  $4s \leq j < 5s$ , then

$$b_{ij} = \begin{cases} -e_{7(j+m+1)} \otimes w_{7j+3 \rightarrow 7(j+1)}, & i = s + (j+1)_s; \\ -w_{7(j+m)+2 \rightarrow 7(j+m)+1} \otimes e_{7j+3}, & i = j + s; \\ w_{7(j+m)+6 \rightarrow 7(j+m)+1} \otimes w_{7j+3 \rightarrow 7j+6}, & i = j + 6s; \\ 0, & \text{otherwise.} \end{cases}$$

If  $5s \leq j < 7s$ , then  $b_{ij} = 0$ .

If  $7s \leq j < 8s$ , then

$$b_{ij} = \begin{cases} e_{7(j+m+1)+5} \otimes w_{7j+6 \rightarrow 7(j+1)+2}, & i = 4s + (j+1)_s; \\ 0, & \text{otherwise.} \end{cases}$$

If  $8s \leq j < 9s$ , then  $b_{ij} = 0$ .

If  $9s \leq j < 10s$ , then

$$b_{ij} = \begin{cases} -e_{7(j+m+1)+1} \otimes w_{7j+6 \rightarrow 7(j+1)+2}, & i = 3s + (j+1)_s; \\ 0, & \text{otherwise.} \end{cases}$$

(8) If  $r_0 = 7$ , then  $\Omega^7(Y_t^{(6)})$  is described with  $(12s \times 10s)$ -matrix with the following elements  $b_{ij}$ :

If  $0 \leq j < s$ , then

$$b_{ij} = \begin{cases} -e_{7(j+m+1)} \otimes w_{7j \rightarrow 7j+1}, & i = j + 3s; \\ w_{7(j+m)+6 \rightarrow 7(j+m+1)} \otimes w_{7j \rightarrow 7j+2}, & i = j + 4s; \\ 0, & \text{otherwise.} \end{cases}$$

If  $s \leq j < 2s$ , then

$$b_{ij} = \begin{cases} -w_{7(j+m+1)+2 \rightarrow 7(j+m+1)+3} \otimes w_{7j+1 \rightarrow 7(j+1)}, & i = (j+1)_s; \\ 0, & \text{otherwise.} \end{cases}$$

If  $2s \leq j < 3s$ , then

$$b_{ij} = \begin{cases} -e_{7(j+m+1)+4} \otimes w_{7j+1 \rightarrow 7(j+1)}, & i = 2s + (j+1)_s; \\ 0, & \text{otherwise.} \end{cases}$$

If  $3s \leq j < 4s$ , then

$$b_{ij} = \begin{cases} e_{7(j+m+1)+5} \otimes w_{7j+2 \rightarrow 7(j+1)}, & i = s + (j+1)_s; \\ -w_{7(j+m+1)+4 \rightarrow 7(j+m+1)+5} \otimes w_{7j+2 \rightarrow 7(j+1)}, & i = 2s + (j+1)_s; \\ w_{7(j+m)+6 \rightarrow 7(j+m+1)+5} \otimes e_{7j+2}, & i = j + s; \\ 0, & \text{otherwise.} \end{cases}$$

If  $4s \leq j < 5s$ , then

$$b_{ij} = \begin{cases} -w_{7(j+m+1) \rightarrow 7(j+m+1)+1} \otimes e_{7j+3}, & i = j + s; \\ -e_{7(j+m+1)+1} \otimes w_{7j+3 \rightarrow 7j+6}, & i = j + 7s; \\ 0, & \text{otherwise.} \end{cases}$$

If  $5s \leq j < 10s$ , then  $b_{ij} = 0$ .

(9) If  $r_0 = 8$ , then  $\Omega^8(Y_t^{(6)})$  is described with  $(13s \times 9s)$ -matrix with the following elements  $b_{ij}$ :

If  $0 \leq j < s$ , then

$$b_{ij} = \begin{cases} -w_{7(j+m)+1 \rightarrow 7(j+m)+3} \otimes w_{7j \rightarrow 7j+1}, & i = j + 2s; \\ -w_{7(j+m)+2 \rightarrow 7(j+m)+3} \otimes w_{7j \rightarrow 7j+2}, & i = j + 4s; \\ 0, & \text{otherwise.} \end{cases}$$

If  $s \leq j < 2s$ , then

$$b_{ij} = \begin{cases} -e_{7(j+m)+5} \otimes w_{7j \rightarrow 7j+1}, & i = j + 2s; \\ 0, & \text{otherwise.} \end{cases}$$

If  $2s \leq j < 3s$ , then

$$b_{ij} = \begin{cases} -e_{7(j+m)+6} \otimes w_{7j+1 \rightarrow 7(j+1)}, & i = (j+1)_s; \\ -w_{7(j+m)+1 \rightarrow 7(j+m)+6} \otimes e_{7j+1}, & i = j; \\ w_{7(j+m)+5 \rightarrow 7(j+m)+6} \otimes e_{7j+1}, & i = j + s; \\ 0, & \text{otherwise.} \end{cases}$$

If  $3s \leq j < 4s$ , then

$$b_{ij} = \begin{cases} w_{7(j+m)+6 \rightarrow 7(j+m+1)} \otimes w_{7j+2 \rightarrow 7(j+1)}, & i = (j+1)_s; \\ -e_{7(j+m+1)} \otimes w_{7j+2 \rightarrow 7(j+1)}, & i = s + (j+1)_s; \\ w_{7(j+m)+2 \rightarrow 7(j+m+1)} \otimes e_{7j+2}, & i = j + s; \\ 0, & \text{otherwise.} \end{cases}$$

If  $4s \leq j < 5s$ , then

$$b_{ij} = \begin{cases} -w_{7(j+m+1) \rightarrow 7(j+m+1)+1} \otimes w_{7j+3 \rightarrow 7(j+1)}, & i = s + (j+1)_s; \\ -w_{7(j+m)+3 \rightarrow 7(j+m+1)+1} \otimes e_{7j+3}, & i = j + s; \\ w_{7(j+m+1) \rightarrow 7(j+m+1)+1} \otimes w_{7j+3 \rightarrow 7j+6}, & i = j + 8s; \\ 0, & \text{otherwise.} \end{cases}$$

If  $5s \leq j < 7s$ , then  $b_{ij} = 0$ .

If  $7s \leq j < 8s$ , then

$$b_{ij} = \begin{cases} w_{7(j+m+1)+1 \rightarrow 7(j+m+1)+2} \otimes w_{7j+6 \rightarrow 7(j+1)+1}, & i = 2s + (j+1)_s; \\ e_{7(j+m+1)+2} \otimes w_{7j+6 \rightarrow 7(j+1)+2}, & i = 4s + (j+1)_s; \\ 0, & \text{otherwise.} \end{cases}$$

If  $8s \leq j < 9s$ , then  $b_{ij} = 0$ .

(10) If  $r_0 = 9$ , then  $\Omega^9(Y_t^{(6)})$  is described with  $(12s \times 7s)$ -matrix with the following elements  $b_{ij}$ :

If  $0 \leq j < s$ , then

$$b_{ij} = \begin{cases} e_{7(j+m)+6} \otimes w_{7j \rightarrow 7j+1}, & i = j + 3s; \\ 0, & \text{otherwise.} \end{cases}$$

If  $s \leq j < 2s$ , then

$$b_{ij} = \begin{cases} -e_{7(j+m+1)+5} \otimes w_{7j+1 \rightarrow 7(j+1)}, & i = (j+1)_s; \\ -w_{7(j+m)+6 \rightarrow 7(j+m+1)+5} \otimes e_{7j+1}, & i = j + 2s; \\ 0, & \text{otherwise.} \end{cases}$$

If  $2s \leq j < 3s$ , then

$$b_{ij} = \begin{cases} w_{7(j+m+1) \rightarrow 7(j+m+1)+1} \otimes e_{7j+2}, & i = j + 2s; \\ 0, & \text{otherwise.} \end{cases}$$

If  $3s \leq j < 4s$ , then

$$b_{ij} = \begin{cases} -w_{7(j+m+1)+1 \rightarrow 7(j+m+1)+2} \otimes w_{7j+3 \rightarrow 7(j+1)}, & i = 2s + (j+1)_s; \\ -w_{7(j+m)+6 \rightarrow 7(j+m+1)+2} \otimes e_{7j+3}, & i = j + 2s; \\ e_{7(j+m+1)+2} \otimes w_{7j+3 \rightarrow 7j+6}, & i = j + 6s; \\ 0, & \text{otherwise.} \end{cases}$$

If  $4s \leq j < 6s$ , then  $b_{ij} = 0$ .

If  $6s \leq j < 7s$ , then

$$b_{ij} = \begin{cases} -w_{7(j+m+1)+6 \rightarrow 7(j+m+2)} \otimes w_{7j+6 \rightarrow 7(j+1)+1}, & i = 3s + (j+1)_s; \\ 0, & \text{otherwise.} \end{cases}$$

(11) If  $r_0 = 10$ , then  $\Omega^{10}(Y_t^{(6)})$  is described with  $(12s \times 8s)$ -matrix with the following elements  $b_{ij}$ :

If  $0 \leq j < s$ , then

$$b_{ij} = \begin{cases} e_{7(j+m)+6} \otimes w_{7j \rightarrow 7(j+1)}, & i = (j+1)_s; \\ -w_{7(j+m)+2 \rightarrow 7(j+m)+6} \otimes w_{7j \rightarrow 7j+1}, & i = j+2s; \\ -w_{7(j+m)+3 \rightarrow 7(j+m)+6} \otimes w_{7j \rightarrow 7j+2}, & i = j+3s; \\ 0, & \text{otherwise.} \end{cases}$$

If  $s \leq j < 2s$ , then

$$b_{ij} = \begin{cases} -w_{7(j+m)+6 \rightarrow 7(j+m+1)} \otimes w_{7j+1 \rightarrow 7(j+1)}, & i = (j+1)_s; \\ -e_{7(j+m+1)} \otimes w_{7j+1 \rightarrow 7(j+1)}, & i = s + (j+1)_s; \\ -w_{7(j+m)+2 \rightarrow 7(j+m+1)} \otimes e_{7j+1}, & i = j+s; \\ 0, & \text{otherwise.} \end{cases}$$

If  $2s \leq j < 3s$ , then

$$b_{ij} = \begin{cases} w_{7(j+m)+6 \rightarrow 7(j+m+1)+1} \otimes w_{7j+2 \rightarrow 7(j+1)}, & i = (j+1)_s; \\ -w_{7(j+m+1) \rightarrow 7(j+m+1)+1} \otimes w_{7j+2 \rightarrow 7(j+1)}, & i = s + (j+1)_s; \\ w_{7(j+m)+3 \rightarrow 7(j+m+1)+1} \otimes e_{7j+2}, & i = j+s; \\ 0, & \text{otherwise.} \end{cases}$$

If  $3s \leq j < 4s$ , then

$$b_{ij} = \begin{cases} w_{7(j+m)+6 \rightarrow 7(j+m+1)+2} \otimes w_{7j+3 \rightarrow 7(j+1)}, & i = (j+1)_s; \\ w_{7(j+m+1) \rightarrow 7(j+m+1)+2} \otimes w_{7j+3 \rightarrow 7(j+1)}, & i = s + (j+1)_s; \\ w_{7(j+m)+6 \rightarrow 7(j+m+1)+2} \otimes w_{7j+3 \rightarrow 7j+6}, & i = j+7s; \\ 0, & \text{otherwise.} \end{cases}$$

If  $4s \leq j < 6s$ , then  $b_{ij} = 0$ .

If  $6s \leq j < 7s$ , then

$$b_{ij} = \begin{cases} w_{7(j+m+1)+2 \rightarrow 7(j+m+1)+3} \otimes w_{7j+6 \rightarrow 7(j+1)+1}, & i = 2s + (j+1)_s; \\ e_{7(j+m+1)+3} \otimes w_{7j+6 \rightarrow 7(j+1)+2}, & i = 3s + (j+1)_s; \\ 0, & \text{otherwise.} \end{cases}$$

If  $7s \leq j < 8s$ , then  $b_{ij} = 0$ .

(12) If  $r_0 = 11$ , then  $\Omega^{11}(Y_t^{(6)})$  is described with  $(10s \times 7s)$ -matrix with the following elements  $b_{ij}$ :

If  $0 \leq j < s$ , then

$$b_{ij} = \begin{cases} e_{7(j+m+1)} \otimes w_{7j \rightarrow 7j+1}, & i = j+2s; \\ 0, & \text{otherwise.} \end{cases}$$

If  $s \leq j < 2s$ , then

$$b_{ij} = \begin{cases} -w_{7(j+m+1) \rightarrow 7(j+m+1)+1} \otimes e_{7j+1}, & i = j+s; \\ 0, & \text{otherwise.} \end{cases}$$



If  $2s \leq j < 3s$ , then

$$b_{ij} = \begin{cases} w_{7(j+m)+6 \rightarrow 7(j+m+1)+2} \otimes e_{7j+2}, & i = j + s; \\ 0, & \text{otherwise.} \end{cases}$$

If  $3s \leq j < 4s$ , then

$$b_{ij} = \begin{cases} w_{7(j+m+1)+2 \rightarrow 7(j+m+1)+3} \otimes w_{7j+3 \rightarrow 7(j+1)}, & i = (j+1)s; \\ e_{7(j+m+1)+3} \otimes w_{7j+3 \rightarrow 7j+6}, & i = j + 5s; \\ 0, & \text{otherwise.} \end{cases}$$

If  $4s \leq j < 7s$ , then  $b_{ij} = 0$ .

(13) If  $r_0 = 12$ , then  $\Omega^{12}(Y_t^{(6)})$  is described with  $(10s \times 7s)$ -matrix with the following elements  $b_{ij}$ :

If  $0 \leq j < s$ , then

$$b_{ij} = \begin{cases} e_{7(j+m+1)} \otimes w_{7j \rightarrow 7(j+1)}, & i = (j+1)s; \\ w_{7(j+m)+3 \rightarrow 7(j+m+1)} \otimes w_{7j \rightarrow 7j+1}, & i = j + s; \\ w_{7(j+m)+4 \rightarrow 7(j+m+1)} \otimes w_{7j \rightarrow 7j+1}, & i = j + 2s; \\ 0, & \text{otherwise.} \end{cases}$$

If  $s \leq j < 2s$ , then

$$b_{ij} = \begin{cases} -w_{7(j+m+1) \rightarrow 7(j+m+1)+1} \otimes w_{7j+1 \rightarrow 7(j+1)}, & i = (j+1)s; \\ -w_{7(j+m)+3 \rightarrow 7(j+m+1)+1} \otimes e_{7j+1}, & i = j; \\ 0, & \text{otherwise.} \end{cases}$$

If  $2s \leq j < 3s$ , then

$$b_{ij} = \begin{cases} w_{7(j+m+1) \rightarrow 7(j+m+1)+2} \otimes w_{7j+2 \rightarrow 7(j+1)}, & i = (j+1)s; \\ w_{7(j+m)+6 \rightarrow 7(j+m+1)+2} \otimes w_{7j+2 \rightarrow 7j+6}, & i = j + 6s; \\ 0, & \text{otherwise.} \end{cases}$$

If  $3s \leq j < 4s$ , then

$$b_{ij} = \begin{cases} -e_{7(j+m+1)+3} \otimes w_{7j+3 \rightarrow 7(j+1)+1}, & i = s + (j+1)s; \\ -w_{7(j+m)+6 \rightarrow 7(j+m+1)+3} \otimes w_{7j+3 \rightarrow 7j+6}, & i = j + 5s; \\ 0, & \text{otherwise.} \end{cases}$$

If  $4s \leq j < 6s$ , then  $b_{ij} = 0$ .

If  $6s \leq j < 7s$ , then

$$b_{ij} = \begin{cases} -w_{7(j+m+1)+3 \rightarrow 7(j+m+1)+6} \otimes w_{7j+6 \rightarrow 7(j+1)+1}, & i = s + (j+1)s; \\ -w_{7(j+m+1)+4 \rightarrow 7(j+m+1)+6} \otimes w_{7j+6 \rightarrow 7(j+1)+1}, & i = 2s + (j+1)s; \\ 0, & \text{otherwise.} \end{cases}$$

(14) If  $r_0 = 13$ , then  $\Omega^{13}(Y_t^{(6)})$  is described with  $(9s \times 8s)$ -matrix with the following elements  $b_{ij}$ :

If  $s \leq j < 2s$ , then

$$b_{ij} = \begin{cases} -w_{7(j+m)+6 \rightarrow 7(j+m+1)+4} \otimes w_{7j \rightarrow 7j+1}, & i = j + s; \\ -w_{7(j+m+1) \rightarrow 7(j+m+1)+4} \otimes w_{7j \rightarrow 7j+2}, & i = j + 2s; \\ -w_{7(j+m+1) \rightarrow 7(j+m+1)+4} \otimes w_{7j \rightarrow 7j+5}, & i = j + 5s; \\ 0, & \text{otherwise.} \end{cases}$$

If  $2s \leq j < 3s$ , then

$$b_{ij} = \begin{cases} w_{7(j+m)+6 \rightarrow 7(j+m+1)+2} \otimes e_{7j+1}, & i = j; \\ 0, & \text{otherwise.} \end{cases}$$

If  $3s \leq j < 4s$ , then

$$b_{ij} = \begin{cases} -e_{7(j+m+1)+3} \otimes w_{7j+2 \rightarrow 7(j+1)}, & i = (j+1)_s; \\ 0, & \text{otherwise.} \end{cases}$$

If  $4s \leq j < 5s$ , then

$$b_{ij} = \begin{cases} w_{7(j+m+1)+3 \rightarrow 7(j+m+1)+6} \otimes w_{7j+3 \rightarrow 7(j+1)}, & i = (j+1)_s; \\ -w_{7(j+m+1)+1 \rightarrow 7(j+m+1)+6} \otimes e_{7j+3}, & i = j; \\ -w_{7(j+m+1)+4 \rightarrow 7(j+m+1)+6} \otimes w_{7j+3 \rightarrow 7j+6}, & i = j + 4s; \\ 0, & \text{otherwise.} \end{cases}$$

If  $5s \leq j < 8s$ , then  $b_{ij} = 0$ .

(15) If  $r_0 = 14$ , then  $\Omega^{14}(Y_t^{(6)})$  is described with  $(7s \times 7s)$ -matrix with the following elements  $b_{ij}$ :

If  $0 \leq j < s$ , then

$$b_{ij} = \begin{cases} w_{7(j+m-1)+6 \rightarrow 7(j+m)+6} \otimes e_{7j}, & i = j; \\ e_{7(j+m)+6} \otimes w_{7j \rightarrow 7(j+1)}, & i = (j+1)_s; \\ w_{7(j+m)+5 \rightarrow 7(j+m)+6} \otimes w_{7j \rightarrow 7j+1}, & i = j + s; \\ -w_{7(j+m)+2 \rightarrow 7(j+m)+6} \otimes w_{7j \rightarrow 7j+3}, & i = j + 3s; \\ w_{7(j+m)+3 \rightarrow 7(j+m)+6} \otimes w_{7j \rightarrow 7j+4}, & i = j + 4s; \\ 0, & \text{otherwise.} \end{cases}$$

If  $s \leq j < 2s$ , then

$$b_{ij} = \begin{cases} w_{7(j+m)+6 \rightarrow 7(j+m+1)+2} \otimes w_{7j+1 \rightarrow 7(j+1)}, & i = (j+1)_s; \\ 0, & \text{otherwise.} \end{cases}$$

If  $2s \leq j < 3s$ , then

$$b_{ij} = \begin{cases} -w_{7(j+m)+6 \rightarrow 7(j+m+1)+3} \otimes w_{7j+2 \rightarrow 7(j+1)}, & i = (j+1)_s; \\ 0, & \text{otherwise.} \end{cases}$$

If  $3s \leq j < 4s$ , then

$$b_{ij} = \begin{cases} -w_{7(j+m+1) \rightarrow 7(j+m+1)+4} \otimes w_{7j+3 \rightarrow 7j+6}, & i = j + 3s; \\ 0, & \text{otherwise.} \end{cases}$$

If  $4s \leq j < 6s$ , then  $b_{ij} = 0$ .

If  $6s \leq j < 7s$ , then

$$b_{ij} = \begin{cases} -w_{7(j+m+1)+5 \rightarrow 7(j+m+2)} \otimes w_{7j+6 \rightarrow 7(j+1)+1}, & i = s + (j+1)_s; \\ w_{7(j+m+1)+1 \rightarrow 7(j+m+2)} \otimes w_{7j+6 \rightarrow 7(j+1)+2}, & i = 2s + (j+1)_s; \\ 0, & \text{otherwise.} \end{cases}$$

(16) If  $r_0 = 15$ , then  $\Omega^{15}(Y_t^{(6)})$  is described with  $(8s \times 9s)$ -matrix with the following elements  $b_{ij}$ :

If  $0 \leq j < s$ , then

$$b_{ij} = \begin{cases} w_{7(j+m+1) \rightarrow 7(j+m+1)+2} \otimes w_{7j \rightarrow 7j+1}, & i = j + s; \\ -w_{7(j+m+1) \rightarrow 7(j+m+1)+2} \otimes w_{7j \rightarrow 7j+4}, & i = j + 4s; \\ 0, & \text{otherwise.} \end{cases}$$

If  $s \leq j < 2s$ , then

$$b_{ij} = \begin{cases} w_{7(j+m+1) \rightarrow 7(j+m+1)+5} \otimes w_{7j \rightarrow 7j+1}, & i = j; \\ 0, & \text{otherwise.} \end{cases}$$

If  $2s \leq j < 3s$ , then  $b_{ij} = 0$ .

If  $3s \leq j < 4s$ , then

$$b_{ij} = \begin{cases} e_{7(j+m+1)+6} \otimes w_{7j+2 \rightarrow 7(j+1)}, & i = (j+1)_s; \\ w_{7(j+m+1)+1 \rightarrow 7(j+m+1)+6} \otimes e_{7j+2}, & i = j - s; \\ 0, & \text{otherwise.} \end{cases}$$

If  $4s \leq j < 5s$ , then

$$b_{ij} = \begin{cases} -w_{7(j+m+1)+2 \rightarrow 7(j+m+2)} \otimes e_{7j+3}, & i = j - s; \\ 0, & \text{otherwise.} \end{cases}$$

If  $5s \leq j < 6s$ , then

$$b_{ij} = \begin{cases} e_{7(j+m+1)+6} \otimes w_{7j+4 \rightarrow 7(j+1)}, & i = (j+1)_s; \\ 0, & \text{otherwise.} \end{cases}$$

If  $6s \leq j < 7s$ , then  $b_{ij} = 0$ .

If  $7s \leq j < 8s$ , then

$$b_{ij} = \begin{cases} -w_{7(j+m+1)+6 \rightarrow 7(j+m+2)+1} \otimes w_{7j+6 \rightarrow 7(j+1)}, & i = (j+1)_s; \\ 0, & \text{otherwise.} \end{cases}$$

If  $8s \leq j < 9s$ , then

$$b_{ij} = \begin{cases} -w_{7(j+m+2) \rightarrow 7(j+m+2)+4} \otimes w_{7j+6 \rightarrow 7(j+1)+1}, & i = s + (j+1)_s; \\ 0, & \text{otherwise.} \end{cases}$$

(17) If  $r_0 = 16$ , then  $\Omega^{16}(Y_t^{(6)})$  is described with  $(7s \times 10s)$ -matrix with the following elements  $b_{ij}$ :

If  $0 \leq j < s$ , then

$$b_{ij} = \begin{cases} -w_{7(j+m)+1 \rightarrow 7(j+m)+6} \otimes w_{7j \rightarrow 7j+1}, & i = j + s; \\ -w_{7(j+m)+2 \rightarrow 7(j+m)+6} \otimes w_{7j \rightarrow 7j+2}, & i = j + 2s; \\ w_{7(j+m)+3 \rightarrow 7(j+m)+6} \otimes w_{7j \rightarrow 7j+3}, & i = j + 3s; \\ -w_{7(j+m)+4 \rightarrow 7(j+m)+6} \otimes w_{7j \rightarrow 7j+4}, & i = j + 4s; \\ w_{7(j+m)+5 \rightarrow 7(j+m)+6} \otimes w_{7j \rightarrow 7j+5}, & i = j + 5s; \\ -e_{7(j+m)+6} \otimes w_{7j \rightarrow 7j+6}, & i = j + 6s; \\ 0, & \text{otherwise.} \end{cases}$$

If  $s \leq j < 2s$ , then

$$b_{ij} = \begin{cases} w_{7(j+m) \rightarrow 7(j+m+1)} \otimes e_{7j}, & i = j - s; \\ -w_{7(j+m)+3 \rightarrow 7(j+m+1)} \otimes w_{7j \rightarrow 7j+3}, & i = j + 2s; \\ w_{7(j+m)+4 \rightarrow 7(j+m+1)} \otimes w_{7j \rightarrow 7j+4}, & i = j + 3s; \\ -w_{7(j+m)+5 \rightarrow 7(j+m+1)} \otimes w_{7j \rightarrow 7j+5}, & i = j + 4s; \\ w_{7(j+m)+6 \rightarrow 7(j+m+1)} \otimes w_{7j \rightarrow 7j+6}, & i = j + 5s; \\ 0, & \text{otherwise.} \end{cases}$$

If  $2s \leq j < 3s$ , then

$$b_{ij} = \begin{cases} w_{7(j+m+1) \rightarrow 7(j+m+1)+3} \otimes w_{7j+1 \rightarrow 7(j+1)}, & i = (j+1)_s; \\ w_{7(j+m+1)+1 \rightarrow 7(j+m+1)+3} \otimes w_{7j+1 \rightarrow 7(j+1)+1}, & i = s + (j+1)_s; \\ 0, & \text{otherwise.} \end{cases}$$

If  $3s \leq j < 4s$ , then

$$b_{ij} = \begin{cases} -w_{7(j+m+1) \rightarrow 7(j+m+1)+4} \otimes w_{7j+2 \rightarrow 7(j+1)}, & i = (j+1)_s; \\ 0, & \text{otherwise.} \end{cases}$$

If  $4s \leq j < 5s$ , then

$$b_{ij} = \begin{cases} w_{7(j+m)+3 \rightarrow 7(j+m+1)+1} \otimes e_{7j+3}, & i = j - s; \\ -w_{7(j+m)+6 \rightarrow 7(j+m+1)+1} \otimes w_{7j+3 \rightarrow 7j+6}, & i = j + 2s; \\ 0, & \text{otherwise.} \end{cases}$$

If  $5s \leq j < 7s$ , then  $b_{ij} = 0$ .

If  $7s \leq j < 8s$ , then

$$b_{ij} = \begin{cases} w_{7(j+m+1) \rightarrow 7(j+m+1)+2} \otimes w_{7j+5 \rightarrow 7(j+1)}, & i = (j+1)_s; \\ 0, & \text{otherwise.} \end{cases}$$

If  $8s \leq j < 9s$ , then  $b_{ij} = 0$ .

If  $9s \leq j < 10s$ , then

$$b_{ij} = \begin{cases} -w_{7(j+m+1)+1 \rightarrow 7(j+m+1)+6} \otimes w_{7j+6 \rightarrow 7(j+1)+1}, & i = s + (j+1)_s; \\ -w_{7(j+m+1)+2 \rightarrow 7(j+m+1)+6} \otimes w_{7j+6 \rightarrow 7(j+1)+2}, & i = 2s + (j+1)_s; \\ w_{7(j+m+1)+3 \rightarrow 7(j+m+1)+6} \otimes w_{7j+6 \rightarrow 7(j+1)+3}, & i = 3s + (j+1)_s; \\ -w_{7(j+m+1)+4 \rightarrow 7(j+m+1)+6} \otimes w_{7j+6 \rightarrow 7(j+1)+4}, & i = 4s + (j+1)_s; \\ w_{7(j+m+1)+5 \rightarrow 7(j+m+1)+6} \otimes w_{7j+6 \rightarrow 7(j+1)+5}, & i = 5s + (j+1)_s; \\ w_{7(j+m)+6 \rightarrow 7(j+m+1)+6} \otimes e_{7j+6}, & i = j - 3s; \\ -e_{7(j+m+1)+6} \otimes w_{7j+6 \rightarrow 7(j+1)+6}, & i = 6s + (j+1)_s; \\ 0, & \text{otherwise.} \end{cases}$$

(II) Represent an arbitrary  $t_0 \in \mathbb{N}$  in the form  $t_0 = 17\ell_0 + r_0$ , where  $0 \leq r_0 \leq 16$ . Then  $\Omega^{t_0}(Y_t^{(6)})$  is a  $\Omega^{r_0}(Y_t^{(6)})$ , whose left components twisted by  $\sigma^{\ell_0}$ , and coefficients multiplied by  $(-1)^{\ell_0}$ .

**Proposition 6** (Translates for the case 7). (I) Let  $r_0 \in \mathbb{N}$ ,  $r_0 < 17$ .  $r_0$ -translates of the elements  $Y_t^{(7)}$  are described by the following way.

(1) If  $r_0 = 0$ , then  $\Omega^0(Y_t^{(7)})$  is described with  $(7s \times 12s)$ -matrix with one nonzero element that is of the following form:

$$b_{j-4s, 10s+(3)_s} = w_{7(j+m)+6 \rightarrow 7(j+m+1)+6} \otimes e_{7j+6}.$$

(2) If  $r_0 = 1$ , then  $\Omega^1(Y_t^{(7)})$  is described with  $(8s \times 12s)$ -matrix with the following two nonzero elements:

$$\begin{aligned} b_{j, 4s+(3)_s} &= -w_{7(j+m)+6 \rightarrow 7(j+m+1)+6} \otimes w_{7j+2 \rightarrow 7j+3}; \\ b_{j-s, 7s+(3)_s} &= w_{7(j+m)+6 \rightarrow 7(j+m+1)+6} \otimes e_{7j+5}. \end{aligned}$$

(3) If  $r_0 = 2$ , then  $\Omega^2(Y_t^{(7)})$  is described with  $(7s \times 13s)$ -matrix with one nonzero element that is of the following form:

$$b_{j, (3)_s} = -w_{7(j+m-1)+6 \rightarrow 7(j+m)+6} \otimes e_{7j}.$$

(4) If  $r_0 = 3$ , then  $\Omega^3(Y_t^{(7)})$  is described with  $(9s \times 12s)$ -matrix with the following two nonzero elements:

$$\begin{aligned} b_{s+(j+1)_s, 3s+(2)_s} &= w_{7(j+m+1)+5 \rightarrow 7(j+m+1)+6} \otimes w_{7j+1 \rightarrow 7(j+1)}; \\ b_{(j+1)_s, 6s+(2)_s} &= w_{7(j+m+1)+2 \rightarrow 7(j+m+1)+6} \otimes w_{7j+4 \rightarrow 7(j+1)}. \end{aligned}$$

(5) If  $r_0 = 4$ , then  $\Omega^4(Y_t^{(7)})$  is described with  $(10s \times 12s)$ -matrix with the following nonzero elements:

$$\begin{aligned} b_{(j+1)_s, (2)_s} &= -e_{7(j+m)+6} \otimes w_{7j \rightarrow 7(j+1)}; \\ b_{(j+1)_s, s+(2)_s} &= w_{7(j+m)+6 \rightarrow 7(j+m+1)} \otimes w_{7j \rightarrow 7(j+1)}; \\ b_{s+(j+1)_s, s+(2)_s} &= e_{7(j+m+1)} \otimes w_{7j \rightarrow 7(j+1)}. \end{aligned}$$

(6) If  $r_0 = 5$ , then  $\Omega^5(Y_t^{(7)})$  is described with  $(10s \times 10s)$ -matrix with the following two nonzero elements:

$$\begin{aligned} b_{2s+(j+1)_s, (2)_s} &= w_{7(j+m+1)+1 \rightarrow 7(j+m+1)+2} \otimes w_{7j \rightarrow 7(j+1)}; \\ b_{(j+1)_s, s+(2)_s} &= e_{7(j+m+1)+4} \otimes w_{7j \rightarrow 7(j+1)}. \end{aligned}$$

(7) If  $r_0 = 6$ , then  $\Omega^6(Y_t^{(7)})$  is described with  $(12s \times 10s)$ -matrix with the following two nonzero elements:

$$b_{(j+1)_s, (2)_s} = -w_{7(j+m)+6 \rightarrow 7(j+m+1)} \otimes w_{7j \rightarrow 7(j+1)};$$

$$b_{s+(j+1)s,(2)s} = -e_{7(j+m+1)} \otimes w_{7j \rightarrow 7(j+1)}.$$

(8) If  $r_0 = 7$ , then  $\Omega^7(Y_t^{(7)})$  is described with  $(12s \times 9s)$ -matrix with the following nonzero elements:

$$b_{(j+1)s,(2)s} = -w_{7(j+m+1)+2 \rightarrow 7(j+m+1)+3} \otimes w_{7j \rightarrow 7(j+1)};$$

$$b_{s+(j+1)s,s+(2)s} = -e_{7(j+m+1)+5} \otimes w_{7j \rightarrow 7(j+1)};$$

$$b_{2s+(j+1)s,s+(2)s} = -w_{7(j+m+1)+4 \rightarrow 7(j+m+1)+5} \otimes w_{7j \rightarrow 7(j+1)}.$$

(9) If  $r_0 = 8$ , then  $\Omega^8(Y_t^{(7)})$  is described with  $(13s \times 7s)$ -matrix with one nonzero element that is of the following form:

$$b_{(j+1)s,(2)s} = -e_{7(j+m)+6} \otimes w_{7j \rightarrow 7(j+1)}.$$

(10) If  $r_0 = 9$ , then  $\Omega^9(Y_t^{(7)})$  is described with  $(12s \times 8s)$ -matrix with one nonzero element that is of the following form:

$$b_{s+(j+1)s,(2)s} = -w_{7(j+m+1)+3 \rightarrow 7(j+m+1)+6} \otimes w_{7j \rightarrow 7(j+1)}.$$

(11) If  $r_0 = 10$ , then  $\Omega^{10}(Y_t^{(7)})$  is described with  $(12s \times 7s)$ -matrix with one nonzero element that is of the following form:

$$b_{s+(j+1)s,(2)s} = -e_{7(j+m+1)} \otimes w_{7j \rightarrow 7(j+1)}.$$

(12) If  $r_0 = 11$ , then  $\Omega^{11}(Y_t^{(7)})$  is described with  $(10s \times 7s)$ -matrix with one nonzero element that is of the following form:

$$b_{(j+1)s,(2)s} = -w_{7(j+m+1)+2 \rightarrow 7(j+m+2)} \otimes w_{7j \rightarrow 7(j+1)}.$$

(13) If  $r_0 = 12$ , then  $\Omega^{12}(Y_t^{(7)})$  is described with  $(10s \times 8s)$ -matrix with one nonzero element that is of the following form:

$$b_{(j+1)s,(2)s} = w_{7(j+m+1) \rightarrow 7(j+m+1)+1} \otimes w_{7j \rightarrow 7(j+1)}.$$

(14) If  $r_0 = 13$ , then  $\Omega^{13}(Y_t^{(7)})$  is described with  $(9s \times 7s)$ -matrix with one nonzero element that is of the following form:

$$b_{(j+1)s,(2)s} = -w_{7(j+m+1)+3 \rightarrow 7(j+m+1)+6} \otimes w_{7j \rightarrow 7(j+1)}.$$

(15) If  $r_0 = 14$ , then  $\Omega^{14}(Y_t^{(7)})$  is described with  $(7s \times 9s)$ -matrix with one nonzero element that is of the following form:

$$b_{(j+1)s,(2)s} = w_{7(j+m)+6 \rightarrow 7(j+m+1)+2} \otimes w_{7j \rightarrow 7(j+1)}.$$

(16) If  $r_0 = 15$ , then  $\Omega^{15}(Y_t^{(7)})$  is described with  $(8s \times 10s)$ -matrix with one nonzero element that is of the following form:

$$b_{j,(2)s} = -w_{7(j+m)+6 \rightarrow 7(j+m+1)+6} \otimes e_{7j}.$$

(17) If  $r_0 = 16$ , then  $\Omega^{16}(Y_t^{(7)})$  is described with  $(7s \times 10s)$ -matrix with the following two nonzero elements:

$$b_{j+3s,3s+(1)s} = w_{7(j+m)+6 \rightarrow 7(j+m+1)+6} \otimes w_{7j+1 \rightarrow 7j+6};$$

$$b_{j+s,5s+(1)s} = -w_{7(j+m)+6 \rightarrow 7(j+m+1)+6} \otimes w_{7j+3 \rightarrow 7j+6}.$$

(II) Represent an arbitrary  $t_0 \in \mathbb{N}$  in the form  $t_0 = 17\ell_0 + r_0$ , where  $0 \leq r_0 \leq 16$ . Then  $\Omega^{t_0}(Y_t^{(7)})$  is a  $\Omega^{r_0}(Y_t^{(7)})$ , whose left components twisted by  $\sigma^{\ell_0}$ .

**Proposition 7** (Translates for the case 8). (I) Let  $r_0 \in \mathbb{N}$ ,  $r_0 < 17$ .  $r_0$ -translates of the elements  $Y_t^{(8)}$  are described by the following way.

(1) If  $r_0 = 0$ , then  $\Omega^0(Y_t^{(8)})$  is described with  $(7s \times 12s)$ -matrix with the following elements  $b_{ij}$ :  
If  $2s \leq j < 3s$ , then

$$b_{ij} = \begin{cases} w_{7(j+m) \rightarrow 7(j+m)+4} \otimes e_{7j}, & i = j - 2s; \\ 0, & \text{otherwise.} \end{cases}$$

If  $3s \leq j < 7s$ , then  $b_{ij} = 0$ .

If  $7s \leq j < 8s$ , then

$$b_{ij} = \begin{cases} w_{7(j+m)+5 \rightarrow 7(j+m)+6} \otimes e_{7j+5}, & i = j - 2s; \\ 0, & \text{otherwise.} \end{cases}$$

If  $8s \leq j < 9s$ , then  $b_{ij} = 0$ .

If  $9s \leq j < 10s$ , then

$$b_{ij} = \begin{cases} w_{7(j+m)+6 \rightarrow 7(j+m+1)+4} \otimes e_{7j+6}, & i = j - 3s; \\ 0, & \text{otherwise.} \end{cases}$$

If  $10s \leq j < 12s$ , then  $b_{ij} = 0$ .

(2) If  $r_0 = 1$ , then  $\Omega^1(Y_t^{(8)})$  is described with  $(8s \times 13s)$ -matrix with the following elements  $b_{ij}$ :  
If  $0 \leq j < s$ , then

$$b_{ij} = \begin{cases} -w_{7(j+m)+4 \rightarrow 7(j+m)+6} \otimes e_{7j}, & i = j + s; \\ -w_{7(j+m)+5 \rightarrow 7(j+m)+6} \otimes w_{7j \rightarrow 7j+4}, & i = j + 5s; \\ 0, & \text{otherwise.} \end{cases}$$

If  $s \leq j < 3s$ , then  $b_{ij} = 0$ .

If  $3s \leq j < 4s$ , then

$$b_{ij} = \begin{cases} -w_{7(j+m+1)+4 \rightarrow 7(j+m+1)+5} \otimes w_{7j+1 \rightarrow 7(j+1)}, & i = s + (j + 1)s; \\ 0, & \text{otherwise.} \end{cases}$$

If  $4s \leq j < 6s$ , then  $b_{ij} = 0$ .

If  $6s \leq j < 7s$ , then

$$b_{ij} = \begin{cases} -e_{7(j+m+1)+4} \otimes w_{7j+3 \rightarrow 7(j+1)}, & i = s + (j + 1)s; \\ -w_{7(j+m)+6 \rightarrow 7(j+m+1)+4} \otimes e_{7j+3}, & i = j - 2s; \\ 0, & \text{otherwise.} \end{cases}$$

If  $7s \leq j < 9s$ , then  $b_{ij} = 0$ .

If  $9s \leq j < 10s$ , then

$$b_{ij} = \begin{cases} -w_{7(j+m)+6 \rightarrow 7(j+m+1)+4} \otimes e_{7j+5}, & i = j - 3s; \\ 0, & \text{otherwise.} \end{cases}$$

If  $10s \leq j < 11s$ , then  $b_{ij} = 0$ .

If  $11s \leq j < 12s$ , then

$$b_{ij} = \begin{cases} w_{7(j+m+1) \rightarrow 7(j+m+1)+6} \otimes e_{7j+6}, & i = j - 4s; \\ 0, & \text{otherwise.} \end{cases}$$

If  $12s \leq j < 13s$ , then

$$b_{ij} = \begin{cases} w_{7(j+m+1) \rightarrow 7(j+m+2)} \otimes e_{7j+6}, & i = j - 5s; \\ 0, & \text{otherwise.} \end{cases}$$

(3) If  $r_0 = 2$ , then  $\Omega^2(Y_t^{(8)})$  is described with  $(7s \times 12s)$ -matrix with the following elements  $b_{ij}$ :  
If  $0 \leq j < s$ , then

$$b_{ij} = \begin{cases} w_{7(j+m-1)+6 \rightarrow 7(j+m)+5} \otimes e_{7j}, & i = j; \\ 0, & \text{otherwise.} \end{cases}$$

If  $s \leq j < 4s$ , then  $b_{ij} = 0$ .

If  $4s \leq j < 5s$ , then

$$b_{ij} = \begin{cases} -w_{7(j+m)+6 \rightarrow 7(j+m+1)} \otimes w_{7j+2 \rightarrow 7(j+1)}, & i = (j+1)_s; \\ w_{7(j+m)+3 \rightarrow 7(j+m+1)} \otimes e_{7j+2}, & i = j - 2s; \\ 0, & \text{otherwise.} \end{cases}$$

If  $5s \leq j < 6s$ , then

$$b_{ij} = \begin{cases} w_{7(j+m)+4 \rightarrow 7(j+m)+6} \otimes e_{7j+3}, & i = j - 2s; \\ 0, & \text{otherwise.} \end{cases}$$

If  $6s \leq j < 7s$ , then

$$b_{ij} = \begin{cases} w_{7(j+m)+5 \rightarrow 7(j+m)+6} \otimes e_{7j+4}, & i = j - 2s; \\ 0, & \text{otherwise.} \end{cases}$$

If  $7s \leq j < 11s$ , then  $b_{ij} = 0$ .

If  $11s \leq j < 12s$ , then

$$b_{ij} = \begin{cases} -w_{7(j+m)+6 \rightarrow 7(j+m+1)+4} \otimes w_{7j+6 \rightarrow 7(j+1)}, & i = (j+1)_s; \\ 0, & \text{otherwise.} \end{cases}$$

(4) If  $r_0 = 3$ , then  $\Omega^3(Y_t^{(8)})$  is described with  $(9s \times 12s)$ -matrix with the following elements  $b_{ij}$ :  
If  $0 \leq j < s$ , then

$$b_{ij} = \begin{cases} -w_{7(j+m)+5 \rightarrow 7(j+m)+6} \otimes e_{7j}, & i = j + s; \\ 0, & \text{otherwise.} \end{cases}$$

If  $s \leq j < 2s$ , then

$$b_{ij} = \begin{cases} -w_{7(j+m)+5 \rightarrow 7(j+m+1)} \otimes e_{7j}, & i = j; \\ w_{7(j+m)+6 \rightarrow 7(j+m+1)} \otimes w_{7j \rightarrow 7j+2}, & i = j + 2s; \\ 0, & \text{otherwise.} \end{cases}$$

If  $2s \leq j < 3s$ , then

$$b_{ij} = \begin{cases} w_{7(j+m)+6 \rightarrow 7(j+m+1)+2} \otimes w_{7j+1 \rightarrow 7j+2}, & i = j + s; \\ 0, & \text{otherwise.} \end{cases}$$



If  $3s \leq j < 4s$ , then

$$b_{ij} = \begin{cases} -w_{7(j+m)+6 \rightarrow 7(j+m+1)+3} \otimes e_{7j+2}, & i = j; \\ 0, & \text{otherwise.} \end{cases}$$

If  $4s \leq j < 6s$ , then  $b_{ij} = 0$ .

If  $6s \leq j < 7s$ , then

$$b_{ij} = \begin{cases} -w_{7(j+m)+6 \rightarrow 7(j+m+1)+4} \otimes e_{7j+4}, & i = j - s; \\ 0, & \text{otherwise.} \end{cases}$$

If  $7s \leq j < 12s$ , then  $b_{ij} = 0$ .

(5) If  $r_0 = 4$ , then  $\Omega^4(Y_t^{(8)})$  is described with  $(10s \times 10s)$ -matrix with the following elements  $b_{ij}$ :

If  $s \leq j < 2s$ , then

$$b_{ij} = \begin{cases} w_{7(j+m-1)+6 \rightarrow 7(j+m)+4} \otimes e_{7j}, & i = j - s; \\ 0, & \text{otherwise.} \end{cases}$$

If  $2s \leq j < 3s$ , then

$$b_{ij} = \begin{cases} e_{7(j+m+1)} \otimes w_{7j+1 \rightarrow 7(j+1)}, & i = s + (j + 1)_s; \\ 0, & \text{otherwise.} \end{cases}$$

If  $3s \leq j < 4s$ , then

$$b_{ij} = \begin{cases} w_{7(j+m)+4 \rightarrow 7(j+m)+6} \otimes e_{7j+2}, & i = j; \\ -w_{7(j+m)+5 \rightarrow 7(j+m)+6} \otimes w_{7j+2 \rightarrow 7j+3}, & i = j + 2s; \\ 0, & \text{otherwise.} \end{cases}$$

If  $4s \leq j < 7s$ , then  $b_{ij} = 0$ .

If  $7s \leq j < 8s$ , then

$$b_{ij} = \begin{cases} w_{7(j+m+1)+4 \rightarrow 7(j+m+1)+5} \otimes w_{7j+6 \rightarrow 7(j+1)+2}, & i = 3s + (j + 1)_s; \\ -e_{7(j+m+1)+5} \otimes w_{7j+6 \rightarrow 7(j+1)+3}, & i = 5s + (j + 1)_s; \\ 0, & \text{otherwise.} \end{cases}$$

If  $8s \leq j < 10s$ , then  $b_{ij} = 0$ .

(6) If  $r_0 = 5$ , then  $\Omega^5(Y_t^{(8)})$  is described with  $(10s \times 10s)$ -matrix with the following elements  $b_{ij}$ :

If  $0 \leq j < s$ , then

$$b_{ij} = \begin{cases} -e_{7(j+m+1)} \otimes w_{7j \rightarrow 7j+2}, & i = j + 4s; \\ 0, & \text{otherwise.} \end{cases}$$

If  $s \leq j < 2s$ , then

$$b_{ij} = \begin{cases} -w_{7(j+m+1)+1 \rightarrow 7(j+m+1)+3} \otimes w_{7j+1 \rightarrow 7(j+1)}, & i = 2s + (j + 1)_s; \\ 0, & \text{otherwise.} \end{cases}$$

If  $2s \leq j < 3s$ , then

$$b_{ij} = \begin{cases} e_{7(j+m+1)+4} \otimes w_{7j+1 \rightarrow 7(j+1)}, & i = (j+1)_s; \\ 0, & \text{otherwise.} \end{cases}$$

If  $3s \leq j < 4s$ , then

$$b_{ij} = \begin{cases} w_{7(j+m+1)+4 \rightarrow 7(j+m+1)+5} \otimes w_{7j+2 \rightarrow 7(j+1)}, & i = (j+1)_s; \\ w_{7(j+m+1) \rightarrow 7(j+m+1)+5} \otimes e_{7j+2}, & i = j+s; \\ 0, & \text{otherwise.} \end{cases}$$

If  $4s \leq j < 10s$ , then  $b_{ij} = 0$ .

(7) If  $r_0 = 6$ , then  $\Omega^6(Y_t^{(8)})$  is described with  $(12s \times 9s)$ -matrix with the following elements  $b_{ij}$ :  
If  $0 \leq j < s$ , then

$$b_{ij} = \begin{cases} w_{7(j+m)+1 \rightarrow 7(j+m)+3} \otimes w_{7j \rightarrow 7j+2}, & i = j+3s; \\ 0, & \text{otherwise.} \end{cases}$$

If  $s \leq j < 2s$ , then  $b_{ij} = 0$ .

If  $2s \leq j < 3s$ , then

$$b_{ij} = \begin{cases} w_{7(j+m)+1 \rightarrow 7(j+m)+6} \otimes w_{7j+1 \rightarrow 7j+2}, & i = j+s; \\ 0, & \text{otherwise.} \end{cases}$$

If  $3s \leq j < 4s$ , then

$$b_{ij} = \begin{cases} w_{7(j+m)+6 \rightarrow 7(j+m+1)} \otimes w_{7j+2 \rightarrow 7(j+1)}, & i = (j+1)_s; \\ e_{7(j+m+1)} \otimes w_{7j+2 \rightarrow 7(j+1)}, & i = s + (j+1)_s; \\ w_{7(j+m)+1 \rightarrow 7(j+m+1)} \otimes e_{7j+2}, & i = j; \\ 0, & \text{otherwise.} \end{cases}$$

If  $4s \leq j < 5s$ , then

$$b_{ij} = \begin{cases} e_{7(j+m+1)+1} \otimes w_{7j+3 \rightarrow 7(j+1)+2}, & i = 3s + (j+1)_s; \\ 0, & \text{otherwise.} \end{cases}$$

If  $5s \leq j < 7s$ , then  $b_{ij} = 0$ .

If  $7s \leq j < 8s$ , then

$$b_{ij} = \begin{cases} w_{7(j+m+1)+1 \rightarrow 7(j+m+1)+2} \otimes w_{7j+6 \rightarrow 7(j+1)+2}, & i = 3s + (j+1)_s; \\ 0, & \text{otherwise.} \end{cases}$$

If  $8s \leq j < 9s$ , then  $b_{ij} = 0$ .

(8) If  $r_0 = 7$ , then  $\Omega^7(Y_t^{(8)})$  is described with  $(12s \times 7s)$ -matrix with the following elements  $b_{ij}$ :  
If  $s \leq j < 2s$ , then

$$b_{ij} = \begin{cases} -e_{7(j+m+1)+5} \otimes w_{7j+1 \rightarrow 7(j+1)}, & i = s + (j+1)_s; \\ -w_{7(j+m+1)+4 \rightarrow 7(j+m+1)+5} \otimes w_{7j+1 \rightarrow 7(j+1)}, & i = 2s + (j+1)_s; \\ 0, & \text{otherwise.} \end{cases}$$

If  $2s \leq j < 3s$ , then

$$b_{ij} = \begin{cases} -w_{7(j+m)+6 \rightarrow 7(j+m+1)+1} \otimes e_{7j+2}, & i = j + 2s; \\ -w_{7(j+m+1) \rightarrow 7(j+m+1)+1} \otimes w_{7j+2 \rightarrow 7j+3}, & i = j + 3s; \\ -e_{7(j+m+1)+1} \otimes w_{7j+2 \rightarrow 7j+6}, & i = j + 9s; \\ 0, & \text{otherwise.} \end{cases}$$

If  $3s \leq j < 7s$ , then  $b_{ij} = 0$ .

(9) If  $r_0 = 8$ , then  $\Omega^8(Y_t^{(8)})$  is described with  $(13s \times 8s)$ -matrix with the following elements  $b_{ij}$ :

If  $0 \leq j < s$ , then

$$b_{ij} = \begin{cases} w_{7(j+m)+1 \rightarrow 7(j+m)+6} \otimes w_{7j \rightarrow 7j+1}, & i = j + 2s; \\ -w_{7(j+m)+5 \rightarrow 7(j+m)+6} \otimes w_{7j \rightarrow 7j+1}, & i = j + 3s; \\ 0, & \text{otherwise.} \end{cases}$$

If  $s \leq j < 2s$ , then

$$b_{ij} = \begin{cases} w_{7(j+m)+1 \rightarrow 7(j+m+1)} \otimes e_{7j+1}, & i = j + s; \\ -w_{7(j+m)+5 \rightarrow 7(j+m+1)} \otimes e_{7j+1}, & i = j + 2s; \\ 0, & \text{otherwise.} \end{cases}$$

If  $2s \leq j < 3s$ , then

$$b_{ij} = \begin{cases} w_{7(j+m)+6 \rightarrow 7(j+m+1)+1} \otimes w_{7j+2 \rightarrow 7(j+1)}, & i = (j+1)s; \\ w_{7(j+m)+2 \rightarrow 7(j+m+1)+1} \otimes e_{7j+2}, & i = j + 2s; \\ 0, & \text{otherwise.} \end{cases}$$

If  $3s \leq j < 4s$ , then

$$b_{ij} = \begin{cases} e_{7(j+m+1)+2} \otimes w_{7j+3 \rightarrow 7(j+1)+2}, & i = 4s + (j+1)s; \\ 0, & \text{otherwise.} \end{cases}$$

If  $4s \leq j < 6s$ , then  $b_{ij} = 0$ .

If  $6s \leq j < 7s$ , then

$$b_{ij} = \begin{cases} w_{7(j+m+1)+2 \rightarrow 7(j+m+1)+3} \otimes w_{7j+6 \rightarrow 7(j+1)+2}, & i = 4s + (j+1)s; \\ 0, & \text{otherwise.} \end{cases}$$

If  $7s \leq j < 8s$ , then  $b_{ij} = 0$ .

(10) If  $r_0 = 9$ , then  $\Omega^9(Y_t^{(8)})$  is described with  $(12s \times 7s)$ -matrix with the following elements  $b_{ij}$ :

If  $s \leq j < 2s$ , then

$$b_{ij} = \begin{cases} -w_{7(j+m)+6 \rightarrow 7(j+m+1)+1} \otimes e_{7j+1}, & i = j + 2s; \\ 0, & \text{otherwise.} \end{cases}$$

If  $2s \leq j < 3s$ , then

$$b_{ij} = \begin{cases} w_{7(j+m+1)+1 \rightarrow 7(j+m+1)+2} \otimes w_{7j+2 \rightarrow 7(j+1)}, & i = 2s + (j+1)_s; \\ -w_{7(j+m+1) \rightarrow 7(j+m+1)+2} \otimes e_{7j+2}, & i = j + 2s; \\ -w_{7(j+m)+6 \rightarrow 7(j+m+1)+2} \otimes w_{7j+2 \rightarrow 7j+3}, & i = j + 3s; \\ e_{7(j+m+1)+2} \otimes w_{7j+2 \rightarrow 7j+6}, & i = j + 7s; \\ 0, & \text{otherwise.} \end{cases}$$

If  $3s \leq j < 6s$ , then  $b_{ij} = 0$ .

If  $6s \leq j < 7s$ , then

$$b_{ij} = \begin{cases} e_{7(j+m+1)+6} \otimes w_{7j+6 \rightarrow 7(j+1)+1}, & i = 3s + (j+1)_s; \\ 0, & \text{otherwise.} \end{cases}$$

(11) If  $r_0 = 10$ , then  $\Omega^{10}(Y_t^{(8)})$  is described with  $(12s \times 7s)$ -matrix with the following elements  $b_{ij}$ :

If  $0 \leq j < s$ , then

$$b_{ij} = \begin{cases} w_{7(j+m)+2 \rightarrow 7(j+m+1)} \otimes w_{7j \rightarrow 7j+1}, & i = j + 2s; \\ 0, & \text{otherwise.} \end{cases}$$

If  $s \leq j < 2s$ , then

$$b_{ij} = \begin{cases} w_{7(j+m)+2 \rightarrow 7(j+m+1)+1} \otimes e_{7j+1}, & i = j + s; \\ 0, & \text{otherwise.} \end{cases}$$

If  $2s \leq j < 3s$ , then

$$b_{ij} = \begin{cases} w_{7(j+m+1) \rightarrow 7(j+m+1)+2} \otimes w_{7j+2 \rightarrow 7(j+1)}, & i = s + (j+1)_s; \\ w_{7(j+m)+3 \rightarrow 7(j+m+1)+2} \otimes e_{7j+2}, & i = j + s; \\ 0, & \text{otherwise.} \end{cases}$$

If  $3s \leq j < 4s$ , then

$$b_{ij} = \begin{cases} e_{7(j+m+1)+3} \otimes w_{7j+3 \rightarrow 7(j+1)+2}, & i = 3s + (j+1)_s; \\ 0, & \text{otherwise.} \end{cases}$$

If  $4s \leq j < 6s$ , then  $b_{ij} = 0$ .

If  $6s \leq j < 7s$ , then

$$b_{ij} = \begin{cases} w_{7(j+m+1)+3 \rightarrow 7(j+m+1)+6} \otimes w_{7j+6 \rightarrow 7(j+1)+2}, & i = 3s + (j+1)_s; \\ 0, & \text{otherwise.} \end{cases}$$

(12) If  $r_0 = 11$ , then  $\Omega^{11}(Y_t^{(8)})$  is described with  $(10s \times 8s)$ -matrix with the following elements  $b_{ij}$ :

If  $2s \leq j < 3s$ , then

$$b_{ij} = \begin{cases} w_{7(j+m+1) \rightarrow 7(j+m+1)+2} \otimes e_{7j+1}, & i = j; \\ 0, & \text{otherwise.} \end{cases}$$

If  $3s \leq j < 4s$ , then

$$b_{ij} = \begin{cases} w_{7(j+m+1)+2 \rightarrow 7(j+m+1)+3} \otimes w_{7j+2 \rightarrow 7(j+1)}, & i = (j+1)_s; \\ w_{7(j+m)+6 \rightarrow 7(j+m+1)+3} \otimes e_{7j+2}, & i = j; \\ -e_{7(j+m+1)+3} \otimes w_{7j+2 \rightarrow 7j+6}, & i = j+5s; \\ 0, & \text{otherwise.} \end{cases}$$

If  $4s \leq j < 7s$ , then  $b_{ij} = 0$ .

If  $7s \leq j < 8s$ , then

$$b_{ij} = \begin{cases} -e_{7(j+m+2)} \otimes w_{7j+6 \rightarrow 7(j+1)+1}, & i = 2s + (j+1)_s; \\ 0, & \text{otherwise.} \end{cases}$$

(13) If  $r_0 = 12$ , then  $\Omega^{12}(Y_t^{(8)})$  is described with  $(10s \times 7s)$ -matrix with the following elements  $b_{ij}$ :

If  $0 \leq j < s$ , then

$$b_{ij} = \begin{cases} w_{7(j+m)+3 \rightarrow 7(j+m)+6} \otimes w_{7j \rightarrow 7j+1}, & i = j+s; \\ 0, & \text{otherwise.} \end{cases}$$

If  $s \leq j < 2s$ , then

$$b_{ij} = \begin{cases} w_{7(j+m)+3 \rightarrow 7(j+m+1)+2} \otimes e_{7j+1}, & i = j; \\ 0, & \text{otherwise.} \end{cases}$$

If  $2s \leq j < 3s$ , then

$$b_{ij} = \begin{cases} w_{7(j+m)+6 \rightarrow 7(j+m+1)+3} \otimes w_{7j+2 \rightarrow 7j+6}, & i = j+6s; \\ 0, & \text{otherwise.} \end{cases}$$

If  $3s \leq j < 4s$ , then

$$b_{ij} = \begin{cases} -e_{7(j+m+1)+4} \otimes w_{7j+3 \rightarrow 7(j+1)+1}, & i = 2s + (j+1)_s; \\ 0, & \text{otherwise.} \end{cases}$$

If  $4s \leq j < 6s$ , then  $b_{ij} = 0$ .

If  $6s \leq j < 7s$ , then

$$b_{ij} = \begin{cases} w_{7(j+m+1)+3 \rightarrow 7(j+m+2)} \otimes w_{7j+6 \rightarrow 7(j+1)+1}, & i = s + (j+1)_s; \\ -w_{7(j+m+1)+4 \rightarrow 7(j+m+2)} \otimes w_{7j+6 \rightarrow 7(j+1)+1}, & i = 2s + (j+1)_s; \\ 0, & \text{otherwise.} \end{cases}$$

(14) If  $r_0 = 13$ , then  $\Omega^{13}(Y_t^{(8)})$  is described with  $(9s \times 9s)$ -matrix with the following elements  $b_{ij}$ :

If  $2s \leq j < 3s$ , then

$$b_{ij} = \begin{cases} w_{7(j+m)+6 \rightarrow 7(j+m+1)+3} \otimes e_{7j+1}, & i = j; \\ 0, & \text{otherwise.} \end{cases}$$

If  $3s \leq j < 4s$ , then

$$b_{ij} = \begin{cases} w_{7(j+m+1)+3 \rightarrow 7(j+m+1)+6} \otimes w_{7j+2 \rightarrow 7(j+1)}, & i = (j+1)_s; \\ w_{7(j+m+1) \rightarrow 7(j+m+1)+6} \otimes e_{7j+2}, & i = j; \\ -w_{7(j+m+1)+4 \rightarrow 7(j+m+1)+6} \otimes w_{7j+2 \rightarrow 7j+6}, & i = j+5s; \\ 0, & \text{otherwise.} \end{cases}$$

If  $4s \leq j < 8s$ , then  $b_{ij} = 0$ .

If  $8s \leq j < 9s$ , then

$$b_{ij} = \begin{cases} w_{7(j+m+1)+6 \rightarrow 7(j+m+2)+4} \otimes w_{7j+6 \rightarrow 7(j+1)+1}, & i = 2s + (j+1)_s; \\ w_{7(j+m+2) \rightarrow 7(j+m+2)+4} \otimes w_{7j+6 \rightarrow 7(j+1)+2}, & i = 3s + (j+1)_s; \\ w_{7(j+m+2) \rightarrow 7(j+m+2)+4} \otimes w_{7j+6 \rightarrow 7(j+1)+5}, & i = 6s + (j+1)_s; \\ 0, & \text{otherwise.} \end{cases}$$

(15) If  $r_0 = 14$ , then  $\Omega^{14}(Y_t^{(8)})$  is described with  $(7s \times 10s)$ -matrix with the following elements  $b_{ij}$ :

If  $0 \leq j < s$ , then

$$b_{ij} = \begin{cases} e_{7(j+m)+6} \otimes w_{7j \rightarrow 7(j+1)}, & i = (j+1)_s; \\ w_{7(j+m)+5 \rightarrow 7(j+m)+6} \otimes w_{7j \rightarrow 7j+1}, & i = j+s; \\ 0, & \text{otherwise.} \end{cases}$$

If  $s \leq j < 2s$ , then  $b_{ij} = 0$ .

If  $2s \leq j < 3s$ , then

$$b_{ij} = \begin{cases} w_{7(j+m)+6 \rightarrow 7(j+m+1)+3} \otimes w_{7j+1 \rightarrow 7(j+1)}, & i = (j+1)_s; \\ 0, & \text{otherwise.} \end{cases}$$

If  $3s \leq j < 4s$ , then

$$b_{ij} = \begin{cases} w_{7(j+m+1) \rightarrow 7(j+m+1)+4} \otimes w_{7j+2 \rightarrow 7j+6}, & i = j+3s; \\ 0, & \text{otherwise.} \end{cases}$$

If  $4s \leq j < 5s$ , then  $b_{ij} = 0$ .

If  $5s \leq j < 6s$ , then

$$b_{ij} = \begin{cases} e_{7(j+m+1)+5} \otimes w_{7j+3 \rightarrow 7(j+1)+1}, & i = s + (j+1)_s; \\ 0, & \text{otherwise.} \end{cases}$$

If  $6s \leq j < 8s$ , then  $b_{ij} = 0$ .

If  $8s \leq j < 9s$ , then

$$b_{ij} = \begin{cases} e_{7(j+m+1)+4} \otimes w_{7j+5 \rightarrow 7(j+1)+5}, & i = 5s + (j+1)_s; \\ 0, & \text{otherwise.} \end{cases}$$

If  $9s \leq j < 10s$ , then

$$b_{ij} = \begin{cases} -w_{7(j+m)+6 \rightarrow 7(j+m+1)+6} \otimes w_{7j+6 \rightarrow 7(j+1)}, & i = (j+1)_s; \\ w_{7(j+m+1)+5 \rightarrow 7(j+m+1)+6} \otimes w_{7j+6 \rightarrow 7(j+1)+1}, & i = s + (j+1)_s; \\ -w_{7(j+m+1)+1 \rightarrow 7(j+m+1)+6} \otimes w_{7j+6 \rightarrow 7(j+1)+2}, & i = 2s + (j+1)_s; \\ w_{7(j+m+1)+2 \rightarrow 7(j+m+1)+6} \otimes w_{7j+6 \rightarrow 7(j+1)+3}, & i = 3s + (j+1)_s; \\ -w_{7(j+m+1)+3 \rightarrow 7(j+m+1)+6} \otimes w_{7j+6 \rightarrow 7(j+1)+4}, & i = 4s + (j+1)_s; \\ 0, & \text{otherwise.} \end{cases}$$

(16) If  $r_0 = 15$ , then  $\Omega^{15}(Y_t^{(8)})$  is described with  $(8s \times 10s)$ -matrix with the following elements  $b_{ij}$ :

If  $0 \leq j < s$ , then

$$b_{ij} = \begin{cases} w_{7(j+m+1) \rightarrow 7(j+m+1)+4} \otimes w_{7j \rightarrow 7j+1}, & i = j + s; \\ 0, & \text{otherwise.} \end{cases}$$

If  $s \leq j < 3s$ , then  $b_{ij} = 0$ .

If  $3s \leq j < 4s$ , then

$$b_{ij} = \begin{cases} w_{7(j+m+1) \rightarrow 7(j+m+1)+6} \otimes e_{7j+1}, & i = j - 2s; \\ 0, & \text{otherwise.} \end{cases}$$

If  $4s \leq j < 5s$ , then

$$b_{ij} = \begin{cases} w_{7(j+m+1)+6 \rightarrow 7(j+m+2)} \otimes w_{7j+2 \rightarrow 7(j+1)}, & i = (j+1)_s; \\ w_{7(j+m+1)+1 \rightarrow 7(j+m+2)} \otimes e_{7j+2}, & i = j - 2s; \\ 0, & \text{otherwise.} \end{cases}$$

If  $5s \leq j < 6s$ , then

$$b_{ij} = \begin{cases} e_{7(j+m+1)+6} \otimes w_{7j+3 \rightarrow 7(j+1)}, & i = (j+1)_s; \\ 0, & \text{otherwise.} \end{cases}$$

If  $6s \leq j < 7s$ , then  $b_{ij} = 0$ .

If  $7s \leq j < 8s$ , then

$$b_{ij} = \begin{cases} e_{7(j+m+1)+6} \otimes w_{7j+5 \rightarrow 7(j+1)}, & i = (j+1)_s; \\ 0, & \text{otherwise.} \end{cases}$$

If  $8s \leq j < 9s$ , then

$$b_{ij} = \begin{cases} -w_{7(j+m+1)+6 \rightarrow 7(j+m+2)+2} \otimes w_{7j+6 \rightarrow 7(j+1)}, & i = (j+1)_s; \\ 0, & \text{otherwise.} \end{cases}$$

If  $9s \leq j < 10s$ , then

$$b_{ij} = \begin{cases} w_{7(j+m+2) \rightarrow 7(j+m+2)+5} \otimes w_{7j+6 \rightarrow 7(j+1)+1}, & i = s + (j+1)_s; \\ 0, & \text{otherwise.} \end{cases}$$

(17) If  $r_0 = 16$ , then  $\Omega^{16}(Y_t^{(8)})$  is described with  $(7s \times 12s)$ -matrix with the following elements  $b_{ij}$ :

If  $s \leq j < 2s$ , then

$$b_{ij} = \begin{cases} w_{7(j+m) \rightarrow 7(j+m+1)} \otimes e_{7j}, & i = j - s; \\ w_{7(j+m)+2 \rightarrow 7(j+m+1)} \otimes w_{7j \rightarrow 7j+2}, & i = j + s; \\ -w_{7(j+m)+3 \rightarrow 7(j+m+1)} \otimes w_{7j \rightarrow 7j+3}, & i = j + 2s; \\ w_{7(j+m)+4 \rightarrow 7(j+m+1)} \otimes w_{7j \rightarrow 7j+4}, & i = j + 3s; \\ -w_{7(j+m)+5 \rightarrow 7(j+m+1)} \otimes w_{7j \rightarrow 7j+5}, & i = j + 4s; \\ w_{7(j+m)+6 \rightarrow 7(j+m+1)} \otimes w_{7j \rightarrow 7j+6}, & i = j + 5s; \\ 0, & \text{otherwise.} \end{cases}$$

If  $2s \leq j < 3s$ , then

$$b_{ij} = \begin{cases} w_{7(j+m+1) \rightarrow 7(j+m+1)+4} \otimes w_{7j+1 \rightarrow 7(j+1)}, & i = (j+1)_s; \\ 0, & \text{otherwise.} \end{cases}$$

If  $3s \leq j < 4s$ , then

$$b_{ij} = \begin{cases} w_{7(j+m)+2 \rightarrow 7(j+m+1)+1} \otimes e_{7j+2}, & i = j - s; \\ -w_{7(j+m)+3 \rightarrow 7(j+m+1)+1} \otimes w_{7j+2 \rightarrow 7j+3}, & i = j; \\ w_{7(j+m)+6 \rightarrow 7(j+m+1)+1} \otimes w_{7j+2 \rightarrow 7j+6}, & i = j + 3s; \\ 0, & \text{otherwise.} \end{cases}$$

If  $4s \leq j < 9s$ , then  $b_{ij} = 0$ .

If  $9s \leq j < 10s$ , then

$$b_{ij} = \begin{cases} w_{7(j+m+1) \rightarrow 7(j+m+1)+5} \otimes w_{7j+5 \rightarrow 7(j+1)}, & i = (j+1)_s; \\ w_{7(j+m+1)+4 \rightarrow 7(j+m+1)+5} \otimes w_{7j+5 \rightarrow 7(j+1)+4}, & i = 4s + (j+1)_s; \\ -e_{7(j+m+1)+5} \otimes w_{7j+5 \rightarrow 7(j+1)+5}, & i = 5s + (j+1)_s; \\ 0, & \text{otherwise.} \end{cases}$$

If  $10s \leq j < 11s$ , then

$$b_{ij} = \begin{cases} -w_{7(j+m)+6 \rightarrow 7(j+m+1)+6} \otimes e_{7j+6}, & i = j - 4s; \\ 0, & \text{otherwise.} \end{cases}$$

If  $11s \leq j < 12s$ , then

$$b_{ij} = \begin{cases} w_{7(j+m+1) \rightarrow 7(j+m+2)} \otimes w_{7j+6 \rightarrow 7(j+1)}, & i = (j+1)_s; \\ w_{7(j+m+1)+2 \rightarrow 7(j+m+2)} \otimes w_{7j+6 \rightarrow 7(j+1)+2}, & i = 2s + (j+1)_s; \\ -w_{7(j+m+1)+3 \rightarrow 7(j+m+2)} \otimes w_{7j+6 \rightarrow 7(j+1)+3}, & i = 3s + (j+1)_s; \\ w_{7(j+m+1)+4 \rightarrow 7(j+m+2)} \otimes w_{7j+6 \rightarrow 7(j+1)+4}, & i = 4s + (j+1)_s; \\ -w_{7(j+m+1)+5 \rightarrow 7(j+m+2)} \otimes w_{7j+6 \rightarrow 7(j+1)+5}, & i = 5s + (j+1)_s; \\ w_{7(j+m+1)+6 \rightarrow 7(j+m+2)} \otimes w_{7j+6 \rightarrow 7(j+1)+6}, & i = 6s + (j+1)_s; \\ 0, & \text{otherwise.} \end{cases}$$

(II) Represent an arbitrary  $t_0 \in \mathbb{N}$  in the form  $t_0 = 17\ell_0 + r_0$ , where  $0 \leq r_0 \leq 16$ . Then  $\Omega^{t_0}(Y_t^{(8)})$  is a  $\Omega^{r_0}(Y_t^{(8)})$ , whose left components twisted by  $\sigma^{\ell_0}$ .



**Proposition 8** (Translates for the case 9). (I) Let  $r_0 \in \mathbb{N}$ ,  $r_0 < 17$ .  $r_0$ -translates of the elements  $Y_t^{(9)}$  are described by the following way.

(1) If  $r_0 = 0$ , then  $\Omega^0(Y_t^{(9)})$  is described with  $(7s \times 13s)$ -matrix with the following elements  $b_{ij}$ :  
If  $s \leq j < 2s$ , then

$$b_{ij} = \begin{cases} e_{7(j+m)} \otimes e_{7j}, & i = j - s; \\ 0, & \text{otherwise.} \end{cases}$$

If  $2s \leq j < 3s$ , then

$$b_{ij} = \begin{cases} -e_{7(j+m)+1} \otimes e_{7j+1}, & i = j - s; \\ 0, & \text{otherwise.} \end{cases}$$

If  $3s \leq j < 4s$ , then  $b_{ij} = 0$ .

If  $4s \leq j < 5s$ , then

$$b_{ij} = \begin{cases} -e_{7(j+m)+2} \otimes e_{7j+2}, & i = j - 2s; \\ 0, & \text{otherwise.} \end{cases}$$

If  $5s \leq j < 6s$ , then

$$b_{ij} = \begin{cases} -e_{7(j+m)+3} \otimes e_{7j+3}, & i = j - 2s; \\ 0, & \text{otherwise.} \end{cases}$$

If  $6s \leq j < 8s$ , then  $b_{ij} = 0$ .

If  $8s \leq j < 9s$ , then

$$b_{ij} = \begin{cases} w_{7(j+m)+4 \rightarrow 7(j+m)+5} \otimes e_{7j+4}, & i = j - 4s; \\ 0, & \text{otherwise.} \end{cases}$$

If  $9s \leq j < 11s$ , then  $b_{ij} = 0$ .

If  $11s \leq j < 12s$ , then

$$b_{ij} = \begin{cases} e_{7(j+m)+6} \otimes e_{7j+6}, & i = j - 5s; \\ 0, & \text{otherwise.} \end{cases}$$

If  $12s \leq j < 13s$ , then

$$b_{ij} = \begin{cases} -w_{7(j+m)+6 \rightarrow 7(j+m)+1} \otimes e_{7j+6}, & i = j - 6s; \\ 0, & \text{otherwise.} \end{cases}$$

(2) If  $r_0 = 1$ , then  $\Omega^1(Y_t^{(9)})$  is described with  $(8s \times 12s)$ -matrix with the following elements  $b_{ij}$ :  
If  $0 \leq j < s$ , then

$$b_{ij} = \begin{cases} w_{7(j+m)+4 \rightarrow 7(j+m)+5} \otimes e_{7j}, & i = j + s; \\ 0, & \text{otherwise.} \end{cases}$$

If  $s \leq j < 2s$ , then

$$b_{ij} = \begin{cases} e_{7(j+m)+3} \otimes w_{7j \rightarrow 7j+2}, & i = j + 2s; \\ 0, & \text{otherwise.} \end{cases}$$

If  $2s \leq j < 3s$ , then

$$b_{ij} = \begin{cases} e_{7(j+m)+1} \otimes e_{7j}, & i = j - 2s; \\ 0, & \text{otherwise.} \end{cases}$$

If  $3s \leq j < 4s$ , then

$$b_{ij} = \begin{cases} -w_{7(j+m)+2 \rightarrow 7(j+m)+6} \otimes e_{7j+1}, & i = j - s; \\ 0, & \text{otherwise.} \end{cases}$$

If  $4s \leq j < 5s$ , then

$$b_{ij} = \begin{cases} -w_{7(j+m)+3 \rightarrow 7(j+m)+1} \otimes e_{7j+2}, & i = j - s; \\ -e_{7(j+m)+1} \otimes w_{7j+2 \rightarrow 7j+6}, & i = j + 3s; \\ 0, & \text{otherwise.} \end{cases}$$

If  $5s \leq j < 6s$ , then

$$b_{ij} = \begin{cases} -e_{7(j+m)+6} \otimes e_{7j+3}, & i = j - s; \\ 0, & \text{otherwise.} \end{cases}$$

If  $6s \leq j < 7s$ , then

$$b_{ij} = \begin{cases} -w_{7(j+m)+5 \rightarrow 7(j+m)+6} \otimes e_{7j+4}, & i = j - s; \\ -e_{7(j+m)+6} \otimes w_{7j+4 \rightarrow 7j+5}, & i = j; \\ 0, & \text{otherwise.} \end{cases}$$

If  $7s \leq j < 8s$ , then

$$b_{ij} = \begin{cases} w_{7(j+m)+5 \rightarrow 7(j+m)+1} \otimes e_{7j+4}, & i = j - 2s; \\ w_{7(j+m)+6 \rightarrow 7(j+m)+1} \otimes w_{7j+4 \rightarrow 7j+5}, & i = j - s; \\ e_{7(j+m)+1} \otimes w_{7j+4 \rightarrow 7j+6}, & i = j; \\ 0, & \text{otherwise.} \end{cases}$$

If  $8s \leq j < 9s$ , then  $b_{ij} = 0$ .

If  $9s \leq j < 10s$ , then

$$b_{ij} = \begin{cases} e_{7(j+m+1)+2} \otimes w_{7j+6 \rightarrow 7(j+1)+1}, & i = 2s + (j+1)s; \\ 0, & \text{otherwise.} \end{cases}$$

If  $10s \leq j < 11s$ , then

$$b_{ij} = \begin{cases} w_{7(j+m+1)+4 \rightarrow 7(j+m+1)+5} \otimes w_{7j+6 \rightarrow 7(j+1)}, & i = s + (j+1)s; \\ w_{7(j+m+1) \rightarrow 7(j+m+1)+5} \otimes e_{7j+6}, & i = j - 3s; \\ 0, & \text{otherwise.} \end{cases}$$

If  $11s \leq j < 12s$ , then

$$b_{ij} = \begin{cases} -w_{7(j+m+1) \rightarrow 7(j+m+1)+4} \otimes e_{7j+6}, & i = j - 4s; \\ 0, & \text{otherwise.} \end{cases}$$

(3) If  $r_0 = 2$ , then  $\Omega^2(Y_t^{(9)})$  is described with  $(7s \times 12s)$ -matrix with the following elements  $b_{ij}$ :

If  $0 \leq j < s$ , then

$$b_{ij} = \begin{cases} -e_{7(j+m-1)+6} \otimes e_{7j}, & i = j; \\ 0, & \text{otherwise.} \end{cases}$$

If  $s \leq j < 2s$ , then  $b_{ij} = 0$ .

If  $2s \leq j < 3s$ , then

$$b_{ij} = \begin{cases} -e_{7(j+m)+2} \otimes e_{7j+1}, & i = j - s; \\ 0, & \text{otherwise.} \end{cases}$$

If  $3s \leq j < 4s$ , then

$$b_{ij} = \begin{cases} -e_{7(j+m)+3} \otimes e_{7j+2}, & i = j - s; \\ 0, & \text{otherwise.} \end{cases}$$

If  $4s \leq j < 5s$ , then  $b_{ij} = 0$ .

If  $5s \leq j < 6s$ , then

$$b_{ij} = \begin{cases} -w_{7(j+m)+4 \rightarrow 7(j+m)+5} \otimes e_{7j+3}, & i = j - 2s; \\ 0, & \text{otherwise.} \end{cases}$$

If  $6s \leq j < 7s$ , then  $b_{ij} = 0$ .

If  $7s \leq j < 8s$ , then

$$b_{ij} = \begin{cases} e_{7(j+m)+1} \otimes w_{7j+4 \rightarrow 7j+5}, & i = j - 2s; \\ 0, & \text{otherwise.} \end{cases}$$

If  $8s \leq j < 11s$ , then  $b_{ij} = 0$ .

If  $11s \leq j < 12s$ , then

$$b_{ij} = \begin{cases} -w_{7(j+m)+6 \rightarrow 7(j+m+1)} \otimes w_{7j+6 \rightarrow 7(j+1)}, & i = (j+1)s; \\ e_{7(j+m+1)} \otimes e_{7j+6}, & i = j - 5s; \\ 0, & \text{otherwise.} \end{cases}$$

(4) If  $r_0 = 3$ , then  $\Omega^3(Y_t^{(9)})$  is described with  $(9s \times 10s)$ -matrix with the following elements  $b_{ij}$ :

If  $0 \leq j < s$ , then

$$b_{ij} = \begin{cases} -e_{7(j+m)+2} \otimes e_{7j}, & i = j; \\ 0, & \text{otherwise.} \end{cases}$$

If  $s \leq j < 2s$ , then  $b_{ij} = 0$ .

If  $2s \leq j < 3s$ , then

$$b_{ij} = \begin{cases} -w_{7(j+m)+3 \rightarrow 7(j+m+1)} \otimes e_{7j+1}, & i = j; \\ 0, & \text{otherwise.} \end{cases}$$

If  $3s \leq j < 4s$ , then

$$b_{ij} = \begin{cases} -e_{7(j+m)+6} \otimes e_{7j+2}, & i = j; \\ 0, & \text{otherwise.} \end{cases}$$

If  $4s \leq j < 5s$ , then

$$b_{ij} = \begin{cases} -e_{7(j+m+1)} \otimes e_{7j+3}, & i = j; \\ 0, & \text{otherwise.} \end{cases}$$

If  $5s \leq j < 6s$ , then

$$b_{ij} = \begin{cases} -e_{7(j+m+1)} \otimes w_{7j+4 \rightarrow 7j+5}, & i = j + s; \\ 0, & \text{otherwise.} \end{cases}$$

If  $6s \leq j < 7s$ , then  $b_{ij} = 0$ .

If  $7s \leq j < 8s$ , then

$$b_{ij} = \begin{cases} w_{7(j+m+1)+4 \rightarrow 7(j+m+1)+5} \otimes e_{7j+6}, & i = j + s; \\ 0, & \text{otherwise.} \end{cases}$$

If  $8s \leq j < 9s$ , then

$$b_{ij} = \begin{cases} e_{7(j+m+1)+3} \otimes w_{7j+6 \rightarrow 7(j+1)+1}, & i = 2s + (j + 1)s; \\ 0, & \text{otherwise.} \end{cases}$$

If  $9s \leq j < 10s$ , then

$$b_{ij} = \begin{cases} e_{7(j+m+1)+1} \otimes e_{7j+6}, & i = j - 2s; \\ 0, & \text{otherwise.} \end{cases}$$

(5) If  $r_0 = 4$ , then  $\Omega^4(Y_t^{(9)})$  is described with  $(10s \times 10s)$ -matrix with the following elements  $b_{ij}$ :

If  $0 \leq j < s$ , then

$$b_{ij} = \begin{cases} -w_{7(j+m-1)+6 \rightarrow 7(j+m)} \otimes e_{7j}, & i = j; \\ -e_{7(j+m)} \otimes e_{7j}, & i = j + s; \\ 0, & \text{otherwise.} \end{cases}$$

If  $s \leq j < 2s$ , then

$$b_{ij} = \begin{cases} -e_{7(j+m)+3} \otimes e_{7j+1}, & i = j + s; \\ 0, & \text{otherwise.} \end{cases}$$

If  $2s \leq j < 3s$ , then  $b_{ij} = 0$ .

If  $3s \leq j < 4s$ , then

$$b_{ij} = \begin{cases} -w_{7(j+m)+4 \rightarrow 7(j+m)+5} \otimes e_{7j+2}, & i = j; \\ 0, & \text{otherwise.} \end{cases}$$

If  $4s \leq j < 5s$ , then

$$b_{ij} = \begin{cases} -e_{7(j+m)+1} \otimes e_{7j+3}, & i = j; \\ 0, & \text{otherwise.} \end{cases}$$

If  $5s \leq j < 6s$ , then

$$b_{ij} = \begin{cases} -e_{7(j+m)+2} \otimes w_{7j+4 \rightarrow 7j+5}, & i = j + 2s; \\ 0, & \text{otherwise.} \end{cases}$$

If  $6s \leq j < 7s$ , then

$$b_{ij} = \begin{cases} -w_{7(j+m)+4 \rightarrow 7(j+m)+5} \otimes w_{7j+4 \rightarrow 7j+5}, & i = j + 2s; \\ 0, & \text{otherwise.} \end{cases}$$

If  $7s \leq j < 8s$ , then  $b_{ij} = 0$ .

If  $8s \leq j < 9s$ , then

$$b_{ij} = \begin{cases} -e_{7(j+m)+6} \otimes e_{7j+6}, & i = j + s; \\ 0, & \text{otherwise.} \end{cases}$$

If  $9s \leq j < 10s$ , then  $b_{ij} = 0$ .

(6) If  $r_0 = 5$ , then  $\Omega^5(Y_t^{(9)})$  is described with  $(10s \times 9s)$ -matrix with the following elements  $b_{ij}$ :  
If  $0 \leq j < s$ , then

$$b_{ij} = \begin{cases} -e_{7(j+m)+3} \otimes e_{7j}, & i = j + s; \\ -w_{7(j+m)+1 \rightarrow 7(j+m)+3} \otimes e_{7j}, & i = j + 2s; \\ 0, & \text{otherwise.} \end{cases}$$

If  $s \leq j < 2s$ , then

$$b_{ij} = \begin{cases} -w_{7(j+m)+4 \rightarrow 7(j+m)+5} \otimes e_{7j}, & i = j - s; \\ 0, & \text{otherwise.} \end{cases}$$

If  $2s \leq j < 3s$ , then

$$b_{ij} = \begin{cases} -e_{7(j+m)+6} \otimes e_{7j+1}, & i = j + s; \\ -e_{7(j+m)+6} \otimes w_{7j+1 \rightarrow 7j+3}, & i = j + 3s; \\ 0, & \text{otherwise.} \end{cases}$$

If  $3s \leq j < 4s$ , then

$$b_{ij} = \begin{cases} -e_{7(j+m+1)} \otimes e_{7j+2}, & i = j + s; \\ w_{7(j+m)+6 \rightarrow 7(j+m+1)} \otimes w_{7j+2 \rightarrow 7j+3}, & i = j + 2s; \\ 0, & \text{otherwise.} \end{cases}$$

If  $4s \leq j < 5s$ , then

$$b_{ij} = \begin{cases} -e_{7(j+m+1)+1} \otimes w_{7j+3 \rightarrow 7(j+1)}, & i = 2s + (j+1)s; \\ -w_{7(j+m)+6 \rightarrow 7(j+m+1)+1} \otimes e_{7j+3}, & i = j + s; \\ 0, & \text{otherwise.} \end{cases}$$

If  $5s \leq j < 6s$ , then

$$b_{ij} = \begin{cases} -e_{7(j+m)+6} \otimes w_{7j+4 \rightarrow 7j+5}, & i = j + 2s; \\ 0, & \text{otherwise.} \end{cases}$$

If  $6s \leq j < 7s$ , then  $b_{ij} = 0$ .

If  $7s \leq j < 8s$ , then

$$b_{ij} = \begin{cases} -e_{7(j+m+1)+2} \otimes e_{7j+6}, & i = j + s; \\ 0, & \text{otherwise.} \end{cases}$$

If  $8s \leq j < 9s$ , then  $b_{ij} = 0$ .

(7) If  $r_0 = 6$ , then  $\Omega^6(Y_t^{(9)})$  is described with  $(12s \times 7s)$ -matrix with the following elements  $b_{ij}$ :  
If  $0 \leq j < s$ , then

$$b_{ij} = \begin{cases} e_{7(j+m-1)+6} \otimes e_{7j}, & i = j; \\ 0, & \text{otherwise.} \end{cases}$$

If  $s \leq j < 2s$ , then

$$b_{ij} = \begin{cases} -w_{7(j+m)+4 \rightarrow 7(j+m)+5} \otimes e_{7j+1}, & i = j + s; \\ 0, & \text{otherwise.} \end{cases}$$

If  $2s \leq j < 3s$ , then

$$b_{ij} = \begin{cases} -e_{7(j+m)+1} \otimes e_{7j+2}, & i = j + s; \\ 0, & \text{otherwise.} \end{cases}$$

If  $3s \leq j < 4s$ , then

$$b_{ij} = \begin{cases} -e_{7(j+m)+2} \otimes e_{7j+3}, & i = j + 2s; \\ 0, & \text{otherwise.} \end{cases}$$

If  $4s \leq j < 5s$ , then

$$b_{ij} = \begin{cases} -e_{7(j+m)+3} \otimes w_{7j+4 \rightarrow 7j+5}, & i = j + 4s; \\ 0, & \text{otherwise.} \end{cases}$$

If  $5s \leq j < 6s$ , then  $b_{ij} = 0$ .

If  $6s \leq j < 7s$ , then

$$b_{ij} = \begin{cases} -w_{7(j+m)+6 \rightarrow 7(j+m)+1} \otimes e_{7j+6}, & i = j + 4s; \\ -e_{7(j+m)+1} \otimes e_{7j+6}, & i = j + 5s; \\ 0, & \text{otherwise.} \end{cases}$$

(8) If  $r_0 = 7$ , then  $\Omega^7(Y_t^{(9)})$  is described with  $(12s \times 8s)$ -matrix with the following elements  $b_{ij}$ :  
If  $0 \leq j < s$ , then

$$b_{ij} = \begin{cases} w_{7(j+m)+2 \rightarrow 7(j+m)+6} \otimes e_{7j}, & i = j; \\ -w_{7(j+m)+4 \rightarrow 7(j+m)+6} \otimes e_{7j}, & i = j + 2s; \\ e_{7(j+m)+6} \otimes w_{7j \rightarrow 7j+4}, & i = j + 6s; \\ 0, & \text{otherwise.} \end{cases}$$

If  $s \leq j < 2s$ , then

$$b_{ij} = \begin{cases} -e_{7(j+m)+1} \otimes e_{7j+1}, & i = j + 2s; \\ -e_{7(j+m)+1} \otimes w_{7j+1 \rightarrow 7j+3}, & i = j + 4s; \\ 0, & \text{otherwise.} \end{cases}$$

If  $2s \leq j < 3s$ , then

$$b_{ij} = \begin{cases} -w_{7(j+m)+6 \rightarrow 7(j+m)+1} \otimes e_{7j+2}, & i = j + 2s; \\ -e_{7(j+m)+1} \otimes w_{7j+2 \rightarrow 7j+6}, & i = j + 9s; \\ 0, & \text{otherwise.} \end{cases}$$

If  $3s \leq j < 4s$ , then

$$b_{ij} = \begin{cases} e_{7(j+m)+2} \otimes w_{7j+3 \rightarrow 7(j+1)}, & i = (j+1)s; \\ -w_{7(j+m)+1 \rightarrow 7(j+m)+2} \otimes e_{7j+3}, & i = j + 2s; \\ 0, & \text{otherwise.} \end{cases}$$

If  $4s \leq j < 5s$ , then

$$b_{ij} = \begin{cases} -w_{7(j+m)+6 \rightarrow 7(j+m+1)} \otimes w_{7j+4 \rightarrow 7j+5}, & i = j + 3s; \\ -e_{7(j+m+1)} \otimes w_{7j+4 \rightarrow 7j+5}, & i = j + 4s; \\ 0, & \text{otherwise.} \end{cases}$$

If  $5s \leq j < 6s$ , then

$$b_{ij} = \begin{cases} w_{7(j+m)+6 \rightarrow 7(j+m+1)+4} \otimes e_{7j+5}, & i = j + 2s; \\ w_{7(j+m+1) \rightarrow 7(j+m+1)+4} \otimes e_{7j+5}, & i = j + 3s; \\ 0, & \text{otherwise.} \end{cases}$$

If  $6s \leq j < 7s$ , then

$$b_{ij} = \begin{cases} -e_{7(j+m+1)+3} \otimes e_{7j+6}, & i = j + 4s; \\ -w_{7(j+m+1)+1 \rightarrow 7(j+m+1)+3} \otimes e_{7j+6}, & i = j + 5s; \\ 0, & \text{otherwise.} \end{cases}$$

If  $7s \leq j < 8s$ , then

$$b_{ij} = \begin{cases} -w_{7(j+m+1)+4 \rightarrow 7(j+m+1)+5} \otimes e_{7j+6}, & i = j + 2s; \\ 0, & \text{otherwise.} \end{cases}$$

(9) If  $r_0 = 8$ , then  $\Omega^8(Y_t^{(9)})$  is described with  $(13s \times 7s)$ -matrix with the following elements  $b_{ij}$ :  
If  $0 \leq j < s$ , then

$$b_{ij} = \begin{cases} w_{7(j+m-1)+6 \rightarrow 7(j+m)} \otimes e_{7j}, & i = j; \\ e_{7(j+m)} \otimes e_{7j}, & i = j + s; \\ 0, & \text{otherwise.} \end{cases}$$

If  $s \leq j < 2s$ , then

$$b_{ij} = \begin{cases} -e_{7(j+m)+1} \otimes e_{7j+1}, & i = j + s; \\ 0, & \text{otherwise.} \end{cases}$$

If  $2s \leq j < 3s$ , then

$$b_{ij} = \begin{cases} -e_{7(j+m)+2} \otimes e_{7j+2}, & i = j + 2s; \\ 0, & \text{otherwise.} \end{cases}$$

If  $3s \leq j < 4s$ , then

$$b_{ij} = \begin{cases} -e_{7(j+m)+3} \otimes e_{7j+3}, & i = j + 2s; \\ 0, & \text{otherwise.} \end{cases}$$

If  $4s \leq j < 5s$ , then  $b_{ij} = 0$ .

If  $5s \leq j < 6s$ , then

$$b_{ij} = \begin{cases} w_{7(j+m)+4 \rightarrow 7(j+m)+5} \otimes e_{7j+5}, & i = j + 4s; \\ 0, & \text{otherwise.} \end{cases}$$

If  $6s \leq j < 7s$ , then

$$b_{ij} = \begin{cases} e_{7(j+m)+6} \otimes e_{7j+6}, & i = j + 5s; \\ 0, & \text{otherwise.} \end{cases}$$

(10) If  $r_0 = 9$ , then  $\Omega^9(Y_t^{(9)})$  is described with  $(12s \times 7s)$ -matrix with the following elements  $b_{ij}$ :

If  $0 \leq j < s$ , then

$$b_{ij} = \begin{cases} w_{7(j+m)+5 \rightarrow 7(j+m+1)} \otimes e_{7j}, & i = j; \\ w_{7(j+m)+6 \rightarrow 7(j+m+1)} \otimes w_{7j \rightarrow 7j+1}, & i = j + 3s; \\ w_{7(j+m)+6 \rightarrow 7(j+m+1)} \otimes w_{7j \rightarrow 7j+3}, & i = j + 5s; \\ e_{7(j+m+1)} \otimes w_{7j \rightarrow 7j+4}, & i = j + 7s; \\ 0, & \text{otherwise.} \end{cases}$$

If  $s \leq j < 2s$ , then

$$b_{ij} = \begin{cases} e_{7(j+m+1)+1} \otimes w_{7j+1 \rightarrow 7(j+1)}, & i = 2s + (j+1)s; \\ -w_{7(j+m)+6 \rightarrow 7(j+m+1)+1} \otimes e_{7j+1}, & i = j + 2s; \\ -w_{7(j+m)+6 \rightarrow 7(j+m+1)+1} \otimes w_{7j+1 \rightarrow 7j+3}, & i = j + 4s; \\ 0, & \text{otherwise.} \end{cases}$$

If  $2s \leq j < 3s$ , then

$$b_{ij} = \begin{cases} -w_{7(j+m+1) \rightarrow 7(j+m+1)+2} \otimes e_{7j+2}, & i = j + 2s; \\ e_{7(j+m+1)+2} \otimes w_{7j+2 \rightarrow 7j+6}, & i = j + 7s; \\ 0, & \text{otherwise.} \end{cases}$$

If  $3s \leq j < 4s$ , then

$$b_{ij} = \begin{cases} e_{7(j+m+1)+3} \otimes w_{7j+3 \rightarrow 7(j+1)}, & i = s + (j+1)s; \\ w_{7(j+m+1)+1 \rightarrow 7(j+m+1)+3} \otimes w_{7j+3 \rightarrow 7(j+1)}, & i = 2s + (j+1)s; \\ -w_{7(j+m)+6 \rightarrow 7(j+m+1)+3} \otimes e_{7j+3}, & i = j + 2s; \\ 0, & \text{otherwise.} \end{cases}$$

If  $4s \leq j < 5s$ , then

$$b_{ij} = \begin{cases} w_{7(j+m)+6 \rightarrow 7(j+m+1)+4} \otimes e_{7j+4}, & i = j + 2s; \\ w_{7(j+m+1) \rightarrow 7(j+m+1)+4} \otimes e_{7j+4}, & i = j + 3s; \\ 0, & \text{otherwise.} \end{cases}$$

If  $5s \leq j < 6s$ , then

$$b_{ij} = \begin{cases} e_{7(j+m+1)+5} \otimes w_{7j+5 \rightarrow 7(j+1)}, & i = (j+1)s; \\ -e_{7(j+m+1)+5} \otimes w_{7j+5 \rightarrow 7j+6}, & i = j + 5s; \\ 0, & \text{otherwise.} \end{cases}$$

If  $6s \leq j < 7s$ , then

$$b_{ij} = \begin{cases} -w_{7(j+m+1)+5 \rightarrow 7(j+m+1)+6} \otimes w_{7j+6 \rightarrow 7(j+1)}, & i = (j+1)s; \\ -e_{7(j+m+1)+6} \otimes w_{7j+6 \rightarrow 7(j+1)+1}, & i = 3s + (j+1)s; \\ -e_{7(j+m+1)+6} \otimes w_{7j+6 \rightarrow 7(j+1)+3}, & i = 5s + (j+1)s; \\ w_{7(j+m+1)+5 \rightarrow 7(j+m+1)+6} \otimes e_{7j+6}, & i = j + 4s; \\ 0, & \text{otherwise.} \end{cases}$$



(11) If  $r_0 = 10$ , then  $\Omega^{10}(Y_t^{(9)})$  is described with  $(12s \times 8s)$ -matrix with the following elements  $b_{ij}$ :

If  $0 \leq j < s$ , then

$$b_{ij} = \begin{cases} -e_{7(j+m)+1} \otimes w_{7j \rightarrow 7j+4}, & i = j + 7s; \\ 0, & \text{otherwise.} \end{cases}$$

If  $s \leq j < 2s$ , then

$$b_{ij} = \begin{cases} w_{7(j+m-1)+6 \rightarrow 7(j+m)+4} \otimes e_{7j}, & i = j - s; \\ 0, & \text{otherwise.} \end{cases}$$

If  $2s \leq j < 3s$ , then

$$b_{ij} = \begin{cases} e_{7(j+m)+2} \otimes e_{7j+1}, & i = j; \\ 0, & \text{otherwise.} \end{cases}$$

If  $3s \leq j < 4s$ , then

$$b_{ij} = \begin{cases} e_{7(j+m)+3} \otimes e_{7j+2}, & i = j; \\ 0, & \text{otherwise.} \end{cases}$$

If  $4s \leq j < 5s$ , then

$$b_{ij} = \begin{cases} e_{7(j+m)+6} \otimes w_{7j+3 \rightarrow 7(j+1)}, & i = (j+1)_s; \\ w_{7(j+m)+5 \rightarrow 7(j+m)+6} \otimes e_{7j+3}, & i = j + s; \\ 0, & \text{otherwise.} \end{cases}$$

If  $5s \leq j < 6s$ , then

$$b_{ij} = \begin{cases} -w_{7(j+m)+4 \rightarrow 7(j+m)+5} \otimes e_{7j+4}, & i = j + s; \\ e_{7(j+m)+5} \otimes w_{7j+4 \rightarrow 7j+5}, & i = j + 4s; \\ 0, & \text{otherwise.} \end{cases}$$

If  $6s \leq j < 7s$ , then  $b_{ij} = 0$ .

If  $7s \leq j < 8s$ , then

$$b_{ij} = \begin{cases} -e_{7(j+m+1)} \otimes e_{7j+6}, & i = j + 4s; \\ 0, & \text{otherwise.} \end{cases}$$

(12) If  $r_0 = 11$ , then  $\Omega^{11}(Y_t^{(9)})$  is described with  $(10s \times 7s)$ -matrix with the following elements  $b_{ij}$ :

If  $0 \leq j < s$ , then

$$b_{ij} = \begin{cases} -w_{7(j+m)+2 \rightarrow 7(j+m)+6} \otimes e_{7j}, & i = j; \\ w_{7(j+m)+4 \rightarrow 7(j+m)+6} \otimes e_{7j}, & i = j + s; \\ -e_{7(j+m)+6} \otimes w_{7j \rightarrow 7j+2}, & i = j + 3s; \\ -e_{7(j+m)+6} \otimes w_{7j \rightarrow 7j+5}, & i = j + 6s; \\ 0, & \text{otherwise.} \end{cases}$$

If  $s \leq j < 2s$ , then

$$b_{ij} = \begin{cases} -e_{7(j+m+1)+2} \otimes w_{7j+1 \rightarrow 7(j+1)}, & i = (j+1)_s; \\ -w_{7(j+m+1) \rightarrow 7(j+m+1)+2} \otimes e_{7j+1}, & i = j+s; \\ -w_{7(j+m+1) \rightarrow 7(j+m+1)+2} \otimes w_{7j+1 \rightarrow 7j+3}, & i = j+3s; \\ 0, & \text{otherwise.} \end{cases}$$

If  $2s \leq j < 3s$ , then

$$b_{ij} = \begin{cases} -w_{7(j+m)+6 \rightarrow 7(j+m+1)+3} \otimes e_{7j+2}, & i = j+s; \\ w_{7(j+m+1) \rightarrow 7(j+m+1)+3} \otimes w_{7j+2 \rightarrow 7j+3}, & i = j+2s; \\ e_{7(j+m+1)+3} \otimes w_{7j+2 \rightarrow 7j+6}, & i = j+6s; \\ 0, & \text{otherwise.} \end{cases}$$

If  $3s \leq j < 4s$ , then

$$b_{ij} = \begin{cases} -w_{7(j+m+1) \rightarrow 7(j+m+1)+4} \otimes e_{7j+3}, & i = j+s; \\ 0, & \text{otherwise.} \end{cases}$$

If  $4s \leq j < 5s$ , then

$$b_{ij} = \begin{cases} w_{7(j+m+1)+4 \rightarrow 7(j+m+1)+5} \otimes w_{7j+4 \rightarrow 7(j+1)}, & i = s + (j+1)_s; \\ w_{7(j+m+1) \rightarrow 7(j+m+1)+5} \otimes e_{7j+4}, & i = j+s; \\ 0, & \text{otherwise.} \end{cases}$$

If  $5s \leq j < 6s$ , then

$$b_{ij} = \begin{cases} e_{7(j+m+1)+1} \otimes w_{7j+5 \rightarrow 7j+6}, & i = j+4s; \\ 0, & \text{otherwise.} \end{cases}$$

If  $6s \leq j < 7s$ , then

$$b_{ij} = \begin{cases} w_{7(j+m+1)+4 \rightarrow 7(j+m+2)} \otimes w_{7j+6 \rightarrow 7(j+1)}, & i = s + (j+1)_s; \\ -e_{7(j+m+2)} \otimes w_{7j+6 \rightarrow 7(j+1)+1}, & i = 2s + (j+1)_s; \\ -2e_{7(j+m+2)} \otimes w_{7j+6 \rightarrow 7(j+1)+3}, & i = 4s + (j+1)_s; \\ e_{7(j+m+2)} \otimes w_{7j+6 \rightarrow 7(j+1)+4}, & i = 5s + (j+1)_s; \\ w_{7(j+m+1)+5 \rightarrow 7(j+m+2)} \otimes e_{7j+6}, & i = j+s; \\ 0, & \text{otherwise.} \end{cases}$$

(13) If  $r_0 = 12$ , then  $\Omega^{12}(Y_t^{(9)})$  is described with  $(10s \times 9s)$ -matrix with the following elements  $b_{ij}$ :

If  $0 \leq j < s$ , then

$$b_{ij} = \begin{cases} w_{7(j+m) \rightarrow 7(j+m)+2} \otimes e_{7j}, & i = j; \\ e_{7(j+m)+2} \otimes w_{7j \rightarrow 7j+4}, & i = j+5s; \\ 0, & \text{otherwise.} \end{cases}$$

If  $s \leq j < 2s$ , then

$$b_{ij} = \begin{cases} -w_{7(j+m) \rightarrow 7(j+m)+5} \otimes e_{7j}, & i = j - s; \\ w_{7(j+m)+4 \rightarrow 7(j+m)+5} \otimes w_{7j \rightarrow 7j+1}, & i = j + s; \\ 0, & \text{otherwise.} \end{cases}$$

If  $2s \leq j < 3s$ , then

$$b_{ij} = \begin{cases} e_{7(j+m)+3} \otimes e_{7j+1}, & i = j - s; \\ 0, & \text{otherwise.} \end{cases}$$

If  $3s \leq j < 4s$ , then

$$b_{ij} = \begin{cases} w_{7(j+m)+5 \rightarrow 7(j+m)+6} \otimes e_{7j+2}, & i = j; \\ -w_{7(j+m)+1 \rightarrow 7(j+m)+6} \otimes w_{7j+2 \rightarrow 7j+3}, & i = j + s; \\ e_{7(j+m)+6} \otimes w_{7j+2 \rightarrow 7j+6}, & i = j + 5s; \\ 0, & \text{otherwise.} \end{cases}$$

If  $4s \leq j < 5s$ , then

$$b_{ij} = \begin{cases} 2e_{7(j+m+1)} \otimes w_{7j+3 \rightarrow 7(j+1)}, & i = (j+1)_s; \\ w_{7(j+m)+1 \rightarrow 7(j+m+1)} \otimes e_{7j+3}, & i = j; \\ -w_{7(j+m)+6 \rightarrow 7(j+m+1)} \otimes w_{7j+3 \rightarrow 7j+6}, & i = j + 4s; \\ -e_{7(j+m+1)} \otimes w_{7j+3 \rightarrow 7j+6}, & i = j + 5s; \\ 0, & \text{otherwise.} \end{cases}$$

If  $5s \leq j < 6s$ , then

$$b_{ij} = \begin{cases} -w_{7(j+m)+2 \rightarrow 7(j+m)+6} \otimes e_{7j+4}, & i = j; \\ 0, & \text{otherwise.} \end{cases}$$

If  $6s \leq j < 7s$ , then

$$b_{ij} = \begin{cases} e_{7(j+m+1)} \otimes w_{7j+5 \rightarrow 7(j+1)}, & i = (j+1)_s; \\ -w_{7(j+m)+3 \rightarrow 7(j+m+1)} \otimes e_{7j+5}, & i = j + s; \\ -w_{7(j+m)+6 \rightarrow 7(j+m+1)} \otimes w_{7j+5 \rightarrow 7j+6}, & i = j + 2s; \\ 0, & \text{otherwise.} \end{cases}$$

If  $7s \leq j < 8s$ , then

$$b_{ij} = \begin{cases} w_{7(j+m+1) \rightarrow 7(j+m+1)+1} \otimes w_{7j+6 \rightarrow 7(j+1)}, & i = (j+1)_s; \\ e_{7(j+m+1)+1} \otimes w_{7j+6 \rightarrow 7(j+1)+3}, & i = 4s + (j+1)_s; \\ 0, & \text{otherwise.} \end{cases}$$

If  $8s \leq j < 9s$ , then

$$b_{ij} = \begin{cases} -w_{7(j+m+1) \rightarrow 7(j+m+1)+4} \otimes w_{7j+6 \rightarrow 7(j+1)}, & i = (j+1)_s; \\ w_{7(j+m)+6 \rightarrow 7(j+m+1)+4} \otimes e_{7j+6}, & i = j; \\ 0, & \text{otherwise.} \end{cases}$$

(14) If  $r_0 = 13$ , then  $\Omega^{13}(Y_t^{(9)})$  is described with  $(9s \times 10s)$ -matrix with the following elements  $b_{ij}$ :

If  $0 \leq j < s$ , then

$$b_{ij} = \begin{cases} -e_{7(j+m)+6} \otimes w_{7j \rightarrow 7j+1}, & i = j + 2s; \\ 0, & \text{otherwise.} \end{cases}$$

If  $s \leq j < 2s$ , then

$$b_{ij} = \begin{cases} -w_{7(j+m)+3 \rightarrow 7(j+m+1)} \otimes e_{7j}, & i = j - s; \\ -w_{7(j+m)+6 \rightarrow 7(j+m+1)} \otimes w_{7j \rightarrow 7j+1}, & i = j + s; \\ -e_{7(j+m+1)} \otimes w_{7j \rightarrow 7j+2}, & i = j + 2s; \\ 0, & \text{otherwise.} \end{cases}$$

If  $2s \leq j < 3s$ , then

$$b_{ij} = \begin{cases} -e_{7(j+m+1)+3} \otimes w_{7j+1 \rightarrow 7(j+1)}, & i = (j + 1)_s; \\ -w_{7(j+m)+6 \rightarrow 7(j+m+1)+3} \otimes e_{7j+1}, & i = j; \\ 0, & \text{otherwise.} \end{cases}$$

If  $3s \leq j < 4s$ , then

$$b_{ij} = \begin{cases} -w_{7(j+m+1) \rightarrow 7(j+m+1)+4} \otimes e_{7j+2}, & i = j; \\ 0, & \text{otherwise.} \end{cases}$$

If  $4s \leq j < 5s$ , then

$$b_{ij} = \begin{cases} -e_{7(j+m+1)+1} \otimes e_{7j+3}, & i = j; \\ 0, & \text{otherwise.} \end{cases}$$

If  $5s \leq j < 6s$ , then

$$b_{ij} = \begin{cases} w_{7(j+m+1)+4 \rightarrow 7(j+m+1)+5} \otimes w_{7j+3 \rightarrow 7j+6}, & i = j + 3s; \\ 0, & \text{otherwise.} \end{cases}$$

If  $6s \leq j < 7s$ , then

$$b_{ij} = \begin{cases} -w_{7(j+m)+6 \rightarrow 7(j+m+1)+1} \otimes e_{7j+4}, & i = j - s; \\ 0, & \text{otherwise.} \end{cases}$$

If  $7s \leq j < 8s$ , then

$$b_{ij} = \begin{cases} -w_{7(j+m+1) \rightarrow 7(j+m+1)+2} \otimes e_{7j+5}, & i = j - s; \\ -e_{7(j+m+1)+2} \otimes w_{7j+5 \rightarrow 7j+6}, & i = j; \\ 0, & \text{otherwise.} \end{cases}$$

If  $8s \leq j < 9s$ , then  $b_{ij} = 0$ .

If  $9s \leq j < 10s$ , then

$$b_{ij} = \begin{cases} -e_{7(j+m+1)+6} \otimes w_{7j+6 \rightarrow 7(j+1)+1}, & i = 2s + (j + 1)_s; \\ -w_{7(j+m+1)+2 \rightarrow 7(j+m+1)+6} \otimes e_{7j+6}, & i = j - 2s; \\ w_{7(j+m+1)+4 \rightarrow 7(j+m+1)+6} \otimes e_{7j+6}, & i = j - s; \\ 0, & \text{otherwise.} \end{cases}$$

(15) If  $r_0 = 14$ , then  $\Omega^{14}(Y_t^{(9)})$  is described with  $(7s \times 10s)$ -matrix with the following elements  $b_{ij}$ :

If  $s \leq j < 2s$ , then

$$b_{ij} = \begin{cases} e_{7(j+m)+3} \otimes w_{7j \rightarrow 7j+4}, & i = j + 3s; \\ 0, & \text{otherwise.} \end{cases}$$

If  $2s \leq j < 3s$ , then

$$b_{ij} = \begin{cases} w_{7(j+m-1)+6 \rightarrow 7(j+m)+1} \otimes e_{7j}, & i = j - 2s; \\ e_{7(j+m)+1} \otimes w_{7j \rightarrow 7j+2}, & i = j; \\ 0, & \text{otherwise.} \end{cases}$$

If  $3s \leq j < 4s$ , then

$$b_{ij} = \begin{cases} e_{7(j+m)+6} \otimes w_{7j+1 \rightarrow 7(j+1)}, & i = (j+1)_s; \\ w_{7(j+m)+5 \rightarrow 7(j+m)+6} \otimes e_{7j+1}, & i = j - 2s; \\ 0, & \text{otherwise.} \end{cases}$$

If  $4s \leq j < 5s$ , then

$$b_{ij} = \begin{cases} w_{7(j+m)+1 \rightarrow 7(j+m+1)} \otimes e_{7j+2}, & i = j - 2s; \\ -w_{7(j+m)+2 \rightarrow 7(j+m+1)} \otimes w_{7j+2 \rightarrow 7j+3}, & i = j - s; \\ e_{7(j+m+1)} \otimes w_{7j+2 \rightarrow 7j+6}, & i = j + 2s; \\ 0, & \text{otherwise.} \end{cases}$$

If  $5s \leq j < 6s$ , then

$$b_{ij} = \begin{cases} w_{7(j+m)+2 \rightarrow 7(j+m)+6} \otimes e_{7j+3}, & i = j - 2s; \\ 0, & \text{otherwise.} \end{cases}$$

If  $6s \leq j < 7s$ , then

$$b_{ij} = \begin{cases} -w_{7(j+m)+3 \rightarrow 7(j+m+1)} \otimes e_{7j+4}, & i = j - 2s; \\ 0, & \text{otherwise.} \end{cases}$$

If  $7s \leq j < 8s$ , then

$$b_{ij} = \begin{cases} -w_{7(j+m)+4 \rightarrow 7(j+m)+6} \otimes e_{7j+5}, & i = j - 2s; \\ 0, & \text{otherwise.} \end{cases}$$

If  $8s \leq j < 9s$ , then

$$b_{ij} = \begin{cases} e_{7(j+m+1)+2} \otimes w_{7j+6 \rightarrow 7(j+1)+3}, & i = 3s + (j+1)_s; \\ w_{7(j+m+1) \rightarrow 7(j+m+1)+2} \otimes e_{7j+6}, & i = j - 2s; \\ 0, & \text{otherwise.} \end{cases}$$

If  $9s \leq j < 10s$ , then

$$b_{ij} = \begin{cases} -e_{7(j+m+1)+5} \otimes w_{7j+6 \rightarrow 7(j+1)+1}, & i = s + (j+1)_s; \\ 0, & \text{otherwise.} \end{cases}$$

(16) If  $r_0 = 15$ , then  $\Omega^{15}(Y_t^{(9)})$  is described with  $(8s \times 12s)$ -matrix with the following elements  $b_{ij}$ :

If  $0 \leq j < s$ , then

$$b_{ij} = \begin{cases} e_{7(j+m)+6} \otimes e_{7j}, & i = j; \\ 0, & \text{otherwise.} \end{cases}$$

If  $s \leq j < 2s$ , then

$$b_{ij} = \begin{cases} -e_{7(j+m+1)} \otimes w_{7j \rightarrow 7j+1}, & i = j; \\ 0, & \text{otherwise.} \end{cases}$$

If  $2s \leq j < 3s$ , then

$$b_{ij} = \begin{cases} -w_{7(j+m+1) \rightarrow 7(j+m+1)+4} \otimes e_{7j+1}, & i = j - s; \\ 0, & \text{otherwise.} \end{cases}$$

If  $3s \leq j < 4s$ , then

$$b_{ij} = \begin{cases} -e_{7(j+m+1)+1} \otimes e_{7j+2}, & i = j - s; \\ 0, & \text{otherwise.} \end{cases}$$

If  $4s \leq j < 5s$ , then

$$b_{ij} = \begin{cases} -e_{7(j+m+1)+5} \otimes w_{7j+2 \rightarrow 7j+6}, & i = j + 3s; \\ 0, & \text{otherwise.} \end{cases}$$

If  $5s \leq j < 6s$ , then

$$b_{ij} = \begin{cases} -e_{7(j+m+1)+2} \otimes e_{7j+3}, & i = j - 2s; \\ 0, & \text{otherwise.} \end{cases}$$

If  $6s \leq j < 7s$ , then

$$b_{ij} = \begin{cases} -w_{7(j+m+1) \rightarrow 7(j+m+1)+2} \otimes e_{7j+4}, & i = j - 2s; \\ 0, & \text{otherwise.} \end{cases}$$

If  $7s \leq j < 8s$ , then  $b_{ij} = 0$ .

If  $8s \leq j < 9s$ , then

$$b_{ij} = \begin{cases} -e_{7(j+m+1)+3} \otimes w_{7j+5 \rightarrow 7j+6}, & i = j - 2s; \\ 0, & \text{otherwise.} \end{cases}$$

If  $9s \leq j < 10s$ , then  $b_{ij} = 0$ .

If  $10s \leq j < 11s$ , then

$$b_{ij} = \begin{cases} w_{7(j+m+1)+3 \rightarrow 7(j+m+1)+6} \otimes e_{7j+6}, & i = j - 4s; \\ 0, & \text{otherwise.} \end{cases}$$

If  $11s \leq j < 12s$ , then

$$b_{ij} = \begin{cases} -e_{7(j+m+2)} \otimes w_{7j+6 \rightarrow 7(j+1)+1}, & i = s + (j+1)_s; \\ 0, & \text{otherwise.} \end{cases}$$

(17) If  $r_0 = 16$ , then  $\Omega^{16}(Y_t^{(9)})$  is described with  $(7s \times 12s)$ -matrix with the following elements  $b_{ij}$ :

If  $0 \leq j < s$ , then

$$b_{ij} = \begin{cases} -w_{7(j+m) \rightarrow 7(j+m)+2} \otimes e_{7j}, & i = j; \\ -e_{7(j+m)+2} \otimes w_{7j \rightarrow 7j+2}, & i = j + 2s; \\ 0, & \text{otherwise.} \end{cases}$$

If  $s \leq j < 2s$ , then

$$b_{ij} = \begin{cases} w_{7(j+m) \rightarrow 7(j+m)+5} \otimes e_{7j}, & i = j - s; \\ w_{7(j+m)+4 \rightarrow 7(j+m)+5} \otimes w_{7j \rightarrow 7j+4}, & i = j + 3s; \\ -e_{7(j+m)+5} \otimes w_{7j \rightarrow 7j+5}, & i = j + 4s; \\ 0, & \text{otherwise.} \end{cases}$$

If  $2s \leq j < 3s$ , then  $b_{ij} = 0$ .

If  $3s \leq j < 4s$ , then

$$b_{ij} = \begin{cases} e_{7(j+m)+1} \otimes w_{7j+1 \rightarrow 7(j+1)}, & i = (j+1)_s; \\ w_{7(j+m)+1 \rightarrow 7(j+m)+1} \otimes e_{7j+1}, & i = j - 2s; \\ 0, & \text{otherwise.} \end{cases}$$

If  $4s \leq j < 5s$ , then

$$b_{ij} = \begin{cases} w_{7(j+m)+2 \rightarrow 7(j+m)+6} \otimes e_{7j+2}, & i = j - 2s; \\ e_{7(j+m)+6} \otimes w_{7j+2 \rightarrow 7j+6}, & i = j + 2s; \\ 0, & \text{otherwise.} \end{cases}$$

If  $5s \leq j < 6s$ , then

$$b_{ij} = \begin{cases} w_{7(j+m)+3 \rightarrow 7(j+m)+1} \otimes e_{7j+3}, & i = j - 2s; \\ 0, & \text{otherwise.} \end{cases}$$

If  $6s \leq j < 7s$ , then

$$b_{ij} = \begin{cases} -w_{7(j+m)+4 \rightarrow 7(j+m)+6} \otimes e_{7j+4}, & i = j - 2s; \\ w_{7(j+m)+5 \rightarrow 7(j+m)+6} \otimes w_{7j+4 \rightarrow 7j+5}, & i = j - s; \\ -e_{7(j+m)+6} \otimes w_{7j+4 \rightarrow 7j+6}, & i = j; \\ 0, & \text{otherwise.} \end{cases}$$

If  $7s \leq j < 10s$ , then  $b_{ij} = 0$ .

If  $10s \leq j < 11s$ , then

$$b_{ij} = \begin{cases} e_{7(j+m)+1+3} \otimes w_{7j+6 \rightarrow 7(j+1)+3}, & i = 3s + (j+1)_s; \\ w_{7(j+m)+6 \rightarrow 7(j+m)+1+3} \otimes e_{7j+6}, & i = j - 4s; \\ 0, & \text{otherwise.} \end{cases}$$

If  $11s \leq j < 12s$ , then

$$b_{ij} = \begin{cases} e_{7(j+m)+1+1} \otimes w_{7j+6 \rightarrow 7(j+1)+1}, & i = s + (j+1)_s; \\ 0, & \text{otherwise.} \end{cases}$$

(II) Represent an arbitrary  $t_0 \in \mathbb{N}$  in the form  $t_0 = 17\ell_0 + r_0$ , where  $0 \leq r_0 \leq 16$ . Then  $\Omega^{t_0}(Y_t^{(9)})$  is a  $\Omega^{r_0}(Y_t^{(9)})$ , whose left components twisted by  $\sigma^{\ell_0}$ .

**Proposition 9** (Translates for the case 12). (I) Let  $r_0 \in \mathbb{N}$ ,  $r_0 < 17$ .  $r_0$ -translates of the elements  $Y_t^{(12)}$  are described by the following way.

(1) If  $r_0 = 0$ , then  $\Omega^0(Y_t^{(12)})$  is described with  $(7s \times 12s)$ -matrix with the following elements  $b_{ij}$ :

If  $s \leq j < 2s$ , then

$$b_{ij} = \begin{cases} e_{7(j+m)} \otimes e_{7j}, & i = j - s; \\ 0, & \text{otherwise.} \end{cases}$$

If  $2s \leq j < 3s$ , then

$$b_{ij} = \begin{cases} w_{7(j+m)+1 \rightarrow 7(j+m)+2} \otimes e_{7j+1}, & i = j - s; \\ 0, & \text{otherwise.} \end{cases}$$

If  $3s \leq j < 4s$ , then

$$b_{ij} = \begin{cases} w_{7(j+m)+2 \rightarrow 7(j+m)+3} \otimes e_{7j+2}, & i = j - s; \\ 0, & \text{otherwise.} \end{cases}$$

If  $4s \leq j < 6s$ , then  $b_{ij} = 0$ .

If  $6s \leq j < 7s$ , then

$$b_{ij} = \begin{cases} e_{7(j+m)+4} \otimes e_{7j+4}, & i = j - 2s; \\ 0, & \text{otherwise.} \end{cases}$$

If  $7s \leq j < 9s$ , then  $b_{ij} = 0$ .

If  $9s \leq j < 10s$ , then

$$b_{ij} = \begin{cases} e_{7(j+m)+5} \otimes e_{7j+5}, & i = j - 4s; \\ 0, & \text{otherwise.} \end{cases}$$

If  $10s \leq j < 11s$ , then

$$b_{ij} = \begin{cases} e_{7(j+m)+6} \otimes e_{7j+6}, & i = j - 4s; \\ 0, & \text{otherwise.} \end{cases}$$

If  $11s \leq j < 12s$ , then  $b_{ij} = 0$ .

(2) If  $r_0 = 1$ , then  $\Omega^1(Y_t^{(12)})$  is described with  $(8s \times 10s)$ -matrix with the following elements  $b_{ij}$ :

If  $0 \leq j < s$ , then

$$b_{ij} = \begin{cases} w_{7(j+m)+1 \rightarrow 7(j+m)+2} \otimes e_{7j}, & i = j; \\ 0, & \text{otherwise.} \end{cases}$$

If  $s \leq j < 2s$ , then

$$b_{ij} = \begin{cases} e_{7(j+m)+4} \otimes e_{7j}, & i = j; \\ 0, & \text{otherwise.} \end{cases}$$



If  $2s \leq j < 3s$ , then

$$b_{ij} = \begin{cases} -w_{7(j+m)+2 \rightarrow 7(j+m+1)} \otimes e_{7j+1}, & i = j; \\ w_{7(j+m)+3 \rightarrow 7(j+m+1)} \otimes w_{7j+1 \rightarrow 7j+2}, & i = j + s; \\ w_{7(j+m)+6 \rightarrow 7(j+m+1)} \otimes w_{7j+1 \rightarrow 7j+3}, & i = j + 2s; \\ e_{7(j+m+1)} \otimes w_{7j+1 \rightarrow 7j+6}, & i = j + 5s; \\ 0, & \text{otherwise.} \end{cases}$$

If  $3s \leq j < 4s$ , then

$$b_{ij} = \begin{cases} -w_{7(j+m)+3 \rightarrow 7(j+m)+6} \otimes e_{7j+2}, & i = j; \\ -e_{7(j+m)+6} \otimes w_{7j+2 \rightarrow 7j+3}, & i = j + s; \\ 0, & \text{otherwise.} \end{cases}$$

If  $4s \leq j < 5s$ , then  $b_{ij} = 0$ .

If  $5s \leq j < 6s$ , then

$$b_{ij} = \begin{cases} -w_{7(j+m)+5 \rightarrow 7(j+m+1)} \otimes e_{7j+4}, & i = j; \\ w_{7(j+m)+6 \rightarrow 7(j+m+1)} \otimes w_{7j+4 \rightarrow 7j+5}, & i = j + s; \\ e_{7(j+m+1)} \otimes w_{7j+4 \rightarrow 7j+6}, & i = j + 2s; \\ 0, & \text{otherwise.} \end{cases}$$

If  $6s \leq j < 7s$ , then

$$b_{ij} = \begin{cases} e_{7(j+m)+6} \otimes e_{7j+5}, & i = j; \\ 0, & \text{otherwise.} \end{cases}$$

If  $7s \leq j < 8s$ , then

$$b_{ij} = \begin{cases} -w_{7(j+m+1)+4 \rightarrow 7(j+m+1)+5} \otimes w_{7j+6 \rightarrow 7(j+1)}, & i = s + (j+1)_s; \\ -e_{7(j+m+1)+5} \otimes w_{7j+6 \rightarrow 7(j+1)+4}, & i = 5s + (j+1)_s; \\ w_{7(j+m+1) \rightarrow 7(j+m+1)+5} \otimes e_{7j+6}, & i = j; \\ 0, & \text{otherwise.} \end{cases}$$

If  $8s \leq j < 9s$ , then

$$b_{ij} = \begin{cases} w_{7(j+m+1)+1 \rightarrow 7(j+m+1)+3} \otimes w_{7j+6 \rightarrow 7(j+1)}, & i = (j+1)_s; \\ -w_{7(j+m+1)+2 \rightarrow 7(j+m+1)+3} \otimes w_{7j+6 \rightarrow 7(j+1)+1}, & i = 2s + (j+1)_s; \\ w_{7(j+m+1) \rightarrow 7(j+m+1)+3} \otimes e_{7j+6}, & i = j - s; \\ 0, & \text{otherwise.} \end{cases}$$

If  $9s \leq j < 10s$ , then  $b_{ij} = 0$ .

(3) If  $r_0 = 2$ , then  $\Omega^2(Y_t^{(12)})$  is described with  $(7s \times 10s)$ -matrix with the following elements  $b_{ij}$ :

If  $0 \leq j < s$ , then

$$b_{ij} = \begin{cases} -w_{7(j+m-1)+6 \rightarrow 7(j+m)} \otimes e_{7j}, & i = j; \\ 0, & \text{otherwise.} \end{cases}$$

If  $s \leq j < 2s$ , then

$$b_{ij} = \begin{cases} w_{7(j+m)+2 \rightarrow 7(j+m)+3} \otimes e_{7j+1}, & i = j; \\ 0, & \text{otherwise.} \end{cases}$$

If  $2s \leq j < 3s$ , then

$$b_{ij} = \begin{cases} e_{7(j+m)+4} \otimes w_{7j+1 \rightarrow 7j+3}, & i = j + s; \\ 0, & \text{otherwise.} \end{cases}$$

If  $3s \leq j < 4s$ , then

$$b_{ij} = \begin{cases} -w_{7(j+m)+4 \rightarrow 7(j+m)+5} \otimes w_{7j+2 \rightarrow 7j+3}, & i = j; \\ 0, & \text{otherwise.} \end{cases}$$

If  $4s \leq j < 5s$ , then  $b_{ij} = 0$ .

If  $5s \leq j < 6s$ , then

$$b_{ij} = \begin{cases} w_{7(j+m)+1 \rightarrow 7(j+m)+2} \otimes w_{7j+4 \rightarrow 7j+5}, & i = j; \\ 0, & \text{otherwise.} \end{cases}$$

If  $6s \leq j < 7s$ , then

$$b_{ij} = \begin{cases} e_{7(j+m)+5} \otimes e_{7j+4}, & i = j - 2s; \\ 0, & \text{otherwise.} \end{cases}$$

If  $7s \leq j < 8s$ , then

$$b_{ij} = \begin{cases} w_{7(j+m)+1 \rightarrow 7(j+m)+3} \otimes e_{7j+5}, & i = j - 2s; \\ 0, & \text{otherwise.} \end{cases}$$

If  $8s \leq j < 9s$ , then

$$b_{ij} = \begin{cases} -e_{7(j+m)+6} \otimes w_{7j+6 \rightarrow 7(j+1)}, & i = (j+1)s; \\ 0, & \text{otherwise.} \end{cases}$$

If  $9s \leq j < 10s$ , then

$$b_{ij} = \begin{cases} e_{7(j+m+1)} \otimes e_{7j+6}, & i = j - 3s; \\ 0, & \text{otherwise.} \end{cases}$$

(4) If  $r_0 = 3$ , then  $\Omega^3(Y_t^{(12)})$  is described with  $(9s \times 9s)$ -matrix with the following elements  $b_{ij}$ :  
If  $0 \leq j < s$ , then

$$b_{ij} = \begin{cases} w_{7(j+m)+2 \rightarrow 7(j+m)+3} \otimes e_{7j}, & i = j; \\ 0, & \text{otherwise.} \end{cases}$$

If  $s \leq j < 2s$ , then

$$b_{ij} = \begin{cases} e_{7(j+m)+5} \otimes e_{7j}, & i = j; \\ 0, & \text{otherwise.} \end{cases}$$

If  $2s \leq j < 3s$ , then

$$b_{ij} = \begin{cases} -w_{7(j+m)+3 \rightarrow 7(j+m)+6} \otimes e_{7j+1}, & i = j; \\ -e_{7(j+m)+6} \otimes w_{7j+1 \rightarrow 7j+2}, & i = j + s; \\ 0, & \text{otherwise.} \end{cases}$$

If  $3s \leq j < 4s$ , then

$$b_{ij} = \begin{cases} -e_{7(j+m+1)} \otimes w_{7j+2 \rightarrow 7j+3}, & i = j + s; \\ 0, & \text{otherwise.} \end{cases}$$

If  $4s \leq j < 5s$ , then

$$b_{ij} = \begin{cases} -w_{7(j+m+1) \rightarrow 7(j+m+1)+1} \otimes e_{7j+3}, & i = j; \\ 0, & \text{otherwise.} \end{cases}$$

If  $5s \leq j < 6s$ , then

$$b_{ij} = \begin{cases} e_{7(j+m)+6} \otimes e_{7j+4}, & i = j; \\ 0, & \text{otherwise.} \end{cases}$$

If  $6s \leq j < 7s$ , then

$$b_{ij} = \begin{cases} e_{7(j+m+1)} \otimes e_{7j+5}, & i = j; \\ 0, & \text{otherwise.} \end{cases}$$

If  $7s \leq j < 8s$ , then

$$b_{ij} = \begin{cases} w_{7(j+m+1)+1 \rightarrow 7(j+m+1)+2} \otimes e_{7j+6}, & i = j; \\ 0, & \text{otherwise.} \end{cases}$$

If  $8s \leq j < 9s$ , then

$$b_{ij} = \begin{cases} e_{7(j+m+1)+4} \otimes e_{7j+6}, & i = j; \\ 0, & \text{otherwise.} \end{cases}$$

(5) If  $r_0 = 4$ , then  $\Omega^4(Y_t^{(12)})$  is described with  $(10s \times 7s)$ -matrix with the following elements  $b_{ij}$ :

If  $0 \leq j < s$ , then

$$b_{ij} = \begin{cases} -e_{7(j+m-1)+6} \otimes e_{7j}, & i = j; \\ 0, & \text{otherwise.} \end{cases}$$

If  $s \leq j < 2s$ , then

$$b_{ij} = \begin{cases} -w_{7(j+m)+4 \rightarrow 7(j+m)+5} \otimes w_{7j+1 \rightarrow 7j+2}, & i = j + 2s; \\ -e_{7(j+m)+5} \otimes w_{7j+1 \rightarrow 7j+3}, & i = j + 4s; \\ 0, & \text{otherwise.} \end{cases}$$

If  $2s \leq j < 3s$ , then  $b_{ij} = 0$ .

If  $3s \leq j < 4s$ , then

$$b_{ij} = \begin{cases} w_{7(j+m)+1 \rightarrow 7(j+m)+2} \otimes e_{7j+3}, & i = j + s; \\ 0, & \text{otherwise.} \end{cases}$$

If  $4s \leq j < 5s$ , then

$$b_{ij} = \begin{cases} w_{7(j+m)+1 \rightarrow 7(j+m)+3} \otimes e_{7j+4}, & i = j + 2s; \\ w_{7(j+m)+2 \rightarrow 7(j+m)+3} \otimes w_{7j+4 \rightarrow 7j+5}, & i = j + 3s; \\ 0, & \text{otherwise.} \end{cases}$$

If  $5s \leq j < 6s$ , then

$$b_{ij} = \begin{cases} e_{7(j+m)+4} \otimes e_{7j+5}, & i = j + 3s; \\ 0, & \text{otherwise.} \end{cases}$$

If  $6s \leq j < 7s$ , then

$$b_{ij} = \begin{cases} -w_{7(j+m)+6 \rightarrow 7(j+m)+1} \otimes w_{7j+6 \rightarrow 7(j+1)}, & i = (j+1)_s; \\ -e_{7(j+m)+1} \otimes w_{7j+6 \rightarrow 7(j+1)}, & i = s + (j+1)_s; \\ -w_{7(j+m)+6 \rightarrow 7(j+m)+1} \otimes e_{7j+6}, & i = j + 3s; \\ 0, & \text{otherwise.} \end{cases}$$

(6) If  $r_0 = 5$ , then  $\Omega^5(Y_t^{(12)})$  is described with  $(10s \times 8s)$ -matrix with the following elements  $b_{ij}$ :

If  $0 \leq j < s$ , then

$$b_{ij} = \begin{cases} -w_{7(j+m)+4 \rightarrow 7(j+m)+6} \otimes e_{7j}, & i = j; \\ -w_{7(j+m)+3 \rightarrow 7(j+m)+6} \otimes e_{7j}, & i = j + s; \\ w_{7(j+m)+1 \rightarrow 7(j+m)+6} \otimes e_{7j}, & i = j + 2s; \\ -e_{7(j+m)+6} \otimes w_{7j \rightarrow 7j+1}, & i = j + 3s; \\ 0, & \text{otherwise.} \end{cases}$$

If  $s \leq j < 2s$ , then

$$b_{ij} = \begin{cases} -e_{7(j+m)+1} \otimes w_{7j+1 \rightarrow 7j+2}, & i = j + 3s; \\ -w_{7(j+m)+6 \rightarrow 7(j+m)+1} \otimes w_{7j+1 \rightarrow 7j+3}, & i = j + 4s; \\ 0, & \text{otherwise.} \end{cases}$$

If  $2s \leq j < 3s$ , then

$$b_{ij} = \begin{cases} e_{7(j+m)+1} \otimes w_{7j+2 \rightarrow 7(j+1)}, & i = 2s + (j+1)_s; \\ -w_{7(j+m)+6 \rightarrow 7(j+m)+1} \otimes w_{7j+2 \rightarrow 7j+3}, & i = j + 3s; \\ 0, & \text{otherwise.} \end{cases}$$

If  $3s \leq j < 4s$ , then

$$b_{ij} = \begin{cases} w_{7(j+m)+1 \rightarrow 7(j+m)+2} \otimes w_{7j+3 \rightarrow 7(j+1)}, & i = 2s + (j+1)_s; \\ -w_{7(j+m)+6 \rightarrow 7(j+m)+2} \otimes e_{7j+3}, & i = j + 2s; \\ 0, & \text{otherwise.} \end{cases}$$

If  $4s \leq j < 5s$ , then

$$b_{ij} = \begin{cases} e_{7(j+m)+1} \otimes e_{7j+4}, & i = j + 2s; \\ -w_{7(j+m)+6 \rightarrow 7(j+m)+1} \otimes w_{7j+4 \rightarrow 7j+5}, & i = j + 3s; \\ 0, & \text{otherwise.} \end{cases}$$

If  $5s \leq j < 6s$ , then

$$b_{ij} = \begin{cases} -e_{7(j+m+1)+4} \otimes w_{7j+5 \rightarrow 7(j+1)}, & i = (j+1)_s; \\ w_{7(j+m)+6 \rightarrow 7(j+m+1)+4} \otimes e_{7j+5}, & i = j+2s; \\ 0, & \text{otherwise.} \end{cases}$$

If  $6s \leq j < 7s$ , then

$$b_{ij} = \begin{cases} -w_{7(j+m+1)+1 \rightarrow 7(j+m+1)+3} \otimes w_{7j+6 \rightarrow 7(j+1)}, & i = 2s + (j+1)_s; \\ w_{7(j+m+1)+2 \rightarrow 7(j+m+1)+3} \otimes e_{7j+6}, & i = j+2s; \\ 0, & \text{otherwise.} \end{cases}$$

If  $7s \leq j < 8s$ , then

$$b_{ij} = \begin{cases} w_{7(j+m+1)+4 \rightarrow 7(j+m+1)+5} \otimes w_{7j+6 \rightarrow 7(j+1)}, & i = (j+1)_s; \\ e_{7(j+m+1)+5} \otimes e_{7j+6}, & i = j+2s; \\ 0, & \text{otherwise.} \end{cases}$$

(7) If  $r_0 = 6$ , then  $\Omega^6(Y_t^{(12)})$  is described with  $(12s \times 7s)$ -matrix with the following elements  $b_{ij}$ :

If  $0 \leq j < s$ , then

$$b_{ij} = \begin{cases} w_{7(j+m-1)+6 \rightarrow 7(j+m)} \otimes e_{7j}, & i = j; \\ -e_{7(j+m)} \otimes e_{7j}, & i = j+s; \\ 0, & \text{otherwise.} \end{cases}$$

If  $s \leq j < 2s$ , then

$$b_{ij} = \begin{cases} e_{7(j+m)+1} \otimes w_{7j+1 \rightarrow 7j+2}, & i = j+2s; \\ 0, & \text{otherwise.} \end{cases}$$

If  $2s \leq j < 3s$ , then  $b_{ij} = 0$ .

If  $3s \leq j < 4s$ , then

$$b_{ij} = \begin{cases} w_{7(j+m)+2 \rightarrow 7(j+m)+3} \otimes e_{7j+3}, & i = j+2s; \\ 0, & \text{otherwise.} \end{cases}$$

If  $4s \leq j < 5s$ , then

$$b_{ij} = \begin{cases} e_{7(j+m)+4} \otimes e_{7j+4}, & i = j+3s; \\ 0, & \text{otherwise.} \end{cases}$$

If  $5s \leq j < 6s$ , then

$$b_{ij} = \begin{cases} -e_{7(j+m)+5} \otimes e_{7j+5}, & i = j+4s; \\ 0, & \text{otherwise.} \end{cases}$$

If  $6s \leq j < 7s$ , then

$$b_{ij} = \begin{cases} -e_{7(j+m)+6} \otimes e_{7j+6}, & i = j+4s; \\ 0, & \text{otherwise.} \end{cases}$$

(8) If  $r_0 = 7$ , then  $\Omega^7(Y_t^{(12)})$  is described with  $(12s \times 7s)$ -matrix with the following elements  $b_{ij}$ :

If  $0 \leq j < s$ , then

$$b_{ij} = \begin{cases} -w_{7(j+m)+5 \rightarrow 7(j+m+1)} \otimes e_{7j}, & i = j + s; \\ w_{7(j+m)+4 \rightarrow 7(j+m+1)} \otimes e_{7j}, & i = j + 2s; \\ -e_{7(j+m+1)} \otimes w_{7j \rightarrow 7j+1}, & i = j + 3s; \\ w_{7(j+m)+6 \rightarrow 7(j+m+1)} \otimes w_{7j \rightarrow 7j+2}, & i = j + 4s; \\ 0, & \text{otherwise.} \end{cases}$$

If  $s \leq j < 2s$ , then

$$b_{ij} = \begin{cases} -w_{7(j+m+1) \rightarrow 7(j+m+1)+1} \otimes e_{7j+1}, & i = j + 2s; \\ w_{7(j+m)+6 \rightarrow 7(j+m+1)+1} \otimes w_{7j+1 \rightarrow 7j+2}, & i = j + 3s; \\ 0, & \text{otherwise.} \end{cases}$$

If  $2s \leq j < 3s$ , then

$$b_{ij} = \begin{cases} e_{7(j+m+1)+2} \otimes w_{7j+2 \rightarrow 7(j+1)}, & i = (j+1)_s; \\ w_{7(j+m)+6 \rightarrow 7(j+m+1)+2} \otimes e_{7j+2}, & i = j + 2s; \\ 0, & \text{otherwise.} \end{cases}$$

If  $3s \leq j < 4s$ , then

$$b_{ij} = \begin{cases} w_{7(j+m+1)+2 \rightarrow 7(j+m+1)+3} \otimes w_{7j+3 \rightarrow 7(j+1)}, & i = (j+1)_s; \\ e_{7(j+m+1)+3} \otimes w_{7j+3 \rightarrow 7j+6}, & i = j + 7s; \\ 0, & \text{otherwise.} \end{cases}$$

If  $4s \leq j < 5s$ , then

$$b_{ij} = \begin{cases} e_{7(j+m+1)+4} \otimes w_{7j+4 \rightarrow 7(j+1)}, & i = 2s + (j+1)_s; \\ w_{7(j+m)+6 \rightarrow 7(j+m+1)+4} \otimes e_{7j+4}, & i = j + 2s; \\ -w_{7(j+m)+6 \rightarrow 7(j+m+1)+4} \otimes w_{7j+4 \rightarrow 7j+5}, & i = j + 3s; \\ 0, & \text{otherwise.} \end{cases}$$

If  $5s \leq j < 6s$ , then

$$b_{ij} = \begin{cases} -e_{7(j+m+1)+5} \otimes w_{7j+5 \rightarrow 7(j+1)}, & i = s + (j+1)_s; \\ w_{7(j+m+1)+4 \rightarrow 7(j+m+1)+5} \otimes w_{7j+5 \rightarrow 7(j+1)}, & i = 2s + (j+1)_s; \\ -w_{7(j+m)+6 \rightarrow 7(j+m+1)+5} \otimes e_{7j+5}, & i = j + 2s; \\ 0, & \text{otherwise.} \end{cases}$$

If  $6s \leq j < 7s$ , then

$$b_{ij} = \begin{cases} -w_{7(j+m+1)+2 \rightarrow 7(j+m+1)+6} \otimes w_{7j+6 \rightarrow 7(j+1)}, & i = (j+1)_s; \\ -w_{7(j+m+1)+5 \rightarrow 7(j+m+1)+6} \otimes w_{7j+6 \rightarrow 7(j+1)}, & i = s + (j+1)_s; \\ -w_{7(j+m+1)+4 \rightarrow 7(j+m+1)+6} \otimes w_{7j+6 \rightarrow 7(j+1)}, & i = 2s + (j+1)_s; \\ e_{7(j+m+1)+6} \otimes w_{7j+6 \rightarrow 7(j+1)+2}, & i = 4s + (j+1)_s; \\ -e_{7(j+m+1)+6} \otimes w_{7j+6 \rightarrow 7(j+1)+4}, & i = 6s + (j+1)_s; \\ w_{7(j+m+1)+3 \rightarrow 7(j+m+1)+6} \otimes e_{7j+6}, & i = j + 4s; \\ 0, & \text{otherwise.} \end{cases}$$

(9) If  $r_0 = 8$ , then  $\Omega^8(Y_t^{(12)})$  is described with  $(13s \times 8s)$ -matrix with the following elements  $b_{ij}$ :

If  $s \leq j < 2s$ , then

$$b_{ij} = \begin{cases} -w_{7(j+m-1)+6 \rightarrow 7(j+m)+4} \otimes e_{7j}, & i = j - s; \\ w_{7(j+m) \rightarrow 7(j+m)+4} \otimes e_{7j}, & i = j; \\ e_{7(j+m)+4} \otimes w_{7j \rightarrow 7j+3}, & i = j + 5s; \\ -e_{7(j+m)+4} \otimes w_{7j \rightarrow 7j+5}, & i = j + 8s; \\ 0, & \text{otherwise.} \end{cases}$$

If  $2s \leq j < 3s$ , then

$$b_{ij} = \begin{cases} -w_{7(j+m)+1 \rightarrow 7(j+m)+2} \otimes e_{7j+1}, & i = j; \\ e_{7(j+m)+2} \otimes w_{7j+1 \rightarrow 7j+2}, & i = j + 2s; \\ 0, & \text{otherwise.} \end{cases}$$

If  $3s \leq j < 4s$ , then

$$b_{ij} = \begin{cases} w_{7(j+m)+2 \rightarrow 7(j+m)+3} \otimes e_{7j+2}, & i = j + s; \\ -e_{7(j+m)+3} \otimes w_{7j+2 \rightarrow 7j+3}, & i = j + 2s; \\ 0, & \text{otherwise.} \end{cases}$$

If  $4s \leq j < 5s$ , then

$$b_{ij} = \begin{cases} -e_{7(j+m)+6} \otimes w_{7j+3 \rightarrow 7(j+1)}, & i = (j + 1)s; \\ 0, & \text{otherwise.} \end{cases}$$

If  $5s \leq j < 6s$ , then

$$b_{ij} = \begin{cases} e_{7(j+m)+5} \otimes e_{7j+4}, & i = j + 3s; \\ 0, & \text{otherwise.} \end{cases}$$

If  $6s \leq j < 7s$ , then

$$b_{ij} = \begin{cases} -w_{7(j+m)+4 \rightarrow 7(j+m)+6} \otimes e_{7j+5}, & i = j + 3s; \\ w_{7(j+m)+1 \rightarrow 7(j+m)+6} \otimes e_{7j+5}, & i = j + 4s; \\ e_{7(j+m)+6} \otimes w_{7j+5 \rightarrow 7j+6}, & i = j + 5s; \\ 0, & \text{otherwise.} \end{cases}$$

If  $7s \leq j < 8s$ , then

$$b_{ij} = \begin{cases} e_{7(j+m)+1} \otimes e_{7j+6}, & i = j + 5s; \\ 0, & \text{otherwise.} \end{cases}$$

(10) If  $r_0 = 9$ , then  $\Omega^9(Y_t^{(12)})$  is described with  $(12s \times 7s)$ -matrix with the following elements  $b_{ij}$ :

If  $0 \leq j < s$ , then

$$b_{ij} = \begin{cases} w_{7(j+m)+5 \rightarrow 7(j+m)+6} \otimes e_{7j}, & i = j; \\ w_{7(j+m)+1 \rightarrow 7(j+m)+6} \otimes e_{7j}, & i = j + 2s; \\ e_{7(j+m)+6} \otimes w_{7j \rightarrow 7j+1}, & i = j + 3s; \\ -e_{7(j+m)+6} \otimes w_{7j \rightarrow 7j+3}, & i = j + 5s; \\ 0, & \text{otherwise.} \end{cases}$$

If  $s \leq j < 2s$ , then

$$b_{ij} = \begin{cases} -w_{7(j+m+1)+1 \rightarrow 7(j+m+1)+2} \otimes w_{7j+1 \rightarrow 7(j+1)}, & i = 2s + (j + 1)_s; \\ -w_{7(j+m)+6 \rightarrow 7(j+m+1)+2} \otimes e_{7j+1}, & i = j + 2s; \\ w_{7(j+m+1) \rightarrow 7(j+m+1)+2} \otimes w_{7j+1 \rightarrow 7j+2}, & i = j + 3s; \\ 0, & \text{otherwise.} \end{cases}$$

If  $2s \leq j < 3s$ , then

$$b_{ij} = \begin{cases} e_{7(j+m+1)+3} \otimes w_{7j+2 \rightarrow 7(j+1)}, & i = s + (j + 1)_s; \\ -w_{7(j+m+1)+1 \rightarrow 7(j+m+1)+3} \otimes w_{7j+2 \rightarrow 7(j+1)}, & i = 2s + (j + 1)_s; \\ w_{7(j+m+1) \rightarrow 7(j+m+1)+3} \otimes e_{7j+2}, & i = j + 2s; \\ 0, & \text{otherwise.} \end{cases}$$

If  $3s \leq j < 4s$ , then

$$b_{ij} = \begin{cases} e_{7(j+m+1)+4} \otimes w_{7j+3 \rightarrow 7j+6}, & i = j + 8s; \\ 0, & \text{otherwise.} \end{cases}$$

If  $4s \leq j < 5s$ , then

$$b_{ij} = \begin{cases} -e_{7(j+m+1)+5} \otimes w_{7j+4 \rightarrow 7(j+1)}, & i = (j + 1)_s; \\ w_{7(j+m+1) \rightarrow 7(j+m+1)+5} \otimes e_{7j+4}, & i = j + 3s; \\ -w_{7(j+m+1) \rightarrow 7(j+m+1)+5} \otimes w_{7j+4 \rightarrow 7j+5}, & i = j + 4s; \\ 0, & \text{otherwise.} \end{cases}$$

If  $5s \leq j < 6s$ , then

$$b_{ij} = \begin{cases} -w_{7(j+m+1) \rightarrow 7(j+m+1)+1} \otimes e_{7j+5}, & i = j + 3s; \\ 0, & \text{otherwise.} \end{cases}$$

If  $6s \leq j < 7s$ , then

$$b_{ij} = \begin{cases} e_{7(j+m+2)} \otimes w_{7j+6 \rightarrow 7(j+1)+2}, & i = 4s + (j + 1)_s; \\ w_{7(j+m+1)+2 \rightarrow 7(j+m+2)} \otimes e_{7j+6}, & i = j + 3s; \\ 0, & \text{otherwise.} \end{cases}$$

(11) If  $r_0 = 10$ , then  $\Omega^{10}(Y_t^{(12)})$  is described with  $(12s \times 9s)$ -matrix with the following elements  $b_{ij}$ :



If  $0 \leq j < s$ , then

$$b_{ij} = \begin{cases} -w_{7(j+m-1)+6 \rightarrow 7(j+m)+2} \otimes e_{7j}, & i = j; \\ -w_{7(j+m) \rightarrow 7(j+m)+2} \otimes e_{7j}, & i = j + s; \\ w_{7(j+m)+1 \rightarrow 7(j+m)+2} \otimes w_{7j \rightarrow 7j+4}, & i = j + 7s; \\ 0, & \text{otherwise.} \end{cases}$$

If  $s \leq j < 2s$ , then

$$b_{ij} = \begin{cases} w_{7(j+m-1)+6 \rightarrow 7(j+m)+5} \otimes e_{7j}, & i = j - s; \\ w_{7(j+m) \rightarrow 7(j+m)+5} \otimes e_{7j}, & i = j; \\ -w_{7(j+m)+4 \rightarrow 7(j+m)+5} \otimes w_{7j \rightarrow 7j+2}, & i = j + 3s; \\ e_{7(j+m)+5} \otimes w_{7j \rightarrow 7j+3}, & i = j + 4s; \\ e_{7(j+m)+5} \otimes w_{7j \rightarrow 7j+5}, & i = j + 8s; \\ 0, & \text{otherwise.} \end{cases}$$

If  $2s \leq j < 3s$ , then

$$b_{ij} = \begin{cases} -w_{7(j+m)+2 \rightarrow 7(j+m)+3} \otimes e_{7j+1}, & i = j; \\ e_{7(j+m)+3} \otimes w_{7j+1 \rightarrow 7j+2}, & i = j + s; \\ 0, & \text{otherwise.} \end{cases}$$

If  $3s \leq j < 4s$ , then

$$b_{ij} = \begin{cases} -e_{7(j+m)+6} \otimes w_{7j+2 \rightarrow 7(j+1)}, & i = (j + 1)s; \\ w_{7(j+m)+4 \rightarrow 7(j+m)+6} \otimes e_{7j+2}, & i = j + s; \\ 0, & \text{otherwise.} \end{cases}$$

If  $4s \leq j < 5s$ , then

$$b_{ij} = \begin{cases} -w_{7(j+m)+6 \rightarrow 7(j+m+1)} \otimes w_{7j+3 \rightarrow 7(j+1)}, & i = (j + 1)s; \\ -e_{7(j+m+1)} \otimes w_{7j+3 \rightarrow 7(j+1)}, & i = s + (j + 1)s; \\ w_{7(j+m)+5 \rightarrow 7(j+m+1)} \otimes e_{7j+3}, & i = j + s; \\ -w_{7(j+m)+6 \rightarrow 7(j+m+1)} \otimes w_{7j+3 \rightarrow 7j+6}, & i = j + 6s; \\ 0, & \text{otherwise.} \end{cases}$$

If  $5s \leq j < 6s$ , then

$$b_{ij} = \begin{cases} w_{7(j+m)+1 \rightarrow 7(j+m)+6} \otimes e_{7j+4}, & i = j + 2s; \\ 0, & \text{otherwise.} \end{cases}$$

If  $6s \leq j < 7s$ , then

$$b_{ij} = \begin{cases} -w_{7(j+m)+2 \rightarrow 7(j+m+1)} \otimes e_{7j+5}, & i = j + 2s; \\ 0, & \text{otherwise.} \end{cases}$$

If  $7s \leq j < 8s$ , then

$$b_{ij} = \begin{cases} w_{7(j+m)+6 \rightarrow 7(j+m+1)+1} \otimes w_{7j+6 \rightarrow 7(j+1)}, & i = (j+1)_s; \\ w_{7(j+m+1) \rightarrow 7(j+m+1)+1} \otimes w_{7j+6 \rightarrow 7(j+1)}, & i = s + (j+1)_s; \\ -e_{7(j+m+1)+1} \otimes w_{7j+6 \rightarrow 7(j+1)+4}, & i = 7s + (j+1)_s; \\ w_{7(j+m)+6 \rightarrow 7(j+m+1)+1} \otimes e_{7j+6}, & i = j + 3s; \\ 0, & \text{otherwise.} \end{cases}$$

If  $8s \leq j < 9s$ , then

$$b_{ij} = \begin{cases} e_{7(j+m+1)+4} \otimes w_{7j+6 \rightarrow 7(j+1)+2}, & i = 4s + (j+1)_s; \\ 0, & \text{otherwise.} \end{cases}$$

(12) If  $r_0 = 11$ , then  $\Omega^{11}(Y_t^{(12)})$  is described with  $(10s \times 10s)$ -matrix with the following elements  $b_{ij}$ :

If  $0 \leq j < s$ , then

$$b_{ij} = \begin{cases} w_{7(j+m)+2 \rightarrow 7(j+m)+6} \otimes e_{7j}, & i = j; \\ e_{7(j+m)+6} \otimes w_{7j \rightarrow 7j+2}, & i = j + 3s; \\ e_{7(j+m)+6} \otimes w_{7j \rightarrow 7j+5}, & i = j + 6s; \\ 0, & \text{otherwise.} \end{cases}$$

If  $s \leq j < 2s$ , then

$$b_{ij} = \begin{cases} -w_{7(j+m)+2 \rightarrow 7(j+m+1)} \otimes e_{7j}, & i = j - s; \\ -w_{7(j+m)+4 \rightarrow 7(j+m+1)} \otimes e_{7j}, & i = j; \\ -e_{7(j+m+1)} \otimes w_{7j \rightarrow 7j+1}, & i = j + s; \\ -w_{7(j+m)+6 \rightarrow 7(j+m+1)} \otimes w_{7j \rightarrow 7j+2}, & i = j + 2s; \\ e_{7(j+m+1)} \otimes w_{7j \rightarrow 7j+3}, & i = j + 3s; \\ -e_{7(j+m+1)} \otimes w_{7j \rightarrow 7j+4}, & i = j + 4s; \\ 0, & \text{otherwise.} \end{cases}$$

If  $2s \leq j < 3s$ , then

$$b_{ij} = \begin{cases} w_{7(j+m+1)+2 \rightarrow 7(j+m+1)+3} \otimes w_{7j+1 \rightarrow 7(j+1)}, & i = (j+1)_s; \\ -w_{7(j+m+1) \rightarrow 7(j+m+1)+3} \otimes e_{7j+1}, & i = j; \\ 0, & \text{otherwise.} \end{cases}$$

If  $3s \leq j < 4s$ , then

$$b_{ij} = \begin{cases} -e_{7(j+m+1)+4} \otimes w_{7j+2 \rightarrow 7(j+1)}, & i = s + (j+1)_s; \\ -w_{7(j+m)+6 \rightarrow 7(j+m+1)+4} \otimes e_{7j+2}, & i = j; \\ 0, & \text{otherwise.} \end{cases}$$

If  $4s \leq j < 5s$ , then  $b_{ij} = 0$ .

If  $5s \leq j < 6s$ , then

$$b_{ij} = \begin{cases} w_{7(j+m+1) \rightarrow 7(j+m+1)+5} \otimes e_{7j+3}, & i = j - s; \\ -e_{7(j+m+1)+5} \otimes w_{7j+3 \rightarrow 7j+6}, & i = j + 2s; \\ 0, & \text{otherwise.} \end{cases}$$

If  $6s \leq j < 7s$ , then

$$b_{ij} = \begin{cases} -w_{7(j+m+1) \rightarrow 7(j+m+1)+1} \otimes e_{7j+4}, & i = j - s; \\ -w_{7(j+m)+6 \rightarrow 7(j+m+1)+1} \otimes w_{7j+4 \rightarrow 7j+5}, & i = j; \\ e_{7(j+m+1)+1} \otimes w_{7j+4 \rightarrow 7j+6}, & i = j + 3s; \\ 0, & \text{otherwise.} \end{cases}$$

If  $7s \leq j < 8s$ , then

$$b_{ij} = \begin{cases} -w_{7(j+m)+6 \rightarrow 7(j+m+1)+2} \otimes e_{7j+5}, & i = j - s; \\ 0, & \text{otherwise.} \end{cases}$$

If  $8s \leq j < 9s$ , then  $b_{ij} = 0$ .

If  $9s \leq j < 10s$ , then

$$b_{ij} = \begin{cases} w_{7(j+m+1)+3 \rightarrow 7(j+m+1)+6} \otimes e_{7j+6}, & i = j - s; \\ 0, & \text{otherwise.} \end{cases}$$

(13) If  $r_0 = 12$ , then  $\Omega^{12}(Y_t^{(12)})$  is described with  $(10s \times 10s)$ -matrix with the following elements  $b_{ij}$ :

If  $0 \leq j < s$ , then

$$b_{ij} = \begin{cases} w_{7(j+m) \rightarrow 7(j+m)+4} \otimes e_{7j}, & i = j; \\ e_{7(j+m)+4} \otimes w_{7j \rightarrow 7j+1}, & i = j + 2s; \\ 0, & \text{otherwise.} \end{cases}$$

If  $s \leq j < 2s$ , then

$$b_{ij} = \begin{cases} w_{7(j+m) \rightarrow 7(j+m)+3} \otimes e_{7j}, & i = j - s; \\ -w_{7(j+m)+1 \rightarrow 7(j+m)+3} \otimes w_{7j \rightarrow 7j+3}, & i = j + 3s; \\ -w_{7(j+m)+2 \rightarrow 7(j+m)+3} \otimes w_{7j \rightarrow 7j+4}, & i = j + 4s; \\ 0, & \text{otherwise.} \end{cases}$$

If  $2s \leq j < 3s$ , then

$$b_{ij} = \begin{cases} -w_{7(j+m) \rightarrow 7(j+m)+1} \otimes e_{7j}, & i = j - 2s; \\ -e_{7(j+m)+1} \otimes w_{7j \rightarrow 7j+3}, & i = j + 2s; \\ 0, & \text{otherwise.} \end{cases}$$

If  $3s \leq j < 4s$ , then

$$b_{ij} = \begin{cases} -w_{7(j+m)+4 \rightarrow 7(j+m)+6} \otimes e_{7j+1}, & i = j - s; \\ w_{7(j+m)+5 \rightarrow 7(j+m)+6} \otimes w_{7j+1 \rightarrow 7j+2}, & i = j; \\ 0, & \text{otherwise.} \end{cases}$$

If  $4s \leq j < 5s$ , then

$$b_{ij} = \begin{cases} e_{7(j+m+1)} \otimes w_{7j+2 \rightarrow 7(j+1)}, & i = (j+1)_s; \\ -w_{7(j+m)+5 \rightarrow 7(j+m+1)} \otimes e_{7j+2}, & i = j - s; \\ 0, & \text{otherwise.} \end{cases}$$

If  $5s \leq j < 6s$ , then

$$b_{ij} = \begin{cases} -w_{7(j+m)+1 \rightarrow 7(j+m)+6} \otimes e_{7j+3}, & i = j - s; \\ e_{7(j+m)+6} \otimes w_{7j+3 \rightarrow 7j+6}, & i = j + 3s; \\ 0, & \text{otherwise.} \end{cases}$$

If  $6s \leq j < 7s$ , then

$$b_{ij} = \begin{cases} e_{7(j+m+1)} \otimes w_{7j+4 \rightarrow 7(j+1)}, & i = (j+1)_s; \\ -w_{7(j+m)+2 \rightarrow 7(j+m+1)} \otimes e_{7j+4}, & i = j - s; \\ 0, & \text{otherwise.} \end{cases}$$

If  $7s \leq j < 8s$ , then

$$b_{ij} = \begin{cases} -w_{7(j+m)+3 \rightarrow 7(j+m)+6} \otimes e_{7j+5}, & i = j; \\ 0, & \text{otherwise.} \end{cases}$$

If  $8s \leq j < 9s$ , then

$$b_{ij} = \begin{cases} w_{7(j+m+1) \rightarrow 7(j+m+1)+2} \otimes w_{7j+6 \rightarrow 7(j+1)}, & i = (j+1)_s; \\ w_{7(j+m+1)+1 \rightarrow 7(j+m+1)+2} \otimes w_{7j+6 \rightarrow 7(j+1)+3}, & i = 4s + (j+1)_s; \\ -e_{7(j+m+1)+2} \otimes w_{7j+6 \rightarrow 7(j+1)+4}, & i = 5s + (j+1)_s; \\ -w_{7(j+m)+6 \rightarrow 7(j+m+1)+2} \otimes e_{7j+6}, & i = j; \\ 0, & \text{otherwise.} \end{cases}$$

If  $9s \leq j < 10s$ , then

$$b_{ij} = \begin{cases} e_{7(j+m+1)+5} \otimes w_{7j+6 \rightarrow 7(j+1)+2}, & i = 3s + (j+1)_s; \\ 0, & \text{otherwise.} \end{cases}$$

(14) If  $r_0 = 13$ , then  $\Omega^{13}(Y_t^{(12)})$  is described with  $(9s \times 12s)$ -matrix with the following elements  $b_{ij}$ :

If  $0 \leq j < s$ , then

$$b_{ij} = \begin{cases} w_{7(j+m)+3 \rightarrow 7(j+m)+6} \otimes e_{7j}, & i = j; \\ e_{7(j+m)+6} \otimes w_{7j \rightarrow 7j+1}, & i = j + 2s; \\ 0, & \text{otherwise.} \end{cases}$$

If  $s \leq j < 2s$ , then

$$b_{ij} = \begin{cases} w_{7(j+m)+3 \rightarrow 7(j+m+1)} \otimes e_{7j}, & i = j - s; \\ w_{7(j+m)+6 \rightarrow 7(j+m+1)} \otimes w_{7j \rightarrow 7j+1}, & i = j + s; \\ e_{7(j+m+1)} \otimes w_{7j \rightarrow 7j+2}, & i = j + 2s; \\ e_{7(j+m+1)} \otimes w_{7j \rightarrow 7j+5}, & i = j + 5s; \\ 0, & \text{otherwise.} \end{cases}$$

If  $2s \leq j < 3s$ , then

$$b_{ij} = \begin{cases} w_{7(j+m)+6 \rightarrow 7(j+m+1)+4} \otimes e_{7j+1}, & i = j; \\ w_{7(j+m+1) \rightarrow 7(j+m+1)+4} \otimes w_{7j+1 \rightarrow 7j+2}, & i = j + s; \\ -e_{7(j+m+1)+4} \otimes w_{7j+1 \rightarrow 7j+6}, & i = j + 6s; \\ 0, & \text{otherwise.} \end{cases}$$

If  $3s \leq j < 4s$ , then  $b_{ij} = 0$ .

If  $4s \leq j < 5s$ , then

$$b_{ij} = \begin{cases} e_{7(j+m+1)+5} \otimes w_{7j+2 \rightarrow 7(j+1)}, & i = s + (j+1)s; \\ -w_{7(j+m+1) \rightarrow 7(j+m+1)+5} \otimes e_{7j+2}, & i = j - s; \\ w_{7(j+m+1)+4 \rightarrow 7(j+m+1)+5} \otimes w_{7j+2 \rightarrow 7j+6}, & i = j + 4s; \\ 0, & \text{otherwise.} \end{cases}$$

If  $5s \leq j < 6s$ , then  $b_{ij} = 0$ .

If  $6s \leq j < 7s$ , then

$$b_{ij} = \begin{cases} -w_{7(j+m)+6 \rightarrow 7(j+m+1)+2} \otimes e_{7j+4}, & i = j - s; \\ w_{7(j+m+1) \rightarrow 7(j+m+1)+2} \otimes w_{7j+4 \rightarrow 7j+5}, & i = j; \\ e_{7(j+m+1)+2} \otimes w_{7j+4 \rightarrow 7j+6}, & i = j + s; \\ 0, & \text{otherwise.} \end{cases}$$

If  $7s \leq j < 8s$ , then  $b_{ij} = 0$ .

If  $8s \leq j < 9s$ , then

$$b_{ij} = \begin{cases} -w_{7(j+m+1) \rightarrow 7(j+m+1)+3} \otimes e_{7j+5}, & i = j - 2s; \\ -w_{7(j+m+1)+2 \rightarrow 7(j+m+1)+3} \otimes w_{7j+5 \rightarrow 7j+6}, & i = j - s; \\ 0, & \text{otherwise.} \end{cases}$$

If  $9s \leq j < 10s$ , then  $b_{ij} = 0$ .

If  $10s \leq j < 11s$ , then

$$b_{ij} = \begin{cases} -w_{7(j+m+1)+2 \rightarrow 7(j+m+1)+6} \otimes e_{7j+6}, & i = j - 3s; \\ w_{7(j+m+1)+4 \rightarrow 7(j+m+1)+6} \otimes e_{7j+6}, & i = j - 2s; \\ 0, & \text{otherwise.} \end{cases}$$

If  $11s \leq j < 12s$ , then  $b_{ij} = 0$ .

(15) If  $r_0 = 14$ , then  $\Omega^{14}(Y_t^{(12)})$  is described with  $(7s \times 12s)$ -matrix with the following elements  $b_{ij}$ :

If  $0 \leq j < s$ , then

$$b_{ij} = \begin{cases} -w_{7(j+m-1)+6 \rightarrow 7(j+m)+2} \otimes e_{7j}, & i = j; \\ w_{7(j+m)+1 \rightarrow 7(j+m)+2} \otimes w_{7j \rightarrow 7j+2}, & i = j + 2s; \\ -e_{7(j+m)+2} \otimes w_{7j \rightarrow 7j+3}, & i = j + 3s; \\ 0, & \text{otherwise.} \end{cases}$$

If  $s \leq j < 2s$ , then

$$b_{ij} = \begin{cases} -e_{7(j+m)+5} \otimes w_{7j \rightarrow 7j+1}, & i = j; \\ 0, & \text{otherwise.} \end{cases}$$

If  $2s \leq j < 3s$ , then

$$b_{ij} = \begin{cases} e_{7(j+m)+4} \otimes w_{7j \rightarrow 7j+5}, & i = j + 3s; \\ 0, & \text{otherwise.} \end{cases}$$

If  $3s \leq j < 4s$ , then

$$b_{ij} = \begin{cases} w_{7(j+m)+6 \rightarrow 7(j+m+1)} \otimes w_{7j+1 \rightarrow 7(j+1)}, & i = (j+1)_s; \\ w_{7(j+m)+5 \rightarrow 7(j+m+1)} \otimes e_{7j+1}, & i = j - 2s; \\ 0, & \text{otherwise.} \end{cases}$$

If  $4s \leq j < 5s$ , then

$$b_{ij} = \begin{cases} e_{7(j+m)+6} \otimes w_{7j+2 \rightarrow 7(j+1)}, & i = (j+1)_s; \\ w_{7(j+m)+1 \rightarrow 7(j+m)+6} \otimes e_{7j+2}, & i = j - 2s; \\ -w_{7(j+m)+2 \rightarrow 7(j+m)+6} \otimes w_{7j+2 \rightarrow 7j+3}, & i = j - s; \\ 0, & \text{otherwise.} \end{cases}$$

If  $5s \leq j < 6s$ , then

$$b_{ij} = \begin{cases} e_{7(j+m+1)} \otimes w_{7j+3 \rightarrow 7j+6}, & i = j + s; \\ 0, & \text{otherwise.} \end{cases}$$

If  $6s \leq j < 7s$ , then

$$b_{ij} = \begin{cases} -w_{7(j+m)+3 \rightarrow 7(j+m)+6} \otimes e_{7j+4}, & i = j - 2s; \\ 0, & \text{otherwise.} \end{cases}$$

If  $7s \leq j < 8s$ , then

$$b_{ij} = \begin{cases} -w_{7(j+m)+4 \rightarrow 7(j+m)+6} \otimes e_{7j+5}, & i = j - 2s; \\ 0, & \text{otherwise.} \end{cases}$$

If  $8s \leq j < 9s$ , then  $b_{ij} = 0$ .

If  $9s \leq j < 10s$ , then

$$b_{ij} = \begin{cases} e_{7(j+m+1)+4} \otimes w_{7j+6 \rightarrow 7(j+1)+5}, & i = 5s + (j+1)_s; \\ -w_{7(j+m+1) \rightarrow 7(j+m+1)+4} \otimes e_{7j+6}, & i = j - 3s; \\ 0, & \text{otherwise.} \end{cases}$$

If  $10s \leq j < 11s$ , then

$$b_{ij} = \begin{cases} w_{7(j+m)+6 \rightarrow 7(j+m+1)+3} \otimes w_{7j+6 \rightarrow 7(j+1)}, & i = (j+1)_s; \\ e_{7(j+m+1)+3} \otimes w_{7j+6 \rightarrow 7(j+1)+4}, & i = 4s + (j+1)_s; \\ 0, & \text{otherwise.} \end{cases}$$

If  $11s \leq j < 12s$ , then  $b_{ij} = 0$ .

(16) If  $r_0 = 15$ , then  $\Omega^{15}(Y_t^{(12)})$  is described with  $(8s \times 13s)$ -matrix with the following elements  $b_{ij}$ :

If  $0 \leq j < s$ , then

$$b_{ij} = \begin{cases} -e_{7(j+m)+6} \otimes e_{7j}, & i = j; \\ 0, & \text{otherwise.} \end{cases}$$

If  $s \leq j < 2s$ , then

$$b_{ij} = \begin{cases} e_{7(j+m+1)} \otimes w_{7j \rightarrow 7j+1}, & i = j; \\ 0, & \text{otherwise.} \end{cases}$$

If  $2s \leq j < 3s$ , then

$$b_{ij} = \begin{cases} -w_{7(j+m+1) \rightarrow 7(j+m+1)+1} \otimes e_{7j+1}, & i = j - s; \\ 0, & \text{otherwise.} \end{cases}$$

If  $3s \leq j < 4s$ , then

$$b_{ij} = \begin{cases} w_{7(j+m+1) \rightarrow 7(j+m+1)+5} \otimes e_{7j+1}, & i = j - 2s; \\ e_{7(j+m+1)+5} \otimes w_{7j+1 \rightarrow 7j+6}, & i = j + 4s; \\ 0, & \text{otherwise.} \end{cases}$$

If  $4s \leq j < 5s$ , then

$$b_{ij} = \begin{cases} w_{7(j+m+1)+1 \rightarrow 7(j+m+1)+2} \otimes e_{7j+2}, & i = j - 2s; \\ 0, & \text{otherwise.} \end{cases}$$

If  $5s \leq j < 6s$ , then

$$b_{ij} = \begin{cases} -w_{7(j+m+1)+2 \rightarrow 7(j+m+1)+3} \otimes e_{7j+3}, & i = j - 2s; \\ 0, & \text{otherwise.} \end{cases}$$

If  $6s \leq j < 7s$ , then  $b_{ij} = 0$ .

If  $7s \leq j < 8s$ , then

$$b_{ij} = \begin{cases} -w_{7(j+m+1) \rightarrow 7(j+m+1)+3} \otimes e_{7j+4}, & i = j - 3s; \\ -e_{7(j+m+1)+3} \otimes w_{7j+4 \rightarrow 7j+6}, & i = j - s; \\ 0, & \text{otherwise.} \end{cases}$$

If  $8s \leq j < 9s$ , then  $b_{ij} = 0$ .

If  $9s \leq j < 10s$ , then

$$b_{ij} = \begin{cases} -e_{7(j+m+1)+4} \otimes e_{7j+5}, & i = j - 4s; \\ 0, & \text{otherwise.} \end{cases}$$

If  $10s \leq j < 11s$ , then  $b_{ij} = 0$ .

If  $11s \leq j < 12s$ , then

$$b_{ij} = \begin{cases} -w_{7(j+m+1)+3 \rightarrow 7(j+m+1)+6} \otimes e_{7j+6}, & i = j - 5s; \\ 0, & \text{otherwise.} \end{cases}$$

If  $12s \leq j < 13s$ , then

$$b_{ij} = \begin{cases} -w_{7(j+m+1)+6 \rightarrow 7(j+m+2)} \otimes w_{7j+6 \rightarrow 7(j+1)}, & i = (j+1)s; \\ 0, & \text{otherwise.} \end{cases}$$

(17) If  $r_0 = 16$ , then  $\Omega^{16}(Y_t^{(12)})$  is described with  $(7s \times 12s)$ -matrix with the following elements  $b_{ij}$ :

If  $0 \leq j < s$ , then

$$b_{ij} = \begin{cases} -w_{7(j+m) \rightarrow 7(j+m)+5} \otimes e_{7j}, & i = j; \\ -w_{7(j+m)+4 \rightarrow 7(j+m)+5} \otimes w_{7j \rightarrow 7j+4}, & i = j + 4s; \\ -e_{7(j+m)+5} \otimes w_{7j \rightarrow 7j+5}, & i = j + 5s; \\ 0, & \text{otherwise.} \end{cases}$$

If  $s \leq j < 2s$ , then

$$b_{ij} = \begin{cases} -w_{7(j+m) \rightarrow 7(j+m)+3} \otimes e_{7j}, & i = j - s; \\ w_{7(j+m)+1 \rightarrow 7(j+m)+3} \otimes w_{7j \rightarrow 7j+1}, & i = j; \\ w_{7(j+m)+2 \rightarrow 7(j+m)+3} \otimes w_{7j \rightarrow 7j+2}, & i = j + s; \\ e_{7(j+m)+3} \otimes w_{7j \rightarrow 7j+3}, & i = j + 2s; \\ 0, & \text{otherwise.} \end{cases}$$

If  $2s \leq j < 3s$ , then  $b_{ij} = 0$ .

If  $3s \leq j < 4s$ , then

$$b_{ij} = \begin{cases} w_{7(j+m)+1 \rightarrow 7(j+m)+6} \otimes e_{7j+1}, & i = j - 2s; \\ w_{7(j+m)+2 \rightarrow 7(j+m)+6} \otimes w_{7j+1 \rightarrow 7j+2}, & i = j - s; \\ -w_{7(j+m)+3 \rightarrow 7(j+m)+6} \otimes w_{7j+1 \rightarrow 7j+3}, & i = j; \\ e_{7(j+m)+6} \otimes w_{7j+1 \rightarrow 7j+6}, & i = j + 3s; \\ 0, & \text{otherwise.} \end{cases}$$

If  $4s \leq j < 5s$ , then

$$b_{ij} = \begin{cases} e_{7(j+m)+1} \otimes w_{7j+2 \rightarrow 7(j+1)}, & i = (j+1)_s; \\ w_{7(j+m)+2 \rightarrow 7(j+m)+1} \otimes e_{7j+2}, & i = j - 2s; \\ 0, & \text{otherwise.} \end{cases}$$

If  $5s \leq j < 6s$ , then

$$b_{ij} = \begin{cases} -w_{7(j+m)+3 \rightarrow 7(j+m)+6} \otimes e_{7j+3}, & i = j - 2s; \\ 0, & \text{otherwise.} \end{cases}$$

If  $6s \leq j < 7s$ , then

$$b_{ij} = \begin{cases} -w_{7(j+m)+4 \rightarrow 7(j+m)+6} \otimes e_{7j+4}, & i = j - 2s; \\ -w_{7(j+m)+5 \rightarrow 7(j+m)+6} \otimes w_{7j+4 \rightarrow 7j+5}, & i = j - s; \\ e_{7(j+m)+6} \otimes w_{7j+4 \rightarrow 7j+6}, & i = j; \\ 0, & \text{otherwise.} \end{cases}$$

If  $7s \leq j < 8s$ , then  $b_{ij} = 0$ .

If  $8s \leq j < 9s$ , then

$$b_{ij} = \begin{cases} -w_{7(j+m)+5 \rightarrow 7(j+m)+1} \otimes e_{7j+5}, & i = j - 3s; \\ w_{7(j+m)+6 \rightarrow 7(j+m)+1} \otimes w_{7j+5 \rightarrow 7j+6}, & i = j - 2s; \\ 0, & \text{otherwise.} \end{cases}$$



If  $9s \leq j < 10s$ , then

$$b_{ij} = \begin{cases} w_{7(j+m+1)+1 \rightarrow 7(j+m+1)+2} \otimes w_{7j+6 \rightarrow 7(j+1)+1}, & i = s + (j+1)_s; \\ -w_{7(j+m)+6 \rightarrow 7(j+m+1)+2} \otimes e_{7j+6}, & i = j - 3s; \\ 0, & \text{otherwise.} \end{cases}$$

If  $10s \leq j < 11s$ , then  $b_{ij} = 0$ .

If  $11s \leq j < 12s$ , then

$$b_{ij} = \begin{cases} w_{7(j+m+1) \rightarrow 7(j+m+1)+4} \otimes w_{7j+6 \rightarrow 7(j+1)}, & i = (j+1)_s; \\ e_{7(j+m+1)+4} \otimes w_{7j+6 \rightarrow 7(j+1)+4}, & i = 4s + (j+1)_s; \\ 0, & \text{otherwise.} \end{cases}$$

(II) Represent an arbitrary  $t_0 \in \mathbb{N}$  in the form  $t_0 = 17\ell_0 + r_0$ , where  $0 \leq r_0 \leq 16$ . Then  $\Omega^{t_0}(Y_t^{(12)})$  is a  $\Omega^{r_0}(Y_t^{(12)})$ , whose left components twisted by  $\sigma^{\ell_0}$ , and coefficients multiplied by  $(-1)^{\ell_0}$ .

**Proposition 10** (Translates for the case 13). (I) Let  $r_0 \in \mathbb{N}$ ,  $r_0 < 17$ .  $r_0$ -translates of the elements  $Y_t^{(13)}$  are described by the following way.

(1) If  $r_0 = 0$ , then  $\Omega^0(Y_t^{(13)})$  is described with  $(7s \times 10s)$ -matrix with the following two nonzero elements:

$$\begin{aligned} b_{j-s, 2s+(3)_s} &= w_{7(j+m)+1 \rightarrow 7(j+m+1)} \otimes e_{7j+1}; \\ b_{j-s, 5s+(3)_s} &= w_{7(j+m)+4 \rightarrow 7(j+m+1)} \otimes e_{7j+4}. \end{aligned}$$

(2) If  $r_0 = 1$ , then  $\Omega^1(Y_t^{(13)})$  is described with  $(8s \times 10s)$ -matrix with the following nonzero elements:

$$\begin{aligned} b_{j, (3)_s} &= -w_{7(j+m)+1 \rightarrow 7(j+m+1)} \otimes e_{7j}; \\ b_{j+s, (3)_s} &= w_{7(j+m)+4 \rightarrow 7(j+m+1)} \otimes e_{7j}; \\ b_{(j+1)_s, 9s+(2)_s} &= -w_{7(j+m+1)+1 \rightarrow 7(j+m+2)} \otimes w_{7j+6 \rightarrow 7(j+1)}; \\ b_{j-2s, 9s+(2)_s} &= -w_{7(j+m+1) \rightarrow 7(j+m+2)} \otimes e_{7j+6}. \end{aligned}$$

(3) If  $r_0 = 2$ , then  $\Omega^2(Y_t^{(13)})$  is described with  $(7s \times 9s)$ -matrix with the following nonzero elements:

$$\begin{aligned} b_{(j+1)_s, 3s+(2)_s} &= w_{7(j+m)+6 \rightarrow 7(j+m+1)} \otimes w_{7j+2 \rightarrow 7(j+1)}; \\ b_{j-s, 3s+(2)_s} &= -w_{7(j+m)+3 \rightarrow 7(j+m+1)} \otimes e_{7j+2}; \\ b_{j-s, 6s+(2)_s} &= w_{7(j+m)+1 \rightarrow 7(j+m+1)} \otimes e_{7j+5}. \end{aligned}$$

(4) If  $r_0 = 3$ , then  $\Omega^3(Y_t^{(13)})$  is described with  $(9s \times 7s)$ -matrix with the following nonzero elements:

$$\begin{aligned} b_{s+(j+1)_s, s+(2)_s} &= -e_{7(j+m+1)+5} \otimes w_{7j+1 \rightarrow 7(j+1)}; \\ b_{j+s, 2s+(2)_s} &= w_{7(j+m)+6 \rightarrow 7(j+m+1)+1} \otimes e_{7j+2}; \\ b_{(j+1)_s, 6s+(1)_s} &= w_{7(j+m+1)+2 \rightarrow 7(j+m+2)} \otimes w_{7j+6 \rightarrow 7(j+1)}; \\ b_{2s+(j+1)_s, 6s+(1)_s} &= w_{7(j+m+1)+3 \rightarrow 7(j+m+2)} \otimes w_{7j+6 \rightarrow 7(j+1)+1}. \end{aligned}$$

(5) If  $r_0 = 4$ , then  $\Omega^4(Y_t^{(13)})$  is described with  $(10s \times 8s)$ -matrix with the following nonzero elements:

$$\begin{aligned} b_{(j+1)_s, (2)_s} &= e_{7(j+m)+6} \otimes w_{7j \rightarrow 7(j+1)}; \\ b_{j+2s, (2)_s} &= -w_{7(j+m)+3 \rightarrow 7(j+m)+6} \otimes w_{7j \rightarrow 7j+1}; \end{aligned}$$

$$\begin{aligned}
b_{(j+1)s, s+(1)s} &= -w_{7(j+m)+6 \rightarrow 7(j+m+1)} \otimes w_{7j+1 \rightarrow 7(j+1)}; \\
b_{s+(j+1)s, s+(1)s} &= -e_{7(j+m+1)} \otimes w_{7j+1 \rightarrow 7(j+1)}; \\
b_{s+(j+1)s, s+(2)s} &= -e_{7(j+m+1)} \otimes w_{7j+1 \rightarrow 7(j+1)}; \\
b_{(j+1)s, 2s+(1)s} &= -w_{7(j+m)+6 \rightarrow 7(j+m+1)+1} \otimes w_{7j+2 \rightarrow 7(j+1)}; \\
b_{(j+1)s, 3s+(1)s} &= -w_{7(j+m)+6 \rightarrow 7(j+m+1)+2} \otimes w_{7j+3 \rightarrow 7(j+1)}; \\
b_{(j+1)s, 4s+(1)s} &= -w_{7(j+m)+6 \rightarrow 7(j+m+1)} \otimes w_{7j+4 \rightarrow 7(j+1)}; \\
b_{s+(j+1)s, 4s+(1)s} &= -e_{7(j+m+1)} \otimes w_{7j+4 \rightarrow 7(j+1)}; \\
b_{2s+(j+1)s, 6s+(1)s} &= -e_{7(j+m+1)+3} \otimes w_{7j+6 \rightarrow 7(j+1)+1}.
\end{aligned}$$

(6) If  $r_0 = 5$ , then  $\Omega^5(Y_t^{(13)})$  is described with  $(10s \times 7s)$ -matrix with the following nonzero elements:

$$\begin{aligned}
b_{j+3s, (2)s} &= w_{7(j+m)+6 \rightarrow 7(j+m+1)} \otimes w_{7j \rightarrow 7j+1}; \\
b_{j+4s, (2)s} &= e_{7(j+m+1)} \otimes w_{7j \rightarrow 7j+2}; \\
b_{2s+(j+1)s, s+(1)s} &= e_{7(j+m+1)+1} \otimes w_{7j+1 \rightarrow 7(j+1)}; \\
b_{2s+(j+1)s, s+(2)s} &= e_{7(j+m+1)+1} \otimes w_{7j+1 \rightarrow 7(j+1)}; \\
b_{s+(j+1)s, 3s+(1)s} &= e_{7(j+m+1)+3} \otimes w_{7j+3 \rightarrow 7(j+1)}; \\
b_{(j+1)s, 4s+(1)s} &= -e_{7(j+m+1)+4} \otimes w_{7j+4 \rightarrow 7(j+1)}.
\end{aligned}$$

(7) If  $r_0 = 6$ , then  $\Omega^6(Y_t^{(13)})$  is described with  $(12s \times 7s)$ -matrix with the following nonzero elements:

$$\begin{aligned}
b_{(j+1)s, (1)s} &= w_{7(j+m)+6 \rightarrow 7(j+m+1)} \otimes w_{7j \rightarrow 7(j+1)}; \\
b_{(j+1)s, (2)s} &= w_{7(j+m)+6 \rightarrow 7(j+m+1)} \otimes w_{7j \rightarrow 7(j+1)}; \\
b_{s+(j+1)s, (2)s} &= e_{7(j+m+1)} \otimes w_{7j \rightarrow 7(j+1)}; \\
b_{j+2s, (2)s} &= -w_{7(j+m)+4 \rightarrow 7(j+m+1)} \otimes w_{7j \rightarrow 7j+1}; \\
b_{(j+1)s, s+(1)s} &= w_{7(j+m)+6 \rightarrow 7(j+m+1)+1} \otimes w_{7j+1 \rightarrow 7(j+1)}; \\
b_{(j+1)s, s+(2)s} &= w_{7(j+m)+6 \rightarrow 7(j+m+1)+1} \otimes w_{7j+1 \rightarrow 7(j+1)}; \\
b_{s+(j+1)s, s+(2)s} &= w_{7(j+m+1) \rightarrow 7(j+m+1)+1} \otimes w_{7j+1 \rightarrow 7(j+1)}; \\
b_{s+(j+1)s, 2s+(1)s} &= -w_{7(j+m+1) \rightarrow 7(j+m+1)+2} \otimes w_{7j+2 \rightarrow 7(j+1)}; \\
b_{s+(j+1)s, 3s+(1)s} &= -w_{7(j+m+1) \rightarrow 7(j+m+1)+3} \otimes w_{7j+3 \rightarrow 7(j+1)}; \\
b_{(j+1)s, 4s+(1)s} &= w_{7(j+m)+6 \rightarrow 7(j+m+1)+4} \otimes w_{7j+4 \rightarrow 7(j+1)}; \\
b_{2s+(j+1)s, 6s+(1)s} &= -w_{7(j+m+1)+4 \rightarrow 7(j+m+1)+6} \otimes w_{7j+6 \rightarrow 7(j+1)+1}.
\end{aligned}$$

(8) If  $r_0 = 7$ , then  $\Omega^7(Y_t^{(13)})$  is described with  $(12s \times 8s)$ -matrix with the following nonzero elements:

$$\begin{aligned}
b_{j+2s, s+(2)s} &= -w_{7(j+m+1) \rightarrow 7(j+m+1)+4} \otimes w_{7j \rightarrow 7j+1}; \\
b_{(j+1)s, 2s+(1)s} &= e_{7(j+m+1)+2} \otimes w_{7j+1 \rightarrow 7(j+1)}; \\
b_{(j+1)s, 2s+(2)s} &= e_{7(j+m+1)+2} \otimes w_{7j+1 \rightarrow 7(j+1)}; \\
b_{2s+(j+1)s, 4s+(1)s} &= -w_{7(j+m+1)+4 \rightarrow 7(j+m+1)+6} \otimes w_{7j+3 \rightarrow 7(j+1)}; \\
b_{s+(j+1)s, 5s+(1)s} &= e_{7(j+m+1)+5} \otimes w_{7j+4 \rightarrow 7(j+1)}.
\end{aligned}$$

(9) If  $r_0 = 8$ , then  $\Omega^8(Y_t^{(13)})$  is described with  $(13s \times 7s)$ -matrix with the following nonzero elements:

$$\begin{aligned}
b_{(j+1)s, (1)s} &= e_{7(j+m)+6} \otimes w_{7j \rightarrow 7(j+1)}; \\
b_{(j+1)s, (2)s} &= e_{7(j+m)+6} \otimes w_{7j \rightarrow 7(j+1)};
\end{aligned}$$

$$\begin{aligned}
b_{j+3s,(2)_s} &= w_{7(j+m)+5 \rightarrow 7(j+m)+6} \otimes w_{7j \rightarrow 7j+1}; \\
b_{(j+1)_s, s+(1)_s} &= w_{7(j+m)+6 \rightarrow 7(j+m+1)+2} \otimes w_{7j+1 \rightarrow 7(j+1)}; \\
b_{(j+1)_s, s+(2)_s} &= w_{7(j+m)+6 \rightarrow 7(j+m+1)+2} \otimes w_{7j+1 \rightarrow 7(j+1)}; \\
b_{(j+1)_s, 3s+(1)_s} &= w_{7(j+m)+6 \rightarrow 7(j+m+1)+4} \otimes w_{7j+3 \rightarrow 7(j+1)}; \\
b_{s+(j+1)_s, 3s+(1)_s} &= w_{7(j+m+1) \rightarrow 7(j+m+1)+4} \otimes w_{7j+3 \rightarrow 7(j+1)}; \\
b_{6s+(j+1)_s, 3s+(1)_s} &= e_{7(j+m+1)+4} \otimes w_{7j+3 \rightarrow 7(j+1)+3}; \\
b_{s+(j+1)_s, 4s+(1)_s} &= w_{7(j+m+1) \rightarrow 7(j+m+1)+5} \otimes w_{7j+4 \rightarrow 7(j+1)}.
\end{aligned}$$

(10) If  $r_0 = 9$ , then  $\Omega^9(Y_t^{(13)})$  is described with  $(12s \times 9s)$ -matrix with the following nonzero elements:

$$\begin{aligned}
b_{j+2s, s+(2)_s} &= -w_{7(j+m)+6 \rightarrow 7(j+m+1)+5} \otimes w_{7j \rightarrow 7j+1}; \\
b_{s+(j+1)_s, 2s+(1)_s} &= e_{7(j+m+1)+3} \otimes w_{7j+1 \rightarrow 7(j+1)}; \\
b_{s+(j+1)_s, 2s+(2)_s} &= e_{7(j+m+1)+3} \otimes w_{7j+1 \rightarrow 7(j+1)}; \\
b_{(j+1)_s, 3s+(1)_s} &= -w_{7(j+m+1)+5 \rightarrow 7(j+m+1)+6} \otimes w_{7j+2 \rightarrow 7(j+1)}; \\
b_{(j+1)_s, 4s+(1)_s} &= w_{7(j+m+1)+5 \rightarrow 7(j+m+2)} \otimes w_{7j+3 \rightarrow 7(j+1)}; \\
b_{2s+(j+1)_s, 5s+(1)_s} &= w_{7(j+m+1)+1 \rightarrow 7(j+m+1)+6} \otimes w_{7j+4 \rightarrow 7(j+1)}.
\end{aligned}$$

(11) If  $r_0 = 10$ , then  $\Omega^{10}(Y_t^{(13)})$  is described with  $(12s \times 10s)$ -matrix with the following nonzero elements:

$$\begin{aligned}
b_{(j+1)_s, (1)_s} &= -e_{7(j+m)+6} \otimes w_{7j \rightarrow 7(j+1)}; \\
b_{j+2s, (2)_s} &= w_{7(j+m)+2 \rightarrow 7(j+m)+6} \otimes w_{7j \rightarrow 7j+1}; \\
b_{j+3s, (2)_s} &= -w_{7(j+m)+3 \rightarrow 7(j+m)+6} \otimes w_{7j \rightarrow 7j+2}; \\
b_{(j+1)_s, s+(1)_s} &= w_{7(j+m)+6 \rightarrow 7(j+m+1)} \otimes w_{7j \rightarrow 7(j+1)}; \\
b_{s+(j+1)_s, s+(1)_s} &= e_{7(j+m+1)} \otimes w_{7j \rightarrow 7(j+1)}; \\
b_{s+(j+1)_s, 2s+(1)_s} &= w_{7(j+m+1) \rightarrow 7(j+m+1)+3} \otimes w_{7j+1 \rightarrow 7(j+1)}; \\
b_{s+(j+1)_s, 2s+(2)_s} &= w_{7(j+m+1) \rightarrow 7(j+m+1)+3} \otimes w_{7j+1 \rightarrow 7(j+1)}; \\
b_{(j+1)_s, 5s+(1)_s} &= w_{7(j+m)+6 \rightarrow 7(j+m+1)+5} \otimes w_{7j+3 \rightarrow 7(j+1)}; \\
b_{5s+(j+1)_s, 5s+(1)_s} &= -e_{7(j+m+1)+5} \otimes w_{7j+3 \rightarrow 7(j+1)+3}; \\
b_{j+s, 6s+(1)_s} &= w_{7(j+m)+1 \rightarrow 7(j+m+1)+1} \otimes e_{7j+4}.
\end{aligned}$$

(12) If  $r_0 = 11$ , then  $\Omega^{11}(Y_t^{(13)})$  is described with  $(10s \times 10s)$ -matrix with the following nonzero elements:

$$\begin{aligned}
b_{s+(j+1)_s, (1)_s} &= e_{7(j+m+1)+4} \otimes w_{7j \rightarrow 7(j+1)}; \\
b_{(j+1)_s, s+(1)_s} &= -w_{7(j+m+1)+2 \rightarrow 7(j+m+1)+3} \otimes w_{7j \rightarrow 7(j+1)}; \\
b_{j+s, s+(2)_s} &= w_{7(j+m+1) \rightarrow 7(j+m+1)+3} \otimes w_{7j \rightarrow 7j+1}; \\
b_{j+2s, 2s+(1)_s} &= w_{7(j+m+1) \rightarrow 7(j+m+1)+1} \otimes w_{7j \rightarrow 7j+3}; \\
b_{j+3s, 2s+(1)_s} &= -w_{7(j+m+1) \rightarrow 7(j+m+1)+1} \otimes w_{7j \rightarrow 7j+4}; \\
b_{(j+1)_s, 3s+(1)_s} &= w_{7(j+m+1)+2 \rightarrow 7(j+m+1)+6} \otimes w_{7j+1 \rightarrow 7(j+1)}; \\
b_{s+(j+1)_s, 3s+(2)_s} &= w_{7(j+m+1)+4 \rightarrow 7(j+m+1)+6} \otimes w_{7j+1 \rightarrow 7(j+1)}; \\
b_{(j+1)_s, 5s+(1)_s} &= -w_{7(j+m+1)+2 \rightarrow 7(j+m+1)+6} \otimes w_{7j+3 \rightarrow 7(j+1)}; \\
b_{s+(j+1)_s, 5s+(1)_s} &= w_{7(j+m+1)+4 \rightarrow 7(j+m+1)+6} \otimes w_{7j+3 \rightarrow 7(j+1)}; \\
b_{3s+(j+1)_s, 5s+(1)_s} &= -e_{7(j+m+1)+6} \otimes w_{7j+3 \rightarrow 7(j+1)+2}; \\
b_{2s+(j+1)_s, 8s+(1)_s} &= -w_{7(j+m+2) \rightarrow 7(j+m+2)+2} \otimes w_{7j+6 \rightarrow 7(j+1)+1}.
\end{aligned}$$

(13) If  $r_0 = 12$ , then  $\Omega^{12}(Y_t^{(13)})$  is described with  $(10s \times 12s)$ -matrix with the following nonzero elements:

$$\begin{aligned}
b_{j+4s,(1)_s} &= -w_{7(j+m)+1 \rightarrow 7(j+m)+6} \otimes w_{7j \rightarrow 7j+3}; \\
b_{j+5s,(1)_s} &= w_{7(j+m)+2 \rightarrow 7(j+m)+6} \otimes w_{7j \rightarrow 7j+4}; \\
b_{j+2s,(2)_s} &= -w_{7(j+m)+4 \rightarrow 7(j+m)+6} \otimes w_{7j \rightarrow 7j+1}; \\
b_{j+s,(2)_s} &= w_{7(j+m)+4 \rightarrow 7(j+m)+1} \otimes w_{7j \rightarrow 7j+1}; \\
b_{j,2s+(2)_s} &= w_{7(j+m)+4 \rightarrow 7(j+m)+1+4} \otimes e_{7j+1}; \\
b_{(j+1)_s,4s+(1)_s} &= w_{7(j+m+1) \rightarrow 7(j+m+1)+5} \otimes w_{7j+2 \rightarrow 7(j+1)}; \\
b_{2s+(j+1)_s,4s+(1)_s} &= -w_{7(j+m+1)+4 \rightarrow 7(j+m+1)+5} \otimes w_{7j+2 \rightarrow 7(j+1)+1}; \\
b_{4s+(j+1)_s,5s} &= w_{7(j+m+1)+1 \rightarrow 7(j+m+1)+2} \otimes w_{7j+3 \rightarrow 7(j+1)+3}; \\
b_{(j+1)_s,5s+(1)_s} &= -w_{7(j+m+1) \rightarrow 7(j+m+1)+2} \otimes w_{7j+3 \rightarrow 7(j+1)}; \\
b_{4s+(j+1)_s,5s+(1)_s} &= w_{7(j+m+1)+1 \rightarrow 7(j+m+1)+2} \otimes w_{7j+3 \rightarrow 7(j+1)+3}; \\
b_{5s+(j+1)_s,8s} &= -w_{7(j+m+1)+2 \rightarrow 7(j+m+1)+3} \otimes w_{7j+5 \rightarrow 7(j+1)+4}; \\
b_{4s+(j+1)_s,10s} &= w_{7(j+m+1)+1 \rightarrow 7(j+m+1)+6} \otimes w_{7j+6 \rightarrow 7(j+1)+3}; \\
b_{5s+(j+1)_s,10s} &= -w_{7(j+m+1)+2 \rightarrow 7(j+m+1)+6} \otimes w_{7j+6 \rightarrow 7(j+1)+4}.
\end{aligned}$$

(14) If  $r_0 = 13$ , then  $\Omega^{13}(Y_t^{(13)})$  is described with  $(9s \times 12s)$ -matrix with the following nonzero elements:

$$\begin{aligned}
b_{j,(1)_s} &= w_{7(j+m)+3 \rightarrow 7(j+m+1)+2} \otimes e_{7j}; \\
b_{j+2s,(1)_s} &= w_{7(j+m)+6 \rightarrow 7(j+m+1)+2} \otimes w_{7j \rightarrow 7j+1}; \\
b_{j+3s,(1)_s} &= w_{7(j+m+1) \rightarrow 7(j+m+1)+2} \otimes w_{7j \rightarrow 7j+2}; \\
b_{j+6s,(1)_s} &= w_{7(j+m+1) \rightarrow 7(j+m+1)+2} \otimes w_{7j \rightarrow 7j+5}; \\
b_{s+(j+1)_s,s+(1)_s} &= -e_{7(j+m+1)+5} \otimes w_{7j \rightarrow 7(j+1)}; \\
b_{s+(j+1)_s,5s+(1)_s} &= -w_{7(j+m+1)+5 \rightarrow 7(j+m+2)} \otimes w_{7j+3 \rightarrow 7(j+1)}; \\
b_{3s+(j+1)_s,5s+(1)_s} &= -e_{7(j+m+2)} \otimes w_{7j+3 \rightarrow 7(j+1)+2}; \\
b_{2s+(j+1)_s,9s+(1)_s} &= w_{7(j+m+1)+6 \rightarrow 7(j+m+2)+4} \otimes w_{7j+6 \rightarrow 7(j+1)+1}; \\
b_{3s+(j+1)_s,9s+(1)_s} &= w_{7(j+m+2) \rightarrow 7(j+m+2)+4} \otimes w_{7j+6 \rightarrow 7(j+1)+2}; \\
b_{6s+(j+1)_s,9s+(1)_s} &= w_{7(j+m+2) \rightarrow 7(j+m+2)+4} \otimes w_{7j+6 \rightarrow 7(j+1)+5}.
\end{aligned}$$

(15) If  $r_0 = 14$ , then  $\Omega^{14}(Y_t^{(13)})$  is described with  $(7s \times 13s)$ -matrix with the following nonzero elements:

$$\begin{aligned}
b_{j,(1)_s} &= w_{7(j+m-1)+6 \rightarrow 7(j+m)+6} \otimes e_{7j}; \\
b_{(j+1)_s,(1)_s} &= -e_{7(j+m)+6} \otimes w_{7j \rightarrow 7(j+1)}; \\
b_{j+2s,(1)_s} &= w_{7(j+m)+1 \rightarrow 7(j+m)+6} \otimes w_{7j \rightarrow 7j+2}; \\
b_{j+3s,(1)_s} &= -w_{7(j+m)+2 \rightarrow 7(j+m)+6} \otimes w_{7j \rightarrow 7j+3}; \\
b_{j+4s,(1)_s} &= w_{7(j+m)+3 \rightarrow 7(j+m)+6} \otimes w_{7j \rightarrow 7j+4}; \\
b_{(j+1)_s,4s} &= -w_{7(j+m)+6 \rightarrow 7(j+m+1)+2} \otimes w_{7j+2 \rightarrow 7(j+1)}; \\
b_{2s+(j+1)_s,4s} &= -w_{7(j+m+1)+1 \rightarrow 7(j+m+1)+2} \otimes w_{7j+2 \rightarrow 7(j+1)+2}; \\
b_{2s+(j+1)_s,4s+(1)_s} &= -w_{7(j+m+1)+1 \rightarrow 7(j+m+1)+2} \otimes w_{7j+2 \rightarrow 7(j+1)+2}; \\
b_{(j+1)_s,5s} &= -w_{7(j+m)+6 \rightarrow 7(j+m+1)+3} \otimes w_{7j+3 \rightarrow 7(j+1)}; \\
b_{2s+(j+1)_s,5s} &= -w_{7(j+m+1)+1 \rightarrow 7(j+m+1)+3} \otimes w_{7j+3 \rightarrow 7(j+1)+2}; \\
b_{3s+(j+1)_s,5s} &= w_{7(j+m+1)+2 \rightarrow 7(j+m+1)+3} \otimes w_{7j+3 \rightarrow 7(j+1)+3};
\end{aligned}$$

$$\begin{aligned}
b_{2s+(j+1)s,5s+(1)s} &= -w_{7(j+m+1)+1 \rightarrow 7(j+m+1)+3} \otimes w_{7j+3 \rightarrow 7(j+1)+2}; \\
b_{3s+(j+1)s,5s+(1)s} &= w_{7(j+m+1)+2 \rightarrow 7(j+m+1)+3} \otimes w_{7j+3 \rightarrow 7(j+1)+3}; \\
b_{(j+1)s,6s+(1)s} &= w_{7(j+m)+6 \rightarrow 7(j+m+1)+4} \otimes w_{7j+3 \rightarrow 7(j+1)}; \\
b_{5s+(j+1)s,9s+(1)s} &= e_{7(j+m+1)+4} \otimes w_{7j+5 \rightarrow 7(j+1)+5}; \\
b_{(j+1)s,11s} &= w_{7(j+m)+6 \rightarrow 7(j+m+1)+6} \otimes w_{7j+6 \rightarrow 7(j+1)}; \\
b_{2s+(j+1)s,11s} &= w_{7(j+m+1)+1 \rightarrow 7(j+m+1)+6} \otimes w_{7j+6 \rightarrow 7(j+1)+2}; \\
b_{3s+(j+1)s,11s} &= -w_{7(j+m+1)+2 \rightarrow 7(j+m+1)+6} \otimes w_{7j+6 \rightarrow 7(j+1)+3}; \\
b_{4s+(j+1)s,11s} &= w_{7(j+m+1)+3 \rightarrow 7(j+m+1)+6} \otimes w_{7j+6 \rightarrow 7(j+1)+4}; \\
b_{(j+1)s,11s+(1)s} &= w_{7(j+m)+6 \rightarrow 7(j+m+1)+6} \otimes w_{7j+6 \rightarrow 7(j+1)}; \\
b_{2s+(j+1)s,11s+(1)s} &= w_{7(j+m+1)+1 \rightarrow 7(j+m+1)+6} \otimes w_{7j+6 \rightarrow 7(j+1)+2}; \\
b_{3s+(j+1)s,11s+(1)s} &= -w_{7(j+m+1)+2 \rightarrow 7(j+m+1)+6} \otimes w_{7j+6 \rightarrow 7(j+1)+3}; \\
b_{4s+(j+1)s,11s+(1)s} &= w_{7(j+m+1)+3 \rightarrow 7(j+m+1)+6} \otimes w_{7j+6 \rightarrow 7(j+1)+4}; \\
b_{2s+(j+1)s,12s} &= -w_{7(j+m+1)+1 \rightarrow 7(j+m+2)} \otimes w_{7j+6 \rightarrow 7(j+1)+2}; \\
b_{3s+(j+1)s,12s} &= w_{7(j+m+1)+2 \rightarrow 7(j+m+2)} \otimes w_{7j+6 \rightarrow 7(j+1)+3}; \\
b_{4s+(j+1)s,12s} &= -w_{7(j+m+1)+3 \rightarrow 7(j+m+2)} \otimes w_{7j+6 \rightarrow 7(j+1)+4}.
\end{aligned}$$

(16) If  $r_0 = 15$ , then  $\Omega^{15}(Y_t^{(13)})$  is described with  $(8s \times 12s)$ -matrix with the following nonzero elements:

$$\begin{aligned}
b_{j,s+(1)s} &= -w_{7(j+m+1) \rightarrow 7(j+m+1)+3} \otimes w_{7j \rightarrow 7j+1}; \\
b_{j+3s,s+(1)s} &= w_{7(j+m+1) \rightarrow 7(j+m+1)+3} \otimes w_{7j \rightarrow 7j+4}; \\
b_{(j+1)s,6s+(1)s} &= e_{7(j+m+1)+6} \otimes w_{7j+4 \rightarrow 7(j+1)}; \\
b_{(j+1)s,8s+(1)s} &= -w_{7(j+m+1)+6 \rightarrow 7(j+m+2)} \otimes w_{7j+5 \rightarrow 7(j+1)}; \\
b_{(j+1)s,9s+(1)s} &= w_{7(j+m+1)+6 \rightarrow 7(j+m+2)+2} \otimes w_{7j+6 \rightarrow 7(j+1)}.
\end{aligned}$$

(17) If  $r_0 = 16$ , then  $\Omega^{16}(Y_t^{(13)})$  is described with  $(7s \times 12s)$ -matrix with the following nonzero elements:

$$\begin{aligned}
b_{j+s,(1)s} &= w_{7(j+m)+1 \rightarrow 7(j+m)+6} \otimes w_{7j \rightarrow 7j+1}; \\
b_{j+2s,(1)s} &= -w_{7(j+m)+2 \rightarrow 7(j+m)+6} \otimes w_{7j \rightarrow 7j+2}; \\
b_{j+3s,(1)s} &= w_{7(j+m)+3 \rightarrow 7(j+m)+6} \otimes w_{7j \rightarrow 7j+3}; \\
b_{j+4s,(1)s} &= -w_{7(j+m)+4 \rightarrow 7(j+m)+6} \otimes w_{7j \rightarrow 7j+4}; \\
b_{j+5s,(1)s} &= w_{7(j+m)+5 \rightarrow 7(j+m)+6} \otimes w_{7j \rightarrow 7j+5}; \\
b_{j+6s,(1)s} &= -e_{7(j+m)+6} \otimes w_{7j \rightarrow 7j+6}; \\
b_{j-s,s+(1)s} &= -w_{7(j+m) \rightarrow 7(j+m+1)} \otimes e_{7j}; \\
b_{j,2s+(1)s} &= -w_{7(j+m)+2 \rightarrow 7(j+m+1)+2} \otimes w_{7j+1 \rightarrow 7j+2}; \\
b_{j+s,2s+(1)s} &= w_{7(j+m)+3 \rightarrow 7(j+m+1)+2} \otimes w_{7j+1 \rightarrow 7j+3}; \\
b_{j+4s,2s+(1)s} &= -w_{7(j+m)+6 \rightarrow 7(j+m+1)+2} \otimes w_{7j+1 \rightarrow 7j+6}; \\
b_{s+(j+1)s,3s} &= w_{7(j+m+1)+1 \rightarrow 7(j+m+1)+3} \otimes w_{7j+2 \rightarrow 7(j+1)+1}; \\
b_{2s+(j+1)s,3s} &= -w_{7(j+m+1)+2 \rightarrow 7(j+m+1)+3} \otimes w_{7j+2 \rightarrow 7(j+1)+2}; \\
b_{j,3s+(1)s} &= w_{7(j+m)+3 \rightarrow 7(j+m+1)+3} \otimes w_{7j+2 \rightarrow 7j+3}; \\
b_{j+3s,3s+(1)s} &= -w_{7(j+m)+6 \rightarrow 7(j+m+1)+3} \otimes w_{7j+2 \rightarrow 7j+6}; \\
b_{j-4s,9s+(1)s} &= w_{7(j+m)+5 \rightarrow 7(j+m+1)+5} \otimes e_{7j+5}; \\
b_{j-3s,9s+(1)s} &= -w_{7(j+m)+6 \rightarrow 7(j+m+1)+5} \otimes w_{7j+5 \rightarrow 7j+6};
\end{aligned}$$

$$b_{j-4s, 10s+(1)_s} = w_{7(j+m)+6 \rightarrow 7(j+m+1)+6} \otimes e_{7j+6}.$$

(II) Represent an arbitrary  $t_0 \in \mathbb{N}$  in the form  $t_0 = 17\ell_0 + r_0$ , where  $0 \leq r_0 \leq 16$ . Then  $\Omega^{t_0}(Y_t^{(13)})$  is a  $\Omega^{r_0}(Y_t^{(13)})$ , whose left components twisted by  $\sigma^{\ell_0}$ .

**Proposition 11** (Translates for the case 14). (I) Let  $r_0 \in \mathbb{N}$ ,  $r_0 < 17$ .  $r_0$ -translates of the elements  $Y_t^{(14)}$  are described by the following way.

(1) If  $r_0 = 0$ , then  $\Omega^0(Y_t^{(14)})$  is described with  $(7s \times 10s)$ -matrix with the following elements  $b_{ij}$ :

If  $0 \leq j < s$ , then

$$b_{ij} = \begin{cases} e_{7(j+m)} \otimes e_{7j}, & i = j; \\ 0, & \text{otherwise.} \end{cases}$$

If  $s \leq j < 2s$ , then

$$b_{ij} = \begin{cases} w_{7(j+m)+1 \rightarrow 7(j+m)+3} \otimes e_{7j+1}, & i = j; \\ 0, & \text{otherwise.} \end{cases}$$

If  $2s \leq j < 6s$ , then  $b_{ij} = 0$ .

If  $6s \leq j < 7s$ , then

$$b_{ij} = \begin{cases} -w_{7(j+m)+4 \rightarrow 7(j+m)+5} \otimes e_{7j+4}, & i = j - 2s; \\ 0, & \text{otherwise.} \end{cases}$$

If  $7s \leq j < 8s$ , then  $b_{ij} = 0$ .

If  $8s \leq j < 9s$ , then

$$b_{ij} = \begin{cases} e_{7(j+m)+6} \otimes e_{7j+6}, & i = j - 2s; \\ 0, & \text{otherwise.} \end{cases}$$

If  $9s \leq j < 10s$ , then  $b_{ij} = 0$ .

(2) If  $r_0 = 1$ , then  $\Omega^1(Y_t^{(14)})$  is described with  $(8s \times 9s)$ -matrix with the following elements  $b_{ij}$ :

If  $0 \leq j < s$ , then

$$b_{ij} = \begin{cases} w_{7(j+m)+1 \rightarrow 7(j+m)+3} \otimes e_{7j}, & i = j; \\ 0, & \text{otherwise.} \end{cases}$$

If  $s \leq j < 2s$ , then

$$b_{ij} = \begin{cases} w_{7(j+m)+4 \rightarrow 7(j+m)+5} \otimes e_{7j}, & i = j; \\ 0, & \text{otherwise.} \end{cases}$$

If  $2s \leq j < 3s$ , then

$$b_{ij} = \begin{cases} w_{7(j+m)+2 \rightarrow 7(j+m)+6} \otimes e_{7j+1}, & i = j; \\ w_{7(j+m)+3 \rightarrow 7(j+m)+6} \otimes w_{7j+1 \rightarrow 7j+2}, & i = j + s; \\ e_{7(j+m)+6} \otimes w_{7j+1 \rightarrow 7j+3}, & i = j + 2s; \\ 0, & \text{otherwise.} \end{cases}$$

If  $3s \leq j < 4s$ , then

$$b_{ij} = \begin{cases} e_{7(j+m+1)} \otimes w_{7j+2 \rightarrow 7j+6}, & i = j + 4s; \\ 0, & \text{otherwise.} \end{cases}$$

If  $4s \leq j < 5s$ , then

$$b_{ij} = \begin{cases} -w_{7(j+m+1) \rightarrow 7(j+m+1)+1} \otimes w_{7j+3 \rightarrow 7j+6}, & i = j + 3s; \\ 0, & \text{otherwise.} \end{cases}$$

If  $5s \leq j < 6s$ , then

$$b_{ij} = \begin{cases} w_{7(j+m)+5 \rightarrow 7(j+m)+6} \otimes e_{7j+4}, & i = j; \\ e_{7(j+m)+6} \otimes w_{7j+4 \rightarrow 7j+5}, & i = j + s; \\ 0, & \text{otherwise.} \end{cases}$$

If  $6s \leq j < 7s$ , then  $b_{ij} = 0$ .

If  $7s \leq j < 8s$ , then

$$b_{ij} = \begin{cases} w_{7(j+m+1) \rightarrow 7(j+m+1)+2} \otimes e_{7j+6}, & i = j; \\ 0, & \text{otherwise.} \end{cases}$$

If  $8s \leq j < 9s$ , then  $b_{ij} = 0$ .

(3) If  $r_0 = 2$ , then  $\Omega^2(Y_t^{(14)})$  is described with  $(7s \times 7s)$ -matrix with the following elements  $b_{ij}$ :

If  $0 \leq j < s$ , then

$$b_{ij} = \begin{cases} e_{7(j+m-1)+6} \otimes e_{7j}, & i = j; \\ 0, & \text{otherwise.} \end{cases}$$

If  $s \leq j < 2s$ , then

$$b_{ij} = \begin{cases} w_{7(j+m)+4 \rightarrow 7(j+m)+5} \otimes w_{7j+1 \rightarrow 7j+3}, & i = j + 2s; \\ 0, & \text{otherwise.} \end{cases}$$

If  $2s \leq j < 4s$ , then  $b_{ij} = 0$ .

If  $4s \leq j < 5s$ , then

$$b_{ij} = \begin{cases} w_{7(j+m)+1 \rightarrow 7(j+m)+3} \otimes w_{7j+4 \rightarrow 7j+5}, & i = j + s; \\ 0, & \text{otherwise.} \end{cases}$$

If  $5s \leq j < 6s$ , then  $b_{ij} = 0$ .

If  $6s \leq j < 7s$ , then

$$b_{ij} = \begin{cases} e_{7(j+m+1)} \otimes e_{7j+6}, & i = j; \\ 0, & \text{otherwise.} \end{cases}$$

(4) If  $r_0 = 3$ , then  $\Omega^3(Y_t^{(14)})$  is described with  $(9s \times 8s)$ -matrix with the following elements  $b_{ij}$ :

If  $0 \leq j < s$ , then

$$b_{ij} = \begin{cases} w_{7(j+m)+2 \rightarrow 7(j+m)+6} \otimes e_{7j}, & i = j; \\ w_{7(j+m)+3 \rightarrow 7(j+m)+6} \otimes w_{7j \rightarrow 7j+1}, & i = j + 2s; \\ e_{7(j+m)+6} \otimes w_{7j \rightarrow 7j+2}, & i = j + 3s; \\ 0, & \text{otherwise.} \end{cases}$$

If  $s \leq j < 2s$ , then

$$b_{ij} = \begin{cases} e_{7(j+m+1)} \otimes w_{7j+1 \rightarrow 7j+3}, & i = j + 3s; \\ 0, & \text{otherwise.} \end{cases}$$

If  $2s \leq j < 3s$ , then

$$b_{ij} = \begin{cases} -w_{7(j+m+1) \rightarrow 7(j+m+1)+1} \otimes w_{7j+2 \rightarrow 7j+3}, & i = j + 2s; \\ 0, & \text{otherwise.} \end{cases}$$

If  $3s \leq j < 4s$ , then

$$b_{ij} = \begin{cases} w_{7(j+m+1) \rightarrow 7(j+m+1)+2} \otimes e_{7j+3}, & i = j + s; \\ 0, & \text{otherwise.} \end{cases}$$

If  $4s \leq j < 5s$ , then

$$b_{ij} = \begin{cases} e_{7(j+m+1)} \otimes w_{7j+4 \rightarrow 7j+5}, & i = j + 2s; \\ 0, & \text{otherwise.} \end{cases}$$

If  $5s \leq j < 6s$ , then

$$b_{ij} = \begin{cases} -w_{7(j+m+1) \rightarrow 7(j+m+1)+4} \otimes e_{7j+5}, & i = j + s; \\ 0, & \text{otherwise.} \end{cases}$$

If  $6s \leq j < 7s$ , then

$$b_{ij} = \begin{cases} w_{7(j+m+1)+1 \rightarrow 7(j+m+1)+3} \otimes e_{7j+6}, & i = j + s; \\ 0, & \text{otherwise.} \end{cases}$$

If  $7s \leq j < 8s$ , then

$$b_{ij} = \begin{cases} w_{7(j+m+1)+4 \rightarrow 7(j+m+1)+5} \otimes e_{7j+6}, & i = j + s; \\ 0, & \text{otherwise.} \end{cases}$$

(5) If  $r_0 = 4$ , then  $\Omega^4(Y_t^{(14)})$  is described with  $(10s \times 7s)$ -matrix with the following elements  $b_{ij}$ :

If  $0 \leq j < s$ , then

$$b_{ij} = \begin{cases} w_{7(j+m-1)+6 \rightarrow 7(j+m)} \otimes e_{7j}, & i = j; \\ e_{7(j+m)} \otimes e_{7j}, & i = j + s; \\ 0, & \text{otherwise.} \end{cases}$$

If  $s \leq j < 3s$ , then  $b_{ij} = 0$ .

If  $3s \leq j < 4s$ , then

$$b_{ij} = \begin{cases} w_{7(j+m)+1 \rightarrow 7(j+m)+3} \otimes e_{7j+3}, & i = j + s; \\ 0, & \text{otherwise.} \end{cases}$$

If  $4s \leq j < 5s$ , then  $b_{ij} = 0$ .

If  $5s \leq j < 6s$ , then

$$b_{ij} = \begin{cases} -w_{7(j+m)+4 \rightarrow 7(j+m)+5} \otimes e_{7j+5}, & i = j + 3s; \\ 0, & \text{otherwise.} \end{cases}$$

If  $6s \leq j < 7s$ , then

$$b_{ij} = \begin{cases} e_{7(j+m)+6} \otimes e_{7j+6}, & i = j + 3s; \\ 0, & \text{otherwise.} \end{cases}$$



(6) If  $r_0 = 5$ , then  $\Omega^5(Y_t^{(14)})$  is described with  $(10s \times 7s)$ -matrix with the following elements  $b_{ij}$ :

If  $0 \leq j < s$ , then

$$b_{ij} = \begin{cases} w_{7(j+m)+4 \rightarrow 7(j+m+1)} \otimes e_{7j}, & i = j; \\ e_{7(j+m+1)} \otimes w_{7j \rightarrow 7j+2}, & i = j + 4s; \\ -w_{7(j+m)+6 \rightarrow 7(j+m+1)} \otimes w_{7j \rightarrow 7j+3}, & i = j + 5s; \\ 0, & \text{otherwise.} \end{cases}$$

If  $s \leq j < 2s$ , then

$$b_{ij} = \begin{cases} e_{7(j+m+1)+1} \otimes w_{7j+1 \rightarrow 7(j+1)}, & i = 2s + (j+1)_s; \\ w_{7(j+m)+6 \rightarrow 7(j+m+1)+1} \otimes w_{7j+1 \rightarrow 7j+3}, & i = j + 4s; \\ 0, & \text{otherwise.} \end{cases}$$

If  $2s \leq j < 3s$ , then

$$b_{ij} = \begin{cases} -w_{7(j+m+1)+1 \rightarrow 7(j+m+1)+2} \otimes w_{7j+2 \rightarrow 7(j+1)}, & i = 2s + (j+1)_s; \\ -w_{7(j+m)+6 \rightarrow 7(j+m+1)+2} \otimes w_{7j+2 \rightarrow 7j+3}, & i = j + 3s; \\ 0, & \text{otherwise.} \end{cases}$$

If  $3s \leq j < 4s$ , then

$$b_{ij} = \begin{cases} w_{7(j+m+1)+1 \rightarrow 7(j+m+1)+3} \otimes w_{7j+3 \rightarrow 7(j+1)}, & i = 2s + (j+1)_s; \\ w_{7(j+m)+6 \rightarrow 7(j+m+1)+3} \otimes e_{7j+3}, & i = j + 2s; \\ 0, & \text{otherwise.} \end{cases}$$

If  $4s \leq j < 5s$ , then

$$b_{ij} = \begin{cases} -e_{7(j+m+1)+4} \otimes w_{7j+4 \rightarrow 7(j+1)}, & i = (j+1)_s; \\ -w_{7(j+m)+6 \rightarrow 7(j+m+1)+4} \otimes w_{7j+4 \rightarrow 7j+5}, & i = j + 3s; \\ 0, & \text{otherwise.} \end{cases}$$

If  $5s \leq j < 6s$ , then

$$b_{ij} = \begin{cases} w_{7(j+m+1)+4 \rightarrow 7(j+m+1)+5} \otimes w_{7j+5 \rightarrow 7(j+1)}, & i = (j+1)_s; \\ w_{7(j+m)+6 \rightarrow 7(j+m+1)+5} \otimes e_{7j+5}, & i = j + 2s; \\ 0, & \text{otherwise.} \end{cases}$$

If  $6s \leq j < 7s$ , then

$$b_{ij} = \begin{cases} -w_{7(j+m+1)+4 \rightarrow 7(j+m+1)+6} \otimes w_{7j+6 \rightarrow 7(j+1)}, & i = (j+1)_s; \\ w_{7(j+m+1)+3 \rightarrow 7(j+m+1)+6} \otimes w_{7j+6 \rightarrow 7(j+1)}, & i = s + (j+1)_s; \\ w_{7(j+m+1)+1 \rightarrow 7(j+m+1)+6} \otimes w_{7j+6 \rightarrow 7(j+1)}, & i = 2s + (j+1)_s; \\ e_{7(j+m+1)+6} \otimes w_{7j+6 \rightarrow 7(j+1)+1}, & i = 3s + (j+1)_s; \\ e_{7(j+m+1)+6} \otimes w_{7j+6 \rightarrow 7(j+1)+3}, & i = 5s + (j+1)_s; \\ w_{7(j+m+1)+2 \rightarrow 7(j+m+1)+6} \otimes e_{7j+6}, & i = j + 2s; \\ 0, & \text{otherwise.} \end{cases}$$

(7) If  $r_0 = 6$ , then  $\Omega^6(Y_t^{(14)})$  is described with  $(12s \times 8s)$ -matrix with the following elements  $b_{ij}$ :

If  $0 \leq j < s$ , then

$$b_{ij} = \begin{cases} -e_{7(j+m)+1} \otimes w_{7j \rightarrow 7j+2}, & i = j + 3s; \\ 0, & \text{otherwise.} \end{cases}$$

If  $s \leq j < 2s$ , then

$$b_{ij} = \begin{cases} w_{7(j+m-1)+6 \rightarrow 7(j+m)+4} \otimes e_{7j}, & i = j - s; \\ e_{7(j+m)+4} \otimes w_{7j \rightarrow 7j+1}, & i = j + s; \\ 0, & \text{otherwise.} \end{cases}$$

If  $2s \leq j < 4s$ , then  $b_{ij} = 0$ .

If  $4s \leq j < 5s$ , then

$$b_{ij} = \begin{cases} e_{7(j+m)+6} \otimes w_{7j+3 \rightarrow 7(j+1)}, & i = (j+1)_s; \\ -w_{7(j+m)+2 \rightarrow 7(j+m)+6} \otimes e_{7j+3}, & i = j + s; \\ 0, & \text{otherwise.} \end{cases}$$

If  $5s \leq j < 6s$ , then  $b_{ij} = 0$ .

If  $6s \leq j < 7s$ , then

$$b_{ij} = \begin{cases} -w_{7(j+m)+3 \rightarrow 7(j+m)+6} \otimes e_{7j+5}, & i = j + 2s; \\ 0, & \text{otherwise.} \end{cases}$$

If  $7s \leq j < 8s$ , then

$$b_{ij} = \begin{cases} -w_{7(j+m)+6 \rightarrow 7(j+m+1)} \otimes e_{7j+6}, & i = j + 3s; \\ -e_{7(j+m+1)} \otimes e_{7j+6}, & i = j + 4s; \\ 0, & \text{otherwise.} \end{cases}$$

(8) If  $r_0 = 7$ , then  $\Omega^7(Y_t^{(14)})$  is described with  $(12s \times 7s)$ -matrix with the following elements  $b_{ij}$ :

If  $0 \leq j < s$ , then

$$b_{ij} = \begin{cases} -w_{7(j+m)+2 \rightarrow 7(j+m)+6} \otimes e_{7j}, & i = j; \\ w_{7(j+m)+4 \rightarrow 7(j+m)+6} \otimes e_{7j}, & i = j + 2s; \\ -e_{7(j+m)+6} \otimes w_{7j \rightarrow 7j+4}, & i = j + 6s; \\ 0, & \text{otherwise.} \end{cases}$$

If  $s \leq j < 2s$ , then

$$b_{ij} = \begin{cases} -e_{7(j+m+1)+2} \otimes w_{7j+1 \rightarrow 7(j+1)}, & i = (j+1)_s; \\ w_{7(j+m+1) \rightarrow 7(j+m+1)+2} \otimes w_{7j+1 \rightarrow 7j+3}, & i = j + 4s; \\ 0, & \text{otherwise.} \end{cases}$$

If  $2s \leq j < 3s$ , then

$$b_{ij} = \begin{cases} w_{7(j+m+1)+2 \rightarrow 7(j+m+1)+3} \otimes w_{7j+2 \rightarrow 7(j+1)}, & i = (j+1)_s; \\ -w_{7(j+m+1) \rightarrow 7(j+m+1)+3} \otimes w_{7j+2 \rightarrow 7j+3}, & i = j + 3s; \\ 0, & \text{otherwise.} \end{cases}$$

If  $3s \leq j < 4s$ , then

$$b_{ij} = \begin{cases} -e_{7(j+m+1)+4} \otimes w_{7j+3 \rightarrow 7(j+1)}, & i = 2s + (j+1)_s; \\ w_{7(j+m+1) \rightarrow 7(j+m+1)+4} \otimes e_{7j+3}, & i = j + 2s; \\ 0, & \text{otherwise.} \end{cases}$$

If  $4s \leq j < 5s$ , then

$$b_{ij} = \begin{cases} -e_{7(j+m+1)+5} \otimes w_{7j+4 \rightarrow 7(j+1)}, & i = s + (j+1)_s; \\ -w_{7(j+m)+6 \rightarrow 7(j+m+1)+5} \otimes w_{7j+4 \rightarrow 7j+5}, & i = j + 3s; \\ -w_{7(j+m+1) \rightarrow 7(j+m+1)+5} \otimes w_{7j+4 \rightarrow 7j+5}, & i = j + 4s; \\ 0, & \text{otherwise.} \end{cases}$$

If  $5s \leq j < 6s$ , then

$$b_{ij} = \begin{cases} -w_{7(j+m)+6 \rightarrow 7(j+m+1)+1} \otimes e_{7j+5}, & i = j + 2s; \\ -w_{7(j+m+1) \rightarrow 7(j+m+1)+1} \otimes e_{7j+5}, & i = j + 3s; \\ 0, & \text{otherwise.} \end{cases}$$

If  $6s \leq j < 7s$ , then

$$b_{ij} = \begin{cases} e_{7(j+m+2)} \otimes w_{7j+6 \rightarrow 7(j+1)+1}, & i = 3s + (j+1)_s; \\ e_{7(j+m+2)} \otimes w_{7j+6 \rightarrow 7(j+1)+3}, & i = 5s + (j+1)_s; \\ w_{7(j+m+1)+4 \rightarrow 7(j+m+2)} \otimes e_{7j+6}, & i = j + 3s; \\ 0, & \text{otherwise.} \end{cases}$$

(9) If  $r_0 = 8$ , then  $\Omega^8(Y_t^{(14)})$  is described with  $(13s \times 9s)$ -matrix with the following elements  $b_{ij}$ :

If  $0 \leq j < s$ , then

$$b_{ij} = \begin{cases} w_{7(j+m-1)+6 \rightarrow 7(j+m)+2} \otimes e_{7j}, & i = j; \\ w_{7(j+m) \rightarrow 7(j+m)+2} \otimes e_{7j}, & i = j + s; \\ w_{7(j+m)+1 \rightarrow 7(j+m)+2} \otimes w_{7j \rightarrow 7j+1}, & i = j + 2s; \\ -e_{7(j+m)+2} \otimes w_{7j \rightarrow 7j+2}, & i = j + 4s; \\ 0, & \text{otherwise.} \end{cases}$$

If  $s \leq j < 2s$ , then

$$b_{ij} = \begin{cases} -w_{7(j+m-1)+6 \rightarrow 7(j+m)+5} \otimes e_{7j}, & i = j - s; \\ -w_{7(j+m) \rightarrow 7(j+m)+5} \otimes e_{7j}, & i = j; \\ -e_{7(j+m)+5} \otimes w_{7j \rightarrow 7j+1}, & i = j + 2s; \\ 0, & \text{otherwise.} \end{cases}$$

If  $2s \leq j < 4s$ , then  $b_{ij} = 0$ .

If  $4s \leq j < 5s$ , then

$$b_{ij} = \begin{cases} w_{7(j+m)+6 \rightarrow 7(j+m+1)} \otimes w_{7j+3 \rightarrow 7(j+1)}, & i = (j+1)_s; \\ e_{7(j+m+1)} \otimes w_{7j+3 \rightarrow 7(j+1)}, & i = s + (j+1)_s; \\ -w_{7(j+m)+4 \rightarrow 7(j+m+1)} \otimes e_{7j+3}, & i = j + 2s; \\ 0, & \text{otherwise.} \end{cases}$$

If  $5s \leq j < 6s$ , then

$$b_{ij} = \begin{cases} -e_{7(j+m)+6} \otimes w_{7j+4 \rightarrow 7(j+1)}, & i = (j+1)_s; \\ 0, & \text{otherwise.} \end{cases}$$

If  $6s \leq j < 7s$ , then

$$b_{ij} = \begin{cases} -w_{7(j+m)+4 \rightarrow 7(j+m+1)} \otimes e_{7j+5}, & i = j + 3s; \\ 0, & \text{otherwise.} \end{cases}$$

If  $7s \leq j < 8s$ , then

$$b_{ij} = \begin{cases} w_{7(j+m)+6 \rightarrow 7(j+m+1)+1} \otimes w_{7j+6 \rightarrow 7(j+1)}, & i = (j+1)_s; \\ w_{7(j+m+1) \rightarrow 7(j+m+1)+1} \otimes w_{7j+6 \rightarrow 7(j+1)}, & i = s + (j+1)_s; \\ 0, & \text{otherwise.} \end{cases}$$

If  $8s \leq j < 9s$ , then

$$b_{ij} = \begin{cases} -w_{7(j+m)+6 \rightarrow 7(j+m+1)+4} \otimes w_{7j+6 \rightarrow 7(j+1)}, & i = (j+1)_s; \\ -w_{7(j+m+1) \rightarrow 7(j+m+1)+4} \otimes w_{7j+6 \rightarrow 7(j+1)}, & i = s + (j+1)_s; \\ -e_{7(j+m+1)+4} \otimes w_{7j+6 \rightarrow 7(j+1)+3}, & i = 6s + (j+1)_s; \\ e_{7(j+m+1)+4} \otimes w_{7j+6 \rightarrow 7(j+1)+5}, & i = 9s + (j+1)_s; \\ w_{7(j+m)+6 \rightarrow 7(j+m+1)+4} \otimes e_{7j+6}, & i = j + 3s; \\ 0, & \text{otherwise.} \end{cases}$$

(10) If  $r_0 = 9$ , then  $\Omega^9(Y_t^{(14)})$  is described with  $(12s \times 10s)$ -matrix with the following elements  $b_{ij}$ :

If  $0 \leq j < s$ , then

$$b_{ij} = \begin{cases} e_{7(j+m)+6} \otimes w_{7j \rightarrow 7j+1}, & i = j + 3s; \\ 0, & \text{otherwise.} \end{cases}$$

If  $s \leq j < 2s$ , then

$$b_{ij} = \begin{cases} -w_{7(j+m)+5 \rightarrow 7(j+m+1)} \otimes e_{7j}, & i = j - s; \\ -e_{7(j+m+1)} \otimes w_{7j \rightarrow 7j+4}, & i = j + 6s; \\ 0, & \text{otherwise.} \end{cases}$$

If  $2s \leq j < 3s$ , then

$$b_{ij} = \begin{cases} -e_{7(j+m+1)+3} \otimes w_{7j+1 \rightarrow 7(j+1)}, & i = s + (j+1)_s; \\ -w_{7(j+m+1)+1 \rightarrow 7(j+m+1)+3} \otimes w_{7j+1 \rightarrow 7(j+1)}, & i = 2s + (j+1)_s; \\ 0, & \text{otherwise.} \end{cases}$$

If  $3s \leq j < 4s$ , then

$$b_{ij} = \begin{cases} w_{7(j+m)+6 \rightarrow 7(j+m+1)+4} \otimes w_{7j+2 \rightarrow 7j+3}, & i = j + 2s; \\ 0, & \text{otherwise.} \end{cases}$$

If  $4s \leq j < 5s$ , then  $b_{ij} = 0$ .

If  $5s \leq j < 6s$ , then

$$b_{ij} = \begin{cases} e_{7(j+m+1)+5} \otimes w_{7j+3 \rightarrow 7(j+1)}, & i = (j+1)s; \\ -w_{7(j+m)+6 \rightarrow 7(j+m+1)+5} \otimes e_{7j+3}, & i = j; \\ 0, & \text{otherwise.} \end{cases}$$

If  $6s \leq j < 7s$ , then

$$b_{ij} = \begin{cases} e_{7(j+m+1)+1} \otimes w_{7j+4 \rightarrow 7(j+1)}, & i = 2s + (j+1)s; \\ 0, & \text{otherwise.} \end{cases}$$

If  $7s \leq j < 8s$ , then  $b_{ij} = 0$ .

If  $8s \leq j < 9s$ , then

$$b_{ij} = \begin{cases} -w_{7(j+m+1) \rightarrow 7(j+m+1)+4} \otimes e_{7j+5}, & i = j; \\ -e_{7(j+m+1)+4} \otimes w_{7j+5 \rightarrow 7j+6}, & i = j+3s; \\ 0, & \text{otherwise.} \end{cases}$$

If  $9s \leq j < 10s$ , then

$$b_{ij} = \begin{cases} w_{7(j+m+1)+5 \rightarrow 7(j+m+1)+6} \otimes w_{7j+6 \rightarrow 7(j+1)}, & i = (j+1)s; \\ e_{7(j+m+1)+6} \otimes w_{7j+6 \rightarrow 7(j+1)+1}, & i = 3s + (j+1)s; \\ -w_{7(j+m+1)+5 \rightarrow 7(j+m+1)+6} \otimes e_{7j+6}, & i = j+s; \\ 0, & \text{otherwise.} \end{cases}$$

(11) If  $r_0 = 10$ , then  $\Omega^{10}(Y_t^{(14)})$  is described with  $(12s \times 10s)$ -matrix with the following elements  $b_{ij}$ :

If  $0 \leq j < s$ , then

$$b_{ij} = \begin{cases} -w_{7(j+m-1)+6 \rightarrow 7(j+m)+4} \otimes e_{7j}, & i = j; \\ -w_{7(j+m) \rightarrow 7(j+m)+4} \otimes e_{7j}, & i = j+s; \\ e_{7(j+m)+4} \otimes w_{7j \rightarrow 7j+2}, & i = j+4s; \\ 0, & \text{otherwise.} \end{cases}$$

If  $s \leq j < 2s$ , then

$$b_{ij} = \begin{cases} w_{7(j+m)+2 \rightarrow 7(j+m)+3} \otimes w_{7j \rightarrow 7j+1}, & i = j+s; \\ -e_{7(j+m)+3} \otimes w_{7j \rightarrow 7j+2}, & i = j+2s; \\ 0, & \text{otherwise.} \end{cases}$$

If  $2s \leq j < 3s$ , then

$$b_{ij} = \begin{cases} e_{7(j+m)+1} \otimes w_{7j \rightarrow 7j+4}, & i = j+5s; \\ 0, & \text{otherwise.} \end{cases}$$

If  $3s \leq j < 4s$ , then

$$b_{ij} = \begin{cases} -e_{7(j+m)+6} \otimes w_{7j+1 \rightarrow 7(j+1)}, & i = (j+1)s; \\ 0, & \text{otherwise.} \end{cases}$$

If  $4s \leq j < 5s$ , then  $b_{ij} = 0$ .

If  $5s \leq j < 6s$ , then

$$b_{ij} = \begin{cases} -w_{7(j+m)+5 \rightarrow 7(j+m)+6} \otimes e_{7j+3}, & i = j; \\ 0, & \text{otherwise.} \end{cases}$$

If  $6s \leq j < 7s$ , then

$$b_{ij} = \begin{cases} -w_{7(j+m)+6 \rightarrow 7(j+m)+1} \otimes w_{7j+4 \rightarrow 7(j+1)}, & i = (j+1)_s; \\ -e_{7(j+m)+1} \otimes w_{7j+4 \rightarrow 7(j+1)}, & i = s + (j+1)_s; \\ 0, & \text{otherwise.} \end{cases}$$

If  $7s \leq j < 8s$ , then

$$b_{ij} = \begin{cases} w_{7(j+m)+5 \rightarrow 7(j+m)+6} \otimes e_{7j+5}, & i = j + 2s; \\ 0, & \text{otherwise.} \end{cases}$$

If  $8s \leq j < 9s$ , then

$$b_{ij} = \begin{cases} w_{7(j+m+1)+1 \rightarrow 7(j+m+1)+2} \otimes w_{7j+6 \rightarrow 7(j+1)+4}, & i = 7s + (j+1)_s; \\ 0, & \text{otherwise.} \end{cases}$$

If  $9s \leq j < 10s$ , then

$$b_{ij} = \begin{cases} w_{7(j+m)+6 \rightarrow 7(j+m+1)+5} \otimes e_{7j+6}, & i = j + s; \\ 0, & \text{otherwise.} \end{cases}$$

(12) If  $r_0 = 11$ , then  $\Omega^{11}(Y_t^{(14)})$  is described with  $(10s \times 12s)$ -matrix with the following elements  $b_{ij}$ :

If  $0 \leq j < s$ , then

$$b_{ij} = \begin{cases} -w_{7(j+m)+2 \rightarrow 7(j+m)+6} \otimes e_{7j}, & i = j; \\ -e_{7(j+m)+6} \otimes w_{7j \rightarrow 7j+2}, & i = j + 3s; \\ -e_{7(j+m)+6} \otimes w_{7j \rightarrow 7j+5}, & i = j + 6s; \\ 0, & \text{otherwise.} \end{cases}$$

If  $s \leq j < 2s$ , then

$$b_{ij} = \begin{cases} e_{7(j+m+1)} \otimes w_{7j \rightarrow 7j+1}, & i = j + s; \\ 0, & \text{otherwise.} \end{cases}$$

If  $2s \leq j < 3s$ , then

$$b_{ij} = \begin{cases} -e_{7(j+m+1)+4} \otimes w_{7j+1 \rightarrow 7(j+1)}, & i = s + (j+1)_s; \\ 0, & \text{otherwise.} \end{cases}$$

If  $3s \leq j < 4s$ , then  $b_{ij} = 0$ .

If  $4s \leq j < 5s$ , then

$$b_{ij} = \begin{cases} w_{7(j+m+1)+4 \rightarrow 7(j+m+1)+5} \otimes w_{7j+2 \rightarrow 7(j+1)}, & i = s + (j+1)_s; \\ -w_{7(j+m)+6 \rightarrow 7(j+m+1)+5} \otimes e_{7j+2}, & i = j - s; \\ 0, & \text{otherwise.} \end{cases}$$

If  $5s \leq j < 6s$ , then  $b_{ij} = 0$ .

If  $6s \leq j < 7s$ , then

$$b_{ij} = \begin{cases} -e_{7(j+m+1)+2} \otimes w_{7j+4 \rightarrow 7(j+1)}, & i = (j+1)_s; \\ 0, & \text{otherwise.} \end{cases}$$

If  $7s \leq j < 9s$ , then  $b_{ij} = 0$ .

If  $9s \leq j < 10s$ , then

$$b_{ij} = \begin{cases} -w_{7(j+m)+6 \rightarrow 7(j+m+1)+5} \otimes e_{7j+5}, & i = j - 3s; \\ 0, & \text{otherwise.} \end{cases}$$

If  $10s \leq j < 11s$ , then

$$b_{ij} = \begin{cases} w_{7(j+m+1)+3 \rightarrow 7(j+m+1)+6} \otimes e_{7j+6}, & i = j - 2s; \\ 0, & \text{otherwise.} \end{cases}$$

If  $11s \leq j < 12s$ , then  $b_{ij} = 0$ .

(13) If  $r_0 = 12$ , then  $\Omega^{12}(Y_t^{(14)})$  is described with  $(10s \times 12s)$ -matrix with the following elements  $b_{ij}$ :

If  $0 \leq j < s$ , then

$$b_{ij} = \begin{cases} w_{7(j+m) \rightarrow 7(j+m)+2} \otimes e_{7j}, & i = j; \\ -w_{7(j+m)+1 \rightarrow 7(j+m)+2} \otimes w_{7j \rightarrow 7j+3}, & i = j + 4s; \\ e_{7(j+m)+2} \otimes w_{7j \rightarrow 7j+4}, & i = j + 5s; \\ 0, & \text{otherwise.} \end{cases}$$

If  $s \leq j < 2s$ , then  $b_{ij} = 0$ .

If  $2s \leq j < 3s$ , then

$$b_{ij} = \begin{cases} e_{7(j+m)+4} \otimes w_{7j \rightarrow 7j+1}, & i = j; \\ 0, & \text{otherwise.} \end{cases}$$

If  $3s \leq j < 4s$ , then

$$b_{ij} = \begin{cases} -e_{7(j+m+1)} \otimes w_{7j+1 \rightarrow 7(j+1)}, & i = (j+1)_s; \\ 0, & \text{otherwise.} \end{cases}$$

If  $4s \leq j < 5s$ , then

$$b_{ij} = \begin{cases} -w_{7(j+m)+5 \rightarrow 7(j+m)+6} \otimes e_{7j+2}, & i = j - s; \\ w_{7(j+m)+1 \rightarrow 7(j+m)+6} \otimes w_{7j+2 \rightarrow 7j+3}, & i = j; \\ -e_{7(j+m)+6} \otimes w_{7j+2 \rightarrow 7j+6}, & i = j + 4s; \\ 0, & \text{otherwise.} \end{cases}$$

If  $5s \leq j < 6s$ , then

$$b_{ij} = \begin{cases} e_{7(j+m+1)} \otimes w_{7j+3 \rightarrow 7j+6}, & i = j + 4s; \\ 0, & \text{otherwise.} \end{cases}$$

If  $6s \leq j < 7s$ , then  $b_{ij} = 0$ .

If  $7s \leq j < 8s$ , then

$$b_{ij} = \begin{cases} -w_{7(j+m)+3 \rightarrow 7(j+m)+6} \otimes e_{7j+5}, & i = j; \\ 0, & \text{otherwise.} \end{cases}$$

If  $8s \leq j < 10s$ , then  $b_{ij} = 0$ .

If  $10s \leq j < 11s$ , then

$$b_{ij} = \begin{cases} -w_{7(j+m)+6 \rightarrow 7(j+m+1)+3} \otimes e_{7j+6}, & i = j - 2s; \\ 0, & \text{otherwise.} \end{cases}$$

If  $11s \leq j < 12s$ , then  $b_{ij} = 0$ .

(14) If  $r_0 = 13$ , then  $\Omega^{13}(Y_t^{(14)})$  is described with  $(9s \times 13s)$ -matrix with the following elements  $b_{ij}$ :

If  $0 \leq j < s$ , then

$$b_{ij} = \begin{cases} w_{7(j+m)+3 \rightarrow 7(j+m)+6} \otimes e_{7j}, & i = j; \\ e_{7(j+m)+6} \otimes w_{7j \rightarrow 7j+1}, & i = j + 2s; \\ 0, & \text{otherwise.} \end{cases}$$

If  $s \leq j < 2s$ , then

$$b_{ij} = \begin{cases} -e_{7(j+m+1)} \otimes w_{7j \rightarrow 7j+2}, & i = j + 2s; \\ 0, & \text{otherwise.} \end{cases}$$

If  $2s \leq j < 3s$ , then

$$b_{ij} = \begin{cases} -w_{7(j+m+1) \rightarrow 7(j+m+1)+1} \otimes w_{7j+1 \rightarrow 7j+2}, & i = j + s; \\ 0, & \text{otherwise.} \end{cases}$$

If  $3s \leq j < 4s$ , then

$$b_{ij} = \begin{cases} e_{7(j+m+1)+5} \otimes w_{7j+1 \rightarrow 7(j+1)}, & i = s + (j + 1)s; \\ 0, & \text{otherwise.} \end{cases}$$

If  $4s \leq j < 5s$ , then

$$b_{ij} = \begin{cases} w_{7(j+m+1) \rightarrow 7(j+m+1)+2} \otimes e_{7j+2}, & i = j - s; \\ 0, & \text{otherwise.} \end{cases}$$

If  $5s \leq j < 6s$ , then

$$b_{ij} = \begin{cases} w_{7(j+m+1)+1 \rightarrow 7(j+m+1)+3} \otimes e_{7j+3}, & i = j - s; \\ 0, & \text{otherwise.} \end{cases}$$

If  $6s \leq j < 7s$ , then

$$b_{ij} = \begin{cases} e_{7(j+m+1)+4} \otimes w_{7j+3 \rightarrow 7j+6}, & i = j + 2s; \\ 0, & \text{otherwise.} \end{cases}$$

If  $7s \leq j < 8s$ , then

$$b_{ij} = \begin{cases} w_{7(j+m)+6 \rightarrow 7(j+m+1)+3} \otimes e_{7j+4}, & i = j - 2s; \\ 0, & \text{otherwise.} \end{cases}$$



If  $8s \leq j < 11s$ , then  $b_{ij} = 0$ .

If  $11s \leq j < 12s$ , then

$$b_{ij} = \begin{cases} -w_{7(j+m+1)+2 \rightarrow 7(j+m+1)+6} \otimes e_{7j+6}, & i = j - 4s; \\ w_{7(j+m+1)+4 \rightarrow 7(j+m+1)+6} \otimes e_{7j+6}, & i = j - 3s; \\ 0, & \text{otherwise.} \end{cases}$$

If  $12s \leq j < 13s$ , then

$$b_{ij} = \begin{cases} w_{7(j+m+1)+3 \rightarrow 7(j+m+2)} \otimes w_{7j+6 \rightarrow 7(j+1)}, & i = (j+1)_s; \\ w_{7(j+m+1)+6 \rightarrow 7(j+m+2)} \otimes w_{7j+6 \rightarrow 7(j+1)+1}, & i = 2s + (j+1)_s; \\ e_{7(j+m+2)} \otimes w_{7j+6 \rightarrow 7(j+1)+2}, & i = 3s + (j+1)_s; \\ e_{7(j+m+2)} \otimes w_{7j+6 \rightarrow 7(j+1)+5}, & i = 6s + (j+1)_s; \\ 0, & \text{otherwise.} \end{cases}$$

(15) If  $r_0 = 14$ , then  $\Omega^{14}(Y_t^{(14)})$  is described with  $(7s \times 12s)$ -matrix with the following elements  $b_{ij}$ :

If  $0 \leq j < s$ , then

$$b_{ij} = \begin{cases} e_{7(j+m)+5} \otimes w_{7j \rightarrow 7j+1}, & i = j + s; \\ 0, & \text{otherwise.} \end{cases}$$

If  $s \leq j < 2s$ , then

$$b_{ij} = \begin{cases} w_{7(j+m-1)+6 \rightarrow 7(j+m)+3} \otimes e_{7j}, & i = j - s; \\ w_{7(j+m)+1 \rightarrow 7(j+m)+3} \otimes w_{7j \rightarrow 7j+2}, & i = j + s; \\ 0, & \text{otherwise.} \end{cases}$$

If  $2s \leq j < 3s$ , then  $b_{ij} = 0$ .

If  $3s \leq j < 4s$ , then

$$b_{ij} = \begin{cases} -e_{7(j+m)+6} \otimes w_{7j+1 \rightarrow 7(j+1)}, & i = (j+1)_s; \\ 0, & \text{otherwise.} \end{cases}$$

If  $4s \leq j < 5s$ , then

$$b_{ij} = \begin{cases} -w_{7(j+m)+1 \rightarrow 7(j+m+1)} \otimes e_{7j+2}, & i = j - 2s; \\ 0, & \text{otherwise.} \end{cases}$$

If  $5s \leq j < 6s$ , then

$$b_{ij} = \begin{cases} -w_{7(j+m)+2 \rightarrow 7(j+m)+6} \otimes e_{7j+3}, & i = j - 2s; \\ 0, & \text{otherwise.} \end{cases}$$

If  $6s \leq j < 7s$ , then

$$b_{ij} = \begin{cases} -w_{7(j+m)+3 \rightarrow 7(j+m)+6} \otimes e_{7j+4}, & i = j - 2s; \\ w_{7(j+m)+4 \rightarrow 7(j+m)+6} \otimes w_{7j+4 \rightarrow 7j+5}, & i = j - s; \\ 0, & \text{otherwise.} \end{cases}$$

If  $7s \leq j < 8s$ , then  $b_{ij} = 0$ .

If  $8s \leq j < 9s$ , then

$$b_{ij} = \begin{cases} -e_{7(j+m+1)} \otimes w_{7j+5 \rightarrow 7j+6}, & i = j - 2s; \\ 0, & \text{otherwise.} \end{cases}$$

If  $9s \leq j < 10s$ , then

$$b_{ij} = \begin{cases} w_{7(j+m+1) \rightarrow 7(j+m+1)+2} \otimes e_{7j+6}, & i = j - 3s; \\ 0, & \text{otherwise.} \end{cases}$$

If  $10s \leq j < 11s$ , then  $b_{ij} = 0$ .

If  $11s \leq j < 12s$ , then

$$b_{ij} = \begin{cases} e_{7(j+m+1)+4} \otimes w_{7j+6 \rightarrow 7(j+1)+5}, & i = 5s + (j+1)_s; \\ 0, & \text{otherwise.} \end{cases}$$

(16) If  $r_0 = 15$ , then  $\Omega^{15}(Y_t^{(14)})$  is described with  $(8s \times 12s)$ -matrix with the following elements  $b_{ij}$ :

If  $0 \leq j < s$ , then

$$b_{ij} = \begin{cases} e_{7(j+m)+6} \otimes e_{7j}, & i = j; \\ 0, & \text{otherwise.} \end{cases}$$

If  $s \leq j < 2s$ , then

$$b_{ij} = \begin{cases} w_{7(j+m)+6 \rightarrow 7(j+m+1)} \otimes e_{7j}, & i = j - s; \\ e_{7(j+m+1)} \otimes w_{7j \rightarrow 7j+1}, & i = j; \\ 0, & \text{otherwise.} \end{cases}$$

If  $2s \leq j < 3s$ , then

$$b_{ij} = \begin{cases} w_{7(j+m+1) \rightarrow 7(j+m+1)+2} \otimes e_{7j+1}, & i = j - s; \\ 0, & \text{otherwise.} \end{cases}$$

If  $3s \leq j < 4s$ , then

$$b_{ij} = \begin{cases} w_{7(j+m+1)+1 \rightarrow 7(j+m+1)+3} \otimes e_{7j+2}, & i = j - s; \\ 0, & \text{otherwise.} \end{cases}$$

If  $4s \leq j < 6s$ , then  $b_{ij} = 0$ .

If  $6s \leq j < 7s$ , then

$$b_{ij} = \begin{cases} w_{7(j+m+1) \rightarrow 7(j+m+1)+4} \otimes e_{7j+4}, & i = j - 2s; \\ 0, & \text{otherwise.} \end{cases}$$

If  $7s \leq j < 9s$ , then  $b_{ij} = 0$ .

If  $9s \leq j < 10s$ , then

$$b_{ij} = \begin{cases} w_{7(j+m+1)+4 \rightarrow 7(j+m+1)+5} \otimes e_{7j+5}, & i = j - 4s; \\ 0, & \text{otherwise.} \end{cases}$$

If  $10s \leq j < 11s$ , then

$$b_{ij} = \begin{cases} e_{7(j+m+1)+6} \otimes w_{7j+6 \rightarrow 7(j+1)}, & i = (j+1)_s; \\ w_{7(j+m+1)+3 \rightarrow 7(j+m+1)+6} \otimes e_{7j+6}, & i = j - 4s; \\ 0, & \text{otherwise.} \end{cases}$$

If  $11s \leq j < 12s$ , then  $b_{ij} = 0$ .

(17) If  $r_0 = 16$ , then  $\Omega^{16}(Y_t^{(14)})$  is described with  $(7s \times 10s)$ -matrix with the following elements  $b_{ij}$ :

If  $s \leq j < 2s$ , then

$$b_{ij} = \begin{cases} w_{7(j+m) \rightarrow 7(j+m)+4} \otimes e_{7j}, & i = j - s; \\ 0, & \text{otherwise.} \end{cases}$$

If  $2s \leq j < 3s$ , then

$$b_{ij} = \begin{cases} -e_{7(j+m+1)} \otimes w_{7j+1 \rightarrow 7(j+1)}, & i = (j+1)_s; \\ -w_{7(j+m)+1 \rightarrow 7(j+m+1)} \otimes e_{7j+1}, & i = j - s; \\ 0, & \text{otherwise.} \end{cases}$$

If  $3s \leq j < 4s$ , then

$$b_{ij} = \begin{cases} -w_{7(j+m)+2 \rightarrow 7(j+m)+6} \otimes e_{7j+2}, & i = j - s; \\ w_{7(j+m)+3 \rightarrow 7(j+m)+6} \otimes w_{7j+2 \rightarrow 7j+3}, & i = j; \\ 0, & \text{otherwise.} \end{cases}$$

If  $4s \leq j < 5s$ , then  $b_{ij} = 0$ .

If  $5s \leq j < 6s$ , then

$$b_{ij} = \begin{cases} -w_{7(j+m)+4 \rightarrow 7(j+m+1)} \otimes e_{7j+4}, & i = j - s; \\ 0, & \text{otherwise.} \end{cases}$$

If  $6s \leq j < 7s$ , then

$$b_{ij} = \begin{cases} w_{7(j+m)+5 \rightarrow 7(j+m)+6} \otimes e_{7j+5}, & i = j - s; \\ -e_{7(j+m)+6} \otimes w_{7j+5 \rightarrow 7j+6}, & i = j; \\ 0, & \text{otherwise.} \end{cases}$$

If  $7s \leq j < 8s$ , then

$$b_{ij} = \begin{cases} w_{7(j+m+1) \rightarrow 7(j+m+1)+5} \otimes w_{7j+6 \rightarrow 7(j+1)}, & i = (j+1)_s; \\ w_{7(j+m+1)+4 \rightarrow 7(j+m+1)+5} \otimes w_{7j+6 \rightarrow 7(j+1)+4}, & i = 4s + (j+1)_s; \\ 0, & \text{otherwise.} \end{cases}$$

If  $8s \leq j < 9s$ , then

$$b_{ij} = \begin{cases} w_{7(j+m+1)+1 \rightarrow 7(j+m+1)+3} \otimes w_{7j+6 \rightarrow 7(j+1)+1}, & i = s + (j+1)_s; \\ w_{7(j+m)+6 \rightarrow 7(j+m+1)+3} \otimes e_{7j+6}, & i = j - 2s; \\ 0, & \text{otherwise.} \end{cases}$$

If  $9s \leq j < 10s$ , then  $b_{ij} = 0$ .

(II) Represent an arbitrary  $t_0 \in \mathbb{N}$  in the form  $t_0 = 17\ell_0 + r_0$ , where  $0 \leq r_0 \leq 16$ . Then  $\Omega^{t_0}(Y_t^{(14)})$  is a  $\Omega^{r_0}(Y_t^{(14)})$ , whose left components twisted by  $\sigma^{\ell_0}$ .

**Proposition 12** (Translates for the case 16). (I) Let  $r_0 \in \mathbb{N}$ ,  $r_0 < 17$ .  $r_0$ -translates of the elements  $Y_t^{(16)}$  are described by the following way.

(1) If  $r_0 = 0$ , then  $\Omega^0(Y_t^{(16)})$  is described with  $(7s \times 8s)$ -matrix with the following elements  $b_{ij}$ :  
If  $0 \leq j < s$ , then

$$b_{ij} = \begin{cases} w_{7(j+m) \rightarrow 7(j+m)+6} \otimes e_{7j}, & i = j; \\ 0, & \text{otherwise.} \end{cases}$$

If  $s \leq j < 4s$ , then  $b_{ij} = 0$ .

If  $4s \leq j < 5s$ , then

$$b_{ij} = \begin{cases} -w_{7(j+m)+4 \rightarrow 7(j+m+1)} \otimes e_{7j+4}, & i = j; \\ 0, & \text{otherwise.} \end{cases}$$

If  $5s \leq j < 6s$ , then

$$b_{ij} = \begin{cases} w_{7(j+m)+5 \rightarrow 7(j+m+1)+4} \otimes e_{7j+5}, & i = j; \\ 0, & \text{otherwise.} \end{cases}$$

If  $6s \leq j < 7s$ , then  $b_{ij} = 0$ .

If  $7s \leq j < 8s$ , then

$$b_{ij} = \begin{cases} -w_{7(j+m)+6 \rightarrow 7(j+m+1)+5} \otimes e_{7j+6}, & i = j - s; \\ 0, & \text{otherwise.} \end{cases}$$

(2) If  $r_0 = 1$ , then  $\Omega^1(Y_t^{(16)})$  is described with  $(8s \times 7s)$ -matrix with the following elements  $b_{ij}$ :  
If  $0 \leq j < s$ , then

$$b_{ij} = \begin{cases} -w_{7(j+m)+4 \rightarrow 7(j+m+1)} \otimes e_{7j}, & i = j + s; \\ 0, & \text{otherwise.} \end{cases}$$

If  $s \leq j < 4s$ , then  $b_{ij} = 0$ .

If  $4s \leq j < 5s$ , then

$$b_{ij} = \begin{cases} -w_{7(j+m)+5 \rightarrow 7(j+m+1)+4} \otimes e_{7j+4}, & i = j + s; \\ 0, & \text{otherwise.} \end{cases}$$

If  $5s \leq j < 6s$ , then

$$b_{ij} = \begin{cases} -w_{7(j+m)+6 \rightarrow 7(j+m+1)+5} \otimes e_{7j+5}, & i = j + s; \\ 0, & \text{otherwise.} \end{cases}$$

If  $6s \leq j < 7s$ , then

$$b_{ij} = \begin{cases} -w_{7(j+m+1) \rightarrow 7(j+m+1)+6} \otimes e_{7j+6}, & i = j + s; \\ 0, & \text{otherwise.} \end{cases}$$

(3) If  $r_0 = 2$ , then  $\Omega^2(Y_t^{(16)})$  is described with  $(7s \times 7s)$ -matrix with the following elements  $b_{ij}$ :

If  $0 \leq j < s$ , then

$$b_{ij} = \begin{cases} -w_{7(j+m)+6 \rightarrow 7(j+m+1)} \otimes w_{7j \rightarrow 7(j+1)}, & i = (j+1)_s; \\ w_{7(j+m)+2 \rightarrow 7(j+m+1)} \otimes w_{7j \rightarrow 7j+1}, & i = j+s; \\ 0, & \text{otherwise.} \end{cases}$$

If  $s \leq j < 4s$ , then  $b_{ij} = 0$ .

If  $4s \leq j < 5s$ , then

$$b_{ij} = \begin{cases} -w_{7(j+m)+6 \rightarrow 7(j+m+1)+4} \otimes w_{7j+4 \rightarrow 7(j+1)}, & i = (j+1)_s; \\ 0, & \text{otherwise.} \end{cases}$$

If  $5s \leq j < 6s$ , then

$$b_{ij} = \begin{cases} -w_{7(j+m)+6 \rightarrow 7(j+m+1)+5} \otimes w_{7j+5 \rightarrow 7(j+1)}, & i = (j+1)_s; \\ 0, & \text{otherwise.} \end{cases}$$

If  $6s \leq j < 7s$ , then

$$b_{ij} = \begin{cases} -w_{7(j+m)+6 \rightarrow 7(j+m+1)+6} \otimes w_{7j+6 \rightarrow 7(j+1)}, & i = (j+1)_s; \\ w_{7(j+m+1)+2 \rightarrow 7(j+m+1)+6} \otimes w_{7j+6 \rightarrow 7(j+1)+1}, & i = s + (j+1)_s; \\ 0, & \text{otherwise.} \end{cases}$$

(4) If  $r_0 = 3$ , then  $\Omega^3(Y_t^{(16)})$  is described with  $(9s \times 8s)$ -matrix with the following elements  $b_{ij}$ :  
If  $0 \leq j < s$ , then

$$b_{ij} = \begin{cases} w_{7(j+m)+3 \rightarrow 7(j+m+1)+1} \otimes w_{7j \rightarrow 7j+1}, & i = j+2s; \\ w_{7(j+m)+6 \rightarrow 7(j+m+1)+1} \otimes w_{7j \rightarrow 7j+2}, & i = j+3s; \\ 0, & \text{otherwise.} \end{cases}$$

If  $s \leq j < 4s$ , then  $b_{ij} = 0$ .

If  $4s \leq j < 5s$ , then

$$b_{ij} = \begin{cases} w_{7(j+m+1)+2 \rightarrow 7(j+m+1)+6} \otimes w_{7j+3 \rightarrow 7(j+1)}, & i = (j+1)_s; \\ 0, & \text{otherwise.} \end{cases}$$

If  $5s \leq j < 8s$ , then  $b_{ij} = 0$ .

(5) If  $r_0 = 4$ , then  $\Omega^4(Y_t^{(16)})$  is described with  $(10s \times 7s)$ -matrix with the following elements  $b_{ij}$ :

If  $0 \leq j < s$ , then

$$b_{ij} = \begin{cases} w_{7(j+m)+3 \rightarrow 7(j+m)+6} \otimes w_{7j \rightarrow 7j+1}, & i = j+2s; \\ 0, & \text{otherwise.} \end{cases}$$

If  $s \leq j < 2s$ , then

$$b_{ij} = \begin{cases} w_{7(j+m)+6 \rightarrow 7(j+m+1)+2} \otimes w_{7j+1 \rightarrow 7(j+1)}, & i = (j+1)_s; \\ 0, & \text{otherwise.} \end{cases}$$

If  $2s \leq j < 3s$ , then

$$b_{ij} = \begin{cases} w_{7(j+m)+6 \rightarrow 7(j+m+1)+3} \otimes w_{7j+2 \rightarrow 7(j+1)}, & i = (j+1)_s; \\ 0, & \text{otherwise.} \end{cases}$$

If  $3s \leq j < 7s$ , then  $b_{ij} = 0$ .

(6) If  $r_0 = 5$ , then  $\Omega^5(Y_t^{(16)})$  is described with  $(10s \times 9s)$ -matrix with the following elements  $b_{ij}$ :

If  $0 \leq j < s$ , then

$$b_{ij} = \begin{cases} w_{7(j+m)+6 \rightarrow 7(j+m+1)+2} \otimes w_{7j \rightarrow 7j+1}, & i = j + 3s; \\ 0, & \text{otherwise.} \end{cases}$$

If  $s \leq j < 3s$ , then  $b_{ij} = 0$ .

If  $3s \leq j < 4s$ , then

$$b_{ij} = \begin{cases} w_{7(j+m+1)+3 \rightarrow 7(j+m+1)+6} \otimes w_{7j+2 \rightarrow 7(j+1)}, & i = s + (j+1)_s; \\ 0, & \text{otherwise.} \end{cases}$$

If  $4s \leq j < 5s$ , then

$$b_{ij} = \begin{cases} -w_{7(j+m+1)+3 \rightarrow 7(j+m+2)} \otimes w_{7j+3 \rightarrow 7(j+1)}, & i = s + (j+1)_s; \\ 0, & \text{otherwise.} \end{cases}$$

If  $5s \leq j < 7s$ , then  $b_{ij} = 0$ .

If  $7s \leq j < 8s$ , then

$$b_{ij} = \begin{cases} -w_{7(j+m+1)+6 \rightarrow 7(j+m+2)+1} \otimes w_{7j+6 \rightarrow 7(j+1)+1}, & i = 3s + (j+1)_s; \\ 0, & \text{otherwise.} \end{cases}$$

If  $8s \leq j < 9s$ , then  $b_{ij} = 0$ .

(7) If  $r_0 = 6$ , then  $\Omega^6(Y_t^{(16)})$  is described with  $(12s \times 10s)$ -matrix with the following elements  $b_{ij}$ :

If  $0 \leq j < s$ , then

$$b_{ij} = \begin{cases} -e_{7(j+m)+6} \otimes w_{7j \rightarrow 7(j+1)}, & i = (j+1)_s; \\ w_{7(j+m)+4 \rightarrow 7(j+m)+6} \otimes w_{7j \rightarrow 7j+1}, & i = j + 2s; \\ -w_{7(j+m)+1 \rightarrow 7(j+m)+6} \otimes w_{7j \rightarrow 7j+2}, & i = j + 3s; \\ 0, & \text{otherwise.} \end{cases}$$

If  $s \leq j < 2s$ , then

$$b_{ij} = \begin{cases} -e_{7(j+m+1)} \otimes w_{7j \rightarrow 7(j+1)}, & i = s + (j+1)_s; \\ 0, & \text{otherwise.} \end{cases}$$

If  $2s \leq j < 3s$ , then

$$b_{ij} = \begin{cases} -w_{7(j+m)+6 \rightarrow 7(j+m+1)+3} \otimes w_{7j+1 \rightarrow 7(j+1)}, & i = (j+1)_s; \\ 0, & \text{otherwise.} \end{cases}$$

If  $3s \leq j < 4s$ , then  $b_{ij} = 0$ .

If  $4s \leq j < 5s$ , then

$$b_{ij} = \begin{cases} -w_{7(j+m+1) \rightarrow 7(j+m+1)+1} \otimes w_{7j+3 \rightarrow 7(j+1)}, & i = s + (j+1)_s; \\ e_{7(j+m+1)+1} \otimes w_{7j+3 \rightarrow 7(j+1)+2}, & i = 3s + (j+1)_s; \\ 0, & \text{otherwise.} \end{cases}$$

If  $5s \leq j < 10s$ , then  $b_{ij} = 0$ .

(8) If  $r_0 = 7$ , then  $\Omega^7(Y_t^{(16)})$  is described with  $(12s \times 10s)$ -matrix with the following elements  $b_{ij}$ :

If  $0 \leq j < s$ , then

$$b_{ij} = \begin{cases} w_{7(j+m+1) \rightarrow 7(j+m+1)+4} \otimes w_{7j \rightarrow 7j+1}, & i = j + 3s; \\ 0, & \text{otherwise.} \end{cases}$$

If  $s \leq j < 3s$ , then  $b_{ij} = 0$ .

If  $3s \leq j < 4s$ , then

$$b_{ij} = \begin{cases} -w_{7(j+m+1)+5 \rightarrow 7(j+m+1)+6} \otimes w_{7j+1 \rightarrow 7(j+1)}, & i = s + (j+1)_s; \\ 0, & \text{otherwise.} \end{cases}$$

If  $4s \leq j < 5s$ , then  $b_{ij} = 0$ .

If  $5s \leq j < 6s$ , then

$$b_{ij} = \begin{cases} -w_{7(j+m+1)+4 \rightarrow 7(j+m+1)+6} \otimes w_{7j+3 \rightarrow 7(j+1)}, & i = 2s + (j+1)_s; \\ 0, & \text{otherwise.} \end{cases}$$

If  $6s \leq j < 10s$ , then  $b_{ij} = 0$ .

(9) If  $r_0 = 8$ , then  $\Omega^8(Y_t^{(16)})$  is described with  $(13s \times 12s)$ -matrix with the following elements  $b_{ij}$ :

If  $0 \leq j < s$ , then

$$b_{ij} = \begin{cases} w_{7(j+m)+5 \rightarrow 7(j+m)+6} \otimes w_{7j \rightarrow 7j+1}, & i = j + 3s; \\ 0, & \text{otherwise.} \end{cases}$$

If  $s \leq j < 2s$ , then

$$b_{ij} = \begin{cases} -e_{7(j+m+1)} \otimes w_{7j \rightarrow 7(j+1)}, & i = s + (j+1)_s; \\ 0, & \text{otherwise.} \end{cases}$$

If  $2s \leq j < 3s$ , then

$$b_{ij} = \begin{cases} -w_{7(j+m+1) \rightarrow 7(j+m+1)+4} \otimes w_{7j+1 \rightarrow 7(j+1)}, & i = s + (j+1)_s; \\ 0, & \text{otherwise.} \end{cases}$$

If  $3s \leq j < 4s$ , then  $b_{ij} = 0$ .

If  $4s \leq j < 5s$ , then

$$b_{ij} = \begin{cases} -w_{7(j+m)+6 \rightarrow 7(j+m+1)+5} \otimes w_{7j+2 \rightarrow 7(j+1)}, & i = (j+1)_s; \\ -w_{7(j+m+1) \rightarrow 7(j+m+1)+5} \otimes w_{7j+2 \rightarrow 7(j+1)}, & i = s + (j+1)_s; \\ 0, & \text{otherwise.} \end{cases}$$

If  $5s \leq j < 12s$ , then  $b_{ij} = 0$ .

(10) If  $r_0 = 9$ , then  $\Omega^9(Y_t^{(16)})$  is described with  $(12s \times 12s)$ -matrix with the following elements  $b_{ij}$ :

If  $0 \leq j < s$ , then

$$b_{ij} = \begin{cases} -w_{7(j+m+1)+1 \rightarrow 7(j+m+1)+2} \otimes w_{7j \rightarrow 7(j+1)}, & i = 2s + (j+1)_s; \\ 0, & \text{otherwise.} \end{cases}$$

If  $s \leq j < 2s$ , then

$$b_{ij} = \begin{cases} -w_{7(j+m)+6 \rightarrow 7(j+m+1)+5} \otimes w_{7j \rightarrow 7j+1}, & i = j + 2s; \\ 0, & \text{otherwise.} \end{cases}$$

If  $2s \leq j < 3s$ , then  $b_{ij} = 0$ .

If  $3s \leq j < 4s$ , then

$$b_{ij} = \begin{cases} -w_{7(j+m+1)+5 \rightarrow 7(j+m+2)} \otimes w_{7j+1 \rightarrow 7(j+1)}, & i = (j+1)_s; \\ 0, & \text{otherwise.} \end{cases}$$

If  $4s \leq j < 5s$ , then

$$b_{ij} = \begin{cases} w_{7(j+m+1)+5 \rightarrow 7(j+m+1)+6} \otimes w_{7j+2 \rightarrow 7(j+1)}, & i = (j+1)_s; \\ 0, & \text{otherwise.} \end{cases}$$

If  $5s \leq j < 12s$ , then  $b_{ij} = 0$ .

(11) If  $r_0 = 10$ , then  $\Omega^{10}(Y_t^{(16)})$  is described with  $(12s \times 13s)$ -matrix with the following elements  $b_{ij}$ :

If  $0 \leq j < s$ , then

$$b_{ij} = \begin{cases} e_{7(j+m)+6} \otimes w_{7j \rightarrow 7(j+1)}, & i = (j+1)_s; \\ w_{7(j+m)+2 \rightarrow 7(j+m)+6} \otimes w_{7j \rightarrow 7j+1}, & i = j + 2s; \\ -w_{7(j+m)+3 \rightarrow 7(j+m)+6} \otimes w_{7j \rightarrow 7j+2}, & i = j + 3s; \\ 0, & \text{otherwise.} \end{cases}$$

If  $s \leq j < 3s$ , then  $b_{ij} = 0$ .

If  $3s \leq j < 4s$ , then

$$b_{ij} = \begin{cases} -w_{7(j+m)+6 \rightarrow 7(j+m+1)+5} \otimes w_{7j+1 \rightarrow 7(j+1)}, & i = (j+1)_s; \\ 0, & \text{otherwise.} \end{cases}$$

If  $4s \leq j < 13s$ , then  $b_{ij} = 0$ .

(12) If  $r_0 = 11$ , then  $\Omega^{11}(Y_t^{(16)})$  is described with  $(10s \times 12s)$ -matrix with the following elements  $b_{ij}$ :

If  $s \leq j < 2s$ , then

$$b_{ij} = \begin{cases} w_{7(j+m+1)+2 \rightarrow 7(j+m+1)+3} \otimes w_{7j \rightarrow 7(j+1)}, & i = (j+1)_s; \\ w_{7(j+m+1) \rightarrow 7(j+m+1)+3} \otimes w_{7j \rightarrow 7j+1}, & i = j + s; \\ 0, & \text{otherwise.} \end{cases}$$

If  $2s \leq j < 3s$ , then  $b_{ij} = 0$ .



If  $3s \leq j < 4s$ , then

$$b_{ij} = \begin{cases} w_{7(j+m+1)+2 \rightarrow 7(j+m+1)+6} \otimes w_{7j+1 \rightarrow 7(j+1)}, & i = (j+1)_s; \\ -w_{7(j+m+1)+4 \rightarrow 7(j+m+1)+6} \otimes w_{7j+1 \rightarrow 7(j+1)}, & i = s + (j+1)_s; \\ 0, & \text{otherwise.} \end{cases}$$

If  $4s \leq j < 5s$ , then

$$b_{ij} = \begin{cases} e_{7(j+m+2)} \otimes w_{7j+2 \rightarrow 7(j+1)+1}, & i = 2s + (j+1)_s; \\ 0, & \text{otherwise.} \end{cases}$$

If  $5s \leq j < 12s$ , then  $b_{ij} = 0$ .

(13) If  $r_0 = 12$ , then  $\Omega^{12}(Y_t^{(16)})$  is described with  $(10s \times 12s)$ -matrix with the following elements  $b_{ij}$ :

If  $0 \leq j < s$ , then

$$b_{ij} = \begin{cases} -w_{7(j+m)+4 \rightarrow 7(j+m)+6} \otimes w_{7j \rightarrow 7j+1}, & i = j + 2s; \\ 0, & \text{otherwise.} \end{cases}$$

If  $s \leq j < 2s$ , then

$$b_{ij} = \begin{cases} e_{7(j+m+1)} \otimes w_{7j \rightarrow 7(j+1)}, & i = (j+1)_s; \\ w_{7(j+m)+4 \rightarrow 7(j+m+1)} \otimes w_{7j \rightarrow 7j+1}, & i = j + s; \\ 0, & \text{otherwise.} \end{cases}$$

If  $2s \leq j < 3s$ , then

$$b_{ij} = \begin{cases} w_{7(j+m+1) \rightarrow 7(j+m+1)+2} \otimes w_{7j+1 \rightarrow 7(j+1)}, & i = (j+1)_s; \\ 0, & \text{otherwise.} \end{cases}$$

If  $3s \leq j < 4s$ , then  $b_{ij} = 0$ .

If  $4s \leq j < 5s$ , then

$$b_{ij} = \begin{cases} e_{7(j+m+1)+4} \otimes w_{7j+2 \rightarrow 7(j+1)+1}, & i = 2s + (j+1)_s; \\ 0, & \text{otherwise.} \end{cases}$$

If  $5s \leq j < 12s$ , then  $b_{ij} = 0$ .

(14) If  $r_0 = 13$ , then  $\Omega^{13}(Y_t^{(16)})$  is described with  $(9s \times 10s)$ -matrix with the following elements  $b_{ij}$ :

If  $s \leq j < 2s$ , then

$$b_{ij} = \begin{cases} -w_{7(j+m)+6 \rightarrow 7(j+m+1)+4} \otimes w_{7j \rightarrow 7j+1}, & i = j + s; \\ -w_{7(j+m+1) \rightarrow 7(j+m+1)+4} \otimes w_{7j \rightarrow 7j+2}, & i = j + 2s; \\ -w_{7(j+m+1) \rightarrow 7(j+m+1)+4} \otimes w_{7j \rightarrow 7j+5}, & i = j + 5s; \\ 0, & \text{otherwise.} \end{cases}$$

If  $2s \leq j < 3s$ , then

$$b_{ij} = \begin{cases} w_{7(j+m+1)+5 \rightarrow 7(j+m+2)} \otimes w_{7j+1 \rightarrow 7(j+1)}, & i = s + (j+1)_s; \\ 0, & \text{otherwise.} \end{cases}$$

If  $3s \leq j < 10s$ , then  $b_{ij} = 0$ .

(15) If  $r_0 = 14$ , then  $\Omega^{14}(Y_t^{(16)})$  is described with  $(7s \times 10s)$ -matrix with the following elements  $b_{ij}$ :

If  $0 \leq j < s$ , then

$$b_{ij} = \begin{cases} -w_{7(j+m)+6 \rightarrow 7(j+m+1)} \otimes w_{7j \rightarrow 7(j+1)}, & i = (j+1)_s; \\ w_{7(j+m)+1 \rightarrow 7(j+m+1)} \otimes w_{7j \rightarrow 7j+2}, & i = j+2s; \\ -w_{7(j+m)+2 \rightarrow 7(j+m+1)} \otimes w_{7j \rightarrow 7j+3}, & i = j+3s; \\ w_{7(j+m)+3 \rightarrow 7(j+m+1)} \otimes w_{7j \rightarrow 7j+4}, & i = j+4s; \\ 0, & \text{otherwise.} \end{cases}$$

If  $s \leq j < 2s$ , then  $b_{ij} = 0$ .

If  $2s \leq j < 3s$ , then

$$b_{ij} = \begin{cases} -w_{7(j+m)+6 \rightarrow 7(j+m+1)+4} \otimes w_{7j+1 \rightarrow 7(j+1)}, & i = (j+1)_s; \\ 0, & \text{otherwise.} \end{cases}$$

If  $3s \leq j < 4s$ , then

$$b_{ij} = \begin{cases} e_{7(j+m+1)+5} \otimes w_{7j+2 \rightarrow 7(j+1)+1}, & i = s + (j+1)_s; \\ 0, & \text{otherwise.} \end{cases}$$

If  $4s \leq j < 10s$ , then  $b_{ij} = 0$ .

(16) If  $r_0 = 15$ , then  $\Omega^{15}(Y_t^{(16)})$  is described with  $(8s \times 9s)$ -matrix with the following elements  $b_{ij}$ :

If  $0 \leq j < s$ , then

$$b_{ij} = \begin{cases} -w_{7(j+m+1) \rightarrow 7(j+m+1)+3} \otimes w_{7j \rightarrow 7j+1}, & i = j+s; \\ w_{7(j+m+1) \rightarrow 7(j+m+1)+3} \otimes w_{7j \rightarrow 7j+4}, & i = j+4s; \\ 0, & \text{otherwise.} \end{cases}$$

If  $s \leq j < 2s$ , then  $b_{ij} = 0$ .

If  $2s \leq j < 3s$ , then

$$b_{ij} = \begin{cases} e_{7(j+m+1)+6} \otimes w_{7j+1 \rightarrow 7(j+1)}, & i = (j+1)_s; \\ 0, & \text{otherwise.} \end{cases}$$

If  $3s \leq j < 4s$ , then

$$b_{ij} = \begin{cases} -w_{7(j+m+1)+6 \rightarrow 7(j+m+2)} \otimes w_{7j+2 \rightarrow 7(j+1)}, & i = (j+1)_s; \\ 0, & \text{otherwise.} \end{cases}$$

If  $4s \leq j < 5s$ , then

$$b_{ij} = \begin{cases} w_{7(j+m+1)+6 \rightarrow 7(j+m+2)+1} \otimes w_{7j+3 \rightarrow 7(j+1)}, & i = (j+1)_s; \\ 0, & \text{otherwise.} \end{cases}$$

If  $5s \leq j < 7s$ , then  $b_{ij} = 0$ .

If  $7s \leq j < 8s$ , then

$$b_{ij} = \begin{cases} -w_{7(j+m+1)+6 \rightarrow 7(j+m+2)+2} \otimes w_{7j+6 \rightarrow 7(j+1)}, & i = (j+1)_s; \\ 0, & \text{otherwise.} \end{cases}$$

If  $8s \leq j < 9s$ , then  $b_{ij} = 0$ .

(17) If  $r_0 = 16$ , then  $\Omega^{16}(Y_t^{(16)})$  is described with  $(7s \times 7s)$ -matrix with the following elements  $b_{ij}$ :

If  $0 \leq j < s$ , then

$$b_{ij} = \begin{cases} -w_{7(j+m)+1 \rightarrow 7(j+m)+6} \otimes w_{7j \rightarrow 7j+1}, & i = j + s; \\ w_{7(j+m)+2 \rightarrow 7(j+m)+6} \otimes w_{7j \rightarrow 7j+2}, & i = j + 2s; \\ -w_{7(j+m)+3 \rightarrow 7(j+m)+6} \otimes w_{7j \rightarrow 7j+3}, & i = j + 3s; \\ w_{7(j+m)+4 \rightarrow 7(j+m)+6} \otimes w_{7j \rightarrow 7j+4}, & i = j + 4s; \\ -w_{7(j+m)+5 \rightarrow 7(j+m)+6} \otimes w_{7j \rightarrow 7j+5}, & i = j + 5s; \\ e_{7(j+m)+6} \otimes w_{7j \rightarrow 7j+6}, & i = j + 6s; \\ 0, & \text{otherwise.} \end{cases}$$

If  $s \leq j < 4s$ , then  $b_{ij} = 0$ .

If  $4s \leq j < 5s$ , then

$$b_{ij} = \begin{cases} -w_{7(j+m+1) \rightarrow 7(j+m+1)+3} \otimes w_{7j+4 \rightarrow 7(j+1)}, & i = (j+1)s; \\ 0, & \text{otherwise.} \end{cases}$$

If  $5s \leq j < 6s$ , then  $b_{ij} = 0$ .

If  $6s \leq j < 7s$ , then

$$b_{ij} = \begin{cases} -w_{7(j+m+1)+1 \rightarrow 7(j+m+2)} \otimes w_{7j+6 \rightarrow 7(j+1)+1}, & i = s + (j+1)s; \\ w_{7(j+m+1)+2 \rightarrow 7(j+m+2)} \otimes w_{7j+6 \rightarrow 7(j+1)+2}, & i = 2s + (j+1)s; \\ -w_{7(j+m+1)+3 \rightarrow 7(j+m+2)} \otimes w_{7j+6 \rightarrow 7(j+1)+3}, & i = 3s + (j+1)s; \\ w_{7(j+m+1)+4 \rightarrow 7(j+m+2)} \otimes w_{7j+6 \rightarrow 7(j+1)+4}, & i = 4s + (j+1)s; \\ -w_{7(j+m+1)+5 \rightarrow 7(j+m+2)} \otimes w_{7j+6 \rightarrow 7(j+1)+5}, & i = 5s + (j+1)s; \\ w_{7(j+m+1)+6 \rightarrow 7(j+m+2)} \otimes w_{7j+6 \rightarrow 7(j+1)+6}, & i = 6s + (j+1)s; \\ 0, & \text{otherwise.} \end{cases}$$

(II) Represent an arbitrary  $t_0 \in \mathbb{N}$  in the form  $t_0 = 17\ell_0 + r_0$ , where  $0 \leq r_0 \leq 16$ . Then  $\Omega^{t_0}(Y_t^{(16)})$  is a  $\Omega^{r_0}(Y_t^{(16)})$ , whose left components twisted by  $\sigma^{\ell_0}$ .

**Proposition 13** (Translates for the case 17). (I) Let  $r_0 \in \mathbb{N}$ ,  $r_0 < 17$ .  $r_0$ -translates of the elements  $Y_t^{(17)}$  are described by the following way.

(1) If  $r_0 = 0$ , then  $\Omega^0(Y_t^{(17)})$  is described with  $(7s \times 7s)$ -matrix with the following elements  $b_{ij}$ :

If  $0 \leq j < s$ , then

$$b_{ij} = \begin{cases} e_{7(j+m)} \otimes e_{7j}, & i = j; \\ 0, & \text{otherwise.} \end{cases}$$

If  $s \leq j < 2s$ , then

$$b_{ij} = \begin{cases} e_{7(j+m)+1} \otimes e_{7j+1}, & i = j; \\ 0, & \text{otherwise.} \end{cases}$$

If  $2s \leq j < 3s$ , then

$$b_{ij} = \begin{cases} e_{7(j+m)+2} \otimes e_{7j+2}, & i = j; \\ 0, & \text{otherwise.} \end{cases}$$

If  $3s \leq j < 4s$ , then

$$b_{ij} = \begin{cases} e_{7(j+m)+3} \otimes e_{7j+3}, & i = j; \\ 0, & \text{otherwise.} \end{cases}$$

If  $4s \leq j < 6s$ , then  $b_{ij} = 0$ .

If  $6s \leq j < 7s$ , then

$$b_{ij} = \begin{cases} e_{7(j+m)+6} \otimes e_{7j+6}, & i = j; \\ 0, & \text{otherwise.} \end{cases}$$

(2) If  $r_0 = 1$ , then  $\Omega^1(Y_t^{(17)})$  is described with  $(8s \times 7s)$ -matrix with the following elements  $b_{ij}$ :  
If  $0 \leq j < s$ , then

$$b_{ij} = \begin{cases} w_{7(j+m)+1 \rightarrow 7(j+m+1)} \otimes e_{7j}, & i = j; \\ w_{7(j+m)+3 \rightarrow 7(j+m+1)} \otimes w_{7j \rightarrow 7j+2}, & i = j + 3s; \\ e_{7(j+m+1)} \otimes w_{7j \rightarrow 7j+6}, & i = j + 7s; \\ 0, & \text{otherwise.} \end{cases}$$

If  $s \leq j < 2s$ , then

$$b_{ij} = \begin{cases} e_{7(j+m+1)+1} \otimes w_{7j+1 \rightarrow 7(j+1)}, & i = (j+1)_s; \\ w_{7(j+m)+2 \rightarrow 7(j+m+1)+1} \otimes e_{7j+1}, & i = j + s; \\ w_{7(j+m)+6 \rightarrow 7(j+m+1)+1} \otimes w_{7j+1 \rightarrow 7j+3}, & i = j + 3s; \\ 0, & \text{otherwise.} \end{cases}$$

If  $2s \leq j < 3s$ , then

$$b_{ij} = \begin{cases} e_{7(j+m+1)+2} \otimes w_{7j+2 \rightarrow 7(j+1)+1}, & i = 2s + (j+1)_s; \\ w_{7(j+m)+3 \rightarrow 7(j+m+1)+2} \otimes e_{7j+2}, & i = j + s; \\ w_{7(j+m+1) \rightarrow 7(j+m+1)+2} \otimes w_{7j+2 \rightarrow 7j+6}, & i = j + 5s; \\ 0, & \text{otherwise.} \end{cases}$$

If  $3s \leq j < 4s$ , then

$$b_{ij} = \begin{cases} w_{7(j+m+1)+1 \rightarrow 7(j+m+1)+3} \otimes w_{7j+3 \rightarrow 7(j+1)}, & i = (j+1)_s; \\ e_{7(j+m+1)+3} \otimes w_{7j+3 \rightarrow 7(j+1)+2}, & i = 3s + (j+1)_s; \\ w_{7(j+m)+6 \rightarrow 7(j+m+1)+3} \otimes e_{7j+3}, & i = j + s; \\ 0, & \text{otherwise.} \end{cases}$$

If  $4s \leq j < 5s$ , then

$$b_{ij} = \begin{cases} w_{7(j+m+1) \rightarrow 7(j+m+1)+4} \otimes w_{7j+4 \rightarrow 7j+6}, & i = j + 3s; \\ 0, & \text{otherwise.} \end{cases}$$

If  $5s \leq j < 6s$ , then

$$b_{ij} = \begin{cases} -w_{7(j+m+1) \rightarrow 7(j+m+1)+5} \otimes w_{7j+5 \rightarrow 7j+6}, & i = j + 2s; \\ 0, & \text{otherwise.} \end{cases}$$

If  $6s \leq j < 7s$ , then

$$b_{ij} = \begin{cases} w_{7(j+m+1)+2 \rightarrow 7(j+m+1)+6} \otimes w_{7j+6 \rightarrow 7(j+1)+1}, & i = 2s + (j+1)_s; \\ e_{7(j+m+1)+6} \otimes w_{7j+6 \rightarrow 7(j+1)+3}, & i = 4s + (j+1)_s; \\ w_{7(j+m+1) \rightarrow 7(j+m+1)+6} \otimes e_{7j+6}, & i = j + s; \\ 0, & \text{otherwise.} \end{cases}$$

(3) If  $r_0 = 2$ , then  $\Omega^2(Y_t^{(17)})$  is described with  $(7s \times 8s)$ -matrix with the following elements  $b_{ij}$ :  
If  $0 \leq j < s$ , then

$$b_{ij} = \begin{cases} -w_{7(j+m-1)+6 \rightarrow 7(j+m)+1} \otimes e_{7j}, & i = j; \\ -e_{7(j+m)+1} \otimes w_{7j \rightarrow 7j+5}, & i = j + 5s; \\ 0, & \text{otherwise.} \end{cases}$$

If  $s \leq j < 2s$ , then  $b_{ij} = 0$ .

If  $2s \leq j < 3s$ , then

$$b_{ij} = \begin{cases} -e_{7(j+m)+2} \otimes e_{7j+1}, & i = j - s; \\ 0, & \text{otherwise.} \end{cases}$$

If  $3s \leq j < 4s$ , then

$$b_{ij} = \begin{cases} -e_{7(j+m)+3} \otimes e_{7j+2}, & i = j - s; \\ 0, & \text{otherwise.} \end{cases}$$

If  $4s \leq j < 5s$ , then

$$b_{ij} = \begin{cases} -e_{7(j+m)+6} \otimes w_{7j+3 \rightarrow 7(j+1)}, & i = (j+1)_s; \\ -w_{7(j+m)+4 \rightarrow 7(j+m)+6} \otimes e_{7j+3}, & i = j - s; \\ 0, & \text{otherwise.} \end{cases}$$

If  $5s \leq j < 7s$ , then  $b_{ij} = 0$ .

If  $7s \leq j < 8s$ , then

$$b_{ij} = \begin{cases} -e_{7(j+m+1)} \otimes e_{7j+6}, & i = j - s; \\ 0, & \text{otherwise.} \end{cases}$$

(4) If  $r_0 = 3$ , then  $\Omega^3(Y_t^{(17)})$  is described with  $(9s \times 7s)$ -matrix with the following elements  $b_{ij}$ :  
If  $0 \leq j < s$ , then

$$b_{ij} = \begin{cases} w_{7(j+m)+2 \rightarrow 7(j+m)+6} \otimes e_{7j}, & i = j; \\ e_{7(j+m)+6} \otimes w_{7j \rightarrow 7j+2}, & i = j + 3s; \\ 0, & \text{otherwise.} \end{cases}$$

If  $s \leq j < 2s$ , then

$$b_{ij} = \begin{cases} e_{7(j+m+1)+2} \otimes w_{7j+1 \rightarrow 7(j+1)}, & i = (j+1)_s; \\ w_{7(j+m)+3 \rightarrow 7(j+m+1)+2} \otimes e_{7j+1}, & i = j + s; \\ w_{7(j+m+1) \rightarrow 7(j+m+1)+2} \otimes w_{7j+1 \rightarrow 7j+3}, & i = j + 3s; \\ 0, & \text{otherwise.} \end{cases}$$

If  $2s \leq j < 3s$ , then

$$b_{ij} = \begin{cases} e_{7(j+m+1)+3} \otimes w_{7j+2 \rightarrow 7(j+1)+1}, & i = 2s + (j+1)_s; \\ w_{7(j+m)+6 \rightarrow 7(j+m+1)+3} \otimes e_{7j+2}, & i = j + s; \\ -w_{7(j+m+1) \rightarrow 7(j+m+1)+3} \otimes w_{7j+2 \rightarrow 7j+3}, & i = j + 2s; \\ 0, & \text{otherwise.} \end{cases}$$

If  $3s \leq j < 4s$ , then

$$b_{ij} = \begin{cases} w_{7(j+m+1) \rightarrow 7(j+m+1)+4} \otimes e_{7j+3}, & i = j + s; \\ 0, & \text{otherwise.} \end{cases}$$

If  $4s \leq j < 5s$ , then

$$b_{ij} = \begin{cases} -w_{7(j+m+1) \rightarrow 7(j+m+1)+5} \otimes w_{7j+4 \rightarrow 7j+5}, & i = j + 2s; \\ 0, & \text{otherwise.} \end{cases}$$

If  $5s \leq j < 6s$ , then

$$b_{ij} = \begin{cases} e_{7(j+m+1)+1} \otimes w_{7j+5 \rightarrow 7j+6}, & i = j + 2s; \\ 0, & \text{otherwise.} \end{cases}$$

If  $6s \leq j < 7s$ , then

$$b_{ij} = \begin{cases} w_{7(j+m+1)+3 \rightarrow 7(j+m+2)} \otimes w_{7j+6 \rightarrow 7(j+1)+1}, & i = 2s + (j+1)_s; \\ e_{7(j+m+2)} \otimes w_{7j+6 \rightarrow 7(j+1)+3}, & i = 4s + (j+1)_s; \\ w_{7(j+m+1)+1 \rightarrow 7(j+m+2)} \otimes e_{7j+6}, & i = j + s; \\ 0, & \text{otherwise.} \end{cases}$$

(5) If  $r_0 = 4$ , then  $\Omega^4(Y_t^{(17)})$  is described with  $(10s \times 9s)$ -matrix with the following elements  $b_{ij}$ :

If  $0 \leq j < s$ , then

$$b_{ij} = \begin{cases} -w_{7(j+m-1)+6 \rightarrow 7(j+m)+2} \otimes e_{7j}, & i = j; \\ -w_{7(j+m) \rightarrow 7(j+m)+2} \otimes e_{7j}, & i = j + s; \\ -e_{7(j+m)+2} \otimes w_{7j \rightarrow 7j+5}, & i = j + 7s; \\ 0, & \text{otherwise.} \end{cases}$$

If  $s \leq j < 2s$ , then

$$b_{ij} = \begin{cases} w_{7(j+m-1)+6 \rightarrow 7(j+m)+5} \otimes e_{7j}, & i = j - s; \\ w_{7(j+m) \rightarrow 7(j+m)+5} \otimes e_{7j}, & i = j; \\ 0, & \text{otherwise.} \end{cases}$$

If  $2s \leq j < 3s$ , then

$$b_{ij} = \begin{cases} -e_{7(j+m)+3} \otimes e_{7j+1}, & i = j; \\ 0, & \text{otherwise.} \end{cases}$$

If  $3s \leq j < 4s$ , then

$$b_{ij} = \begin{cases} -e_{7(j+m)+6} \otimes w_{7j+2 \rightarrow 7(j+1)}, & i = (j+1)_s; \\ -w_{7(j+m)+4 \rightarrow 7(j+m)+6} \otimes e_{7j+2}, & i = j; \\ w_{7(j+m)+5 \rightarrow 7(j+m)+6} \otimes w_{7j+2 \rightarrow 7j+3}, & i = j+2s; \\ 0, & \text{otherwise.} \end{cases}$$

If  $4s \leq j < 5s$ , then

$$b_{ij} = \begin{cases} -w_{7(j+m)+6 \rightarrow 7(j+m)+1} \otimes w_{7j+3 \rightarrow 7(j+1)}, & i = (j+1)_s; \\ -e_{7(j+m)+1} \otimes w_{7j+3 \rightarrow 7(j+1)}, & i = s + (j+1)_s; \\ -w_{7(j+m)+1 \rightarrow 7(j+m)+1} \otimes e_{7j+3}, & i = j; \\ 0, & \text{otherwise.} \end{cases}$$

If  $5s \leq j < 6s$ , then

$$b_{ij} = \begin{cases} w_{7(j+m)+2 \rightarrow 7(j+m)+6} \otimes w_{7j+4 \rightarrow 7j+5}, & i = j+2s; \\ 0, & \text{otherwise.} \end{cases}$$

If  $6s \leq j < 7s$ , then  $b_{ij} = 0$ .

If  $7s \leq j < 8s$ , then

$$b_{ij} = \begin{cases} -e_{7(j+m)+1} \otimes w_{7j+6 \rightarrow 7(j+1)+3}, & i = 4s + (j+1)_s; \\ -w_{7(j+m)+6 \rightarrow 7(j+m)+1} \otimes e_{7j+6}, & i = j+2s; \\ 0, & \text{otherwise.} \end{cases}$$

If  $8s \leq j < 9s$ , then  $b_{ij} = 0$ .

(6) If  $r_0 = 5$ , then  $\Omega^5(Y_t^{(17)})$  is described with  $(10s \times 10s)$ -matrix with the following elements  $b_{ij}$ :

If  $0 \leq j < s$ , then

$$b_{ij} = \begin{cases} e_{7(j+m)+6} \otimes w_{7j \rightarrow 7j+1}, & i = j+3s; \\ 0, & \text{otherwise.} \end{cases}$$

If  $s \leq j < 2s$ , then

$$b_{ij} = \begin{cases} w_{7(j+m)+3 \rightarrow 7(j+m)+1} \otimes e_{7j}, & i = j; \\ w_{7(j+m)+1 \rightarrow 7(j+m)+1} \otimes e_{7j}, & i = j+s; \\ w_{7(j+m)+6 \rightarrow 7(j+m)+1} \otimes w_{7j \rightarrow 7j+1}, & i = j+2s; \\ e_{7(j+m)+1} \otimes w_{7j \rightarrow 7j+2}, & i = j+3s; \\ 0, & \text{otherwise.} \end{cases}$$

If  $2s \leq j < 3s$ , then

$$b_{ij} = \begin{cases} e_{7(j+m)+3} \otimes w_{7j+1 \rightarrow 7(j+1)}, & i = s + (j+1)_s; \\ w_{7(j+m)+1 \rightarrow 7(j+m)+3} \otimes w_{7j+1 \rightarrow 7(j+1)}, & i = 2s + (j+1)_s; \\ w_{7(j+m)+6 \rightarrow 7(j+m)+3} \otimes e_{7j+1}, & i = j+s; \\ 0, & \text{otherwise.} \end{cases}$$

If  $3s \leq j < 4s$ , then

$$b_{ij} = \begin{cases} w_{7(j+m+1) \rightarrow 7(j+m+1)+4} \otimes e_{7j+2}, & i = j + s; \\ 0, & \text{otherwise.} \end{cases}$$

If  $4s \leq j < 5s$ , then

$$b_{ij} = \begin{cases} e_{7(j+m+1)+1} \otimes w_{7j+3 \rightarrow 7(j+1)}, & i = 2s + (j+1)_s; \\ w_{7(j+m)+6 \rightarrow 7(j+m+1)+1} \otimes e_{7j+3}, & i = j + s; \\ 0, & \text{otherwise.} \end{cases}$$

If  $5s \leq j < 6s$ , then  $b_{ij} = 0$ .

If  $6s \leq j < 7s$ , then

$$b_{ij} = \begin{cases} w_{7(j+m)+6 \rightarrow 7(j+m+1)+1} \otimes w_{7j+4 \rightarrow 7j+5}, & i = j + s; \\ 0, & \text{otherwise.} \end{cases}$$

If  $7s \leq j < 8s$ , then

$$b_{ij} = \begin{cases} e_{7(j+m+1)+2} \otimes w_{7j+5 \rightarrow 7j+6}, & i = j + s; \\ 0, & \text{otherwise.} \end{cases}$$

If  $8s \leq j < 9s$ , then  $b_{ij} = 0$ .

If  $9s \leq j < 10s$ , then

$$b_{ij} = \begin{cases} e_{7(j+m+1)+6} \otimes w_{7j+6 \rightarrow 7(j+1)+1}, & i = 3s + (j+1)_s; \\ w_{7(j+m+1)+2 \rightarrow 7(j+m+1)+6} \otimes e_{7j+6}, & i = j - s; \\ 0, & \text{otherwise.} \end{cases}$$

(7) If  $r_0 = 6$ , then  $\Omega^6(Y_t^{(17)})$  is described with  $(12s \times 10s)$ -matrix with the following elements  $b_{ij}$ :

If  $s \leq j < 2s$ , then

$$b_{ij} = \begin{cases} -e_{7(j+m)+3} \otimes w_{7j \rightarrow 7j+5}, & i = j + 7s; \\ 0, & \text{otherwise.} \end{cases}$$

If  $2s \leq j < 3s$ , then

$$b_{ij} = \begin{cases} w_{7(j+m-1)+6 \rightarrow 7(j+m)+1} \otimes e_{7j}, & i = j - 2s; \\ -e_{7(j+m)+1} \otimes w_{7j \rightarrow 7j+2}, & i = j + s; \\ 0, & \text{otherwise.} \end{cases}$$

If  $3s \leq j < 4s$ , then

$$b_{ij} = \begin{cases} e_{7(j+m)+6} \otimes w_{7j+1 \rightarrow 7(j+1)}, & i = (j+1)_s; \\ -w_{7(j+m)+4 \rightarrow 7(j+m)+6} \otimes e_{7j+1}, & i = j - s; \\ 0, & \text{otherwise.} \end{cases}$$

If  $4s \leq j < 5s$ , then

$$b_{ij} = \begin{cases} -e_{7(j+m+1)} \otimes w_{7j+2 \rightarrow 7(j+1)}, & i = s + (j+1)_s; \\ -w_{7(j+m)+1 \rightarrow 7(j+m+1)} \otimes e_{7j+2}, & i = j - s; \\ 0, & \text{otherwise.} \end{cases}$$



If  $5s \leq j < 6s$ , then

$$b_{ij} = \begin{cases} -w_{7(j+m)+2 \rightarrow 7(j+m)+6} \otimes e_{7j+3}, & i = j; \\ 0, & \text{otherwise.} \end{cases}$$

If  $6s \leq j < 7s$ , then

$$b_{ij} = \begin{cases} -w_{7(j+m)+6 \rightarrow 7(j+m)+1} \otimes w_{7j+4 \rightarrow 7(j+1)}, & i = (j+1)_s; \\ w_{7(j+m)+2 \rightarrow 7(j+m)+1} \otimes e_{7j+4}, & i = j; \\ -w_{7(j+m)+4 \rightarrow 7(j+m)+1} \otimes e_{7j+4}, & i = j+s; \\ 0, & \text{otherwise.} \end{cases}$$

If  $7s \leq j < 8s$ , then  $b_{ij} = 0$ .

If  $8s \leq j < 9s$ , then

$$b_{ij} = \begin{cases} -w_{7(j+m+1)+1 \rightarrow 7(j+m+1)+2} \otimes w_{7j+6 \rightarrow 7(j+1)+2}, & i = 3s + (j+1)_s; \\ -e_{7(j+m+1)+2} \otimes w_{7j+6 \rightarrow 7(j+1)+3}, & i = 5s + (j+1)_s; \\ -w_{7(j+m)+6 \rightarrow 7(j+m)+1} \otimes e_{7j+6}, & i = j+2s; \\ 0, & \text{otherwise.} \end{cases}$$

If  $9s \leq j < 10s$ , then

$$b_{ij} = \begin{cases} w_{7(j+m+1)+4 \rightarrow 7(j+m+1)+5} \otimes w_{7j+6 \rightarrow 7(j+1)+1}, & i = 2s + (j+1)_s; \\ 0, & \text{otherwise.} \end{cases}$$

(8) If  $r_0 = 7$ , then  $\Omega^7(Y_t^{(17)})$  is described with  $(12s \times 12s)$ -matrix with the following elements  $b_{ij}$ :

If  $0 \leq j < s$ , then

$$b_{ij} = \begin{cases} w_{7(j+m)+2 \rightarrow 7(j+m)+6} \otimes e_{7j}, & i = j; \\ -w_{7(j+m)+4 \rightarrow 7(j+m)+6} \otimes e_{7j}, & i = j+2s; \\ e_{7(j+m)+6} \otimes w_{7j \rightarrow 7j+4}, & i = j+6s; \\ 0, & \text{otherwise.} \end{cases}$$

If  $s \leq j < 2s$ , then

$$b_{ij} = \begin{cases} e_{7(j+m+1)} \otimes w_{7j \rightarrow 7j+1}, & i = j+2s; \\ w_{7(j+m)+6 \rightarrow 7(j+m)+1} \otimes w_{7j \rightarrow 7j+4}, & i = j+5s; \\ 0, & \text{otherwise.} \end{cases}$$

If  $2s \leq j < 3s$ , then

$$b_{ij} = \begin{cases} w_{7(j+m+1) \rightarrow 7(j+m+1)+4} \otimes e_{7j+1}, & i = j+s; \\ 0, & \text{otherwise.} \end{cases}$$

If  $3s \leq j < 4s$ , then

$$b_{ij} = \begin{cases} w_{7(j+m)+6 \rightarrow 7(j+m+1)+1} \otimes e_{7j+2}, & i = j+s; \\ w_{7(j+m+1) \rightarrow 7(j+m+1)+1} \otimes w_{7j+2 \rightarrow 7j+3}, & i = j+2s; \\ e_{7(j+m+1)+1} \otimes w_{7j+2 \rightarrow 7j+6}, & i = j+8s; \\ 0, & \text{otherwise.} \end{cases}$$

If  $4s \leq j < 5s$ , then

$$b_{ij} = \begin{cases} w_{7(j+m+1)+4 \rightarrow 7(j+m+1)+5} \otimes w_{7j+2 \rightarrow 7(j+1)}, & i = 2s + (j+1)_s; \\ 0, & \text{otherwise.} \end{cases}$$

If  $5s \leq j < 6s$ , then

$$b_{ij} = \begin{cases} -e_{7(j+m+1)+2} \otimes w_{7j+3 \rightarrow 7(j+1)}, & i = (j+1)_s; \\ w_{7(j+m+1) \rightarrow 7(j+m+1)+2} \otimes e_{7j+3}, & i = j; \\ w_{7(j+m+1)+1 \rightarrow 7(j+m+1)+2} \otimes w_{7j+3 \rightarrow 7j+6}, & i = j + 6s; \\ 0, & \text{otherwise.} \end{cases}$$

If  $6s \leq j < 7s$ , then

$$b_{ij} = \begin{cases} w_{7(j+m)+6 \rightarrow 7(j+m+1)+2} \otimes e_{7j+4}, & i = j; \\ w_{7(j+m)+6 \rightarrow 7(j+m+1)+2} \otimes w_{7j+4 \rightarrow 7j+5}, & i = j + s; \\ 0, & \text{otherwise.} \end{cases}$$

If  $7s \leq j < 8s$ , then

$$b_{ij} = \begin{cases} w_{7(j+m)+6 \rightarrow 7(j+m+1)+4} \otimes e_{7j+4}, & i = j - s; \\ 0, & \text{otherwise.} \end{cases}$$

If  $8s \leq j < 9s$ , then

$$b_{ij} = \begin{cases} e_{7(j+m+1)+3} \otimes w_{7j+5 \rightarrow 7j+6}, & i = j + 2s; \\ 0, & \text{otherwise.} \end{cases}$$

If  $9s \leq j < 10s$ , then  $b_{ij} = 0$ .

If  $10s \leq j < 11s$ , then

$$b_{ij} = \begin{cases} -w_{7(j+m+1)+3 \rightarrow 7(j+m+1)+6} \otimes e_{7j+6}, & i = j; \\ 0, & \text{otherwise.} \end{cases}$$

If  $11s \leq j < 12s$ , then

$$b_{ij} = \begin{cases} e_{7(j+m+2)} \otimes w_{7j+6 \rightarrow 7(j+1)+1}, & i = 3s + (j+1)_s; \\ 0, & \text{otherwise.} \end{cases}$$

(9) If  $r_0 = 8$ , then  $\Omega^8(Y_t^{(17)})$  is described with  $(13s \times 12s)$ -matrix with the following elements  $b_{ij}$ :

If  $0 \leq j < s$ , then

$$b_{ij} = \begin{cases} -w_{7(j+m-1)+6 \rightarrow 7(j+m)+2} \otimes e_{7j}, & i = j; \\ w_{7(j+m)+1 \rightarrow 7(j+m)+2} \otimes w_{7j \rightarrow 7j+1}, & i = j + 2s; \\ e_{7(j+m)+2} \otimes w_{7j \rightarrow 7j+2}, & i = j + 4s; \\ 0, & \text{otherwise.} \end{cases}$$

If  $s \leq j < 2s$ , then

$$b_{ij} = \begin{cases} -e_{7(j+m)+5} \otimes w_{7j \rightarrow 7j+1}, & i = j + 2s; \\ e_{7(j+m)+5} \otimes w_{7j \rightarrow 7j+4}, & i = j + 7s; \\ 0, & \text{otherwise.} \end{cases}$$

If  $2s \leq j < 3s$ , then  $b_{ij} = 0$ .

If  $3s \leq j < 4s$ , then

$$b_{ij} = \begin{cases} w_{7(j+m)+6 \rightarrow 7(j+m+1)} \otimes w_{7j+1 \rightarrow 7(j+1)}, & i = (j+1)_s; \\ e_{7(j+m+1)} \otimes w_{7j+1 \rightarrow 7(j+1)}, & i = s + (j+1)_s; \\ -w_{7(j+m)+1 \rightarrow 7(j+m+1)} \otimes e_{7j+1}, & i = j - s; \\ 0, & \text{otherwise.} \end{cases}$$

If  $4s \leq j < 5s$ , then

$$b_{ij} = \begin{cases} -w_{7(j+m)+2 \rightarrow 7(j+m)+6} \otimes e_{7j+2}, & i = j; \\ -w_{7(j+m)+3 \rightarrow 7(j+m)+6} \otimes w_{7j+2 \rightarrow 7j+3}, & i = j + s; \\ 0, & \text{otherwise.} \end{cases}$$

If  $5s \leq j < 6s$ , then

$$b_{ij} = \begin{cases} -w_{7(j+m)+3 \rightarrow 7(j+m+1)} \otimes e_{7j+3}, & i = j; \\ 0, & \text{otherwise.} \end{cases}$$

If  $6s \leq j < 7s$ , then

$$b_{ij} = \begin{cases} -e_{7(j+m)+6} \otimes w_{7j+4 \rightarrow 7(j+1)}, & i = (j+1)_s; \\ w_{7(j+m)+3 \rightarrow 7(j+m)+6} \otimes e_{7j+4}, & i = j + s; \\ -w_{7(j+m)+5 \rightarrow 7(j+m)+6} \otimes e_{7j+4}, & i = j + 2s; \\ 0, & \text{otherwise.} \end{cases}$$

If  $7s \leq j < 10s$ , then  $b_{ij} = 0$ .

If  $10s \leq j < 11s$ , then

$$b_{ij} = \begin{cases} -e_{7(j+m+1)+3} \otimes w_{7j+6 \rightarrow 7(j+1)+3}, & i = 5s + (j+1)_s; \\ w_{7(j+m)+6 \rightarrow 7(j+m+1)+3} \otimes e_{7j+6}, & i = j + s; \\ 0, & \text{otherwise.} \end{cases}$$

If  $11s \leq j < 12s$ , then

$$b_{ij} = \begin{cases} -e_{7(j+m+1)+1} \otimes w_{7j+6 \rightarrow 7(j+1)+1}, & i = 2s + (j+1)_s; \\ 0, & \text{otherwise.} \end{cases}$$

(10) If  $r_0 = 9$ , then  $\Omega^9(Y_t^{(17)})$  is described with  $(12s \times 13s)$ -matrix with the following elements  $b_{ij}$ :

If  $0 \leq j < s$ , then

$$b_{ij} = \begin{cases} -w_{7(j+m)+3 \rightarrow 7(j+m)+6} \otimes e_{7j}, & i = j + s; \\ e_{7(j+m)+6} \otimes w_{7j \rightarrow 7j+1}, & i = j + 3s; \\ 0, & \text{otherwise.} \end{cases}$$

If  $s \leq j < 2s$ , then

$$b_{ij} = \begin{cases} w_{7(j+m)+6 \rightarrow 7(j+m+1)} \otimes w_{7j \rightarrow 7j+1}, & i = j + 2s; \\ e_{7(j+m+1)} \otimes w_{7j \rightarrow 7j+4}, & i = j + 6s; \\ 0, & \text{otherwise.} \end{cases}$$

If  $2s \leq j < 3s$ , then

$$b_{ij} = \begin{cases} -e_{7(j+m+1)+1} \otimes w_{7j+1 \rightarrow 7(j+1)}, & i = 2s + (j+1)_s; \\ w_{7(j+m)+6 \rightarrow 7(j+m+1)+1} \otimes e_{7j+1}, & i = j + s; \\ 0, & \text{otherwise.} \end{cases}$$

If  $3s \leq j < 4s$ , then

$$b_{ij} = \begin{cases} -e_{7(j+m+1)+5} \otimes w_{7j+1 \rightarrow 7(j+1)}, & i = (j+1)_s; \\ 0, & \text{otherwise.} \end{cases}$$

If  $4s \leq j < 5s$ , then

$$b_{ij} = \begin{cases} -w_{7(j+m+1)+1 \rightarrow 7(j+m+1)+2} \otimes w_{7j+2 \rightarrow 7(j+1)}, & i = 2s + (j+1)_s; \\ w_{7(j+m+1) \rightarrow 7(j+m+1)+2} \otimes e_{7j+2}, & i = j; \\ w_{7(j+m)+6 \rightarrow 7(j+m+1)+2} \otimes w_{7j+2 \rightarrow 7j+3}, & i = j + s; \\ -e_{7(j+m+1)+2} \otimes w_{7j+2 \rightarrow 7j+6}, & i = j + 5s; \\ 0, & \text{otherwise.} \end{cases}$$

If  $5s \leq j < 6s$ , then

$$b_{ij} = \begin{cases} -e_{7(j+m+1)+3} \otimes w_{7j+3 \rightarrow 7(j+1)}, & i = s + (j+1)_s; \\ w_{7(j+m)+6 \rightarrow 7(j+m+1)+3} \otimes e_{7j+3}, & i = j; \\ 0, & \text{otherwise.} \end{cases}$$

If  $6s \leq j < 7s$ , then  $b_{ij} = 0$ .

If  $7s \leq j < 8s$ , then

$$b_{ij} = \begin{cases} w_{7(j+m)+6 \rightarrow 7(j+m+1)+3} \otimes e_{7j+4}, & i = j - s; \\ 0, & \text{otherwise.} \end{cases}$$

If  $8s \leq j < 9s$ , then

$$b_{ij} = \begin{cases} -e_{7(j+m+1)+5} \otimes w_{7j+4 \rightarrow 7(j+1)}, & i = (j+1)_s; \\ -w_{7(j+m+1) \rightarrow 7(j+m+1)+5} \otimes e_{7j+4}, & i = j - s; \\ 0, & \text{otherwise.} \end{cases}$$

If  $9s \leq j < 11s$ , then  $b_{ij} = 0$ .

If  $11s \leq j < 12s$ , then

$$b_{ij} = \begin{cases} -w_{7(j+m+1)+3 \rightarrow 7(j+m+1)+6} \otimes w_{7j+6 \rightarrow 7(j+1)}, & i = s + (j+1)_s; \\ w_{7(j+m+1)+5 \rightarrow 7(j+m+1)+6} \otimes e_{7j+6}, & i = j - s; \\ 0, & \text{otherwise.} \end{cases}$$

If  $12s \leq j < 13s$ , then

$$b_{ij} = \begin{cases} -w_{7(j+m+1)+3 \rightarrow 7(j+m+2)} \otimes w_{7j+6 \rightarrow 7(j+1)}, & i = s + (j+1)_s; \\ -e_{7(j+m+2)} \otimes w_{7j+6 \rightarrow 7(j+1)+4}, & i = 7s + (j+1)_s; \\ 0, & \text{otherwise.} \end{cases}$$

(11) If  $r_0 = 10$ , then  $\Omega^{10}(Y_t^{(17)})$  is described with  $(12s \times 12s)$ -matrix with the following elements  $b_{ij}$ :

If  $s \leq j < 2s$ , then

$$b_{ij} = \begin{cases} w_{7(j+m-1)+6 \rightarrow 7(j+m)+3} \otimes e_{7j}, & i = j - s; \\ e_{7(j+m)+3} \otimes w_{7j \rightarrow 7j+2}, & i = j + 2s; \\ 0, & \text{otherwise.} \end{cases}$$

If  $2s \leq j < 3s$ , then

$$b_{ij} = \begin{cases} -e_{7(j+m)+1} \otimes w_{7j \rightarrow 7j+4}, & i = j + 5s; \\ 0, & \text{otherwise.} \end{cases}$$

If  $3s \leq j < 4s$ , then

$$b_{ij} = \begin{cases} -e_{7(j+m)+6} \otimes w_{7j+1 \rightarrow 7(j+1)}, & i = (j+1)_s; \\ -w_{7(j+m)+2 \rightarrow 7(j+m)+6} \otimes e_{7j+1}, & i = j - s; \\ 0, & \text{otherwise.} \end{cases}$$

If  $4s \leq j < 5s$ , then

$$b_{ij} = \begin{cases} -w_{7(j+m)+3 \rightarrow 7(j+m+1)} \otimes e_{7j+2}, & i = j - s; \\ 0, & \text{otherwise.} \end{cases}$$

If  $5s \leq j < 6s$ , then

$$b_{ij} = \begin{cases} -w_{7(j+m)+5 \rightarrow 7(j+m)+6} \otimes e_{7j+3}, & i = j; \\ 0, & \text{otherwise.} \end{cases}$$

If  $6s \leq j < 7s$ , then

$$b_{ij} = \begin{cases} -w_{7(j+m)+4 \rightarrow 7(j+m)+6} \otimes e_{7j+4}, & i = j; \\ w_{7(j+m)+5 \rightarrow 7(j+m)+6} \otimes w_{7j+4 \rightarrow 7j+5}, & i = j + 3s; \\ 0, & \text{otherwise.} \end{cases}$$

If  $7s \leq j < 8s$ , then

$$b_{ij} = \begin{cases} -w_{7(j+m)+6 \rightarrow 7(j+m+1)} \otimes w_{7j+4 \rightarrow 7(j+1)}, & i = (j+1)_s; \\ -e_{7(j+m+1)} \otimes w_{7j+4 \rightarrow 7(j+1)}, & i = s + (j+1)_s; \\ -w_{7(j+m)+1 \rightarrow 7(j+m+1)} \otimes e_{7j+4}, & i = j; \\ 0, & \text{otherwise.} \end{cases}$$

If  $8s \leq j < 9s$ , then

$$b_{ij} = \begin{cases} e_{7(j+m+1)} \otimes w_{7j+5 \rightarrow 7j+6}, & i = j + 3s; \\ 0, & \text{otherwise.} \end{cases}$$

If  $9s \leq j < 10s$ , then

$$b_{ij} = \begin{cases} e_{7(j+m+1)+2} \otimes w_{7j+6 \rightarrow 7(j+1)+1}, & i = 2s + (j+1)_s; \\ -w_{7(j+m+1)+1 \rightarrow 7(j+m+1)+2} \otimes w_{7j+6 \rightarrow 7(j+1)+4}, & i = 7s + (j+1)_s; \\ 0, & \text{otherwise.} \end{cases}$$

If  $10s \leq j < 11s$ , then

$$b_{ij} = \begin{cases} w_{7(j+m)+6 \rightarrow 7(j+m+1)+5} \otimes w_{7j+6 \rightarrow 7(j+1)}, & i = (j+1)_s; \\ w_{7(j+m+1) \rightarrow 7(j+m+1)+5} \otimes w_{7j+6 \rightarrow 7(j+1)}, & i = s + (j+1)_s; \\ -w_{7(j+m+1)+4 \rightarrow 7(j+m+1)+5} \otimes w_{7j+6 \rightarrow 7(j+1)+2}, & i = 4s + (j+1)_s; \\ -e_{7(j+m+1)+5} \otimes w_{7j+6 \rightarrow 7(j+1)+3}, & i = 5s + (j+1)_s; \\ -e_{7(j+m+1)+5} \otimes w_{7j+6 \rightarrow 7(j+1)+5}, & i = 9s + (j+1)_s; \\ -w_{7(j+m)+6 \rightarrow 7(j+m+1)+5} \otimes e_{7j+6}, & i = j; \\ 0, & \text{otherwise.} \end{cases}$$

If  $11s \leq j < 12s$ , then  $b_{ij} = 0$ .

(12) If  $r_0 = 11$ , then  $\Omega^{11}(Y_t^{(17)})$  is described with  $(10s \times 12s)$ -matrix with the following elements  $b_{ij}$ :

If  $0 \leq j < s$ , then

$$b_{ij} = \begin{cases} w_{7(j+m)+2 \rightarrow 7(j+m)+6} \otimes e_{7j}, & i = j; \\ -w_{7(j+m)+4 \rightarrow 7(j+m)+6} \otimes e_{7j}, & i = j + s; \\ e_{7(j+m)+6} \otimes w_{7j \rightarrow 7j+2}, & i = j + 3s; \\ e_{7(j+m)+6} \otimes w_{7j \rightarrow 7j+5}, & i = j + 6s; \\ 0, & \text{otherwise.} \end{cases}$$

If  $s \leq j < 2s$ , then

$$b_{ij} = \begin{cases} e_{7(j+m+1)} \otimes w_{7j \rightarrow 7j+4}, & i = j + 4s; \\ 0, & \text{otherwise.} \end{cases}$$

If  $2s \leq j < 3s$ , then

$$b_{ij} = \begin{cases} e_{7(j+m+1)+2} \otimes w_{7j+1 \rightarrow 7(j+1)}, & i = (j+1)_s; \\ w_{7(j+m+1) \rightarrow 7(j+m+1)+2} \otimes e_{7j+1}, & i = j; \\ 0, & \text{otherwise.} \end{cases}$$

If  $3s \leq j < 4s$ , then

$$b_{ij} = \begin{cases} w_{7(j+m)+6 \rightarrow 7(j+m+1)+3} \otimes e_{7j+2}, & i = j; \\ -e_{7(j+m+1)+3} \otimes w_{7j+2 \rightarrow 7j+6}, & i = j + 5s; \\ 0, & \text{otherwise.} \end{cases}$$

If  $4s \leq j < 5s$ , then  $b_{ij} = 0$ .

If  $5s \leq j < 6s$ , then

$$b_{ij} = \begin{cases} -w_{7(j+m+1) \rightarrow 7(j+m+1)+5} \otimes e_{7j+3}, & i = j - s; \\ e_{7(j+m+1)+5} \otimes w_{7j+3 \rightarrow 7j+6}, & i = j + 2s; \\ 0, & \text{otherwise.} \end{cases}$$

If  $6s \leq j < 7s$ , then

$$b_{ij} = \begin{cases} w_{7(j+m+1) \rightarrow 7(j+m+1)+4} \otimes e_{7j+4}, & i = j - s; \\ 0, & \text{otherwise.} \end{cases}$$

If  $7s \leq j < 8s$ , then

$$b_{ij} = \begin{cases} -w_{7(j+m+1) \rightarrow 7(j+m+1)+1} \otimes e_{7j+4}, & i = j - 2s; \\ e_{7(j+m+1)+1} \otimes w_{7j+4 \rightarrow 7j+6}, & i = j + 2s; \\ 0, & \text{otherwise.} \end{cases}$$

If  $8s \leq j < 9s$ , then

$$b_{ij} = \begin{cases} w_{7(j+m+1)+1 \rightarrow 7(j+m+1)+2} \otimes w_{7j+5 \rightarrow 7j+6}, & i = j + s; \\ 0, & \text{otherwise.} \end{cases}$$

If  $9s \leq j < 10s$ , then

$$b_{ij} = \begin{cases} -e_{7(j+m+1)+5} \otimes w_{7j+5 \rightarrow 7j+6}, & i = j - 2s; \\ 0, & \text{otherwise.} \end{cases}$$

If  $10s \leq j < 11s$ , then

$$b_{ij} = \begin{cases} w_{7(j+m+1)+2 \rightarrow 7(j+m+1)+6} \otimes w_{7j+6 \rightarrow 7(j+1)}, & i = (j+1)_s; \\ e_{7(j+m+1)+6} \otimes w_{7j+6 \rightarrow 7(j+1)+2}, & i = 3s + (j+1)_s; \\ e_{7(j+m+1)+6} \otimes w_{7j+6 \rightarrow 7(j+1)+5}, & i = 6s + (j+1)_s; \\ -w_{7(j+m+1)+3 \rightarrow 7(j+m+1)+6} \otimes e_{7j+6}, & i = j - 2s; \\ 0, & \text{otherwise.} \end{cases}$$

If  $11s \leq j < 12s$ , then

$$b_{ij} = \begin{cases} w_{7(j+m+1)+4 \rightarrow 7(j+m+2)} \otimes w_{7j+6 \rightarrow 7(j+1)}, & i = s + (j+1)_s; \\ -e_{7(j+m+2)} \otimes w_{7j+6 \rightarrow 7(j+1)+3}, & i = 4s + (j+1)_s; \\ e_{7(j+m+2)} \otimes w_{7j+6 \rightarrow 7(j+1)+4}, & i = 5s + (j+1)_s; \\ 0, & \text{otherwise.} \end{cases}$$

(13) If  $r_0 = 12$ , then  $\Omega^{12}(Y_t^{(17)})$  is described with  $(10s \times 10s)$ -matrix with the following elements  $b_{ij}$ :

If  $0 \leq j < s$ , then

$$b_{ij} = \begin{cases} -w_{7(j+m) \rightarrow 7(j+m)+2} \otimes e_{7j}, & i = j; \\ w_{7(j+m)+1 \rightarrow 7(j+m)+2} \otimes w_{7j \rightarrow 7j+3}, & i = j + 4s; \\ -e_{7(j+m)+2} \otimes w_{7j \rightarrow 7j+4}, & i = j + 5s; \\ 0, & \text{otherwise.} \end{cases}$$

If  $s \leq j < 2s$ , then  $b_{ij} = 0$ .

If  $2s \leq j < 3s$ , then

$$b_{ij} = \begin{cases} -w_{7(j+m)+3 \rightarrow 7(j+m+1)} \otimes e_{7j+1}, & i = j - s; \\ 0, & \text{otherwise.} \end{cases}$$

If  $3s \leq j < 4s$ , then

$$b_{ij} = \begin{cases} -w_{7(j+m)+5 \rightarrow 7(j+m)+6} \otimes e_{7j+2}, & i = j; \\ 0, & \text{otherwise.} \end{cases}$$

If  $4s \leq j < 5s$ , then

$$b_{ij} = \begin{cases} -e_{7(j+m+1)} \otimes w_{7j+3 \rightarrow 7(j+1)}, & i = (j+1)_s; \\ -w_{7(j+m)+1 \rightarrow 7(j+m+1)} \otimes e_{7j+3}, & i = j; \\ w_{7(j+m)+6 \rightarrow 7(j+m+1)} \otimes w_{7j+3 \rightarrow 7j+6}, & i = j + 4s; \\ e_{7(j+m+1)} \otimes w_{7j+3 \rightarrow 7j+6}, & i = j + 5s; \\ 0, & \text{otherwise.} \end{cases}$$

If  $5s \leq j < 6s$ , then

$$b_{ij} = \begin{cases} w_{7(j+m)+2 \rightarrow 7(j+m+1)} \otimes e_{7j+4}, & i = j; \\ -w_{7(j+m)+5 \rightarrow 7(j+m+1)} \otimes e_{7j+4}, & i = j + s; \\ 0, & \text{otherwise.} \end{cases}$$

If  $6s \leq j < 7s$ , then

$$b_{ij} = \begin{cases} -e_{7(j+m)+6} \otimes w_{7j+5 \rightarrow 7j+6}, & i = j + 2s; \\ 0, & \text{otherwise.} \end{cases}$$

If  $7s \leq j < 8s$ , then  $b_{ij} = 0$ .

If  $8s \leq j < 9s$ , then

$$b_{ij} = \begin{cases} e_{7(j+m+1)+3} \otimes w_{7j+6 \rightarrow 7(j+1)+1}, & i = s + (j+1)_s; \\ w_{7(j+m)+6 \rightarrow 7(j+m+1)+3} \otimes e_{7j+6}, & i = j; \\ 0, & \text{otherwise.} \end{cases}$$

If  $9s \leq j < 10s$ , then

$$b_{ij} = \begin{cases} e_{7(j+m+1)+1} \otimes w_{7j+6 \rightarrow 7(j+1)+3}, & i = 4s + (j+1)_s; \\ 0, & \text{otherwise.} \end{cases}$$

(14) If  $r_0 = 13$ , then  $\Omega^{13}(Y_t^{(17)})$  is described with  $(9s \times 10s)$ -matrix with the following elements  $b_{ij}$ :

If  $0 \leq j < s$ , then

$$b_{ij} = \begin{cases} w_{7(j+m)+5 \rightarrow 7(j+m+1)} \otimes e_{7j}, & i = j + s; \\ -w_{7(j+m)+6 \rightarrow 7(j+m+1)} \otimes w_{7j \rightarrow 7j+1}, & i = j + 2s; \\ e_{7(j+m+1)} \otimes w_{7j \rightarrow 7j+2}, & i = j + 3s; \\ 0, & \text{otherwise.} \end{cases}$$

If  $s \leq j < 2s$ , then

$$b_{ij} = \begin{cases} e_{7(j+m+1)+3} \otimes w_{7j+1 \rightarrow 7(j+1)}, & i = (j+1)_s; \\ w_{7(j+m)+6 \rightarrow 7(j+m+1)+3} \otimes e_{7j+1}, & i = j + s; \\ 0, & \text{otherwise.} \end{cases}$$

If  $2s \leq j < 3s$ , then  $b_{ij} = 0$ .



If  $3s \leq j < 4s$ , then

$$b_{ij} = \begin{cases} -w_{7(j+m+1) \rightarrow 7(j+m+1)+5} \otimes e_{7j+2}, & i = j; \\ 0, & \text{otherwise.} \end{cases}$$

If  $4s \leq j < 5s$ , then

$$b_{ij} = \begin{cases} e_{7(j+m+1)+1} \otimes e_{7j+3}, & i = j; \\ 0, & \text{otherwise.} \end{cases}$$

If  $5s \leq j < 6s$ , then

$$b_{ij} = \begin{cases} w_{7(j+m)+6 \rightarrow 7(j+m+1)+2} \otimes e_{7j+4}, & i = j; \\ w_{7(j+m+1) \rightarrow 7(j+m+1)+2} \otimes w_{7j+4 \rightarrow 7j+5}, & i = j + s; \\ e_{7(j+m+1)+2} \otimes w_{7j+4 \rightarrow 7j+6}, & i = j + 2s; \\ 0, & \text{otherwise.} \end{cases}$$

If  $6s \leq j < 7s$ , then

$$b_{ij} = \begin{cases} -w_{7(j+m)+6 \rightarrow 7(j+m+1)+5} \otimes e_{7j+4}, & i = j - s; \\ 0, & \text{otherwise.} \end{cases}$$

If  $7s \leq j < 8s$ , then  $b_{ij} = 0$ .

If  $8s \leq j < 9s$ , then

$$b_{ij} = \begin{cases} e_{7(j+m+1)+6} \otimes w_{7j+6 \rightarrow 7(j+1)+1}, & i = 2s + (j + 1)s; \\ w_{7(j+m+1)+2 \rightarrow 7(j+m+1)+6} \otimes e_{7j+6}, & i = j - s; \\ -w_{7(j+m+1)+4 \rightarrow 7(j+m+1)+6} \otimes e_{7j+6}, & i = j; \\ 0, & \text{otherwise.} \end{cases}$$

If  $9s \leq j < 10s$ , then  $b_{ij} = 0$ .

(15) If  $r_0 = 14$ , then  $\Omega^{14}(Y_t^{(17)})$  is described with  $(7s \times 9s)$ -matrix with the following elements  $b_{ij}$ :

If  $0 \leq j < s$ , then

$$b_{ij} = \begin{cases} -w_{7(j+m)+1 \rightarrow 7(j+m)+3} \otimes w_{7j \rightarrow 7j+2}, & i = j + 2s; \\ -e_{7(j+m)+3} \otimes w_{7j \rightarrow 7j+4}, & i = j + 4s; \\ 0, & \text{otherwise.} \end{cases}$$

If  $s \leq j < 2s$ , then

$$b_{ij} = \begin{cases} w_{7(j+m-1)+6 \rightarrow 7(j+m)+5} \otimes e_{7j}, & i = j - s; \\ 0, & \text{otherwise.} \end{cases}$$

If  $2s \leq j < 3s$ , then

$$b_{ij} = \begin{cases} -e_{7(j+m)+6} \otimes w_{7j+1 \rightarrow 7(j+1)}, & i = (j + 1)s; \\ -w_{7(j+m)+5 \rightarrow 7(j+m)+6} \otimes e_{7j+1}, & i = j - s; \\ -w_{7(j+m)+2 \rightarrow 7(j+m)+6} \otimes w_{7j+1 \rightarrow 7j+3}, & i = j + s; \\ 0, & \text{otherwise.} \end{cases}$$

If  $3s \leq j < 4s$ , then

$$b_{ij} = \begin{cases} w_{7(j+m)+6 \rightarrow 7(j+m+1)} \otimes w_{7j+2 \rightarrow 7(j+1)}, & i = (j+1)_s; \\ -w_{7(j+m)+1 \rightarrow 7(j+m+1)} \otimes e_{7j+2}, & i = j - s; \\ -e_{7(j+m+1)} \otimes w_{7j+2 \rightarrow 7j+6}, & i = j + 3s; \\ 0, & \text{otherwise.} \end{cases}$$

If  $4s \leq j < 5s$ , then

$$b_{ij} = \begin{cases} -e_{7(j+m+1)+1} \otimes w_{7j+3 \rightarrow 7(j+1)+2}, & i = 2s + (j+1)_s; \\ -w_{7(j+m)+2 \rightarrow 7(j+m+1)+1} \otimes e_{7j+3}, & i = j - s; \\ 0, & \text{otherwise.} \end{cases}$$

If  $5s \leq j < 6s$ , then

$$b_{ij} = \begin{cases} w_{7(j+m)+4 \rightarrow 7(j+m)+6} \otimes w_{7j+4 \rightarrow 7j+5}, & i = j; \\ 0, & \text{otherwise.} \end{cases}$$

If  $6s \leq j < 7s$ , then  $b_{ij} = 0$ .

If  $7s \leq j < 8s$ , then

$$b_{ij} = \begin{cases} w_{7(j+m)+6 \rightarrow 7(j+m+1)+2} \otimes w_{7j+6 \rightarrow 7(j+1)}, & i = (j+1)_s; \\ -e_{7(j+m+1)+2} \otimes w_{7j+6 \rightarrow 7(j+1)+3}, & i = 3s + (j+1)_s; \\ -w_{7(j+m+1) \rightarrow 7(j+m+1)+2} \otimes e_{7j+6}, & i = j - s; \\ 0, & \text{otherwise.} \end{cases}$$

If  $8s \leq j < 9s$ , then  $b_{ij} = 0$ .

(16) If  $r_0 = 15$ , then  $\Omega^{15}(Y_t^{(17)})$  is described with  $(8s \times 7s)$ -matrix with the following elements  $b_{ij}$ :

If  $0 \leq j < s$ , then

$$b_{ij} = \begin{cases} e_{7(j+m)+6} \otimes e_{7j}, & i = j; \\ 0, & \text{otherwise.} \end{cases}$$

If  $s \leq j < 2s$ , then

$$b_{ij} = \begin{cases} -w_{7(j+m+1) \rightarrow 7(j+m+1)+5} \otimes e_{7j+1}, & i = j; \\ 0, & \text{otherwise.} \end{cases}$$

If  $2s \leq j < 3s$ , then

$$b_{ij} = \begin{cases} e_{7(j+m+1)+1} \otimes e_{7j+2}, & i = j; \\ 0, & \text{otherwise.} \end{cases}$$

If  $3s \leq j < 4s$ , then

$$b_{ij} = \begin{cases} e_{7(j+m+1)+2} \otimes e_{7j+3}, & i = j; \\ 0, & \text{otherwise.} \end{cases}$$

If  $4s \leq j < 5s$ , then

$$b_{ij} = \begin{cases} e_{7(j+m+1)+3} \otimes w_{7j+4 \rightarrow 7j+6}, & i = j + 2s; \\ 0, & \text{otherwise.} \end{cases}$$

If  $5s \leq j < 6s$ , then  $b_{ij} = 0$ .

If  $6s \leq j < 7s$ , then

$$b_{ij} = \begin{cases} e_{7(j+m+2)} \otimes w_{7j+6 \rightarrow 7(j+1)+1}, & i = s + (j+1)_s; \\ w_{7(j+m+1)+3 \rightarrow 7(j+m+2)} \otimes e_{7j+6}, & i = j; \\ 0, & \text{otherwise.} \end{cases}$$

(17) If  $r_0 = 16$ , then  $\Omega^{16}(Y_t^{(17)})$  is described with  $(7s \times 8s)$ -matrix with the following elements  $b_{ij}$ :

If  $0 \leq j < s$ , then

$$b_{ij} = \begin{cases} -w_{7(j+m) \rightarrow 7(j+m)+6} \otimes e_{7j}, & i = j; \\ -w_{7(j+m)+2 \rightarrow 7(j+m)+6} \otimes w_{7j \rightarrow 7j+2}, & i = j + 2s; \\ -w_{7(j+m)+4 \rightarrow 7(j+m)+6} \otimes w_{7j \rightarrow 7j+4}, & i = j + 4s; \\ w_{7(j+m)+5 \rightarrow 7(j+m)+6} \otimes w_{7j \rightarrow 7j+5}, & i = j + 5s; \\ -e_{7(j+m)+6} \otimes w_{7j \rightarrow 7j+6}, & i = j + 6s; \\ 0, & \text{otherwise.} \end{cases}$$

If  $s \leq j < 2s$ , then

$$b_{ij} = \begin{cases} -e_{7(j+m+1)} \otimes w_{7j+1 \rightarrow 7(j+1)}, & i = (j+1)_s; \\ -w_{7(j+m)+1 \rightarrow 7(j+m+1)} \otimes e_{7j+1}, & i = j; \\ -w_{7(j+m)+3 \rightarrow 7(j+m+1)} \otimes w_{7j+1 \rightarrow 7j+3}, & i = j + 2s; \\ 0, & \text{otherwise.} \end{cases}$$

If  $2s \leq j < 3s$ , then

$$b_{ij} = \begin{cases} -e_{7(j+m+1)+1} \otimes w_{7j+2 \rightarrow 7(j+1)+1}, & i = s + (j+1)_s; \\ -w_{7(j+m)+2 \rightarrow 7(j+m+1)+1} \otimes e_{7j+2}, & i = j; \\ -w_{7(j+m)+6 \rightarrow 7(j+m+1)+1} \otimes w_{7j+2 \rightarrow 7j+6}, & i = j + 4s; \\ 0, & \text{otherwise.} \end{cases}$$

If  $3s \leq j < 4s$ , then

$$b_{ij} = \begin{cases} -w_{7(j+m+1) \rightarrow 7(j+m+1)+2} \otimes w_{7j+3 \rightarrow 7(j+1)}, & i = (j+1)_s; \\ -e_{7(j+m+1)+2} \otimes w_{7j+3 \rightarrow 7(j+1)+2}, & i = 2s + (j+1)_s; \\ -w_{7(j+m)+3 \rightarrow 7(j+m+1)+2} \otimes e_{7j+3}, & i = j; \\ 0, & \text{otherwise.} \end{cases}$$

If  $4s \leq j < 6s$ , then  $b_{ij} = 0$ .

If  $6s \leq j < 7s$ , then

$$b_{ij} = \begin{cases} -w_{7(j+m+1)+1 \rightarrow 7(j+m+1)+3} \otimes w_{7j+6 \rightarrow 7(j+1)+1}, & i = s + (j+1)_s; \\ -e_{7(j+m+1)+3} \otimes w_{7j+6 \rightarrow 7(j+1)+3}, & i = 3s + (j+1)_s; \\ -w_{7(j+m)+6 \rightarrow 7(j+m+1)+3} \otimes e_{7j+6}, & i = j; \\ 0, & \text{otherwise.} \end{cases}$$

If  $7s \leq j < 8s$ , then  $b_{ij} = 0$ .

(II) Represent an arbitrary  $t_0 \in \mathbb{N}$  in the form  $t_0 = 17\ell_0 + r_0$ , where  $0 \leq r_0 \leq 16$ . Then  $\Omega^{t_0}(Y_t^{(17)})$  is a  $\Omega^{r_0}(Y_t^{(17)})$ , whose left components twisted by  $\sigma^{\ell_0}$ .

**Proposition 14** (Translates for the case 19). (I) Let  $r_0 \in \mathbb{N}$ ,  $r_0 < 17$ .  $r_0$ -translates of the elements  $Y_t^{(19)}$  are described by the following way.

(1) If  $r_0 = 0$ , then  $\Omega^0(Y_t^{(19)})$  is described with  $(7s \times 7s)$ -matrix with one nonzero element that is of the following form:

$$b_{j,0} = w_{7(j+m) \rightarrow 7(j+m+1)} \otimes e_{7j}.$$

(2) If  $r_0 = 1$ , then  $\Omega^1(Y_t^{(19)})$  is described with  $(8s \times 8s)$ -matrix with one nonzero element that is of the following form:

$$b_{j,7s} = w_{7(j+m+1) \rightarrow 7(j+m+2)} \otimes e_{7j+6}.$$

(3) If  $r_0 = 2$ , then  $\Omega^2(Y_t^{(19)})$  is described with  $(7s \times 7s)$ -matrix with one nonzero element that is of the following form:

$$b_{j,6s} = w_{7(j+m+1) \rightarrow 7(j+m+2)} \otimes e_{7j+6}.$$

(4) If  $r_0 = 3$ , then  $\Omega^3(Y_t^{(19)})$  is described with  $(9s \times 9s)$ -matrix with the following two nonzero elements:

$$b_{j,4s} = w_{7(j+m+1) \rightarrow 7(j+m+2)} \otimes e_{7j+3};$$

$$b_{j,6s} = w_{7(j+m+1) \rightarrow 7(j+m+2)} \otimes e_{7j+5}.$$

(5) If  $r_0 = 4$ , then  $\Omega^4(Y_t^{(19)})$  is described with  $(10s \times 10s)$ -matrix with one nonzero element that is of the following form:

$$b_{j,s} = w_{7(j+m) \rightarrow 7(j+m+1)} \otimes e_{7j}.$$

(6) If  $r_0 = 5$ , then  $\Omega^5(Y_t^{(19)})$  is described with  $(10s \times 10s)$ -matrix with the following two nonzero elements:

$$b_{j,4s} = w_{7(j+m+1) \rightarrow 7(j+m+2)} \otimes e_{7j+2};$$

$$b_{j,6s} = w_{7(j+m+1) \rightarrow 7(j+m+2)} \otimes e_{7j+4}.$$

(7) If  $r_0 = 6$ , then  $\Omega^6(Y_t^{(19)})$  is described with  $(12s \times 12s)$ -matrix with the following two nonzero elements:

$$b_{j,s} = w_{7(j+m) \rightarrow 7(j+m+1)} \otimes e_{7j};$$

$$b_{j,11s} = w_{7(j+m+1) \rightarrow 7(j+m+2)} \otimes e_{7j+6}.$$

(8) If  $r_0 = 7$ , then  $\Omega^7(Y_t^{(19)})$  is described with  $(12s \times 12s)$ -matrix with the following nonzero elements:

$$b_{j,3s} = w_{7(j+m+1) \rightarrow 7(j+m+2)} \otimes e_{7j+1};$$

$$b_{j,5s} = w_{7(j+m+1) \rightarrow 7(j+m+2)} \otimes e_{7j+3};$$

$$b_{j,8s} = w_{7(j+m+1) \rightarrow 7(j+m+2)} \otimes e_{7j+5}.$$

(9) If  $r_0 = 8$ , then  $\Omega^8(Y_t^{(19)})$  is described with  $(13s \times 13s)$ -matrix with the following two nonzero elements:

$$b_{j,s} = w_{7(j+m) \rightarrow 7(j+m+1)} \otimes e_{7j};$$

$$b_{j,12s} = w_{7(j+m+1) \rightarrow 7(j+m+2)} \otimes e_{7j+6}.$$

(10) If  $r_0 = 9$ , then  $\Omega^9(Y_t^{(19)})$  is described with  $(12s \times 12s)$ -matrix with the following nonzero elements:

$$b_{j,4s} = w_{7(j+m+1) \rightarrow 7(j+m+2)} \otimes e_{7j+2};$$

$$b_{j,7s} = w_{7(j+m+1) \rightarrow 7(j+m+2)} \otimes e_{7j+4};$$

$$b_{j,8s} = w_{7(j+m+1) \rightarrow 7(j+m+2)} \otimes e_{7j+5}.$$

(11) If  $r_0 = 10$ , then  $\Omega^{10}(Y_t^{(19)})$  is described with  $(12s \times 12s)$ -matrix with the following two nonzero elements:

$$\begin{aligned} b_{j,s} &= w_{7(j+m) \rightarrow 7(j+m+1)} \otimes e_{7j}; \\ b_{j,11s} &= w_{7(j+m+1) \rightarrow 7(j+m+2)} \otimes e_{7j+6}. \end{aligned}$$

(12) If  $r_0 = 11$ , then  $\Omega^{11}(Y_t^{(19)})$  is described with  $(10s \times 10s)$ -matrix with the following nonzero elements:

$$\begin{aligned} b_{j,2s} &= w_{7(j+m+1) \rightarrow 7(j+m+2)} \otimes e_{7j+1}; \\ b_{j,4s} &= w_{7(j+m+1) \rightarrow 7(j+m+2)} \otimes e_{7j+3}; \\ b_{j,5s} &= w_{7(j+m+1) \rightarrow 7(j+m+2)} \otimes e_{7j+4}. \end{aligned}$$

(13) If  $r_0 = 12$ , then  $\Omega^{12}(Y_t^{(19)})$  is described with  $(10s \times 10s)$ -matrix with the following two nonzero elements:

$$\begin{aligned} b_{j,0} &= w_{7(j+m) \rightarrow 7(j+m+1)} \otimes e_{7j}; \\ b_{j,9s} &= w_{7(j+m+1) \rightarrow 7(j+m+2)} \otimes e_{7j+6}. \end{aligned}$$

(14) If  $r_0 = 13$ , then  $\Omega^{13}(Y_t^{(19)})$  is described with  $(9s \times 9s)$ -matrix with the following two nonzero elements:

$$\begin{aligned} b_{j,3s} &= w_{7(j+m+1) \rightarrow 7(j+m+2)} \otimes e_{7j+2}; \\ b_{j,6s} &= w_{7(j+m+1) \rightarrow 7(j+m+2)} \otimes e_{7j+5}. \end{aligned}$$

(15) If  $r_0 = 14$ , then  $\Omega^{14}(Y_t^{(19)})$  is described with  $(7s \times 7s)$ -matrix with one nonzero element that is of the following form:

$$b_{j,6s} = w_{7(j+m+1) \rightarrow 7(j+m+2)} \otimes e_{7j+6}.$$

(16) If  $r_0 = 15$ , then  $\Omega^{15}(Y_t^{(19)})$  is described with  $(8s \times 8s)$ -matrix with the following two nonzero elements:

$$\begin{aligned} b_{j,s} &= w_{7(j+m+1) \rightarrow 7(j+m+2)} \otimes e_{7j+1}; \\ b_{j,4s} &= w_{7(j+m+1) \rightarrow 7(j+m+2)} \otimes e_{7j+4}. \end{aligned}$$

(17) If  $r_0 = 16$ , then  $\Omega^{16}(Y_t^{(19)})$  is described with  $(7s \times 7s)$ -matrix with one nonzero element that is of the following form:

$$b_{j,0} = w_{7(j+m) \rightarrow 7(j+m+1)} \otimes e_{7j}.$$

(II) Represent an arbitrary  $t_0 \in \mathbb{N}$  in the form  $t_0 = 17\ell_0 + r_0$ , where  $0 \leq r_0 \leq 16$ . Then  $\Omega^{t_0}(Y_t^{(19)})$  is a  $\Omega^{r_0}(Y_t^{(19)})$ , whose left components twisted by  $\sigma^{\ell_0}$ , and coefficients multiplied by  $(-1)^{\ell_0}$ .

**Proposition 15** (Translates for the case 20). (I) Let  $r_0 \in \mathbb{N}$ ,  $r_0 < 17$ .  $r_0$ -translates of the elements  $Y_t^{(20)}$  are described by the following way.

(1) If  $r_0 = 0$ , then  $\Omega^0(Y_t^{(20)})$  is described with  $(7s \times 7s)$ -matrix with one nonzero element that is of the following form:

$$b_{j,4s} = w_{7(j+m)+4 \rightarrow 7(j+m+1)+4} \otimes e_{7j+4}.$$

(2) If  $r_0 = 1$ , then  $\Omega^1(Y_t^{(20)})$  is described with  $(8s \times 8s)$ -matrix with one nonzero element that is of the following form:

$$b_{j,s} = w_{7(j+m)+4 \rightarrow 7(j+m+1)+4} \otimes e_{7j}.$$

(3) If  $r_0 = 2$ , then  $\Omega^2(Y_t^{(20)})$  is described with  $(7s \times 7s)$ -matrix with one nonzero element that is of the following form:

$$b_{j,3s} = w_{7(j+m)+4 \rightarrow 7(j+m+1)+4} \otimes e_{7j+3}.$$

(4) If  $r_0 = 3$ , then  $\Omega^3(Y_t^{(20)})$  is described with  $(9s \times 9s)$ -matrix with one nonzero element that is of the following form:

$$b_{j,8s} = w_{7(j+m)+4 \rightarrow 7(j+m+1)+4} \otimes e_{7j+6}.$$

(5) If  $r_0 = 4$ , then  $\Omega^4(Y_t^{(20)})$  is described with  $(10s \times 10s)$ -matrix with the following two nonzero elements:

$$b_{j,3s} = w_{7(j+m)+4 \rightarrow 7(j+m+1)+4} \otimes e_{7j+2};$$

$$b_{j,8s} = w_{7(j+m)+4 \rightarrow 7(j+m+1)+4} \otimes e_{7j+5}.$$

(6) If  $r_0 = 5$ , then  $\Omega^5(Y_t^{(20)})$  is described with  $(10s \times 10s)$ -matrix with one nonzero element that is of the following form:

$$b_{j,0} = w_{7(j+m)+4 \rightarrow 7(j+m+1)+4} \otimes e_{7j}.$$

(7) If  $r_0 = 6$ , then  $\Omega^6(Y_t^{(20)})$  is described with  $(12s \times 12s)$ -matrix with the following two nonzero elements:

$$b_{j,2s} = w_{7(j+m)+4 \rightarrow 7(j+m+1)+4} \otimes e_{7j+1};$$

$$b_{j,7s} = w_{7(j+m)+4 \rightarrow 7(j+m+1)+4} \otimes e_{7j+4}.$$

(8) If  $r_0 = 7$ , then  $\Omega^7(Y_t^{(20)})$  is described with  $(12s \times 12s)$ -matrix with the following two nonzero elements:

$$b_{j,2s} = w_{7(j+m)+4 \rightarrow 7(j+m+1)+4} \otimes e_{7j};$$

$$b_{j,9s} = w_{7(j+m)+4 \rightarrow 7(j+m+1)+4} \otimes e_{7j+6}.$$

(9) If  $r_0 = 8$ , then  $\Omega^8(Y_t^{(20)})$  is described with  $(13s \times 13s)$ -matrix with the following two nonzero elements:

$$b_{j,6s} = w_{7(j+m)+4 \rightarrow 7(j+m+1)+4} \otimes e_{7j+3};$$

$$b_{j,9s} = w_{7(j+m)+4 \rightarrow 7(j+m+1)+4} \otimes e_{7j+5}.$$

(10) If  $r_0 = 9$ , then  $\Omega^9(Y_t^{(20)})$  is described with  $(12s \times 12s)$ -matrix with one nonzero element that is of the following form:

$$b_{j,11s} = w_{7(j+m)+4 \rightarrow 7(j+m+1)+4} \otimes e_{7j+6}.$$

(11) If  $r_0 = 10$ , then  $\Omega^{10}(Y_t^{(20)})$  is described with  $(12s \times 12s)$ -matrix with the following two nonzero elements:

$$b_{j,4s} = w_{7(j+m)+4 \rightarrow 7(j+m+1)+4} \otimes e_{7j+2};$$

$$b_{j,6s} = w_{7(j+m)+4 \rightarrow 7(j+m+1)+4} \otimes e_{7j+4}.$$

(12) If  $r_0 = 11$ , then  $\Omega^{11}(Y_t^{(20)})$  is described with  $(10s \times 10s)$ -matrix with one nonzero element that is of the following form:

$$b_{j,s} = w_{7(j+m)+4 \rightarrow 7(j+m+1)+4} \otimes e_{7j}.$$

(13) If  $r_0 = 12$ , then  $\Omega^{12}(Y_t^{(20)})$  is described with  $(10s \times 10s)$ -matrix with one nonzero element that is of the following form:

$$b_{j,2s} = w_{7(j+m)+4 \rightarrow 7(j+m+1)+4} \otimes e_{7j+1}.$$

(14) If  $r_0 = 13$ , then  $\Omega^{13}(Y_t^{(20)})$  is described with  $(9s \times 9s)$ -matrix with one nonzero element that is of the following form:

$$b_{j,8s} = w_{7(j+m)+4 \rightarrow 7(j+m+1)+4} \otimes e_{7j+6}.$$

(15) If  $r_0 = 14$ , then  $\Omega^{14}(Y_t^{(20)})$  is described with  $(7s \times 7s)$ -matrix with one nonzero element that is of the following form:

$$b_{j,5s} = w_{7(j+m)+4 \rightarrow 7(j+m+1)+4} \otimes e_{7j+5}.$$

(16) If  $r_0 = 15$ , then  $\Omega^{15}(Y_t^{(20)})$  is described with  $(8s \times 8s)$ -matrix with one nonzero element that is of the following form:

$$b_{j,5s} = w_{7(j+m)+4 \rightarrow 7(j+m+1)+4} \otimes e_{7j+5}.$$

(17) If  $r_0 = 16$ , then  $\Omega^{16}(Y_t^{(20)})$  is described with  $(7s \times 7s)$ -matrix with one nonzero element that is of the following form:

$$b_{j,4s} = w_{7(j+m)+4 \rightarrow 7(j+m+1)+4} \otimes e_{7j+4}.$$

(II) Represent an arbitrary  $t_0 \in \mathbb{N}$  in the form  $t_0 = 17\ell_0 + r_0$ , where  $0 \leq r_0 \leq 16$ . Then  $\Omega^{t_0}(Y_t^{(20)})$  is a  $\Omega^{r_0}(Y_t^{(20)})$ , whose left components twisted by  $\sigma^{\ell_0}$ , and coefficients multiplied by  $(-1)^{\ell_0}$ .

**Proposition 16** (Translates for the case 21). (I) Let  $r_0 \in \mathbb{N}$ ,  $r_0 < 17$ .  $r_0$ -translates of the elements  $Y_t^{(21)}$  are described by the following way.

(1) If  $r_0 = 0$ , then  $\Omega^0(Y_t^{(21)})$  is described with  $(7s \times 7s)$ -matrix with one nonzero element that is of the following form:

$$b_{j,5s} = w_{7(j+m)+5 \rightarrow 7(j+m+1)+5} \otimes e_{7j+5}.$$

(2) If  $r_0 = 1$ , then  $\Omega^1(Y_t^{(21)})$  is described with  $(8s \times 8s)$ -matrix with one nonzero element that is of the following form:

$$b_{j,5s} = w_{7(j+m)+5 \rightarrow 7(j+m+1)+5} \otimes e_{7j+4}.$$

(3) If  $r_0 = 2$ , then  $\Omega^2(Y_t^{(21)})$  is described with  $(7s \times 7s)$ -matrix with one nonzero element that is of the following form:

$$b_{j,4s} = w_{7(j+m)+5 \rightarrow 7(j+m+1)+5} \otimes e_{7j+4}.$$

(4) If  $r_0 = 3$ , then  $\Omega^3(Y_t^{(21)})$  is described with  $(9s \times 9s)$ -matrix with one nonzero element that is of the following form:

$$b_{j,s} = w_{7(j+m)+5 \rightarrow 7(j+m+1)+5} \otimes e_{7j}.$$

(5) If  $r_0 = 4$ , then  $\Omega^4(Y_t^{(21)})$  is described with  $(10s \times 10s)$ -matrix with one nonzero element that is of the following form:

$$b_{j,5s} = w_{7(j+m)+5 \rightarrow 7(j+m+1)+5} \otimes e_{7j+3}.$$

(6) If  $r_0 = 5$ , then  $\Omega^5(Y_t^{(21)})$  is described with  $(10s \times 10s)$ -matrix with one nonzero element that is of the following form:

$$b_{j,9s} = w_{7(j+m)+5 \rightarrow 7(j+m+1)+5} \otimes e_{7j+6}.$$

(7) If  $r_0 = 6$ , then  $\Omega^6(Y_t^{(21)})$  is described with  $(12s \times 12s)$ -matrix with the following two nonzero elements:

$$b_{j,4s} = w_{7(j+m)+5 \rightarrow 7(j+m+1)+5} \otimes e_{7j+2};$$

$$b_{j,9s} = w_{7(j+m)+5 \rightarrow 7(j+m+1)+5} \otimes e_{7j+5}.$$

(8) If  $r_0 = 7$ , then  $\Omega^7(Y_t^{(21)})$  is described with  $(12s \times 12s)$ -matrix with one nonzero element that is of the following form:

$$b_{j,s} = w_{7(j+m)+5 \rightarrow 7(j+m+1)+5} \otimes e_{7j}.$$

(9) If  $r_0 = 8$ , then  $\Omega^8(Y_t^{(21)})$  is described with  $(13s \times 13s)$ -matrix with the following two nonzero elements:

$$b_{j,3s} = w_{7(j+m)+5 \rightarrow 7(j+m+1)+5} \otimes e_{7j+1};$$

$$b_{j,8s} = w_{7(j+m)+5 \rightarrow 7(j+m+1)+5} \otimes e_{7j+4}.$$

(10) If  $r_0 = 9$ , then  $\Omega^9(Y_t^{(21)})$  is described with  $(12s \times 12s)$ -matrix with the following two nonzero elements:

$$b_{j,0} = w_{7(j+m)+5 \rightarrow 7(j+m+1)+5} \otimes e_{7j};$$

$$b_{j,10s} = w_{7(j+m)+5 \rightarrow 7(j+m+1)+5} \otimes e_{7j+6}.$$

(11) If  $r_0 = 10$ , then  $\Omega^{10}(Y_t^{(21)})$  is described with  $(12s \times 12s)$ -matrix with the following two nonzero elements:

$$b_{j,5s} = w_{7(j+m)+5 \rightarrow 7(j+m+1)+5} \otimes e_{7j+3};$$

$$b_{j,9s} = w_{7(j+m)+5 \rightarrow 7(j+m+1)+5} \otimes e_{7j+5}.$$

(12) If  $r_0 = 11$ , then  $\Omega^{11}(Y_t^{(21)})$  is described with  $(10s \times 10s)$ -matrix with one nonzero element that is of the following form:

$$b_{j,7s} = w_{7(j+m)+5 \rightarrow 7(j+m+1)+5} \otimes e_{7j+6}.$$

(13) If  $r_0 = 12$ , then  $\Omega^{12}(Y_t^{(21)})$  is described with  $(10s \times 10s)$ -matrix with the following two nonzero elements:

$$b_{j,3s} = w_{7(j+m)+5 \rightarrow 7(j+m+1)+5} \otimes e_{7j+2};$$

$$b_{j,6s} = w_{7(j+m)+5 \rightarrow 7(j+m+1)+5} \otimes e_{7j+4}.$$

(14) If  $r_0 = 13$ , then  $\Omega^{13}(Y_t^{(21)})$  is described with  $(9s \times 9s)$ -matrix with one nonzero element that is of the following form:

$$b_{j,s} = w_{7(j+m)+5 \rightarrow 7(j+m+1)+5} \otimes e_{7j}.$$

(15) If  $r_0 = 14$ , then  $\Omega^{14}(Y_t^{(21)})$  is described with  $(7s \times 7s)$ -matrix with one nonzero element that is of the following form:

$$b_{j,s} = w_{7(j+m)+5 \rightarrow 7(j+m+1)+5} \otimes e_{7j+1}.$$

(16) If  $r_0 = 15$ , then  $\Omega^{15}(Y_t^{(21)})$  is described with  $(8s \times 8s)$ -matrix with one nonzero element that is of the following form:

$$b_{j,7s} = w_{7(j+m)+5 \rightarrow 7(j+m+1)+5} \otimes e_{7j+6}.$$

(17) If  $r_0 = 16$ , then  $\Omega^{16}(Y_t^{(21)})$  is described with  $(7s \times 7s)$ -matrix with one nonzero element that is of the following form:

$$b_{j,5s} = w_{7(j+m)+5 \rightarrow 7(j+m+1)+5} \otimes e_{7j+5}.$$

(II) Represent an arbitrary  $t_0 \in \mathbb{N}$  in the form  $t_0 = 17\ell_0 + r_0$ , where  $0 \leq r_0 \leq 16$ . Then  $\Omega^{t_0}(Y_t^{(21)})$  is a  $\Omega^{r_0}(Y_t^{(21)})$ , whose left components twisted by  $\sigma^{\ell_0}$ , and coefficients multiplied by  $(-1)^{\ell_0}$ .



**Proposition 17** (Translates for the case 22). (I) Let  $r_0 \in \mathbb{N}$ ,  $r_0 < 17$ .  $r_0$ -translates of the elements  $Y_t^{(22)}$  are described by the following way.

(1) If  $r_0 = 0$ , then  $\Omega^0(Y_t^{(22)})$  is described with  $(7s \times 7s)$ -matrix with one nonzero element that is of the following form:

$$b_{j,3s} = w_{7(j+m)+3 \rightarrow 7(j+m+1)+3} \otimes e_{7j+3}.$$

(2) If  $r_0 = 1$ , then  $\Omega^1(Y_t^{(22)})$  is described with  $(8s \times 8s)$ -matrix with one nonzero element that is of the following form:

$$b_{j,3s} = w_{7(j+m)+3 \rightarrow 7(j+m+1)+3} \otimes e_{7j+2}.$$

(3) If  $r_0 = 2$ , then  $\Omega^2(Y_t^{(22)})$  is described with  $(7s \times 7s)$ -matrix with one nonzero element that is of the following form:

$$b_{j,2s} = w_{7(j+m)+3 \rightarrow 7(j+m+1)+3} \otimes e_{7j+2}.$$

(4) If  $r_0 = 3$ , then  $\Omega^3(Y_t^{(22)})$  is described with  $(9s \times 9s)$ -matrix with one nonzero element that is of the following form:

$$b_{j,2s} = w_{7(j+m)+3 \rightarrow 7(j+m+1)+3} \otimes e_{7j+1}.$$

(5) If  $r_0 = 4$ , then  $\Omega^4(Y_t^{(22)})$  is described with  $(10s \times 10s)$ -matrix with one nonzero element that is of the following form:

$$b_{j,2s} = w_{7(j+m)+3 \rightarrow 7(j+m+1)+3} \otimes e_{7j+1}.$$

(6) If  $r_0 = 5$ , then  $\Omega^5(Y_t^{(22)})$  is described with  $(10s \times 10s)$ -matrix with one nonzero element that is of the following form:

$$b_{j,s} = w_{7(j+m)+3 \rightarrow 7(j+m+1)+3} \otimes e_{7j}.$$

(7) If  $r_0 = 6$ , then  $\Omega^6(Y_t^{(22)})$  is described with  $(12s \times 12s)$ -matrix with one nonzero element that is of the following form:

$$b_{j,8s} = w_{7(j+m)+3 \rightarrow 7(j+m+1)+3} \otimes e_{7j+5}.$$

(8) If  $r_0 = 7$ , then  $\Omega^7(Y_t^{(22)})$  is described with  $(12s \times 12s)$ -matrix with one nonzero element that is of the following form:

$$b_{j,10s} = w_{7(j+m)+3 \rightarrow 7(j+m+1)+3} \otimes e_{7j+6}.$$

(9) If  $r_0 = 8$ , then  $\Omega^8(Y_t^{(22)})$  is described with  $(13s \times 13s)$ -matrix with the following two nonzero elements:

$$b_{j,5s} = w_{7(j+m)+3 \rightarrow 7(j+m+1)+3} \otimes e_{7j+3};$$

$$b_{j,7s} = w_{7(j+m)+3 \rightarrow 7(j+m+1)+3} \otimes e_{7j+4}.$$

(10) If  $r_0 = 9$ , then  $\Omega^9(Y_t^{(22)})$  is described with  $(12s \times 12s)$ -matrix with one nonzero element that is of the following form:

$$b_{j,s} = w_{7(j+m)+3 \rightarrow 7(j+m+1)+3} \otimes e_{7j}.$$

(11) If  $r_0 = 10$ , then  $\Omega^{10}(Y_t^{(22)})$  is described with  $(12s \times 12s)$ -matrix with one nonzero element that is of the following form:

$$b_{j,3s} = w_{7(j+m)+3 \rightarrow 7(j+m+1)+3} \otimes e_{7j+2}.$$

(12) If  $r_0 = 11$ , then  $\Omega^{11}(Y_t^{(22)})$  is described with  $(10s \times 10s)$ -matrix with one nonzero element that is of the following form:

$$b_{j,8s} = w_{7(j+m)+3 \rightarrow 7(j+m+1)+3} \otimes e_{7j+6}.$$

(13) If  $r_0 = 12$ , then  $\Omega^{12}(Y_t^{(22)})$  is described with  $(10s \times 10s)$ -matrix with the following two nonzero elements:

$$b_{j,s} = w_{7(j+m)+3 \rightarrow 7(j+m+1)+3} \otimes e_{7j+1};$$

$$b_{j,7s} = w_{7(j+m)+3 \rightarrow 7(j+m+1)+3} \otimes e_{7j+5}.$$

(14) If  $r_0 = 13$ , then  $\Omega^{13}(Y_t^{(22)})$  is described with  $(9s \times 9s)$ -matrix with one nonzero element that is of the following form:

$$b_{j,0} = w_{7(j+m)+3 \rightarrow 7(j+m+1)+3} \otimes e_{7j}.$$

(15) If  $r_0 = 14$ , then  $\Omega^{14}(Y_t^{(22)})$  is described with  $(7s \times 7s)$ -matrix with one nonzero element that is of the following form:

$$b_{j,4s} = w_{7(j+m)+3 \rightarrow 7(j+m+1)+3} \otimes e_{7j+4}.$$

(16) If  $r_0 = 15$ , then  $\Omega^{15}(Y_t^{(22)})$  is described with  $(8s \times 8s)$ -matrix with one nonzero element that is of the following form:

$$b_{j,6s} = w_{7(j+m)+3 \rightarrow 7(j+m+1)+3} \otimes e_{7j+6}.$$

(17) If  $r_0 = 16$ , then  $\Omega^{16}(Y_t^{(22)})$  is described with  $(7s \times 7s)$ -matrix with one nonzero element that is of the following form:

$$b_{j,3s} = w_{7(j+m)+3 \rightarrow 7(j+m+1)+3} \otimes e_{7j+3}.$$

(II) Represent an arbitrary  $t_0 \in \mathbb{N}$  in the form  $t_0 = 17\ell_0 + r_0$ , where  $0 \leq r_0 \leq 16$ . Then  $\Omega^{t_0}(Y_t^{(22)})$  is a  $\Omega^{r_0}(Y_t^{(22)})$ , whose left components twisted by  $\sigma^{\ell_0}$ , and coefficients multiplied by  $(-1)^{\ell_0}$ .

**Proposition 18** (Translates for the case 23). (I) Let  $r_0 \in \mathbb{N}$ ,  $r_0 < 17$ .  $r_0$ -translates of the elements  $Y_t^{(23)}$  are described by the following way.

(1) If  $r_0 = 0$ , then  $\Omega^0(Y_t^{(23)})$  is described with  $(7s \times 7s)$ -matrix with one nonzero element that is of the following form:

$$b_{j,s} = w_{7(j+m)+1 \rightarrow 7(j+m+1)+1} \otimes e_{7j+1}.$$

(2) If  $r_0 = 1$ , then  $\Omega^1(Y_t^{(23)})$  is described with  $(8s \times 8s)$ -matrix with one nonzero element that is of the following form:

$$b_{j,0} = w_{7(j+m)+1 \rightarrow 7(j+m+1)+1} \otimes e_{7j}.$$

(3) If  $r_0 = 2$ , then  $\Omega^2(Y_t^{(23)})$  is described with  $(7s \times 7s)$ -matrix with one nonzero element that is of the following form:

$$b_{j,5s} = w_{7(j+m)+1 \rightarrow 7(j+m+1)+1} \otimes e_{7j+5}.$$

(4) If  $r_0 = 3$ , then  $\Omega^3(Y_t^{(23)})$  is described with  $(9s \times 9s)$ -matrix with one nonzero element that is of the following form:

$$b_{j,7s} = w_{7(j+m)+1 \rightarrow 7(j+m+1)+1} \otimes e_{7j+6}.$$

(5) If  $r_0 = 4$ , then  $\Omega^4(Y_t^{(23)})$  is described with  $(10s \times 10s)$ -matrix with the following two nonzero elements:

$$b_{j,4s} = w_{7(j+m)+1 \rightarrow 7(j+m+1)+1} \otimes e_{7j+3};$$

$$b_{j,6s} = w_{7(j+m)+1 \rightarrow 7(j+m+1)+1} \otimes e_{7j+4}.$$

(6) If  $r_0 = 5$ , then  $\Omega^5(Y_t^{(23)})$  is described with  $(10s \times 10s)$ -matrix with one nonzero element that is of the following form:

$$b_{j,2s} = w_{7(j+m)+1 \rightarrow 7(j+m+1)+1} \otimes e_{7j}.$$

(7) If  $r_0 = 6$ , then  $\Omega^6(Y_t^{(23)})$  is described with  $(12s \times 12s)$ -matrix with one nonzero element that is of the following form:

$$b_{j,3s} = w_{7(j+m)+1 \rightarrow 7(j+m+1)+1} \otimes e_{7j+2}.$$

(8) If  $r_0 = 7$ , then  $\Omega^7(Y_t^{(23)})$  is described with  $(12s \times 12s)$ -matrix with one nonzero element that is of the following form:

$$b_{j,11s} = w_{7(j+m)+1 \rightarrow 7(j+m+1)+1} \otimes e_{7j+6}.$$

(9) If  $r_0 = 8$ , then  $\Omega^8(Y_t^{(23)})$  is described with  $(13s \times 13s)$ -matrix with the following two nonzero elements:

$$b_{j,2s} = w_{7(j+m)+1 \rightarrow 7(j+m+1)+1} \otimes e_{7j+1};$$

$$b_{j,10s} = w_{7(j+m)+1 \rightarrow 7(j+m+1)+1} \otimes e_{7j+5}.$$

(10) If  $r_0 = 9$ , then  $\Omega^9(Y_t^{(23)})$  is described with  $(12s \times 12s)$ -matrix with one nonzero element that is of the following form:

$$b_{j,2s} = w_{7(j+m)+1 \rightarrow 7(j+m+1)+1} \otimes e_{7j}.$$

(11) If  $r_0 = 10$ , then  $\Omega^{10}(Y_t^{(23)})$  is described with  $(12s \times 12s)$ -matrix with one nonzero element that is of the following form:

$$b_{j,7s} = w_{7(j+m)+1 \rightarrow 7(j+m+1)+1} \otimes e_{7j+4}.$$

(12) If  $r_0 = 11$ , then  $\Omega^{11}(Y_t^{(23)})$  is described with  $(10s \times 10s)$ -matrix with one nonzero element that is of the following form:

$$b_{j,9s} = w_{7(j+m)+1 \rightarrow 7(j+m+1)+1} \otimes e_{7j+6}.$$

(13) If  $r_0 = 12$ , then  $\Omega^{12}(Y_t^{(23)})$  is described with  $(10s \times 10s)$ -matrix with one nonzero element that is of the following form:

$$b_{j,4s} = w_{7(j+m)+1 \rightarrow 7(j+m+1)+1} \otimes e_{7j+3}.$$

(14) If  $r_0 = 13$ , then  $\Omega^{13}(Y_t^{(23)})$  is described with  $(9s \times 9s)$ -matrix with one nonzero element that is of the following form:

$$b_{j,4s} = w_{7(j+m)+1 \rightarrow 7(j+m+1)+1} \otimes e_{7j+3}.$$

(15) If  $r_0 = 14$ , then  $\Omega^{14}(Y_t^{(23)})$  is described with  $(7s \times 7s)$ -matrix with one nonzero element that is of the following form:

$$b_{j,2s} = w_{7(j+m)+1 \rightarrow 7(j+m+1)+1} \otimes e_{7j+2}.$$

(16) If  $r_0 = 15$ , then  $\Omega^{15}(Y_t^{(23)})$  is described with  $(8s \times 8s)$ -matrix with one nonzero element that is of the following form:

$$b_{j,2s} = w_{7(j+m)+1 \rightarrow 7(j+m+1)+1} \otimes e_{7j+2}.$$

(17) If  $r_0 = 16$ , then  $\Omega^{16}(Y_t^{(23)})$  is described with  $(7s \times 7s)$ -matrix with one nonzero element that is of the following form:

$$b_{j,s} = w_{7(j+m)+1 \rightarrow 7(j+m+1)+1} \otimes e_{7j+1}.$$

(II) Represent an arbitrary  $t_0 \in \mathbb{N}$  in the form  $t_0 = 17\ell_0 + r_0$ , where  $0 \leq r_0 \leq 16$ . Then  $\Omega^{t_0}(Y_t^{(23)})$  is a  $\Omega^{r_0}(Y_t^{(23)})$ , whose left components twisted by  $\sigma^{\ell_0}$ , and coefficients multiplied by  $(-1)^{\ell_0}$ .

**Proposition 19** (Translates for the case 24). (I) Let  $r_0 \in \mathbb{N}$ ,  $r_0 < 17$ .  $r_0$ -translates of the elements  $Y_t^{(24)}$  are described by the following way.

(1) If  $r_0 = 0$ , then  $\Omega^0(Y_t^{(24)})$  is described with  $(7s \times 7s)$ -matrix with one nonzero element that is of the following form:

$$b_{j,2s} = w_{7(j+m)+2 \rightarrow 7(j+m+1)+2} \otimes e_{7j+2}.$$

(2) If  $r_0 = 1$ , then  $\Omega^1(Y_t^{(24)})$  is described with  $(8s \times 8s)$ -matrix with one nonzero element that is of the following form:

$$b_{j,2s} = w_{7(j+m)+2 \rightarrow 7(j+m+1)+2} \otimes e_{7j+1}.$$

(3) If  $r_0 = 2$ , then  $\Omega^2(Y_t^{(24)})$  is described with  $(7s \times 7s)$ -matrix with one nonzero element that is of the following form:

$$b_{j,s} = w_{7(j+m)+2 \rightarrow 7(j+m+1)+2} \otimes e_{7j+1}.$$

(4) If  $r_0 = 3$ , then  $\Omega^3(Y_t^{(24)})$  is described with  $(9s \times 9s)$ -matrix with one nonzero element that is of the following form:

$$b_{j,0} = w_{7(j+m)+2 \rightarrow 7(j+m+1)+2} \otimes e_{7j}.$$

(5) If  $r_0 = 4$ , then  $\Omega^4(Y_t^{(24)})$  is described with  $(10s \times 10s)$ -matrix with one nonzero element that is of the following form:

$$b_{j,7s} = w_{7(j+m)+2 \rightarrow 7(j+m+1)+2} \otimes e_{7j+5}.$$

(6) If  $r_0 = 5$ , then  $\Omega^5(Y_t^{(24)})$  is described with  $(10s \times 10s)$ -matrix with one nonzero element that is of the following form:

$$b_{j,8s} = w_{7(j+m)+2 \rightarrow 7(j+m+1)+2} \otimes e_{7j+6}.$$

(7) If  $r_0 = 6$ , then  $\Omega^6(Y_t^{(24)})$  is described with  $(12s \times 12s)$ -matrix with the following two nonzero elements:

$$b_{j,5s} = w_{7(j+m)+2 \rightarrow 7(j+m+1)+2} \otimes e_{7j+3};$$

$$b_{j,6s} = w_{7(j+m)+2 \rightarrow 7(j+m+1)+2} \otimes e_{7j+4}.$$

(8) If  $r_0 = 7$ , then  $\Omega^7(Y_t^{(24)})$  is described with  $(12s \times 12s)$ -matrix with one nonzero element that is of the following form:

$$b_{j,0} = w_{7(j+m)+2 \rightarrow 7(j+m+1)+2} \otimes e_{7j}.$$

(9) If  $r_0 = 8$ , then  $\Omega^8(Y_t^{(24)})$  is described with  $(13s \times 13s)$ -matrix with one nonzero element that is of the following form:

$$b_{j,4s} = w_{7(j+m)+2 \rightarrow 7(j+m+1)+2} \otimes e_{7j+2}.$$

(10) If  $r_0 = 9$ , then  $\Omega^9(Y_t^{(24)})$  is described with  $(12s \times 12s)$ -matrix with one nonzero element that is of the following form:

$$b_{j,9s} = w_{7(j+m)+2 \rightarrow 7(j+m+1)+2} \otimes e_{7j+6}.$$

(11) If  $r_0 = 10$ , then  $\Omega^{10}(Y_t^{(24)})$  is described with  $(12s \times 12s)$ -matrix with the following two nonzero elements:

$$b_{j,2s} = w_{7(j+m)+2 \rightarrow 7(j+m+1)+2} \otimes e_{7j+1};$$

$$b_{j,8s} = w_{7(j+m)+2 \rightarrow 7(j+m+1)+2} \otimes e_{7j+5}.$$

(12) If  $r_0 = 11$ , then  $\Omega^{11}(Y_t^{(24)})$  is described with  $(10s \times 10s)$ -matrix with one nonzero element that is of the following form:

$$b_{j,0} = w_{7(j+m)+2 \rightarrow 7(j+m+1)+2} \otimes e_{7j}.$$

(13) If  $r_0 = 12$ , then  $\Omega^{12}(Y_t^{(24)})$  is described with  $(10s \times 10s)$ -matrix with one nonzero element that is of the following form:

$$b_{j,5s} = w_{7(j+m)+2 \rightarrow 7(j+m+1)+2} \otimes e_{7j+4}.$$

(14) If  $r_0 = 13$ , then  $\Omega^{13}(Y_t^{(24)})$  is described with  $(9s \times 9s)$ -matrix with one nonzero element that is of the following form:

$$b_{j,7s} = w_{7(j+m)+2 \rightarrow 7(j+m+1)+2} \otimes e_{7j+6}.$$

(15) If  $r_0 = 14$ , then  $\Omega^{14}(Y_t^{(24)})$  is described with  $(7s \times 7s)$ -matrix with one nonzero element that is of the following form:

$$b_{j,3s} = w_{7(j+m)+2 \rightarrow 7(j+m+1)+2} \otimes e_{7j+3}.$$

(16) If  $r_0 = 15$ , then  $\Omega^{15}(Y_t^{(24)})$  is described with  $(8s \times 8s)$ -matrix with one nonzero element that is of the following form:

$$b_{j,3s} = w_{7(j+m)+2 \rightarrow 7(j+m+1)+2} \otimes e_{7j+3}.$$

(17) If  $r_0 = 16$ , then  $\Omega^{16}(Y_t^{(24)})$  is described with  $(7s \times 7s)$ -matrix with one nonzero element that is of the following form:

$$b_{j,2s} = w_{7(j+m)+2 \rightarrow 7(j+m+1)+2} \otimes e_{7j+2}.$$

(II) Represent an arbitrary  $t_0 \in \mathbb{N}$  in the form  $t_0 = 17\ell_0 + r_0$ , where  $0 \leq r_0 \leq 16$ . Then  $\Omega^{t_0}(Y_t^{(24)})$  is a  $\Omega^{r_0}(Y_t^{(24)})$ , whose left components twisted by  $\sigma^{\ell_0}$ , and coefficients multiplied by  $(-1)^{\ell_0}$ .

**Proposition 20** (Translates for the case 25). (I) Let  $r_0 \in \mathbb{N}$ ,  $r_0 < 17$ .  $r_0$ -translates of the elements  $Y_t^{(25)}$  are described by the following way.

(1) If  $r_0 = 0$ , then  $\Omega^0(Y_t^{(25)})$  is described with  $(7s \times 7s)$ -matrix with one nonzero element that is of the following form:

$$b_{j,6s} = w_{7(j+m)+6 \rightarrow 7(j+m+1)+6} \otimes e_{7j+6}.$$

(2) If  $r_0 = 1$ , then  $\Omega^1(Y_t^{(25)})$  is described with  $(8s \times 8s)$ -matrix with the following two nonzero elements:

$$\begin{aligned} b_{j,4s} &= w_{7(j+m)+6 \rightarrow 7(j+m+1)+6} \otimes e_{7j+3}; \\ b_{j,6s} &= w_{7(j+m)+6 \rightarrow 7(j+m+1)+6} \otimes e_{7j+5}. \end{aligned}$$

(3) If  $r_0 = 2$ , then  $\Omega^2(Y_t^{(25)})$  is described with  $(7s \times 7s)$ -matrix with one nonzero element that is of the following form:

$$b_{j,0} = w_{7(j+m)+6 \rightarrow 7(j+m+1)+6} \otimes e_{7j}.$$

(4) If  $r_0 = 3$ , then  $\Omega^3(Y_t^{(25)})$  is described with  $(9s \times 9s)$ -matrix with the following two nonzero elements:

$$\begin{aligned} b_{j,3s} &= w_{7(j+m)+6 \rightarrow 7(j+m+1)+6} \otimes e_{7j+2}; \\ b_{j,5s} &= w_{7(j+m)+6 \rightarrow 7(j+m+1)+6} \otimes e_{7j+4}. \end{aligned}$$

(5) If  $r_0 = 4$ , then  $\Omega^4(Y_t^{(25)})$  is described with  $(10s \times 10s)$ -matrix with the following two nonzero elements:

$$\begin{aligned} b_{j,0} &= w_{7(j+m)+6 \rightarrow 7(j+m+1)+6} \otimes e_{7j}; \\ b_{j,9s} &= w_{7(j+m)+6 \rightarrow 7(j+m+1)+6} \otimes e_{7j+6}. \end{aligned}$$

(6) If  $r_0 = 5$ , then  $\Omega^5(Y_t^{(25)})$  is described with  $(10s \times 10s)$ -matrix with the following nonzero elements:

$$\begin{aligned} b_{j,3s} &= w_{7(j+m)+6 \rightarrow 7(j+m+1)+6} \otimes e_{7j+1}; \\ b_{j,5s} &= w_{7(j+m)+6 \rightarrow 7(j+m+1)+6} \otimes e_{7j+3}; \\ b_{j,7s} &= w_{7(j+m)+6 \rightarrow 7(j+m+1)+6} \otimes e_{7j+5}. \end{aligned}$$

(7) If  $r_0 = 6$ , then  $\Omega^6(Y_t^{(25)})$  is described with  $(12s \times 12s)$ -matrix with the following two nonzero elements:

$$\begin{aligned} b_{j,0} &= w_{7(j+m)+6 \rightarrow 7(j+m+1)+6} \otimes e_{7j}; \\ b_{j,10s} &= w_{7(j+m)+6 \rightarrow 7(j+m+1)+6} \otimes e_{7j+6}. \end{aligned}$$

(8) If  $r_0 = 7$ , then  $\Omega^7(Y_t^{(25)})$  is described with  $(12s \times 12s)$ -matrix with the following nonzero elements:

$$\begin{aligned} b_{j,4s} &= w_{7(j+m)+6 \rightarrow 7(j+m+1)+6} \otimes e_{7j+2}; \\ b_{j,6s} &= w_{7(j+m)+6 \rightarrow 7(j+m+1)+6} \otimes e_{7j+4}; \\ b_{j,7s} &= w_{7(j+m)+6 \rightarrow 7(j+m+1)+6} \otimes e_{7j+5}. \end{aligned}$$

(9) If  $r_0 = 8$ , then  $\Omega^8(Y_t^{(25)})$  is described with  $(13s \times 13s)$ -matrix with the following two nonzero elements:

$$\begin{aligned} b_{j,0} &= w_{7(j+m)+6 \rightarrow 7(j+m+1)+6} \otimes e_{7j}; \\ b_{j,11s} &= w_{7(j+m)+6 \rightarrow 7(j+m+1)+6} \otimes e_{7j+6}. \end{aligned}$$

(10) If  $r_0 = 9$ , then  $\Omega^9(Y_t^{(25)})$  is described with  $(12s \times 12s)$ -matrix with the following nonzero elements:

$$\begin{aligned} b_{j,3s} &= w_{7(j+m)+6 \rightarrow 7(j+m+1)+6} \otimes e_{7j+1}; \\ b_{j,5s} &= w_{7(j+m)+6 \rightarrow 7(j+m+1)+6} \otimes e_{7j+3}; \\ b_{j,6s} &= w_{7(j+m)+6 \rightarrow 7(j+m+1)+6} \otimes e_{7j+4}. \end{aligned}$$

(11) If  $r_0 = 10$ , then  $\Omega^{10}(Y_t^{(25)})$  is described with  $(12s \times 12s)$ -matrix with the following two nonzero elements:

$$b_{j,0} = w_{7(j+m)+6 \rightarrow 7(j+m+1)+6} \otimes e_{7j};$$

$$b_{j,10s} = w_{7(j+m)+6 \rightarrow 7(j+m+1)+6} \otimes e_{7j+6}.$$

(12) If  $r_0 = 11$ , then  $\Omega^{11}(Y_t^{(25)})$  is described with  $(10s \times 10s)$ -matrix with the following two nonzero elements:

$$b_{j,3s} = w_{7(j+m)+6 \rightarrow 7(j+m+1)+6} \otimes e_{7j+2};$$

$$b_{j,6s} = w_{7(j+m)+6 \rightarrow 7(j+m+1)+6} \otimes e_{7j+5}.$$

(13) If  $r_0 = 12$ , then  $\Omega^{12}(Y_t^{(25)})$  is described with  $(10s \times 10s)$ -matrix with one nonzero element that is of the following form:

$$b_{j,8s} = w_{7(j+m)+6 \rightarrow 7(j+m+1)+6} \otimes e_{7j+6}.$$

(14) If  $r_0 = 13$ , then  $\Omega^{13}(Y_t^{(25)})$  is described with  $(9s \times 9s)$ -matrix with the following two nonzero elements:

$$b_{j,2s} = w_{7(j+m)+6 \rightarrow 7(j+m+1)+6} \otimes e_{7j+1};$$

$$b_{j,5s} = w_{7(j+m)+6 \rightarrow 7(j+m+1)+6} \otimes e_{7j+4}.$$

(15) If  $r_0 = 14$ , then  $\Omega^{14}(Y_t^{(25)})$  is described with  $(7s \times 7s)$ -matrix with one nonzero element that is of the following form:

$$b_{j,0} = w_{7(j+m)+6 \rightarrow 7(j+m+1)+6} \otimes e_{7j}.$$

(16) If  $r_0 = 15$ , then  $\Omega^{15}(Y_t^{(25)})$  is described with  $(8s \times 8s)$ -matrix with one nonzero element that is of the following form:

$$b_{j,0} = w_{7(j+m)+6 \rightarrow 7(j+m+1)+6} \otimes e_{7j}.$$

(17) If  $r_0 = 16$ , then  $\Omega^{16}(Y_t^{(25)})$  is described with  $(7s \times 7s)$ -matrix with one nonzero element that is of the following form:

$$b_{j,6s} = w_{7(j+m)+6 \rightarrow 7(j+m+1)+6} \otimes e_{7j+6}.$$

(II) Represent an arbitrary  $t_0 \in \mathbb{N}$  in the form  $t_0 = 17\ell_0 + r_0$ , where  $0 \leq r_0 \leq 16$ . Then  $\Omega^{t_0}(Y_t^{(25)})$  is a  $\Omega^{r_0}(Y_t^{(25)})$ , whose left components twisted by  $\sigma^{\ell_0}$ , and coefficients multiplied by  $(-1)^{\ell_0}$ .
