# Supplementary material for: Hochschild cohomology rings for self-injective algebras of tree classes $E_7$ and $E_8$
Source: arXiv:1910.03043 ancillary file (2021-02-14)
Supplement: Supplementary file 3 [file e8-differentials.pdf]

## TREE CLASS $E_8$ : DIFFERENTIALS OF THE BIMODULE RESOLUTION

Since  $Q_i$  are direct sums, their elements can be concerned as column vectors. Hence the differentials can be described by matrixes (which are multiplied by column vectors from the right). Now we describe the entries of the matrices of the differentials.

*Remark 1.* The numeration of rows and columns always starts with zero.

### Notation.

- (1) Denote by  $w_{i \rightarrow j}$  a path from the  $i$ th vertex to the  $j$ th vertex.
- (2) For the  $j$ th column of the differential matrix, denote by  $j_2$  the integral part of  $j$  modulo  $s$ .

### Description of $d_0$

$d_0 : Q_1 \rightarrow Q_0$  - is an  $(8s \times 9s)$  matrix.

If  $0 \leq j < s$ , then

$$(d_0)_{ij} = \begin{cases} w_{8(j+m) \rightarrow 8(j+m)+1} \otimes e_{8j}, & i = j; \\ -e_{8(j+m)+1} \otimes w_{8j \rightarrow 8j+1}, & i = j + s; \\ 0, & \text{otherwise.} \end{cases}$$

If  $s \leq j < 2s$ , then

$$(d_0)_{ij} = \begin{cases} w_{8(j+m) \rightarrow 8(j+m)+5} \otimes e_{8j}, & i = j; \\ -e_{8(j+m)+5} \otimes w_{8j \rightarrow 8j+5}, & i = j + 4s; \\ 0, & \text{otherwise.} \end{cases}$$

If  $2s \leq j < 5s$ , then

$$(d_0)_{ij} = \begin{cases} w_{8(j+m)+j_2-1 \rightarrow 8(j+m)+j_2} \otimes e_{8j+j_2-1}, & i = j - s; \\ -e_{8(j+m)+j_2} \otimes w_{8j+j_2-1 \rightarrow 8j+j_2}, & i = j; \\ 0, & \text{otherwise.} \end{cases}$$

If  $5s \leq j < 6s$ , then

$$(d_0)_{ij} = \begin{cases} w_{8(j+m)+4 \rightarrow 8(j+m)+7} \otimes e_{8j+4}, & i = j - s; \\ -e_{8(j+m)+7} \otimes w_{8j+4 \rightarrow 8j+7}, & i = j + 2s; \\ 0, & \text{otherwise.} \end{cases}$$

If  $6s \leq j < 8s$ , then

$$(d_0)_{ij} = \begin{cases} w_{8(j+m)+j_2-1 \rightarrow 8(j+m)+j_2} \otimes e_{8j+j_2-1}, & i = j - s; \\ -e_{8(j+m)+j_2} \otimes w_{8j+j_2-1 \rightarrow 8j+j_2}, & i = j; \\ 0, & \text{otherwise.} \end{cases}$$

If  $8s \leq j < 9s$ , then

$$(d_0)_{ij} = \begin{cases} -e_{8(j+m)+1} \otimes w_{8j+7 \rightarrow 8(j+1)}, & i = (j+1)s; \\ w_{8(j+m)+7 \rightarrow 8(j+m)+1} \otimes e_{8j+7}, & i = j - s; \\ 0, & \text{otherwise.} \end{cases}$$

### Description of $d_1$

$d_1 : Q_2 \rightarrow Q_1$  - is an  $(9s \times 8s)$  matrix.

If  $0 \leq j < s$ , then

$$(d_1)_{ij} = \begin{cases} w_{8(j+m)+1 \rightarrow 8(j+m)+7} \otimes e_{8j}, & i = j; \\ -w_{8(j+m)+5 \rightarrow 8(j+m)+7} \otimes e_{8j}, & i = j + s; \\ (1 - 2f(j_1, 5, 6))w_{8(j+m)+j_1+1+2f(j_1,4) \rightarrow 8(j+m)+7} \otimes w_{8j \rightarrow 8j+j_1}, \\ \quad i = j + (j_1 + 1)s, \ 1 \leq j_1 \leq 6; \\ 0, & \text{otherwise.} \end{cases}$$

If  $s \leq j < 2s$ , then

$$(d_1)_{ij} = \begin{cases} w_{8(j+m+1)+1+j_1 \rightarrow 8(j+m+1)+2} \otimes w_{8j+1 \rightarrow 8(j+1)+j_1}, & i = 2j_1s + (j + 1)s, \ 0 \leq j_1 \leq 1; \\ w_{8(j+m)+1+j_1+2f(j_1,4) \rightarrow 8(j+m+1)+2} \otimes w_{8j+1 \rightarrow 8j+j_1}, & i = j + j_1s, \ 1 \leq j_1 \leq 4; \\ w_{8(j+m+1) \rightarrow 8(j+m+1)+2} \otimes w_{8j+1 \rightarrow 8j+7}, & i = j + 7s; \\ 0, & \text{otherwise.} \end{cases}$$

If  $2s \leq j < 3s$ , then

$$(d_1)_{ij} = \begin{cases} w_{8(j+m+1)+j_1 \rightarrow 8(j+m+1)+3} \otimes w_{8j+2 \rightarrow 8(j+1)+j_1-1}, \\ \quad i = (j_1 - f(j_1, 1))s + (j + 1)s, \ 1 \leq j_1 \leq 3; \\ w_{8(j+m)+2+j_1+2f(j_1,3) \rightarrow 8(j+m+1)+3} \otimes w_{8j+2 \rightarrow 8j+1+j_1}, & i = j + j_1s, \ 1 \leq j_1 \leq 3; \\ w_{8(j+m+1) \rightarrow 8(j+m+1)+3} \otimes w_{8j+2 \rightarrow 8j+7}, & i = j + 6s; \\ 0, & \text{otherwise.} \end{cases}$$

If  $3s \leq j < 4s$ , then

$$(d_1)_{ij} = \begin{cases} w_{8(j+m+1)+j_1 \rightarrow 8(j+m+1)+4} \otimes w_{8j+3 \rightarrow 8(j+1)+j_1-1}, \\ \quad i = (j_1 - f(j_1, 1))s + (j + 1)s, \ 1 \leq j_1 \leq 4; \\ w_{8(j+m)+4 \rightarrow 8(j+m+1)+4} \otimes e_{8j+3}, & i = j + s; \\ w_{8(j+m)+7 \rightarrow 8(j+m+1)+4} \otimes w_{8j+3 \rightarrow 8j+4}, & i = j + 2s; \\ w_{8(j+m+1) \rightarrow 8(j+m+1)+4} \otimes w_{8j+3 \rightarrow 8j+7}, & i = j + 5s; \\ 0, & \text{otherwise.} \end{cases}$$

If  $4s \leq j < 5s$ , then

$$(d_1)_{ij} = \begin{cases} e_{8(j+m+1)+5} \otimes w_{8j+4 \rightarrow 8(j+1)}, & i = s + (j + 1)s; \\ w_{8(j+m)+7 \rightarrow 8(j+m+1)+5} \otimes e_{8j+4}, & i = j + s; \\ w_{8(j+m+1) \rightarrow 8(j+m+1)+5} \otimes w_{8j+4 \rightarrow 8j+7}, & i = j + 4s; \\ 0, & \text{otherwise.} \end{cases}$$

If  $5s \leq j < 6s$ , then

$$(d_1)_{ij} = \begin{cases} w_{8(j+m+1)+5 \rightarrow 8(j+m+1)+6} \otimes w_{8j+5 \rightarrow 8(j+1)}, & i = s + (j + 1)s; \\ e_{8(j+m+1)+6} \otimes w_{8j+5 \rightarrow 8(j+1)+5}, & i = 6s + (j + 1)s; \\ w_{8(j+m)+5+j_1 \rightarrow 8(j+m+1)+6} \otimes w_{8j+5 \rightarrow 8j+4+j_1}, & i = j + j_1s, \ 1 \leq j_1 \leq 3; \\ 0, & \text{otherwise.} \end{cases}$$

If  $6s \leq j < 7s$ , then

$$(d_1)_{ij} = \begin{cases} e_{8(j+m+1)+1} \otimes w_{8j+6 \rightarrow 8(j+1)}, & i = (j+1)_s; \\ w_{8(j+m)+6+j_1 \rightarrow 8(j+m+1)+1} \otimes w_{8j+6 \rightarrow 8j+5+j_1}, & i = j + j_1 s, \ 1 \leq j_1 \leq 2; \\ 0, & \text{otherwise.} \end{cases}$$

If  $7s \leq j < 8s$ , then

$$(d_1)_{ij} = \begin{cases} w_{8(j+m+1)+j_1+2f(j_1,5,6) \rightarrow 8(j+m+2)} \otimes w_{8j+7 \rightarrow 8(j+1)+j_1-1+2f(j_1,6)}, \\ \quad i = (j_1 - f(j_1, 1) + 2f(j_1, 6))s + (j+1)_s, \ 1 \leq j_1 \leq 6; \\ w_{8(j+m+1) \rightarrow 8(j+m+2)} \otimes e_{8j+7}, & i = j + s; \\ 0, & \text{otherwise.} \end{cases}$$

### Description of $d_2$

$d_2 : Q_3 \rightarrow Q_2$  - is an  $(8s \times 10s)$  matrix.

If  $0 \leq j < s$ , then

$$(d_2)_{ij} = \begin{cases} (-1)^{j_1} w_{8(j+m-1)+7+3j_1 \rightarrow 8(j+m)+2} \otimes w_{8j \rightarrow 8j+j_1}, & i = j + j_1 s, \ 0 \leq j_1 \leq 1; \\ w_{8(j+m)+1 \rightarrow 8(j+m)+2} \otimes w_{8j \rightarrow 8j+6}, & i = j + 6s; \\ 0, & \text{otherwise.} \end{cases}$$

If  $s \leq j < 2s$ , then

$$(d_2)_{ij} = \begin{cases} w_{8(j+m-1)+7 \rightarrow 8(j+m)+6} \otimes e_{8j}, & i = j_s; \\ (-1)^{j_1} w_{8(j+m)+2+j_1 \rightarrow 8(j+m)+6} \otimes w_{8j \rightarrow 8j+j_1+1}, & i = j + j_1 s, \ 3 \leq j_1 \leq 4; \\ 0, & \text{otherwise.} \end{cases}$$

If  $2s \leq j < 4s$ , then

$$(d_2)_{ij} = \begin{cases} w_{8(j+m)+j_2 \rightarrow 8(j+m)+j_2+1} \otimes e_{8j+j_2-1}, & i = j - s; \\ -e_{8(j+m)+j_2+1} \otimes w_{8j+j_2-1 \rightarrow 8j+j_2}, & i = j; \\ 0, & \text{otherwise.} \end{cases}$$

If  $4s \leq j < 5s$ , then

$$(d_2)_{ij} = \begin{cases} -e_{8(j+m)+7} \otimes w_{8j+3 \rightarrow 8(j+1)}, & i = (j+1)_s; \\ (-1)^{j_1} w_{8(j+m)+4+j_1 \rightarrow 8(j+m)+7} \otimes w_{8j+3 \rightarrow 8j+3+j_1}, & i = j + (j_1 - 1)s, \ 0 \leq j_1 \leq 1; \\ 0, & \text{otherwise.} \end{cases}$$

If  $5s \leq j < 6s$ , then

$$(d_2)_{ij} = \begin{cases} w_{8(j+m)+7 \rightarrow 8(j+m+1)} \otimes w_{8j+4 \rightarrow 8(j+1)}, & i = (j+1)_s; \\ (-1)^{j_1} w_{8(j+m)+5+3j_1 \rightarrow 8(j+m+1)} \otimes w_{8j+4 \rightarrow 8j+4+3j_1}, \\ \quad i = j + (3j_1 - 1)s, \ 0 \leq j_1 \leq 1; \\ 0, & \text{otherwise.} \end{cases}$$

If  $6s \leq j < 7s$ , then

$$(d_2)_{ij} = \begin{cases} e_{8(j+m)+7} \otimes w_{8j+5 \rightarrow 8(j+1)}, & i = (j+1)_s; \\ (-1)^{j_1} w_{8(j+m)+6-5j_1 \rightarrow 8(j+m)+7} \otimes w_{8j+5 \rightarrow 8j+5+j_1}, & i = j + (j_1 - 1)s, \ 0 \leq j_1 \leq 1; \\ 0, & \text{otherwise.} \end{cases}$$

If  $7s \leq j < 8s$ , then

$$(d_2)_{ij} = \begin{cases} (-1)^{j_1} w_{8(j+m)+1+7j_1 \rightarrow 8(j+m+1)} \otimes w_{8j+6 \rightarrow 8j+6+j_1}, & i = j + (j_1 - 1)s, \ 0 \leq j_1 \leq 1; \\ 0, & \text{otherwise.} \end{cases}$$

If  $8s \leq j < 9s$ , then

$$(d_2)_{ij} = \begin{cases} -w_{8(j+m)+7 \rightarrow 8(j+m+1)+1} \otimes w_{8j+7 \rightarrow 8(j+1)}, & i = (j+1)s; \\ -e_{8(j+m+1)+1} \otimes w_{8j+7 \rightarrow 8(j+1)+6}, & i = 6s + (j+1)s; \\ w_{8(j+m+1) \rightarrow 8(j+m+1)+1} \otimes e_{8j+7}, & i = j - s; \\ 0, & \text{otherwise.} \end{cases}$$

If  $9s \leq j < 10s$ , then

$$(d_2)_{ij} = \begin{cases} -e_{8(j+m+1)+5} \otimes w_{8j+7 \rightarrow 8(j+1)+4}, & i = 4s + (j+1)s; \\ w_{8(j+m+1) \rightarrow 8(j+m+1)+5} \otimes e_{8j+7}, & i = j - 2s; \\ 0, & \text{otherwise.} \end{cases}$$

### Description of $d_3$

$d_3 : Q_4 \rightarrow Q_3$  - is an  $(10s \times 11s)$  matrix.

If  $0 \leq j < s$ , then

$$(d_3)_{ij} = \begin{cases} (-1)^{j_1} w_{8(j+m)+2+4j_1 \rightarrow 8(j+m)+7} \otimes e_{8j}, & i = j + j_1s, \ 0 \leq j_1 \leq 1; \\ w_{8(j+m)+2+j_1+2f(j_1,3) \rightarrow 8(j+m)+7} \otimes w_{8j \rightarrow 8j+j_1}, & i = j + (j_1 + 1)s, \ 1 \leq j_1 \leq 3; \\ e_{8(j+m)+7} \otimes w_{8j \rightarrow 8j+5}, & i = j + 6s; \\ 0, & \text{otherwise.} \end{cases}$$

If  $s \leq j < 2s$ , then

$$(d_3)_{ij} = \begin{cases} w_{8(j+m)+6+2j_1 \rightarrow 8(j+m+1)} \otimes w_{8j \rightarrow 8j+4j_1}, & i = j + 4j_1s, \ 0 \leq j_1 \leq 1; \\ -w_{8(j+m)+2+j_1 \rightarrow 8(j+m+1)} \otimes w_{8j \rightarrow 8j+j_1}, & i = j + j_1s, \ 5 \leq j_1 \leq 6; \\ 0, & \text{otherwise.} \end{cases}$$

If  $2s \leq j < 3s$ , then

$$(d_3)_{ij} = \begin{cases} w_{8(j+m+1)+2+j_1 \rightarrow 8(j+m+1)+3} \otimes w_{8j+1 \rightarrow 8(j+1)+j_1}, & i = 2j_1s + (j+1)s, \ 0 \leq j_1 \leq 1; \\ w_{8(j+m)+3+j_1+2f(j_1,2) \rightarrow 8(j+m+1)+3} \otimes w_{8j+1 \rightarrow 8j+1+j_1}, & i = j + j_1s, \ 0 \leq j_1 \leq 2; \\ 0, & \text{otherwise.} \end{cases}$$

If  $3s \leq j < 4s$ , then

$$(d_3)_{ij} = \begin{cases} w_{8(j+m+1)+2+j_1 \rightarrow 8(j+m+1)+4} \otimes w_{8j+2 \rightarrow 8(j+1)+j_1}, & \\ i = (1 + j_1 - f(j_1, 0))s + (j+1)s, \ 0 \leq j_1 \leq 2; \\ w_{8(j+m)+4+3j_1 \rightarrow 8(j+m+1)+4} \otimes w_{8j+2 \rightarrow 8j+2+j_1}, & i = j + j_1s, \ 0 \leq j_1 \leq 1; \\ 0, & \text{otherwise.} \end{cases}$$

If  $4s \leq j < 5s$ , then

$$(d_3)_{ij} = \begin{cases} w_{8(j+m)+7+j_1 \rightarrow 8(j+m+1)+5} \otimes w_{8j+3 \rightarrow 8j+3+j_1}, & i = j + j_1s, \ 0 \leq j_1 \leq 1; \\ e_{8(j+m+1)+5} \otimes w_{8j+3 \rightarrow 8j+7}, & i = j + 5s; \\ 0, & \text{otherwise.} \end{cases}$$

If  $5s \leq j < 6s$ , then

$$(d_3)_{ij} = \begin{cases} -e_{8(j+m+1)+6} \otimes w_{8j+4 \rightarrow 8(j+1)}, & i = s + (j+1)s; \\ w_{8(j+m+1)+5j_1 \rightarrow 8(j+m+1)+6} \otimes w_{8j+4 \rightarrow 8j+4+3j_1}, & i = j + 4j_1s, \ 0 \leq j_1 \leq 1; \\ 0, & \text{otherwise.} \end{cases}$$

If  $6s \leq j < 7s$ , then

$$(d_3)_{ij} = \begin{cases} w_{8(j+m+1)+j_1 \rightarrow 8(j+m+1)+1} \otimes w_{8j+4 \rightarrow 8j+4+3j_1}, & i = j + (3j_1 - 1)s, \ 0 \leq j_1 \leq 1; \\ 0, & \text{otherwise.} \end{cases}$$

If  $7s \leq j < 8s$ , then

$$(d_3)_{ij} = \begin{cases} w_{8(j+m)+7+j_1 \rightarrow 8(j+m+1)+1} \otimes w_{8j+5 \rightarrow 8j+5+j_1}, & i = j + (j_1 - 1)s, \ 0 \leq j_1 \leq 2; \\ 0, & \text{otherwise.} \end{cases}$$

If  $8s \leq j < 9s$ , then

$$(d_3)_{ij} = \begin{cases} e_{8(j+m+1)+2} \otimes w_{8j+6 \rightarrow 8(j+1)}, & i = (j+1)s; \\ w_{8(j+m+1)+j_1 \rightarrow 8(j+m+1)+2} \otimes w_{8j+6 \rightarrow 8j+6+j_1}, & i = j + (j_1 - 1)s, \ 0 \leq j_1 \leq 1; \\ 0, & \text{otherwise.} \end{cases}$$

If  $9s \leq j < 10s$ , then

$$(d_3)_{ij} = \begin{cases} w_{8(j+m+1)+5j_1 \rightarrow 8(j+m+1)+5} \otimes w_{8j+6 \rightarrow 8j+6+j_1}, & i = j + (2j_1 - 2)s, \ 0 \leq j_1 \leq 1; \\ 0, & \text{otherwise.} \end{cases}$$

If  $10s \leq j < 11s$ , then

$$(d_3)_{ij} = \begin{cases} w_{8(j+m+1)+1+j_1+2f(j_1,4) \rightarrow 8(j+m+1)+7} \otimes w_{8j+7 \rightarrow 8(j+1)+j_1-1}, & i = (j_1 - f(j_1, 1))s + (j+1)s, \ 1 \leq j_1 \leq 4; \\ (-1)^{j_1} w_{8(j+m+1)+1+4j_1 \rightarrow 8(j+m+1)+7} \otimes e_{8j+7}, & i = j + (j_1 - 2)s, \ 0 \leq j_1 \leq 1; \\ 0, & \text{otherwise.} \end{cases}$$

#### Description of $d_4$

$d_4 : Q_5 \rightarrow Q_4$  - is an  $(11s \times 11s)$  matrix.

If  $0 \leq j < s$ , then

$$(d_4)_{ij} = \begin{cases} w_{8(j+m-1)+7+j_1 \rightarrow 8(j+m)+5} \otimes e_{8j}, & i = j + j_1s, \ 0 \leq j_1 \leq 1; \\ -e_{8(j+m)+5} \otimes w_{8j \rightarrow 8j+3}, & i = j + 4s; \\ e_{8(j+m)+5} \otimes w_{8j \rightarrow 8j+6}, & i = j + 9s; \\ 0, & \text{otherwise.} \end{cases}$$

If  $s \leq j < 2s$ , then

$$(d_4)_{ij} = \begin{cases} w_{8(j+m-1)+7 \rightarrow 8(j+m)+3} \otimes e_{8j}, & i = j_s; \\ -e_{8(j+m)+3} \otimes w_{8j \rightarrow 8j+1}, & i = j + s; \\ (-1)^{j_1} w_{8(j+m)+j_1 \rightarrow 8(j+m)+3} \otimes w_{8j \rightarrow 8j+4+j_1}, & i = j + (5 + j_1)s, \ 1 \leq j_1 \leq 2; \\ 0, & \text{otherwise.} \end{cases}$$

If  $2s \leq j < 3s$ , then

$$(d_4)_{ij} = \begin{cases} w_{8(j+m) \rightarrow 8(j+m)+1} \otimes e_{8j}, & i = j - s; \\ (-1)^{j_1+1} e_{8(j+m)+1} \otimes w_{8j \rightarrow 8j+j_1}, & i = j + j_1 s, \ 4 \leq j_1 \leq 5; \\ 0, & \text{otherwise.} \end{cases}$$

If  $3s \leq j < 4s$ , then

$$(d_4)_{ij} = \begin{cases} (-1)^{j_1} w_{8(j+m)+3+j_1 \rightarrow 8(j+m)+4} \otimes w_{8j+1 \rightarrow 8j+1+j_1}, & i = j + (j_1 - 1)s, \ 0 \leq j_1 \leq 1; \\ 0, & \text{otherwise.} \end{cases}$$

If  $4s \leq j < 5s$ , then

$$(d_4)_{ij} = \begin{cases} -e_{8(j+m)+7} \otimes w_{8j+2 \rightarrow 8(j+1)}, & i = (j+1)_s; \\ (-1)^{j_1} w_{8(j+m)+4+j_1 \rightarrow 8(j+m)+7} \otimes w_{8j+2 \rightarrow 8j+2+j_1}, & i = j + (j_1 - 1)s, \ 0 \leq j_1 \leq 2; \\ 0, & \text{otherwise.} \end{cases}$$

If  $5s \leq j < 6s$ , then

$$(d_4)_{ij} = \begin{cases} -e_{8(j+m)+1} \otimes w_{8j+3 \rightarrow 8(j+1)}, & i = s + (j+1)_s; \\ (-1)^{j_1} w_{8(j+m)+5+j_1 \rightarrow 8(j+m)+1} \otimes w_{8j+3 \rightarrow 8j+3+j_1}, & i = j + (j_1 - 1)s, \ 0 \leq j_1 \leq 1; \\ 0, & \text{otherwise.} \end{cases}$$

If  $6s \leq j < 7s$ , then

$$(d_4)_{ij} = \begin{cases} -e_{8(j+m)+7} \otimes w_{8j+4 \rightarrow 8(j+1)}, & i = (j+1)_s; \\ w_{8(j+m)+6 \rightarrow 8(j+m)+7} \otimes e_{8j+4}, & i = j - s; \\ -w_{8(j+m)+1 \rightarrow 8(j+m)+7} \otimes e_{8j+4}, & i = j; \\ e_{8(j+m)+7} \otimes w_{8j+4 \rightarrow 8j+7}, & i = j + 4s; \\ 0, & \text{otherwise.} \end{cases}$$

If  $7s \leq j < 8s$ , then

$$(d_4)_{ij} = \begin{cases} w_{8(j+m)+7+j_1 \rightarrow 8(j+m)+1} \otimes w_{8j+5 \rightarrow 8(j+1)}, & i = j_1 s + (j+1)_s, \ 0 \leq j_1 \leq 1; \\ (-1)^{j_1} w_{8(j+m)+1+j_1 \rightarrow 8(j+m)+1} \otimes w_{8j+5 \rightarrow 8j+5+j_1}, & i = j + j_1 s, \ 0 \leq j_1 \leq 1; \\ 0, & \text{otherwise.} \end{cases}$$

If  $8s \leq j < 9s$ , then

$$(d_4)_{ij} = \begin{cases} w_{8(j+m)+2 \rightarrow 8(j+m)+7} \otimes e_{8j+6}, & i = j; \\ -w_{8(j+m)+5+2j_1 \rightarrow 8(j+m)+7} \otimes w_{8j+6 \rightarrow 8j+6+j_1}, & i = j + (j_1 + 1)s, \ 0 \leq j_1 \leq 1; \\ 0, & \text{otherwise.} \end{cases}$$

If  $9s \leq j < 10s$ , then

$$(d_4)_{ij} = \begin{cases} -w_{8(j+m)+7+j_1 \rightarrow 8(j+m)+2} \otimes w_{8j+7 \rightarrow 8(j+1)}, & i = j_1 s + (j+1)_s, \ 0 \leq j_1 \leq 1; \\ w_{8(j+m)+1 \rightarrow 8(j+m)+2} \otimes w_{8j+7 \rightarrow 8(j+1)+4}, & i = 6s + (j+1)_s; \\ -e_{8(j+m)+2} \otimes w_{8j+7 \rightarrow 8(j+1)+6}, & i = 8s + (j+1)_s; \\ w_{8(j+m)+7 \rightarrow 8(j+m)+2} \otimes e_{8j+7}, & i = j + s; \\ 0, & \text{otherwise.} \end{cases}$$

If  $10s \leq j < 11s$ , then

$$(d_4)_{ij} = \begin{cases} (-1)^{j_1+1} w_{8(j+m+1)+5+j_1 \rightarrow 8(j+m+1)+6} \otimes w_{8j+7 \rightarrow 8(j+1)+3+j_1}, \\ \quad i = (4+j_1)s + (j+1)_s, \quad 0 \leq j_1 \leq 1; \\ w_{8(j+m)+7 \rightarrow 8(j+m+1)+6} \otimes e_{8j+7}, \quad i = j; \\ 0, \quad \text{otherwise.} \end{cases}$$

**Description of  $d_5$**

$d_5 : Q_6 \rightarrow Q_5$  – is an  $(11s \times 13s)$  matrix.

If  $0 \leq j < s$ , then

$$(d_5)_{ij} = \begin{cases} w_{8(j+m)+5 \rightarrow 8(j+m)+7} \otimes e_{8j}, \quad i = j; \\ -w_{8(j+m)+3 \rightarrow 8(j+m)+7} \otimes e_{8j}, \quad i = j + s; \\ -w_{8(j+m)+1 \rightarrow 8(j+m)+7} \otimes e_{8j}, \quad i = j + 2s; \\ -w_{8(j+m)+4 \rightarrow 8(j+m)+7} \otimes w_{8j \rightarrow 8j+1}, \quad i = j + 3s; \\ (1 - 2f(j_1, 0))e_{8(j+m)+7} \otimes w_{8j \rightarrow 8j+2(j_1+1)}, \quad i = j + 2(2+j_1)s, \quad 0 \leq j_1 \leq 2; \\ 0, \quad \text{otherwise.} \end{cases}$$

If  $s \leq j < 2s$ , then

$$(d_5)_{ij} = \begin{cases} w_{8(j+m)+3+j_1+2f(j_1,2,3) \rightarrow 8(j+m+1)} \otimes w_{8j \rightarrow 8j+j_1}, \\ \quad i = j + (1+j_1 - f(j_1, 0))s, \quad 0 \leq j_1 \leq 3; \\ e_{8(j+m+1)} \otimes w_{8j \rightarrow 8j+5}, \quad i = j + 6s; \\ 0, \quad \text{otherwise.} \end{cases}$$

If  $2s \leq j < 3s$ , then

$$(d_5)_{ij} = \begin{cases} w_{8(j+m+1)+3+j_1 \rightarrow 8(j+m+1)+4} \otimes w_{8j+1 \rightarrow 8(j+1)+j_1}, \\ \quad i = (2j_1+1)s + (j+1)_s, \quad 0 \leq j_1 \leq 1; \\ w_{8(j+m)+1+3j_1 \rightarrow 8(j+m+1)+4} \otimes w_{8j+1 \rightarrow 8j+j_1}, \quad i = j + j_1s, \quad 1 \leq j_1 \leq 2; \\ 0, \quad \text{otherwise.} \end{cases}$$

If  $3s \leq j < 4s$ , then

$$(d_5)_{ij} = \begin{cases} e_{8(j+m+1)+5} \otimes w_{8j+2 \rightarrow 8(j+1)}, \quad i = (j+1)_s; \\ w_{8(j+m)+6+j_1 \rightarrow 8(j+m+1)+5} \otimes w_{8j+2 \rightarrow 8j+1+j_1}, \quad i = j + j_1s, \quad 1 \leq j_1 \leq 2; \\ 0, \quad \text{otherwise.} \end{cases}$$

If  $4s \leq j < 5s$ , then

$$(d_5)_{ij} = \begin{cases} w_{8(j+m+1)+5 \rightarrow 8(j+m+1)+6} \otimes w_{8j+3 \rightarrow 8(j+1)}, \quad i = (j+1)_s; \\ w_{8(j+m+1)-j_1 \rightarrow 8(j+m+1)+6} \otimes w_{8j+3 \rightarrow 8j+3+j_1}, \quad i = j + (j_1+1)s, \quad 0 \leq j_1 \leq 1; \\ -e_{8(j+m+1)+6} \otimes w_{8j+3 \rightarrow 8j+7}, \quad i = j + 6s; \\ 0, \quad \text{otherwise.} \end{cases}$$

If  $5s \leq j < 6s$ , then

$$(d_5)_{ij} = \begin{cases} e_{8(j+m+1)+1} \otimes w_{8j+3 \rightarrow 8(j+1)}, \quad i = 2s + (j+1)_s; \\ w_{8(j+m+1) \rightarrow 8(j+m+1)+1} \otimes e_{8j+3}, \quad i = j; \\ 0, \quad \text{otherwise.} \end{cases}$$

If  $6s \leq j < 7s$ , then

$$(d_5)_{ij} = \begin{cases} -w_{8(j+m+1)+1 \rightarrow 8(j+m+1)+2} \otimes w_{8j+4 \rightarrow 8(j+1)}, & i = 2s + (j+1)_s; \\ (-1)^{j_1} w_{8(j+m)+7+3j_1 \rightarrow 8(j+m+1)+2} \otimes w_{8j+4 \rightarrow 8j+4+3j_1}, & i = j + 3j_1s, \ 0 \leq j_1 \leq 1; \\ 0, & \text{otherwise.} \end{cases}$$

If  $7s \leq j < 8s$ , then

$$(d_5)_{ij} = \begin{cases} w_{8(j+m+1)-j_1+4f(j_1,2) \rightarrow 8(j+m+1)+2} \otimes w_{8j+5 \rightarrow 8j+5+j_1}, & i = j + j_1s, \ 0 \leq j_1 \leq 2; \\ 0, & \text{otherwise.} \end{cases}$$

If  $8s \leq j < 9s$ , then

$$(d_5)_{ij} = \begin{cases} -e_{8(j+m+1)+5} \otimes w_{8j+5 \rightarrow 8(j+1)}, & i = (j+1)_s; \\ w_{8(j+m+1) \rightarrow 8(j+m+1)+5} \otimes e_{8j+5}, & i = j - s; \\ 0, & \text{otherwise.} \end{cases}$$

If  $9s \leq j < 10s$ , then

$$(d_5)_{ij} = \begin{cases} w_{8(j+m+1)+3-2j_1 \rightarrow 8(j+m+1)+3} \otimes w_{8j+6 \rightarrow 8(j+1)}, & i = (j_1+1)s + (j+1)_s, \ 0 \leq j_1 \leq 1; \\ w_{8(j+m)+7+3j_1 \rightarrow 8(j+m+1)+3} \otimes w_{8j+6 \rightarrow 8j+6+j_1}, & i = j + (j_1-1)s, \ 0 \leq j_1 \leq 1; \\ 0, & \text{otherwise.} \end{cases}$$

If  $10s \leq j < 11s$ , then

$$(d_5)_{ij} = \begin{cases} w_{8(j+m)+7(j_1+1) \rightarrow 8(j+m+1)+6} \otimes w_{8j+6 \rightarrow 8j+6+j_1}, & i = j + 2(j_1-1)s, \ 0 \leq j_1 \leq 1; \\ 0, & \text{otherwise.} \end{cases}$$

If  $11s \leq j < 12s$ , then

$$(d_5)_{ij} = \begin{cases} w_{8(j+m+1)+3 \rightarrow 8(j+m+1)+7} \otimes w_{8j+7 \rightarrow 8(j+1)}, & i = s + (j+1)_s; \\ w_{8(j+m+1)+1+3j_1 \rightarrow 8(j+m+1)+7} \otimes w_{8j+7 \rightarrow 8(j+1)+j_1}, & i = (j_1+2)s + (j+1)_s, \ 0 \leq j_1 \leq 2; \\ (-1)^{j_1} w_{8(j+m+1)+2+4j_1 \rightarrow 8(j+m+1)+7} \otimes e_{8j+7}, & i = j + (j_1-2)s, \ 0 \leq j_1 \leq 1; \\ 0, & \text{otherwise.} \end{cases}$$

If  $12s \leq j < 13s$ , then

$$(d_5)_{ij} = \begin{cases} e_{8(j+m+2)} \otimes w_{8j+7 \rightarrow 8(j+1)+3}, & i = 5s + (j+1)_s; \\ w_{8(j+m+1)+6 \rightarrow 8(j+m+2)} \otimes e_{8j+7}, & i = j - 2s; \\ 0, & \text{otherwise.} \end{cases}$$

### Description of $d_6$

$d_6 : Q_7 \rightarrow Q_6$  - is an  $(13s \times 14s)$  matrix.

If  $0 \leq j < s$ , then

$$(d_6)_{ij} = \begin{cases} w_{8(j+m-1)+7+j_1 \rightarrow 8(j+m)+2} \otimes e_{8j}, & i = j + j_1s, \ 0 \leq j_1 \leq 1; \\ -w_{8(j+m)+2-f(j_1,0) \rightarrow 8(j+m)+2} \otimes w_{8j \rightarrow 8j+3+j_1}, & i = j + (5+j_1)s, \ 0 \leq j_1 \leq 2; \\ 0, & \text{otherwise.} \end{cases}$$



If  $s \leq j < 2s$ , then

$$(d_6)_{ij} = \begin{cases} (-1)^{j_1} w_{8(j+m)+4j_1 \rightarrow 8(j+m)+4} \otimes w_{8j \rightarrow 8j+j_1}, & i = j + j_1 s, \ 0 \leq j_1 \leq 1; \\ (-1 + 2f(j_1, 2)) w_{8(j+m)+1+j_1 \rightarrow 8(j+m)+4} \otimes w_{8j \rightarrow 8j+j_1+4-f(j_1, 0)}, \\ \quad i = j + 2(2 + j_1)s, \ 0 \leq j_1 \leq 2; \\ 0, & \text{otherwise.} \end{cases}$$

If  $2s \leq j < 3s$ , then

$$(d_6)_{ij} = \begin{cases} w_{8(j+m-1)+7 \rightarrow 8(j+m)+6} \otimes e_{8j}, & i = j_s; \\ (-1)^{j_1} w_{8(j+m)+5+j_1 \rightarrow 8(j+m)+6} \otimes w_{8j \rightarrow 8j+2+j_1}, & i = j + (1 + j_1)s, \ 0 \leq j_1 \leq 1; \\ -e_{8(j+m)+6} \otimes w_{8j \rightarrow 8j+6}, & i = j + 8s; \\ 0, & \text{otherwise.} \end{cases}$$

If  $3s \leq j < 4s$ , then

$$(d_6)_{ij} = \begin{cases} (-1)^{j_1} w_{8(j+m)+5j_1 \rightarrow 8(j+m)+5} \otimes w_{8j \rightarrow 8j+2j_1}, & i = j + 2(j_1 - 1)s, \ 0 \leq j_1 \leq 1; \\ -e_{8(j+m)+5} \otimes w_{8j \rightarrow 8j+5}, & i = j + 5s; \\ 0, & \text{otherwise.} \end{cases}$$

If  $4s \leq j < 5s$ , then

$$(d_6)_{ij} = \begin{cases} e_{8(j+m)+7} \otimes w_{8j+1 \rightarrow 8(j+1)}, & i = (j + 1)_s; \\ (-1)^{j_1} w_{8(j+m)+4+j_1-5f(j_1, 2) \rightarrow 8(j+m)+7} \otimes w_{8j+1 \rightarrow 8j+1+j_1}, \\ \quad i = j + (j_1 - 2 + f(j_1, 2))s, \ 0 \leq j_1 \leq 2; \\ 0, & \text{otherwise.} \end{cases}$$

If  $5s \leq j < 6s$ , then

$$(d_6)_{ij} = \begin{cases} -w_{8(j+m)+7+j_1 \rightarrow 8(j+m)+1} \otimes w_{8j+2 \rightarrow 8(j+1)}, & i = j_1 s + (j + 1)_s, \ 0 \leq j_1 \leq 1; \\ (-1)^{j_1} w_{8(j+m)+5-4j_1 \rightarrow 8(j+m)+1} \otimes w_{8j+2 \rightarrow 8j+2+j_1}, & i = j + 2(j_1 - 1)s, \ 0 \leq j_1 \leq 1; \\ 0, & \text{otherwise.} \end{cases}$$

If  $6s \leq j < 7s$ , then

$$(d_6)_{ij} = \begin{cases} -e_{8(j+m)+7} \otimes w_{8j+3 \rightarrow 8(j+1)}, & i = (j + 1)_s; \\ w_{8(j+m)+6 \rightarrow 8(j+m)+7} \otimes e_{8j+3}, & i = j - 2s; \\ -w_{8(j+m)+1+j_1 \rightarrow 8(j+m)+7} \otimes w_{8j+3 \rightarrow 8j+3+j_1}, & i = j + (j_1 - 1)s, \ 0 \leq j_1 \leq 1; \\ -e_{8(j+m)+7} \otimes w_{8j+3 \rightarrow 8j+7}, & i = j + 5s; \\ 0, & \text{otherwise.} \end{cases}$$

If  $7s \leq j < 8s$ , then

$$(d_6)_{ij} = \begin{cases} -e_{8(j+m)+1} \otimes w_{8j+4 \rightarrow 8(j+1)}, & i = s + (j + 1)_s; \\ w_{8(j+m)+2 \rightarrow 8(j+m)+1} \otimes e_{8j+4}, & i = j - s; \\ w_{8(j+m)+7+j_1 \rightarrow 8(j+m)+1} \otimes w_{8j+4 \rightarrow 8j+7}, & i = j + (4 + j_1)s, \ 0 \leq j_1 \leq 1; \\ 0, & \text{otherwise.} \end{cases}$$

If  $8s \leq j < 9s$ , then

$$(d_6)_{ij} = \begin{cases} -e_{8(j+m)+7} \otimes w_{8j+5 \rightarrow 8(j+1)}, & i = (j+1)_s; \\ (-1)^{j_1} w_{8(j+m)+2+3j_1 \rightarrow 8(j+m)+7} \otimes e_{8j+5}, & i = j + (j_1 - 1)s, \ 0 \leq j_1 \leq 1; \\ -w_{8(j+m)+3 \rightarrow 8(j+m)+7} \otimes w_{8j+5 \rightarrow 8j+6}, & i = j + s; \\ 0, & \text{otherwise.} \end{cases}$$

If  $9s \leq j < 10s$ , then

$$(d_6)_{ij} = \begin{cases} w_{8(j+m)+3 \rightarrow 8(j+m)+7} \otimes e_{8j+6}, & i = j; \\ -w_{8(j+m)+6+j_1 \rightarrow 8(j+m)+7} \otimes w_{8j+6 \rightarrow 8j+6+j_1}, & i = j + (j_1 + 1)s, \ 0 \leq j_1 \leq 1; \\ 0, & \text{otherwise.} \end{cases}$$

If  $10s \leq j < 11s$ , then

$$(d_6)_{ij} = \begin{cases} (-1)^{j_1} w_{8(j+m)+6+2j_1 \rightarrow 8(j+m)+7} \otimes w_{8j+6 \rightarrow 8j+6+j_1}, & i = j + 2j_1s, \ 0 \leq j_1 \leq 1; \\ 0, & \text{otherwise.} \end{cases}$$

If  $11s \leq j < 12s$ , then

$$(d_6)_{ij} = \begin{cases} -e_{8(j+m)+5} \otimes w_{8j+7 \rightarrow 8(j+1)+2}, & i = 3s + (j+1)_s; \\ w_{8(j+m)+7+j_1 \rightarrow 8(j+m)+5} \otimes e_{8j+7}, & i = j + j_1s, \ 0 \leq j_1 \leq 1; \\ 0, & \text{otherwise.} \end{cases}$$

If  $12s \leq j < 13s$ , then

$$(d_6)_{ij} = \begin{cases} w_{8(j+m)+7 \rightarrow 8(j+m)+3} \otimes w_{8j+7 \rightarrow 8(j+1)}, & i = (j+1)_s; \\ -w_{8(j+m)+j_1 \rightarrow 8(j+m)+3} \otimes w_{8j+7 \rightarrow 8(j+1)+2j_1}, & i = 3j_1s + (j+1)_s, \ 2 \leq j_1 \leq 3; \\ w_{8(j+m)+7 \rightarrow 8(j+m)+3} \otimes e_{8j+7}, & i = j - s; \\ 0, & \text{otherwise.} \end{cases}$$

If  $13s \leq j < 14s$ , then

$$(d_6)_{ij} = \begin{cases} -e_{8(j+m)+1} \otimes w_{8j+7 \rightarrow 8(j+1)+3}, & i = 5s + (j+1)_s; \\ w_{8(j+m)+1 \rightarrow 8(j+m)+1} \otimes e_{8j+7}, & i = j - s; \\ 0, & \text{otherwise.} \end{cases}$$

### Description of $d_7$

$d_7 : Q_8 \rightarrow Q_7$  – is an  $(14s \times 16s)$  matrix.

If  $0 \leq j < s$ , then

$$(d_7)_{ij} = \begin{cases} (-1 + 2f(j_1, 0)) w_{8(j+m)+7-j_1-5f(j_1, 0) \rightarrow 8(j+m)+7} \otimes e_{8j}, & i = j + (1 + j_1 - f(j_1, 0))s, \ 0 \leq j_1 \leq 2; \\ (1 - 2f(j_1, 0)) e_{8(j+m)+7} \otimes w_{8j \rightarrow 8j+4+j_1-f(j_1, 0)}, & i = j + (7 + j_1 - f(j_1, 0))s, \ 0 \leq j_1 \leq 2; \\ 0, & \text{otherwise.} \end{cases}$$

If  $s \leq j < 2s$ , then

$$(d_7)_{ij} = \begin{cases} (-1)^{j_1} w_{8(j+m)+4+j_1 \rightarrow 8(j+m)+7} \otimes e_{8j}, & i = j + 2j_1s, \ 0 \leq j_1 \leq 1; \\ e_{8(j+m)+7} \otimes w_{8j \rightarrow 8j+1+4j_1}, & i = j + (3 + 4j_1)s, \ 0 \leq j_1 \leq 1; \\ 0, & \text{otherwise.} \end{cases}$$

If  $2s \leq j < 3s$ , then

$$(d_7)_{ij} = \begin{cases} w_{8(j+m)+6 \rightarrow 8(j+m+1)} \otimes e_{8j}, & i = j; \\ (1 - 2f(j_1, 0))w_{8(j+m+1)-f(j_1, 1) \rightarrow 8(j+m+1)} \otimes w_{8j \rightarrow 8j+2+j_1}, \\ \quad i = j + (3 + j_1)s, \quad 0 \leq j_1 \leq 2; \\ e_{8(j+m+1)} \otimes w_{8j \rightarrow 8j+6}, & i = j + 8s; \\ 0, & \text{otherwise.} \end{cases}$$

If  $3s \leq j < 4s$ , then

$$(d_7)_{ij} = \begin{cases} e_{8(j+m+1)+5} \otimes w_{8j+1 \rightarrow 8(j+1)}, & i = 3s + (j+1)s; \\ w_{8(j+m)+6+j_1 \rightarrow 8(j+m+1)+5} \otimes w_{8j+1 \rightarrow 8j+j_1}, & i = j + j_1s, \quad 1 \leq j_1 \leq 2; \\ 0, & \text{otherwise.} \end{cases}$$

If  $4s \leq j < 5s$ , then

$$(d_7)_{ij} = \begin{cases} w_{8(j+m+1)+6-j_1 \rightarrow 8(j+m+1)+6} \otimes w_{8j+2 \rightarrow 8(j+1)}, & i = (2 + j_1)s + (j+1)s, \quad 0 \leq j_1 \leq 1; \\ w_{8(j+m+1) \rightarrow 8(j+m+1)+6} \otimes e_{8j+2}, & i = j + s; \\ 0, & \text{otherwise.} \end{cases}$$

If  $5s \leq j < 6s$ , then

$$(d_7)_{ij} = \begin{cases} (-1 + 2f(j_1, 0))w_{8(j+m+1)-f(j_1, 1) \rightarrow 8(j+m+1)+1} \otimes w_{8j+2 \rightarrow 8j+2+j_1}, \\ \quad i = j + j_1s, \quad 0 \leq j_1 \leq 2; \\ e_{8(j+m+1)+1} \otimes w_{8j+2 \rightarrow 8j+7}, & i = j + 8s; \\ 0, & \text{otherwise.} \end{cases}$$

If  $6s \leq j < 7s$ , then

$$(d_7)_{ij} = \begin{cases} e_{8(j+m+1)+2} \otimes w_{8j+3 \rightarrow 8(j+1)}, & i = (j+1)s; \\ w_{8(j+m)+7+j_1 \rightarrow 8(j+m+1)+2} \otimes w_{8j+3 \rightarrow 8j+3+j_1}, & i = j + j_1s, \quad 0 \leq j_1 \leq 1; \\ -w_{8(j+m+1)+1 \rightarrow 8(j+m+1)+2} \otimes w_{8j+3 \rightarrow 8j+7}, & i = j + 7s; \\ 0, & \text{otherwise.} \end{cases}$$

If  $7s \leq j < 8s$ , then

$$(d_7)_{ij} = \begin{cases} w_{8(j+m+1)+2 \rightarrow 8(j+m+1)+3} \otimes w_{8j+4 \rightarrow 8(j+1)}, & i = (j+1)s; \\ w_{8(j+m+1) \rightarrow 8(j+m+1)+3} \otimes e_{8j+4}, & i = j; \\ -w_{8(j+m+1)+3-2j_1 \rightarrow 8(j+m+1)+3} \otimes w_{8j+4 \rightarrow 8j+7}, & i = j + (5 + j_1)s, \quad 0 \leq j_1 \leq 1; \\ 0, & \text{otherwise.} \end{cases}$$

If  $8s \leq j < 9s$ , then

$$(d_7)_{ij} = \begin{cases} e_{8(j+m+1)+5} \otimes w_{8j+4 \rightarrow 8(j+1)}, & i = 3s + (j+1)s; \\ (-1)^{j_1}w_{8(j+m+1)+5j_1 \rightarrow 8(j+m+1)+5} \otimes w_{8j+4 \rightarrow 8j+4+3j_1}, \\ \quad i = j + (4j_1 - 1)s, \quad 0 \leq j_1 \leq 1; \\ 0, & \text{otherwise.} \end{cases}$$

If  $9s \leq j < 10s$ , then

$$(d_7)_{ij} = \begin{cases} w_{8(j+m)+7+4f(j_1,2) \rightarrow 8(j+m+1)+3} \otimes w_{8j+5 \rightarrow 8j+5+j_1}, \\ \quad i = j + (j_1 - 1 + 2f(j_1, 2))s, \quad 0 \leq j_1 \leq 2; \\ 0, \quad \text{otherwise.} \end{cases}$$

If  $10s \leq j < 11s$ , then

$$(d_7)_{ij} = \begin{cases} e_{8(j+m+1)+6} \otimes w_{8j+5 \rightarrow 8(j+1)}, \quad i = 2s + (j + 1)_s; \\ w_{8(j+m)+7 \rightarrow 8(j+m+1)+6} \otimes e_{8j+5}, \quad i = j - 2s; \\ 0, \quad \text{otherwise.} \end{cases}$$

If  $11s \leq j < 12s$ , then

$$(d_7)_{ij} = \begin{cases} w_{8(j+m)+7+j_1+4f(j_1,2) \rightarrow 8(j+m+1)+5} \otimes w_{8j+6 \rightarrow 8j+6+f(j_1,2)}, \\ \quad i = j + (j_1 - 2)s, \quad 0 \leq j_1 \leq 2; \\ 0, \quad \text{otherwise.} \end{cases}$$

If  $12s \leq j < 13s$ , then

$$(d_7)_{ij} = \begin{cases} (-1)^{j_1+1} w_{8(j+m+1)+2+2j_1 \rightarrow 8(j+m+1)+4} \otimes w_{8j+6 \rightarrow 8(j+1)}, \\ \quad i = j_1s + (j + 1)_s, \quad 0 \leq j_1 \leq 1; \\ w_{8(j+m)+7+4j_1 \rightarrow 8(j+m+1)+4} \otimes w_{8j+6 \rightarrow 8j+6+j_1}, \quad i = j + 3(j_1 - 1)s, \quad 0 \leq j_1 \leq 1; \\ 0, \quad \text{otherwise.} \end{cases}$$

If  $13s \leq j < 14s$ , then

$$(d_7)_{ij} = \begin{cases} w_{8(j+m+1)+j_1 \rightarrow 8(j+m+1)+1} \otimes w_{8j+6 \rightarrow 8j+6+j_1}, \quad i = j + 3(j_1 - 1)s, \quad 0 \leq j_1 \leq 1; \\ 0, \quad \text{otherwise.} \end{cases}$$

If  $14s \leq j < 15s$ , then

$$(d_7)_{ij} = \begin{cases} (-1)^{j_1} w_{8(j+m+1)+2+2j_1 \rightarrow 8(j+m+1)+7} \otimes w_{8j+7 \rightarrow 8(j+1)}, \\ \quad i = j_1s + (j + 1)_s, \quad 0 \leq j_1 \leq 1; \\ -e_{8(j+m+1)+7} \otimes w_{8j+7 \rightarrow 8(j+1)+1}, \quad i = 4s + (j + 1)_s; \\ (-1 + 2f(j_1, 0)) w_{8(j+m+1)+5-2j_1 \rightarrow 8(j+m+1)+7} \otimes e_{8j+7}, \quad i = j + (j_1 - 3)s, \quad 0 \leq j_1 \leq 2; \\ 0, \quad \text{otherwise.} \end{cases}$$

If  $15s \leq j < 16s$ , then

$$(d_7)_{ij} = \begin{cases} (-1)^{j_1+1} w_{8(j+m+1)+2+2j_1 \rightarrow 8(j+m+2)} \otimes w_{8j+7 \rightarrow 8(j+1)}, \\ \quad i = j_1s + (j + 1)_s, \quad 0 \leq j_1 \leq 1; \\ w_{8(j+m+1)+7+j_1 \rightarrow 8(j+m+2)} \otimes w_{8j+7 \rightarrow 8(j+1)+1+j_1}, \quad i = (4 + j_1)s + (j + 1)_s, \quad 0 \leq j_1 \leq 1; \\ w_{8(j+m+1)+3 \rightarrow 8(j+m+2)} \otimes e_{8j+7}, \quad i = j - 3s; \\ 0, \quad \text{otherwise.} \end{cases}$$

### Description of $d_8$

$d_8 : Q_9 \rightarrow Q_8$  – is an  $(16s \times 16s)$  matrix.

If  $0 \leq j < s$ , then

$$(d_8)_{ij} = \begin{cases} (1 - 2f(j_1, 1))w_{8(j+m-1)+7+f(j_1,2)+6f(j_1,3) \rightarrow 8(j+m)+5} \otimes w_{8j \rightarrow 8j+f(j_1,3)}, \\ \quad i = j + j_1 s, \quad 0 \leq j_1 \leq 3; \\ -e_{8(j+m)+5} \otimes w_{8j \rightarrow 8j+4}, \quad i = j + 8s; \\ -e_{8(j+m)+5} \otimes w_{8j \rightarrow 8j+6}, \quad i = j + 11s; \\ 0, \quad \text{otherwise.} \end{cases}$$

If  $s \leq j < 2s$ , then

$$(d_8)_{ij} = \begin{cases} w_{8(j+m-1)+7 \rightarrow 8(j+m)+3} \otimes e_{8j}, \quad i = j_s; \\ (-1)^{j_1} w_{8(j+m)+2+j_1 \rightarrow 8(j+m)+3} \otimes w_{8j \rightarrow 8j+3+j_1}, \quad i = j + (5 + j_1)s, \quad 0 \leq j_1 \leq 1; \\ -e_{8(j+m)+3} \otimes w_{8j \rightarrow 8j+5}, \quad i = j + 8s; \\ 0, \quad \text{otherwise.} \end{cases}$$

If  $2s \leq j < 3s$ , then

$$(d_8)_{ij} = \begin{cases} (-1)^{j_1} w_{8(j+m)+4+j_1-5f(j_1,0) \rightarrow 8(j+m)+6} \otimes w_{8j \rightarrow 8j+j_1}, \\ \quad i = j + (j_1 - f(j_1, 0))s, \quad 0 \leq j_1 \leq 2; \\ -e_{8(j+m)+6} \otimes w_{8j \rightarrow 8j+5}, \quad i = j + 8s; \\ 0, \quad \text{otherwise.} \end{cases}$$

If  $3s \leq j < 4s$ , then

$$(d_8)_{ij} = \begin{cases} w_{8(j+m)+j_1 \rightarrow 8(j+m)+1} \otimes w_{8j \rightarrow 8j+2j_1}, \quad i = j + (3j_1 - 1)s, \quad 0 \leq j_1 \leq 1; \\ -e_{8(j+m)+1} \otimes w_{8j \rightarrow 8j+6}, \quad i = j + 10s; \\ 0, \quad \text{otherwise.} \end{cases}$$

If  $4s \leq j < 5s$ , then

$$(d_8)_{ij} = \begin{cases} e_{8(j+m+1)} \otimes w_{8j+1 \rightarrow 8(j+1)}, \quad i = 2s + (j + 1)s; \\ (-1)^{j_1} w_{8(j+m)+5+j_1 \rightarrow 8(j+m)+1} \otimes w_{8j+1 \rightarrow 8j+1+j_1}, \quad i = j + (j_1 - 1)s, \quad 0 \leq j_1 \leq 1; \\ 0, \quad \text{otherwise.} \end{cases}$$

If  $5s \leq j < 6s$ , then

$$(d_8)_{ij} = \begin{cases} e_{8(j+m)+7} \otimes w_{8j+2 \rightarrow 8(j+1)}, \quad i = (j + 1)s; \\ w_{8(j+m)+6 \rightarrow 8(j+m)+7} \otimes e_{8j+2}, \quad i = j - s; \\ -w_{8(j+m)+1+j_1 \rightarrow 8(j+m)+7} \otimes w_{8j+2 \rightarrow 8j+2+j_1}, \quad i = j + j_1 s, \quad 0 \leq j_1 \leq 1; \\ 0, \quad \text{otherwise.} \end{cases}$$

If  $6s \leq j < 7s$ , then

$$(d_8)_{ij} = \begin{cases} (-1)^{j_1+1} w_{8(j+m)+7+f(j_1,2) \rightarrow 8(j+m)+1} \otimes w_{8j+3 \rightarrow 8(j+1)}, \\ \quad i = j_1 s + (j + 1)s, \quad 0 \leq j_1 \leq 2; \\ (-1)^{j_1} w_{8(j+m)+2+j_1 \rightarrow 8(j+m)+1} \otimes w_{8j+3 \rightarrow 8j+3+j_1}, \quad i = j + j_1 s, \quad 0 \leq j_1 \leq 1; \\ -e_{8(j+m)+1} \otimes w_{8j+3 \rightarrow 8j+7}, \quad i = j + 9s; \\ 0, \quad \text{otherwise.} \end{cases}$$

If  $7s \leq j < 8s$ , then

$$(d_8)_{ij} = \begin{cases} -e_{8(j+m)+7} \otimes w_{8j+4 \rightarrow 8(j+1)}, & i = s + (j+1)_s; \\ (-1)^{j_1} w_{8(j+m)+3+2j_1 \rightarrow 8(j+m)+7} \otimes e_{8j+4}, & i = j + j_1 s, \ 0 \leq j_1 \leq 1; \\ -e_{8(j+m)+7} \otimes w_{8j+4 \rightarrow 8j+7}, & i = j + 7s; \\ 0, & \text{otherwise.} \end{cases}$$

If  $8s \leq j < 9s$ , then

$$(d_8)_{ij} = \begin{cases} (-1)^{j_1+1} e_{8(j+m)+7} \otimes w_{8j+5 \rightarrow 8(j+1)}, & i = j_1 s + (j+1)_s, \ 0 \leq j_1 \leq 1; \\ (-1)^{j_1} w_{8(j+m)+3+3j_1 \rightarrow 8(j+m)+7} \otimes e_{8j+5}, & i = j + (j_1+1)s, \ 0 \leq j_1 \leq 1; \\ -w_{8(j+m)+4 \rightarrow 8(j+m)+7} \otimes w_{8j+5 \rightarrow 8j+6}, & i = j + 4s; \\ 0, & \text{otherwise.} \end{cases}$$

If  $9s \leq j < 10s$ , then

$$(d_8)_{ij} = \begin{cases} -e_{8(j+m+1)} \otimes w_{8j+5 \rightarrow 8(j+1)}, & i = 2s + (j+1)_s; \\ w_{8(j+m)+6 \rightarrow 8(j+m+1)} \otimes e_{8j+5}, & i = j + s; \\ 0, & \text{otherwise.} \end{cases}$$

If  $10s \leq j < 11s$ , then

$$(d_8)_{ij} = \begin{cases} (-1 + 2f(j_1, 1)) w_{8(j+m)+6-j_1-2f(j_1, 3)+5f(j_1, 4) \rightarrow 8(j+m)+7} \otimes w_{8j+6 \rightarrow 8j+6+f(j_1, 4)}, & i = j + j_1 s, \ 1 \leq j_1 \leq 4; \\ 0, & \text{otherwise.} \end{cases}$$

If  $11s \leq j < 12s$ , then

$$(d_8)_{ij} = \begin{cases} w_{8(j+m)+4 \rightarrow 8(j+m+1)} \otimes e_{8j+6}, & i = j + s; \\ -e_{8(j+m+1)} \otimes w_{8j+6 \rightarrow 8j+7}, & i = j + 4s; \\ 0, & \text{otherwise.} \end{cases}$$

If  $12s \leq j < 13s$ , then

$$(d_8)_{ij} = \begin{cases} -w_{8(j+m+1)+1+j_1 \rightarrow 8(j+m+1)+2} \otimes w_{8j+7 \rightarrow 8(j+1)+2+j_1}, & i = (5+j_1)s + (j+1)_s, \ 0 \leq j_1 \leq 1; \\ w_{8(j+m)+7+j_1 \rightarrow 8(j+m+1)+2} \otimes e_{8j+7}, & i = j + (2+j_1)s, \ 0 \leq j_1 \leq 1; \\ 0, & \text{otherwise.} \end{cases}$$

If  $13s \leq j < 14s$ , then

$$(d_8)_{ij} = \begin{cases} (-1)^{j_1} w_{8(j+m)+7 \rightarrow 8(j+m+1)+4} \otimes w_{8j+7 \rightarrow 8(j+1)}, & i = j_1 s + (j+1)_s, \ 0 \leq j_1 \leq 1; \\ -w_{8(j+m+1)+2+j_1-f(j_1, 0) \rightarrow 8(j+m+1)+4} \otimes w_{8j+7 \rightarrow 8(j+1)+2(j_1+1)}, & i = (5+2j_1+3f(j_1, 2))s + (j+1)_s, \ 0 \leq j_1 \leq 2; \\ w_{8(j+m+1) \rightarrow 8(j+m+1)+4} \otimes e_{8j+7}, & i = j + 2s; \\ 0, & \text{otherwise.} \end{cases}$$

If  $14s \leq j < 15s$ , then

$$(d_8)_{ij} = \begin{cases} (-1)^{j_1} w_{8(j+m+1)+5+j_1 \rightarrow 8(j+m+1)+6} \otimes w_{8j+7 \rightarrow 8(j+1)+1+j_1}, & i = (3+j_1)s + (j+1)_s, \ 0 \leq j_1 \leq 1; \\ w_{8(j+m)+7 \rightarrow 8(j+m+1)+6} \otimes e_{8j+7}, & i = j; \\ 0, & \text{otherwise.} \end{cases}$$

If  $15s \leq j < 16s$ , then

$$(d_8)_{ij} = \begin{cases} -e_{8(j+m+1)+5} \otimes w_{8j+7 \rightarrow 8(j+1)+1}, & i = 3s + (j+1)_s; \\ w_{8(j+m+1) \rightarrow 8(j+m+1)+5} \otimes e_{8j+7}, & i = j; \\ 0, & \text{otherwise.} \end{cases}$$

### Description of $d_9$

$d_9 : Q_{10} \rightarrow Q_9$  – is an  $(16s \times 19s)$  matrix.

If  $0 \leq j < s$ , then

$$(d_9)_{ij} = \begin{cases} (-1)^{j_1} w_{8(j+m)+5-2j_1+5f(j_1,2)+2f(j_1,3) \rightarrow 8(j+m)+7} \otimes e_{8j}, & i = j + j_1s, \ 0 \leq j_1 \leq 3; \\ -e_{8(j+m)+7} \otimes w_{8j \rightarrow 8j+2}, & i = j + 5s; \\ (-1 + 2f(j_1, 2))e_{8(j+m)+7} \otimes w_{8j \rightarrow 8j+4+j_1}, & i = j + (7 + j_1 + f(j_1, 2))s, \ 0 \leq j_1 \leq 2; \\ 0, & \text{otherwise.} \end{cases}$$

If  $s \leq j < 2s$ , then

$$(d_9)_{ij} = \begin{cases} w_{8(j+m)+3 \rightarrow 8(j+m+1)} \otimes e_{8j}, & i = j; \\ -e_{8(j+m+1)} \otimes w_{8j \rightarrow 8j+3}, & i = j + 5s; \\ w_{8(j+m)+7+j_1-f(j_1,2) \rightarrow 8(j+m+1)} \otimes w_{8j \rightarrow 8j+5+f(j_1,2)}, & i = j + (7 + j_1 + f(j_1, 2))s, \ 0 \leq j_1 \leq 2; \\ 0, & \text{otherwise.} \end{cases}$$

If  $2s \leq j < 3s$ , then

$$(d_9)_{ij} = \begin{cases} w_{8(j+m)+6+2j_1 \rightarrow 8(j+m+1)} \otimes w_{8j \rightarrow 8j+j_1}, & i = j + 2j_1s, \ 0 \leq j_1 \leq 1; \\ e_{8(j+m+1)} \otimes w_{8j \rightarrow 8j+5}, & i = j + 7s; \\ 0, & \text{otherwise.} \end{cases}$$

If  $3s \leq j < 4s$ , then

$$(d_9)_{ij} = \begin{cases} -w_{8(j+m+1)+5+j_1 \rightarrow 8(j+m+1)+6} \otimes w_{8j+1 \rightarrow 8(j+1)}, & i = 2j_1s + (j+1)_s, \ 0 \leq j_1 \leq 1; \\ w_{8(j+m+1)+1-j_1 \rightarrow 8(j+m+1)+6} \otimes w_{8j+1 \rightarrow 8j+j_1}, & i = j + j_1s, \ 1 \leq j_1 \leq 2; \\ 0, & \text{otherwise.} \end{cases}$$

If  $4s \leq j < 5s$ , then

$$(d_9)_{ij} = \begin{cases} -e_{8(j+m+1)+1} \otimes w_{8j+1 \rightarrow 8(j+1)}, & i = 3s + (j+1)_s; \\ w_{8(j+m+1) \rightarrow 8(j+m+1)+1} \otimes e_{8j+1}, & i = j; \\ 0, & \text{otherwise.} \end{cases}$$

If  $5s \leq j < 6s$ , then

$$(d_9)_{ij} = \begin{cases} w_{8(j+m+1)+1 \rightarrow 8(j+m+1)+2} \otimes w_{8j+2 \rightarrow 8(j+1)}, & i = 3s + (j+1)_s; \\ w_{8(j+m)+7 \rightarrow 8(j+m+1)+2} \otimes w_{8j+2 \rightarrow 8j+2+j_1}, & i = j + j_1s, \ 0 \leq j_1 \leq 2; \\ e_{8(j+m+1)+2} \otimes w_{8j+2 \rightarrow 8j+7}, & i = j + 7s; \\ 0, & \text{otherwise.} \end{cases}$$

If  $6s \leq j < 7s$ , then

$$(d_9)_{ij} = \begin{cases} e_{8(j+m+1)+3} \otimes w_{8j+3 \rightarrow 8(j+1)}, & i = s + (j+1)_s; \\ w_{8(j+m+1)+1 \rightarrow 8(j+m+1)+3} \otimes w_{8j+3 \rightarrow 8(j+1)}, & i = 3s + (j+1)_s; \\ w_{8(j+m+1)-j_1 \rightarrow 8(j+m+1)+3} \otimes w_{8j+3 \rightarrow 8j+3+j_1}, & i = j + j_1s, \ 0 \leq j_1 \leq 1; \\ w_{8(j+m+1)+2 \rightarrow 8(j+m+1)+3} \otimes w_{8j+3 \rightarrow 8j+7}, & i = j + 6s; \\ 0, & \text{otherwise.} \end{cases}$$

If  $7s \leq j < 8s$ , then

$$(d_9)_{ij} = \begin{cases} e_{8(j+m+1)+5} \otimes w_{8j+3 \rightarrow 8(j+1)}, & i = (j+1)_s; \\ w_{8(j+m+1) \rightarrow 8(j+m+1)+5} \otimes e_{8j+3}, & i = j - s; \\ e_{8(j+m+1)+5} \otimes w_{8j+3 \rightarrow 8j+7}, & i = j + 8s; \\ 0, & \text{otherwise.} \end{cases}$$

If  $8s \leq j < 9s$ , then

$$(d_9)_{ij} = \begin{cases} w_{8(j+m+1)+3 \rightarrow 8(j+m+1)+4} \otimes w_{8j+4 \rightarrow 8(j+1)}, & i = s + (j+1)_s; \\ w_{8(j+m)+7 \rightarrow 8(j+m+1)+4} \otimes e_{8j+4}, & i = j - s; \\ (-1)^{j_1} w_{8(j+m+1)+2+2j_1 \rightarrow 8(j+m+1)+4} \otimes w_{8j+4 \rightarrow 8j+7}, & i = j + (4+j_1)s, \ 0 \leq j_1 \leq 1; \\ 0, & \text{otherwise.} \end{cases}$$

If  $9s \leq j < 10s$ , then

$$(d_9)_{ij} = \begin{cases} e_{8(j+m+1)+6} \otimes w_{8j+4 \rightarrow 8(j+1)}, & i = 2s + (j+1)_s; \\ w_{8(j+m)+7 \rightarrow 8(j+m+1)+6} \otimes e_{8j+4}, & i = j - 2s; \\ e_{8(j+m+1)+6} \otimes w_{8j+4 \rightarrow 8j+7}, & i = j + 5s; \\ 0, & \text{otherwise.} \end{cases}$$

If  $10s \leq j < 11s$ , then

$$(d_9)_{ij} = \begin{cases} e_{8(j+m+1)+5} \otimes w_{8j+5 \rightarrow 8(j+1)}, & i = (j+1)_s; \\ w_{8(j+m)+7+j_1 \rightarrow 8(j+m+1)+5} \otimes e_{8j+5}, & i = j + (j_1 - 2)s, \ 0 \leq j_1 \leq 1; \\ 0, & \text{otherwise.} \end{cases}$$

If  $11s \leq j < 12s$ , then

$$(d_9)_{ij} = \begin{cases} w_{8(j+m)+7 \rightarrow 8(j+m+1)+4} \otimes e_{8j+5}, & i = j - 3s; \\ w_{8(j+m+1)+4j_1 \rightarrow 8(j+m+1)+4} \otimes w_{8j+5 \rightarrow 8j+6+j_1}, & i = j + 2j_1s, \ 0 \leq j_1 \leq 1; \\ 0, & \text{otherwise.} \end{cases}$$



If  $12s \leq j < 13s$ , then

$$(d_9)_{ij} = \begin{cases} e_{8(j+m+1)+1} \otimes w_{8j+5 \rightarrow 8(j+1)}, & i = 3s + (j+1)_s; \\ w_{8(j+m+1) \rightarrow 8(j+m+1)+1} \otimes e_{8j+5}, & i = j - 3s; \\ 0, & \text{otherwise.} \end{cases}$$

If  $13s \leq j < 14s$ , then

$$(d_9)_{ij} = \begin{cases} w_{8(j+m)+7+j_1+f(j_1,2) \rightarrow 8(j+m+1)+2} \otimes w_{8j+6 \rightarrow 8j+6+f(j_1,2)}, \\ \quad i = j + (j_1 - 3)s, \quad 0 \leq j_1 \leq 2; \\ 0, & \text{otherwise.} \end{cases}$$

If  $14s \leq j < 15s$ , then

$$(d_9)_{ij} = \begin{cases} w_{8(j+m)+7 \rightarrow 8(j+m+1)+6} \otimes e_{8j+6}, & i = j - 4s; \\ e_{8(j+m+1)+6} \otimes w_{8j+6 \rightarrow 8j+7}, & i = j; \\ 0, & \text{otherwise.} \end{cases}$$

If  $15s \leq j < 16s$ , then

$$(d_9)_{ij} = \begin{cases} w_{8(j+m+1) \rightarrow 8(j+m+1)+5} \otimes e_{8j+6}, & i = j - 4s; \\ e_{8(j+m+1)+5} \otimes w_{8j+6 \rightarrow 8j+7}, & i = j; \\ 0, & \text{otherwise.} \end{cases}$$

If  $16s \leq j < 17s$ , then

$$(d_9)_{ij} = \begin{cases} -e_{8(j+m+1)+7} \otimes w_{8j+7 \rightarrow 8(j+1)+2}, & i = 5s + (j+1)_s; \\ w_{8(j+m+1)+2 \rightarrow 8(j+m+1)+7} \otimes e_{8j+7}, & i = j - 4s; \\ -w_{8(j+m+1)+6-j_1 \rightarrow 8(j+m+1)+7} \otimes e_{8j+7}, & i = j + (j_1 - 2)s, \quad 0 \leq j_1 \leq 1; \\ 0, & \text{otherwise.} \end{cases}$$

If  $17s \leq j < 18s$ , then

$$(d_9)_{ij} = \begin{cases} (-1)^{j_1} w_{8(j+m+1)+3j_1 \rightarrow 8(j+m+1)+7} \otimes w_{8j+7 \rightarrow 8(j+1)}, \\ \quad i = j_1 s + (j+1)_s, \quad 1 \leq j_1 \leq 2; \\ -e_{8(j+m+1)+7} \otimes w_{8j+7 \rightarrow 8(j+1)+2+3j_1}, & i = (5+3j_1)s + (j+1)_s, \quad 0 \leq j_1 \leq 1; \\ (-1)^{j_1} w_{8(j+m+1)+4+j_1 \rightarrow 8(j+m+1)+7} \otimes e_{8j+7}, & i = j + 2(j_1 - 2)s, \quad 0 \leq j_1 \leq 1; \\ 0, & \text{otherwise.} \end{cases}$$

If  $18s \leq j < 19s$ , then

$$(d_9)_{ij} = \begin{cases} -e_{8(j+m+2)} \otimes w_{8j+7 \rightarrow 8(j+1)+1}, & i = 4s + (j+1)_s; \\ w_{8(j+m+1)+6 \rightarrow 8(j+m+2)} \otimes e_{8j+7}, & i = j - 4s; \\ 0, & \text{otherwise.} \end{cases}$$

#### Description of $d_{10}$

$d_{10} : Q_{11} \rightarrow Q_{10}$  - is an  $(19s \times 18s)$  matrix.

If  $0 \leq j < s$ , then

$$(d_{10})_{ij} = \begin{cases} w_{8(j+m-1)+7+j_1 \rightarrow 8(j+m)+2} \otimes e_{8j}, & i = j + j_1 s, \ 0 \leq j_1 \leq 1; \\ e_{8(j+m)+2} \otimes w_{8j \rightarrow 8j+2}, & i = j + 5s; \\ -w_{8(j+m)+1+j_1 \rightarrow 8(j+m)+2} \otimes w_{8j \rightarrow 8j+5+j_1}, & i = j + (12 + j_1)s, \ 0 \leq j_1 \leq 1; \\ 0, & \text{otherwise.} \end{cases}$$

If  $s \leq j < 2s$ , then

$$(d_{10})_{ij} = \begin{cases} w_{8(j+m-1)+7 \rightarrow 8(j+m)+6} \otimes e_{8j}, & i = j_s; \\ (-1)^{j_1+1} w_{8(j+m)+6j_1 \rightarrow 8(j+m)+6} \otimes w_{8j \rightarrow 8j+j_1}, & i = j + (j_1 + 1)s, \ 0 \leq j_1 \leq 1; \\ (1 - 2f(j_1, 2)) w_{8(j+m)+6-f(j_1, 1) \rightarrow 8(j+m)+6} \otimes w_{8j \rightarrow 8j+4+j_1}, \\ \quad i = j + (8 + j_1 + 3f(j_1, 2))s, \ 0 \leq j_1 \leq 2; \\ 0, & \text{otherwise.} \end{cases}$$

If  $2s \leq j < 3s$ , then

$$(d_{10})_{ij} = \begin{cases} w_{8(j+m) \rightarrow 8(j+m)+4} \otimes e_{8j}, & i = j - s; \\ (-1 + 2f(j_1, 0)) w_{8(j+m)+4-f(j_1, 0) \rightarrow 8(j+m)+4} \otimes w_{8j \rightarrow 8j+3+j_1}, \\ \quad i = j + (4 + 2j_1 + f(j_1, 2))s, \ 0 \leq j_1 \leq 2; \\ -w_{8(j+m)+1 \rightarrow 8(j+m)+4} \otimes w_{8j \rightarrow 8j+5}, & i = j + 10s; \\ 0, & \text{otherwise.} \end{cases}$$

If  $3s \leq j < 4s$ , then

$$(d_{10})_{ij} = \begin{cases} (-1)^{j_1} w_{8(j+m)+j_1 \rightarrow 8(j+m)+1} \otimes w_{8j \rightarrow 8j+j_1}, & i = j + (2j_1 - 1)s, \ 0 \leq j_1 \leq 1; \\ -e_{8(j+m)+1} \otimes w_{8j \rightarrow 8j+5}, & i = j + 9s; \\ 0, & \text{otherwise.} \end{cases}$$

If  $4s \leq j < 5s$ , then

$$(d_{10})_{ij} = \begin{cases} w_{8(j+m) \rightarrow 8(j+m)+5} \otimes e_{8j}, & i = j - 3s; \\ e_{8(j+m)+5} \otimes w_{8j \rightarrow 8j+3}, & i = j + 3s; \\ -e_{8(j+m)+5} \otimes w_{8j \rightarrow 8j+5}, & i = j + 6s; \\ -e_{8(j+m)+5} \otimes w_{8j \rightarrow 8j+6}, & i = j + 11s; \\ 0, & \text{otherwise.} \end{cases}$$

If  $5s \leq j < 6s$ , then

$$(d_{10})_{ij} = \begin{cases} e_{8(j+m)+7} \otimes w_{8j+1 \rightarrow 8(j+1)}, & i = (j + 1)s; \\ w_{8(j+m)+6 \rightarrow 8(j+m)+7} \otimes e_{8j+1}, & i = j - 2s; \\ (-1 + 2f(j_1, 2)) w_{8(j+m)+1+j_1 \rightarrow 8(j+m)+7} \otimes w_{8j+1 \rightarrow 8j+1+j_1}, \\ \quad i = j + (j_1 - 1)s, \ 0 \leq j_1 \leq 2; \\ 0, & \text{otherwise.} \end{cases}$$

If  $6s \leq j < 7s$ , then

$$(d_{10})_{ij} = \begin{cases} e_{8(j+m+1)} \otimes w_{8j+2 \rightarrow 8(j+1)}, & i = s + (j+1)_s; \\ (-1)^{j_1} w_{8(j+m)+2+j_1 \rightarrow 8(j+m+1)} \otimes w_{8j+2 \rightarrow 8j+2+j_1}, & i = j + (j_1 - 1)s, \ 0 \leq j_1 \leq 1; \\ 0, & \text{otherwise.} \end{cases}$$

If  $7s \leq j < 8s$ , then

$$(d_{10})_{ij} = \begin{cases} e_{8(j+m)+7} \otimes w_{8j+3 \rightarrow 8(j+1)}, & i = (j+1)_s; \\ w_{8(j+m)+3 \rightarrow 8(j+m)+7} \otimes e_{8j+3}, & i = j - s; \\ -w_{8(j+m)+5+j_1 \rightarrow 8(j+m)+7} \otimes w_{8j+3 \rightarrow 8j+3+j_1+2f(j_1,2)}, & \\ \quad i = j + (2j_1 + 5f(j_1,2))s, \ 0 \leq j_1 \leq 2; \\ 0, & \text{otherwise.} \end{cases}$$

If  $8s \leq j < 9s$ , then

$$(d_{10})_{ij} = \begin{cases} (-1)^{j_1} w_{8(j+m)+4+2j_1 \rightarrow 8(j+m)+7} \otimes e_{8j+4}, & i = j + j_1s, \ 0 \leq j_1 \leq 1; \\ (-1)^{j_1+1} e_{8(j+m)+7} \otimes w_{8j+4 \rightarrow 8j+7}, & i = j + (8 + j_1)s, \ 0 \leq j_1 \leq 1; \\ 0, & \text{otherwise.} \end{cases}$$

If  $9s \leq j < 10s$ , then

$$(d_{10})_{ij} = \begin{cases} -e_{8(j+m+1)} \otimes w_{8j+4 \rightarrow 8(j+1)}, & i = 2s + (j+1)_s; \\ w_{8(j+m)+6 \rightarrow 8(j+m+1)} \otimes e_{8j+4}, & i = j; \\ -e_{8(j+m+1)} \otimes w_{8j+4 \rightarrow 8j+7}, & i = j + 9s; \\ 0, & \text{otherwise.} \end{cases}$$

If  $10s \leq j < 11s$ , then

$$(d_{10})_{ij} = \begin{cases} -e_{8(j+m)+7} \otimes w_{8j+5 \rightarrow 8(j+1)}, & i = (j+1)_s; \\ (-1 + 2f(j_1, 0)) w_{8(j+m)+5-j_1-2f(j_1,2) \rightarrow 8(j+m)+7} \otimes e_{8j+5}, & i = j + j_1s, \ 0 \leq j_1 \leq 2; \\ w_{8(j+m)+5+2j_1 \rightarrow 8(j+m)+7} \otimes w_{8j+5 \rightarrow 8j+6+j_1}, & i = j + (5 + 2j_1)s, \ 0 \leq j_1 \leq 1; \\ 0, & \text{otherwise.} \end{cases}$$

If  $11s \leq j < 12s$ , then

$$(d_{10})_{ij} = \begin{cases} (-1)^{j_1} e_{8(j+m+1)} \otimes w_{8j+5 \rightarrow 8(j+1)}, & i = j_1s + (j+1)_s, \ 1 \leq j_1 \leq 2; \\ (-1 + 2f(j_1, 0)) w_{8(j+m)+4+j_1+f(j_1,2) \rightarrow 8(j+m+1)} \otimes w_{8j+5 \rightarrow 8j+5+j_1}, & \\ \quad i = j + (4j_1 - 2f(j_1,2))s, \ 0 \leq j_1 \leq 2; \\ 0, & \text{otherwise.} \end{cases}$$

If  $12s \leq j < 13s$ , then

$$(d_{10})_{ij} = \begin{cases} (-1 + 2f(j_1, 1)) w_{8(j+m)+8-j_1-5f(j_1,1)+3f(j_1,4) \rightarrow 8(j+m)+7} \otimes w_{8j+6 \rightarrow 8j+6+f(j_1,4)}, & \\ \quad i = j + j_1s, \ 1 \leq j_1 \leq 4; \\ 0, & \text{otherwise.} \end{cases}$$

If  $13s \leq j < 14s$ , then

$$(d_{10})_{ij} = \begin{cases} w_{8(j+m)+6 \rightarrow 8(j+m+1)} \otimes e_{8j+6}, & i = j + s; \\ -e_{8(j+m+1)} \otimes w_{8j+6 \rightarrow 8j+7}, & i = j + 5s; \\ 0, & \text{otherwise.} \end{cases}$$

If  $14s \leq j < 15s$ , then

$$(d_{10})_{ij} = \begin{cases} w_{8(j+m+1) \rightarrow 8(j+m+1)+5} \otimes w_{8j+7 \rightarrow 8(j+1)}, & i = 2s + (j+1)_s; \\ -e_{8(j+m+1)+5} \otimes w_{8j+7 \rightarrow 8(j+1)+5}, & i = 10s + (j+1)_s; \\ (-1)^{j_1} w_{8(j+m)+7+f(j_1,2) \rightarrow 8(j+m+1)+5} \otimes e_{8j+7}, & i = j + (2+j_1)s, \ 0 \leq j_1 \leq 2; \\ 0, & \text{otherwise.} \end{cases}$$

If  $15s \leq j < 16s$ , then

$$(d_{10})_{ij} = \begin{cases} (-1)^{j_1} w_{8(j+m+1)+2+j_1 \rightarrow 8(j+m+1)+3} \otimes w_{8j+7 \rightarrow 8(j+1)+2+j_1}, \\ \quad i = (5+j_1)s + (j+1)_s, \ 0 \leq j_1 \leq 1; \\ w_{8(j+m)+7 \rightarrow 8(j+m+1)+3} \otimes e_{8j+7}, & i = j + s; \\ 0, & \text{otherwise.} \end{cases}$$

If  $16s \leq j < 17s$ , then

$$(d_{10})_{ij} = \begin{cases} (-1)^{j_1+1} w_{8(j+m+1)+6j_1 \rightarrow 8(j+m+1)+6} \otimes w_{8j+7 \rightarrow 8(j+1)+j_1}, \\ \quad i = (2+j_1)s + (j+1)_s, \ 0 \leq j_1 \leq 1; \\ w_{8(j+m+1)+5 \rightarrow 8(j+m+1)+6} \otimes w_{8j+7 \rightarrow 8(j+1)+5}, & i = 10s + (j+1)_s; \\ w_{8(j+m)+7 \rightarrow 8(j+m+1)+6} \otimes e_{8j+7}, & i = j + s; \\ 0, & \text{otherwise.} \end{cases}$$

If  $17s \leq j < 18s$ , then

$$(d_{10})_{ij} = \begin{cases} e_{8(j+m+1)+1} \otimes w_{8j+7 \rightarrow 8(j+1)+1}, & i = 4s + (j+1)_s; \\ w_{8(j+m+1) \rightarrow 8(j+m+1)+1} \otimes e_{8j+7}, & i = j + s; \\ 0, & \text{otherwise.} \end{cases}$$

### Description of $d_{11}$

$d_{11} : Q_{12} \rightarrow Q_{11}$  - is an  $(18s \times 19s)$  matrix.

If  $0 \leq j < s$ , then

$$(d_{11})_{ij} = \begin{cases} (-1 + 2f(j_1, 0)) w_{8(j+m)+2+4j_1-9f(j_1,2) \rightarrow 8(j+m)+7} \otimes e_{8j}, \\ \quad i = j + (j_1 + f(j_1, 2))s, \ 0 \leq j_1 \leq 2; \\ -w_{8(j+m)+5 \rightarrow 8(j+m)+7} \otimes e_{8j}, & i = j + 4s; \\ (-1)^{j_1} e_{8(j+m)+7} \otimes w_{8j \rightarrow 8j+1+2j_1+f(j_1,2)}, & i = j + (5 + 2j_1 + 3f(j_1, 2))s, \ 0 \leq j_1 \leq 2; \\ 0, & \text{otherwise.} \end{cases}$$

If  $s \leq j < 2s$ , then

$$(d_{11})_{ij} = \begin{cases} w_{8(j+m)+2 \rightarrow 8(j+m+1)} \otimes e_{8j}, & i = j_s; \\ -w_{8(j+m)+4 \rightarrow 8(j+m+1)} \otimes e_{8j}, & i = j + s; \\ -w_{8(j+m+1)-f(j_1,1) \rightarrow 8(j+m+1)} \otimes w_{8j \rightarrow 8j+4-2f(j_1,0)}, \\ \quad i = j + (6 + j_1 - f(j_1,0))s, & 0 \leq j_1 \leq 2; \\ (1 - 2f(j_1,0))w_{8(j+m+1)-f(j_1,1) \rightarrow 8(j+m+1)} \otimes w_{8j \rightarrow 8j+6-f(j_1,0)}, \\ \quad i = j + (10 + j_1)s, & 0 \leq j_1 \leq 2; \\ 0, & \text{otherwise.} \end{cases}$$

If  $2s \leq j < 3s$ , then

$$(d_{11})_{ij} = \begin{cases} w_{8(j+m)+4 \rightarrow 8(j+m)+7} \otimes e_{8j}, & i = j; \\ -w_{8(j+m)+5 \rightarrow 8(j+m)+7} \otimes e_{8j}, & i = j + 2s; \\ (-1)^{j_1+1}e_{8(j+m)+7} \otimes w_{8j \rightarrow 8j+3+j_1}, & i = j + (5 + j_1 + f(j_1,2))s, \quad 0 \leq j_1 \leq 2; \\ 0, & \text{otherwise.} \end{cases}$$

If  $3s \leq j < 4s$ , then

$$(d_{11})_{ij} = \begin{cases} -e_{8(j+m+1)+2} \otimes w_{8j+1 \rightarrow 8(j+1)}, & i = (j+1)_s; \\ w_{8(j+m)+7+j_1 \rightarrow 8(j+m+1)+2} \otimes w_{8j+1 \rightarrow 8j+1+j_1}, & i = j + (2 + j_1)s, \quad 0 \leq j_1 \leq 1; \\ 0, & \text{otherwise.} \end{cases}$$

If  $4s \leq j < 5s$ , then

$$(d_{11})_{ij} = \begin{cases} -w_{8(j+m+1)+2 \rightarrow 8(j+m+1)+3} \otimes w_{8j+2 \rightarrow 8(j+1)}, & i = (j+1)_s; \\ w_{8(j+m+1)-j_1 \rightarrow 8(j+m+1)+3} \otimes w_{8j+2 \rightarrow 8j+2+j_1}, & i = j + (2 + j_1)s, \quad 0 \leq j_1 \leq 1; \\ e_{8(j+m+1)+3} \otimes w_{8j+2 \rightarrow 8j+7}, & i = j + 11s; \\ 0, & \text{otherwise.} \end{cases}$$

If  $5s \leq j < 6s$ , then

$$(d_{11})_{ij} = \begin{cases} -e_{8(j+m+1)+5} \otimes w_{8j+2 \rightarrow 8(j+1)}, & i = 4s + (j+1)_s; \\ w_{8(j+m+1) \rightarrow 8(j+m+1)+5} \otimes e_{8j+2}, & i = j + s; \\ 0, & \text{otherwise.} \end{cases}$$

If  $6s \leq j < 7s$ , then

$$(d_{11})_{ij} = \begin{cases} -w_{8(j+m+1)+2 \rightarrow 8(j+m+1)+4} \otimes w_{8j+3 \rightarrow 8(j+1)}, & i = (j+1)_s; \\ e_{8(j+m+1)+4} \otimes w_{8j+3 \rightarrow 8(j+1)}, & i = 2s + (j+1)_s; \\ w_{8(j+m)+7 \rightarrow 8(j+m+1)+4} \otimes e_{8j+3}, & i = j + s; \\ w_{8(j+m+1)+3 \rightarrow 8(j+m+1)+4} \otimes w_{8j+3 \rightarrow 8j+7}, & i = j + 9s; \\ 0, & \text{otherwise.} \end{cases}$$

If  $7s \leq j < 8s$ , then

$$(d_{11})_{ij} = \begin{cases} -e_{8(j+m+1)+6} \otimes w_{8j+3 \rightarrow 8(j+1)}, & i = s + (j+1)_s; \\ (-1)^{j_1} w_{8(j+m)+7 \rightarrow 8(j+m+1)+6} \otimes w_{8j+3 \rightarrow 8j+3+j_1}, & i = j + j_1 s, \ 0 \leq j_1 \leq 1; \\ e_{8(j+m+1)+6} \otimes w_{8j+3 \rightarrow 8j+7}, & i = j + 9s; \\ 0, & \text{otherwise.} \end{cases}$$

If  $8s \leq j < 9s$ , then

$$(d_{11})_{ij} = \begin{cases} w_{8(j+m)+7+j_1 \rightarrow 8(j+m+1)+5} \otimes e_{8j+4}, & i = j + j_1 s, \ 0 \leq j_1 \leq 1; \\ e_{8(j+m+1)+5} \otimes w_{8j+4 \rightarrow 8j+7}, & i = j + 6s; \\ 0, & \text{otherwise.} \end{cases}$$

If  $9s \leq j < 10s$ , then

$$(d_{11})_{ij} = \begin{cases} e_{8(j+m+1)+1} \otimes w_{8j+4 \rightarrow 8(j+1)}, & i = 3s + (j+1)_s; \\ w_{8(j+m+1) \rightarrow 8(j+m+1)+1} \otimes e_{8j+4}, & i = j; \\ e_{8(j+m+1)+1} \otimes w_{8j+4 \rightarrow 8j+7}, & i = j + 8s; \\ 0, & \text{otherwise.} \end{cases}$$

If  $10s \leq j < 11s$ , then

$$(d_{11})_{ij} = \begin{cases} e_{8(j+m+1)+2} \otimes w_{8j+5 \rightarrow 8(j+1)}, & i = (j+1)_s; \\ -w_{8(j+m+1)+1 \rightarrow 8(j+m+1)+2} \otimes w_{8j+5 \rightarrow 8(j+1)}, & i = 3s + (j+1)_s; \\ w_{8(j+m)+7+j_1 \rightarrow 8(j+m+1)+2} \otimes e_{8j+5}, & i = j + j_1 s, \ 0 \leq j_1 \leq 1; \\ 0, & \text{otherwise.} \end{cases}$$

If  $11s \leq j < 12s$ , then

$$(d_{11})_{ij} = \begin{cases} e_{8(j+m+1)+6} \otimes w_{8j+5 \rightarrow 8(j+1)}, & i = s + (j+1)_s; \\ w_{8(j+m)+7 \rightarrow 8(j+m+1)+6} \otimes e_{8j+5}, & i = j - s; \\ w_{8(j+m)+7+j_1+4f(j_1,2) \rightarrow 8(j+m+1)+6} \otimes w_{8j+5 \rightarrow 8j+6+f(j_1,2)}, & i = j + (j_1+1)s, \ 0 \leq j_1 \leq 2; \\ 0, & \text{otherwise.} \end{cases}$$

If  $12s \leq j < 13s$ , then

$$(d_{11})_{ij} = \begin{cases} e_{8(j+m+1)+5} \otimes w_{8j+5 \rightarrow 8(j+1)}, & i = 4s + (j+1)_s; \\ w_{8(j+m+1) \rightarrow 8(j+m+1)+5} \otimes e_{8j+5}, & i = j - s; \\ -w_{8(j+m)+7+j_1+4f(j_1,2) \rightarrow 8(j+m+1)+5} \otimes w_{8j+5 \rightarrow 8j+6+f(j_1,2)}, & i = j + j_1 s, \ 0 \leq j_1 \leq 2; \\ 0, & \text{otherwise.} \end{cases}$$

If  $13s \leq j < 14s$ , then

$$(d_{11})_{ij} = \begin{cases} w_{8(j+m)+7+j_1+4f(j_1,2) \rightarrow 8(j+m+1)+6} \otimes w_{8j+6 \rightarrow 8j+6+f(j_1,2)}, & i = j + (j_1-1)s, \ 0 \leq j_1 \leq 2; \\ e_{8(j+m+1)+6} \otimes w_{8j+6 \rightarrow 8j+7}, & i = j + 3s; \\ 0, & \text{otherwise.} \end{cases}$$

If  $14s \leq j < 15s$ , then

$$(d_{11})_{ij} = \begin{cases} w_{8(j+m)+7 \rightarrow 8(j+m+1)+3} \otimes e_{8j+6}, & i = j - 2s; \\ e_{8(j+m+1)+3} \otimes w_{8j+6 \rightarrow 8j+7}, & i = j + s; \\ 0, & \text{otherwise.} \end{cases}$$

If  $15s \leq j < 16s$ , then

$$(d_{11})_{ij} = \begin{cases} w_{8(j+m+1) \rightarrow 8(j+m+1)+1} \otimes e_{8j+6}, & i = j - 2s; \\ e_{8(j+m+1)+1} \otimes w_{8j+6 \rightarrow 8j+7}, & i = j + 2s; \\ 0, & \text{otherwise.} \end{cases}$$

If  $16s \leq j < 17s$ , then

$$(d_{11})_{ij} = \begin{cases} -e_{8(j+m+1)+7} \otimes w_{8j+7 \rightarrow 8(j+1)+1}, & i = 5s + (j+1)_s; \\ (-1)^{j_1} w_{8(j+m+1)+5-2j_1+5f(j_1,2)+2f(j_1,3) \rightarrow 8(j+m+1)+7} \otimes e_{8j+7}, & i = j + (j_1 - 2)s, \ 0 \leq j_1 \leq 3; \\ 0, & \text{otherwise.} \end{cases}$$

If  $17s \leq j < 18s$ , then

$$(d_{11})_{ij} = \begin{cases} -e_{8(j+m+2)} \otimes w_{8j+7 \rightarrow 8(j+1)+2}, & i = 6s + (j+1)_s; \\ w_{8(j+m+1)+3 \rightarrow 8(j+m+2)} \otimes e_{8j+7}, & i = j - 2s; \\ 0, & \text{otherwise.} \end{cases}$$

If  $18s \leq j < 19s$ , then

$$(d_{11})_{ij} = \begin{cases} (1 - 2f(j_1, 0)) w_{8(j+m+1)+4-3j_1+7f(j_1,2) \rightarrow 8(j+m+2)} \otimes w_{8j+7 \rightarrow 8(j+1)}, & i = (2 + j_1)s + (j+1)_s, \ 0 \leq j_1 \leq 2; \\ (-1 + 2f(j_1, 2)) w_{8(j+m+1)+7+f(j_1,1) \rightarrow 8(j+m+2)} \otimes w_{8j+7 \rightarrow 8(j+1)+1+j_1}, & i = (5 + j_1)s + (j+1)_s, \ 0 \leq j_1 \leq 3; \\ -e_{8(j+m+2)} \otimes w_{8j+7 \rightarrow 8(j+1)+5}, & i = 11s + (j+1)_s; \\ w_{8(j+m+1)+6 \rightarrow 8(j+m+2)} \otimes e_{8j+7}, & i = j - 2s; \\ 0, & \text{otherwise.} \end{cases}$$

### Description of $d_{12}$

$d_{12} : Q_{13} \rightarrow Q_{12}$  - is an  $(19s \times 18s)$  matrix.

If  $0 \leq j < s$ , then

$$(d_{12})_{ij} = \begin{cases} (-1 + 2f(j_1, 0)) w_{8(j+m-1)+7+f(j_1,1)+3f(j_1,3) \rightarrow 8(j+m)+2} \otimes w_{8j \rightarrow 8j+f(j_1,3)}, & i = j + j_1s, \ 0 \leq j_1 \leq 3; \\ (-1 + 2f(j_1, 2)) w_{8(j+m)+1+f(j_1,1) \rightarrow 8(j+m)+2} \otimes w_{8j \rightarrow 8j+4+j_1}, & i = j + (9 + j_1 + 4f(j_1, 2))s, \ 0 \leq j_1 \leq 2; \\ 0, & \text{otherwise.} \end{cases}$$

If  $s \leq j < 2s$ , then

$$(d_{12})_{ij} = \begin{cases} w_{8(j+m-1)+7 \rightarrow 8(j+m)+3} \otimes e_{8j}, & i = j_s; \\ (-1)^{j_1} w_{8(j+m)+1+j_1 \rightarrow 8(j+m)+3} \otimes w_{8j \rightarrow 8j+j_1}, & i = j + (1+j_1)s, \ 1 \leq j_1 \leq 2; \\ -e_{8(j+m)+3} \otimes w_{8j \rightarrow 8j+6}, & i = j + 13s; \\ 0, & \text{otherwise.} \end{cases}$$

If  $2s \leq j < 3s$ , then

$$(d_{12})_{ij} = \begin{cases} w_{8(j+m-1)+7 \rightarrow 8(j+m)+6} \otimes e_{8j}, & i = j; \\ e_{8(j+m)+6} \otimes w_{8j \rightarrow 8j+3+2j_1}, & i = j + (5+4j_1)s, \ 0 \leq j_1 \leq 1; \\ -e_{8(j+m)+6} \otimes w_{8j \rightarrow 8j+6}, & i = j + 11s; \\ 0, & \text{otherwise.} \end{cases}$$

If  $3s \leq j < 4s$ , then

$$(d_{12})_{ij} = \begin{cases} w_{8(j+m) \rightarrow 8(j+m)+5} \otimes e_{8j}, & i = j - 2s; \\ e_{8(j+m)+5} \otimes w_{8j \rightarrow 8j+2+2j_1-f(j_1,2)}, & i = j + (2+3j_1+f(j_1,2))s, \ 0 \leq j_1 \leq 2; \\ 0, & \text{otherwise.} \end{cases}$$

If  $4s \leq j < 5s$ , then

$$(d_{12})_{ij} = \begin{cases} w_{8(j+m+1)-j_1 \rightarrow 8(j+m+1)} \otimes w_{8j+1 \rightarrow 8(j+1)}, & i = (1+j_1)s + (j+1)s, \ 0 \leq j_1 \leq 1; \\ (-1)^{j_1} w_{8(j+m)+2+3j_1 \rightarrow 8(j+m+1)} \otimes w_{8j+1 \rightarrow 8j+1+j_1}, & i = j + (2j_1-1)s, \ 0 \leq j_1 \leq 1; \\ 0, & \text{otherwise.} \end{cases}$$

If  $5s \leq j < 6s$ , then

$$(d_{12})_{ij} = \begin{cases} e_{8(j+m)+7} \otimes w_{8j+2 \rightarrow 8(j+1)}, & i = 2s + (j+1)s; \\ (-1 + 2f(j_1, 0)) w_{8(j+m)+3+2j_1-3f(j_1,2) \rightarrow 8(j+m)+7} \otimes w_{8j+2 \rightarrow 8j+2+f(j_1,2)}, & i = j + (j_1-1)s, \ 0 \leq j_1 \leq 2; \\ 0, & \text{otherwise.} \end{cases}$$

If  $6s \leq j < 7s$ , then

$$(d_{12})_{ij} = \begin{cases} e_{8(j+m)+7} \otimes w_{8j+3 \rightarrow 8(j+1)}, & i = (j+1)s; \\ -e_{8(j+m)+7} \otimes w_{8j+3 \rightarrow 8(j+1)}, & i = 2s + (j+1)s; \\ (1 - 2f(j_1, 1, 2)) w_{8(j+m)+4+2j_1-3f(j_1,2)-9f(j_1,3) \rightarrow 8(j+m)+7} \otimes w_{8j+3 \rightarrow 8j+3+f(j_1,2,3)}, & i = j + j_1s, \ 0 \leq j_1 \leq 3; \\ e_{8(j+m)+7} \otimes w_{8j+3 \rightarrow 8j+7}, & i = j + 10s; \\ 0, & \text{otherwise.} \end{cases}$$



If  $7s \leq j < 8s$ , then

$$(d_{12})_{ij} = \begin{cases} (1 - 2f(j_1, 0))w_{8(j+m)+7+f(j_1,1) \rightarrow 8(j+m+1)} \otimes w_{8j+3 \rightarrow 8(j+1)}, \\ \quad i = j_1s + (j+1)s, \quad 0 \leq j_1 \leq 2; \\ (1 - 2f(j_1, 2))w_{8(j+m)+6-j_1-3f(j_1,2) \rightarrow 8(j+m+1)} \otimes w_{8j+3 \rightarrow 8j+4-f(j_1,0)}, \\ \quad i = j + j_1s, \quad 0 \leq j_1 \leq 2; \\ -w_{8(j+m)+7+j_1 \rightarrow 8(j+m+1)} \otimes w_{8j+3 \rightarrow 8j+7}, \quad i = j + (9+j_1)s, \quad 0 \leq j_1 \leq 1; \\ 0, \quad \text{otherwise.} \end{cases}$$

If  $8s \leq j < 9s$ , then

$$(d_{12})_{ij} = \begin{cases} w_{8(j+m)+7 \rightarrow 8(j+m+1)} \otimes w_{8j+4 \rightarrow 8(j+1)}, \quad i = 2s + (j+1)s; \\ (-1)^{j_1}w_{8(j+m)+5-4j_1 \rightarrow 8(j+m+1)} \otimes e_{8j+4}, \quad i = j + j_1s, \quad 0 \leq j_1 \leq 1; \\ (-1 + 2f(j_1, 2))w_{8(j+m+1)-f(j_1,0) \rightarrow 8(j+m+1)} \otimes w_{8j+4 \rightarrow 8j+7}, \\ \quad i = j + (8+j_1)s, \quad 0 \leq j_1 \leq 2; \\ 0, \quad \text{otherwise.} \end{cases}$$

If  $9s \leq j < 10s$ , then

$$(d_{12})_{ij} = \begin{cases} -e_{8(j+m)+7} \otimes w_{8j+5 \rightarrow 8(j+1)}, \quad i = (j+1)s; \\ (-1 + 2f(j_1, 0))w_{8(j+m)+2+4j_1-5f(j_1,2) \rightarrow 8(j+m)+7} \otimes e_{8j+5}, \quad i = j + (j_1+1)s, \quad 0 \leq j_1 \leq 2; \\ 0, \quad \text{otherwise.} \end{cases}$$

If  $10s \leq j < 11s$ , then

$$(d_{12})_{ij} = \begin{cases} (-1)^{j_1}w_{8(j+m)+7+j_1 \rightarrow 8(j+m+1)} \otimes w_{8j+5 \rightarrow 8(j+1)}, \quad i = j_1s + (j+1)s, \quad 0 \leq j_1 \leq 1; \\ (-1)^{j_1}w_{8(j+m)+6+2f(j_1,2) \rightarrow 8(j+m+1)} \otimes w_{8j+5 \rightarrow 8j+5+j_1}, \\ \quad i = j + (1+2j_1+3f(j_1,2))s, \quad 0 \leq j_1 \leq 2; \\ 0, \quad \text{otherwise.} \end{cases}$$

If  $11s \leq j < 12s$ , then

$$(d_{12})_{ij} = \begin{cases} (-1 + 2f(j_1, 0))w_{8(j+m)+1+2j_1+5f(j_1,0)-4f(j_1,2) \rightarrow 8(j+m)+7} \otimes w_{8j+6 \rightarrow 8j+6+f(j_1,3)}, \\ \quad i = j + (2+j_1)s, \quad 0 \leq j_1 \leq 3; \\ 0, \quad \text{otherwise.} \end{cases}$$

If  $12s \leq j < 13s$ , then

$$(d_{12})_{ij} = \begin{cases} w_{8(j+m)+3 \rightarrow 8(j+m+1)} \otimes e_{8j+6}, \quad i = j + 2s; \\ -e_{8(j+m+1)} \otimes w_{8j+6 \rightarrow 8j+7}, \quad i = j + 5s; \\ 0, \quad \text{otherwise.} \end{cases}$$

If  $13s \leq j < 14s$ , then

$$(d_{12})_{ij} = \begin{cases} e_{8(j+m+1)+2} \otimes w_{8j+7 \rightarrow 8(j+1)+1}, \quad i = 3s + (j+1)s; \\ w_{8(j+m)+7+j_1 \rightarrow 8(j+m+1)+2} \otimes e_{8j+7}, \quad i = j + (3+j_1)s, \quad 0 \leq j_1 \leq 1; \\ 0, \quad \text{otherwise.} \end{cases}$$

If  $14s \leq j < 15s$ , then

$$(d_{12})_{ij} = \begin{cases} (-1)^{j_1} w_{8(j+m+1)-j_1 \rightarrow 8(j+m+1)+6} \otimes w_{8j+7 \rightarrow 8(j+1)}, \\ \quad i = (j_1 + 1)s + (j + 1)_s, \quad 0 \leq j_1 \leq 1; \\ w_{8(j+m+1)+5 \rightarrow 8(j+m+1)+6} \otimes w_{8j+7 \rightarrow 8(j+1)+4}, \quad i = 8s + (j + 1)_s; \\ -e_{8(j+m+1)+6} \otimes w_{8j+7 \rightarrow 8(j+1)+5}, \quad i = 11s + (j + 1)_s; \\ w_{8(j+m)+7 \rightarrow 8(j+m+1)+6} \otimes e_{8j+7}, \quad i = j + 2s; \\ -w_{8(j+m+1) \rightarrow 8(j+m+1)+6} \otimes e_{8j+7}, \quad i = j + 4s; \\ 0, \quad \text{otherwise.} \end{cases}$$

If  $15s \leq j < 16s$ , then

$$(d_{12})_{ij} = \begin{cases} (-1)^{j_1} w_{8(j+m+1)+3+j_1 \rightarrow 8(j+m+1)+4} \otimes w_{8j+7 \rightarrow 8(j+1)+2+j_1}, \\ \quad i = (4 + 2j_1)s + (j + 1)_s, \quad 0 \leq j_1 \leq 1; \\ w_{8(j+m+1) \rightarrow 8(j+m+1)+4} \otimes e_{8j+7}, \quad i = j + 2s; \\ 0, \quad \text{otherwise.} \end{cases}$$

If  $16s \leq j < 17s$ , then

$$(d_{12})_{ij} = \begin{cases} (-1)^{j_1} w_{8(j+m)+7+j_1 \rightarrow 8(j+m+1)+1} \otimes w_{8j+7 \rightarrow 8(j+1)}, \quad i = j_1s + (j + 1)_s, \quad 0 \leq j_1 \leq 1; \\ -e_{8(j+m+1)+1} \otimes w_{8j+7 \rightarrow 8(j+1)+4}, \quad i = 9s + (j + 1)_s; \\ e_{8(j+m+1)+1} \otimes w_{8j+7 \rightarrow 8(j+1)+6}, \quad i = 15s + (j + 1)_s; \\ w_{8(j+m+1) \rightarrow 8(j+m+1)+1} \otimes e_{8j+7}, \quad i = j + 2s; \\ 0, \quad \text{otherwise.} \end{cases}$$

If  $17s \leq j < 18s$ , then

$$(d_{12})_{ij} = \begin{cases} e_{8(j+m+1)+5} \otimes w_{8j+7 \rightarrow 8(j+1)+2}, \quad i = 5s + (j + 1)_s; \\ w_{8(j+m+1) \rightarrow 8(j+m+1)+5} \otimes e_{8j+7}, \quad i = j; \\ 0, \quad \text{otherwise.} \end{cases}$$

### Description of $d_{13}$

$d_{13} : Q_{14} \rightarrow Q_{13}$  - is an  $(18s \times 20s)$  matrix.

If  $0 \leq j < s$ , then

$$(d_{13})_{ij} = \begin{cases} (1 - 2f(j_1, 1))w_{8(j+m)+2+j_1+2f(j_1, 2) \rightarrow 8(j+m)+7} \otimes e_{8j}, \quad i = j + j_1s, \quad 0 \leq j_1 \leq 3; \\ e_{8(j+m)+7} \otimes w_{8j \rightarrow 8j+2+j_1+f(j_1, 2, 3)}, \quad i = j + (5 + j_1 + 2f(j_1, 2) + 3f(j_1, 3))s, \quad 0 \leq j_1 \leq 3; \\ 0, \quad \text{otherwise.} \end{cases}$$

If  $s \leq j < 2s$ , then

$$(d_{13})_{ij} = \begin{cases} w_{8(j+m)+3 \rightarrow 8(j+m+1)} \otimes e_{8j}, \quad i = j; \\ (-1 + 2f(j_1, 0))w_{8(j+m+1)-f(j_1, 1, 2) \rightarrow 8(j+m+1)} \otimes w_{8j \rightarrow 8j+1+j_1-f(j_1, 3)}, \\ \quad i = j + (3 + j_1)s, \quad 0 \leq j_1 \leq 3; \\ e_{8(j+m+1)} \otimes w_{8j \rightarrow 8j+6}, \quad i = j + 11s; \\ 0, \quad \text{otherwise.} \end{cases}$$

If  $2s \leq j < 3s$ , then

$$(d_{13})_{ij} = \begin{cases} w_{8(j+m)+6 \rightarrow 8(j+m+1)} \otimes e_{8j}, & i = j; \\ -e_{8(j+m+1)} \otimes w_{8j \rightarrow 8j+3}, & i = j + 5s; \\ e_{8(j+m+1)} \otimes w_{8j \rightarrow 8j+4}, & i = j + 6s; \\ -e_{8(j+m+1)} \otimes w_{8j \rightarrow 8j+5}, & i = j + 8s; \\ 0, & \text{otherwise.} \end{cases}$$

If  $3s \leq j < 4s$ , then

$$(d_{13})_{ij} = \begin{cases} w_{8(j+m+1)+2 \rightarrow 8(j+m+1)+3} \otimes w_{8j+1 \rightarrow 8(j+1)}, & i = (j+1)_s; \\ -e_{8(j+m+1)+3} \otimes w_{8j+1 \rightarrow 8(j+1)}, & i = s + (j+1)_s; \\ w_{8(j+m+1) \rightarrow 8(j+m+1)+3} \otimes e_{8j+1}, & i = j + s; \\ 0, & \text{otherwise.} \end{cases}$$

If  $4s \leq j < 5s$ , then

$$(d_{13})_{ij} = \begin{cases} -e_{8(j+m+1)+5} \otimes w_{8j+1 \rightarrow 8(j+1)}, & i = 3s + (j+1)_s; \\ w_{8(j+m+1) \rightarrow 8(j+m+1)+5} \otimes e_{8j+1}, & i = j; \\ -w_{8(j+m)+7 \rightarrow 8(j+m+1)+5} \otimes w_{8j+1 \rightarrow 8j+2}, & i = j + s; \\ 0, & \text{otherwise.} \end{cases}$$

If  $5s \leq j < 6s$ , then

$$(d_{13})_{ij} = \begin{cases} w_{8(j+m+1)+2 \rightarrow 8(j+m+1)+4} \otimes w_{8j+2 \rightarrow 8(j+1)}, & i = (j+1)_s; \\ -w_{8(j+m+1)+3 \rightarrow 8(j+m+1)+4} \otimes w_{8j+2 \rightarrow 8(j+1)}, & i = s + (j+1)_s; \\ w_{8(j+m)+7+f(j_1,2) \rightarrow 8(j+m+1)+4} \otimes w_{8j+2 \rightarrow 8j+3-f(j_1,0)}, & i = j + j_1s, \ 0 \leq j_1 \leq 2; \\ e_{8(j+m+1)+4} \otimes w_{8j+2 \rightarrow 8j+7}, & i = j + 10s; \\ 0, & \text{otherwise.} \end{cases}$$

If  $6s \leq j < 7s$ , then

$$(d_{13})_{ij} = \begin{cases} -e_{8(j+m+1)+6} \otimes w_{8j+2 \rightarrow 8(j+1)}, & i = 2s + (j+1)_s; \\ w_{8(j+m)+7 \rightarrow 8(j+m+1)+6} \otimes e_{8j+2}, & i = j - s; \\ 0, & \text{otherwise.} \end{cases}$$

If  $7s \leq j < 8s$ , then

$$(d_{13})_{ij} = \begin{cases} -e_{8(j+m+1)+5} \otimes w_{8j+3 \rightarrow 8(j+1)}, & i = 3s + (j+1)_s; \\ w_{8(j+m)+7 \rightarrow 8(j+m+1)+5} \otimes e_{8j+3}, & i = j - s; \\ w_{8(j+m+1) \rightarrow 8(j+m+1)+5} \otimes e_{8j+3}, & i = j; \\ e_{8(j+m+1)+5} \otimes w_{8j+3 \rightarrow 8j+7}, & i = j + 10s; \\ 0, & \text{otherwise.} \end{cases}$$

If  $8s \leq j < 9s$ , then

$$(d_{13})_{ij} = \begin{cases} w_{8(j+m+1) \rightarrow 8(j+m+1)+1} \otimes e_{8j+3}, & i = j - s; \\ -w_{8(j+m+1) \rightarrow 8(j+m+1)+1} \otimes w_{8j+3 \rightarrow 8j+4}, & i = j; \\ e_{8(j+m+1)+1} \otimes w_{8j+3 \rightarrow 8j+7}, & i = j + 8s; \\ 0, & \text{otherwise.} \end{cases}$$

If  $9s \leq j < 10s$ , then

$$(d_{13})_{ij} = \begin{cases} e_{8(j+m+1)+2} \otimes w_{8j+4 \rightarrow 8(j+1)}, & i = (j+1)_s; \\ w_{8(j+m+1) \rightarrow 8(j+m+1)+2} \otimes e_{8j+4}, & i = j - s; \\ e_{8(j+m+1)+2} \otimes w_{8j+4 \rightarrow 8j+7}, & i = j + 4s; \\ -w_{8(j+m+1)+1 \rightarrow 8(j+m+1)+2} \otimes w_{8j+4 \rightarrow 8j+7}, & i = j + 7s; \\ 0, & \text{otherwise.} \end{cases}$$

If  $10s \leq j < 11s$ , then

$$(d_{13})_{ij} = \begin{cases} -w_{8(j+m+1)+5 \rightarrow 8(j+m+1)+6} \otimes w_{8j+4 \rightarrow 8(j+1)}, & i = 3s + (j+1)_s; \\ w_{8(j+m+1) \rightarrow 8(j+m+1)+6} \otimes e_{8j+4}, & i = j - 2s; \\ e_{8(j+m+1)+6} \otimes w_{8j+4 \rightarrow 8j+7}, & i = j + 4s; \\ w_{8(j+m+1)+5 \rightarrow 8(j+m+1)+6} \otimes w_{8j+4 \rightarrow 8j+7}, & i = j + 7s; \\ 0, & \text{otherwise.} \end{cases}$$

If  $11s \leq j < 12s$ , then

$$(d_{13})_{ij} = \begin{cases} e_{8(j+m+1)+6} \otimes w_{8j+5 \rightarrow 8(j+1)}, & i = 2s + (j+1)_s; \\ w_{8(j+m)+7 \rightarrow 8(j+m+1)+6} \otimes w_{8j+5 \rightarrow 8j+5+f(j_1,2)}, & i = j + (j_1 - 2)s, \ 0 \leq j_1 \leq 2; \\ e_{8(j+m+1)+6} \otimes w_{8j+5 \rightarrow 8j+7}, & i = j + 3s; \\ 0, & \text{otherwise.} \end{cases}$$

If  $12s \leq j < 13s$ , then

$$(d_{13})_{ij} = \begin{cases} e_{8(j+m+1)+3} \otimes w_{8j+5 \rightarrow 8(j+1)}, & i = s + (j+1)_s; \\ w_{8(j+m)+7 \rightarrow 8(j+m+1)+3} \otimes e_{8j+5}, & i = j - 3s; \\ 0, & \text{otherwise.} \end{cases}$$

If  $13s \leq j < 14s$ , then

$$(d_{13})_{ij} = \begin{cases} w_{8(j+m+1) \rightarrow 8(j+m+1)+1} \otimes e_{8j+5}, & i = j - 3s; \\ -e_{8(j+m+1)+1} \otimes w_{8j+5 \rightarrow 8j+7}, & i = j + 3s; \\ 0, & \text{otherwise.} \end{cases}$$

If  $14s \leq j < 15s$ , then

$$(d_{13})_{ij} = \begin{cases} w_{8(j+m)+7 \rightarrow 8(j+m+1)+2} \otimes e_{8j+6}, & i = j - 3s; \\ w_{8(j+m+1) \rightarrow 8(j+m+1)+2} \otimes e_{8j+6}, & i = j - 2s; \\ e_{8(j+m+1)+2} \otimes w_{8j+6 \rightarrow 8j+7}, & i = j - s; \\ 0, & \text{otherwise.} \end{cases}$$

If  $15s \leq j < 16s$ , then

$$(d_{13})_{ij} = \begin{cases} w_{8(j+m+1) \rightarrow 8(j+m+1)+4} \otimes e_{8j+6}, & i = j - 3s; \\ e_{8(j+m+1)+4} \otimes w_{8j+6 \rightarrow 8j+7}, & i = j; \\ 0, & \text{otherwise.} \end{cases}$$

If  $16s \leq j < 17s$ , then

$$(d_{13})_{ij} = \begin{cases} w_{8(j+m+1) \rightarrow 8(j+m+1)+5} \otimes e_{8j+6}, & i = j - 4s; \\ e_{8(j+m+1)+5} \otimes w_{8j+6 \rightarrow 8j+7}, & i = j + s; \\ 0, & \text{otherwise.} \end{cases}$$

If  $17s \leq j < 18s$ , then

$$(d_{13})_{ij} = \begin{cases} w_{8(j+m+1)+2 \rightarrow 8(j+m+1)+7} \otimes w_{8j+7 \rightarrow 8(j+1)}, & i = (j+1)_s; \\ w_{8(j+m+1)+5 \rightarrow 8(j+m+1)+7} \otimes w_{8j+7 \rightarrow 8(j+1)}, & i = 3s + (j+1)_s; \\ e_{8(j+m+1)+7} \otimes w_{8j+7 \rightarrow 8(j+1)+5}, & i = 9s + (j+1)_s; \\ w_{8(j+m+1)+2 \rightarrow 8(j+m+1)+7} \otimes e_{8j+7}, & i = j - 4s; \\ -w_{8(j+m+1)+6 \rightarrow 8(j+m+1)+7} \otimes e_{8j+7}, & i = j - 3s; \\ -w_{8(j+m+1)+1 \rightarrow 8(j+m+1)+7} \otimes e_{8j+7}, & i = j - s; \\ -w_{8(j+m+1)+5 \rightarrow 8(j+m+1)+7} \otimes e_{8j+7}, & i = j; \\ 0, & \text{otherwise.} \end{cases}$$

If  $18s \leq j < 19s$ , then

$$(d_{13})_{ij} = \begin{cases} -e_{8(j+m+2)} \otimes w_{8j+7 \rightarrow 8(j+1)+1}, & i = 4s + (j+1)_s; \\ w_{8(j+m+1)+7 \rightarrow 8(j+m+2)} \otimes w_{8j+7 \rightarrow 8(j+1)+2}, & i = 5s + (j+1)_s; \\ w_{8(j+m+1)+2 \rightarrow 8(j+m+2)} \otimes e_{8j+7}, & i = j - 5s; \\ -w_{8(j+m+1)+4 \rightarrow 8(j+m+2)} \otimes e_{8j+7}, & i = j - 3s; \\ 0, & \text{otherwise.} \end{cases}$$

If  $19s \leq j < 20s$ , then

$$(d_{13})_{ij} = \begin{cases} -e_{8(j+m+1)+7} \otimes w_{8j+7 \rightarrow 8(j+1)+2}, & i = 5s + (j+1)_s; \\ w_{8(j+m+1)+4 \rightarrow 8(j+m+1)+7} \otimes e_{8j+7}, & i = j - 4s; \\ -w_{8(j+m+1)+5 \rightarrow 8(j+m+1)+7} \otimes e_{8j+7}, & i = j - 2s; \\ 0, & \text{otherwise.} \end{cases}$$

### Description of $d_{14}$

$d_{14} : Q_{15} \rightarrow Q_{14}$  - is an  $(20s \times 18s)$  matrix.

If  $0 \leq j < s$ , then

$$(d_{14})_{ij} = \begin{cases} w_{8(j+m-1)+7 \rightarrow 8(j+m)+3} \otimes e_{8j}, & i = j; \\ w_{8(j+m) \rightarrow 8(j+m)+3} \otimes e_{8j}, & i = j + s; \\ -e_{8(j+m)+3} \otimes w_{8j \rightarrow 8j+1}, & i = j + 3s; \\ (1 - 2f(j_1, 2, 3))w_{8(j+m)+1+j_1-2f(j_1, 3) \rightarrow 8(j+m)+3} \otimes w_{8j \rightarrow 8j+3+j_1}, & i = j + (8 + j_1 + 2f(j_1, 2) + 3f(j_1, 3))s, \ 0 \leq j_1 \leq 3; \\ 0, & \text{otherwise.} \end{cases}$$

If  $s \leq j < 2s$ , then

$$(d_{14})_{ij} = \begin{cases} w_{8(j+m-1)+7 \rightarrow 8(j+m)+6} \otimes e_{8j}, & i = j_s; \\ -w_{8(j+m) \rightarrow 8(j+m)+6} \otimes e_{8j}, & i = j + s; \\ (-1 + 2f(j_1, 2))w_{8(j+m)+6-f(j_1, 1) \rightarrow 8(j+m)+6} \otimes w_{8j \rightarrow 8j+2+j_1}, \\ \quad i = j + (5 + j_1 + 2f(j_1, 2, 3))s, \quad 0 \leq j_1 \leq 3; \\ 0, & \text{otherwise.} \end{cases}$$

If  $2s \leq j < 3s$ , then

$$(d_{14})_{ij} = \begin{cases} w_{8(j+m) \rightarrow 8(j+m)+4} \otimes e_{8j}, & i = j - s; \\ -w_{8(j+m)+3 \rightarrow 8(j+m)+4} \otimes w_{8j \rightarrow 8j+1}, & i = j + s; \\ e_{8(j+m)+4} \otimes w_{8j \rightarrow 8j+2}, & i = j + 3s; \\ -e_{8(j+m)+4} \otimes w_{8j \rightarrow 8j+6}, & i = j + 13s; \\ 0, & \text{otherwise.} \end{cases}$$

If  $3s \leq j < 4s$ , then

$$(d_{14})_{ij} = \begin{cases} w_{8(j+m) \rightarrow 8(j+m)+1} \otimes e_{8j}, & i = j - s; \\ e_{8(j+m)+1} \otimes w_{8j \rightarrow 8j+3}, & i = j + 5s; \\ e_{8(j+m)+1} \otimes w_{8j \rightarrow 8j+5}, & i = j + 10s; \\ 0, & \text{otherwise.} \end{cases}$$

If  $4s \leq j < 5s$ , then

$$(d_{14})_{ij} = \begin{cases} w_{8(j+m) \rightarrow 8(j+m)+5} \otimes e_{8j}, & i = j - 3s; \\ -e_{8(j+m)+5} \otimes w_{8j \rightarrow 8j+1}, & i = j; \\ e_{8(j+m)+5} \otimes w_{8j \rightarrow 8j+3}, & i = j + 3s; \\ -e_{8(j+m)+5} \otimes w_{8j \rightarrow 8j+6}, & i = j + 12s; \\ 0, & \text{otherwise.} \end{cases}$$

If  $5s \leq j < 6s$ , then

$$(d_{14})_{ij} = \begin{cases} -e_{8(j+m)+7} \otimes w_{8j+1 \rightarrow 8(j+1)}, & i = (j+1)_s; \\ w_{8(j+m)+3 \rightarrow 8(j+m)+7} \otimes e_{8j+1}, & i = j - 2s; \\ -w_{8(j+m)+5 \rightarrow 8(j+m)+7} \otimes e_{8j+1}, & i = j - s; \\ -w_{8(j+m)+6 \rightarrow 8(j+m)+7} \otimes w_{8j+1 \rightarrow 8j+2}, & i = j + s; \\ 0, & \text{otherwise.} \end{cases}$$

If  $6s \leq j < 7s$ , then

$$(d_{14})_{ij} = \begin{cases} -e_{8(j+m)+7} \otimes w_{8j+2 \rightarrow 8(j+1)}, & i = (j+1)_s; \\ w_{8(j+m)+4 \rightarrow 8(j+m)+7} \otimes e_{8j+2}, & i = j - s; \\ -w_{8(j+m)+6 \rightarrow 8(j+m)+7} \otimes e_{8j+2}, & i = j; \\ -w_{8(j+m)+5 \rightarrow 8(j+m)+7} \otimes w_{8j+2 \rightarrow 8j+3}, & i = j + s; \\ -e_{8(j+m)+7} \otimes w_{8j+2 \rightarrow 8j+7}, & i = j + 13s; \\ 0, & \text{otherwise.} \end{cases}$$

If  $7s \leq j < 8s$ , then

$$(d_{14})_{ij} = \begin{cases} e_{8(j+m+1)} \otimes w_{8j+2 \rightarrow 8(j+1)}, & i = 2s + (j+1)s; \\ w_{8(j+m)+6 \rightarrow 8(j+m+1)} \otimes e_{8j+2}, & i = j - s; \\ 0, & \text{otherwise.} \end{cases}$$

If  $8s \leq j < 9s$ , then

$$(d_{14})_{ij} = \begin{cases} (1 - 2f(j_1, 2))w_{8(j+m+1)-f(j_1,0) \rightarrow 8(j+m+1)} \otimes w_{8j+3 \rightarrow 8(j+1)}, \\ \quad i = j_1s + (j+1)s, \quad 0 \leq j_1 \leq 2; \\ (-1 + 2f(j_1, 0))w_{8(j+m)+j_1+5f(j_1,0) \rightarrow 8(j+m+1)} \otimes w_{8j+3 \rightarrow 8j+3+f(j_1,2)}, \\ \quad i = j + (j_1 - 1)s, \quad 0 \leq j_1 \leq 2; \\ e_{8(j+m+1)} \otimes w_{8j+3 \rightarrow 8j+7}, \quad i = j + 10s; \\ w_{8(j+m)+7 \rightarrow 8(j+m+1)} \otimes w_{8j+3 \rightarrow 8j+7}, \quad i = j + 11s; \\ 0, & \text{otherwise.} \end{cases}$$

If  $9s \leq j < 10s$ , then

$$(d_{14})_{ij} = \begin{cases} w_{8(j+m)+2 \rightarrow 8(j+m)+7} \otimes e_{8j+4}, & i = j; \\ -w_{8(j+m)+6 \rightarrow 8(j+m)+7} \otimes e_{8j+4}, & i = j + s; \\ -e_{8(j+m)+7} \otimes w_{8j+4 \rightarrow 8j+7}, & i = j + 8s; \\ 0, & \text{otherwise.} \end{cases}$$

If  $10s \leq j < 11s$ , then

$$(d_{14})_{ij} = \begin{cases} -e_{8(j+m)+7} \otimes w_{8j+5 \rightarrow 8(j+1)}, & i = (j+1)s; \\ (-1 + 2f(j_1, 1))w_{8(j+m)+j_1-2+7f(j_1,1)+3f(j_1,2) \rightarrow 8(j+m)+7} \otimes w_{8j+5 \rightarrow 8j+5+f(j_1,4)}, \\ \quad i = j + j_1s, \quad 1 \leq j_1 \leq 4; \\ w_{8(j+m)+5 \rightarrow 8(j+m)+7} \otimes w_{8j+5 \rightarrow 8j+6}, & i = j + 6s; \\ e_{8(j+m)+7} \otimes w_{8j+5 \rightarrow 8j+7}, & i = j + 7s; \\ 0, & \text{otherwise.} \end{cases}$$

If  $11s \leq j < 12s$ , then

$$(d_{14})_{ij} = \begin{cases} -e_{8(j+m+1)} \otimes w_{8j+5 \rightarrow 8(j+1)}, & i = s + (j+1)s; \\ w_{8(j+m)+3 \rightarrow 8(j+m+1)} \otimes e_{8j+5}, & i = j + s; \\ 0, & \text{otherwise.} \end{cases}$$

If  $12s \leq j < 13s$ , then

$$(d_{14})_{ij} = \begin{cases} w_{8(j+m)+2 \rightarrow 8(j+m+1)} \otimes e_{8j+6}, & i = j + 2s; \\ -w_{8(j+m)+4 \rightarrow 8(j+m+1)} \otimes e_{8j+6}, & i = j + 3s; \\ -e_{8(j+m+1)} \otimes w_{8j+6 \rightarrow 8j+7}, & i = j + 6s; \\ 0, & \text{otherwise.} \end{cases}$$

If  $13s \leq j < 14s$ , then

$$(d_{14})_{ij} = \begin{cases} w_{8(j+m)+4 \rightarrow 8(j+m)+7} \otimes e_{8j+6}, & i = j + 2s; \\ -w_{8(j+m)+5 \rightarrow 8(j+m)+7} \otimes e_{8j+6}, & i = j + 3s; \\ -e_{8(j+m)+7} \otimes w_{8j+6 \rightarrow 8j+7}, & i = j + 6s; \\ 0, & \text{otherwise.} \end{cases}$$

If  $14s \leq j < 15s$ , then

$$(d_{14})_{ij} = \begin{cases} -w_{8(j+m)+7 \rightarrow 8(j+m+1)+2} \otimes w_{8j+7 \rightarrow 8(j+1)}, & i = (j+1)_s; \\ -w_{8(j+m+1) \rightarrow 8(j+m+1)+2} \otimes w_{8j+7 \rightarrow 8(j+1)}, & i = s + (j+1)_s; \\ -w_{8(j+m+1)+1 \rightarrow 8(j+m+1)+2} \otimes w_{8j+7 \rightarrow 8(j+1)+3}, & i = 8s + (j+1)_s; \\ -e_{8(j+m+1)+2} \otimes w_{8j+7 \rightarrow 8(j+1)+4}, & i = 9s + (j+1)_s; \\ e_{8(j+m+1)+2} \otimes w_{8j+7 \rightarrow 8(j+1)+6}, & i = 14s + (j+1)_s; \\ (-1 + 2f(j_1, 0))w_{8(j+m)+7+f(j_1,1) \rightarrow 8(j+m+1)+2} \otimes e_{8j+7}, & i = j + (3 + j_1)s, \ 0 \leq j_1 \leq 2; \\ 0, & \text{otherwise.} \end{cases}$$

If  $15s \leq j < 16s$ , then

$$(d_{14})_{ij} = \begin{cases} -e_{8(j+m+1)+3} \otimes w_{8j+7 \rightarrow 8(j+1)+5}, & i = 12s + (j+1)_s; \\ w_{8(j+m)+7 \rightarrow 8(j+m+1)+3} \otimes e_{8j+7}, & i = j + 2s; \\ 0, & \text{otherwise.} \end{cases}$$

If  $16s \leq j < 17s$ , then

$$(d_{14})_{ij} = \begin{cases} e_{8(j+m+1)+6} \otimes w_{8j+7 \rightarrow 8(j+1)+2}, & i = 6s + (j+1)_s; \\ w_{8(j+m)+7 \rightarrow 8(j+m+1)+6} \otimes e_{8j+7}, & i = j + 3s; \\ 0, & \text{otherwise.} \end{cases}$$

If  $17s \leq j < 18s$ , then

$$(d_{14})_{ij} = \begin{cases} e_{8(j+m+1)+5} \otimes w_{8j+7 \rightarrow 8(j+1)+1}, & i = 4s + (j+1)_s; \\ w_{8(j+m+1) \rightarrow 8(j+m+1)+5} \otimes e_{8j+7}, & i = j + s; \\ 0, & \text{otherwise.} \end{cases}$$

### Description of $d_{15}$

$d_{15} : Q_{16} \rightarrow Q_{15}$  - is an  $(18s \times 19s)$  matrix.

If  $0 \leq j < s$ , then

$$(d_{15})_{ij} = \begin{cases} (-1 + 2f(j_1, 0))w_{8(j+m)+3-j_1+4f(j_1,1)+5f(j_1,3) \rightarrow 8(j+m)+7} \otimes e_{8j}, \\ \quad i = j + (j_1 + f(j_1, 2, 3))s, \ 0 \leq j_1 \leq 3; \\ e_{8(j+m)+7} \otimes w_{8j \rightarrow 8j+1}, & i = j + 5s; \\ -e_{8(j+m)+7} \otimes w_{8j \rightarrow 8j+4}, & i = j + 9s; \\ -e_{8(j+m)+7} \otimes w_{8j \rightarrow 8j+5}, & i = j + 10s; \\ 0, & \text{otherwise.} \end{cases}$$



If  $s \leq j < 2s$ , then

$$(d_{15})_{ij} = \begin{cases} w_{8(j+m)+3 \rightarrow 8(j+m+1)} \otimes e_{8j}, & i = j_s; \\ -w_{8(j+m)+4 \rightarrow 8(j+m+1)} \otimes e_{8j}, & i = j + s; \\ w_{8(j+m+1)-f(j_1,0) \rightarrow 8(j+m+1)} \otimes w_{8j \rightarrow 8j+2+f(j_1,2)}, & i = j + (5 + j_1)s, \ 0 \leq j_1 \leq 2; \\ e_{8(j+m+1)} \otimes w_{8j \rightarrow 8j+5}, & i = j + 10s; \\ e_{8(j+m+1)} \otimes w_{8j \rightarrow 8j+6}, & i = j + 11s; \\ 0, & \text{otherwise.} \end{cases}$$

If  $2s \leq j < 3s$ , then

$$(d_{15})_{ij} = \begin{cases} w_{8(j+m)+4 \rightarrow 8(j+m)+7} \otimes e_{8j}, & i = j; \\ (-1)^{j_1+1} w_{8(j+m)+7-2f(j_1,0) \rightarrow 8(j+m)+7} \otimes w_{8j \rightarrow 8j+j_1}, & i = j + (2 + j_1)s, \ 0 \leq j_1 \leq 2; \\ e_{8(j+m)+7} \otimes w_{8j \rightarrow 8j+6}, & i = j + 11s; \\ 0, & \text{otherwise.} \end{cases}$$

If  $3s \leq j < 4s$ , then

$$(d_{15})_{ij} = \begin{cases} w_{8(j+m+1)+3 \rightarrow 8(j+m+1)+4} \otimes w_{8j+1 \rightarrow 8(j+1)}, & i = (j + 1)_s; \\ -e_{8(j+m+1)+4} \otimes w_{8j+1 \rightarrow 8(j+1)}, & i = 2s + (j + 1)_s; \\ w_{8(j+m)+7 \rightarrow 8(j+m+1)+4} \otimes e_{8j+1}, & i = j + 2s; \\ 0, & \text{otherwise.} \end{cases}$$

If  $4s \leq j < 5s$ , then

$$(d_{15})_{ij} = \begin{cases} e_{8(j+m+1)+6} \otimes w_{8j+1 \rightarrow 8(j+1)}, & i = s + (j + 1)_s; \\ w_{8(j+m)+7 \rightarrow 8(j+m+1)+6} \otimes e_{8j+1}, & i = j + s; \\ w_{8(j+m+1) \rightarrow 8(j+m+1)+6} \otimes w_{8j+1 \rightarrow 8j+2}, & i = j + 3s; \\ 0, & \text{otherwise.} \end{cases}$$

If  $5s \leq j < 6s$ , then

$$(d_{15})_{ij} = \begin{cases} -e_{8(j+m+1)+5} \otimes w_{8j+2 \rightarrow 8(j+1)}, & i = 4s + (j + 1)_s; \\ w_{8(j+m+1)-f(j_1,1) \rightarrow 8(j+m+1)+5} \otimes w_{8j+2 \rightarrow 8j+2+f(j_1,3)}, & i = j + j_1s, \ 1 \leq j_1 \leq 3; \\ -e_{8(j+m+1)+5} \otimes w_{8j+2 \rightarrow 8j+7}, & i = j + 12s; \\ 0, & \text{otherwise.} \end{cases}$$

If  $6s \leq j < 7s$ , then

$$(d_{15})_{ij} = \begin{cases} -e_{8(j+m+1)+1} \otimes w_{8j+2 \rightarrow 8(j+1)}, & i = 3s + (j + 1)_s; \\ w_{8(j+m+1) \rightarrow 8(j+m+1)+1} \otimes e_{8j+2}, & i = j + s; \\ 0, & \text{otherwise.} \end{cases}$$

If  $7s \leq j < 8s$ , then

$$(d_{15})_{ij} = \begin{cases} w_{8(j+m+1)+1 \rightarrow 8(j+m+1)+2} \otimes w_{8j+3 \rightarrow 8(j+1)}, & i = 3s + (j+1)_s; \\ w_{8(j+m+1) \rightarrow 8(j+m+1)+2} \otimes e_{8j+3}, & i = j + s; \\ w_{8(j+m)+7 \rightarrow 8(j+m+1)+2} \otimes w_{8j+3 \rightarrow 8j+4}, & i = j + 2s; \\ e_{8(j+m+1)+2} \otimes w_{8j+3 \rightarrow 8j+7}, & i = j + 7s; \\ 0, & \text{otherwise.} \end{cases}$$

If  $8s \leq j < 9s$ , then

$$(d_{15})_{ij} = \begin{cases} -e_{8(j+m+1)+6} \otimes w_{8j+3 \rightarrow 8(j+1)}, & i = s + (j+1)_s; \\ -w_{8(j+m+1)+5 \rightarrow 8(j+m+1)+6} \otimes w_{8j+3 \rightarrow 8(j+1)}, & i = 4s + (j+1)_s; \\ w_{8(j+m+1) \rightarrow 8(j+m+1)+6} \otimes e_{8j+3}, & i = j; \\ -e_{8(j+m+1)+6} \otimes w_{8j+3 \rightarrow 8j+7}, & i = j + 8s; \\ -w_{8(j+m+1)+5 \rightarrow 8(j+m+1)+6} \otimes w_{8j+3 \rightarrow 8j+7}, & i = j + 9s; \\ 0, & \text{otherwise.} \end{cases}$$

If  $9s \leq j < 10s$ , then

$$(d_{15})_{ij} = \begin{cases} w_{8(j+m)+7 \rightarrow 8(j+m+1)+3} \otimes e_{8j+4}, & i = j; \\ e_{8(j+m+1)+3} \otimes w_{8j+4 \rightarrow 8j+7}, & i = j + 6s; \\ 0, & \text{otherwise.} \end{cases}$$

If  $10s \leq j < 11s$ , then

$$(d_{15})_{ij} = \begin{cases} (1 - 2f(j_1, 4))w_{8(j+m+1)-f(j_1,0)-f(j_1,3)+2f(j_1,4) \rightarrow 8(j+m+1)+2} \otimes w_{8j+5 \rightarrow 8j+4+j_1+f(j_1,0)-f(j_1,3,4)}, \\ i = j + j_1s, \ 0 \leq j_1 \leq 4; \\ 0, & \text{otherwise.} \end{cases}$$

If  $11s \leq j < 12s$ , then

$$(d_{15})_{ij} = \begin{cases} e_{8(j+m+1)+4} \otimes w_{8j+5 \rightarrow 8(j+1)}, & i = 2s + (j+1)_s; \\ w_{8(j+m+1) \rightarrow 8(j+m+1)+4} \otimes e_{8j+5}, & i = j; \\ 0, & \text{otherwise.} \end{cases}$$

If  $12s \leq j < 13s$ , then

$$(d_{15})_{ij} = \begin{cases} e_{8(j+m+1)+5} \otimes w_{8j+5 \rightarrow 8(j+1)}, & i = 4s + (j+1)_s; \\ w_{8(j+m+1) \rightarrow 8(j+m+1)+5} \otimes e_{8j+5}, & i = j - s; \\ 0, & \text{otherwise.} \end{cases}$$

If  $13s \leq j < 14s$ , then

$$(d_{15})_{ij} = \begin{cases} -e_{8(j+m+1)+3} \otimes w_{8j+6 \rightarrow 8(j+1)}, & i = (j+1)_s; \\ (1 - 2f(j_1, 2))w_{8(j+m+1)+j_1-2f(j_1,1) \rightarrow 8(j+m+1)+3} \otimes w_{8j+6 \rightarrow 8j+6+f(j_1,2,3)}, \\ i = j + (j_1 - 1)s, \ 0 \leq j_1 \leq 3; \\ 0, & \text{otherwise.} \end{cases}$$

If  $14s \leq j < 15s$ , then

$$(d_{15})_{ij} = \begin{cases} w_{8(j+m)+7 \rightarrow 8(j+m+1)+6} \otimes e_{8j+6}, & i = j - s; \\ e_{8(j+m+1)+6} \otimes w_{8j+6 \rightarrow 8j+7}, & i = j + 2s; \\ 0, & \text{otherwise.} \end{cases}$$

If  $15s \leq j < 16s$ , then

$$(d_{15})_{ij} = \begin{cases} w_{8(j+m+1) \rightarrow 8(j+m+1)+5} \otimes e_{8j+6}, & i = j - 3s; \\ e_{8(j+m+1)+5} \otimes w_{8j+6 \rightarrow 8j+7}, & i = j + 2s; \\ 0, & \text{otherwise.} \end{cases}$$

If  $16s \leq j < 17s$ , then

$$(d_{15})_{ij} = \begin{cases} w_{8(j+m+1)+3 \rightarrow 8(j+m+1)+7} \otimes w_{8j+7 \rightarrow 8(j+1)}, & i = (j+1)_s; \\ e_{8(j+m+1)+7} \otimes w_{8j+7 \rightarrow 8(j+1)+1}, & i = 5s + (j+1)_s; \\ (1 - 2f(j_1, 1))w_{8(j+m+1)+2+j_1+2f(j_1, 2) \rightarrow 8(j+m+1)+7} \otimes e_{8j+7}, & i = j + (j_1 - 2)s, \ 0 \leq j_1 \leq 3; \\ 0, & \text{otherwise.} \end{cases}$$

If  $17s \leq j < 18s$ , then

$$(d_{15})_{ij} = \begin{cases} e_{8(j+m+2)} \otimes w_{8j+7 \rightarrow 8(j+1)+5}, & i = 11s + (j+1)_s; \\ w_{8(j+m+1)+3 \rightarrow 8(j+m+2)} \otimes e_{8j+7}, & i = j - 2s; \\ 0, & \text{otherwise.} \end{cases}$$

If  $18s \leq j < 19s$ , then

$$(d_{15})_{ij} = \begin{cases} -e_{8(j+m+2)} \otimes w_{8j+7 \rightarrow 8(j+1)+2}, & i = 7s + (j+1)_s; \\ w_{8(j+m+1)+6 \rightarrow 8(j+m+2)} \otimes e_{8j+7}, & i = j - 2s; \\ 0, & \text{otherwise.} \end{cases}$$

### Description of $d_{16}$

$d_{16} : Q_{17} \rightarrow Q_{16}$  - is an  $(19s \times 18s)$  matrix.

If  $0 \leq j < s$ , then

$$(d_{16})_{ij} = \begin{cases} (-1 + 2f(j_1, 0))w_{8(j+m-1)+7+f(j_1, 1) \rightarrow 8(j+m)+2} \otimes e_{8j}, & i = j + j_1s, \ 0 \leq j_1 \leq 2; \\ w_{8(j+m)+1 \rightarrow 8(j+m)+2} \otimes w_{8j \rightarrow 8j+2}, & i = j + 6s; \\ e_{8(j+m)+2} \otimes w_{8j \rightarrow 8j+3}, & i = j + 7s; \\ e_{8(j+m)+2} \otimes w_{8j \rightarrow 8j+5}, & i = j + 10s; \\ 0, & \text{otherwise.} \end{cases}$$

If  $s \leq j < 2s$ , then

$$(d_{16})_{ij} = \begin{cases} w_{8(j+m-1)+7 \rightarrow 8(j+m)+4} \otimes e_{8j}, & i = j_s; \\ (1 - 2f(j_1, 0))w_{8(j+m)+4-j_1 \rightarrow 8(j+m)+4} \otimes w_{8j \rightarrow 8j+3+j_1-2f(j_1, 0)}, & i = j + (7 + j_1 - 5f(j_1, 0))s, \ 0 \leq j_1 \leq 2; \\ -e_{8(j+m)+4} \otimes w_{8j \rightarrow 8j+5}, & i = j + 10s; \\ -w_{8(j+m)+3 \rightarrow 8(j+m)+4} \otimes w_{8j \rightarrow 8j+6}, & i = j + 12s; \\ 0, & \text{otherwise.} \end{cases}$$

If  $2s \leq j < 3s$ , then

$$(d_{16})_{ij} = \begin{cases} (-1)^{j_1} w_{8(j+m)+6-7f(j_1,0)-f(j_1,2) \rightarrow 8(j+m)+6} \otimes w_{8j \rightarrow 8j+j_1}, \\ \quad i = j + (2j_1 - f(j_1, 2))s, \quad 0 \leq j_1 \leq 3; \\ -e_{8(j+m)+6} \otimes w_{8j \rightarrow 8j+6}, \quad i = j + 12s; \\ 0, \quad \text{otherwise.} \end{cases}$$

If  $3s \leq j < 4s$ , then

$$(d_{16})_{ij} = \begin{cases} w_{8(j+m) \rightarrow 8(j+m)+5} \otimes e_{8j}, \quad i = j - 2s; \\ -e_{8(j+m)+5} \otimes w_{8j \rightarrow 8j+2}, \quad i = j + 2s; \\ -e_{8(j+m)+5} \otimes w_{8j \rightarrow 8j+5}, \quad i = j + 9s; \\ -e_{8(j+m)+5} \otimes w_{8j \rightarrow 8j+6}, \quad i = j + 12s; \\ 0, \quad \text{otherwise.} \end{cases}$$

If  $4s \leq j < 5s$ , then

$$(d_{16})_{ij} = \begin{cases} -e_{8(j+m)+7} \otimes w_{8j+1 \rightarrow 8(j+1)}, \quad i = (j+1)_s; \\ e_{8(j+m)+7} \otimes w_{8j+1 \rightarrow 8(j+1)}, \quad i = 2s + (j+1)_s; \\ w_{8(j+m)+4 \rightarrow 8(j+m)+7} \otimes e_{8j+1}, \quad i = j - s; \\ -w_{8(j+m)+6 \rightarrow 8(j+m)+7} \otimes e_{8j+1}, \quad i = j; \\ w_{8(j+m)+1 \rightarrow 8(j+m)+7} \otimes w_{8j+1 \rightarrow 8j+2}, \quad i = j + 2s; \\ 0, \quad \text{otherwise.} \end{cases}$$

If  $5s \leq j < 6s$ , then

$$(d_{16})_{ij} = \begin{cases} (-1 + 2f(j_1, 0)) w_{8(j+m)+7+f(j_1,1) \rightarrow 8(j+m+1)} \otimes w_{8j+1 \rightarrow 8(j+1)}, \\ \quad i = j_1 s + (j+1)_s, \quad 0 \leq j_1 \leq 2; \\ w_{8(j+m)+6 \rightarrow 8(j+m+1)} \otimes e_{8j+1}, \quad i = j - s; \\ -w_{8(j+m)+1 \rightarrow 8(j+m+1)} \otimes w_{8j+1 \rightarrow 8j+2}, \quad i = j + s; \\ 0, \quad \text{otherwise.} \end{cases}$$

If  $6s \leq j < 7s$ , then

$$(d_{16})_{ij} = \begin{cases} (-1 + 2f(j_1, 0)) w_{8(j+m)+7+f(j_1,1) \rightarrow 8(j+m+1)} \otimes w_{8j+2 \rightarrow 8(j+1)}, \\ \quad i = j_1 s + (j+1)_s, \quad 0 \leq j_1 \leq 2; \\ w_{8(j+m)+5 \rightarrow 8(j+m+1)} \otimes e_{8j+2}, \quad i = j - s; \\ -w_{8(j+m)+1 \rightarrow 8(j+m+1)} \otimes e_{8j+2}, \quad i = j; \\ -w_{8(j+m)+6 \rightarrow 8(j+m+1)} \otimes w_{8j+2 \rightarrow 8j+3}, \quad i = j + 2s; \\ -e_{8(j+m+1)} \otimes w_{8j+2 \rightarrow 8j+7}, \quad i = j + 12s; \\ 0, \quad \text{otherwise.} \end{cases}$$

If  $7s \leq j < 8s$ , then

$$(d_{16})_{ij} = \begin{cases} e_{8(j+m)+7} \otimes w_{8j+3 \rightarrow 8(j+1)}, & i = (j+1)_s; \\ (-1 + 2f(j_1, 0))w_{8(j+m)+2+4f(j_1,1)+f(j_1,2) \rightarrow 8(j+m)+7} \otimes w_{8j+3 \rightarrow 8j+3+f(j_1,2)}, \\ \quad i = j + j_1s, \ 0 \leq j_1 \leq 2; \\ -e_{8(j+m)+7} \otimes w_{8j+3 \rightarrow 8j+7}, & i = j + 9s; \\ 0, & \text{otherwise.} \end{cases}$$

If  $8s \leq j < 9s$ , then

$$(d_{16})_{ij} = \begin{cases} w_{8(j+m)+3 \rightarrow 8(j+m+1)} \otimes e_{8j+4}, & i = j + s; \\ -e_{8(j+m+1)} \otimes w_{8j+4 \rightarrow 8j+7}, & i = j + 9s; \\ 0, & \text{otherwise.} \end{cases}$$

If  $9s \leq j < 10s$ , then

$$(d_{16})_{ij} = \begin{cases} -e_{8(j+m+1)} \otimes w_{8j+5 \rightarrow 8(j+1)}, & i = s + (j+1)_s; \\ w_{8(j+m)+2 \rightarrow 8(j+m+1)} \otimes e_{8j+5}, & i = j + s; \\ (-1 + 2f(j_1, 2))w_{8(j+m)+4-j_1+6f(j_1,2) \rightarrow 8(j+m+1)} \otimes w_{8j+5 \rightarrow 8j+5+j_1}, \\ \quad i = j + 2(1 + j_1 + f(j_1, 2))s, \ 0 \leq j_1 \leq 2; \\ 0, & \text{otherwise.} \end{cases}$$

If  $10s \leq j < 11s$ , then

$$(d_{16})_{ij} = \begin{cases} -e_{8(j+m)+7} \otimes w_{8j+5 \rightarrow 8(j+1)}, & i = 2s + (j+1)_s; \\ w_{8(j+m)+4 \rightarrow 8(j+m)+7} \otimes e_{8j+5}, & i = j + s; \\ -w_{8(j+m)+5 \rightarrow 8(j+m)+7} \otimes e_{8j+5}, & i = j + 2s; \\ 0, & \text{otherwise.} \end{cases}$$

If  $11s \leq j < 12s$ , then

$$(d_{16})_{ij} = \begin{cases} (1 - 2f(j_1, 1, 2))w_{8(j+m)+3+j_1+2f(j_1,1)+f(j_1,3) \rightarrow 8(j+m)+7} \otimes w_{8j+6 \rightarrow 8j+6+f(j_1,3)}, \\ \quad i = j + (2 + j_1)s, \ 0 \leq j_1 \leq 3; \\ 0, & \text{otherwise.} \end{cases}$$

If  $12s \leq j < 13s$ , then

$$(d_{16})_{ij} = \begin{cases} w_{8(j+m)+6 \rightarrow 8(j+m+1)} \otimes e_{8j+6}, & i = j + 2s; \\ -e_{8(j+m+1)} \otimes w_{8j+6 \rightarrow 8j+7}, & i = j + 6s; \\ 0, & \text{otherwise.} \end{cases}$$

If  $13s \leq j < 14s$ , then

$$(d_{16})_{ij} = \begin{cases} -w_{8(j+m+1) \rightarrow 8(j+m+1)+3} \otimes w_{8j+7 \rightarrow 8(j+1)}, & i = s + (j+1)_s; \\ -w_{8(j+m)+7 \rightarrow 8(j+m+1)+3} \otimes w_{8j+7 \rightarrow 8(j+1)}, & i = 2s + (j+1)_s; \\ (1 - 2f(j_1, 2))w_{8(j+m+1)+1+j_1 \rightarrow 8(j+m+1)+3} \otimes w_{8j+7 \rightarrow 8(j+1)+2+j_1}, \\ \quad i = (6 + j_1 + f(j_1, 2))s + (j+1)_s, & 0 \leq j_1 \leq 2; \\ e_{8(j+m+1)+3} \otimes w_{8j+7 \rightarrow 8(j+1)+6}, & i = 13s + (j+1)_s; \\ w_{8(j+m)+7 \rightarrow 8(j+m+1)+3} \otimes e_{8j+7}, & i = j + 3s; \\ w_{8(j+m+1) \rightarrow 8(j+m+1)+3} \otimes e_{8j+7}, & i = j + 4s; \\ 0, & \text{otherwise.} \end{cases}$$

If  $14s \leq j < 15s$ , then

$$(d_{16})_{ij} = \begin{cases} -e_{8(j+m+1)+6} \otimes w_{8j+7 \rightarrow 8(j+1)+1}, & i = 4s + (j+1)_s; \\ w_{8(j+m)+7 \rightarrow 8(j+m+1)+6} \otimes e_{8j+7}, & i = j + 2s; \\ -w_{8(j+m+1) \rightarrow 8(j+m+1)+6} \otimes e_{8j+7}, & i = j + 4s; \\ 0, & \text{otherwise.} \end{cases}$$

If  $15s \leq j < 16s$ , then

$$(d_{16})_{ij} = \begin{cases} -e_{8(j+m+1)+4} \otimes w_{8j+7 \rightarrow 8(j+1)+5}, & i = 11s + (j+1)_s; \\ w_{8(j+m+1) \rightarrow 8(j+m+1)+4} \otimes e_{8j+7}, & i = j + 2s; \\ 0, & \text{otherwise.} \end{cases}$$

If  $16s \leq j < 17s$ , then

$$(d_{16})_{ij} = \begin{cases} e_{8(j+m+1)+1} \otimes w_{8j+7 \rightarrow 8(j+1)+2}, & i = 6s + (j+1)_s; \\ w_{8(j+m+1) \rightarrow 8(j+m+1)+1} \otimes e_{8j+7}, & i = j + 2s; \\ 0, & \text{otherwise.} \end{cases}$$

If  $17s \leq j < 18s$ , then

$$(d_{16})_{ij} = \begin{cases} -e_{8(j+m+1)+5} \otimes w_{8j+7 \rightarrow 8(j+1)+5}, & i = 12s + (j+1)_s; \\ w_{8(j+m+1) \rightarrow 8(j+m+1)+5} \otimes e_{8j+7}, & i = j; \\ 0, & \text{otherwise.} \end{cases}$$

### Description of $d_{17}$

$d_{17} : Q_{18} \rightarrow Q_{17}$  – is an  $(18s \times 19s)$  matrix.

If  $0 \leq j < s$ , then

$$(d_{17})_{ij} = \begin{cases} (1 - 2f(j_1, 1) - 2f(j_1, 4))w_{8(j+m)+2+2j_1-3f(j_1, 3, 4) \rightarrow 8(j+m)+7} \otimes w_{8j \rightarrow 8j+f(j_1, 4)}, \\ \quad i = j + j_1s, & 0 \leq j_1 \leq 4; \\ -e_{8(j+m)+7} \otimes w_{8j \rightarrow 8j+3}, & i = j + 7s; \\ -e_{8(j+m)+7} \otimes w_{8j \rightarrow 8j+5}, & i = j + 10s; \\ -e_{8(j+m)+7} \otimes w_{8j \rightarrow 8j+6}, & i = j + 11s; \\ 0, & \text{otherwise.} \end{cases}$$

If  $s \leq j < 2s$ , then

$$(d_{17})_{ij} = \begin{cases} w_{8(j+m)+6+j_1-2f(j_1,0) \rightarrow 8(j+m+1)} \otimes w_{8j \rightarrow 8j+1-f(j_1,0)}, \\ \quad i = j + (2 + j_1 - 2f(j_1, 0))s, \quad 0 \leq j_1 \leq 2; \\ -e_{8(j+m+1)} \otimes w_{8j \rightarrow 8j+4}, \quad i = j + 7s; \\ -e_{8(j+m+1)} \otimes w_{8j \rightarrow 8j+5}, \quad i = j + 8s; \\ 0, \quad \text{otherwise.} \end{cases}$$

If  $2s \leq j < 3s$ , then

$$(d_{17})_{ij} = \begin{cases} (1 - 2f(j_1, 2))w_{8(j+m+1)-2f(j_1,0) \rightarrow 8(j+m+1)} \otimes w_{8j \rightarrow 8j+j_1}, \\ \quad i = j + (2 + j_1 - 2f(j_1, 0))s, \quad 0 \leq j_1 \leq 2; \\ e_{8(j+m+1)} \otimes w_{8j \rightarrow 8j+6}, \quad i = j + 10s; \\ 0, \quad \text{otherwise.} \end{cases}$$

If  $3s \leq j < 4s$ , then

$$(d_{17})_{ij} = \begin{cases} e_{8(j+m+1)+5} \otimes w_{8j+1 \rightarrow 8(j+1)}, \quad i = 3s + (j + 1)s; \\ w_{8(j+m)+7 \rightarrow 8(j+m+1)+5} \otimes e_{8j+1}, \quad i = j + s; \\ w_{8(j+m+1) \rightarrow 8(j+m+1)+5} \otimes e_{8j+1}, \quad i = j + 2s; \\ 0, \quad \text{otherwise.} \end{cases}$$

If  $4s \leq j < 5s$ , then

$$(d_{17})_{ij} = \begin{cases} w_{8(j+m+1) \rightarrow 8(j+m+1)+1} \otimes e_{8j+1}, \quad i = j + s; \\ -w_{8(j+m+1) \rightarrow 8(j+m+1)+1} \otimes w_{8j+1 \rightarrow 8j+2}, \quad i = j + 2s; \\ -e_{8(j+m+1)+1} \otimes w_{8j+1 \rightarrow 8j+7}, \quad i = j + 12s; \\ 0, \quad \text{otherwise.} \end{cases}$$

If  $5s \leq j < 6s$ , then

$$(d_{17})_{ij} = \begin{cases} -e_{8(j+m+1)+2} \otimes w_{8j+2 \rightarrow 8(j+1)}, \quad i = (j + 1)s; \\ w_{8(j+m+1) \rightarrow 8(j+m+1)+2} \otimes e_{8j+2}, \quad i = j + s; \\ w_{8(j+m+1)+1 \rightarrow 8(j+m+1)+2} \otimes w_{8j+2 \rightarrow 8j+7}, \quad i = j + 11s; \\ 0, \quad \text{otherwise.} \end{cases}$$

If  $6s \leq j < 7s$ , then

$$(d_{17})_{ij} = \begin{cases} e_{8(j+m+1)+6} \otimes w_{8j+2 \rightarrow 8(j+1)}, \quad i = 2s + (j + 1)s; \\ w_{8(j+m+1)+5 \rightarrow 8(j+m+1)+6} \otimes w_{8j+2 \rightarrow 8(j+1)}, \quad i = 3s + (j + 1)s; \\ w_{8(j+m+1) \rightarrow 8(j+m+1)+6} \otimes e_{8j+2}, \quad i = j; \\ -w_{8(j+m)+7 \rightarrow 8(j+m+1)+6} \otimes w_{8j+2 \rightarrow 8j+3}, \quad i = j + s; \\ -e_{8(j+m+1)+6} \otimes w_{8j+2 \rightarrow 8j+7}, \quad i = j + 8s; \\ 0, \quad \text{otherwise.} \end{cases}$$

If  $7s \leq j < 8s$ , then

$$(d_{17})_{ij} = \begin{cases} -w_{8(j+m+1)+2 \rightarrow 8(j+m+1)+3} \otimes w_{8j+3 \rightarrow 8(j+1)}, & i = (j+1)_s; \\ w_{8(j+m)+7 \rightarrow 8(j+m+1)+3} \otimes e_{8j+3}, & i = j; \\ w_{8(j+m+1) \rightarrow 8(j+m+1)+3} \otimes w_{8j+3 \rightarrow 8j+4}, & i = j+s; \\ e_{8(j+m+1)+3} \otimes w_{8j+3 \rightarrow 8j+7}, & i = j+6s; \\ 0, & \text{otherwise.} \end{cases}$$

If  $8s \leq j < 9s$ , then

$$(d_{17})_{ij} = \begin{cases} w_{8(j+m+1) \rightarrow 8(j+m+1)+4} \otimes e_{8j+4}, & i = j; \\ e_{8(j+m+1)+4} \otimes w_{8j+4 \rightarrow 8j+7}, & i = j+7s; \\ 0, & \text{otherwise.} \end{cases}$$

If  $9s \leq j < 10s$ , then

$$(d_{17})_{ij} = \begin{cases} w_{8(j+m+1) \rightarrow 8(j+m+1)+5} \otimes e_{8j+4}, & i = j-s; \\ e_{8(j+m+1)+5} \otimes w_{8j+4 \rightarrow 8j+7}, & i = j+8s; \\ 0, & \text{otherwise.} \end{cases}$$

If  $10s \leq j < 11s$ , then

$$(d_{17})_{ij} = \begin{cases} w_{8(j+m)+7+f(j_1,0) \rightarrow 8(j+m+1)+3} \otimes w_{8j+5 \rightarrow 8j+5+f(j_1,2)}, & i = j + (j_1 - 1)s, \ 0 \leq j_1 \leq 2; \\ -e_{8(j+m+1)+3} \otimes w_{8j+5 \rightarrow 8j+7}, & i = j+3s; \\ 0, & \text{otherwise.} \end{cases}$$

If  $11s \leq j < 12s$ , then

$$(d_{17})_{ij} = \begin{cases} e_{8(j+m+1)+6} \otimes w_{8j+5 \rightarrow 8(j+1)}, & i = 2s + (j+1)_s; \\ w_{8(j+m)+7 \rightarrow 8(j+m+1)+6} \otimes e_{8j+5}, & i = j-s; \\ 0, & \text{otherwise.} \end{cases}$$

If  $12s \leq j < 13s$ , then

$$(d_{17})_{ij} = \begin{cases} e_{8(j+m+1)+5} \otimes w_{8j+5 \rightarrow 8(j+1)}, & i = 3s + (j+1)_s; \\ w_{8(j+m+1) \rightarrow 8(j+m+1)+5} \otimes e_{8j+5}, & i = j-3s; \\ -e_{8(j+m+1)+5} \otimes w_{8j+5 \rightarrow 8j+7}, & i = j+5s; \\ 0, & \text{otherwise.} \end{cases}$$

If  $13s \leq j < 14s$ , then

$$(d_{17})_{ij} = \begin{cases} w_{8(j+m)+7 \rightarrow 8(j+m+1)+6} \otimes e_{8j+6}, & i = j-2s; \\ w_{8(j+m+1) \rightarrow 8(j+m+1)+6} \otimes e_{8j+6}, & i = j-s; \\ -e_{8(j+m+1)+6} \otimes w_{8j+6 \rightarrow 8j+7}, & i = j+s; \\ 0, & \text{otherwise.} \end{cases}$$



If  $14s \leq j < 15s$ , then

$$(d_{17})_{ij} = \begin{cases} w_{8(j+m+1)+2 \rightarrow 8(j+m+1)+4} \otimes w_{8j+6 \rightarrow 8(j+1)}, & i = (j+1)_s; \\ -e_{8(j+m+1)+4} \otimes w_{8j+6 \rightarrow 8(j+1)}, & i = s + (j+1)_s; \\ w_{8(j+m)+7 \rightarrow 8(j+m+1)+4} \otimes e_{8j+6}, & i = j - 3s; \\ -w_{8(j+m+1)+3 \rightarrow 8(j+m+1)+4} \otimes w_{8j+6 \rightarrow 8j+7}, & i = j - s; \\ e_{8(j+m+1)+4} \otimes w_{8j+6 \rightarrow 8j+7}, & i = j + s; \\ 0, & \text{otherwise.} \end{cases}$$

If  $15s \leq j < 16s$ , then

$$(d_{17})_{ij} = \begin{cases} w_{8(j+m+1) \rightarrow 8(j+m+1)+1} \otimes e_{8j+6}, & i = j - 3s; \\ e_{8(j+m+1)+1} \otimes w_{8j+6 \rightarrow 8j+7}, & i = j + s; \\ 0, & \text{otherwise.} \end{cases}$$

If  $16s \leq j < 17s$ , then

$$(d_{17})_{ij} = \begin{cases} -w_{8(j+m+1)+2 \rightarrow 8(j+m+1)+7} \otimes w_{8j+7 \rightarrow 8(j+1)}, & i = (j+1)_s; \\ w_{8(j+m+1)+4 \rightarrow 8(j+m+1)+7} \otimes w_{8j+7 \rightarrow 8(j+1)}, & i = s + (j+1)_s; \\ e_{8(j+m+1)+7} \otimes w_{8j+7 \rightarrow 8(j+1)+1}, & i = 4s + (j+1)_s; \\ e_{8(j+m+1)+7} \otimes w_{8j+7 \rightarrow 8(j+1)+5}, & i = 10s + (j+1)_s; \\ (-1 + 2f(j_1, 0))w_{8(j+m+1)+3-j_1+4f(j_1,1)+5f(j_1,3) \rightarrow 8(j+m+1)+7} \otimes e_{8j+7}, & i = j + (j_1 - 3 + f(j_1, 2, 3))s, \ 0 \leq j_1 \leq 3; \\ 0, & \text{otherwise.} \end{cases}$$

If  $17s \leq j < 18s$ , then

$$(d_{17})_{ij} = \begin{cases} (1 - 2f(j_1, 0))w_{8(j+m+1)+2+2j_1+f(j_1,2) \rightarrow 8(j+m+2)} \otimes w_{8j+7 \rightarrow 8(j+1)+f(j_1,2,3)}, & i = (j_1 + 2f(j_1, 2, 3))s + (j+1)_s, \ 0 \leq j_1 \leq 3; \\ w_{8(j+m+1)+3 \rightarrow 8(j+m+2)} \otimes e_{8j+7}, & i = j - 4s; \\ -w_{8(j+m+1)+4 \rightarrow 8(j+m+2)} \otimes e_{8j+7}, & i = j - 2s; \\ 0, & \text{otherwise.} \end{cases}$$

If  $18s \leq j < 19s$ , then

$$(d_{17})_{ij} = \begin{cases} e_{8(j+m+1)+7} \otimes w_{8j+7 \rightarrow 8(j+1)+5}, & i = 10s + (j+1)_s; \\ w_{8(j+m+1)+4 \rightarrow 8(j+m+1)+7} \otimes e_{8j+7}, & i = j - 3s; \\ -w_{8(j+m+1)+5 \rightarrow 8(j+m+1)+7} \otimes e_{8j+7}, & i = j - s; \\ 0, & \text{otherwise.} \end{cases}$$

### Description of $d_{18}$

$d_{18} : Q_{19} \rightarrow Q_{18}$  - is an  $(19s \times 16s)$  matrix.

If  $0 \leq j < s$ , then

$$(d_{18})_{ij} = \begin{cases} w_{8(j+m-1)+7 \rightarrow 8(j+m)+3} \otimes e_{8j}, & i = j; \\ (1 - 2f(j_1, 1, 2))w_{8(j+m)+j_1 \rightarrow 8(j+m)+3} \otimes w_{8j \rightarrow 8j+j_1}, \\ \quad i = j + (j_1 + 3 - 2f(j_1, 0) + f(j_1, 3))s, & 0 \leq j_1 \leq 3; \\ e_{8(j+m)+3} \otimes w_{8j \rightarrow 8j+5}, & i = j + 10s; \\ 0, & \text{otherwise.} \end{cases}$$

If  $s \leq j < 2s$ , then

$$(d_{18})_{ij} = \begin{cases} w_{8(j+m-1)+7 \rightarrow 8(j+m)+6} \otimes e_{8j}, & i = j_s; \\ (-1)^{j_1+1}w_{8(j+m)+4+j_1-4f(j_1,0) \rightarrow 8(j+m)+6} \otimes w_{8j \rightarrow 8j+j_1}, \\ \quad i = j + (j_1 + 1 + 2f(j_1, 2))s, & 0 \leq j_1 \leq 2; \\ e_{8(j+m)+6} \otimes w_{8j \rightarrow 8j+5}, & i = j + 10s; \\ e_{8(j+m)+6} \otimes w_{8j \rightarrow 8j+6}, & i = j + 12s; \\ 0, & \text{otherwise.} \end{cases}$$

If  $2s \leq j < 3s$ , then

$$(d_{18})_{ij} = \begin{cases} w_{8(j+m) \rightarrow 8(j+m)+1} \otimes e_{8j}, & i = j; \\ -e_{8(j+m)+1} \otimes w_{8j \rightarrow 8j+1}, & i = j + 2s; \\ -e_{8(j+m)+1} \otimes w_{8j \rightarrow 8j+6}, & i = j + 13s; \\ 0, & \text{otherwise.} \end{cases}$$

If  $3s \leq j < 4s$ , then

$$(d_{18})_{ij} = \begin{cases} w_{8(j+m) \rightarrow 8(j+m)+5} \otimes e_{8j}, & i = j - 2s; \\ -e_{8(j+m)+5} \otimes w_{8j \rightarrow 8j+1}, & i = j; \\ e_{8(j+m)+5} \otimes w_{8j \rightarrow 8j+4}, & i = j + 6s; \\ e_{8(j+m)+5} \otimes w_{8j \rightarrow 8j+5}, & i = j + 9s; \\ 0, & \text{otherwise.} \end{cases}$$

If  $4s \leq j < 5s$ , then

$$(d_{18})_{ij} = \begin{cases} (-1 + 2f(j_1, 2))w_{8(j+m+1)-f(j_1,0) \rightarrow 8(j+m+1)} \otimes w_{8j+1 \rightarrow 8(j+1)}, \\ \quad i = j_1s + (j + 1)_s, & 0 \leq j_1 \leq 2; \\ (-1 + 2f(j_1, 0))w_{8(j+m)+j_1+5f(j_1,0) \rightarrow 8(j+m+1)} \otimes w_{8j+1 \rightarrow 8j+1+f(j_1,2)}, \\ \quad i = j + (j_1 - 1)s, & 0 \leq j_1 \leq 2; \\ 0, & \text{otherwise.} \end{cases}$$

If  $5s \leq j < 6s$ , then

$$(d_{18})_{ij} = \begin{cases} e_{8(j+m)+7} \otimes w_{8j+2 \rightarrow 8(j+1)}, & i = (j + 1)_s; \\ -w_{8(j+m)+6 \rightarrow 8(j+m)+7} \otimes e_{8j+2}, & i = j + s; \\ (-1)^{j_1}w_{8(j+m)+2+j_1+f(j_1,2) \rightarrow 8(j+m)+7} \otimes w_{8j+2 \rightarrow 8j+2+j_1}, \\ \quad i = j + 2j_1s, & 0 \leq j_1 \leq 2; \\ e_{8(j+m)+7} \otimes w_{8j+2 \rightarrow 8j+7}, & i = j + 11s; \\ 0, & \text{otherwise.} \end{cases}$$

If  $6s \leq j < 7s$ , then

$$(d_{18})_{ij} = \begin{cases} e_{8(j+m+1)} \otimes w_{8j+3 \rightarrow 8(j+1)}, & i = s + (j+1)_s; \\ w_{8(j+m)+3 \rightarrow 8(j+m+1)} \otimes e_{8j+3}, & i = j + s; \\ -w_{8(j+m)+4 \rightarrow 8(j+m+1)} \otimes w_{8j+3 \rightarrow 8j+4}, & i = j + 2s; \\ -e_{8(j+m+1)} \otimes w_{8j+3 \rightarrow 8j+7}, & i = j + 11s; \\ 0, & \text{otherwise.} \end{cases}$$

If  $7s \leq j < 8s$ , then

$$(d_{18})_{ij} = \begin{cases} w_{8(j+m)+4 \rightarrow 8(j+m)+7} \otimes e_{8j+4}, & i = j + s; \\ -w_{8(j+m)+5 \rightarrow 8(j+m)+7} \otimes e_{8j+4}, & i = j + 2s; \\ -e_{8(j+m)+7} \otimes w_{8j+4 \rightarrow 8j+7}, & i = j + 11s; \\ 0, & \text{otherwise.} \end{cases}$$

If  $8s \leq j < 9s$ , then

$$(d_{18})_{ij} = \begin{cases} e_{8(j+m)+7} \otimes w_{8j+5 \rightarrow 8(j+1)}, & i = (j+1)_s; \\ (-1 + 2f(j_1, 0))w_{8(j+m)+3+j_1+2f(j_1, 1) \rightarrow 8(j+m)+7} \otimes e_{8j+5}, & i = j + (2 + j_1)s, \ 0 \leq j_1 \leq 2; \\ -w_{8(j+m)+6 \rightarrow 8(j+m)+7} \otimes w_{8j+5 \rightarrow 8j+6}, & i = j + 5s; \\ w_{8(j+m)+1 \rightarrow 8(j+m)+7} \otimes w_{8j+5 \rightarrow 8j+6}, & i = j + 7s; \\ e_{8(j+m)+7} \otimes w_{8j+5 \rightarrow 8j+7}, & i = j + 8s; \\ 0, & \text{otherwise.} \end{cases}$$

If  $9s \leq j < 10s$ , then

$$(d_{18})_{ij} = \begin{cases} -e_{8(j+m+1)} \otimes w_{8j+5 \rightarrow 8(j+1)}, & i = 2s + (j+1)_s; \\ w_{8(j+m)+6 \rightarrow 8(j+m+1)} \otimes e_{8j+5}, & i = j + 2s; \\ 0, & \text{otherwise.} \end{cases}$$

If  $10s \leq j < 11s$ , then

$$(d_{18})_{ij} = \begin{cases} (-1 + 2f(j_1, 0))w_{8(j+m)+6-2j_1-f(j_1, 2) \rightarrow 8(j+m)+7} \otimes e_{8j+6}, & i = j + (3 + j_1)s, \ 0 \leq j_1 \leq 2; \\ -e_{8(j+m)+7} \otimes w_{8j+6 \rightarrow 8j+7}, & i = j + 6s; \\ e_{8(j+m)+7} \otimes w_{8j+6 \rightarrow 8j+7}, & i = j + 8s; \\ 0, & \text{otherwise.} \end{cases}$$

If  $11s \leq j < 12s$ , then

$$(d_{18})_{ij} = \begin{cases} w_{8(j+m)+4 \rightarrow 8(j+m+1)} \otimes e_{8j+6}, & i = j + 3s; \\ e_{8(j+m+1)} \otimes w_{8j+6 \rightarrow 8j+7}, & i = j + 6s; \\ 0, & \text{otherwise.} \end{cases}$$

If  $12s \leq j < 13s$ , then

$$(d_{18})_{ij} = \begin{cases} w_{8(j+m+1)+1 \rightarrow 8(j+m+1)+2} \otimes w_{8j+7 \rightarrow 8(j+1)+1}, & i = 4s + (j+1)_s; \\ e_{8(j+m+1)+2} \otimes w_{8j+7 \rightarrow 8(j+1)+2}, & i = 5s + (j+1)_s; \\ (-1 + 2f(j_1, 0))w_{8(j+m)+7+f(j_1, 1) \rightarrow 8(j+m+1)+2} \otimes e_{8j+7}, & i = j + (4 + j_1)s, \ 0 \leq j_1 \leq 2; \\ 0, & \text{otherwise.} \end{cases}$$

If  $13s \leq j < 14s$ , then

$$(d_{18})_{ij} = \begin{cases} w_{8(j+m)+7 \rightarrow 8(j+m+1)+4} \otimes w_{8j+7 \rightarrow 8(j+1)}, & i = (j+1)_s; \\ w_{8(j+m+1)+3 \rightarrow 8(j+m+1)+4} \otimes w_{8j+7 \rightarrow 8(j+1)+3}, & i = 7s + (j+1)_s; \\ -e_{8(j+m+1)+4} \otimes w_{8j+7 \rightarrow 8(j+1)+4}, & i = 8s + (j+1)_s; \\ e_{8(j+m+1)+4} \otimes w_{8j+7 \rightarrow 8(j+1)+6}, & i = 14s + (j+1)_s; \\ w_{8(j+m)+7 \rightarrow 8(j+m+1)+4} \otimes e_{8j+7}, & i = j + 3s; \\ 0, & \text{otherwise.} \end{cases}$$

If  $14s \leq j < 15s$ , then

$$(d_{18})_{ij} = \begin{cases} -e_{8(j+m+1)+6} \otimes w_{8j+7 \rightarrow 8(j+1)+5}, & i = 11s + (j+1)_s; \\ w_{8(j+m)+7 \rightarrow 8(j+m+1)+6} \otimes e_{8j+7}, & i = j + 4s; \\ 0, & \text{otherwise.} \end{cases}$$

If  $15s \leq j < 16s$ , then

$$(d_{18})_{ij} = \begin{cases} -e_{8(j+m+1)+5} \otimes w_{8j+7 \rightarrow 8(j+1)+1}, & i = 3s + (j+1)_s; \\ w_{8(j+m+1) \rightarrow 8(j+m+1)+5} \otimes e_{8j+7}, & i = j + 2s; \\ 0, & \text{otherwise.} \end{cases}$$

### Description of $d_{19}$

$d_{19} : Q_{20} \rightarrow Q_{19}$  is an  $(16s \times 16s)$  matrix.

If  $0 \leq j < s$ , then

$$(d_{19})_{ij} = \begin{cases} (-1 + 2f(j_1, 0))w_{8(j+m)+3-j_1+4f(j_1,1)+5f(j_1,3) \rightarrow 8(j+m)+7} \otimes e_{8j}, & i = j + j_1s, \ 0 \leq j_1 \leq 3; \\ e_{8(j+m)+7} \otimes w_{8j \rightarrow 8j+2}, & i = j + 5s; \\ -e_{8(j+m)+7} \otimes w_{8j \rightarrow 8j+5}, & i = j + 8s; \\ 0, & \text{otherwise.} \end{cases}$$

If  $s \leq j < 2s$ , then

$$(d_{19})_{ij} = \begin{cases} w_{8(j+m)+3 \rightarrow 8(j+m+1)} \otimes e_{8j}, & i = j_s; \\ -w_{8(j+m)+5 \rightarrow 8(j+m+1)} \otimes e_{8j}, & i = j + 2s; \\ -e_{8(j+m+1)} \otimes w_{8j \rightarrow 8j+1}, & i = j + 3s; \\ -w_{8(j+m+1)-f(j_1,1,2)-f(j_1,4) \rightarrow 8(j+m+1)} \otimes w_{8j \rightarrow 8j+3+j_1-f(j_1,3,4)-2f(j_1,5)}, & i = j + (5 + j_1)s, \ 0 \leq j_1 \leq 5; \\ 0, & \text{otherwise.} \end{cases}$$

If  $2s \leq j < 3s$ , then

$$(d_{19})_{ij} = \begin{cases} -w_{8(j+m+1)+1 \rightarrow 8(j+m+1)+2} \otimes w_{8j+1 \rightarrow 8(j+1)}, & i = 2s + (j+1)_s; \\ w_{8(j+m+1)-f(j_1,1)-f(j_1,3) \rightarrow 8(j+m+1)+2} \otimes w_{8j+1 \rightarrow 8j+1+j_1}, & i = j + (2 + j_1)s, \ 0 \leq j_1 \leq 3; \\ -e_{8(j+m+1)+2} \otimes w_{8j+1 \rightarrow 8j+7}, & i = j + 10s; \\ 0, & \text{otherwise.} \end{cases}$$

If  $3s \leq j < 4s$ , then

$$(d_{19})_{ij} = \begin{cases} e_{8(j+m+1)+6} \otimes w_{8j+1 \rightarrow 8(j+1)}, & i = s + (j+1)_s; \\ w_{8(j+m+1)+5 \rightarrow 8(j+m+1)+6} \otimes w_{8j+1 \rightarrow 8(j+1)}, & i = 3s + (j+1)_s; \\ w_{8(j+m+1) \rightarrow 8(j+m+1)+6} \otimes e_{8j+1}, & i = j + s; \\ 0, & \text{otherwise.} \end{cases}$$

If  $4s \leq j < 5s$ , then

$$(d_{19})_{ij} = \begin{cases} -e_{8(j+m+1)+3} \otimes w_{8j+2 \rightarrow 8(j+1)}, & i = (j+1)_s; \\ w_{8(j+m)+7+f(j_1,1) \rightarrow 8(j+m+1)+3} \otimes w_{8j+2 \rightarrow 8j+2+j_1}, & i = j + (j_1+1)s, \ 0 \leq j_1 \leq 2; \\ -w_{8(j+m+1)+2 \rightarrow 8(j+m+1)+3} \otimes w_{8j+2 \rightarrow 8j+7}, & i = j + 8s; \\ 0, & \text{otherwise.} \end{cases}$$

If  $5s \leq j < 6s$ , then

$$(d_{19})_{ij} = \begin{cases} -w_{8(j+m+1)+3 \rightarrow 8(j+m+1)+4} \otimes w_{8j+3 \rightarrow 8(j+1)}, & i = (j+1)_s; \\ w_{8(j+m+1) \rightarrow 8(j+m+1)+4} \otimes e_{8j+3}, & i = j + s; \\ w_{8(j+m)+7 \rightarrow 8(j+m+1)+4} \otimes w_{8j+3 \rightarrow 8j+4}, & i = j + 2s; \\ -w_{8(j+m+1)+2 \rightarrow 8(j+m+1)+4} \otimes w_{8j+3 \rightarrow 8j+7}, & i = j + 7s; \\ e_{8(j+m+1)+4} \otimes w_{8j+3 \rightarrow 8j+7}, & i = j + 8s; \\ 0, & \text{otherwise.} \end{cases}$$

If  $6s \leq j < 7s$ , then

$$(d_{19})_{ij} = \begin{cases} -e_{8(j+m+1)+5} \otimes w_{8j+3 \rightarrow 8(j+1)}, & i = 3s + (j+1)_s; \\ w_{8(j+m+1) \rightarrow 8(j+m+1)+5} \otimes e_{8j+3}, & i = j; \\ e_{8(j+m+1)+5} \otimes w_{8j+3 \rightarrow 8j+7}, & i = j + 9s; \\ 0, & \text{otherwise.} \end{cases}$$

If  $7s \leq j < 8s$ , then

$$(d_{19})_{ij} = \begin{cases} w_{8(j+m)+7 \rightarrow 8(j+m+1)+6} \otimes e_{8j+4}, & i = j; \\ e_{8(j+m+1)+6} \otimes w_{8j+4 \rightarrow 8j+7}, & i = j + 7s; \\ 0, & \text{otherwise.} \end{cases}$$

If  $8s \leq j < 9s$ , then

$$(d_{19})_{ij} = \begin{cases} -e_{8(j+m+1)+6} \otimes w_{8j+5 \rightarrow 8(j+1)}, & i = s + (j+1)_s; \\ w_{8(j+m)+7+f(j_1,1) \rightarrow 8(j+m+1)+6} \otimes w_{8j+5 \rightarrow 8j+5+f(j_1,2)}, & i = j + j_1s, \ 0 \leq j_1 \leq 2; \\ -e_{8(j+m+1)+6} \otimes w_{8j+5 \rightarrow 8j+7}, & i = j + 6s; \\ 0, & \text{otherwise.} \end{cases}$$

If  $9s \leq j < 10s$ , then

$$(d_{19})_{ij} = \begin{cases} w_{8(j+m)+7 \rightarrow 8(j+m+1)+4} \otimes e_{8j+5}, & i = j - s; \\ -e_{8(j+m+1)+4} \otimes w_{8j+5 \rightarrow 8j+7}, & i = j + 4s; \\ 0, & \text{otherwise.} \end{cases}$$

If  $10s \leq j < 11s$ , then

$$(d_{19})_{ij} = \begin{cases} e_{8(j+m+1)+1} \otimes w_{8j+5 \rightarrow 8(j+1)}, & i = 2s + (j+1)_s; \\ w_{8(j+m+1) \rightarrow 8(j+m+1)+1} \otimes e_{8j+5}, & i = j - s; \\ 0, & \text{otherwise.} \end{cases}$$

If  $11s \leq j < 12s$ , then

$$(d_{19})_{ij} = \begin{cases} w_{8(j+m)+7+j_1+f(j_1,2) \rightarrow 8(j+m+1)+2} \otimes w_{8j+6 \rightarrow 8j+6+f(j_1,2)}, \\ \quad i = j + (j_1 - 1)s, \quad 0 \leq j_1 \leq 2; \\ 0, & \text{otherwise.} \end{cases}$$

If  $12s \leq j < 13s$ , then

$$(d_{19})_{ij} = \begin{cases} w_{8(j+m+1) \rightarrow 8(j+m+1)+5} \otimes e_{8j+6}, & i = j - s; \\ -e_{8(j+m+1)+5} \otimes w_{8j+6 \rightarrow 8j+7}, & i = j + 3s; \\ 0, & \text{otherwise.} \end{cases}$$

If  $13s \leq j < 14s$ , then

$$(d_{19})_{ij} = \begin{cases} w_{8(j+m+1)+6 \rightarrow 8(j+m+1)+7} \otimes w_{8j+7 \rightarrow 8(j+1)}, & i = s + (j+1)_s; \\ (-1 + 2f(j_1, 0))w_{8(j+m+1)+7-6f(j_1,0) \rightarrow 8(j+m+1)+7} \otimes w_{8j+7 \rightarrow 8(j+1)+2j_1}, \\ \quad i = (3 + 2j_1 - f(j_1, 0) + f(j_1, 3))s + (j+1)_s, \quad 0 \leq j_1 \leq 3; \\ (1 - 2f(j_1, 1))w_{8(j+m+1)+2(j_1+1)-3f(j_1,3) \rightarrow 8(j+m+1)+7} \otimes e_{8j+7}, & i = j + (j_1 - 1)s, \quad 0 \leq j_1 \leq 3; \\ 0, & \text{otherwise.} \end{cases}$$

If  $14s \leq j < 15s$ , then

$$(d_{19})_{ij} = \begin{cases} -w_{8(j+m+1)+6 \rightarrow 8(j+m+2)} \otimes w_{8j+7 \rightarrow 8(j+1)}, & i = s + (j+1)_s; \\ (1 - 2f(j_1, 0))w_{8(j+m+2)+1-j_1-8f(j_1,0) \rightarrow 8(j+m+2)} \otimes w_{8j+7 \rightarrow 8(j+1)+j_1}, \\ \quad i = (3 + j_1 - f(j_1, 0))s + (j+1)_s, \quad 0 \leq j_1 \leq 2; \\ w_{8(j+m+1)+7+f(j_1,1) \rightarrow 8(j+m+2)} \otimes w_{8j+7 \rightarrow 8(j+1)+4+j_1}, \\ \quad i = (8 + j_1 - f(j_1, 0))s + (j+1)_s, \quad 0 \leq j_1 \leq 2; \\ w_{8(j+m+1)+4 \rightarrow 8(j+m+2)} \otimes e_{8j+7}, & i = j - s; \\ 0, & \text{otherwise.} \end{cases}$$

If  $15s \leq j < 16s$ , then

$$(d_{19})_{ij} = \begin{cases} e_{8(j+m+2)} \otimes w_{8j+7 \rightarrow 8(j+1)+5}, & i = 9s + (j+1)_s; \\ w_{8(j+m+1)+6 \rightarrow 8(j+m+2)} \otimes e_{8j+7}, & i = j - s; \\ 0, & \text{otherwise.} \end{cases}$$

### Description of $d_{20}$

$d_{20} : Q_{21} \rightarrow Q_{20}$  - is an  $(16s \times 14s)$  matrix.

If  $0 \leq j < s$ , then

$$(d_{20})_{ij} = \begin{cases} (-1 + 2f(j_1, 0))w_{8(j+m-1)+7+j_1+f(j_1, 2) \rightarrow 8(j+m)+2} \otimes w_{8j \rightarrow 8j+f(j_1, 2)}, \\ \quad i = j + j_1 s, \quad 0 \leq j_1 \leq 2; \\ -w_{8(j+m)+1 \rightarrow 8(j+m)+2} \otimes w_{8j \rightarrow 8j+5}, \quad i = j + 10s; \\ -e_{8(j+m)+2} \otimes w_{8j \rightarrow 8j+6}, \quad i = j + 11s; \\ 0, \quad \text{otherwise.} \end{cases}$$

If  $s \leq j < 2s$ , then

$$(d_{20})_{ij} = \begin{cases} (1 - 2f(j_1, 2))w_{8(j+m)+j_1+1-f(j_1, 0) \rightarrow 8(j+m)+4} \otimes w_{8j \rightarrow 8j+j_1}, \\ \quad i = j + (j_1 + f(j_1, 2, 3))s, \quad 0 \leq j_1 \leq 3; \\ e_{8(j+m)+4} \otimes w_{8j \rightarrow 8j+5}, \quad i = j + 8s; \\ w_{8(j+m)+1 \rightarrow 8(j+m)+4} \otimes w_{8j \rightarrow 8j+5}, \quad i = j + 9s; \\ w_{8(j+m)+2 \rightarrow 8(j+m)+4} \otimes w_{8j \rightarrow 8j+6}, \quad i = j + 10s; \\ 0, \quad \text{otherwise.} \end{cases}$$

If  $2s \leq j < 3s$ , then

$$(d_{20})_{ij} = \begin{cases} w_{8(j+m) \rightarrow 8(j+m)+6} \otimes e_{8j}, \quad i = j - s; \\ e_{8(j+m)+6} \otimes w_{8j \rightarrow 8j+1}, \quad i = j + s; \\ w_{8(j+m)+5+f(j_1, 1, 2) \rightarrow 8(j+m)+6} \otimes w_{8j \rightarrow 8j+3+j_1}, \\ \quad i = j + (4 + j_1 + 3f(j_1, 3))s, \quad 0 \leq j_1 \leq 3; \\ 0, \quad \text{otherwise.} \end{cases}$$

If  $3s \leq j < 4s$ , then

$$(d_{20})_{ij} = \begin{cases} -e_{8(j+m)+7} \otimes w_{8j+1 \rightarrow 8(j+1)}, \quad i = (j + 1)s; \\ (-1 + 2f(j_1, 0))w_{8(j+m)+9-3j_1-7f(j_1, 0) \rightarrow 8(j+m)+7} \otimes w_{8j+1 \rightarrow 8j+1+f(j_1, 2)}, \\ \quad i = j + (j_1 - 1)s, \quad 0 \leq j_1 \leq 2; \\ 0, \quad \text{otherwise.} \end{cases}$$

If  $4s \leq j < 5s$ , then

$$(d_{20})_{ij} = \begin{cases} -w_{8(j+m)+7 \rightarrow 8(j+m+1)} \otimes w_{8j+2 \rightarrow 8(j+1)}, \quad i = (j + 1)s; \\ e_{8(j+m+1)} \otimes w_{8j+2 \rightarrow 8(j+1)}, \quad i = s + (j + 1)s; \\ w_{8(j+m)+3 \rightarrow 8(j+m+1)} \otimes e_{8j+2}, \quad i = j; \\ -w_{8(j+m)+4 \rightarrow 8(j+m+1)} \otimes w_{8j+2 \rightarrow 8j+3}, \quad i = j + s; \\ e_{8(j+m+1)} \otimes w_{8j+2 \rightarrow 8j+7}, \quad i = j + 10s; \\ 0, \quad \text{otherwise.} \end{cases}$$

If  $5s \leq j < 6s$ , then

$$(d_{20})_{ij} = \begin{cases} e_{8(j+m)+7} \otimes w_{8j+3 \rightarrow 8(j+1)}, \quad i = (j + 1)s; \\ (1 - 2f(j_1, 1, 2))w_{8(j+m)+4+j_1 \rightarrow 8(j+m)+7} \otimes w_{8j+3 \rightarrow 8j+3+f(j_1, 2)+4f(j_1, 3)}, \\ \quad i = j + (j_1 + 5f(j_1, 3))s, \quad 0 \leq j_1 \leq 3; \\ 0, \quad \text{otherwise.} \end{cases}$$

If  $6s \leq j < 7s$ , then

$$(d_{20})_{ij} = \begin{cases} w_{8(j+m)+6 \rightarrow 8(j+m+1)} \otimes e_{8j+4}, & i = j + s; \\ -e_{8(j+m+1)} \otimes w_{8j+4 \rightarrow 8j+7}, & i = j + 9s; \\ 0, & \text{otherwise.} \end{cases}$$

If  $7s \leq j < 8s$ , then

$$(d_{20})_{ij} = \begin{cases} (-1 + 2f(j_1, 0))w_{8(j+m)+6-2j_1-f(j_1,2) \rightarrow 8(j+m)+7} \otimes e_{8j+5}, & i = j + (1 + j_1)s, \ 0 \leq j_1 \leq 2; \\ (1 - 2f(j_1, 0))w_{8(j+m)+3+2j_1-f(j_1,0) \rightarrow 8(j+m)+7} \otimes w_{8j+5 \rightarrow 8j+6+f(j_1,2)}, \\ \quad i = j + (4 + j_1)s, \ 0 \leq j_1 \leq 2; \\ 0, & \text{otherwise.} \end{cases}$$

If  $8s \leq j < 9s$ , then

$$(d_{20})_{ij} = \begin{cases} -w_{8(j+m)+7 \rightarrow 8(j+m+1)} \otimes w_{8j+5 \rightarrow 8(j+1)}, & i = (j + 1)_s; \\ e_{8(j+m+1)} \otimes w_{8j+5 \rightarrow 8(j+1)}, & i = s + (j + 1)_s; \\ w_{8(j+m)+4 \rightarrow 8(j+m+1)} \otimes e_{8j+5}, & i = j + s; \\ e_{8(j+m+1)} \otimes w_{8j+5 \rightarrow 8j+7}, & i = j + 6s; \\ 0, & \text{otherwise.} \end{cases}$$

If  $9s \leq j < 10s$ , then

$$(d_{20})_{ij} = \begin{cases} w_{8(j+m)+2 \rightarrow 8(j+m+1)} \otimes e_{8j+6}, & i = j + 2s; \\ -w_{8(j+m)+5 \rightarrow 8(j+m+1)} \otimes e_{8j+6}, & i = j + 3s; \\ (-1 + 2f(j_1, 2))w_{8(j+m+1)-f(j_1,0) \rightarrow 8(j+m+1)} \otimes w_{8j+6 \rightarrow 8j+7}, \\ \quad i = j + (4 + j_1)s, \ 0 \leq j_1 \leq 2; \\ 0, & \text{otherwise.} \end{cases}$$

If  $10s \leq j < 11s$ , then

$$(d_{20})_{ij} = \begin{cases} -w_{8(j+m+1)+2 \rightarrow 8(j+m+1)+3} \otimes w_{8j+7 \rightarrow 8(j+1)+1}, & i = 2s + (j + 1)_s; \\ e_{8(j+m+1)+3} \otimes w_{8j+7 \rightarrow 8(j+1)+2}, & i = 4s + (j + 1)_s; \\ -w_{8(j+m+1)+1 \rightarrow 8(j+m+1)+3} \otimes w_{8j+7 \rightarrow 8(j+1)+5}, & i = 10s + (j + 1)_s; \\ w_{8(j+m)+7 \rightarrow 8(j+m+1)+3} \otimes e_{8j+7}, & i = j + 3s; \\ w_{8(j+m+1) \rightarrow 8(j+m+1)+3} \otimes e_{8j+7}, & i = j + 4s; \\ 0, & \text{otherwise.} \end{cases}$$

If  $11s \leq j < 12s$ , then

$$(d_{20})_{ij} = \begin{cases} w_{8(j+m)+7 \rightarrow 8(j+m+1)+6} \otimes w_{8j+7 \rightarrow 8(j+1)}, & i = (j + 1)_s; \\ e_{8(j+m+1)+6} \otimes w_{8j+7 \rightarrow 8(j+1)+4}, & i = 7s + (j + 1)_s; \\ e_{8(j+m+1)+6} \otimes w_{8j+7 \rightarrow 8(j+1)+5}, & i = 8s + (j + 1)_s; \\ w_{8(j+m)+7 \rightarrow 8(j+m+1)+6} \otimes e_{8j+7}, & i = j + 2s; \\ -w_{8(j+m+1) \rightarrow 8(j+m+1)+6} \otimes e_{8j+7}, & i = j + 4s; \\ 0, & \text{otherwise.} \end{cases}$$



If  $12s \leq j < 13s$ , then

$$(d_{20})_{ij} = \begin{cases} -e_{8(j+m+1)+1} \otimes w_{8j+7 \rightarrow 8(j+1)+5}, & i = 10s + (j+1)_s; \\ w_{8(j+m+1) \rightarrow 8(j+m+1)+1} \otimes e_{8j+7}, & i = j + 3s; \\ 0, & \text{otherwise.} \end{cases}$$

If  $13s \leq j < 14s$ , then

$$(d_{20})_{ij} = \begin{cases} -w_{8(j+m)+7 \rightarrow 8(j+m+1)+5} \otimes w_{8j+7 \rightarrow 8(j+1)}, & i = (j+1)_s; \\ w_{8(j+m+1)+5-5f(j_1,0) \rightarrow 8(j+m+1)+5} \otimes w_{8j+7 \rightarrow 8(j+1)+3j_1}, \\ \quad i = (6j_1 + f(j_1,0))s + (j+1)_s, & 0 \leq j_1 \leq 2; \\ w_{8(j+m+1) \rightarrow 8(j+m+1)+5} \otimes e_{8j+7}, & i = j + s; \\ 0, & \text{otherwise.} \end{cases}$$

### Description of $d_{21}$

$d_{21} : Q_{22} \rightarrow Q_{21}$  - is an  $(14s \times 13s)$  matrix.

If  $0 \leq j < s$ , then

$$(d_{21})_{ij} = \begin{cases} w_{8(j+m)+4 \rightarrow 8(j+m+1)} \otimes e_{8j}, & i = j + s; \\ (1 - 2f(j_1, 2))w_{8(j+m+1)-6f(j_1,0) \rightarrow 8(j+m+1)} \otimes w_{8j \rightarrow 8j+2j_1+f(j_1,2)}, \\ \quad i = j + 4j_1s, & 0 \leq j_1 \leq 2; \\ 0, & \text{otherwise.} \end{cases}$$

If  $s \leq j < 2s$ , then

$$(d_{21})_{ij} = \begin{cases} w_{8(j+m)+4 \rightarrow 8(j+m)+7} \otimes e_{8j}, & i = j; \\ -w_{8(j+m)+6 \rightarrow 8(j+m)+7} \otimes e_{8j}, & i = j + s; \\ (-1 + 2f(j_1, 2))e_{8(j+m)+7} \otimes w_{8j \rightarrow 8j+1+2j_1}, & i = j + 2(j_1 + 1)s, \quad 0 \leq j_1 \leq 2; \\ 0, & \text{otherwise.} \end{cases}$$

If  $2s \leq j < 3s$ , then

$$(d_{21})_{ij} = \begin{cases} w_{8(j+m+1)+2 \rightarrow 8(j+m+1)+3} \otimes w_{8j+1 \rightarrow 8(j+1)}, & i = (j+1)_s; \\ w_{8(j+m)+7+f(j_1,2) \rightarrow 8(j+m+1)+3} \otimes w_{8j+1 \rightarrow 8j+j_1}, & i = j + j_1s, \quad 1 \leq j_1 \leq 3; \\ -e_{8(j+m+1)+3} \otimes w_{8j+1 \rightarrow 8j+7}, & i = j + 8s; \\ 0, & \text{otherwise.} \end{cases}$$

If  $3s \leq j < 4s$ , then

$$(d_{21})_{ij} = \begin{cases} -e_{8(j+m+1)+4} \otimes w_{8j+2 \rightarrow 8(j+1)}, & i = s + (j+1)_s; \\ w_{8(j+m+1) \rightarrow 8(j+m+1)+4} \otimes e_{8j+2}, & i = j + s; \\ w_{8(j+m)+7 \rightarrow 8(j+m+1)+4} \otimes w_{8j+2 \rightarrow 8j+3}, & i = j + 2s; \\ -w_{8(j+m+1)+3 \rightarrow 8(j+m+1)+4} \otimes w_{8j+2 \rightarrow 8j+7}, & i = j + 7s; \\ 0, & \text{otherwise.} \end{cases}$$

If  $4s \leq j < 5s$ , then

$$(d_{21})_{ij} = \begin{cases} w_{8(j+m+1) \rightarrow 8(j+m+1)+5} \otimes e_{8j+2}, & i = j; \\ -e_{8(j+m+1)+5} \otimes w_{8j+2 \rightarrow 8j+7}, & i = j + 9s; \\ 0, & \text{otherwise.} \end{cases}$$

If  $5s \leq j < 6s$ , then

$$(d_{21})_{ij} = \begin{cases} w_{8(j+m)+7 \rightarrow 8(j+m+1)+6} \otimes e_{8j+3}, & i = j; \\ w_{8(j+m+1) \rightarrow 8(j+m+1)+6} \otimes w_{8j+3 \rightarrow 8j+4}, & i = j + s; \\ -e_{8(j+m+1)+6} \otimes w_{8j+3 \rightarrow 8j+7}, & i = j + 6s; \\ 0, & \text{otherwise.} \end{cases}$$

If  $6s \leq j < 7s$ , then

$$(d_{21})_{ij} = \begin{cases} w_{8(j+m+1) \rightarrow 8(j+m+1)+1} \otimes e_{8j+4}, & i = j; \\ e_{8(j+m+1)+1} \otimes w_{8j+4 \rightarrow 8j+7}, & i = j + 6s; \\ 0, & \text{otherwise.} \end{cases}$$

If  $7s \leq j < 8s$ , then

$$(d_{21})_{ij} = \begin{cases} e_{8(j+m+1)+2} \otimes w_{8j+5 \rightarrow 8(j+1)}, & i = (j+1)_s; \\ (1 - 2f(j_1, 3))w_{8(j+m)+7+j_1-f(j_1, 2, 3) \rightarrow 8(j+m+1)+2} \otimes w_{8j+5 \rightarrow 8j+4+j_1+f(j_1, 0)}, & \\ i = j + (j_1 + 2f(j_1, 3))s, & 0 \leq j_1 \leq 3; \\ 0, & \text{otherwise.} \end{cases}$$

If  $8s \leq j < 9s$ , then

$$(d_{21})_{ij} = \begin{cases} w_{8(j+m+1) \rightarrow 8(j+m+1)+5} \otimes e_{8j+5}, & i = j; \\ -e_{8(j+m+1)+5} \otimes w_{8j+5 \rightarrow 8j+7}, & i = j + 5s; \\ 0, & \text{otherwise.} \end{cases}$$

If  $9s \leq j < 10s$ , then

$$(d_{21})_{ij} = \begin{cases} w_{8(j+m+1) \rightarrow 8(j+m+1)+3} \otimes e_{8j+6}, & i = j; \\ e_{8(j+m+1)+3} \otimes w_{8j+6 \rightarrow 8j+7}, & i = j + s; \\ -w_{8(j+m+1)+1 \rightarrow 8(j+m+1)+3} \otimes w_{8j+6 \rightarrow 8j+7}, & i = j + 3s; \\ 0, & \text{otherwise.} \end{cases}$$

If  $10s \leq j < 11s$ , then

$$(d_{21})_{ij} = \begin{cases} -e_{8(j+m+1)+6} \otimes w_{8j+6 \rightarrow 8(j+1)}, & i = 2s + (j+1)_s; \\ w_{8(j+m+1)+7-j_1-7f(j_1, 0) \rightarrow 8(j+m+1)+6} \otimes w_{8j+6 \rightarrow 8j+7-f(j_1, 0)}, & \\ i = j + (2j_1 - 1)s, & 0 \leq j_1 \leq 2; \\ 0, & \text{otherwise.} \end{cases}$$

If  $11s \leq j < 12s$ , then

$$(d_{21})_{ij} = \begin{cases} w_{8(j+m+1)+6 \rightarrow 8(j+m+1)+7} \otimes w_{8j+7 \rightarrow 8(j+1)}, & i = 2s + (j+1)_s; \\ e_{8(j+m+1)+7} \otimes w_{8j+7 \rightarrow 8(j+1)+1}, & i = 3s + (j+1)_s; \\ (-1 + 2f(j_1, 0))w_{8(j+m+1)+3-j_1+4f(j_1, 1)+5f(j_1, 3) \rightarrow 8(j+m+1)+7} \otimes e_{8j+7}, & \\ i = j + (j_1 - 1)s, & 0 \leq j_1 \leq 3; \\ 0, & \text{otherwise.} \end{cases}$$

If  $12s \leq j < 13s$ , then

$$(d_{21})_{ij} = \begin{cases} -w_{8(j+m+1)+2 \rightarrow 8(j+m+2)} \otimes w_{8j+7 \rightarrow 8(j+1)}, & i = (j+1)_s; \\ -w_{8(j+m+2)-f(j_1,1) \rightarrow 8(j+m+2)} \otimes w_{8j+7 \rightarrow 8(j+1)+2+j_1}, \\ \quad i = (4+j_1)s + (j+1)_s, \quad 0 \leq j_1 \leq 2; \\ -e_{8(j+m+2)} \otimes w_{8j+7 \rightarrow 8(j+1)+6}, & i = 9s + (j+1)_s; \\ w_{8(j+m+1)+3 \rightarrow 8(j+m+2)} \otimes e_{8j+7}, & i = j - 2s; \\ -w_{8(j+m+1)+5 \rightarrow 8(j+m+2)} \otimes e_{8j+7}, & i = j + s; \\ 0, & \text{otherwise.} \end{cases}$$

**Description of  $d_{22}$**

$d_{22} : Q_{23} \rightarrow Q_{22}$  is an  $(13s \times 11s)$  matrix.

If  $0 \leq j < s$ , then

$$(d_{22})_{ij} = \begin{cases} (-1 + 2f(j_1, 0))w_{8(j+m)-j_1+5f(j_1,2) \rightarrow 8(j+m)+3} \otimes w_{8j \rightarrow 8j+f(j_1,2)}, \\ \quad i = j + j_1s, \quad 0 \leq j_1 \leq 2; \\ w_{8(j+m)+2 \rightarrow 8(j+m)+3} \otimes w_{8j \rightarrow 8j+5}, & i = j + 7s; \\ -e_{8(j+m)+3} \otimes w_{8j \rightarrow 8j+6}, & i = j + 9s; \\ 0, & \text{otherwise.} \end{cases}$$

If  $s \leq j < 2s$ , then

$$(d_{22})_{ij} = \begin{cases} w_{8(j+m) \rightarrow 8(j+m)+5} \otimes e_{8j}, & i = j_s; \\ -e_{8(j+m)+5} \otimes w_{8j \rightarrow 8j+2}, & i = j + 3s; \\ e_{8(j+m)+5} \otimes w_{8j \rightarrow 8j+5}, & i = j + 7s; \\ 0, & \text{otherwise.} \end{cases}$$

If  $2s \leq j < 3s$ , then

$$(d_{22})_{ij} = \begin{cases} -e_{8(j+m+1)} \otimes w_{8j+1 \rightarrow 8(j+1)}, & i = (j+1)_s; \\ w_{8(j+m)+3 \rightarrow 8(j+m+1)} \otimes e_{8j+1}, & i = j; \\ -w_{8(j+m)+4 \rightarrow 8(j+m+1)} \otimes w_{8j+1 \rightarrow 8j+2}, & i = j + s; \\ 0, & \text{otherwise.} \end{cases}$$

If  $3s \leq j < 4s$ , then

$$(d_{22})_{ij} = \begin{cases} e_{8(j+m)+7} \otimes w_{8j+2 \rightarrow 8(j+1)}, & i = s + (j+1)_s; \\ (1 - 2f(j_1, 1, 2))w_{8(j+m)+4+j_1-6f(j_1,3) \rightarrow 8(j+m)+7} \otimes w_{8j+2 \rightarrow 8j+1+j_1+f(j_1,0)}, \\ \quad i = j + j_1s, \quad 0 \leq j_1 \leq 3; \\ e_{8(j+m)+7} \otimes w_{8j+2 \rightarrow 8j+7}, & i = j + 8s; \\ 0, & \text{otherwise.} \end{cases}$$

If  $4s \leq j < 5s$ , then

$$(d_{22})_{ij} = \begin{cases} e_{8(j+m+1)} \otimes w_{8j+3 \rightarrow 8(j+1)}, & i = (j+1)_s; \\ -w_{8(j+m)+7 \rightarrow 8(j+m+1)} \otimes w_{8j+3 \rightarrow 8(j+1)}, & i = s + (j+1)_s; \\ w_{8(j+m)+6 \rightarrow 8(j+m+1)} \otimes e_{8j+3}, & i = j + s; \\ -w_{8(j+m)+1 \rightarrow 8(j+m+1)} \otimes w_{8j+3 \rightarrow 8j+4}, & i = j + 2s; \\ -w_{8(j+m)+7 \rightarrow 8(j+m+1)} \otimes w_{8j+3 \rightarrow 8j+7}, & i = j + 7s; \\ e_{8(j+m+1)} \otimes w_{8j+3 \rightarrow 8j+7}, & i = j + 8s; \\ 0, & \text{otherwise.} \end{cases}$$

If  $5s \leq j < 6s$ , then

$$(d_{22})_{ij} = \begin{cases} -w_{8(j+m+1) \rightarrow 8(j+m+1)+1} \otimes w_{8j+4 \rightarrow 8(j+1)}, & i = (j+1)_s; \\ w_{8(j+m)+7 \rightarrow 8(j+m+1)+1} \otimes w_{8j+4 \rightarrow 8(j+1)}, & i = s + (j+1)_s; \\ w_{8(j+m)+1 \rightarrow 8(j+m+1)+1} \otimes e_{8j+4}, & i = j + s; \\ -e_{8(j+m+1)+1} \otimes w_{8j+4 \rightarrow 8(j+1)+4}, & i = 6s + (j+1)_s; \\ w_{8(j+m)+7 \rightarrow 8(j+m+1)+1} \otimes w_{8j+4 \rightarrow 8j+7}, & i = j + 6s; \\ -w_{8(j+m+1) \rightarrow 8(j+m+1)+1} \otimes w_{8j+4 \rightarrow 8j+7}, & i = j + 7s; \\ 0, & \text{otherwise.} \end{cases}$$

If  $6s \leq j < 7s$ , then

$$(d_{22})_{ij} = \begin{cases} (1 - 2f(j_1, 1, 2))w_{8(j+m)+2+3j_1-5f(j_1,2)-3f(j_1,3) \rightarrow 8(j+m+1)} \otimes w_{8j+5 \rightarrow 8j+4+j_1+f(j_1,0)}, \\ i = j + (j_1 + 1 + 2f(j_1, 3))s, & 0 \leq j_1 \leq 3; \\ 0, & \text{otherwise.} \end{cases}$$

If  $7s \leq j < 8s$ , then

$$(d_{22})_{ij} = \begin{cases} (-1 + 2f(j_1, 0))w_{8(j+m)+5+j_1-2f(j_1,0) \rightarrow 8(j+m)+7} \otimes w_{8j+6 \rightarrow 8j+6+f(j_1,2)}, \\ i = j + (2 + j_1)s, & 0 \leq j_1 \leq 2; \\ 0, & \text{otherwise.} \end{cases}$$

If  $8s \leq j < 9s$ , then

$$(d_{22})_{ij} = \begin{cases} -w_{8(j+m+1) \rightarrow 8(j+m+1)+2} \otimes w_{8j+7 \rightarrow 8(j+1)}, & i = (j+1)_s; \\ w_{8(j+m)+7 \rightarrow 8(j+m+1)+2} \otimes w_{8j+7 \rightarrow 8(j+1)}, & i = s + (j+1)_s; \\ -w_{8(j+m+1)+1 \rightarrow 8(j+m+1)+2} \otimes w_{8j+7 \rightarrow 8(j+1)+4}, & i = 6s + (j+1)_s; \\ -e_{8(j+m+1)+2} \otimes w_{8j+7 \rightarrow 8(j+1)+5}, & i = 7s + (j+1)_s; \\ w_{8(j+m)+7 \rightarrow 8(j+m+1)+2} \otimes e_{8j+7}, & i = j + 3s; \\ -w_{8(j+m+1) \rightarrow 8(j+m+1)+2} \otimes e_{8j+7}, & i = j + 4s; \\ 0, & \text{otherwise.} \end{cases}$$

If  $9s \leq j < 10s$ , then

$$(d_{22})_{ij} = \begin{cases} (1 - 2f(j_1, 1, 2))w_{8(j+m+1)+1+j_1-f(j_1,0)-3f(j_1,1) \rightarrow 8(j+m+1)+4} \otimes w_{8j+7 \rightarrow 8(j+1)-1+j_1+f(j_1,0)}, \\ \quad i = j_1s + (j+1)_s, \quad 0 \leq j_1 \leq 3; \\ w_{8(j+m+1)+1 \rightarrow 8(j+m+1)+4} \otimes w_{8j+7 \rightarrow 8(j+1)+4}, & i = 6s + (j+1)_s; \\ w_{8(j+m+1)+2 \rightarrow 8(j+m+1)+4} \otimes w_{8j+7 \rightarrow 8(j+1)+5}, & i = 7s + (j+1)_s; \\ w_{8(j+m+1) \rightarrow 8(j+m+1)+4} \otimes e_{8j+7}, & i = j + 3s; \\ 0, & \text{otherwise.} \end{cases}$$

If  $10s \leq j < 11s$ , then

$$(d_{22})_{ij} = \begin{cases} w_{8(j+m+1)+5 \rightarrow 8(j+m+1)+6} \otimes w_{8j+7 \rightarrow 8(j+1)+2}, & i = 4s + (j+1)_s; \\ e_{8(j+m+1)+6} \otimes w_{8j+7 \rightarrow 8(j+1)+3}, & i = 5s + (j+1)_s; \\ e_{8(j+m+1)+6} \otimes w_{8j+7 \rightarrow 8(j+1)+6}, & i = 10s + (j+1)_s; \\ w_{8(j+m+1) \rightarrow 8(j+m+1)+6} \otimes e_{8j+7}, & i = j + 2s; \\ 0, & \text{otherwise.} \end{cases}$$

### Description of $d_{23}$

$d_{23} : Q_{24} \rightarrow Q_{23}$  - is an  $(11s \times 11s)$  matrix.

If  $0 \leq j < s$ , then

$$(d_{23})_{ij} = \begin{cases} (1 - 2f(j_1, 1))w_{8(j+m+1)-5f(j_1,0)-3f(j_1,1)-f(j_1,3) \rightarrow 8(j+m+1)} \otimes w_{8j \rightarrow 8j-1+j_1+f(j_1,0)}, \\ \quad i = j + j_1s, \quad 0 \leq j_1 \leq 4; \\ -e_{8(j+m+1)} \otimes w_{8j \rightarrow 8j+5}, & i = j + 6s; \\ 0, & \text{otherwise.} \end{cases}$$

If  $s \leq j < 2s$ , then

$$(d_{23})_{ij} = \begin{cases} w_{8(j+m+1)+3 \rightarrow 8(j+m+1)+4} \otimes w_{8j+1 \rightarrow 8(j+1)}, & i = (j+1)_s; \\ w_{8(j+m+1)-f(j_1,2) \rightarrow 8(j+m+1)+4} \otimes w_{8j+1 \rightarrow 8j+j_1}, & i = j + j_1s, \quad 1 \leq j_1 \leq 3; \\ -e_{8(j+m+1)+4} \otimes w_{8j+1 \rightarrow 8j+7}, & i = j + 8s; \\ 0, & \text{otherwise.} \end{cases}$$

If  $2s \leq j < 3s$ , then

$$(d_{23})_{ij} = \begin{cases} e_{8(j+m+1)+5} \otimes w_{8j+1 \rightarrow 8(j+1)}, & i = s + (j+1)_s; \\ w_{8(j+m+1) \rightarrow 8(j+m+1)+5} \otimes e_{8j+1}, & i = j; \\ 0, & \text{otherwise.} \end{cases}$$

If  $3s \leq j < 4s$ , then

$$(d_{23})_{ij} = \begin{cases} -w_{8(j+m+1)+5 \rightarrow 8(j+m+1)+6} \otimes w_{8j+2 \rightarrow 8(j+1)}, & i = s + (j+1)_s; \\ w_{8(j+m+1)+7 \rightarrow 8(j+m+1)+6} \otimes e_{8j+2}, & i = j; \\ w_{8(j+m+1) \rightarrow 8(j+m+1)+6} \otimes w_{8j+2 \rightarrow 8j+3}, & i = j + s; \\ -e_{8(j+m+1)+6} \otimes w_{8j+2 \rightarrow 8j+7}, & i = j + 7s; \\ 0, & \text{otherwise.} \end{cases}$$

If  $4s \leq j < 5s$ , then

$$(d_{23})_{ij} = \begin{cases} w_{8(j+m+1) \rightarrow 8(j+m+1)+1} \otimes e_{8j+3}, & i = j; \\ e_{8(j+m+1)+1} \otimes w_{8j+3 \rightarrow 8j+4}, & i = j + s; \\ 0, & \text{otherwise.} \end{cases}$$

If  $5s \leq j < 6s$ , then

$$(d_{23})_{ij} = \begin{cases} w_{8(j+m+1)+1 \rightarrow 8(j+m+1)+2} \otimes e_{8j+4}, & i = j; \\ -e_{8(j+m+1)+2} \otimes w_{8j+4 \rightarrow 8j+7}, & i = j + 3s; \\ 0, & \text{otherwise.} \end{cases}$$

If  $6s \leq j < 7s$ , then

$$(d_{23})_{ij} = \begin{cases} e_{8(j+m+1)+3} \otimes w_{8j+5 \rightarrow 8(j+1)}, & i = (j+1)_s; \\ w_{8(j+m+1)+j_1-2f(j_1,1) \rightarrow 8(j+m+1)+3} \otimes w_{8j+5 \rightarrow 8j+5+j_1}, & i = j + j_1s, \ 0 \leq j_1 \leq 2; \\ 0, & \text{otherwise.} \end{cases}$$

If  $7s \leq j < 8s$ , then

$$(d_{23})_{ij} = \begin{cases} w_{8(j+m+1) \rightarrow 8(j+m+1)+6} \otimes e_{8j+5}, & i = j - s; \\ -e_{8(j+m+1)+6} \otimes w_{8j+5 \rightarrow 8j+7}, & i = j + 3s; \\ 0, & \text{otherwise.} \end{cases}$$

If  $8s \leq j < 9s$ , then

$$(d_{23})_{ij} = \begin{cases} w_{8(j+m+1)+2j_1-f(j_1,0) \rightarrow 8(j+m+1)+4} \otimes w_{8j+6 \rightarrow 8j+7-f(j_1,0)}, & \\ i = j + (j_1 - 1)s, \ 0 \leq j_1 \leq 2; \\ 0, & \text{otherwise.} \end{cases}$$

If  $9s \leq j < 10s$ , then

$$(d_{23})_{ij} = \begin{cases} e_{8(j+m+2)} \otimes w_{8j+7 \rightarrow 8(j+1)+1}, & i = 2s + (j+1)_s; \\ w_{8(j+m+1)+2 \rightarrow 8(j+m+2)} \otimes e_{8j+7}, & i = j - s; \\ w_{8(j+m+1)+4 \rightarrow 8(j+m+2)} \otimes e_{8j+7}, & i = j; \\ 0, & \text{otherwise.} \end{cases}$$

If  $10s \leq j < 11s$ , then

$$(d_{23})_{ij} = \begin{cases} -w_{8(j+m+1)+3 \rightarrow 8(j+m+1)+7} \otimes w_{8j+7 \rightarrow 8(j+1)}, & i = (j+1)_s; \\ -e_{8(j+m+1)+7} \otimes w_{8j+7 \rightarrow 8(j+1)+2}, & i = 3s + (j+1)_s; \\ -e_{8(j+m+1)+7} \otimes w_{8j+7 \rightarrow 8(j+1)+6}, & i = 7s + (j+1)_s; \\ w_{8(j+m+1)+4 \rightarrow 8(j+m+1)+7} \otimes e_{8j+7}, & i = j - s; \\ -w_{8(j+m+1)+6 \rightarrow 8(j+m+1)+7} \otimes e_{8j+7}, & i = j; \\ 0, & \text{otherwise.} \end{cases}$$

#### Description of $d_{24}$

$d_{24} : Q_{25} \rightarrow Q_{24}$  - is an  $(11s \times 10s)$  matrix.

If  $0 \leq j < s$ , then

$$(d_{24})_{ij} = \begin{cases} w_{8(j+m) \rightarrow 8(j+m)+4} \otimes e_{8j}, & i = j; \\ -e_{8(j+m)+4} \otimes w_{8j \rightarrow 8j+1}, & i = j + s; \\ w_{8(j+m)+3 \rightarrow 8(j+m)+4} \otimes w_{8j \rightarrow 8j+5}, & i = j + 6s; \\ -e_{8(j+m)+4} \otimes w_{8j \rightarrow 8j+6}, & i = j + 8s; \\ 0, & \text{otherwise.} \end{cases}$$

If  $s \leq j < 2s$ , then

$$(d_{24})_{ij} = \begin{cases} w_{8(j+m) \rightarrow 8(j+m)+6} \otimes e_{8j}, & i = j_s; \\ (-1 + 2f(j_1, 3))w_{8(j+m)+6-f(j_1, 1) \rightarrow 8(j+m)+6} \otimes w_{8j \rightarrow 8j+j_1+2f(j_1, 3)}, \\ \quad i = j + (j_1 + 3f(j_1, 3))s, \quad 1 \leq j_1 \leq 3; \\ 0, & \text{otherwise.} \end{cases}$$

If  $2s \leq j < 3s$ , then

$$(d_{24})_{ij} = \begin{cases} w_{8(j+m)+4 \rightarrow 8(j+m)+7} \otimes e_{8j+1}, & i = j - s; \\ -w_{8(j+m)+5 \rightarrow 8(j+m)+7} \otimes e_{8j+1}, & i = j; \\ -w_{8(j+m)+6 \rightarrow 8(j+m)+7} \otimes w_{8j+1 \rightarrow 8j+2}, & i = j + s; \\ e_{8(j+m)+7} \otimes w_{8j+1 \rightarrow 8j+7}, & i = j + 8s; \\ 0, & \text{otherwise.} \end{cases}$$

If  $3s \leq j < 4s$ , then

$$(d_{24})_{ij} = \begin{cases} -e_{8(j+m+1)} \otimes w_{8j+2 \rightarrow 8(j+1)}, & i = (j+1)_s; \\ (-1)^{j_1} w_{8(j+m)+j_1+6f(j_1, 0) \rightarrow 8(j+m+1)} \otimes w_{8j+2 \rightarrow 8j+2+j_1}, \\ \quad i = j + j_1s, \quad 0 \leq j_1 \leq 2; \\ e_{8(j+m+1)} \otimes w_{8j+2 \rightarrow 8j+7}, & i = j + 6s; \\ -w_{8(j+m)+7 \rightarrow 8(j+m+1)} \otimes w_{8j+2 \rightarrow 8j+7}, & i = j + 7s; \\ 0, & \text{otherwise.} \end{cases}$$

If  $4s \leq j < 5s$ , then

$$(d_{24})_{ij} = \begin{cases} w_{8(j+m+1) \rightarrow 8(j+m+1)+1} \otimes w_{8j+3 \rightarrow 8(j+1)}, & i = (j+1)_s; \\ w_{8(j+m)+1 \rightarrow 8(j+m+1)+1} \otimes e_{8j+3}, & i = j; \\ -e_{8(j+m+1)+1} \otimes w_{8j+3 \rightarrow 8(j+1)+3}, & i = 4s + (j+1)_s; \\ -w_{8(j+m)+2 \rightarrow 8(j+m+1)+1} \otimes w_{8j+3 \rightarrow 8j+4}, & i = j + s; \\ -w_{8(j+m+1) \rightarrow 8(j+m+1)+1} \otimes w_{8j+3 \rightarrow 8j+7}, & i = j + 5s; \\ w_{8(j+m)+7 \rightarrow 8(j+m+1)+1} \otimes w_{8j+3 \rightarrow 8j+7}, & i = j + 6s; \\ 0, & \text{otherwise.} \end{cases}$$

If  $5s \leq j < 6s$ , then

$$(d_{24})_{ij} = \begin{cases} -w_{8(j+m+1) \rightarrow 8(j+m+1)+2} \otimes w_{8j+4 \rightarrow 8(j+1)}, & i = (j+1)_s; \\ w_{8(j+m+1)+1 \rightarrow 8(j+m+1)+2} \otimes w_{8j+4 \rightarrow 8(j+1)+3}, & i = 4s + (j+1)_s; \\ w_{8(j+m)+2 \rightarrow 8(j+m+1)+2} \otimes e_{8j+4}, & i = j; \\ -e_{8(j+m+1)+2} \otimes w_{8j+4 \rightarrow 8(j+1)+4}, & i = 5s + (j+1)_s; \\ w_{8(j+m+1) \rightarrow 8(j+m+1)+2} \otimes w_{8j+4 \rightarrow 8j+7}, & i = j + 4s; \\ -w_{8(j+m)+7 \rightarrow 8(j+m+1)+2} \otimes w_{8j+4 \rightarrow 8j+7}, & i = j + 5s; \\ 0, & \text{otherwise.} \end{cases}$$

If  $6s \leq j < 7s$ , then

$$(d_{24})_{ij} = \begin{cases} w_{8(j+m)+3 \rightarrow 8(j+m)+7} \otimes e_{8j+5}, & i = j; \\ (-1 + 2f(j_1, 2))w_{8(j+m)+6-2j_1+5f(j_1, 2) \rightarrow 8(j+m)+7} \otimes w_{8j+5 \rightarrow 8j+5+j_1}, \\ \quad i = j + (1 + j_1 + f(j_1, 2))s, & 0 \leq j_1 \leq 2; \\ 0, & \text{otherwise.} \end{cases}$$

If  $7s \leq j < 8s$ , then

$$(d_{24})_{ij} = \begin{cases} w_{8(j+m)+4 \rightarrow 8(j+m+1)} \otimes e_{8j+6}, & i = j + s; \\ -e_{8(j+m+1)} \otimes w_{8j+6 \rightarrow 8j+7}, & i = j + 2s; \\ 0, & \text{otherwise.} \end{cases}$$

If  $8s \leq j < 9s$ , then

$$(d_{24})_{ij} = \begin{cases} -w_{8(j+m+1) \rightarrow 8(j+m+1)+3} \otimes w_{8j+7 \rightarrow 8(j+1)}, & i = (j+1)_s; \\ (-1 + 2f(j_1, 0))w_{8(j+m+1)+1+j_1 \rightarrow 8(j+m+1)+3} \otimes w_{8j+7 \rightarrow 8(j+1)+3+j_1}, \\ \quad i = (4 + j_1)s + (j+1)_s, & 0 \leq j_1 \leq 2; \\ w_{8(j+m+1) \rightarrow 8(j+m+1)+3} \otimes e_{8j+7}, & i = j + s; \\ -w_{8(j+m)+7 \rightarrow 8(j+m+1)+3} \otimes e_{8j+7}, & i = j + 2s; \\ 0, & \text{otherwise.} \end{cases}$$

If  $9s \leq j < 10s$ , then

$$(d_{24})_{ij} = \begin{cases} -e_{8(j+m+1)+5} \otimes w_{8j+7 \rightarrow 8(j+1)+1}, & i = 2s + (j+1)_s; \\ w_{8(j+m+1) \rightarrow 8(j+m+1)+5} \otimes e_{8j+7}, & i = j; \\ 0, & \text{otherwise.} \end{cases}$$

### Description of $d_{25}$

$d_{25} : Q_{26} \rightarrow Q_{25}$  - is an  $(10s \times 8s)$  matrix.

If  $0 \leq j < s$ , then

$$(d_{25})_{ij} = \begin{cases} (-1)^{j_1} w_{8(j+m)+5+j_1-f(j_1, 0) \rightarrow 8(j+m)+7} \otimes w_{8j \rightarrow 8j+f(j_1, 2)}, \\ \quad i = j + j_1s, & 0 \leq j_1 \leq 2; \\ -e_{8(j+m)+7} \otimes w_{8j \rightarrow 8j+5}, & i = j + 6s; \\ 0, & \text{otherwise.} \end{cases}$$



If  $s \leq j < 2s$ , then

$$(d_{25})_{ij} = \begin{cases} e_{8(j+m+1)+6} \otimes w_{8j+1 \rightarrow 8(j+1)}, & i = s + (j+1)_s; \\ w_{8(j+m)+7 \rightarrow 8(j+m+1)+6} \otimes e_{8j+1}, & i = j + s; \\ w_{8(j+m+1) \rightarrow 8(j+m+1)+6} \otimes w_{8j+1 \rightarrow 8j+2}, & i = j + 2s; \\ -w_{8(j+m+1)+5 \rightarrow 8(j+m+1)+6} \otimes w_{8j+1 \rightarrow 8j+7}, & i = j + 8s; \\ 0, & \text{otherwise.} \end{cases}$$

If  $2s \leq j < 3s$ , then

$$(d_{25})_{ij} = \begin{cases} w_{8(j+m+1) \rightarrow 8(j+m+1)+1} \otimes e_{8j+2}, & i = j + s; \\ e_{8(j+m+1)+1} \otimes w_{8j+2 \rightarrow 8j+3}, & i = j + 2s; \\ 0, & \text{otherwise.} \end{cases}$$

If  $3s \leq j < 4s$ , then

$$(d_{25})_{ij} = \begin{cases} w_{8(j+m+1)+1 \rightarrow 8(j+m+1)+2} \otimes e_{8j+3}, & i = j + s; \\ e_{8(j+m+1)+2} \otimes w_{8j+3 \rightarrow 8j+4}, & i = j + 2s; \\ 0, & \text{otherwise.} \end{cases}$$

If  $4s \leq j < 5s$ , then

$$(d_{25})_{ij} = \begin{cases} w_{8(j+m+1)+2 \rightarrow 8(j+m+1)+3} \otimes e_{8j+4}, & i = j + s; \\ -e_{8(j+m+1)+3} \otimes w_{8j+4 \rightarrow 8j+7}, & i = j + 4s; \\ 0, & \text{otherwise.} \end{cases}$$

If  $5s \leq j < 6s$ , then

$$(d_{25})_{ij} = \begin{cases} e_{8(j+m+1)+4} \otimes w_{8j+5 \rightarrow 8(j+1)}, & i = (j+1)_s; \\ w_{8(j+m)+6+j_1+2f(j_1,3) \rightarrow 8(j+m+1)+4} \otimes w_{8j+5 \rightarrow 8j+4+j_1}, & i = j + j_1s, \ 1 \leq j_1 \leq 3; \\ 0, & \text{otherwise.} \end{cases}$$

If  $6s \leq j < 7s$ , then

$$(d_{25})_{ij} = \begin{cases} w_{8(j+m+1) \rightarrow 8(j+m+1)+5} \otimes e_{8j+6}, & i = j + s; \\ e_{8(j+m+1)+5} \otimes w_{8j+6 \rightarrow 8j+7}, & i = j + 3s; \\ 0, & \text{otherwise.} \end{cases}$$

If  $7s \leq j < 8s$ , then

$$(d_{25})_{ij} = \begin{cases} w_{8(j+m+1)+6+j_1-2f(j_1,0) \rightarrow 8(j+m+2)} \otimes w_{8j+7 \rightarrow 8(j+1)+j_1}, \\ \quad i = (1 + j_1 - f(j_1, 0))s + (j+1)_s, \ 0 \leq j_1 \leq 2; \\ e_{8(j+m+2)} \otimes w_{8j+7 \rightarrow 8(j+1)+6}, & i = 7s + (j+1)_s; \\ w_{8(j+m+1)+3 \rightarrow 8(j+m+2)} \otimes e_{8j+7}, & i = j + s; \\ -w_{8(j+m+1)+5 \rightarrow 8(j+m+2)} \otimes e_{8j+7}, & i = j + 2s; \\ 0, & \text{otherwise.} \end{cases}$$

#### Description of $d_{26}$

$d_{26} : Q_{27} \rightarrow Q_{26}$  – is an  $(8s \times 9s)$  matrix.

If  $0 \leq j < s$ , then

$$(d_{26})_{ij} = \begin{cases} -e_{8(j+m)+7} \otimes w_{8j \rightarrow 8(j+1)}, & i = (j+1)_s; \\ ((-1)^{j_1} + 2f(j_1, 5) - 2f(j_1, 6))w_{8(j+m-1)+7+j_1+6f(j_1, 1) \rightarrow 8(j+m)+7} \otimes w_{8j \rightarrow 8j+j_1}, \\ & i = j + j_1s, \quad 0 \leq j_1 \leq 6; \\ 0, & \text{otherwise.} \end{cases}$$

If  $s \leq j < 2s$ , then

$$(d_{26})_{ij} = \begin{cases} w_{8(j+m)+7 \rightarrow 8(j+m+1)} \otimes w_{8j+1 \rightarrow 8(j+1)}, & i = (j+1)_s; \\ (-1)^{j_1} w_{8(j+m)+j_1+6f(j_1, 0) \rightarrow 8(j+m+1)} \otimes w_{8j+1 \rightarrow 8j+1+j_1}, \\ & i = j + j_1s, \quad 0 \leq j_1 \leq 3; \\ -e_{8(j+m+1)} \otimes w_{8j+1 \rightarrow 8j+7}, & i = j + 6s; \\ 0, & \text{otherwise.} \end{cases}$$

If  $2s \leq j < 3s$ , then

$$(d_{26})_{ij} = \begin{cases} -w_{8(j+m)+7 \rightarrow 8(j+m+1)+1} \otimes w_{8j+2 \rightarrow 8(j+1)}, & i = (j+1)_s; \\ -e_{8(j+m+1)+1} \otimes w_{8j+2 \rightarrow 8(j+1)+2}, & i = 2s + (j+1)_s; \\ (-1)^{j_1} w_{8(j+m)+1+j_1 \rightarrow 8(j+m+1)+1} \otimes w_{8j+2 \rightarrow 8j+2+j_1}, & i = j + j_1s, \quad 0 \leq j_1 \leq 2; \\ w_{8(j+m+1) \rightarrow 8(j+m+1)+1} \otimes w_{8j+2 \rightarrow 8j+7}, & i = j + 5s; \\ 0, & \text{otherwise.} \end{cases}$$

If  $3s \leq j < 4s$ , then

$$(d_{26})_{ij} = \begin{cases} w_{8(j+m)+7 \rightarrow 8(j+m+1)+2} \otimes w_{8j+3 \rightarrow 8(j+1)}, & i = (j+1)_s; \\ w_{8(j+m+1)+1 \rightarrow 8(j+m+1)+2} \otimes w_{8j+3 \rightarrow 8(j+1)+2}, & i = 2s + (j+1)_s; \\ -e_{8(j+m+1)+2} \otimes w_{8j+3 \rightarrow 8(j+1)+3}, & i = 3s + (j+1)_s; \\ w_{8(j+m)+2 \rightarrow 8(j+m+1)+2} \otimes e_{8j+3}, & i = j; \\ -w_{8(j+m)+3 \rightarrow 8(j+m+1)+2} \otimes w_{8j+3 \rightarrow 8j+4}, & i = j + s; \\ -w_{8(j+m+1) \rightarrow 8(j+m+1)+2} \otimes w_{8j+3 \rightarrow 8j+7}, & i = j + 4s; \\ 0, & \text{otherwise.} \end{cases}$$

If  $4s \leq j < 5s$ , then

$$(d_{26})_{ij} = \begin{cases} -w_{8(j+m)+7 \rightarrow 8(j+m+1)+3} \otimes w_{8j+4 \rightarrow 8(j+1)}, & i = (j+1)_s; \\ (-1)^{j_1} w_{8(j+m+1)+j_1 \rightarrow 8(j+m+1)+3} \otimes w_{8j+4 \rightarrow 8(j+1)+1+j_1}, \\ & i = (1+j_1)s + (j+1)_s, \quad 1 \leq j_1 \leq 3; \\ w_{8(j+m)+3 \rightarrow 8(j+m+1)+3} \otimes e_{8j+4}, & i = j; \\ w_{8(j+m+1) \rightarrow 8(j+m+1)+3} \otimes w_{8j+4 \rightarrow 8j+7}, & i = j + 3s; \\ 0, & \text{otherwise.} \end{cases}$$

If  $5s \leq j < 6s$ , then

$$(d_{26})_{ij} = \begin{cases} (-1 + 2f(j_1, 0))w_{8(j+m)+4+j_1+2f(j_1, 2) \rightarrow 8(j+m+1)} \otimes w_{8j+5 \rightarrow 8j+5+j_1}, \\ & i = j + j_1s, \quad 0 \leq j_1 \leq 2; \\ 0, & \text{otherwise.} \end{cases}$$

If  $6s \leq j < 7s$ , then

$$(d_{26})_{ij} = \begin{cases} w_{8(j+m)+5 \rightarrow 8(j+m+1)+5} \otimes e_{8j+6}, & i = j; \\ -e_{8(j+m+1)+5} \otimes w_{8j+6 \rightarrow 8(j+1)+6}, & i = 6s + (j+1)_s; \\ w_{8(j+m+1) \rightarrow 8(j+m+1)+5} \otimes w_{8j+6 \rightarrow 8j+7}, & i = j + s; \\ 0, & \text{otherwise.} \end{cases}$$

If  $7s \leq j < 8s$ , then

$$(d_{26})_{ij} = \begin{cases} -w_{8(j+m)+7 \rightarrow 8(j+m+1)+4} \otimes w_{8j+7 \rightarrow 8(j+1)}, & i = (j+1)_s; \\ (-1 + 2f(j_1, 2))w_{8(j+m+1)+j_1 \rightarrow 8(j+m+1)+4} \otimes w_{8j+7 \rightarrow 8(j+1)+1+j_1}, & i = (1+j_1)s + (j+1)_s, \ 1 \leq j_1 \leq 4; \\ w_{8(j+m+1) \rightarrow 8(j+m+1)+4} \otimes e_{8j+7}, & i = j; \\ 0, & \text{otherwise.} \end{cases}$$

If  $8s \leq j < 9s$ , then

$$(d_{26})_{ij} = \begin{cases} -e_{8(j+m+1)+6} \otimes w_{8j+7 \rightarrow 8(j+1)+1}, & i = s + (j+1)_s; \\ -w_{8(j+m+1)+5 \rightarrow 8(j+m+1)+6} \otimes w_{8j+7 \rightarrow 8(j+1)+6}, & i = 6s + (j+1)_s; \\ w_{8(j+m+1) \rightarrow 8(j+m+1)+6} \otimes e_{8j+7}, & i = j - s; \\ 0, & \text{otherwise.} \end{cases}$$

### Description of $d_{27}$

$d_{27} : Q_{28} \rightarrow Q_{27}$  - is an  $(9s \times 8s)$  matrix.

If  $0 \leq j < s$ , then

$$(d_{27})_{ij} = \begin{cases} w_{8(j+m)+7 \rightarrow 8(j+m+1)} \otimes e_{8j}, & i = j; \\ e_{8(j+m+1)} \otimes w_{8j \rightarrow 8j+1}, & i = j + s; \\ -e_{8(j+m+1)} \otimes w_{8j \rightarrow 8j+5}, & i = j + 5s; \\ 0, & \text{otherwise.} \end{cases}$$

If  $s \leq j < 2s$ , then

$$(d_{27})_{ij} = \begin{cases} w_{8(j+m+1) \rightarrow 8(j+m+1)+1} \otimes e_{8j+1}, & i = j; \\ e_{8(j+m+1)+1} \otimes w_{8j+1 \rightarrow 8j+2}, & i = j + s; \\ 0, & \text{otherwise.} \end{cases}$$

If  $2s \leq j < 3s$ , then

$$(d_{27})_{ij} = \begin{cases} w_{8(j+m+1)+1 \rightarrow 8(j+m+1)+2} \otimes e_{8j+2}, & i = j; \\ e_{8(j+m+1)+2} \otimes w_{8j+2 \rightarrow 8j+3}, & i = j + s; \\ 0, & \text{otherwise.} \end{cases}$$

If  $3s \leq j < 4s$ , then

$$(d_{27})_{ij} = \begin{cases} w_{8(j+m+1)+2 \rightarrow 8(j+m+1)+3} \otimes e_{8j+3}, & i = j; \\ e_{8(j+m+1)+3} \otimes w_{8j+3 \rightarrow 8j+4}, & i = j + s; \\ 0, & \text{otherwise.} \end{cases}$$

If  $4s \leq j < 5s$ , then

$$(d_{27})_{ij} = \begin{cases} w_{8(j+m+1)+3 \rightarrow 8(j+m+1)+4} \otimes e_{8j+4}, & i = j; \\ -e_{8(j+m+1)+4} \otimes w_{8j+4 \rightarrow 8j+7}, & i = j + 3s; \\ 0, & \text{otherwise.} \end{cases}$$

If  $5s \leq j < 6s$ , then

$$(d_{27})_{ij} = \begin{cases} w_{8(j+m+1) \rightarrow 8(j+m+1)+5} \otimes e_{8j+5}, & i = j; \\ e_{8(j+m+1)+5} \otimes w_{8j+5 \rightarrow 8j+6}, & i = j + s; \\ 0, & \text{otherwise.} \end{cases}$$

If  $6s \leq j < 7s$ , then

$$(d_{27})_{ij} = \begin{cases} w_{8(j+m+1)+5 \rightarrow 8(j+m+1)+6} \otimes e_{8j+6}, & i = j; \\ -e_{8(j+m+1)+6} \otimes w_{8j+6 \rightarrow 8j+7}, & i = j + 2s; \\ 0, & \text{otherwise.} \end{cases}$$

If  $7s \leq j < 8s$ , then

$$(d_{27})_{ij} = \begin{cases} e_{8(j+m+1)+7} \otimes w_{8j+7 \rightarrow 8(j+1)}, & i = (j+1)_s; \\ w_{8(j+m+1)+4 \rightarrow 8(j+m+1)+7} \otimes e_{8j+7}, & i = j; \\ -w_{8(j+m+1)+6 \rightarrow 8(j+m+1)+7} \otimes e_{8j+7}, & i = j + s; \\ 0, & \text{otherwise.} \end{cases}$$

### Description of $d_{28}$

$d_{28} : Q_{29} \rightarrow Q_{28}$  - is an  $(8s \times 8s)$  matrix.

If  $0 \leq j < s$ , then

$$(d_{28})_{ij} = \begin{cases} -e_{8(j+m+1)} \otimes w_{8j \rightarrow 8(j+1)}, & i = (j+1)_s; \\ ((-1)^{j_1} + 2f(j_1, 5) - 2f(j_1, 6) + 2f(j_1, 7))w_{8(j+m)+j_1 \rightarrow 8(j+m+1)} \otimes w_{8j \rightarrow 8j+j_1}, & i = j + j_1s, \ 0 \leq j_1 \leq 7; \\ 0, & \text{otherwise.} \end{cases}$$

If  $s \leq j < 2s$ , then

$$(d_{28})_{ij} = \begin{cases} (-1)^{j_1} w_{8(j+m+1)+j_1 \rightarrow 8(j+m+1)+1} \otimes w_{8j+1 \rightarrow 8(j+1)+j_1}, & i = j_1s + (j+1)_s, \ 0 \leq j_1 \leq 1; \\ (-1)^{j_1} w_{8(j+m)+1+j_1 \rightarrow 8(j+m+1)+1} \otimes w_{8j+1 \rightarrow 8j+1+j_1}, & i = j + j_1s, \ 0 \leq j_1 \leq 3; \\ -w_{8(j+m)+7 \rightarrow 8(j+m+1)+1} \otimes w_{8j+1 \rightarrow 8j+7}, & i = j + 6s; \\ 0, & \text{otherwise.} \end{cases}$$

If  $2s \leq j < 3s$ , then

$$(d_{28})_{ij} = \begin{cases} (-1)^{j_1+1} w_{8(j+m+1)+j_1 \rightarrow 8(j+m+1)+2} \otimes w_{8j+2 \rightarrow 8(j+1)+j_1}, & i = j_1s + (j+1)_s, \ 0 \leq j_1 \leq 2; \\ (-1)^{j_1} w_{8(j+m)+2+j_1 \rightarrow 8(j+m+1)+2} \otimes w_{8j+2 \rightarrow 8j+2+j_1}, & i = j + j_1s, \ 0 \leq j_1 \leq 2; \\ w_{8(j+m)+7 \rightarrow 8(j+m+1)+2} \otimes w_{8j+2 \rightarrow 8j+7}, & i = j + 5s; \\ 0, & \text{otherwise.} \end{cases}$$

If  $3s \leq j < 4s$ , then

$$(d_{28})_{ij} = \begin{cases} (-1)^{j_1} w_{8(j+m+1)+j_1 \rightarrow 8(j+m+1)+3} \otimes w_{8j+3 \rightarrow 8(j+1)+j_1}, \\ \quad i = j_1 s + (j+1)_s, \quad 0 \leq j_1 \leq 3; \\ (-1)^{j_1} w_{8(j+m)+3+j_1 \rightarrow 8(j+m+1)+3} \otimes w_{8j+3 \rightarrow 8j+3+j_1}, \quad i = j + j_1 s, \quad 0 \leq j_1 \leq 1; \\ -w_{8(j+m)+7 \rightarrow 8(j+m+1)+3} \otimes w_{8j+3 \rightarrow 8j+7}, \quad i = j + 4s; \\ 0, \quad \text{otherwise.} \end{cases}$$

If  $4s \leq j < 5s$ , then

$$(d_{28})_{ij} = \begin{cases} (-1)^{j_1+1} w_{8(j+m+1)+j_1 \rightarrow 8(j+m+1)+4} \otimes w_{8j+4 \rightarrow 8(j+1)+j_1}, \\ \quad i = j_1 s + (j+1)_s, \quad 0 \leq j_1 \leq 4; \\ w_{8(j+m)+4 \rightarrow 8(j+m+1)+4} \otimes e_{8j+4}, \quad i = j; \\ w_{8(j+m)+7 \rightarrow 8(j+m+1)+4} \otimes w_{8j+4 \rightarrow 8j+7}, \quad i = j + 3s; \\ 0, \quad \text{otherwise.} \end{cases}$$

If  $5s \leq j < 6s$ , then

$$(d_{28})_{ij} = \begin{cases} -w_{8(j+m+1) \rightarrow 8(j+m+1)+5} \otimes w_{8j+5 \rightarrow 8(j+1)}, \quad i = (j+1)_s; \\ -e_{8(j+m+1)+5} \otimes w_{8j+5 \rightarrow 8(j+1)+5}, \quad i = 5s + (j+1)_s; \\ (-1)^{j_1} w_{8(j+m)+5+j_1 \rightarrow 8(j+m+1)+5} \otimes w_{8j+5 \rightarrow 8j+5+j_1}, \quad i = j + j_1 s, \quad 0 \leq j_1 \leq 2; \\ 0, \quad \text{otherwise.} \end{cases}$$

If  $6s \leq j < 7s$ , then

$$(d_{28})_{ij} = \begin{cases} w_{8(j+m+1) \rightarrow 8(j+m+1)+6} \otimes w_{8j+6 \rightarrow 8(j+1)}, \quad i = (j+1)_s; \\ (-1)^{j_1} w_{8(j+m+1)+5+j_1 \rightarrow 8(j+m+1)+6} \otimes w_{8j+6 \rightarrow 8(j+1)+5+j_1}, \\ \quad i = (5+j_1)s + (j+1)_s, \quad 0 \leq j_1 \leq 1; \\ (-1)^{j_1} w_{8(j+m)+6+j_1 \rightarrow 8(j+m+1)+6} \otimes w_{8j+6 \rightarrow 8j+6+j_1}, \quad i = j + j_1 s, \quad 0 \leq j_1 \leq 1; \\ 0, \quad \text{otherwise.} \end{cases}$$

If  $7s \leq j < 8s$ , then

$$(d_{28})_{ij} = \begin{cases} ((-1)^{j_1+1} - 2f(j_1, 5) + 2f(j_1, 6) - 2f(j_1, 7)) w_{8(j+m+1)+j_1 \rightarrow 8(j+m+1)+7} \otimes w_{8j+7 \rightarrow 8(j+1)+j_1}, \\ \quad i = j_1 s + (j+1)_s, \quad 0 \leq j_1 \leq 7; \\ w_{8(j+m)+7 \rightarrow 8(j+m+1)+7} \otimes e_{8j+7}, \quad i = j; \\ 0, \quad \text{otherwise.} \end{cases}$$
