# Supplementary material for: Hochschild cohomology rings for self-injective algebras of tree classes $E_7$ and $E_8$
Source: arXiv:1910.03043 ancillary file (2021-02-14)
Supplement: Supplementary file 4 [file e8-omega-shifts.pdf]

TREE CLASS  $E_8$ :  $\Omega$ -SHIFTS OF GENERATORS OF THE ALGEBRA  $\mathrm{HH}^*(R)$

**Notation.** The degree  $t$  is represented in the form  $t = 29\ell + r$  ( $0 \leq r \leq 28$ ).

**Proposition 1** (Translates for the case 1). (I) *Let  $r_0 \in \mathbb{N}$ ,  $r_0 < 29$ .  $r_0$ -translates of the elements  $Z_t^{(1)}$  are described by the following way.*

(1) *If  $r_0 = 0$ , then  $\Omega^0(Z_t^{(1)})$  is described with  $(8s \times 8s)$  matrix, whose entries  $b_{ij}$  have the following form:*

*If  $0 \leq j < 8s$ , then*

$$b_{ij} = \begin{cases} e_{8(j+m)+j_2} \otimes e_{8j+j_2}, & i = j; \\ 0, & \text{otherwise.} \end{cases}$$

(2) *If  $r_0 = 1$ , then  $\Omega^1(Z_t^{(1)})$  is described with  $(9s \times 9s)$  matrix, whose entries  $b_{ij}$  have the following form:*

*If  $0 \leq j < s$ , then*

$$b_{ij} = \begin{cases} e_{8(j+m)+1} \otimes e_{8j}, & i = j; \\ 0, & \text{otherwise.} \end{cases}$$

*If  $s \leq j < 2s$ , then*

$$b_{ij} = \begin{cases} e_{8(j+m)+5} \otimes e_{8j}, & i = j; \\ 0, & \text{otherwise.} \end{cases}$$

*If  $2s \leq j < 9s$ , then*

$$b_{ij} = \begin{cases} e_{8(j+m)+j_2+2f(j_2,5)} \otimes e_{8j+j_2-1}, & i = j; \\ 0, & \text{otherwise.} \end{cases}$$

(3) *If  $r_0 = 2$ , then  $\Omega^2(Z_t^{(1)})$  is described with  $(8s \times 8s)$  matrix, whose entries  $b_{ij}$  have the following form:*

*If  $0 \leq j < 8s$ , then*

$$b_{ij} = \begin{cases} e_{8(j+m)+j_2+1-2f(j_2,0)-6f(j_2,6)} \otimes e_{8j+j_2}, & i = j; \\ 0, & \text{otherwise.} \end{cases}$$

(4) *If  $r_0 = 3$ , then  $\Omega^3(Z_t^{(1)})$  is described with  $(10s \times 10s)$  matrix, whose entries  $b_{ij}$  have the following form:*

*If  $0 \leq j < s$ , then*

$$b_{ij} = \begin{cases} e_{8(j+m)+2} \otimes e_{8j}, & i = j; \\ 0, & \text{otherwise.} \end{cases}$$

*If  $s \leq j < 2s$ , then*

$$b_{ij} = \begin{cases} e_{8(j+m)+6} \otimes e_{8j}, & i = j; \\ 0, & \text{otherwise.} \end{cases}$$

*If  $2s \leq j < 9s$ , then*

$$b_{ij} = \begin{cases} e_{8(j+m)+j_2+1+2f(j_2,4,5)} \otimes e_{8j+j_2-1}, & i = j; \\ 0, & \text{otherwise.} \end{cases}$$

If  $9s \leq j < 10s$ , then

$$b_{ij} = \begin{cases} e_{8(j+m+1)+5} \otimes e_{8j+7}, & i = j; \\ 0, & \text{otherwise.} \end{cases}$$

(5) If  $r_0 = 4$ , then  $\Omega^4(Z_t^{(1)})$  is described with  $(11s \times 11s)$  matrix, whose entries  $b_{ij}$  have the following form:

If  $0 \leq j < s$ , then

$$b_{ij} = \begin{cases} e_{8(j+m-1)+7} \otimes e_{8j}, & i = j; \\ 0, & \text{otherwise.} \end{cases}$$

If  $s \leq j < 2s$ , then

$$b_{ij} = \begin{cases} e_{8(j+m)} \otimes e_{8j}, & i = j; \\ 0, & \text{otherwise.} \end{cases}$$

If  $2s \leq j < 6s$ , then

$$b_{ij} = \begin{cases} e_{8(j+m)+j_2+1} \otimes e_{8j+j_2-1}, & i = j; \\ 0, & \text{otherwise.} \end{cases}$$

If  $6s \leq j < 9s$ , then

$$b_{ij} = \begin{cases} e_{8(j+m)+1+f(j_2,8)} \otimes e_{8j+j_2-2}, & i = j; \\ 0, & \text{otherwise.} \end{cases}$$

If  $9s \leq j < 10s$ , then

$$b_{ij} = \begin{cases} e_{8(j+m)+5} \otimes e_{8j+6}, & i = j; \\ 0, & \text{otherwise.} \end{cases}$$

If  $10s \leq j < 11s$ , then

$$b_{ij} = \begin{cases} e_{8(j+m)+7} \otimes e_{8j+7}, & i = j; \\ 0, & \text{otherwise.} \end{cases}$$

(6) If  $r_0 = 5$ , then  $\Omega^5(Z_t^{(1)})$  is described with  $(11s \times 11s)$  matrix, whose entries  $b_{ij}$  have the following form:

If  $0 \leq j < 3s$ , then

$$b_{ij} = \begin{cases} e_{8(j+m)+5-2j_2} \otimes e_{8j}, & i = j; \\ 0, & \text{otherwise.} \end{cases}$$

If  $3s \leq j < 4s$ , then

$$b_{ij} = \begin{cases} e_{8(j+m)+4} \otimes e_{8j+1}, & i = j; \\ 0, & \text{otherwise.} \end{cases}$$

If  $4s \leq j < 9s$ , then

$$b_{ij} = \begin{cases} e_{8(j+m)+7+f(j_2,5)+f(j_2,7)} \otimes e_{8j+j_2-2}, & i = j; \\ 0, & \text{otherwise.} \end{cases}$$

If  $9s \leq j < 10s$ , then

$$b_{ij} = \begin{cases} e_{8(j+m+1)+2} \otimes e_{8j+7}, & i = j; \\ 0, & \text{otherwise.} \end{cases}$$

If  $10s \leq j < 11s$ , then

$$b_{ij} = \begin{cases} e_{8(j+m+1)+6} \otimes e_{8j+7}, & i = j; \\ 0, & \text{otherwise.} \end{cases}$$

(7) If  $r_0 = 6$ , then  $\Omega^6(Z_t^{(1)})$  is described with  $(13s \times 13s)$  matrix, whose entries  $b_{ij}$  have the following form:

If  $0 \leq j < 2s$ , then

$$b_{ij} = \begin{cases} e_{8(j+m-1)+7+j_2} \otimes e_{8j}, & i = j; \\ 0, & \text{otherwise.} \end{cases}$$

If  $2s \leq j < 5s$ , then

$$b_{ij} = \begin{cases} e_{8(j+m)+j_2+2} \otimes e_{8j+j_2-1}, & i = j; \\ 0, & \text{otherwise.} \end{cases}$$

If  $5s \leq j < 6s$ , then

$$b_{ij} = \begin{cases} e_{8(j+m)+1} \otimes e_{8j+3}, & i = j; \\ 0, & \text{otherwise.} \end{cases}$$

If  $6s \leq j < 7s$ , then

$$b_{ij} = \begin{cases} e_{8(j+m)+2} \otimes e_{8j+4}, & i = j; \\ 0, & \text{otherwise.} \end{cases}$$

If  $7s \leq j < 8s$ , then

$$b_{ij} = \begin{cases} e_{8(j+m)+2} \otimes e_{8j+5}, & i = j; \\ 0, & \text{otherwise.} \end{cases}$$

If  $8s \leq j < 9s$ , then

$$b_{ij} = \begin{cases} e_{8(j+m)+5} \otimes e_{8j+5}, & i = j; \\ 0, & \text{otherwise.} \end{cases}$$

If  $9s \leq j < 10s$ , then

$$b_{ij} = \begin{cases} e_{8(j+m)+3} \otimes e_{8j+6}, & i = j; \\ 0, & \text{otherwise.} \end{cases}$$

If  $10s \leq j < 13s$ , then

$$b_{ij} = \begin{cases} e_{8(j+m)+j_2-4} \otimes e_{8j+7-f(j_2,10)}, & i = j; \\ 0, & \text{otherwise.} \end{cases}$$

(8) If  $r_0 = 7$ , then  $\Omega^7(Z_t^{(1)})$  is described with  $(14s \times 14s)$  matrix, whose entries  $b_{ij}$  have the following form:

If  $0 \leq j < s$ , then

$$b_{ij} = \begin{cases} e_{8(j+m)+2} \otimes e_{8j}, & i = j; \\ 0, & \text{otherwise.} \end{cases}$$

If  $s \leq j < 2s$ , then

$$b_{ij} = \begin{cases} e_{8(j+m)+4} \otimes e_{8j}, & i = j; \\ 0, & \text{otherwise.} \end{cases}$$

If  $2s \leq j < 3s$ , then

$$b_{ij} = \begin{cases} e_{8(j+m)+6} \otimes e_{8j}, & i = j; \\ 0, & \text{otherwise.} \end{cases}$$

If  $3s \leq j < 4s$ , then

$$b_{ij} = \begin{cases} e_{8(j+m)+5} \otimes e_{8j}, & i = j; \\ 0, & \text{otherwise.} \end{cases}$$

If  $4s \leq j < 10s$ , then

$$b_{ij} = \begin{cases} e_{8(j+m)+7+f(j_2,5)+f(j_2,7)} \otimes e_{8j+j_2-3}, & i = j; \\ 0, & \text{otherwise.} \end{cases}$$

If  $10s \leq j < 11s$ , then

$$b_{ij} = \begin{cases} e_{8(j+m+1)} \otimes e_{8j+6}, & i = j; \\ 0, & \text{otherwise.} \end{cases}$$

If  $11s \leq j < 14s$ , then

$$b_{ij} = \begin{cases} e_{8(j+m+1)+27-2j_2} \otimes e_{8j+7}, & i = j; \\ 0, & \text{otherwise.} \end{cases}$$

(9) If  $r_0 = 8$ , then  $\Omega^8(Z_t^{(1)})$  is described with  $(16s \times 16s)$  matrix, whose entries  $b_{ij}$  have the following form:

If  $0 \leq j < 3s$ , then

$$b_{ij} = \begin{cases} e_{8(j+m-1)+7+f(j_2,2)} \otimes e_{8j}, & i = j; \\ 0, & \text{otherwise.} \end{cases}$$

If  $3s \leq j < 5s$ , then

$$b_{ij} = \begin{cases} e_{8(j+m)+j_2+2} \otimes e_{8j+j_2-2}, & i = j; \\ 0, & \text{otherwise.} \end{cases}$$

If  $5s \leq j < 8s$ , then

$$b_{ij} = \begin{cases} e_{8(j+m)+j_2-4} \otimes e_{8j+j_2-3}, & i = j; \\ 0, & \text{otherwise.} \end{cases}$$

If  $8s \leq j < 9s$ , then

$$b_{ij} = \begin{cases} e_{8(j+m)+5} \otimes e_{8j+4}, & i = j; \\ 0, & \text{otherwise.} \end{cases}$$

If  $9s \leq j < 10s$ , then

$$b_{ij} = \begin{cases} e_{8(j+m)+3} \otimes e_{8j+5}, & i = j; \\ 0, & \text{otherwise.} \end{cases}$$

If  $10s \leq j < 13s$ , then

$$b_{ij} = \begin{cases} e_{8(j+m)+16-j_2} \otimes e_{8j+6-f(j_2,10)}, & i = j; \\ 0, & \text{otherwise.} \end{cases}$$

If  $13s \leq j < 14s$ , then

$$b_{ij} = \begin{cases} e_{8(j+m)+1} \otimes e_{8j+6}, & i = j; \\ 0, & \text{otherwise.} \end{cases}$$

If  $14s \leq j < 16s$ , then

$$b_{ij} = \begin{cases} e_{8(j+m)+j_2-7} \otimes e_{8j+7}, & i = j; \\ 0, & \text{otherwise.} \end{cases}$$

(10) If  $r_0 = 9$ , then  $\Omega^9(Z_t^{(1)})$  is described with  $(16s \times 16s)$  matrix, whose entries  $b_{ij}$  have the following form:

If  $0 \leq j < s$ , then

$$b_{ij} = \begin{cases} e_{8(j+m)+5} \otimes e_{8j}, & i = j; \\ 0, & \text{otherwise.} \end{cases}$$

If  $s \leq j < 2s$ , then

$$b_{ij} = \begin{cases} e_{8(j+m)+3} \otimes e_{8j}, & i = j; \\ 0, & \text{otherwise.} \end{cases}$$

If  $2s \leq j < 3s$ , then

$$b_{ij} = \begin{cases} e_{8(j+m)+6} \otimes e_{8j}, & i = j; \\ 0, & \text{otherwise.} \end{cases}$$

If  $3s \leq j < 4s$ , then

$$b_{ij} = \begin{cases} e_{8(j+m)+1} \otimes e_{8j}, & i = j; \\ 0, & \text{otherwise.} \end{cases}$$

If  $4s \leq j < 12s$ , then

$$b_{ij} = \begin{cases} e_{8(j+m+1)-f(j_2,5)-f(j_2,7,8)-f(j_2,10)} \otimes e_{8j+j_2-3-f(j_2,9,11)-f(j_2,11)}, & i = j; \\ 0, & \text{otherwise.} \end{cases}$$

If  $12s \leq j < 15s$ , then

$$b_{ij} = \begin{cases} e_{8(j+m+1)+2(j_2-11)} \otimes e_{8j+7}, & i = j; \\ 0, & \text{otherwise.} \end{cases}$$

If  $15s \leq j < 16s$ , then

$$b_{ij} = \begin{cases} e_{8(j+m+1)+5} \otimes e_{8j+7}, & i = j; \\ 0, & \text{otherwise.} \end{cases}$$

(11) If  $r_0 = 10$ , then  $\Omega^{10}(Z_t^{(1)})$  is described with  $(19s \times 19s)$  matrix, whose entries  $b_{ij}$  have the following form:

If  $0 \leq j < 3s$ , then

$$b_{ij} = \begin{cases} e_{8(j+m)-f(j_2,0)} \otimes e_{8j}, & i = j; \\ 0, & \text{otherwise.} \end{cases}$$

If  $3s \leq j < 4s$ , then

$$b_{ij} = \begin{cases} e_{8(j+m)+6} \otimes e_{8j+1}, & i = j; \\ 0, & \text{otherwise.} \end{cases}$$

If  $4s \leq j < 7s$ , then

$$b_{ij} = \begin{cases} e_{8(j+m)+j_2-3} \otimes e_{8j+j_2-3}, & i = j; \\ 0, & \text{otherwise.} \end{cases}$$

If  $7s \leq j < 8s$ , then

$$b_{ij} = \begin{cases} e_{8(j+m)+5} \otimes e_{8j+3}, & i = j; \\ 0, & \text{otherwise.} \end{cases}$$

If  $8s \leq j < 9s$ , then

$$b_{ij} = \begin{cases} e_{8(j+m)+4} \otimes e_{8j+4}, & i = j; \\ 0, & \text{otherwise.} \end{cases}$$

If  $9s \leq j < 12s$ , then

$$b_{ij} = \begin{cases} e_{8(j+m)+15-j_2} \otimes e_{8j+5-f(j_2,9)}, & i = j; \\ 0, & \text{otherwise.} \end{cases}$$

If  $12s \leq j < 14s$ , then

$$b_{ij} = \begin{cases} e_{8(j+m)+j_2-11} \otimes e_{8j+j_2-7}, & i = j; \\ 0, & \text{otherwise.} \end{cases}$$

If  $14s \leq j < 15s$ , then

$$b_{ij} = \begin{cases} e_{8(j+m)+6} \otimes e_{8j+6}, & i = j; \\ 0, & \text{otherwise.} \end{cases}$$

If  $15s \leq j < 16s$ , then

$$b_{ij} = \begin{cases} e_{8(j+m)+5} \otimes e_{8j+6}, & i = j; \\ 0, & \text{otherwise.} \end{cases}$$

If  $16s \leq j < 19s$ , then

$$b_{ij} = \begin{cases} e_{8(j+m)+7+f(j_2,18)} \otimes e_{8j+7}, & i = j; \\ 0, & \text{otherwise.} \end{cases}$$

(12) If  $r_0 = 11$ , then  $\Omega^{11}(Z_t^{(1)})$  is described with  $(18s \times 18s)$  matrix, whose entries  $b_{ij}$  have the following form:

If  $0 \leq j < s$ , then

$$b_{ij} = \begin{cases} e_{8(j+m)+2} \otimes e_{8j}, & i = j; \\ 0, & \text{otherwise.} \end{cases}$$

If  $s \leq j < 2s$ , then

$$b_{ij} = \begin{cases} e_{8(j+m)+6} \otimes e_{8j}, & i = j; \\ 0, & \text{otherwise.} \end{cases}$$

If  $2s \leq j < 3s$ , then

$$b_{ij} = \begin{cases} e_{8(j+m)+4} \otimes e_{8j}, & i = j; \\ 0, & \text{otherwise.} \end{cases}$$

If  $3s \leq j < 4s$ , then

$$b_{ij} = \begin{cases} e_{8(j+m)+1} \otimes e_{8j}, & i = j; \\ 0, & \text{otherwise.} \end{cases}$$

If  $4s \leq j < 5s$ , then

$$b_{ij} = \begin{cases} e_{8(j+m)+5} \otimes e_{8j}, & i = j; \\ 0, & \text{otherwise.} \end{cases}$$

If  $5s \leq j < 14s$ , then

$$b_{ij} = \begin{cases} e_{8(j+m)+7+f(j_2,6)+f(j_2,9)+f(j_2,11)+f(j_2,13)} \otimes e_{8j+j_2-4-f(j_2,9,13)-f(j_2,11,13)-f(j_2,13)}, & i = j; \\ 0, & \text{otherwise.} \end{cases}$$

If  $14s \leq j < 15s$ , then

$$b_{ij} = \begin{cases} e_{8(j+m+1)+5} \otimes e_{8j+7}, & i = j; \\ 0, & \text{otherwise.} \end{cases}$$

If  $15s \leq j < 16s$ , then

$$b_{ij} = \begin{cases} e_{8(j+m+1)+3} \otimes e_{8j+7}, & i = j; \\ 0, & \text{otherwise.} \end{cases}$$

If  $16s \leq j < 17s$ , then

$$b_{ij} = \begin{cases} e_{8(j+m+1)+6} \otimes e_{8j+7}, & i = j; \\ 0, & \text{otherwise.} \end{cases}$$

If  $17s \leq j < 18s$ , then

$$b_{ij} = \begin{cases} e_{8(j+m+1)+1} \otimes e_{8j+7}, & i = j; \\ 0, & \text{otherwise.} \end{cases}$$

(13) If  $r_0 = 12$ , then  $\Omega^{12}(Z_t^{(1)})$  is described with  $(19s \times 19s)$  matrix, whose entries  $b_{ij}$  have the following form:

If  $0 \leq j < 3s$ , then

$$b_{ij} = \begin{cases} e_{8(j+m-1)+7+f(j_2,1)} \otimes e_{8j}, & i = j; \\ 0, & \text{otherwise.} \end{cases}$$

If  $3s \leq j < 4s$ , then

$$b_{ij} = \begin{cases} e_{8(j+m)+2} \otimes e_{8j+1}, & i = j; \\ 0, & \text{otherwise.} \end{cases}$$

If  $4s \leq j < 5s$ , then

$$b_{ij} = \begin{cases} e_{8(j+m)+3} \otimes e_{8j+2}, & i = j; \\ 0, & \text{otherwise.} \end{cases}$$

If  $5s \leq j < 6s$ , then

$$b_{ij} = \begin{cases} e_{8(j+m)+5} \otimes e_{8j+2}, & i = j; \\ 0, & \text{otherwise.} \end{cases}$$

If  $6s \leq j < 7s$ , then

$$b_{ij} = \begin{cases} e_{8(j+m)+4} \otimes e_{8j+3}, & i = j; \\ 0, & \text{otherwise.} \end{cases}$$

If  $7s \leq j < 8s$ , then

$$b_{ij} = \begin{cases} e_{8(j+m)+6} \otimes e_{8j+3}, & i = j; \\ 0, & \text{otherwise.} \end{cases}$$

If  $8s \leq j < 9s$ , then

$$b_{ij} = \begin{cases} e_{8(j+m)+5} \otimes e_{8j+4}, & i = j; \\ 0, & \text{otherwise.} \end{cases}$$

If  $9s \leq j < 11s$ , then

$$b_{ij} = \begin{cases} e_{8(j+m)+j_2-8} \otimes e_{8j+j_2-5}, & i = j; \\ 0, & \text{otherwise.} \end{cases}$$

If  $11s \leq j < 12s$ , then

$$b_{ij} = \begin{cases} e_{8(j+m)+6} \otimes e_{8j+5}, & i = j; \\ 0, & \text{otherwise.} \end{cases}$$

If  $12s \leq j < 13s$ , then

$$b_{ij} = \begin{cases} e_{8(j+m)+5} \otimes e_{8j+5}, & i = j; \\ 0, & \text{otherwise.} \end{cases}$$

If  $13s \leq j < 16s$ , then

$$b_{ij} = \begin{cases} e_{8(j+m)+6-3f(j_2,14)-5f(j_2,15)} \otimes e_{8j+6}, & i = j; \\ 0, & \text{otherwise.} \end{cases}$$

If  $16s \leq j < 19s$ , then

$$b_{ij} = \begin{cases} e_{8(j+m+1)-f(j_2,16)} \otimes e_{8j+7}, & i = j; \\ 0, & \text{otherwise.} \end{cases}$$

(14) If  $r_0 = 13$ , then  $\Omega^{13}(Z_t^{(1)})$  is described with  $(18s \times 18s)$  matrix, whose entries  $b_{ij}$  have the following form:

If  $0 \leq j < 4s$ , then

$$b_{ij} = \begin{cases} e_{8(j+m)+2+j_2+2f(j_2,2)} \otimes e_{8j}, & i = j; \\ 0, & \text{otherwise.} \end{cases}$$

If  $4s \leq j < 5s$ , then

$$b_{ij} = \begin{cases} e_{8(j+m+1)} \otimes e_{8j+1}, & i = j; \\ 0, & \text{otherwise.} \end{cases}$$

If  $5s \leq j < 13s$ , then

$$b_{ij} = \begin{cases} e_{8(j+m)+7+f(j_2,7,8)+f(j_2,10)+f(j_2,12)} \otimes e_{8j+j_2-3-f(j_2,7,12)-f(j_2,10,12)-f(j_2,12)}, & i = j; \\ 0, & \text{otherwise.} \end{cases}$$



If  $13s \leq j < 16s$ , then

$$b_{ij} = \begin{cases} e_{8(j+m+1)+j_2-11+3f(j_2,14)} \otimes e_{8j+7}, & i = j; \\ 0, & \text{otherwise.} \end{cases}$$

If  $16s \leq j < 17s$ , then

$$b_{ij} = \begin{cases} e_{8(j+m+1)+1} \otimes e_{8j+7}, & i = j; \\ 0, & \text{otherwise.} \end{cases}$$

If  $17s \leq j < 18s$ , then

$$b_{ij} = \begin{cases} e_{8(j+m+1)+5} \otimes e_{8j+7}, & i = j; \\ 0, & \text{otherwise.} \end{cases}$$

(15) If  $r_0 = 14$ , then  $\Omega^{14}(Z_t^{(1)})$  is described with  $(20s \times 20s)$  matrix, whose entries  $b_{ij}$  have the following form:

If  $0 \leq j < 3s$ , then

$$b_{ij} = \begin{cases} e_{8(j+m)-f(j_2,0)} \otimes e_{8j}, & i = j; \\ 0, & \text{otherwise.} \end{cases}$$

If  $3s \leq j < 4s$ , then

$$b_{ij} = \begin{cases} e_{8(j+m)+3} \otimes e_{8j+1}, & i = j; \\ 0, & \text{otherwise.} \end{cases}$$

If  $4s \leq j < 5s$ , then

$$b_{ij} = \begin{cases} e_{8(j+m)+5} \otimes e_{8j+1}, & i = j; \\ 0, & \text{otherwise.} \end{cases}$$

If  $5s \leq j < 6s$ , then

$$b_{ij} = \begin{cases} e_{8(j+m)+4} \otimes e_{8j+2}, & i = j; \\ 0, & \text{otherwise.} \end{cases}$$

If  $6s \leq j < 7s$ , then

$$b_{ij} = \begin{cases} e_{8(j+m)+6} \otimes e_{8j+2}, & i = j; \\ 0, & \text{otherwise.} \end{cases}$$

If  $7s \leq j < 8s$ , then

$$b_{ij} = \begin{cases} e_{8(j+m)+5} \otimes e_{8j+3}, & i = j; \\ 0, & \text{otherwise.} \end{cases}$$

If  $8s \leq j < 9s$ , then

$$b_{ij} = \begin{cases} e_{8(j+m)+1} \otimes e_{8j+3}, & i = j; \\ 0, & \text{otherwise.} \end{cases}$$

If  $9s \leq j < 10s$ , then

$$b_{ij} = \begin{cases} e_{8(j+m)+2} \otimes e_{8j+4}, & i = j; \\ 0, & \text{otherwise.} \end{cases}$$

If  $10s \leq j < 11s$ , then

$$b_{ij} = \begin{cases} e_{8(j+m)+6} \otimes e_{8j+4}, & i = j; \\ 0, & \text{otherwise.} \end{cases}$$

If  $11s \leq j < 14s$ , then

$$b_{ij} = \begin{cases} e_{8(j+m)+6-3f(j_2,12)-5f(j_2,13)} \otimes e_{8j+5}, & i = j; \\ 0, & \text{otherwise.} \end{cases}$$

If  $14s \leq j < 17s$ , then

$$b_{ij} = \begin{cases} e_{8(j+m)+j_2-11-f(j_2,14)} \otimes e_{8j+6}, & i = j; \\ 0, & \text{otherwise.} \end{cases}$$

If  $17s \leq j < 20s$ , then

$$b_{ij} = \begin{cases} e_{8(j+m)+7+f(j_2,18)} \otimes e_{8j+7}, & i = j; \\ 0, & \text{otherwise.} \end{cases}$$

(16) If  $r_0 = 15$ , then  $\Omega^{15}(Z_t^{(1)})$  is described with  $(18s \times 18s)$  matrix, whose entries  $b_{ij}$  have the following form:

If  $0 \leq j < 3s$ , then

$$b_{ij} = \begin{cases} e_{8(j+m)+3(j_2+1)-5f(j_2,2)} \otimes e_{8j}, & i = j; \\ 0, & \text{otherwise.} \end{cases}$$

If  $3s \leq j < 4s$ , then

$$b_{ij} = \begin{cases} e_{8(j+m)+1} \otimes e_{8j}, & i = j; \\ 0, & \text{otherwise.} \end{cases}$$

If  $4s \leq j < 5s$ , then

$$b_{ij} = \begin{cases} e_{8(j+m)+5} \otimes e_{8j}, & i = j; \\ 0, & \text{otherwise.} \end{cases}$$

If  $5s \leq j < 14s$ , then

$$b_{ij} = \begin{cases} e_{8(j+m)+7+f(j_2,7,8)+f(j_2,11,12)} \otimes e_{8j+j_2-4-f(j_2,7,13)-f(j_2,11,13)-f(j_2,13)}, & i = j; \\ 0, & \text{otherwise.} \end{cases}$$

If  $14s \leq j < 18s$ , then

$$b_{ij} = \begin{cases} e_{8(j+m+1)+j_2-12+2f(j_2,16)} \otimes e_{8j+7}, & i = j; \\ 0, & \text{otherwise.} \end{cases}$$

(17) If  $r_0 = 16$ , then  $\Omega^{16}(Z_t^{(1)})$  is described with  $(19s \times 19s)$  matrix, whose entries  $b_{ij}$  have the following form:

If  $0 \leq j < 3s$ , then

$$b_{ij} = \begin{cases} e_{8(j+m-1)+7+f(j_2,1)} \otimes e_{8j}, & i = j; \\ 0, & \text{otherwise.} \end{cases}$$

If  $3s \leq j < 4s$ , then

$$b_{ij} = \begin{cases} e_{8(j+m)+4} \otimes e_{8j+1}, & i = j; \\ 0, & \text{otherwise.} \end{cases}$$

If  $4s \leq j < 5s$ , then

$$b_{ij} = \begin{cases} e_{8(j+m)+6} \otimes e_{8j+1}, & i = j; \\ 0, & \text{otherwise.} \end{cases}$$

If  $5s \leq j < 6s$ , then

$$b_{ij} = \begin{cases} e_{8(j+m)+5} \otimes e_{8j+2}, & i = j; \\ 0, & \text{otherwise.} \end{cases}$$

If  $6s \leq j < 7s$ , then

$$b_{ij} = \begin{cases} e_{8(j+m)+1} \otimes e_{8j+2}, & i = j; \\ 0, & \text{otherwise.} \end{cases}$$

If  $7s \leq j < 8s$ , then

$$b_{ij} = \begin{cases} e_{8(j+m)+2} \otimes e_{8j+3}, & i = j; \\ 0, & \text{otherwise.} \end{cases}$$

If  $8s \leq j < 9s$ , then

$$b_{ij} = \begin{cases} e_{8(j+m)+6} \otimes e_{8j+3}, & i = j; \\ 0, & \text{otherwise.} \end{cases}$$

If  $9s \leq j < 10s$ , then

$$b_{ij} = \begin{cases} e_{8(j+m)+3} \otimes e_{8j+4}, & i = j; \\ 0, & \text{otherwise.} \end{cases}$$

If  $10s \leq j < 13s$ , then

$$b_{ij} = \begin{cases} e_{8(j+m)+j_2-7-f(j_2,10)} \otimes e_{8j+5}, & i = j; \\ 0, & \text{otherwise.} \end{cases}$$

If  $13s \leq j < 16s$ , then

$$b_{ij} = \begin{cases} e_{8(j+m)+j_2-10+2f(j_2,14)} \otimes e_{8j+6}, & i = j; \\ 0, & \text{otherwise.} \end{cases}$$

If  $16s \leq j < 19s$ , then

$$b_{ij} = \begin{cases} e_{8(j+m+1)-f(j_2,16)} \otimes e_{8j+7}, & i = j; \\ 0, & \text{otherwise.} \end{cases}$$

(18) If  $r_0 = 17$ , then  $\Omega^{17}(Z_t^{(1)})$  is described with  $(18s \times 18s)$  matrix, whose entries  $b_{ij}$  have the following form:

If  $0 \leq j < 4s$ , then

$$b_{ij} = \begin{cases} e_{8(j+m)+2(j_2+1)-3f(j_2,3)} \otimes e_{8j}, & i = j; \\ 0, & \text{otherwise.} \end{cases}$$

If  $4s \leq j < 13s$ , then

$$b_{ij} = \begin{cases} e_{8(j+m)+7+f(j_2,5,6)+f(j_2,8,9)+f(j_2,12)} \otimes e_{8j+j_2-3-f(j_2,5,12)-f(j_2,10,12)-f(j_2,12)}, & i = j; \\ 0, & \text{otherwise.} \end{cases}$$

If  $13s \leq j < 16s$ , then

$$b_{ij} = \begin{cases} e_{8(j+m+1)+3(j_2-12)-5f(j_2,15)} \otimes e_{8j+7}, & i = j; \\ 0, & \text{otherwise.} \end{cases}$$

If  $16s \leq j < 17s$ , then

$$b_{ij} = \begin{cases} e_{8(j+m+1)+1} \otimes e_{8j+7}, & i = j; \\ 0, & \text{otherwise.} \end{cases}$$

If  $17s \leq j < 18s$ , then

$$b_{ij} = \begin{cases} e_{8(j+m+1)+5} \otimes e_{8j+7}, & i = j; \\ 0, & \text{otherwise.} \end{cases}$$

(19) If  $r_0 = 18$ , then  $\Omega^{18}(Z_t^{(1)})$  is described with  $(19s \times 19s)$  matrix, whose entries  $b_{ij}$  have the following form:

If  $0 \leq j < 3s$ , then

$$b_{ij} = \begin{cases} e_{8(j+m)-f(j_2,0)} \otimes e_{8j}, & i = j; \\ 0, & \text{otherwise.} \end{cases}$$

If  $3s \leq j < 4s$ , then

$$b_{ij} = \begin{cases} e_{8(j+m)+5} \otimes e_{8j+1}, & i = j; \\ 0, & \text{otherwise.} \end{cases}$$

If  $4s \leq j < 6s$ , then

$$b_{ij} = \begin{cases} e_{8(j+m)+j_2-3} \otimes e_{8j+j_2-3}, & i = j; \\ 0, & \text{otherwise.} \end{cases}$$

If  $6s \leq j < 7s$ , then

$$b_{ij} = \begin{cases} e_{8(j+m)+6} \otimes e_{8j+2}, & i = j; \\ 0, & \text{otherwise.} \end{cases}$$

If  $7s \leq j < 10s$ , then

$$b_{ij} = \begin{cases} e_{8(j+m)+j_2-4} \otimes e_{8j+4-f(j_2,7)}, & i = j; \\ 0, & \text{otherwise.} \end{cases}$$

If  $10s \leq j < 13s$ , then

$$b_{ij} = \begin{cases} e_{8(j+m)+j_2-7+2f(j_2,11)} \otimes e_{8j+5}, & i = j; \\ 0, & \text{otherwise.} \end{cases}$$

If  $13s \leq j < 16s$ , then

$$b_{ij} = \begin{cases} e_{8(j+m)+2(16-j_2)-f(j_2,15)} \otimes e_{8j+6}, & i = j; \\ 0, & \text{otherwise.} \end{cases}$$

If  $16s \leq j < 19s$ , then

$$b_{ij} = \begin{cases} e_{8(j+m)+7+f(j_2,17)} \otimes e_{8j+7}, & i = j; \\ 0, & \text{otherwise.} \end{cases}$$

(20) If  $r_0 = 19$ , then  $\Omega^{19}(Z_t^{(1)})$  is described with  $(16s \times 16s)$  matrix, whose entries  $b_{ij}$  have the following form:

If  $0 \leq j < 3s$ , then

$$b_{ij} = \begin{cases} e_{8(j+m)+3-j_2+4f(j_2,1)} \otimes e_{8j}, & i = j; \\ 0, & \text{otherwise.} \end{cases}$$

If  $3s \leq j < 4s$ , then

$$b_{ij} = \begin{cases} e_{8(j+m)+5} \otimes e_{8j}, & i = j; \\ 0, & \text{otherwise.} \end{cases}$$

If  $4s \leq j < 12s$ , then

$$b_{ij} = \begin{cases} e_{8(j+m+1)-f(j_2,5)-f(j_2,7,8)-f(j_2,10)} \otimes e_{8j+j_2-3-f(j_2,9,11)-f(j_2,11)}, & i = j; \\ 0, & \text{otherwise.} \end{cases}$$

If  $12s \leq j < 16s$ , then

$$b_{ij} = \begin{cases} e_{8(j+m+1)+2(j_2-11)-3f(j_2,15)} \otimes e_{8j+7}, & i = j; \\ 0, & \text{otherwise.} \end{cases}$$

(21) If  $r_0 = 20$ , then  $\Omega^{20}(Z_t^{(1)})$  is described with  $(16s \times 16s)$  matrix, whose entries  $b_{ij}$  have the following form:

If  $0 \leq j < 2s$ , then

$$b_{ij} = \begin{cases} e_{8(j+m-1)+7+j_2} \otimes e_{8j}, & i = j; \\ 0, & \text{otherwise.} \end{cases}$$

If  $2s \leq j < 3s$ , then

$$b_{ij} = \begin{cases} e_{8(j+m)+2} \otimes e_{8j+1}, & i = j; \\ 0, & \text{otherwise.} \end{cases}$$

If  $3s \leq j < 4s$ , then

$$b_{ij} = \begin{cases} e_{8(j+m)+6} \otimes e_{8j+1}, & i = j; \\ 0, & \text{otherwise.} \end{cases}$$

If  $4s \leq j < 8s$ , then

$$b_{ij} = \begin{cases} e_{8(j+m)+j_2-1} \otimes e_{8j+j_2-2-f(j_2,6,7)}, & i = j; \\ 0, & \text{otherwise.} \end{cases}$$

If  $8s \leq j < 11s$ , then

$$b_{ij} = \begin{cases} e_{8(j+m)+2(11-j_2)-f(j_2,10)} \otimes e_{8j+5}, & i = j; \\ 0, & \text{otherwise.} \end{cases}$$

If  $11s \leq j < 12s$ , then

$$b_{ij} = \begin{cases} e_{8(j+m)+2} \otimes e_{8j+6}, & i = j; \\ 0, & \text{otherwise.} \end{cases}$$

If  $12s \leq j < 13s$ , then

$$b_{ij} = \begin{cases} e_{8(j+m)+5} \otimes e_{8j+6}, & i = j; \\ 0, & \text{otherwise.} \end{cases}$$

If  $13s \leq j < 16s$ , then

$$b_{ij} = \begin{cases} e_{8(j+m+1)-f(j_2,13)} \otimes e_{8j+7}, & i = j; \\ 0, & \text{otherwise.} \end{cases}$$

(22) If  $r_0 = 21$ , then  $\Omega^{21}(Z_t^{(1)})$  is described with  $(14s \times 14s)$  matrix, whose entries  $b_{ij}$  have the following form:

If  $0 \leq j < 3s$ , then

$$b_{ij} = \begin{cases} e_{8(j+m)+2(j_2+1)} \otimes e_{8j}, & i = j; \\ 0, & \text{otherwise.} \end{cases}$$

If  $3s \leq j < 10s$ , then

$$b_{ij} = \begin{cases} e_{8(j+m+1)-f(j_2,3)-f(j_2,5)-f(j_2,7)} \otimes e_{8j+j_2-2-f(j_2,8,9)}, & i = j; \\ 0, & \text{otherwise.} \end{cases}$$

If  $10s \leq j < 13s$ , then

$$b_{ij} = \begin{cases} e_{8(j+m+1)+3(j_2-9)-8f(j_2,12)} \otimes e_{8j+7}, & i = j; \\ 0, & \text{otherwise.} \end{cases}$$

If  $13s \leq j < 14s$ , then

$$b_{ij} = \begin{cases} e_{8(j+m+1)+5} \otimes e_{8j+7}, & i = j; \\ 0, & \text{otherwise.} \end{cases}$$

(23) If  $r_0 = 22$ , then  $\Omega^{22}(Z_t^{(1)})$  is described with  $(13s \times 13s)$  matrix, whose entries  $b_{ij}$  have the following form:

If  $0 \leq j < s$ , then

$$b_{ij} = \begin{cases} e_{8(j+m)} \otimes e_{8j}, & i = j; \\ 0, & \text{otherwise.} \end{cases}$$

If  $s \leq j < 2s$ , then

$$b_{ij} = \begin{cases} e_{8(j+m-1)+7} \otimes e_{8j}, & i = j; \\ 0, & \text{otherwise.} \end{cases}$$

If  $2s \leq j < 6s$ , then

$$b_{ij} = \begin{cases} e_{8(j+m)+j_2+1} \otimes e_{8j+j_2-1-f(j_2,4,5)}, & i = j; \\ 0, & \text{otherwise.} \end{cases}$$

If  $6s \leq j < 7s$ , then

$$b_{ij} = \begin{cases} e_{8(j+m)+1} \otimes e_{8j+4}, & i = j; \\ 0, & \text{otherwise.} \end{cases}$$

If  $7s \leq j < 8s$ , then

$$b_{ij} = \begin{cases} e_{8(j+m)+2} \otimes e_{8j+5}, & i = j; \\ 0, & \text{otherwise.} \end{cases}$$

If  $8s \leq j < 9s$ , then

$$b_{ij} = \begin{cases} e_{8(j+m)+5} \otimes e_{8j+5}, & i = j; \\ 0, & \text{otherwise.} \end{cases}$$

If  $9s \leq j < 10s$ , then

$$b_{ij} = \begin{cases} e_{8(j+m)+3} \otimes e_{8j+6}, & i = j; \\ 0, & \text{otherwise.} \end{cases}$$

If  $10s \leq j < 11s$ , then

$$b_{ij} = \begin{cases} e_{8(j+m)+6} \otimes e_{8j+6}, & i = j; \\ 0, & \text{otherwise.} \end{cases}$$

If  $11s \leq j < 12s$ , then

$$b_{ij} = \begin{cases} e_{8(j+m)+7} \otimes e_{8j+7}, & i = j; \\ 0, & \text{otherwise.} \end{cases}$$

If  $12s \leq j < 13s$ , then

$$b_{ij} = \begin{cases} e_{8(j+m+1)} \otimes e_{8j+7}, & i = j; \\ 0, & \text{otherwise.} \end{cases}$$

(24) If  $r_0 = 23$ , then  $\Omega^{23}(Z_t^{(1)})$  is described with  $(11s \times 11s)$  matrix, whose entries  $b_{ij}$  have the following form:

If  $0 \leq j < s$ , then

$$b_{ij} = \begin{cases} e_{8(j+m)+3} \otimes e_{8j}, & i = j; \\ 0, & \text{otherwise.} \end{cases}$$

If  $s \leq j < 2s$ , then

$$b_{ij} = \begin{cases} e_{8(j+m)+5} \otimes e_{8j}, & i = j; \\ 0, & \text{otherwise.} \end{cases}$$

If  $2s \leq j < 5s$ , then

$$b_{ij} = \begin{cases} e_{8(j+m+1)-f(j_2,3)} \otimes e_{8j+j_2-1}, & i = j; \\ 0, & \text{otherwise.} \end{cases}$$

If  $5s \leq j < 8s$ , then

$$b_{ij} = \begin{cases} e_{8(j+m+1)+6-j_2} \otimes e_{8j+j_2-1}, & i = j; \\ 0, & \text{otherwise.} \end{cases}$$

If  $8s \leq j < 11s$ , then

$$b_{ij} = \begin{cases} e_{8(j+m+1)+2(j_2-7)} \otimes e_{8j+7}, & i = j; \\ 0, & \text{otherwise.} \end{cases}$$

(25) If  $r_0 = 24$ , then  $\Omega^{24}(Z_t^{(1)})$  is described with  $(11s \times 11s)$  matrix, whose entries  $b_{ij}$  have the following form:

If  $0 \leq j < s$ , then

$$b_{ij} = \begin{cases} e_{8(j+m)} \otimes e_{8j}, & i = j; \\ 0, & \text{otherwise.} \end{cases}$$

If  $s \leq j < 4s$ , then

$$b_{ij} = \begin{cases} e_{8(j+m)+3+j_2} \otimes e_{8j+1+f(j_2,3)}, & i = j; \\ 0, & \text{otherwise.} \end{cases}$$

If  $4s \leq j < 7s$ , then

$$b_{ij} = \begin{cases} e_{8(j+m)+j_2-3} \otimes e_{8j+j_2-1}, & i = j; \\ 0, & \text{otherwise.} \end{cases}$$

If  $7s \leq j < 8s$ , then

$$b_{ij} = \begin{cases} e_{8(j+m)+6} \otimes e_{8j+5}, & i = j; \\ 0, & \text{otherwise.} \end{cases}$$

If  $8s \leq j < 9s$ , then

$$b_{ij} = \begin{cases} e_{8(j+m)+4} \otimes e_{8j+6}, & i = j; \\ 0, & \text{otherwise.} \end{cases}$$

If  $9s \leq j < 10s$ , then

$$b_{ij} = \begin{cases} e_{8(j+m+1)} \otimes e_{8j+7}, & i = j; \\ 0, & \text{otherwise.} \end{cases}$$

If  $10s \leq j < 11s$ , then

$$b_{ij} = \begin{cases} e_{8(j+m)+7} \otimes e_{8j+7}, & i = j; \\ 0, & \text{otherwise.} \end{cases}$$

(26) If  $r_0 = 25$ , then  $\Omega^{25}(Z_t^{(1)})$  is described with  $(10s \times 10s)$  matrix, whose entries  $b_{ij}$  have the following form:

If  $0 \leq j < s$ , then

$$b_{ij} = \begin{cases} e_{8(j+m)+4} \otimes e_{8j}, & i = j; \\ 0, & \text{otherwise.} \end{cases}$$

If  $s \leq j < 6s$ , then

$$b_{ij} = \begin{cases} e_{8(j+m)+5+j_2} \otimes e_{8j+j_2-1}, & i = j; \\ 0, & \text{otherwise.} \end{cases}$$

If  $6s \leq j < 7s$ , then

$$b_{ij} = \begin{cases} e_{8(j+m)+7} \otimes e_{8j+5}, & i = j; \\ 0, & \text{otherwise.} \end{cases}$$



If  $7s \leq j < 8s$ , then

$$b_{ij} = \begin{cases} e_{8(j+m+1)} \otimes e_{8j+6}, & i = j; \\ 0, & \text{otherwise.} \end{cases}$$

If  $8s \leq j < 9s$ , then

$$b_{ij} = \begin{cases} e_{8(j+m+1)+3} \otimes e_{8j+7}, & i = j; \\ 0, & \text{otherwise.} \end{cases}$$

If  $9s \leq j < 10s$ , then

$$b_{ij} = \begin{cases} e_{8(j+m+1)+5} \otimes e_{8j+7}, & i = j; \\ 0, & \text{otherwise.} \end{cases}$$

(27) If  $r_0 = 26$ , then  $\Omega^{26}(Z_t^{(1)})$  is described with  $(8s \times 8s)$  matrix, whose entries  $b_{ij}$  have the following form:

If  $0 \leq j < 8s$ , then

$$b_{ij} = \begin{cases} e_{8(j+m-1)+7+j_2+6f(j_2,1)+2f(j_2,7)} \otimes e_{8j+j_2}, & i = j; \\ 0, & \text{otherwise.} \end{cases}$$

(28) If  $r_0 = 27$ , then  $\Omega^{27}(Z_t^{(1)})$  is described with  $(9s \times 9s)$  matrix, whose entries  $b_{ij}$  have the following form:

If  $0 \leq j < 7s$ , then

$$b_{ij} = \begin{cases} e_{8(j+m)+7+j_2-4f(j_2,5)} \otimes e_{8j+j_2}, & i = j; \\ 0, & \text{otherwise.} \end{cases}$$

If  $7s \leq j < 8s$ , then

$$b_{ij} = \begin{cases} e_{8(j+m+1)+4} \otimes e_{8j+7}, & i = j; \\ 0, & \text{otherwise.} \end{cases}$$

If  $8s \leq j < 9s$ , then

$$b_{ij} = \begin{cases} e_{8(j+m+1)+6} \otimes e_{8j+7}, & i = j; \\ 0, & \text{otherwise.} \end{cases}$$

(29) If  $r_0 = 28$ , then  $\Omega^{28}(Z_t^{(1)})$  is described with  $(8s \times 8s)$  matrix, whose entries  $b_{ij}$  have the following form:

If  $0 \leq j < 8s$ , then

$$b_{ij} = \begin{cases} e_{8(j+m)+j_2} \otimes e_{8j+j_2}, & i = j; \\ 0, & \text{otherwise.} \end{cases}$$

(II) Represent an arbitrary  $t_0 \in \mathbb{N}$  in the form  $t_0 = 29\ell_0 + r_0$ , where  $0 \leq r_0 \leq 28$ . Then  $\Omega^{t_0}(Z_t^{(1)})$  is a  $\Omega^{r_0}(Z_t^{(1)})$ , whose left components twisted by  $\sigma^{\ell_0}$ .

**Proposition 2** (Translates for the case 2). (I) Let  $r_0 \in \mathbb{N}$ ,  $r_0 < 29$ .  $r_0$ -translates of the elements  $Z_t^{(2)}$  are described by the following way.

(1) If  $r_0 = 0$ , then  $\Omega^0(Z_t^{(2)})$  is described with  $(8s \times 9s)$  matrix with two nonzero entries:

$$\begin{aligned} b_{j,(2)_s} &= w_{8(j+m) \rightarrow 8(j+m)+1} \otimes e_{8j}; \\ b_{j-s,s+(2)_s} &= w_{8(j+m) \rightarrow 8(j+m)+5} \otimes e_{8j}. \end{aligned}$$

(2) If  $r_0 = 1$ , then  $\Omega^1(Z_t^{(2)})$  is described with  $(9s \times 8s)$  matrix with the following nonzero entries:

$$\begin{aligned}
b_{(j+1)s, s+(1)s} &= w_{8(j+m+1)+1 \rightarrow 8(j+m+1)+2} \otimes w_{8j+1 \rightarrow 8(j+1)}; \\
b_{2s+(j+1)s, s+(1)s} &= e_{8(j+m+1)+2} \otimes w_{8j+1 \rightarrow 8(j+1)+1}; \\
b_{(j_1+1-f(j_1,0))s+(j+1)s, 2s+(1)s} &= w_{8(j+m+1)+j_1+1 \rightarrow 8(j+m+1)+3} \otimes w_{8j+2 \rightarrow 8(j+1)+j_1}, \quad 0 \leq j_1 \leq 2; \\
b_{(j_1+1-f(j_1,0))s+(j+1)s, 3s+(1)s} &= w_{8(j+m+1)+j_1+1 \rightarrow 8(j+m+1)+4} \otimes w_{8j+3 \rightarrow 8(j+1)+j_1}, \quad 0 \leq j_1 \leq 3; \\
b_{s+(j+1)s, 4s+(1)s} &= e_{8(j+m+1)+5} \otimes w_{8j+4 \rightarrow 8(j+1)}; \\
b_{s+(j+1)s, 5s+(1)s} &= w_{8(j+m+1)+5 \rightarrow 8(j+m+1)+6} \otimes w_{8j+5 \rightarrow 8(j+1)}; \\
b_{6s+(j+1)s, 5s+(1)s} &= e_{8(j+m+1)+6} \otimes w_{8j+5 \rightarrow 8(j+1)+5}; \\
b_{(j+1)s, 6s+(1)s} &= e_{8(j+m+1)+1} \otimes w_{8j+6 \rightarrow 8(j+1)}; \\
b_{j+s, 7s+(1)s} &= -w_{8(j+m+1) \rightarrow 8(j+m+2)} \otimes e_{8j+7}.
\end{aligned}$$

(3) If  $r_0 = 2$ , then  $\Omega^2(Z_t^{(2)})$  is described with  $(8s \times 10s)$  matrix with the following nonzero entries:

$$\begin{aligned}
b_{(j+1)s, 4s+(1)s} &= e_{8(j+m)+7} \otimes w_{8j+3 \rightarrow 8(j+1)}; \\
b_{j-s, 5s+(1)s} &= w_{8(j+m)+5 \rightarrow 8(j+m+1)} \otimes e_{8j+4}; \\
b_{(j+1)s, 6s+(1)s} &= -e_{8(j+m)+7} \otimes w_{8j+5 \rightarrow 8(j+1)}; \\
b_{j-s, 7s+(1)s} &= w_{8(j+m)+1 \rightarrow 8(j+m+1)} \otimes e_{8j+6}.
\end{aligned}$$

(4) If  $r_0 = 3$ , then  $\Omega^3(Z_t^{(2)})$  is described with  $(10s \times 11s)$  matrix with the following nonzero entries:

$$\begin{aligned}
b_{j+(j_1-f(j_1,0))s, s+(1)s} &= -w_{8(j+m)+2+j_1+2f(j_1,3) \rightarrow 8(j+m+1)} \otimes w_{8j \rightarrow 8j+j_1}, \quad 0 \leq j_1 \leq 3; \\
b_{(j+1)s, 2s+(1)s} &= w_{8(j+m+1)+2 \rightarrow 8(j+m+1)+3} \otimes w_{8j+1 \rightarrow 8(j+1)}; \\
b_{2s+(j+1)s, 2s+(1)s} &= e_{8(j+m+1)+3} \otimes w_{8j+1 \rightarrow 8(j+1)+1}; \\
b_{(j_1+1-f(j_1,0))s+(j+1)s, 3s+(1)s} &= w_{8(j+m+1)+2+j_1 \rightarrow 8(j+m+1)+4} \otimes w_{8j+2 \rightarrow 8(j+1)+j_1}, \quad 0 \leq j_1 \leq 2; \\
b_{j, 4s+(1)s} &= -w_{8(j+m)+7 \rightarrow 8(j+m+1)+5} \otimes e_{8j+3}; \\
b_{j-s, 7s+(1)s} &= -w_{8(j+m)+7 \rightarrow 8(j+m+1)+1} \otimes e_{8j+5}.
\end{aligned}$$

(5) If  $r_0 = 4$ , then  $\Omega^4(Z_t^{(2)})$  is described with  $(11s \times 11s)$  matrix with the following nonzero entries:

$$\begin{aligned}
b_{j-s, s+(1)s} &= w_{8(j+m-1)+7 \rightarrow 8(j+m)+3} \otimes e_{8j}; \\
b_{j+s, s+(1)s} &= -e_{8(j+m)+3} \otimes w_{8j \rightarrow 8j+1}; \\
b_{j-2s, 2s+(1)s} &= -w_{8(j+m-1)+7 \rightarrow 8(j+m)+1} \otimes e_{8j}; \\
b_{j-s, 4s+(1)s} &= w_{8(j+m)+4 \rightarrow 8(j+m)+7} \otimes e_{8j+2}; \\
b_{(j+1)s, 5s} &= w_{8(j+m)+7 \rightarrow 8(j+m+1)} \otimes w_{8j+3 \rightarrow 8(j+1)}; \\
b_{s+(j+1)s, 5s} &= e_{8(j+m+1)} \otimes w_{8j+3 \rightarrow 8(j+1)}; \\
b_{(j+1)s, 7s} &= -w_{8(j+m)+7 \rightarrow 8(j+m+1)} \otimes w_{8j+5 \rightarrow 8(j+1)}; \\
b_{s+(j+1)s, 7s} &= -e_{8(j+m+1)} \otimes w_{8j+5 \rightarrow 8(j+1)}; \\
b_{(j+1)s, 9s} &= w_{8(j+m)+7 \rightarrow 8(j+m+1)+2} \otimes w_{8j+7 \rightarrow 8(j+1)}; \\
b_{s+(j+1)s, 9s} &= w_{8(j+m+1) \rightarrow 8(j+m+1)+2} \otimes w_{8j+7 \rightarrow 8(j+1)}; \\
b_{6s+(j+1)s, 9s} &= -w_{8(j+m+1)+1 \rightarrow 8(j+m+1)+2} \otimes w_{8j+7 \rightarrow 8(j+1)+4}; \\
b_{8s+(j+1)s, 9s} &= e_{8(j+m+1)+2} \otimes w_{8j+7 \rightarrow 8(j+1)+6};
\end{aligned}$$

$$b_{4s+(j+1)s,10s} = w_{8(j+m+1)+5 \rightarrow 8(j+m+1)+6} \otimes w_{8j+7 \rightarrow 8(j+1)+3};$$

$$b_{5s+(j+1)s,10s} = -e_{8(j+m+1)+6} \otimes w_{8j+7 \rightarrow 8(j+1)+4}.$$

(6) If  $r_0 = 5$ , then  $\Omega^5(Z_t^{(2)})$  is described with  $(11s \times 13s)$  matrix with the following nonzero entries:

$$b_{j+3s,(1)s} = w_{8(j+m)+4 \rightarrow 8(j+m)+7} \otimes w_{8j \rightarrow 8j+1};$$

$$b_{j+2s,s+(1)s} = -w_{8(j+m)+4 \rightarrow 8(j+m+1)} \otimes w_{8j \rightarrow 8j+1};$$

$$b_{s+(j+1)s,2s} = w_{8(j+m+1)+3 \rightarrow 8(j+m+1)+4} \otimes w_{8j+1 \rightarrow 8(j+1)};$$

$$b_{j+s,2s+(1)s} = -w_{8(j+m)+4 \rightarrow 8(j+m+1)+4} \otimes e_{8j+1};$$

$$b_{(j+1)s,3s} = e_{8(j+m+1)+5} \otimes w_{8j+2 \rightarrow 8(j+1)};$$

$$b_{(j+1)s,4s} = w_{8(j+m+1)+5 \rightarrow 8(j+m+1)+6} \otimes w_{8j+3 \rightarrow 8(j+1)};$$

$$b_{2s+(j+1)s,5s} = e_{8(j+m+1)+1} \otimes w_{8j+3 \rightarrow 8(j+1)};$$

$$b_{2s+(j+1)s,6s} = -w_{8(j+m+1)+1 \rightarrow 8(j+m+1)+2} \otimes w_{8j+4 \rightarrow 8(j+1)};$$

$$b_{(j+1)s,8s} = -e_{8(j+m+1)+5} \otimes w_{8j+5 \rightarrow 8(j+1)};$$

$$b_{s+(j+1)s,9s} = e_{8(j+m+1)+3} \otimes w_{8j+6 \rightarrow 8(j+1)};$$

$$b_{2s+(j+1)s,9s} = w_{8(j+m+1)+1 \rightarrow 8(j+m+1)+3} \otimes w_{8j+6 \rightarrow 8(j+1)};$$

$$b_{s+(j+1)s,11s} = w_{8(j+m+1)+3 \rightarrow 8(j+m+1)+7} \otimes w_{8j+7 \rightarrow 8(j+1)};$$

$$b_{2s+(j+1)s,11s} = w_{8(j+m+1)+1 \rightarrow 8(j+m+1)+7} \otimes w_{8j+7 \rightarrow 8(j+1)};$$

$$b_{4s+(j+1)s,11s} = e_{8(j+m+1)+7} \otimes w_{8j+7 \rightarrow 8(j+1)+2};$$

$$b_{5s+(j+1)s,12s} = e_{8(j+m+2)} \otimes w_{8j+7 \rightarrow 8(j+1)+3}.$$

(7) If  $r_0 = 6$ , then  $\Omega^6(Z_t^{(2)})$  is described with  $(13s \times 14s)$  matrix with the following nonzero entries:

$$b_{(j+1)s,4s} = -e_{8(j+m)+7} \otimes w_{8j+1 \rightarrow 8(j+1)};$$

$$b_{(j+1)s,5s} = w_{8(j+m)+7 \rightarrow 8(j+m+1)} \otimes w_{8j+2 \rightarrow 8(j+1)};$$

$$b_{s+(j+1)s,5s} = e_{8(j+m+1)} \otimes w_{8j+2 \rightarrow 8(j+1)};$$

$$b_{(j+1)s,6s} = e_{8(j+m)+7} \otimes w_{8j+3 \rightarrow 8(j+1)};$$

$$b_{s+(j+1)s,7s} = e_{8(j+m+1)} \otimes w_{8j+4 \rightarrow 8(j+1)};$$

$$b_{(j+1)s,8s} = e_{8(j+m)+7} \otimes w_{8j+5 \rightarrow 8(j+1)};$$

$$b_{3s+(j+1)s,11s} = e_{8(j+m+1)+5} \otimes w_{8j+7 \rightarrow 8(j+1)+2};$$

$$b_{(j+1)s,12s} = -w_{8(j+m)+7 \rightarrow 8(j+m+1)+3} \otimes w_{8j+7 \rightarrow 8(j+1)};$$

$$b_{6s+(j+1)s,12s} = w_{8(j+m+1)+2 \rightarrow 8(j+m+1)+3} \otimes w_{8j+7 \rightarrow 8(j+1)+4};$$

$$b_{9s+(j+1)s,12s} = e_{8(j+m+1)+3} \otimes w_{8j+7 \rightarrow 8(j+1)+6};$$

$$b_{5s+(j+1)s,13s} = e_{8(j+m+1)+1} \otimes w_{8j+7 \rightarrow 8(j+1)+3}.$$

(8) If  $r_0 = 7$ , then  $\Omega^7(Z_t^{(2)})$  is described with  $(14s \times 16s)$  matrix with the following nonzero entries:

$$b_{3s+(j+1)s,3s} = e_{8(j+m+1)+5} \otimes w_{8j+1 \rightarrow 8(j+1)};$$

$$b_{2s+(j+1)s,4s} = e_{8(j+m+1)+6} \otimes w_{8j+2 \rightarrow 8(j+1)};$$

$$b_{3s+(j+1)s,4s} = w_{8(j+m+1)+5 \rightarrow 8(j+m+1)+6} \otimes w_{8j+2 \rightarrow 8(j+1)};$$

$$b_{(j+1)s,6s} = e_{8(j+m+1)+2} \otimes w_{8j+3 \rightarrow 8(j+1)};$$

$$b_{(j+1)s,7s} = w_{8(j+m+1)+2 \rightarrow 8(j+m+1)+3} \otimes w_{8j+4 \rightarrow 8(j+1)};$$

$$b_{3s+(j+1)s,8s} = e_{8(j+m+1)+5} \otimes w_{8j+4 \rightarrow 8(j+1)};$$

$$\begin{aligned}
b_{2s+(j+1)s,10s} &= e_{8(j+m+1)+6} \otimes w_{8j+5 \rightarrow 8(j+1)}; \\
b_{(j+1)s,12s} &= -w_{8(j+m+1)+2 \rightarrow 8(j+m+1)+4} \otimes w_{8j+6 \rightarrow 8(j+1)}; \\
b_{s+(j+1)s,12s} &= e_{8(j+m+1)+4} \otimes w_{8j+6 \rightarrow 8(j+1)}; \\
b_{(j+1)s,14s} &= w_{8(j+m+1)+2 \rightarrow 8(j+m+1)+7} \otimes w_{8j+7 \rightarrow 8(j+1)}; \\
b_{s+(j+1)s,14s} &= -w_{8(j+m+1)+4 \rightarrow 8(j+m+1)+7} \otimes w_{8j+7 \rightarrow 8(j+1)}; \\
b_{4s+(j+1)s,14s} &= -e_{8(j+m+1)+7} \otimes w_{8j+7 \rightarrow 8(j+1)+1}; \\
b_{(j+1)s,15s} &= -w_{8(j+m+1)+2 \rightarrow 8(j+m+2)} \otimes w_{8j+7 \rightarrow 8(j+1)}; \\
b_{s+(j+1)s,15s} &= w_{8(j+m+1)+4 \rightarrow 8(j+m+2)} \otimes w_{8j+7 \rightarrow 8(j+1)}; \\
b_{4s+(j+1)s,15s} &= w_{8(j+m+1)+7 \rightarrow 8(j+m+2)} \otimes w_{8j+7 \rightarrow 8(j+1)+1}; \\
b_{5s+(j+1)s,15s} &= e_{8(j+m+2)} \otimes w_{8j+7 \rightarrow 8(j+1)+2}.
\end{aligned}$$

(9) If  $r_0 = 8$ , then  $\Omega^8(Z_t^{(2)})$  is described with  $(16s \times 16s)$  matrix with the following nonzero entries:

$$\begin{aligned}
b_{2s+(j+1)s,4s} &= -e_{8(j+m+1)} \otimes w_{8j+1 \rightarrow 8(j+1)}; \\
b_{(j+1)s,5s} &= -e_{8(j+m)+7} \otimes w_{8j+2 \rightarrow 8(j+1)}; \\
b_{j_1s+(j+1)s,6s} &= (-1)^{j_1} w_{8(j+m)+7 \rightarrow 8(j+m+1)} \otimes w_{8j+3 \rightarrow 8(j+1)}, \quad 0 \leq j_1 \leq 2; \\
b_{s+(j+1)s,7s} &= e_{8(j+m)+7} \otimes w_{8j+4 \rightarrow 8(j+1)}; \\
b_{(j+1)s,8s} &= e_{8(j+m)+7} \otimes w_{8j+5 \rightarrow 8(j+1)}; \\
b_{s+(j+1)s,8s} &= -e_{8(j+m)+7} \otimes w_{8j+5 \rightarrow 8(j+1)}; \\
b_{2s+(j+1)s,9s} &= e_{8(j+m+1)} \otimes w_{8j+5 \rightarrow 8(j+1)}; \\
b_{5s+(j+1)s,12s} &= w_{8(j+m+1)+1 \rightarrow 8(j+m+1)+2} \otimes w_{8j+7 \rightarrow 8(j+1)+2}; \\
b_{6s+(j+1)s,12s} &= e_{8(j+m+1)+2} \otimes w_{8j+7 \rightarrow 8(j+1)+3}; \\
b_{(j+1)s,13s} &= -w_{8(j+m)+7 \rightarrow 8(j+m+1)+4} \otimes w_{8j+7 \rightarrow 8(j+1)}; \\
b_{s+(j+1)s,13s} &= w_{8(j+m)+7 \rightarrow 8(j+m+1)+4} \otimes w_{8j+7 \rightarrow 8(j+1)}; \\
b_{5s+(j+1)s,13s} &= w_{8(j+m+1)+1 \rightarrow 8(j+m+1)+4} \otimes w_{8j+7 \rightarrow 8(j+1)+2}; \\
b_{7s+(j+1)s,13s} &= w_{8(j+m+1)+3 \rightarrow 8(j+m+1)+4} \otimes w_{8j+7 \rightarrow 8(j+1)+4}; \\
b_{12s+(j+1)s,13s} &= e_{8(j+m+1)+4} \otimes w_{8j+7 \rightarrow 8(j+1)+6}; \\
b_{3s+(j+1)s,14s} &= -w_{8(j+m+1)+5 \rightarrow 8(j+m+1)+6} \otimes w_{8j+7 \rightarrow 8(j+1)+1}; \\
b_{4s+(j+1)s,14s} &= e_{8(j+m+1)+6} \otimes w_{8j+7 \rightarrow 8(j+1)+2}; \\
b_{3s+(j+1)s,15s} &= e_{8(j+m+1)+5} \otimes w_{8j+7 \rightarrow 8(j+1)+1}.
\end{aligned}$$

(10) If  $r_0 = 9$ , then  $\Omega^9(Z_t^{(2)})$  is described with  $(16s \times 19s)$  matrix with the following nonzero entries:

$$\begin{aligned}
b_{(j+1)s,3s} &= -w_{8(j+m+1)+5 \rightarrow 8(j+m+1)+6} \otimes w_{8j+1 \rightarrow 8(j+1)}; \\
b_{2s+(j+1)s,3s} &= -e_{8(j+m+1)+6} \otimes w_{8j+1 \rightarrow 8(j+1)}; \\
b_{3s+(j+1)s,4s} &= -e_{8(j+m+1)+1} \otimes w_{8j+1 \rightarrow 8(j+1)}; \\
b_{3s+(j+1)s,5s} &= w_{8(j+m+1)+1 \rightarrow 8(j+m+1)+2} \otimes w_{8j+2 \rightarrow 8(j+1)}; \\
b_{s+(j+1)s,6s} &= e_{8(j+m+1)+3} \otimes w_{8j+3 \rightarrow 8(j+1)}; \\
b_{3s+(j+1)s,6s} &= w_{8(j+m+1)+1 \rightarrow 8(j+m+1)+3} \otimes w_{8j+3 \rightarrow 8(j+1)}; \\
b_{(j+1)s,7s} &= e_{8(j+m+1)+5} \otimes w_{8j+3 \rightarrow 8(j+1)}; \\
b_{s+(j+1)s,8s} &= w_{8(j+m+1)+3 \rightarrow 8(j+m+1)+4} \otimes w_{8j+4 \rightarrow 8(j+1)}; \\
b_{2s+(j+1)s,9s} &= e_{8(j+m+1)+6} \otimes w_{8j+4 \rightarrow 8(j+1)};
\end{aligned}$$

$$\begin{aligned}
b_{(j+1)s,10s} &= e_{8(j+m+1)+5} \otimes w_{8j+5 \rightarrow 8(j+1)}; \\
b_{3s+(j+1)s,12s} &= e_{8(j+m+1)+1} \otimes w_{8j+5 \rightarrow 8(j+1)}; \\
b_{5s+(j+1)s,16s} &= -e_{8(j+m+1)+7} \otimes w_{8j+7 \rightarrow 8(j+1)+2}; \\
b_{s+(j+1)s,17s} &= -w_{8(j+m+1)+3 \rightarrow 8(j+m+1)+7} \otimes w_{8j+7 \rightarrow 8(j+1)}; \\
b_{2s+(j+1)s,17s} &= w_{8(j+m+1)+6 \rightarrow 8(j+m+1)+7} \otimes w_{8j+7 \rightarrow 8(j+1)}; \\
b_{5s+(j+1)s,17s} &= -e_{8(j+m+1)+7} \otimes w_{8j+7 \rightarrow 8(j+1)+2}; \\
b_{8s+(j+1)s,17s} &= -e_{8(j+m+1)+7} \otimes w_{8j+7 \rightarrow 8(j+1)+5}; \\
b_{4s+(j+1)s,18s} &= -e_{8(j+m+2)} \otimes w_{8j+7 \rightarrow 8(j+1)+1}.
\end{aligned}$$

(11) If  $r_0 = 10$ , then  $\Omega^{10}(Z_t^{(2)})$  is described with  $(19s \times 18s)$  matrix with the following nonzero entries:

$$\begin{aligned}
b_{(j+1)s,5s} &= -e_{8(j+m)+7} \otimes w_{8j+1 \rightarrow 8(j+1)}; \\
b_{s+(j+1)s,6s} &= -e_{8(j+m+1)} \otimes w_{8j+2 \rightarrow 8(j+1)}; \\
b_{(j+1)s,7s} &= -e_{8(j+m)+7} \otimes w_{8j+3 \rightarrow 8(j+1)}; \\
b_{2s+(j+1)s,9s} &= e_{8(j+m+1)} \otimes w_{8j+4 \rightarrow 8(j+1)}; \\
b_{(j+1)s,10s} &= e_{8(j+m)+7} \otimes w_{8j+5 \rightarrow 8(j+1)}; \\
b_{s+(j+1)s,11s} &= e_{8(j+m+1)} \otimes w_{8j+5 \rightarrow 8(j+1)}; \\
b_{2s+(j+1)s,11s} &= -e_{8(j+m+1)} \otimes w_{8j+5 \rightarrow 8(j+1)}; \\
b_{2s+(j+1)s,14s} &= -w_{8(j+m+1) \rightarrow 8(j+m+1)+5} \otimes w_{8j+7 \rightarrow 8(j+1)}; \\
b_{10s+(j+1)s,14s} &= e_{8(j+m+1)+5} \otimes w_{8j+7 \rightarrow 8(j+1)+5}; \\
b_{5s+(j+1)s,15s} &= -w_{8(j+m+1)+2 \rightarrow 8(j+m+1)+3} \otimes w_{8j+7 \rightarrow 8(j+1)+2}; \\
b_{6s+(j+1)s,15s} &= e_{8(j+m+1)+3} \otimes w_{8j+7 \rightarrow 8(j+1)+3}; \\
b_{2s+(j+1)s,16s} &= w_{8(j+m+1) \rightarrow 8(j+m+1)+6} \otimes w_{8j+7 \rightarrow 8(j+1)}; \\
b_{3s+(j+1)s,16s} &= -e_{8(j+m+1)+6} \otimes w_{8j+7 \rightarrow 8(j+1)+1}; \\
b_{10s+(j+1)s,16s} &= -w_{8(j+m+1)+5 \rightarrow 8(j+m+1)+6} \otimes w_{8j+7 \rightarrow 8(j+1)+5}; \\
b_{4s+(j+1)s,17s} &= -e_{8(j+m+1)+1} \otimes w_{8j+7 \rightarrow 8(j+1)+1}.
\end{aligned}$$

(12) If  $r_0 = 11$ , then  $\Omega^{11}(Z_t^{(2)})$  is described with  $(18s \times 19s)$  matrix with the following nonzero entries:

$$\begin{aligned}
b_{(j+1)s,3s} &= -e_{8(j+m+1)+2} \otimes w_{8j+1 \rightarrow 8(j+1)}; \\
b_{(j+1)s,4s} &= -w_{8(j+m+1)+2 \rightarrow 8(j+m+1)+3} \otimes w_{8j+2 \rightarrow 8(j+1)}; \\
b_{4s+(j+1)s,5s} &= -e_{8(j+m+1)+5} \otimes w_{8j+2 \rightarrow 8(j+1)}; \\
b_{(j+1)s,6s} &= -w_{8(j+m+1)+2 \rightarrow 8(j+m+1)+4} \otimes w_{8j+3 \rightarrow 8(j+1)}; \\
b_{2s+(j+1)s,6s} &= e_{8(j+m+1)+4} \otimes w_{8j+3 \rightarrow 8(j+1)}; \\
b_{s+(j+1)s,7s} &= -e_{8(j+m+1)+6} \otimes w_{8j+3 \rightarrow 8(j+1)}; \\
b_{3s+(j+1)s,9s} &= e_{8(j+m+1)+1} \otimes w_{8j+4 \rightarrow 8(j+1)}; \\
b_{(j+1)s,10s} &= e_{8(j+m+1)+2} \otimes w_{8j+5 \rightarrow 8(j+1)}; \\
b_{3s+(j+1)s,10s} &= -w_{8(j+m+1)+1 \rightarrow 8(j+m+1)+2} \otimes w_{8j+5 \rightarrow 8(j+1)}; \\
b_{s+(j+1)s,11s} &= e_{8(j+m+1)+6} \otimes w_{8j+5 \rightarrow 8(j+1)}; \\
b_{4s+(j+1)s,12s} &= e_{8(j+m+1)+5} \otimes w_{8j+5 \rightarrow 8(j+1)}; \\
b_{5s+(j+1)s,16s} &= -e_{8(j+m+1)+7} \otimes w_{8j+7 \rightarrow 8(j+1)+1}; \\
b_{6s+(j+1)s,17s} &= -e_{8(j+m+2)} \otimes w_{8j+7 \rightarrow 8(j+1)+2};
\end{aligned}$$

$$\begin{aligned}
b_{3s+(j+1)s,18s} &= w_{8(j+m+1)+1 \rightarrow 8(j+m+2)} \otimes w_{8j+7 \rightarrow 8(j+1)}; \\
b_{5s+(j+1)s,18s} &= -w_{8(j+m+1)+7 \rightarrow 8(j+m+2)} \otimes w_{8j+7 \rightarrow 8(j+1)+1}; \\
b_{6s+(j+1)s,18s} &= -e_{8(j+m+2)} \otimes w_{8j+7 \rightarrow 8(j+1)+2}; \\
b_{10s+(j+1)s,18s} &= -w_{8(j+m+1)+7 \rightarrow 8(j+m+2)} \otimes w_{8j+7 \rightarrow 8(j+1)+5}; \\
b_{11s+(j+1)s,18s} &= -e_{8(j+m+2)} \otimes w_{8j+7 \rightarrow 8(j+1)+5}.
\end{aligned}$$

(13) If  $r_0 = 12$ , then  $\Omega^{12}(Z_t^{(2)})$  is described with  $(19s \times 18s)$  matrix with the following nonzero entries:

$$\begin{aligned}
b_{s+(j+1)s,4s} &= -e_{8(j+m+1)} \otimes w_{8j+1 \rightarrow 8(j+1)}; \\
b_{2s+(j+1)s,4s} &= -w_{8(j+m)+7 \rightarrow 8(j+m+1)} \otimes w_{8j+1 \rightarrow 8(j+1)}; \\
b_{2s+(j+1)s,5s} &= -e_{8(j+m)+7} \otimes w_{8j+2 \rightarrow 8(j+1)}; \\
b_{(j+1)s,6s} &= -e_{8(j+m)+7} \otimes w_{8j+3 \rightarrow 8(j+1)}; \\
b_{2s+(j+1)s,6s} &= e_{8(j+m)+7} \otimes w_{8j+3 \rightarrow 8(j+1)}; \\
b_{j_1s+(j+1)s,7s} &= (-1 + 2f(j_1, 0))w_{8(j+m)+7+f(j_1,1) \rightarrow 8(j+m+1)} \otimes w_{8j+3 \rightarrow 8(j+1)}, \quad 0 \leq j_1 \leq 2; \\
b_{(j+1)s,9s} &= e_{8(j+m)+7} \otimes w_{8j+5 \rightarrow 8(j+1)}; \\
b_{j_1s+(j+1)s,10s} &= (1 - 2f(j_1, 0))w_{8(j+m)+7+f(j_1,1) \rightarrow 8(j+m+1)} \otimes w_{8j+5 \rightarrow 8(j+1)}, \quad 0 \leq j_1 \leq 2; \\
b_{3s+(j+1)s,13s} &= -e_{8(j+m+1)+2} \otimes w_{8j+7 \rightarrow 8(j+1)+1}; \\
b_{s+(j+1)s,14s} &= -w_{8(j+m+1) \rightarrow 8(j+m+1)+6} \otimes w_{8j+7 \rightarrow 8(j+1)}; \\
b_{8s+(j+1)s,14s} &= -w_{8(j+m+1)+5 \rightarrow 8(j+m+1)+6} \otimes w_{8j+7 \rightarrow 8(j+1)+4}; \\
b_{11s+(j+1)s,14s} &= e_{8(j+m+1)+6} \otimes w_{8j+7 \rightarrow 8(j+1)+5}; \\
b_{4s+(j+1)s,15s} &= -w_{8(j+m+1)+3 \rightarrow 8(j+m+1)+4} \otimes w_{8j+7 \rightarrow 8(j+1)+2}; \\
b_{6s+(j+1)s,15s} &= e_{8(j+m+1)+4} \otimes w_{8j+7 \rightarrow 8(j+1)+3}; \\
b_{(j+1)s,16s} &= -w_{8(j+m)+7 \rightarrow 8(j+m+1)+1} \otimes w_{8j+7 \rightarrow 8(j+1)}; \\
b_{s+(j+1)s,16s} &= w_{8(j+m+1) \rightarrow 8(j+m+1)+1} \otimes w_{8j+7 \rightarrow 8(j+1)}; \\
b_{2s+(j+1)s,16s} &= w_{8(j+m)+7 \rightarrow 8(j+m+1)+1} \otimes w_{8j+7 \rightarrow 8(j+1)}; \\
b_{9s+(j+1)s,16s} &= e_{8(j+m+1)+1} \otimes w_{8j+7 \rightarrow 8(j+1)+4}; \\
b_{15s+(j+1)s,16s} &= -e_{8(j+m+1)+1} \otimes w_{8j+7 \rightarrow 8(j+1)+6}; \\
b_{5s+(j+1)s,17s} &= -e_{8(j+m+1)+5} \otimes w_{8j+7 \rightarrow 8(j+1)+2}.
\end{aligned}$$

(14) If  $r_0 = 13$ , then  $\Omega^{13}(Z_t^{(2)})$  is described with  $(18s \times 20s)$  matrix with the following nonzero entries:

$$\begin{aligned}
b_{(j+1)s,3s} &= w_{8(j+m+1)+2 \rightarrow 8(j+m+1)+3} \otimes w_{8j+1 \rightarrow 8(j+1)}; \\
b_{s+(j+1)s,3s} &= -e_{8(j+m+1)+3} \otimes w_{8j+1 \rightarrow 8(j+1)}; \\
b_{3s+(j+1)s,4s} &= -e_{8(j+m+1)+5} \otimes w_{8j+1 \rightarrow 8(j+1)}; \\
b_{(j+1)s,5s} &= w_{8(j+m+1)+2 \rightarrow 8(j+m+1)+4} \otimes w_{8j+2 \rightarrow 8(j+1)}; \\
b_{s+(j+1)s,5s} &= -w_{8(j+m+1)+3 \rightarrow 8(j+m+1)+4} \otimes w_{8j+2 \rightarrow 8(j+1)}; \\
b_{2s+(j+1)s,6s} &= -e_{8(j+m+1)+6} \otimes w_{8j+2 \rightarrow 8(j+1)}; \\
b_{3s+(j+1)s,7s} &= -e_{8(j+m+1)+5} \otimes w_{8j+3 \rightarrow 8(j+1)}; \\
b_{(j+1)s,9s} &= e_{8(j+m+1)+2} \otimes w_{8j+4 \rightarrow 8(j+1)}; \\
b_{3s+(j+1)s,10s} &= -w_{8(j+m+1)+5 \rightarrow 8(j+m+1)+6} \otimes w_{8j+4 \rightarrow 8(j+1)}; \\
b_{2s+(j+1)s,11s} &= e_{8(j+m+1)+6} \otimes w_{8j+5 \rightarrow 8(j+1)}; \\
b_{s+(j+1)s,12s} &= e_{8(j+m+1)+3} \otimes w_{8j+5 \rightarrow 8(j+1)};
\end{aligned}$$

$$\begin{aligned}
b_{(j+1)s,17s} &= w_{8(j+m+1)+2 \rightarrow 8(j+m+1)+7} \otimes w_{8j+7 \rightarrow 8(j+1)}; \\
b_{3s+(j+1)s,17s} &= w_{8(j+m+1)+5 \rightarrow 8(j+m+1)+7} \otimes w_{8j+7 \rightarrow 8(j+1)}; \\
b_{9s+(j+1)s,17s} &= e_{8(j+m+1)+7} \otimes w_{8j+7 \rightarrow 8(j+1)+5}; \\
b_{4s+(j+1)s,18s} &= -e_{8(j+m+2)} \otimes w_{8j+7 \rightarrow 8(j+1)+1}; \\
b_{5s+(j+1)s,18s} &= w_{8(j+m+1)+7 \rightarrow 8(j+m+2)} \otimes w_{8j+7 \rightarrow 8(j+1)+2}; \\
b_{5s+(j+1)s,19s} &= -e_{8(j+m+1)+7} \otimes w_{8j+7 \rightarrow 8(j+1)+2}.
\end{aligned}$$

(15) If  $r_0 = 14$ , then  $\Omega^{14}(Z_t^{(2)})$  is described with  $(20s \times 18s)$  matrix with the following nonzero entries:

$$\begin{aligned}
b_{(j+1)s,5s} &= e_{8(j+m)+7} \otimes w_{8j+1 \rightarrow 8(j+1)}; \\
b_{(j+1)s,6s} &= e_{8(j+m)+7} \otimes w_{8j+2 \rightarrow 8(j+1)}; \\
b_{2s+(j+1)s,7s} &= -e_{8(j+m+1)} \otimes w_{8j+2 \rightarrow 8(j+1)}; \\
b_{j_1s+(j+1)s,8s} &= (-1 + 2f(j_1, 2))w_{8(j+m+1)-f(j_1,0) \rightarrow 8(j+m+1)} \otimes w_{8j+3 \rightarrow 8(j+1)}, \quad 0 \leq j_1 \leq 2; \\
b_{(j+1)s,10s} &= e_{8(j+m)+7} \otimes w_{8j+5 \rightarrow 8(j+1)}; \\
b_{s+(j+1)s,11s} &= e_{8(j+m+1)} \otimes w_{8j+5 \rightarrow 8(j+1)}; \\
b_{(j+1)s,14s} &= w_{8(j+m)+7 \rightarrow 8(j+m+1)+2} \otimes w_{8j+7 \rightarrow 8(j+1)}; \\
b_{s+(j+1)s,14s} &= w_{8(j+m+1) \rightarrow 8(j+m+1)+2} \otimes w_{8j+7 \rightarrow 8(j+1)}; \\
b_{8s+(j+1)s,14s} &= w_{8(j+m+1)+1 \rightarrow 8(j+m+1)+2} \otimes w_{8j+7 \rightarrow 8(j+1)+3}; \\
b_{9s+(j+1)s,14s} &= e_{8(j+m+1)+2} \otimes w_{8j+7 \rightarrow 8(j+1)+4}; \\
b_{14s+(j+1)s,14s} &= -e_{8(j+m+1)+2} \otimes w_{8j+7 \rightarrow 8(j+1)+6}; \\
b_{12s+(j+1)s,15s} &= e_{8(j+m+1)+3} \otimes w_{8j+7 \rightarrow 8(j+1)+5}; \\
b_{6s+(j+1)s,16s} &= -e_{8(j+m+1)+6} \otimes w_{8j+7 \rightarrow 8(j+1)+2}; \\
b_{4s+(j+1)s,17s} &= -e_{8(j+m+1)+5} \otimes w_{8j+7 \rightarrow 8(j+1)+1}.
\end{aligned}$$

(16) If  $r_0 = 15$ , then  $\Omega^{15}(Z_t^{(2)})$  is described with  $(18s \times 19s)$  matrix with the following nonzero entries:

$$\begin{aligned}
b_{(j+1)s,3s} &= w_{8(j+m+1)+3 \rightarrow 8(j+m+1)+4} \otimes w_{8j+1 \rightarrow 8(j+1)}; \\
b_{2s+(j+1)s,3s} &= -e_{8(j+m+1)+4} \otimes w_{8j+1 \rightarrow 8(j+1)}; \\
b_{s+(j+1)s,4s} &= e_{8(j+m+1)+6} \otimes w_{8j+1 \rightarrow 8(j+1)}; \\
b_{4s+(j+1)s,5s} &= -e_{8(j+m+1)+5} \otimes w_{8j+2 \rightarrow 8(j+1)}; \\
b_{3s+(j+1)s,6s} &= -e_{8(j+m+1)+1} \otimes w_{8j+2 \rightarrow 8(j+1)}; \\
b_{3s+(j+1)s,7s} &= w_{8(j+m+1)+1 \rightarrow 8(j+m+1)+2} \otimes w_{8j+3 \rightarrow 8(j+1)}; \\
b_{s+(j+1)s,8s} &= -e_{8(j+m+1)+6} \otimes w_{8j+3 \rightarrow 8(j+1)}; \\
b_{4s+(j+1)s,8s} &= -w_{8(j+m+1)+5 \rightarrow 8(j+m+1)+6} \otimes w_{8j+3 \rightarrow 8(j+1)}; \\
b_{2s+(j+1)s,11s} &= e_{8(j+m+1)+4} \otimes w_{8j+5 \rightarrow 8(j+1)}; \\
b_{4s+(j+1)s,12s} &= e_{8(j+m+1)+5} \otimes w_{8j+5 \rightarrow 8(j+1)}; \\
b_{(j+1)s,13s} &= -e_{8(j+m+1)+3} \otimes w_{8j+6 \rightarrow 8(j+1)}; \\
b_{(j+1)s,16s} &= w_{8(j+m+1)+3 \rightarrow 8(j+m+1)+7} \otimes w_{8j+7 \rightarrow 8(j+1)}; \\
b_{5s+(j+1)s,16s} &= e_{8(j+m+1)+7} \otimes w_{8j+7 \rightarrow 8(j+1)+1}; \\
b_{11s+(j+1)s,17s} &= e_{8(j+m+2)} \otimes w_{8j+7 \rightarrow 8(j+1)+5}; \\
b_{7s+(j+1)s,18s} &= -e_{8(j+m+2)} \otimes w_{8j+7 \rightarrow 8(j+1)+2}.
\end{aligned}$$

(17) If  $r_0 = 16$ , then  $\Omega^{16}(Z_t^{(2)})$  is described with  $(19s \times 18s)$  matrix with the following nonzero entries:

$$\begin{aligned}
b_{(j+1)s,4s} &= e_{8(j+m)+7} \otimes w_{8j+1 \rightarrow 8(j+1)}; \\
b_{2s+(j+1)s,4s} &= -e_{8(j+m)+7} \otimes w_{8j+1 \rightarrow 8(j+1)}; \\
b_{j_1s+(j+1)s,5s} &= (1 - 2f(j_1, 0))w_{8(j+m)+7+f(j_1,1) \rightarrow 8(j+m+1)} \otimes w_{8j+1 \rightarrow 8(j+1)}, \quad 0 \leq j_1 \leq 2; \\
b_{j_1s+(j+1)s,6s} &= (1 - 2f(j_1, 0))w_{8(j+m)+7+f(j_1,1) \rightarrow 8(j+m+1)} \otimes w_{8j+2 \rightarrow 8(j+1)}, \quad 0 \leq j_1 \leq 2; \\
b_{(j+1)s,7s} &= -e_{8(j+m)+7} \otimes w_{8j+3 \rightarrow 8(j+1)}; \\
b_{s+(j+1)s,9s} &= e_{8(j+m+1)} \otimes w_{8j+5 \rightarrow 8(j+1)}; \\
b_{2s+(j+1)s,10s} &= e_{8(j+m)+7} \otimes w_{8j+5 \rightarrow 8(j+1)}; \\
b_{s+(j+1)s,13s} &= w_{8(j+m+1) \rightarrow 8(j+m+1)+3} \otimes w_{8j+7 \rightarrow 8(j+1)}; \\
b_{2s+(j+1)s,13s} &= w_{8(j+m)+7 \rightarrow 8(j+m+1)+3} \otimes w_{8j+7 \rightarrow 8(j+1)}; \\
b_{6s+(j+1)s,13s} &= -w_{8(j+m+1)+1 \rightarrow 8(j+m+1)+3} \otimes w_{8j+7 \rightarrow 8(j+1)+2}; \\
b_{7s+(j+1)s,13s} &= -w_{8(j+m+1)+2 \rightarrow 8(j+m+1)+3} \otimes w_{8j+7 \rightarrow 8(j+1)+3}; \\
b_{9s+(j+1)s,13s} &= e_{8(j+m+1)+3} \otimes w_{8j+7 \rightarrow 8(j+1)+4}; \\
b_{13s+(j+1)s,13s} &= -e_{8(j+m+1)+3} \otimes w_{8j+7 \rightarrow 8(j+1)+6}; \\
b_{4s+(j+1)s,14s} &= e_{8(j+m+1)+6} \otimes w_{8j+7 \rightarrow 8(j+1)+1}; \\
b_{11s+(j+1)s,15s} &= e_{8(j+m+1)+4} \otimes w_{8j+7 \rightarrow 8(j+1)+5}; \\
b_{6s+(j+1)s,16s} &= -e_{8(j+m+1)+1} \otimes w_{8j+7 \rightarrow 8(j+1)+2}; \\
b_{12s+(j+1)s,17s} &= e_{8(j+m+1)+5} \otimes w_{8j+7 \rightarrow 8(j+1)+5}.
\end{aligned}$$

(18) If  $r_0 = 17$ , then  $\Omega^{17}(Z_t^{(2)})$  is described with  $(18s \times 19s)$  matrix with the following nonzero entries:

$$\begin{aligned}
b_{3s+(j+1)s,3s} &= e_{8(j+m+1)+5} \otimes w_{8j+1 \rightarrow 8(j+1)}; \\
b_{(j+1)s,5s} &= -e_{8(j+m+1)+2} \otimes w_{8j+2 \rightarrow 8(j+1)}; \\
b_{2s+(j+1)s,6s} &= e_{8(j+m+1)+6} \otimes w_{8j+2 \rightarrow 8(j+1)}; \\
b_{3s+(j+1)s,6s} &= w_{8(j+m+1)+5 \rightarrow 8(j+m+1)+6} \otimes w_{8j+2 \rightarrow 8(j+1)}; \\
b_{(j+1)s,7s} &= -w_{8(j+m+1)+2 \rightarrow 8(j+m+1)+3} \otimes w_{8j+3 \rightarrow 8(j+1)}; \\
b_{2s+(j+1)s,11s} &= e_{8(j+m+1)+6} \otimes w_{8j+5 \rightarrow 8(j+1)}; \\
b_{3s+(j+1)s,12s} &= e_{8(j+m+1)+5} \otimes w_{8j+5 \rightarrow 8(j+1)}; \\
b_{(j+1)s,14s} &= w_{8(j+m+1)+2 \rightarrow 8(j+m+1)+4} \otimes w_{8j+6 \rightarrow 8(j+1)}; \\
b_{s+(j+1)s,14s} &= -e_{8(j+m+1)+4} \otimes w_{8j+6 \rightarrow 8(j+1)}; \\
b_{(j+1)s,16s} &= -w_{8(j+m+1)+2 \rightarrow 8(j+m+1)+7} \otimes w_{8j+7 \rightarrow 8(j+1)}; \\
b_{s+(j+1)s,16s} &= w_{8(j+m+1)+4 \rightarrow 8(j+m+1)+7} \otimes w_{8j+7 \rightarrow 8(j+1)}; \\
b_{4s+(j+1)s,16s} &= e_{8(j+m+1)+7} \otimes w_{8j+7 \rightarrow 8(j+1)+1}; \\
b_{10s+(j+1)s,16s} &= e_{8(j+m+1)+7} \otimes w_{8j+7 \rightarrow 8(j+1)+5}; \\
b_{(j+1)s,17s} &= -w_{8(j+m+1)+2 \rightarrow 8(j+m+2)} \otimes w_{8j+7 \rightarrow 8(j+1)}; \\
b_{s+(j+1)s,17s} &= w_{8(j+m+1)+4 \rightarrow 8(j+m+2)} \otimes w_{8j+7 \rightarrow 8(j+1)}; \\
b_{4s+(j+1)s,17s} &= w_{8(j+m+1)+7 \rightarrow 8(j+m+2)} \otimes w_{8j+7 \rightarrow 8(j+1)+1}; \\
b_{5s+(j+1)s,17s} &= e_{8(j+m+2)} \otimes w_{8j+7 \rightarrow 8(j+1)+1}; \\
b_{10s+(j+1)s,18s} &= e_{8(j+m+1)+7} \otimes w_{8j+7 \rightarrow 8(j+1)+5}.
\end{aligned}$$



(19) If  $r_0 = 18$ , then  $\Omega^{18}(Z_t^{(2)})$  is described with  $(19s \times 16s)$  matrix with the following nonzero entries:

$$\begin{aligned}
b_{j_1s+(j+1)s,4s} &= (1 - 2f(j_1, 2))w_{8(j+m+1)-f(j_1,0) \rightarrow 8(j+m+1)} \otimes w_{8j+1 \rightarrow 8(j+1)}, \quad 0 \leq j_1 \leq 2; \\
b_{(j+1)s,5s} &= -e_{8(j+m)+7} \otimes w_{8j+2 \rightarrow 8(j+1)}; \\
b_{s+(j+1)s,6s} &= -e_{8(j+m+1)} \otimes w_{8j+3 \rightarrow 8(j+1)}; \\
b_{(j+1)s,8s} &= -e_{8(j+m)+7} \otimes w_{8j+5 \rightarrow 8(j+1)}; \\
b_{2s+(j+1)s,9s} &= e_{8(j+m+1)} \otimes w_{8j+5 \rightarrow 8(j+1)}; \\
b_{4s+(j+1)s,12s} &= -w_{8(j+m+1)+1 \rightarrow 8(j+m+1)+2} \otimes w_{8j+7 \rightarrow 8(j+1)+1}; \\
b_{5s+(j+1)s,12s} &= -e_{8(j+m+1)+2} \otimes w_{8j+7 \rightarrow 8(j+1)+2}; \\
b_{(j+1)s,13s} &= -w_{8(j+m)+7 \rightarrow 8(j+m+1)+4} \otimes w_{8j+7 \rightarrow 8(j+1)}; \\
b_{7s+(j+1)s,13s} &= -w_{8(j+m+1)+3 \rightarrow 8(j+m+1)+4} \otimes w_{8j+7 \rightarrow 8(j+1)+3}; \\
b_{8s+(j+1)s,13s} &= e_{8(j+m+1)+4} \otimes w_{8j+7 \rightarrow 8(j+1)+4}; \\
b_{14s+(j+1)s,13s} &= -e_{8(j+m+1)+4} \otimes w_{8j+7 \rightarrow 8(j+1)+6}; \\
b_{11s+(j+1)s,14s} &= e_{8(j+m+1)+6} \otimes w_{8j+7 \rightarrow 8(j+1)+5}; \\
b_{3s+(j+1)s,15s} &= e_{8(j+m+1)+5} \otimes w_{8j+7 \rightarrow 8(j+1)+1}.
\end{aligned}$$

(20) If  $r_0 = 19$ , then  $\Omega^{19}(Z_t^{(2)})$  is described with  $(16s \times 16s)$  matrix with the following nonzero entries:

$$\begin{aligned}
b_{2s+(j+1)s,2s} &= -w_{8(j+m+1)+1 \rightarrow 8(j+m+1)+2} \otimes w_{8j+1 \rightarrow 8(j+1)}; \\
b_{s+(j+1)s,3s} &= e_{8(j+m+1)+6} \otimes w_{8j+1 \rightarrow 8(j+1)}; \\
b_{3s+(j+1)s,3s} &= w_{8(j+m+1)+5 \rightarrow 8(j+m+1)+6} \otimes w_{8j+1 \rightarrow 8(j+1)}; \\
b_{(j+1)s,4s} &= -e_{8(j+m+1)+3} \otimes w_{8j+2 \rightarrow 8(j+1)}; \\
b_{(j+1)s,5s} &= -w_{8(j+m+1)+3 \rightarrow 8(j+m+1)+4} \otimes w_{8j+3 \rightarrow 8(j+1)}; \\
b_{3s+(j+1)s,6s} &= -e_{8(j+m+1)+5} \otimes w_{8j+3 \rightarrow 8(j+1)}; \\
b_{s+(j+1)s,8s} &= -e_{8(j+m+1)+6} \otimes w_{8j+5 \rightarrow 8(j+1)}; \\
b_{2s+(j+1)s,10s} &= e_{8(j+m+1)+1} \otimes w_{8j+5 \rightarrow 8(j+1)}; \\
b_{s+(j+1)s,13s} &= w_{8(j+m+1)+6 \rightarrow 8(j+m+1)+7} \otimes w_{8j+7 \rightarrow 8(j+1)}; \\
b_{2s+(j+1)s,13s} &= w_{8(j+m+1)+1 \rightarrow 8(j+m+1)+7} \otimes w_{8j+7 \rightarrow 8(j+1)}; \\
b_{5s+(j+1)s,13s} &= -e_{8(j+m+1)+7} \otimes w_{8j+7 \rightarrow 8(j+1)+2}; \\
b_{7s+(j+1)s,13s} &= -e_{8(j+m+1)+7} \otimes w_{8j+7 \rightarrow 8(j+1)+4}; \\
b_{10s+(j+1)s,13s} &= -e_{8(j+m+1)+7} \otimes w_{8j+7 \rightarrow 8(j+1)+6}; \\
b_{s+(j+1)s,14s} &= -w_{8(j+m+1)+6 \rightarrow 8(j+m+2)} \otimes w_{8j+7 \rightarrow 8(j+1)}; \\
b_{2s+(j+1)s,14s} &= -w_{8(j+m+1)+1 \rightarrow 8(j+m+2)} \otimes w_{8j+7 \rightarrow 8(j+1)}; \\
b_{4s+(j+1)s,14s} &= e_{8(j+m+2)} \otimes w_{8j+7 \rightarrow 8(j+1)+1}; \\
b_{5s+(j+1)s,14s} &= w_{8(j+m+1)+7 \rightarrow 8(j+m+2)} \otimes w_{8j+7 \rightarrow 8(j+1)+2}; \\
b_{7s+(j+1)s,14s} &= w_{8(j+m+1)+7 \rightarrow 8(j+m+2)} \otimes w_{8j+7 \rightarrow 8(j+1)+4}; \\
b_{9s+(j+1)s,14s} &= e_{8(j+m+2)} \otimes w_{8j+7 \rightarrow 8(j+1)+5}; \\
b_{10s+(j+1)s,14s} &= w_{8(j+m+1)+7 \rightarrow 8(j+m+2)} \otimes w_{8j+7 \rightarrow 8(j+1)+6}; \\
b_{9s+(j+1)s,15s} &= e_{8(j+m+2)} \otimes w_{8j+7 \rightarrow 8(j+1)+5}.
\end{aligned}$$

(21) If  $r_0 = 20$ , then  $\Omega^{20}(Z_t^{(2)})$  is described with  $(16s \times 14s)$  matrix with the following nonzero entries:

$$\begin{aligned}
b_{(j+1)s,3s} &= e_{8(j+m)+7} \otimes w_{8j+1 \rightarrow 8(j+1)}; \\
b_{(j+1)s,4s} &= w_{8(j+m)+7 \rightarrow 8(j+m+1)} \otimes w_{8j+2 \rightarrow 8(j+1)}; \\
b_{s+(j+1)s,4s} &= -e_{8(j+m)+1} \otimes w_{8j+2 \rightarrow 8(j+1)}; \\
b_{(j+1)s,5s} &= -e_{8(j+m)+7} \otimes w_{8j+3 \rightarrow 8(j+1)}; \\
b_{(j+1)s,8s} &= w_{8(j+m)+7 \rightarrow 8(j+m+1)} \otimes w_{8j+5 \rightarrow 8(j+1)}; \\
b_{s+(j+1)s,8s} &= -e_{8(j+m)+1} \otimes w_{8j+5 \rightarrow 8(j+1)}; \\
b_{2s+(j+1)s,10s} &= w_{8(j+m+1)+2 \rightarrow 8(j+m+1)+3} \otimes w_{8j+7 \rightarrow 8(j+1)+1}; \\
b_{4s+(j+1)s,10s} &= -e_{8(j+m+1)+3} \otimes w_{8j+7 \rightarrow 8(j+1)+2}; \\
b_{10s+(j+1)s,10s} &= w_{8(j+m+1)+1 \rightarrow 8(j+m+1)+3} \otimes w_{8j+7 \rightarrow 8(j+1)+5}; \\
b_{(j+1)s,11s} &= -w_{8(j+m)+7 \rightarrow 8(j+m+1)+6} \otimes w_{8j+7 \rightarrow 8(j+1)}; \\
b_{7s+(j+1)s,11s} &= -e_{8(j+m+1)+6} \otimes w_{8j+7 \rightarrow 8(j+1)+4}; \\
b_{8s+(j+1)s,11s} &= -e_{8(j+m+1)+6} \otimes w_{8j+7 \rightarrow 8(j+1)+5}; \\
b_{10s+(j+1)s,12s} &= e_{8(j+m+1)+1} \otimes w_{8j+7 \rightarrow 8(j+1)+5}; \\
b_{(j+1)s,13s} &= w_{8(j+m)+7 \rightarrow 8(j+m+1)+5} \otimes w_{8j+7 \rightarrow 8(j+1)}; \\
b_{s+(j+1)s,13s} &= -w_{8(j+m+1) \rightarrow 8(j+m+1)+5} \otimes w_{8j+7 \rightarrow 8(j+1)}; \\
b_{6s+(j+1)s,13s} &= -e_{8(j+m+1)+5} \otimes w_{8j+7 \rightarrow 8(j+1)+3}; \\
b_{12s+(j+1)s,13s} &= -e_{8(j+m+1)+5} \otimes w_{8j+7 \rightarrow 8(j+1)+6}.
\end{aligned}$$

(22) If  $r_0 = 21$ , then  $\Omega^{21}(Z_t^{(2)})$  is described with  $(14s \times 13s)$  matrix with the following nonzero entries:

$$\begin{aligned}
b_{(j+1)s,2s} &= w_{8(j+m+1)+2 \rightarrow 8(j+m+1)+3} \otimes w_{8j+1 \rightarrow 8(j+1)}; \\
b_{s+(j+1)s,3s} &= -e_{8(j+m+1)+4} \otimes w_{8j+2 \rightarrow 8(j+1)}; \\
b_{(j+1)s,7s} &= e_{8(j+m+1)+2} \otimes w_{8j+5 \rightarrow 8(j+1)}; \\
b_{2s+(j+1)s,10s} &= -e_{8(j+m+1)+6} \otimes w_{8j+6 \rightarrow 8(j+1)}; \\
b_{2s+(j+1)s,11s} &= w_{8(j+m+1)+6 \rightarrow 8(j+m+1)+7} \otimes w_{8j+7 \rightarrow 8(j+1)}; \\
b_{3s+(j+1)s,11s} &= e_{8(j+m+1)+7} \otimes w_{8j+7 \rightarrow 8(j+1)+1}; \\
b_{(j+1)s,12s} &= -w_{8(j+m+1)+2 \rightarrow 8(j+m+2)} \otimes w_{8j+7 \rightarrow 8(j+1)}; \\
b_{4s+(j+1)s,12s} &= -e_{8(j+m+2)} \otimes w_{8j+7 \rightarrow 8(j+1)+2}; \\
b_{5s+(j+1)s,12s} &= -w_{8(j+m+1)+7 \rightarrow 8(j+m+2)} \otimes w_{8j+7 \rightarrow 8(j+1)+3}; \\
b_{6s+(j+1)s,12s} &= -e_{8(j+m+2)} \otimes w_{8j+7 \rightarrow 8(j+1)+4}; \\
b_{9s+(j+1)s,12s} &= -e_{8(j+m+2)} \otimes w_{8j+7 \rightarrow 8(j+1)+6}.
\end{aligned}$$

(23) If  $r_0 = 22$ , then  $\Omega^{22}(Z_t^{(2)})$  is described with  $(13s \times 11s)$  matrix with the following nonzero entries:

$$\begin{aligned}
b_{(j+1)s,2s} &= e_{8(j+m+1)} \otimes w_{8j+1 \rightarrow 8(j+1)}; \\
b_{s+(j+1)s,3s} &= -e_{8(j+m)+7} \otimes w_{8j+2 \rightarrow 8(j+1)}; \\
b_{(j+1)s,4s} &= -e_{8(j+m+1)} \otimes w_{8j+3 \rightarrow 8(j+1)}; \\
b_{s+(j+1)s,4s} &= w_{8(j+m)+7 \rightarrow 8(j+m+1)} \otimes w_{8j+3 \rightarrow 8(j+1)}; \\
b_{(j+1)s,5s} &= w_{8(j+m+1) \rightarrow 8(j+m+1)+1} \otimes w_{8j+4 \rightarrow 8(j+1)}; \\
b_{s+(j+1)s,5s} &= -w_{8(j+m)+7 \rightarrow 8(j+m+1)+1} \otimes w_{8j+4 \rightarrow 8(j+1)};
\end{aligned}$$

$$\begin{aligned}
b_{6s+(j+1)s,5s} &= e_{8(j+m+1)+1} \otimes w_{8j+4 \rightarrow 8(j+1)+4}; \\
b_{(j+1)s,8s} &= w_{8(j+m+1) \rightarrow 8(j+m+1)+2} \otimes w_{8j+7 \rightarrow 8(j+1)}; \\
b_{s+(j+1)s,8s} &= -w_{8(j+m)+7 \rightarrow 8(j+m+1)+2} \otimes w_{8j+7 \rightarrow 8(j+1)}; \\
b_{6s+(j+1)s,8s} &= w_{8(j+m+1)+1 \rightarrow 8(j+m+1)+2} \otimes w_{8j+7 \rightarrow 8(j+1)+4}; \\
b_{7s+(j+1)s,8s} &= e_{8(j+m+1)+2} \otimes w_{8j+7 \rightarrow 8(j+1)+5}; \\
b_{(j+1)s,9s} &= -w_{8(j+m+1) \rightarrow 8(j+m+1)+4} \otimes w_{8j+7 \rightarrow 8(j+1)}; \\
b_{s+(j+1)s,9s} &= w_{8(j+m)+7 \rightarrow 8(j+m+1)+4} \otimes w_{8j+7 \rightarrow 8(j+1)}; \\
b_{2s+(j+1)s,9s} &= w_{8(j+m+1)+3 \rightarrow 8(j+m+1)+4} \otimes w_{8j+7 \rightarrow 8(j+1)+1}; \\
b_{3s+(j+1)s,9s} &= -e_{8(j+m+1)+4} \otimes w_{8j+7 \rightarrow 8(j+1)+2}; \\
b_{6s+(j+1)s,9s} &= -w_{8(j+m+1)+1 \rightarrow 8(j+m+1)+4} \otimes w_{8j+7 \rightarrow 8(j+1)+4}; \\
b_{7s+(j+1)s,9s} &= -w_{8(j+m+1)+2 \rightarrow 8(j+m+1)+4} \otimes w_{8j+7 \rightarrow 8(j+1)+5}; \\
b_{4s+(j+1)s,10s} &= -w_{8(j+m+1)+5 \rightarrow 8(j+m+1)+6} \otimes w_{8j+7 \rightarrow 8(j+1)+2}; \\
b_{5s+(j+1)s,10s} &= -e_{8(j+m+1)+6} \otimes w_{8j+7 \rightarrow 8(j+1)+3}; \\
b_{10s+(j+1)s,10s} &= -e_{8(j+m+1)+6} \otimes w_{8j+7 \rightarrow 8(j+1)+6}.
\end{aligned}$$

(24) If  $r_0 = 23$ , then  $\Omega^{23}(Z_t^{(2)})$  is described with  $(11s \times 11s)$  matrix with the following nonzero entries:

$$\begin{aligned}
b_{(j+1)s,s} &= w_{8(j+m+1)+3 \rightarrow 8(j+m+1)+4} \otimes w_{8j+1 \rightarrow 8(j+1)}; \\
b_{s+(j+1)s,2s} &= e_{8(j+m+1)+5} \otimes w_{8j+1 \rightarrow 8(j+1)}; \\
b_{s+(j+1)s,3s} &= -w_{8(j+m+1)+5 \rightarrow 8(j+m+1)+6} \otimes w_{8j+2 \rightarrow 8(j+1)}; \\
b_{(j+1)s,6s} &= e_{8(j+m+1)+3} \otimes w_{8j+5 \rightarrow 8(j+1)}; \\
b_{2s+(j+1)s,9s} &= e_{8(j+m+2)} \otimes w_{8j+7 \rightarrow 8(j+1)+1}; \\
b_{(j+1)s,10s} &= -w_{8(j+m+1)+3 \rightarrow 8(j+m+1)+7} \otimes w_{8j+7 \rightarrow 8(j+1)}; \\
b_{3s+(j+1)s,10s} &= -e_{8(j+m+1)+7} \otimes w_{8j+7 \rightarrow 8(j+1)+2}; \\
b_{7s+(j+1)s,10s} &= -e_{8(j+m+1)+7} \otimes w_{8j+7 \rightarrow 8(j+1)+6}.
\end{aligned}$$

(25) If  $r_0 = 24$ , then  $\Omega^{24}(Z_t^{(2)})$  is described with  $(11s \times 10s)$  matrix with the following nonzero entries:

$$\begin{aligned}
b_{(j+1)s,3s} &= e_{8(j+m+1)} \otimes w_{8j+2 \rightarrow 8(j+1)}; \\
b_{(j+1)s,4s} &= -w_{8(j+m+1) \rightarrow 8(j+m+1)+1} \otimes w_{8j+3 \rightarrow 8(j+1)}; \\
b_{4s+(j+1)s,4s} &= e_{8(j+m+1)+1} \otimes w_{8j+3 \rightarrow 8(j+1)+3}; \\
b_{(j+1)s,5s} &= w_{8(j+m+1) \rightarrow 8(j+m+1)+2} \otimes w_{8j+4 \rightarrow 8(j+1)}; \\
b_{4s+(j+1)s,5s} &= -w_{8(j+m+1)+1 \rightarrow 8(j+m+1)+2} \otimes w_{8j+4 \rightarrow 8(j+1)+3}; \\
b_{5s+(j+1)s,5s} &= e_{8(j+m+1)+2} \otimes w_{8j+4 \rightarrow 8(j+1)+4}; \\
b_{(j+1)s,8s} &= w_{8(j+m+1) \rightarrow 8(j+m+1)+3} \otimes w_{8j+7 \rightarrow 8(j+1)}; \\
b_{(3+j_1)s+(j+1)s,8s} &= (1 - 2f(j_1, 1))w_{8(j+m+1)+j_1 \rightarrow 8(j+m+1)+3} \otimes w_{8j+7 \rightarrow 8(j+1)+2+j_1}, \quad 1 \leq j_1 \leq 3; \\
b_{2s+(j+1)s,9s} &= e_{8(j+m+1)+5} \otimes w_{8j+7 \rightarrow 8(j+1)+1}.
\end{aligned}$$

(26) If  $r_0 = 25$ , then  $\Omega^{25}(Z_t^{(2)})$  is described with  $(10s \times 8s)$  matrix with the following nonzero entries:

$$\begin{aligned}
b_{s+(j+1)s,s} &= e_{8(j+m+1)+6} \otimes w_{8j+1 \rightarrow 8(j+1)}; \\
b_{(j+1)s,5s} &= e_{8(j+m+1)+4} \otimes w_{8j+5 \rightarrow 8(j+1)}; \\
b_{(j+1)s,7s} &= w_{8(j+m+1)+4 \rightarrow 8(j+m+2)} \otimes w_{8j+7 \rightarrow 8(j+1)};
\end{aligned}$$

$$\begin{aligned}
b_{2s+(j+1)s,7s} &= w_{8(j+m+1)+7 \rightarrow 8(j+m+2)} \otimes w_{8j+7 \rightarrow 8(j+1)+1}; \\
b_{3s+(j+1)s,7s} &= e_{8(j+m+2)} \otimes w_{8j+7 \rightarrow 8(j+1)+2}; \\
b_{7s+(j+1)s,7s} &= e_{8(j+m+2)} \otimes w_{8j+7 \rightarrow 8(j+1)+6}.
\end{aligned}$$

(27) If  $r_0 = 26$ , then  $\Omega^{26}(Z_t^{(2)})$  is described with  $(8s \times 9s)$  matrix with the following nonzero entries:

$$\begin{aligned}
b_{(j+1)s,0} &= e_{8(j+m)+7} \otimes w_{8j \rightarrow 8(j+1)}; \\
b_{(j+1)s,s} &= -w_{8(j+m)+7 \rightarrow 8(j+m+1)} \otimes w_{8j+1 \rightarrow 8(j+1)}; \\
b_{(j+1)s,2s} &= w_{8(j+m)+7 \rightarrow 8(j+m+1)+1} \otimes w_{8j+2 \rightarrow 8(j+1)}; \\
b_{2s+(j+1)s,2s} &= e_{8(j+m+1)+1} \otimes w_{8j+2 \rightarrow 8(j+1)+2}; \\
b_{(j+1)s,3s} &= -w_{8(j+m)+7 \rightarrow 8(j+m+1)+2} \otimes w_{8j+3 \rightarrow 8(j+1)}; \\
b_{2s+(j+1)s,3s} &= -w_{8(j+m+1)+1 \rightarrow 8(j+m+1)+2} \otimes w_{8j+3 \rightarrow 8(j+1)+2}; \\
b_{3s+(j+1)s,3s} &= e_{8(j+m+1)+2} \otimes w_{8j+3 \rightarrow 8(j+1)+3}; \\
b_{(j+1)s,4s} &= w_{8(j+m)+7 \rightarrow 8(j+m+1)+3} \otimes w_{8j+4 \rightarrow 8(j+1)}; \\
b_{(1+j_1)s+(j+1)s,4s} &= (-1)^{j_1+1} w_{8(j+m+1)+j_1 \rightarrow 8(j+m+1)+3} \otimes w_{8j+4 \rightarrow 8(j+1)+1+j_1}, \quad 1 \leq j_1 \leq 3; \\
b_{6s+(j+1)s,6s} &= e_{8(j+m+1)+5} \otimes w_{8j+6 \rightarrow 8(j+1)+6}; \\
b_{(j+1)s,7s} &= w_{8(j+m)+7 \rightarrow 8(j+m+1)+4} \otimes w_{8j+7 \rightarrow 8(j+1)}; \\
b_{(1+j_1)s+(j+1)s,7s} &= (1 - 2f(j_1, 2)) w_{8(j+m+1)+j_1 \rightarrow 8(j+m+1)+4} \otimes w_{8j+7 \rightarrow 8(j+1)+1+j_1}, \quad 1 \leq j_1 \leq 4; \\
b_{s+(j+1)s,8s} &= e_{8(j+m+1)+6} \otimes w_{8j+7 \rightarrow 8(j+1)+1}; \\
b_{6s+(j+1)s,8s} &= w_{8(j+m+1)+5 \rightarrow 8(j+m+1)+6} \otimes w_{8j+7 \rightarrow 8(j+1)+6}.
\end{aligned}$$

(28) If  $r_0 = 27$ , then  $\Omega^{27}(Z_t^{(2)})$  is described with  $(9s \times 8s)$  matrix with two nonzero entries:

$$\begin{aligned}
b_{j,7s} &= -w_{8(j+m+1)+4 \rightarrow 8(j+m+1)+7} \otimes e_{8j+7}; \\
b_{j+s,7s} &= w_{8(j+m+1)+6 \rightarrow 8(j+m+1)+7} \otimes e_{8j+7}.
\end{aligned}$$

(29) If  $r_0 = 28$ , then  $\Omega^{28}(Z_t^{(2)})$  is described with  $(8s \times 8s)$  matrix with the following nonzero entries:

$$\begin{aligned}
b_{(j+1)s,0} &= e_{8(j+m+1)} \otimes w_{8j \rightarrow 8(j+1)}; \\
b_{j+7s,0} &= -w_{8(j+m)+7 \rightarrow 8(j+m+1)} \otimes w_{8j \rightarrow 8j+7}; \\
b_{j+j_1s,s} &= (-1)^{j_1} w_{8(j+m)+1+j_1 \rightarrow 8(j+m+1)+1} \otimes w_{8j+1 \rightarrow 8j+1+j_1}, \quad 0 \leq j_1 \leq 3; \\
b_{j+j_1s,2s} &= (-1)^{j_1} w_{8(j+m)+2+j_1 \rightarrow 8(j+m+1)+2} \otimes w_{8j+2 \rightarrow 8j+2+j_1}, \quad 0 \leq j_1 \leq 2; \\
b_{j,3s} &= w_{8(j+m)+3 \rightarrow 8(j+m+1)+3} \otimes e_{8j+3}; \\
b_{j+s,3s} &= -w_{8(j+m)+4 \rightarrow 8(j+m+1)+3} \otimes w_{8j+3 \rightarrow 8j+4}; \\
b_{j,4s} &= w_{8(j+m)+4 \rightarrow 8(j+m+1)+4} \otimes e_{8j+4}; \\
b_{j,5s} &= w_{8(j+m)+5 \rightarrow 8(j+m+1)+5} \otimes e_{8j+5}; \\
b_{j+s,5s} &= -w_{8(j+m)+6 \rightarrow 8(j+m+1)+5} \otimes w_{8j+5 \rightarrow 8j+6}; \\
b_{j,6s} &= w_{8(j+m)+6 \rightarrow 8(j+m+1)+6} \otimes e_{8j+6}; \\
b_{7s+(j+1)s,7s+(-1)s} &= e_{8(j+m+1)+7} \otimes w_{8j+7 \rightarrow 8(j+1)+7}.
\end{aligned}$$

(II) Represent an arbitrary  $t_0 \in \mathbb{N}$  in the form  $t_0 = 29\ell_0 + r_0$ , where  $0 \leq r_0 \leq 28$ . Then  $\Omega^{t_0}(Z_t^{(2)})$  is a  $\Omega^{r_0}(Z_t^{(2)})$ , whose left components twisted by  $\sigma^{\ell_0}$ , and coefficients multiplied by  $(-1)^{\ell_0}$ .

**Proposition 3** (Translates for the case 3). (I) Let  $r_0 \in \mathbb{N}$ ,  $r_0 < 29$ .  $r_0$ -translates of the elements  $Z_t^{(3)}$  are described by the following way.

(1) If  $r_0 = 0$ , then  $\Omega^0(Z_t^{(3)})$  is described with  $(8s \times 10s)$  matrix, whose entries  $b_{ij}$  have the following form:

If  $0 \leq j < 2s$ , then

$$b_{ij} = \begin{cases} (-1)^{j_2} w_{8(j+m) \rightarrow 8(j+m)+2+4j_2} \otimes e_{8j}, & i = j - j_2 s; \\ 0, & \text{otherwise.} \end{cases}$$

If  $2s \leq j < 5s$ , then  $b_{ij} = 0$ .

If  $5s \leq j < 6s$ , then

$$b_{ij} = \begin{cases} w_{8(j+m)+4 \rightarrow 8(j+m+1)} \otimes e_{8j+4}, & i = j - s; \\ 0, & \text{otherwise.} \end{cases}$$

If  $6s \leq j < 8s$ , then  $b_{ij} = 0$ .

If  $8s \leq j < 9s$ , then

$$b_{ij} = \begin{cases} w_{8(j+m)+7 \rightarrow 8(j+m+1)+1} \otimes e_{8j+7}, & i = j - s; \\ 0, & \text{otherwise.} \end{cases}$$

If  $9s \leq j < 10s$ , then  $b_{ij} = 0$ .

(2) If  $r_0 = 1$ , then  $\Omega^1(Z_t^{(3)})$  is described with  $(9s \times 11s)$  matrix, whose entries  $b_{ij}$  have the following form:

If  $s \leq j < 2s$ , then

$$b_{ij} = \begin{cases} -w_{8(j+m)+1 \rightarrow 8(j+m+1)} \otimes e_{8j}, & i = j - s; \\ -w_{8(j+m)+j_1+1 \rightarrow 8(j+m+1)} \otimes w_{8j \rightarrow 8j+j_1}, & i = j + j_1 s, \ 1 \leq j_1 \leq 3; \\ 0, & \text{otherwise.} \end{cases}$$

If  $2s \leq j < 3s$ , then

$$b_{ij} = \begin{cases} -w_{8(j+m+1)+1 \rightarrow 8(j+m+1)+3} \otimes w_{8j+1 \rightarrow 8(j+1)}, & i = (j+1)s; \\ -w_{8(j+m+1)+2 \rightarrow 8(j+m+1)+3} \otimes w_{8j+1 \rightarrow 8(j+1)+1}, & i = 2s + (j+1)s; \\ 0, & \text{otherwise.} \end{cases}$$

If  $3s \leq j < 4s$ , then

$$b_{ij} = \begin{cases} w_{8(j+m+1)+1 \rightarrow 8(j+m+1)+4} \otimes w_{8j+2 \rightarrow 8(j+1)}, & i = (j+1)s; \\ w_{8(j+m+1)+2 \rightarrow 8(j+m+1)+4} \otimes w_{8j+2 \rightarrow 8(j+1)+1}, & i = 2s + (j+1)s; \\ w_{8(j+m+1)+3 \rightarrow 8(j+m+1)+4} \otimes w_{8j+2 \rightarrow 8(j+1)+2}, & i = 3s + (j+1)s; \\ 0, & \text{otherwise.} \end{cases}$$

If  $4s \leq j < 5s$ , then  $b_{ij} = 0$ .

If  $5s \leq j < 6s$ , then

$$b_{ij} = \begin{cases} w_{8(j+m+1)+5 \rightarrow 8(j+m+1)+6} \otimes w_{8j+4 \rightarrow 8(j+1)}, & i = s + (j+1)s; \\ 0, & \text{otherwise.} \end{cases}$$

If  $6s \leq j < 8s$ , then

$$b_{ij} = \begin{cases} -w_{8(j+m)+7 \rightarrow 8(j+m+1)+1} \otimes w_{8j+j_2-2 \rightarrow 8j+2(j_2-4)}, & i = j + (j_2 - 7)s; \\ 0, & \text{otherwise.} \end{cases}$$

If  $8s \leq j < 9s$ , then

$$b_{ij} = \begin{cases} w_{8(j+m+1)+1 \rightarrow 8(j+m+1)+2} \otimes w_{8j+6 \rightarrow 8(j+1)}, & i = (j+1)s; \\ w_{8(j+m)+7 \rightarrow 8(j+m+1)+2} \otimes e_{8j+6}, & i = j - s; \\ 0, & \text{otherwise.} \end{cases}$$

If  $9s \leq j < 10s$ , then  $b_{ij} = 0$ .

If  $10s \leq j < 11s$ , then

$$b_{ij} = \begin{cases} -w_{8(j+m+1) \rightarrow 8(j+m+1)+7} \otimes e_{8j+7}, & i = j - 2s; \\ 0, & \text{otherwise.} \end{cases}$$

(3) If  $r_0 = 2$ , then  $\Omega^2(Z_t^{(3)})$  is described with  $(8s \times 11s)$  matrix, whose entries  $b_{ij}$  have the following form:

If  $2s \leq j < 3s$ , then

$$b_{ij} = \begin{cases} w_{8(j+m-1)+7 \rightarrow 8(j+m)+1} \otimes e_{8j}, & i = j - 2s; \\ 0, & \text{otherwise.} \end{cases}$$

If  $3s \leq j < 4s$ , then  $b_{ij} = 0$ .

If  $4s \leq j < 6s$ , then

$$b_{ij} = \begin{cases} w_{8(j+m)+7 \rightarrow 8(j+m)+j_2+3} \otimes w_{8j+j_2-2 \rightarrow 8(j+1)}, & i = (j+1)s; \\ 0, & \text{otherwise.} \end{cases}$$

If  $6s \leq j < 7s$ , then

$$b_{ij} = \begin{cases} -w_{8(j+m)+5 \rightarrow 8(j+m)+7} \otimes e_{8j+4}, & i = j - 2s; \\ 0, & \text{otherwise.} \end{cases}$$

If  $7s \leq j < 8s$ , then  $b_{ij} = 0$ .

If  $8s \leq j < 9s$ , then

$$b_{ij} = \begin{cases} w_{8(j+m)+1 \rightarrow 8(j+m)+7} \otimes e_{8j+6}, & i = j - 2s; \\ 0, & \text{otherwise.} \end{cases}$$

If  $9s \leq j < 10s$ , then

$$b_{ij} = \begin{cases} w_{8(j+m)+7 \rightarrow 8(j+m+1)+2} \otimes w_{8j+7 \rightarrow 8(j+1)}, & i = (j+1)s; \\ 0, & \text{otherwise.} \end{cases}$$

If  $10s \leq j < 11s$ , then  $b_{ij} = 0$ .

(4) If  $r_0 = 3$ , then  $\Omega^3(Z_t^{(3)})$  is described with  $(10s \times 13s)$  matrix, whose entries  $b_{ij}$  have the following form:

If  $0 \leq j < s$ , then

$$b_{ij} = \begin{cases} w_{8(j+m)+2 \rightarrow 8(j+m)+7} \otimes e_{8j}, & i = j; \\ w_{8(j+m)+3 \rightarrow 8(j+m)+7} \otimes w_{8j \rightarrow 8j+1}, & i = j + 2s; \\ w_{8(j+m)+4 \rightarrow 8(j+m)+7} \otimes w_{8j \rightarrow 8j+2}, & i = j + 3s; \\ e_{8(j+m)+7} \otimes w_{8j \rightarrow 8j+3}, & i = j + 4s; \\ 0, & \text{otherwise.} \end{cases}$$

If  $s \leq j < 2s$ , then  $b_{ij} = 0$ .

If  $2s \leq j < 3s$ , then

$$b_{ij} = \begin{cases} -w_{8(j+m+1)+2 \rightarrow 8(j+m+1)+4} \otimes w_{8j+1 \rightarrow 8(j+1)}, & i = (j+1)_s; \\ -w_{8(j+m+1)+3 \rightarrow 8(j+m+1)+4} \otimes w_{8j+1 \rightarrow 8(j+1)+1}, & i = 2s + (j+1)_s; \\ 0, & \text{otherwise.} \end{cases}$$

If  $3s \leq j < 4s$ , then  $b_{ij} = 0$ .

If  $4s \leq j < 5s$ , then

$$b_{ij} = \begin{cases} -e_{8(j+m+1)+6} \otimes w_{8j+3 \rightarrow 8(j+1)}, & i = s + (j+1)_s; \\ 0, & \text{otherwise.} \end{cases}$$

If  $5s \leq j < 7s$ , then  $b_{ij} = 0$ .

If  $7s \leq j < 8s$ , then

$$b_{ij} = \begin{cases} e_{8(j+m+1)+2} \otimes w_{8j+5 \rightarrow 8(j+1)}, & i = (j+1)_s; \\ 0, & \text{otherwise.} \end{cases}$$

If  $8s \leq j < 13s$ , then  $b_{ij} = 0$ .

(5) If  $r_0 = 4$ , then  $\Omega^4(Z_t^{(3)})$  is described with  $(11s \times 14s)$  matrix, whose entries  $b_{ij}$  have the following form:

If  $0 \leq j < s$ , then

$$b_{ij} = \begin{cases} -w_{8(j+m-1)+7 \rightarrow 8(j+m)+2} \otimes e_{8j}, & i = j; \\ -w_{8(j+m) \rightarrow 8(j+m)+2} \otimes e_{8j}, & i = j + s; \\ w_{8(j+m)+1 \rightarrow 8(j+m)+2} \otimes w_{8j \rightarrow 8j+4}, & i = j + 6s; \\ -e_{8(j+m)+2} \otimes w_{8j \rightarrow 8j+6}, & i = j + 8s; \\ 0, & \text{otherwise.} \end{cases}$$

If  $s \leq j < 2s$ , then  $b_{ij} = 0$ .

If  $2s \leq j < 3s$ , then

$$b_{ij} = \begin{cases} w_{8(j+m)+5 \rightarrow 8(j+m)+6} \otimes w_{8j \rightarrow 8j+3}, & i = j + 2s; \\ -e_{8(j+m)+6} \otimes w_{8j \rightarrow 8j+4}, & i = j + 3s; \\ 0, & \text{otherwise.} \end{cases}$$

If  $3s \leq j < 5s$ , then  $b_{ij} = 0$ .

If  $5s \leq j < 6s$ , then

$$b_{ij} = \begin{cases} w_{8(j+m)+7 \rightarrow 8(j+m+1)} \otimes w_{8j+2 \rightarrow 8(j+1)}, & i = (j+1)_s; \\ e_{8(j+m+1)} \otimes w_{8j+2 \rightarrow 8(j+1)}, & i = s + (j+1)_s; \\ 0, & \text{otherwise.} \end{cases}$$

If  $6s \leq j < 7s$ , then

$$b_{ij} = \begin{cases} -e_{8(j+m)+7} \otimes w_{8j+3 \rightarrow 8(j+1)}, & i = (j+1)_s; \\ 0, & \text{otherwise.} \end{cases}$$

If  $7s \leq j < 12s$ , then  $b_{ij} = 0$ .

If  $12s \leq j < 13s$ , then

$$b_{ij} = \begin{cases} e_{8(j+m+1)+3} \otimes w_{8j+7 \rightarrow 8(j+1)+1}, & i = 2s + (j+1)_s; \\ 0, & \text{otherwise.} \end{cases}$$

If  $13s \leq j < 14s$ , then  $b_{ij} = 0$ .

(6) If  $r_0 = 5$ , then  $\Omega^5(Z_t^{(3)})$  is described with  $(11s \times 16s)$  matrix, whose entries  $b_{ij}$  have the following form:

If  $0 \leq j < s$ , then

$$b_{ij} = \begin{cases} -w_{8(j+m)+3 \rightarrow 8(j+m)+7} \otimes e_{8j}, & i = j + s; \\ -w_{8(j+m)+1 \rightarrow 8(j+m)+7} \otimes e_{8j}, & i = j + 2s; \\ -w_{8(j+m)+4 \rightarrow 8(j+m)+7} \otimes w_{8j \rightarrow 8j+1}, & i = j + 3s; \\ -e_{8(j+m)+7} \otimes w_{8j \rightarrow 8j+2}, & i = j + 4s; \\ 0, & \text{otherwise.} \end{cases}$$

If  $s \leq j < 2s$ , then  $b_{ij} = 0$ .

If  $2s \leq j < 3s$ , then

$$b_{ij} = \begin{cases} e_{8(j+m+1)} \otimes w_{8j \rightarrow 8j+3}, & i = j + 3s; \\ 0, & \text{otherwise.} \end{cases}$$

If  $3s \leq j < 5s$ , then

$$b_{ij} = \begin{cases} (-1)^{j_2+1} w_{8(j+m+1)+5 \rightarrow 8(j+m+1)+j_2+2} \otimes w_{8j+j_2-2 \rightarrow 8(j+1)}, & i = (j+1)_s; \\ 0, & \text{otherwise.} \end{cases}$$

If  $5s \leq j < 7s$ , then

$$b_{ij} = \begin{cases} -w_{8(j+m+1)+1 \rightarrow 8(j+m+1)+j_2-4} \otimes w_{8j+j_2-3 \rightarrow 8(j+1)}, & i = 2s + (j+1)_s; \\ 0, & \text{otherwise.} \end{cases}$$

If  $7s \leq j < 8s$ , then

$$b_{ij} = \begin{cases} e_{8(j+m+1)+3} \otimes w_{8j+4 \rightarrow 8(j+1)}, & i = s + (j+1)_s; \\ w_{8(j+m+1)+1 \rightarrow 8(j+m+1)+3} \otimes w_{8j+4 \rightarrow 8(j+1)}, & i = 2s + (j+1)_s; \\ 0, & \text{otherwise.} \end{cases}$$

If  $8s \leq j < 12s$ , then  $b_{ij} = 0$ .



If  $12s \leq j < 13s$ , then

$$b_{ij} = \begin{cases} w_{8(j+m+1)+3 \rightarrow 8(j+m+1)+4} \otimes w_{8j+6 \rightarrow 8(j+1)}, & i = s + (j+1)_s; \\ w_{8(j+m+1)+1 \rightarrow 8(j+m+1)+4} \otimes w_{8j+6 \rightarrow 8(j+1)}, & i = 2s + (j+1)_s; \\ 0, & \text{otherwise.} \end{cases}$$

If  $13s \leq j < 14s$ , then  $b_{ij} = 0$ .

If  $14s \leq j < 16s$ , then

$$b_{ij} = \begin{cases} -w_{8(j+m+1)+3 \rightarrow 8(j+m+1)+j_2-7} \otimes w_{8j+7 \rightarrow 8(j+1)}, & i = s + (j+1)_s; \\ -w_{8(j+m+1)+1 \rightarrow 8(j+m+1)+j_2-7} \otimes w_{8j+7 \rightarrow 8(j+1)}, & i = 2s + (j+1)_s; \\ 0, & \text{otherwise.} \end{cases}$$

(7) If  $r_0 = 6$ , then  $\Omega^6(Z_t^{(3)})$  is described with  $(13s \times 16s)$  matrix, whose entries  $b_{ij}$  have the following form:

If  $0 \leq j < s$ , then

$$b_{ij} = \begin{cases} e_{8(j+m)+5} \otimes w_{8j \rightarrow 8j+2}, & i = j + 3s; \\ 0, & \text{otherwise.} \end{cases}$$

If  $s \leq j < 2s$ , then

$$b_{ij} = \begin{cases} w_{8(j+m-1)+7 \rightarrow 8(j+m)+3} \otimes e_{8j}, & i = j - s; \\ -w_{8(j+m)+2 \rightarrow 8(j+m)+3} \otimes w_{8j \rightarrow 8j+4}, & i = j + 5s; \\ -e_{8(j+m)+3} \otimes w_{8j \rightarrow 8j+6}, & i = j + 8s; \\ 0, & \text{otherwise.} \end{cases}$$

If  $2s \leq j < 3s$ , then  $b_{ij} = 0$ .

If  $3s \leq j < 4s$ , then

$$b_{ij} = \begin{cases} -e_{8(j+m)+1} \otimes w_{8j \rightarrow 8j+3}, & i = j + 2s; \\ 0, & \text{otherwise.} \end{cases}$$

If  $4s \leq j < 5s$ , then  $b_{ij} = 0$ .

If  $5s \leq j < 7s$ , then

$$b_{ij} = \begin{cases} (-1)^{j_2+1} e_{8(j+m)+j_2+2} \otimes w_{8j+j_2-3 \rightarrow 8(j+1)}, & i = (j_2 - 5)s + (j+1)_s; \\ 0, & \text{otherwise.} \end{cases}$$

If  $7s \leq j < 13s$ , then  $b_{ij} = 0$ .

If  $13s \leq j < 14s$ , then

$$b_{ij} = \begin{cases} e_{8(j+m+1)+4} \otimes w_{8j+7 \rightarrow 8(j+1)+1}, & i = 2s + (j+1)_s; \\ 0, & \text{otherwise.} \end{cases}$$

If  $14s \leq j < 16s$ , then  $b_{ij} = 0$ .

(8) If  $r_0 = 7$ , then  $\Omega^7(Z_t^{(3)})$  is described with  $(14s \times 19s)$  matrix, whose entries  $b_{ij}$  have the following form:

If  $0 \leq j < s$ , then

$$b_{ij} = \begin{cases} w_{8(j+m)+2 \rightarrow 8(j+m)+7} \otimes e_{8j}, & i = j; \\ -w_{8(j+m)+4 \rightarrow 8(j+m)+7} \otimes e_{8j}, & i = j + s; \\ -e_{8(j+m)+7} \otimes w_{8j \rightarrow 8j+1}, & i = j + 4s; \\ 0, & \text{otherwise.} \end{cases}$$

If  $s \leq j < 2s$ , then

$$b_{ij} = \begin{cases} w_{8(j+m)+2 \rightarrow 8(j+m+1)} \otimes e_{8j}, & i = j - s; \\ -w_{8(j+m)+4 \rightarrow 8(j+m+1)} \otimes e_{8j}, & i = j; \\ -w_{8(j+m)+7 \rightarrow 8(j+m+1)} \otimes w_{8j \rightarrow 8j+1}, & i = j + 3s; \\ -e_{8(j+m+1)} \otimes w_{8j \rightarrow 8j+2}, & i = j + 4s; \\ 0, & \text{otherwise.} \end{cases}$$

If  $2s \leq j < 3s$ , then  $b_{ij} = 0$ .

If  $3s \leq j < 4s$ , then

$$b_{ij} = \begin{cases} e_{8(j+m+1)+6} \otimes w_{8j+1 \rightarrow 8(j+1)}, & i = 2s + (j+1)_s; \\ 0, & \text{otherwise.} \end{cases}$$

If  $4s \leq j < 5s$ , then  $b_{ij} = 0$ .

If  $5s \leq j < 7s$ , then

$$b_{ij} = \begin{cases} (-1)^{j_2} w_{8(j+m+1)+2 \rightarrow 8(j+m+1)+j_2-3} \otimes w_{8j+j_2-3 \rightarrow 8(j+1)}, & i = (j+1)_s; \\ 0, & \text{otherwise.} \end{cases}$$

If  $7s \leq j < 8s$ , then

$$b_{ij} = \begin{cases} -e_{8(j+m+1)+5} \otimes w_{8j+3 \rightarrow 8(j+1)}, & i = 3s + (j+1)_s; \\ 0, & \text{otherwise.} \end{cases}$$

If  $8s \leq j < 9s$ , then

$$b_{ij} = \begin{cases} -w_{8(j+m+1)+2 \rightarrow 8(j+m+1)+4} \otimes w_{8j+4 \rightarrow 8(j+1)}, & i = (j+1)_s; \\ e_{8(j+m+1)+4} \otimes w_{8j+4 \rightarrow 8(j+1)}, & i = s + (j+1)_s; \\ 0, & \text{otherwise.} \end{cases}$$

If  $9s \leq j < 17s$ , then  $b_{ij} = 0$ .

If  $17s \leq j < 18s$ , then

$$b_{ij} = \begin{cases} w_{8(j+m+1)+2 \rightarrow 8(j+m+1)+7} \otimes w_{8j+7 \rightarrow 8(j+1)}, & i = (j+1)_s; \\ -w_{8(j+m+1)+4 \rightarrow 8(j+m+1)+7} \otimes w_{8j+7 \rightarrow 8(j+1)}, & i = s + (j+1)_s; \\ 0, & \text{otherwise.} \end{cases}$$

If  $18s \leq j < 19s$ , then  $b_{ij} = 0$ .

(9) If  $r_0 = 8$ , then  $\Omega^8(Z_t^{(3)})$  is described with  $(16s \times 18s)$  matrix, whose entries  $b_{ij}$  have the following form:

If  $0 \leq j < s$ , then

$$b_{ij} = \begin{cases} -w_{8(j+m)+1 \rightarrow 8(j+m)+2} \otimes w_{8j \rightarrow 8j+2}, & i = j + 5s; \\ -e_{8(j+m)+2} \otimes w_{8j \rightarrow 8j+3}, & i = j + 6s; \\ 0, & \text{otherwise.} \end{cases}$$

If  $s \leq j < 2s$ , then

$$b_{ij} = \begin{cases} -w_{8(j+m)+5 \rightarrow 8(j+m)+6} \otimes w_{8j \rightarrow 8j+1}, & i = j + 2s; \\ e_{8(j+m)+6} \otimes w_{8j \rightarrow 8j+2}, & i = j + 3s; \\ 0, & \text{otherwise.} \end{cases}$$

If  $2s \leq j < 3s$ , then

$$b_{ij} = \begin{cases} w_{8(j+m-1)+7 \rightarrow 8(j+m)+4} \otimes e_{8j}, & i = j - 2s; \\ -w_{8(j+m-1)+7 \rightarrow 8(j+m)+4} \otimes e_{8j}, & i = j - s; \\ -w_{8(j+m)+1 \rightarrow 8(j+m)+4} \otimes w_{8j \rightarrow 8j+2}, & i = j + 3s; \\ -w_{8(j+m)+3 \rightarrow 8(j+m)+4} \otimes w_{8j \rightarrow 8j+4}, & i = j + 5s; \\ -e_{8(j+m)+4} \otimes w_{8j \rightarrow 8j+6}, & i = j + 10s; \\ 0, & \text{otherwise.} \end{cases}$$

If  $3s \leq j < 4s$ , then  $b_{ij} = 0$ .

If  $4s \leq j < 5s$ , then

$$b_{ij} = \begin{cases} -e_{8(j+m)+5} \otimes w_{8j \rightarrow 8j+1}, & i = j - s; \\ 0, & \text{otherwise.} \end{cases}$$

If  $5s \leq j < 6s$ , then

$$b_{ij} = \begin{cases} e_{8(j+m)+7} \otimes w_{8j+1 \rightarrow 8(j+1)}, & i = (j+1)_s; \\ -e_{8(j+m)+7} \otimes w_{8j+1 \rightarrow 8(j+1)}, & i = s + (j+1)_s; \\ 0, & \text{otherwise.} \end{cases}$$

If  $6s \leq j < 7s$ , then

$$b_{ij} = \begin{cases} w_{8(j+m)+7 \rightarrow 8(j+m+1)} \otimes w_{8j+2 \rightarrow 8(j+1)}, & i = (j+1)_s; \\ -w_{8(j+m)+7 \rightarrow 8(j+m+1)} \otimes w_{8j+2 \rightarrow 8(j+1)}, & i = s + (j+1)_s; \\ e_{8(j+m+1)} \otimes w_{8j+2 \rightarrow 8(j+1)}, & i = 2s + (j+1)_s; \\ 0, & \text{otherwise.} \end{cases}$$

If  $7s \leq j < 8s$ , then

$$b_{ij} = \begin{cases} -e_{8(j+m)+7} \otimes w_{8j+3 \rightarrow 8(j+1)}, & i = s + (j+1)_s; \\ 0, & \text{otherwise.} \end{cases}$$

If  $8s \leq j < 18s$ , then  $b_{ij} = 0$ .

(10) If  $r_0 = 9$ , then  $\Omega^9(Z_t^{(3)})$  is described with  $(16s \times 19s)$  matrix, whose entries  $b_{ij}$  have the following form:

If  $0 \leq j < s$ , then

$$b_{ij} = \begin{cases} e_{8(j+m)+7} \otimes w_{8j \rightarrow 8j+2}, & i = j + 5s; \\ 0, & \text{otherwise.} \end{cases}$$

If  $s \leq j < 2s$ , then

$$b_{ij} = \begin{cases} w_{8(j+m)+3 \rightarrow 8(j+m+1)} \otimes e_{8j}, & i = j; \\ -w_{8(j+m)+6 \rightarrow 8(j+m+1)} \otimes e_{8j}, & i = j + s; \\ -e_{8(j+m+1)} \otimes w_{8j \rightarrow 8j+1}, & i = j + 3s; \\ w_{8(j+m)+7 \rightarrow 8(j+m+1)} \otimes w_{8j \rightarrow 8j+5}, & i = j + 7s; \\ 0, & \text{otherwise.} \end{cases}$$

If  $2s \leq j < 3s$ , then

$$b_{ij} = \begin{cases} w_{8(j+m)+3 \rightarrow 8(j+m)+7} \otimes e_{8j}, & i = j - s; \\ -w_{8(j+m)+6 \rightarrow 8(j+m)+7} \otimes e_{8j}, & i = j; \\ e_{8(j+m)+7} \otimes w_{8j \rightarrow 8j+2}, & i = j + 3s; \\ e_{8(j+m)+7} \otimes w_{8j \rightarrow 8j+5}, & i = j + 6s; \\ 0, & \text{otherwise.} \end{cases}$$

If  $3s \leq j < 4s$ , then

$$b_{ij} = \begin{cases} w_{8(j+m+1)+1 \rightarrow 8(j+m+1)+2} \otimes w_{8j+1 \rightarrow 8(j+1)}, & i = 3s + (j + 1)_s; \\ 0, & \text{otherwise.} \end{cases}$$

If  $4s \leq j < 5s$ , then

$$b_{ij} = \begin{cases} -e_{8(j+m+1)+3} \otimes w_{8j+2 \rightarrow 8(j+1)}, & i = s + (j + 1)_s; \\ -w_{8(j+m+1)+1 \rightarrow 8(j+m+1)+3} \otimes w_{8j+2 \rightarrow 8(j+1)}, & i = 3s + (j + 1)_s; \\ 0, & \text{otherwise.} \end{cases}$$

If  $5s \leq j < 6s$ , then

$$b_{ij} = \begin{cases} e_{8(j+m+1)+5} \otimes w_{8j+2 \rightarrow 8(j+1)}, & i = (j + 1)_s; \\ 0, & \text{otherwise.} \end{cases}$$

If  $6s \leq j < 7s$ , then

$$b_{ij} = \begin{cases} w_{8(j+m+1)+3 \rightarrow 8(j+m+1)+4} \otimes w_{8j+3 \rightarrow 8(j+1)}, & i = s + (j + 1)_s; \\ 0, & \text{otherwise.} \end{cases}$$

If  $7s \leq j < 8s$ , then

$$b_{ij} = \begin{cases} -e_{8(j+m+1)+6} \otimes w_{8j+3 \rightarrow 8(j+1)}, & i = 2s + (j + 1)_s; \\ 0, & \text{otherwise.} \end{cases}$$

If  $8s \leq j < 18s$ , then  $b_{ij} = 0$ .

If  $18s \leq j < 19s$ , then

$$b_{ij} = \begin{cases} w_{8(j+m+1)+3 \rightarrow 8(j+m+2)} \otimes w_{8j+7 \rightarrow 8(j+1)}, & i = s + (j+1)_s; \\ -w_{8(j+m+1)+6 \rightarrow 8(j+m+2)} \otimes w_{8j+7 \rightarrow 8(j+1)}, & i = 2s + (j+1)_s; \\ w_{8(j+m+1)+7 \rightarrow 8(j+m+2)} \otimes w_{8j+7 \rightarrow 8(j+1)+2}, & i = 5s + (j+1)_s; \\ w_{8(j+m+1)+7 \rightarrow 8(j+m+2)} \otimes w_{8j+7 \rightarrow 8(j+1)+5}, & i = 8s + (j+1)_s; \\ 0, & \text{otherwise.} \end{cases}$$

(11) If  $r_0 = 10$ , then  $\Omega^{10}(Z_t^{(3)})$  is described with  $(19s \times 18s)$  matrix, whose entries  $b_{ij}$  have the following form:

If  $0 \leq j < s$ , then

$$b_{ij} = \begin{cases} w_{8(j+m)+1 \rightarrow 8(j+m)+2} \otimes w_{8j \rightarrow 8j+1}, & i = j + 4s; \\ 0, & \text{otherwise.} \end{cases}$$

If  $s \leq j < 2s$ , then

$$b_{ij} = \begin{cases} w_{8(j+m)+2 \rightarrow 8(j+m)+3} \otimes w_{8j \rightarrow 8j+2}, & i = j + 4s; \\ -e_{8(j+m)+3} \otimes w_{8j \rightarrow 8j+3}, & i = j + 5s; \\ 0, & \text{otherwise.} \end{cases}$$

If  $2s \leq j < 3s$ , then

$$b_{ij} = \begin{cases} -w_{8(j+m) \rightarrow 8(j+m)+6} \otimes e_{8j}, & i = j; \\ e_{8(j+m)+6} \otimes w_{8j \rightarrow 8j+1}, & i = j + s; \\ w_{8(j+m)+5 \rightarrow 8(j+m)+6} \otimes w_{8j \rightarrow 8j+5}, & i = j + 8s; \\ 0, & \text{otherwise.} \end{cases}$$

If  $3s \leq j < 4s$ , then

$$b_{ij} = \begin{cases} -w_{8(j+m) \rightarrow 8(j+m)+5} \otimes e_{8j}, & i = j - s; \\ e_{8(j+m)+5} \otimes w_{8j \rightarrow 8j+5}, & i = j + 7s; \\ 0, & \text{otherwise.} \end{cases}$$

If  $4s \leq j < 5s$ , then

$$b_{ij} = \begin{cases} w_{8(j+m)+7 \rightarrow 8(j+m+1)} \otimes w_{8j+1 \rightarrow 8(j+1)}, & i = (j+1)_s; \\ e_{8(j+m+1)} \otimes w_{8j+1 \rightarrow 8(j+1)}, & i = s + (j+1)_s; \\ -e_{8(j+m+1)} \otimes w_{8j+1 \rightarrow 8(j+1)}, & i = 2s + (j+1)_s; \\ 0, & \text{otherwise.} \end{cases}$$

If  $5s \leq j < 6s$ , then

$$b_{ij} = \begin{cases} -e_{8(j+m)+7} \otimes w_{8j+2 \rightarrow 8(j+1)}, & i = (j+1)_s; \\ 0, & \text{otherwise.} \end{cases}$$

If  $6s \leq j < 7s$ , then  $b_{ij} = 0$ .

If  $7s \leq j < 8s$ , then

$$b_{ij} = \begin{cases} -e_{8(j+m+1)} \otimes w_{8j+3 \rightarrow 8(j+1)}, & i = 2s + (j+1)_s; \\ 0, & \text{otherwise.} \end{cases}$$

If  $8s \leq j < 14s$ , then  $b_{ij} = 0$ .

If  $14s \leq j < 15s$ , then

$$b_{ij} = \begin{cases} w_{8(j+m+1) \rightarrow 8(j+m+1)+6} \otimes w_{8j+7 \rightarrow 8(j+1)}, & i = 2s + (j+1)_s; \\ -w_{8(j+m+1)+5 \rightarrow 8(j+m+1)+6} \otimes w_{8j+7 \rightarrow 8(j+1)+5}, & i = 10s + (j+1)_s; \\ 0, & \text{otherwise.} \end{cases}$$

If  $15s \leq j < 16s$ , then  $b_{ij} = 0$ .

If  $16s \leq j < 17s$ , then

$$b_{ij} = \begin{cases} -e_{8(j+m+1)+1} \otimes w_{8j+7 \rightarrow 8(j+1)+1}, & i = 4s + (j+1)_s; \\ 0, & \text{otherwise.} \end{cases}$$

If  $17s \leq j < 18s$ , then  $b_{ij} = 0$ .

(12) If  $r_0 = 11$ , then  $\Omega^{11}(Z_t^{(3)})$  is described with  $(18s \times 20s)$  matrix, whose entries  $b_{ij}$  have the following form:

If  $0 \leq j < s$ , then

$$b_{ij} = \begin{cases} -e_{8(j+m)+7} \otimes w_{8j \rightarrow 8j+1}, & i = j + 5s; \\ 0, & \text{otherwise.} \end{cases}$$

If  $s \leq j < 2s$ , then

$$b_{ij} = \begin{cases} e_{8(j+m+1)} \otimes w_{8j \rightarrow 8j+2}, & i = j + 5s; \\ 0, & \text{otherwise.} \end{cases}$$

If  $2s \leq j < 3s$ , then

$$b_{ij} = \begin{cases} -w_{8(j+m)+1 \rightarrow 8(j+m+1)} \otimes e_{8j}, & i = j + s; \\ w_{8(j+m)+7 \rightarrow 8(j+m+1)} \otimes w_{8j \rightarrow 8j+1}, & i = j + 3s; \\ e_{8(j+m+1)} \otimes w_{8j \rightarrow 8j+2}, & i = j + 4s; \\ w_{8(j+m)+7 \rightarrow 8(j+m+1)} \otimes w_{8j \rightarrow 8j+5}, & i = j + 8s; \\ e_{8(j+m+1)} \otimes w_{8j \rightarrow 8j+5}, & i = j + 9s; \\ 0, & \text{otherwise.} \end{cases}$$

If  $3s \leq j < 4s$ , then

$$b_{ij} = \begin{cases} -w_{8(j+m+1)+2 \rightarrow 8(j+m+1)+3} \otimes w_{8j+1 \rightarrow 8(j+1)}, & i = (j+1)_s; \\ w_{8(j+m+1)+1 \rightarrow 8(j+m+1)+3} \otimes w_{8j+1 \rightarrow 8(j+1)}, & i = 3s + (j+1)_s; \\ 0, & \text{otherwise.} \end{cases}$$

If  $4s \leq j < 5s$ , then

$$b_{ij} = \begin{cases} e_{8(j+m+1)+5} \otimes w_{8j+1 \rightarrow 8(j+1)}, & i = 4s + (j+1)_s; \\ 0, & \text{otherwise.} \end{cases}$$

If  $5s \leq j < 6s$ , then

$$b_{ij} = \begin{cases} w_{8(j+m+1)+2 \rightarrow 8(j+m+1)+4} \otimes w_{8j+2 \rightarrow 8(j+1)}, & i = (j+1)_s; \\ -e_{8(j+m+1)+4} \otimes w_{8j+2 \rightarrow 8(j+1)}, & i = 2s + (j+1)_s; \\ -w_{8(j+m+1)+1 \rightarrow 8(j+m+1)+4} \otimes w_{8j+2 \rightarrow 8(j+1)}, & i = 3s + (j+1)_s; \\ 0, & \text{otherwise.} \end{cases}$$

If  $6s \leq j < 7s$ , then

$$b_{ij} = \begin{cases} -e_{8(j+m+1)+6} \otimes w_{8j+2 \rightarrow 8(j+1)}, & i = s + (j+1)s; \\ 0, & \text{otherwise.} \end{cases}$$

If  $7s \leq j < 8s$ , then  $b_{ij} = 0$ .

If  $8s \leq j < 9s$ , then

$$b_{ij} = \begin{cases} e_{8(j+m+1)+1} \otimes w_{8j+3 \rightarrow 8(j+1)}, & i = 3s + (j+1)s; \\ 0, & \text{otherwise.} \end{cases}$$

If  $9s \leq j < 20s$ , then  $b_{ij} = 0$ .

(13) If  $r_0 = 12$ , then  $\Omega^{12}(Z_t^{(3)})$  is described with  $(19s \times 18s)$  matrix, whose entries  $b_{ij}$  have the following form:

If  $0 \leq j < s$ , then

$$b_{ij} = \begin{cases} -w_{8(j+m)+2 \rightarrow 8(j+m)+3} \otimes w_{8j \rightarrow 8j+1}, & i = j + 3s; \\ 0, & \text{otherwise.} \end{cases}$$

If  $s \leq j < 2s$ , then

$$b_{ij} = \begin{cases} -w_{8(j+m) \rightarrow 8(j+m)+6} \otimes e_{8j}, & i = j; \\ -w_{8(j+m)+5 \rightarrow 8(j+m)+6} \otimes w_{8j \rightarrow 8j+4}, & i = j + 7s; \\ e_{8(j+m)+6} \otimes w_{8j \rightarrow 8j+5}, & i = j + 10s; \\ 0, & \text{otherwise.} \end{cases}$$

If  $2s \leq j < 3s$ , then

$$b_{ij} = \begin{cases} w_{8(j+m)+3 \rightarrow 8(j+m)+4} \otimes w_{8j \rightarrow 8j+2}, & i = j + 2s; \\ -e_{8(j+m)+4} \otimes w_{8j \rightarrow 8j+3}, & i = j + 4s; \\ 0, & \text{otherwise.} \end{cases}$$

If  $3s \leq j < 4s$ , then

$$b_{ij} = \begin{cases} -w_{8(j+m-1)+7 \rightarrow 8(j+m)+1} \otimes e_{8j}, & i = j - 3s; \\ w_{8(j+m) \rightarrow 8(j+m)+1} \otimes e_{8j}, & i = j - 2s; \\ w_{8(j+m-1)+7 \rightarrow 8(j+m)+1} \otimes e_{8j}, & i = j - s; \\ e_{8(j+m)+1} \otimes w_{8j \rightarrow 8j+4}, & i = j + 6s; \\ -e_{8(j+m)+1} \otimes w_{8j \rightarrow 8j+6}, & i = j + 12s; \\ 0, & \text{otherwise.} \end{cases}$$

If  $4s \leq j < 5s$ , then

$$b_{ij} = \begin{cases} e_{8(j+m)+5} \otimes w_{8j \rightarrow 8j+2}, & i = j + s; \\ 0, & \text{otherwise.} \end{cases}$$

If  $5s \leq j < 6s$ , then

$$b_{ij} = \begin{cases} e_{8(j+m)+7} \otimes w_{8j+1 \rightarrow 8(j+1)}, & i = (j+1)s; \\ 0, & \text{otherwise.} \end{cases}$$

If  $6s \leq j < 7s$ , then

$$b_{ij} = \begin{cases} e_{8(j+m)+7} \otimes w_{8j+2 \rightarrow 8(j+1)}, & i = (j+1)_s; \\ -e_{8(j+m)+7} \otimes w_{8j+2 \rightarrow 8(j+1)}, & i = 2s + (j+1)_s; \\ 0, & \text{otherwise.} \end{cases}$$

If  $7s \leq j < 8s$ , then

$$b_{ij} = \begin{cases} w_{8(j+m)+7 \rightarrow 8(j+m+1)} \otimes w_{8j+2 \rightarrow 8(j+1)}, & i = (j+1)_s; \\ -e_{8(j+m+1)} \otimes w_{8j+2 \rightarrow 8(j+1)}, & i = s + (j+1)_s; \\ -w_{8(j+m)+7 \rightarrow 8(j+m+1)} \otimes w_{8j+2 \rightarrow 8(j+1)}, & i = 2s + (j+1)_s; \\ 0, & \text{otherwise.} \end{cases}$$

If  $8s \leq j < 14s$ , then  $b_{ij} = 0$ .

If  $14s \leq j < 15s$ , then

$$b_{ij} = \begin{cases} -e_{8(j+m+1)+2} \otimes w_{8j+7 \rightarrow 8(j+1)+1}, & i = 3s + (j+1)_s; \\ 0, & \text{otherwise.} \end{cases}$$

If  $15s \leq j < 18s$ , then  $b_{ij} = 0$ .

(14) If  $r_0 = 13$ , then  $\Omega^{13}(Z_t^{(3)})$  is described with  $(18s \times 19s)$  matrix, whose entries  $b_{ij}$  have the following form:

If  $0 \leq j < s$ , then

$$b_{ij} = \begin{cases} -w_{8(j+m)+2 \rightarrow 8(j+m)+7} \otimes e_{8j}, & i = j; \\ -w_{8(j+m)+5 \rightarrow 8(j+m)+7} \otimes e_{8j}, & i = j + 3s; \\ -e_{8(j+m)+7} \otimes w_{8j \rightarrow 8j+5}, & i = j + 9s; \\ 0, & \text{otherwise.} \end{cases}$$

If  $s \leq j < 2s$ , then

$$b_{ij} = \begin{cases} -e_{8(j+m+1)} \otimes w_{8j \rightarrow 8j+1}, & i = j + 3s; \\ w_{8(j+m)+7 \rightarrow 8(j+m+1)} \otimes w_{8j \rightarrow 8j+2}, & i = j + 4s; \\ 0, & \text{otherwise.} \end{cases}$$

If  $2s \leq j < 3s$ , then

$$b_{ij} = \begin{cases} e_{8(j+m)+7} \otimes w_{8j \rightarrow 8j+2}, & i = j + 3s; \\ 0, & \text{otherwise.} \end{cases}$$

If  $3s \leq j < 4s$ , then

$$b_{ij} = \begin{cases} -w_{8(j+m+1)+3 \rightarrow 8(j+m+1)+4} \otimes w_{8j+1 \rightarrow 8(j+1)}, & i = s + (j+1)_s; \\ 0, & \text{otherwise.} \end{cases}$$

If  $4s \leq j < 5s$ , then

$$b_{ij} = \begin{cases} e_{8(j+m+1)+6} \otimes w_{8j+1 \rightarrow 8(j+1)}, & i = 2s + (j+1)_s; \\ 0, & \text{otherwise.} \end{cases}$$



If  $5s \leq j < 6s$ , then

$$b_{ij} = \begin{cases} -e_{8(j+m+1)+5} \otimes w_{8j+2 \rightarrow 8(j+1)}, & i = 3s + (j+1)_s; \\ 0, & \text{otherwise.} \end{cases}$$

If  $6s \leq j < 7s$ , then  $b_{ij} = 0$ .

If  $7s \leq j < 8s$ , then

$$b_{ij} = \begin{cases} e_{8(j+m+1)+2} \otimes w_{8j+3 \rightarrow 8(j+1)}, & i = (j+1)_s; \\ 0, & \text{otherwise.} \end{cases}$$

If  $8s \leq j < 9s$ , then

$$b_{ij} = \begin{cases} w_{8(j+m+1)+5 \rightarrow 8(j+m+1)+6} \otimes w_{8j+3 \rightarrow 8(j+1)}, & i = 3s + (j+1)_s; \\ 0, & \text{otherwise.} \end{cases}$$

If  $9s \leq j < 19s$ , then  $b_{ij} = 0$ .

(15) If  $r_0 = 14$ , then  $\Omega^{14}(Z_t^{(3)})$  is described with  $(20s \times 18s)$  matrix, whose entries  $b_{ij}$  have the following form:

If  $0 \leq j < s$ , then

$$b_{ij} = \begin{cases} w_{8(j+m-1)+7 \rightarrow 8(j+m)+2} \otimes e_{8j}, & i = j; \\ w_{8(j+m) \rightarrow 8(j+m)+2} \otimes e_{8j}, & i = j + s; \\ w_{8(j+m)+1 \rightarrow 8(j+m)+2} \otimes w_{8j \rightarrow 8j+3}, & i = j + 8s; \\ e_{8(j+m)+2} \otimes w_{8j \rightarrow 8j+4}, & i = j + 9s; \\ -e_{8(j+m)+2} \otimes w_{8j \rightarrow 8j+6}, & i = j + 14s; \\ 0, & \text{otherwise.} \end{cases}$$

If  $s \leq j < 2s$ , then

$$b_{ij} = \begin{cases} w_{8(j+m)+3 \rightarrow 8(j+m)+4} \otimes w_{8j \rightarrow 8j+5}, & i = j + 11s; \\ 0, & \text{otherwise.} \end{cases}$$

If  $2s \leq j < 3s$ , then

$$b_{ij} = \begin{cases} e_{8(j+m)+6} \otimes w_{8j \rightarrow 8j+2}, & i = j + 4s; \\ 0, & \text{otherwise.} \end{cases}$$

If  $3s \leq j < 4s$ , then

$$b_{ij} = \begin{cases} -e_{8(j+m)+5} \otimes w_{8j \rightarrow 8j+1}, & i = j + s; \\ 0, & \text{otherwise.} \end{cases}$$

If  $4s \leq j < 5s$ , then

$$b_{ij} = \begin{cases} e_{8(j+m)+7} \otimes w_{8j+1 \rightarrow 8(j+1)}, & i = (j+1)_s; \\ 0, & \text{otherwise.} \end{cases}$$

If  $5s \leq j < 6s$ , then

$$b_{ij} = \begin{cases} w_{8(j+m)+7 \rightarrow 8(j+m+1)} \otimes w_{8j+1 \rightarrow 8(j+1)}, & i = (j+1)_s; \\ e_{8(j+m+1)} \otimes w_{8j+1 \rightarrow 8(j+1)}, & i = s + (j+1)_s; \\ 0, & \text{otherwise.} \end{cases}$$

If  $6s \leq j < 7s$ , then

$$b_{ij} = \begin{cases} w_{8(j+m)+7 \rightarrow 8(j+m+1)} \otimes w_{8j+2 \rightarrow 8(j+1)}, & i = (j+1)_s; \\ e_{8(j+m+1)} \otimes w_{8j+2 \rightarrow 8(j+1)}, & i = s + (j+1)_s; \\ -e_{8(j+m+1)} \otimes w_{8j+2 \rightarrow 8(j+1)}, & i = 2s + (j+1)_s; \\ 0, & \text{otherwise.} \end{cases}$$

If  $7s \leq j < 13s$ , then  $b_{ij} = 0$ .

If  $13s \leq j < 14s$ , then

$$b_{ij} = \begin{cases} -e_{8(j+m+1)+3} \otimes w_{8j+7 \rightarrow 8(j+1)+1}, & i = 3s + (j+1)_s; \\ 0, & \text{otherwise.} \end{cases}$$

If  $14s \leq j < 18s$ , then  $b_{ij} = 0$ .

(16) If  $r_0 = 15$ , then  $\Omega^{15}(Z_t^{(3)})$  is described with  $(18s \times 19s)$  matrix, whose entries  $b_{ij}$  have the following form:

If  $0 \leq j < s$ , then

$$b_{ij} = \begin{cases} w_{8(j+m)+3 \rightarrow 8(j+m)+7} \otimes e_{8j}, & i = j; \\ e_{8(j+m)+7} \otimes w_{8j \rightarrow 8j+1}, & i = j + 5s; \\ 0, & \text{otherwise.} \end{cases}$$

If  $s \leq j < 2s$ , then

$$b_{ij} = \begin{cases} -e_{8(j+m+1)} \otimes w_{8j \rightarrow 8j+5}, & i = j + 10s; \\ 0, & \text{otherwise.} \end{cases}$$

If  $2s \leq j < 3s$ , then

$$b_{ij} = \begin{cases} e_{8(j+m+1)} \otimes w_{8j \rightarrow 8j+2}, & i = j + 5s; \\ 0, & \text{otherwise.} \end{cases}$$

If  $3s \leq j < 4s$ , then

$$b_{ij} = \begin{cases} e_{8(j+m+1)+5} \otimes w_{8j+1 \rightarrow 8(j+1)}, & i = 4s + (j+1)_s; \\ 0, & \text{otherwise.} \end{cases}$$

If  $4s \leq j < 6s$ , then

$$b_{ij} = \begin{cases} -w_{8(j+m+1)+1 \rightarrow 8(j+m+1)+j_2-3} \otimes w_{8j+j_2-3 \rightarrow 8(j+1)}, & i = 3s + (j+1)_s; \\ 0, & \text{otherwise.} \end{cases}$$

If  $6s \leq j < 7s$ , then

$$b_{ij} = \begin{cases} -e_{8(j+m+1)+6} \otimes w_{8j+2 \rightarrow 8(j+1)}, & i = s + (j+1)_s; \\ -w_{8(j+m+1)+5 \rightarrow 8(j+m+1)+6} \otimes w_{8j+2 \rightarrow 8(j+1)}, & i = 4s + (j+1)_s; \\ 0, & \text{otherwise.} \end{cases}$$

If  $7s \leq j < 8s$ , then

$$b_{ij} = \begin{cases} e_{8(j+m+1)+3} \otimes w_{8j+3 \rightarrow 8(j+1)}, & i = (j+1)_s; \\ 0, & \text{otherwise.} \end{cases}$$

If  $8s \leq j < 14s$ , then  $b_{ij} = 0$ .

If  $14s \leq j < 15s$ , then

$$b_{ij} = \begin{cases} w_{8(j+m+1)+3 \rightarrow 8(j+m+1)+4} \otimes w_{8j+6 \rightarrow 8(j+1)}, & i = (j+1)_s; \\ 0, & \text{otherwise.} \end{cases}$$

If  $15s \leq j < 16s$ , then  $b_{ij} = 0$ .

If  $16s \leq j < 18s$ , then

$$b_{ij} = \begin{cases} (-1)^{j_2+1} w_{8(j+m+1)+3 \rightarrow 8(j+m+1)+j_2-9} \otimes w_{8j+7 \rightarrow 8(j+1)}, & i = (j+1)_s; \\ 0, & \text{otherwise.} \end{cases}$$

If  $18s \leq j < 19s$ , then  $b_{ij} = 0$ .

(17) If  $r_0 = 16$ , then  $\Omega^{16}(Z_t^{(3)})$  is described with  $(19s \times 16s)$  matrix, whose entries  $b_{ij}$  have the following form:

If  $0 \leq j < s$ , then

$$b_{ij} = \begin{cases} w_{8(j+m) \rightarrow 8(j+m)+3} \otimes e_{8j}, & i = j + s; \\ w_{8(j+m-1)+7 \rightarrow 8(j+m)+3} \otimes e_{8j}, & i = j + 2s; \\ -w_{8(j+m)+1 \rightarrow 8(j+m)+3} \otimes w_{8j \rightarrow 8j+2}, & i = j + 6s; \\ -w_{8(j+m)+2 \rightarrow 8(j+m)+3} \otimes w_{8j \rightarrow 8j+3}, & i = j + 7s; \\ e_{8(j+m)+3} \otimes w_{8j \rightarrow 8j+4}, & i = j + 9s; \\ -e_{8(j+m)+3} \otimes w_{8j \rightarrow 8j+6}, & i = j + 13s; \\ 0, & \text{otherwise.} \end{cases}$$

If  $s \leq j < 2s$ , then

$$b_{ij} = \begin{cases} e_{8(j+m)+6} \otimes w_{8j \rightarrow 8j+1}, & i = j + 3s; \\ 0, & \text{otherwise.} \end{cases}$$

If  $2s \leq j < 3s$ , then

$$b_{ij} = \begin{cases} -e_{8(j+m)+1} \otimes w_{8j \rightarrow 8j+2}, & i = j + 4s; \\ 0, & \text{otherwise.} \end{cases}$$

If  $3s \leq j < 4s$ , then

$$b_{ij} = \begin{cases} -e_{8(j+m)+5} \otimes w_{8j \rightarrow 8j+5}, & i = j + 9s; \\ 0, & \text{otherwise.} \end{cases}$$

If  $4s \leq j < 5s$ , then

$$b_{ij} = \begin{cases} e_{8(j+m+1)} \otimes w_{8j+1 \rightarrow 8(j+1)}, & i = s + (j+1)_s; \\ w_{8(j+m)+7 \rightarrow 8(j+m+1)} \otimes w_{8j+1 \rightarrow 8(j+1)}, & i = 2s + (j+1)_s; \\ 0, & \text{otherwise.} \end{cases}$$

If  $5s \leq j < 6s$ , then

$$b_{ij} = \begin{cases} e_{8(j+m)+7} \otimes w_{8j+2 \rightarrow 8(j+1)}, & i = (j+1)_s; \\ 0, & \text{otherwise.} \end{cases}$$

If  $6s \leq j < 13s$ , then  $b_{ij} = 0$ .

If  $13s \leq j < 14s$ , then

$$b_{ij} = \begin{cases} -e_{8(j+m+1)+4} \otimes w_{8j+7 \rightarrow 8(j+1)+1}, & i = 3s + (j+1)_s; \\ 0, & \text{otherwise.} \end{cases}$$

If  $14s \leq j < 16s$ , then  $b_{ij} = 0$ .

(18) If  $r_0 = 17$ , then  $\Omega^{17}(Z_t^{(3)})$  is described with  $(18s \times 16s)$  matrix, whose entries  $b_{ij}$  have the following form:

If  $0 \leq j < s$ , then

$$b_{ij} = \begin{cases} w_{8(j+m)+2 \rightarrow 8(j+m)+7} \otimes e_{8j}, & i = j; \\ -w_{8(j+m)+4 \rightarrow 8(j+m)+7} \otimes e_{8j}, & i = j + s; \\ -e_{8(j+m)+7} \otimes w_{8j \rightarrow 8j+1}, & i = j + 4s; \\ -e_{8(j+m)+7} \otimes w_{8j \rightarrow 8j+5}, & i = j + 10s; \\ 0, & \text{otherwise.} \end{cases}$$

If  $s \leq j < 2s$ , then

$$b_{ij} = \begin{cases} -w_{8(j+m)+2 \rightarrow 8(j+m+1)} \otimes e_{8j}, & i = j - s; \\ w_{8(j+m)+4 \rightarrow 8(j+m+1)} \otimes e_{8j}, & i = j; \\ w_{8(j+m)+7 \rightarrow 8(j+m+1)} \otimes w_{8j \rightarrow 8j+1}, & i = j + 3s; \\ e_{8(j+m+1)} \otimes w_{8j \rightarrow 8j+1}, & i = j + 4s; \\ w_{8(j+m)+7 \rightarrow 8(j+m+1)} \otimes w_{8j \rightarrow 8j+5}, & i = j + 9s; \\ 0, & \text{otherwise.} \end{cases}$$

If  $2s \leq j < 3s$ , then

$$b_{ij} = \begin{cases} -e_{8(j+m+1)+2} \otimes w_{8j+1 \rightarrow 8(j+1)}, & i = (j+1)_s; \\ 0, & \text{otherwise.} \end{cases}$$

If  $3s \leq j < 4s$ , then

$$b_{ij} = \begin{cases} -e_{8(j+m+1)+6} \otimes w_{8j+1 \rightarrow 8(j+1)}, & i = 2s + (j+1)_s; \\ -w_{8(j+m+1)+5 \rightarrow 8(j+m+1)+6} \otimes w_{8j+1 \rightarrow 8(j+1)}, & i = 3s + (j+1)_s; \\ 0, & \text{otherwise.} \end{cases}$$

If  $4s \leq j < 5s$ , then

$$b_{ij} = \begin{cases} w_{8(j+m+1)+2 \rightarrow 8(j+m+1)+3} \otimes w_{8j+2 \rightarrow 8(j+1)}, & i = (j+1)_s; \\ 0, & \text{otherwise.} \end{cases}$$

If  $5s \leq j < 6s$ , then

$$b_{ij} = \begin{cases} -w_{8(j+m+1)+2 \rightarrow 8(j+m+1)+4} \otimes w_{8j+3 \rightarrow 8(j+1)}, & i = (j+1)_s; \\ e_{8(j+m+1)+4} \otimes w_{8j+3 \rightarrow 8(j+1)}, & i = s + (j+1)_s; \\ 0, & \text{otherwise.} \end{cases}$$

If  $6s \leq j < 13s$ , then  $b_{ij} = 0$ .

If  $13s \leq j < 15s$ , then

$$b_{ij} = \begin{cases} w_{8(j+m+1)+7 \rightarrow 8(j+m+1)+j_2-6} \otimes w_{8j+7 \rightarrow 8(j+1)+1}, & i = 4s + (j+1)_s; \\ 0, & \text{otherwise.} \end{cases}$$

If  $15s \leq j < 16s$ , then  $b_{ij} = 0$ .

(19) If  $r_0 = 18$ , then  $\Omega^{18}(Z_t^{(3)})$  is described with  $(19s \times 14s)$  matrix, whose entries  $b_{ij}$  have the following form:

If  $0 \leq j < s$ , then

$$b_{ij} = \begin{cases} -w_{8(j+m)+1 \rightarrow 8(j+m)+2} \otimes w_{8j \rightarrow 8j+1}, & i = j + 4s; \\ -e_{8(j+m)+2} \otimes w_{8j \rightarrow 8j+2}, & i = j + 5s; \\ 0, & \text{otherwise.} \end{cases}$$

If  $s \leq j < 2s$ , then

$$b_{ij} = \begin{cases} -w_{8(j+m-1)+7 \rightarrow 8(j+m)+4} \otimes e_{8j}, & i = j - s; \\ w_{8(j+m)+1 \rightarrow 8(j+m)+4} \otimes w_{8j \rightarrow 8j+1}, & i = j + 3s; \\ w_{8(j+m)+2 \rightarrow 8(j+m)+4} \otimes w_{8j \rightarrow 8j+2}, & i = j + 4s; \\ -w_{8(j+m)+3 \rightarrow 8(j+m)+4} \otimes w_{8j \rightarrow 8j+3}, & i = j + 6s; \\ e_{8(j+m)+4} \otimes w_{8j \rightarrow 8j+4}, & i = j + 7s; \\ -e_{8(j+m)+4} \otimes w_{8j \rightarrow 8j+6}, & i = j + 13s; \\ 0, & \text{otherwise.} \end{cases}$$

If  $2s \leq j < 3s$ , then

$$b_{ij} = \begin{cases} -w_{8(j+m)+5 \rightarrow 8(j+m)+6} \otimes w_{8j \rightarrow 8j+1}, & i = j + s; \\ -e_{8(j+m)+6} \otimes w_{8j \rightarrow 8j+5}, & i = j + 9s; \\ 0, & \text{otherwise.} \end{cases}$$

If  $3s \leq j < 5s$ , then

$$b_{ij} = \begin{cases} (-1)^{j_2} e_{8(j+m)+j_2+4} \otimes w_{8j+j_2-2 \rightarrow 8(j+1)}, & i = (j_2 - 3)s + (j+1)_s; \\ 0, & \text{otherwise.} \end{cases}$$

If  $5s \leq j < 11s$ , then  $b_{ij} = 0$ .

If  $11s \leq j < 12s$ , then

$$b_{ij} = \begin{cases} -e_{8(j+m+1)+6} \otimes w_{8j+7 \rightarrow 8(j+1)+5}, & i = 11s + (j+1)_s; \\ 0, & \text{otherwise.} \end{cases}$$

If  $12s \leq j < 13s$ , then  $b_{ij} = 0$ .

If  $13s \leq j < 14s$ , then

$$b_{ij} = \begin{cases} e_{8(j+m+1)+5} \otimes w_{8j+7 \rightarrow 8(j+1)+1}, & i = 3s + (j+1)_s; \\ 0, & \text{otherwise.} \end{cases}$$

(20) If  $r_0 = 19$ , then  $\Omega^{19}(Z_t^{(3)})$  is described with  $(16s \times 13s)$  matrix, whose entries  $b_{ij}$  have the following form:

If  $0 \leq j < s$ , then

$$b_{ij} = \begin{cases} w_{8(j+m)+6 \rightarrow 8(j+m+1)} \otimes e_{8j}, & i = j + s; \\ w_{8(j+m)+1 \rightarrow 8(j+m+1)} \otimes e_{8j}, & i = j + 2s; \\ -e_{8(j+m+1)} \otimes w_{8j \rightarrow 8j+1}, & i = j + 4s; \\ -w_{8(j+m)+7 \rightarrow 8(j+m+1)} \otimes w_{8j \rightarrow 8j+2}, & i = j + 5s; \\ -w_{8(j+m)+7 \rightarrow 8(j+m+1)} \otimes w_{8j \rightarrow 8j+4}, & i = j + 7s; \\ -e_{8(j+m+1)} \otimes w_{8j \rightarrow 8j+5}, & i = j + 9s; \\ -w_{8(j+m)+7 \rightarrow 8(j+m+1)} \otimes w_{8j \rightarrow 8j+6}, & i = j + 10s; \\ 0, & \text{otherwise.} \end{cases}$$

If  $s \leq j < 2s$ , then

$$b_{ij} = \begin{cases} -w_{8(j+m)+6 \rightarrow 8(j+m)+7} \otimes e_{8j}, & i = j; \\ -w_{8(j+m)+1 \rightarrow 8(j+m)+7} \otimes e_{8j}, & i = j + s; \\ e_{8(j+m)+7} \otimes w_{8j \rightarrow 8j+2}, & i = j + 4s; \\ e_{8(j+m)+7} \otimes w_{8j \rightarrow 8j+4}, & i = j + 6s; \\ e_{8(j+m)+7} \otimes w_{8j \rightarrow 8j+6}, & i = j + 9s; \\ 0, & \text{otherwise.} \end{cases}$$

If  $2s \leq j < 4s$ , then

$$b_{ij} = \begin{cases} (-1)^{j_2+1} w_{8(j+m+1)+3 \rightarrow 8(j+m+1)+j_2+1} \otimes w_{8j+j_2-1 \rightarrow 8(j+1)}, & i = (j+1)_s; \\ 0, & \text{otherwise.} \end{cases}$$

If  $4s \leq j < 5s$ , then

$$b_{ij} = \begin{cases} e_{8(j+m+1)+5} \otimes w_{8j+2 \rightarrow 8(j+1)}, & i = 3s + (j+1)_s; \\ 0, & \text{otherwise.} \end{cases}$$

If  $5s \leq j < 12s$ , then  $b_{ij} = 0$ .

If  $12s \leq j < 13s$ , then

$$b_{ij} = \begin{cases} e_{8(j+m+2)} \otimes w_{8j+7 \rightarrow 8(j+1)+1}, & i = 4s + (j+1)_s; \\ 0, & \text{otherwise.} \end{cases}$$

(21) If  $r_0 = 20$ , then  $\Omega^{20}(Z_t^{(3)})$  is described with  $(16s \times 11s)$  matrix, whose entries  $b_{ij}$  have the following form:

If  $0 \leq j < s$ , then

$$b_{ij} = \begin{cases} w_{8(j+m)+2 \rightarrow 8(j+m)+3} \otimes w_{8j \rightarrow 8j+1}, & i = j + 2s; \\ -e_{8(j+m)+3} \otimes w_{8j \rightarrow 8j+2}, & i = j + 4s; \\ w_{8(j+m)+1 \rightarrow 8(j+m)+3} \otimes w_{8j \rightarrow 8j+5}, & i = j + 10s; \\ 0, & \text{otherwise.} \end{cases}$$

If  $s \leq j < 2s$ , then

$$b_{ij} = \begin{cases} -w_{8(j+m-1)+7 \rightarrow 8(j+m)+5} \otimes e_{8j}, & i = j - s; \\ w_{8(j+m) \rightarrow 8(j+m)+5} \otimes e_{8j}, & i = j; \\ e_{8(j+m)+5} \otimes w_{8j \rightarrow 8j+3}, & i = j + 5s; \\ e_{8(j+m)+5} \otimes w_{8j \rightarrow 8j+6}, & i = j + 11s; \\ 0, & \text{otherwise.} \end{cases}$$

If  $2s \leq j < 3s$ , then

$$b_{ij} = \begin{cases} w_{8(j+m)+7 \rightarrow 8(j+m+1)} \otimes w_{8j+1 \rightarrow 8(j+1)}, & i = (j + 1)_s; \\ -e_{8(j+m+1)} \otimes w_{8j+1 \rightarrow 8(j+1)}, & i = s + (j + 1)_s; \\ 0, & \text{otherwise.} \end{cases}$$

If  $3s \leq j < 4s$ , then

$$b_{ij} = \begin{cases} e_{8(j+m)+7} \otimes w_{8j+2 \rightarrow 8(j+1)}, & i = (j + 1)_s; \\ 0, & \text{otherwise.} \end{cases}$$

If  $4s \leq j < 8s$ , then  $b_{ij} = 0$ .

If  $8s \leq j < 10s$ , then

$$b_{ij} = \begin{cases} (-1)^{j_2} w_{8(j+m+1)+1 \rightarrow 8(j+m+1)+2(j_2-7)} \otimes w_{8j+7 \rightarrow 8(j+1)+5}, & i = 10s + (j + 1)_s; \\ 0, & \text{otherwise.} \end{cases}$$

If  $10s \leq j < 11s$ , then

$$b_{ij} = \begin{cases} -e_{8(j+m+1)+6} \otimes w_{8j+7 \rightarrow 8(j+1)+1}, & i = 3s + (j + 1)_s; \\ 0, & \text{otherwise.} \end{cases}$$

(22) If  $r_0 = 21$ , then  $\Omega^{21}(Z_t^{(3)})$  is described with  $(14s \times 11s)$  matrix, whose entries  $b_{ij}$  have the following form:

If  $0 \leq j < s$ , then

$$b_{ij} = \begin{cases} -w_{8(j+m)+2 \rightarrow 8(j+m+1)} \otimes e_{8j}, & i = j; \\ -e_{8(j+m+1)} \otimes w_{8j \rightarrow 8j+2}, & i = j + 4s; \\ -w_{8(j+m)+7 \rightarrow 8(j+m+1)} \otimes w_{8j \rightarrow 8j+3}, & i = j + 5s; \\ -e_{8(j+m+1)} \otimes w_{8j \rightarrow 8j+4}, & i = j + 6s; \\ -e_{8(j+m+1)} \otimes w_{8j \rightarrow 8j+6}, & i = j + 9s; \\ 0, & \text{otherwise.} \end{cases}$$

If  $s \leq j < 2s$ , then

$$b_{ij} = \begin{cases} -e_{8(j+m+1)+4} \otimes w_{8j+1 \rightarrow 8(j+1)}, & i = s + (j+1)_s; \\ 0, & \text{otherwise.} \end{cases}$$

If  $2s \leq j < 3s$ , then  $b_{ij} = 0$ .

If  $3s \leq j < 4s$ , then

$$b_{ij} = \begin{cases} e_{8(j+m+1)+6} \otimes w_{8j+2 \rightarrow 8(j+1)}, & i = 2s + (j+1)_s; \\ 0, & \text{otherwise.} \end{cases}$$

If  $4s \leq j < 10s$ , then  $b_{ij} = 0$ .

If  $10s \leq j < 11s$ , then

$$b_{ij} = \begin{cases} e_{8(j+m+1)+7} \otimes w_{8j+7 \rightarrow 8(j+1)+1}, & i = 3s + (j+1)_s; \\ 0, & \text{otherwise.} \end{cases}$$

(23) If  $r_0 = 22$ , then  $\Omega^{22}(Z_t^{(3)})$  is described with  $(13s \times 10s)$  matrix, whose entries  $b_{ij}$  have the following form:

If  $0 \leq j < s$ , then

$$b_{ij} = \begin{cases} -w_{8(j+m) \rightarrow 8(j+m)+4} \otimes e_{8j}, & i = j; \\ w_{8(j+m-1)+7 \rightarrow 8(j+m)+4} \otimes e_{8j}, & i = j + s; \\ w_{8(j+m)+3 \rightarrow 8(j+m)+4} \otimes w_{8j \rightarrow 8j+1}, & i = j + 2s; \\ -e_{8(j+m)+4} \otimes w_{8j \rightarrow 8j+2}, & i = j + 3s; \\ -w_{8(j+m)+1 \rightarrow 8(j+m)+4} \otimes w_{8j \rightarrow 8j+4}, & i = j + 6s; \\ -w_{8(j+m)+2 \rightarrow 8(j+m)+4} \otimes w_{8j \rightarrow 8j+5}, & i = j + 7s; \\ 0, & \text{otherwise.} \end{cases}$$

If  $s \leq j < 2s$ , then

$$b_{ij} = \begin{cases} w_{8(j+m)+5 \rightarrow 8(j+m)+6} \otimes w_{8j \rightarrow 8j+2}, & i = j + 3s; \\ e_{8(j+m)+6} \otimes w_{8j \rightarrow 8j+3}, & i = j + 4s; \\ e_{8(j+m)+6} \otimes w_{8j \rightarrow 8j+6}, & i = j + 9s; \\ 0, & \text{otherwise.} \end{cases}$$

If  $2s \leq j < 3s$ , then

$$b_{ij} = \begin{cases} -e_{8(j+m)+7} \otimes w_{8j+1 \rightarrow 8(j+1)}, & i = s + (j+1)_s; \\ 0, & \text{otherwise.} \end{cases}$$

If  $3s \leq j < 5s$ , then

$$b_{ij} = \begin{cases} w_{8(j+m+1) \rightarrow 8(j+m+1)+j_2-3} \otimes w_{8j+j_2-1 \rightarrow 8(j+1)}, & i = (j+1)_s; \\ -w_{8(j+m)+7 \rightarrow 8(j+m+1)+j_2-3} \otimes w_{8j+j_2-1 \rightarrow 8(j+1)}, & i = s + (j+1)_s; \\ 0, & \text{otherwise.} \end{cases}$$



If  $5s \leq j < 6s$ , then

$$b_{ij} = \begin{cases} w_{8(j+m+1) \rightarrow 8(j+m+1)+2} \otimes w_{8j+4 \rightarrow 8(j+1)}, & i = (j+1)_s; \\ -w_{8(j+m)+7 \rightarrow 8(j+m+1)+2} \otimes w_{8j+4 \rightarrow 8(j+1)}, & i = s + (j+1)_s; \\ w_{8(j+m+1)+1 \rightarrow 8(j+m+1)+2} \otimes w_{8j+4 \rightarrow 8(j+1)+4}, & i = 6s + (j+1)_s; \\ 0, & \text{otherwise.} \end{cases}$$

If  $6s \leq j < 8s$ , then  $b_{ij} = 0$ .

If  $8s \leq j < 9s$ , then

$$b_{ij} = \begin{cases} -w_{8(j+m+1) \rightarrow 8(j+m+1)+3} \otimes w_{8j+7 \rightarrow 8(j+1)}, & i = (j+1)_s; \\ w_{8(j+m)+7 \rightarrow 8(j+m+1)+3} \otimes w_{8j+7 \rightarrow 8(j+1)}, & i = s + (j+1)_s; \\ -w_{8(j+m+1)+1 \rightarrow 8(j+m+1)+3} \otimes w_{8j+7 \rightarrow 8(j+1)+4}, & i = 6s + (j+1)_s; \\ -w_{8(j+m+1)+2 \rightarrow 8(j+m+1)+3} \otimes w_{8j+7 \rightarrow 8(j+1)+5}, & i = 7s + (j+1)_s; \\ 0, & \text{otherwise.} \end{cases}$$

If  $9s \leq j < 10s$ , then  $b_{ij} = 0$ .

(24) If  $r_0 = 23$ , then  $\Omega^{23}(Z_t^{(3)})$  is described with  $(11s \times 8s)$  matrix, whose entries  $b_{ij}$  have the following form:

If  $0 \leq j < s$ , then

$$b_{ij} = \begin{cases} -w_{8(j+m)+3 \rightarrow 8(j+m)+7} \otimes e_{8j}, & i = j; \\ -e_{8(j+m)+7} \otimes w_{8j \rightarrow 8j+2}, & i = j + 3s; \\ -e_{8(j+m)+7} \otimes w_{8j \rightarrow 8j+6}, & i = j + 7s; \\ 0, & \text{otherwise.} \end{cases}$$

If  $s \leq j < 2s$ , then

$$b_{ij} = \begin{cases} -w_{8(j+m+1)+5 \rightarrow 8(j+m+1)+6} \otimes w_{8j+1 \rightarrow 8(j+1)}, & i = s + (j+1)_s; \\ 0, & \text{otherwise.} \end{cases}$$

If  $2s \leq j < 7s$ , then  $b_{ij} = 0$ .

If  $7s \leq j < 8s$ , then

$$b_{ij} = \begin{cases} -e_{8(j+m+2)} \otimes w_{8j+7 \rightarrow 8(j+1)+1}, & i = 2s + (j+1)_s; \\ 0, & \text{otherwise.} \end{cases}$$

(25) If  $r_0 = 24$ , then  $\Omega^{24}(Z_t^{(3)})$  is described with  $(11s \times 9s)$  matrix, whose entries  $b_{ij}$  have the following form:

If  $0 \leq j < s$ , then

$$b_{ij} = \begin{cases} w_{8(j+m) \rightarrow 8(j+m)+7} \otimes e_{8j}, & i = j; \\ -w_{8(j+m)+5 \rightarrow 8(j+m)+7} \otimes w_{8j \rightarrow 8j+1}, & i = j + 2s; \\ (1 - 2f(j_1, 1))w_{8(j+m)+j_1 \rightarrow 8(j+m)+7} \otimes w_{8j \rightarrow 8j+2+j_1}, & i = j + (j_1 + 3)s, \ 1 \leq j_1 \leq 3; \\ 0, & \text{otherwise.} \end{cases}$$

If  $s \leq j < 3s$ , then

$$b_{ij} = \begin{cases} w_{8(j+m+1) \rightarrow 8(j+m+1)+j_2-1} \otimes w_{8j+j_2 \rightarrow 8(j+1)}, & i = (j+1)_s; \\ 0, & \text{otherwise.} \end{cases}$$

If  $3s \leq j < 4s$ , then

$$b_{ij} = \begin{cases} w_{8(j+m+1) \rightarrow 8(j+m+1)+2} \otimes w_{8j+3 \rightarrow 8(j+1)}, & i = (j+1)_s; \\ -w_{8(j+m+1)+1 \rightarrow 8(j+m+1)+2} \otimes w_{8j+3 \rightarrow 8(j+1)+3}, & i = 4s + (j+1)_s; \\ 0, & \text{otherwise.} \end{cases}$$

If  $4s \leq j < 5s$ , then

$$b_{ij} = \begin{cases} w_{8(j+m+1) \rightarrow 8(j+m+1)+3} \otimes w_{8j+4 \rightarrow 8(j+1)}, & i = (j+1)_s; \\ -w_{8(j+m+1)+1 \rightarrow 8(j+m+1)+3} \otimes w_{8j+4 \rightarrow 8(j+1)+3}, & i = 4s + (j+1)_s; \\ w_{8(j+m+1)+2 \rightarrow 8(j+m+1)+3} \otimes w_{8j+4 \rightarrow 8(j+1)+4}, & i = 5s + (j+1)_s; \\ 0, & \text{otherwise.} \end{cases}$$

If  $5s \leq j < 7s$ , then  $b_{ij} = 0$ .

If  $7s \leq j < 8s$ , then

$$b_{ij} = \begin{cases} -w_{8(j+m+1) \rightarrow 8(j+m+1)+4} \otimes w_{8j+7 \rightarrow 8(j+1)}, & i = (j+1)_s; \\ (-1 + 2f(j_1, 1))w_{8(j+m+1)+j_1 \rightarrow 8(j+m+1)+4} \otimes w_{8j+7 \rightarrow 8(j+1)+j_1+2}, & i = (j_1 + 3)s + (j+1)_s, \ 1 \leq j_1 \leq 3; \\ 0, & \text{otherwise.} \end{cases}$$

If  $8s \leq j < 9s$ , then

$$b_{ij} = \begin{cases} w_{8(j+m+1)+5 \rightarrow 8(j+m+1)+6} \otimes w_{8j+7 \rightarrow 8(j+1)+1}, & i = 2s + (j+1)_s; \\ 0, & \text{otherwise.} \end{cases}$$

(26) If  $r_0 = 25$ , then  $\Omega^{25}(Z_t^{(3)})$  is described with  $(10s \times 8s)$  matrix, whose entries  $b_{ij}$  have the following form:

If  $0 \leq j < s$ , then

$$b_{ij} = \begin{cases} -w_{8(j+m)+4 \rightarrow 8(j+m+1)} \otimes e_{8j}, & i = j; \\ -w_{8(j+m)+7 \rightarrow 8(j+m+1)} \otimes w_{8j \rightarrow 8j+1}, & i = j + 2s; \\ -e_{8(j+m+1)} \otimes w_{8j \rightarrow 8j+2}, & i = j + 3s; \\ -e_{8(j+m+1)} \otimes w_{8j \rightarrow 8j+6}, & i = j + 7s; \\ 0, & \text{otherwise.} \end{cases}$$

If  $s \leq j < 8s$ , then  $b_{ij} = 0$ .

(27) If  $r_0 = 26$ , then  $\Omega^{26}(Z_t^{(3)})$  is described with  $(8s \times 8s)$  matrix, whose entries  $b_{ij}$  have the following form:

If  $0 \leq j < s$ , then

$$b_{ij} = \begin{cases} (1 - 2f(j_1, 2))w_{8(j+m)+j_1 \rightarrow 8(j+m+1)} \otimes w_{8j \rightarrow 8j+j_1+1}, & i = j + (j_1 + 1)s, \ 1 \leq j_1 \leq 4; \\ 0, & \text{otherwise.} \end{cases}$$

If  $s \leq j < 2s$ , then

$$b_{ij} = \begin{cases} w_{8(j+m)+7 \rightarrow 8(j+m+1)+1} \otimes w_{8j+1 \rightarrow 8(j+1)}, & i = (j+1)_s; \\ 0, & \text{otherwise.} \end{cases}$$

If  $2s \leq j < 3s$ , then

$$b_{ij} = \begin{cases} w_{8(j+m)+7 \rightarrow 8(j+m+1)+2} \otimes w_{8j+2 \rightarrow 8(j+1)}, & i = (j+1)_s; \\ w_{8(j+m+1)+1 \rightarrow 8(j+m+1)+2} \otimes w_{8j+2 \rightarrow 8(j+1)+2}, & i = 2s + (j+1)_s; \\ 0, & \text{otherwise.} \end{cases}$$

If  $3s \leq j < 4s$ , then

$$b_{ij} = \begin{cases} w_{8(j+m)+7 \rightarrow 8(j+m+1)+3} \otimes w_{8j+3 \rightarrow 8(j+1)}, & i = (j+1)_s; \\ w_{8(j+m+1)+1 \rightarrow 8(j+m+1)+3} \otimes w_{8j+3 \rightarrow 8(j+1)+2}, & i = 2s + (j+1)_s; \\ -w_{8(j+m+1)+2 \rightarrow 8(j+m+1)+3} \otimes w_{8j+3 \rightarrow 8(j+1)+3}, & i = 3s + (j+1)_s; \\ 0, & \text{otherwise.} \end{cases}$$

If  $4s \leq j < 5s$ , then

$$b_{ij} = \begin{cases} w_{8(j+m)+7 \rightarrow 8(j+m+1)+4} \otimes w_{8j+4 \rightarrow 8(j+1)}, & i = (j+1)_s; \\ (-1)^{j_1+1} w_{8(j+m+1)+j_1 \rightarrow 8(j+m+1)+4} \otimes w_{8j+4 \rightarrow 8(j+1)+j_1+1}, & i = (j_1+1)s + (j+1)_s, \ 1 \leq j_1 \leq 3; \\ 0, & \text{otherwise.} \end{cases}$$

If  $5s \leq j < 6s$ , then  $b_{ij} = 0$ .

If  $6s \leq j < 7s$ , then

$$b_{ij} = \begin{cases} w_{8(j+m+1)+5 \rightarrow 8(j+m+1)+6} \otimes w_{8j+6 \rightarrow 8(j+1)+6}, & i = 6s + (j+1)_s; \\ 0, & \text{otherwise.} \end{cases}$$

If  $7s \leq j < 8s$ , then

$$b_{ij} = \begin{cases} w_{8(j+m)+7 \rightarrow 8(j+m+1)+7} \otimes w_{8j+7 \rightarrow 8(j+1)}, & i = (j+1)_s; \\ (1 - 2f(j_1, 2)) w_{8(j+m+1)+j_1 \rightarrow 8(j+m+1)+7} \otimes w_{8j+7 \rightarrow 8(j+1)+j_1+1}, & i = (j_1+1)s + (j+1)_s, \ 1 \leq j_1 \leq 4; \\ 0, & \text{otherwise.} \end{cases}$$

(28) If  $r_0 = 27$ , then  $\Omega^{27}(Z_t^{(3)})$  is described with  $(9s \times 9s)$  matrix, whose entries  $b_{ij}$  have the following form:

If  $0 \leq j < s$ , then

$$b_{ij} = \begin{cases} -w_{8(j+m+1) \rightarrow 8(j+m+1)+1} \otimes w_{8j \rightarrow 8j+1}, & i = j + s; \\ w_{8(j+m+1) \rightarrow 8(j+m+1)+1} \otimes w_{8j \rightarrow 8j+5}, & i = j + 5s; \\ 0, & \text{otherwise.} \end{cases}$$

If  $s \leq j < 7s$ , then  $b_{ij} = 0$ .

If  $7s \leq j < 8s$ , then

$$b_{ij} = \begin{cases} -e_{8(j+m+1)+7} \otimes w_{8j+6 \rightarrow 8(j+1)}, & i = (j+1)_s; \\ 0, & \text{otherwise.} \end{cases}$$

If  $8s \leq j < 9s$ , then  $b_{ij} = 0$ .

(29) If  $r_0 = 28$ , then  $\Omega^{28}(Z_t^{(3)})$  is described with  $(8s \times 8s)$  matrix, whose entries  $b_{ij}$  have the following form:

If  $0 \leq j < s$ , then

$$b_{ij} = \begin{cases} (1 - 2(f(j_1, 1) + f(j_1, 3) + f(j_1, 6)))w_{8(j+m)+j_1 \rightarrow 8(j+m)+7} \otimes w_{8j \rightarrow 8j+j_1}, \\ i = j + j_1s, \quad 1 \leq j_1 \leq 7; \\ 0, \quad \text{otherwise.} \end{cases}$$

If  $s \leq j < 2s$ , then

$$b_{ij} = \begin{cases} -w_{8(j+m+1)+1 \rightarrow 8(j+m+1)+2} \otimes w_{8j+1 \rightarrow 8(j+1)+1}, & i = s + (j+1)_s; \\ 0, & \text{otherwise.} \end{cases}$$

If  $2s \leq j < 3s$ , then

$$b_{ij} = \begin{cases} -w_{8(j+m+1)+1 \rightarrow 8(j+m+1)+3} \otimes w_{8j+2 \rightarrow 8(j+1)+1}, & i = s + (j+1)_s; \\ w_{8(j+m+1)+2 \rightarrow 8(j+m+1)+3} \otimes w_{8j+2 \rightarrow 8(j+1)+2}, & i = 2s + (j+1)_s; \\ 0, & \text{otherwise.} \end{cases}$$

If  $3s \leq j < 4s$ , then

$$b_{ij} = \begin{cases} (-1)^{j_1} w_{8(j+m+1)+j_1 \rightarrow 8(j+m+1)+4} \otimes w_{8j+3 \rightarrow 8(j+1)+j_1}, & i = j_1s + (j+1)_s, \quad 1 \leq j_1 \leq 3; \\ 0, & \text{otherwise.} \end{cases}$$

If  $4s \leq j < 5s$ , then  $b_{ij} = 0$ .

If  $5s \leq j < 6s$ , then

$$b_{ij} = \begin{cases} -w_{8(j+m+1) \rightarrow 8(j+m+1)+6} \otimes w_{8j+5 \rightarrow 8(j+1)}, & i = (j+1)_s; \\ -w_{8(j+m+1)+5 \rightarrow 8(j+m+1)+6} \otimes w_{8j+5 \rightarrow 8(j+1)+5}, & i = 5s + (j+1)_s; \\ 0, & \text{otherwise.} \end{cases}$$

If  $6s \leq j < 8s$ , then

$$b_{ij} = \begin{cases} -w_{8(j+m+1) \rightarrow 8(j+m+1)+1+7(j_2-6)} \otimes w_{8j+j_2 \rightarrow 8(j+1)}, & i = (j+1)_s; \\ 0, & \text{otherwise.} \end{cases}$$

(II) Represent an arbitrary  $t_0 \in \mathbb{N}$  in the form  $t_0 = 29\ell_0 + r_0$ , where  $0 \leq r_0 \leq 28$ . Then  $\Omega^{t_0}(Z_t^{(3)})$  is a  $\Omega^{r_0}(Z_t^{(3)})$ , whose left components twisted by  $\sigma^{\ell_0}$ .

**Proposition 4** (Translates for the case 4). (I) Let  $r_0 \in \mathbb{N}$ ,  $r_0 < 29$ .  $r_0$ -translates of the elements  $Z_t^{(4)}$  are described by the following way.

(1) If  $r_0 = 0$ , then  $\Omega^0(Z_t^{(4)})$  is described with  $(8s \times 11s)$  matrix with unique nonzero entry:

$$b_{j,(1)_s} = w_{8(j+m) \rightarrow 8(j+m)+7} \otimes e_{8j}.$$

(2) If  $r_0 = 1$ , then  $\Omega^1(Z_t^{(4)})$  is described with  $(9s \times 11s)$  matrix with the following nonzero entries:

$$\begin{aligned} b_{s+(j+1)_s, 4s} &= -w_{8(j+m+1)+5 \rightarrow 8(j+m+1)+7} \otimes w_{8j+2 \rightarrow 8(j+1)}; \\ b_{s+(j+1)_s, 6s} &= -w_{8(j+m+1)+5 \rightarrow 8(j+m+1)+7} \otimes w_{8j+4 \rightarrow 8(j+1)}; \\ b_{(j+1)_s, 7s} &= -w_{8(j+m+1)+1 \rightarrow 8(j+m+2)} \otimes w_{8j+5 \rightarrow 8(j+1)}. \end{aligned}$$

(3) If  $r_0 = 2$ , then  $\Omega^2(Z_t^{(4)})$  is described with  $(8s \times 13s)$  matrix with two nonzero entries:

$$b_{(j+1)_s, s} = -w_{8(j+m)+7 \rightarrow 8(j+m+1)} \otimes w_{8j \rightarrow 8(j+1)};$$

$$b_{(j+1)s,3s} = -w_{8(j+m)+7 \rightarrow 8(j+m+1)+5} \otimes w_{8j+2 \rightarrow 8(j+1)}.$$

(4) If  $r_0 = 3$ , then  $\Omega^3(Z_t^{(4)})$  is described with  $(10s \times 14s)$  matrix with the following nonzero entries:

$$\begin{aligned} b_{(j+1)s,0} &= -e_{8(j+m+1)+2} \otimes w_{8j \rightarrow 8(j+1)}; \\ b_{(j+1)s,s} &= -w_{8(j+m+1)+2 \rightarrow 8(j+m+1)+4} \otimes w_{8j \rightarrow 8(j+1)}; \\ b_{s+(j+1)s,2s} &= e_{8(j+m+1)+6} \otimes w_{8j \rightarrow 8(j+1)}; \\ b_{s+(j+1)s,4s} &= w_{8(j+m+1)+6 \rightarrow 8(j+m+1)+7} \otimes w_{8j+1 \rightarrow 8(j+1)}. \end{aligned}$$

(5) If  $r_0 = 4$ , then  $\Omega^4(Z_t^{(4)})$  is described with  $(11s \times 16s)$  matrix with the following nonzero entries:

$$\begin{aligned} b_{(j+1)s,0} &= -e_{8(j+m)+7} \otimes w_{8j \rightarrow 8(j+1)}; \\ b_{(j+1)s,s} &= -e_{8(j+m)+7} \otimes w_{8j \rightarrow 8(j+1)}; \\ b_{s+(j+1)s,2s} &= e_{8(j+m+1)} \otimes w_{8j \rightarrow 8(j+1)}; \\ b_{(j+1)s,3s} &= w_{8(j+m)+7 \rightarrow 8(j+m+1)+5} \otimes w_{8j+1 \rightarrow 8(j+1)}. \end{aligned}$$

(6) If  $r_0 = 5$ , then  $\Omega^5(Z_t^{(4)})$  is described with  $(11s \times 16s)$  matrix with the following nonzero entries:

$$\begin{aligned} b_{(j+1)s,0} &= e_{8(j+m+1)+5} \otimes w_{8j \rightarrow 8(j+1)}; \\ b_{s+(j+1)s,s} &= -e_{8(j+m+1)+3} \otimes w_{8j \rightarrow 8(j+1)}; \\ b_{2s+(j+1)s,3s} &= -e_{8(j+m+1)+1} \otimes w_{8j \rightarrow 8(j+1)}. \end{aligned}$$

(7) If  $r_0 = 6$ , then  $\Omega^6(Z_t^{(4)})$  is described with  $(13s \times 19s)$  matrix with two nonzero entries:

$$\begin{aligned} b_{(j+1)s,0} &= e_{8(j+m)+7} \otimes w_{8j \rightarrow 8(j+1)}; \\ b_{s+(j+1)s,s} &= -e_{8(j+m+1)} \otimes w_{8j \rightarrow 8(j+1)}. \end{aligned}$$

(8) If  $r_0 = 7$ , then  $\Omega^7(Z_t^{(4)})$  is described with  $(14s \times 18s)$  matrix with the following nonzero entries:

$$\begin{aligned} b_{(j+1)s,0} &= -e_{8(j+m+1)+2} \otimes w_{8j \rightarrow 8(j+1)}; \\ b_{2s+(j+1)s,s} &= e_{8(j+m+1)+6} \otimes w_{8j \rightarrow 8(j+1)}; \\ b_{s+(j+1)s,2s} &= -e_{8(j+m+1)+4} \otimes w_{8j \rightarrow 8(j+1)}; \\ b_{3s+(j+1)s,4s} &= -e_{8(j+m+1)+5} \otimes w_{8j \rightarrow 8(j+1)}. \end{aligned}$$

(9) If  $r_0 = 8$ , then  $\Omega^8(Z_t^{(4)})$  is described with  $(16s \times 19s)$  matrix with the following nonzero entries:

$$\begin{aligned} b_{(j+1)s,0} &= -e_{8(j+m)+7} \otimes w_{8j \rightarrow 8(j+1)}; \\ b_{(j+1)s,s} &= w_{8(j+m)+7 \rightarrow 8(j+m+1)} \otimes w_{8j \rightarrow 8(j+1)}; \\ b_{s+(j+1)s,s} &= -w_{8(j+m)+7 \rightarrow 8(j+m+1)} \otimes w_{8j \rightarrow 8(j+1)}; \\ b_{2s+(j+1)s,s} &= e_{8(j+m+1)} \otimes w_{8j \rightarrow 8(j+1)}; \\ b_{s+(j+1)s,2s} &= -e_{8(j+m)+7} \otimes w_{8j \rightarrow 8(j+1)}. \end{aligned}$$

(10) If  $r_0 = 9$ , then  $\Omega^9(Z_t^{(4)})$  is described with  $(16s \times 18s)$  matrix with the following nonzero entries:

$$\begin{aligned} b_{3s+(j+1)s,0} &= -w_{8(j+m+1)+1 \rightarrow 8(j+m+1)+2} \otimes w_{8j \rightarrow 8(j+1)}; \\ b_{s+(j+1)s,s} &= -e_{8(j+m+1)+3} \otimes w_{8j \rightarrow 8(j+1)}; \\ b_{2s+(j+1)s,2s} &= -e_{8(j+m+1)+6} \otimes w_{8j \rightarrow 8(j+1)}; \\ b_{(j+1)s,3s} &= e_{8(j+m+1)+5} \otimes w_{8j \rightarrow 8(j+1)}. \end{aligned}$$

(11) If  $r_0 = 10$ , then  $\Omega^{10}(Z_t^{(4)})$  is described with  $(19s \times 20s)$  matrix with the following nonzero entries:

$$\begin{aligned} b_{(j+1)s,0} &= e_{8(j+m)+7} \otimes w_{8j \rightarrow 8(j+1)}; \\ b_{s+(j+1)s,s} &= -e_{8(j+m+1)} \otimes w_{8j \rightarrow 8(j+1)}; \\ b_{2s+(j+1)s,2s} &= -e_{8(j+m+1)} \otimes w_{8j \rightarrow 8(j+1)}. \end{aligned}$$

(12) If  $r_0 = 11$ , then  $\Omega^{11}(Z_t^{(4)})$  is described with  $(18s \times 18s)$  matrix with the following nonzero entries:

$$\begin{aligned} b_{(j+1)s,0} &= w_{8(j+m+1)+2 \rightarrow 8(j+m+1)+3} \otimes w_{8j \rightarrow 8(j+1)}; \\ b_{s+(j+1)s,s} &= e_{8(j+m+1)+6} \otimes w_{8j \rightarrow 8(j+1)}; \\ b_{2s+(j+1)s,2s} &= -e_{8(j+m+1)+4} \otimes w_{8j \rightarrow 8(j+1)}; \\ b_{3s+(j+1)s,3s} &= e_{8(j+m+1)+1} \otimes w_{8j \rightarrow 8(j+1)}; \\ b_{4s+(j+1)s,4s} &= -e_{8(j+m+1)+5} \otimes w_{8j \rightarrow 8(j+1)}. \end{aligned}$$

(13) If  $r_0 = 12$ , then  $\Omega^{12}(Z_t^{(4)})$  is described with  $(19s \times 19s)$  matrix with the following nonzero entries:

$$\begin{aligned} b_{(j+1)s,0} &= -e_{8(j+m)+7} \otimes w_{8j \rightarrow 8(j+1)}; \\ b_{s+(j+1)s,s} &= e_{8(j+m+1)} \otimes w_{8j \rightarrow 8(j+1)}; \\ b_{2s+(j+1)s,2s} &= -e_{8(j+m)+7} \otimes w_{8j \rightarrow 8(j+1)}. \end{aligned}$$

(14) If  $r_0 = 13$ , then  $\Omega^{13}(Z_t^{(4)})$  is described with  $(18s \times 18s)$  matrix with the following nonzero entries:

$$\begin{aligned} b_{(j+1)s,0} &= e_{8(j+m+1)+2} \otimes w_{8j \rightarrow 8(j+1)}; \\ b_{s+(j+1)s,s} &= w_{8(j+m+1)+3 \rightarrow 8(j+m+1)+4} \otimes w_{8j \rightarrow 8(j+1)}; \\ b_{2s+(j+1)s,2s} &= -e_{8(j+m+1)+6} \otimes w_{8j \rightarrow 8(j+1)}; \\ b_{3s+(j+1)s,3s} &= e_{8(j+m+1)+5} \otimes w_{8j \rightarrow 8(j+1)}. \end{aligned}$$

(15) If  $r_0 = 14$ , then  $\Omega^{14}(Z_t^{(4)})$  is described with  $(20s \times 19s)$  matrix with the following nonzero entries:

$$\begin{aligned} b_{(j+1)s,0} &= e_{8(j+m)+7} \otimes w_{8j \rightarrow 8(j+1)}; \\ b_{s+(j+1)s,s} &= -e_{8(j+m+1)} \otimes w_{8j \rightarrow 8(j+1)}; \\ b_{2s+(j+1)s,2s} &= -e_{8(j+m+1)} \otimes w_{8j \rightarrow 8(j+1)}. \end{aligned}$$

(16) If  $r_0 = 15$ , then  $\Omega^{15}(Z_t^{(4)})$  is described with  $(18s \times 16s)$  matrix with the following nonzero entries:

$$\begin{aligned} b_{(j+1)s,0} &= e_{8(j+m+1)+3} \otimes w_{8j \rightarrow 8(j+1)}; \\ b_{s+(j+1)s,s} &= e_{8(j+m+1)+6} \otimes w_{8j \rightarrow 8(j+1)}; \\ b_{3s+(j+1)s,2s} &= e_{8(j+m+1)+1} \otimes w_{8j \rightarrow 8(j+1)}; \\ b_{4s+(j+1)s,3s} &= -e_{8(j+m+1)+5} \otimes w_{8j \rightarrow 8(j+1)}. \end{aligned}$$

(17) If  $r_0 = 16$ , then  $\Omega^{16}(Z_t^{(4)})$  is described with  $(19s \times 16s)$  matrix with the following nonzero entries:

$$\begin{aligned} b_{(j+1)s,0} &= -e_{8(j+m)+7} \otimes w_{8j \rightarrow 8(j+1)}; \\ b_{s+(j+1)s,s} &= e_{8(j+m+1)} \otimes w_{8j \rightarrow 8(j+1)}; \\ b_{2s+(j+1)s,s} &= w_{8(j+m)+7 \rightarrow 8(j+m+1)} \otimes w_{8j \rightarrow 8(j+1)}. \end{aligned}$$

(18) If  $r_0 = 17$ , then  $\Omega^{17}(Z_t^{(4)})$  is described with  $(18s \times 14s)$  matrix with the following nonzero entries:

$$\begin{aligned} b_{(j+1)s,0} &= e_{8(j+m+1)+2} \otimes w_{8j \rightarrow 8(j+1)}; \\ b_{(j+1)s,s} &= -w_{8(j+m+1)+2 \rightarrow 8(j+m+1)+4} \otimes w_{8j \rightarrow 8(j+1)}; \\ b_{s+(j+1)s,s} &= e_{8(j+m+1)+4} \otimes w_{8j \rightarrow 8(j+1)}; \\ b_{2s+(j+1)s,2s} &= -e_{8(j+m+1)+6} \otimes w_{8j \rightarrow 8(j+1)}; \\ b_{3s+(j+1)s,2s} &= -w_{8(j+m+1)+5 \rightarrow 8(j+m+1)+6} \otimes w_{8j \rightarrow 8(j+1)}. \end{aligned}$$

(19) If  $r_0 = 18$ , then  $\Omega^{18}(Z_t^{(4)})$  is described with  $(19s \times 13s)$  matrix with two nonzero entries:

$$\begin{aligned} b_{s+(j+1)s,0} &= -e_{8(j+m+1)} \otimes w_{8j \rightarrow 8(j+1)}; \\ b_{(j+1)s,s} &= -e_{8(j+m)+7} \otimes w_{8j \rightarrow 8(j+1)}. \end{aligned}$$

(20) If  $r_0 = 19$ , then  $\Omega^{19}(Z_t^{(4)})$  is described with  $(16s \times 11s)$  matrix with two nonzero entries:

$$\begin{aligned} b_{(j+1)s,0} &= e_{8(j+m+1)+3} \otimes w_{8j \rightarrow 8(j+1)}; \\ b_{3s+(j+1)s,s} &= -e_{8(j+m+1)+5} \otimes w_{8j \rightarrow 8(j+1)}. \end{aligned}$$

(21) If  $r_0 = 20$ , then  $\Omega^{20}(Z_t^{(4)})$  is described with  $(16s \times 11s)$  matrix with unique nonzero entry:

$$b_{s+(j+1)s,0} = e_{8(j+m+1)} \otimes w_{8j \rightarrow 8(j+1)}.$$

(22) If  $r_0 = 21$ , then  $\Omega^{21}(Z_t^{(4)})$  is described with  $(14s \times 10s)$  matrix with two nonzero entries:

$$\begin{aligned} b_{s+(j+1)s,0} &= e_{8(j+m+1)+4} \otimes w_{8j \rightarrow 8(j+1)}; \\ b_{2s+(j+1)s,s} &= -e_{8(j+m+1)+6} \otimes w_{8j \rightarrow 8(j+1)}. \end{aligned}$$

(23) If  $r_0 = 22$ , then  $\Omega^{22}(Z_t^{(4)})$  is described with  $(13s \times 8s)$  matrix with unique nonzero entry:

$$b_{s+(j+1)s,0} = e_{8(j+m)+7} \otimes w_{8j \rightarrow 8(j+1)}.$$

(24) If  $r_0 = 23$ , then  $\Omega^{23}(Z_t^{(4)})$  is described with  $(11s \times 9s)$  matrix with two nonzero entries:

$$\begin{aligned} b_{(j+1)s,0} &= w_{8(j+m+1)+3 \rightarrow 8(j+m+1)+7} \otimes w_{8j \rightarrow 8(j+1)}; \\ b_{s+(j+1)s,0} &= -w_{8(j+m+1)+5 \rightarrow 8(j+m+1)+7} \otimes w_{8j \rightarrow 8(j+1)}. \end{aligned}$$

(25) If  $r_0 = 24$ , then  $\Omega^{24}(Z_t^{(4)})$  is described with  $(11s \times 8s)$  matrix with unique nonzero entry:

$$b_{(j+1)s,0} = -e_{8(j+m+1)} \otimes w_{8j \rightarrow 8(j+1)}.$$

(26) If  $r_0 = 25$ , then  $\Omega^{25}(Z_t^{(4)})$  is described with  $(10s \times 8s)$  matrix with unique nonzero entry:

$$b_{(j+1)s,0} = w_{8(j+m+1)+4 \rightarrow 8(j+m+2)} \otimes w_{8j \rightarrow 8(j+1)}.$$

(27) If  $r_0 = 26$ , then  $\Omega^{26}(Z_t^{(4)})$  is described with  $(8s \times 9s)$  matrix with unique nonzero entry:

$$b_{(j+1)s,0} = w_{8(j+m)+7 \rightarrow 8(j+m+1)+1} \otimes w_{8j \rightarrow 8(j+1)}.$$

(28) If  $r_0 = 27$ , then  $\Omega^{27}(Z_t^{(4)})$  is described with  $(9s \times 8s)$  matrix with unique nonzero entry:

$$b_{(j+1)s,0} = e_{8(j+m+1)+7} \otimes w_{8j \rightarrow 8(j+1)}.$$

(29) If  $r_0 = 28$ , then  $\Omega^{28}(Z_t^{(4)})$  is described with  $(8s \times 10s)$  matrix with the following nonzero entries:

$$\begin{aligned} b_{(j+1)s,0} &= w_{8(j+m+1) \rightarrow 8(j+m+1)+2} \otimes w_{8j \rightarrow 8(j+1)}; \\ b_{j+5s,s} &= -w_{8(j+m)+6 \rightarrow 8(j+m+1)+6} \otimes w_{8j \rightarrow 8j+6}; \end{aligned}$$

$$b_{j+6s,s} = w_{8(j+m)+7 \rightarrow 8(j+m+1)+6} \otimes w_{8j \rightarrow 8j+7}.$$

(II) Represent an arbitrary  $t_0 \in \mathbb{N}$  in the form  $t_0 = 29\ell_0 + r_0$ , where  $0 \leq r_0 \leq 28$ . Then  $\Omega^{t_0}(Z_t^{(4)})$  is a  $\Omega^{r_0}(Z_t^{(4)})$ , whose left components twisted by  $\sigma^{\ell_0}$ , and coefficients multiplied by  $(-1)^{\ell_0}$ .

**Proposition 5** (Translates for the case 6). (I) Let  $r_0 \in \mathbb{N}$ ,  $r_0 < 29$ .  $r_0$ -translates of the elements  $Z_t^{(6)}$  are described by the following way.

(1) If  $r_0 = 0$ , then  $\Omega^0(Z_t^{(6)})$  is described with  $(8s \times 13s)$  matrix with unique nonzero entry:

$$b_{j-s,s+(2)_s} = -w_{8(j+m) \rightarrow 8(j+m+1)} \otimes e_{8j}.$$

(2) If  $r_0 = 1$ , then  $\Omega^1(Z_t^{(6)})$  is described with  $(9s \times 14s)$  matrix with two nonzero entries:

$$b_{s+(j+1)_s, 5s+(1)_s} = w_{8(j+m+1)+5 \rightarrow 8(j+m+2)} \otimes w_{8j+2 \rightarrow 8(j+1)};$$

$$b_{s+(j+1)_s, 7s+(1)_s} = w_{8(j+m+1)+5 \rightarrow 8(j+m+2)} \otimes w_{8j+4 \rightarrow 8(j+1)}.$$

(3) If  $r_0 = 2$ , then  $\Omega^2(Z_t^{(6)})$  is described with  $(8s \times 16s)$  matrix with two nonzero entries:

$$b_{(j+1)_s, 3s+(1)_s} = -w_{8(j+m)+7 \rightarrow 8(j+m+1)+5} \otimes w_{8j+1 \rightarrow 8(j+1)};$$

$$b_{j-4s, 8s+(1)_s} = w_{8(j+m)+5 \rightarrow 8(j+m+1)+5} \otimes e_{8j+4}.$$

(4) If  $r_0 = 3$ , then  $\Omega^3(Z_t^{(6)})$  is described with  $(10s \times 16s)$  matrix with two nonzero entries:

$$b_{j+4s, (1)_s} = w_{8(j+m)+7 \rightarrow 8(j+m+1)+5} \otimes w_{8j \rightarrow 8j+3};$$

$$b_{s+(j+1)_s, 2s+(1)_s} = e_{8(j+m+1)+6} \otimes w_{8j \rightarrow 8(j+1)}.$$

(5) If  $r_0 = 4$ , then  $\Omega^4(Z_t^{(6)})$  is described with  $(11s \times 19s)$  matrix with the following nonzero entries:

$$b_{(j+1)_s, (1)_s} = -e_{8(j+m)+7} \otimes w_{8j \rightarrow 8(j+1)};$$

$$b_{j+2s, (1)_s} = w_{8(j+m)+3 \rightarrow 8(j+m)+7} \otimes w_{8j \rightarrow 8j+1};$$

$$b_{s+(j+1)_s, 2s+(1)_s} = e_{8(j+m+1)} \otimes w_{8j \rightarrow 8(j+1)};$$

$$b_{(j+1)_s, 7s} = w_{8(j+m)+7 \rightarrow 8(j+m+1)+5} \otimes w_{8j+3 \rightarrow 8(j+1)};$$

$$b_{s+(j+1)_s, 7s} = w_{8(j+m+1) \rightarrow 8(j+m+1)+5} \otimes w_{8j+3 \rightarrow 8(j+1)}.$$

(6) If  $r_0 = 5$ , then  $\Omega^5(Z_t^{(6)})$  is described with  $(11s \times 18s)$  matrix with the following nonzero entries:

$$b_{j+3s, (1)_s} = w_{8(j+m)+4 \rightarrow 8(j+m+1)+2} \otimes w_{8j \rightarrow 8j+1};$$

$$b_{j+4s, (1)_s} = w_{8(j+m)+7 \rightarrow 8(j+m+1)+2} \otimes w_{8j \rightarrow 8j+2};$$

$$b_{(j+1)_s, s+(1)_s} = -w_{8(j+m+1)+5 \rightarrow 8(j+m+1)+6} \otimes w_{8j \rightarrow 8(j+1)};$$

$$b_{2s+(j+1)_s, 3s+(1)_s} = e_{8(j+m+1)+1} \otimes w_{8j \rightarrow 8(j+1)};$$

$$b_{(j+1)_s, 4s} = e_{8(j+m+1)+5} \otimes w_{8j \rightarrow 8(j+1)};$$

$$b_{(j+1)_s, 5s} = w_{8(j+m+1)+5 \rightarrow 8(j+m+1)+7} \otimes w_{8j+1 \rightarrow 8(j+1)};$$

$$b_{s+(j+1)_s, 5s} = -w_{8(j+m+1)+3 \rightarrow 8(j+m+1)+7} \otimes w_{8j+1 \rightarrow 8(j+1)};$$

$$b_{2s+(j+1)_s, 5s} = -w_{8(j+m+1)+1 \rightarrow 8(j+m+1)+7} \otimes w_{8j+1 \rightarrow 8(j+1)};$$

$$b_{s+(j+1)_s, 7s} = -w_{8(j+m+1)+3 \rightarrow 8(j+m+1)+7} \otimes w_{8j+3 \rightarrow 8(j+1)};$$

$$b_{2s+(j+1)_s, 7s} = -w_{8(j+m+1)+1 \rightarrow 8(j+m+1)+7} \otimes w_{8j+3 \rightarrow 8(j+1)}.$$



(7) If  $r_0 = 6$ , then  $\Omega^6(Z_t^{(6)})$  is described with  $(13s \times 19s)$  matrix with the following nonzero entries:

$$\begin{aligned} b_{(j+1)s,(1)s} &= e_{8(j+m)+7} \otimes w_{8j \rightarrow 8(j+1)}; \\ b_{j+2s,(1)s} &= w_{8(j+m)+4 \rightarrow 8(j+m)+7} \otimes w_{8j \rightarrow 8j+1}; \\ b_{(j+1)s,2s} &= -e_{8(j+m)+7} \otimes w_{8j \rightarrow 8(j+1)}; \\ b_{(j+1)s,3s} &= w_{8(j+m)+7 \rightarrow 8(j+m+1)+2} \otimes w_{8j+1 \rightarrow 8(j+1)}; \\ b_{(j+1)s,4s} &= w_{8(j+m)+7 \rightarrow 8(j+m+1)+3} \otimes w_{8j+2 \rightarrow 8(j+1)}; \\ b_{(j+1)s,6s} &= w_{8(j+m)+7 \rightarrow 8(j+m+1)+4} \otimes w_{8j+3 \rightarrow 8(j+1)}. \end{aligned}$$

(8) If  $r_0 = 7$ , then  $\Omega^7(Z_t^{(6)})$  is described with  $(14s \times 18s)$  matrix with the following nonzero entries:

$$\begin{aligned} b_{j+4s,(1)s} &= w_{8(j+m)+7 \rightarrow 8(j+m+1)+2} \otimes w_{8j \rightarrow 8j+1}; \\ b_{j+3s,s+(1)s} &= w_{8(j+m)+7 \rightarrow 8(j+m+1)+3} \otimes w_{8j \rightarrow 8j+1}; \\ b_{2s+(j+1)s,2s} &= -e_{8(j+m+1)+6} \otimes w_{8j \rightarrow 8(j+1)}; \\ b_{(j+1)s,6s} &= w_{8(j+m+1)+2 \rightarrow 8(j+m+1)+7} \otimes w_{8j+3 \rightarrow 8(j+1)}; \\ b_{s+(j+1)s,6s} &= -w_{8(j+m+1)+4 \rightarrow 8(j+m+1)+7} \otimes w_{8j+3 \rightarrow 8(j+1)}; \\ b_{(j+1)s,7s} &= -w_{8(j+m+1)+2 \rightarrow 8(j+m+2)} \otimes w_{8j+3 \rightarrow 8(j+1)}; \\ b_{s+(j+1)s,7s} &= w_{8(j+m+1)+4 \rightarrow 8(j+m+2)} \otimes w_{8j+3 \rightarrow 8(j+1)}; \\ b_{4s+(j+1)s,16s} &= w_{8(j+m+1)+7 \rightarrow 8(j+m+2)+1} \otimes w_{8j+7 \rightarrow 8(j+1)+1}; \\ b_{5s+(j+1)s,16s} &= w_{8(j+m+2) \rightarrow 8(j+m+2)+1} \otimes w_{8j+7 \rightarrow 8(j+1)+2}. \end{aligned}$$

(9) If  $r_0 = 8$ , then  $\Omega^8(Z_t^{(6)})$  is described with  $(16s \times 20s)$  matrix with the following nonzero entries:

$$\begin{aligned} b_{(j+1)s,0} &= e_{8(j+m)+7} \otimes w_{8j \rightarrow 8(j+1)}; \\ b_{s+(j+1)s,0} &= -e_{8(j+m)+7} \otimes w_{8j \rightarrow 8(j+1)}; \\ b_{(j+1)s,2s} &= w_{8(j+m)+7 \rightarrow 8(j+m+1)} \otimes w_{8j \rightarrow 8(j+1)}; \\ b_{s+(j+1)s,2s} &= -w_{8(j+m)+7 \rightarrow 8(j+m+1)} \otimes w_{8j \rightarrow 8(j+1)}; \\ b_{(j+1)s,8s} &= -w_{8(j+m)+7 \rightarrow 8(j+m+1)+1} \otimes w_{8j+3 \rightarrow 8(j+1)}; \\ b_{s+(j+1)s,8s} &= w_{8(j+m)+7 \rightarrow 8(j+m+1)+1} \otimes w_{8j+3 \rightarrow 8(j+1)}; \\ b_{2s+(j+1)s,8s} &= -w_{8(j+m+1) \rightarrow 8(j+m+1)+1} \otimes w_{8j+3 \rightarrow 8(j+1)}; \\ b_{2s+(j+1)s,9s} &= w_{8(j+m+1) \rightarrow 8(j+m+1)+2} \otimes w_{8j+4 \rightarrow 8(j+1)}; \\ b_{6s+(j+1)s,9s} &= -e_{8(j+m+1)+2} \otimes w_{8j+4 \rightarrow 8(j+1)+3}; \\ b_{4s+(j+1)s,17s} &= -w_{8(j+m+1)+6 \rightarrow 8(j+m+1)+7} \otimes w_{8j+7 \rightarrow 8(j+1)+2}. \end{aligned}$$

(10) If  $r_0 = 9$ , then  $\Omega^9(Z_t^{(6)})$  is described with  $(16s \times 18s)$  matrix with the following nonzero entries:

$$\begin{aligned} b_{3s+(j+1)s,3s} &= -e_{8(j+m+1)+1} \otimes w_{8j \rightarrow 8(j+1)}; \\ b_{s+(j+1)s,8s} &= w_{8(j+m+1)+3 \rightarrow 8(j+m+2)} \otimes w_{8j+3 \rightarrow 8(j+1)}; \\ b_{3s+(j+1)s,9s} &= w_{8(j+m+1)+1 \rightarrow 8(j+m+1)+7} \otimes w_{8j+4 \rightarrow 8(j+1)}; \\ b_{5s+(j+1)s,9s} &= e_{8(j+m+1)+7} \otimes w_{8j+4 \rightarrow 8(j+1)+2}. \end{aligned}$$

(11) If  $r_0 = 10$ , then  $\Omega^{10}(Z_t^{(6)})$  is described with  $(19s \times 19s)$  matrix with the following nonzero entries:

$$b_{s+(j+1)s,s} = e_{8(j+m+1)} \otimes w_{8j \rightarrow 8(j+1)};$$

$$\begin{aligned}
b_{(j+1)s,7s} &= -w_{8(j+m)+7 \rightarrow 8(j+m+1)+2} \otimes w_{8j+3 \rightarrow 8(j+1)}; \\
b_{(j+1)s,9s} &= -w_{8(j+m)+7 \rightarrow 8(j+m+1)+3} \otimes w_{8j+4 \rightarrow 8(j+1)}; \\
b_{s+(j+1)s,9s} &= -w_{8(j+m+1) \rightarrow 8(j+m+1)+3} \otimes w_{8j+4 \rightarrow 8(j+1)}; \\
b_{6s+(j+1)s,9s} &= -e_{8(j+m+1)+3} \otimes w_{8j+4 \rightarrow 8(j+1)+3}.
\end{aligned}$$

(12) If  $r_0 = 11$ , then  $\Omega^{11}(Z_t^{(6)})$  is described with  $(18s \times 18s)$  matrix with the following nonzero entries:

$$\begin{aligned}
b_{(j+1)s,0} &= -e_{8(j+m+1)+2} \otimes w_{8j \rightarrow 8(j+1)}; \\
b_{(j+1)s,s} &= -w_{8(j+m+1)+2 \rightarrow 8(j+m+1)+4} \otimes w_{8j \rightarrow 8(j+1)}; \\
b_{4s+(j+1)s,3s} &= e_{8(j+m+1)+5} \otimes w_{8j \rightarrow 8(j+1)}; \\
b_{2s+(j+1)s,7s} &= w_{8(j+m+1)+4 \rightarrow 8(j+m+1)+7} \otimes w_{8j+3 \rightarrow 8(j+1)}; \\
b_{(j+1)s,8s} &= -w_{8(j+m+1)+2 \rightarrow 8(j+m+2)} \otimes w_{8j+4 \rightarrow 8(j+1)}; \\
b_{6s+(j+1)s,8s} &= e_{8(j+m+2)} \otimes w_{8j+4 \rightarrow 8(j+1)+2}.
\end{aligned}$$

(13) If  $r_0 = 12$ , then  $\Omega^{12}(Z_t^{(6)})$  is described with  $(19s \times 19s)$  matrix with the following nonzero entries:

$$\begin{aligned}
b_{2s+(j+1)s,0} &= -e_{8(j+m)+7} \otimes w_{8j \rightarrow 8(j+1)}; \\
b_{s+(j+1)s,7s} &= -w_{8(j+m+1) \rightarrow 8(j+m+1)+3} \otimes w_{8j+3 \rightarrow 8(j+1)}; \\
b_{(j+1)s,8s} &= -w_{8(j+m)+7 \rightarrow 8(j+m+1)+4} \otimes w_{8j+4 \rightarrow 8(j+1)}; \\
b_{3s+(j+1)s,8s} &= w_{8(j+m+1)+2 \rightarrow 8(j+m+1)+4} \otimes w_{8j+4 \rightarrow 8(j+1)+1}; \\
b_{6s+(j+1)s,8s} &= -e_{8(j+m+1)+4} \otimes w_{8j+4 \rightarrow 8(j+1)+3}; \\
b_{5s+(j+1)s,9s} &= e_{8(j+m+1)+5} \otimes w_{8j+4 \rightarrow 8(j+1)+2}.
\end{aligned}$$

(14) If  $r_0 = 13$ , then  $\Omega^{13}(Z_t^{(6)})$  is described with  $(18s \times 16s)$  matrix with the following nonzero entries:

$$\begin{aligned}
b_{(j+1)s,0} &= w_{8(j+m+1)+2 \rightarrow 8(j+m+1)+3} \otimes w_{8j \rightarrow 8(j+1)}; \\
b_{s+(j+1)s,0} &= -e_{8(j+m+1)+3} \otimes w_{8j \rightarrow 8(j+1)}; \\
b_{2s+(j+1)s,s} &= -e_{8(j+m+1)+6} \otimes w_{8j \rightarrow 8(j+1)}; \\
b_{3s+(j+1)s,5s} &= w_{8(j+m+1)+5 \rightarrow 8(j+m+1)+7} \otimes w_{8j+2 \rightarrow 8(j+1)}; \\
b_{s+(j+1)s,6s} &= w_{8(j+m+1)+3 \rightarrow 8(j+m+2)} \otimes w_{8j+3 \rightarrow 8(j+1)}; \\
b_{3s+(j+1)s,6s} &= -w_{8(j+m+1)+5 \rightarrow 8(j+m+2)} \otimes w_{8j+3 \rightarrow 8(j+1)}; \\
b_{5s+(j+1)s,6s} &= -w_{8(j+m+1)+7 \rightarrow 8(j+m+2)} \otimes w_{8j+3 \rightarrow 8(j+1)+2}; \\
b_{s+(j+1)s,7s} &= -w_{8(j+m+1)+3 \rightarrow 8(j+m+1)+7} \otimes w_{8j+4 \rightarrow 8(j+1)}; \\
b_{5s+(j+1)s,7s} &= e_{8(j+m+1)+7} \otimes w_{8j+4 \rightarrow 8(j+1)+2}.
\end{aligned}$$

(15) If  $r_0 = 14$ , then  $\Omega^{14}(Z_t^{(6)})$  is described with  $(20s \times 16s)$  matrix with the following nonzero entries:

$$\begin{aligned}
b_{(j+1)s,0} &= e_{8(j+m)+7} \otimes w_{8j \rightarrow 8(j+1)}; \\
b_{(j+1)s,s} &= w_{8(j+m)+7 \rightarrow 8(j+m+1)} \otimes w_{8j \rightarrow 8(j+1)}; \\
b_{2s+(j+1)s,s} &= -e_{8(j+m+1)} \otimes w_{8j \rightarrow 8(j+1)}; \\
b_{(j+1)s,6s} &= -w_{8(j+m)+7 \rightarrow 8(j+m+1)+5} \otimes w_{8j+3 \rightarrow 8(j+1)}; \\
b_{s+(j+1)s,6s} &= -w_{8(j+m+1) \rightarrow 8(j+m+1)+5} \otimes w_{8j+3 \rightarrow 8(j+1)}; \\
b_{2s+(j+1)s,6s} &= w_{8(j+m+1) \rightarrow 8(j+m+1)+5} \otimes w_{8j+3 \rightarrow 8(j+1)}; \\
b_{4s+(j+1)s,6s} &= e_{8(j+m+1)+5} \otimes w_{8j+3 \rightarrow 8(j+1)+1};
\end{aligned}$$

$$b_{6s+(j+1)s,7s} = e_{8(j+m+1)+6} \otimes w_{8j+4 \rightarrow 8(j+1)+2}.$$

(16) If  $r_0 = 15$ , then  $\Omega^{15}(Z_t^{(6)})$  is described with  $(18s \times 14s)$  matrix with the following nonzero entries:

$$\begin{aligned} b_{3s+(j+1)s,0} &= w_{8(j+m+1)+1 \rightarrow 8(j+m+1)+2} \otimes w_{8j \rightarrow 8(j+1)}; \\ b_{(j+1)s,s} &= w_{8(j+m+1)+3 \rightarrow 8(j+m+1)+4} \otimes w_{8j \rightarrow 8(j+1)}; \\ b_{2s+(j+1)s,s} &= -e_{8(j+m+1)+4} \otimes w_{8j \rightarrow 8(j+1)}; \\ b_{3s+(j+1)s,s} &= -w_{8(j+m+1)+1 \rightarrow 8(j+m+1)+4} \otimes w_{8j \rightarrow 8(j+1)}; \\ b_{4s+(j+1)s,2s} &= -w_{8(j+m+1)+5 \rightarrow 8(j+m+1)+6} \otimes w_{8j \rightarrow 8(j+1)}; \\ b_{s+(j+1)s,5s} &= w_{8(j+m+1)+6 \rightarrow 8(j+m+1)+7} \otimes w_{8j+3 \rightarrow 8(j+1)}; \\ b_{4s+(j+1)s,5s} &= w_{8(j+m+1)+5 \rightarrow 8(j+m+1)+7} \otimes w_{8j+3 \rightarrow 8(j+1)}; \\ b_{7s+(j+1)s,6s} &= e_{8(j+m+2)} \otimes w_{8j+4 \rightarrow 8(j+1)+2}. \end{aligned}$$

(17) If  $r_0 = 16$ , then  $\Omega^{16}(Z_t^{(6)})$  is described with  $(19s \times 13s)$  matrix with the following nonzero entries:

$$\begin{aligned} b_{s+(j+1)s,0} &= e_{8(j+m+1)} \otimes w_{8j \rightarrow 8(j+1)}; \\ b_{(j+1)s,s} &= e_{8(j+m)+7} \otimes w_{8j \rightarrow 8(j+1)}; \\ b_{2s+(j+1)s,s} &= -e_{8(j+m)+7} \otimes w_{8j \rightarrow 8(j+1)}; \\ b_{(j+1)s,5s} &= -w_{8(j+m)+7 \rightarrow 8(j+m+1)+6} \otimes w_{8j+3 \rightarrow 8(j+1)}; \\ b_{4s+(j+1)s,5s} &= e_{8(j+m+1)+6} \otimes w_{8j+3 \rightarrow 8(j+1)+1}; \\ b_{6s+(j+1)s,6s} &= e_{8(j+m+1)+1} \otimes w_{8j+4 \rightarrow 8(j+1)+2}. \end{aligned}$$

(18) If  $r_0 = 17$ , then  $\Omega^{17}(Z_t^{(6)})$  is described with  $(18s \times 11s)$  matrix with the following nonzero entries:

$$\begin{aligned} b_{(j+1)s,0} &= -w_{8(j+m+1)+2 \rightarrow 8(j+m+1)+3} \otimes w_{8j \rightarrow 8(j+1)}; \\ b_{3s+(j+1)s,s} &= e_{8(j+m+1)+5} \otimes w_{8j \rightarrow 8(j+1)}; \\ b_{(j+1)s,3s} &= w_{8(j+m+1)+2 \rightarrow 8(j+m+1)+7} \otimes w_{8j+2 \rightarrow 8(j+1)}; \\ b_{2s+(j+1)s,3s} &= w_{8(j+m+1)+6 \rightarrow 8(j+m+1)+7} \otimes w_{8j+2 \rightarrow 8(j+1)}; \\ b_{3s+(j+1)s,3s} &= w_{8(j+m+1)+5 \rightarrow 8(j+m+1)+7} \otimes w_{8j+2 \rightarrow 8(j+1)}; \\ b_{s+(j+1)s,4s} &= -w_{8(j+m+1)+4 \rightarrow 8(j+m+2)} \otimes w_{8j+3 \rightarrow 8(j+1)}; \\ b_{4s+(j+1)s,4s} &= -w_{8(j+m+1)+7 \rightarrow 8(j+m+2)} \otimes w_{8j+3 \rightarrow 8(j+1)+1}; \\ b_{5s+(j+1)s,5s} &= -w_{8(j+m+2) \rightarrow 8(j+m+2)+1} \otimes w_{8j+4 \rightarrow 8(j+1)+1}. \end{aligned}$$

(19) If  $r_0 = 18$ , then  $\Omega^{18}(Z_t^{(6)})$  is described with  $(19s \times 11s)$  matrix with the following nonzero entries:

$$\begin{aligned} b_{s+(j+1)s,0} &= -e_{8(j+m+1)} \otimes w_{8j \rightarrow 8(j+1)}; \\ b_{2s+(j+1)s,0} &= e_{8(j+m+1)} \otimes w_{8j \rightarrow 8(j+1)}; \\ b_{(j+1)s,s} &= w_{8(j+m)+7 \rightarrow 8(j+m+1)+4} \otimes w_{8j+1 \rightarrow 8(j+1)}; \\ b_{(j+1)s,3s} &= w_{8(j+m)+7 \rightarrow 8(j+m+1)+6} \otimes w_{8j+2 \rightarrow 8(j+1)}; \\ b_{s+(j+1)s,4s} &= -w_{8(j+m+1) \rightarrow 8(j+m+1)+1} \otimes w_{8j+3 \rightarrow 8(j+1)}; \\ b_{2s+(j+1)s,5s} &= -w_{8(j+m+1) \rightarrow 8(j+m+1)+2} \otimes w_{8j+4 \rightarrow 8(j+1)}; \\ b_{5s+(j+1)s,5s} &= -e_{8(j+m+1)+2} \otimes w_{8j+4 \rightarrow 8(j+1)+2}. \end{aligned}$$

(20) If  $r_0 = 19$ , then  $\Omega^{19}(Z_t^{(6)})$  is described with  $(16s \times 10s)$  matrix with the following nonzero entries:

$$\begin{aligned}
b_{(j+1)s,0} &= -w_{8(j+m+1)+3 \rightarrow 8(j+m+1)+4} \otimes w_{8j \rightarrow 8(j+1)}; \\
b_{2s+(j+1)s,0} &= w_{8(j+m+1)+1 \rightarrow 8(j+m+1)+4} \otimes w_{8j \rightarrow 8(j+1)}; \\
b_{s+(j+1)s,s} &= -e_{8(j+m+1)+6} \otimes w_{8j \rightarrow 8(j+1)}; \\
b_{3s+(j+1)s,s} &= -w_{8(j+m+1)+5 \rightarrow 8(j+m+1)+6} \otimes w_{8j \rightarrow 8(j+1)}; \\
b_{(j+1)s,3s} &= w_{8(j+m+1)+3 \rightarrow 8(j+m+2)} \otimes w_{8j+2 \rightarrow 8(j+1)}; \\
b_{2s+(j+1)s,3s} &= -w_{8(j+m+1)+1 \rightarrow 8(j+m+2)} \otimes w_{8j+2 \rightarrow 8(j+1)}; \\
b_{2s+(j+1)s,4s} &= w_{8(j+m+1)+1 \rightarrow 8(j+m+2)+1} \otimes w_{8j+3 \rightarrow 8(j+1)}; \\
b_{4s+(j+1)s,4s} &= -w_{8(j+m+2) \rightarrow 8(j+m+2)+1} \otimes w_{8j+3 \rightarrow 8(j+1)+1}; \\
b_{4s+(j+1)s,5s} &= w_{8(j+m+2) \rightarrow 8(j+m+2)+2} \otimes w_{8j+4 \rightarrow 8(j+1)+1}.
\end{aligned}$$

(21) If  $r_0 = 20$ , then  $\Omega^{20}(Z_t^{(6)})$  is described with  $(16s \times 8s)$  matrix with the following nonzero entries:

$$\begin{aligned}
b_{(j+1)s,0} &= -e_{8(j+m)+7} \otimes w_{8j \rightarrow 8(j+1)}; \\
b_{s+(j+1)s,2s} &= w_{8(j+m+1) \rightarrow 8(j+m+1)+1} \otimes w_{8j+2 \rightarrow 8(j+1)}; \\
b_{(j+1)s,4s} &= w_{8(j+m)+7 \rightarrow 8(j+m+1)+3} \otimes w_{8j+4 \rightarrow 8(j+1)}; \\
b_{s+(j+1)s,4s} &= -w_{8(j+m+1) \rightarrow 8(j+m+1)+3} \otimes w_{8j+4 \rightarrow 8(j+1)}; \\
b_{4s+(j+1)s,4s} &= -e_{8(j+m+1)+3} \otimes w_{8j+4 \rightarrow 8(j+1)+2}.
\end{aligned}$$

(22) If  $r_0 = 21$ , then  $\Omega^{21}(Z_t^{(6)})$  is described with  $(14s \times 9s)$  matrix with the following nonzero entries:

$$\begin{aligned}
b_{(j+1)s,2s} &= w_{8(j+m+1)+2 \rightarrow 8(j+m+2)+1} \otimes w_{8j+2 \rightarrow 8(j+1)}; \\
b_{s+(j+1)s,2s} &= w_{8(j+m+1)+4 \rightarrow 8(j+m+2)+1} \otimes w_{8j+2 \rightarrow 8(j+1)}; \\
b_{(j+1)s,3s} &= -w_{8(j+m+1)+2 \rightarrow 8(j+m+2)+2} \otimes w_{8j+3 \rightarrow 8(j+1)}; \\
b_{3s+(j+1)s,3s} &= -w_{8(j+m+1)+7 \rightarrow 8(j+m+2)+2} \otimes w_{8j+3 \rightarrow 8(j+1)+1}; \\
b_{3s+(j+1)s,4s} &= w_{8(j+m+1)+7 \rightarrow 8(j+m+2)+3} \otimes w_{8j+4 \rightarrow 8(j+1)+1}.
\end{aligned}$$

(23) If  $r_0 = 22$ , then  $\Omega^{22}(Z_t^{(6)})$  is described with  $(13s \times 8s)$  matrix with the following nonzero entries:

$$\begin{aligned}
b_{(j+1)s,s} &= w_{8(j+m+1) \rightarrow 8(j+m+1)+1} \otimes w_{8j+1 \rightarrow 8(j+1)}; \\
b_{s+(j+1)s,2s} &= w_{8(j+m)+7 \rightarrow 8(j+m+1)+2} \otimes w_{8j+2 \rightarrow 8(j+1)}; \\
b_{(j+1)s,4s} &= w_{8(j+m+1) \rightarrow 8(j+m+1)+4} \otimes w_{8j+4 \rightarrow 8(j+1)}; \\
b_{s+(j+1)s,4s} &= -w_{8(j+m)+7 \rightarrow 8(j+m+1)+4} \otimes w_{8j+4 \rightarrow 8(j+1)}; \\
b_{3s+(j+1)s,4s} &= -e_{8(j+m+1)+4} \otimes w_{8j+4 \rightarrow 8(j+1)+2}.
\end{aligned}$$

(24) If  $r_0 = 23$ , then  $\Omega^{23}(Z_t^{(6)})$  is described with  $(11s \times 8s)$  matrix with the following nonzero entries:

$$\begin{aligned}
b_{(j+1)s,2s} &= w_{8(j+m+1)+3 \rightarrow 8(j+m+2)+2} \otimes w_{8j+2 \rightarrow 8(j+1)}; \\
b_{2s+(j+1)s,2s} &= w_{8(j+m+2) \rightarrow 8(j+m+2)+2} \otimes w_{8j+2 \rightarrow 8(j+1)+1}; \\
b_{(j+1)s,3s} &= -w_{8(j+m+1)+3 \rightarrow 8(j+m+2)+3} \otimes w_{8j+3 \rightarrow 8(j+1)}; \\
b_{2s+(j+1)s,3s} &= -w_{8(j+m+2) \rightarrow 8(j+m+2)+3} \otimes w_{8j+3 \rightarrow 8(j+1)+1}; \\
b_{2s+(j+1)s,4s} &= w_{8(j+m+2) \rightarrow 8(j+m+2)+4} \otimes w_{8j+4 \rightarrow 8(j+1)+1}.
\end{aligned}$$

(25) If  $r_0 = 24$ , then  $\Omega^{24}(Z_t^{(6)})$  is described with  $(11s \times 9s)$  matrix with two nonzero entries:

$$b_{(j+1)s, 2s} = -w_{8(j+m+1) \rightarrow 8(j+m+1)+2} \otimes w_{8j+1 \rightarrow 8(j+1)};$$

$$b_{2s+(j+1)s, 5s} = w_{8(j+m+1)+5 \rightarrow 8(j+m+1)+7} \otimes w_{8j+4 \rightarrow 8(j+1)+1}.$$

(26) If  $r_0 = 25$ , then  $\Omega^{25}(Z_t^{(6)})$  is described with  $(10s \times 8s)$  matrix with the following nonzero entries:

$$b_{(j+1)s, 0} = -w_{8(j+m+1)+4 \rightarrow 8(j+m+1)+7} \otimes w_{8j \rightarrow 8(j+1)};$$

$$b_{s+(j+1)s, 4s} = w_{8(j+m+1)+6 \rightarrow 8(j+m+2)+5} \otimes w_{8j+4 \rightarrow 8(j+1)};$$

$$b_{3s+(j+1)s, 4s} = w_{8(j+m+2) \rightarrow 8(j+m+2)+5} \otimes w_{8j+4 \rightarrow 8(j+1)+2}.$$

(27) If  $r_0 = 26$ , then  $\Omega^{26}(Z_t^{(6)})$  is described with  $(8s \times 10s)$  matrix with the following nonzero entries:

$$b_{(j+1)s, 0} = w_{8(j+m)+7 \rightarrow 8(j+m+1)+2} \otimes w_{8j \rightarrow 8(j+1)};$$

$$b_{(j+1)s, s} = -w_{8(j+m)+7 \rightarrow 8(j+m+1)+6} \otimes w_{8j \rightarrow 8(j+1)};$$

$$b_{(j+1)s, 4s} = w_{8(j+m)+7 \rightarrow 8(j+m+1)+7} \otimes w_{8j+3 \rightarrow 8(j+1)};$$

$$b_{s+(j+1)s, 4s} = -w_{8(j+m+1)+6 \rightarrow 8(j+m+1)+7} \otimes w_{8j+3 \rightarrow 8(j+1)+1};$$

$$b_{s+(j+1)s, 5s} = -w_{8(j+m+1)+6 \rightarrow 8(j+m+2)} \otimes w_{8j+4 \rightarrow 8(j+1)+1}.$$

(28) If  $r_0 = 27$ , then  $\Omega^{27}(Z_t^{(6)})$  is described with  $(9s \times 11s)$  matrix with two nonzero entries:

$$b_{(j+1)s, 0} = e_{8(j+m+1)+7} \otimes w_{8j \rightarrow 8(j+1)};$$

$$b_{(j+1)s, 5s} = -w_{8(j+m+1)+7 \rightarrow 8(j+m+2)+6} \otimes w_{8j+4 \rightarrow 8(j+1)}.$$

(29) If  $r_0 = 28$ , then  $\Omega^{28}(Z_t^{(6)})$  is described with  $(8s \times 11s)$  matrix with the following nonzero entries:

$$b_{(j+1)s, 0} = -w_{8(j+m+1) \rightarrow 8(j+m+1)+5} \otimes w_{8j \rightarrow 8(j+1)};$$

$$b_{(j+1)s, s} = w_{8(j+m+1) \rightarrow 8(j+m+1)+3} \otimes w_{8j \rightarrow 8(j+1)};$$

$$b_{(j+1)s, 4s} = w_{8(j+m+1) \rightarrow 8(j+m+1)+7} \otimes w_{8j+2 \rightarrow 8(j+1)};$$

$$b_{s+(j+1)s, 4s} = -w_{8(j+m+1)+1 \rightarrow 8(j+m+1)+7} \otimes w_{8j+2 \rightarrow 8(j+1)+1};$$

$$b_{2s+(j+1)s, 4s} = w_{8(j+m+1)+2 \rightarrow 8(j+m+1)+7} \otimes w_{8j+2 \rightarrow 8(j+1)+2};$$

$$b_{j+s, 6s} = w_{8(j+m)+7 \rightarrow 8(j+m+1)+7} \otimes w_{8j+4 \rightarrow 8j+7}.$$

(II) Represent an arbitrary  $t_0 \in \mathbb{N}$  in the form  $t_0 = 29\ell_0 + r_0$ , where  $0 \leq r_0 \leq 28$ . Then  $\Omega^{t_0}(Z_t^{(6)})$  is a  $\Omega^{r_0}(Z_t^{(6)})$ , whose left components twisted by  $\sigma^{\ell_0}$ .

**Proposition 6** (Translates for the case 7). (I) Let  $r_0 \in \mathbb{N}$ ,  $r_0 < 29$ .  $r_0$ -translates of the elements  $Z_t^{(7)}$  are described by the following way.

(1) If  $r_0 = 0$ , then  $\Omega^0(Z_t^{(7)})$  is described with  $(8s \times 14s)$  matrix, whose entries  $b_{ij}$  have the following form:

If  $0 \leq j < s$ , then

$$b_{ij} = \begin{cases} -w_{8(j+m) \rightarrow 8(j+m)+2} \otimes e_{8j}, & i = j; \\ 0, & \text{otherwise.} \end{cases}$$

If  $s \leq j < 2s$ , then  $b_{ij} = 0$ .

If  $2s \leq j < 3s$ , then

$$b_{ij} = \begin{cases} w_{8(j+m) \rightarrow 8(j+m)+6} \otimes e_{8j}, & i = j - 2s; \\ 0, & \text{otherwise.} \end{cases}$$

If  $3s \leq j < 5s$ , then  $b_{ij} = 0$ .

If  $5s \leq j < 6s$ , then

$$b_{ij} = \begin{cases} w_{8(j+m)+2 \rightarrow 8(j+m+1)} \otimes e_{8j+2}, & i = j - 3s; \\ 0, & \text{otherwise.} \end{cases}$$

If  $6s \leq j < 13s$ , then  $b_{ij} = 0$ .

If  $13s \leq j < 14s$ , then

$$b_{ij} = \begin{cases} w_{8(j+m)+7 \rightarrow 8(j+m+1)+1} \otimes e_{8j+7}, & i = j - 6s; \\ 0, & \text{otherwise.} \end{cases}$$

(2) If  $r_0 = 1$ , then  $\Omega^1(Z_t^{(7)})$  is described with  $(9s \times 16s)$  matrix, whose entries  $b_{ij}$  have the following form:

If  $2s \leq j < 3s$ , then

$$b_{ij} = \begin{cases} w_{8(j+m)+1 \rightarrow 8(j+m+1)} \otimes e_{8j}, & i = j - 2s; \\ w_{8(j+m)+2 \rightarrow 8(j+m+1)} \otimes w_{8j \rightarrow 8j+1}, & i = j; \\ 0, & \text{otherwise.} \end{cases}$$

If  $3s \leq j < 4s$ , then  $b_{ij} = 0$ .

If  $4s \leq j < 5s$ , then

$$b_{ij} = \begin{cases} w_{8(j+m+1)+5 \rightarrow 8(j+m+1)+6} \otimes w_{8j+2 \rightarrow 8(j+1)}, & i = s + (j + 1)_s; \\ 0, & \text{otherwise.} \end{cases}$$

If  $5s \leq j < 6s$ , then

$$b_{ij} = \begin{cases} -w_{8(j+m)+3 \rightarrow 8(j+m+1)+1} \otimes e_{8j+2}, & i = j - 2s; \\ -w_{8(j+m)+4 \rightarrow 8(j+m+1)+1} \otimes w_{8j+2 \rightarrow 8j+3}, & i = j - s; \\ -w_{8(j+m)+7 \rightarrow 8(j+m+1)+1} \otimes w_{8j+2 \rightarrow 8j+4}, & i = j; \\ 0, & \text{otherwise.} \end{cases}$$

If  $6s \leq j < 7s$ , then

$$b_{ij} = \begin{cases} w_{8(j+m+1) \rightarrow 8(j+m+1)+2} \otimes w_{8j+3 \rightarrow 8j+7}, & i = j + 2s; \\ 0, & \text{otherwise.} \end{cases}$$

If  $7s \leq j < 8s$ , then

$$b_{ij} = \begin{cases} -w_{8(j+m+1) \rightarrow 8(j+m+1)+3} \otimes w_{8j+4 \rightarrow 8j+7}, & i = j + s; \\ 0, & \text{otherwise.} \end{cases}$$

If  $8s \leq j < 10s$ , then  $b_{ij} = 0$ .

If  $10s \leq j < 11s$ , then

$$b_{ij} = \begin{cases} w_{8(j+m+1)+5 \rightarrow 8(j+m+1)+6} \otimes w_{8j+5 \rightarrow 8(j+1)}, & i = s + (j+1)_s; \\ e_{8(j+m+1)+6} \otimes w_{8j+5 \rightarrow 8(j+1)+5}, & i = 6s + (j+1)_s; \\ 0, & \text{otherwise.} \end{cases}$$

If  $11s \leq j < 12s$ , then  $b_{ij} = 0$ .

If  $12s \leq j < 13s$ , then

$$b_{ij} = \begin{cases} w_{8(j+m+1)+1 \rightarrow 8(j+m+1)+4} \otimes w_{8j+6 \rightarrow 8(j+1)}, & i = (j+1)_s; \\ 0, & \text{otherwise.} \end{cases}$$

If  $13s \leq j < 14s$ , then

$$b_{ij} = \begin{cases} -w_{8(j+m)+7 \rightarrow 8(j+m+1)+1} \otimes e_{8j+6}, & i = j - 6s; \\ 0, & \text{otherwise.} \end{cases}$$

If  $14s \leq j < 15s$ , then

$$b_{ij} = \begin{cases} w_{8(j+m+1) \rightarrow 8(j+m+1)+7} \otimes e_{8j+7}, & i = j - 6s; \\ 0, & \text{otherwise.} \end{cases}$$

If  $15s \leq j < 16s$ , then

$$b_{ij} = \begin{cases} -w_{8(j+m+1)+1 \rightarrow 8(j+m+2)} \otimes w_{8j+7 \rightarrow 8(j+1)}, & i = (j+1)_s; \\ -w_{8(j+m+1)+2 \rightarrow 8(j+m+2)} \otimes w_{8j+7 \rightarrow 8(j+1)+1}, & i = 2s + (j+1)_s; \\ 0, & \text{otherwise.} \end{cases}$$

(3) If  $r_0 = 2$ , then  $\Omega^2(Z_t^{(7)})$  is described with  $(8s \times 16s)$  matrix, whose entries  $b_{ij}$  have the following form:

If  $3s \leq j < 4s$ , then

$$b_{ij} = \begin{cases} -w_{8(j+m-1)+7 \rightarrow 8(j+m)+1} \otimes e_{8j}, & i = j - 3s; \\ 0, & \text{otherwise.} \end{cases}$$

If  $4s \leq j < 5s$ , then

$$b_{ij} = \begin{cases} w_{8(j+m)+7 \rightarrow 8(j+m+1)} \otimes w_{8j+1 \rightarrow 8(j+1)}, & i = (j+1)_s; \\ 0, & \text{otherwise.} \end{cases}$$

If  $5s \leq j < 6s$ , then

$$b_{ij} = \begin{cases} e_{8(j+m)+7} \otimes w_{8j+2 \rightarrow 8(j+1)}, & i = (j+1)_s; \\ -w_{8(j+m)+3 \rightarrow 8(j+m)+7} \otimes e_{8j+2}, & i = j - 3s; \\ 0, & \text{otherwise.} \end{cases}$$

If  $6s \leq j < 8s$ , then  $b_{ij} = 0$ .

If  $8s \leq j < 9s$ , then

$$b_{ij} = \begin{cases} -e_{8(j+m)+7} \otimes w_{8j+5 \rightarrow 8(j+1)}, & i = (j+1)_s; \\ 0, & \text{otherwise.} \end{cases}$$

If  $9s \leq j < 10s$ , then

$$b_{ij} = \begin{cases} -w_{8(j+m)+7 \rightarrow 8(j+m+1)} \otimes w_{8j+5 \rightarrow 8(j+1)}, & i = (j+1)_s; \\ 0, & \text{otherwise.} \end{cases}$$

If  $10s \leq j < 11s$ , then

$$b_{ij} = \begin{cases} -w_{8(j+m)+1 \rightarrow 8(j+m)+7} \otimes e_{8j+6}, & i = j - 4s; \\ 0, & \text{otherwise.} \end{cases}$$

If  $11s \leq j < 12s$ , then  $b_{ij} = 0$ .

If  $12s \leq j < 13s$ , then

$$b_{ij} = \begin{cases} -e_{8(j+m+1)+2} \otimes w_{8j+7 \rightarrow 8(j+1)+1}, & i = s + (j+1)_s; \\ 0, & \text{otherwise.} \end{cases}$$

If  $13s \leq j < 14s$ , then

$$b_{ij} = \begin{cases} -w_{8(j+m+1)+2 \rightarrow 8(j+m+1)+4} \otimes w_{8j+7 \rightarrow 8(j+1)+1}, & i = s + (j+1)_s; \\ 0, & \text{otherwise.} \end{cases}$$

If  $14s \leq j < 16s$ , then  $b_{ij} = 0$ .

(4) If  $r_0 = 3$ , then  $\Omega^3(Z_t^{(7)})$  is described with  $(10s \times 19s)$  matrix, whose entries  $b_{ij}$  have the following form:

If  $0 \leq j < s$ , then

$$b_{ij} = \begin{cases} -w_{8(j+m)+2 \rightarrow 8(j+m)+7} \otimes e_{8j}, & i = j; \\ -w_{8(j+m)+3 \rightarrow 8(j+m)+7} \otimes w_{8j \rightarrow 8j+1}, & i = j + 2s; \\ 0, & \text{otherwise.} \end{cases}$$

If  $s \leq j < 5s$ , then  $b_{ij} = 0$ .

If  $5s \leq j < 6s$ , then

$$b_{ij} = \begin{cases} e_{8(j+m+1)+2} \otimes w_{8j+2 \rightarrow 8(j+1)}, & i = (j+1)_s; \\ w_{8(j+m)+4 \rightarrow 8(j+m+1)+2} \otimes e_{8j+2}, & i = j - 2s; \\ w_{8(j+m)+7 \rightarrow 8(j+m+1)+2} \otimes w_{8j+2 \rightarrow 8j+3}, & i = j - s; \\ 0, & \text{otherwise.} \end{cases}$$

If  $6s \leq j < 7s$ , then

$$b_{ij} = \begin{cases} -w_{8(j+m+1)+2 \rightarrow 8(j+m+1)+3} \otimes w_{8j+3 \rightarrow 8(j+1)}, & i = (j+1)_s; \\ 0, & \text{otherwise.} \end{cases}$$

If  $7s \leq j < 11s$ , then  $b_{ij} = 0$ .

If  $11s \leq j < 12s$ , then

$$b_{ij} = \begin{cases} w_{8(j+m+1)+2 \rightarrow 8(j+m+1)+4} \otimes w_{8j+5 \rightarrow 8(j+1)}, & i = (j+1)_s; \\ 0, & \text{otherwise.} \end{cases}$$

If  $12s \leq j < 16s$ , then  $b_{ij} = 0$ .



If  $16s \leq j < 17s$ , then

$$b_{ij} = \begin{cases} -w_{8(j+m+1)+3 \rightarrow 8(j+m+1)+7} \otimes w_{8j+7 \rightarrow 8(j+1)+1}, & i = 2s + (j+1)_s; \\ 0, & \text{otherwise.} \end{cases}$$

If  $17s \leq j < 18s$ , then

$$b_{ij} = \begin{cases} -w_{8(j+m+1)+3 \rightarrow 8(j+m+1)+7} \otimes w_{8j+7 \rightarrow 8(j+1)+1}, & i = 2s + (j+1)_s; \\ 0, & \text{otherwise.} \end{cases}$$

If  $18s \leq j < 19s$ , then  $b_{ij} = 0$ .

(5) If  $r_0 = 4$ , then  $\Omega^4(Z_t^{(7)})$  is described with  $(11s \times 18s)$  matrix, whose entries  $b_{ij}$  have the following form:

If  $0 \leq j < s$ , then

$$b_{ij} = \begin{cases} w_{8(j+m-1)+7 \rightarrow 8(j+m)+2} \otimes e_{8j}, & i = j; \\ w_{8(j+m) \rightarrow 8(j+m)+2} \otimes e_{8j}, & i = j + s; \\ -w_{8(j+m)+1 \rightarrow 8(j+m)+2} \otimes w_{8j \rightarrow 8j+4}, & i = j + 6s; \\ e_{8(j+m)+2} \otimes w_{8j \rightarrow 8j+6}, & i = j + 8s; \\ 0, & \text{otherwise.} \end{cases}$$

If  $s \leq j < 5s$ , then  $b_{ij} = 0$ .

If  $5s \leq j < 6s$ , then

$$b_{ij} = \begin{cases} -w_{8(j+m)+3 \rightarrow 8(j+m)+7} \otimes e_{8j+1}, & i = j - 3s; \\ 0, & \text{otherwise.} \end{cases}$$

If  $6s \leq j < 11s$ , then  $b_{ij} = 0$ .

If  $11s \leq j < 12s$ , then

$$b_{ij} = \begin{cases} -w_{8(j+m)+7 \rightarrow 8(j+m+1)} \otimes w_{8j+5 \rightarrow 8(j+1)}, & i = (j+1)_s; \\ -e_{8(j+m+1)} \otimes w_{8j+5 \rightarrow 8(j+1)}, & i = s + (j+1)_s; \\ 0, & \text{otherwise.} \end{cases}$$

If  $12s \leq j < 15s$ , then  $b_{ij} = 0$ .

If  $15s \leq j < 16s$ , then

$$b_{ij} = \begin{cases} -e_{8(j+m+1)+3} \otimes w_{8j+7 \rightarrow 8(j+1)+1}, & i = 2s + (j+1)_s; \\ 0, & \text{otherwise.} \end{cases}$$

If  $16s \leq j < 18s$ , then  $b_{ij} = 0$ .

(6) If  $r_0 = 5$ , then  $\Omega^5(Z_t^{(7)})$  is described with  $(11s \times 19s)$  matrix, whose entries  $b_{ij}$  have the following form:

If  $0 \leq j < s$ , then

$$b_{ij} = \begin{cases} w_{8(j+m)+3 \rightarrow 8(j+m)+7} \otimes e_{8j}, & i = j + s; \\ w_{8(j+m)+1 \rightarrow 8(j+m)+7} \otimes e_{8j}, & i = j + 2s; \\ 0, & \text{otherwise.} \end{cases}$$

If  $s \leq j < 2s$ , then

$$b_{ij} = \begin{cases} -w_{8(j+m)+3 \rightarrow 8(j+m+1)} \otimes e_{8j}, & i = j; \\ -w_{8(j+m)+1 \rightarrow 8(j+m+1)} \otimes e_{8j}, & i = j + s; \\ -w_{8(j+m)+4 \rightarrow 8(j+m+1)} \otimes w_{8j \rightarrow 8j+1}, & i = j + 2s; \\ -w_{8(j+m)+7 \rightarrow 8(j+m+1)} \otimes w_{8j \rightarrow 8j+2}, & i = j + 3s; \\ -e_{8(j+m+1)} \otimes w_{8j \rightarrow 8j+3}, & i = j + 4s; \\ 0, & \text{otherwise.} \end{cases}$$

If  $2s \leq j < 3s$ , then  $b_{ij} = 0$ .

If  $3s \leq j < 4s$ , then

$$b_{ij} = \begin{cases} -w_{8(j+m+1)+1 \rightarrow 8(j+m+1)+2} \otimes w_{8j+1 \rightarrow 8(j+1)}, & i = 2s + (j + 1)_s; \\ w_{8(j+m)+4 \rightarrow 8(j+m+1)+2} \otimes e_{8j+1}, & i = j; \\ w_{8(j+m)+7 \rightarrow 8(j+m+1)+2} \otimes w_{8j+1 \rightarrow 8j+2}, & i = j + s; \\ 0, & \text{otherwise.} \end{cases}$$

If  $4s \leq j < 5s$ , then

$$b_{ij} = \begin{cases} e_{8(j+m+1)+3} \otimes w_{8j+2 \rightarrow 8(j+1)}, & i = s + (j + 1)_s; \\ w_{8(j+m+1)+1 \rightarrow 8(j+m+1)+3} \otimes w_{8j+2 \rightarrow 8(j+1)}, & i = 2s + (j + 1)_s; \\ 0, & \text{otherwise.} \end{cases}$$

If  $5s \leq j < 6s$ , then  $b_{ij} = 0$ .

If  $6s \leq j < 7s$ , then

$$b_{ij} = \begin{cases} -w_{8(j+m+1)+3 \rightarrow 8(j+m+1)+4} \otimes w_{8j+3 \rightarrow 8(j+1)}, & i = s + (j + 1)_s; \\ -w_{8(j+m+1)+1 \rightarrow 8(j+m+1)+4} \otimes w_{8j+3 \rightarrow 8(j+1)}, & i = 2s + (j + 1)_s; \\ 0, & \text{otherwise.} \end{cases}$$

If  $7s \leq j < 12s$ , then  $b_{ij} = 0$ .

If  $12s \leq j < 13s$ , then

$$b_{ij} = \begin{cases} -e_{8(j+m+1)+5} \otimes w_{8j+5 \rightarrow 8(j+1)}, & i = (j + 1)_s; \\ 0, & \text{otherwise.} \end{cases}$$

If  $13s \leq j < 17s$ , then  $b_{ij} = 0$ .

If  $17s \leq j < 18s$ , then

$$b_{ij} = \begin{cases} -w_{8(j+m+1)+4 \rightarrow 8(j+m+2)} \otimes w_{8j+7 \rightarrow 8(j+1)+1}, & i = 3s + (j + 1)_s; \\ -w_{8(j+m+1)+7 \rightarrow 8(j+m+2)} \otimes w_{8j+7 \rightarrow 8(j+1)+2}, & i = 4s + (j + 1)_s; \\ -e_{8(j+m+2)} \otimes w_{8j+7 \rightarrow 8(j+1)+3}, & i = 5s + (j + 1)_s; \\ 0, & \text{otherwise.} \end{cases}$$

If  $18s \leq j < 19s$ , then

$$b_{ij} = \begin{cases} -w_{8(j+m+1)+4 \rightarrow 8(j+m+2)} \otimes w_{8j+7 \rightarrow 8(j+1)+1}, & i = 3s + (j + 1)_s; \\ -w_{8(j+m+1)+7 \rightarrow 8(j+m+2)} \otimes w_{8j+7 \rightarrow 8(j+1)+2}, & i = 4s + (j + 1)_s; \\ -e_{8(j+m+2)} \otimes w_{8j+7 \rightarrow 8(j+1)+3}, & i = 5s + (j + 1)_s; \\ 0, & \text{otherwise.} \end{cases}$$

(7) If  $r_0 = 6$ , then  $\Omega^6(Z_t^{(7)})$  is described with  $(13s \times 18s)$  matrix, whose entries  $b_{ij}$  have the following form:

If  $0 \leq j < s$ , then

$$b_{ij} = \begin{cases} w_{8(j+m)+1 \rightarrow 8(j+m)+2} \otimes w_{8j \rightarrow 8j+3}, & i = j + 5s; \\ 0, & \text{otherwise.} \end{cases}$$

If  $s \leq j < 2s$ , then

$$b_{ij} = \begin{cases} -w_{8(j+m-1)+7 \rightarrow 8(j+m)+3} \otimes e_{8j}, & i = j - s; \\ w_{8(j+m)+2 \rightarrow 8(j+m)+3} \otimes w_{8j \rightarrow 8j+4}, & i = j + 5s; \\ e_{8(j+m)+3} \otimes w_{8j \rightarrow 8j+6}, & i = j + 8s; \\ 0, & \text{otherwise.} \end{cases}$$

If  $2s \leq j < 3s$ , then  $b_{ij} = 0$ .

If  $3s \leq j < 4s$ , then

$$b_{ij} = \begin{cases} -e_{8(j+m)+5} \otimes w_{8j \rightarrow 8j+2}, & i = j; \\ 0, & \text{otherwise.} \end{cases}$$

If  $4s \leq j < 5s$ , then

$$b_{ij} = \begin{cases} -e_{8(j+m+1)} \otimes w_{8j+1 \rightarrow 8(j+1)}, & i = s + (j + 1)_s; \\ 0, & \text{otherwise.} \end{cases}$$

If  $5s \leq j < 9s$ , then  $b_{ij} = 0$ .

If  $9s \leq j < 10s$ , then

$$b_{ij} = \begin{cases} e_{8(j+m)+7} \otimes w_{8j+5 \rightarrow 8(j+1)}, & i = (j + 1)_s; \\ 0, & \text{otherwise.} \end{cases}$$

If  $10s \leq j < 13s$ , then  $b_{ij} = 0$ .

If  $13s \leq j < 14s$ , then

$$b_{ij} = \begin{cases} -w_{8(j+m+1)+1 \rightarrow 8(j+m+1)+2} \otimes w_{8j+7 \rightarrow 8(j+1)+3}, & i = 5s + (j + 1)_s; \\ 0, & \text{otherwise.} \end{cases}$$

If  $14s \leq j < 15s$ , then  $b_{ij} = 0$ .

If  $15s \leq j < 16s$ , then

$$b_{ij} = \begin{cases} -e_{8(j+m+1)+4} \otimes w_{8j+7 \rightarrow 8(j+1)+1}, & i = 2s + (j + 1)_s; \\ -w_{8(j+m+1)+1 \rightarrow 8(j+m+1)+4} \otimes w_{8j+7 \rightarrow 8(j+1)+3}, & i = 5s + (j + 1)_s; \\ 0, & \text{otherwise.} \end{cases}$$

If  $16s \leq j < 17s$ , then  $b_{ij} = 0$ .

If  $17s \leq j < 18s$ , then

$$b_{ij} = \begin{cases} -e_{8(j+m+1)+5} \otimes w_{8j+7 \rightarrow 8(j+1)+2}, & i = 3s + (j + 1)_s; \\ 0, & \text{otherwise.} \end{cases}$$

(8) If  $r_0 = 7$ , then  $\Omega^7(Z_t^{(7)})$  is described with  $(14s \times 20s)$  matrix, whose entries  $b_{ij}$  have the following form:

If  $0 \leq j < s$ , then

$$b_{ij} = \begin{cases} -w_{8(j+m)+2 \rightarrow 8(j+m)+7} \otimes e_{8j}, & i = j; \\ w_{8(j+m)+4 \rightarrow 8(j+m)+7} \otimes e_{8j}, & i = j + s; \\ e_{8(j+m)+7} \otimes w_{8j \rightarrow 8j+1}, & i = j + 4s; \\ 0, & \text{otherwise.} \end{cases}$$

If  $s \leq j < 2s$ , then

$$b_{ij} = \begin{cases} -w_{8(j+m)+2 \rightarrow 8(j+m+1)} \otimes e_{8j}, & i = j - s; \\ w_{8(j+m)+4 \rightarrow 8(j+m+1)} \otimes e_{8j}, & i = j; \\ w_{8(j+m)+7 \rightarrow 8(j+m+1)} \otimes w_{8j \rightarrow 8j+1}, & i = j + 3s; \\ e_{8(j+m+1)} \otimes w_{8j \rightarrow 8j+2}, & i = j + 4s; \\ 0, & \text{otherwise.} \end{cases}$$

If  $2s \leq j < 3s$ , then  $b_{ij} = 0$ .

If  $3s \leq j < 4s$ , then

$$b_{ij} = \begin{cases} w_{8(j+m+1)+2 \rightarrow 8(j+m+1)+3} \otimes w_{8j+1 \rightarrow 8(j+1)}, & i = (j+1)s; \\ 0, & \text{otherwise.} \end{cases}$$

If  $4s \leq j < 5s$ , then

$$b_{ij} = \begin{cases} -e_{8(j+m+1)+5} \otimes w_{8j+1 \rightarrow 8(j+1)}, & i = 3s + (j+1)s; \\ 0, & \text{otherwise.} \end{cases}$$

If  $5s \leq j < 6s$ , then

$$b_{ij} = \begin{cases} -w_{8(j+m+1)+2 \rightarrow 8(j+m+1)+4} \otimes w_{8j+2 \rightarrow 8(j+1)}, & i = (j+1)s; \\ e_{8(j+m+1)+4} \otimes w_{8j+2 \rightarrow 8(j+1)}, & i = s + (j+1)s; \\ 0, & \text{otherwise.} \end{cases}$$

If  $6s \leq j < 11s$ , then  $b_{ij} = 0$ .

If  $11s \leq j < 12s$ , then

$$b_{ij} = \begin{cases} e_{8(j+m+1)+6} \otimes w_{8j+5 \rightarrow 8(j+1)}, & i = 2s + (j+1)s; \\ 0, & \text{otherwise.} \end{cases}$$

If  $12s \leq j < 18s$ , then  $b_{ij} = 0$ .

If  $18s \leq j < 19s$ , then

$$b_{ij} = \begin{cases} -w_{8(j+m+1)+7 \rightarrow 8(j+m+2)} \otimes w_{8j+7 \rightarrow 8(j+1)+1}, & i = 4s + (j+1)s; \\ -e_{8(j+m+2)} \otimes w_{8j+7 \rightarrow 8(j+1)+2}, & i = 5s + (j+1)s; \\ 0, & \text{otherwise.} \end{cases}$$

If  $19s \leq j < 20s$ , then

$$b_{ij} = \begin{cases} -e_{8(j+m+1)+7} \otimes w_{8j+7 \rightarrow 8(j+1)+1}, & i = 4s + (j+1)s; \\ 0, & \text{otherwise.} \end{cases}$$

(9) If  $r_0 = 8$ , then  $\Omega^8(Z_t^{(7)})$  is described with  $(16s \times 18s)$  matrix, whose entries  $b_{ij}$  have the following form:

If  $0 \leq j < s$ , then

$$b_{ij} = \begin{cases} -w_{8(j+m)+1 \rightarrow 8(j+m)+3} \otimes w_{8j \rightarrow 8j+2}, & i = j + 5s; \\ -w_{8(j+m)+2 \rightarrow 8(j+m)+3} \otimes w_{8j \rightarrow 8j+3}, & i = j + 6s; \\ 0, & \text{otherwise.} \end{cases}$$

If  $s \leq j < 2s$ , then

$$b_{ij} = \begin{cases} w_{8(j+m)+5 \rightarrow 8(j+m)+6} \otimes w_{8j \rightarrow 8j+1}, & i = j + 2s; \\ -e_{8(j+m)+6} \otimes w_{8j \rightarrow 8j+2}, & i = j + 3s; \\ 0, & \text{otherwise.} \end{cases}$$

If  $2s \leq j < 3s$ , then

$$b_{ij} = \begin{cases} -w_{8(j+m-1)+7 \rightarrow 8(j+m)+4} \otimes e_{8j}, & i = j - 2s; \\ w_{8(j+m-1)+7 \rightarrow 8(j+m)+4} \otimes e_{8j}, & i = j - s; \\ w_{8(j+m)+1 \rightarrow 8(j+m)+4} \otimes w_{8j \rightarrow 8j+2}, & i = j + 3s; \\ w_{8(j+m)+3 \rightarrow 8(j+m)+4} \otimes w_{8j \rightarrow 8j+4}, & i = j + 5s; \\ e_{8(j+m)+4} \otimes w_{8j \rightarrow 8j+6}, & i = j + 10s; \\ 0, & \text{otherwise.} \end{cases}$$

If  $3s \leq j < 4s$ , then  $b_{ij} = 0$ .

If  $4s \leq j < 5s$ , then

$$b_{ij} = \begin{cases} e_{8(j+m)+5} \otimes w_{8j \rightarrow 8j+1}, & i = j - s; \\ 0, & \text{otherwise.} \end{cases}$$

If  $5s \leq j < 6s$ , then

$$b_{ij} = \begin{cases} -e_{8(j+m)+7} \otimes w_{8j+1 \rightarrow 8(j+1)}, & i = s + (j + 1)_s; \\ 0, & \text{otherwise.} \end{cases}$$

If  $6s \leq j < 10s$ , then  $b_{ij} = 0$ .

If  $10s \leq j < 11s$ , then

$$b_{ij} = \begin{cases} e_{8(j+m)+7} \otimes w_{8j+5 \rightarrow 8(j+1)}, & i = (j + 1)_s; \\ -e_{8(j+m)+7} \otimes w_{8j+5 \rightarrow 8(j+1)}, & i = s + (j + 1)_s; \\ 0, & \text{otherwise.} \end{cases}$$

If  $11s \leq j < 12s$ , then

$$b_{ij} = \begin{cases} w_{8(j+m)+7 \rightarrow 8(j+m+1)} \otimes w_{8j+5 \rightarrow 8(j+1)}, & i = (j + 1)_s; \\ -w_{8(j+m)+7 \rightarrow 8(j+m+1)} \otimes w_{8j+5 \rightarrow 8(j+1)}, & i = s + (j + 1)_s; \\ e_{8(j+m+1)} \otimes w_{8j+5 \rightarrow 8(j+1)}, & i = 2s + (j + 1)_s; \\ 0, & \text{otherwise.} \end{cases}$$

If  $12s \leq j < 16s$ , then  $b_{ij} = 0$ .

If  $16s \leq j < 17s$ , then

$$b_{ij} = \begin{cases} -w_{8(j+m+1)+5 \rightarrow 8(j+m+1)+6} \otimes w_{8j+7 \rightarrow 8(j+1)+1}, & i = 3s + (j+1)_s; \\ e_{8(j+m+1)+6} \otimes w_{8j+7 \rightarrow 8(j+1)+2}, & i = 4s + (j+1)_s; \\ 0, & \text{otherwise.} \end{cases}$$

If  $17s \leq j < 18s$ , then

$$b_{ij} = \begin{cases} -e_{8(j+m+1)+5} \otimes w_{8j+7 \rightarrow 8(j+1)+1}, & i = 3s + (j+1)_s; \\ 0, & \text{otherwise.} \end{cases}$$

(10) If  $r_0 = 9$ , then  $\Omega^9(Z_t^{(7)})$  is described with  $(16s \times 19s)$  matrix, whose entries  $b_{ij}$  have the following form:

If  $0 \leq j < s$ , then

$$b_{ij} = \begin{cases} -e_{8(j+m)+7} \otimes w_{8j \rightarrow 8j+2}, & i = j + 5s; \\ 0, & \text{otherwise.} \end{cases}$$

If  $s \leq j < 2s$ , then

$$b_{ij} = \begin{cases} -w_{8(j+m)+3 \rightarrow 8(j+m+1)} \otimes e_{8j}, & i = j; \\ w_{8(j+m)+6 \rightarrow 8(j+m+1)} \otimes e_{8j}, & i = j + s; \\ e_{8(j+m+1)} \otimes w_{8j \rightarrow 8j+1}, & i = j + 3s; \\ -w_{8(j+m)+7 \rightarrow 8(j+m+1)} \otimes w_{8j \rightarrow 8j+5}, & i = j + 7s; \\ 0, & \text{otherwise.} \end{cases}$$

If  $2s \leq j < 3s$ , then

$$b_{ij} = \begin{cases} -w_{8(j+m)+3 \rightarrow 8(j+m)+7} \otimes e_{8j}, & i = j - s; \\ w_{8(j+m)+6 \rightarrow 8(j+m)+7} \otimes e_{8j}, & i = j; \\ -e_{8(j+m)+7} \otimes w_{8j \rightarrow 8j+2}, & i = j + 3s; \\ -e_{8(j+m)+7} \otimes w_{8j \rightarrow 8j+5}, & i = j + 6s; \\ 0, & \text{otherwise.} \end{cases}$$

If  $3s \leq j < 4s$ , then

$$b_{ij} = \begin{cases} w_{8(j+m+1)+3 \rightarrow 8(j+m+1)+4} \otimes w_{8j+1 \rightarrow 8(j+1)}, & i = s + (j+1)_s; \\ 0, & \text{otherwise.} \end{cases}$$

If  $4s \leq j < 5s$ , then

$$b_{ij} = \begin{cases} -e_{8(j+m+1)+6} \otimes w_{8j+1 \rightarrow 8(j+1)}, & i = 2s + (j+1)_s; \\ 0, & \text{otherwise.} \end{cases}$$

If  $5s \leq j < 10s$ , then  $b_{ij} = 0$ .

If  $10s \leq j < 11s$ , then

$$b_{ij} = \begin{cases} w_{8(j+m+1)+1 \rightarrow 8(j+m+1)+2} \otimes w_{8j+5 \rightarrow 8(j+1)}, & i = 3s + (j+1)_s; \\ 0, & \text{otherwise.} \end{cases}$$

If  $11s \leq j < 12s$ , then

$$b_{ij} = \begin{cases} w_{8(j+m+1)+1 \rightarrow 8(j+m+1)+4} \otimes w_{8j+5 \rightarrow 8(j+1)}, & i = 3s + (j+1)_s; \\ 0, & \text{otherwise.} \end{cases}$$

If  $12s \leq j < 13s$ , then

$$b_{ij} = \begin{cases} e_{8(j+m+1)+5} \otimes w_{8j+5 \rightarrow 8(j+1)}, & i = (j+1)_s; \\ 0, & \text{otherwise.} \end{cases}$$

If  $13s \leq j < 16s$ , then  $b_{ij} = 0$ .

If  $16s \leq j < 17s$ , then

$$b_{ij} = \begin{cases} -e_{8(j+m+1)+7} \otimes w_{8j+7 \rightarrow 8(j+1)+2}, & i = 5s + (j+1)_s; \\ 0, & \text{otherwise.} \end{cases}$$

If  $17s \leq j < 18s$ , then  $b_{ij} = 0$ .

If  $18s \leq j < 19s$ , then

$$b_{ij} = \begin{cases} -e_{8(j+m+2)} \otimes w_{8j+7 \rightarrow 8(j+1)+1}, & i = 4s + (j+1)_s; \\ 0, & \text{otherwise.} \end{cases}$$

(11) If  $r_0 = 10$ , then  $\Omega^{10}(Z_t^{(7)})$  is described with  $(19s \times 18s)$  matrix, whose entries  $b_{ij}$  have the following form:

If  $0 \leq j < s$ , then

$$b_{ij} = \begin{cases} -w_{8(j+m)+1 \rightarrow 8(j+m)+2} \otimes w_{8j \rightarrow 8j+1}, & i = j + 4s; \\ 0, & \text{otherwise.} \end{cases}$$

If  $s \leq j < 2s$ , then

$$b_{ij} = \begin{cases} w_{8(j+m)+2 \rightarrow 8(j+m)+4} \otimes w_{8j \rightarrow 8j+2}, & i = j + 4s; \\ -w_{8(j+m)+3 \rightarrow 8(j+m)+4} \otimes w_{8j \rightarrow 8j+3}, & i = j + 5s; \\ 0, & \text{otherwise.} \end{cases}$$

If  $2s \leq j < 3s$ , then

$$b_{ij} = \begin{cases} w_{8(j+m) \rightarrow 8(j+m)+6} \otimes e_{8j}, & i = j; \\ -e_{8(j+m)+6} \otimes w_{8j \rightarrow 8j+1}, & i = j + s; \\ -w_{8(j+m)+5 \rightarrow 8(j+m)+6} \otimes w_{8j \rightarrow 8j+5}, & i = j + 8s; \\ 0, & \text{otherwise.} \end{cases}$$

If  $3s \leq j < 4s$ , then

$$b_{ij} = \begin{cases} w_{8(j+m) \rightarrow 8(j+m)+5} \otimes e_{8j}, & i = j - s; \\ -e_{8(j+m)+5} \otimes w_{8j \rightarrow 8j+5}, & i = j + 7s; \\ 0, & \text{otherwise.} \end{cases}$$

If  $4s \leq j < 5s$ , then  $b_{ij} = 0$ .

If  $5s \leq j < 6s$ , then

$$b_{ij} = \begin{cases} -e_{8(j+m+1)} \otimes w_{8j+1 \rightarrow 8(j+1)}, & i = 2s + (j+1)_s; \\ 0, & \text{otherwise.} \end{cases}$$

If  $6s \leq j < 9s$ , then  $b_{ij} = 0$ .

If  $9s \leq j < 10s$ , then

$$b_{ij} = \begin{cases} e_{8(j+m+1)} \otimes w_{8j+5 \rightarrow 8(j+1)}, & i = s + (j+1)_s; \\ -e_{8(j+m+1)} \otimes w_{8j+5 \rightarrow 8(j+1)}, & i = 2s + (j+1)_s; \\ 0, & \text{otherwise.} \end{cases}$$

If  $10s \leq j < 11s$ , then

$$b_{ij} = \begin{cases} -e_{8(j+m)+7} \otimes w_{8j+5 \rightarrow 8(j+1)}, & i = (j+1)_s; \\ 0, & \text{otherwise.} \end{cases}$$

If  $11s \leq j < 13s$ , then  $b_{ij} = 0$ .

If  $13s \leq j < 14s$ , then

$$b_{ij} = \begin{cases} w_{8(j+m+1)+1 \rightarrow 8(j+m+1)+3} \otimes w_{8j+7 \rightarrow 8(j+1)+1}, & i = 4s + (j+1)_s; \\ 0, & \text{otherwise.} \end{cases}$$

If  $14s \leq j < 15s$ , then

$$b_{ij} = \begin{cases} -e_{8(j+m+1)+6} \otimes w_{8j+7 \rightarrow 8(j+1)+1}, & i = 3s + (j+1)_s; \\ 0, & \text{otherwise.} \end{cases}$$

If  $15s \leq j < 16s$ , then  $b_{ij} = 0$ .

If  $16s \leq j < 17s$ , then

$$b_{ij} = \begin{cases} e_{8(j+m+1)+1} \otimes w_{8j+7 \rightarrow 8(j+1)+1}, & i = 4s + (j+1)_s; \\ 0, & \text{otherwise.} \end{cases}$$

If  $17s \leq j < 18s$ , then  $b_{ij} = 0$ .

(12) If  $r_0 = 11$ , then  $\Omega^{11}(Z_t^{(7)})$  is described with  $(18s \times 19s)$  matrix, whose entries  $b_{ij}$  have the following form:

If  $0 \leq j < s$ , then

$$b_{ij} = \begin{cases} e_{8(j+m)+7} \otimes w_{8j \rightarrow 8j+1}, & i = j + 5s; \\ 0, & \text{otherwise.} \end{cases}$$

If  $s \leq j < 2s$ , then

$$b_{ij} = \begin{cases} -e_{8(j+m+1)} \otimes w_{8j \rightarrow 8j+2}, & i = j + 5s; \\ 0, & \text{otherwise.} \end{cases}$$



If  $2s \leq j < 3s$ , then

$$b_{ij} = \begin{cases} w_{8(j+m)+1 \rightarrow 8(j+m+1)} \otimes e_{8j}, & i = j + s; \\ -w_{8(j+m)+7 \rightarrow 8(j+m+1)} \otimes w_{8j \rightarrow 8j+1}, & i = j + 3s; \\ -e_{8(j+m+1)} \otimes w_{8j \rightarrow 8j+2}, & i = j + 4s; \\ -w_{8(j+m)+7 \rightarrow 8(j+m+1)} \otimes w_{8j \rightarrow 8j+5}, & i = j + 8s; \\ -e_{8(j+m+1)} \otimes w_{8j \rightarrow 8j+5}, & i = j + 9s; \\ 0, & \text{otherwise.} \end{cases}$$

If  $3s \leq j < 4s$ , then  $b_{ij} = 0$ .

If  $4s \leq j < 5s$ , then

$$b_{ij} = \begin{cases} e_{8(j+m+1)+1} \otimes w_{8j+1 \rightarrow 8(j+1)}, & i = 3s + (j + 1)_s; \\ 0, & \text{otherwise.} \end{cases}$$

If  $5s \leq j < 10s$ , then  $b_{ij} = 0$ .

If  $10s \leq j < 11s$ , then

$$b_{ij} = \begin{cases} -w_{8(j+m+1)+2 \rightarrow 8(j+m+1)+3} \otimes w_{8j+5 \rightarrow 8(j+1)}, & i = (j + 1)_s; \\ w_{8(j+m+1)+1 \rightarrow 8(j+m+1)+3} \otimes w_{8j+5 \rightarrow 8(j+1)}, & i = 3s + (j + 1)_s; \\ 0, & \text{otherwise.} \end{cases}$$

If  $11s \leq j < 12s$ , then

$$b_{ij} = \begin{cases} -e_{8(j+m+1)+6} \otimes w_{8j+5 \rightarrow 8(j+1)}, & i = s + (j + 1)_s; \\ 0, & \text{otherwise.} \end{cases}$$

If  $12s \leq j < 13s$ , then

$$b_{ij} = \begin{cases} e_{8(j+m+1)+5} \otimes w_{8j+5 \rightarrow 8(j+1)}, & i = 4s + (j + 1)_s; \\ 0, & \text{otherwise.} \end{cases}$$

If  $13s \leq j < 16s$ , then  $b_{ij} = 0$ .

If  $16s \leq j < 17s$ , then

$$b_{ij} = \begin{cases} -e_{8(j+m+1)+7} \otimes w_{8j+7 \rightarrow 8(j+1)+1}, & i = 5s + (j + 1)_s; \\ 0, & \text{otherwise.} \end{cases}$$

If  $17s \leq j < 18s$ , then

$$b_{ij} = \begin{cases} -e_{8(j+m+2)} \otimes w_{8j+7 \rightarrow 8(j+1)+2}, & i = 6s + (j + 1)_s; \\ 0, & \text{otherwise.} \end{cases}$$

If  $18s \leq j < 19s$ , then  $b_{ij} = 0$ .

(13) If  $r_0 = 12$ , then  $\Omega^{12}(Z_t^{(7)})$  is described with  $(19s \times 16s)$  matrix, whose entries  $b_{ij}$  have the following form:

If  $0 \leq j < s$ , then

$$b_{ij} = \begin{cases} w_{8(j+m)+2 \rightarrow 8(j+m)+3} \otimes w_{8j \rightarrow 8j+1}, & i = j + 3s; \\ 0, & \text{otherwise.} \end{cases}$$

If  $s \leq j < 2s$ , then

$$b_{ij} = \begin{cases} w_{8(j+m) \rightarrow 8(j+m)+6} \otimes e_{8j}, & i = j; \\ w_{8(j+m)+5 \rightarrow 8(j+m)+6} \otimes w_{8j \rightarrow 8j+4}, & i = j + 7s; \\ -e_{8(j+m)+6} \otimes w_{8j \rightarrow 8j+5}, & i = j + 10s; \\ 0, & \text{otherwise.} \end{cases}$$

If  $2s \leq j < 3s$ , then

$$b_{ij} = \begin{cases} w_{8(j+m-1)+7 \rightarrow 8(j+m)+1} \otimes e_{8j}, & i = j - 2s; \\ -w_{8(j+m) \rightarrow 8(j+m)+1} \otimes e_{8j}, & i = j - s; \\ -w_{8(j+m-1)+7 \rightarrow 8(j+m)+1} \otimes e_{8j}, & i = j; \\ -e_{8(j+m)+1} \otimes w_{8j \rightarrow 8j+4}, & i = j + 7s; \\ e_{8(j+m)+1} \otimes w_{8j \rightarrow 8j+6}, & i = j + 13s; \\ 0, & \text{otherwise.} \end{cases}$$

If  $3s \leq j < 4s$ , then

$$b_{ij} = \begin{cases} -e_{8(j+m)+5} \otimes w_{8j \rightarrow 8j+2}, & i = j + 2s; \\ 0, & \text{otherwise.} \end{cases}$$

If  $4s \leq j < 8s$ , then  $b_{ij} = 0$ .

If  $8s \leq j < 9s$ , then

$$b_{ij} = \begin{cases} e_{8(j+m)+7} \otimes w_{8j+5 \rightarrow 8(j+1)}, & i = (j+1)_s; \\ 0, & \text{otherwise.} \end{cases}$$

If  $9s \leq j < 10s$ , then

$$b_{ij} = \begin{cases} w_{8(j+m)+7 \rightarrow 8(j+m+1)} \otimes w_{8j+5 \rightarrow 8(j+1)}, & i = (j+1)_s; \\ -e_{8(j+m+1)} \otimes w_{8j+5 \rightarrow 8(j+1)}, & i = s + (j+1)_s; \\ -w_{8(j+m)+7 \rightarrow 8(j+m+1)} \otimes w_{8j+5 \rightarrow 8(j+1)}, & i = 2s + (j+1)_s; \\ 0, & \text{otherwise.} \end{cases}$$

If  $10s \leq j < 12s$ , then  $b_{ij} = 0$ .

If  $12s \leq j < 13s$ , then

$$b_{ij} = \begin{cases} e_{8(j+m+1)+2} \otimes w_{8j+7 \rightarrow 8(j+1)+1}, & i = 3s + (j+1)_s; \\ 0, & \text{otherwise.} \end{cases}$$

If  $13s \leq j < 15s$ , then  $b_{ij} = 0$ .

If  $15s \leq j < 16s$ , then

$$b_{ij} = \begin{cases} -e_{8(j+m+1)+5} \otimes w_{8j+7 \rightarrow 8(j+1)+2}, & i = 5s + (j+1)_s; \\ 0, & \text{otherwise.} \end{cases}$$

(14) If  $r_0 = 13$ , then  $\Omega^{13}(Z_t^{(7)})$  is described with  $(18s \times 16s)$  matrix, whose entries  $b_{ij}$  have the following form:

If  $0 \leq j < s$ , then

$$b_{ij} = \begin{cases} w_{8(j+m)+2 \rightarrow 8(j+m)+7} \otimes e_{8j}, & i = j; \\ w_{8(j+m)+5 \rightarrow 8(j+m)+7} \otimes e_{8j}, & i = j + 3s; \\ e_{8(j+m)+7} \otimes w_{8j \rightarrow 8j+5}, & i = j + 9s; \\ 0, & \text{otherwise.} \end{cases}$$

If  $s \leq j < 2s$ , then

$$b_{ij} = \begin{cases} e_{8(j+m+1)} \otimes w_{8j \rightarrow 8j+1}, & i = j + 3s; \\ 0, & \text{otherwise.} \end{cases}$$

If  $2s \leq j < 3s$ , then

$$b_{ij} = \begin{cases} e_{8(j+m+1)+2} \otimes w_{8j+1 \rightarrow 8(j+1)}, & i = (j+1)_s; \\ 0, & \text{otherwise.} \end{cases}$$

If  $3s \leq j < 4s$ , then

$$b_{ij} = \begin{cases} w_{8(j+m+1)+5 \rightarrow 8(j+m+1)+6} \otimes w_{8j+1 \rightarrow 8(j+1)}, & i = 3s + (j+1)_s; \\ 0, & \text{otherwise.} \end{cases}$$

If  $4s \leq j < 8s$ , then  $b_{ij} = 0$ .

If  $8s \leq j < 9s$ , then

$$b_{ij} = \begin{cases} e_{8(j+m+1)+6} \otimes w_{8j+5 \rightarrow 8(j+1)}, & i = 2s + (j+1)_s; \\ 0, & \text{otherwise.} \end{cases}$$

If  $9s \leq j < 10s$ , then

$$b_{ij} = \begin{cases} -w_{8(j+m+1)+3 \rightarrow 8(j+m+1)+4} \otimes w_{8j+5 \rightarrow 8(j+1)}, & i = s + (j+1)_s; \\ 0, & \text{otherwise.} \end{cases}$$

If  $10s \leq j < 13s$ , then  $b_{ij} = 0$ .

If  $13s \leq j < 14s$ , then

$$b_{ij} = \begin{cases} -w_{8(j+m+1)+2 \rightarrow 8(j+m+1)+7} \otimes w_{8j+7 \rightarrow 8(j+1)}, & i = (j+1)_s; \\ -w_{8(j+m+1)+5 \rightarrow 8(j+m+1)+7} \otimes w_{8j+7 \rightarrow 8(j+1)}, & i = 3s + (j+1)_s; \\ -e_{8(j+m+1)+7} \otimes w_{8j+7 \rightarrow 8(j+1)+5}, & i = 9s + (j+1)_s; \\ 0, & \text{otherwise.} \end{cases}$$

If  $14s \leq j < 15s$ , then

$$b_{ij} = \begin{cases} -w_{8(j+m+1)+2 \rightarrow 8(j+m+2)} \otimes w_{8j+7 \rightarrow 8(j+1)}, & i = (j+1)_s; \\ -w_{8(j+m+1)+5 \rightarrow 8(j+m+2)} \otimes w_{8j+7 \rightarrow 8(j+1)}, & i = 3s + (j+1)_s; \\ -e_{8(j+m+2)} \otimes w_{8j+7 \rightarrow 8(j+1)+1}, & i = 4s + (j+1)_s; \\ -w_{8(j+m+1)+7 \rightarrow 8(j+m+2)} \otimes w_{8j+7 \rightarrow 8(j+1)+5}, & i = 9s + (j+1)_s; \\ 0, & \text{otherwise.} \end{cases}$$

If  $15s \leq j < 16s$ , then  $b_{ij} = 0$ .

(15) If  $r_0 = 14$ , then  $\Omega^{14}(Z_t^{(7)})$  is described with  $(20s \times 14s)$  matrix, whose entries  $b_{ij}$  have the following form:

If  $0 \leq j < s$ , then

$$b_{ij} = \begin{cases} -w_{8(j+m-1)+7 \rightarrow 8(j+m)+2} \otimes e_{8j}, & i = j; \\ -w_{8(j+m) \rightarrow 8(j+m)+2} \otimes e_{8j}, & i = j + s; \\ -w_{8(j+m)+1 \rightarrow 8(j+m)+2} \otimes w_{8j \rightarrow 8j+3}, & i = j + 8s; \\ -e_{8(j+m)+2} \otimes w_{8j \rightarrow 8j+4}, & i = j + 9s; \\ e_{8(j+m)+2} \otimes w_{8j \rightarrow 8j+6}, & i = j + 14s; \\ 0, & \text{otherwise.} \end{cases}$$

If  $s \leq j < 2s$ , then

$$b_{ij} = \begin{cases} w_{8(j+m)+3 \rightarrow 8(j+m)+4} \otimes w_{8j \rightarrow 8j+1}, & i = j + 2s; \\ 0, & \text{otherwise.} \end{cases}$$

If  $2s \leq j < 3s$ , then

$$b_{ij} = \begin{cases} -w_{8(j+m)+5 \rightarrow 8(j+m)+6} \otimes w_{8j \rightarrow 8j+1}, & i = j + 2s; \\ -e_{8(j+m)+6} \otimes w_{8j \rightarrow 8j+2}, & i = j + 4s; \\ 0, & \text{otherwise.} \end{cases}$$

If  $3s \leq j < 7s$ , then  $b_{ij} = 0$ .

If  $7s \leq j < 8s$ , then

$$b_{ij} = \begin{cases} -e_{8(j+m)+7} \otimes w_{8j+5 \rightarrow 8(j+1)}, & i = (j+1)_s; \\ 0, & \text{otherwise.} \end{cases}$$

If  $8s \leq j < 9s$ , then

$$b_{ij} = \begin{cases} e_{8(j+m+1)} \otimes w_{8j+5 \rightarrow 8(j+1)}, & i = s + (j+1)_s; \\ 0, & \text{otherwise.} \end{cases}$$

If  $9s \leq j < 10s$ , then  $b_{ij} = 0$ .

If  $10s \leq j < 11s$ , then

$$b_{ij} = \begin{cases} e_{8(j+m+1)+3} \otimes w_{8j+7 \rightarrow 8(j+1)+1}, & i = 3s + (j+1)_s; \\ 0, & \text{otherwise.} \end{cases}$$

If  $11s \leq j < 14s$ , then  $b_{ij} = 0$ .

(16) If  $r_0 = 15$ , then  $\Omega^{15}(Z_t^{(7)})$  is described with  $(18s \times 13s)$  matrix, whose entries  $b_{ij}$  have the following form:

If  $0 \leq j < s$ , then

$$b_{ij} = \begin{cases} w_{8(j+m)+3 \rightarrow 8(j+m+1)} \otimes e_{8j}, & i = j; \\ e_{8(j+m+1)} \otimes w_{8j \rightarrow 8j+5}, & i = j + 11s; \\ 0, & \text{otherwise.} \end{cases}$$

If  $s \leq j < 2s$ , then

$$b_{ij} = \begin{cases} e_{8(j+m)+7} \otimes w_{8j \rightarrow 8j+1}, & i = j + 4s; \\ 0, & \text{otherwise.} \end{cases}$$

If  $2s \leq j < 3s$ , then

$$b_{ij} = \begin{cases} e_{8(j+m+1)+3} \otimes w_{8j+1 \rightarrow 8(j+1)}, & i = (j+1)_s; \\ 0, & \text{otherwise.} \end{cases}$$

If  $3s \leq j < 8s$ , then  $b_{ij} = 0$ .

If  $8s \leq j < 9s$ , then

$$b_{ij} = \begin{cases} e_{8(j+m+1)+5} \otimes w_{8j+5 \rightarrow 8(j+1)}, & i = 4s + (j+1)_s; \\ 0, & \text{otherwise.} \end{cases}$$

If  $9s \leq j < 11s$ , then  $b_{ij} = 0$ .

If  $11s \leq j < 12s$ , then

$$b_{ij} = \begin{cases} -e_{8(j+m+1)+7} \otimes w_{8j+7 \rightarrow 8(j+1)+1}, & i = 5s + (j+1)_s; \\ 0, & \text{otherwise.} \end{cases}$$

If  $12s \leq j < 13s$ , then

$$b_{ij} = \begin{cases} -w_{8(j+m+1)+3 \rightarrow 8(j+m+2)} \otimes w_{8j+7 \rightarrow 8(j+1)}, & i = (j+1)_s; \\ -e_{8(j+m+2)} \otimes w_{8j+7 \rightarrow 8(j+1)+5}, & i = 11s + (j+1)_s; \\ 0, & \text{otherwise.} \end{cases}$$

(17) If  $r_0 = 16$ , then  $\Omega^{16}(Z_t^{(7)})$  is described with  $(19s \times 11s)$  matrix, whose entries  $b_{ij}$  have the following form:

If  $0 \leq j < s$ , then

$$b_{ij} = \begin{cases} -w_{8(j+m) \rightarrow 8(j+m)+3} \otimes e_{8j}, & i = j + s; \\ -w_{8(j+m-1)+7 \rightarrow 8(j+m)+3} \otimes e_{8j}, & i = j + 2s; \\ w_{8(j+m)+1 \rightarrow 8(j+m)+3} \otimes w_{8j \rightarrow 8j+2}, & i = j + 6s; \\ w_{8(j+m)+2 \rightarrow 8(j+m)+3} \otimes w_{8j \rightarrow 8j+3}, & i = j + 7s; \\ -e_{8(j+m)+3} \otimes w_{8j \rightarrow 8j+4}, & i = j + 9s; \\ e_{8(j+m)+3} \otimes w_{8j \rightarrow 8j+6}, & i = j + 13s; \\ 0, & \text{otherwise.} \end{cases}$$

If  $s \leq j < 2s$ , then

$$b_{ij} = \begin{cases} e_{8(j+m)+5} \otimes w_{8j \rightarrow 8j+5}, & i = j + 11s; \\ 0, & \text{otherwise.} \end{cases}$$

If  $2s \leq j < 6s$ , then  $b_{ij} = 0$ .

If  $6s \leq j < 7s$ , then

$$b_{ij} = \begin{cases} -e_{8(j+m+1)} \otimes w_{8j+5 \rightarrow 8(j+1)}, & i = s + (j+1)_s; \\ -w_{8(j+m)+7 \rightarrow 8(j+m+1)} \otimes w_{8j+5 \rightarrow 8(j+1)}, & i = 2s + (j+1)_s; \\ 0, & \text{otherwise.} \end{cases}$$

If  $7s \leq j < 9s$ , then  $b_{ij} = 0$ .

If  $9s \leq j < 10s$ , then

$$b_{ij} = \begin{cases} e_{8(j+m+1)+4} \otimes w_{8j+7 \rightarrow 8(j+1)+1}, & i = 3s + (j+1)_s; \\ 0, & \text{otherwise.} \end{cases}$$

If  $10s \leq j < 11s$ , then

$$b_{ij} = \begin{cases} w_{8(j+m+1)+5 \rightarrow 8(j+m+1)+6} \otimes w_{8j+7 \rightarrow 8(j+1)+5}, & i = 12s + (j+1)_s; \\ 0, & \text{otherwise.} \end{cases}$$

(18) If  $r_0 = 17$ , then  $\Omega^{17}(Z_t^{(7)})$  is described with  $(18s \times 11s)$  matrix, whose entries  $b_{ij}$  have the following form:

If  $0 \leq j < s$ , then

$$b_{ij} = \begin{cases} w_{8(j+m)+2 \rightarrow 8(j+m+1)} \otimes e_{8j}, & i = j; \\ -w_{8(j+m)+4 \rightarrow 8(j+m+1)} \otimes e_{8j}, & i = j + s; \\ -w_{8(j+m)+7 \rightarrow 8(j+m+1)} \otimes w_{8j \rightarrow 8j+1}, & i = j + 4s; \\ -e_{8(j+m+1)} \otimes w_{8j \rightarrow 8j+1}, & i = j + 5s; \\ -w_{8(j+m)+7 \rightarrow 8(j+m+1)} \otimes w_{8j \rightarrow 8j+5}, & i = j + 10s; \\ 0, & \text{otherwise.} \end{cases}$$

If  $s \leq j < 2s$ , then

$$b_{ij} = \begin{cases} -w_{8(j+m+1)+2 \rightarrow 8(j+m+1)+4} \otimes w_{8j+1 \rightarrow 8(j+1)}, & i = (j+1)_s; \\ e_{8(j+m+1)+4} \otimes w_{8j+1 \rightarrow 8(j+1)}, & i = s + (j+1)_s; \\ 0, & \text{otherwise.} \end{cases}$$

If  $2s \leq j < 7s$ , then  $b_{ij} = 0$ .

If  $7s \leq j < 8s$ , then

$$b_{ij} = \begin{cases} e_{8(j+m+1)+6} \otimes w_{8j+5 \rightarrow 8(j+1)}, & i = 2s + (j+1)_s; \\ w_{8(j+m+1)+5 \rightarrow 8(j+m+1)+6} \otimes w_{8j+5 \rightarrow 8(j+1)}, & i = 3s + (j+1)_s; \\ 0, & \text{otherwise.} \end{cases}$$

If  $8s \leq j < 9s$ , then  $b_{ij} = 0$ .

If  $9s \leq j < 10s$ , then

$$b_{ij} = \begin{cases} -w_{8(j+m+1)+7 \rightarrow 8(j+m+2)} \otimes w_{8j+7 \rightarrow 8(j+1)+1}, & i = 4s + (j+1)_s; \\ -e_{8(j+m+2)} \otimes w_{8j+7 \rightarrow 8(j+1)+1}, & i = 5s + (j+1)_s; \\ 0, & \text{otherwise.} \end{cases}$$

If  $10s \leq j < 11s$ , then

$$b_{ij} = \begin{cases} w_{8(j+m+1)+2 \rightarrow 8(j+m+1)+7} \otimes w_{8j+7 \rightarrow 8(j+1)}, & i = (j+1)_s; \\ -w_{8(j+m+1)+4 \rightarrow 8(j+m+1)+7} \otimes w_{8j+7 \rightarrow 8(j+1)}, & i = s + (j+1)_s; \\ -e_{8(j+m+1)+7} \otimes w_{8j+7 \rightarrow 8(j+1)+5}, & i = 10s + (j+1)_s; \\ 0, & \text{otherwise.} \end{cases}$$

(19) If  $r_0 = 18$ , then  $\Omega^{18}(Z_t^{(7)})$  is described with  $(19s \times 10s)$  matrix, whose entries  $b_{ij}$  have the following form:

If  $0 \leq j < s$ , then

$$b_{ij} = \begin{cases} w_{8(j+m-1)+7 \rightarrow 8(j+m)+4} \otimes e_{8j}, & i = j; \\ -w_{8(j+m)+1 \rightarrow 8(j+m)+4} \otimes w_{8j \rightarrow 8j+1}, & i = j + 4s; \\ -w_{8(j+m)+2 \rightarrow 8(j+m)+4} \otimes w_{8j \rightarrow 8j+2}, & i = j + 5s; \\ w_{8(j+m)+3 \rightarrow 8(j+m)+4} \otimes w_{8j \rightarrow 8j+3}, & i = j + 7s; \\ -e_{8(j+m)+4} \otimes w_{8j \rightarrow 8j+4}, & i = j + 8s; \\ e_{8(j+m)+4} \otimes w_{8j \rightarrow 8j+6}, & i = j + 14s; \\ 0, & \text{otherwise.} \end{cases}$$

If  $s \leq j < 2s$ , then

$$b_{ij} = \begin{cases} w_{8(j+m)+5 \rightarrow 8(j+m)+6} \otimes w_{8j \rightarrow 8j+1}, & i = j + 2s; \\ e_{8(j+m)+6} \otimes w_{8j \rightarrow 8j+5}, & i = j + 10s; \\ 0, & \text{otherwise.} \end{cases}$$

If  $2s \leq j < 6s$ , then  $b_{ij} = 0$ .

If  $6s \leq j < 7s$ , then

$$b_{ij} = \begin{cases} e_{8(j+m)+7} \otimes w_{8j+5 \rightarrow 8(j+1)}, & i = (j+1)_s; \\ 0, & \text{otherwise.} \end{cases}$$

If  $7s \leq j < 9s$ , then  $b_{ij} = 0$ .

If  $9s \leq j < 10s$ , then

$$b_{ij} = \begin{cases} -e_{8(j+m+1)+5} \otimes w_{8j+7 \rightarrow 8(j+1)+1}, & i = 3s + (j+1)_s; \\ 0, & \text{otherwise.} \end{cases}$$

(20) If  $r_0 = 19$ , then  $\Omega^{19}(Z_t^{(7)})$  is described with  $(16s \times 8s)$  matrix, whose entries  $b_{ij}$  have the following form:

If  $0 \leq j < s$ , then

$$b_{ij} = \begin{cases} w_{8(j+m)+6 \rightarrow 8(j+m)+7} \otimes e_{8j}, & i = j + s; \\ w_{8(j+m)+1 \rightarrow 8(j+m)+7} \otimes e_{8j}, & i = j + 2s; \\ -e_{8(j+m)+7} \otimes w_{8j \rightarrow 8j+2}, & i = j + 5s; \\ -e_{8(j+m)+7} \otimes w_{8j \rightarrow 8j+4}, & i = j + 7s; \\ -e_{8(j+m)+7} \otimes w_{8j \rightarrow 8j+6}, & i = j + 10s; \\ 0, & \text{otherwise.} \end{cases}$$

If  $s \leq j < 7s$ , then  $b_{ij} = 0$ .

If  $7s \leq j < 8s$ , then

$$b_{ij} = \begin{cases} -w_{8(j+m+1)+6 \rightarrow 8(j+m+2)} \otimes w_{8j+7 \rightarrow 8(j+1)}, & i = s + (j+1)_s; \\ -w_{8(j+m+1)+1 \rightarrow 8(j+m+2)} \otimes w_{8j+7 \rightarrow 8(j+1)}, & i = 2s + (j+1)_s; \\ w_{8(j+m+1)+7 \rightarrow 8(j+m+2)} \otimes w_{8j+7 \rightarrow 8(j+1)+2}, & i = 5s + (j+1)_s; \\ w_{8(j+m+1)+7 \rightarrow 8(j+m+2)} \otimes w_{8j+7 \rightarrow 8(j+1)+4}, & i = 7s + (j+1)_s; \\ e_{8(j+m+2)} \otimes w_{8j+7 \rightarrow 8(j+1)+5}, & i = 9s + (j+1)_s; \\ w_{8(j+m+1)+7 \rightarrow 8(j+m+2)} \otimes w_{8j+7 \rightarrow 8(j+1)+6}, & i = 10s + (j+1)_s; \\ 0, & \text{otherwise.} \end{cases}$$

(21) If  $r_0 = 20$ , then  $\Omega^{20}(Z_t^{(7)})$  is described with  $(16s \times 9s)$  matrix, whose entries  $b_{ij}$  have the following form:

If  $0 \leq j < s$ , then

$$b_{ij} = \begin{cases} w_{8(j+m-1)+7 \rightarrow 8(j+m)+7} \otimes e_{8j}, & i = j; \\ w_{8(j+m)+6 \rightarrow 8(j+m)+7} \otimes w_{8j \rightarrow 8j+4}, & i = j + 7s; \\ w_{8(j+m)+6 \rightarrow 8(j+m)+7} \otimes w_{8j \rightarrow 8j+5}, & i = j + 8s; \\ -w_{8(j+m)+1 \rightarrow 8(j+m)+7} \otimes w_{8j \rightarrow 8j+5}, & i = j + 10s; \\ 0, & \text{otherwise.} \end{cases}$$

If  $s \leq j < 5s$ , then  $b_{ij} = 0$ .

If  $5s \leq j < 6s$ , then

$$b_{ij} = \begin{cases} -w_{8(j+m)+7 \rightarrow 8(j+m+1)} \otimes w_{8j+5 \rightarrow 8(j+1)}, & i = (j+1)_s; \\ e_{8(j+m+1)} \otimes w_{8j+5 \rightarrow 8(j+1)}, & i = s + (j+1)_s; \\ 0, & \text{otherwise.} \end{cases}$$

If  $6s \leq j < 7s$ , then

$$b_{ij} = \begin{cases} w_{8(j+m)+7 \rightarrow 8(j+m+1)+5} \otimes w_{8j+6 \rightarrow 8(j+1)}, & i = (j+1)_s; \\ -w_{8(j+m+1) \rightarrow 8(j+m+1)+5} \otimes w_{8j+6 \rightarrow 8(j+1)}, & i = s + (j+1)_s; \\ -e_{8(j+m+1)+5} \otimes w_{8j+6 \rightarrow 8(j+1)+6}, & i = 12s + (j+1)_s; \\ 0, & \text{otherwise.} \end{cases}$$

If  $7s \leq j < 8s$ , then

$$b_{ij} = \begin{cases} w_{8(j+m+1)+1 \rightarrow 8(j+m+1)+4} \otimes w_{8j+7 \rightarrow 8(j+1)+5}, & i = 10s + (j+1)_s; \\ 0, & \text{otherwise.} \end{cases}$$

If  $8s \leq j < 9s$ , then

$$b_{ij} = \begin{cases} -w_{8(j+m)+7 \rightarrow 8(j+m+1)+6} \otimes w_{8j+7 \rightarrow 8(j+1)}, & i = (j+1)_s; \\ -e_{8(j+m+1)+6} \otimes w_{8j+7 \rightarrow 8(j+1)+4}, & i = 7s + (j+1)_s; \\ -e_{8(j+m+1)+6} \otimes w_{8j+7 \rightarrow 8(j+1)+5}, & i = 8s + (j+1)_s; \\ 0, & \text{otherwise.} \end{cases}$$

(22) If  $r_0 = 21$ , then  $\Omega^{21}(Z_t^{(7)})$  is described with  $(14s \times 8s)$  matrix, whose entries  $b_{ij}$  have the following form:



If  $0 \leq j < s$ , then

$$b_{ij} = \begin{cases} -w_{8(j+m)+2 \rightarrow 8(j+m+1)} \otimes e_{8j}, & i = j; \\ -w_{8(j+m)+6 \rightarrow 8(j+m+1)} \otimes e_{8j}, & i = j + 2s; \\ -w_{8(j+m)+7 \rightarrow 8(j+m+1)} \otimes w_{8j \rightarrow 8j+1}, & i = j + 3s; \\ -e_{8(j+m+1)} \otimes w_{8j \rightarrow 8j+2}, & i = j + 4s; \\ -w_{8(j+m)+7 \rightarrow 8(j+m+1)} \otimes w_{8j \rightarrow 8j+3}, & i = j + 5s; \\ -e_{8(j+m+1)} \otimes w_{8j \rightarrow 8j+4}, & i = j + 6s; \\ -e_{8(j+m+1)} \otimes w_{8j \rightarrow 8j+6}, & i = j + 9s; \\ 0, & \text{otherwise.} \end{cases}$$

If  $s \leq j < 6s$ , then  $b_{ij} = 0$ .

If  $6s \leq j < 7s$ , then

$$b_{ij} = \begin{cases} e_{8(j+m+1)+6} \otimes w_{8j+6 \rightarrow 8(j+1)}, & i = 2s + (j+1)_s; \\ 0, & \text{otherwise.} \end{cases}$$

If  $7s \leq j < 8s$ , then  $b_{ij} = 0$ .

(23) If  $r_0 = 22$ , then  $\Omega^{22}(Z_t^{(7)})$  is described with  $(13s \times 8s)$  matrix, whose entries  $b_{ij}$  have the following form:

If  $0 \leq j < s$ , then

$$b_{ij} = \begin{cases} w_{8(j+m) \rightarrow 8(j+m+1)} \otimes e_{8j}, & i = j; \\ w_{8(j+m)+1 \rightarrow 8(j+m+1)} \otimes w_{8j \rightarrow 8j+4}, & i = j + 6s; \\ w_{8(j+m)+2 \rightarrow 8(j+m+1)} \otimes w_{8j \rightarrow 8j+5}, & i = j + 7s; \\ 0, & \text{otherwise.} \end{cases}$$

If  $s \leq j < 2s$ , then

$$b_{ij} = \begin{cases} w_{8(j+m+1) \rightarrow 8(j+m+1)+1} \otimes w_{8j+1 \rightarrow 8(j+1)}, & i = (j+1)_s; \\ -w_{8(j+m)+7 \rightarrow 8(j+m+1)+1} \otimes w_{8j+1 \rightarrow 8(j+1)}, & i = s + (j+1)_s; \\ 0, & \text{otherwise.} \end{cases}$$

If  $2s \leq j < 3s$ , then

$$b_{ij} = \begin{cases} w_{8(j+m+1) \rightarrow 8(j+m+1)+2} \otimes w_{8j+2 \rightarrow 8(j+1)}, & i = (j+1)_s; \\ -w_{8(j+m)+7 \rightarrow 8(j+m+1)+2} \otimes w_{8j+2 \rightarrow 8(j+1)}, & i = s + (j+1)_s; \\ 0, & \text{otherwise.} \end{cases}$$

If  $3s \leq j < 4s$ , then

$$b_{ij} = \begin{cases} w_{8(j+m+1) \rightarrow 8(j+m+1)+3} \otimes w_{8j+3 \rightarrow 8(j+1)}, & i = (j+1)_s; \\ -w_{8(j+m)+7 \rightarrow 8(j+m+1)+3} \otimes w_{8j+3 \rightarrow 8(j+1)}, & i = s + (j+1)_s; \\ 0, & \text{otherwise.} \end{cases}$$

If  $4s \leq j < 5s$ , then

$$b_{ij} = \begin{cases} w_{8(j+m+1) \rightarrow 8(j+m+1)+4} \otimes w_{8j+4 \rightarrow 8(j+1)}, & i = (j+1)_s; \\ -w_{8(j+m)+7 \rightarrow 8(j+m+1)+4} \otimes w_{8j+4 \rightarrow 8(j+1)}, & i = s + (j+1)_s; \\ w_{8(j+m+1)+1 \rightarrow 8(j+m+1)+4} \otimes w_{8j+4 \rightarrow 8(j+1)+4}, & i = 6s + (j+1)_s; \\ 0, & \text{otherwise.} \end{cases}$$

If  $5s \leq j < 6s$ , then  $b_{ij} = 0$ .

If  $6s \leq j < 7s$ , then

$$b_{ij} = \begin{cases} e_{8(j+m+1)+6} \otimes w_{8j+6 \rightarrow 8(j+1)+6}, & i = 10s + (j+1)_s; \\ 0, & \text{otherwise.} \end{cases}$$

If  $7s \leq j < 8s$ , then

$$b_{ij} = \begin{cases} w_{8(j+m+1) \rightarrow 8(j+m+1)+7} \otimes w_{8j+7 \rightarrow 8(j+1)}, & i = (j+1)_s; \\ -w_{8(j+m)+7 \rightarrow 8(j+m+1)+7} \otimes w_{8j+7 \rightarrow 8(j+1)}, & i = s + (j+1)_s; \\ w_{8(j+m+1)+1 \rightarrow 8(j+m+1)+7} \otimes w_{8j+7 \rightarrow 8(j+1)+4}, & i = 6s + (j+1)_s; \\ w_{8(j+m+1)+2 \rightarrow 8(j+m+1)+7} \otimes w_{8j+7 \rightarrow 8(j+1)+5}, & i = 7s + (j+1)_s; \\ 0, & \text{otherwise.} \end{cases}$$

(24) If  $r_0 = 23$ , then  $\Omega^{23}(Z_t^{(7)})$  is described with  $(11s \times 9s)$  matrix, whose entries  $b_{ij}$  have the following form:

If  $0 \leq j < s$ , then

$$b_{ij} = \begin{cases} w_{8(j+m)+3 \rightarrow 8(j+m+1)+1} \otimes e_{8j}, & i = j; \\ w_{8(j+m+1) \rightarrow 8(j+m+1)+1} \otimes w_{8j \rightarrow 8j+1}, & i = j + 2s; \\ w_{8(j+m)+7 \rightarrow 8(j+m+1)+1} \otimes w_{8j \rightarrow 8j+2}, & i = j + 3s; \\ w_{8(j+m)+7 \rightarrow 8(j+m+1)+1} \otimes w_{8j \rightarrow 8j+6}, & i = j + 7s; \\ 0, & \text{otherwise.} \end{cases}$$

If  $s \leq j < 7s$ , then  $b_{ij} = 0$ .

If  $7s \leq j < 8s$ , then

$$b_{ij} = \begin{cases} -w_{8(j+m+1)+3 \rightarrow 8(j+m+1)+7} \otimes w_{8j+6 \rightarrow 8(j+1)}, & i = (j+1)_s; \\ -e_{8(j+m+1)+7} \otimes w_{8j+6 \rightarrow 8(j+1)+6}, & i = 7s + (j+1)_s; \\ 0, & \text{otherwise.} \end{cases}$$

If  $8s \leq j < 9s$ , then  $b_{ij} = 0$ .

(25) If  $r_0 = 24$ , then  $\Omega^{24}(Z_t^{(7)})$  is described with  $(11s \times 8s)$  matrix, whose entries  $b_{ij}$  have the following form:

If  $0 \leq j < s$ , then

$$b_{ij} = \begin{cases} w_{8(j+m) \rightarrow 8(j+m)+7} \otimes e_{8j}, & i = j; \\ -w_{8(j+m)+1 \rightarrow 8(j+m)+7} \otimes w_{8j \rightarrow 8j+3}, & i = j + 4s; \\ w_{8(j+m)+2 \rightarrow 8(j+m)+7} \otimes w_{8j \rightarrow 8j+4}, & i = j + 5s; \\ w_{8(j+m)+3 \rightarrow 8(j+m)+7} \otimes w_{8j \rightarrow 8j+5}, & i = j + 6s; \\ 0, & \text{otherwise.} \end{cases}$$

If  $s \leq j < 2s$ , then

$$b_{ij} = \begin{cases} w_{8(j+m+1) \rightarrow 8(j+m+1)+2} \otimes w_{8j+1 \rightarrow 8(j+1)}, & i = (j+1)_s; \\ 0, & \text{otherwise.} \end{cases}$$

If  $2s \leq j < 3s$ , then

$$b_{ij} = \begin{cases} w_{8(j+m+1) \rightarrow 8(j+m+1)+3} \otimes w_{8j+2 \rightarrow 8(j+1)}, & i = (j+1)_s; \\ 0, & \text{otherwise.} \end{cases}$$

If  $3s \leq j < 4s$ , then

$$b_{ij} = \begin{cases} w_{8(j+m+1) \rightarrow 8(j+m+1)+4} \otimes w_{8j+3 \rightarrow 8(j+1)}, & i = (j+1)_s; \\ -w_{8(j+m+1)+1 \rightarrow 8(j+m+1)+4} \otimes w_{8j+3 \rightarrow 8(j+1)+3}, & i = 4s + (j+1)_s; \\ 0, & \text{otherwise.} \end{cases}$$

If  $4s \leq j < 7s$ , then  $b_{ij} = 0$ .

If  $7s \leq j < 8s$ , then

$$b_{ij} = \begin{cases} w_{8(j+m+1)+5 \rightarrow 8(j+m+2)} \otimes w_{8j+7 \rightarrow 8(j+1)+1}, & i = 2s + (j+1)_s; \\ 0, & \text{otherwise.} \end{cases}$$

(26) If  $r_0 = 25$ , then  $\Omega^{25}(Z_t^{(7)})$  is described with  $(10s \times 10s)$  matrix, whose entries  $b_{ij}$  have the following form:

If  $0 \leq j < s$ , then

$$b_{ij} = \begin{cases} w_{8(j+m)+4 \rightarrow 8(j+m+1)+2} \otimes e_{8j}, & i = j; \\ w_{8(j+m)+7 \rightarrow 8(j+m+1)+2} \otimes w_{8j \rightarrow 8j+1}, & i = j + 2s; \\ w_{8(j+m+1) \rightarrow 8(j+m+1)+2} \otimes w_{8j \rightarrow 8j+2}, & i = j + 3s; \\ w_{8(j+m+1) \rightarrow 8(j+m+1)+2} \otimes w_{8j \rightarrow 8j+6}, & i = j + 7s; \\ 0, & \text{otherwise.} \end{cases}$$

If  $s \leq j < 5s$ , then  $b_{ij} = 0$ .

If  $5s \leq j < 6s$ , then

$$b_{ij} = \begin{cases} w_{8(j+m+1)+6 \rightarrow 8(j+m+2)} \otimes w_{8j+4 \rightarrow 8(j+1)}, & i = s + (j+1)_s; \\ e_{8(j+m+2)} \otimes w_{8j+4 \rightarrow 8(j+1)+2}, & i = 3s + (j+1)_s; \\ 0, & \text{otherwise.} \end{cases}$$

If  $6s \leq j < 7s$ , then

$$b_{ij} = \begin{cases} w_{8(j+m+1)+4 \rightarrow 8(j+m+1)+7} \otimes w_{8j+5 \rightarrow 8(j+1)}, & i = (j+1)_s; \\ 0, & \text{otherwise.} \end{cases}$$

If  $7s \leq j < 8s$ , then  $b_{ij} = 0$ .

If  $8s \leq j < 9s$ , then

$$b_{ij} = \begin{cases} -w_{8(j+m+1)+4 \rightarrow 8(j+m+2)+1} \otimes w_{8j+7 \rightarrow 8(j+1)}, & i = (j+1)_s; \\ -w_{8(j+m+1)+7 \rightarrow 8(j+m+2)+1} \otimes w_{8j+7 \rightarrow 8(j+1)+1}, & i = 2s + (j+1)_s; \\ -w_{8(j+m+2) \rightarrow 8(j+m+2)+1} \otimes w_{8j+7 \rightarrow 8(j+1)+2}, & i = 3s + (j+1)_s; \\ -w_{8(j+m+2) \rightarrow 8(j+m+2)+1} \otimes w_{8j+7 \rightarrow 8(j+1)+6}, & i = 7s + (j+1)_s; \\ 0, & \text{otherwise.} \end{cases}$$

If  $9s \leq j < 10s$ , then

$$b_{ij} = \begin{cases} -w_{8(j+m+1)+7 \rightarrow 8(j+m+2)+5} \otimes w_{8j+7 \rightarrow 8(j+1)+1}, & i = 2s + (j+1)_s; \\ -w_{8(j+m+2) \rightarrow 8(j+m+2)+5} \otimes w_{8j+7 \rightarrow 8(j+1)+2}, & i = 3s + (j+1)_s; \\ -w_{8(j+m+2) \rightarrow 8(j+m+2)+5} \otimes w_{8j+7 \rightarrow 8(j+1)+6}, & i = 7s + (j+1)_s; \\ 0, & \text{otherwise.} \end{cases}$$

(27) If  $r_0 = 26$ , then  $\Omega^{26}(Z_t^{(7)})$  is described with  $(8s \times 11s)$  matrix, whose entries  $b_{ij}$  have the following form:

If  $0 \leq j < s$ , then

$$b_{ij} = \begin{cases} w_{8(j+m-1)+7 \rightarrow 8(j+m)+7} \otimes e_{8j}, & i = j; \\ w_{8(j+m)+1 \rightarrow 8(j+m)+7} \otimes w_{8j \rightarrow 8j+2}, & i = j + 2s; \\ -w_{8(j+m)+2 \rightarrow 8(j+m)+7} \otimes w_{8j \rightarrow 8j+3}, & i = j + 3s; \\ w_{8(j+m)+3 \rightarrow 8(j+m)+7} \otimes w_{8j \rightarrow 8j+4}, & i = j + 4s; \\ w_{8(j+m)+4 \rightarrow 8(j+m)+7} \otimes w_{8j \rightarrow 8j+5}, & i = j + 5s; \\ 0, & \text{otherwise.} \end{cases}$$

If  $s \leq j < 2s$ , then

$$b_{ij} = \begin{cases} -w_{8(j+m)+7 \rightarrow 8(j+m+1)} \otimes w_{8j \rightarrow 8(j+1)}, & i = (j+1)_s; \\ 0, & \text{otherwise.} \end{cases}$$

If  $2s \leq j < 3s$ , then

$$b_{ij} = \begin{cases} w_{8(j+m)+7 \rightarrow 8(j+m+1)+3} \otimes w_{8j+1 \rightarrow 8(j+1)}, & i = (j+1)_s; \\ 0, & \text{otherwise.} \end{cases}$$

If  $3s \leq j < 4s$ , then

$$b_{ij} = \begin{cases} w_{8(j+m)+7 \rightarrow 8(j+m+1)+4} \otimes w_{8j+2 \rightarrow 8(j+1)}, & i = (j+1)_s; \\ w_{8(j+m+1)+1 \rightarrow 8(j+m+1)+4} \otimes w_{8j+2 \rightarrow 8(j+1)+2}, & i = 2s + (j+1)_s; \\ 0, & \text{otherwise.} \end{cases}$$

If  $4s \leq j < 5s$ , then

$$b_{ij} = \begin{cases} -w_{8(j+m)+7 \rightarrow 8(j+m+1)+5} \otimes w_{8j+3 \rightarrow 8(j+1)}, & i = (j+1)_s; \\ 0, & \text{otherwise.} \end{cases}$$

If  $5s \leq j < 6s$ , then

$$b_{ij} = \begin{cases} -w_{8(j+m)+7 \rightarrow 8(j+m+1)+6} \otimes w_{8j+4 \rightarrow 8(j+1)}, & i = (j+1)_s; \\ 0, & \text{otherwise.} \end{cases}$$

If  $6s \leq j < 7s$ , then

$$b_{ij} = \begin{cases} -w_{8(j+m)+7 \rightarrow 8(j+m+1)+1} \otimes w_{8j+4 \rightarrow 8(j+1)}, & i = (j+1)_s; \\ 0, & \text{otherwise.} \end{cases}$$

If  $7s \leq j < 9s$ , then  $b_{ij} = 0$ .

If  $9s \leq j < 10s$ , then

$$b_{ij} = \begin{cases} -e_{8(j+m+1)+5} \otimes w_{8j+6 \rightarrow 8(j+1)+6}, & i = 6s + (j+1)_s; \\ 0, & \text{otherwise.} \end{cases}$$

If  $10s \leq j < 11s$ , then

$$b_{ij} = \begin{cases} w_{8(j+m)+7 \rightarrow 8(j+m+1)+7} \otimes w_{8j+7 \rightarrow 8(j+1)}, & i = (j+1)_s; \\ w_{8(j+m+1)+1 \rightarrow 8(j+m+1)+7} \otimes w_{8j+7 \rightarrow 8(j+1)+2}, & i = 2s + (j+1)_s; \\ -w_{8(j+m+1)+2 \rightarrow 8(j+m+1)+7} \otimes w_{8j+7 \rightarrow 8(j+1)+3}, & i = 3s + (j+1)_s; \\ w_{8(j+m+1)+3 \rightarrow 8(j+m+1)+7} \otimes w_{8j+7 \rightarrow 8(j+1)+4}, & i = 4s + (j+1)_s; \\ w_{8(j+m+1)+4 \rightarrow 8(j+m+1)+7} \otimes w_{8j+7 \rightarrow 8(j+1)+5}, & i = 5s + (j+1)_s; \\ 0, & \text{otherwise.} \end{cases}$$

(28) If  $r_0 = 27$ , then  $\Omega^{27}(Z_t^{(7)})$  is described with  $(9s \times 11s)$  matrix, whose entries  $b_{ij}$  have the following form:

If  $s \leq j < 2s$ , then

$$b_{ij} = \begin{cases} -w_{8(j+m+1) \rightarrow 8(j+m+1)+3} \otimes w_{8j \rightarrow 8j+1}, & i = j; \\ w_{8(j+m+1) \rightarrow 8(j+m+1)+3} \otimes w_{8j \rightarrow 8j+5}, & i = j + 4s; \\ 0, & \text{otherwise.} \end{cases}$$

If  $2s \leq j < 7s$ , then  $b_{ij} = 0$ .

If  $7s \leq j < 8s$ , then

$$b_{ij} = \begin{cases} w_{8(j+m+1)+7 \rightarrow 8(j+m+2)} \otimes w_{8j+5 \rightarrow 8(j+1)}, & i = (j+1)_s; \\ 0, & \text{otherwise.} \end{cases}$$

If  $8s \leq j < 9s$ , then

$$b_{ij} = \begin{cases} -e_{8(j+m+1)+7} \otimes w_{8j+6 \rightarrow 8(j+1)}, & i = (j+1)_s; \\ 0, & \text{otherwise.} \end{cases}$$

If  $9s \leq j < 11s$ , then  $b_{ij} = 0$ .

(29) If  $r_0 = 28$ , then  $\Omega^{28}(Z_t^{(7)})$  is described with  $(8s \times 13s)$  matrix, whose entries  $b_{ij}$  have the following form:

If  $0 \leq j < s$ , then

$$b_{ij} = \begin{cases} (-1 + 2(f(j_1, 1) + f(j_1, 3) + f(j_1, 6)))w_{8(j+m)+j_1 \rightarrow 8(j+m)+7} \otimes w_{8j \rightarrow 8j+j_1}, & i = j + j_1s, \ 1 \leq j_1 \leq 7; \\ 0, & \text{otherwise.} \end{cases}$$

If  $s \leq j < 2s$ , then

$$b_{ij} = \begin{cases} (1 - 2(f(j_1, 0) + f(j_1, 2) + f(j_1, 5)))w_{8(j+m)+j_1+1 \rightarrow 8(j+m+1)} \otimes w_{8j \rightarrow 8j+j_1+1}, \\ i = j + j_1s, \ 0 \leq j_1 \leq 6; \\ 0, \text{ otherwise.} \end{cases}$$

If  $2s \leq j < 3s$ , then

$$b_{ij} = \begin{cases} -w_{8(j+m+1)+1 \rightarrow 8(j+m+1)+4} \otimes w_{8j+1 \rightarrow 8(j+1)+1}, & i = s + (j+1)_s; \\ 0, & \text{otherwise.} \end{cases}$$

If  $3s \leq j < 8s$ , then  $b_{ij} = 0$ .

If  $8s \leq j < 9s$ , then

$$b_{ij} = \begin{cases} w_{8(j+m+1) \rightarrow 8(j+m+1)+5} \otimes w_{8j+5 \rightarrow 8(j+1)}, & i = (j+1)_s; \\ e_{8(j+m+1)+5} \otimes w_{8j+5 \rightarrow 8(j+1)+5}, & i = 5s + (j+1)_s; \\ 0, & \text{otherwise.} \end{cases}$$

If  $9s \leq j < 10s$ , then

$$b_{ij} = \begin{cases} -w_{8(j+m+1) \rightarrow 8(j+m+1)+3} \otimes w_{8j+6 \rightarrow 8(j+1)}, & i = (j+1)_s; \\ 0, & \text{otherwise.} \end{cases}$$

If  $10s \leq j < 11s$ , then

$$b_{ij} = \begin{cases} w_{8(j+m)+6 \rightarrow 8(j+m+1)+6} \otimes e_{8j+6}, & i = j - 4s; \\ -w_{8(j+m)+7 \rightarrow 8(j+m+1)+6} \otimes w_{8j+6 \rightarrow 8j+7}, & i = j - 3s; \\ 0, & \text{otherwise.} \end{cases}$$

If  $11s \leq j < 12s$ , then

$$b_{ij} = \begin{cases} (1 - 2(f(j_1, 1) + f(j_1, 3) + f(j_1, 6)))w_{8(j+m+1)+j_1 \rightarrow 8(j+m+1)+7} \otimes w_{8j+7 \rightarrow 8(j+1)+j_1}, \\ i = j_1s + (j+1)_s, \ 1 \leq j_1 \leq 7; \\ 0, \text{ otherwise.} \end{cases}$$

If  $12s \leq j < 13s$ , then  $b_{ij} = 0$ .

(II) Represent an arbitrary  $t_0 \in \mathbb{N}$  in the form  $t_0 = 29\ell_0 + r_0$ , where  $0 \leq r_0 \leq 28$ . Then  $\Omega^{t_0}(Z_t^{(7)})$  is a  $\Omega^{r_0}(Z_t^{(7)})$ , whose left components twisted by  $\sigma^{\ell_0}$ .

**Proposition 7** (Translates for the case 8). (I) Let  $r_0 \in \mathbb{N}$ ,  $r_0 < 29$ .  $r_0$ -translates of the elements  $Z_t^{(8)}$  are described by the following way.

(1) If  $r_0 = 0$ , then  $\Omega^0(Z_t^{(8)})$  is described with  $(8s \times 16s)$  matrix with unique nonzero entry:

$$b_{j,(3)_s} = -w_{8(j+m) \rightarrow 8(j+m)+7} \otimes e_{8j}.$$

(2) If  $r_0 = 1$ , then  $\Omega^1(Z_t^{(8)})$  is described with  $(9s \times 16s)$  matrix with the following nonzero entries:

$$\begin{aligned} b_{s+(j+1)_s, 5s+(2)_s} &= -w_{8(j+m+1)+5 \rightarrow 8(j+m+1)+7} \otimes w_{8j+2 \rightarrow 8(j+1)}; \\ b_{s+(j+1)_s, 6s+(2)_s} &= -w_{8(j+m+1)+5 \rightarrow 8(j+m+2)} \otimes w_{8j+3 \rightarrow 8(j+1)}; \\ b_{(j+1)_s, 8s+(2)_s} &= w_{8(j+m+1)+1 \rightarrow 8(j+m+1)+7} \otimes w_{8j+5 \rightarrow 8(j+1)}. \end{aligned}$$

(3) If  $r_0 = 2$ , then  $\Omega^2(Z_t^{(8)})$  is described with  $(8s \times 19s)$  matrix with the following nonzero entries:

$$\begin{aligned} b_{(j+1)s, (2)s} &= -e_{8(j+m)+7} \otimes w_{8j \rightarrow 8(j+1)}; \\ b_{(j+1)s, s+(2)s} &= -w_{8(j+m)+7 \rightarrow 8(j+m+1)} \otimes w_{8j \rightarrow 8(j+1)}; \\ b_{(j+1)s, 7s+(2)s} &= w_{8(j+m)+7 \rightarrow 8(j+m+1)+5} \otimes w_{8j+3 \rightarrow 8(j+1)}. \end{aligned}$$

(4) If  $r_0 = 3$ , then  $\Omega^3(Z_t^{(8)})$  is described with  $(10s \times 18s)$  matrix with the following nonzero entries:

$$\begin{aligned} b_{s+(j+1)s, s+(2)s} &= -e_{8(j+m+1)+6} \otimes w_{8j \rightarrow 8(j+1)}; \\ b_{(j+1)s, 2s+(2)s} &= -w_{8(j+m+1)+2 \rightarrow 8(j+m+1)+4} \otimes w_{8j \rightarrow 8(j+1)}; \\ b_{s+(j+1)s, 7s+(2)s} &= -w_{8(j+m+1)+6 \rightarrow 8(j+m+1)+7} \otimes w_{8j+3 \rightarrow 8(j+1)}. \end{aligned}$$

(5) If  $r_0 = 4$ , then  $\Omega^4(Z_t^{(8)})$  is described with  $(11s \times 19s)$  matrix with the following nonzero entries:

$$\begin{aligned} b_{(j+1)s, s+(2)s} &= -w_{8(j+m)+7 \rightarrow 8(j+m+1)} \otimes w_{8j \rightarrow 8(j+1)}; \\ b_{s+(j+1)s, s+(2)s} &= -e_{8(j+m+1)} \otimes w_{8j \rightarrow 8(j+1)}; \\ b_{(j+1)s, 2s+(2)s} &= -e_{8(j+m)+7} \otimes w_{8j \rightarrow 8(j+1)}; \\ b_{s+(j+1)s, 7s+(2)s} &= -w_{8(j+m+1) \rightarrow 8(j+m+1)+6} \otimes w_{8j+3 \rightarrow 8(j+1)}. \end{aligned}$$

(6) If  $r_0 = 5$ , then  $\Omega^5(Z_t^{(8)})$  is described with  $(11s \times 18s)$  matrix with the following nonzero entries:

$$\begin{aligned} b_{2s+(j+1)s, (2)s} &= w_{8(j+m+1)+1 \rightarrow 8(j+m+1)+2} \otimes w_{8j \rightarrow 8(j+1)}; \\ b_{(j+1)s, 2s+(2)s} &= -w_{8(j+m+1)+5 \rightarrow 8(j+m+1)+6} \otimes w_{8j \rightarrow 8(j+1)}; \\ b_{(j+1)s, 3s+(2)s} &= -e_{8(j+m+1)+5} \otimes w_{8j \rightarrow 8(j+1)}; \\ b_{2s+(j+1)s, 6s+(2)s} &= -w_{8(j+m+1)+1 \rightarrow 8(j+m+1)+7} \otimes w_{8j+3 \rightarrow 8(j+1)}; \\ b_{2s+(j+1)s, 7s+(2)s} &= -w_{8(j+m+1)+1 \rightarrow 8(j+m+2)} \otimes w_{8j+3 \rightarrow 8(j+1)}. \end{aligned}$$

(7) If  $r_0 = 6$ , then  $\Omega^6(Z_t^{(8)})$  is described with  $(13s \times 20s)$  matrix with the following nonzero entries:

$$\begin{aligned} b_{(j+1)s, 2s+(2)s} &= -w_{8(j+m)+7 \rightarrow 8(j+m+1)} \otimes w_{8j \rightarrow 8(j+1)}; \\ b_{s+(j+1)s, 2s+(2)s} &= -e_{8(j+m+1)} \otimes w_{8j \rightarrow 8(j+1)}; \\ b_{j-3s, 8s+(2)s} &= w_{8(j+m)+1 \rightarrow 8(j+m+1)+1} \otimes e_{8j+3}. \end{aligned}$$

(8) If  $r_0 = 7$ , then  $\Omega^7(Z_t^{(8)})$  is described with  $(14s \times 18s)$  matrix with the following nonzero entries:

$$\begin{aligned} b_{2s+(j+1)s, s+(2)s} &= -e_{8(j+m+1)+6} \otimes w_{8j \rightarrow 8(j+1)}; \\ b_{3s+(j+1)s, s+(2)s} &= -w_{8(j+m+1)+5 \rightarrow 8(j+m+1)+6} \otimes w_{8j \rightarrow 8(j+1)}; \\ b_{j+2s, 3s+(2)s} &= -w_{8(j+m+1) \rightarrow 8(j+m+1)+1} \otimes w_{8j \rightarrow 8j+2}. \end{aligned}$$

(9) If  $r_0 = 8$ , then  $\Omega^8(Z_t^{(8)})$  is described with  $(16s \times 19s)$  matrix with the following nonzero entries:

$$\begin{aligned} b_{j+4s, (2)s} &= -w_{8(j+m)+6 \rightarrow 8(j+m)+7} \otimes w_{8j \rightarrow 8j+2}; \\ b_{2s+(j+1)s, 6s+(1)s} &= -w_{8(j+m+1) \rightarrow 8(j+m+1)+1} \otimes w_{8j+2 \rightarrow 8(j+1)}; \\ b_{2s+(j+1)s, 7s+(1)s} &= -w_{8(j+m+1) \rightarrow 8(j+m+1)+2} \otimes w_{8j+3 \rightarrow 8(j+1)}; \\ b_{6s+(j+1)s, 7s+(1)s} &= e_{8(j+m+1)+2} \otimes w_{8j+3 \rightarrow 8(j+1)+3}. \end{aligned}$$

(10) If  $r_0 = 9$ , then  $\Omega^9(Z_t^{(8)})$  is described with  $(16s \times 18s)$  matrix with the following nonzero entries:

$$\begin{aligned}
b_{(j+1)s, 4s+(1)s} &= w_{8(j+m+1)+5 \rightarrow 8(j+m+1)+7} \otimes w_{8j+1 \rightarrow 8(j+1)}; \\
b_{s+(j+1)s, 4s+(1)s} &= -w_{8(j+m+1)+3 \rightarrow 8(j+m+1)+7} \otimes w_{8j+1 \rightarrow 8(j+1)}; \\
b_{2s+(j+1)s, 4s+(1)s} &= w_{8(j+m+1)+6 \rightarrow 8(j+m+1)+7} \otimes w_{8j+1 \rightarrow 8(j+1)}; \\
b_{(j+1)s, 5s+(1)s} &= w_{8(j+m+1)+5 \rightarrow 8(j+m+2)} \otimes w_{8j+1 \rightarrow 8(j+1)}; \\
b_{2s+(j+1)s, 5s+(1)s} &= w_{8(j+m+1)+6 \rightarrow 8(j+m+2)} \otimes w_{8j+1 \rightarrow 8(j+1)}; \\
b_{(j+1)s, 6s+(1)s} &= w_{8(j+m+1)+5 \rightarrow 8(j+m+2)} \otimes w_{8j+2 \rightarrow 8(j+1)}; \\
b_{2s+(j+1)s, 6s+(1)s} &= w_{8(j+m+1)+6 \rightarrow 8(j+m+2)} \otimes w_{8j+2 \rightarrow 8(j+1)}; \\
b_{(j+1)s, 7s+(1)s} &= -w_{8(j+m+1)+5 \rightarrow 8(j+m+1)+7} \otimes w_{8j+3 \rightarrow 8(j+1)}; \\
b_{s+(j+1)s, 7s+(1)s} &= w_{8(j+m+1)+3 \rightarrow 8(j+m+1)+7} \otimes w_{8j+3 \rightarrow 8(j+1)}; \\
b_{2s+(j+1)s, 7s+(1)s} &= -w_{8(j+m+1)+6 \rightarrow 8(j+m+1)+7} \otimes w_{8j+3 \rightarrow 8(j+1)}.
\end{aligned}$$

(11) If  $r_0 = 10$ , then  $\Omega^{10}(Z_t^{(8)})$  is described with  $(19s \times 19s)$  matrix with two nonzero entries:

$$\begin{aligned}
b_{s+(j+1)s, s+(1)s} &= e_{8(j+m+1)} \otimes w_{8j \rightarrow 8(j+1)}; \\
b_{j-s, 7s+(1)s} &= w_{8(j+m)+3 \rightarrow 8(j+m+1)+3} \otimes e_{8j+3}.
\end{aligned}$$

(12) If  $r_0 = 11$ , then  $\Omega^{11}(Z_t^{(8)})$  is described with  $(18s \times 16s)$  matrix with the following nonzero entries:

$$\begin{aligned}
b_{(j+1)s, (1)s} &= -w_{8(j+m+1)+2 \rightarrow 8(j+m+1)+3} \otimes w_{8j \rightarrow 8(j+1)}; \\
b_{j+5s, (1)s} &= w_{8(j+m)+7 \rightarrow 8(j+m+1)+3} \otimes w_{8j \rightarrow 8j+1}; \\
b_{4s+(j+1)s, 3s+(1)s} &= e_{8(j+m+1)+5} \otimes w_{8j \rightarrow 8(j+1)}.
\end{aligned}$$

(13) If  $r_0 = 12$ , then  $\Omega^{12}(Z_t^{(8)})$  is described with  $(19s \times 16s)$  matrix with the following nonzero entries:

$$\begin{aligned}
b_{j+3s, (1)s} &= -w_{8(j+m)+2 \rightarrow 8(j+m)+7} \otimes w_{8j \rightarrow 8j+1}; \\
b_{j+5s, (1)s} &= w_{8(j+m)+5 \rightarrow 8(j+m)+7} \otimes w_{8j \rightarrow 8j+2}; \\
b_{s+(j+1)s, s+(1)s} &= -e_{8(j+m+1)} \otimes w_{8j \rightarrow 8(j+1)}; \\
b_{2s+(j+1)s, s+(1)s} &= -w_{8(j+m)+7 \rightarrow 8(j+m+1)} \otimes w_{8j \rightarrow 8(j+1)}; \\
b_{(j+1)s, 4s} &= -w_{8(j+m)+7 \rightarrow 8(j+m+1)+3} \otimes w_{8j+2 \rightarrow 8(j+1)}; \\
b_{(j+1)s, 5s} &= w_{8(j+m)+7 \rightarrow 8(j+m+1)+4} \otimes w_{8j+3 \rightarrow 8(j+1)}; \\
b_{6s+(j+1)s, 5s} &= e_{8(j+m+1)+4} \otimes w_{8j+3 \rightarrow 8(j+1)+3}.
\end{aligned}$$

(14) If  $r_0 = 13$ , then  $\Omega^{13}(Z_t^{(8)})$  is described with  $(18s \times 14s)$  matrix with the following nonzero entries:

$$\begin{aligned}
b_{j+4s, (1)s} &= w_{8(j+m+1) \rightarrow 8(j+m+1)+2} \otimes w_{8j \rightarrow 8j+1}; \\
b_{(j+1)s, s+(1)s} &= w_{8(j+m+1)+2 \rightarrow 8(j+m+1)+4} \otimes w_{8j \rightarrow 8(j+1)}; \\
b_{s+(j+1)s, s+(1)s} &= -w_{8(j+m+1)+3 \rightarrow 8(j+m+1)+4} \otimes w_{8j \rightarrow 8(j+1)}; \\
b_{2s+(j+1)s, 2s+(1)s} &= e_{8(j+m+1)+6} \otimes w_{8j \rightarrow 8(j+1)}; \\
b_{3s+(j+1)s, 2s+(1)s} &= w_{8(j+m+1)+5 \rightarrow 8(j+m+1)+6} \otimes w_{8j \rightarrow 8(j+1)}; \\
b_{s+(j+1)s, 3s} &= -w_{8(j+m+1)+3 \rightarrow 8(j+m+1)+7} \otimes w_{8j+1 \rightarrow 8(j+1)}; \\
b_{(j+1)s, 4s} &= w_{8(j+m+1)+2 \rightarrow 8(j+m+2)} \otimes w_{8j+2 \rightarrow 8(j+1)}; \\
b_{3s+(j+1)s, 4s} &= w_{8(j+m+1)+5 \rightarrow 8(j+m+2)} \otimes w_{8j+2 \rightarrow 8(j+1)};
\end{aligned}$$



$$\begin{aligned}
b_{s+(j+1)s,5s} &= w_{8(j+m+1)+3 \rightarrow 8(j+m+1)+7} \otimes w_{8j+3 \rightarrow 8(j+1)}; \\
b_{5s+(j+1)s,5s} &= -e_{8(j+m+1)+7} \otimes w_{8j+3 \rightarrow 8(j+1)+2}; \\
b_{4s+(j+1)s,13s} &= -w_{8(j+m+2) \rightarrow 8(j+m+2)+5} \otimes w_{8j+7 \rightarrow 8(j+1)+1}.
\end{aligned}$$

(15) If  $r_0 = 14$ , then  $\Omega^{14}(Z_t^{(8)})$  is described with  $(20s \times 13s)$  matrix with the following nonzero entries:

$$\begin{aligned}
b_{(j+1)s,(1)s} &= -w_{8(j+m)+7 \rightarrow 8(j+m+1)} \otimes w_{8j \rightarrow 8(j+1)}; \\
b_{2s+(j+1)s,(1)s} &= e_{8(j+m+1)} \otimes w_{8j \rightarrow 8(j+1)}; \\
b_{j+4s,(1)s} &= -w_{8(j+m)+5 \rightarrow 8(j+m+1)} \otimes w_{8j \rightarrow 8j+1}; \\
b_{(j+1)s,0} &= w_{8(j+m)+7 \rightarrow 8(j+m+1)} \otimes w_{8j \rightarrow 8(j+1)}; \\
b_{s+(j+1)s,0} &= e_{8(j+m+1)} \otimes w_{8j \rightarrow 8(j+1)}; \\
b_{2s+(j+1)s,0} &= -e_{8(j+m+1)} \otimes w_{8j \rightarrow 8(j+1)}; \\
b_{(j+1)s,s+(1)s} &= e_{8(j+m)+7} \otimes w_{8j \rightarrow 8(j+1)}; \\
b_{(j+1)s,2s} &= -w_{8(j+m)+7 \rightarrow 8(j+m+1)+3} \otimes w_{8j+1 \rightarrow 8(j+1)}; \\
b_{s+(j+1)s,2s} &= -w_{8(j+m+1) \rightarrow 8(j+m+1)+3} \otimes w_{8j+1 \rightarrow 8(j+1)}; \\
b_{(j+1)s,3s} &= w_{8(j+m)+7 \rightarrow 8(j+m+1)+4} \otimes w_{8j+2 \rightarrow 8(j+1)}; \\
b_{(j+1)s,4s} &= w_{8(j+m)+7 \rightarrow 8(j+m+1)+5} \otimes w_{8j+2 \rightarrow 8(j+1)}; \\
b_{s+(j+1)s,4s} &= w_{8(j+m+1) \rightarrow 8(j+m+1)+5} \otimes w_{8j+2 \rightarrow 8(j+1)}; \\
b_{2s+(j+1)s,4s} &= -w_{8(j+m+1) \rightarrow 8(j+m+1)+5} \otimes w_{8j+2 \rightarrow 8(j+1)}; \\
b_{(j+1)s,5s} &= -w_{8(j+m)+7 \rightarrow 8(j+m+1)+6} \otimes w_{8j+3 \rightarrow 8(j+1)}; \\
b_{s+(j+1)s,5s} &= -w_{8(j+m+1) \rightarrow 8(j+m+1)+6} \otimes w_{8j+3 \rightarrow 8(j+1)}; \\
b_{2s+(j+1)s,5s} &= w_{8(j+m+1) \rightarrow 8(j+m+1)+6} \otimes w_{8j+3 \rightarrow 8(j+1)}; \\
b_{4s+(j+1)s,5s} &= w_{8(j+m+1)+5 \rightarrow 8(j+m+1)+6} \otimes w_{8j+3 \rightarrow 8(j+1)+1}; \\
b_{3s+(j+1)s,11s} &= w_{8(j+m+1)+3 \rightarrow 8(j+m+1)+7} \otimes w_{8j+7 \rightarrow 8(j+1)+1}.
\end{aligned}$$

(16) If  $r_0 = 15$ , then  $\Omega^{15}(Z_t^{(8)})$  is described with  $(18s \times 11s)$  matrix with the following nonzero entries:

$$\begin{aligned}
b_{3s+(j+1)s,(1)s} &= -w_{8(j+m+1)+1 \rightarrow 8(j+m+1)+3} \otimes w_{8j \rightarrow 8(j+1)}; \\
b_{3s+(j+1)s,0} &= w_{8(j+m+1)+1 \rightarrow 8(j+m+1)+3} \otimes w_{8j \rightarrow 8(j+1)}; \\
b_{j+4s,s+(1)s} &= w_{8(j+m)+7 \rightarrow 8(j+m+1)+5} \otimes w_{8j \rightarrow 8j+1}; \\
b_{j+6s,s+(1)s} &= w_{8(j+m+1) \rightarrow 8(j+m+1)+5} \otimes w_{8j \rightarrow 8j+2}; \\
b_{4s+(j+1)s,2s} &= -w_{8(j+m+1)+5 \rightarrow 8(j+m+2)} \otimes w_{8j+1 \rightarrow 8(j+1)}; \\
b_{(j+1)s,3s} &= -w_{8(j+m+1)+3 \rightarrow 8(j+m+1)+7} \otimes w_{8j+2 \rightarrow 8(j+1)}; \\
b_{3s+(j+1)s,3s} &= 2w_{8(j+m+1)+1 \rightarrow 8(j+m+1)+7} \otimes w_{8j+2 \rightarrow 8(j+1)}; \\
b_{4s+(j+1)s,3s} &= -w_{8(j+m+1)+5 \rightarrow 8(j+m+1)+7} \otimes w_{8j+2 \rightarrow 8(j+1)}; \\
b_{(j+1)s,4s} &= -w_{8(j+m+1)+3 \rightarrow 8(j+m+2)} \otimes w_{8j+3 \rightarrow 8(j+1)}; \\
b_{3s+(j+1)s,4s} &= w_{8(j+m+1)+1 \rightarrow 8(j+m+2)} \otimes w_{8j+3 \rightarrow 8(j+1)}; \\
b_{5s+(j+1)s,5s} &= w_{8(j+m+1)+7 \rightarrow 8(j+m+2)+1} \otimes w_{8j+4 \rightarrow 8(j+1)+1}; \\
b_{5s+(j+1)s,8s} &= -w_{8(j+m+1)+7 \rightarrow 8(j+m+2)+2} \otimes w_{8j+7 \rightarrow 8(j+1)+1}.
\end{aligned}$$

(17) If  $r_0 = 16$ , then  $\Omega^{16}(Z_t^{(8)})$  is described with  $(19s \times 11s)$  matrix with the following nonzero entries:

$$b_{(j+1)s,(1)s} = w_{8(j+m)+7 \rightarrow 8(j+m+1)} \otimes w_{8j \rightarrow 8(j+1)};$$

$$\begin{aligned}
b_{s+(j+1)s,(1)s} &= -e_{8(j+m+1)} \otimes w_{8j \rightarrow 8(j+1)}; \\
b_{2s+(j+1)s,(1)s} &= -w_{8(j+m)+7 \rightarrow 8(j+m+1)} \otimes w_{8j \rightarrow 8(j+1)}; \\
b_{j+4s,(1)s} &= w_{8(j+m)+6 \rightarrow 8(j+m+1)} \otimes w_{8j \rightarrow 8j+1}; \\
b_{2s+(j+1)s,2s} &= w_{8(j+m)+7 \rightarrow 8(j+m+1)+5} \otimes w_{8j+1 \rightarrow 8(j+1)}; \\
b_{s+(j+1)s,3s} &= w_{8(j+m+1) \rightarrow 8(j+m+1)+6} \otimes w_{8j+2 \rightarrow 8(j+1)}; \\
b_{2s+(j+1)s,3s} &= w_{8(j+m)+7 \rightarrow 8(j+m+1)+6} \otimes w_{8j+2 \rightarrow 8(j+1)}; \\
b_{(j+1)s,4s} &= w_{8(j+m)+7 \rightarrow 8(j+m+1)+1} \otimes w_{8j+3 \rightarrow 8(j+1)}.
\end{aligned}$$

(18) If  $r_0 = 17$ , then  $\Omega^{17}(Z_t^{(8)})$  is described with  $(18s \times 10s)$  matrix with the following nonzero entries:

$$\begin{aligned}
b_{(j+1)s,(1)s} &= w_{8(j+m+1)+2 \rightarrow 8(j+m+1)+4} \otimes w_{8j \rightarrow 8(j+1)}; \\
b_{3s+(j+1)s,s+(1)s} &= w_{8(j+m+1)+5 \rightarrow 8(j+m+1)+6} \otimes w_{8j \rightarrow 8(j+1)}; \\
b_{j+3s,s+(1)s} &= w_{8(j+m)+7 \rightarrow 8(j+m+1)+6} \otimes w_{8j \rightarrow 8j+1}; \\
b_{3s+(j+1)s,s} &= -w_{8(j+m+1)+5 \rightarrow 8(j+m+1)+6} \otimes w_{8j \rightarrow 8(j+1)}; \\
b_{3s+(j+1)s,2s} &= w_{8(j+m+1)+5 \rightarrow 8(j+m+1)+7} \otimes w_{8j+1 \rightarrow 8(j+1)}; \\
b_{2s+(j+1)s,3s} &= w_{8(j+m+1)+6 \rightarrow 8(j+m+2)} \otimes w_{8j+2 \rightarrow 8(j+1)}; \\
b_{3s+(j+1)s,3s} &= w_{8(j+m+1)+5 \rightarrow 8(j+m+2)} \otimes w_{8j+2 \rightarrow 8(j+1)}.
\end{aligned}$$

(19) If  $r_0 = 18$ , then  $\Omega^{18}(Z_t^{(8)})$  is described with  $(19s \times 8s)$  matrix with the following nonzero entries:

$$\begin{aligned}
b_{j+3s,(1)s} &= w_{8(j+m)+5 \rightarrow 8(j+m)+7} \otimes w_{8j \rightarrow 8j+1}; \\
b_{j+4s,(1)s} &= -w_{8(j+m)+1 \rightarrow 8(j+m)+7} \otimes w_{8j \rightarrow 8j+1}; \\
b_{j+5s,(1)s} &= -w_{8(j+m)+2 \rightarrow 8(j+m)+7} \otimes w_{8j \rightarrow 8j+2}; \\
b_{(j+1)s,s} &= -w_{8(j+m)+7 \rightarrow 8(j+m+1)+6} \otimes w_{8j+1 \rightarrow 8(j+1)}.
\end{aligned}$$

(20) If  $r_0 = 19$ , then  $\Omega^{19}(Z_t^{(8)})$  is described with  $(16s \times 9s)$  matrix with the following nonzero entries:

$$\begin{aligned}
b_{s+(j+1)s,0} &= -w_{8(j+m+1)+6 \rightarrow 8(j+m+1)+7} \otimes w_{8j \rightarrow 8(j+1)}; \\
b_{2s+(j+1)s,0} &= -w_{8(j+m+1)+1 \rightarrow 8(j+m+1)+7} \otimes w_{8j \rightarrow 8(j+1)}; \\
b_{s+(j+1)s,s} &= -w_{8(j+m+1)+6 \rightarrow 8(j+m+2)} \otimes w_{8j+1 \rightarrow 8(j+1)}; \\
b_{2s+(j+1)s,s} &= -w_{8(j+m+1)+1 \rightarrow 8(j+m+2)} \otimes w_{8j+1 \rightarrow 8(j+1)}; \\
b_{(j+1)s,2s} &= -w_{8(j+m+1)+3 \rightarrow 8(j+m+2)+1} \otimes w_{8j+2 \rightarrow 8(j+1)}; \\
b_{4s+(j+1)s,3s} &= -w_{8(j+m+2) \rightarrow 8(j+m+2)+2} \otimes w_{8j+3 \rightarrow 8(j+1)+1}.
\end{aligned}$$

(21) If  $r_0 = 20$ , then  $\Omega^{20}(Z_t^{(8)})$  is described with  $(16s \times 8s)$  matrix with the following nonzero entries:

$$\begin{aligned}
b_{(j+1)s,s} &= -w_{8(j+m)+7 \rightarrow 8(j+m+1)+1} \otimes w_{8j+1 \rightarrow 8(j+1)}; \\
b_{s+(j+1)s,2s} &= w_{8(j+m+1) \rightarrow 8(j+m+1)+2} \otimes w_{8j+2 \rightarrow 8(j+1)}; \\
b_{(j+1)s,3s} &= w_{8(j+m)+7 \rightarrow 8(j+m+1)+3} \otimes w_{8j+3 \rightarrow 8(j+1)}; \\
b_{s+(j+1)s,3s} &= -w_{8(j+m+1) \rightarrow 8(j+m+1)+3} \otimes w_{8j+3 \rightarrow 8(j+1)}; \\
b_{4s+(j+1)s,3s} &= -e_{8(j+m+1)+3} \otimes w_{8j+3 \rightarrow 8(j+1)+2}.
\end{aligned}$$

(22) If  $r_0 = 21$ , then  $\Omega^{21}(Z_t^{(8)})$  is described with  $(14s \times 8s)$  matrix with the following nonzero entries:

$$b_{(j+1)s,2s} = -w_{8(j+m+1)+2 \rightarrow 8(j+m+2)+2} \otimes w_{8j+2 \rightarrow 8(j+1)};$$

$$b_{s+(j+1)s,2s} = -w_{8(j+m+1)+4 \rightarrow 8(j+m+2)+2} \otimes w_{8j+2 \rightarrow 8(j+1)};$$

$$b_{3s+(j+1)s,3s} = -w_{8(j+m+1)+7 \rightarrow 8(j+m+2)+3} \otimes w_{8j+3 \rightarrow 8(j+1)+1}.$$

(23) If  $r_0 = 22$ , then  $\Omega^{22}(Z_t^{(8)})$  is described with  $(13s \times 9s)$  matrix with the following nonzero entries:

$$b_{(j+1)s,2s} = w_{8(j+m+1) \rightarrow 8(j+m+1)+2} \otimes w_{8j+1 \rightarrow 8(j+1)};$$

$$b_{s+(j+1)s,3s} = -w_{8(j+m)+7 \rightarrow 8(j+m+1)+3} \otimes w_{8j+2 \rightarrow 8(j+1)};$$

$$b_{(j+1)s,4s} = -w_{8(j+m+1) \rightarrow 8(j+m+1)+4} \otimes w_{8j+3 \rightarrow 8(j+1)};$$

$$b_{s+(j+1)s,4s} = w_{8(j+m)+7 \rightarrow 8(j+m+1)+4} \otimes w_{8j+3 \rightarrow 8(j+1)};$$

$$b_{3s+(j+1)s,4s} = e_{8(j+m+1)+4} \otimes w_{8j+3 \rightarrow 8(j+1)+2}.$$

(24) If  $r_0 = 23$ , then  $\Omega^{23}(Z_t^{(8)})$  is described with  $(11s \times 8s)$  matrix with the following nonzero entries:

$$b_{(j+1)s,2s} = -w_{8(j+m+1)+3 \rightarrow 8(j+m+2)+3} \otimes w_{8j+2 \rightarrow 8(j+1)};$$

$$b_{2s+(j+1)s,2s} = -w_{8(j+m+2) \rightarrow 8(j+m+2)+3} \otimes w_{8j+2 \rightarrow 8(j+1)+1};$$

$$b_{2s+(j+1)s,3s} = -w_{8(j+m+2) \rightarrow 8(j+m+2)+4} \otimes w_{8j+3 \rightarrow 8(j+1)+1}.$$

(25) If  $r_0 = 24$ , then  $\Omega^{24}(Z_t^{(8)})$  is described with  $(11s \times 10s)$  matrix with two nonzero entries:

$$b_{(j+1)s,2s} = w_{8(j+m+1) \rightarrow 8(j+m+1)+3} \otimes w_{8j+1 \rightarrow 8(j+1)};$$

$$b_{2s+(j+1)s,4s} = -w_{8(j+m+1)+5 \rightarrow 8(j+m+1)+7} \otimes w_{8j+3 \rightarrow 8(j+1)+1}.$$

(26) If  $r_0 = 25$ , then  $\Omega^{25}(Z_t^{(8)})$  is described with  $(10s \times 11s)$  matrix with the following nonzero entries:

$$b_{(j+1)s,0} = w_{8(j+m+1)+4 \rightarrow 8(j+m+1)+7} \otimes w_{8j \rightarrow 8(j+1)};$$

$$b_{s+(j+1)s,4s} = w_{8(j+m+1)+6 \rightarrow 8(j+m+2)+5} \otimes w_{8j+3 \rightarrow 8(j+1)};$$

$$b_{3s+(j+1)s,4s} = w_{8(j+m+2) \rightarrow 8(j+m+2)+5} \otimes w_{8j+3 \rightarrow 8(j+1)+2}.$$

(27) If  $r_0 = 26$ , then  $\Omega^{26}(Z_t^{(8)})$  is described with  $(8s \times 11s)$  matrix with the following nonzero entries:

$$b_{(j+1)s,0} = w_{8(j+m)+7 \rightarrow 8(j+m+1)+5} \otimes w_{8j \rightarrow 8(j+1)};$$

$$b_{(j+1)s,s} = w_{8(j+m)+7 \rightarrow 8(j+m+1)+3} \otimes w_{8j \rightarrow 8(j+1)};$$

$$b_{(j+1)s,4s} = w_{8(j+m)+7 \rightarrow 8(j+m+1)+7} \otimes w_{8j+2 \rightarrow 8(j+1)};$$

$$b_{s+(j+1)s,4s} = -w_{8(j+m+1)+6 \rightarrow 8(j+m+1)+7} \otimes w_{8j+2 \rightarrow 8(j+1)+1};$$

$$b_{s+(j+1)s,5s} = w_{8(j+m+1)+6 \rightarrow 8(j+m+2)} \otimes w_{8j+3 \rightarrow 8(j+1)+1}.$$

(28) If  $r_0 = 27$ , then  $\Omega^{27}(Z_t^{(8)})$  is described with  $(9s \times 13s)$  matrix with two nonzero entries:

$$b_{(j+1)s,0} = -e_{8(j+m+1)+7} \otimes w_{8j \rightarrow 8(j+1)};$$

$$b_{(j+1)s,4s} = -w_{8(j+m+1)+7 \rightarrow 8(j+m+2)+6} \otimes w_{8j+3 \rightarrow 8(j+1)}.$$

(29) If  $r_0 = 28$ , then  $\Omega^{28}(Z_t^{(8)})$  is described with  $(8s \times 14s)$  matrix with two nonzero entries:

$$b_{(j+1)s,0} = -w_{8(j+m+1) \rightarrow 8(j+m+1)+2} \otimes w_{8j \rightarrow 8(j+1)};$$

$$b_{j+s,6s} = -w_{8(j+m)+7 \rightarrow 8(j+m+1)+7} \otimes w_{8j+3 \rightarrow 8j+7}.$$

(II) Represent an arbitrary  $t_0 \in \mathbb{N}$  in the form  $t_0 = 29\ell_0 + r_0$ , where  $0 \leq r_0 \leq 28$ . Then  $\Omega^{t_0}(Z_t^{(8)})$  is a  $\Omega^{r_0}(Z_t^{(8)})$ , whose left components twisted by  $\sigma^{\ell_0}$ , and coefficients multiplied by  $(-1)^{\ell_0}$ .

**Proposition 8** (Translates for the case 9). (I) Let  $r_0 \in \mathbb{N}$ ,  $r_0 < 29$ .  $r_0$ -translates of the elements  $Z_t^{(9)}$  are described by the following way.

(1) If  $r_0 = 0$ , then  $\Omega^0(Z_t^{(9)})$  is described with  $(8s \times 16s)$  matrix, whose entries  $b_{ij}$  have the following form:

If  $s \leq j < 2s$ , then

$$b_{ij} = \begin{cases} w_{8(j+m) \rightarrow 8(j+m)+3} \otimes e_{8j}, & i = j - s; \\ 0, & \text{otherwise.} \end{cases}$$

If  $2s \leq j < 3s$ , then  $b_{ij} = 0$ .

If  $3s \leq j < 4s$ , then

$$b_{ij} = \begin{cases} w_{8(j+m) \rightarrow 8(j+m)+1} \otimes e_{8j}, & i = j - 3s; \\ 0, & \text{otherwise.} \end{cases}$$

If  $4s \leq j < 5s$ , then

$$b_{ij} = \begin{cases} w_{8(j+m)+1 \rightarrow 8(j+m)+1} \otimes e_{8j+1}, & i = j - 3s; \\ 0, & \text{otherwise.} \end{cases}$$

If  $5s \leq j < 6s$ , then

$$b_{ij} = \begin{cases} w_{8(j+m)+2 \rightarrow 8(j+m)+7} \otimes e_{8j+2}, & i = j - 3s; \\ 0, & \text{otherwise.} \end{cases}$$

If  $6s \leq j < 7s$ , then

$$b_{ij} = \begin{cases} w_{8(j+m)+3 \rightarrow 8(j+m)+1} \otimes e_{8j+3}, & i = j - 3s; \\ 0, & \text{otherwise.} \end{cases}$$

If  $7s \leq j < 8s$ , then

$$b_{ij} = \begin{cases} w_{8(j+m)+4 \rightarrow 8(j+m)+7} \otimes e_{8j+4}, & i = j - 3s; \\ 0, & \text{otherwise.} \end{cases}$$

If  $8s \leq j < 9s$ , then

$$b_{ij} = \begin{cases} w_{8(j+m)+5 \rightarrow 8(j+m)+7} \otimes e_{8j+5}, & i = j - 3s; \\ 0, & \text{otherwise.} \end{cases}$$

If  $9s \leq j < 10s$ , then

$$b_{ij} = \begin{cases} -w_{8(j+m)+5 \rightarrow 8(j+m)+1} \otimes e_{8j+5}, & i = j - 4s; \\ 0, & \text{otherwise.} \end{cases}$$

If  $10s \leq j < 12s$ , then  $b_{ij} = 0$ .

If  $12s \leq j < 13s$ , then

$$b_{ij} = \begin{cases} w_{8(j+m)+7 \rightarrow 8(j+m)+2} \otimes e_{8j+7}, & i = j - 5s; \\ 0, & \text{otherwise.} \end{cases}$$

If  $13s \leq j < 14s$ , then

$$b_{ij} = \begin{cases} -2w_{8(j+m)+7 \rightarrow 8(j+m+1)+4} \otimes e_{8j+7}, & i = j - 6s; \\ 0, & \text{otherwise.} \end{cases}$$

If  $14s \leq j < 16s$ , then  $b_{ij} = 0$ .

(2) If  $r_0 = 1$ , then  $\Omega^1(Z_t^{(9)})$  is described with  $(9s \times 19s)$  matrix, whose entries  $b_{ij}$  have the following form:

If  $0 \leq j < s$ , then

$$b_{ij} = \begin{cases} 2w_{8(j+m)+1 \rightarrow 8(j+m)+7} \otimes e_{8j}, & i = j; \\ w_{8(j+m)+5 \rightarrow 8(j+m)+7} \otimes e_{8j}, & i = j + s; \\ 2w_{8(j+m)+2 \rightarrow 8(j+m)+7} \otimes w_{8j \rightarrow 8j+1}, & i = j + 2s; \\ w_{8(j+m)+3 \rightarrow 8(j+m)+7} \otimes w_{8j \rightarrow 8j+2}, & i = j + 3s; \\ w_{8(j+m)+4 \rightarrow 8(j+m)+7} \otimes w_{8j \rightarrow 8j+3}, & i = j + 4s; \\ 0, & \text{otherwise.} \end{cases}$$

If  $s \leq j < 2s$ , then

$$b_{ij} = \begin{cases} w_{8(j+m)+1 \rightarrow 8(j+m+1)} \otimes e_{8j}, & i = j - s; \\ w_{8(j+m)+2 \rightarrow 8(j+m+1)} \otimes w_{8j \rightarrow 8j+1}, & i = j + s; \\ w_{8(j+m)+3 \rightarrow 8(j+m+1)} \otimes w_{8j \rightarrow 8j+2}, & i = j + 2s; \\ 0, & \text{otherwise.} \end{cases}$$

If  $2s \leq j < 3s$ , then

$$b_{ij} = \begin{cases} -w_{8(j+m)+1 \rightarrow 8(j+m+1)} \otimes e_{8j}, & i = j - 2s; \\ w_{8(j+m)+5 \rightarrow 8(j+m+1)} \otimes e_{8j}, & i = j - s; \\ 0, & \text{otherwise.} \end{cases}$$

If  $3s \leq j < 4s$ , then  $b_{ij} = 0$ .

If  $4s \leq j < 5s$ , then

$$b_{ij} = \begin{cases} w_{8(j+m)+2 \rightarrow 8(j+m+1)+1} \otimes e_{8j+1}, & i = j - 2s; \\ w_{8(j+m)+3 \rightarrow 8(j+m+1)+1} \otimes w_{8j+1 \rightarrow 8j+2}, & i = j - s; \\ w_{8(j+m)+4 \rightarrow 8(j+m+1)+1} \otimes w_{8j+1 \rightarrow 8j+3}, & i = j; \\ w_{8(j+m)+7 \rightarrow 8(j+m+1)+1} \otimes w_{8j+1 \rightarrow 8j+4}, & i = j + s; \\ w_{8(j+m+1) \rightarrow 8(j+m+1)+1} \otimes w_{8j+1 \rightarrow 8j+7}, & i = j + 4s; \\ 0, & \text{otherwise.} \end{cases}$$

If  $5s \leq j < 6s$ , then

$$b_{ij} = \begin{cases} w_{8(j+m)+3 \rightarrow 8(j+m+1)+2} \otimes e_{8j+2}, & i = j - 2s; \\ 2w_{8(j+m)+4 \rightarrow 8(j+m+1)+2} \otimes w_{8j+2 \rightarrow 8j+3}, & i = j - s; \\ -2w_{8(j+m)+7 \rightarrow 8(j+m+1)+2} \otimes w_{8j+2 \rightarrow 8j+4}, & i = j; \\ -w_{8(j+m+1) \rightarrow 8(j+m+1)+2} \otimes w_{8j+2 \rightarrow 8j+7}, & i = j + 3s; \\ 0, & \text{otherwise.} \end{cases}$$

If  $6s \leq j < 7s$ , then

$$b_{ij} = \begin{cases} w_{8(j+m)+4 \rightarrow 8(j+m+1)+3} \otimes e_{8j+3}, & i = j - 2s; \\ 2w_{8(j+m)+7 \rightarrow 8(j+m+1)+3} \otimes w_{8j+3 \rightarrow 8j+4}, & i = j - s; \\ -2w_{8(j+m+1) \rightarrow 8(j+m+1)+3} \otimes w_{8j+3 \rightarrow 8j+7}, & i = j + 2s; \\ 0, & \text{otherwise.} \end{cases}$$

If  $7s \leq j < 8s$ , then  $b_{ij} = 0$ .

If  $8s \leq j < 9s$ , then

$$b_{ij} = \begin{cases} w_{8(j+m)+7 \rightarrow 8(j+m+1)+4} \otimes e_{8j+4}, & i = j - 3s; \\ -w_{8(j+m+1) \rightarrow 8(j+m+1)+4} \otimes w_{8j+4 \rightarrow 8j+7}, & i = j; \\ 0, & \text{otherwise.} \end{cases}$$

If  $9s \leq j < 11s$ , then  $b_{ij} = 0$ .

If  $11s \leq j < 12s$ , then

$$b_{ij} = \begin{cases} 2w_{8(j+m)+7 \rightarrow 8(j+m+1)+4} \otimes w_{8j+5 \rightarrow 8j+6}, & i = j - 4s; \\ 0, & \text{otherwise.} \end{cases}$$

If  $12s \leq j < 13s$ , then

$$b_{ij} = \begin{cases} e_{8(j+m+1)+1} \otimes w_{8j+5 \rightarrow 8(j+1)}, & i = (j+1)_s; \\ 0, & \text{otherwise.} \end{cases}$$

If  $13s \leq j < 14s$ , then

$$b_{ij} = \begin{cases} -w_{8(j+m)+7 \rightarrow 8(j+m+1)+2} \otimes e_{8j+6}, & i = j - 6s; \\ 0, & \text{otherwise.} \end{cases}$$

If  $14s \leq j < 16s$ , then  $b_{ij} = 0$ .

If  $16s \leq j < 17s$ , then

$$b_{ij} = \begin{cases} w_{8(j+m+1)+1 \rightarrow 8(j+m+1)+7} \otimes w_{8j+7 \rightarrow 8(j+1)}, & i = (j+1)_s; \\ w_{8(j+m+1)+2 \rightarrow 8(j+m+1)+7} \otimes w_{8j+7 \rightarrow 8(j+1)+1}, & i = 2s + (j+1)_s; \\ w_{8(j+m+1) \rightarrow 8(j+m+1)+7} \otimes e_{8j+7}, & i = j - 8s; \\ 0, & \text{otherwise.} \end{cases}$$

If  $17s \leq j < 18s$ , then

$$b_{ij} = \begin{cases} w_{8(j+m+1)+1 \rightarrow 8(j+m+1)+7} \otimes w_{8j+7 \rightarrow 8(j+1)}, & i = (j+1)_s; \\ w_{8(j+m+1)+5 \rightarrow 8(j+m+1)+7} \otimes w_{8j+7 \rightarrow 8(j+1)}, & i = s + (j+1)_s; \\ w_{8(j+m+1)+2 \rightarrow 8(j+m+1)+7} \otimes w_{8j+7 \rightarrow 8(j+1)+1}, & i = 2s + (j+1)_s; \\ -2w_{8(j+m+1) \rightarrow 8(j+m+1)+7} \otimes e_{8j+7}, & i = j - 9s; \\ 0, & \text{otherwise.} \end{cases}$$

If  $18s \leq j < 19s$ , then

$$b_{ij} = \begin{cases} w_{8(j+m+1)+1 \rightarrow 8(j+m+2)} \otimes w_{8j+7 \rightarrow 8(j+1)}, & i = (j+1)_s; \\ w_{8(j+m+1) \rightarrow 8(j+m+2)} \otimes e_{8j+7}, & i = j - 10s; \\ 0, & \text{otherwise.} \end{cases}$$

(3) If  $r_0 = 2$ , then  $\Omega^2(Z_t^{(9)})$  is described with  $(8s \times 18s)$  matrix, whose entries  $b_{ij}$  have the following form:

If  $0 \leq j < s$ , then

$$b_{ij} = \begin{cases} -w_{8(j+m-1)+7 \rightarrow 8(j+m)+2} \otimes e_{8j}, & i = j; \\ -e_{8(j+m)+2} \otimes w_{8j \rightarrow 8j+1}, & i = j + s; \\ 0, & \text{otherwise.} \end{cases}$$

If  $s \leq j < 2s$ , then  $b_{ij} = 0$ .

If  $2s \leq j < 3s$ , then

$$b_{ij} = \begin{cases} 2w_{8(j+m-1)+7 \rightarrow 8(j+m)+4} \otimes e_{8j}, & i = j - 2s; \\ -w_{8(j+m)+2 \rightarrow 8(j+m)+4} \otimes w_{8j \rightarrow 8j+1}, & i = j - s; \\ 0, & \text{otherwise.} \end{cases}$$

If  $3s \leq j < 4s$ , then

$$b_{ij} = \begin{cases} -w_{8(j+m-1)+7 \rightarrow 8(j+m)+1} \otimes e_{8j}, & i = j - 3s; \\ -e_{8(j+m)+1} \otimes w_{8j \rightarrow 8j+6}, & i = j + 3s; \\ 0, & \text{otherwise.} \end{cases}$$

If  $4s \leq j < 5s$ , then  $b_{ij} = 0$ .

If  $5s \leq j < 6s$ , then

$$b_{ij} = \begin{cases} -e_{8(j+m)+7} \otimes w_{8j+1 \rightarrow 8(j+1)}, & i = (j+1)_s; \\ -2w_{8(j+m)+2 \rightarrow 8(j+m)+7} \otimes e_{8j+1}, & i = j - 4s; \\ 0, & \text{otherwise.} \end{cases}$$

If  $6s \leq j < 7s$ , then

$$b_{ij} = \begin{cases} w_{8(j+m)+3 \rightarrow 8(j+m+1)} \otimes e_{8j+2}, & i = j - 4s; \\ 0, & \text{otherwise.} \end{cases}$$

If  $7s \leq j < 8s$ , then

$$b_{ij} = \begin{cases} -e_{8(j+m)+7} \otimes w_{8j+3 \rightarrow 8(j+1)}, & i = (j+1)_s; \\ 2w_{8(j+m)+4 \rightarrow 8(j+m)+7} \otimes e_{8j+3}, & i = j - 4s; \\ 0, & \text{otherwise.} \end{cases}$$

If  $8s \leq j < 9s$ , then

$$b_{ij} = \begin{cases} w_{8(j+m)+5 \rightarrow 8(j+m)+7} \otimes e_{8j+4}, & i = j - 4s; \\ 0, & \text{otherwise.} \end{cases}$$

If  $9s \leq j < 10s$ , then

$$b_{ij} = \begin{cases} -w_{8(j+m)+5 \rightarrow 8(j+m+1)} \otimes e_{8j+4}, & i = j - 5s; \\ 0, & \text{otherwise.} \end{cases}$$

If  $10s \leq j < 11s$ , then

$$b_{ij} = \begin{cases} -2e_{8(j+m)+7} \otimes w_{8j+5 \rightarrow 8(j+1)}, & i = (j+1)_s; \\ -2w_{8(j+m)+6 \rightarrow 8(j+m)+7} \otimes e_{8j+5}, & i = j - 5s; \\ 0, & \text{otherwise.} \end{cases}$$

If  $11s \leq j < 12s$ , then

$$b_{ij} = \begin{cases} 2w_{8(j+m)+7 \rightarrow 8(j+m)+1} \otimes w_{8j+5 \rightarrow 8(j+1)}, & i = (j+1)_s; \\ 2w_{8(j+m)+6 \rightarrow 8(j+m)+1} \otimes e_{8j+5}, & i = j - 6s; \\ 0, & \text{otherwise.} \end{cases}$$

If  $12s \leq j < 13s$ , then

$$b_{ij} = \begin{cases} -w_{8(j+m)+1 \rightarrow 8(j+m)+7} \otimes e_{8j+6}, & i = j - 6s; \\ 0, & \text{otherwise.} \end{cases}$$

If  $13s \leq j < 14s$ , then

$$b_{ij} = \begin{cases} -w_{8(j+m)+1 \rightarrow 8(j+m)+1} \otimes e_{8j+6}, & i = j - 7s; \\ 0, & \text{otherwise.} \end{cases}$$

If  $14s \leq j < 15s$ , then  $b_{ij} = 0$ .

If  $15s \leq j < 16s$ , then

$$b_{ij} = \begin{cases} w_{8(j+m)+2 \rightarrow 8(j+m)+3} \otimes w_{8j+7 \rightarrow 8(j+1)+1}, & i = s + (j+1)_s; \\ 0, & \text{otherwise.} \end{cases}$$

If  $16s \leq j < 17s$ , then  $b_{ij} = 0$ .

If  $17s \leq j < 18s$ , then

$$b_{ij} = \begin{cases} w_{8(j+m)+7 \rightarrow 8(j+m)+1} \otimes w_{8j+7 \rightarrow 8(j+1)}, & i = (j+1)_s; \\ e_{8(j+m)+1} \otimes w_{8j+7 \rightarrow 8(j+1)+6}, & i = 6s + (j+1)_s; \\ 0, & \text{otherwise.} \end{cases}$$

(4) If  $r_0 = 3$ , then  $\Omega^3(Z_t^{(9)})$  is described with  $(10s \times 19s)$  matrix, whose entries  $b_{ij}$  have the following form:

If  $0 \leq j < s$ , then

$$b_{ij} = \begin{cases} 2w_{8(j+m)+3 \rightarrow 8(j+m)+7} \otimes w_{8j \rightarrow 8j+1}, & i = j + 2s; \\ 2w_{8(j+m)+4 \rightarrow 8(j+m)+7} \otimes w_{8j \rightarrow 8j+2}, & i = j + 3s; \\ 0, & \text{otherwise.} \end{cases}$$

If  $s \leq j < 2s$ , then

$$b_{ij} = \begin{cases} -2w_{8(j+m)+2 \rightarrow 8(j+m)+1} \otimes e_{8j}, & i = j - s; \\ -2w_{8(j+m)+6 \rightarrow 8(j+m)+1} \otimes e_{8j}, & i = j; \\ -2w_{8(j+m)+3 \rightarrow 8(j+m)+1} \otimes w_{8j \rightarrow 8j+1}, & i = j + s; \\ 2w_{8(j+m)+4 \rightarrow 8(j+m)+1} \otimes w_{8j \rightarrow 8j+2}, & i = j + 2s; \\ 2w_{8(j+m)+7 \rightarrow 8(j+m)+1} \otimes w_{8j \rightarrow 8j+3}, & i = j + 3s; \\ 0, & \text{otherwise.} \end{cases}$$



If  $2s \leq j < 3s$ , then

$$b_{ij} = \begin{cases} 2w_{8(j+m)+6 \rightarrow 8(j+m)+7} \otimes e_{8j}, & i = j - s; \\ -w_{8(j+m)+3 \rightarrow 8(j+m)+7} \otimes w_{8j \rightarrow 8j+1}, & i = j; \\ -w_{8(j+m)+4 \rightarrow 8(j+m)+7} \otimes w_{8j \rightarrow 8j+2}, & i = j + s; \\ 2e_{8(j+m)+7} \otimes w_{8j \rightarrow 8j+3}, & i = j + 2s; \\ 0, & \text{otherwise.} \end{cases}$$

If  $3s \leq j < 4s$ , then

$$b_{ij} = \begin{cases} -e_{8(j+m+1)+2} \otimes w_{8j+1 \rightarrow 8(j+1)}, & i = (j+1)_s; \\ -2w_{8(j+m)+3 \rightarrow 8(j+m+1)+2} \otimes e_{8j+1}, & i = j - s; \\ -w_{8(j+m)+4 \rightarrow 8(j+m+1)+2} \otimes w_{8j+1 \rightarrow 8j+2}, & i = j; \\ -w_{8(j+m)+7 \rightarrow 8(j+m+1)+2} \otimes w_{8j+1 \rightarrow 8j+3}, & i = j + s; \\ 0, & \text{otherwise.} \end{cases}$$

If  $4s \leq j < 5s$ , then

$$b_{ij} = \begin{cases} -2w_{8(j+m+1)+2 \rightarrow 8(j+m+1)+3} \otimes w_{8j+2 \rightarrow 8(j+1)}, & i = (j+1)_s; \\ w_{8(j+m)+4 \rightarrow 8(j+m+1)+3} \otimes e_{8j+2}, & i = j - s; \\ -2w_{8(j+m)+7 \rightarrow 8(j+m+1)+3} \otimes w_{8j+2 \rightarrow 8j+3}, & i = j; \\ 0, & \text{otherwise.} \end{cases}$$

If  $5s \leq j < 6s$ , then  $b_{ij} = 0$ .

If  $6s \leq j < 7s$ , then

$$b_{ij} = \begin{cases} -w_{8(j+m+1)+2 \rightarrow 8(j+m+1)+4} \otimes w_{8j+3 \rightarrow 8(j+1)}, & i = (j+1)_s; \\ 2w_{8(j+m)+7 \rightarrow 8(j+m+1)+4} \otimes e_{8j+3}, & i = j - 2s; \\ 0, & \text{otherwise.} \end{cases}$$

If  $7s \leq j < 8s$ , then

$$b_{ij} = \begin{cases} -e_{8(j+m+1)+6} \otimes w_{8j+3 \rightarrow 8(j+1)}, & i = s + (j+1)_s; \\ 0, & \text{otherwise.} \end{cases}$$

If  $8s \leq j < 11s$ , then  $b_{ij} = 0$ .

If  $11s \leq j < 12s$ , then

$$b_{ij} = \begin{cases} -2w_{8(j+m)+7 \rightarrow 8(j+m+1)+6} \otimes e_{8j+5}, & i = j - 5s; \\ 0, & \text{otherwise.} \end{cases}$$

If  $12s \leq j < 13s$ , then

$$b_{ij} = \begin{cases} 2w_{8(j+m)+7 \rightarrow 8(j+m+1)+5} \otimes e_{8j+5}, & i = j - 6s; \\ 0, & \text{otherwise.} \end{cases}$$

If  $13s \leq j < 15s$ , then  $b_{ij} = 0$ .

If  $15s \leq j < 16s$ , then

$$b_{ij} = \begin{cases} -w_{8(j+m+1) \rightarrow 8(j+m+1)+1} \otimes e_{8j+6}, & i = j - 8s; \\ -e_{8(j+m+1)+1} \otimes w_{8j+6 \rightarrow 8j+7}, & i = j - 7s; \\ 0, & \text{otherwise.} \end{cases}$$

If  $16s \leq j < 17s$ , then

$$b_{ij} = \begin{cases} -w_{8(j+m+1)+2 \rightarrow 8(j+m+1)+7} \otimes w_{8j+7 \rightarrow 8(j+1)}, & i = (j+1)_s; \\ 0, & \text{otherwise.} \end{cases}$$

If  $17s \leq j < 18s$ , then

$$b_{ij} = \begin{cases} w_{8(j+m+1)+3 \rightarrow 8(j+m+2)} \otimes w_{8j+7 \rightarrow 8(j+1)+1}, & i = 2s + (j+1)_s; \\ 0, & \text{otherwise.} \end{cases}$$

If  $18s \leq j < 19s$ , then

$$b_{ij} = \begin{cases} -w_{8(j+m+1)+2 \rightarrow 8(j+m+2)} \otimes w_{8j+7 \rightarrow 8(j+1)}, & i = (j+1)_s; \\ -2w_{8(j+m+1)+6 \rightarrow 8(j+m+2)} \otimes w_{8j+7 \rightarrow 8(j+1)}, & i = s + (j+1)_s; \\ 2w_{8(j+m+1)+3 \rightarrow 8(j+m+2)} \otimes w_{8j+7 \rightarrow 8(j+1)+1}, & i = 2s + (j+1)_s; \\ w_{8(j+m+1)+4 \rightarrow 8(j+m+2)} \otimes w_{8j+7 \rightarrow 8(j+1)+2}, & i = 3s + (j+1)_s; \\ -2w_{8(j+m+1)+7 \rightarrow 8(j+m+2)} \otimes w_{8j+7 \rightarrow 8(j+1)+3}, & i = 4s + (j+1)_s; \\ 0, & \text{otherwise.} \end{cases}$$

(5) If  $r_0 = 4$ , then  $\Omega^4(Z_t^{(9)})$  is described with  $(11s \times 18s)$  matrix, whose entries  $b_{ij}$  have the following form:

If  $0 \leq j < s$ , then

$$b_{ij} = \begin{cases} 2w_{8(j+m-1)+7 \rightarrow 8(j+m)+2} \otimes e_{8j}, & i = j; \\ 2w_{8(j+m) \rightarrow 8(j+m)+2} \otimes e_{8j}, & i = j + s; \\ -2w_{8(j+m)+1 \rightarrow 8(j+m)+2} \otimes w_{8j \rightarrow 8j+4}, & i = j + 6s; \\ e_{8(j+m)+2} \otimes w_{8j \rightarrow 8j+6}, & i = j + 8s; \\ 0, & \text{otherwise.} \end{cases}$$

If  $s \leq j < 2s$ , then

$$b_{ij} = \begin{cases} -e_{8(j+m)+3} \otimes w_{8j \rightarrow 8j+1}, & i = j + s; \\ 0, & \text{otherwise.} \end{cases}$$

If  $2s \leq j < 3s$ , then

$$b_{ij} = \begin{cases} -2w_{8(j+m-1)+7 \rightarrow 8(j+m)+6} \otimes e_{8j}, & i = j - 2s; \\ -w_{8(j+m)+5 \rightarrow 8(j+m)+6} \otimes w_{8j \rightarrow 8j+3}, & i = j + 2s; \\ e_{8(j+m)+6} \otimes w_{8j \rightarrow 8j+4}, & i = j + 3s; \\ 0, & \text{otherwise.} \end{cases}$$

If  $3s \leq j < 4s$ , then

$$b_{ij} = \begin{cases} 2w_{8(j+m-1)+7 \rightarrow 8(j+m)+5} \otimes e_{8j}, & i = j - 3s; \\ 0, & \text{otherwise.} \end{cases}$$

If  $4s \leq j < 5s$ , then

$$b_{ij} = \begin{cases} 2w_{8(j+m)+7 \rightarrow 8(j+m+1)} \otimes w_{8j+1 \rightarrow 8(j+1)}, & i = (j+1)_s; \\ 2e_{8(j+m+1)} \otimes w_{8j+1 \rightarrow 8(j+1)}, & i = s + (j+1)_s; \\ 0, & \text{otherwise.} \end{cases}$$

If  $5s \leq j < 6s$ , then

$$b_{ij} = \begin{cases} -2e_{8(j+m)+7} \otimes w_{8j+2 \rightarrow 8(j+1)}, & i = (j+1)_s; \\ w_{8(j+m)+4 \rightarrow 8(j+m)+7} \otimes e_{8j+2}, & i = j - 2s; \\ 0, & \text{otherwise.} \end{cases}$$

If  $6s \leq j < 7s$ , then

$$b_{ij} = \begin{cases} -2e_{8(j+m)+7} \otimes w_{8j+3 \rightarrow 8(j+1)}, & i = (j+1)_s; \\ 2w_{8(j+m)+5 \rightarrow 8(j+m)+7} \otimes e_{8j+3}, & i = j - 2s; \\ -2w_{8(j+m)+6 \rightarrow 8(j+m)+7} \otimes w_{8j+3 \rightarrow 8j+4}, & i = j - s; \\ 0, & \text{otherwise.} \end{cases}$$

If  $7s \leq j < 8s$ , then

$$b_{ij} = \begin{cases} -w_{8(j+m)+7 \rightarrow 8(j+m+1)} \otimes w_{8j+3 \rightarrow 8(j+1)}, & i = (j+1)_s; \\ -2e_{8(j+m+1)} \otimes w_{8j+3 \rightarrow 8(j+1)}, & i = s + (j+1)_s; \\ 0, & \text{otherwise.} \end{cases}$$

If  $8s \leq j < 10s$ , then  $b_{ij} = 0$ .

If  $10s \leq j < 11s$ , then

$$b_{ij} = \begin{cases} w_{8(j+m)+7 \rightarrow 8(j+m+1)} \otimes w_{8j+5 \rightarrow 8(j+1)}, & i = (j+1)_s; \\ e_{8(j+m+1)} \otimes w_{8j+5 \rightarrow 8(j+1)}, & i = s + (j+1)_s; \\ 0, & \text{otherwise.} \end{cases}$$

If  $11s \leq j < 12s$ , then

$$b_{ij} = \begin{cases} w_{8(j+m)+2 \rightarrow 8(j+m)+7} \otimes e_{8j+6}, & i = j - 3s; \\ 0, & \text{otherwise.} \end{cases}$$

If  $12s \leq j < 13s$ , then  $b_{ij} = 0$ .

If  $13s \leq j < 14s$ , then

$$b_{ij} = \begin{cases} -w_{8(j+m)+7 \rightarrow 8(j+m+1)+2} \otimes w_{8j+7 \rightarrow 8(j+1)}, & i = (j+1)_s; \\ -w_{8(j+m+1) \rightarrow 8(j+m+1)+2} \otimes w_{8j+7 \rightarrow 8(j+1)}, & i = s + (j+1)_s; \\ w_{8(j+m+1)+1 \rightarrow 8(j+m+1)+2} \otimes w_{8j+7 \rightarrow 8(j+1)+4}, & i = 6s + (j+1)_s; \\ -e_{8(j+m+1)+2} \otimes w_{8j+7 \rightarrow 8(j+1)+6}, & i = 8s + (j+1)_s; \\ 0, & \text{otherwise.} \end{cases}$$

If  $14s \leq j < 15s$ , then

$$b_{ij} = \begin{cases} 2w_{8(j+m)+7 \rightarrow 8(j+m+1)+6} \otimes w_{8j+7 \rightarrow 8(j+1)}, & i = (j+1)_s; \\ 0, & \text{otherwise.} \end{cases}$$

If  $15s \leq j < 16s$ , then

$$b_{ij} = \begin{cases} w_{8(j+m+1)+3 \rightarrow 8(j+m+1)+4} \otimes w_{8j+7 \rightarrow 8(j+1)+1}, & i = 2s + (j+1)_s; \\ 0, & \text{otherwise.} \end{cases}$$

If  $16s \leq j < 17s$ , then

$$b_{ij} = \begin{cases} w_{8(j+m)+7 \rightarrow 8(j+m+1)+1} \otimes w_{8j+7 \rightarrow 8(j+1)}, & i = (j+1)_s; \\ w_{8(j+m+1) \rightarrow 8(j+m+1)+1} \otimes w_{8j+7 \rightarrow 8(j+1)}, & i = s + (j+1)_s; \\ -e_{8(j+m+1)+1} \otimes w_{8j+7 \rightarrow 8(j+1)+4}, & i = 6s + (j+1)_s; \\ 0, & \text{otherwise.} \end{cases}$$

If  $17s \leq j < 18s$ , then  $b_{ij} = 0$ .

(6) If  $r_0 = 5$ , then  $\Omega^5(Z_t^{(9)})$  is described with  $(11s \times 20s)$  matrix, whose entries  $b_{ij}$  have the following form:

If  $0 \leq j < s$ , then

$$b_{ij} = \begin{cases} 2w_{8(j+m)+3 \rightarrow 8(j+m)+7} \otimes e_{8j}, & i = j + s; \\ 2w_{8(j+m)+1 \rightarrow 8(j+m)+7} \otimes e_{8j}, & i = j + 2s; \\ -2w_{8(j+m)+4 \rightarrow 8(j+m)+7} \otimes w_{8j \rightarrow 8j+1}, & i = j + 3s; \\ -e_{8(j+m)+7} \otimes w_{8j \rightarrow 8j+2}, & i = j + 4s; \\ 0, & \text{otherwise.} \end{cases}$$

If  $s \leq j < 2s$ , then

$$b_{ij} = \begin{cases} -w_{8(j+m)+4 \rightarrow 8(j+m+1)} \otimes w_{8j \rightarrow 8j+1}, & i = j + 2s; \\ -2w_{8(j+m)+7 \rightarrow 8(j+m+1)} \otimes w_{8j \rightarrow 8j+2}, & i = j + 3s; \\ e_{8(j+m+1)} \otimes w_{8j \rightarrow 8j+3}, & i = j + 4s; \\ 0, & \text{otherwise.} \end{cases}$$

If  $2s \leq j < 3s$ , then

$$b_{ij} = \begin{cases} -e_{8(j+m+1)} \otimes w_{8j \rightarrow 8j+3}, & i = j + 3s; \\ 0, & \text{otherwise.} \end{cases}$$

If  $3s \leq j < 4s$ , then

$$b_{ij} = \begin{cases} -e_{8(j+m+1)+3} \otimes w_{8j+1 \rightarrow 8(j+1)}, & i = s + (j+1)_s; \\ -w_{8(j+m+1)+1 \rightarrow 8(j+m+1)+3} \otimes w_{8j+1 \rightarrow 8(j+1)}, & i = 2s + (j+1)_s; \\ 0, & \text{otherwise.} \end{cases}$$

If  $4s \leq j < 5s$ , then

$$b_{ij} = \begin{cases} 2e_{8(j+m+1)+5} \otimes w_{8j+1 \rightarrow 8(j+1)}, & i = (j+1)_s; \\ 0, & \text{otherwise.} \end{cases}$$

If  $5s \leq j < 6s$ , then

$$b_{ij} = \begin{cases} -2w_{8(j+m+1)+3 \rightarrow 8(j+m+1)+4} \otimes w_{8j+2 \rightarrow 8(j+1)}, & i = s + (j+1)_s; \\ w_{8(j+m)+7 \rightarrow 8(j+m+1)+4} \otimes e_{8j+2}, & i = j - s; \\ 0, & \text{otherwise.} \end{cases}$$

If  $6s \leq j < 7s$ , then  $b_{ij} = 0$ .

If  $7s \leq j < 8s$ , then

$$b_{ij} = \begin{cases} 2w_{8(j+m+1) \rightarrow 8(j+m+1)+5} \otimes e_{8j+3}, & i = j - 2s; \\ 0, & \text{otherwise.} \end{cases}$$

If  $8s \leq j < 9s$ , then

$$b_{ij} = \begin{cases} -e_{8(j+m+1)+1} \otimes w_{8j+3 \rightarrow 8(j+1)}, & i = 2s + (j+1)_s; \\ 0, & \text{otherwise.} \end{cases}$$

If  $9s \leq j < 11s$ , then  $b_{ij} = 0$ .

If  $11s \leq j < 12s$ , then

$$b_{ij} = \begin{cases} w_{8(j+m+1)+5 \rightarrow 8(j+m+1)+6} \otimes w_{8j+5 \rightarrow 8(j+1)}, & i = (j+1)_s; \\ 0, & \text{otherwise.} \end{cases}$$

If  $12s \leq j < 14s$ , then  $b_{ij} = 0$ .

If  $14s \leq j < 15s$ , then

$$b_{ij} = \begin{cases} w_{8(j+m)+7 \rightarrow 8(j+m+1)+2} \otimes e_{8j+6}, & i = j - 6s; \\ e_{8(j+m+1)+2} \otimes w_{8j+6 \rightarrow 8j+7}, & i = j - 5s; \\ 0, & \text{otherwise.} \end{cases}$$

If  $15s \leq j < 18s$ , then  $b_{ij} = 0$ .

If  $18s \leq j < 19s$ , then

$$b_{ij} = \begin{cases} -w_{8(j+m+1)+3 \rightarrow 8(j+m+2)} \otimes w_{8j+7 \rightarrow 8(j+1)}, & i = s + (j+1)_s; \\ -w_{8(j+m+1)+1 \rightarrow 8(j+m+2)} \otimes w_{8j+7 \rightarrow 8(j+1)}, & i = 2s + (j+1)_s; \\ -2w_{8(j+m+1)+4 \rightarrow 8(j+m+2)} \otimes w_{8j+7 \rightarrow 8(j+1)+1}, & i = 3s + (j+1)_s; \\ -w_{8(j+m+1)+7 \rightarrow 8(j+m+2)} \otimes w_{8j+7 \rightarrow 8(j+1)+2}, & i = 4s + (j+1)_s; \\ -e_{8(j+m+2)} \otimes w_{8j+7 \rightarrow 8(j+1)+3}, & i = 5s + (j+1)_s; \\ 0, & \text{otherwise.} \end{cases}$$

If  $19s \leq j < 20s$ , then

$$b_{ij} = \begin{cases} w_{8(j+m+1)+4 \rightarrow 8(j+m+1)+7} \otimes w_{8j+7 \rightarrow 8(j+1)+1}, & i = 3s + (j+1)_s; \\ 0, & \text{otherwise.} \end{cases}$$

(7) If  $r_0 = 6$ , then  $\Omega^6(Z_t^{(9)})$  is described with  $(13s \times 18s)$  matrix, whose entries  $b_{ij}$  have the following form:

If  $0 \leq j < s$ , then

$$b_{ij} = \begin{cases} -2w_{8(j+m-1)+7 \rightarrow 8(j+m)+3} \otimes e_{8j}, & i = j; \\ w_{8(j+m)+1 \rightarrow 8(j+m)+3} \otimes w_{8j \rightarrow 8j+3}, & i = j + 5s; \\ 2w_{8(j+m)+2 \rightarrow 8(j+m)+3} \otimes w_{8j \rightarrow 8j+4}, & i = j + 6s; \\ e_{8(j+m)+3} \otimes w_{8j \rightarrow 8j+6}, & i = j + 9s; \\ 0, & \text{otherwise.} \end{cases}$$

If  $s \leq j < 2s$ , then

$$b_{ij} = \begin{cases} -w_{8(j+m)+5 \rightarrow 8(j+m)+6} \otimes w_{8j \rightarrow 8j+2}, & i = j + 2s; \\ 0, & \text{otherwise.} \end{cases}$$

If  $2s \leq j < 3s$ , then

$$b_{ij} = \begin{cases} -e_{8(j+m)+4} \otimes w_{8j \rightarrow 8j+1}, & i = j; \\ w_{8(j+m)+1 \rightarrow 8(j+m)+4} \otimes w_{8j \rightarrow 8j+3}, & i = j + 3s; \\ 0, & \text{otherwise.} \end{cases}$$

If  $3s \leq j < 4s$ , then

$$b_{ij} = \begin{cases} -e_{8(j+m)+1} \otimes w_{8j \rightarrow 8j+3}, & i = j + 2s; \\ 0, & \text{otherwise.} \end{cases}$$

If  $4s \leq j < 5s$ , then

$$b_{ij} = \begin{cases} -2e_{8(j+m)+5} \otimes w_{8j \rightarrow 8j+2}, & i = j - s; \\ 0, & \text{otherwise.} \end{cases}$$

If  $5s \leq j < 6s$ , then

$$b_{ij} = \begin{cases} -2e_{8(j+m)+7} \otimes w_{8j+1 \rightarrow 8(j+1)}, & i = (j+1)_s; \\ 0, & \text{otherwise.} \end{cases}$$

If  $6s \leq j < 7s$ , then

$$b_{ij} = \begin{cases} -e_{8(j+m)+7} \otimes w_{8j+2 \rightarrow 8(j+1)}, & i = (j+1)_s; \\ w_{8(j+m)+5 \rightarrow 8(j+m)+7} \otimes e_{8j+2}, & i = j - 3s; \\ 2w_{8(j+m)+1 \rightarrow 8(j+m)+7} \otimes w_{8j+2 \rightarrow 8j+3}, & i = j - s; \\ 0, & \text{otherwise.} \end{cases}$$

If  $7s \leq j < 8s$ , then  $b_{ij} = 0$ .

If  $8s \leq j < 9s$ , then

$$b_{ij} = \begin{cases} e_{8(j+m)+1} \otimes w_{8j+3 \rightarrow 8(j+1)}, & i = s + (j+1)_s; \\ 2w_{8(j+m)+1 \rightarrow 8(j+m)+1} \otimes e_{8j+3}, & i = j - 3s; \\ 0, & \text{otherwise.} \end{cases}$$

If  $9s \leq j < 10s$ , then  $b_{ij} = 0$ .

If  $10s \leq j < 11s$ , then

$$b_{ij} = \begin{cases} 2e_{8(j+m)+7} \otimes w_{8j+5 \rightarrow 8(j+1)}, & i = (j+1)_s; \\ -w_{8(j+m)+2 \rightarrow 8(j+m)+7} \otimes e_{8j+5}, & i = j - 3s; \\ w_{8(j+m)+5 \rightarrow 8(j+m)+7} \otimes e_{8j+5}, & i = j - 2s; \\ 0, & \text{otherwise.} \end{cases}$$

If  $11s \leq j < 12s$ , then  $b_{ij} = 0$ .

If  $12s \leq j < 13s$ , then

$$b_{ij} = \begin{cases} w_{8(j+m)+3 \rightarrow 8(j+m+1)} \otimes e_{8j+6}, & i = j - 3s; \\ 0, & \text{otherwise.} \end{cases}$$

If  $13s \leq j < 14s$ , then  $b_{ij} = 0$ .

If  $14s \leq j < 15s$ , then

$$b_{ij} = \begin{cases} w_{8(j+m)+7 \rightarrow 8(j+m+1)+2} \otimes w_{8j+7 \rightarrow 8(j+1)}, & i = (j+1)_s; \\ -e_{8(j+m+1)+2} \otimes w_{8j+7 \rightarrow 8(j+1)+4}, & i = 6s + (j+1)_s; \\ 0, & \text{otherwise.} \end{cases}$$

If  $15s \leq j < 17s$ , then  $b_{ij} = 0$ .

If  $17s \leq j < 18s$ , then

$$b_{ij} = \begin{cases} -e_{8(j+m+1)+5} \otimes w_{8j+7 \rightarrow 8(j+1)+2}, & i = 3s + (j+1)_s; \\ 0, & \text{otherwise.} \end{cases}$$

(8) If  $r_0 = 7$ , then  $\Omega^7(Z_t^{(9)})$  is described with  $(14s \times 19s)$  matrix, whose entries  $b_{ij}$  have the following form:

If  $0 \leq j < s$ , then

$$b_{ij} = \begin{cases} -2w_{8(j+m)+2 \rightarrow 8(j+m)+7} \otimes e_{8j}, & i = j; \\ w_{8(j+m)+4 \rightarrow 8(j+m)+7} \otimes e_{8j}, & i = j + s; \\ w_{8(j+m)+5 \rightarrow 8(j+m)+7} \otimes e_{8j}, & i = j + 3s; \\ e_{8(j+m)+7} \otimes w_{8j \rightarrow 8j+1}, & i = j + 4s; \\ 0, & \text{otherwise.} \end{cases}$$

If  $s \leq j < 2s$ , then

$$b_{ij} = \begin{cases} -2w_{8(j+m)+2 \rightarrow 8(j+m+1)} \otimes e_{8j}, & i = j - s; \\ 2w_{8(j+m)+4 \rightarrow 8(j+m+1)} \otimes e_{8j}, & i = j; \\ -2w_{8(j+m)+7 \rightarrow 8(j+m+1)} \otimes w_{8j \rightarrow 8j+1}, & i = j + 3s; \\ -e_{8(j+m+1)} \otimes w_{8j \rightarrow 8j+2}, & i = j + 4s; \\ 0, & \text{otherwise.} \end{cases}$$

If  $2s \leq j < 3s$ , then

$$b_{ij} = \begin{cases} -e_{8(j+m)+7} \otimes w_{8j \rightarrow 8j+1}, & i = j + 2s; \\ 0, & \text{otherwise.} \end{cases}$$

If  $3s \leq j < 4s$ , then

$$b_{ij} = \begin{cases} w_{8(j+m+1)+2 \rightarrow 8(j+m+1)+4} \otimes w_{8j+1 \rightarrow 8(j+1)}, & i = (j+1)_s; \\ -e_{8(j+m+1)+4} \otimes w_{8j+1 \rightarrow 8(j+1)}, & i = s + (j+1)_s; \\ 0, & \text{otherwise.} \end{cases}$$

If  $4s \leq j < 5s$ , then

$$b_{ij} = \begin{cases} -2e_{8(j+m+1)+6} \otimes w_{8j+1 \rightarrow 8(j+1)}, & i = 2s + (j+1)_s; \\ 0, & \text{otherwise.} \end{cases}$$

If  $5s \leq j < 6s$ , then

$$b_{ij} = \begin{cases} 2e_{8(j+m+1)+5} \otimes w_{8j+2 \rightarrow 8(j+1)}, & i = 3s + (j+1)_s; \\ w_{8(j+m+1) \rightarrow 8(j+m+1)+5} \otimes e_{8j+2}, & i = j; \\ 0, & \text{otherwise.} \end{cases}$$

If  $6s \leq j < 7s$ , then  $b_{ij} = 0$ .

If  $7s \leq j < 8s$ , then

$$b_{ij} = \begin{cases} e_{8(j+m+1)+2} \otimes w_{8j+3 \rightarrow 8(j+1)}, & i = (j+1)_s; \\ 0, & \text{otherwise.} \end{cases}$$

If  $8s \leq j < 9s$ , then

$$b_{ij} = \begin{cases} w_{8(j+m+1)+5 \rightarrow 8(j+m+1)+6} \otimes w_{8j+3 \rightarrow 8(j+1)}, & i = 3s + (j+1)_s; \\ 0, & \text{otherwise.} \end{cases}$$

If  $9s \leq j < 10s$ , then  $b_{ij} = 0$ .

If  $10s \leq j < 11s$ , then

$$b_{ij} = \begin{cases} -w_{8(j+m)+7 \rightarrow 8(j+m+1)+2} \otimes e_{8j+5}, & i = j - 2s; \\ 0, & \text{otherwise.} \end{cases}$$

If  $11s \leq j < 13s$ , then  $b_{ij} = 0$ .

If  $13s \leq j < 14s$ , then

$$b_{ij} = \begin{cases} w_{8(j+m)+7 \rightarrow 8(j+m+1)+3} \otimes e_{8j+6}, & i = j - 4s; \\ e_{8(j+m+1)+3} \otimes w_{8j+6 \rightarrow 8j+7}, & i = j - s; \\ 0, & \text{otherwise.} \end{cases}$$

If  $14s \leq j < 16s$ , then  $b_{ij} = 0$ .

If  $16s \leq j < 17s$ , then

$$b_{ij} = \begin{cases} -w_{8(j+m+1)+2 \rightarrow 8(j+m+1)+7} \otimes w_{8j+7 \rightarrow 8(j+1)}, & i = (j+1)_s; \\ w_{8(j+m+1)+4 \rightarrow 8(j+m+1)+7} \otimes w_{8j+7 \rightarrow 8(j+1)}, & i = s + (j+1)_s; \\ e_{8(j+m+1)+7} \otimes w_{8j+7 \rightarrow 8(j+1)+1}, & i = 4s + (j+1)_s; \\ 0, & \text{otherwise.} \end{cases}$$

If  $17s \leq j < 19s$ , then  $b_{ij} = 0$ .

(9) If  $r_0 = 8$ , then  $\Omega^8(Z_t^{(9)})$  is described with  $(16s \times 18s)$  matrix, whose entries  $b_{ij}$  have the following form:

If  $0 \leq j < s$ , then

$$b_{ij} = \begin{cases} -w_{8(j+m-1)+7 \rightarrow 8(j+m)+2} \otimes e_{8j}, & i = j + s; \\ w_{8(j+m)+1 \rightarrow 8(j+m)+2} \otimes w_{8j \rightarrow 8j+2}, & i = j + 5s; \\ e_{8(j+m)+2} \otimes w_{8j \rightarrow 8j+3}, & i = j + 6s; \\ 0, & \text{otherwise.} \end{cases}$$



If  $s \leq j < 2s$ , then

$$b_{ij} = \begin{cases} -2w_{8(j+m-1)+7 \rightarrow 8(j+m)+4} \otimes e_{8j}, & i = j - s; \\ w_{8(j+m-1)+7 \rightarrow 8(j+m)+4} \otimes e_{8j}, & i = j; \\ -2w_{8(j+m)+2 \rightarrow 8(j+m)+4} \otimes w_{8j \rightarrow 8j+3}, & i = j + 5s; \\ 2w_{8(j+m)+3 \rightarrow 8(j+m)+4} \otimes w_{8j \rightarrow 8j+4}, & i = j + 6s; \\ e_{8(j+m)+4} \otimes w_{8j \rightarrow 8j+6}, & i = j + 11s; \\ 0, & \text{otherwise.} \end{cases}$$

If  $2s \leq j < 3s$ , then

$$b_{ij} = \begin{cases} -w_{8(j+m)+5 \rightarrow 8(j+m)+6} \otimes w_{8j \rightarrow 8j+1}, & i = j + s; \\ 2e_{8(j+m)+6} \otimes w_{8j \rightarrow 8j+2}, & i = j + 2s; \\ 0, & \text{otherwise.} \end{cases}$$

If  $3s \leq j < 4s$ , then

$$b_{ij} = \begin{cases} -2e_{8(j+m)+5} \otimes w_{8j \rightarrow 8j+1}, & i = j; \\ 0, & \text{otherwise.} \end{cases}$$

If  $4s \leq j < 5s$ , then

$$b_{ij} = \begin{cases} -2e_{8(j+m)+7} \otimes w_{8j+1 \rightarrow 8(j+1)}, & i = (j+1)_s; \\ -2e_{8(j+m)+7} \otimes w_{8j+1 \rightarrow 8(j+1)}, & i = s + (j+1)_s; \\ 0, & \text{otherwise.} \end{cases}$$

If  $5s \leq j < 6s$ , then

$$b_{ij} = \begin{cases} -w_{8(j+m)+7 \rightarrow 8(j+m)+1} \otimes w_{8j+1 \rightarrow 8(j+1)}, & i = s + (j+1)_s; \\ -2e_{8(j+m)+1} \otimes w_{8j+1 \rightarrow 8(j+1)}, & i = 2s + (j+1)_s; \\ 0, & \text{otherwise.} \end{cases}$$

If  $6s \leq j < 7s$ , then

$$b_{ij} = \begin{cases} -w_{8(j+m)+7 \rightarrow 8(j+m)+1} \otimes w_{8j+2 \rightarrow 8(j+1)}, & i = s + (j+1)_s; \\ -e_{8(j+m)+1} \otimes w_{8j+2 \rightarrow 8(j+1)}, & i = 2s + (j+1)_s; \\ w_{8(j+m)+6 \rightarrow 8(j+m)+1} \otimes e_{8j+2}, & i = j - 2s; \\ 0, & \text{otherwise.} \end{cases}$$

If  $7s \leq j < 9s$ , then  $b_{ij} = 0$ .

If  $9s \leq j < 10s$ , then

$$b_{ij} = \begin{cases} 2w_{8(j+m)+7 \rightarrow 8(j+m)+1} \otimes w_{8j+5 \rightarrow 8(j+1)}, & i = (j+1)_s; \\ -2w_{8(j+m)+7 \rightarrow 8(j+m)+1} \otimes w_{8j+5 \rightarrow 8(j+1)}, & i = s + (j+1)_s; \\ 2e_{8(j+m)+1} \otimes w_{8j+5 \rightarrow 8(j+1)}, & i = 2s + (j+1)_s; \\ -w_{8(j+m)+3 \rightarrow 8(j+m)+1} \otimes e_{8j+5}, & i = j; \\ 0, & \text{otherwise.} \end{cases}$$

If  $10s \leq j < 11s$ , then  $b_{ij} = 0$ .

If  $11s \leq j < 12s$ , then

$$b_{ij} = \begin{cases} w_{8(j+m)+4 \rightarrow 8(j+m)+7} \otimes e_{8j+6}, & i = j + s; \\ 0, & \text{otherwise.} \end{cases}$$

If  $12s \leq j < 13s$ , then  $b_{ij} = 0$ .

If  $13s \leq j < 14s$ , then

$$b_{ij} = \begin{cases} w_{8(j+m)+7 \rightarrow 8(j+m+1)+3} \otimes w_{8j+7 \rightarrow 8(j+1)}, & i = (j+1)_s; \\ -w_{8(j+m)+7 \rightarrow 8(j+m+1)+3} \otimes w_{8j+7 \rightarrow 8(j+1)}, & i = s + (j+1)_s; \\ w_{8(j+m+1)+1 \rightarrow 8(j+m+1)+3} \otimes w_{8j+7 \rightarrow 8(j+1)+2}, & i = 5s + (j+1)_s; \\ 2w_{8(j+m+1)+2 \rightarrow 8(j+m+1)+3} \otimes w_{8j+7 \rightarrow 8(j+1)+3}, & i = 6s + (j+1)_s; \\ -e_{8(j+m+1)+3} \otimes w_{8j+7 \rightarrow 8(j+1)+4}, & i = 7s + (j+1)_s; \\ 0, & \text{otherwise.} \end{cases}$$

If  $14s \leq j < 15s$ , then

$$b_{ij} = \begin{cases} w_{8(j+m+1)+5 \rightarrow 8(j+m+1)+6} \otimes w_{8j+7 \rightarrow 8(j+1)+1}, & i = 3s + (j+1)_s; \\ -e_{8(j+m+1)+6} \otimes w_{8j+7 \rightarrow 8(j+1)+2}, & i = 4s + (j+1)_s; \\ 0, & \text{otherwise.} \end{cases}$$

If  $15s \leq j < 18s$ , then  $b_{ij} = 0$ .

(10) If  $r_0 = 9$ , then  $\Omega^9(Z_t^{(9)})$  is described with  $(16s \times 19s)$  matrix, whose entries  $b_{ij}$  have the following form:

If  $0 \leq j < s$ , then

$$b_{ij} = \begin{cases} 2w_{8(j+m)+3 \rightarrow 8(j+m)+7} \otimes e_{8j}, & i = j + s; \\ -2w_{8(j+m)+6 \rightarrow 8(j+m)+7} \otimes e_{8j}, & i = j + 2s; \\ -e_{8(j+m)+7} \otimes w_{8j \rightarrow 8j+2}, & i = j + 5s; \\ 2e_{8(j+m)+7} \otimes w_{8j \rightarrow 8j+5}, & i = j + 8s; \\ 0, & \text{otherwise.} \end{cases}$$

If  $s \leq j < 2s$ , then

$$b_{ij} = \begin{cases} -2w_{8(j+m)+3 \rightarrow 8(j+m+1)} \otimes e_{8j}, & i = j; \\ w_{8(j+m)+6 \rightarrow 8(j+m+1)} \otimes e_{8j}, & i = j + s; \\ e_{8(j+m+1)} \otimes w_{8j \rightarrow 8j+1}, & i = j + 3s; \\ -w_{8(j+m)+7 \rightarrow 8(j+m+1)} \otimes w_{8j \rightarrow 8j+5}, & i = j + 7s; \\ 0, & \text{otherwise.} \end{cases}$$

If  $2s \leq j < 3s$ , then

$$b_{ij} = \begin{cases} -e_{8(j+m+1)} \otimes w_{8j \rightarrow 8j+1}, & i = j + 2s; \\ 0, & \text{otherwise.} \end{cases}$$

If  $3s \leq j < 4s$ , then

$$b_{ij} = \begin{cases} -2e_{8(j+m+1)+5} \otimes w_{8j+1 \rightarrow 8(j+1)}, & i = (j+1)_s; \\ 0, & \text{otherwise.} \end{cases}$$

If  $4s \leq j < 5s$ , then

$$b_{ij} = \begin{cases} -e_{8(j+m+1)+1} \otimes w_{8j+1 \rightarrow 8(j+1)}, & i = 3s + (j+1)_s; \\ 0, & \text{otherwise.} \end{cases}$$

If  $5s \leq j < 6s$ , then

$$b_{ij} = \begin{cases} -w_{8(j+m+1)+1 \rightarrow 8(j+m+1)+2} \otimes w_{8j+2 \rightarrow 8(j+1)}, & i = 3s + (j+1)_s; \\ 0, & \text{otherwise.} \end{cases}$$

If  $6s \leq j < 7s$ , then

$$b_{ij} = \begin{cases} -w_{8(j+m+1)+5 \rightarrow 8(j+m+1)+6} \otimes w_{8j+2 \rightarrow 8(j+1)}, & i = (j+1)_s; \\ -2e_{8(j+m+1)+6} \otimes w_{8j+2 \rightarrow 8(j+1)}, & i = 2s + (j+1)_s; \\ w_{8(j+m)+7 \rightarrow 8(j+m+1)+6} \otimes e_{8j+2}, & i = j - s; \\ 0, & \text{otherwise.} \end{cases}$$

If  $7s \leq j < 8s$ , then

$$b_{ij} = \begin{cases} e_{8(j+m+1)+3} \otimes w_{8j+3 \rightarrow 8(j+1)}, & i = s + (j+1)_s; \\ 0, & \text{otherwise.} \end{cases}$$

If  $8s \leq j < 10s$ , then  $b_{ij} = 0$ .

If  $10s \leq j < 11s$ , then

$$b_{ij} = \begin{cases} 2w_{8(j+m+1)+1 \rightarrow 8(j+m+1)+3} \otimes w_{8j+5 \rightarrow 8(j+1)}, & i = 3s + (j+1)_s; \\ -w_{8(j+m)+7 \rightarrow 8(j+m+1)+3} \otimes e_{8j+5}, & i = j - 2s; \\ 0, & \text{otherwise.} \end{cases}$$

If  $11s \leq j < 12s$ , then  $b_{ij} = 0$ .

If  $12s \leq j < 13s$ , then

$$b_{ij} = \begin{cases} 2e_{8(j+m+1)+5} \otimes w_{8j+5 \rightarrow 8(j+1)}, & i = (j+1)_s; \\ 0, & \text{otherwise.} \end{cases}$$

If  $13s \leq j < 14s$ , then  $b_{ij} = 0$ .

If  $14s \leq j < 15s$ , then

$$b_{ij} = \begin{cases} w_{8(j+m+1) \rightarrow 8(j+m+1)+4} \otimes e_{8j+6}, & i = j - 3s; \\ e_{8(j+m+1)+4} \otimes w_{8j+6 \rightarrow 8j+7}, & i = j - s; \\ 0, & \text{otherwise.} \end{cases}$$

If  $15s \leq j < 16s$ , then  $b_{ij} = 0$ .

If  $16s \leq j < 17s$ , then

$$b_{ij} = \begin{cases} -w_{8(j+m+1)+3 \rightarrow 8(j+m+1)+7} \otimes w_{8j+7 \rightarrow 8(j+1)}, & i = s + (j+1)_s; \\ w_{8(j+m+1)+6 \rightarrow 8(j+m+1)+7} \otimes w_{8j+7 \rightarrow 8(j+1)}, & i = 2s + (j+1)_s; \\ -e_{8(j+m+1)+7} \otimes w_{8j+7 \rightarrow 8(j+1)+5}, & i = 8s + (j+1)_s; \\ 0, & \text{otherwise.} \end{cases}$$

If  $17s \leq j < 18s$ , then

$$b_{ij} = \begin{cases} -w_{8(j+m+1)+3 \rightarrow 8(j+m+2)} \otimes w_{8j+7 \rightarrow 8(j+1)}, & i = s + (j+1)_s; \\ w_{8(j+m+1)+6 \rightarrow 8(j+m+2)} \otimes w_{8j+7 \rightarrow 8(j+1)}, & i = 2s + (j+1)_s; \\ e_{8(j+m+2)} \otimes w_{8j+7 \rightarrow 8(j+1)+1}, & i = 4s + (j+1)_s; \\ -w_{8(j+m+1)+7 \rightarrow 8(j+m+2)} \otimes w_{8j+7 \rightarrow 8(j+1)+5}, & i = 8s + (j+1)_s; \\ 0, & \text{otherwise.} \end{cases}$$

If  $18s \leq j < 19s$ , then  $b_{ij} = 0$ .

(11) If  $r_0 = 10$ , then  $\Omega^{10}(Z_t^{(9)})$  is described with  $(19s \times 16s)$  matrix, whose entries  $b_{ij}$  have the following form:

If  $0 \leq j < s$ , then

$$b_{ij} = \begin{cases} w_{8(j+m)+1 \rightarrow 8(j+m)+3} \otimes w_{8j \rightarrow 8j+1}, & i = j + 4s; \\ -w_{8(j+m)+2 \rightarrow 8(j+m)+3} \otimes w_{8j \rightarrow 8j+2}, & i = j + 5s; \\ e_{8(j+m)+3} \otimes w_{8j \rightarrow 8j+3}, & i = j + 6s; \\ 0, & \text{otherwise.} \end{cases}$$

If  $s \leq j < 2s$ , then

$$b_{ij} = \begin{cases} -2w_{8(j+m) \rightarrow 8(j+m)+6} \otimes e_{8j}, & i = j + s; \\ -2e_{8(j+m)+6} \otimes w_{8j \rightarrow 8j+1}, & i = j + 2s; \\ 2w_{8(j+m)+5 \rightarrow 8(j+m)+6} \otimes w_{8j \rightarrow 8j+5}, & i = j + 9s; \\ 0, & \text{otherwise.} \end{cases}$$

If  $2s \leq j < 3s$ , then

$$b_{ij} = \begin{cases} -e_{8(j+m)+1} \otimes w_{8j \rightarrow 8j+1}, & i = j + 2s; \\ 0, & \text{otherwise.} \end{cases}$$

If  $3s \leq j < 4s$ , then

$$b_{ij} = \begin{cases} w_{8(j+m) \rightarrow 8(j+m)+5} \otimes e_{8j}, & i = j - s; \\ -e_{8(j+m)+5} \otimes w_{8j \rightarrow 8j+5}, & i = j + 7s; \\ 0, & \text{otherwise.} \end{cases}$$

If  $4s \leq j < 5s$ , then

$$b_{ij} = \begin{cases} -2w_{8(j+m)+7 \rightarrow 8(j+m+1)} \otimes w_{8j+1 \rightarrow 8(j+1)}, & i = (j+1)_s; \\ -2e_{8(j+m+1)} \otimes w_{8j+1 \rightarrow 8(j+1)}, & i = s + (j+1)_s; \\ -2e_{8(j+m+1)} \otimes w_{8j+1 \rightarrow 8(j+1)}, & i = 2s + (j+1)_s; \\ 0, & \text{otherwise.} \end{cases}$$

If  $5s \leq j < 6s$ , then

$$b_{ij} = \begin{cases} e_{8(j+m)+7} \otimes w_{8j+2 \rightarrow 8(j+1)}, & i = (j+1)_s; \\ -w_{8(j+m)+2 \rightarrow 8(j+m)+7} \otimes e_{8j+2}, & i = j; \\ w_{8(j+m)+3 \rightarrow 8(j+m)+7} \otimes w_{8j+2 \rightarrow 8j+3}, & i = j + s; \\ 0, & \text{otherwise.} \end{cases}$$

If  $6s \leq j < 8s$ , then  $b_{ij} = 0$ .

If  $8s \leq j < 9s$ , then

$$b_{ij} = \begin{cases} -e_{8(j+m)+7} \otimes w_{8j+5 \rightarrow 8(j+1)}, & i = (j+1)_s; \\ -w_{8(j+m)+5 \rightarrow 8(j+m)+7} \otimes e_{8j+5}, & i = j+2s; \\ w_{8(j+m)+1 \rightarrow 8(j+m)+7} \otimes e_{8j+5}, & i = j+4s; \\ 0, & \text{otherwise.} \end{cases}$$

If  $9s \leq j < 10s$ , then  $b_{ij} = 0$ .

If  $10s \leq j < 11s$ , then

$$b_{ij} = \begin{cases} -w_{8(j+m)+5 \rightarrow 8(j+m)+7} \otimes e_{8j+6}, & i = j+5s; \\ -e_{8(j+m)+7} \otimes w_{8j+6 \rightarrow 8j+7}, & i = j+7s; \\ 0, & \text{otherwise.} \end{cases}$$

If  $11s \leq j < 12s$ , then

$$b_{ij} = \begin{cases} w_{8(j+m)+5 \rightarrow 8(j+m+1)} \otimes e_{8j+6}, & i = j+4s; \\ w_{8(j+m)+7 \rightarrow 8(j+m+1)} \otimes w_{8j+6 \rightarrow 8j+7}, & i = j+6s; \\ 0, & \text{otherwise.} \end{cases}$$

If  $12s \leq j < 13s$ , then

$$b_{ij} = \begin{cases} -w_{8(j+m+1)+1 \rightarrow 8(j+m+1)+2} \otimes w_{8j+7 \rightarrow 8(j+1)+1}, & i = 4s + (j+1)_s; \\ 0, & \text{otherwise.} \end{cases}$$

If  $13s \leq j < 14s$ , then

$$b_{ij} = \begin{cases} w_{8(j+m+1) \rightarrow 8(j+m+1)+4} \otimes w_{8j+7 \rightarrow 8(j+1)}, & i = s + (j+1)_s; \\ -w_{8(j+m+1) \rightarrow 8(j+m+1)+4} \otimes w_{8j+7 \rightarrow 8(j+1)}, & i = 2s + (j+1)_s; \\ w_{8(j+m+1)+1 \rightarrow 8(j+m+1)+4} \otimes w_{8j+7 \rightarrow 8(j+1)+1}, & i = 4s + (j+1)_s; \\ -w_{8(j+m+1)+2 \rightarrow 8(j+m+1)+4} \otimes w_{8j+7 \rightarrow 8(j+1)+2}, & i = 5s + (j+1)_s; \\ 2w_{8(j+m+1)+3 \rightarrow 8(j+m+1)+4} \otimes w_{8j+7 \rightarrow 8(j+1)+3}, & i = 6s + (j+1)_s; \\ -e_{8(j+m+1)+4} \otimes w_{8j+7 \rightarrow 8(j+1)+4}, & i = 8s + (j+1)_s; \\ 0, & \text{otherwise.} \end{cases}$$

If  $14s \leq j < 15s$ , then  $b_{ij} = 0$ .

If  $15s \leq j < 16s$ , then

$$b_{ij} = \begin{cases} w_{8(j+m+1) \rightarrow 8(j+m+1)+5} \otimes w_{8j+7 \rightarrow 8(j+1)}, & i = 2s + (j+1)_s; \\ -e_{8(j+m+1)+5} \otimes w_{8j+7 \rightarrow 8(j+1)+5}, & i = 10s + (j+1)_s; \\ 0, & \text{otherwise.} \end{cases}$$

(12) If  $r_0 = 11$ , then  $\Omega^{11}(Z_t^{(9)})$  is described with  $(18s \times 16s)$  matrix, whose entries  $b_{ij}$  have the following form:

If  $0 \leq j < s$ , then

$$b_{ij} = \begin{cases} w_{8(j+m)+1 \rightarrow 8(j+m)+7} \otimes e_{8j}, & i = j+3s; \\ 2e_{8(j+m)+7} \otimes w_{8j \rightarrow 8j+1}, & i = j+5s; \\ 0, & \text{otherwise.} \end{cases}$$

If  $s \leq j < 2s$ , then

$$b_{ij} = \begin{cases} 2w_{8(j+m)+4 \rightarrow 8(j+m+1)} \otimes e_{8j}, & i = j + s; \\ -w_{8(j+m)+1 \rightarrow 8(j+m+1)} \otimes e_{8j}, & i = j + 2s; \\ -2w_{8(j+m)+5 \rightarrow 8(j+m+1)} \otimes e_{8j}, & i = j + 3s; \\ -e_{8(j+m+1)} \otimes w_{8j \rightarrow 8j+2}, & i = j + 5s; \\ -2w_{8(j+m)+7 \rightarrow 8(j+m+1)} \otimes w_{8j \rightarrow 8j+3}, & i = j + 6s; \\ 2w_{8(j+m)+7 \rightarrow 8(j+m+1)} \otimes w_{8j \rightarrow 8j+4}, & i = j + 7s; \\ 2e_{8(j+m+1)} \otimes w_{8j \rightarrow 8j+5}, & i = j + 10s; \\ 0, & \text{otherwise.} \end{cases}$$

If  $2s \leq j < 3s$ , then

$$b_{ij} = \begin{cases} -2e_{8(j+m+1)+2} \otimes w_{8j+1 \rightarrow 8(j+1)}, & i = (j+1)_s; \\ -2w_{8(j+m+1)+1 \rightarrow 8(j+m+1)+2} \otimes w_{8j+1 \rightarrow 8(j+1)}, & i = 3s + (j+1)_s; \\ w_{8(j+m)+7 \rightarrow 8(j+m+1)+2} \otimes e_{8j+1}, & i = j + 3s; \\ 0, & \text{otherwise.} \end{cases}$$

If  $3s \leq j < 4s$ , then

$$b_{ij} = \begin{cases} -2e_{8(j+m+1)+6} \otimes w_{8j+1 \rightarrow 8(j+1)}, & i = s + (j+1)_s; \\ -2w_{8(j+m+1)+5 \rightarrow 8(j+m+1)+6} \otimes w_{8j+1 \rightarrow 8(j+1)}, & i = 4s + (j+1)_s; \\ 0, & \text{otherwise.} \end{cases}$$

If  $4s \leq j < 5s$ , then

$$b_{ij} = \begin{cases} w_{8(j+m+1)+2 \rightarrow 8(j+m+1)+3} \otimes w_{8j+2 \rightarrow 8(j+1)}, & i = (j+1)_s; \\ -w_{8(j+m+1) \rightarrow 8(j+m+1)+3} \otimes e_{8j+2}, & i = j + 2s; \\ 0, & \text{otherwise.} \end{cases}$$

If  $5s \leq j < 6s$ , then

$$b_{ij} = \begin{cases} e_{8(j+m+1)+4} \otimes w_{8j+3 \rightarrow 8(j+1)}, & i = 2s + (j+1)_s; \\ -w_{8(j+m+1)+1 \rightarrow 8(j+m+1)+4} \otimes w_{8j+3 \rightarrow 8(j+1)}, & i = 3s + (j+1)_s; \\ 0, & \text{otherwise.} \end{cases}$$

If  $6s \leq j < 8s$ , then  $b_{ij} = 0$ .

If  $8s \leq j < 9s$ , then

$$b_{ij} = \begin{cases} -2e_{8(j+m+1)+6} \otimes w_{8j+5 \rightarrow 8(j+1)}, & i = s + (j+1)_s; \\ -w_{8(j+m)+7 \rightarrow 8(j+m+1)+6} \otimes e_{8j+5}, & i = j + 2s; \\ 0, & \text{otherwise.} \end{cases}$$

If  $9s \leq j < 10s$ , then

$$b_{ij} = \begin{cases} -w_{8(j+m+1)+2 \rightarrow 8(j+m+1)+4} \otimes w_{8j+5 \rightarrow 8(j+1)}, & i = (j+1)_s; \\ w_{8(j+m+1)+1 \rightarrow 8(j+m+1)+4} \otimes w_{8j+5 \rightarrow 8(j+1)}, & i = 3s + (j+1)_s; \\ 0, & \text{otherwise.} \end{cases}$$

If  $10s \leq j < 12s$ , then  $b_{ij} = 0$ .

If  $12s \leq j < 13s$ , then

$$b_{ij} = \begin{cases} -w_{8(j+m)+7 \rightarrow 8(j+m+1)+5} \otimes e_{8j+6}, & i = j; \\ -w_{8(j+m+1) \rightarrow 8(j+m+1)+5} \otimes e_{8j+6}, & i = j + s; \\ -e_{8(j+m+1)+5} \otimes w_{8j+6 \rightarrow 8j+7}, & i = j + 2s; \\ 0, & \text{otherwise.} \end{cases}$$

If  $13s \leq j < 14s$ , then

$$b_{ij} = \begin{cases} -w_{8(j+m+1)+5 \rightarrow 8(j+m+1)+7} \otimes w_{8j+7 \rightarrow 8(j+1)}, & i = 4s + (j + 1)_s; \\ -2e_{8(j+m+1)+7} \otimes w_{8j+7 \rightarrow 8(j+1)+1}, & i = 5s + (j + 1)_s; \\ -e_{8(j+m+1)+7} \otimes w_{8j+7 \rightarrow 8(j+1)+3}, & i = 7s + (j + 1)_s; \\ e_{8(j+m+1)+7} \otimes w_{8j+7 \rightarrow 8(j+1)+4}, & i = 8s + (j + 1)_s; \\ 0, & \text{otherwise.} \end{cases}$$

If  $14s \leq j < 15s$ , then

$$b_{ij} = \begin{cases} -w_{8(j+m+1)+4 \rightarrow 8(j+m+2)} \otimes w_{8j+7 \rightarrow 8(j+1)}, & i = 2s + (j + 1)_s; \\ w_{8(j+m+1)+1 \rightarrow 8(j+m+2)} \otimes w_{8j+7 \rightarrow 8(j+1)}, & i = 3s + (j + 1)_s; \\ 2w_{8(j+m+1)+5 \rightarrow 8(j+m+2)} \otimes w_{8j+7 \rightarrow 8(j+1)}, & i = 4s + (j + 1)_s; \\ 2w_{8(j+m+1)+7 \rightarrow 8(j+m+2)} \otimes w_{8j+7 \rightarrow 8(j+1)+1}, & i = 5s + (j + 1)_s; \\ 2w_{8(j+m+1)+7 \rightarrow 8(j+m+2)} \otimes w_{8j+7 \rightarrow 8(j+1)+3}, & i = 7s + (j + 1)_s; \\ -2w_{8(j+m+1)+7 \rightarrow 8(j+m+2)} \otimes w_{8j+7 \rightarrow 8(j+1)+4}, & i = 8s + (j + 1)_s; \\ -e_{8(j+m+2)} \otimes w_{8j+7 \rightarrow 8(j+1)+5}, & i = 11s + (j + 1)_s; \\ 0, & \text{otherwise.} \end{cases}$$

If  $15s \leq j < 16s$ , then  $b_{ij} = 0$ .

(13) If  $r_0 = 12$ , then  $\Omega^{12}(Z_t^{(9)})$  is described with  $(19s \times 14s)$  matrix, whose entries  $b_{ij}$  have the following form:

If  $0 \leq j < s$ , then

$$b_{ij} = \begin{cases} -2w_{8(j+m-1)+7 \rightarrow 8(j+m)+2} \otimes e_{8j}, & i = j + 2s; \\ e_{8(j+m)+2} \otimes w_{8j \rightarrow 8j+1}, & i = j + 3s; \\ -2e_{8(j+m)+2} \otimes w_{8j \rightarrow 8j+5}, & i = j + 10s; \\ 0, & \text{otherwise.} \end{cases}$$

If  $s \leq j < 2s$ , then

$$b_{ij} = \begin{cases} 2w_{8(j+m-1)+7 \rightarrow 8(j+m)+4} \otimes e_{8j}, & i = j + s; \\ w_{8(j+m)+2 \rightarrow 8(j+m)+4} \otimes w_{8j \rightarrow 8j+1}, & i = j + 2s; \\ -w_{8(j+m)+3 \rightarrow 8(j+m)+4} \otimes w_{8j \rightarrow 8j+2}, & i = j + 3s; \\ e_{8(j+m)+4} \otimes w_{8j \rightarrow 8j+3}, & i = j + 5s; \\ 2w_{8(j+m)+2 \rightarrow 8(j+m)+4} \otimes w_{8j \rightarrow 8j+5}, & i = j + 9s; \\ 0, & \text{otherwise.} \end{cases}$$

If  $2s \leq j < 3s$ , then

$$b_{ij} = \begin{cases} -2w_{8(j+m) \rightarrow 8(j+m)+6} \otimes e_{8j}, & i = j - s; \\ 2w_{8(j+m-1)+7 \rightarrow 8(j+m)+6} \otimes e_{8j}, & i = j; \\ 2w_{8(j+m)+5 \rightarrow 8(j+m)+6} \otimes w_{8j \rightarrow 8j+2}, & i = j + 3s; \\ -2w_{8(j+m)+5 \rightarrow 8(j+m)+6} \otimes w_{8j \rightarrow 8j+4}, & i = j + 6s; \\ e_{8(j+m)+6} \otimes w_{8j \rightarrow 8j+5}, & i = j + 9s; \\ 0, & \text{otherwise.} \end{cases}$$

If  $3s \leq j < 4s$ , then

$$b_{ij} = \begin{cases} -2e_{8(j+m)+7} \otimes w_{8j+1 \rightarrow 8(j+1)}, & i = (j+1)_s; \\ w_{8(j+m)+2 \rightarrow 8(j+m)+7} \otimes e_{8j+1}, & i = j; \\ 0, & \text{otherwise.} \end{cases}$$

If  $4s \leq j < 5s$ , then

$$b_{ij} = \begin{cases} e_{8(j+m+1)} \otimes w_{8j+2 \rightarrow 8(j+1)}, & i = s + (j+1)_s; \\ w_{8(j+m)+7 \rightarrow 8(j+m+1)} \otimes w_{8j+2 \rightarrow 8(j+1)}, & i = 2s + (j+1)_s; \\ -w_{8(j+m)+5 \rightarrow 8(j+m+1)} \otimes e_{8j+2}, & i = j + s; \\ 0, & \text{otherwise.} \end{cases}$$

If  $5s \leq j < 6s$ , then

$$b_{ij} = \begin{cases} e_{8(j+m)+7} \otimes w_{8j+3 \rightarrow 8(j+1)}, & i = 2s + (j+1)_s; \\ 0, & \text{otherwise.} \end{cases}$$

If  $6s \leq j < 7s$ , then  $b_{ij} = 0$ .

If  $7s \leq j < 8s$ , then

$$b_{ij} = \begin{cases} e_{8(j+m)+7} \otimes w_{8j+5 \rightarrow 8(j+1)}, & i = (j+1)_s; \\ -w_{8(j+m)+6 \rightarrow 8(j+m)+7} \otimes e_{8j+5}, & i = j + 4s; \\ 0, & \text{otherwise.} \end{cases}$$

If  $8s \leq j < 9s$ , then

$$b_{ij} = \begin{cases} -e_{8(j+m+1)} \otimes w_{8j+5 \rightarrow 8(j+1)}, & i = s + (j+1)_s; \\ 0, & \text{otherwise.} \end{cases}$$

If  $9s \leq j < 10s$ , then

$$b_{ij} = \begin{cases} w_{8(j+m)+6 \rightarrow 8(j+m+1)} \otimes e_{8j+6}, & i = j + 4s; \\ -e_{8(j+m+1)} \otimes w_{8j+6 \rightarrow 8j+7}, & i = j + 9s; \\ 0, & \text{otherwise.} \end{cases}$$

If  $10s \leq j < 11s$ , then

$$b_{ij} = \begin{cases} -w_{8(j+m)+7 \rightarrow 8(j+m+1)+3} \otimes w_{8j+7 \rightarrow 8(j+1)}, & i = 2s + (j+1)_s; \\ -w_{8(j+m+1)+2 \rightarrow 8(j+m+1)+3} \otimes w_{8j+7 \rightarrow 8(j+1)+1}, & i = 3s + (j+1)_s; \\ -w_{8(j+m+1)+2 \rightarrow 8(j+m+1)+3} \otimes w_{8j+7 \rightarrow 8(j+1)+5}, & i = 10s + (j+1)_s; \\ 0, & \text{otherwise.} \end{cases}$$



If  $11s \leq j < 12s$ , then

$$b_{ij} = \begin{cases} w_{8(j+m)+7 \rightarrow 8(j+m+1)+6} \otimes w_{8j+7 \rightarrow 8(j+1)}, & i = 2s + (j+1)_s; \\ 0, & \text{otherwise.} \end{cases}$$

If  $12s \leq j < 13s$ , then  $b_{ij} = 0$ .

If  $13s \leq j < 14s$ , then

$$b_{ij} = \begin{cases} -w_{8(j+m+1) \rightarrow 8(j+m+1)+5} \otimes w_{8j+7 \rightarrow 8(j+1)}, & i = s + (j+1)_s; \\ -2e_{8(j+m+1)+5} \otimes w_{8j+7 \rightarrow 8(j+1)+2}, & i = 5s + (j+1)_s; \\ -e_{8(j+m+1)+5} \otimes w_{8j+7 \rightarrow 8(j+1)+4}, & i = 8s + (j+1)_s; \\ 0, & \text{otherwise.} \end{cases}$$

(14) If  $r_0 = 13$ , then  $\Omega^{13}(Z_t^{(9)})$  is described with  $(18s \times 13s)$  matrix, whose entries  $b_{ij}$  have the following form:

If  $0 \leq j < s$ , then

$$b_{ij} = \begin{cases} 2e_{8(j+m+1)} \otimes w_{8j \rightarrow 8j+1}, & i = j + 4s; \\ -w_{8(j+m)+7 \rightarrow 8(j+m+1)} \otimes w_{8j \rightarrow 8j+2}, & i = j + 5s; \\ 0, & \text{otherwise.} \end{cases}$$

If  $s \leq j < 2s$ , then

$$b_{ij} = \begin{cases} 2w_{8(j+m)+5 \rightarrow 8(j+m)+7} \otimes e_{8j}, & i = j + 2s; \\ -e_{8(j+m)+7} \otimes w_{8j \rightarrow 8j+2}, & i = j + 4s; \\ 2e_{8(j+m)+7} \otimes w_{8j \rightarrow 8j+5}, & i = j + 8s; \\ 0, & \text{otherwise.} \end{cases}$$

If  $2s \leq j < 3s$ , then

$$b_{ij} = \begin{cases} -w_{8(j+m+1)+2 \rightarrow 8(j+m+1)+3} \otimes w_{8j+1 \rightarrow 8(j+1)}, & i = (j+1)_s; \\ -e_{8(j+m+1)+3} \otimes w_{8j+1 \rightarrow 8(j+1)}, & i = s + (j+1)_s; \\ 0, & \text{otherwise.} \end{cases}$$

If  $3s \leq j < 4s$ , then

$$b_{ij} = \begin{cases} -w_{8(j+m+1)+2 \rightarrow 8(j+m+1)+4} \otimes w_{8j+2 \rightarrow 8(j+1)}, & i = (j+1)_s; \\ w_{8(j+m+1)+3 \rightarrow 8(j+m+1)+4} \otimes w_{8j+2 \rightarrow 8(j+1)}, & i = s + (j+1)_s; \\ 0, & \text{otherwise.} \end{cases}$$

If  $4s \leq j < 5s$ , then

$$b_{ij} = \begin{cases} 2e_{8(j+m+1)+5} \otimes w_{8j+2 \rightarrow 8(j+1)}, & i = 3s + (j+1)_s; \\ w_{8(j+m)+7 \rightarrow 8(j+m+1)+5} \otimes e_{8j+2}, & i = j + s; \\ 0, & \text{otherwise.} \end{cases}$$

If  $5s \leq j < 7s$ , then  $b_{ij} = 0$ .

If  $7s \leq j < 8s$ , then

$$b_{ij} = \begin{cases} 2e_{8(j+m+1)+2} \otimes w_{8j+5 \rightarrow 8(j+1)}, & i = (j+1)_s; \\ -w_{8(j+m+1) \rightarrow 8(j+m+1)+2} \otimes e_{8j+5}, & i = j+3s; \\ 0, & \text{otherwise.} \end{cases}$$

If  $8s \leq j < 9s$ , then  $b_{ij} = 0$ .

If  $9s \leq j < 10s$ , then

$$b_{ij} = \begin{cases} w_{8(j+m+1)+2 \rightarrow 8(j+m+1)+3} \otimes w_{8j+6 \rightarrow 8(j+1)}, & i = (j+1)_s; \\ -w_{8(j+m+1)+1 \rightarrow 8(j+m+1)+3} \otimes w_{8j+6 \rightarrow 8j+7}, & i = j+7s; \\ 0, & \text{otherwise.} \end{cases}$$

If  $10s \leq j < 11s$ , then

$$b_{ij} = \begin{cases} w_{8(j+m)+7 \rightarrow 8(j+m+1)+6} \otimes e_{8j+6}, & i = j+s; \\ e_{8(j+m+1)+6} \otimes w_{8j+6 \rightarrow 8j+7}, & i = j+4s; \\ 0, & \text{otherwise.} \end{cases}$$

If  $11s \leq j < 12s$ , then

$$b_{ij} = \begin{cases} -w_{8(j+m+1)+5 \rightarrow 8(j+m+1)+7} \otimes w_{8j+7 \rightarrow 8(j+1)}, & i = 3s + (j+1)_s; \\ -e_{8(j+m+1)+7} \otimes w_{8j+7 \rightarrow 8(j+1)+5}, & i = 9s + (j+1)_s; \\ 0, & \text{otherwise.} \end{cases}$$

If  $12s \leq j < 13s$ , then

$$b_{ij} = \begin{cases} w_{8(j+m+1)+6 \rightarrow 8(j+m+2)} \otimes w_{8j+7 \rightarrow 8(j+1)}, & i = 2s + (j+1)_s; \\ w_{8(j+m+1)+5 \rightarrow 8(j+m+2)} \otimes w_{8j+7 \rightarrow 8(j+1)}, & i = 3s + (j+1)_s; \\ -2e_{8(j+m+2)} \otimes w_{8j+7 \rightarrow 8(j+1)+1}, & i = 4s + (j+1)_s; \\ -e_{8(j+m+2)} \otimes w_{8j+7 \rightarrow 8(j+1)+3}, & i = 7s + (j+1)_s; \\ e_{8(j+m+2)} \otimes w_{8j+7 \rightarrow 8(j+1)+4}, & i = 8s + (j+1)_s; \\ w_{8(j+m+1)+7 \rightarrow 8(j+m+2)} \otimes w_{8j+7 \rightarrow 8(j+1)+5}, & i = 9s + (j+1)_s; \\ 0, & \text{otherwise.} \end{cases}$$

(15) If  $r_0 = 14$ , then  $\Omega^{14}(Z_t^{(9)})$  is described with  $(20s \times 11s)$  matrix, whose entries  $b_{ij}$  have the following form:

If  $0 \leq j < s$ , then

$$b_{ij} = \begin{cases} w_{8(j+m) \rightarrow 8(j+m)+3} \otimes e_{8j}, & i = j+2s; \\ 2e_{8(j+m)+3} \otimes w_{8j \rightarrow 8j+1}, & i = j+3s; \\ w_{8(j+m)+1 \rightarrow 8(j+m)+3} \otimes w_{8j \rightarrow 8j+3}, & i = j+8s; \\ -2e_{8(j+m)+3} \otimes w_{8j \rightarrow 8j+5}, & i = j+12s; \\ 0, & \text{otherwise.} \end{cases}$$

If  $s \leq j < 2s$ , then

$$b_{ij} = \begin{cases} 2e_{8(j+m)+5} \otimes w_{8j \rightarrow 8j+1}, & i = j+3s; \\ 0, & \text{otherwise.} \end{cases}$$

If  $2s \leq j < 3s$ , then

$$b_{ij} = \begin{cases} -2e_{8(j+m+1)} \otimes w_{8j+1 \rightarrow 8(j+1)}, & i = s + (j+1)_s; \\ 0, & \text{otherwise.} \end{cases}$$

If  $3s \leq j < 4s$ , then

$$b_{ij} = \begin{cases} -e_{8(j+m)+7} \otimes w_{8j+2 \rightarrow 8(j+1)}, & i = (j+1)_s; \\ -w_{8(j+m)+6 \rightarrow 8(j+m)+7} \otimes e_{8j+2}, & i = j + 3s; \\ 0, & \text{otherwise.} \end{cases}$$

If  $4s \leq j < 5s$ , then

$$b_{ij} = \begin{cases} e_{8(j+m+1)} \otimes w_{8j+3 \rightarrow 8(j+1)}, & i = 2s + (j+1)_s; \\ 0, & \text{otherwise.} \end{cases}$$

If  $5s \leq j < 6s$ , then

$$b_{ij} = \begin{cases} -w_{8(j+m+1) \rightarrow 8(j+m+1)+1} \otimes w_{8j+4 \rightarrow 8(j+1)}, & i = 2s + (j+1)_s; \\ 0, & \text{otherwise.} \end{cases}$$

If  $6s \leq j < 7s$ , then

$$b_{ij} = \begin{cases} w_{8(j+m)+7 \rightarrow 8(j+m+1)} \otimes w_{8j+5 \rightarrow 8(j+1)}, & i = (j+1)_s; \\ e_{8(j+m+1)} \otimes w_{8j+5 \rightarrow 8(j+1)}, & i = s + (j+1)_s; \\ -w_{8(j+m)+1 \rightarrow 8(j+m+1)} \otimes e_{8j+5}, & i = j + 7s; \\ 0, & \text{otherwise.} \end{cases}$$

If  $7s \leq j < 8s$ , then

$$b_{ij} = \begin{cases} -w_{8(j+m)+2 \rightarrow 8(j+m)+7} \otimes e_{8j+6}, & i = j + 7s; \\ w_{8(j+m)+5 \rightarrow 8(j+m)+7} \otimes e_{8j+6}, & i = j + 9s; \\ e_{8(j+m)+7} \otimes w_{8j+6 \rightarrow 8j+7}, & i = j + 10s; \\ 0, & \text{otherwise.} \end{cases}$$

If  $8s \leq j < 9s$ , then

$$b_{ij} = \begin{cases} -w_{8(j+m+1) \rightarrow 8(j+m+1)+2} \otimes w_{8j+7 \rightarrow 8(j+1)}, & i = 2s + (j+1)_s; \\ 0, & \text{otherwise.} \end{cases}$$

If  $9s \leq j < 10s$ , then

$$b_{ij} = \begin{cases} w_{8(j+m+1) \rightarrow 8(j+m+1)+4} \otimes w_{8j+7 \rightarrow 8(j+1)}, & i = 2s + (j+1)_s; \\ -w_{8(j+m+1)+3 \rightarrow 8(j+m+1)+4} \otimes w_{8j+7 \rightarrow 8(j+1)+5}, & i = 12s + (j+1)_s; \\ 0, & \text{otherwise.} \end{cases}$$

If  $10s \leq j < 11s$ , then

$$b_{ij} = \begin{cases} w_{8(j+m)+7 \rightarrow 8(j+m+1)+6} \otimes w_{8j+7 \rightarrow 8(j+1)}, & i = (j+1)_s; \\ -2w_{8(j+m+1)+5 \rightarrow 8(j+m+1)+6} \otimes w_{8j+7 \rightarrow 8(j+1)+1}, & i = 4s + (j+1)_s; \\ -2e_{8(j+m+1)+6} \otimes w_{8j+7 \rightarrow 8(j+1)+2}, & i = 6s + (j+1)_s; \\ -w_{8(j+m+1)+5 \rightarrow 8(j+m+1)+6} \otimes w_{8j+7 \rightarrow 8(j+1)+3}, & i = 7s + (j+1)_s; \\ e_{8(j+m+1)+6} \otimes w_{8j+7 \rightarrow 8(j+1)+4}, & i = 10s + (j+1)_s; \\ 0, & \text{otherwise.} \end{cases}$$

(16) If  $r_0 = 15$ , then  $\Omega^{15}(Z_t^{(9)})$  is described with  $(18s \times 11s)$  matrix, whose entries  $b_{ij}$  have the following form:

If  $0 \leq j < s$ , then

$$b_{ij} = \begin{cases} w_{8(j+m)+1 \rightarrow 8(j+m+1)} \otimes e_{8j}, & i = j + 3s; \\ 2w_{8(j+m)+7 \rightarrow 8(j+m+1)} \otimes w_{8j \rightarrow 8j+1}, & i = j + 5s; \\ e_{8(j+m+1)} \otimes w_{8j \rightarrow 8j+2}, & i = j + 7s; \\ -2e_{8(j+m+1)} \otimes w_{8j \rightarrow 8j+5}, & i = j + 11s; \\ 0, & \text{otherwise.} \end{cases}$$

If  $s \leq j < 2s$ , then

$$b_{ij} = \begin{cases} -w_{8(j+m+1)+3 \rightarrow 8(j+m+1)+4} \otimes w_{8j+1 \rightarrow 8(j+1)}, & i = (j+1)_s; \\ -e_{8(j+m+1)+4} \otimes w_{8j+1 \rightarrow 8(j+1)}, & i = 2s + (j+1)_s; \\ w_{8(j+m+1)+1 \rightarrow 8(j+m+1)+4} \otimes w_{8j+1 \rightarrow 8(j+1)}, & i = 3s + (j+1)_s; \\ 0, & \text{otherwise.} \end{cases}$$

If  $2s \leq j < 3s$ , then

$$b_{ij} = \begin{cases} -2e_{8(j+m+1)+5} \otimes w_{8j+1 \rightarrow 8(j+1)}, & i = 4s + (j+1)_s; \\ 0, & \text{otherwise.} \end{cases}$$

If  $3s \leq j < 4s$ , then

$$b_{ij} = \begin{cases} -2e_{8(j+m+1)+6} \otimes w_{8j+2 \rightarrow 8(j+1)}, & i = s + (j+1)_s; \\ -w_{8(j+m+1) \rightarrow 8(j+m+1)+6} \otimes e_{8j+2}, & i = j + 4s; \\ 0, & \text{otherwise.} \end{cases}$$

If  $4s \leq j < 6s$ , then  $b_{ij} = 0$ .

If  $6s \leq j < 7s$ , then

$$b_{ij} = \begin{cases} 2e_{8(j+m+1)+3} \otimes w_{8j+5 \rightarrow 8(j+1)}, & i = (j+1)_s; \\ w_{8(j+m)+7 \rightarrow 8(j+m+1)+3} \otimes e_{8j+5}, & i = j + 4s; \\ w_{8(j+m+1) \rightarrow 8(j+m+1)+3} \otimes e_{8j+5}, & i = j + 5s; \\ 0, & \text{otherwise.} \end{cases}$$

If  $7s \leq j < 8s$ , then

$$b_{ij} = \begin{cases} w_{8(j+m+1)+5 \rightarrow 8(j+m+1)+6} \otimes w_{8j+5 \rightarrow 8(j+1)}, & i = 4s + (j+1)_s; \\ 0, & \text{otherwise.} \end{cases}$$

If  $8s \leq j < 9s$ , then

$$b_{ij} = \begin{cases} w_{8(j+m+1)+3 \rightarrow 8(j+m+1)+4} \otimes w_{8j+6 \rightarrow 8(j+1)}, & i = (j+1)_s; \\ -w_{8(j+m+1) \rightarrow 8(j+m+1)+4} \otimes e_{8j+6}, & i = j+4s; \\ -w_{8(j+m)+7 \rightarrow 8(j+m+1)+4} \otimes e_{8j+6}, & i = j+5s; \\ w_{8(j+m+1)+2 \rightarrow 8(j+m+1)+4} \otimes w_{8j+6 \rightarrow 8j+7}, & i = j+6s; \\ 0, & \text{otherwise.} \end{cases}$$

If  $9s \leq j < 10s$ , then

$$b_{ij} = \begin{cases} -e_{8(j+m+2)} \otimes w_{8j+7 \rightarrow 8(j+1)+5}, & i = 11s + (j+1)_s; \\ 0, & \text{otherwise.} \end{cases}$$

If  $10s \leq j < 11s$ , then

$$b_{ij} = \begin{cases} -w_{8(j+m+1)+3 \rightarrow 8(j+m+1)+7} \otimes w_{8j+7 \rightarrow 8(j+1)}, & i = (j+1)_s; \\ w_{8(j+m+1)+5 \rightarrow 8(j+m+1)+7} \otimes w_{8j+7 \rightarrow 8(j+1)}, & i = 4s + (j+1)_s; \\ 2e_{8(j+m+1)+7} \otimes w_{8j+7 \rightarrow 8(j+1)+1}, & i = 5s + (j+1)_s; \\ e_{8(j+m+1)+7} \otimes w_{8j+7 \rightarrow 8(j+1)+4}, & i = 9s + (j+1)_s; \\ 0, & \text{otherwise.} \end{cases}$$

(17) If  $r_0 = 16$ , then  $\Omega^{16}(Z_t^{(9)})$  is described with  $(19s \times 10s)$  matrix, whose entries  $b_{ij}$  have the following form:

If  $0 \leq j < s$ , then

$$b_{ij} = \begin{cases} -w_{8(j+m-1)+7 \rightarrow 8(j+m)+4} \otimes e_{8j}, & i = j; \\ w_{8(j+m) \rightarrow 8(j+m)+4} \otimes e_{8j}, & i = j+s; \\ w_{8(j+m-1)+7 \rightarrow 8(j+m)+4} \otimes e_{8j}, & i = j+2s; \\ 2e_{8(j+m)+4} \otimes w_{8j \rightarrow 8j+1}, & i = j+3s; \\ -w_{8(j+m)+2 \rightarrow 8(j+m)+4} \otimes w_{8j \rightarrow 8j+3}, & i = j+7s; \\ -2e_{8(j+m)+4} \otimes w_{8j \rightarrow 8j+5}, & i = j+11s; \\ 0, & \text{otherwise.} \end{cases}$$

If  $s \leq j < 2s$ , then

$$b_{ij} = \begin{cases} 2e_{8(j+m)+6} \otimes w_{8j \rightarrow 8j+1}, & i = j+3s; \\ -2w_{8(j+m)+5 \rightarrow 8(j+m)+6} \otimes w_{8j \rightarrow 8j+5}, & i = j+11s; \\ 0, & \text{otherwise.} \end{cases}$$

If  $2s \leq j < 3s$ , then

$$b_{ij} = \begin{cases} -e_{8(j+m)+7} \otimes w_{8j+1 \rightarrow 8(j+1)}, & i = (j+1)_s; \\ -2e_{8(j+m)+7} \otimes w_{8j+1 \rightarrow 8(j+1)}, & i = 2s + (j+1)_s; \\ -w_{8(j+m)+4 \rightarrow 8(j+m)+7} \otimes e_{8j+1}, & i = j+s; \\ w_{8(j+m)+6 \rightarrow 8(j+m)+7} \otimes e_{8j+1}, & i = j+2s; \\ 0, & \text{otherwise.} \end{cases}$$

If  $3s \leq j < 4s$ , then

$$b_{ij} = \begin{cases} 2w_{8(j+m)+7 \rightarrow 8(j+m+1)} \otimes w_{8j+2 \rightarrow 8(j+1)}, & i = (j+1)_s; \\ -e_{8(j+m+1)} \otimes w_{8j+2 \rightarrow 8(j+1)}, & i = s + (j+1)_s; \\ -w_{8(j+m)+7 \rightarrow 8(j+m+1)} \otimes w_{8j+2 \rightarrow 8(j+1)}, & i = 2s + (j+1)_s; \\ -w_{8(j+m)+1 \rightarrow 8(j+m+1)} \otimes e_{8j+2}, & i = j + 3s; \\ 0, & \text{otherwise.} \end{cases}$$

If  $4s \leq j < 5s$ , then

$$b_{ij} = \begin{cases} -w_{8(j+m)+7 \rightarrow 8(j+m+1)+1} \otimes w_{8j+3 \rightarrow 8(j+1)}, & i = (j+1)_s; \\ e_{8(j+m+1)+1} \otimes w_{8j+3 \rightarrow 8(j+1)+2}, & i = 6s + (j+1)_s; \\ 0, & \text{otherwise.} \end{cases}$$

If  $5s \leq j < 6s$ , then

$$b_{ij} = \begin{cases} w_{8(j+m)+7 \rightarrow 8(j+m+1)+2} \otimes w_{8j+4 \rightarrow 8(j+1)}, & i = (j+1)_s; \\ -w_{8(j+m+1)+1 \rightarrow 8(j+m+1)+2} \otimes w_{8j+4 \rightarrow 8(j+1)+2}, & i = 6s + (j+1)_s; \\ 0, & \text{otherwise.} \end{cases}$$

If  $6s \leq j < 7s$ , then

$$b_{ij} = \begin{cases} w_{8(j+m)+2 \rightarrow 8(j+m)+7} \otimes e_{8j+5}, & i = j + 4s; \\ 0, & \text{otherwise.} \end{cases}$$

If  $7s \leq j < 8s$ , then

$$b_{ij} = \begin{cases} -w_{8(j+m)+3 \rightarrow 8(j+m+1)} \otimes e_{8j+6}, & i = j + 6s; \\ e_{8(j+m+1)} \otimes w_{8j+6 \rightarrow 8j+7}, & i = j + 10s; \\ 0, & \text{otherwise.} \end{cases}$$

If  $8s \leq j < 9s$ , then

$$b_{ij} = \begin{cases} w_{8(j+m)+7 \rightarrow 8(j+m+1)+3} \otimes w_{8j+7 \rightarrow 8(j+1)}, & i = (j+1)_s; \\ -w_{8(j+m+1)+1 \rightarrow 8(j+m+1)+3} \otimes w_{8j+7 \rightarrow 8(j+1)+2}, & i = 6s + (j+1)_s; \\ 0, & \text{otherwise.} \end{cases}$$

If  $9s \leq j < 10s$ , then

$$b_{ij} = \begin{cases} -e_{8(j+m+1)+5} \otimes w_{8j+7 \rightarrow 8(j+1)+5}, & i = 12s + (j+1)_s; \\ 0, & \text{otherwise.} \end{cases}$$

(18) If  $r_0 = 17$ , then  $\Omega^{17}(Z_t^{(9)})$  is described with  $(18s \times 8s)$  matrix, whose entries  $b_{ij}$  have the following form:

If  $0 \leq j < s$ , then

$$b_{ij} = \begin{cases} -w_{8(j+m)+2 \rightarrow 8(j+m)+7} \otimes e_{8j}, & i = j; \\ e_{8(j+m)+7} \otimes w_{8j \rightarrow 8j+1}, & i = j + 4s; \\ -2e_{8(j+m)+7} \otimes w_{8j \rightarrow 8j+5}, & i = j + 10s; \\ 0, & \text{otherwise.} \end{cases}$$

If  $s \leq j < 2s$ , then

$$b_{ij} = \begin{cases} -2e_{8(j+m+1)+6} \otimes w_{8j+1 \rightarrow 8(j+1)}, & i = 2s + (j+1)_s; \\ -w_{8(j+m+1)+5 \rightarrow 8(j+m+1)+6} \otimes w_{8j+1 \rightarrow 8(j+1)}, & i = 3s + (j+1)_s; \\ -w_{8(j+m)+7 \rightarrow 8(j+m+1)+6} \otimes e_{8j+1}, & i = j + 3s; \\ 0, & \text{otherwise.} \end{cases}$$

If  $2s \leq j < 3s$ , then

$$b_{ij} = \begin{cases} w_{8(j+m+1) \rightarrow 8(j+m+1)+1} \otimes e_{8j+2}, & i = j + 4s; \\ e_{8(j+m+1)+1} \otimes w_{8j+2 \rightarrow 8j+7}, & i = j + 14s; \\ 0, & \text{otherwise.} \end{cases}$$

If  $3s \leq j < 5s$ , then  $b_{ij} = 0$ .

If  $5s \leq j < 6s$ , then

$$b_{ij} = \begin{cases} -2w_{8(j+m+1)+2 \rightarrow 8(j+m+1)+4} \otimes w_{8j+5 \rightarrow 8(j+1)}, & i = (j+1)_s; \\ 2e_{8(j+m+1)+4} \otimes w_{8j+5 \rightarrow 8(j+1)}, & i = s + (j+1)_s; \\ w_{8(j+m+1) \rightarrow 8(j+m+1)+4} \otimes e_{8j+5}, & i = j + 4s; \\ w_{8(j+m)+7 \rightarrow 8(j+m+1)+4} \otimes e_{8j+5}, & i = j + 5s; \\ 0, & \text{otherwise.} \end{cases}$$

If  $6s \leq j < 7s$ , then

$$b_{ij} = \begin{cases} e_{8(j+m+1)+5} \otimes w_{8j+6 \rightarrow 8j+7}, & i = j + 11s; \\ 0, & \text{otherwise.} \end{cases}$$

If  $7s \leq j < 8s$ , then

$$b_{ij} = \begin{cases} -w_{8(j+m+1)+2 \rightarrow 8(j+m+2)} \otimes w_{8j+7 \rightarrow 8(j+1)}, & i = (j+1)_s; \\ w_{8(j+m+1)+4 \rightarrow 8(j+m+2)} \otimes w_{8j+7 \rightarrow 8(j+1)}, & i = s + (j+1)_s; \\ 2w_{8(j+m+1)+7 \rightarrow 8(j+m+2)} \otimes w_{8j+7 \rightarrow 8(j+1)+1}, & i = 4s + (j+1)_s; \\ -2e_{8(j+m+2)} \otimes w_{8j+7 \rightarrow 8(j+1)+1}, & i = 5s + (j+1)_s; \\ -e_{8(j+m+2)} \otimes w_{8j+7 \rightarrow 8(j+1)+4}, & i = 8s + (j+1)_s; \\ -w_{8(j+m+1)+7 \rightarrow 8(j+m+2)} \otimes w_{8j+7 \rightarrow 8(j+1)+5}, & i = 10s + (j+1)_s; \\ 0, & \text{otherwise.} \end{cases}$$

(19) If  $r_0 = 18$ , then  $\Omega^{18}(Z_t^{(9)})$  is described with  $(19s \times 9s)$  matrix, whose entries  $b_{ij}$  have the following form:

If  $0 \leq j < s$ , then

$$b_{ij} = \begin{cases} 3e_{8(j+m)+7} \otimes w_{8j \rightarrow 8(j+1)}, & i = (j+1)_s; \\ -w_{8(j+m) \rightarrow 8(j+m)+7} \otimes e_{8j}, & i = j + s; \\ -2w_{8(j+m)+5 \rightarrow 8(j+m)+7} \otimes w_{8j \rightarrow 8j+1}, & i = j + 3s; \\ -2w_{8(j+m)+1 \rightarrow 8(j+m)+7} \otimes w_{8j \rightarrow 8j+1}, & i = j + 4s; \\ -w_{8(j+m)+2 \rightarrow 8(j+m)+7} \otimes w_{8j \rightarrow 8j+2}, & i = j + 5s; \\ -w_{8(j+m)+5 \rightarrow 8(j+m)+7} \otimes w_{8j \rightarrow 8j+4}, & i = j + 9s; \\ -w_{8(j+m)+6 \rightarrow 8(j+m)+7} \otimes w_{8j \rightarrow 8j+5}, & i = j + 11s; \\ 0, & \text{otherwise.} \end{cases}$$

If  $s \leq j < 2s$ , then

$$b_{ij} = \begin{cases} -e_{8(j+m+1)} \otimes w_{8j+1 \rightarrow 8(j+1)}, & i = s + (j+1)_s; \\ -2e_{8(j+m+1)} \otimes w_{8j+1 \rightarrow 8(j+1)}, & i = 2s + (j+1)_s; \\ -w_{8(j+m)+5 \rightarrow 8(j+m+1)} \otimes e_{8j+1}, & i = j + 2s; \\ w_{8(j+m)+1 \rightarrow 8(j+m+1)} \otimes e_{8j+1}, & i = j + 3s; \\ 0, & \text{otherwise.} \end{cases}$$

If  $2s \leq j < 3s$ , then

$$b_{ij} = \begin{cases} w_{8(j+m)+7 \rightarrow 8(j+m+1)+1} \otimes w_{8j+2 \rightarrow 8(j+1)}, & i = (j+1)_s; \\ 2w_{8(j+m+1) \rightarrow 8(j+m+1)+1} \otimes w_{8j+2 \rightarrow 8(j+1)}, & i = s + (j+1)_s; \\ w_{8(j+m+1) \rightarrow 8(j+m+1)+1} \otimes w_{8j+2 \rightarrow 8(j+1)}, & i = 2s + (j+1)_s; \\ w_{8(j+m)+2 \rightarrow 8(j+m+1)+1} \otimes e_{8j+2}, & i = j + 3s; \\ 0, & \text{otherwise.} \end{cases}$$

If  $3s \leq j < 4s$ , then

$$b_{ij} = \begin{cases} -w_{8(j+m+1) \rightarrow 8(j+m+1)+2} \otimes w_{8j+3 \rightarrow 8(j+1)}, & i = s + (j+1)_s; \\ -2w_{8(j+m+1) \rightarrow 8(j+m+1)+2} \otimes w_{8j+3 \rightarrow 8(j+1)}, & i = 2s + (j+1)_s; \\ -e_{8(j+m+1)+2} \otimes w_{8j+3 \rightarrow 8(j+1)+2}, & i = 5s + (j+1)_s; \\ 0, & \text{otherwise.} \end{cases}$$

If  $4s \leq j < 5s$ , then

$$b_{ij} = \begin{cases} w_{8(j+m+1) \rightarrow 8(j+m+1)+3} \otimes w_{8j+4 \rightarrow 8(j+1)}, & i = s + (j+1)_s; \\ 2w_{8(j+m+1) \rightarrow 8(j+m+1)+3} \otimes w_{8j+4 \rightarrow 8(j+1)}, & i = 2s + (j+1)_s; \\ w_{8(j+m+1)+2 \rightarrow 8(j+m+1)+3} \otimes w_{8j+4 \rightarrow 8(j+1)+2}, & i = 5s + (j+1)_s; \\ 0, & \text{otherwise.} \end{cases}$$

If  $5s \leq j < 6s$ , then

$$b_{ij} = \begin{cases} -w_{8(j+m)+7 \rightarrow 8(j+m+1)} \otimes w_{8j+5 \rightarrow 8(j+1)}, & i = (j+1)_s; \\ e_{8(j+m+1)} \otimes w_{8j+5 \rightarrow 8(j+1)}, & i = 2s + (j+1)_s; \\ w_{8(j+m)+5 \rightarrow 8(j+m+1)} \otimes e_{8j+5}, & i = j + 7s; \\ 0, & \text{otherwise.} \end{cases}$$



If  $6s \leq j < 7s$ , then

$$b_{ij} = \begin{cases} w_{8(j+m)+6 \rightarrow 8(j+m+1)+5} \otimes e_{8j+6}, & i = j + 7s; \\ -w_{8(j+m)+7 \rightarrow 8(j+m+1)+5} \otimes w_{8j+6 \rightarrow 8j+7}, & i = j + 10s; \\ 0, & \text{otherwise.} \end{cases}$$

If  $7s \leq j < 8s$ , then

$$b_{ij} = \begin{cases} w_{8(j+m+1) \rightarrow 8(j+m+1)+4} \otimes w_{8j+7 \rightarrow 8(j+1)}, & i = s + (j + 1)_s; \\ 2w_{8(j+m+1)+1 \rightarrow 8(j+m+1)+4} \otimes w_{8j+7 \rightarrow 8(j+1)+1}, & i = 4s + (j + 1)_s; \\ w_{8(j+m+1)+2 \rightarrow 8(j+m+1)+4} \otimes w_{8j+7 \rightarrow 8(j+1)+2}, & i = 5s + (j + 1)_s; \\ 0, & \text{otherwise.} \end{cases}$$

If  $8s \leq j < 9s$ , then

$$b_{ij} = \begin{cases} -2w_{8(j+m+1)+5 \rightarrow 8(j+m+1)+6} \otimes w_{8j+7 \rightarrow 8(j+1)+1}, & i = 3s + (j + 1)_s; \\ -w_{8(j+m+1)+5 \rightarrow 8(j+m+1)+6} \otimes w_{8j+7 \rightarrow 8(j+1)+4}, & i = 9s + (j + 1)_s; \\ -e_{8(j+m+1)+6} \otimes w_{8j+7 \rightarrow 8(j+1)+5}, & i = 11s + (j + 1)_s; \\ 0, & \text{otherwise.} \end{cases}$$

(20) If  $r_0 = 19$ , then  $\Omega^{19}(Z_t^{(9)})$  is described with  $(16s \times 8s)$  matrix, whose entries  $b_{ij}$  have the following form:

If  $0 \leq j < s$ , then

$$b_{ij} = \begin{cases} -w_{8(j+m)+5 \rightarrow 8(j+m+1)} \otimes e_{8j}, & i = j + 3s; \\ e_{8(j+m+1)} \otimes w_{8j \rightarrow 8j+1}, & i = j + 4s; \\ -e_{8(j+m+1)} \otimes w_{8j \rightarrow 8j+5}, & i = j + 9s; \\ 0, & \text{otherwise.} \end{cases}$$

If  $s \leq j < 2s$ , then

$$b_{ij} = \begin{cases} -w_{8(j+m+1) \rightarrow 8(j+m+1)+1} \otimes e_{8j+1}, & i = j + 3s; \\ 0, & \text{otherwise.} \end{cases}$$

If  $2s \leq j < 3s$ , then

$$b_{ij} = \begin{cases} -w_{8(j+m+1)+1 \rightarrow 8(j+m+1)+2} \otimes w_{8j+2 \rightarrow 8(j+1)}, & i = 2s + (j + 1)_s; \\ w_{8(j+m)+7 \rightarrow 8(j+m+1)+2} \otimes e_{8j+2}, & i = j + 3s; \\ w_{8(j+m+1) \rightarrow 8(j+m+1)+2} \otimes w_{8j+2 \rightarrow 8j+3}, & i = j + 4s; \\ w_{8(j+m)+7 \rightarrow 8(j+m+1)+2} \otimes w_{8j+2 \rightarrow 8j+4}, & i = j + 5s; \\ -e_{8(j+m+1)+2} \otimes w_{8j+2 \rightarrow 8j+7}, & i = j + 10s; \\ 0, & \text{otherwise.} \end{cases}$$

If  $3s \leq j < 4s$ , then  $b_{ij} = 0$ .

If  $4s \leq j < 5s$ , then

$$b_{ij} = \begin{cases} 2w_{8(j+m+1)+1 \rightarrow 8(j+m+1)+4} \otimes w_{8j+4 \rightarrow 8(j+1)}, & i = 2s + (j + 1)_s; \\ 0, & \text{otherwise.} \end{cases}$$

If  $5s \leq j < 6s$ , then

$$b_{ij} = \begin{cases} -w_{8(j+m)+7 \rightarrow 8(j+m+1)+5} \otimes e_{8j+5}, & i = j + 3s; \\ -w_{8(j+m+1) \rightarrow 8(j+m+1)+5} \otimes e_{8j+5}, & i = j + 4s; \\ 0, & \text{otherwise.} \end{cases}$$

If  $6s \leq j < 7s$ , then

$$b_{ij} = \begin{cases} w_{8(j+m)+7 \rightarrow 8(j+m+1)+6} \otimes e_{8j+6}, & i = j + 4s; \\ -e_{8(j+m+1)+6} \otimes w_{8j+6 \rightarrow 8j+7}, & i = j + 8s; \\ 0, & \text{otherwise.} \end{cases}$$

If  $7s \leq j < 8s$ , then  $b_{ij} = 0$ .

(21) If  $r_0 = 20$ , then  $\Omega^{20}(Z_t^{(9)})$  is described with  $(16s \times 8s)$  matrix, whose entries  $b_{ij}$  have the following form:

If  $0 \leq j < s$ , then

$$b_{ij} = \begin{cases} 3w_{8(j+m)+7 \rightarrow 8(j+m+1)} \otimes w_{8j \rightarrow 8(j+1)}, & i = (j+1)_s; \\ 2e_{8(j+m+1)} \otimes w_{8j \rightarrow 8(j+1)}, & i = s + (j+1)_s; \\ w_{8(j+m)+2 \rightarrow 8(j+m+1)} \otimes w_{8j \rightarrow 8j+1}, & i = j + 2s; \\ w_{8(j+m)+6 \rightarrow 8(j+m+1)} \otimes w_{8j \rightarrow 8j+1}, & i = j + 3s; \\ -w_{8(j+m)+6 \rightarrow 8(j+m+1)} \otimes w_{8j \rightarrow 8j+4}, & i = j + 7s; \\ -2w_{8(j+m)+6 \rightarrow 8(j+m+1)} \otimes w_{8j \rightarrow 8j+5}, & i = j + 8s; \\ 0, & \text{otherwise.} \end{cases}$$

If  $s \leq j < 2s$ , then

$$b_{ij} = \begin{cases} 2w_{8(j+m)+7 \rightarrow 8(j+m+1)+1} \otimes w_{8j+1 \rightarrow 8(j+1)}, & i = (j+1)_s; \\ -2w_{8(j+m+1) \rightarrow 8(j+m+1)+1} \otimes w_{8j+1 \rightarrow 8(j+1)}, & i = s + (j+1)_s; \\ -w_{8(j+m)+2 \rightarrow 8(j+m+1)+1} \otimes e_{8j+1}, & i = j + s; \\ 0, & \text{otherwise.} \end{cases}$$

If  $2s \leq j < 3s$ , then

$$b_{ij} = \begin{cases} -w_{8(j+m)+7 \rightarrow 8(j+m+1)+2} \otimes w_{8j+2 \rightarrow 8(j+1)}, & i = (j+1)_s; \\ 2w_{8(j+m+1) \rightarrow 8(j+m+1)+2} \otimes w_{8j+2 \rightarrow 8(j+1)}, & i = s + (j+1)_s; \\ w_{8(j+m)+3 \rightarrow 8(j+m+1)+2} \otimes e_{8j+2}, & i = j + 2s; \\ 0, & \text{otherwise.} \end{cases}$$

If  $3s \leq j < 4s$ , then

$$b_{ij} = \begin{cases} 2w_{8(j+m)+7 \rightarrow 8(j+m+1)+3} \otimes w_{8j+3 \rightarrow 8(j+1)}, & i = (j+1)_s; \\ -2w_{8(j+m+1) \rightarrow 8(j+m+1)+3} \otimes w_{8j+3 \rightarrow 8(j+1)}, & i = s + (j+1)_s; \\ -e_{8(j+m+1)+3} \otimes w_{8j+3 \rightarrow 8(j+1)+2}, & i = 4s + (j+1)_s; \\ 0, & \text{otherwise.} \end{cases}$$

If  $4s \leq j < 5s$ , then

$$b_{ij} = \begin{cases} -2w_{8(j+m)+7 \rightarrow 8(j+m+1)+4} \otimes w_{8j+4 \rightarrow 8(j+1)}, & i = (j+1)_s; \\ 2w_{8(j+m+1) \rightarrow 8(j+m+1)+4} \otimes w_{8j+4 \rightarrow 8(j+1)}, & i = s + (j+1)_s; \\ w_{8(j+m+1)+3 \rightarrow 8(j+m+1)+4} \otimes w_{8j+4 \rightarrow 8(j+1)+2}, & i = 4s + (j+1)_s; \\ 0, & \text{otherwise.} \end{cases}$$

If  $5s \leq j < 6s$ , then

$$b_{ij} = \begin{cases} w_{8(j+m)+7 \rightarrow 8(j+m+1)+5} \otimes w_{8j+5 \rightarrow 8(j+1)}, & i = (j+1)_s; \\ -2w_{8(j+m+1) \rightarrow 8(j+m+1)+5} \otimes w_{8j+5 \rightarrow 8(j+1)}, & i = s + (j+1)_s; \\ -w_{8(j+m)+6 \rightarrow 8(j+m+1)+5} \otimes e_{8j+5}, & i = j + 3s; \\ 0, & \text{otherwise.} \end{cases}$$

If  $6s \leq j < 7s$ , then

$$b_{ij} = \begin{cases} -w_{8(j+m)+7 \rightarrow 8(j+m+1)+6} \otimes w_{8j+6 \rightarrow 8(j+1)}, & i = (j+1)_s; \\ -2e_{8(j+m+1)+6} \otimes w_{8j+6 \rightarrow 8(j+1)+5}, & i = 8s + (j+1)_s; \\ -w_{8(j+m)+7 \rightarrow 8(j+m+1)+6} \otimes w_{8j+6 \rightarrow 8j+7}, & i = j + 7s; \\ 0, & \text{otherwise.} \end{cases}$$

If  $7s \leq j < 8s$ , then

$$b_{ij} = \begin{cases} -w_{8(j+m+1)+2 \rightarrow 8(j+m+1)+7} \otimes w_{8j+7 \rightarrow 8(j+1)+1}, & i = 2s + (j+1)_s; \\ -w_{8(j+m+1)+6 \rightarrow 8(j+m+1)+7} \otimes w_{8j+7 \rightarrow 8(j+1)+1}, & i = 3s + (j+1)_s; \\ w_{8(j+m+1)+6 \rightarrow 8(j+m+1)+7} \otimes w_{8j+7 \rightarrow 8(j+1)+5}, & i = 8s + (j+1)_s; \\ w_{8(j+m+1)+1 \rightarrow 8(j+m+1)+7} \otimes w_{8j+7 \rightarrow 8(j+1)+5}, & i = 10s + (j+1)_s; \\ 0, & \text{otherwise.} \end{cases}$$

(22) If  $r_0 = 21$ , then  $\Omega^{21}(Z_t^{(9)})$  is described with  $(14s \times 9s)$  matrix, whose entries  $b_{ij}$  have the following form:

If  $s \leq j < 2s$ , then

$$b_{ij} = \begin{cases} -w_{8(j+m)+6 \rightarrow 8(j+m+1)+5} \otimes e_{8j}, & i = j + s; \\ -2w_{8(j+m)+7 \rightarrow 8(j+m+1)+5} \otimes w_{8j \rightarrow 8j+1}, & i = j + 2s; \\ -w_{8(j+m+1) \rightarrow 8(j+m+1)+5} \otimes w_{8j \rightarrow 8j+2}, & i = j + 3s; \\ -w_{8(j+m)+7 \rightarrow 8(j+m+1)+5} \otimes w_{8j \rightarrow 8j+3}, & i = j + 4s; \\ -w_{8(j+m+1) \rightarrow 8(j+m+1)+5} \otimes w_{8j \rightarrow 8j+4}, & i = j + 5s; \\ -w_{8(j+m+1) \rightarrow 8(j+m+1)+5} \otimes w_{8j \rightarrow 8j+6}, & i = j + 8s; \\ 0, & \text{otherwise.} \end{cases}$$

If  $2s \leq j < 3s$ , then

$$b_{ij} = \begin{cases} w_{8(j+m)+7 \rightarrow 8(j+m+1)+2} \otimes e_{8j+1}, & i = j + s; \\ 0, & \text{otherwise.} \end{cases}$$

If  $3s \leq j < 4s$ , then

$$b_{ij} = \begin{cases} -w_{8(j+m+1)+2 \rightarrow 8(j+m+1)+3} \otimes w_{8j+2 \rightarrow 8(j+1)}, & i = (j+1)_s; \\ -w_{8(j+m+1) \rightarrow 8(j+m+1)+3} \otimes e_{8j+2}, & i = j+s; \\ -w_{8(j+m)+7 \rightarrow 8(j+m+1)+3} \otimes w_{8j+2 \rightarrow 8j+3}, & i = j+2s; \\ e_{8(j+m+1)+3} \otimes w_{8j+2 \rightarrow 8j+7}, & i = j+7s; \\ 0, & \text{otherwise.} \end{cases}$$

If  $4s \leq j < 5s$ , then  $b_{ij} = 0$ .

If  $5s \leq j < 6s$ , then

$$b_{ij} = \begin{cases} -2w_{8(j+m+1)+2 \rightarrow 8(j+m+1)+7} \otimes w_{8j+4 \rightarrow 8(j+1)}, & i = (j+1)_s; \\ -e_{8(j+m+1)+7} \otimes w_{8j+4 \rightarrow 8(j+1)+1}, & i = 3s + (j+1)_s; \\ 0, & \text{otherwise.} \end{cases}$$

If  $6s \leq j < 7s$ , then

$$b_{ij} = \begin{cases} 2e_{8(j+m+1)+6} \otimes w_{8j+5 \rightarrow 8(j+1)}, & i = 2s + (j+1)_s; \\ w_{8(j+m)+7 \rightarrow 8(j+m+1)+6} \otimes e_{8j+5}, & i = j+s; \\ 0, & \text{otherwise.} \end{cases}$$

If  $7s \leq j < 8s$ , then

$$b_{ij} = \begin{cases} w_{8(j+m+1) \rightarrow 8(j+m+1)+7} \otimes e_{8j+6}, & i = j+2s; \\ w_{8(j+m+1)+3 \rightarrow 8(j+m+1)+7} \otimes w_{8j+6 \rightarrow 8j+7}, & i = j+3s; \\ w_{8(j+m+1)+6 \rightarrow 8(j+m+1)+7} \otimes w_{8j+6 \rightarrow 8j+7}, & i = j+4s; \\ 0, & \text{otherwise.} \end{cases}$$

If  $8s \leq j < 9s$ , then

$$b_{ij} = \begin{cases} w_{8(j+m+1)+2 \rightarrow 8(j+m+2)} \otimes w_{8j+7 \rightarrow 8(j+1)}, & i = (j+1)_s; \\ w_{8(j+m+1)+6 \rightarrow 8(j+m+2)} \otimes w_{8j+7 \rightarrow 8(j+1)}, & i = 2s + (j+1)_s; \\ w_{8(j+m+1)+7 \rightarrow 8(j+m+2)} \otimes w_{8j+7 \rightarrow 8(j+1)+1}, & i = 3s + (j+1)_s; \\ e_{8(j+m+2)} \otimes w_{8j+7 \rightarrow 8(j+1)+2}, & i = 4s + (j+1)_s; \\ w_{8(j+m+1)+7 \rightarrow 8(j+m+2)} \otimes w_{8j+7 \rightarrow 8(j+1)+3}, & i = 5s + (j+1)_s; \\ e_{8(j+m+2)} \otimes w_{8j+7 \rightarrow 8(j+1)+4}, & i = 6s + (j+1)_s; \\ e_{8(j+m+2)} \otimes w_{8j+7 \rightarrow 8(j+1)+6}, & i = 9s + (j+1)_s; \\ 0, & \text{otherwise.} \end{cases}$$

(23) If  $r_0 = 22$ , then  $\Omega^{22}(Z_t^{(9)})$  is described with  $(13s \times 8s)$  matrix, whose entries  $b_{ij}$  have the following form:

If  $0 \leq j < s$ , then

$$b_{ij} = \begin{cases} w_{8(j+m-1)+7 \rightarrow 8(j+m)+7} \otimes e_{8j}, & i = j + s; \\ 3e_{8(j+m)+7} \otimes w_{8j \rightarrow 8(j+1)}, & i = s + (j+1)_s; \\ -w_{8(j+m)+3 \rightarrow 8(j+m)+7} \otimes w_{8j \rightarrow 8j+1}, & i = j + 2s; \\ -2w_{8(j+m)+4 \rightarrow 8(j+m)+7} \otimes w_{8j \rightarrow 8j+2}, & i = j + 3s; \\ w_{8(j+m)+6 \rightarrow 8(j+m)+7} \otimes w_{8j \rightarrow 8j+3}, & i = j + 5s; \\ 0, & \text{otherwise.} \end{cases}$$

If  $s \leq j < 2s$ , then

$$b_{ij} = \begin{cases} -2w_{8(j+m+1) \rightarrow 8(j+m+1)+2} \otimes w_{8j+1 \rightarrow 8(j+1)}, & i = (j+1)_s; \\ 2w_{8(j+m)+7 \rightarrow 8(j+m+1)+2} \otimes w_{8j+1 \rightarrow 8(j+1)}, & i = s + (j+1)_s; \\ -w_{8(j+m)+3 \rightarrow 8(j+m+1)+2} \otimes e_{8j+1}, & i = j + s; \\ 0, & \text{otherwise.} \end{cases}$$

If  $2s \leq j < 3s$ , then

$$b_{ij} = \begin{cases} -2w_{8(j+m+1) \rightarrow 8(j+m+1)+3} \otimes w_{8j+2 \rightarrow 8(j+1)}, & i = (j+1)_s; \\ -2w_{8(j+m)+7 \rightarrow 8(j+m+1)+3} \otimes w_{8j+2 \rightarrow 8(j+1)}, & i = s + (j+1)_s; \\ w_{8(j+m)+4 \rightarrow 8(j+m+1)+3} \otimes e_{8j+2}, & i = j + s; \\ 0, & \text{otherwise.} \end{cases}$$

If  $3s \leq j < 4s$ , then

$$b_{ij} = \begin{cases} -2w_{8(j+m+1) \rightarrow 8(j+m+1)+4} \otimes w_{8j+3 \rightarrow 8(j+1)}, & i = (j+1)_s; \\ 2w_{8(j+m)+7 \rightarrow 8(j+m+1)+4} \otimes w_{8j+3 \rightarrow 8(j+1)}, & i = s + (j+1)_s; \\ -e_{8(j+m+1)+4} \otimes w_{8j+3 \rightarrow 8(j+1)+2}, & i = 3s + (j+1)_s; \\ 0, & \text{otherwise.} \end{cases}$$

If  $4s \leq j < 5s$ , then  $b_{ij} = 0$ .

If  $5s \leq j < 6s$ , then

$$b_{ij} = \begin{cases} w_{8(j+m)+7 \rightarrow 8(j+m+1)+6} \otimes w_{8j+5 \rightarrow 8(j+1)}, & i = s + (j+1)_s; \\ w_{8(j+m)+6 \rightarrow 8(j+m+1)+6} \otimes w_{8j+5 \rightarrow 8j+6}, & i = j + 5s; \\ 0, & \text{otherwise.} \end{cases}$$

If  $6s \leq j < 7s$ , then

$$b_{ij} = \begin{cases} w_{8(j+m+1) \rightarrow 8(j+m+1)+1} \otimes w_{8j+6 \rightarrow 8j+7}, & i = j + 6s; \\ 0, & \text{otherwise.} \end{cases}$$

If  $7s \leq j < 8s$ , then

$$b_{ij} = \begin{cases} -w_{8(j+m+1) \rightarrow 8(j+m+2)} \otimes w_{8j+7 \rightarrow 8(j+1)}, & i = (j+1)_s; \\ -w_{8(j+m+1)+3 \rightarrow 8(j+m+2)} \otimes w_{8j+7 \rightarrow 8(j+1)+1}, & i = 2s + (j+1)_s; \\ -w_{8(j+m+1)+1 \rightarrow 8(j+m+2)} \otimes w_{8j+7 \rightarrow 8(j+1)+4}, & i = 6s + (j+1)_s; \\ -w_{8(j+m+1)+2 \rightarrow 8(j+m+2)} \otimes w_{8j+7 \rightarrow 8(j+1)+5}, & i = 7s + (j+1)_s; \\ 0, & \text{otherwise.} \end{cases}$$

(24) If  $r_0 = 23$ , then  $\Omega^{23}(Z_t^{(9)})$  is described with  $(11s \times 10s)$  matrix, whose entries  $b_{ij}$  have the following form:

If  $0 \leq j < s$ , then

$$b_{ij} = \begin{cases} 2w_{8(j+m+1) \rightarrow 8(j+m+1)+2} \otimes w_{8j \rightarrow 8j+1}, & i = j + 2s; \\ -w_{8(j+m)+7 \rightarrow 8(j+m+1)+2} \otimes w_{8j \rightarrow 8j+2}, & i = j + 3s; \\ -w_{8(j+m+1) \rightarrow 8(j+m+1)+2} \otimes w_{8j \rightarrow 8j+3}, & i = j + 4s; \\ 0, & \text{otherwise.} \end{cases}$$

If  $s \leq j < 2s$ , then

$$b_{ij} = \begin{cases} -w_{8(j+m)+7 \rightarrow 8(j+m+1)+6} \otimes w_{8j \rightarrow 8j+2}, & i = j + 2s; \\ -w_{8(j+m)+7 \rightarrow 8(j+m+1)+6} \otimes w_{8j \rightarrow 8j+6}, & i = j + 6s; \\ 0, & \text{otherwise.} \end{cases}$$

If  $2s \leq j < 3s$ , then

$$b_{ij} = \begin{cases} w_{8(j+m+1) \rightarrow 8(j+m+1)+3} \otimes e_{8j+1}, & i = j; \\ 0, & \text{otherwise.} \end{cases}$$

If  $3s \leq j < 4s$ , then

$$b_{ij} = \begin{cases} -w_{8(j+m+1)+3 \rightarrow 8(j+m+1)+4} \otimes w_{8j+2 \rightarrow 8(j+1)}, & i = (j+1)_s; \\ -w_{8(j+m)+7 \rightarrow 8(j+m+1)+4} \otimes e_{8j+2}, & i = j; \\ -w_{8(j+m+1) \rightarrow 8(j+m+1)+4} \otimes w_{8j+2 \rightarrow 8j+3}, & i = j + s; \\ e_{8(j+m+1)+4} \otimes w_{8j+2 \rightarrow 8j+7}, & i = j + 6s; \\ 0, & \text{otherwise.} \end{cases}$$

If  $4s \leq j < 5s$ , then

$$b_{ij} = \begin{cases} -w_{8(j+m+1)+3 \rightarrow 8(j+m+1)+7} \otimes w_{8j+3 \rightarrow 8(j+1)}, & i = (j+1)_s; \\ -w_{8(j+m+1)+5 \rightarrow 8(j+m+1)+7} \otimes w_{8j+3 \rightarrow 8(j+1)}, & i = s + (j+1)_s; \\ e_{8(j+m+1)+7} \otimes w_{8j+3 \rightarrow 8(j+1)+2}, & i = 3s + (j+1)_s; \\ 0, & \text{otherwise.} \end{cases}$$

If  $5s \leq j < 6s$ , then

$$b_{ij} = \begin{cases} 2w_{8(j+m+1)+3 \rightarrow 8(j+m+2)} \otimes w_{8j+4 \rightarrow 8(j+1)}, & i = (j+1)_s; \\ -w_{8(j+m+1)+5 \rightarrow 8(j+m+2)} \otimes w_{8j+4 \rightarrow 8(j+1)}, & i = s + (j+1)_s; \\ -e_{8(j+m+2)} \otimes w_{8j+4 \rightarrow 8(j+1)+1}, & i = 2s + (j+1)_s; \\ w_{8(j+m+1)+7 \rightarrow 8(j+m+2)} \otimes w_{8j+4 \rightarrow 8(j+1)+2}, & i = 3s + (j+1)_s; \\ 0, & \text{otherwise.} \end{cases}$$

If  $6s \leq j < 7s$ , then

$$b_{ij} = \begin{cases} w_{8(j+m+1) \rightarrow 8(j+m+1)+7} \otimes e_{8j+5}, & i = j; \\ 0, & \text{otherwise.} \end{cases}$$

If  $7s \leq j < 8s$ , then

$$b_{ij} = \begin{cases} -w_{8(j+m+1)+2 \rightarrow 8(j+m+2)} \otimes w_{8j+6 \rightarrow 8j+7}, & i = j + s; \\ 0, & \text{otherwise.} \end{cases}$$

If  $8s \leq j < 9s$ , then

$$b_{ij} = \begin{cases} w_{8(j+m+1)+3 \rightarrow 8(j+m+2)+1} \otimes w_{8j+7 \rightarrow 8(j+1)}, & i = (j+1)_s; \\ -2w_{8(j+m+2) \rightarrow 8(j+m+2)+1} \otimes w_{8j+7 \rightarrow 8(j+1)+1}, & i = 2s + (j+1)_s; \\ -w_{8(j+m+2) \rightarrow 8(j+m+2)+1} \otimes w_{8j+7 \rightarrow 8(j+1)+3}, & i = 4s + (j+1)_s; \\ w_{8(j+m+1)+7 \rightarrow 8(j+m+2)+1} \otimes w_{8j+7 \rightarrow 8(j+1)+6}, & i = 7s + (j+1)_s; \\ 0, & \text{otherwise.} \end{cases}$$

If  $9s \leq j < 10s$ , then  $b_{ij} = 0$ .

(25) If  $r_0 = 24$ , then  $\Omega^{24}(Z_t^{(9)})$  is described with  $(11s \times 11s)$  matrix, whose entries  $b_{ij}$  have the following form:

If  $0 \leq j < s$ , then

$$b_{ij} = \begin{cases} -2w_{8(j+m) \rightarrow 8(j+m)+7} \otimes e_{8j}, & i = j; \\ -w_{8(j+m)+4 \rightarrow 8(j+m)+7} \otimes w_{8j \rightarrow 8j+1}, & i = j + s; \\ -w_{8(j+m)+5 \rightarrow 8(j+m)+7} \otimes w_{8j \rightarrow 8j+1}, & i = j + 2s; \\ w_{8(j+m)+1 \rightarrow 8(j+m)+7} \otimes w_{8j \rightarrow 8j+3}, & i = j + 4s; \\ -w_{8(j+m)+2 \rightarrow 8(j+m)+7} \otimes w_{8j \rightarrow 8j+4}, & i = j + 5s; \\ -w_{8(j+m)+3 \rightarrow 8(j+m)+7} \otimes w_{8j \rightarrow 8j+5}, & i = j + 6s; \\ 0, & \text{otherwise.} \end{cases}$$

If  $s \leq j < 2s$ , then

$$b_{ij} = \begin{cases} -w_{8(j+m) \rightarrow 8(j+m+1)} \otimes e_{8j}, & i = j - s; \\ 2e_{8(j+m+1)} \otimes w_{8j \rightarrow 8(j+1)}, & i = (j+1)_s; \\ w_{8(j+m)+5 \rightarrow 8(j+m+1)} \otimes w_{8j \rightarrow 8j+1}, & i = j + s; \\ w_{8(j+m)+1 \rightarrow 8(j+m+1)} \otimes w_{8j \rightarrow 8j+3}, & i = j + 3s; \\ -w_{8(j+m)+2 \rightarrow 8(j+m+1)} \otimes w_{8j \rightarrow 8j+4}, & i = j + 4s; \\ 0, & \text{otherwise.} \end{cases}$$

If  $2s \leq j < 3s$ , then

$$b_{ij} = \begin{cases} -w_{8(j+m+1) \rightarrow 8(j+m+1)+3} \otimes w_{8j+1 \rightarrow 8(j+1)}, & i = (j+1)_s; \\ -w_{8(j+m)+4 \rightarrow 8(j+m+1)+3} \otimes e_{8j+1}, & i = j - s; \\ 0, & \text{otherwise.} \end{cases}$$

If  $3s \leq j < 4s$ , then

$$b_{ij} = \begin{cases} 2w_{8(j+m+1) \rightarrow 8(j+m+1)+4} \otimes w_{8j+2 \rightarrow 8(j+1)}, & i = (j+1)_s; \\ -w_{8(j+m+1) \rightarrow 8(j+m+1)+4} \otimes w_{8j+2 \rightarrow 8j+7}, & i = j + 6s; \\ 0, & \text{otherwise.} \end{cases}$$

If  $4s \leq j < 5s$ , then

$$b_{ij} = \begin{cases} -e_{8(j+m+1)+5} \otimes w_{8j+3 \rightarrow 8(j+1)+1}, & i = 2s + (j+1)_s; \\ 0, & \text{otherwise.} \end{cases}$$

If  $5s \leq j < 6s$ , then

$$b_{ij} = \begin{cases} w_{8(j+m+1)+5 \rightarrow 8(j+m+1)+6} \otimes w_{8j+4 \rightarrow 8(j+1)+1}, & i = 2s + (j+1)_s; \\ 0, & \text{otherwise.} \end{cases}$$

If  $6s \leq j < 7s$ , then

$$b_{ij} = \begin{cases} -w_{8(j+m+1) \rightarrow 8(j+m+1)+1} \otimes w_{8j+4 \rightarrow 8(j+1)}, & i = (j+1)_s; \\ 0, & \text{otherwise.} \end{cases}$$

If  $7s \leq j < 8s$ , then

$$b_{ij} = \begin{cases} w_{8(j+m)+3 \rightarrow 8(j+m+1)+1} \otimes e_{8j+5}, & i = j - s; \\ 0, & \text{otherwise.} \end{cases}$$

If  $8s \leq j < 9s$ , then

$$b_{ij} = \begin{cases} -w_{8(j+m)+4 \rightarrow 8(j+m+1)+2} \otimes e_{8j+6}, & i = j; \\ w_{8(j+m)+7 \rightarrow 8(j+m+1)+2} \otimes w_{8j+6 \rightarrow 8j+7}, & i = j + 2s; \\ 0, & \text{otherwise.} \end{cases}$$

If  $9s \leq j < 10s$ , then  $b_{ij} = 0$ .

If  $10s \leq j < 11s$ , then

$$b_{ij} = \begin{cases} -w_{8(j+m+1) \rightarrow 8(j+m+1)+7} \otimes w_{8j+7 \rightarrow 8(j+1)}, & i = (j+1)_s; \\ -w_{8(j+m+1)+4 \rightarrow 8(j+m+1)+7} \otimes w_{8j+7 \rightarrow 8(j+1)+1}, & i = s + (j+1)_s; \\ w_{8(j+m+1)+1 \rightarrow 8(j+m+1)+7} \otimes w_{8j+7 \rightarrow 8(j+1)+3}, & i = 4s + (j+1)_s; \\ -w_{8(j+m+1)+2 \rightarrow 8(j+m+1)+7} \otimes w_{8j+7 \rightarrow 8(j+1)+4}, & i = 5s + (j+1)_s; \\ -w_{8(j+m+1)+3 \rightarrow 8(j+m+1)+7} \otimes w_{8j+7 \rightarrow 8(j+1)+5}, & i = 6s + (j+1)_s; \\ 0, & \text{otherwise.} \end{cases}$$

(26) If  $r_0 = 25$ , then  $\Omega^{25}(Z_t^{(9)})$  is described with  $(10s \times 11s)$  matrix, whose entries  $b_{ij}$  have the following form:

If  $0 \leq j < s$ , then

$$b_{ij} = \begin{cases} -2w_{8(j+m)+7 \rightarrow 8(j+m+1)+5} \otimes w_{8j \rightarrow 8j+1}, & i = j + 2s; \\ -2w_{8(j+m+1) \rightarrow 8(j+m+1)+5} \otimes w_{8j \rightarrow 8j+2}, & i = j + 3s; \\ -2w_{8(j+m+1) \rightarrow 8(j+m+1)+5} \otimes w_{8j \rightarrow 8j+6}, & i = j + 7s; \\ 0, & \text{otherwise.} \end{cases}$$



If  $s \leq j < 2s$ , then

$$b_{ij} = \begin{cases} -2w_{8(j+m)+4 \rightarrow 8(j+m+1)+3} \otimes e_{8j}, & i = j - s; \\ -2w_{8(j+m)+7 \rightarrow 8(j+m+1)+3} \otimes w_{8j \rightarrow 8j+1}, & i = j + s; \\ -w_{8(j+m+1) \rightarrow 8(j+m+1)+3} \otimes w_{8j \rightarrow 8j+2}, & i = j + 2s; \\ -w_{8(j+m+1) \rightarrow 8(j+m+1)+3} \otimes w_{8j \rightarrow 8j+6}, & i = j + 6s; \\ 0, & \text{otherwise.} \end{cases}$$

If  $2s \leq j < 3s$ , then

$$b_{ij} = \begin{cases} w_{8(j+m)+4 \rightarrow 8(j+m+1)+1} \otimes e_{8j}, & i = j - 2s; \\ w_{8(j+m)+7 \rightarrow 8(j+m+1)+1} \otimes w_{8j \rightarrow 8j+1}, & i = j; \\ w_{8(j+m+1) \rightarrow 8(j+m+1)+1} \otimes w_{8j \rightarrow 8j+2}, & i = j + s; \\ w_{8(j+m+1) \rightarrow 8(j+m+1)+1} \otimes w_{8j \rightarrow 8j+6}, & i = j + 5s; \\ 0, & \text{otherwise.} \end{cases}$$

If  $3s \leq j < 4s$ , then

$$b_{ij} = \begin{cases} w_{8(j+m)+7 \rightarrow 8(j+m+1)+4} \otimes e_{8j+1}, & i = j - s; \\ w_{8(j+m+1) \rightarrow 8(j+m+1)+4} \otimes w_{8j+1 \rightarrow 8j+2}, & i = j; \\ 0, & \text{otherwise.} \end{cases}$$

If  $4s \leq j < 5s$ , then

$$b_{ij} = \begin{cases} -w_{8(j+m+1)+4 \rightarrow 8(j+m+1)+7} \otimes w_{8j+2 \rightarrow 8(j+1)}, & i = (j+1)_s; \\ -w_{8(j+m+1)+5 \rightarrow 8(j+m+1)+7} \otimes w_{8j+2 \rightarrow 8j+7}, & i = j + 5s; \\ 0, & \text{otherwise.} \end{cases}$$

If  $5s \leq j < 6s$ , then

$$b_{ij} = \begin{cases} w_{8(j+m+1)+6 \rightarrow 8(j+m+2)} \otimes w_{8j+3 \rightarrow 8(j+1)}, & i = s + (j+1)_s; \\ e_{8(j+m+2)} \otimes w_{8j+3 \rightarrow 8(j+1)+2}, & i = 3s + (j+1)_s; \\ 0, & \text{otherwise.} \end{cases}$$

If  $6s \leq j < 7s$ , then  $b_{ij} = 0$ .

If  $7s \leq j < 8s$ , then

$$b_{ij} = \begin{cases} w_{8(j+m+1)+4 \rightarrow 8(j+m+2)} \otimes w_{8j+5 \rightarrow 8(j+1)}, & i = (j+1)_s; \\ 0, & \text{otherwise.} \end{cases}$$

If  $8s \leq j < 9s$ , then

$$b_{ij} = \begin{cases} -w_{8(j+m+1) \rightarrow 8(j+m+1)+7} \otimes e_{8j+6}, & i = j - s; \\ -w_{8(j+m+1)+3 \rightarrow 8(j+m+1)+7} \otimes w_{8j+6 \rightarrow 8j+7}, & i = j; \\ 0, & \text{otherwise.} \end{cases}$$

If  $9s \leq j < 10s$ , then

$$b_{ij} = \begin{cases} w_{8(j+m+2) \rightarrow 8(j+m+2)+2} \otimes w_{8j+7 \rightarrow 8(j+1)+2}, & i = 3s + (j+1)_s; \\ w_{8(j+m+2) \rightarrow 8(j+m+2)+2} \otimes w_{8j+7 \rightarrow 8(j+1)+6}, & i = 7s + (j+1)_s; \\ 0, & \text{otherwise.} \end{cases}$$

If  $10s \leq j < 11s$ , then  $b_{ij} = 0$ .

(27) If  $r_0 = 26$ , then  $\Omega^{26}(Z_t^{(9)})$  is described with  $(8s \times 13s)$  matrix, whose entries  $b_{ij}$  have the following form:

If  $0 \leq j < s$ , then

$$b_{ij} = \begin{cases} 2w_{8(j+m-1)+7 \rightarrow 8(j+m)+7} \otimes e_{8j}, & i = j; \\ -e_{8(j+m)+7} \otimes w_{8j \rightarrow 8(j+1)}, & i = (j+1)_s; \\ -w_{8(j+m)+6 \rightarrow 8(j+m)+7} \otimes w_{8j \rightarrow 8j+1}, & i = j+s; \\ -2w_{8(j+m)+1 \rightarrow 8(j+m)+7} \otimes w_{8j \rightarrow 8j+2}, & i = j+2s; \\ 2w_{8(j+m)+2 \rightarrow 8(j+m)+7} \otimes w_{8j \rightarrow 8j+3}, & i = j+3s; \\ -2w_{8(j+m)+3 \rightarrow 8(j+m)+7} \otimes w_{8j \rightarrow 8j+4}, & i = j+4s; \\ 2w_{8(j+m)+4 \rightarrow 8(j+m)+7} \otimes w_{8j \rightarrow 8j+5}, & i = j+5s; \\ 0, & \text{otherwise.} \end{cases}$$

If  $s \leq j < 2s$ , then

$$b_{ij} = \begin{cases} 3w_{8(j+m)+7 \rightarrow 8(j+m+1)} \otimes w_{8j \rightarrow 8(j+1)}, & i = (j+1)_s; \\ -w_{8(j+m)+6 \rightarrow 8(j+m+1)} \otimes w_{8j \rightarrow 8j+1}, & i = j; \\ -w_{8(j+m)+1 \rightarrow 8(j+m+1)} \otimes w_{8j \rightarrow 8j+2}, & i = j+s; \\ w_{8(j+m)+2 \rightarrow 8(j+m+1)} \otimes w_{8j \rightarrow 8j+3}, & i = j+2s; \\ -w_{8(j+m)+3 \rightarrow 8(j+m+1)} \otimes w_{8j \rightarrow 8j+4}, & i = j+3s; \\ -w_{8(j+m)+4 \rightarrow 8(j+m+1)} \otimes w_{8j \rightarrow 8j+5}, & i = j+4s; \\ 0, & \text{otherwise.} \end{cases}$$

If  $2s \leq j < 3s$ , then

$$b_{ij} = \begin{cases} -2w_{8(j+m)+7 \rightarrow 8(j+m+1)+4} \otimes w_{8j+1 \rightarrow 8(j+1)}, & i = (j+1)_s; \\ 0, & \text{otherwise.} \end{cases}$$

If  $3s \leq j < 4s$ , then

$$b_{ij} = \begin{cases} -w_{8(j+m)+7 \rightarrow 8(j+m+1)+5} \otimes w_{8j+2 \rightarrow 8(j+1)}, & i = (j+1)_s; \\ -w_{8(j+m+1) \rightarrow 8(j+m+1)+5} \otimes w_{8j+2 \rightarrow 8j+7}, & i = j+4s; \\ 0, & \text{otherwise.} \end{cases}$$

If  $4s \leq j < 5s$ , then

$$b_{ij} = \begin{cases} w_{8(j+m)+7 \rightarrow 8(j+m+1)+6} \otimes w_{8j+3 \rightarrow 8(j+1)}, & i = (j+1)_s; \\ e_{8(j+m+1)+6} \otimes w_{8j+3 \rightarrow 8(j+1)+1}, & i = s + (j+1)_s; \\ 0, & \text{otherwise.} \end{cases}$$

If  $5s \leq j < 6s$ , then

$$b_{ij} = \begin{cases} w_{8(j+m)+7 \rightarrow 8(j+m+1)+1} \otimes w_{8j+3 \rightarrow 8(j+1)}, & i = (j+1)_s; \\ 0, & \text{otherwise.} \end{cases}$$

If  $6s \leq j < 7s$ , then

$$b_{ij} = \begin{cases} w_{8(j+m)+7 \rightarrow 8(j+m+1)+2} \otimes w_{8j+4 \rightarrow 8(j+1)}, & i = (j+1)_s; \\ 0, & \text{otherwise.} \end{cases}$$

If  $7s \leq j < 8s$ , then

$$b_{ij} = \begin{cases} w_{8(j+m)+4 \rightarrow 8(j+m+1)+2} \otimes e_{8j+5}, & i = j - 2s; \\ 0, & \text{otherwise.} \end{cases}$$

If  $8s \leq j < 9s$ , then  $b_{ij} = 0$ .

If  $9s \leq j < 10s$ , then

$$b_{ij} = \begin{cases} -w_{8(j+m+1) \rightarrow 8(j+m+1)+3} \otimes w_{8j+6 \rightarrow 8j+7}, & i = j - 2s; \\ 0, & \text{otherwise.} \end{cases}$$

If  $10s \leq j < 11s$ , then  $b_{ij} = 0$ .

If  $11s \leq j < 12s$ , then

$$b_{ij} = \begin{cases} w_{8(j+m)+7 \rightarrow 8(j+m+1)+7} \otimes w_{8j+7 \rightarrow 8(j+1)}, & i = (j+1)_s; \\ w_{8(j+m+1)+6 \rightarrow 8(j+m+1)+7} \otimes w_{8j+7 \rightarrow 8(j+1)+1}, & i = s + (j+1)_s; \\ w_{8(j+m+1)+1 \rightarrow 8(j+m+1)+7} \otimes w_{8j+7 \rightarrow 8(j+1)+2}, & i = 2s + (j+1)_s; \\ -w_{8(j+m+1)+2 \rightarrow 8(j+m+1)+7} \otimes w_{8j+7 \rightarrow 8(j+1)+3}, & i = 3s + (j+1)_s; \\ w_{8(j+m+1)+3 \rightarrow 8(j+m+1)+7} \otimes w_{8j+7 \rightarrow 8(j+1)+4}, & i = 4s + (j+1)_s; \\ w_{8(j+m+1)+4 \rightarrow 8(j+m+1)+7} \otimes w_{8j+7 \rightarrow 8(j+1)+5}, & i = 5s + (j+1)_s; \\ 0, & \text{otherwise.} \end{cases}$$

If  $12s \leq j < 13s$ , then  $b_{ij} = 0$ .

(28) If  $r_0 = 27$ , then  $\Omega^{27}(Z_t^{(9)})$  is described with  $(9s \times 14s)$  matrix, whose entries  $b_{ij}$  have the following form:

If  $0 \leq j < s$ , then

$$b_{ij} = \begin{cases} -w_{8(j+m+1) \rightarrow 8(j+m+1)+2} \otimes w_{8j \rightarrow 8j+1}, & i = j + s; \\ w_{8(j+m+1) \rightarrow 8(j+m+1)+2} \otimes w_{8j \rightarrow 8j+5}, & i = j + 5s; \\ 0, & \text{otherwise.} \end{cases}$$

If  $s \leq j < 2s$ , then

$$b_{ij} = \begin{cases} w_{8(j+m+1) \rightarrow 8(j+m+1)+4} \otimes w_{8j \rightarrow 8j+1}, & i = j; \\ -2w_{8(j+m+1) \rightarrow 8(j+m+1)+4} \otimes w_{8j \rightarrow 8j+5}, & i = j + 4s; \\ 0, & \text{otherwise.} \end{cases}$$

If  $2s \leq j < 3s$ , then

$$b_{ij} = \begin{cases} -w_{8(j+m+1) \rightarrow 8(j+m+1)+6} \otimes w_{8j \rightarrow 8j+1}, & i = j - s; \\ 0, & \text{otherwise.} \end{cases}$$

If  $3s \leq j < 4s$ , then

$$b_{ij} = \begin{cases} -w_{8(j+m+1) \rightarrow 8(j+m+1)+5} \otimes w_{8j \rightarrow 8j+1}, & i = j - 2s; \\ 0, & \text{otherwise.} \end{cases}$$

If  $4s \leq j < 5s$ , then

$$b_{ij} = \begin{cases} e_{8(j+m+1)+7} \otimes w_{8j+1 \rightarrow 8(j+1)}, & i = (j+1)_s; \\ -w_{8(j+m+1) \rightarrow 8(j+m+1)+7} \otimes e_{8j+1}, & i = j - 3s; \\ 0, & \text{otherwise.} \end{cases}$$

If  $5s \leq j < 6s$ , then

$$b_{ij} = \begin{cases} w_{8(j+m+1)+1 \rightarrow 8(j+m+2)} \otimes e_{8j+2}, & i = j - 3s; \\ 0, & \text{otherwise.} \end{cases}$$

If  $6s \leq j < 7s$ , then

$$b_{ij} = \begin{cases} e_{8(j+m+1)+7} \otimes w_{8j+3 \rightarrow 8(j+1)}, & i = (j+1)_s; \\ 0, & \text{otherwise.} \end{cases}$$

If  $7s \leq j < 8s$ , then  $b_{ij} = 0$ .

If  $8s \leq j < 9s$ , then

$$b_{ij} = \begin{cases} -2e_{8(j+m+1)+7} \otimes w_{8j+5 \rightarrow 8(j+1)}, & i = (j+1)_s; \\ w_{8(j+m+1) \rightarrow 8(j+m+1)+7} \otimes e_{8j+5}, & i = j - 3s; \\ 0, & \text{otherwise.} \end{cases}$$

If  $9s \leq j < 10s$ , then

$$b_{ij} = \begin{cases} -e_{8(j+m+1)+7} \otimes w_{8j+6 \rightarrow 8(j+1)}, & i = (j+1)_s; \\ w_{8(j+m+1)+5 \rightarrow 8(j+m+1)+7} \otimes e_{8j+6}, & i = j - 3s; \\ 0, & \text{otherwise.} \end{cases}$$

If  $10s \leq j < 11s$ , then  $b_{ij} = 0$ .

If  $11s \leq j < 12s$ , then

$$b_{ij} = \begin{cases} -w_{8(j+m+2) \rightarrow 8(j+m+2)+5} \otimes w_{8j+7 \rightarrow 8(j+1)+1}, & i = s + (j+1)_s; \\ 0, & \text{otherwise.} \end{cases}$$

If  $12s \leq j < 13s$ , then

$$b_{ij} = \begin{cases} -2w_{8(j+m+1)+7 \rightarrow 8(j+m+2)+3} \otimes w_{8j+7 \rightarrow 8(j+1)}, & i = (j+1)_s; \\ -w_{8(j+m+2) \rightarrow 8(j+m+2)+3} \otimes w_{8j+7 \rightarrow 8(j+1)+1}, & i = s + (j+1)_s; \\ 0, & \text{otherwise.} \end{cases}$$

If  $13s \leq j < 14s$ , then  $b_{ij} = 0$ .

(29) If  $r_0 = 28$ , then  $\Omega^{28}(Z_t^{(9)})$  is described with  $(8s \times 16s)$  matrix, whose entries  $b_{ij}$  have the following form:

If  $0 \leq j < s$ , then

$$b_{ij} = \begin{cases} -w_{8(j+m)+1 \rightarrow 8(j+m)+7} \otimes w_{8j \rightarrow 8j+1}, & i = j + s; \\ w_{8(j+m)+2 \rightarrow 8(j+m)+7} \otimes w_{8j \rightarrow 8j+2}, & i = j + 2s; \\ -w_{8(j+m)+3 \rightarrow 8(j+m)+7} \otimes w_{8j \rightarrow 8j+3}, & i = j + 3s; \\ w_{8(j+m)+4 \rightarrow 8(j+m)+7} \otimes w_{8j \rightarrow 8j+4}, & i = j + 4s; \\ 2w_{8(j+m)+5 \rightarrow 8(j+m)+7} \otimes w_{8j \rightarrow 8j+5}, & i = j + 5s; \\ -w_{8(j+m)+6 \rightarrow 8(j+m)+7} \otimes w_{8j \rightarrow 8j+6}, & i = j + 6s; \\ e_{8(j+m)+7} \otimes w_{8j \rightarrow 8j+7}, & i = j + 7s; \\ 0, & \text{otherwise.} \end{cases}$$

If  $s \leq j < 2s$ , then

$$b_{ij} = \begin{cases} w_{8(j+m)+1 \rightarrow 8(j+m)+7} \otimes w_{8j \rightarrow 8j+1}, & i = j; \\ -w_{8(j+m)+2 \rightarrow 8(j+m)+7} \otimes w_{8j \rightarrow 8j+2}, & i = j + s; \\ w_{8(j+m)+3 \rightarrow 8(j+m)+7} \otimes w_{8j \rightarrow 8j+3}, & i = j + 2s; \\ -w_{8(j+m)+4 \rightarrow 8(j+m)+7} \otimes w_{8j \rightarrow 8j+4}, & i = j + 3s; \\ -w_{8(j+m)+5 \rightarrow 8(j+m)+7} \otimes w_{8j \rightarrow 8j+5}, & i = j + 4s; \\ w_{8(j+m)+6 \rightarrow 8(j+m)+7} \otimes w_{8j \rightarrow 8j+6}, & i = j + 5s; \\ -e_{8(j+m)+7} \otimes w_{8j \rightarrow 8j+7}, & i = j + 6s; \\ 0, & \text{otherwise.} \end{cases}$$

If  $2s \leq j < 3s$ , then

$$b_{ij} = \begin{cases} -w_{8(j+m) \rightarrow 8(j+m+1)} \otimes e_{8j}, & i = j - 2s; \\ -w_{8(j+m)+2 \rightarrow 8(j+m+1)} \otimes w_{8j \rightarrow 8j+2}, & i = j; \\ w_{8(j+m)+3 \rightarrow 8(j+m+1)} \otimes w_{8j \rightarrow 8j+3}, & i = j + s; \\ -w_{8(j+m)+4 \rightarrow 8(j+m+1)} \otimes w_{8j \rightarrow 8j+4}, & i = j + 2s; \\ -w_{8(j+m)+5 \rightarrow 8(j+m+1)} \otimes w_{8j \rightarrow 8j+5}, & i = j + 3s; \\ w_{8(j+m)+6 \rightarrow 8(j+m+1)} \otimes w_{8j \rightarrow 8j+6}, & i = j + 4s; \\ -w_{8(j+m)+7 \rightarrow 8(j+m+1)} \otimes w_{8j \rightarrow 8j+7}, & i = j + 5s; \\ 0, & \text{otherwise.} \end{cases}$$

If  $3s \leq j < 4s$ , then

$$b_{ij} = \begin{cases} -w_{8(j+m+1) \rightarrow 8(j+m+1)+5} \otimes w_{8j+1 \rightarrow 8(j+1)}, & i = (j+1)_s; \\ 0, & \text{otherwise.} \end{cases}$$

If  $4s \leq j < 5s$ , then  $b_{ij} = 0$ .

If  $5s \leq j < 6s$ , then

$$b_{ij} = \begin{cases} -w_{8(j+m)+2 \rightarrow 8(j+m+1)+1} \otimes e_{8j+2}, & i = j - 3s; \\ w_{8(j+m)+3 \rightarrow 8(j+m+1)+1} \otimes w_{8j+2 \rightarrow 8j+3}, & i = j - 2s; \\ -w_{8(j+m)+4 \rightarrow 8(j+m+1)+1} \otimes w_{8j+2 \rightarrow 8j+4}, & i = j - s; \\ -w_{8(j+m)+7 \rightarrow 8(j+m+1)+1} \otimes w_{8j+2 \rightarrow 8j+7}, & i = j + 2s; \\ 0, & \text{otherwise.} \end{cases}$$

If  $6s \leq j < 7s$ , then

$$b_{ij} = \begin{cases} -w_{8(j+m+1) \rightarrow 8(j+m+1)+2} \otimes w_{8j+3 \rightarrow 8(j+1)}, & i = (j+1)_s; \\ 0, & \text{otherwise.} \end{cases}$$

If  $7s \leq j < 8s$ , then

$$b_{ij} = \begin{cases} 2w_{8(j+m+1) \rightarrow 8(j+m+1)+3} \otimes w_{8j+4 \rightarrow 8(j+1)}, & i = (j+1)_s; \\ 0, & \text{otherwise.} \end{cases}$$

If  $8s \leq j < 10s$ , then  $b_{ij} = 0$ .

If  $10s \leq j < 11s$ , then

$$b_{ij} = \begin{cases} -2w_{8(j+m+1) \rightarrow 8(j+m+1)+6} \otimes w_{8j+5 \rightarrow 8(j+1)}, & i = (j+1)_s; \\ 3w_{8(j+m+1)+5 \rightarrow 8(j+m+1)+6} \otimes w_{8j+5 \rightarrow 8(j+1)+5}, & i = 5s + (j+1)_s; \\ 0, & \text{otherwise.} \end{cases}$$

If  $11s \leq j < 12s$ , then

$$b_{ij} = \begin{cases} -w_{8(j+m)+6 \rightarrow 8(j+m+1)+5} \otimes e_{8j+6}, & i = j - 5s; \\ w_{8(j+m)+7 \rightarrow 8(j+m+1)+5} \otimes w_{8j+6 \rightarrow 8j+7}, & i = j - 4s; \\ 0, & \text{otherwise.} \end{cases}$$

If  $12s \leq j < 13s$ , then

$$b_{ij} = \begin{cases} -2w_{8(j+m+1) \rightarrow 8(j+m+1)+4} \otimes w_{8j+6 \rightarrow 8(j+1)}, & i = (j+1)_s; \\ 0, & \text{otherwise.} \end{cases}$$

If  $13s \leq j < 14s$ , then  $b_{ij} = 0$ .

If  $14s \leq j < 15s$ , then

$$b_{ij} = \begin{cases} 2w_{8(j+m+1) \rightarrow 8(j+m+1)+7} \otimes w_{8j+7 \rightarrow 8(j+1)}, & i = (j+1)_s; \\ w_{8(j+m)+7 \rightarrow 8(j+m+1)+7} \otimes e_{8j+7}, & i = j - 7s; \\ 0, & \text{otherwise.} \end{cases}$$

If  $15s \leq j < 16s$ , then

$$b_{ij} = \begin{cases} 2w_{8(j+m+1) \rightarrow 8(j+m+2)} \otimes w_{8j+7 \rightarrow 8(j+1)}, & i = (j+1)_s; \\ w_{8(j+m+1)+1 \rightarrow 8(j+m+2)} \otimes w_{8j+7 \rightarrow 8(j+1)+1}, & i = s + (j+1)_s; \\ 0, & \text{otherwise.} \end{cases}$$

(II) Represent an arbitrary  $t_0 \in \mathbb{N}$  in the form  $t_0 = 29\ell_0 + r_0$ , where  $0 \leq r_0 \leq 28$ . Then  $\Omega^{t_0}(Z_t^{(9)})$  is a  $\Omega^{r_0}(Z_t^{(9)})$ , whose left components twisted by  $\sigma^{\ell_0}$ , and coefficients multiplied by  $(-1)^{\ell_0}$ .

**Proposition 9** (Translates for the case 12). (I) Let  $r_0 \in \mathbb{N}$ ,  $r_0 < 29$ .  $r_0$ -translates of the elements  $Z_t^{(12)}$  are described by the following way.

(1) If  $r_0 = 0$ , then  $\Omega^0(Z_t^{(12)})$  is described with  $(8s \times 18s)$  matrix with the following nonzero entries:

$$\begin{aligned} b_{j,0} &= -w_{8(j+m) \rightarrow 8(j+m)+2} \otimes e_{8j}; \\ b_{j-s,s} &= w_{8(j+m) \rightarrow 8(j+m)+6} \otimes e_{8j}; \\ b_{j-4s,6s} &= w_{8(j+m)+2 \rightarrow 8(j+m+1)} \otimes e_{8j+2}. \end{aligned}$$

(2) If  $r_0 = 1$ , then  $\Omega^1(Z_t^{(12)})$  is described with  $(9s \times 19s)$  matrix with the following nonzero entries:

$$\begin{aligned}
b_{j-s,s} &= w_{8(j+m)+1 \rightarrow 8(j+m+1)} \otimes e_{8j}; \\
b_{j+s,s} &= w_{8(j+m)+2 \rightarrow 8(j+m+1)} \otimes w_{8j \rightarrow 8j+1}; \\
b_{j-s,3s} &= -w_{8(j+m)+2 \rightarrow 8(j+m+1)+2} \otimes e_{8j+1}; \\
b_{(j+1)s,3s+(-1)s} &= w_{8(j+m+1)+1 \rightarrow 8(j+m+1)+2} \otimes w_{8j+1 \rightarrow 8(j+1)}; \\
b_{2s+(j+1)s,3s+(-1)s} &= e_{8(j+m+1)+2} \otimes w_{8j+1 \rightarrow 8(j+1)+1}; \\
b_{(j+1)s,4s+(-1)s} &= -w_{8(j+m+1)+1 \rightarrow 8(j+m+1)+3} \otimes w_{8j+2 \rightarrow 8(j+1)}; \\
b_{2s+(j+1)s,4s+(-1)s} &= -w_{8(j+m+1)+2 \rightarrow 8(j+m+1)+3} \otimes w_{8j+2 \rightarrow 8(j+1)+1}; \\
b_{3s+(j+1)s,4s+(-1)s} &= -e_{8(j+m+1)+3} \otimes w_{8j+2 \rightarrow 8(j+1)+2}; \\
b_{(j+1)s,6s+(-1)s} &= w_{8(j+m+1)+1 \rightarrow 8(j+m+1)+4} \otimes w_{8j+3 \rightarrow 8(j+1)}; \\
b_{2s+(j+1)s,6s+(-1)s} &= w_{8(j+m+1)+2 \rightarrow 8(j+m+1)+4} \otimes w_{8j+3 \rightarrow 8(j+1)+1}; \\
b_{3s+(j+1)s,6s+(-1)s} &= w_{8(j+m+1)+3 \rightarrow 8(j+m+1)+4} \otimes w_{8j+3 \rightarrow 8(j+1)+2}; \\
b_{4s+(j+1)s,6s+(-1)s} &= e_{8(j+m+1)+4} \otimes w_{8j+3 \rightarrow 8(j+1)+3}; \\
b_{s+(j+1)s,7s+(-1)s} &= -w_{8(j+m+1)+5 \rightarrow 8(j+m+1)+6} \otimes w_{8j+3 \rightarrow 8(j+1)}; \\
b_{(j+1)s,10s+(-1)s} &= -w_{8(j+m+1)+1 \rightarrow 8(j+m+1)+2} \otimes w_{8j+5 \rightarrow 8(j+1)}; \\
b_{s+(j+1)s,11s+(-1)s} &= w_{8(j+m+1)+5 \rightarrow 8(j+m+1)+6} \otimes w_{8j+5 \rightarrow 8(j+1)}; \\
b_{6s+(j+1)s,11s+(-1)s} &= e_{8(j+m+1)+6} \otimes w_{8j+5 \rightarrow 8(j+1)+5}; \\
b_{(j+1)s,17s+(-1)s} &= w_{8(j+m+1)+1 \rightarrow 8(j+m+2)} \otimes w_{8j+7 \rightarrow 8(j+1)}; \\
b_{2s+(j+1)s,17s+(-1)s} &= w_{8(j+m+1)+2 \rightarrow 8(j+m+2)} \otimes w_{8j+7 \rightarrow 8(j+1)+1}; \\
b_{j-9s,17s+(-1)s} &= w_{8(j+m+1) \rightarrow 8(j+m+2)} \otimes e_{8j+7}; \\
b_{(j+1)s,18s+(-1)s} &= w_{8(j+m+1)+1 \rightarrow 8(j+m+2)} \otimes w_{8j+7 \rightarrow 8(j+1)}; \\
b_{2s+(j+1)s,18s+(-1)s} &= w_{8(j+m+1)+2 \rightarrow 8(j+m+2)} \otimes w_{8j+7 \rightarrow 8(j+1)+1}; \\
b_{j-10s,18s+(-1)s} &= w_{8(j+m+1) \rightarrow 8(j+m+2)} \otimes e_{8j+7}.
\end{aligned}$$

(3) If  $r_0 = 2$ , then  $\Omega^2(Z_t^{(12)})$  is described with  $(8s \times 18s)$  matrix with the following nonzero entries:

$$\begin{aligned}
b_{(j+1)s,6s+(-1)s} &= e_{8(j+m)+7} \otimes w_{8j+3 \rightarrow 8(j+1)}; \\
b_{(j+1)s,7s+(-1)s} &= w_{8(j+m)+7 \rightarrow 8(j+m+1)} \otimes w_{8j+3 \rightarrow 8(j+1)}; \\
b_{j-4s,7s+(-1)s} &= -w_{8(j+m)+4 \rightarrow 8(j+m+1)} \otimes e_{8j+3}; \\
b_{(j+1)s,9s+(-1)s} &= -e_{8(j+m)+7} \otimes w_{8j+5 \rightarrow 8(j+1)}; \\
b_{j-5s,10s+(-1)s} &= w_{8(j+m)+6 \rightarrow 8(j+m+1)} \otimes e_{8j+5}; \\
b_{j-6s,12s+(-1)s} &= -w_{8(j+m)+1 \rightarrow 8(j+m+1)} \otimes e_{8j+6}.
\end{aligned}$$

(4) If  $r_0 = 3$ , then  $\Omega^3(Z_t^{(12)})$  is described with  $(10s \times 20s)$  matrix with the following nonzero entries:

$$\begin{aligned}
b_{j-s,s+(-1)s} &= -w_{8(j+m)+2 \rightarrow 8(j+m+1)} \otimes e_{8j}; \\
b_{j+s,s+(-1)s} &= -w_{8(j+m)+3 \rightarrow 8(j+m+1)} \otimes w_{8j \rightarrow 8j+1}; \\
b_{j+2s,s+(-1)s} &= -w_{8(j+m)+4 \rightarrow 8(j+m+1)} \otimes w_{8j \rightarrow 8j+2}; \\
b_{j-s,2s+(-1)s} &= -w_{8(j+m)+6 \rightarrow 8(j+m+1)} \otimes e_{8j}; \\
b_{j+2s,2s+(-1)s} &= w_{8(j+m)+7 \rightarrow 8(j+m+1)} \otimes w_{8j \rightarrow 8j+3}; \\
b_{j-2s,5s+(-1)s} &= w_{8(j+m)+4 \rightarrow 8(j+m+1)+4} \otimes e_{8j+2};
\end{aligned}$$

$$\begin{aligned}
b_{j-4s,8s+(-1)_s} &= w_{8(j+m)+7 \rightarrow 8(j+m+1)+1} \otimes e_{8j+3}; \\
b_{j-5s,11s+(-1)_s} &= -w_{8(j+m)+7 \rightarrow 8(j+m+1)+6} \otimes e_{8j+5}; \\
b_{(j+1)_s,12s+(-1)_s} &= -w_{8(j+m+1)+2 \rightarrow 8(j+m+1)+3} \otimes w_{8j+5 \rightarrow 8(j+1)}.
\end{aligned}$$

(5) If  $r_0 = 4$ , then  $\Omega^4(Z_t^{(12)})$  is described with  $(11s \times 18s)$  matrix with the following nonzero entries:

$$\begin{aligned}
b_{j+2s,(-1)_s} &= e_{8(j+m)+3} \otimes w_{8j \rightarrow 8j+1}; \\
b_{j-s,s+(-1)_s} &= w_{8(j+m-1)+7 \rightarrow 8(j+m)+6} \otimes e_{8j}; \\
b_{s+(j+1)_s,7s+(-2)_s} &= -e_{8(j+m+1)} \otimes w_{8j+2 \rightarrow 8(j+1)}; \\
b_{(j+1)_s,8s+(-2)_s} &= -w_{8(j+m)+7 \rightarrow 8(j+m+1)} \otimes w_{8j+3 \rightarrow 8(j+1)}; \\
b_{j-3s,10s+(-1)_s} &= w_{8(j+m)+1 \rightarrow 8(j+m)+7} \otimes e_{8j+5}; \\
b_{j-2s,10s+(-1)_s} &= -w_{8(j+m)+2 \rightarrow 8(j+m)+7} \otimes w_{8j+5 \rightarrow 8j+6}; \\
b_{(j+1)_s,11s+(-2)_s} &= w_{8(j+m)+7 \rightarrow 8(j+m+1)} \otimes w_{8j+5 \rightarrow 8(j+1)}; \\
b_{s+(j+1)_s,11s+(-2)_s} &= e_{8(j+m+1)} \otimes w_{8j+5 \rightarrow 8(j+1)}; \\
b_{(j+1)_s,11s+(-1)_s} &= -w_{8(j+m)+7 \rightarrow 8(j+m+1)} \otimes w_{8j+5 \rightarrow 8(j+1)}; \\
b_{s+(j+1)_s,11s+(-1)_s} &= -e_{8(j+m+1)} \otimes w_{8j+5 \rightarrow 8(j+1)}; \\
b_{(j+1)_s,14s+(-2)_s} &= w_{8(j+m)+7 \rightarrow 8(j+m+1)+2} \otimes w_{8j+7 \rightarrow 8(j+1)}; \\
b_{s+(j+1)_s,14s+(-2)_s} &= w_{8(j+m+1) \rightarrow 8(j+m+1)+2} \otimes w_{8j+7 \rightarrow 8(j+1)}; \\
b_{6s+(j+1)_s,14s+(-2)_s} &= -w_{8(j+m+1)+1 \rightarrow 8(j+m+1)+2} \otimes w_{8j+7 \rightarrow 8(j+1)+4}; \\
b_{8s+(j+1)_s,14s+(-2)_s} &= e_{8(j+m+1)+2} \otimes w_{8j+7 \rightarrow 8(j+1)+6}.
\end{aligned}$$

(6) If  $r_0 = 5$ , then  $\Omega^5(Z_t^{(12)})$  is described with  $(11s \times 19s)$  matrix with the following nonzero entries:

$$\begin{aligned}
b_{j+s,(-1)_s} &= w_{8(j+m)+3 \rightarrow 8(j+m)+7} \otimes e_{8j}; \\
b_{j+2s,s+(-1)_s} &= w_{8(j+m)+4 \rightarrow 8(j+m+1)} \otimes w_{8j \rightarrow 8j+1}; \\
b_{j+3s,s+(-1)_s} &= w_{8(j+m)+7 \rightarrow 8(j+m+1)} \otimes w_{8j \rightarrow 8j+2}; \\
b_{j+4s,s+(-1)_s} &= e_{8(j+m+1)} \otimes w_{8j \rightarrow 8j+3}; \\
b_{3s+(j+1)_s,3s+(-2)_s} &= -e_{8(j+m+1)+4} \otimes w_{8j+1 \rightarrow 8(j+1)+1}; \\
b_{(j+1)_s,4s+(-2)_s} &= w_{8(j+m+1)+5 \rightarrow 8(j+m+1)+6} \otimes w_{8j+1 \rightarrow 8(j+1)}; \\
b_{(j+1)_s,5s+(-2)_s} &= -e_{8(j+m+1)+5} \otimes w_{8j+2 \rightarrow 8(j+1)}; \\
b_{2s+(j+1)_s,6s+(-2)_s} &= e_{8(j+m+1)+1} \otimes w_{8j+2 \rightarrow 8(j+1)}; \\
b_{2s+(j+1)_s,7s+(-2)_s} &= w_{8(j+m+1)+1 \rightarrow 8(j+m+1)+2} \otimes w_{8j+3 \rightarrow 8(j+1)}; \\
b_{j-3s,10s+(-1)_s} &= -w_{8(j+m+1) \rightarrow 8(j+m+1)+2} \otimes e_{8j+5}; \\
b_{s+(j+1)_s,11s+(-2)_s} &= w_{8(j+m+1)+3 \rightarrow 8(j+m+1)+4} \otimes w_{8j+5 \rightarrow 8(j+1)}; \\
b_{2s+(j+1)_s,11s+(-2)_s} &= w_{8(j+m+1)+1 \rightarrow 8(j+m+1)+4} \otimes w_{8j+5 \rightarrow 8(j+1)}; \\
b_{s+(j+1)_s,11s+(-1)_s} &= -w_{8(j+m+1)+3 \rightarrow 8(j+m+1)+4} \otimes w_{8j+5 \rightarrow 8(j+1)}; \\
b_{2s+(j+1)_s,11s+(-1)_s} &= -w_{8(j+m+1)+1 \rightarrow 8(j+m+1)+4} \otimes w_{8j+5 \rightarrow 8(j+1)}; \\
b_{(j+1)_s,12s+(-2)_s} &= e_{8(j+m+1)+5} \otimes w_{8j+5 \rightarrow 8(j+1)}; \\
b_{(j+1)_s,12s+(-1)_s} &= -e_{8(j+m+1)+5} \otimes w_{8j+5 \rightarrow 8(j+1)}; \\
b_{s+(j+1)_s,13s+(-2)_s} &= e_{8(j+m+1)+3} \otimes w_{8j+6 \rightarrow 8(j+1)}; \\
b_{2s+(j+1)_s,13s+(-2)_s} &= w_{8(j+m+1)+1 \rightarrow 8(j+m+1)+3} \otimes w_{8j+6 \rightarrow 8(j+1)}; \\
b_{s+(j+1)_s,16s+(-2)_s} &= w_{8(j+m+1)+3 \rightarrow 8(j+m+1)+7} \otimes w_{8j+7 \rightarrow 8(j+1)};
\end{aligned}$$



$$b_{2s+(j+1)s,16s+(-2)s} = w_{8(j+m+1)+1 \rightarrow 8(j+m+1)+7} \otimes w_{8j+7 \rightarrow 8(j+1)}.$$

(7) If  $r_0 = 6$ , then  $\Omega^6(Z_t^{(12)})$  is described with  $(13s \times 18s)$  matrix with the following nonzero entries:

$$\begin{aligned} b_{j+s,(-1)s} &= -w_{8(j+m) \rightarrow 8(j+m)+2} \otimes e_{8j}; \\ b_{j,s+(-1)s} &= -w_{8(j+m) \rightarrow 8(j+m)+4} \otimes e_{8j}; \\ b_{j+s,s+(-1)s} &= e_{8(j+m)+4} \otimes w_{8j \rightarrow 8j+1}; \\ b_{j+4s,s+(-1)s} &= w_{8(j+m)+1 \rightarrow 8(j+m)+4} \otimes w_{8j \rightarrow 8j+3}; \\ b_{j,3s+(-1)s} &= e_{8(j+m)+5} \otimes w_{8j \rightarrow 8j+2}; \\ b_{(j+1)s,4s+(-2)s} &= e_{8(j+m)+7} \otimes w_{8j+1 \rightarrow 8(j+1)}; \\ b_{(j+1)s,5s+(-2)s} &= w_{8(j+m)+7 \rightarrow 8(j+m+1)} \otimes w_{8j+1 \rightarrow 8(j+1)}; \\ b_{(j+1)s,6s+(-2)s} &= w_{8(j+m)+7 \rightarrow 8(j+m+1)} \otimes w_{8j+2 \rightarrow 8(j+1)}; \\ b_{(j+1)s,9s+(-1)s} &= w_{8(j+m)+7 \rightarrow 8(j+m+1)} \otimes w_{8j+5 \rightarrow 8(j+1)}; \\ b_{j-s,9s+(-1)s} &= w_{8(j+m)+5 \rightarrow 8(j+m+1)} \otimes e_{8j+5}; \\ b_{(j+1)s,10s+(-2)s} &= -e_{8(j+m)+7} \otimes w_{8j+5 \rightarrow 8(j+1)}; \\ b_{(j+1)s,10s+(-1)s} &= e_{8(j+m)+7} \otimes w_{8j+5 \rightarrow 8(j+1)}; \\ b_{(j+1)s,13s+(-2)s} &= -w_{8(j+m)+7 \rightarrow 8(j+m+1)+3} \otimes w_{8j+7 \rightarrow 8(j+1)}; \\ b_{5s+(j+1)s,13s+(-2)s} &= w_{8(j+m+1)+1 \rightarrow 8(j+m+1)+3} \otimes w_{8j+7 \rightarrow 8(j+1)+3}; \\ b_{6s+(j+1)s,13s+(-2)s} &= w_{8(j+m+1)+2 \rightarrow 8(j+m+1)+3} \otimes w_{8j+7 \rightarrow 8(j+1)+4}; \\ b_{9s+(j+1)s,13s+(-2)s} &= e_{8(j+m+1)+3} \otimes w_{8j+7 \rightarrow 8(j+1)+6}. \end{aligned}$$

(8) If  $r_0 = 7$ , then  $\Omega^7(Z_t^{(12)})$  is described with  $(14s \times 19s)$  matrix with the following nonzero entries:

$$\begin{aligned} b_{j+4s,(-1)s} &= -e_{8(j+m)+7} \otimes w_{8j \rightarrow 8j+1}; \\ b_{j+2s,s+(-1)s} &= w_{8(j+m)+5 \rightarrow 8(j+m+1)} \otimes e_{8j}; \\ b_{j+3s,s+(-1)s} &= -w_{8(j+m)+7 \rightarrow 8(j+m+1)} \otimes w_{8j \rightarrow 8j+1}; \\ b_{(j+1)s,5s+(-2)s} &= e_{8(j+m+1)+2} \otimes w_{8j+2 \rightarrow 8(j+1)}; \\ b_{2s+(j+1)s,6s+(-2)s} &= -e_{8(j+m+1)+6} \otimes w_{8j+2 \rightarrow 8(j+1)}; \\ b_{(j+1)s,7s+(-2)s} &= -w_{8(j+m+1)+2 \rightarrow 8(j+m+1)+3} \otimes w_{8j+3 \rightarrow 8(j+1)}; \\ b_{2s+(j+1)s,11s+(-2)s} &= -e_{8(j+m+1)+6} \otimes w_{8j+5 \rightarrow 8(j+1)}; \\ b_{2s+(j+1)s,11s+(-1)s} &= e_{8(j+m+1)+6} \otimes w_{8j+5 \rightarrow 8(j+1)}; \\ b_{j-4s,12s+(-1)s} &= -w_{8(j+m)+7 \rightarrow 8(j+m+1)+5} \otimes e_{8j+5}; \\ b_{(j+1)s,14s+(-2)s} &= -w_{8(j+m+1)+2 \rightarrow 8(j+m+1)+4} \otimes w_{8j+6 \rightarrow 8(j+1)}; \\ b_{s+(j+1)s,14s+(-2)s} &= e_{8(j+m+1)+4} \otimes w_{8j+6 \rightarrow 8(j+1)}; \\ b_{(j+1)s,16s+(-2)s} &= w_{8(j+m+1)+2 \rightarrow 8(j+m+1)+7} \otimes w_{8j+7 \rightarrow 8(j+1)}; \\ b_{s+(j+1)s,16s+(-2)s} &= -w_{8(j+m+1)+4 \rightarrow 8(j+m+1)+7} \otimes w_{8j+7 \rightarrow 8(j+1)}; \\ b_{(j+1)s,17s+(-2)s} &= -w_{8(j+m+1)+2 \rightarrow 8(j+m+2)} \otimes w_{8j+7 \rightarrow 8(j+1)}; \\ b_{s+(j+1)s,17s+(-2)s} &= w_{8(j+m+1)+4 \rightarrow 8(j+m+2)} \otimes w_{8j+7 \rightarrow 8(j+1)}. \end{aligned}$$

(9) If  $r_0 = 8$ , then  $\Omega^8(Z_t^{(12)})$  is described with  $(16s \times 16s)$  matrix with the following nonzero entries:

$$\begin{aligned} b_{j+2s,s+(-1)s} &= -w_{8(j+m)+5 \rightarrow 8(j+m)+6} \otimes w_{8j \rightarrow 8j+1}; \\ b_{j+3s,s+(-1)s} &= e_{8(j+m)+6} \otimes w_{8j \rightarrow 8j+2}; \end{aligned}$$

$$\begin{aligned}
b_{j-2s,3s+(-1)_s} &= -w_{8(j+m-1)+7 \rightarrow 8(j+m)+5} \otimes e_{8j}; \\
b_{(j+1)_s,4s+(-2)_s} &= w_{8(j+m)+7 \rightarrow 8(j+m+1)} \otimes w_{8j+1 \rightarrow 8(j+1)}; \\
b_{2s+(j+1)_s,4s+(-2)_s} &= e_{8(j+m+1)} \otimes w_{8j+1 \rightarrow 8(j+1)}; \\
b_{(j+1)_s,5s+(-2)_s} &= e_{8(j+m)+7} \otimes w_{8j+2 \rightarrow 8(j+1)}; \\
b_{s+(j+1)_s,5s+(-2)_s} &= -e_{8(j+m)+7} \otimes w_{8j+2 \rightarrow 8(j+1)}; \\
b_{s+(j+1)_s,6s+(-2)_s} &= -w_{8(j+m)+7 \rightarrow 8(j+m+1)} \otimes w_{8j+3 \rightarrow 8(j+1)}; \\
b_{(j+1)_s,8s+(-2)_s} &= e_{8(j+m)+7} \otimes w_{8j+5 \rightarrow 8(j+1)}; \\
b_{s+(j+1)_s,8s+(-2)_s} &= -e_{8(j+m)+7} \otimes w_{8j+5 \rightarrow 8(j+1)}; \\
b_{j+2s,8s+(-1)_s} &= w_{8(j+m)+6 \rightarrow 8(j+m)+7} \otimes e_{8j+5}; \\
b_{2s+(j+1)_s,9s+(-2)_s} &= -e_{8(j+m+1)} \otimes w_{8j+5 \rightarrow 8(j+1)}; \\
b_{2s+(j+1)_s,9s+(-1)_s} &= e_{8(j+m+1)} \otimes w_{8j+5 \rightarrow 8(j+1)}; \\
b_{(j+1)_s,13s+(-2)_s} &= -w_{8(j+m)+7 \rightarrow 8(j+m+1)+4} \otimes w_{8j+7 \rightarrow 8(j+1)}; \\
b_{s+(j+1)_s,13s+(-2)_s} &= w_{8(j+m)+7 \rightarrow 8(j+m+1)+4} \otimes w_{8j+7 \rightarrow 8(j+1)}; \\
b_{6s+(j+1)_s,13s+(-2)_s} &= -w_{8(j+m+1)+2 \rightarrow 8(j+m+1)+4} \otimes w_{8j+7 \rightarrow 8(j+1)+3}; \\
b_{7s+(j+1)_s,13s+(-2)_s} &= w_{8(j+m+1)+3 \rightarrow 8(j+m+1)+4} \otimes w_{8j+7 \rightarrow 8(j+1)+4}; \\
b_{12s+(j+1)_s,13s+(-2)_s} &= e_{8(j+m+1)+4} \otimes w_{8j+7 \rightarrow 8(j+1)+6}.
\end{aligned}$$

(10) If  $r_0 = 9$ , then  $\Omega^9(Z_t^{(12)})$  is described with  $(16s \times 16s)$  matrix with the following nonzero entries:

$$\begin{aligned}
b_{j+2s,(-1)_s} &= w_{8(j+m)+6 \rightarrow 8(j+m)+7} \otimes e_{8j}; \\
b_{j+s,(-1)_s} &= -w_{8(j+m)+6 \rightarrow 8(j+m+1)} \otimes e_{8j}; \\
b_{j+3s,(-1)_s} &= -e_{8(j+m+1)} \otimes w_{8j \rightarrow 8j+1}; \\
b_{3s+(j+1)_s,2s+(-2)_s} &= w_{8(j+m+1)+1 \rightarrow 8(j+m+1)+2} \otimes w_{8j+1 \rightarrow 8(j+1)}; \\
b_{(j+1)_s,3s+(-2)_s} &= -w_{8(j+m+1)+5 \rightarrow 8(j+m+1)+6} \otimes w_{8j+1 \rightarrow 8(j+1)}; \\
b_{s+(j+1)_s,4s+(-2)_s} &= e_{8(j+m+1)+3} \otimes w_{8j+2 \rightarrow 8(j+1)}; \\
b_{s+(j+1)_s,5s+(-2)_s} &= -w_{8(j+m+1)+3 \rightarrow 8(j+m+1)+4} \otimes w_{8j+3 \rightarrow 8(j+1)}; \\
b_{(j+1)_s,8s+(-2)_s} &= w_{8(j+m+1)+5 \rightarrow 8(j+m+1)+6} \otimes w_{8j+5 \rightarrow 8(j+1)}; \\
b_{(j+1)_s,8s+(-1)_s} &= -w_{8(j+m+1)+5 \rightarrow 8(j+m+1)+6} \otimes w_{8j+5 \rightarrow 8(j+1)}; \\
b_{j,8s+(-1)_s} &= -w_{8(j+m)+7 \rightarrow 8(j+m+1)+6} \otimes e_{8j+5}; \\
b_{3s+(j+1)_s,10s+(-2)_s} &= e_{8(j+m+1)+1} \otimes w_{8j+5 \rightarrow 8(j+1)}; \\
b_{3s+(j+1)_s,10s+(-1)_s} &= -e_{8(j+m+1)+1} \otimes w_{8j+5 \rightarrow 8(j+1)}; \\
b_{s+(j+1)_s,13s+(-2)_s} &= w_{8(j+m+1)+3 \rightarrow 8(j+m+1)+7} \otimes w_{8j+7 \rightarrow 8(j+1)}; \\
b_{2s+(j+1)_s,13s+(-2)_s} &= -w_{8(j+m+1)+6 \rightarrow 8(j+m+1)+7} \otimes w_{8j+7 \rightarrow 8(j+1)}; \\
b_{8s+(j+1)_s,13s+(-2)_s} &= e_{8(j+m+1)+7} \otimes w_{8j+7 \rightarrow 8(j+1)+5}; \\
b_{s+(j+1)_s,14s+(-2)_s} &= w_{8(j+m+1)+3 \rightarrow 8(j+m+2)} \otimes w_{8j+7 \rightarrow 8(j+1)}; \\
b_{2s+(j+1)_s,14s+(-2)_s} &= -w_{8(j+m+1)+6 \rightarrow 8(j+m+2)} \otimes w_{8j+7 \rightarrow 8(j+1)}; \\
b_{8s+(j+1)_s,14s+(-2)_s} &= w_{8(j+m+1)+7 \rightarrow 8(j+m+2)} \otimes w_{8j+7 \rightarrow 8(j+1)+5}.
\end{aligned}$$

(11) If  $r_0 = 10$ , then  $\Omega^{10}(Z_t^{(12)})$  is described with  $(19s \times 14s)$  matrix with the following nonzero entries:

$$\begin{aligned}
b_{j+4s,(-1)_s} &= w_{8(j+m)+1 \rightarrow 8(j+m)+2} \otimes w_{8j \rightarrow 8j+1}; \\
b_{j+3s,(-1)_s} &= -w_{8(j+m)+1 \rightarrow 8(j+m)+4} \otimes w_{8j \rightarrow 8j+1};
\end{aligned}$$

$$\begin{aligned}
b_{j,2s+(-1)_s} &= w_{8(j+m) \rightarrow 8(j+m)+6} \otimes e_{8j}; \\
b_{j+8s,2s+(-1)_s} &= -w_{8(j+m)+5 \rightarrow 8(j+m)+6} \otimes w_{8j \rightarrow 8j+5}; \\
b_{(j+1)_s,3s+(-2)_s} &= -e_{8(j+m)+7} \otimes w_{8j+1 \rightarrow 8(j+1)}; \\
b_{s+(j+1)_s,4s+(-2)_s} &= e_{8(j+m+1)} \otimes w_{8j+2 \rightarrow 8(j+1)}; \\
b_{2s+(j+1)_s,4s+(-2)_s} &= -e_{8(j+m+1)} \otimes w_{8j+2 \rightarrow 8(j+1)}; \\
b_{(j+1)_s,7s+(-2)_s} &= -e_{8(j+m)+7} \otimes w_{8j+5 \rightarrow 8(j+1)}; \\
b_{j+3s,7s+(-1)_s} &= w_{8(j+m)+5 \rightarrow 8(j+m)+7} \otimes e_{8j+5}; \\
b_{j+5s,7s+(-1)_s} &= -w_{8(j+m)+1 \rightarrow 8(j+m)+7} \otimes e_{8j+5}; \\
b_{s+(j+1)_s,8s+(-2)_s} &= e_{8(j+m+1)} \otimes w_{8j+5 \rightarrow 8(j+1)}; \\
b_{2s+(j+1)_s,8s+(-2)_s} &= -e_{8(j+m+1)} \otimes w_{8j+5 \rightarrow 8(j+1)}; \\
b_{2s+(j+1)_s,13s+(-2)_s} &= -w_{8(j+m+1) \rightarrow 8(j+m+1)+5} \otimes w_{8j+7 \rightarrow 8(j+1)}; \\
b_{10s+(j+1)_s,13s+(-2)_s} &= e_{8(j+m+1)+5} \otimes w_{8j+7 \rightarrow 8(j+1)+5}.
\end{aligned}$$

(12) If  $r_0 = 11$ , then  $\Omega^{11}(Z_t^{(12)})$  is described with  $(18s \times 13s)$  matrix with the following nonzero entries:

$$\begin{aligned}
b_{j+2s,s+(-1)_s} &= w_{8(j+m)+1 \rightarrow 8(j+m)+7} \otimes e_{8j}; \\
b_{(j+1)_s,2s+(-2)_s} &= -w_{8(j+m+1)+2 \rightarrow 8(j+m+1)+3} \otimes w_{8j+1 \rightarrow 8(j+1)}; \\
b_{3s+(j+1)_s,2s+(-2)_s} &= w_{8(j+m+1)+1 \rightarrow 8(j+m+1)+3} \otimes w_{8j+1 \rightarrow 8(j+1)}; \\
b_{2s+(j+1)_s,3s+(-2)_s} &= e_{8(j+m+1)+4} \otimes w_{8j+2 \rightarrow 8(j+1)}; \\
b_{3s+(j+1)_s,3s+(-2)_s} &= -w_{8(j+m+1)+1 \rightarrow 8(j+m+1)+4} \otimes w_{8j+2 \rightarrow 8(j+1)}; \\
b_{4s+(j+1)_s,4s+(-2)_s} &= e_{8(j+m+1)+5} \otimes w_{8j+2 \rightarrow 8(j+1)}; \\
b_{(j+1)_s,7s+(-2)_s} &= e_{8(j+m+1)+2} \otimes w_{8j+5 \rightarrow 8(j+1)}; \\
b_{3s+(j+1)_s,7s+(-2)_s} &= -w_{8(j+m+1)+1 \rightarrow 8(j+m+1)+2} \otimes w_{8j+5 \rightarrow 8(j+1)}; \\
b_{4s+(j+1)_s,8s+(-2)_s} &= e_{8(j+m+1)+5} \otimes w_{8j+5 \rightarrow 8(j+1)}; \\
b_{2s+(j+1)_s,12s+(-2)_s} &= w_{8(j+m+1)+4 \rightarrow 8(j+m+2)} \otimes w_{8j+7 \rightarrow 8(j+1)}; \\
b_{3s+(j+1)_s,12s+(-2)_s} &= -w_{8(j+m+1)+1 \rightarrow 8(j+m+2)} \otimes w_{8j+7 \rightarrow 8(j+1)}; \\
b_{4s+(j+1)_s,12s+(-2)_s} &= -w_{8(j+m+1)+5 \rightarrow 8(j+m+2)} \otimes w_{8j+7 \rightarrow 8(j+1)}; \\
b_{7s+(j+1)_s,12s+(-2)_s} &= -w_{8(j+m+1)+7 \rightarrow 8(j+m+2)} \otimes w_{8j+7 \rightarrow 8(j+1)+3}; \\
b_{8s+(j+1)_s,12s+(-2)_s} &= w_{8(j+m+1)+7 \rightarrow 8(j+m+2)} \otimes w_{8j+7 \rightarrow 8(j+1)+4}; \\
b_{11s+(j+1)_s,12s+(-2)_s} &= e_{8(j+m+2)} \otimes w_{8j+7 \rightarrow 8(j+1)+5}.
\end{aligned}$$

(13) If  $r_0 = 12$ , then  $\Omega^{12}(Z_t^{(12)})$  is described with  $(19s \times 11s)$  matrix with the following nonzero entries:

$$\begin{aligned}
b_{s+(j+1)_s,2s+(-2)_s} &= -e_{8(j+m+1)} \otimes w_{8j+1 \rightarrow 8(j+1)}; \\
b_{2s+(j+1)_s,3s+(-2)_s} &= e_{8(j+m)+7} \otimes w_{8j+2 \rightarrow 8(j+1)}; \\
b_{2s+(j+1)_s,4s+(-2)_s} &= w_{8(j+m)+7 \rightarrow 8(j+m+1)} \otimes w_{8j+3 \rightarrow 8(j+1)}; \\
b_{2s+(j+1)_s,5s+(-2)_s} &= w_{8(j+m)+7 \rightarrow 8(j+m+1)+1} \otimes w_{8j+4 \rightarrow 8(j+1)}; \\
b_{s+(j+1)_s,6s+(-2)_s} &= -e_{8(j+m+1)} \otimes w_{8j+5 \rightarrow 8(j+1)}; \\
b_{2s+(j+1)_s,8s+(-2)_s} &= -w_{8(j+m)+7 \rightarrow 8(j+m+1)+2} \otimes w_{8j+7 \rightarrow 8(j+1)}; \\
b_{10s+(j+1)_s,8s+(-2)_s} &= -e_{8(j+m+1)+2} \otimes w_{8j+7 \rightarrow 8(j+1)+5}; \\
b_{2s+(j+1)_s,9s+(-2)_s} &= w_{8(j+m)+7 \rightarrow 8(j+m+1)+4} \otimes w_{8j+7 \rightarrow 8(j+1)}; \\
b_{10s+(j+1)_s,9s+(-2)_s} &= w_{8(j+m+1)+2 \rightarrow 8(j+m+1)+4} \otimes w_{8j+7 \rightarrow 8(j+1)+5};
\end{aligned}$$

$$\begin{aligned}
b_{s+(j+1)s,10s+(-2)s} &= w_{8(j+m+1) \rightarrow 8(j+m+1)+6} \otimes w_{8j+7 \rightarrow 8(j+1)}; \\
b_{2s+(j+1)s,10s+(-2)s} &= -w_{8(j+m)+7 \rightarrow 8(j+m+1)+6} \otimes w_{8j+7 \rightarrow 8(j+1)}; \\
b_{5s+(j+1)s,10s+(-2)s} &= w_{8(j+m+1)+5 \rightarrow 8(j+m+1)+6} \otimes w_{8j+7 \rightarrow 8(j+1)+2}; \\
b_{8s+(j+1)s,10s+(-2)s} &= w_{8(j+m+1)+5 \rightarrow 8(j+m+1)+6} \otimes w_{8j+7 \rightarrow 8(j+1)+4}; \\
b_{11s+(j+1)s,10s+(-2)s} &= -e_{8(j+m+1)+6} \otimes w_{8j+7 \rightarrow 8(j+1)+5}.
\end{aligned}$$

(14) If  $r_0 = 13$ , then  $\Omega^{13}(Z_t^{(12)})$  is described with  $(18s \times 11s)$  matrix with the following nonzero entries:

$$\begin{aligned}
b_{(j+1)s,s+(-2)s} &= w_{8(j+m+1)+2 \rightarrow 8(j+m+1)+4} \otimes w_{8j+1 \rightarrow 8(j+1)}; \\
b_{s+(j+1)s,s+(-2)s} &= -w_{8(j+m+1)+3 \rightarrow 8(j+m+1)+4} \otimes w_{8j+1 \rightarrow 8(j+1)}; \\
b_{3s+(j+1)s,2s+(-2)s} &= -e_{8(j+m+1)+5} \otimes w_{8j+1 \rightarrow 8(j+1)}; \\
b_{2s+(j+1)s,3s+(-2)s} &= e_{8(j+m+1)+6} \otimes w_{8j+2 \rightarrow 8(j+1)}; \\
b_{3s+(j+1)s,3s+(-2)s} &= -w_{8(j+m+1)+5 \rightarrow 8(j+m+1)+6} \otimes w_{8j+2 \rightarrow 8(j+1)}; \\
b_{(j+1)s,6s+(-2)s} &= -w_{8(j+m+1)+2 \rightarrow 8(j+m+1)+3} \otimes w_{8j+5 \rightarrow 8(j+1)}; \\
b_{s+(j+1)s,6s+(-2)s} &= e_{8(j+m+1)+3} \otimes w_{8j+5 \rightarrow 8(j+1)}; \\
b_{2s+(j+1)s,7s+(-2)s} &= e_{8(j+m+1)+6} \otimes w_{8j+5 \rightarrow 8(j+1)}; \\
b_{3s+(j+1)s,10s+(-2)s} &= w_{8(j+m+1)+5 \rightarrow 8(j+m+1)+7} \otimes w_{8j+7 \rightarrow 8(j+1)}; \\
b_{9s+(j+1)s,10s+(-2)s} &= e_{8(j+m+1)+7} \otimes w_{8j+7 \rightarrow 8(j+1)+5}.
\end{aligned}$$

(15) If  $r_0 = 14$ , then  $\Omega^{14}(Z_t^{(12)})$  is described with  $(20s \times 10s)$  matrix with the following nonzero entries:

$$\begin{aligned}
b_{(j+1)s,2s+(-2)s} &= e_{8(j+m)+7} \otimes w_{8j+1 \rightarrow 8(j+1)}; \\
b_{2s+(j+1)s,3s+(-2)s} &= e_{8(j+m+1)} \otimes w_{8j+2 \rightarrow 8(j+1)}; \\
b_{(j+1)s,6s+(-2)s} &= e_{8(j+m)+7} \otimes w_{8j+5 \rightarrow 8(j+1)}; \\
b_{12s+(j+1)s,8s+(-2)s} &= -e_{8(j+m+1)+3} \otimes w_{8j+7 \rightarrow 8(j+1)+5}.
\end{aligned}$$

(16) If  $r_0 = 15$ , then  $\Omega^{15}(Z_t^{(12)})$  is described with  $(18s \times 8s)$  matrix with the following nonzero entries:

$$\begin{aligned}
b_{s+(j+1)s,s+(-2)s} &= e_{8(j+m+1)+6} \otimes w_{8j+1 \rightarrow 8(j+1)}; \\
b_{3s+(j+1)s,2s+(-2)s} &= -e_{8(j+m+1)+1} \otimes w_{8j+2 \rightarrow 8(j+1)}; \\
b_{(j+1)s,5s+(-2)s} &= -w_{8(j+m+1)+3 \rightarrow 8(j+m+1)+4} \otimes w_{8j+5 \rightarrow 8(j+1)}; \\
b_{2s+(j+1)s,5s+(-2)s} &= e_{8(j+m+1)+4} \otimes w_{8j+5 \rightarrow 8(j+1)}; \\
b_{11s+(j+1)s,7s+(-2)s} &= -e_{8(j+m+2)} \otimes w_{8j+7 \rightarrow 8(j+1)+5}.
\end{aligned}$$

(17) If  $r_0 = 16$ , then  $\Omega^{16}(Z_t^{(12)})$  is described with  $(19s \times 9s)$  matrix with the following nonzero entries:

$$\begin{aligned}
b_{(j+1)s,(-2)s} &= -e_{8(j+m)+7} \otimes w_{8j \rightarrow 8(j+1)}; \\
b_{2s+(j+1)s,(-2)s} &= e_{8(j+m)+7} \otimes w_{8j \rightarrow 8(j+1)}; \\
b_{(j+1)s,s+(-2)s} &= -w_{8(j+m)+7 \rightarrow 8(j+m+1)} \otimes w_{8j+1 \rightarrow 8(j+1)}; \\
b_{s+(j+1)s,s+(-2)s} &= e_{8(j+m+1)} \otimes w_{8j+1 \rightarrow 8(j+1)}; \\
b_{2s+(j+1)s,s+(-2)s} &= w_{8(j+m)+7 \rightarrow 8(j+m+1)} \otimes w_{8j+1 \rightarrow 8(j+1)}; \\
b_{j+4s,2s+(-2)s} &= -w_{8(j+m)+1 \rightarrow 8(j+m+1)+1} \otimes e_{8j+2}; \\
b_{s+(j+1)s,5s+(-2)s} &= e_{8(j+m+1)} \otimes w_{8j+5 \rightarrow 8(j+1)}; \\
b_{12s+(j+1)s,6s+(-2)s} &= -e_{8(j+m+1)+5} \otimes w_{8j+6 \rightarrow 8(j+1)+5};
\end{aligned}$$

$$b_{11s+(j+1)s,7s+(-2)s} = -e_{8(j+m+1)+4} \otimes w_{8j+7 \rightarrow 8(j+1)+5};$$

$$b_{12s+(j+1)s,8s+(-2)s} = w_{8(j+m+1)+5 \rightarrow 8(j+m+1)+6} \otimes w_{8j+7 \rightarrow 8(j+1)+5}.$$

(18) If  $r_0 = 17$ , then  $\Omega^{17}(Z_t^{(12)})$  is described with  $(18s \times 8s)$  matrix with the following nonzero entries:

$$b_{j+4s,s+(-2)s} = w_{8(j+m+1) \rightarrow 8(j+m+1)+1} \otimes e_{8j+1};$$

$$b_{3s+(j+1)s,5s+(-2)s} = e_{8(j+m+1)+5} \otimes w_{8j+5 \rightarrow 8(j+1)};$$

$$b_{10s+(j+1)s,7s+(-2)s} = -e_{8(j+m+1)+7} \otimes w_{8j+7 \rightarrow 8(j+1)+5}.$$

(19) If  $r_0 = 18$ , then  $\Omega^{18}(Z_t^{(12)})$  is described with  $(19s \times 8s)$  matrix with the following nonzero entries:

$$b_{j+3s,(-2)s} = -w_{8(j+m)+5 \rightarrow 8(j+m+1)} \otimes w_{8j \rightarrow 8j+1};$$

$$b_{2s+(j+1)s,s+(-3)s} = -w_{8(j+m+1) \rightarrow 8(j+m+1)+1} \otimes w_{8j+1 \rightarrow 8(j+1)};$$

$$b_{(j+1)s,2s+(-3)s} = -w_{8(j+m)+7 \rightarrow 8(j+m+1)+2} \otimes w_{8j+2 \rightarrow 8(j+1)};$$

$$b_{s+(j+1)s,2s+(-3)s} = -w_{8(j+m+1) \rightarrow 8(j+m+1)+2} \otimes w_{8j+2 \rightarrow 8(j+1)};$$

$$b_{j+3s,2s+(-3)s} = -w_{8(j+m)+2 \rightarrow 8(j+m+1)+2} \otimes e_{8j+2};$$

$$b_{2s+(j+1)s,3s+(-3)s} = -w_{8(j+m+1) \rightarrow 8(j+m+1)+3} \otimes w_{8j+3 \rightarrow 8(j+1)};$$

$$b_{5s+(j+1)s,3s+(-3)s} = -w_{8(j+m+1)+2 \rightarrow 8(j+m+1)+3} \otimes w_{8j+3 \rightarrow 8(j+1)+2};$$

$$b_{2s+(j+1)s,4s+(-3)s} = -w_{8(j+m+1) \rightarrow 8(j+m+1)+4} \otimes w_{8j+4 \rightarrow 8(j+1)};$$

$$b_{5s+(j+1)s,4s+(-3)s} = -w_{8(j+m+1)+2 \rightarrow 8(j+m+1)+4} \otimes w_{8j+4 \rightarrow 8(j+1)+2};$$

$$b_{(j+1)s,5s+(-2)s} = -w_{8(j+m)+7 \rightarrow 8(j+m+1)+5} \otimes w_{8j+5 \rightarrow 8(j+1)};$$

$$b_{2s+(j+1)s,5s+(-2)s} = w_{8(j+m+1) \rightarrow 8(j+m+1)+5} \otimes w_{8j+5 \rightarrow 8(j+1)};$$

$$b_{11s+(j+1)s,6s+(-2)s} = e_{8(j+m+1)+6} \otimes w_{8j+6 \rightarrow 8(j+1)+5};$$

$$b_{11s+(j+1)s,7s+(-2)s} = w_{8(j+m+1)+6 \rightarrow 8(j+m+1)+7} \otimes w_{8j+7 \rightarrow 8(j+1)+5};$$

$$b_{4s+(j+1)s,7s+(-3)s} = -w_{8(j+m+1)+1 \rightarrow 8(j+m+1)+7} \otimes w_{8j+7 \rightarrow 8(j+1)+1};$$

$$b_{5s+(j+1)s,7s+(-3)s} = -w_{8(j+m+1)+2 \rightarrow 8(j+m+1)+7} \otimes w_{8j+7 \rightarrow 8(j+1)+2}.$$

(20) If  $r_0 = 19$ , then  $\Omega^{19}(Z_t^{(12)})$  is described with  $(16s \times 9s)$  matrix with the following nonzero entries:

$$b_{2s+(j+1)s,(-3)s} = e_{8(j+m+1)+1} \otimes w_{8j \rightarrow 8(j+1)};$$

$$b_{3s+(j+1)s,s+(-2)s} = -e_{8(j+m+1)+5} \otimes w_{8j \rightarrow 8(j+1)};$$

$$b_{j+3s,s+(-2)s} = -w_{8(j+m+1) \rightarrow 8(j+m+1)+5} \otimes w_{8j \rightarrow 8j+1};$$

$$b_{j+2s,2s+(-3)s} = -w_{8(j+m+1) \rightarrow 8(j+m+1)+2} \otimes e_{8j+1};$$

$$b_{(j+1)s,3s+(-3)s} = -e_{8(j+m+1)+3} \otimes w_{8j+2 \rightarrow 8(j+1)};$$

$$b_{2s+(j+1)s,3s+(-3)s} = w_{8(j+m+1)+1 \rightarrow 8(j+m+1)+3} \otimes w_{8j+2 \rightarrow 8(j+1)};$$

$$b_{2s+(j+1)s,5s+(-3)s} = -w_{8(j+m+1)+1 \rightarrow 8(j+m+1)+7} \otimes w_{8j+4 \rightarrow 8(j+1)};$$

$$b_{s+(j+1)s,6s+(-2)s} = -e_{8(j+m+1)+6} \otimes w_{8j+5 \rightarrow 8(j+1)};$$

$$b_{9s+(j+1)s,8s+(-2)s} = e_{8(j+m+2)} \otimes w_{8j+7 \rightarrow 8(j+1)+5};$$

$$b_{4s+(j+1)s,8s+(-3)s} = e_{8(j+m+2)} \otimes w_{8j+7 \rightarrow 8(j+1)+1}.$$

(21) If  $r_0 = 20$ , then  $\Omega^{20}(Z_t^{(12)})$  is described with  $(16s \times 8s)$  matrix with the following nonzero entries:

$$b_{(j+1)s,(-3)s} = -e_{8(j+m)+7} \otimes w_{8j \rightarrow 8(j+1)};$$

$$b_{j+3s,(-3)s} = -w_{8(j+m)+6 \rightarrow 8(j+m)+7} \otimes w_{8j \rightarrow 8j+1};$$

$$\begin{aligned}
b_{j+3s,(-2)_s} &= w_{8(j+m)+6 \rightarrow 8(j+m)+7} \otimes w_{8j \rightarrow 8j+1}; \\
b_{(j+1)_s, s+(-4)_s} &= -w_{8(j+m)+7 \rightarrow 8(j+m+1)+2} \otimes w_{8j+1 \rightarrow 8(j+1)}; \\
b_{s+(j+1)_s, s+(-4)_s} &= w_{8(j+m+1) \rightarrow 8(j+m+1)+2} \otimes w_{8j+1 \rightarrow 8(j+1)}; \\
b_{s+(j+1)_s, s+(-3)_s} &= -w_{8(j+m+1) \rightarrow 8(j+m+1)+2} \otimes w_{8j+1 \rightarrow 8(j+1)}; \\
b_{s+(j+1)_s, 2s+(-4)_s} &= w_{8(j+m+1) \rightarrow 8(j+m+1)+3} \otimes w_{8j+2 \rightarrow 8(j+1)}; \\
b_{j+2s, 2s+(-4)_s} &= w_{8(j+m)+3 \rightarrow 8(j+m+1)+3} \otimes e_{8j+2}; \\
b_{s+(j+1)_s, 2s+(-3)_s} &= -w_{8(j+m+1) \rightarrow 8(j+m+1)+3} \otimes w_{8j+2 \rightarrow 8(j+1)}; \\
b_{(j+1)_s, 3s+(-4)_s} &= -w_{8(j+m)+7 \rightarrow 8(j+m+1)+4} \otimes w_{8j+3 \rightarrow 8(j+1)}; \\
b_{s+(j+1)_s, 3s+(-4)_s} &= w_{8(j+m+1) \rightarrow 8(j+m+1)+4} \otimes w_{8j+3 \rightarrow 8(j+1)}; \\
b_{4s+(j+1)_s, 3s+(-4)_s} &= w_{8(j+m+1)+3 \rightarrow 8(j+m+1)+4} \otimes w_{8j+3 \rightarrow 8(j+1)+2}; \\
b_{(j+1)_s, 3s+(-3)_s} &= w_{8(j+m)+7 \rightarrow 8(j+m+1)+4} \otimes w_{8j+3 \rightarrow 8(j+1)}; \\
b_{s+(j+1)_s, 3s+(-3)_s} &= -w_{8(j+m+1) \rightarrow 8(j+m+1)+4} \otimes w_{8j+3 \rightarrow 8(j+1)}; \\
b_{4s+(j+1)_s, 3s+(-3)_s} &= -w_{8(j+m+1)+3 \rightarrow 8(j+m+1)+4} \otimes w_{8j+3 \rightarrow 8(j+1)+2}; \\
b_{(j+1)_s, 5s+(-2)_s} &= w_{8(j+m)+7 \rightarrow 8(j+m+1)+6} \otimes w_{8j+5 \rightarrow 8(j+1)}; \\
b_{s+(j+1)_s, 5s+(-2)_s} &= -w_{8(j+m+1) \rightarrow 8(j+m+1)+6} \otimes w_{8j+5 \rightarrow 8(j+1)}; \\
b_{10s+(j+1)_s, 6s+(-2)_s} &= e_{8(j+m+1)+1} \otimes w_{8j+6 \rightarrow 8(j+1)+5}; \\
b_{3s+(j+1)_s, 7s+(-4)_s} &= -w_{8(j+m+1)+6 \rightarrow 8(j+m+2)} \otimes w_{8j+7 \rightarrow 8(j+1)+1}; \\
b_{3s+(j+1)_s, 7s+(-3)_s} &= w_{8(j+m+1)+6 \rightarrow 8(j+m+2)} \otimes w_{8j+7 \rightarrow 8(j+1)+1}; \\
b_{7s+(j+1)_s, 7s+(-2)_s} &= w_{8(j+m+1)+6 \rightarrow 8(j+m+2)} \otimes w_{8j+7 \rightarrow 8(j+1)+4}; \\
b_{8s+(j+1)_s, 7s+(-2)_s} &= w_{8(j+m+1)+6 \rightarrow 8(j+m+2)} \otimes w_{8j+7 \rightarrow 8(j+1)+5}.
\end{aligned}$$

(22) If  $r_0 = 21$ , then  $\Omega^{21}(Z_t^{(12)})$  is described with  $(14s \times 10s)$  matrix with the following nonzero entries:

$$\begin{aligned}
b_{(j+1)_s, (-4)_s} &= e_{8(j+m+1)+2} \otimes w_{8j \rightarrow 8(j+1)}; \\
b_{(j+1)_s, (-3)_s} &= -e_{8(j+m+1)+2} \otimes w_{8j \rightarrow 8(j+1)}; \\
b_{j+2s, s+(-3)_s} &= w_{8(j+m)+7 \rightarrow 8(j+m+1)+6} \otimes w_{8j \rightarrow 8j+1}; \\
b_{2s+(j+1)_s, s+(-2)_s} &= -e_{8(j+m+1)+6} \otimes w_{8j \rightarrow 8(j+1)}; \\
b_{j+2s, s+(-2)_s} &= -w_{8(j+m)+7 \rightarrow 8(j+m+1)+6} \otimes w_{8j \rightarrow 8j+1}; \\
b_{j+2s, 2s+(-4)_s} &= w_{8(j+m)+7 \rightarrow 8(j+m+1)+3} \otimes e_{8j+1}; \\
b_{(j+1)_s, 3s+(-4)_s} &= w_{8(j+m+1)+2 \rightarrow 8(j+m+1)+4} \otimes w_{8j+2 \rightarrow 8(j+1)}; \\
b_{s+(j+1)_s, 3s+(-4)_s} &= e_{8(j+m+1)+4} \otimes w_{8j+2 \rightarrow 8(j+1)}; \\
b_{(j+1)_s, 3s+(-3)_s} &= -w_{8(j+m+1)+2 \rightarrow 8(j+m+1)+4} \otimes w_{8j+2 \rightarrow 8(j+1)}; \\
b_{s+(j+1)_s, 3s+(-3)_s} &= -e_{8(j+m+1)+4} \otimes w_{8j+2 \rightarrow 8(j+1)}; \\
b_{(j+1)_s, 4s+(-4)_s} &= -w_{8(j+m+1)+2 \rightarrow 8(j+m+1)+7} \otimes w_{8j+3 \rightarrow 8(j+1)}; \\
b_{3s+(j+1)_s, 4s+(-4)_s} &= -e_{8(j+m+1)+7} \otimes w_{8j+3 \rightarrow 8(j+1)+1}; \\
b_{(j+1)_s, 4s+(-3)_s} &= w_{8(j+m+1)+2 \rightarrow 8(j+m+1)+7} \otimes w_{8j+3 \rightarrow 8(j+1)}; \\
b_{3s+(j+1)_s, 4s+(-3)_s} &= e_{8(j+m+1)+7} \otimes w_{8j+3 \rightarrow 8(j+1)+1}; \\
b_{6s+(j+1)_s, 5s+(-2)_s} &= -e_{8(j+m+2)} \otimes w_{8j+4 \rightarrow 8(j+1)+4}; \\
b_{(j+1)_s, 6s+(-2)_s} &= w_{8(j+m+1)+2 \rightarrow 8(j+m+1)+7} \otimes w_{8j+5 \rightarrow 8(j+1)}; \\
b_{(j+1)_s, 7s+(-2)_s} &= -w_{8(j+m+1)+2 \rightarrow 8(j+m+2)} \otimes w_{8j+6 \rightarrow 8(j+1)}; \\
b_{2s+(j+1)_s, 7s+(-2)_s} &= -w_{8(j+m+1)+6 \rightarrow 8(j+m+2)} \otimes w_{8j+6 \rightarrow 8(j+1)};
\end{aligned}$$

$$\begin{aligned}
b_{9s+(j+1)s,7s+(-2)s} &= -e_{8(j+m+2)} \otimes w_{8j+6 \rightarrow 8(j+1)+6}; \\
b_{3s+(j+1)s,9s+(-4)s} &= w_{8(j+m+1)+7 \rightarrow 8(j+m+2)+5} \otimes w_{8j+7 \rightarrow 8(j+1)+1}; \\
b_{3s+(j+1)s,9s+(-3)s} &= -w_{8(j+m+1)+7 \rightarrow 8(j+m+2)+5} \otimes w_{8j+7 \rightarrow 8(j+1)+1}; \\
b_{2s+(j+1)s,9s+(-2)s} &= w_{8(j+m+1)+6 \rightarrow 8(j+m+2)+5} \otimes w_{8j+7 \rightarrow 8(j+1)}; \\
b_{3s+(j+1)s,9s+(-2)s} &= w_{8(j+m+1)+7 \rightarrow 8(j+m+2)+5} \otimes w_{8j+7 \rightarrow 8(j+1)+1}; \\
b_{4s+(j+1)s,9s+(-2)s} &= w_{8(j+m+2) \rightarrow 8(j+m+2)+5} \otimes w_{8j+7 \rightarrow 8(j+1)+2}; \\
b_{5s+(j+1)s,9s+(-2)s} &= w_{8(j+m+1)+7 \rightarrow 8(j+m+2)+5} \otimes w_{8j+7 \rightarrow 8(j+1)+3}; \\
b_{6s+(j+1)s,9s+(-2)s} &= w_{8(j+m+2) \rightarrow 8(j+m+2)+5} \otimes w_{8j+7 \rightarrow 8(j+1)+4}; \\
b_{9s+(j+1)s,9s+(-2)s} &= w_{8(j+m+2) \rightarrow 8(j+m+2)+5} \otimes w_{8j+7 \rightarrow 8(j+1)+6}.
\end{aligned}$$

(23) If  $r_0 = 22$ , then  $\Omega^{22}(Z_t^{(12)})$  is described with  $(13s \times 11s)$  matrix with the following nonzero entries:

$$\begin{aligned}
b_{j+2s,(-4)s} &= w_{8(j+m)+3 \rightarrow 8(j+m)+7} \otimes w_{8j \rightarrow 8j+1}; \\
b_{j+3s,(-4)s} &= -w_{8(j+m)+4 \rightarrow 8(j+m)+7} \otimes w_{8j \rightarrow 8j+2}; \\
b_{j+2s,(-3)s} &= -w_{8(j+m)+3 \rightarrow 8(j+m)+7} \otimes w_{8j \rightarrow 8j+1}; \\
b_{j+3s,(-3)s} &= w_{8(j+m)+4 \rightarrow 8(j+m)+7} \otimes w_{8j \rightarrow 8j+2}; \\
b_{s+(j+1)s,(-2)s} &= -e_{8(j+m)+7} \otimes w_{8j \rightarrow 8(j+1)}; \\
b_{j+2s,(-2)s} &= w_{8(j+m)+3 \rightarrow 8(j+m)+7} \otimes w_{8j \rightarrow 8j+1}; \\
b_{j+3s,(-2)s} &= -w_{8(j+m)+4 \rightarrow 8(j+m)+7} \otimes w_{8j \rightarrow 8j+2}; \\
b_{s+(j+1)s,2s+(-4)s} &= w_{8(j+m)+7 \rightarrow 8(j+m+1)+3} \otimes w_{8j+1 \rightarrow 8(j+1)}; \\
b_{s+(j+1)s,2s+(-3)s} &= -w_{8(j+m)+7 \rightarrow 8(j+m+1)+3} \otimes w_{8j+1 \rightarrow 8(j+1)}; \\
b_{(j+1)s,2s+(-5)s} &= w_{8(j+m+1) \rightarrow 8(j+m+1)+3} \otimes w_{8j+1 \rightarrow 8(j+1)}; \\
b_{s+(j+1)s,2s+(-5)s} &= -w_{8(j+m)+7 \rightarrow 8(j+m+1)+3} \otimes w_{8j+1 \rightarrow 8(j+1)}; \\
b_{s+(j+1)s,3s+(-4)s} &= w_{8(j+m)+7 \rightarrow 8(j+m+1)+4} \otimes w_{8j+2 \rightarrow 8(j+1)}; \\
b_{s+(j+1)s,3s+(-3)s} &= -w_{8(j+m)+7 \rightarrow 8(j+m+1)+4} \otimes w_{8j+2 \rightarrow 8(j+1)}; \\
b_{s+(j+1)s,3s+(-5)s} &= -w_{8(j+m)+7 \rightarrow 8(j+m+1)+4} \otimes w_{8j+2 \rightarrow 8(j+1)}; \\
b_{j,3s+(-5)s} &= -w_{8(j+m)+4 \rightarrow 8(j+m+1)+4} \otimes e_{8j+2}; \\
b_{(j+1)s,4s+(-2)s} &= w_{8(j+m+1) \rightarrow 8(j+m+1)+5} \otimes w_{8j+3 \rightarrow 8(j+1)}; \\
b_{s+(j+1)s,4s+(-2)s} &= -w_{8(j+m)+7 \rightarrow 8(j+m+1)+5} \otimes w_{8j+3 \rightarrow 8(j+1)}; \\
b_{(j+1)s,5s+(-2)s} &= w_{8(j+m+1) \rightarrow 8(j+m+1)+6} \otimes w_{8j+4 \rightarrow 8(j+1)}; \\
b_{s+(j+1)s,5s+(-2)s} &= -w_{8(j+m)+7 \rightarrow 8(j+m+1)+6} \otimes w_{8j+4 \rightarrow 8(j+1)}; \\
b_{6s+(j+1)s,6s+(-2)s} &= -e_{8(j+m+1)+1} \otimes w_{8j+4 \rightarrow 8(j+1)+4}; \\
b_{(j+1)s,8s+(-2)s} &= -w_{8(j+m+1) \rightarrow 8(j+m+1)+2} \otimes w_{8j+6 \rightarrow 8(j+1)}; \\
b_{s+(j+1)s,8s+(-2)s} &= w_{8(j+m)+7 \rightarrow 8(j+m+1)+2} \otimes w_{8j+6 \rightarrow 8(j+1)}; \\
b_{7s+(j+1)s,8s+(-2)s} &= -e_{8(j+m+1)+2} \otimes w_{8j+6 \rightarrow 8(j+1)+5}; \\
b_{2s+(j+1)s,10s+(-4)s} &= -w_{8(j+m+1)+3 \rightarrow 8(j+m+1)+7} \otimes w_{8j+7 \rightarrow 8(j+1)+1}; \\
b_{3s+(j+1)s,10s+(-4)s} &= w_{8(j+m+1)+4 \rightarrow 8(j+m+1)+7} \otimes w_{8j+7 \rightarrow 8(j+1)+2}; \\
b_{2s+(j+1)s,10s+(-3)s} &= w_{8(j+m+1)+3 \rightarrow 8(j+m+1)+7} \otimes w_{8j+7 \rightarrow 8(j+1)+1}; \\
b_{3s+(j+1)s,10s+(-3)s} &= -w_{8(j+m+1)+4 \rightarrow 8(j+m+1)+7} \otimes w_{8j+7 \rightarrow 8(j+1)+2}; \\
b_{(j+1)s,10s+(-2)s} &= -w_{8(j+m+1) \rightarrow 8(j+m+1)+7} \otimes w_{8j+7 \rightarrow 8(j+1)}; \\
b_{s+(j+1)s,10s+(-2)s} &= w_{8(j+m)+7 \rightarrow 8(j+m+1)+7} \otimes w_{8j+7 \rightarrow 8(j+1)};
\end{aligned}$$

$$\begin{aligned}
b_{6s+(j+1)s,10s+(-2)s} &= -w_{8(j+m+1)+1 \rightarrow 8(j+m+1)+7} \otimes w_{8j+7 \rightarrow 8(j+1)+4}; \\
b_{7s+(j+1)s,10s+(-2)s} &= -w_{8(j+m+1)+2 \rightarrow 8(j+m+1)+7} \otimes w_{8j+7 \rightarrow 8(j+1)+5}; \\
b_{2s+(j+1)s,10s+(-5)s} &= w_{8(j+m+1)+3 \rightarrow 8(j+m+1)+7} \otimes w_{8j+7 \rightarrow 8(j+1)+1}; \\
b_{3s+(j+1)s,10s+(-5)s} &= -w_{8(j+m+1)+4 \rightarrow 8(j+m+1)+7} \otimes w_{8j+7 \rightarrow 8(j+1)+2}.
\end{aligned}$$

(24) If  $r_0 = 23$ , then  $\Omega^{23}(Z_t^{(12)})$  is described with  $(11s \times 11s)$  matrix with the following nonzero entries:

$$\begin{aligned}
b_{s+(j+1)s,(-2)s} &= -e_{8(j+m+1)+5} \otimes w_{8j \rightarrow 8(j+1)}; \\
b_{(j+1)s,s+(-4)s} &= e_{8(j+m+1)+3} \otimes w_{8j \rightarrow 8(j+1)}; \\
b_{j+s,s+(-4)s} &= w_{8(j+m+1) \rightarrow 8(j+m+1)+3} \otimes w_{8j \rightarrow 8j+1}; \\
b_{(j+1)s,s+(-3)s} &= -e_{8(j+m+1)+3} \otimes w_{8j \rightarrow 8(j+1)}; \\
b_{j+s,s+(-3)s} &= -w_{8(j+m+1) \rightarrow 8(j+m+1)+3} \otimes w_{8j \rightarrow 8j+1}; \\
b_{j+s,s+(-2)s} &= w_{8(j+m+1) \rightarrow 8(j+m+1)+3} \otimes w_{8j \rightarrow 8j+1}; \\
b_{(j+1)s,s+(-5)s} &= -e_{8(j+m+1)+3} \otimes w_{8j \rightarrow 8(j+1)}; \\
b_{j-s,3s+(-5)s} &= -w_{8(j+m+1) \rightarrow 8(j+m+1)+4} \otimes e_{8j+1}; \\
b_{(j+1)s,4s+(-4)s} &= -w_{8(j+m+1)+3 \rightarrow 8(j+m+1)+7} \otimes w_{8j+2 \rightarrow 8(j+1)}; \\
b_{s+(j+1)s,4s+(-4)s} &= w_{8(j+m+1)+5 \rightarrow 8(j+m+1)+7} \otimes w_{8j+2 \rightarrow 8(j+1)}; \\
b_{3s+(j+1)s,4s+(-4)s} &= -e_{8(j+m+1)+7} \otimes w_{8j+2 \rightarrow 8(j+1)+2}; \\
b_{(j+1)s,4s+(-3)s} &= w_{8(j+m+1)+3 \rightarrow 8(j+m+1)+7} \otimes w_{8j+2 \rightarrow 8(j+1)}; \\
b_{s+(j+1)s,4s+(-3)s} &= -w_{8(j+m+1)+5 \rightarrow 8(j+m+1)+7} \otimes w_{8j+2 \rightarrow 8(j+1)}; \\
b_{3s+(j+1)s,4s+(-3)s} &= e_{8(j+m+1)+7} \otimes w_{8j+2 \rightarrow 8(j+1)+2}; \\
b_{(j+1)s,4s+(-5)s} &= w_{8(j+m+1)+3 \rightarrow 8(j+m+1)+7} \otimes w_{8j+2 \rightarrow 8(j+1)}; \\
b_{s+(j+1)s,4s+(-5)s} &= -w_{8(j+m+1)+5 \rightarrow 8(j+m+1)+7} \otimes w_{8j+2 \rightarrow 8(j+1)}; \\
b_{3s+(j+1)s,4s+(-5)s} &= e_{8(j+m+1)+7} \otimes w_{8j+2 \rightarrow 8(j+1)+2}; \\
b_{(j+1)s,7s+(-2)s} &= w_{8(j+m+1)+3 \rightarrow 8(j+m+2)} \otimes w_{8j+5 \rightarrow 8(j+1)}; \\
b_{(j+1)s,9s+(-2)s} &= -w_{8(j+m+1)+3 \rightarrow 8(j+m+2)+2} \otimes w_{8j+7 \rightarrow 8(j+1)}; \\
b_{2s+(j+1)s,9s+(-2)s} &= -w_{8(j+m+2) \rightarrow 8(j+m+2)+2} \otimes w_{8j+7 \rightarrow 8(j+1)+1}; \\
b_{3s+(j+1)s,9s+(-2)s} &= -w_{8(j+m+1)+7 \rightarrow 8(j+m+2)+2} \otimes w_{8j+7 \rightarrow 8(j+1)+2}; \\
b_{7s+(j+1)s,9s+(-2)s} &= -w_{8(j+m+1)+7 \rightarrow 8(j+m+2)+2} \otimes w_{8j+7 \rightarrow 8(j+1)+6}.
\end{aligned}$$

(25) If  $r_0 = 24$ , then  $\Omega^{24}(Z_t^{(12)})$  is described with  $(11s \times 13s)$  matrix with the following nonzero entries:

$$\begin{aligned}
b_{j+2s,(-4)s} &= -w_{8(j+m)+5 \rightarrow 8(j+m)+7} \otimes w_{8j \rightarrow 8j+1}; \\
b_{j+2s,(-3)s} &= w_{8(j+m)+5 \rightarrow 8(j+m)+7} \otimes w_{8j \rightarrow 8j+1}; \\
b_{j+2s,(-2)s} &= -w_{8(j+m)+5 \rightarrow 8(j+m)+7} \otimes w_{8j \rightarrow 8j+1}; \\
b_{j+2s,(-5)s} &= w_{8(j+m)+5 \rightarrow 8(j+m)+7} \otimes w_{8j \rightarrow 8j+1}; \\
b_{j+s,s+(-4)s} &= w_{8(j+m)+5 \rightarrow 8(j+m+1)} \otimes w_{8j \rightarrow 8j+1}; \\
b_{j+s,s+(-3)s} &= -w_{8(j+m)+5 \rightarrow 8(j+m+1)} \otimes w_{8j \rightarrow 8j+1}; \\
b_{(j+1)s,s+(-2)s} &= e_{8(j+m+1)} \otimes w_{8j \rightarrow 8(j+1)}; \\
b_{j+s,s+(-2)s} &= w_{8(j+m)+5 \rightarrow 8(j+m+1)} \otimes w_{8j \rightarrow 8j+1}; \\
b_{j+s,s+(-5)s} &= -w_{8(j+m)+5 \rightarrow 8(j+m+1)} \otimes w_{8j \rightarrow 8j+1}; \\
b_{(j+1)s,2s+(-4)s} &= -w_{8(j+m+1) \rightarrow 8(j+m+1)+4} \otimes w_{8j+1 \rightarrow 8(j+1)};
\end{aligned}$$



$$\begin{aligned}
b_{(j+1)s, 2s+(-3)_s} &= w_{8(j+m+1) \rightarrow 8(j+m+1)+4} \otimes w_{8j+1 \rightarrow 8(j+1)}; \\
b_{(j+1)s, 2s+(-6)_s} &= -w_{8(j+m+1) \rightarrow 8(j+m+1)+4} \otimes w_{8j+1 \rightarrow 8(j+1)}; \\
b_{(j+1)s, 2s+(-5)_s} &= w_{8(j+m+1) \rightarrow 8(j+m+1)+4} \otimes w_{8j+1 \rightarrow 8(j+1)}; \\
b_{(j+1)s, 3s+(-4)_s} &= -w_{8(j+m+1) \rightarrow 8(j+m+1)+5} \otimes w_{8j+2 \rightarrow 8(j+1)}; \\
b_{2s+(j+1)s, 3s+(-4)_s} &= e_{8(j+m+1)+5} \otimes w_{8j+2 \rightarrow 8(j+1)+1}; \\
b_{(j+1)s, 3s+(-3)_s} &= w_{8(j+m+1) \rightarrow 8(j+m+1)+5} \otimes w_{8j+2 \rightarrow 8(j+1)}; \\
b_{2s+(j+1)s, 3s+(-3)_s} &= -e_{8(j+m+1)+5} \otimes w_{8j+2 \rightarrow 8(j+1)+1}; \\
b_{(j+1)s, 3s+(-5)_s} &= w_{8(j+m+1) \rightarrow 8(j+m+1)+5} \otimes w_{8j+2 \rightarrow 8(j+1)}; \\
b_{2s+(j+1)s, 3s+(-5)_s} &= -e_{8(j+m+1)+5} \otimes w_{8j+2 \rightarrow 8(j+1)+1}; \\
b_{(j+1)s, 6s+(-2)_s} &= w_{8(j+m+1) \rightarrow 8(j+m+1)+2} \otimes w_{8j+4 \rightarrow 8(j+1)}; \\
b_{4s+(j+1)s, 6s+(-2)_s} &= -w_{8(j+m+1)+1 \rightarrow 8(j+m+1)+2} \otimes w_{8j+4 \rightarrow 8(j+1)+3}; \\
b_{5s+(j+1)s, 6s+(-2)_s} &= e_{8(j+m+1)+2} \otimes w_{8j+4 \rightarrow 8(j+1)+4}; \\
b_{(j+1)s, 9s+(-2)_s} &= -w_{8(j+m+1) \rightarrow 8(j+m+1)+3} \otimes w_{8j+6 \rightarrow 8(j+1)}; \\
b_{6s+(j+1)s, 9s+(-2)_s} &= -e_{8(j+m+1)+3} \otimes w_{8j+6 \rightarrow 8(j+1)+5}; \\
b_{2s+(j+1)s, 11s+(-4)_s} &= -w_{8(j+m+1)+5 \rightarrow 8(j+m+1)+7} \otimes w_{8j+7 \rightarrow 8(j+1)+1}; \\
b_{2s+(j+1)s, 11s+(-3)_s} &= w_{8(j+m+1)+5 \rightarrow 8(j+m+1)+7} \otimes w_{8j+7 \rightarrow 8(j+1)+1}; \\
b_{(j+1)s, 11s+(-2)_s} &= -w_{8(j+m+1) \rightarrow 8(j+m+1)+7} \otimes w_{8j+7 \rightarrow 8(j+1)}; \\
b_{4s+(j+1)s, 11s+(-2)_s} &= w_{8(j+m+1)+1 \rightarrow 8(j+m+1)+7} \otimes w_{8j+7 \rightarrow 8(j+1)+3}; \\
b_{5s+(j+1)s, 11s+(-2)_s} &= -w_{8(j+m+1)+2 \rightarrow 8(j+m+1)+7} \otimes w_{8j+7 \rightarrow 8(j+1)+4}; \\
b_{6s+(j+1)s, 11s+(-2)_s} &= -w_{8(j+m+1)+3 \rightarrow 8(j+m+1)+7} \otimes w_{8j+7 \rightarrow 8(j+1)+5}; \\
b_{2s+(j+1)s, 11s+(-5)_s} &= w_{8(j+m+1)+5 \rightarrow 8(j+m+1)+7} \otimes w_{8j+7 \rightarrow 8(j+1)+1}; \\
b_{2s+(j+1)s, 11s+(-6)_s} &= -w_{8(j+m+1)+5 \rightarrow 8(j+m+1)+7} \otimes w_{8j+7 \rightarrow 8(j+1)+1}.
\end{aligned}$$

(26) If  $r_0 = 25$ , then  $\Omega^{25}(Z_t^{(12)})$  is described with  $(10s \times 14s)$  matrix with the following nonzero entries:

$$\begin{aligned}
b_{(j+1)s, s+(-6)_s} &= e_{8(j+m+1)+4} \otimes w_{8j \rightarrow 8(j+1)}; \\
b_{(j+1)s, s+(-5)_s} &= -e_{8(j+m+1)+4} \otimes w_{8j \rightarrow 8(j+1)}; \\
b_{(j+1)s, s+(-4)_s} &= e_{8(j+m+1)+4} \otimes w_{8j \rightarrow 8(j+1)}; \\
b_{(j+1)s, s+(-3)_s} &= -e_{8(j+m+1)+4} \otimes w_{8j \rightarrow 8(j+1)}; \\
b_{s+(j+1)s, 2s+(-5)_s} &= e_{8(j+m+1)+6} \otimes w_{8j \rightarrow 8(j+1)}; \\
b_{s+(j+1)s, 2s+(-4)_s} &= -e_{8(j+m+1)+6} \otimes w_{8j \rightarrow 8(j+1)}; \\
b_{s+(j+1)s, 2s+(-3)_s} &= e_{8(j+m+1)+6} \otimes w_{8j \rightarrow 8(j+1)}; \\
b_{j-s, 3s+(-5)_s} &= w_{8(j+m)+7 \rightarrow 8(j+m+1)+5} \otimes w_{8j \rightarrow 8j+1}; \\
b_{j, 3s+(-5)_s} &= w_{8(j+m+1) \rightarrow 8(j+m+1)+5} \otimes w_{8j \rightarrow 8j+2}; \\
b_{j+4s, 3s+(-5)_s} &= w_{8(j+m+1) \rightarrow 8(j+m+1)+5} \otimes w_{8j \rightarrow 8j+6}; \\
b_{j-s, 3s+(-4)_s} &= -w_{8(j+m)+7 \rightarrow 8(j+m+1)+5} \otimes w_{8j \rightarrow 8j+1}; \\
b_{j, 3s+(-4)_s} &= -w_{8(j+m+1) \rightarrow 8(j+m+1)+5} \otimes w_{8j \rightarrow 8j+2}; \\
b_{j+4s, 3s+(-4)_s} &= -w_{8(j+m+1) \rightarrow 8(j+m+1)+5} \otimes w_{8j \rightarrow 8j+6}; \\
b_{j-s, 3s+(-3)_s} &= w_{8(j+m)+7 \rightarrow 8(j+m+1)+5} \otimes w_{8j \rightarrow 8j+1}; \\
b_{j, 3s+(-3)_s} &= w_{8(j+m+1) \rightarrow 8(j+m+1)+5} \otimes w_{8j \rightarrow 8j+2}; \\
b_{j+4s, 3s+(-3)_s} &= w_{8(j+m+1) \rightarrow 8(j+m+1)+5} \otimes w_{8j \rightarrow 8j+6};
\end{aligned}$$

$$\begin{aligned}
b_{j-s,3s+(-2)_s} &= -w_{8(j+m)+7 \rightarrow 8(j+m+1)+5} \otimes w_{8j \rightarrow 8j+1}; \\
b_{j,3s+(-2)_s} &= -w_{8(j+m+1) \rightarrow 8(j+m+1)+5} \otimes w_{8j \rightarrow 8j+2}; \\
b_{j+4s,3s+(-2)_s} &= -w_{8(j+m+1) \rightarrow 8(j+m+1)+5} \otimes w_{8j \rightarrow 8j+6}; \\
b_{s+(j+1)_s,4s+(-6)_s} &= -w_{8(j+m+1)+6 \rightarrow 8(j+m+1)+7} \otimes w_{8j+1 \rightarrow 8(j+1)}; \\
b_{s+(j+1)_s,5s+(-5)_s} &= w_{8(j+m+1)+6 \rightarrow 8(j+m+2)} \otimes w_{8j+2 \rightarrow 8(j+1)}; \\
b_{3s+(j+1)_s,5s+(-5)_s} &= e_{8(j+m+2)} \otimes w_{8j+2 \rightarrow 8(j+1)+2}; \\
b_{s+(j+1)_s,5s+(-4)_s} &= -w_{8(j+m+1)+6 \rightarrow 8(j+m+2)} \otimes w_{8j+2 \rightarrow 8(j+1)}; \\
b_{3s+(j+1)_s,5s+(-4)_s} &= -e_{8(j+m+2)} \otimes w_{8j+2 \rightarrow 8(j+1)+2}; \\
b_{s+(j+1)_s,5s+(-3)_s} &= w_{8(j+m+1)+6 \rightarrow 8(j+m+2)} \otimes w_{8j+2 \rightarrow 8(j+1)}; \\
b_{3s+(j+1)_s,5s+(-3)_s} &= e_{8(j+m+2)} \otimes w_{8j+2 \rightarrow 8(j+1)+2}; \\
b_{(j+1)_s,8s+(-2)_s} &= w_{8(j+m+1)+4 \rightarrow 8(j+m+1)+7} \otimes w_{8j+5 \rightarrow 8(j+1)}; \\
b_{2s+(j+1)_s,11s+(-6)_s} &= w_{8(j+m+1)+7 \rightarrow 8(j+m+2)+5} \otimes w_{8j+7 \rightarrow 8(j+1)+1}; \\
b_{3s+(j+1)_s,11s+(-6)_s} &= w_{8(j+m+2) \rightarrow 8(j+m+2)+5} \otimes w_{8j+7 \rightarrow 8(j+1)+2}; \\
b_{7s+(j+1)_s,11s+(-6)_s} &= w_{8(j+m+2) \rightarrow 8(j+m+2)+5} \otimes w_{8j+7 \rightarrow 8(j+1)+6}; \\
b_{2s+(j+1)_s,11s+(-5)_s} &= -w_{8(j+m+1)+7 \rightarrow 8(j+m+2)+5} \otimes w_{8j+7 \rightarrow 8(j+1)+1}; \\
b_{3s+(j+1)_s,11s+(-5)_s} &= -w_{8(j+m+2) \rightarrow 8(j+m+2)+5} \otimes w_{8j+7 \rightarrow 8(j+1)+2}; \\
b_{7s+(j+1)_s,11s+(-5)_s} &= -w_{8(j+m+2) \rightarrow 8(j+m+2)+5} \otimes w_{8j+7 \rightarrow 8(j+1)+6}; \\
b_{2s+(j+1)_s,11s+(-4)_s} &= w_{8(j+m+1)+7 \rightarrow 8(j+m+2)+5} \otimes w_{8j+7 \rightarrow 8(j+1)+1}; \\
b_{3s+(j+1)_s,11s+(-4)_s} &= w_{8(j+m+2) \rightarrow 8(j+m+2)+5} \otimes w_{8j+7 \rightarrow 8(j+1)+2}; \\
b_{7s+(j+1)_s,11s+(-4)_s} &= w_{8(j+m+2) \rightarrow 8(j+m+2)+5} \otimes w_{8j+7 \rightarrow 8(j+1)+6}; \\
b_{2s+(j+1)_s,11s+(-3)_s} &= -w_{8(j+m+1)+7 \rightarrow 8(j+m+2)+5} \otimes w_{8j+7 \rightarrow 8(j+1)+1}; \\
b_{3s+(j+1)_s,11s+(-3)_s} &= -w_{8(j+m+2) \rightarrow 8(j+m+2)+5} \otimes w_{8j+7 \rightarrow 8(j+1)+2}; \\
b_{7s+(j+1)_s,11s+(-3)_s} &= -w_{8(j+m+2) \rightarrow 8(j+m+2)+5} \otimes w_{8j+7 \rightarrow 8(j+1)+6}; \\
b_{(j+1)_s,12s+(-2)_s} &= -w_{8(j+m+1)+4 \rightarrow 8(j+m+2)+3} \otimes w_{8j+7 \rightarrow 8(j+1)}; \\
b_{2s+(j+1)_s,12s+(-2)_s} &= -w_{8(j+m+1)+7 \rightarrow 8(j+m+2)+3} \otimes w_{8j+7 \rightarrow 8(j+1)+1}; \\
b_{3s+(j+1)_s,12s+(-2)_s} &= -w_{8(j+m+2) \rightarrow 8(j+m+2)+3} \otimes w_{8j+7 \rightarrow 8(j+1)+2}; \\
b_{7s+(j+1)_s,12s+(-2)_s} &= -w_{8(j+m+2) \rightarrow 8(j+m+2)+3} \otimes w_{8j+7 \rightarrow 8(j+1)+6}.
\end{aligned}$$

(27) If  $r_0 = 26$ , then  $\Omega^{26}(Z_t^{(12)})$  is described with  $(8s \times 16s)$  matrix with the following nonzero entries:

$$\begin{aligned}
b_{j,(-5)_s} &= -w_{8(j+m-1)+7 \rightarrow 8(j+m)+7} \otimes e_{8j}; \\
b_{(j+1)_s,(-5)_s} &= e_{8(j+m)+7} \otimes w_{8j \rightarrow 8(j+1)}; \\
b_{j+2s,(-5)_s} &= -w_{8(j+m)+1 \rightarrow 8(j+m)+7} \otimes w_{8j \rightarrow 8j+2}; \\
b_{j+3s,(-5)_s} &= w_{8(j+m)+2 \rightarrow 8(j+m)+7} \otimes w_{8j \rightarrow 8j+3}; \\
b_{j+4s,(-5)_s} &= -w_{8(j+m)+3 \rightarrow 8(j+m)+7} \otimes w_{8j \rightarrow 8j+4}; \\
b_{j+5s,(-5)_s} &= -w_{8(j+m)+4 \rightarrow 8(j+m)+7} \otimes w_{8j \rightarrow 8j+5}; \\
b_{j,(-4)_s} &= w_{8(j+m-1)+7 \rightarrow 8(j+m)+7} \otimes e_{8j}; \\
b_{(j+1)_s,(-4)_s} &= -e_{8(j+m)+7} \otimes w_{8j \rightarrow 8(j+1)}; \\
b_{j+2s,(-4)_s} &= w_{8(j+m)+1 \rightarrow 8(j+m)+7} \otimes w_{8j \rightarrow 8j+2}; \\
b_{j+3s,(-4)_s} &= -w_{8(j+m)+2 \rightarrow 8(j+m)+7} \otimes w_{8j \rightarrow 8j+3}; \\
b_{j+4s,(-4)_s} &= w_{8(j+m)+3 \rightarrow 8(j+m)+7} \otimes w_{8j \rightarrow 8j+4};
\end{aligned}$$

$$\begin{aligned}
b_{j+5s,(-4)_s} &= w_{8(j+m)+4 \rightarrow 8(j+m)+7} \otimes w_{8j \rightarrow 8j+5}; \\
b_{j,(-3)_s} &= -w_{8(j+m-1)+7 \rightarrow 8(j+m)+7} \otimes e_{8j}; \\
b_{(j+1)_s,(-3)_s} &= e_{8(j+m)+7} \otimes w_{8j \rightarrow 8(j+1)}; \\
b_{j+2s,(-3)_s} &= -w_{8(j+m)+1 \rightarrow 8(j+m)+7} \otimes w_{8j \rightarrow 8j+2}; \\
b_{j+3s,(-3)_s} &= w_{8(j+m)+2 \rightarrow 8(j+m)+7} \otimes w_{8j \rightarrow 8j+3}; \\
b_{j+4s,(-3)_s} &= -w_{8(j+m)+3 \rightarrow 8(j+m)+7} \otimes w_{8j \rightarrow 8j+4}; \\
b_{j+5s,(-3)_s} &= -w_{8(j+m)+4 \rightarrow 8(j+m)+7} \otimes w_{8j \rightarrow 8j+5}; \\
b_{j,(-2)_s} &= w_{8(j+m-1)+7 \rightarrow 8(j+m)+7} \otimes e_{8j}; \\
b_{j+2s,(-2)_s} &= w_{8(j+m)+1 \rightarrow 8(j+m)+7} \otimes w_{8j \rightarrow 8j+2}; \\
b_{j+3s,(-2)_s} &= -w_{8(j+m)+2 \rightarrow 8(j+m)+7} \otimes w_{8j \rightarrow 8j+3}; \\
b_{j+4s,(-2)_s} &= w_{8(j+m)+3 \rightarrow 8(j+m)+7} \otimes w_{8j \rightarrow 8j+4}; \\
b_{j+5s,(-2)_s} &= w_{8(j+m)+4 \rightarrow 8(j+m)+7} \otimes w_{8j \rightarrow 8j+5}; \\
b_{(j+1)_s,s+(-6)_s} &= e_{8(j+m)+7} \otimes w_{8j \rightarrow 8(j+1)}; \\
b_{j-s,s+(-5)_s} &= -w_{8(j+m-1)+7 \rightarrow 8(j+m)+7} \otimes e_{8j}; \\
b_{j+s,s+(-5)_s} &= -w_{8(j+m)+1 \rightarrow 8(j+m)+7} \otimes w_{8j \rightarrow 8j+2}; \\
b_{j+2s,s+(-5)_s} &= w_{8(j+m)+2 \rightarrow 8(j+m)+7} \otimes w_{8j \rightarrow 8j+3}; \\
b_{j+3s,s+(-5)_s} &= -w_{8(j+m)+3 \rightarrow 8(j+m)+7} \otimes w_{8j \rightarrow 8j+4}; \\
b_{j+4s,s+(-5)_s} &= -w_{8(j+m)+4 \rightarrow 8(j+m)+7} \otimes w_{8j \rightarrow 8j+5}; \\
b_{j-s,s+(-4)_s} &= w_{8(j+m-1)+7 \rightarrow 8(j+m)+7} \otimes e_{8j}; \\
b_{j+s,s+(-4)_s} &= w_{8(j+m)+1 \rightarrow 8(j+m)+7} \otimes w_{8j \rightarrow 8j+2}; \\
b_{j+2s,s+(-4)_s} &= -w_{8(j+m)+2 \rightarrow 8(j+m)+7} \otimes w_{8j \rightarrow 8j+3}; \\
b_{j+3s,s+(-4)_s} &= w_{8(j+m)+3 \rightarrow 8(j+m)+7} \otimes w_{8j \rightarrow 8j+4}; \\
b_{j+4s,s+(-4)_s} &= w_{8(j+m)+4 \rightarrow 8(j+m)+7} \otimes w_{8j \rightarrow 8j+5}; \\
b_{j-s,s+(-3)_s} &= -w_{8(j+m-1)+7 \rightarrow 8(j+m)+7} \otimes e_{8j}; \\
b_{j+s,s+(-3)_s} &= -w_{8(j+m)+1 \rightarrow 8(j+m)+7} \otimes w_{8j \rightarrow 8j+2}; \\
b_{j+2s,s+(-3)_s} &= w_{8(j+m)+2 \rightarrow 8(j+m)+7} \otimes w_{8j \rightarrow 8j+3}; \\
b_{j+3s,s+(-3)_s} &= -w_{8(j+m)+3 \rightarrow 8(j+m)+7} \otimes w_{8j \rightarrow 8j+4}; \\
b_{j+4s,s+(-3)_s} &= -w_{8(j+m)+4 \rightarrow 8(j+m)+7} \otimes w_{8j \rightarrow 8j+5}; \\
b_{j-s,s+(-2)_s} &= w_{8(j+m-1)+7 \rightarrow 8(j+m)+7} \otimes e_{8j}; \\
b_{j+s,s+(-2)_s} &= w_{8(j+m)+1 \rightarrow 8(j+m)+7} \otimes w_{8j \rightarrow 8j+2}; \\
b_{j+2s,s+(-2)_s} &= -w_{8(j+m)+2 \rightarrow 8(j+m)+7} \otimes w_{8j \rightarrow 8j+3}; \\
b_{j+3s,s+(-2)_s} &= w_{8(j+m)+3 \rightarrow 8(j+m)+7} \otimes w_{8j \rightarrow 8j+4}; \\
b_{j+4s,s+(-2)_s} &= w_{8(j+m)+4 \rightarrow 8(j+m)+7} \otimes w_{8j \rightarrow 8j+5}; \\
b_{(j+1)_s,3s+(-6)_s} &= w_{8(j+m)+7 \rightarrow 8(j+m+1)+5} \otimes w_{8j+1 \rightarrow 8(j+1)}; \\
b_{(j+1)_s,3s+(-5)_s} &= -w_{8(j+m)+7 \rightarrow 8(j+m+1)+5} \otimes w_{8j+1 \rightarrow 8(j+1)}; \\
b_{(j+1)_s,3s+(-4)_s} &= w_{8(j+m)+7 \rightarrow 8(j+m+1)+5} \otimes w_{8j+1 \rightarrow 8(j+1)}; \\
b_{(j+1)_s,3s+(-3)_s} &= -w_{8(j+m)+7 \rightarrow 8(j+m+1)+5} \otimes w_{8j+1 \rightarrow 8(j+1)}; \\
b_{s+(j+1)_s,4s+(-6)_s} &= e_{8(j+m+1)+6} \otimes w_{8j+2 \rightarrow 8(j+1)+1}; \\
b_{(j+1)_s,4s+(-5)_s} &= -w_{8(j+m)+7 \rightarrow 8(j+m+1)+6} \otimes w_{8j+2 \rightarrow 8(j+1)+1};
\end{aligned}$$



$$\begin{aligned}
b_{5s+(j+1)s,14s+(-2)s} &= w_{8(j+m+1)+4 \rightarrow 8(j+m+1)+7} \otimes w_{8j+7 \rightarrow 8(j+1)+5}; \\
b_{2s+(j+1)s,15s+(-2)s} &= -w_{8(j+m+1)+1 \rightarrow 8(j+m+2)} \otimes w_{8j+7 \rightarrow 8(j+1)+2}; \\
b_{3s+(j+1)s,15s+(-2)s} &= w_{8(j+m+1)+2 \rightarrow 8(j+m+2)} \otimes w_{8j+7 \rightarrow 8(j+1)+3}; \\
b_{4s+(j+1)s,15s+(-2)s} &= -w_{8(j+m+1)+3 \rightarrow 8(j+m+2)} \otimes w_{8j+7 \rightarrow 8(j+1)+4}; \\
b_{5s+(j+1)s,15s+(-2)s} &= -w_{8(j+m+1)+4 \rightarrow 8(j+m+2)} \otimes w_{8j+7 \rightarrow 8(j+1)+5}.
\end{aligned}$$

(28) If  $r_0 = 27$ , then  $\Omega^{27}(Z_t^{(12)})$  is described with  $(9s \times 16s)$  matrix with the following nonzero entries:

$$\begin{aligned}
b_{j,s+(-5)s} &= w_{8(j+m+1) \rightarrow 8(j+m+1)+3} \otimes w_{8j \rightarrow 8j+1}; \\
b_{j+4s,s+(-5)s} &= -w_{8(j+m+1) \rightarrow 8(j+m+1)+3} \otimes w_{8j \rightarrow 8j+5}; \\
b_{j,s+(-4)s} &= -w_{8(j+m+1) \rightarrow 8(j+m+1)+3} \otimes w_{8j \rightarrow 8j+1}; \\
b_{j+4s,s+(-4)s} &= w_{8(j+m+1) \rightarrow 8(j+m+1)+3} \otimes w_{8j \rightarrow 8j+5}; \\
b_{j,s+(-3)s} &= w_{8(j+m+1) \rightarrow 8(j+m+1)+3} \otimes w_{8j \rightarrow 8j+1}; \\
b_{j+4s,s+(-3)s} &= -w_{8(j+m+1) \rightarrow 8(j+m+1)+3} \otimes w_{8j \rightarrow 8j+5}; \\
b_{j,s+(-2)s} &= -w_{8(j+m+1) \rightarrow 8(j+m+1)+3} \otimes w_{8j \rightarrow 8j+1}; \\
b_{j+4s,s+(-2)s} &= w_{8(j+m+1) \rightarrow 8(j+m+1)+3} \otimes w_{8j \rightarrow 8j+5}; \\
b_{(j+1)s,4s+(-6)s} &= w_{8(j+m+1)+7 \rightarrow 8(j+m+2)} \otimes w_{8j+1 \rightarrow 8(j+1)}; \\
b_{(j+1)s,5s+(-6)s} &= -e_{8(j+m+1)+7} \otimes w_{8j+2 \rightarrow 8(j+1)}; \\
b_{(j+1)s,8s+(-2)s} &= e_{8(j+m+1)+7} \otimes w_{8j+5 \rightarrow 8(j+1)}; \\
b_{(j+1)s,10s+(-6)s} &= -e_{8(j+m+1)+7} \otimes w_{8j+6 \rightarrow 8(j+1)}; \\
b_{(j+1)s,10s+(-5)s} &= e_{8(j+m+1)+7} \otimes w_{8j+6 \rightarrow 8(j+1)}; \\
b_{(j+1)s,10s+(-4)s} &= -e_{8(j+m+1)+7} \otimes w_{8j+6 \rightarrow 8(j+1)}; \\
b_{(j+1)s,10s+(-3)s} &= e_{8(j+m+1)+7} \otimes w_{8j+6 \rightarrow 8(j+1)}; \\
b_{(j+1)s,12s+(-6)s} &= w_{8(j+m+1)+7 \rightarrow 8(j+m+2)+2} \otimes w_{8j+7 \rightarrow 8(j+1)}; \\
b_{(j+1)s,12s+(-5)s} &= -w_{8(j+m+1)+7 \rightarrow 8(j+m+2)+2} \otimes w_{8j+7 \rightarrow 8(j+1)}; \\
b_{(j+1)s,12s+(-4)s} &= w_{8(j+m+1)+7 \rightarrow 8(j+m+2)+2} \otimes w_{8j+7 \rightarrow 8(j+1)}; \\
b_{(j+1)s,12s+(-3)s} &= -w_{8(j+m+1)+7 \rightarrow 8(j+m+2)+2} \otimes w_{8j+7 \rightarrow 8(j+1)}; \\
b_{(j+1)s,13s+(-2)s} &= -w_{8(j+m+1)+7 \rightarrow 8(j+m+2)+4} \otimes w_{8j+7 \rightarrow 8(j+1)}.
\end{aligned}$$

(29) If  $r_0 = 28$ , then  $\Omega^{28}(Z_t^{(12)})$  is described with  $(8s \times 19s)$  matrix with the following nonzero entries:

$$\begin{aligned}
b_{j,s,(-5)s} &= -w_{8(j+m)+1 \rightarrow 8(j+m)+7} \otimes w_{8j \rightarrow 8j+1}; \\
b_{j+2s,(-5)s} &= w_{8(j+m)+2 \rightarrow 8(j+m)+7} \otimes w_{8j \rightarrow 8j+2}; \\
b_{j+3s,(-5)s} &= -w_{8(j+m)+3 \rightarrow 8(j+m)+7} \otimes w_{8j \rightarrow 8j+3}; \\
b_{j+4s,(-5)s} &= w_{8(j+m)+4 \rightarrow 8(j+m)+7} \otimes w_{8j \rightarrow 8j+4}; \\
b_{j+5s,(-5)s} &= w_{8(j+m)+5 \rightarrow 8(j+m)+7} \otimes w_{8j \rightarrow 8j+5}; \\
b_{j+6s,(-5)s} &= -w_{8(j+m)+6 \rightarrow 8(j+m)+7} \otimes w_{8j \rightarrow 8j+6}; \\
b_{j+7s,(-5)s} &= e_{8(j+m)+7} \otimes w_{8j \rightarrow 8j+7}; \\
b_{j,s,(-4)s} &= w_{8(j+m)+1 \rightarrow 8(j+m)+7} \otimes w_{8j \rightarrow 8j+1}; \\
b_{j+2s,(-4)s} &= -w_{8(j+m)+2 \rightarrow 8(j+m)+7} \otimes w_{8j \rightarrow 8j+2}; \\
b_{j+3s,(-4)s} &= w_{8(j+m)+3 \rightarrow 8(j+m)+7} \otimes w_{8j \rightarrow 8j+3}; \\
b_{j+4s,(-4)s} &= -w_{8(j+m)+4 \rightarrow 8(j+m)+7} \otimes w_{8j \rightarrow 8j+4};
\end{aligned}$$

$$\begin{aligned}
b_{j+5s,(-4)_s} &= -w_{8(j+m)+5 \rightarrow 8(j+m)+7} \otimes w_{8j \rightarrow 8j+5}; \\
b_{j+6s,(-4)_s} &= w_{8(j+m)+6 \rightarrow 8(j+m)+7} \otimes w_{8j \rightarrow 8j+6}; \\
b_{j+7s,(-4)_s} &= -e_{8(j+m)+7} \otimes w_{8j \rightarrow 8j+7}; \\
b_{j+s,(-3)_s} &= -w_{8(j+m)+1 \rightarrow 8(j+m)+7} \otimes w_{8j \rightarrow 8j+1}; \\
b_{j+2s,(-3)_s} &= w_{8(j+m)+2 \rightarrow 8(j+m)+7} \otimes w_{8j \rightarrow 8j+2}; \\
b_{j+3s,(-3)_s} &= -w_{8(j+m)+3 \rightarrow 8(j+m)+7} \otimes w_{8j \rightarrow 8j+3}; \\
b_{j+4s,(-3)_s} &= w_{8(j+m)+4 \rightarrow 8(j+m)+7} \otimes w_{8j \rightarrow 8j+4}; \\
b_{j+5s,(-3)_s} &= w_{8(j+m)+5 \rightarrow 8(j+m)+7} \otimes w_{8j \rightarrow 8j+5}; \\
b_{j+6s,(-3)_s} &= -w_{8(j+m)+6 \rightarrow 8(j+m)+7} \otimes w_{8j \rightarrow 8j+6}; \\
b_{j+7s,(-3)_s} &= e_{8(j+m)+7} \otimes w_{8j \rightarrow 8j+7}; \\
b_{j+s,(-2)_s} &= w_{8(j+m)+1 \rightarrow 8(j+m)+7} \otimes w_{8j \rightarrow 8j+1}; \\
b_{j+2s,(-2)_s} &= -w_{8(j+m)+2 \rightarrow 8(j+m)+7} \otimes w_{8j \rightarrow 8j+2}; \\
b_{j+3s,(-2)_s} &= w_{8(j+m)+3 \rightarrow 8(j+m)+7} \otimes w_{8j \rightarrow 8j+3}; \\
b_{j+4s,(-2)_s} &= -w_{8(j+m)+4 \rightarrow 8(j+m)+7} \otimes w_{8j \rightarrow 8j+4}; \\
b_{j+5s,(-2)_s} &= -w_{8(j+m)+5 \rightarrow 8(j+m)+7} \otimes w_{8j \rightarrow 8j+5}; \\
b_{j+6s,(-2)_s} &= w_{8(j+m)+6 \rightarrow 8(j+m)+7} \otimes w_{8j \rightarrow 8j+6}; \\
b_{j+7s,(-2)_s} &= -e_{8(j+m)+7} \otimes w_{8j \rightarrow 8j+7}; \\
b_{j-s,s+(-5)_s} &= w_{8(j+m) \rightarrow 8(j+m+1)} \otimes e_{8j}; \\
b_{j-s,s+(-4)_s} &= -w_{8(j+m) \rightarrow 8(j+m+1)} \otimes e_{8j}; \\
b_{j-s,s+(-3)_s} &= w_{8(j+m) \rightarrow 8(j+m+1)} \otimes e_{8j}; \\
b_{j-s,s+(-2)_s} &= -w_{8(j+m) \rightarrow 8(j+m+1)} \otimes e_{8j}; \\
b_{(j+1)_s,s+(-2)_s} &= e_{8(j+m+1)} \otimes w_{8j \rightarrow 8(j+1)}; \\
b_{(j+1)_s,2s+(-6)_s} &= e_{8(j+m+1)} \otimes w_{8j \rightarrow 8(j+1)}; \\
b_{(j+1)_s,4s+(-6)_s} &= w_{8(j+m+1) \rightarrow 8(j+m+1)+1} \otimes w_{8j+1 \rightarrow 8(j+1)}; \\
b_{s+(j+1)_s,4s+(-6)_s} &= -e_{8(j+m+1)+1} \otimes w_{8j+1 \rightarrow 8(j+1)+1}; \\
b_{(j+1)_s,5s+(-5)_s} &= -w_{8(j+m+1) \rightarrow 8(j+m+1)+2} \otimes w_{8j+2 \rightarrow 8(j+1)}; \\
b_{s+(j+1)_s,5s+(-5)_s} &= w_{8(j+m+1)+1 \rightarrow 8(j+m+1)+2} \otimes w_{8j+2 \rightarrow 8(j+1)+1}; \\
b_{2s+(j+1)_s,5s+(-5)_s} &= -e_{8(j+m+1)+2} \otimes w_{8j+2 \rightarrow 8(j+1)+2}; \\
b_{(j+1)_s,5s+(-4)_s} &= w_{8(j+m+1) \rightarrow 8(j+m+1)+2} \otimes w_{8j+2 \rightarrow 8(j+1)}; \\
b_{s+(j+1)_s,5s+(-4)_s} &= -w_{8(j+m+1)+1 \rightarrow 8(j+m+1)+2} \otimes w_{8j+2 \rightarrow 8(j+1)+1}; \\
b_{2s+(j+1)_s,5s+(-4)_s} &= e_{8(j+m+1)+2} \otimes w_{8j+2 \rightarrow 8(j+1)+2}; \\
b_{(j+1)_s,5s+(-3)_s} &= -w_{8(j+m+1) \rightarrow 8(j+m+1)+2} \otimes w_{8j+2 \rightarrow 8(j+1)}; \\
b_{s+(j+1)_s,5s+(-3)_s} &= w_{8(j+m+1)+1 \rightarrow 8(j+m+1)+2} \otimes w_{8j+2 \rightarrow 8(j+1)+1}; \\
b_{2s+(j+1)_s,5s+(-3)_s} &= -e_{8(j+m+1)+2} \otimes w_{8j+2 \rightarrow 8(j+1)+2}; \\
b_{(j+1)_s,6s+(-6)_s} &= w_{8(j+m+1) \rightarrow 8(j+m+1)+3} \otimes w_{8j+3 \rightarrow 8(j+1)}; \\
b_{(j+1)_s,6s+(-5)_s} &= -w_{8(j+m+1) \rightarrow 8(j+m+1)+3} \otimes w_{8j+3 \rightarrow 8(j+1)}; \\
b_{(j+1)_s,6s+(-4)_s} &= w_{8(j+m+1) \rightarrow 8(j+m+1)+3} \otimes w_{8j+3 \rightarrow 8(j+1)}; \\
b_{(j+1)_s,6s+(-3)_s} &= -w_{8(j+m+1) \rightarrow 8(j+m+1)+3} \otimes w_{8j+3 \rightarrow 8(j+1)}; \\
b_{(j+1)_s,8s+(-6)_s} &= w_{8(j+m+1) \rightarrow 8(j+m+1)+4} \otimes w_{8j+4 \rightarrow 8(j+1)};
\end{aligned}$$

$$\begin{aligned}
b_{(j+1)s, 8s+(-5)_s} &= -w_{8(j+m+1) \rightarrow 8(j+m+1)+4} \otimes w_{8j+4 \rightarrow 8(j+1)}; \\
b_{(j+1)s, 8s+(-4)_s} &= w_{8(j+m+1) \rightarrow 8(j+m+1)+4} \otimes w_{8j+4 \rightarrow 8(j+1)}; \\
b_{(j+1)s, 8s+(-3)_s} &= -w_{8(j+m+1) \rightarrow 8(j+m+1)+4} \otimes w_{8j+4 \rightarrow 8(j+1)}; \\
b_{(j+1)s, 8s+(-2)_s} &= w_{8(j+m+1) \rightarrow 8(j+m+1)+4} \otimes w_{8j+4 \rightarrow 8(j+1)}; \\
b_{s+(j+1)s, 8s+(-2)_s} &= -w_{8(j+m+1)+1 \rightarrow 8(j+m+1)+4} \otimes w_{8j+4 \rightarrow 8(j+1)+1}; \\
b_{2s+(j+1)s, 8s+(-2)_s} &= w_{8(j+m+1)+2 \rightarrow 8(j+m+1)+4} \otimes w_{8j+4 \rightarrow 8(j+1)+2}; \\
b_{3s+(j+1)s, 8s+(-2)_s} &= -w_{8(j+m+1)+3 \rightarrow 8(j+m+1)+4} \otimes w_{8j+4 \rightarrow 8(j+1)+3}; \\
b_{4s+(j+1)s, 8s+(-2)_s} &= e_{8(j+m+1)+4} \otimes w_{8j+4 \rightarrow 8(j+1)+4}; \\
b_{(j+1)s, 10s+(-2)_s} &= w_{8(j+m+1) \rightarrow 8(j+m+1)+5} \otimes w_{8j+5 \rightarrow 8(j+1)}; \\
b_{5s+(j+1)s, 10s+(-2)_s} &= e_{8(j+m+1)+5} \otimes w_{8j+5 \rightarrow 8(j+1)+5}; \\
b_{j-8s, 14s+(-6)_s} &= w_{8(j+m)+6 \rightarrow 8(j+m+1)+6} \otimes e_{8j+6}; \\
b_{j-7s, 14s+(-6)_s} &= -w_{8(j+m)+7 \rightarrow 8(j+m+1)+6} \otimes w_{8j+6 \rightarrow 8j+7}; \\
b_{j-8s, 14s+(-5)_s} &= -w_{8(j+m)+6 \rightarrow 8(j+m+1)+6} \otimes e_{8j+6}; \\
b_{j-7s, 14s+(-5)_s} &= w_{8(j+m)+7 \rightarrow 8(j+m+1)+6} \otimes w_{8j+6 \rightarrow 8j+7}; \\
b_{j-8s, 14s+(-4)_s} &= w_{8(j+m)+6 \rightarrow 8(j+m+1)+6} \otimes e_{8j+6}; \\
b_{j-7s, 14s+(-4)_s} &= -w_{8(j+m)+7 \rightarrow 8(j+m+1)+6} \otimes w_{8j+6 \rightarrow 8j+7}; \\
b_{j-8s, 14s+(-3)_s} &= -w_{8(j+m)+6 \rightarrow 8(j+m+1)+6} \otimes e_{8j+6}; \\
b_{j-7s, 14s+(-3)_s} &= w_{8(j+m)+7 \rightarrow 8(j+m+1)+6} \otimes w_{8j+6 \rightarrow 8j+7}; \\
b_{j-9s, 16s+(-6)_s} &= w_{8(j+m)+7 \rightarrow 8(j+m+1)+7} \otimes e_{8j+7}; \\
b_{j-9s, 16s+(-5)_s} &= -w_{8(j+m)+7 \rightarrow 8(j+m+1)+7} \otimes e_{8j+7}; \\
b_{j-9s, 16s+(-4)_s} &= w_{8(j+m)+7 \rightarrow 8(j+m+1)+7} \otimes e_{8j+7}; \\
b_{j-9s, 16s+(-3)_s} &= -w_{8(j+m)+7 \rightarrow 8(j+m+1)+7} \otimes e_{8j+7}; \\
b_{(j+1)s, 17s+(-6)_s} &= -w_{8(j+m+1) \rightarrow 8(j+m+1)+7} \otimes w_{8j+7 \rightarrow 8(j+1)}; \\
b_{j-10s, 17s+(-6)_s} &= w_{8(j+m)+7 \rightarrow 8(j+m+1)+7} \otimes e_{8j+7}; \\
b_{(j+1)s, 17s+(-5)_s} &= w_{8(j+m+1) \rightarrow 8(j+m+1)+7} \otimes w_{8j+7 \rightarrow 8(j+1)}; \\
b_{j-10s, 17s+(-5)_s} &= -w_{8(j+m)+7 \rightarrow 8(j+m+1)+7} \otimes e_{8j+7}; \\
b_{(j+1)s, 17s+(-4)_s} &= -w_{8(j+m+1) \rightarrow 8(j+m+1)+7} \otimes w_{8j+7 \rightarrow 8(j+1)}; \\
b_{j-10s, 17s+(-4)_s} &= w_{8(j+m)+7 \rightarrow 8(j+m+1)+7} \otimes e_{8j+7}; \\
b_{(j+1)s, 17s+(-3)_s} &= w_{8(j+m+1) \rightarrow 8(j+m+1)+7} \otimes w_{8j+7 \rightarrow 8(j+1)}; \\
b_{j-10s, 17s+(-3)_s} &= -w_{8(j+m)+7 \rightarrow 8(j+m+1)+7} \otimes e_{8j+7}; \\
b_{j-10s, 17s+(-2)_s} &= -w_{8(j+m)+7 \rightarrow 8(j+m+1)+7} \otimes e_{8j+7}.
\end{aligned}$$

(II) Represent an arbitrary  $t_0 \in \mathbb{N}$  in the form  $t_0 = 29\ell_0 + r_0$ , where  $0 \leq r_0 \leq 28$ . Then  $\Omega^{t_0}(Z_t^{(12)})$  is a  $\Omega^{r_0}(Z_t^{(12)})$ , whose left components twisted by  $\sigma^{\ell_0}$ .

**Proposition 10** (Translates for the case 13). (I) Let  $r_0 \in \mathbb{N}$ ,  $r_0 < 29$ .  $r_0$ -translates of the elements  $Z_t^{(13)}$  are described by the following way.

(1) If  $r_0 = 0$ , then  $\Omega^0(Z_t^{(13)})$  is described with  $(8s \times 19s)$  matrix, whose entries  $b_{ij}$  have the following form:

If  $s \leq j < 2s$ , then

$$b_{ij} = \begin{cases} e_{8(j+m)} \otimes e_{8j}, & i = j - s; \\ 0, & \text{otherwise.} \end{cases}$$

If  $2s \leq j < 3s$ , then  $b_{ij} = 0$ .

If  $3s \leq j < 4s$ , then

$$b_{ij} = \begin{cases} -w_{8(j+m)+1 \rightarrow 8(j+m)+2} \otimes e_{8j+1}, & i = j - 2s; \\ 0, & \text{otherwise.} \end{cases}$$

If  $4s \leq j < 5s$ , then

$$b_{ij} = \begin{cases} -w_{8(j+m)+2 \rightarrow 8(j+m)+3} \otimes e_{8j+2}, & i = j - 2s; \\ 0, & \text{otherwise.} \end{cases}$$

If  $5s \leq j < 6s$ , then  $b_{ij} = 0$ .

If  $6s \leq j < 7s$ , then

$$b_{ij} = \begin{cases} -w_{8(j+m)+3 \rightarrow 8(j+m)+4} \otimes e_{8j+3}, & i = j - 3s; \\ 0, & \text{otherwise.} \end{cases}$$

If  $7s \leq j < 11s$ , then  $b_{ij} = 0$ .

If  $11s \leq j < 12s$ , then

$$b_{ij} = \begin{cases} w_{8(j+m)+5 \rightarrow 8(j+m)+6} \otimes e_{8j+5}, & i = j - 6s; \\ 0, & \text{otherwise.} \end{cases}$$

If  $12s \leq j < 13s$ , then

$$b_{ij} = \begin{cases} -e_{8(j+m)+5} \otimes e_{8j+5}, & i = j - 7s; \\ 0, & \text{otherwise.} \end{cases}$$

If  $13s \leq j < 14s$ , then

$$b_{ij} = \begin{cases} e_{8(j+m)+6} \otimes e_{8j+6}, & i = j - 7s; \\ 0, & \text{otherwise.} \end{cases}$$

If  $14s \leq j < 16s$ , then  $b_{ij} = 0$ .

If  $16s \leq j < 17s$ , then

$$b_{ij} = \begin{cases} e_{8(j+m)+7} \otimes e_{8j+7}, & i = j - 9s; \\ 0, & \text{otherwise.} \end{cases}$$

If  $17s \leq j < 18s$ , then  $b_{ij} = 0$ .

If  $18s \leq j < 19s$ , then

$$b_{ij} = \begin{cases} w_{8(j+m)+7 \rightarrow 8(j+m)+1} \otimes e_{8j+7}, & i = j - 11s; \\ 0, & \text{otherwise.} \end{cases}$$



(2) If  $r_0 = 1$ , then  $\Omega^1(Z_t^{(13)})$  is described with  $(9s \times 18s)$  matrix, whose entries  $b_{ij}$  have the following form:

If  $0 \leq j < s$ , then

$$b_{ij} = \begin{cases} -w_{8(j+m)+1 \rightarrow 8(j+m)+2} \otimes e_{8j}, & i = j; \\ 0, & \text{otherwise.} \end{cases}$$

If  $s \leq j < 2s$ , then

$$b_{ij} = \begin{cases} w_{8(j+m)+2 \rightarrow 8(j+m)+3} \otimes w_{8j \rightarrow 8j+1}, & i = j + s; \\ 0, & \text{otherwise.} \end{cases}$$

If  $2s \leq j < 3s$ , then

$$b_{ij} = \begin{cases} e_{8(j+m)+6} \otimes w_{8j \rightarrow 8j+5}, & i = j + 4s; \\ 0, & \text{otherwise.} \end{cases}$$

If  $3s \leq j < 4s$ , then

$$b_{ij} = \begin{cases} e_{8(j+m)+5} \otimes e_{8j}, & i = j - 2s; \\ 0, & \text{otherwise.} \end{cases}$$

If  $4s \leq j < 5s$ , then

$$b_{ij} = \begin{cases} -w_{8(j+m)+2 \rightarrow 8(j+m)+1} \otimes e_{8j+1}, & i = j - 2s; \\ -w_{8(j+m)+3 \rightarrow 8(j+m)+1} \otimes w_{8j+1 \rightarrow 8j+2}, & i = j - s; \\ -w_{8(j+m)+4 \rightarrow 8(j+m)+1} \otimes w_{8j+1 \rightarrow 8j+3}, & i = j; \\ -w_{8(j+m)+7 \rightarrow 8(j+m)+1} \otimes w_{8j+1 \rightarrow 8j+4}, & i = j + s; \\ -e_{8(j+m)+1} \otimes w_{8j+1 \rightarrow 8j+7}, & i = j + 4s; \\ 0, & \text{otherwise.} \end{cases}$$

If  $5s \leq j < 6s$ , then

$$b_{ij} = \begin{cases} -w_{8(j+m)+3 \rightarrow 8(j+m)+7} \otimes e_{8j+2}, & i = j - 2s; \\ 0, & \text{otherwise.} \end{cases}$$

If  $6s \leq j < 7s$ , then

$$b_{ij} = \begin{cases} -w_{8(j+m)+4 \rightarrow 8(j+m)+7} \otimes e_{8j+3}, & i = j - 2s; \\ -e_{8(j+m)+7} \otimes w_{8j+3 \rightarrow 8j+4}, & i = j - s; \\ 0, & \text{otherwise.} \end{cases}$$

If  $7s \leq j < 8s$ , then

$$b_{ij} = \begin{cases} -e_{8(j+m)+1} \otimes w_{8j+3 \rightarrow 8j+7}, & i = j + s; \\ 0, & \text{otherwise.} \end{cases}$$

If  $8s \leq j < 10s$ , then  $b_{ij} = 0$ .

If  $10s \leq j < 11s$ , then

$$b_{ij} = \begin{cases} w_{8(j+m)+6 \rightarrow 8(j+m)+1} \otimes e_{8j+5}, & i = j - 4s; \\ e_{8(j+m)+1} \otimes w_{8j+5 \rightarrow 8j+7}, & i = j - 2s; \\ 0, & \text{otherwise.} \end{cases}$$

If  $11s \leq j < 12s$ , then

$$b_{ij} = \begin{cases} e_{8(j+m)+7} \otimes e_{8j+6}, & i = j - 4s; \\ 0, & \text{otherwise.} \end{cases}$$

If  $12s \leq j < 13s$ , then  $b_{ij} = 0$ .

If  $13s \leq j < 14s$ , then

$$b_{ij} = \begin{cases} w_{8(j+m+1)+1 \rightarrow 8(j+m+1)+2} \otimes w_{8j+7 \rightarrow 8(j+1)}, & i = (j+1)_s; \\ w_{8(j+m+1) \rightarrow 8(j+m+1)+2} \otimes e_{8j+7}, & i = j - 5s; \\ 0, & \text{otherwise.} \end{cases}$$

If  $14s \leq j < 15s$ , then

$$b_{ij} = \begin{cases} w_{8(j+m+1)+5 \rightarrow 8(j+m+1)+6} \otimes w_{8j+7 \rightarrow 8(j+1)}, & i = s + (j+1)_s; \\ 0, & \text{otherwise.} \end{cases}$$

If  $15s \leq j < 16s$ , then

$$b_{ij} = \begin{cases} -w_{8(j+m+1)+3 \rightarrow 8(j+m+1)+4} \otimes w_{8j+7 \rightarrow 8(j+1)+2}, & i = 3s + (j+1)_s; \\ 0, & \text{otherwise.} \end{cases}$$

If  $16s \leq j < 17s$ , then

$$b_{ij} = \begin{cases} w_{8(j+m+1) \rightarrow 8(j+m+1)+1} \otimes e_{8j+7}, & i = j - 8s; \\ 0, & \text{otherwise.} \end{cases}$$

If  $17s \leq j < 18s$ , then  $b_{ij} = 0$ .

(3) If  $r_0 = 2$ , then  $\Omega^2(Z_t^{(13)})$  is described with  $(8s \times 20s)$  matrix, whose entries  $b_{ij}$  have the following form:

If  $0 \leq j < s$ , then

$$b_{ij} = \begin{cases} -e_{8(j+m-1)+7} \otimes e_{8j}, & i = j; \\ 0, & \text{otherwise.} \end{cases}$$

If  $s \leq j < 3s$ , then  $b_{ij} = 0$ .

If  $3s \leq j < 4s$ , then

$$b_{ij} = \begin{cases} -w_{8(j+m)+2 \rightarrow 8(j+m)+3} \otimes e_{8j+1}, & i = j - 2s; \\ 0, & \text{otherwise.} \end{cases}$$

If  $4s \leq j < 5s$ , then

$$b_{ij} = \begin{cases} -e_{8(j+m)+5} \otimes w_{8j+1 \rightarrow 8j+4}, & i = j; \\ 0, & \text{otherwise.} \end{cases}$$

If  $5s \leq j < 6s$ , then

$$b_{ij} = \begin{cases} -w_{8(j+m)+3 \rightarrow 8(j+m)+4} \otimes e_{8j+2}, & i = j - 3s; \\ 0, & \text{otherwise.} \end{cases}$$

If  $6s \leq j < 7s$ , then  $b_{ij} = 0$ .

If  $7s \leq j < 8s$ , then

$$b_{ij} = \begin{cases} -e_{8(j+m)+5} \otimes w_{8j+3 \rightarrow 8j+4}, & i = j - 3s; \\ 0, & \text{otherwise.} \end{cases}$$

If  $8s \leq j < 11s$ , then  $b_{ij} = 0$ .

If  $11s \leq j < 12s$ , then

$$b_{ij} = \begin{cases} e_{8(j+m)+6} \otimes e_{8j+5}, & i = j - 6s; \\ 0, & \text{otherwise.} \end{cases}$$

If  $12s \leq j < 14s$ , then  $b_{ij} = 0$ .

If  $14s \leq j < 15s$ , then

$$b_{ij} = \begin{cases} w_{8(j+m)+1 \rightarrow 8(j+m)+2} \otimes e_{8j+6}, & i = j - 8s; \\ 0, & \text{otherwise.} \end{cases}$$

If  $15s \leq j < 18s$ , then  $b_{ij} = 0$ .

If  $18s \leq j < 19s$ , then

$$b_{ij} = \begin{cases} e_{8(j+m+1)} \otimes e_{8j+7}, & i = j - 11s; \\ 0, & \text{otherwise.} \end{cases}$$

If  $19s \leq j < 20s$ , then  $b_{ij} = 0$ .

(4) If  $r_0 = 3$ , then  $\Omega^3(Z_t^{(13)})$  is described with  $(10s \times 18s)$  matrix, whose entries  $b_{ij}$  have the following form:

If  $0 \leq j < s$ , then

$$b_{ij} = \begin{cases} -w_{8(j+m)+2 \rightarrow 8(j+m)+3} \otimes e_{8j}, & i = j; \\ 0, & \text{otherwise.} \end{cases}$$

If  $s \leq j < 2s$ , then

$$b_{ij} = \begin{cases} -e_{8(j+m)+6} \otimes e_{8j}, & i = j; \\ 0, & \text{otherwise.} \end{cases}$$

If  $2s \leq j < 3s$ , then

$$b_{ij} = \begin{cases} w_{8(j+m)+3 \rightarrow 8(j+m)+4} \otimes w_{8j \rightarrow 8j+1}, & i = j; \\ 0, & \text{otherwise.} \end{cases}$$

If  $3s \leq j < 5s$ , then  $b_{ij} = 0$ .

If  $5s \leq j < 6s$ , then

$$b_{ij} = \begin{cases} -w_{8(j+m)+3 \rightarrow 8(j+m)+7} \otimes e_{8j+1}, & i = j - 3s; \\ -w_{8(j+m)+4 \rightarrow 8(j+m)+7} \otimes w_{8j+1 \rightarrow 8j+2}, & i = j - 2s; \\ -e_{8(j+m)+7} \otimes w_{8j+1 \rightarrow 8j+3}, & i = j - s; \\ 0, & \text{otherwise.} \end{cases}$$

If  $6s \leq j < 7s$ , then

$$b_{ij} = \begin{cases} -w_{8(j+m)+4 \rightarrow 8(j+m)+7} \otimes e_{8j+2}, & i = j - 3s; \\ -e_{8(j+m)+7} \otimes w_{8j+2 \rightarrow 8j+3}, & i = j - 2s; \\ 0, & \text{otherwise.} \end{cases}$$

If  $7s \leq j < 8s$ , then  $b_{ij} = 0$ .

If  $8s \leq j < 9s$ , then

$$b_{ij} = \begin{cases} -e_{8(j+m+1)} \otimes w_{8j+3 \rightarrow 8j+4}, & i = j - 3s; \\ 0, & \text{otherwise.} \end{cases}$$

If  $9s \leq j < 10s$ , then  $b_{ij} = 0$ .

If  $10s \leq j < 11s$ , then

$$b_{ij} = \begin{cases} e_{8(j+m)+7} \otimes e_{8j+5}, & i = j - 4s; \\ 0, & \text{otherwise.} \end{cases}$$

If  $11s \leq j < 12s$ , then  $b_{ij} = 0$ .

If  $12s \leq j < 13s$ , then

$$b_{ij} = \begin{cases} e_{8(j+m+1)} \otimes e_{8j+6}, & i = j - 5s; \\ 0, & \text{otherwise.} \end{cases}$$

If  $13s \leq j < 14s$ , then  $b_{ij} = 0$ .

If  $14s \leq j < 15s$ , then

$$b_{ij} = \begin{cases} -w_{8(j+m+1)+1 \rightarrow 8(j+m+1)+2} \otimes e_{8j+7}, & i = j - 6s; \\ 0, & \text{otherwise.} \end{cases}$$

If  $15s \leq j < 17s$ , then  $b_{ij} = 0$ .

If  $17s \leq j < 18s$ , then

$$b_{ij} = \begin{cases} e_{8(j+m+1)+5} \otimes e_{8j+7}, & i = j - 8s; \\ 0, & \text{otherwise.} \end{cases}$$

(5) If  $r_0 = 4$ , then  $\Omega^4(Z_t^{(13)})$  is described with  $(11s \times 19s)$  matrix, whose entries  $b_{ij}$  have the following form:

If  $0 \leq j < s$ , then

$$b_{ij} = \begin{cases} -e_{8(j+m-1)+7} \otimes e_{8j}, & i = j; \\ 0, & \text{otherwise.} \end{cases}$$

If  $s \leq j < 2s$ , then

$$b_{ij} = \begin{cases} -w_{8(j+m-1)+7 \rightarrow 8(j+m)} \otimes e_{8j}, & i = j - s; \\ -e_{8(j+m)} \otimes e_{8j}, & i = j; \\ 0, & \text{otherwise.} \end{cases}$$

If  $2s \leq j < 3s$ , then  $b_{ij} = 0$ .

If  $3s \leq j < 4s$ , then

$$b_{ij} = \begin{cases} -w_{8(j+m)+3 \rightarrow 8(j+m)+4} \otimes e_{8j+1}, & i = j - s; \\ 0, & \text{otherwise.} \end{cases}$$

If  $4s \leq j < 5s$ , then

$$b_{ij} = \begin{cases} -w_{8(j+m)+5 \rightarrow 8(j+m)+6} \otimes w_{8j+1 \rightarrow 8j+3}, & i = j; \\ e_{8(j+m)+6} \otimes w_{8j+1 \rightarrow 8j+4}, & i = j + s; \\ 0, & \text{otherwise.} \end{cases}$$

If  $5s \leq j < 6s$ , then

$$b_{ij} = \begin{cases} -e_{8(j+m)+5} \otimes w_{8j+2 \rightarrow 8j+3}, & i = j - s; \\ 0, & \text{otherwise.} \end{cases}$$

If  $6s \leq j < 7s$ , then  $b_{ij} = 0$ .

If  $7s \leq j < 8s$ , then

$$b_{ij} = \begin{cases} -w_{8(j+m)+1 \rightarrow 8(j+m)+2} \otimes w_{8j+3 \rightarrow 8j+4}, & i = j - s; \\ 0, & \text{otherwise.} \end{cases}$$

If  $8s \leq j < 9s$ , then

$$b_{ij} = \begin{cases} -e_{8(j+m)+6} \otimes w_{8j+3 \rightarrow 8j+4}, & i = j - 3s; \\ 0, & \text{otherwise.} \end{cases}$$

If  $9s \leq j < 10s$ , then  $b_{ij} = 0$ .

If  $10s \leq j < 11s$ , then

$$b_{ij} = \begin{cases} w_{8(j+m)+1 \rightarrow 8(j+m)+2} \otimes e_{8j+5}, & i = j - 3s; \\ 0, & \text{otherwise.} \end{cases}$$

If  $11s \leq j < 13s$ , then  $b_{ij} = 0$ .

If  $13s \leq j < 14s$ , then

$$b_{ij} = \begin{cases} w_{8(j+m)+2 \rightarrow 8(j+m)+3} \otimes e_{8j+6}, & i = j - 5s; \\ 0, & \text{otherwise.} \end{cases}$$

If  $14s \leq j < 15s$ , then  $b_{ij} = 0$ .

If  $15s \leq j < 16s$ , then

$$b_{ij} = \begin{cases} e_{8(j+m)+5} \otimes e_{8j+6}, & i = j - 6s; \\ 0, & \text{otherwise.} \end{cases}$$

If  $16s \leq j < 17s$ , then

$$b_{ij} = \begin{cases} -e_{8(j+m)+7} \otimes e_{8j+7}, & i = j - 6s; \\ 0, & \text{otherwise.} \end{cases}$$

If  $17s \leq j < 19s$ , then  $b_{ij} = 0$ .

(6) If  $r_0 = 5$ , then  $\Omega^5(Z_t^{(13)})$  is described with  $(11s \times 18s)$  matrix, whose entries  $b_{ij}$  have the following form:

If  $0 \leq j < s$ , then

$$b_{ij} = \begin{cases} w_{8(j+m)+1 \rightarrow 8(j+m)+2} \otimes e_{8j}, & i = j + 2s; \\ 0, & \text{otherwise.} \end{cases}$$

If  $s \leq j < 2s$ , then

$$b_{ij} = \begin{cases} -w_{8(j+m)+3 \rightarrow 8(j+m)+4} \otimes e_{8j}, & i = j; \\ 0, & \text{otherwise.} \end{cases}$$

If  $2s \leq j < 3s$ , then  $b_{ij} = 0$ .

If  $3s \leq j < 4s$ , then

$$b_{ij} = \begin{cases} -e_{8(j+m)+5} \otimes e_{8j}, & i = j - 3s; \\ 0, & \text{otherwise.} \end{cases}$$

If  $4s \leq j < 5s$ , then

$$b_{ij} = \begin{cases} -w_{8(j+m)+4 \rightarrow 8(j+m)+7} \otimes e_{8j+1}, & i = j - s; \\ -e_{8(j+m)+7} \otimes w_{8j+1 \rightarrow 8j+2}, & i = j; \\ 0, & \text{otherwise.} \end{cases}$$

If  $5s \leq j < 6s$ , then

$$b_{ij} = \begin{cases} -e_{8(j+m+1)} \otimes w_{8j+1 \rightarrow 8j+3}, & i = j; \\ 0, & \text{otherwise.} \end{cases}$$

If  $6s \leq j < 7s$ , then

$$b_{ij} = \begin{cases} -e_{8(j+m+1)} \otimes w_{8j+2 \rightarrow 8j+3}, & i = j - s; \\ 0, & \text{otherwise.} \end{cases}$$

If  $7s \leq j < 8s$ , then

$$b_{ij} = \begin{cases} e_{8(j+m)+7} \otimes w_{8j+3 \rightarrow 8j+4}, & i = j - s; \\ 0, & \text{otherwise.} \end{cases}$$

If  $8s \leq j < 9s$ , then  $b_{ij} = 0$ .

If  $9s \leq j < 10s$ , then

$$b_{ij} = \begin{cases} e_{8(j+m+1)} \otimes e_{8j+5}, & i = j - 2s; \\ 0, & \text{otherwise.} \end{cases}$$

If  $10s \leq j < 11s$ , then  $b_{ij} = 0$ .

If  $11s \leq j < 12s$ , then

$$b_{ij} = \begin{cases} e_{8(j+m)+7} \otimes e_{8j+6}, & i = j - 3s; \\ 0, & \text{otherwise.} \end{cases}$$

If  $12s \leq j < 13s$ , then  $b_{ij} = 0$ .

If  $13s \leq j < 14s$ , then

$$b_{ij} = \begin{cases} -w_{8(j+m+1)+2 \rightarrow 8(j+m+1)+3} \otimes e_{8j+7}, & i = j - 4s; \\ 0, & \text{otherwise.} \end{cases}$$

If  $14s \leq j < 15s$ , then

$$b_{ij} = \begin{cases} -e_{8(j+m+1)+6} \otimes e_{8j+7}, & i = j - 4s; \\ 0, & \text{otherwise.} \end{cases}$$

If  $15s \leq j < 18s$ , then  $b_{ij} = 0$ .

(7) If  $r_0 = 6$ , then  $\Omega^6(Z_t^{(13)})$  is described with  $(13s \times 19s)$  matrix, whose entries  $b_{ij}$  have the following form:

If  $0 \leq j < s$ , then

$$b_{ij} = \begin{cases} -e_{8(j+m-1)+7} \otimes e_{8j}, & i = j; \\ 0, & \text{otherwise.} \end{cases}$$

If  $s \leq j < 2s$ , then

$$b_{ij} = \begin{cases} -e_{8(j+m)} \otimes e_{8j}, & i = j; \\ 0, & \text{otherwise.} \end{cases}$$

If  $2s \leq j < 3s$ , then  $b_{ij} = 0$ .

If  $3s \leq j < 4s$ , then

$$b_{ij} = \begin{cases} -e_{8(j+m)+5} \otimes w_{8j+1 \rightarrow 8j+2}, & i = j; \\ 0, & \text{otherwise.} \end{cases}$$

If  $4s \leq j < 5s$ , then  $b_{ij} = 0$ .

If  $5s \leq j < 6s$ , then

$$b_{ij} = \begin{cases} -w_{8(j+m)+1 \rightarrow 8(j+m)+2} \otimes w_{8j+2 \rightarrow 8j+3}, & i = j; \\ 0, & \text{otherwise.} \end{cases}$$

If  $6s \leq j < 7s$ , then

$$b_{ij} = \begin{cases} -e_{8(j+m)+6} \otimes w_{8j+2 \rightarrow 8j+3}, & i = j - 2s; \\ 0, & \text{otherwise.} \end{cases}$$

If  $7s \leq j < 8s$ , then

$$b_{ij} = \begin{cases} w_{8(j+m)+2 \rightarrow 8(j+m)+3} \otimes w_{8j+3 \rightarrow 8j+4}, & i = j - s; \\ 0, & \text{otherwise.} \end{cases}$$

If  $8s \leq j < 10s$ , then  $b_{ij} = 0$ .

If  $10s \leq j < 11s$ , then

$$b_{ij} = \begin{cases} w_{8(j+m)+2 \rightarrow 8(j+m)+3} \otimes e_{8j+5}, & i = j - 3s; \\ 0, & \text{otherwise.} \end{cases}$$

If  $11s \leq j < 12s$ , then  $b_{ij} = 0$ .

If  $12s \leq j < 13s$ , then

$$b_{ij} = \begin{cases} e_{8(j+m)+5} \otimes e_{8j+5}, & i = j - 4s; \\ 0, & \text{otherwise.} \end{cases}$$

If  $13s \leq j < 14s$ , then

$$b_{ij} = \begin{cases} e_{8(j+m)+6} \otimes e_{8j+6}, & i = j - 3s; \\ 0, & \text{otherwise.} \end{cases}$$

If  $14s \leq j < 15s$ , then

$$b_{ij} = \begin{cases} w_{8(j+m)+3 \rightarrow 8(j+m)+4} \otimes e_{8j+6}, & i = j - 5s; \\ 0, & \text{otherwise.} \end{cases}$$

If  $15s \leq j < 16s$ , then  $b_{ij} = 0$ .

If  $16s \leq j < 17s$ , then

$$b_{ij} = \begin{cases} -e_{8(j+m)+7} \otimes e_{8j+7}, & i = j - 5s; \\ 0, & \text{otherwise.} \end{cases}$$

If  $17s \leq j < 18s$ , then

$$b_{ij} = \begin{cases} -w_{8(j+m)+7 \rightarrow 8(j+m)+1} \otimes e_{8j+7}, & i = j - 6s; \\ -e_{8(j+m)+1} \otimes e_{8j+7}, & i = j - 5s; \\ 0, & \text{otherwise.} \end{cases}$$

If  $18s \leq j < 19s$ , then  $b_{ij} = 0$ .

(8) If  $r_0 = 7$ , then  $\Omega^7(Z_t^{(13)})$  is described with  $(14s \times 16s)$  matrix, whose entries  $b_{ij}$  have the following form:

If  $0 \leq j < s$ , then

$$b_{ij} = \begin{cases} -w_{8(j+m)+2 \rightarrow 8(j+m)+3} \otimes e_{8j}, & i = j; \\ 0, & \text{otherwise.} \end{cases}$$

If  $s \leq j < 2s$ , then

$$b_{ij} = \begin{cases} -e_{8(j+m)+6} \otimes e_{8j}, & i = j + s; \\ 0, & \text{otherwise.} \end{cases}$$

If  $2s \leq j < 3s$ , then  $b_{ij} = 0$ .

If  $3s \leq j < 4s$ , then

$$b_{ij} = \begin{cases} -e_{8(j+m)+5} \otimes e_{8j}, & i = j; \\ 0, & \text{otherwise.} \end{cases}$$

If  $4s \leq j < 5s$ , then

$$b_{ij} = \begin{cases} -e_{8(j+m)+1} \otimes w_{8j+1 \rightarrow 8j+2}, & i = j + s; \\ 0, & \text{otherwise.} \end{cases}$$

If  $5s \leq j < 6s$ , then

$$b_{ij} = \begin{cases} e_{8(j+m)+7} \otimes w_{8j+2 \rightarrow 8j+3}, & i = j + s; \\ 0, & \text{otherwise.} \end{cases}$$

If  $6s \leq j < 7s$ , then

$$b_{ij} = \begin{cases} e_{8(j+m)+1} \otimes w_{8j+3 \rightarrow 8j+4}, & i = j + s; \\ 0, & \text{otherwise.} \end{cases}$$

If  $7s \leq j < 8s$ , then  $b_{ij} = 0$ .



If  $8s \leq j < 9s$ , then

$$b_{ij} = \begin{cases} e_{8(j+m)+7} \otimes e_{8j+5}, & i = j; \\ e_{8(j+m)+7} \otimes w_{8j+5 \rightarrow 8j+6}, & i = j + s; \\ 0, & \text{otherwise.} \end{cases}$$

If  $9s \leq j < 10s$ , then  $b_{ij} = 0$ .

If  $10s \leq j < 11s$ , then

$$b_{ij} = \begin{cases} -e_{8(j+m)+7} \otimes e_{8j+6}, & i = j - s; \\ 0, & \text{otherwise.} \end{cases}$$

If  $11s \leq j < 12s$ , then

$$b_{ij} = \begin{cases} w_{8(j+m)+7 \rightarrow 8(j+m+1)} \otimes e_{8j+6}, & i = j - 2s; \\ e_{8(j+m+1)} \otimes e_{8j+6}, & i = j - s; \\ 0, & \text{otherwise.} \end{cases}$$

If  $12s \leq j < 13s$ , then

$$b_{ij} = \begin{cases} w_{8(j+m+1)+1 \rightarrow 8(j+m+1)+2} \otimes e_{8j+7}, & i = j + s; \\ 0, & \text{otherwise.} \end{cases}$$

If  $13s \leq j < 14s$ , then

$$b_{ij} = \begin{cases} -w_{8(j+m+1)+3 \rightarrow 8(j+m+1)+4} \otimes e_{8j+7}, & i = j - s; \\ 0, & \text{otherwise.} \end{cases}$$

If  $14s \leq j < 15s$ , then  $b_{ij} = 0$ .

If  $15s \leq j < 16s$ , then

$$b_{ij} = \begin{cases} -e_{8(j+m+1)+5} \otimes e_{8j+7}, & i = j - 4s; \\ 0, & \text{otherwise.} \end{cases}$$

(9) If  $r_0 = 8$ , then  $\Omega^8(Z_t^{(13)})$  is described with  $(16s \times 16s)$  matrix, whose entries  $b_{ij}$  have the following form:

If  $0 \leq j < s$ , then

$$b_{ij} = \begin{cases} -e_{8(j+m-1)+7} \otimes e_{8j}, & i = j; \\ 0, & \text{otherwise.} \end{cases}$$

If  $s \leq j < 2s$ , then

$$b_{ij} = \begin{cases} -w_{8(j+m-1)+7 \rightarrow 8(j+m)} \otimes e_{8j}, & i = j - s; \\ -e_{8(j+m)} \otimes e_{8j}, & i = j + s; \\ 0, & \text{otherwise.} \end{cases}$$

If  $2s \leq j < 3s$ , then

$$b_{ij} = \begin{cases} -w_{8(j+m)+1 \rightarrow 8(j+m)+2} \otimes w_{8j+1 \rightarrow 8j+2}, & i = j + 3s; \\ 0, & \text{otherwise.} \end{cases}$$

If  $3s \leq j < 4s$ , then

$$b_{ij} = \begin{cases} -e_{8(j+m)+6} \otimes w_{8j+1 \rightarrow 8j+2}, & i = j + s; \\ 0, & \text{otherwise.} \end{cases}$$

If  $4s \leq j < 5s$ , then

$$b_{ij} = \begin{cases} w_{8(j+m)+2 \rightarrow 8(j+m)+3} \otimes w_{8j+2 \rightarrow 8j+3}, & i = j + 2s; \\ 0, & \text{otherwise.} \end{cases}$$

If  $5s \leq j < 6s$ , then

$$b_{ij} = \begin{cases} w_{8(j+m)+3 \rightarrow 8(j+m)+4} \otimes w_{8j+3 \rightarrow 8j+4}, & i = j + 2s; \\ 0, & \text{otherwise.} \end{cases}$$

If  $6s \leq j < 7s$ , then

$$b_{ij} = \begin{cases} e_{8(j+m)+5} \otimes w_{8j+3 \rightarrow 8j+4}, & i = j + 2s; \\ 0, & \text{otherwise.} \end{cases}$$

If  $7s \leq j < 8s$ , then  $b_{ij} = 0$ .

If  $8s \leq j < 9s$ , then

$$b_{ij} = \begin{cases} e_{8(j+m)+6} \otimes e_{8j+5}, & i = j + 2s; \\ 0, & \text{otherwise.} \end{cases}$$

If  $9s \leq j < 10s$ , then

$$b_{ij} = \begin{cases} w_{8(j+m)+3 \rightarrow 8(j+m)+4} \otimes e_{8j+5}, & i = j; \\ 0, & \text{otherwise.} \end{cases}$$

If  $10s \leq j < 11s$ , then  $b_{ij} = 0$ .

If  $11s \leq j < 12s$ , then

$$b_{ij} = \begin{cases} w_{8(j+m)+1 \rightarrow 8(j+m)+2} \otimes e_{8j+6}, & i = j + 2s; \\ 0, & \text{otherwise.} \end{cases}$$

If  $12s \leq j < 13s$ , then

$$b_{ij} = \begin{cases} e_{8(j+m)+5} \otimes e_{8j+6}, & i = j - s; \\ 0, & \text{otherwise.} \end{cases}$$

If  $13s \leq j < 14s$ , then

$$b_{ij} = \begin{cases} e_{8(j+m)+7} \otimes w_{8j+7 \rightarrow 8(j+1)}, & i = (j+1)_s; \\ -e_{8(j+m)+7} \otimes w_{8j+7 \rightarrow 8(j+1)}, & i = s + (j+1)_s; \\ -e_{8(j+m)+7} \otimes e_{8j+7}, & i = j + s; \\ 0, & \text{otherwise.} \end{cases}$$

If  $14s \leq j < 15s$ , then

$$b_{ij} = \begin{cases} -w_{8(j+m)+7 \rightarrow 8(j+m+1)} \otimes w_{8j+7 \rightarrow 8(j+1)}, & i = (j+1)_s; \\ w_{8(j+m)+7 \rightarrow 8(j+m+1)} \otimes w_{8j+7 \rightarrow 8(j+1)}, & i = s + (j+1)_s; \\ -e_{8(j+m+1)} \otimes e_{8j+7}, & i = j + s; \\ 0, & \text{otherwise.} \end{cases}$$

If  $15s \leq j < 16s$ , then  $b_{ij} = 0$ .

(10) If  $r_0 = 9$ , then  $\Omega^9(Z_t^{(13)})$  is described with  $(16s \times 14s)$  matrix, whose entries  $b_{ij}$  have the following form:

If  $0 \leq j < s$ , then

$$b_{ij} = \begin{cases} w_{8(j+m)+1 \rightarrow 8(j+m)+2} \otimes e_{8j}, & i = j + 3s; \\ 0, & \text{otherwise.} \end{cases}$$

If  $s \leq j < 2s$ , then

$$b_{ij} = \begin{cases} -w_{8(j+m)+3 \rightarrow 8(j+m)+4} \otimes e_{8j}, & i = j; \\ -w_{8(j+m)+1 \rightarrow 8(j+m)+4} \otimes e_{8j}, & i = j + 2s; \\ 0, & \text{otherwise.} \end{cases}$$

If  $2s \leq j < 3s$ , then

$$b_{ij} = \begin{cases} -w_{8(j+m)+5 \rightarrow 8(j+m)+6} \otimes e_{8j}, & i = j - 2s; \\ -e_{8(j+m)+6} \otimes e_{8j}, & i = j; \\ 0, & \text{otherwise.} \end{cases}$$

If  $3s \leq j < 4s$ , then

$$b_{ij} = \begin{cases} e_{8(j+m)+7} \otimes w_{8j+1 \rightarrow 8j+2}, & i = j + 2s; \\ 0, & \text{otherwise.} \end{cases}$$

If  $4s \leq j < 5s$ , then

$$b_{ij} = \begin{cases} e_{8(j+m+1)} \otimes w_{8j+2 \rightarrow 8j+3}, & i = j + 2s; \\ 0, & \text{otherwise.} \end{cases}$$

If  $5s \leq j < 6s$ , then

$$b_{ij} = \begin{cases} e_{8(j+m)+7} \otimes w_{8j+3 \rightarrow 8j+4}, & i = j + 2s; \\ 0, & \text{otherwise.} \end{cases}$$

If  $6s \leq j < 7s$ , then  $b_{ij} = 0$ .

If  $7s \leq j < 8s$ , then

$$b_{ij} = \begin{cases} -e_{8(j+m)+7} \otimes e_{8j+5}, & i = j + s; \\ e_{8(j+m)+7} \otimes w_{8j+5 \rightarrow 8j+6}, & i = j + 3s; \\ 0, & \text{otherwise.} \end{cases}$$

If  $8s \leq j < 9s$ , then

$$b_{ij} = \begin{cases} w_{8(j+m)+7 \rightarrow 8(j+m+1)} \otimes e_{8j+5}, & i = j; \\ e_{8(j+m+1)} \otimes e_{8j+5}, & i = j + s; \\ e_{8(j+m+1)} \otimes w_{8j+5 \rightarrow 8j+6}, & i = j + 3s; \\ 0, & \text{otherwise.} \end{cases}$$

If  $9s \leq j < 10s$ , then

$$b_{ij} = \begin{cases} -w_{8(j+m)+7 \rightarrow 8(j+m+1)} \otimes e_{8j+6}, & i = j + s; \\ -e_{8(j+m+1)} \otimes e_{8j+6}, & i = j + 2s; \\ 0, & \text{otherwise.} \end{cases}$$

If  $10s \leq j < 11s$ , then

$$b_{ij} = \begin{cases} -w_{8(j+m+1)+2 \rightarrow 8(j+m+1)+3} \otimes e_{8j+7}, & i = j + 2s; \\ 0, & \text{otherwise.} \end{cases}$$

If  $11s \leq j < 12s$ , then

$$b_{ij} = \begin{cases} -e_{8(j+m+1)+6} \otimes w_{8j+7 \rightarrow 8(j+1)}, & i = 2s + (j + 1)s; \\ -e_{8(j+m+1)+6} \otimes e_{8j+7}, & i = j + 3s; \\ 0, & \text{otherwise.} \end{cases}$$

If  $12s \leq j < 13s$ , then  $b_{ij} = 0$ .

If  $13s \leq j < 14s$ , then

$$b_{ij} = \begin{cases} -e_{8(j+m+1)+5} \otimes w_{8j+7 \rightarrow 8(j+1)}, & i = (j + 1)s; \\ -e_{8(j+m+1)+5} \otimes e_{8j+7}, & i = j + 2s; \\ 0, & \text{otherwise.} \end{cases}$$

(11) If  $r_0 = 10$ , then  $\Omega^{10}(Z_t^{(13)})$  is described with  $(19s \times 13s)$  matrix, whose entries  $b_{ij}$  have the following form:

If  $0 \leq j < s$ , then

$$b_{ij} = \begin{cases} -e_{8(j+m)} \otimes e_{8j}, & i = j + s; \\ 0, & \text{otherwise.} \end{cases}$$

If  $s \leq j < 2s$ , then

$$b_{ij} = \begin{cases} e_{8(j+m-1)+7} \otimes e_{8j}, & i = j - s; \\ 0, & \text{otherwise.} \end{cases}$$

If  $2s \leq j < 3s$ , then

$$b_{ij} = \begin{cases} w_{8(j+m)+2 \rightarrow 8(j+m)+3} \otimes w_{8j+1 \rightarrow 8j+2}, & i = j + 3s; \\ 0, & \text{otherwise.} \end{cases}$$

If  $3s \leq j < 4s$ , then

$$b_{ij} = \begin{cases} w_{8(j+m)+3 \rightarrow 8(j+m)+4} \otimes w_{8j+2 \rightarrow 8j+3}, & i = j + 3s; \\ 0, & \text{otherwise.} \end{cases}$$

If  $4s \leq j < 5s$ , then

$$b_{ij} = \begin{cases} e_{8(j+m)+5} \otimes w_{8j+2 \rightarrow 8j+3}, & i = j + 3s; \\ 0, & \text{otherwise.} \end{cases}$$

If  $5s \leq j < 6s$ , then

$$b_{ij} = \begin{cases} e_{8(j+m)+6} \otimes w_{8j+3 \rightarrow 8j+4}, & i = j + 4s; \\ 0, & \text{otherwise.} \end{cases}$$

If  $6s \leq j < 7s$ , then  $b_{ij} = 0$ .

If  $7s \leq j < 8s$ , then

$$b_{ij} = \begin{cases} w_{8(j+m)+1 \rightarrow 8(j+m)+2} \otimes e_{8j+5}, & i = j + 5s; \\ 0, & \text{otherwise.} \end{cases}$$

If  $8s \leq j < 9s$ , then

$$b_{ij} = \begin{cases} e_{8(j+m)+5} \otimes e_{8j+5}, & i = j + 2s; \\ e_{8(j+m)+5} \otimes w_{8j+5 \rightarrow 8j+6}, & i = j + 7s; \\ 0, & \text{otherwise.} \end{cases}$$

If  $9s \leq j < 10s$ , then

$$b_{ij} = \begin{cases} -w_{8(j+m)+2 \rightarrow 8(j+m)+3} \otimes e_{8j+6}, & i = j + 4s; \\ 0, & \text{otherwise.} \end{cases}$$

If  $10s \leq j < 11s$ , then

$$b_{ij} = \begin{cases} -e_{8(j+m)+6} \otimes e_{8j+6}, & i = j + 4s; \\ -w_{8(j+m)+5 \rightarrow 8(j+m)+6} \otimes e_{8j+6}, & i = j + 5s; \\ 0, & \text{otherwise.} \end{cases}$$

If  $11s \leq j < 12s$ , then

$$b_{ij} = \begin{cases} -e_{8(j+m)+7} \otimes e_{8j+7}, & i = j + 5s; \\ 0, & \text{otherwise.} \end{cases}$$

If  $12s \leq j < 13s$ , then

$$b_{ij} = \begin{cases} w_{8(j+m)+7 \rightarrow 8(j+m)+1} \otimes w_{8j+7 \rightarrow 8(j+1)}, & i = (j+1)s; \\ e_{8(j+m)+1} \otimes w_{8j+7 \rightarrow 8(j+1)}, & i = s + (j+1)s; \\ -e_{8(j+m)+1} \otimes w_{8j+7 \rightarrow 8(j+1)}, & i = 2s + (j+1)s; \\ -w_{8(j+m)+7 \rightarrow 8(j+m)+1} \otimes e_{8j+7}, & i = j + 4s; \\ -e_{8(j+m)+1} \otimes e_{8j+7}, & i = j + 6s; \\ 0, & \text{otherwise.} \end{cases}$$

(12) If  $r_0 = 11$ , then  $\Omega^{11}(Z_t^{(13)})$  is described with  $(18s \times 11s)$  matrix, whose entries  $b_{ij}$  have the following form:

If  $0 \leq j < s$ , then

$$b_{ij} = \begin{cases} -w_{8(j+m)+2 \rightarrow 8(j+m)+3} \otimes e_{8j}, & i = j; \\ 0, & \text{otherwise.} \end{cases}$$

If  $s \leq j < 2s$ , then

$$b_{ij} = \begin{cases} -e_{8(j+m)+5} \otimes e_{8j}, & i = j + 3s; \\ 0, & \text{otherwise.} \end{cases}$$

If  $2s \leq j < 3s$ , then

$$b_{ij} = \begin{cases} e_{8(j+m+1)} \otimes w_{8j+1 \rightarrow 8j+2}, & i = j + 4s; \\ 0, & \text{otherwise.} \end{cases}$$

If  $3s \leq j < 4s$ , then

$$b_{ij} = \begin{cases} e_{8(j+m)+7} \otimes w_{8j+2 \rightarrow 8j+3}, & i = j + 4s; \\ 0, & \text{otherwise.} \end{cases}$$

If  $4s \leq j < 5s$ , then

$$b_{ij} = \begin{cases} e_{8(j+m+1)} \otimes w_{8j+3 \rightarrow 8j+4}, & i = j + 5s; \\ 0, & \text{otherwise.} \end{cases}$$

If  $5s \leq j < 6s$ , then

$$b_{ij} = \begin{cases} -w_{8(j+m+1) \rightarrow 8(j+m+1)+1} \otimes e_{8j+4}, & i = j + 4s; \\ 0, & \text{otherwise.} \end{cases}$$

If  $6s \leq j < 7s$ , then

$$b_{ij} = \begin{cases} -w_{8(j+m)+7 \rightarrow 8(j+m+1)} \otimes e_{8j+5}, & i = j + 4s; \\ -e_{8(j+m+1)} \otimes e_{8j+5}, & i = j + 5s; \\ w_{8(j+m)+7 \rightarrow 8(j+m+1)} \otimes w_{8j+5 \rightarrow 8j+6}, & i = j + 6s; \\ e_{8(j+m+1)} \otimes w_{8j+5 \rightarrow 8j+6}, & i = j + 7s; \\ 0, & \text{otherwise.} \end{cases}$$

If  $7s \leq j < 8s$ , then

$$b_{ij} = \begin{cases} -e_{8(j+m)+7} \otimes e_{8j+6}, & i = j + 5s; \\ 0, & \text{otherwise.} \end{cases}$$

If  $8s \leq j < 9s$ , then

$$b_{ij} = \begin{cases} w_{8(j+m+1)+1 \rightarrow 8(j+m+1)+2} \otimes w_{8j+7 \rightarrow 8(j+1)}, & i = 3s + (j+1)s; \\ w_{8(j+m+1)+1 \rightarrow 8(j+m+1)+2} \otimes e_{8j+7}, & i = j + 9s; \\ 0, & \text{otherwise.} \end{cases}$$

If  $9s \leq j < 10s$ , then

$$b_{ij} = \begin{cases} -w_{8(j+m+1)+1 \rightarrow 8(j+m+1)+4} \otimes w_{8j+7 \rightarrow 8(j+1)}, & i = 3s + (j+1)_s; \\ -w_{8(j+m+1)+3 \rightarrow 8(j+m+1)+4} \otimes e_{8j+7}, & i = j + 6s; \\ -w_{8(j+m+1)+1 \rightarrow 8(j+m+1)+4} \otimes e_{8j+7}, & i = j + 8s; \\ 0, & \text{otherwise.} \end{cases}$$

If  $10s \leq j < 11s$ , then

$$b_{ij} = \begin{cases} e_{8(j+m+1)+6} \otimes w_{8j+7 \rightarrow 8(j+1)}, & i = s + (j+1)_s; \\ w_{8(j+m+1)+5 \rightarrow 8(j+m+1)+6} \otimes w_{8j+7 \rightarrow 8(j+1)}, & i = 4s + (j+1)_s; \\ -w_{8(j+m+1)+5 \rightarrow 8(j+m+1)+6} \otimes e_{8j+7}, & i = j + 4s; \\ -e_{8(j+m+1)+6} \otimes e_{8j+7}, & i = j + 6s; \\ 0, & \text{otherwise.} \end{cases}$$

(13) If  $r_0 = 12$ , then  $\Omega^{12}(Z_t^{(13)})$  is described with  $(19s \times 11s)$  matrix, whose entries  $b_{ij}$  have the following form:

If  $0 \leq j < s$ , then

$$b_{ij} = \begin{cases} -e_{8(j+m)} \otimes e_{8j}, & i = j + s; \\ -w_{8(j+m-1)+7 \rightarrow 8(j+m)} \otimes e_{8j}, & i = j + 2s; \\ 0, & \text{otherwise.} \end{cases}$$

If  $s \leq j < 2s$ , then

$$b_{ij} = \begin{cases} w_{8(j+m)+3 \rightarrow 8(j+m)+4} \otimes w_{8j+1 \rightarrow 8j+2}, & i = j + 3s; \\ w_{8(j+m)+1 \rightarrow 8(j+m)+4} \otimes w_{8j+1 \rightarrow 8j+4}, & i = j + 8s; \\ 0, & \text{otherwise.} \end{cases}$$

If  $2s \leq j < 3s$ , then

$$b_{ij} = \begin{cases} e_{8(j+m)+5} \otimes w_{8j+1 \rightarrow 8j+2}, & i = j + 3s; \\ 0, & \text{otherwise.} \end{cases}$$

If  $3s \leq j < 4s$ , then

$$b_{ij} = \begin{cases} e_{8(j+m)+6} \otimes w_{8j+2 \rightarrow 8j+3}, & i = j + 4s; \\ w_{8(j+m)+5 \rightarrow 8(j+m)+6} \otimes w_{8j+2 \rightarrow 8j+4}, & i = j + 5s; \\ 0, & \text{otherwise.} \end{cases}$$

If  $4s \leq j < 5s$ , then  $b_{ij} = 0$ .

If  $5s \leq j < 6s$ , then

$$b_{ij} = \begin{cases} -w_{8(j+m)+1 \rightarrow 8(j+m)+2} \otimes e_{8j+4}, & i = j + 4s; \\ 0, & \text{otherwise.} \end{cases}$$

If  $6s \leq j < 7s$ , then

$$b_{ij} = \begin{cases} -w_{8(j+m)+2 \rightarrow 8(j+m)+3} \otimes e_{8j+5}, & i = j + 4s; \\ w_{8(j+m)+1 \rightarrow 8(j+m)+3} \otimes w_{8j+5 \rightarrow 8j+6}, & i = j + 9s; \\ 0, & \text{otherwise.} \end{cases}$$

If  $7s \leq j < 8s$ , then

$$b_{ij} = \begin{cases} -e_{8(j+m)+6} \otimes e_{8j+5}, & i = j + 4s; \\ -w_{8(j+m)+5 \rightarrow 8(j+m)+6} \otimes e_{8j+5}, & i = j + 5s; \\ e_{8(j+m)+6} \otimes w_{8j+5 \rightarrow 8j+6}, & i = j + 6s; \\ 0, & \text{otherwise.} \end{cases}$$

If  $8s \leq j < 9s$ , then

$$b_{ij} = \begin{cases} -w_{8(j+m)+3 \rightarrow 8(j+m)+4} \otimes e_{8j+6}, & i = j + 6s; \\ 0, & \text{otherwise.} \end{cases}$$

If  $9s \leq j < 10s$ , then

$$b_{ij} = \begin{cases} -e_{8(j+m+1)} \otimes e_{8j+7}, & i = j + 8s; \\ 0, & \text{otherwise.} \end{cases}$$

If  $10s \leq j < 11s$ , then

$$b_{ij} = \begin{cases} e_{8(j+m)+7} \otimes w_{8j+7 \rightarrow 8(j+1)}, & i = (j+1)_s; \\ e_{8(j+m)+7} \otimes e_{8j+7}, & i = j + 6s; \\ 0, & \text{otherwise.} \end{cases}$$

(14) If  $r_0 = 13$ , then  $\Omega^{13}(Z_t^{(13)})$  is described with  $(18s \times 10s)$  matrix, whose entries  $b_{ij}$  have the following form:

If  $0 \leq j < s$ , then

$$b_{ij} = \begin{cases} w_{8(j+m)+2 \rightarrow 8(j+m)+4} \otimes e_{8j}, & i = j; \\ -w_{8(j+m)+3 \rightarrow 8(j+m)+4} \otimes e_{8j}, & i = j + s; \\ 0, & \text{otherwise.} \end{cases}$$

If  $s \leq j < 2s$ , then

$$b_{ij} = \begin{cases} -e_{8(j+m)+6} \otimes e_{8j}, & i = j + s; \\ -w_{8(j+m)+5 \rightarrow 8(j+m)+6} \otimes e_{8j}, & i = j + 2s; \\ 0, & \text{otherwise.} \end{cases}$$

If  $2s \leq j < 3s$ , then

$$b_{ij} = \begin{cases} e_{8(j+m)+7} \otimes w_{8j+1 \rightarrow 8j+2}, & i = j + 3s; \\ e_{8(j+m)+7} \otimes w_{8j+1 \rightarrow 8j+3}, & i = j + 4s; \\ 0, & \text{otherwise.} \end{cases}$$

If  $3s \leq j < 4s$ , then

$$b_{ij} = \begin{cases} e_{8(j+m+1)} \otimes w_{8j+2 \rightarrow 8j+3}, & i = j + 4s; \\ 0, & \text{otherwise.} \end{cases}$$

If  $4s \leq j < 5s$ , then

$$b_{ij} = \begin{cases} -w_{8(j+m+1) \rightarrow 8(j+m+1)+1} \otimes e_{8j+3}, & i = j + 3s; \\ 0, & \text{otherwise.} \end{cases}$$



If  $5s \leq j < 6s$ , then

$$b_{ij} = \begin{cases} -e_{8(j+m+1)+2} \otimes w_{8j+4 \rightarrow 8(j+1)}, & i = (j+1)_s; \\ -e_{8(j+m+1)+2} \otimes w_{8j+4 \rightarrow 8j+7}, & i = j+8s; \\ 0, & \text{otherwise.} \end{cases}$$

If  $6s \leq j < 7s$ , then

$$b_{ij} = \begin{cases} -e_{8(j+m)+7} \otimes e_{8j+5}, & i = j+3s; \\ -e_{8(j+m)+7} \otimes w_{8j+5 \rightarrow 8j+6}, & i = j+5s; \\ 0, & \text{otherwise.} \end{cases}$$

If  $7s \leq j < 8s$ , then

$$b_{ij} = \begin{cases} -e_{8(j+m+1)} \otimes e_{8j+6}, & i = j+5s; \\ 0, & \text{otherwise.} \end{cases}$$

If  $8s \leq j < 9s$ , then

$$b_{ij} = \begin{cases} -w_{8(j+m+1)+2 \rightarrow 8(j+m+1)+3} \otimes w_{8j+7 \rightarrow 8(j+1)}, & i = (j+1)_s; \\ -w_{8(j+m+1)+2 \rightarrow 8(j+m+1)+3} \otimes e_{8j+7}, & i = j+5s; \\ 0, & \text{otherwise.} \end{cases}$$

If  $9s \leq j < 10s$ , then

$$b_{ij} = \begin{cases} -e_{8(j+m+1)+5} \otimes e_{8j+7}, & i = j+8s; \\ 0, & \text{otherwise.} \end{cases}$$

(15) If  $r_0 = 14$ , then  $\Omega^{14}(Z_t^{(13)})$  is described with  $(20s \times 8s)$  matrix, whose entries  $b_{ij}$  have the following form:

If  $0 \leq j < s$ , then

$$b_{ij} = \begin{cases} e_{8(j+m-1)+7} \otimes e_{8j}, & i = j; \\ 0, & \text{otherwise.} \end{cases}$$

If  $s \leq j < 2s$ , then

$$b_{ij} = \begin{cases} e_{8(j+m)+6} \otimes w_{8j+1 \rightarrow 8j+2}, & i = j+5s; \\ w_{8(j+m)+5 \rightarrow 8(j+m)+6} \otimes w_{8j+1 \rightarrow 8j+3}, & i = j+6s; \\ 0, & \text{otherwise.} \end{cases}$$

If  $2s \leq j < 3s$ , then  $b_{ij} = 0$ .

If  $3s \leq j < 4s$ , then

$$b_{ij} = \begin{cases} -w_{8(j+m)+1 \rightarrow 8(j+m)+2} \otimes e_{8j+3}, & i = j+5s; \\ -e_{8(j+m)+2} \otimes w_{8j+3 \rightarrow 8j+4}, & i = j+6s; \\ 0, & \text{otherwise.} \end{cases}$$

If  $4s \leq j < 5s$ , then  $b_{ij} = 0$ .

If  $5s \leq j < 6s$ , then

$$b_{ij} = \begin{cases} -w_{8(j+m)+3 \rightarrow 8(j+m)+4} \otimes e_{8j+5}, & i = j + 7s; \\ -w_{8(j+m)+2 \rightarrow 8(j+m)+4} \otimes w_{8j+5 \rightarrow 8j+6}, & i = j + 9s; \\ 0, & \text{otherwise.} \end{cases}$$

If  $6s \leq j < 7s$ , then

$$b_{ij} = \begin{cases} -e_{8(j+m)+5} \otimes e_{8j+6}, & i = j + 10s; \\ 0, & \text{otherwise.} \end{cases}$$

If  $7s \leq j < 8s$ , then

$$b_{ij} = \begin{cases} -e_{8(j+m+1)} \otimes w_{8j+7 \rightarrow 8(j+1)}, & i = s + (j + 1)s; \\ -e_{8(j+m+1)} \otimes e_{8j+7}, & i = j + 11s; \\ -w_{8(j+m)+7 \rightarrow 8(j+m+1)} \otimes e_{8j+7}, & i = j + 12s; \\ 0, & \text{otherwise.} \end{cases}$$

(16) If  $r_0 = 15$ , then  $\Omega^{15}(Z_t^{(13)})$  is described with  $(18s \times 9s)$  matrix, whose entries  $b_{ij}$  have the following form:

If  $0 \leq j < s$ , then

$$b_{ij} = \begin{cases} w_{8(j+m)+3 \rightarrow 8(j+m)+7} \otimes e_{8j}, & i = j; \\ -w_{8(j+m)+5 \rightarrow 8(j+m)+7} \otimes e_{8j}, & i = j + 4s; \\ e_{8(j+m)+7} \otimes w_{8j \rightarrow 8j+1}, & i = j + 5s; \\ 0, & \text{otherwise.} \end{cases}$$

If  $s \leq j < 2s$ , then

$$b_{ij} = \begin{cases} e_{8(j+m+1)} \otimes w_{8j+1 \rightarrow 8j+2}, & i = j + 6s; \\ e_{8(j+m+1)} \otimes w_{8j+1 \rightarrow 8j+3}, & i = j + 7s; \\ 0, & \text{otherwise.} \end{cases}$$

If  $2s \leq j < 3s$ , then

$$b_{ij} = \begin{cases} -e_{8(j+m+1)+1} \otimes w_{8j+2 \rightarrow 8(j+1)}, & i = 3s + (j + 1)s; \\ -w_{8(j+m+1) \rightarrow 8(j+m+1)+1} \otimes w_{8j+2 \rightarrow 8j+3}, & i = j + 6s; \\ 0, & \text{otherwise.} \end{cases}$$

If  $3s \leq j < 4s$ , then

$$b_{ij} = \begin{cases} w_{8(j+m+1)+1 \rightarrow 8(j+m+1)+2} \otimes w_{8j+3 \rightarrow 8(j+1)}, & i = 3s + (j + 1)s; \\ w_{8(j+m+1) \rightarrow 8(j+m+1)+2} \otimes e_{8j+3}, & i = j + 5s; \\ 0, & \text{otherwise.} \end{cases}$$

If  $4s \leq j < 5s$ , then

$$b_{ij} = \begin{cases} w_{8(j+m)+7 \rightarrow 8(j+m+1)+3} \otimes e_{8j+4}, & i = j + 5s; \\ w_{8(j+m+1)+2 \rightarrow 8(j+m+1)+3} \otimes w_{8j+4 \rightarrow 8j+7}, & i = j + 10s; \\ 0, & \text{otherwise.} \end{cases}$$

If  $5s \leq j < 6s$ , then

$$b_{ij} = \begin{cases} -e_{8(j+m+1)} \otimes e_{8j+5}, & i = j + 6s; \\ -e_{8(j+m+1)} \otimes w_{8j+5 \rightarrow 8j+6}, & i = j + 7s; \\ -w_{8(j+m)+7 \rightarrow 8(j+m+1)} \otimes w_{8j+5 \rightarrow 8j+6}, & i = j + 8s; \\ 0, & \text{otherwise.} \end{cases}$$

If  $6s \leq j < 7s$ , then

$$b_{ij} = \begin{cases} -e_{8(j+m+1)+5} \otimes w_{8j+6 \rightarrow 8(j+1)}, & i = 4s + (j + 1)_s; \\ w_{8(j+m+1) \rightarrow 8(j+m+1)+5} \otimes e_{8j+6}, & i = j + 6s; \\ w_{8(j+m)+7 \rightarrow 8(j+m+1)+5} \otimes e_{8j+6}, & i = j + 7s; \\ 0, & \text{otherwise.} \end{cases}$$

If  $7s \leq j < 8s$ , then

$$b_{ij} = \begin{cases} w_{8(j+m+1)+2 \rightarrow 8(j+m+1)+4} \otimes e_{8j+7}, & i = j + 7s; \\ -w_{8(j+m+1)+3 \rightarrow 8(j+m+1)+4} \otimes e_{8j+7}, & i = j + 8s; \\ 0, & \text{otherwise.} \end{cases}$$

If  $8s \leq j < 9s$ , then

$$b_{ij} = \begin{cases} -w_{8(j+m+1)+5 \rightarrow 8(j+m+1)+6} \otimes w_{8j+7 \rightarrow 8(j+1)}, & i = 4s + (j + 1)_s; \\ -e_{8(j+m+1)+6} \otimes e_{8j+7}, & i = j + 8s; \\ -w_{8(j+m+1)+5 \rightarrow 8(j+m+1)+6} \otimes e_{8j+7}, & i = j + 9s; \\ 0, & \text{otherwise.} \end{cases}$$

(17) If  $r_0 = 16$ , then  $\Omega^{16}(Z_t^{(13)})$  is described with  $(19s \times 8s)$  matrix, whose entries  $b_{ij}$  have the following form:

If  $0 \leq j < s$ , then

$$b_{ij} = \begin{cases} e_{8(j+m)} \otimes e_{8j}, & i = j + s; \\ w_{8(j+m-1)+7 \rightarrow 8(j+m)} \otimes e_{8j}, & i = j + 2s; \\ 0, & \text{otherwise.} \end{cases}$$

If  $s \leq j < 2s$ , then

$$b_{ij} = \begin{cases} e_{8(j+m)+1} \otimes w_{8j+1 \rightarrow 8j+2}, & i = j + 5s; \\ 0, & \text{otherwise.} \end{cases}$$

If  $2s \leq j < 3s$ , then  $b_{ij} = 0$ .

If  $3s \leq j < 4s$ , then

$$b_{ij} = \begin{cases} w_{8(j+m)+2 \rightarrow 8(j+m)+3} \otimes e_{8j+3}, & i = j + 4s; \\ 0, & \text{otherwise.} \end{cases}$$

If  $4s \leq j < 5s$ , then

$$b_{ij} = \begin{cases} w_{8(j+m)+3 \rightarrow 8(j+m)+4} \otimes e_{8j+4}, & i = j + 5s; \\ 0, & \text{otherwise.} \end{cases}$$

If  $5s \leq j < 6s$ , then

$$b_{ij} = \begin{cases} -e_{8(j+m)+5} \otimes e_{8j+5}, & i = j + 7s; \\ 0, & \text{otherwise.} \end{cases}$$

If  $6s \leq j < 7s$ , then

$$b_{ij} = \begin{cases} e_{8(j+m)+6} \otimes e_{8j+6}, & i = j + 8s; \\ w_{8(j+m)+5 \rightarrow 8(j+m)+6} \otimes e_{8j+6}, & i = j + 9s; \\ 0, & \text{otherwise.} \end{cases}$$

If  $7s \leq j < 8s$ , then

$$b_{ij} = \begin{cases} e_{8(j+m)+7} \otimes e_{8j+7}, & i = j + 9s; \\ 0, & \text{otherwise.} \end{cases}$$

(18) If  $r_0 = 17$ , then  $\Omega^{17}(Z_t^{(13)})$  is described with  $(18s \times 8s)$  matrix, whose entries  $b_{ij}$  have the following form:

If  $0 \leq j < s$ , then

$$b_{ij} = \begin{cases} w_{8(j+m)+6 \rightarrow 8(j+m)+1} \otimes e_{8j}, & i = j + 2s; \\ w_{8(j+m)+5 \rightarrow 8(j+m)+1} \otimes e_{8j}, & i = j + 3s; \\ e_{8(j+m)+1} \otimes w_{8j \rightarrow 8j+1}, & i = j + 5s; \\ -w_{8(j+m)+7 \rightarrow 8(j+m)+1} \otimes w_{8j \rightarrow 8j+3}, & i = j + 7s; \\ 0, & \text{otherwise.} \end{cases}$$

If  $s \leq j < 2s$ , then

$$b_{ij} = \begin{cases} -w_{8(j+m)+1 \rightarrow 8(j+m)+1} \otimes e_{8j+1}, & i = j + 4s; \\ w_{8(j+m)+7 \rightarrow 8(j+m)+1} \otimes w_{8j+1 \rightarrow 8j+3}, & i = j + 6s; \\ 0, & \text{otherwise.} \end{cases}$$

If  $2s \leq j < 3s$ , then

$$b_{ij} = \begin{cases} e_{8(j+m)+2} \otimes w_{8j+2 \rightarrow 8(j+1)}, & i = (j+1)_s; \\ -w_{8(j+m)+7 \rightarrow 8(j+m)+2} \otimes w_{8j+2 \rightarrow 8j+3}, & i = j + 5s; \\ 0, & \text{otherwise.} \end{cases}$$

If  $3s \leq j < 4s$ , then

$$b_{ij} = \begin{cases} -w_{8(j+m)+2 \rightarrow 8(j+m)+3} \otimes w_{8j+3 \rightarrow 8(j+1)}, & i = (j+1)_s; \\ w_{8(j+m)+7 \rightarrow 8(j+m)+3} \otimes e_{8j+3}, & i = j + 4s; \\ 0, & \text{otherwise.} \end{cases}$$

If  $4s \leq j < 5s$ , then

$$b_{ij} = \begin{cases} w_{8(j+m)+1 \rightarrow 8(j+m)+4} \otimes e_{8j+4}, & i = j + 4s; \\ w_{8(j+m)+3 \rightarrow 8(j+m)+4} \otimes w_{8j+4 \rightarrow 8j+7}, & i = j + 9s; \\ 0, & \text{otherwise.} \end{cases}$$

If  $5s \leq j < 6s$ , then

$$b_{ij} = \begin{cases} -e_{8(j+m+1)+5} \otimes w_{8j+5 \rightarrow 8(j+1)}, & i = 3s + (j+1)_s; \\ w_{8(j+m)+7 \rightarrow 8(j+m+1)+5} \otimes e_{8j+5}, & i = j + 5s; \\ w_{8(j+m)+7 \rightarrow 8(j+m+1)+5} \otimes w_{8j+5 \rightarrow 8j+6}, & i = j + 6s; \\ 0, & \text{otherwise.} \end{cases}$$

If  $6s \leq j < 7s$ , then

$$b_{ij} = \begin{cases} e_{8(j+m+1)+6} \otimes w_{8j+6 \rightarrow 8(j+1)}, & i = 2s + (j+1)_s; \\ w_{8(j+m+1)+5 \rightarrow 8(j+m+1)+6} \otimes w_{8j+6 \rightarrow 8(j+1)}, & i = 3s + (j+1)_s; \\ -w_{8(j+m)+7 \rightarrow 8(j+m+1)+6} \otimes e_{8j+6}, & i = j + 5s; \\ 0, & \text{otherwise.} \end{cases}$$

If  $7s \leq j < 8s$ , then

$$b_{ij} = \begin{cases} -e_{8(j+m+1)+7} \otimes w_{8j+7 \rightarrow 8(j+1)+5}, & i = 10s + (j+1)_s; \\ -e_{8(j+m+1)+7} \otimes w_{8j+7 \rightarrow 8(j+1)+6}, & i = 11s + (j+1)_s; \\ w_{8(j+m+1)+3 \rightarrow 8(j+m+1)+7} \otimes e_{8j+7}, & i = j + 6s; \\ -w_{8(j+m+1)+4 \rightarrow 8(j+m+1)+7} \otimes e_{8j+7}, & i = j + 8s; \\ 0, & \text{otherwise.} \end{cases}$$

(19) If  $r_0 = 18$ , then  $\Omega^{18}(Z_t^{(13)})$  is described with  $(19s \times 9s)$  matrix, whose entries  $b_{ij}$  have the following form:

If  $s \leq j < 2s$ , then

$$b_{ij} = \begin{cases} w_{8(j+m-1)+7 \rightarrow 8(j+m)+5} \otimes e_{8j}, & i = j - s; \\ e_{8(j+m)+5} \otimes w_{8j \rightarrow 8j+1}, & i = j + 2s; \\ 0, & \text{otherwise.} \end{cases}$$

If  $2s \leq j < 3s$ , then

$$b_{ij} = \begin{cases} w_{8(j+m)+1 \rightarrow 8(j+m)+2} \otimes e_{8j+1}, & i = j + 2s; \\ e_{8(j+m)+2} \otimes w_{8j+1 \rightarrow 8j+2}, & i = j + 3s; \\ 0, & \text{otherwise.} \end{cases}$$

If  $3s \leq j < 4s$ , then  $b_{ij} = 0$ .

If  $4s \leq j < 5s$ , then

$$b_{ij} = \begin{cases} -w_{8(j+m)+3 \rightarrow 8(j+m)+4} \otimes e_{8j+3}, & i = j + 3s; \\ 0, & \text{otherwise.} \end{cases}$$

If  $5s \leq j < 6s$ , then

$$b_{ij} = \begin{cases} w_{8(j+m)+4 \rightarrow 8(j+m)+7} \otimes e_{8j+4}, & i = j + 3s; \\ 0, & \text{otherwise.} \end{cases}$$

If  $6s \leq j < 7s$ , then

$$b_{ij} = \begin{cases} -e_{8(j+m)+6} \otimes e_{8j+5}, & i = j + 5s; \\ 0, & \text{otherwise.} \end{cases}$$

If  $7s \leq j < 8s$ , then

$$b_{ij} = \begin{cases} -e_{8(j+m)+7} \otimes w_{8j+6 \rightarrow 8(j+1)}, & i = (j+1)_s; \\ w_{8(j+m)+4 \rightarrow 8(j+m)+7} \otimes e_{8j+6}, & i = j+7s; \\ 0, & \text{otherwise.} \end{cases}$$

If  $8s \leq j < 9s$ , then

$$b_{ij} = \begin{cases} -w_{8(j+m)+7 \rightarrow 8(j+m)+1} \otimes w_{8j+7 \rightarrow 8(j+1)}, & i = (j+1)_s; \\ -e_{8(j+m)+1} \otimes e_{8j+7}, & i = j+9s; \\ 0, & \text{otherwise.} \end{cases}$$

(20) If  $r_0 = 19$ , then  $\Omega^{19}(Z_t^{(13)})$  is described with  $(16s \times 8s)$  matrix, whose entries  $b_{ij}$  have the following form:

If  $0 \leq j < s$ , then

$$b_{ij} = \begin{cases} -w_{8(j+m)+6 \rightarrow 8(j+m)+7} \otimes e_{8j}, & i = j+s; \\ -w_{8(j+m)+1 \rightarrow 8(j+m)+7} \otimes e_{8j}, & i = j+2s; \\ e_{8(j+m)+7} \otimes w_{8j \rightarrow 8j+2}, & i = j+5s; \\ e_{8(j+m)+7} \otimes w_{8j \rightarrow 8j+4}, & i = j+7s; \\ e_{8(j+m)+7} \otimes w_{8j \rightarrow 8j+6}, & i = j+10s; \\ 0, & \text{otherwise.} \end{cases}$$

If  $s \leq j < 2s$ , then

$$b_{ij} = \begin{cases} -w_{8(j+m+1)+1 \rightarrow 8(j+m+1)+2} \otimes w_{8j+1 \rightarrow 8(j+1)}, & i = 2s + (j+1)_s; \\ w_{8(j+m+1) \rightarrow 8(j+m+1)+2} \otimes e_{8j+1}, & i = j+3s; \\ w_{8(j+m+1) \rightarrow 8(j+m+1)+2} \otimes w_{8j+1 \rightarrow 8j+3}, & i = j+5s; \\ 0, & \text{otherwise.} \end{cases}$$

If  $2s \leq j < 3s$ , then

$$b_{ij} = \begin{cases} e_{8(j+m+1)+3} \otimes w_{8j+2 \rightarrow 8(j+1)}, & i = (j+1)_s; \\ -w_{8(j+m+1) \rightarrow 8(j+m+1)+3} \otimes w_{8j+2 \rightarrow 8j+3}, & i = j+4s; \\ 0, & \text{otherwise.} \end{cases}$$

If  $3s \leq j < 4s$ , then

$$b_{ij} = \begin{cases} -w_{8(j+m+1)+3 \rightarrow 8(j+m+1)+4} \otimes w_{8j+3 \rightarrow 8(j+1)}, & i = (j+1)_s; \\ w_{8(j+m+1) \rightarrow 8(j+m+1)+4} \otimes e_{8j+3}, & i = j+3s; \\ 0, & \text{otherwise.} \end{cases}$$

If  $4s \leq j < 5s$ , then

$$b_{ij} = \begin{cases} -e_{8(j+m+1)+5} \otimes w_{8j+4 \rightarrow 8j+7}, & i = j+11s; \\ 0, & \text{otherwise.} \end{cases}$$

If  $5s \leq j < 6s$ , then

$$b_{ij} = \begin{cases} -e_{8(j+m+1)+6} \otimes w_{8j+5 \rightarrow 8(j+1)}, & i = s + (j+1)_s; \\ w_{8(j+m+1) \rightarrow 8(j+m+1)+6} \otimes e_{8j+5}, & i = j + 4s; \\ w_{8(j+m+1) \rightarrow 8(j+m+1)+6} \otimes w_{8j+5 \rightarrow 8j+6}, & i = j + 6s; \\ 0, & \text{otherwise.} \end{cases}$$

If  $6s \leq j < 7s$ , then

$$b_{ij} = \begin{cases} w_{8(j+m+1) \rightarrow 8(j+m+1)+1} \otimes e_{8j+6}, & i = j + 5s; \\ 0, & \text{otherwise.} \end{cases}$$

If  $7s \leq j < 8s$ , then

$$b_{ij} = \begin{cases} e_{8(j+m+2)} \otimes w_{8j+7 \rightarrow 8(j+1)+3}, & i = 6s + (j+1)_s; \\ -w_{8(j+m+1)+2 \rightarrow 8(j+m+2)} \otimes e_{8j+7}, & i = j + 5s; \\ 0, & \text{otherwise.} \end{cases}$$

(21) If  $r_0 = 20$ , then  $\Omega^{20}(Z_t^{(13)})$  is described with  $(16s \times 10s)$  matrix, whose entries  $b_{ij}$  have the following form:

If  $0 \leq j < s$ , then

$$b_{ij} = \begin{cases} -w_{8(j+m-1)+7 \rightarrow 8(j+m)+2} \otimes e_{8j}, & i = j; \\ w_{8(j+m) \rightarrow 8(j+m)+2} \otimes e_{8j}, & i = j + s; \\ w_{8(j+m)+1 \rightarrow 8(j+m)+2} \otimes w_{8j \rightarrow 8j+5}, & i = j + 10s; \\ 0, & \text{otherwise.} \end{cases}$$

If  $s \leq j < 2s$ , then

$$b_{ij} = \begin{cases} w_{8(j+m-1)+7 \rightarrow 8(j+m)+6} \otimes e_{8j}, & i = j - s; \\ -w_{8(j+m) \rightarrow 8(j+m)+6} \otimes e_{8j}, & i = j; \\ -e_{8(j+m)+6} \otimes w_{8j \rightarrow 8j+1}, & i = j + 2s; \\ -w_{8(j+m)+5 \rightarrow 8(j+m)+6} \otimes w_{8j \rightarrow 8j+3}, & i = j + 5s; \\ 0, & \text{otherwise.} \end{cases}$$

If  $2s \leq j < 3s$ , then

$$b_{ij} = \begin{cases} -w_{8(j+m)+2 \rightarrow 8(j+m)+3} \otimes e_{8j+1}, & i = j; \\ e_{8(j+m)+3} \otimes w_{8j+1 \rightarrow 8j+2}, & i = j + 2s; \\ 0, & \text{otherwise.} \end{cases}$$

If  $3s \leq j < 4s$ , then  $b_{ij} = 0$ .

If  $4s \leq j < 5s$ , then

$$b_{ij} = \begin{cases} -e_{8(j+m)+7} \otimes w_{8j+3 \rightarrow 8(j+1)}, & i = (j+1)_s; \\ w_{8(j+m)+5 \rightarrow 8(j+m)+7} \otimes e_{8j+3}, & i = j + 2s; \\ 0, & \text{otherwise.} \end{cases}$$

If  $5s \leq j < 6s$ , then

$$b_{ij} = \begin{cases} -w_{8(j+m)+7 \rightarrow 8(j+m+1)} \otimes w_{8j+4 \rightarrow 8(j+1)}, & i = (j+1)_s; \\ e_{8(j+m+1)} \otimes w_{8j+4 \rightarrow 8(j+1)}, & i = s + (j+1)_s; \\ -w_{8(j+m)+6 \rightarrow 8(j+m+1)} \otimes e_{8j+4}, & i = j + 2s; \\ w_{8(j+m)+7 \rightarrow 8(j+m+1)} \otimes w_{8j+4 \rightarrow 8j+7}, & i = j + 8s; \\ e_{8(j+m+1)} \otimes w_{8j+4 \rightarrow 8j+7}, & i = j + 9s; \\ 0, & \text{otherwise.} \end{cases}$$

If  $6s \leq j < 7s$ , then

$$b_{ij} = \begin{cases} -w_{8(j+m)+1 \rightarrow 8(j+m)+7} \otimes e_{8j+5}, & i = j + 4s; \\ 0, & \text{otherwise.} \end{cases}$$

If  $7s \leq j < 8s$ , then

$$b_{ij} = \begin{cases} w_{8(j+m)+2 \rightarrow 8(j+m+1)} \otimes e_{8j+6}, & i = j + 4s; \\ 0, & \text{otherwise.} \end{cases}$$

If  $8s \leq j < 9s$ , then

$$b_{ij} = \begin{cases} -w_{8(j+m)+7 \rightarrow 8(j+m+1)+1} \otimes w_{8j+7 \rightarrow 8(j+1)}, & i = (j+1)_s; \\ w_{8(j+m+1) \rightarrow 8(j+m+1)+1} \otimes w_{8j+7 \rightarrow 8(j+1)}, & i = s + (j+1)_s; \\ w_{8(j+m)+7 \rightarrow 8(j+m+1)+1} \otimes e_{8j+7}, & i = j + 5s; \\ w_{8(j+m+1) \rightarrow 8(j+m+1)+1} \otimes e_{8j+7}, & i = j + 6s; \\ 0, & \text{otherwise.} \end{cases}$$

If  $9s \leq j < 10s$ , then

$$b_{ij} = \begin{cases} e_{8(j+m+1)+5} \otimes w_{8j+7 \rightarrow 8(j+1)+3}, & i = 6s + (j+1)_s; \\ 0, & \text{otherwise.} \end{cases}$$

(22) If  $r_0 = 21$ , then  $\Omega^{21}(Z_t^{(13)})$  is described with  $(14s \times 11s)$  matrix, whose entries  $b_{ij}$  have the following form:

If  $0 \leq j < s$ , then

$$b_{ij} = \begin{cases} e_{8(j+m)+7} \otimes w_{8j \rightarrow 8j+1}, & i = j + 3s; \\ 0, & \text{otherwise.} \end{cases}$$

If  $s \leq j < 2s$ , then

$$b_{ij} = \begin{cases} w_{8(j+m)+2 \rightarrow 8(j+m+1)} \otimes e_{8j}, & i = j - s; \\ w_{8(j+m)+7 \rightarrow 8(j+m+1)} \otimes w_{8j \rightarrow 8j+1}, & i = j + 2s; \\ e_{8(j+m+1)} \otimes w_{8j \rightarrow 8j+2}, & i = j + 3s; \\ w_{8(j+m)+7 \rightarrow 8(j+m+1)} \otimes w_{8j \rightarrow 8j+3}, & i = j + 4s; \\ 0, & \text{otherwise.} \end{cases}$$



If  $2s \leq j < 3s$ , then

$$b_{ij} = \begin{cases} w_{8(j+m+1)+2 \rightarrow 8(j+m+1)+3} \otimes w_{8j+1 \rightarrow 8(j+1)}, & i = (j+1)_s; \\ w_{8(j+m)+7 \rightarrow 8(j+m+1)+3} \otimes e_{8j+1}, & i = j+s; \\ 0, & \text{otherwise.} \end{cases}$$

If  $3s \leq j < 4s$ , then

$$b_{ij} = \begin{cases} e_{8(j+m+1)+4} \otimes w_{8j+2 \rightarrow 8(j+1)}, & i = s + (j+1)_s; \\ 0, & \text{otherwise.} \end{cases}$$

If  $4s \leq j < 5s$ , then

$$b_{ij} = \begin{cases} w_{8(j+m)+7 \rightarrow 8(j+m+1)+5} \otimes e_{8j+3}, & i = j+s; \\ e_{8(j+m+1)+5} \otimes w_{8j+3 \rightarrow 8j+7}, & i = j+9s; \\ 0, & \text{otherwise.} \end{cases}$$

If  $5s \leq j < 6s$ , then

$$b_{ij} = \begin{cases} e_{8(j+m+1)+6} \otimes w_{8j+4 \rightarrow 8(j+1)}, & i = 2s + (j+1)_s; \\ w_{8(j+m+1) \rightarrow 8(j+m+1)+6} \otimes e_{8j+4}, & i = j+s; \\ -e_{8(j+m+1)+6} \otimes w_{8j+4 \rightarrow 8j+7}, & i = j+6s; \\ -w_{8(j+m+1)+5 \rightarrow 8(j+m+1)+6} \otimes w_{8j+4 \rightarrow 8j+7}, & i = j+8s; \\ 0, & \text{otherwise.} \end{cases}$$

If  $6s \leq j < 7s$ , then  $b_{ij} = 0$ .

If  $7s \leq j < 8s$ , then

$$b_{ij} = \begin{cases} w_{8(j+m)+7 \rightarrow 8(j+m+1)+1} \otimes e_{8j+5}, & i = j; \\ w_{8(j+m+1) \rightarrow 8(j+m+1)+1} \otimes e_{8j+5}, & i = j+s; \\ 0, & \text{otherwise.} \end{cases}$$

If  $8s \leq j < 9s$ , then

$$b_{ij} = \begin{cases} w_{8(j+m+1) \rightarrow 8(j+m+1)+2} \otimes e_{8j+6}, & i = j+s; \\ -w_{8(j+m+1)+1 \rightarrow 8(j+m+1)+2} \otimes w_{8j+6 \rightarrow 8j+7}, & i = j+4s; \\ 0, & \text{otherwise.} \end{cases}$$

If  $9s \leq j < 10s$ , then  $b_{ij} = 0$ .

If  $10s \leq j < 11s$ , then

$$b_{ij} = \begin{cases} -w_{8(j+m+1)+3 \rightarrow 8(j+m+1)+7} \otimes e_{8j+7}, & i = j; \\ 0, & \text{otherwise.} \end{cases}$$

(23) If  $r_0 = 22$ , then  $\Omega^{22}(Z_t^{(13)})$  is described with  $(13s \times 11s)$  matrix, whose entries  $b_{ij}$  have the following form:

If  $0 \leq j < s$ , then

$$b_{ij} = \begin{cases} e_{8(j+m)+5} \otimes w_{8j \rightarrow 8j+2}, & i = j+4s; \\ 0, & \text{otherwise.} \end{cases}$$

If  $s \leq j < 2s$ , then

$$b_{ij} = \begin{cases} -w_{8(j+m)+2 \rightarrow 8(j+m)+3} \otimes w_{8j \rightarrow 8j+5}, & i = j + 6s; \\ 0, & \text{otherwise.} \end{cases}$$

If  $2s \leq j < 3s$ , then

$$b_{ij} = \begin{cases} -w_{8(j+m) \rightarrow 8(j+m)+1} \otimes e_{8j}, & i = j - 2s; \\ w_{8(j+m-1)+7 \rightarrow 8(j+m)+1} \otimes e_{8j}, & i = j - s; \\ 0, & \text{otherwise.} \end{cases}$$

If  $3s \leq j < 4s$ , then

$$b_{ij} = \begin{cases} -w_{8(j+m)+3 \rightarrow 8(j+m)+4} \otimes e_{8j+1}, & i = j - s; \\ e_{8(j+m)+4} \otimes w_{8j+1 \rightarrow 8j+2}, & i = j; \\ 0, & \text{otherwise.} \end{cases}$$

If  $4s \leq j < 5s$ , then

$$b_{ij} = \begin{cases} e_{8(j+m)+7} \otimes w_{8j+2 \rightarrow 8(j+1)}, & i = s + (j + 1)_s; \\ -w_{8(j+m)+6 \rightarrow 8(j+m)+7} \otimes w_{8j+2 \rightarrow 8j+3}, & i = j + s; \\ 0, & \text{otherwise.} \end{cases}$$

If  $5s \leq j < 6s$ , then

$$b_{ij} = \begin{cases} -e_{8(j+m+1)} \otimes w_{8j+3 \rightarrow 8(j+1)}, & i = (j + 1)_s; \\ w_{8(j+m)+7 \rightarrow 8(j+m+1)} \otimes w_{8j+3 \rightarrow 8(j+1)}, & i = s + (j + 1)_s; \\ -w_{8(j+m)+6 \rightarrow 8(j+m+1)} \otimes e_{8j+3}, & i = j; \\ 0, & \text{otherwise.} \end{cases}$$

If  $6s \leq j < 7s$ , then

$$b_{ij} = \begin{cases} -w_{8(j+m)+1 \rightarrow 8(j+m)+7} \otimes e_{8j+4}, & i = j; \\ -e_{8(j+m)+7} \otimes w_{8j+4 \rightarrow 8j+7}, & i = j + 5s; \\ 0, & \text{otherwise.} \end{cases}$$

If  $7s \leq j < 8s$ , then

$$b_{ij} = \begin{cases} w_{8(j+m)+2 \rightarrow 8(j+m+1)} \otimes e_{8j+5}, & i = j; \\ 0, & \text{otherwise.} \end{cases}$$

If  $8s \leq j < 9s$ , then

$$b_{ij} = \begin{cases} w_{8(j+m)+3 \rightarrow 8(j+m)+7} \otimes e_{8j+6}, & i = j + s; \\ 0, & \text{otherwise.} \end{cases}$$

If  $9s \leq j < 10s$ , then

$$b_{ij} = \begin{cases} -w_{8(j+m+1) \rightarrow 8(j+m+1)+2} \otimes w_{8j+7 \rightarrow 8(j+1)}, & i = (j+1)_s; \\ w_{8(j+m)+7 \rightarrow 8(j+m+1)+2} \otimes w_{8j+7 \rightarrow 8(j+1)}, & i = s + (j+1)_s; \\ -e_{8(j+m+1)+2} \otimes w_{8j+7 \rightarrow 8(j+1)+5}, & i = 7s + (j+1)_s; \\ w_{8(j+m)+7 \rightarrow 8(j+m+1)+2} \otimes e_{8j+7}, & i = j + 2s; \\ 0, & \text{otherwise.} \end{cases}$$

If  $10s \leq j < 11s$ , then

$$b_{ij} = \begin{cases} e_{8(j+m+1)+6} \otimes w_{8j+7 \rightarrow 8(j+1)+3}, & i = 5s + (j+1)_s; \\ 0, & \text{otherwise.} \end{cases}$$

(24) If  $r_0 = 23$ , then  $\Omega^{23}(Z_t^{(13)})$  is described with  $(11s \times 13s)$  matrix, whose entries  $b_{ij}$  have the following form:

If  $0 \leq j < s$ , then

$$b_{ij} = \begin{cases} -w_{8(j+m)+3 \rightarrow 8(j+m)+7} \otimes e_{8j}, & i = j; \\ -e_{8(j+m)+7} \otimes w_{8j \rightarrow 8j+2}, & i = j + 3s; \\ 0, & \text{otherwise.} \end{cases}$$

If  $s \leq j < 2s$ , then

$$b_{ij} = \begin{cases} e_{8(j+m+1)} \otimes w_{8j \rightarrow 8j+1}, & i = j + s; \\ 0, & \text{otherwise.} \end{cases}$$

If  $2s \leq j < 3s$ , then

$$b_{ij} = \begin{cases} w_{8(j+m+1)+3 \rightarrow 8(j+m+1)+4} \otimes w_{8j+1 \rightarrow 8(j+1)}, & i = (j+1)_s; \\ w_{8(j+m+1) \rightarrow 8(j+m+1)+4} \otimes e_{8j+1}, & i = j; \\ 0, & \text{otherwise.} \end{cases}$$

If  $3s \leq j < 4s$ , then

$$b_{ij} = \begin{cases} -e_{8(j+m+1)+5} \otimes w_{8j+2 \rightarrow 8(j+1)}, & i = s + (j+1)_s; \\ 0, & \text{otherwise.} \end{cases}$$

If  $4s \leq j < 5s$ , then

$$b_{ij} = \begin{cases} w_{8(j+m+1) \rightarrow 8(j+m+1)+6} \otimes e_{8j+3}, & i = j; \\ -e_{8(j+m+1)+6} \otimes w_{8j+3 \rightarrow 8j+7}, & i = j + 6s; \\ 0, & \text{otherwise.} \end{cases}$$

If  $5s \leq j < 7s$ , then  $b_{ij} = 0$ .

If  $7s \leq j < 8s$ , then

$$b_{ij} = \begin{cases} w_{8(j+m+1) \rightarrow 8(j+m+1)+2} \otimes e_{8j+5}, & i = j - s; \\ e_{8(j+m+1)+2} \otimes w_{8j+5 \rightarrow 8j+7}, & i = j + s; \\ 0, & \text{otherwise.} \end{cases}$$

If  $8s \leq j < 9s$ , then  $b_{ij} = 0$ .

If  $9s \leq j < 10s$ , then

$$b_{ij} = \begin{cases} w_{8(j+m)+7 \rightarrow 8(j+m+1)+3} \otimes e_{8j+6}, & i = j - 2s; \\ 0, & \text{otherwise.} \end{cases}$$

If  $10s \leq j < 11s$ , then  $b_{ij} = 0$ .

If  $11s \leq j < 12s$ , then

$$b_{ij} = \begin{cases} w_{8(j+m+1)+2 \rightarrow 8(j+m+1)+7} \otimes e_{8j+7}, & i = j - 3s; \\ w_{8(j+m+1)+4 \rightarrow 8(j+m+1)+7} \otimes e_{8j+7}, & i = j - 2s; \\ 0, & \text{otherwise.} \end{cases}$$

If  $12s \leq j < 13s$ , then  $b_{ij} = 0$ .

(25) If  $r_0 = 24$ , then  $\Omega^{24}(Z_t^{(13)})$  is described with  $(11s \times 14s)$  matrix, whose entries  $b_{ij}$  have the following form:

If  $0 \leq j < s$ , then

$$b_{ij} = \begin{cases} w_{8(j+m) \rightarrow 8(j+m)+2} \otimes e_{8j}, & i = j; \\ -w_{8(j+m)+1 \rightarrow 8(j+m)+2} \otimes w_{8j \rightarrow 8j+3}, & i = j + 4s; \\ e_{8(j+m)+2} \otimes w_{8j \rightarrow 8j+4}, & i = j + 5s; \\ 0, & \text{otherwise.} \end{cases}$$

If  $s \leq j < 2s$ , then

$$b_{ij} = \begin{cases} -w_{8(j+m)+3 \rightarrow 8(j+m)+4} \otimes w_{8j \rightarrow 8j+5}, & i = j + 5s; \\ 0, & \text{otherwise.} \end{cases}$$

If  $2s \leq j < 3s$ , then

$$b_{ij} = \begin{cases} -e_{8(j+m)+6} \otimes w_{8j \rightarrow 8j+2}, & i = j + s; \\ 0, & \text{otherwise.} \end{cases}$$

If  $3s \leq j < 4s$ , then

$$b_{ij} = \begin{cases} e_{8(j+m)+5} \otimes w_{8j \rightarrow 8j+1}, & i = j - s; \\ 0, & \text{otherwise.} \end{cases}$$

If  $4s \leq j < 5s$ , then

$$b_{ij} = \begin{cases} w_{8(j+m)+5 \rightarrow 8(j+m)+7} \otimes e_{8j+1}, & i = j - 2s; \\ 0, & \text{otherwise.} \end{cases}$$

If  $5s \leq j < 6s$ , then

$$b_{ij} = \begin{cases} -e_{8(j+m+1)} \otimes w_{8j+2 \rightarrow 8(j+1)}, & i = (j+1)_s; \\ 0, & \text{otherwise.} \end{cases}$$

If  $6s \leq j < 7s$ , then

$$b_{ij} = \begin{cases} -w_{8(j+m)+1 \rightarrow 8(j+m)+7} \otimes e_{8j+3}, & i = j - 2s; \\ w_{8(j+m)+2 \rightarrow 8(j+m)+7} \otimes w_{8j+3 \rightarrow 8j+4}, & i = j - s; \\ -e_{8(j+m)+7} \otimes w_{8j+3 \rightarrow 8j+7}, & i = j + 4s; \\ 0, & \text{otherwise.} \end{cases}$$

If  $7s \leq j < 8s$ , then

$$b_{ij} = \begin{cases} -e_{8(j+m+1)} \otimes w_{8j+4 \rightarrow 8j+7}, & i = j + 2s; \\ 0, & \text{otherwise.} \end{cases}$$

If  $8s \leq j < 9s$ , then

$$b_{ij} = \begin{cases} w_{8(j+m)+3 \rightarrow 8(j+m)+7} \otimes e_{8j+5}, & i = j - 2s; \\ 0, & \text{otherwise.} \end{cases}$$

If  $9s \leq j < 10s$ , then

$$b_{ij} = \begin{cases} -w_{8(j+m)+4 \rightarrow 8(j+m)+7} \otimes e_{8j+6}, & i = j - s; \\ 0, & \text{otherwise.} \end{cases}$$

If  $10s \leq j < 12s$ , then  $b_{ij} = 0$ .

If  $12s \leq j < 13s$ , then

$$b_{ij} = \begin{cases} -w_{8(j+m+1) \rightarrow 8(j+m+1)+3} \otimes w_{8j+7 \rightarrow 8(j+1)}, & i = (j+1)_s; \\ w_{8(j+m+1)+1 \rightarrow 8(j+m+1)+3} \otimes w_{8j+7 \rightarrow 8(j+1)+3}, & i = 4s + (j+1)_s; \\ -w_{8(j+m+1)+2 \rightarrow 8(j+m+1)+3} \otimes w_{8j+7 \rightarrow 8(j+1)+4}, & i = 5s + (j+1)_s; \\ -e_{8(j+m+1)+3} \otimes w_{8j+7 \rightarrow 8(j+1)+5}, & i = 6s + (j+1)_s; \\ w_{8(j+m+1) \rightarrow 8(j+m+1)+3} \otimes e_{8j+7}, & i = j - 3s; \\ 0, & \text{otherwise.} \end{cases}$$

If  $13s \leq j < 14s$ , then  $b_{ij} = 0$ .

(26) If  $r_0 = 25$ , then  $\Omega^{25}(Z_t^{(13)})$  is described with  $(10s \times 16s)$  matrix, whose entries  $b_{ij}$  have the following form:

If  $0 \leq j < s$ , then

$$b_{ij} = \begin{cases} w_{8(j+m)+4 \rightarrow 8(j+m)+7} \otimes e_{8j}, & i = j; \\ e_{8(j+m)+7} \otimes w_{8j \rightarrow 8j+1}, & i = j + 2s; \\ 0, & \text{otherwise.} \end{cases}$$

If  $s \leq j < 2s$ , then  $b_{ij} = 0$ .

If  $2s \leq j < 3s$ , then

$$b_{ij} = \begin{cases} -e_{8(j+m+1)} \otimes w_{8j \rightarrow 8j+2}, & i = j + s; \\ 0, & \text{otherwise.} \end{cases}$$

If  $3s \leq j < 4s$ , then

$$b_{ij} = \begin{cases} w_{8(j+m)+7 \rightarrow 8(j+m+1)+5} \otimes e_{8j+1}, & i = j - s; \\ w_{8(j+m+1) \rightarrow 8(j+m+1)+5} \otimes w_{8j+1 \rightarrow 8j+2}, & i = j; \\ -e_{8(j+m+1)+5} \otimes w_{8j+1 \rightarrow 8j+7}, & i = j + 6s; \\ 0, & \text{otherwise.} \end{cases}$$

If  $4s \leq j < 5s$ , then

$$b_{ij} = \begin{cases} e_{8(j+m+1)+6} \otimes w_{8j+2 \rightarrow 8(j+1)}, & i = s + (j+1)s; \\ 0, & \text{otherwise.} \end{cases}$$

If  $5s \leq j < 6s$ , then

$$b_{ij} = \begin{cases} -w_{8(j+m+1) \rightarrow 8(j+m+1)+1} \otimes e_{8j+2}, & i = j - 2s; \\ 0, & \text{otherwise.} \end{cases}$$

If  $6s \leq j < 7s$ , then

$$b_{ij} = \begin{cases} w_{8(j+m+1)+1 \rightarrow 8(j+m+1)+2} \otimes e_{8j+3}, & i = j - 2s; \\ 0, & \text{otherwise.} \end{cases}$$

If  $7s \leq j < 8s$ , then  $b_{ij} = 0$ .

If  $8s \leq j < 9s$ , then

$$b_{ij} = \begin{cases} -e_{8(j+m+1)+5} \otimes w_{8j+4 \rightarrow 8j+7}, & i = j + s; \\ 0, & \text{otherwise.} \end{cases}$$

If  $9s \leq j < 10s$ , then

$$b_{ij} = \begin{cases} w_{8(j+m)+7 \rightarrow 8(j+m+1)+3} \otimes e_{8j+5}, & i = j - 3s; \\ e_{8(j+m+1)+3} \otimes w_{8j+5 \rightarrow 8j+7}, & i = j - s; \\ 0, & \text{otherwise.} \end{cases}$$

If  $10s \leq j < 12s$ , then  $b_{ij} = 0$ .

If  $12s \leq j < 13s$ , then

$$b_{ij} = \begin{cases} w_{8(j+m+1) \rightarrow 8(j+m+1)+4} \otimes e_{8j+6}, & i = j - 5s; \\ 0, & \text{otherwise.} \end{cases}$$

If  $13s \leq j < 14s$ , then  $b_{ij} = 0$ .

If  $14s \leq j < 15s$ , then

$$b_{ij} = \begin{cases} w_{8(j+m+1)+5 \rightarrow 8(j+m+1)+7} \otimes e_{8j+7}, & i = j - 5s; \\ 0, & \text{otherwise.} \end{cases}$$

If  $15s \leq j < 16s$ , then

$$b_{ij} = \begin{cases} w_{8(j+m+1)+4 \rightarrow 8(j+m+2)} \otimes w_{8j+7 \rightarrow 8(j+1)}, & i = (j+1)_s; \\ w_{8(j+m+1)+7 \rightarrow 8(j+m+2)} \otimes w_{8j+7 \rightarrow 8(j+1)+1}, & i = 2s + (j+1)_s; \\ e_{8(j+m+2)} \otimes w_{8j+7 \rightarrow 8(j+1)+2}, & i = 3s + (j+1)_s; \\ e_{8(j+m+2)} \otimes w_{8j+7 \rightarrow 8(j+1)+6}, & i = 7s + (j+1)_s; \\ w_{8(j+m+1)+3 \rightarrow 8(j+m+2)} \otimes e_{8j+7}, & i = j - 7s; \\ 0, & \text{otherwise.} \end{cases}$$

(27) If  $r_0 = 26$ , then  $\Omega^{26}(Z_t^{(13)})$  is described with  $(8s \times 16s)$  matrix, whose entries  $b_{ij}$  have the following form:

If  $s \leq j < 2s$ , then

$$b_{ij} = \begin{cases} w_{8(j+m-1)+7 \rightarrow 8(j+m)+3} \otimes e_{8j}, & i = j - s; \\ -w_{8(j+m)+2 \rightarrow 8(j+m)+3} \otimes w_{8j \rightarrow 8j+3}, & i = j + 2s; \\ e_{8(j+m)+3} \otimes w_{8j \rightarrow 8j+4}, & i = j + 3s; \\ 0, & \text{otherwise.} \end{cases}$$

If  $2s \leq j < 3s$ , then

$$b_{ij} = \begin{cases} e_{8(j+m)+6} \otimes w_{8j \rightarrow 8j+1}, & i = j - s; \\ 0, & \text{otherwise.} \end{cases}$$

If  $3s \leq j < 4s$ , then  $b_{ij} = 0$ .

If  $4s \leq j < 5s$ , then

$$b_{ij} = \begin{cases} -w_{8(j+m)+6 \rightarrow 8(j+m+1)} \otimes e_{8j+1}, & i = j - 3s; \\ 0, & \text{otherwise.} \end{cases}$$

If  $5s \leq j < 6s$ , then

$$b_{ij} = \begin{cases} e_{8(j+m)+7} \otimes w_{8j+2 \rightarrow 8(j+1)}, & i = (j+1)_s; \\ -w_{8(j+m)+1 \rightarrow 8(j+m)+7} \otimes e_{8j+2}, & i = j - 3s; \\ 0, & \text{otherwise.} \end{cases}$$

If  $6s \leq j < 7s$ , then

$$b_{ij} = \begin{cases} -w_{8(j+m)+2 \rightarrow 8(j+m+1)} \otimes e_{8j+3}, & i = j - 3s; \\ w_{8(j+m)+3 \rightarrow 8(j+m+1)} \otimes w_{8j+3 \rightarrow 8j+4}, & i = j - 2s; \\ 0, & \text{otherwise.} \end{cases}$$

If  $7s \leq j < 8s$ , then  $b_{ij} = 0$ .

If  $8s \leq j < 9s$ , then

$$b_{ij} = \begin{cases} -w_{8(j+m)+4 \rightarrow 8(j+m)+7} \otimes e_{8j+5}, & i = j - 3s; \\ 0, & \text{otherwise.} \end{cases}$$

If  $9s \leq j < 10s$ , then  $b_{ij} = 0$ .

If  $10s \leq j < 11s$ , then

$$b_{ij} = \begin{cases} -w_{8(j+m)+5 \rightarrow 8(j+m)+7} \otimes e_{8j+6}, & i = j - 4s; \\ 0, & \text{otherwise.} \end{cases}$$

If  $11s \leq j < 12s$ , then

$$b_{ij} = \begin{cases} -w_{8(j+m)+5 \rightarrow 8(j+m+1)} \otimes e_{8j+6}, & i = j - 5s; \\ -e_{8(j+m+1)} \otimes w_{8j+6 \rightarrow 8j+7}, & i = j - 4s; \\ 0, & \text{otherwise.} \end{cases}$$

If  $12s \leq j < 13s$ , then

$$b_{ij} = \begin{cases} -w_{8(j+m+1)+1 \rightarrow 8(j+m+1)+2} \otimes w_{8j+7 \rightarrow 8(j+1)+2}, & i = 2s + (j+1)s; \\ w_{8(j+m+1) \rightarrow 8(j+m+1)+2} \otimes e_{8j+7}, & i = j - 5s; \\ 0, & \text{otherwise.} \end{cases}$$

If  $13s \leq j < 14s$ , then  $b_{ij} = 0$ .

If  $14s \leq j < 15s$ , then

$$b_{ij} = \begin{cases} -e_{8(j+m+1)+6} \otimes w_{8j+7 \rightarrow 8(j+1)+1}, & i = s + (j+1)s; \\ 0, & \text{otherwise.} \end{cases}$$

If  $15s \leq j < 16s$ , then

$$b_{ij} = \begin{cases} e_{8(j+m+1)+5} \otimes w_{8j+7 \rightarrow 8(j+1)+6}, & i = 6s + (j+1)s; \\ 0, & \text{otherwise.} \end{cases}$$

(28) If  $r_0 = 27$ , then  $\Omega^{27}(Z_t^{(13)})$  is described with  $(9s \times 19s)$  matrix, whose entries  $b_{ij}$  have the following form:

If  $0 \leq j < s$ , then

$$b_{ij} = \begin{cases} e_{8(j+m)+7} \otimes e_{8j}, & i = j; \\ 0, & \text{otherwise.} \end{cases}$$

If  $s \leq j < 2s$ , then

$$b_{ij} = \begin{cases} w_{8(j+m)+7 \rightarrow 8(j+m+1)} \otimes e_{8j}, & i = j - s; \\ e_{8(j+m+1)} \otimes w_{8j \rightarrow 8j+1}, & i = j; \\ 0, & \text{otherwise.} \end{cases}$$

If  $2s \leq j < 3s$ , then  $b_{ij} = 0$ .

If  $3s \leq j < 4s$ , then

$$b_{ij} = \begin{cases} w_{8(j+m+1) \rightarrow 8(j+m+1)+6} \otimes e_{8j+1}, & i = j - 2s; \\ e_{8(j+m+1)+6} \otimes w_{8j+1 \rightarrow 8j+7}, & i = j + 5s; \\ 0, & \text{otherwise.} \end{cases}$$

If  $4s \leq j < 5s$ , then  $b_{ij} = 0$ .

If  $5s \leq j < 6s$ , then

$$b_{ij} = \begin{cases} w_{8(j+m+1)+1 \rightarrow 8(j+m+1)+2} \otimes e_{8j+2}, & i = j - 3s; \\ 0, & \text{otherwise.} \end{cases}$$



If  $6s \leq j < 7s$ , then

$$b_{ij} = \begin{cases} w_{8(j+m+1)+2 \rightarrow 8(j+m+1)+3} \otimes e_{8j+3}, & i = j - 3s; \\ 0, & \text{otherwise.} \end{cases}$$

If  $7s \leq j < 8s$ , then  $b_{ij} = 0$ .

If  $8s \leq j < 9s$ , then

$$b_{ij} = \begin{cases} w_{8(j+m+1)+3 \rightarrow 8(j+m+1)+4} \otimes e_{8j+4}, & i = j - 4s; \\ 0, & \text{otherwise.} \end{cases}$$

If  $9s \leq j < 11s$ , then  $b_{ij} = 0$ .

If  $11s \leq j < 12s$ , then

$$b_{ij} = \begin{cases} w_{8(j+m+1) \rightarrow 8(j+m+1)+4} \otimes e_{8j+5}, & i = j - 6s; \\ 0, & \text{otherwise.} \end{cases}$$

If  $12s \leq j < 15s$ , then  $b_{ij} = 0$ .

If  $15s \leq j < 16s$ , then

$$b_{ij} = \begin{cases} -e_{8(j+m+1)+5} \otimes e_{8j+6}, & i = j - 9s; \\ 0, & \text{otherwise.} \end{cases}$$

If  $16s \leq j < 17s$ , then

$$b_{ij} = \begin{cases} e_{8(j+m+1)+7} \otimes w_{8j+7 \rightarrow 8(j+1)}, & i = (j+1)_s; \\ w_{8(j+m+1)+4 \rightarrow 8(j+m+1)+7} \otimes e_{8j+7}, & i = j - 9s; \\ 0, & \text{otherwise.} \end{cases}$$

If  $17s \leq j < 18s$ , then

$$b_{ij} = \begin{cases} e_{8(j+m+1)+7} \otimes w_{8j+7 \rightarrow 8(j+1)}, & i = (j+1)_s; \\ 0, & \text{otherwise.} \end{cases}$$

If  $18s \leq j < 19s$ , then  $b_{ij} = 0$ .

(29) If  $r_0 = 28$ , then  $\Omega^{28}(Z_t^{(13)})$  is described with  $(8s \times 18s)$  matrix, whose entries  $b_{ij}$  have the following form:

If  $0 \leq j < s$ , then

$$b_{ij} = \begin{cases} w_{8(j+m)+1 \rightarrow 8(j+m)+2} \otimes w_{8j \rightarrow 8j+1}, & i = j + s; \\ 0, & \text{otherwise.} \end{cases}$$

If  $s \leq j < 2s$ , then

$$b_{ij} = \begin{cases} w_{8(j+m) \rightarrow 8(j+m)+6} \otimes e_{8j}, & i = j - s; \\ w_{8(j+m)+5 \rightarrow 8(j+m)+6} \otimes w_{8j \rightarrow 8j+5}, & i = j + 4s; \\ -e_{8(j+m)+6} \otimes w_{8j \rightarrow 8j+6}, & i = j + 5s; \\ 0, & \text{otherwise.} \end{cases}$$

If  $2s \leq j < 3s$ , then

$$b_{ij} = \begin{cases} w_{8(j+m) \rightarrow 8(j+m)+4} \otimes e_{8j}, & i = j - 2s; \\ -w_{8(j+m)+3 \rightarrow 8(j+m)+4} \otimes w_{8j \rightarrow 8j+3}, & i = j + s; \\ 0, & \text{otherwise.} \end{cases}$$

If  $3s \leq j < 4s$ , then  $b_{ij} = 0$ .

If  $4s \leq j < 5s$ , then

$$b_{ij} = \begin{cases} w_{8(j+m) \rightarrow 8(j+m)+5} \otimes e_{8j}, & i = j - 4s; \\ e_{8(j+m)+5} \otimes w_{8j \rightarrow 8j+5}, & i = j + s; \\ 0, & \text{otherwise.} \end{cases}$$

If  $5s \leq j < 6s$ , then

$$b_{ij} = \begin{cases} -w_{8(j+m)+1 \rightarrow 8(j+m)+7} \otimes e_{8j+1}, & i = j - 4s; \\ -w_{8(j+m)+3 \rightarrow 8(j+m)+7} \otimes w_{8j+1 \rightarrow 8j+3}, & i = j - 2s; \\ w_{8(j+m)+4 \rightarrow 8(j+m)+7} \otimes w_{8j+1 \rightarrow 8j+4}, & i = j - s; \\ e_{8(j+m)+7} \otimes w_{8j+1 \rightarrow 8j+7}, & i = j + 2s; \\ 0, & \text{otherwise.} \end{cases}$$

If  $6s \leq j < 7s$ , then

$$b_{ij} = \begin{cases} e_{8(j+m+1)} \otimes w_{8j+2 \rightarrow 8(j+1)}, & i = (j+1)_s; \\ -w_{8(j+m)+2 \rightarrow 8(j+m+1)} \otimes e_{8j+2}, & i = j - 4s; \\ 0, & \text{otherwise.} \end{cases}$$

If  $7s \leq j < 8s$ , then

$$b_{ij} = \begin{cases} -w_{8(j+m)+3 \rightarrow 8(j+m)+7} \otimes e_{8j+3}, & i = j - 4s; \\ w_{8(j+m)+4 \rightarrow 8(j+m)+7} \otimes w_{8j+3 \rightarrow 8j+4}, & i = j - 3s; \\ 0, & \text{otherwise.} \end{cases}$$

If  $8s \leq j < 9s$ , then

$$b_{ij} = \begin{cases} w_{8(j+m)+4 \rightarrow 8(j+m)+7} \otimes e_{8j+4}, & i = j - 4s; \\ 0, & \text{otherwise.} \end{cases}$$

If  $9s \leq j < 10s$ , then  $b_{ij} = 0$ .

If  $10s \leq j < 11s$ , then

$$b_{ij} = \begin{cases} -w_{8(j+m)+5 \rightarrow 8(j+m)+7} \otimes e_{8j+5}, & i = j - 5s; \\ 0, & \text{otherwise.} \end{cases}$$

If  $11s \leq j < 12s$ , then

$$b_{ij} = \begin{cases} -w_{8(j+m)+5 \rightarrow 8(j+m+1)} \otimes e_{8j+5}, & i = j - 6s; \\ 0, & \text{otherwise.} \end{cases}$$

If  $12s \leq j < 13s$ , then

$$b_{ij} = \begin{cases} w_{8(j+m)+6 \rightarrow 8(j+m)+7} \otimes e_{8j+6}, & i = j - 6s; \\ -e_{8(j+m)+7} \otimes w_{8j+6 \rightarrow 8j+7}, & i = j - 5s; \\ 0, & \text{otherwise.} \end{cases}$$

If  $13s \leq j < 15s$ , then  $b_{ij} = 0$ .

If  $15s \leq j < 16s$ , then

$$b_{ij} = \begin{cases} -w_{8(j+m+1)+2 \rightarrow 8(j+m+1)+3} \otimes w_{8j+7 \rightarrow 8(j+1)+2}, & i = 2s + (j+1)_s; \\ w_{8(j+m)+7 \rightarrow 8(j+m+1)+3} \otimes e_{8j+7}, & i = j - 8s; \\ 0, & \text{otherwise.} \end{cases}$$

If  $16s \leq j < 17s$ , then

$$b_{ij} = \begin{cases} w_{8(j+m+1) \rightarrow 8(j+m+1)+6} \otimes w_{8j+7 \rightarrow 8(j+1)}, & i = (j+1)_s; \\ w_{8(j+m+1)+5 \rightarrow 8(j+m+1)+6} \otimes w_{8j+7 \rightarrow 8(j+1)+5}, & i = 5s + (j+1)_s; \\ -e_{8(j+m+1)+6} \otimes w_{8j+7 \rightarrow 8(j+1)+6}, & i = 6s + (j+1)_s; \\ 0, & \text{otherwise.} \end{cases}$$

If  $17s \leq j < 18s$ , then  $b_{ij} = 0$ .

(II) Represent an arbitrary  $t_0 \in \mathbb{N}$  in the form  $t_0 = 29\ell_0 + r_0$ , where  $0 \leq r_0 \leq 28$ . Then  $\Omega^{t_0}(Z_t^{(13)})$  is a  $\Omega^{r_0}(Z_t^{(13)})$ , whose left components twisted by  $\sigma^{\ell_0}$ .

**Proposition 11** (Translates for the case 14). (I) Let  $r_0 \in \mathbb{N}$ ,  $r_0 < 29$ .  $r_0$ -translates of the elements  $Z_t^{(14)}$  are described by the following way.

(1) If  $r_0 = 0$ , then  $\Omega^0(Z_t^{(14)})$  is described with  $(8s \times 18s)$  matrix with the following nonzero entries:

$$\begin{aligned} b_{j-s,s} &= w_{8(j+m) \rightarrow 8(j+m)+3} \otimes e_{8j}; \\ b_{j-3s,4s} &= -w_{8(j+m)+1 \rightarrow 8(j+m+1)} \otimes e_{8j+1}; \\ b_{j-5s,11s} &= w_{8(j+m)+6 \rightarrow 8(j+m)+7} \otimes e_{8j+6}. \end{aligned}$$

(2) If  $r_0 = 1$ , then  $\Omega^1(Z_t^{(14)})$  is described with  $(9s \times 20s)$  matrix with the following nonzero entries:

$$\begin{aligned} b_{j+s,0} &= -w_{8(j+m)+5 \rightarrow 8(j+m)+7} \otimes e_{8j}; \\ b_{j+6s,0} &= -w_{8(j+m)+6 \rightarrow 8(j+m)+7} \otimes w_{8j \rightarrow 8j+5}; \\ b_{j-s,s} &= w_{8(j+m)+1 \rightarrow 8(j+m+1)} \otimes e_{8j}; \\ b_{(j+1)_s,3s+(-1)_s} &= -w_{8(j+m+1)+1 \rightarrow 8(j+m+1)+3} \otimes w_{8j+1 \rightarrow 8(j+1)}; \\ b_{2s+(j+1)_s,3s+(-1)_s} &= -w_{8(j+m+1)+2 \rightarrow 8(j+m+1)+3} \otimes w_{8j+1 \rightarrow 8(j+1)+1}; \\ b_{(j+1)_s,5s+(-1)_s} &= -w_{8(j+m+1)+1 \rightarrow 8(j+m+1)+4} \otimes w_{8j+2 \rightarrow 8(j+1)}; \\ b_{2s+(j+1)_s,5s+(-1)_s} &= -w_{8(j+m+1)+2 \rightarrow 8(j+m+1)+4} \otimes w_{8j+2 \rightarrow 8(j+1)+1}; \\ b_{3s+(j+1)_s,5s+(-1)_s} &= -w_{8(j+m+1)+3 \rightarrow 8(j+m+1)+4} \otimes w_{8j+2 \rightarrow 8(j+1)+2}; \\ b_{j-5s,11s} &= -w_{8(j+m)+6 \rightarrow 8(j+m+1)+6} \otimes e_{8j+5}; \\ b_{(j+1)_s,12s+(-1)_s} &= w_{8(j+m+1)+1 \rightarrow 8(j+m+1)+3} \otimes w_{8j+5 \rightarrow 8(j+1)}; \\ b_{(j+1)_s,18s+(-1)_s} &= -w_{8(j+m+1)+1 \rightarrow 8(j+m+2)} \otimes w_{8j+7 \rightarrow 8(j+1)}; \\ b_{j-10s,18s+(-1)_s} &= -w_{8(j+m+1) \rightarrow 8(j+m+2)} \otimes e_{8j+7}. \end{aligned}$$

(3) If  $r_0 = 2$ , then  $\Omega^2(Z_t^{(14)})$  is described with  $(8s \times 18s)$  matrix with the following nonzero entries:

$$\begin{aligned} b_{(j+1)s, 5s+(-1)s} &= -e_{8(j+m)+7} \otimes w_{8j+1 \rightarrow 8(j+1)}; \\ b_{(j+1)s, 6s+(-1)s} &= -e_{8(j+m)+7} \otimes w_{8j+2 \rightarrow 8(j+1)}; \\ b_{(j+1)s, 8s+(-1)s} &= w_{8(j+m)+7 \rightarrow 8(j+m+1)} \otimes w_{8j+3 \rightarrow 8(j+1)}; \\ b_{j-5s, 8s+(-1)s} &= -w_{8(j+m)+4 \rightarrow 8(j+m+1)} \otimes e_{8j+3}; \\ b_{(j+1)s, 10s+(-1)s} &= -e_{8(j+m)+7} \otimes w_{8j+5 \rightarrow 8(j+1)}; \\ b_{j-6s, 12s+(-1)s} &= w_{8(j+m)+1 \rightarrow 8(j+m+1)} \otimes e_{8j+6}. \end{aligned}$$

(4) If  $r_0 = 3$ , then  $\Omega^3(Z_t^{(14)})$  is described with  $(10s \times 19s)$  matrix with the following nonzero entries:

$$\begin{aligned} b_{j-s, s+(-1)s} &= w_{8(j+m)+2 \rightarrow 8(j+m+1)} \otimes e_{8j}; \\ b_{j+s, s+(-1)s} &= w_{8(j+m)+3 \rightarrow 8(j+m+1)} \otimes w_{8j \rightarrow 8j+1}; \\ b_{j+2s, s+(-1)s} &= w_{8(j+m)+4 \rightarrow 8(j+m+1)} \otimes w_{8j \rightarrow 8j+2}; \\ b_{(j+1)s, 3s+(-1)s} &= -w_{8(j+m+1)+2 \rightarrow 8(j+m+1)+4} \otimes w_{8j+1 \rightarrow 8(j+1)}; \\ b_{2s+(j+1)s, 3s+(-1)s} &= -w_{8(j+m+1)+3 \rightarrow 8(j+m+1)+4} \otimes w_{8j+1 \rightarrow 8(j+1)+1}; \\ b_{s+(j+1)s, 4s+(-1)s} &= -e_{8(j+m+1)+6} \otimes w_{8j+1 \rightarrow 8(j+1)}; \\ b_{j-3s, 7s+(-1)s} &= -w_{8(j+m)+7 \rightarrow 8(j+m+1)+2} \otimes e_{8j+3}; \\ b_{s+(j+1)s, 8s+(-1)s} &= e_{8(j+m+1)+6} \otimes w_{8j+3 \rightarrow 8(j+1)}; \\ b_{(j+1)s, 10s+(-1)s} &= -e_{8(j+m+1)+2} \otimes w_{8j+5 \rightarrow 8(j+1)}. \end{aligned}$$

(5) If  $r_0 = 4$ , then  $\Omega^4(Z_t^{(14)})$  is described with  $(11s \times 18s)$  matrix with the following nonzero entries:

$$\begin{aligned} b_{j, (-1)s} &= -w_{8(j+m-1)+7 \rightarrow 8(j+m)+2} \otimes e_{8j}; \\ b_{j+s, (-1)s} &= -w_{8(j+m) \rightarrow 8(j+m)+2} \otimes e_{8j}; \\ b_{j+6s, (-1)s} &= w_{8(j+m)+1 \rightarrow 8(j+m)+2} \otimes w_{8j \rightarrow 8j+4}; \\ b_{j+8s, (-1)s} &= -e_{8(j+m)+2} \otimes w_{8j \rightarrow 8j+6}; \\ b_{(j+1)s, 4s+(-1)s} &= -e_{8(j+m)+7} \otimes w_{8j+1 \rightarrow 8(j+1)}; \\ b_{(j+1)s, 5s+(-2)s} &= -w_{8(j+m)+7 \rightarrow 8(j+m+1)} \otimes w_{8j+1 \rightarrow 8(j+1)}; \\ b_{s+(j+1)s, 5s+(-2)s} &= -e_{8(j+m+1)} \otimes w_{8j+1 \rightarrow 8(j+1)}; \\ b_{s+(j+1)s, 5s+(-1)s} &= -e_{8(j+m+1)} \otimes w_{8j+1 \rightarrow 8(j+1)}; \\ b_{(j+1)s, 6s+(-2)s} &= -w_{8(j+m)+7 \rightarrow 8(j+m+1)} \otimes w_{8j+2 \rightarrow 8(j+1)}; \\ b_{s+(j+1)s, 6s+(-2)s} &= -e_{8(j+m+1)} \otimes w_{8j+2 \rightarrow 8(j+1)}; \\ b_{s+(j+1)s, 6s+(-1)s} &= -e_{8(j+m+1)} \otimes w_{8j+2 \rightarrow 8(j+1)}; \\ b_{j-3s, 7s+(-1)s} &= -w_{8(j+m)+5 \rightarrow 8(j+m)+7} \otimes e_{8j+3}; \\ b_{j-2s, 7s+(-1)s} &= w_{8(j+m)+6 \rightarrow 8(j+m)+7} \otimes w_{8j+3 \rightarrow 8j+4}; \\ b_{(j+1)s, 9s+(-2)s} &= -w_{8(j+m)+7 \rightarrow 8(j+m+1)} \otimes w_{8j+5 \rightarrow 8(j+1)}; \\ b_{s+(j+1)s, 9s+(-2)s} &= -e_{8(j+m+1)} \otimes w_{8j+5 \rightarrow 8(j+1)}; \\ b_{(j+1)s, 9s+(-1)s} &= -w_{8(j+m)+7 \rightarrow 8(j+m+1)} \otimes w_{8j+5 \rightarrow 8(j+1)}; \\ b_{s+(j+1)s, 9s+(-1)s} &= -e_{8(j+m+1)} \otimes w_{8j+5 \rightarrow 8(j+1)}; \\ b_{2s+(j+1)s, 13s+(-2)s} &= -e_{8(j+m+1)+3} \otimes w_{8j+7 \rightarrow 8(j+1)+1}. \end{aligned}$$

(6) If  $r_0 = 5$ , then  $\Omega^5(Z_t^{(14)})$  is described with  $(11s \times 19s)$  matrix with the following nonzero entries:

$$\begin{aligned}
b_{j+s,(-1)_s} &= -w_{8(j+m)+3 \rightarrow 8(j+m)+7} \otimes e_{8j}; \\
b_{j+2s,(-1)_s} &= -w_{8(j+m)+1 \rightarrow 8(j+m)+7} \otimes e_{8j}; \\
b_{j+3s,(-1)_s} &= -w_{8(j+m)+4 \rightarrow 8(j+m)+7} \otimes w_{8j \rightarrow 8j+1}; \\
b_{j+4s,(-1)_s} &= -e_{8(j+m)+7} \otimes w_{8j \rightarrow 8j+2}; \\
b_{(j+1)_s,3s+(-2)_s} &= -e_{8(j+m+1)+5} \otimes w_{8j+1 \rightarrow 8(j+1)}; \\
b_{(j+1)_s,3s+(-1)_s} &= -e_{8(j+m+1)+5} \otimes w_{8j+1 \rightarrow 8(j+1)}; \\
b_{2s+(j+1)_s,5s+(-1)_s} &= -w_{8(j+m+1)+1 \rightarrow 8(j+m+1)+2} \otimes w_{8j+2 \rightarrow 8(j+1)}; \\
b_{(j+1)_s,6s+(-2)_s} &= -w_{8(j+m+1)+5 \rightarrow 8(j+m+1)+6} \otimes w_{8j+2 \rightarrow 8(j+1)}; \\
b_{(j+1)_s,6s+(-1)_s} &= -w_{8(j+m+1)+5 \rightarrow 8(j+m+1)+6} \otimes w_{8j+2 \rightarrow 8(j+1)}; \\
b_{j-2s,6s+(-1)_s} &= -w_{8(j+m)+7 \rightarrow 8(j+m+1)+6} \otimes e_{8j+2}; \\
b_{s+(j+1)_s,7s+(-2)_s} &= e_{8(j+m+1)+3} \otimes w_{8j+3 \rightarrow 8(j+1)}; \\
b_{2s+(j+1)_s,7s+(-2)_s} &= w_{8(j+m+1)+1 \rightarrow 8(j+m+1)+3} \otimes w_{8j+3 \rightarrow 8(j+1)}; \\
b_{s+(j+1)_s,10s+(-2)_s} &= -e_{8(j+m+1)+3} \otimes w_{8j+5 \rightarrow 8(j+1)}; \\
b_{2s+(j+1)_s,10s+(-2)_s} &= -w_{8(j+m+1)+1 \rightarrow 8(j+m+1)+3} \otimes w_{8j+5 \rightarrow 8(j+1)}; \\
b_{s+(j+1)_s,10s+(-1)_s} &= -e_{8(j+m+1)+3} \otimes w_{8j+5 \rightarrow 8(j+1)}; \\
b_{2s+(j+1)_s,10s+(-1)_s} &= -w_{8(j+m+1)+1 \rightarrow 8(j+m+1)+3} \otimes w_{8j+5 \rightarrow 8(j+1)}; \\
b_{(j+1)_s,12s+(-2)_s} &= -e_{8(j+m+1)+5} \otimes w_{8j+5 \rightarrow 8(j+1)}; \\
b_{(j+1)_s,12s+(-1)_s} &= -e_{8(j+m+1)+5} \otimes w_{8j+5 \rightarrow 8(j+1)}; \\
b_{s+(j+1)_s,14s+(-2)_s} &= -w_{8(j+m+1)+3 \rightarrow 8(j+m+1)+4} \otimes w_{8j+6 \rightarrow 8(j+1)}; \\
b_{2s+(j+1)_s,14s+(-2)_s} &= -w_{8(j+m+1)+1 \rightarrow 8(j+m+1)+4} \otimes w_{8j+6 \rightarrow 8(j+1)}; \\
b_{s+(j+1)_s,16s+(-2)_s} &= w_{8(j+m+1)+3 \rightarrow 8(j+m+1)+7} \otimes w_{8j+7 \rightarrow 8(j+1)}; \\
b_{2s+(j+1)_s,16s+(-2)_s} &= w_{8(j+m+1)+1 \rightarrow 8(j+m+1)+7} \otimes w_{8j+7 \rightarrow 8(j+1)}; \\
b_{s+(j+1)_s,17s+(-2)_s} &= w_{8(j+m+1)+3 \rightarrow 8(j+m+2)} \otimes w_{8j+7 \rightarrow 8(j+1)}; \\
b_{2s+(j+1)_s,17s+(-2)_s} &= w_{8(j+m+1)+1 \rightarrow 8(j+m+2)} \otimes w_{8j+7 \rightarrow 8(j+1)}.
\end{aligned}$$

(7) If  $r_0 = 6$ , then  $\Omega^6(Z_t^{(14)})$  is described with  $(13s \times 16s)$  matrix with the following nonzero entries:

$$\begin{aligned}
b_{j,(-1)_s} &= w_{8(j+m-1)+7 \rightarrow 8(j+m)+3} \otimes e_{8j}; \\
b_{j+6s,(-1)_s} &= -w_{8(j+m)+2 \rightarrow 8(j+m)+3} \otimes w_{8j \rightarrow 8j+4}; \\
b_{j+9s,(-1)_s} &= -e_{8(j+m)+3} \otimes w_{8j \rightarrow 8j+6}; \\
b_{(j+1)_s,4s+(-2)_s} &= -w_{8(j+m)+7 \rightarrow 8(j+m+1)} \otimes w_{8j+1 \rightarrow 8(j+1)}; \\
b_{(j+1)_s,4s+(-1)_s} &= -w_{8(j+m)+7 \rightarrow 8(j+m+1)} \otimes w_{8j+1 \rightarrow 8(j+1)}; \\
b_{s+(j+1)_s,4s+(-1)_s} &= -e_{8(j+m+1)} \otimes w_{8j+1 \rightarrow 8(j+1)}; \\
b_{(j+1)_s,5s+(-2)_s} &= e_{8(j+m)+7} \otimes w_{8j+2 \rightarrow 8(j+1)}; \\
b_{j-2s,5s+(-1)_s} &= w_{8(j+m)+5 \rightarrow 8(j+m)+7} \otimes e_{8j+2}; \\
b_{j,5s+(-1)_s} &= -w_{8(j+m)+1 \rightarrow 8(j+m)+7} \otimes w_{8j+2 \rightarrow 8j+3}; \\
b_{(j+1)_s,8s+(-2)_s} &= e_{8(j+m)+7} \otimes w_{8j+5 \rightarrow 8(j+1)}; \\
b_{(j+1)_s,8s+(-1)_s} &= e_{8(j+m)+7} \otimes w_{8j+5 \rightarrow 8(j+1)}; \\
b_{2s+(j+1)_s,13s+(-2)_s} &= -e_{8(j+m+1)+4} \otimes w_{8j+7 \rightarrow 8(j+1)+1}.
\end{aligned}$$

(8) If  $r_0 = 7$ , then  $\Omega^7(Z_t^{(14)})$  is described with  $(14s \times 16s)$  matrix with the following nonzero entries:

$$\begin{aligned}
b_{j,(-1)_s} &= w_{8(j+m)+2 \rightarrow 8(j+m)+7} \otimes e_{8j}; \\
b_{j+s,(-1)_s} &= -w_{8(j+m)+4 \rightarrow 8(j+m)+7} \otimes e_{8j}; \\
b_{j+4s,(-1)_s} &= -e_{8(j+m)+7} \otimes w_{8j \rightarrow 8j+1}; \\
b_{j-s,s+(-1)_s} &= w_{8(j+m)+2 \rightarrow 8(j+m)+1} \otimes e_{8j}; \\
b_{j,s+(-1)_s} &= -w_{8(j+m)+4 \rightarrow 8(j+m)+1} \otimes e_{8j}; \\
b_{j+3s,s+(-1)_s} &= -w_{8(j+m)+7 \rightarrow 8(j+m)+1} \otimes w_{8j \rightarrow 8j+1}; \\
b_{j+4s,s+(-1)_s} &= -e_{8(j+m)+1} \otimes w_{8j \rightarrow 8j+2}; \\
b_{(j+1)_s,2s+(-1)_s} &= -e_{8(j+m)+2} \otimes w_{8j+1 \rightarrow 8(j+1)}; \\
b_{2s+(j+1)_s,3s+(-2)_s} &= -e_{8(j+m)+6} \otimes w_{8j+1 \rightarrow 8(j+1)}; \\
b_{2s+(j+1)_s,3s+(-1)_s} &= -e_{8(j+m)+6} \otimes w_{8j+1 \rightarrow 8(j+1)}; \\
b_{3s+(j+1)_s,3s+(-1)_s} &= -w_{8(j+m)+5 \rightarrow 8(j+m)+6} \otimes w_{8j+1 \rightarrow 8(j+1)}; \\
b_{(j+1)_s,5s+(-2)_s} &= -w_{8(j+m)+2 \rightarrow 8(j+m)+4} \otimes w_{8j+3 \rightarrow 8(j+1)}; \\
b_{s+(j+1)_s,5s+(-2)_s} &= e_{8(j+m)+4} \otimes w_{8j+3 \rightarrow 8(j+1)}; \\
b_{2s+(j+1)_s,8s+(-2)_s} &= e_{8(j+m)+6} \otimes w_{8j+5 \rightarrow 8(j+1)}; \\
b_{2s+(j+1)_s,8s+(-1)_s} &= e_{8(j+m)+6} \otimes w_{8j+5 \rightarrow 8(j+1)}; \\
b_{(j+1)_s,9s+(-2)_s} &= w_{8(j+m)+2 \rightarrow 8(j+m)+4} \otimes w_{8j+5 \rightarrow 8(j+1)}; \\
b_{s+(j+1)_s,9s+(-2)_s} &= -e_{8(j+m)+4} \otimes w_{8j+5 \rightarrow 8(j+1)}; \\
b_{(j+1)_s,9s+(-1)_s} &= w_{8(j+m)+2 \rightarrow 8(j+m)+4} \otimes w_{8j+5 \rightarrow 8(j+1)}; \\
b_{s+(j+1)_s,9s+(-1)_s} &= -e_{8(j+m)+4} \otimes w_{8j+5 \rightarrow 8(j+1)}; \\
b_{4s+(j+1)_s,13s+(-2)_s} &= e_{8(j+m)+7} \otimes w_{8j+7 \rightarrow 8(j+1)+1}; \\
b_{4s+(j+1)_s,14s+(-2)_s} &= -w_{8(j+m)+7 \rightarrow 8(j+m)+2} \otimes w_{8j+7 \rightarrow 8(j+1)+1}.
\end{aligned}$$

(9) If  $r_0 = 8$ , then  $\Omega^8(Z_t^{(14)})$  is described with  $(16s \times 14s)$  matrix with the following nonzero entries:

$$\begin{aligned}
b_{j+5s,(-1)_s} &= w_{8(j+m)+1 \rightarrow 8(j+m)+2} \otimes w_{8j \rightarrow 8j+2}; \\
b_{j+6s,(-1)_s} &= e_{8(j+m)+2} \otimes w_{8j \rightarrow 8j+3}; \\
b_{j-s,s+(-1)_s} &= w_{8(j+m)+7 \rightarrow 8(j+m)+4} \otimes e_{8j}; \\
b_{j,s+(-1)_s} &= -w_{8(j+m)+7 \rightarrow 8(j+m)+4} \otimes e_{8j}; \\
b_{j+4s,s+(-1)_s} &= -w_{8(j+m)+1 \rightarrow 8(j+m)+4} \otimes w_{8j \rightarrow 8j+2}; \\
b_{j+6s,s+(-1)_s} &= -w_{8(j+m)+3 \rightarrow 8(j+m)+4} \otimes w_{8j \rightarrow 8j+4}; \\
b_{j+11s,s+(-1)_s} &= -e_{8(j+m)+4} \otimes w_{8j \rightarrow 8j+6}; \\
b_{j+s,2s+(-1)_s} &= -w_{8(j+m)+5 \rightarrow 8(j+m)+6} \otimes w_{8j \rightarrow 8j+1}; \\
b_{(j+1)_s,3s+(-2)_s} &= -e_{8(j+m)+7} \otimes w_{8j+1 \rightarrow 8(j+1)}; \\
b_{s+(j+1)_s,3s+(-2)_s} &= e_{8(j+m)+7} \otimes w_{8j+1 \rightarrow 8(j+1)}; \\
b_{(j+1)_s,3s+(-1)_s} &= -e_{8(j+m)+7} \otimes w_{8j+1 \rightarrow 8(j+1)}; \\
b_{(j+1)_s,4s+(-2)_s} &= w_{8(j+m)+7 \rightarrow 8(j+m)+1} \otimes w_{8j+2 \rightarrow 8(j+1)}; \\
b_{s+(j+1)_s,4s+(-2)_s} &= -w_{8(j+m)+7 \rightarrow 8(j+m)+1} \otimes w_{8j+2 \rightarrow 8(j+1)}; \\
b_{2s+(j+1)_s,4s+(-2)_s} &= e_{8(j+m)+1} \otimes w_{8j+2 \rightarrow 8(j+1)}; \\
b_{(j+1)_s,7s+(-2)_s} &= -e_{8(j+m)+7} \otimes w_{8j+5 \rightarrow 8(j+1)};
\end{aligned}$$

$$\begin{aligned}
b_{s+(j+1)s,7s+(-2)s} &= e_{8(j+m)+7} \otimes w_{8j+5 \rightarrow 8(j+1)}; \\
b_{(j+1)s,7s+(-1)s} &= -e_{8(j+m)+7} \otimes w_{8j+5 \rightarrow 8(j+1)}; \\
b_{s+(j+1)s,7s+(-1)s} &= e_{8(j+m)+7} \otimes w_{8j+5 \rightarrow 8(j+1)}; \\
b_{(j+1)s,8s+(-2)s} &= w_{8(j+m)+7 \rightarrow 8(j+m+1)} \otimes w_{8j+5 \rightarrow 8(j+1)}; \\
b_{s+(j+1)s,8s+(-2)s} &= -w_{8(j+m)+7 \rightarrow 8(j+m+1)} \otimes w_{8j+5 \rightarrow 8(j+1)}; \\
b_{2s+(j+1)s,8s+(-2)s} &= e_{8(j+m+1)} \otimes w_{8j+5 \rightarrow 8(j+1)}; \\
b_{(j+1)s,8s+(-1)s} &= w_{8(j+m)+7 \rightarrow 8(j+m+1)} \otimes w_{8j+5 \rightarrow 8(j+1)}; \\
b_{s+(j+1)s,8s+(-1)s} &= -w_{8(j+m)+7 \rightarrow 8(j+m+1)} \otimes w_{8j+5 \rightarrow 8(j+1)}; \\
b_{2s+(j+1)s,8s+(-1)s} &= e_{8(j+m+1)} \otimes w_{8j+5 \rightarrow 8(j+1)}; \\
b_{3s+(j+1)s,13s+(-2)s} &= -e_{8(j+m+1)+5} \otimes w_{8j+7 \rightarrow 8(j+1)+1}.
\end{aligned}$$

(10) If  $r_0 = 9$ , then  $\Omega^9(Z_t^{(14)})$  is described with  $(16s \times 13s)$  matrix with the following nonzero entries:

$$\begin{aligned}
b_{j+s,(-1)s} &= w_{8(j+m)+3 \rightarrow 8(j+m+1)} \otimes e_{8j}; \\
b_{j+2s,(-1)s} &= -w_{8(j+m)+6 \rightarrow 8(j+m+1)} \otimes e_{8j}; \\
b_{j+4s,(-1)s} &= -e_{8(j+m+1)} \otimes w_{8j \rightarrow 8j+1}; \\
b_{j+8s,(-1)s} &= w_{8(j+m)+7 \rightarrow 8(j+m+1)} \otimes w_{8j \rightarrow 8j+5}; \\
b_{j,s+(-1)s} &= w_{8(j+m)+3 \rightarrow 8(j+m)+7} \otimes e_{8j}; \\
b_{j+s,(-1)s} &= -w_{8(j+m)+6 \rightarrow 8(j+m)+7} \otimes e_{8j}; \\
b_{j+4s,s+(-1)s} &= e_{8(j+m)+7} \otimes w_{8j \rightarrow 8j+2}; \\
b_{j+7s,s+(-1)s} &= e_{8(j+m)+7} \otimes w_{8j \rightarrow 8j+5}; \\
b_{3s+(j+1)s,2s+(-2)s} &= w_{8(j+m+1)+1 \rightarrow 8(j+m+1)+3} \otimes w_{8j+1 \rightarrow 8(j+1)}; \\
b_{s+(j+1)s,2s+(-1)s} &= -e_{8(j+m+1)+3} \otimes w_{8j+1 \rightarrow 8(j+1)}; \\
b_{3s+(j+1)s,3s+(-2)s} &= w_{8(j+m+1)+1 \rightarrow 8(j+m+1)+4} \otimes w_{8j+2 \rightarrow 8(j+1)}; \\
b_{(j+1)s,4s+(-2)s} &= e_{8(j+m+1)+5} \otimes w_{8j+2 \rightarrow 8(j+1)}; \\
b_{3s+(j+1)s,7s+(-2)s} &= w_{8(j+m+1)+1 \rightarrow 8(j+m+1)+2} \otimes w_{8j+5 \rightarrow 8(j+1)}; \\
b_{3s+(j+1)s,7s+(-1)s} &= w_{8(j+m+1)+1 \rightarrow 8(j+m+1)+2} \otimes w_{8j+5 \rightarrow 8(j+1)}; \\
b_{(j+1)s,8s+(-2)s} &= e_{8(j+m+1)+5} \otimes w_{8j+5 \rightarrow 8(j+1)}; \\
b_{(j+1)s,8s+(-1)s} &= e_{8(j+m+1)+5} \otimes w_{8j+5 \rightarrow 8(j+1)}; \\
b_{4s+(j+1)s,12s+(-2)s} &= e_{8(j+m+2)} \otimes w_{8j+7 \rightarrow 8(j+1)+1}; \\
b_{5s+(j+1)s,12s+(-2)s} &= w_{8(j+m+1)+7 \rightarrow 8(j+m+2)} \otimes w_{8j+7 \rightarrow 8(j+1)+2}.
\end{aligned}$$

(11) If  $r_0 = 10$ , then  $\Omega^{10}(Z_t^{(14)})$  is described with  $(19s \times 11s)$  matrix with the following nonzero entries:

$$\begin{aligned}
b_{j+4s,(-1)s} &= -w_{8(j+m)+1 \rightarrow 8(j+m)+3} \otimes w_{8j \rightarrow 8j+1}; \\
b_{j+5s,(-1)s} &= -w_{8(j+m)+2 \rightarrow 8(j+m)+3} \otimes w_{8j \rightarrow 8j+2}; \\
b_{j+6s,(-1)s} &= e_{8(j+m)+3} \otimes w_{8j \rightarrow 8j+3}; \\
b_{j+s,s+(-1)s} &= -w_{8(j+m) \rightarrow 8(j+m)+5} \otimes e_{8j}; \\
b_{j+9s,s+(-1)s} &= e_{8(j+m)+5} \otimes w_{8j \rightarrow 8j+5}; \\
b_{s+(j+1)s,2s+(-2)s} &= -e_{8(j+m+1)} \otimes w_{8j+1 \rightarrow 8(j+1)}; \\
b_{2s+(j+1)s,2s+(-2)s} &= e_{8(j+m+1)} \otimes w_{8j+1 \rightarrow 8(j+1)}; \\
b_{s+(j+1)s,2s+(-1)s} &= -e_{8(j+m+1)} \otimes w_{8j+1 \rightarrow 8(j+1)};
\end{aligned}$$

$$\begin{aligned}
b_{(j+1)s, 3s+(-2)s} &= -e_{8(j+m)+7} \otimes w_{8j+2 \rightarrow 8(j+1)}; \\
b_{(j+1)s, 6s+(-2)s} &= -w_{8(j+m)+7 \rightarrow 8(j+m+1)} \otimes w_{8j+5 \rightarrow 8(j+1)}; \\
b_{s+(j+1)s, 6s+(-2)s} &= -e_{8(j+m+1)} \otimes w_{8j+5 \rightarrow 8(j+1)}; \\
b_{2s+(j+1)s, 6s+(-2)s} &= e_{8(j+m+1)} \otimes w_{8j+5 \rightarrow 8(j+1)}; \\
b_{(j+1)s, 6s+(-1)s} &= -w_{8(j+m)+7 \rightarrow 8(j+m+1)} \otimes w_{8j+5 \rightarrow 8(j+1)}; \\
b_{s+(j+1)s, 6s+(-1)s} &= -e_{8(j+m+1)} \otimes w_{8j+5 \rightarrow 8(j+1)}; \\
b_{2s+(j+1)s, 6s+(-1)s} &= e_{8(j+m+1)} \otimes w_{8j+5 \rightarrow 8(j+1)}; \\
b_{3s+(j+1)s, 10s+(-2)s} &= e_{8(j+m+1)+6} \otimes w_{8j+7 \rightarrow 8(j+1)+1}.
\end{aligned}$$

(12) If  $r_0 = 11$ , then  $\Omega^{11}(Z_t^{(14)})$  is described with  $(18s \times 11s)$  matrix with the following nonzero entries:

$$\begin{aligned}
b_{j+2s, (-1)s} &= -w_{8(j+m)+4 \rightarrow 8(j+m+1)} \otimes e_{8j}; \\
b_{j+3s, (-1)s} &= w_{8(j+m)+1 \rightarrow 8(j+m+1)} \otimes e_{8j}; \\
b_{j+4s, (-1)s} &= w_{8(j+m)+5 \rightarrow 8(j+m+1)} \otimes e_{8j}; \\
b_{j+6s, (-1)s} &= -e_{8(j+m+1)} \otimes w_{8j \rightarrow 8j+2}; \\
b_{j+7s, (-1)s} &= w_{8(j+m)+7 \rightarrow 8(j+m+1)} \otimes w_{8j \rightarrow 8j+3}; \\
b_{j+8s, (-1)s} &= -w_{8(j+m)+7 \rightarrow 8(j+m+1)} \otimes w_{8j \rightarrow 8j+4}; \\
b_{j+11s, (-1)s} &= -e_{8(j+m+1)} \otimes w_{8j \rightarrow 8j+5}; \\
b_{(j+1)s, s+(-2)s} &= -w_{8(j+m+1)+2 \rightarrow 8(j+m+1)+4} \otimes w_{8j+1 \rightarrow 8(j+1)}; \\
b_{3s+(j+1)s, s+(-2)s} &= w_{8(j+m+1)+1 \rightarrow 8(j+m+1)+4} \otimes w_{8j+1 \rightarrow 8(j+1)}; \\
b_{2s+(j+1)s, s+(-1)s} &= -e_{8(j+m+1)+4} \otimes w_{8j+1 \rightarrow 8(j+1)}; \\
b_{4s+(j+1)s, 2s+(-2)s} &= -e_{8(j+m+1)+5} \otimes w_{8j+1 \rightarrow 8(j+1)}; \\
b_{4s+(j+1)s, 2s+(-1)s} &= -e_{8(j+m+1)+5} \otimes w_{8j+1 \rightarrow 8(j+1)}; \\
b_{s+(j+1)s, 3s+(-2)s} &= -e_{8(j+m+1)+6} \otimes w_{8j+2 \rightarrow 8(j+1)}; \\
b_{(j+1)s, 6s+(-2)s} &= -w_{8(j+m+1)+2 \rightarrow 8(j+m+1)+3} \otimes w_{8j+5 \rightarrow 8(j+1)}; \\
b_{3s+(j+1)s, 6s+(-2)s} &= w_{8(j+m+1)+1 \rightarrow 8(j+m+1)+3} \otimes w_{8j+5 \rightarrow 8(j+1)}; \\
b_{(j+1)s, 6s+(-1)s} &= -w_{8(j+m+1)+2 \rightarrow 8(j+m+1)+3} \otimes w_{8j+5 \rightarrow 8(j+1)}; \\
b_{3s+(j+1)s, 6s+(-1)s} &= w_{8(j+m+1)+1 \rightarrow 8(j+m+1)+3} \otimes w_{8j+5 \rightarrow 8(j+1)}; \\
b_{s+(j+1)s, 7s+(-2)s} &= -e_{8(j+m+1)+6} \otimes w_{8j+5 \rightarrow 8(j+1)}; \\
b_{4s+(j+1)s, 7s+(-2)s} &= -w_{8(j+m+1)+5 \rightarrow 8(j+m+1)+6} \otimes w_{8j+5 \rightarrow 8(j+1)}; \\
b_{s+(j+1)s, 7s+(-1)s} &= -e_{8(j+m+1)+6} \otimes w_{8j+5 \rightarrow 8(j+1)}; \\
b_{4s+(j+1)s, 7s+(-1)s} &= -w_{8(j+m+1)+5 \rightarrow 8(j+m+1)+6} \otimes w_{8j+5 \rightarrow 8(j+1)}; \\
b_{5s+(j+1)s, 10s+(-2)s} &= -e_{8(j+m+1)+7} \otimes w_{8j+7 \rightarrow 8(j+1)+1}.
\end{aligned}$$

(13) If  $r_0 = 12$ , then  $\Omega^{12}(Z_t^{(14)})$  is described with  $(19s \times 10s)$  matrix with the following nonzero entries:

$$\begin{aligned}
b_{j+2s, (-1)s} &= -w_{8(j+m-1)+7 \rightarrow 8(j+m)+4} \otimes e_{8j}; \\
b_{j+4s, (-1)s} &= -w_{8(j+m)+3 \rightarrow 8(j+m)+4} \otimes w_{8j \rightarrow 8j+2}; \\
b_{j+6s, (-1)s} &= e_{8(j+m)+4} \otimes w_{8j \rightarrow 8j+3}; \\
b_{j+10s, (-1)s} &= -w_{8(j+m)+2 \rightarrow 8(j+m)+4} \otimes w_{8j \rightarrow 8j+5}; \\
b_{j, s+(-1)s} &= w_{8(j+m) \rightarrow 8(j+m)+6} \otimes e_{8j}; \\
b_{j+s, s+(-1)s} &= -w_{8(j+m-1)+7 \rightarrow 8(j+m)+6} \otimes e_{8j};
\end{aligned}$$



$$\begin{aligned}
b_{j+7s,s+(-1)_s} &= w_{8(j+m)+5 \rightarrow 8(j+m)+6} \otimes w_{8j \rightarrow 8j+4}; \\
b_{j+10s,s+(-1)_s} &= -e_{8(j+m)+6} \otimes w_{8j \rightarrow 8j+5}; \\
b_{(j+1)_s,2s+(-2)_s} &= -e_{8(j+m)+7} \otimes w_{8j+1 \rightarrow 8(j+1)}; \\
b_{2s+(j+1)_s,2s+(-1)_s} &= -e_{8(j+m)+7} \otimes w_{8j+1 \rightarrow 8(j+1)}; \\
b_{(j+1)_s,3s+(-2)_s} &= w_{8(j+m)+7 \rightarrow 8(j+m+1)} \otimes w_{8j+2 \rightarrow 8(j+1)}; \\
b_{s+(j+1)_s,3s+(-2)_s} &= -e_{8(j+m+1)} \otimes w_{8j+2 \rightarrow 8(j+1)}; \\
b_{(j+1)_s,4s+(-2)_s} &= -w_{8(j+m)+7 \rightarrow 8(j+m+1)+1} \otimes w_{8j+3 \rightarrow 8(j+1)}; \\
b_{s+(j+1)_s,4s+(-2)_s} &= w_{8(j+m+1) \rightarrow 8(j+m+1)+1} \otimes w_{8j+3 \rightarrow 8(j+1)}; \\
b_{2s+(j+1)_s,5s+(-2)_s} &= w_{8(j+m)+7 \rightarrow 8(j+m+1)+2} \otimes w_{8j+4 \rightarrow 8(j+1)}; \\
b_{3s+(j+1)_s,5s+(-2)_s} &= e_{8(j+m+1)+2} \otimes w_{8j+4 \rightarrow 8(j+1)+1}; \\
b_{(j+1)_s,6s+(-2)_s} &= -e_{8(j+m)+7} \otimes w_{8j+5 \rightarrow 8(j+1)}; \\
b_{(j+1)_s,6s+(-1)_s} &= -e_{8(j+m)+7} \otimes w_{8j+5 \rightarrow 8(j+1)}; \\
b_{2s+(j+1)_s,8s+(-2)_s} &= w_{8(j+m)+7 \rightarrow 8(j+m+1)+3} \otimes w_{8j+7 \rightarrow 8(j+1)}; \\
b_{3s+(j+1)_s,8s+(-2)_s} &= w_{8(j+m+1)+2 \rightarrow 8(j+m+1)+3} \otimes w_{8j+7 \rightarrow 8(j+1)+1}; \\
b_{10s+(j+1)_s,8s+(-2)_s} &= w_{8(j+m+1)+2 \rightarrow 8(j+m+1)+3} \otimes w_{8j+7 \rightarrow 8(j+1)+5}.
\end{aligned}$$

(14) If  $r_0 = 13$ , then  $\Omega^{13}(Z_t^{(14)})$  is described with  $(18s \times 8s)$  matrix with the following nonzero entries:

$$\begin{aligned}
b_{j+3s,(-1)_s} &= -w_{8(j+m)+5 \rightarrow 8(j+m)+7} \otimes e_{8j}; \\
b_{j+5s,(-1)_s} &= -e_{8(j+m)+7} \otimes w_{8j \rightarrow 8j+2}; \\
b_{j+9s,(-1)_s} &= -e_{8(j+m)+7} \otimes w_{8j \rightarrow 8j+5}; \\
b_{2s+(j+1)_s,s+(-2)_s} &= -e_{8(j+m+1)+6} \otimes w_{8j+1 \rightarrow 8(j+1)}; \\
b_{2s+(j+1)_s,s+(-1)_s} &= -e_{8(j+m+1)+6} \otimes w_{8j+1 \rightarrow 8(j+1)}; \\
b_{(j+1)_s,3s+(-2)_s} &= -e_{8(j+m+1)+2} \otimes w_{8j+3 \rightarrow 8(j+1)}; \\
b_{s+(j+1)_s,5s+(-2)_s} &= -w_{8(j+m+1)+3 \rightarrow 8(j+m+1)+4} \otimes w_{8j+5 \rightarrow 8(j+1)}; \\
b_{s+(j+1)_s,5s+(-1)_s} &= -w_{8(j+m+1)+3 \rightarrow 8(j+m+1)+4} \otimes w_{8j+5 \rightarrow 8(j+1)}; \\
b_{4s+(j+1)_s,7s+(-2)_s} &= e_{8(j+m+2)} \otimes w_{8j+7 \rightarrow 8(j+1)+1}; \\
b_{5s+(j+1)_s,7s+(-2)_s} &= -w_{8(j+m+1)+7 \rightarrow 8(j+m+2)} \otimes w_{8j+7 \rightarrow 8(j+1)+2}.
\end{aligned}$$

(15) If  $r_0 = 14$ , then  $\Omega^{14}(Z_t^{(14)})$  is described with  $(20s \times 9s)$  matrix with the following nonzero entries:

$$\begin{aligned}
b_{(j+1)_s,(-2)_s} &= e_{8(j+m)+7} \otimes w_{8j \rightarrow 8(j+1)}; \\
b_{(j+1)_s,(-1)_s} &= e_{8(j+m)+7} \otimes w_{8j \rightarrow 8(j+1)}; \\
b_{j+3s,(-1)_s} &= -w_{8(j+m)+3 \rightarrow 8(j+m)+7} \otimes w_{8j \rightarrow 8j+1}; \\
b_{j+4s,(-1)_s} &= w_{8(j+m)+5 \rightarrow 8(j+m)+7} \otimes w_{8j \rightarrow 8j+1}; \\
b_{j+12s,(-1)_s} &= -w_{8(j+m)+3 \rightarrow 8(j+m)+7} \otimes w_{8j \rightarrow 8j+5}; \\
b_{(j+1)_s,s+(-2)_s} &= -w_{8(j+m)+7 \rightarrow 8(j+m+1)} \otimes w_{8j+1 \rightarrow 8(j+1)}; \\
b_{s+(j+1)_s,s+(-2)_s} &= -e_{8(j+m+1)} \otimes w_{8j+1 \rightarrow 8(j+1)}; \\
b_{2s+(j+1)_s,s+(-1)_s} &= -e_{8(j+m+1)} \otimes w_{8j+1 \rightarrow 8(j+1)}; \\
b_{(j+1)_s,2s+(-2)_s} &= w_{8(j+m)+7 \rightarrow 8(j+m+1)+1} \otimes w_{8j+2 \rightarrow 8(j+1)}; \\
b_{s+(j+1)_s,2s+(-2)_s} &= w_{8(j+m+1) \rightarrow 8(j+m+1)+1} \otimes w_{8j+2 \rightarrow 8(j+1)}; \\
b_{(j+1)_s,3s+(-2)_s} &= -w_{8(j+m)+7 \rightarrow 8(j+m+1)+2} \otimes w_{8j+3 \rightarrow 8(j+1)};
\end{aligned}$$

$$\begin{aligned}
b_{s+(j+1)s,3s+(-2)s} &= -w_{8(j+m+1) \rightarrow 8(j+m+1)+2} \otimes w_{8j+3 \rightarrow 8(j+1)}; \\
b_{2s+(j+1)s,3s+(-2)s} &= w_{8(j+m+1) \rightarrow 8(j+m+1)+2} \otimes w_{8j+3 \rightarrow 8(j+1)}; \\
b_{3s+(j+1)s,4s+(-2)s} &= e_{8(j+m+1)+3} \otimes w_{8j+4 \rightarrow 8(j+1)+1}; \\
b_{s+(j+1)s,5s+(-2)s} &= -e_{8(j+m+1)} \otimes w_{8j+5 \rightarrow 8(j+1)}; \\
b_{s+(j+1)s,5s+(-1)s} &= -e_{8(j+m+1)} \otimes w_{8j+5 \rightarrow 8(j+1)}; \\
b_{3s+(j+1)s,7s+(-2)s} &= w_{8(j+m+1)+3 \rightarrow 8(j+m+1)+4} \otimes w_{8j+7 \rightarrow 8(j+1)+1}; \\
b_{12s+(j+1)s,7s+(-2)s} &= w_{8(j+m+1)+3 \rightarrow 8(j+m+1)+4} \otimes w_{8j+7 \rightarrow 8(j+1)+5}; \\
b_{4s+(j+1)s,8s+(-2)s} &= w_{8(j+m+1)+5 \rightarrow 8(j+m+1)+6} \otimes w_{8j+7 \rightarrow 8(j+1)+1}.
\end{aligned}$$

(16) If  $r_0 = 15$ , then  $\Omega^{15}(Z_t^{(14)})$  is described with  $(18s \times 8s)$  matrix with the following nonzero entries:

$$\begin{aligned}
b_{j+5s,(-1)s} &= -w_{8(j+m)+7 \rightarrow 8(j+m+1)} \otimes w_{8j \rightarrow 8j+1}; \\
b_{j+7s,(-1)s} &= -e_{8(j+m+1)} \otimes w_{8j \rightarrow 8j+2}; \\
b_{j+11s,(-1)s} &= -e_{8(j+m+1)} \otimes w_{8j \rightarrow 8j+5}; \\
b_{3s+(j+1)s,s+(-1)s} &= -e_{8(j+m+1)+1} \otimes w_{8j+1 \rightarrow 8(j+1)}; \\
b_{3s+(j+1)s,2s+(-2)s} &= w_{8(j+m+1)+1 \rightarrow 8(j+m+1)+2} \otimes w_{8j+2 \rightarrow 8(j+1)}; \\
b_{(j+1)s,3s+(-2)s} &= -e_{8(j+m+1)+3} \otimes w_{8j+3 \rightarrow 8(j+1)}; \\
b_{3s+(j+1)s,3s+(-2)s} &= w_{8(j+m+1)+1 \rightarrow 8(j+m+1)+3} \otimes w_{8j+3 \rightarrow 8(j+1)}; \\
b_{4s+(j+1)s,5s+(-2)s} &= -e_{8(j+m+1)+5} \otimes w_{8j+5 \rightarrow 8(j+1)}; \\
b_{4s+(j+1)s,5s+(-1)s} &= -e_{8(j+m+1)+5} \otimes w_{8j+5 \rightarrow 8(j+1)}.
\end{aligned}$$

(17) If  $r_0 = 16$ , then  $\Omega^{16}(Z_t^{(14)})$  is described with  $(19s \times 8s)$  matrix with the following nonzero entries:

$$\begin{aligned}
b_{2s+(j+1)s,(-2)s} &= w_{8(j+m)+7 \rightarrow 8(j+m+1)} \otimes w_{8j \rightarrow 8(j+1)}; \\
b_{j+3s,(-2)s} &= w_{8(j+m)+4 \rightarrow 8(j+m+1)} \otimes w_{8j \rightarrow 8j+1}; \\
b_{(j+1)s,(-1)s} &= -w_{8(j+m)+7 \rightarrow 8(j+m+1)} \otimes w_{8j \rightarrow 8(j+1)}; \\
b_{2s+(j+1)s,(-1)s} &= 2w_{8(j+m)+7 \rightarrow 8(j+m+1)} \otimes w_{8j \rightarrow 8(j+1)}; \\
b_{j+3s,(-1)s} &= w_{8(j+m)+4 \rightarrow 8(j+m+1)} \otimes w_{8j \rightarrow 8j+1}; \\
b_{j+4s,(-1)s} &= -w_{8(j+m)+6 \rightarrow 8(j+m+1)} \otimes w_{8j \rightarrow 8j+1}; \\
b_{j+11s,(-1)s} &= -w_{8(j+m)+4 \rightarrow 8(j+m+1)} \otimes w_{8j \rightarrow 8j+5}; \\
b_{s+(j+1)s,s+(-2)s} &= -w_{8(j+m+1) \rightarrow 8(j+m+1)+1} \otimes w_{8j+1 \rightarrow 8(j+1)}; \\
b_{2s+(j+1)s,s+(-2)s} &= -w_{8(j+m)+7 \rightarrow 8(j+m+1)+1} \otimes w_{8j+1 \rightarrow 8(j+1)}; \\
b_{(j+1)s,s+(-1)s} &= w_{8(j+m)+7 \rightarrow 8(j+m+1)+1} \otimes w_{8j+1 \rightarrow 8(j+1)}; \\
b_{s+(j+1)s,s+(-1)s} &= -w_{8(j+m+1) \rightarrow 8(j+m+1)+1} \otimes w_{8j+1 \rightarrow 8(j+1)}; \\
b_{2s+(j+1)s,s+(-1)s} &= -w_{8(j+m)+7 \rightarrow 8(j+m+1)+1} \otimes w_{8j+1 \rightarrow 8(j+1)}; \\
b_{s+(j+1)s,2s+(-2)s} &= w_{8(j+m+1) \rightarrow 8(j+m+1)+2} \otimes w_{8j+2 \rightarrow 8(j+1)}; \\
b_{2s+(j+1)s,2s+(-2)s} &= w_{8(j+m)+7 \rightarrow 8(j+m+1)+2} \otimes w_{8j+2 \rightarrow 8(j+1)}; \\
b_{(j+1)s,3s+(-2)s} &= -w_{8(j+m)+7 \rightarrow 8(j+m+1)+3} \otimes w_{8j+3 \rightarrow 8(j+1)}; \\
b_{6s+(j+1)s,3s+(-2)s} &= -w_{8(j+m+1)+1 \rightarrow 8(j+m+1)+3} \otimes w_{8j+3 \rightarrow 8(j+1)+2}; \\
b_{3s+(j+1)s,4s+(-2)s} &= e_{8(j+m+1)+4} \otimes w_{8j+4 \rightarrow 8(j+1)+1}; \\
b_{6s+(j+1)s,4s+(-2)s} &= w_{8(j+m+1)+1 \rightarrow 8(j+m+1)+4} \otimes w_{8j+4 \rightarrow 8(j+1)+2}; \\
b_{s+(j+1)s,5s+(-2)s} &= w_{8(j+m+1) \rightarrow 8(j+m+1)+5} \otimes w_{8j+5 \rightarrow 8(j+1)};
\end{aligned}$$

$$\begin{aligned}
b_{2s+(j+1)_s, 5s+(-2)_s} &= w_{8(j+m)+7 \rightarrow 8(j+m+1)+5} \otimes w_{8j+5 \rightarrow 8(j+1)}; \\
b_{2s+(j+1)_s, 5s+(-1)_s} &= w_{8(j+m)+7 \rightarrow 8(j+m+1)+5} \otimes w_{8j+5 \rightarrow 8(j+1)}; \\
b_{12s+(j+1)_s, 6s+(-2)_s} &= -w_{8(j+m+1)+5 \rightarrow 8(j+m+1)+6} \otimes w_{8j+6 \rightarrow 8(j+1)+5}; \\
b_{4s+(j+1)_s, 7s+(-2)_s} &= w_{8(j+m+1)+6 \rightarrow 8(j+m+1)+7} \otimes w_{8j+7 \rightarrow 8(j+1)+1}; \\
b_{11s+(j+1)_s, 7s+(-2)_s} &= w_{8(j+m+1)+4 \rightarrow 8(j+m+1)+7} \otimes w_{8j+7 \rightarrow 8(j+1)+5}.
\end{aligned}$$

(18) If  $r_0 = 17$ , then  $\Omega^{17}(Z_t^{(14)})$  is described with  $(18s \times 9s)$  matrix with the following nonzero entries:

$$\begin{aligned}
b_{j+4s, (-2)_s} &= -w_{8(j+m)+7 \rightarrow 8(j+m+1)+1} \otimes w_{8j \rightarrow 8j+1}; \\
b_{j+5s, (-2)_s} &= -w_{8(j+m+1) \rightarrow 8(j+m+1)+1} \otimes w_{8j \rightarrow 8j+1}; \\
b_{j+4s, (-1)_s} &= -w_{8(j+m)+7 \rightarrow 8(j+m+1)+1} \otimes w_{8j \rightarrow 8j+1}; \\
b_{j+5s, (-1)_s} &= -w_{8(j+m+1) \rightarrow 8(j+m+1)+1} \otimes w_{8j \rightarrow 8j+1}; \\
b_{j+10s, (-1)_s} &= w_{8(j+m)+7 \rightarrow 8(j+m+1)+1} \otimes w_{8j \rightarrow 8j+5}; \\
b_{3s+(j+1)_s, s+(-2)_s} &= -e_{8(j+m+1)+5} \otimes w_{8j \rightarrow 8(j+1)}; \\
b_{j+3s, s+(-1)_s} &= w_{8(j+m)+7 \rightarrow 8(j+m+1)+5} \otimes w_{8j \rightarrow 8j+1}; \\
b_{(j+1)_s, 2s+(-1)_s} &= -e_{8(j+m+1)+2} \otimes w_{8j+1 \rightarrow 8(j+1)}; \\
b_{(j+1)_s, 3s+(-2)_s} &= w_{8(j+m+1)+2 \rightarrow 8(j+m+1)+3} \otimes w_{8j+2 \rightarrow 8(j+1)}; \\
b_{s+(j+1)_s, 4s+(-2)_s} &= e_{8(j+m+1)+4} \otimes w_{8j+3 \rightarrow 8(j+1)}; \\
b_{4s+(j+1)_s, 5s+(-2)_s} &= e_{8(j+m+1)+7} \otimes w_{8j+4 \rightarrow 8(j+1)+1}; \\
b_{2s+(j+1)_s, 6s+(-2)_s} &= -e_{8(j+m+1)+6} \otimes w_{8j+5 \rightarrow 8(j+1)}; \\
b_{3s+(j+1)_s, 6s+(-2)_s} &= -w_{8(j+m+1)+5 \rightarrow 8(j+m+1)+6} \otimes w_{8j+5 \rightarrow 8(j+1)}; \\
b_{2s+(j+1)_s, 6s+(-1)_s} &= -e_{8(j+m+1)+6} \otimes w_{8j+5 \rightarrow 8(j+1)}; \\
b_{10s+(j+1)_s, 7s+(-2)_s} &= -e_{8(j+m+1)+7} \otimes w_{8j+6 \rightarrow 8(j+1)+5}; \\
b_{4s+(j+1)_s, 8s+(-2)_s} &= -w_{8(j+m+1)+7 \rightarrow 8(j+m+2)} \otimes w_{8j+7 \rightarrow 8(j+1)+1}; \\
b_{5s+(j+1)_s, 8s+(-2)_s} &= -e_{8(j+m+2)} \otimes w_{8j+7 \rightarrow 8(j+1)+1}; \\
b_{4s+(j+1)_s, 8s+(-3)_s} &= -w_{8(j+m+1)+7 \rightarrow 8(j+m+2)} \otimes w_{8j+7 \rightarrow 8(j+1)+1}; \\
b_{5s+(j+1)_s, 8s+(-3)_s} &= -e_{8(j+m+2)} \otimes w_{8j+7 \rightarrow 8(j+1)+1}.
\end{aligned}$$

(19) If  $r_0 = 18$ , then  $\Omega^{18}(Z_t^{(14)})$  is described with  $(19s \times 8s)$  matrix with the following nonzero entries:

$$\begin{aligned}
b_{(j+1)_s, (-2)_s} &= -e_{8(j+m)+7} \otimes w_{8j \rightarrow 8(j+1)}; \\
b_{j+3s, (-2)_s} &= w_{8(j+m)+5 \rightarrow 8(j+m)+7} \otimes w_{8j \rightarrow 8j+1}; \\
b_{j+4s, (-1)_s} &= w_{8(j+m)+1 \rightarrow 8(j+m)+7} \otimes w_{8j \rightarrow 8j+1}; \\
b_{j+5s, (-1)_s} &= w_{8(j+m)+2 \rightarrow 8(j+m)+7} \otimes w_{8j \rightarrow 8j+2}; \\
b_{j+11s, (-1)_s} &= -w_{8(j+m)+6 \rightarrow 8(j+m)+7} \otimes w_{8j \rightarrow 8j+5}; \\
b_{(j+1)_s, s+(-2)_s} &= w_{8(j+m)+7 \rightarrow 8(j+m+1)+2} \otimes w_{8j+1 \rightarrow 8(j+1)}; \\
b_{(j+1)_s, s+(-1)_s} &= w_{8(j+m)+7 \rightarrow 8(j+m+1)+2} \otimes w_{8j+1 \rightarrow 8(j+1)}; \\
b_{s+(j+1)_s, s+(-1)_s} &= w_{8(j+m+1) \rightarrow 8(j+m+1)+2} \otimes w_{8j+1 \rightarrow 8(j+1)}; \\
b_{2s+(j+1)_s, s+(-1)_s} &= -w_{8(j+m+1) \rightarrow 8(j+m+1)+2} \otimes w_{8j+1 \rightarrow 8(j+1)}; \\
b_{(j+1)_s, 2s+(-2)_s} &= -w_{8(j+m)+7 \rightarrow 8(j+m+1)+3} \otimes w_{8j+2 \rightarrow 8(j+1)}; \\
b_{s+(j+1)_s, 3s+(-2)_s} &= -w_{8(j+m+1) \rightarrow 8(j+m+1)+4} \otimes w_{8j+3 \rightarrow 8(j+1)}; \\
b_{2s+(j+1)_s, 3s+(-2)_s} &= w_{8(j+m+1) \rightarrow 8(j+m+1)+4} \otimes w_{8j+3 \rightarrow 8(j+1)};
\end{aligned}$$

$$\begin{aligned}
b_{5s+(j+1)s, 3s+(-2)s} &= w_{8(j+m+1)+2 \rightarrow 8(j+m+1)+4} \otimes w_{8j+3 \rightarrow 8(j+1)+2}; \\
b_{3s+(j+1)s, 4s+(-2)s} &= -e_{8(j+m+1)+5} \otimes w_{8j+4 \rightarrow 8(j+1)+1}; \\
b_{3s+(j+1)s, 4s+(-3)s} &= -e_{8(j+m+1)+5} \otimes w_{8j+4 \rightarrow 8(j+1)+1}; \\
b_{(j+1)s, 5s+(-2)s} &= w_{8(j+m)+7 \rightarrow 8(j+m+1)+6} \otimes w_{8j+5 \rightarrow 8(j+1)}; \\
b_{2s+(j+1)s, 5s+(-1)s} &= w_{8(j+m+1) \rightarrow 8(j+m+1)+6} \otimes w_{8j+5 \rightarrow 8(j+1)}.
\end{aligned}$$

(20) If  $r_0 = 19$ , then  $\Omega^{19}(Z_t^{(14)})$  is described with  $(16s \times 10s)$  matrix with the following nonzero entries:

$$\begin{aligned}
b_{j+4s, (-1)s} &= w_{8(j+m+1) \rightarrow 8(j+m+1)+2} \otimes w_{8j \rightarrow 8j+1}; \\
b_{j+8s, s+(-1)s} &= -w_{8(j+m+1) \rightarrow 8(j+m+1)+6} \otimes w_{8j \rightarrow 8j+5}; \\
b_{(j+1)s, 2s+(-1)s} &= -e_{8(j+m+1)+3} \otimes w_{8j+1 \rightarrow 8(j+1)}; \\
b_{2s+(j+1)s, 2s+(-1)s} &= w_{8(j+m+1)+1 \rightarrow 8(j+m+1)+3} \otimes w_{8j+1 \rightarrow 8(j+1)}; \\
b_{(j+1)s, 3s+(-2)s} &= w_{8(j+m+1)+3 \rightarrow 8(j+m+1)+4} \otimes w_{8j+2 \rightarrow 8(j+1)}; \\
b_{2s+(j+1)s, 3s+(-2)s} &= -w_{8(j+m+1)+1 \rightarrow 8(j+m+1)+4} \otimes w_{8j+2 \rightarrow 8(j+1)}; \\
b_{2s+(j+1)s, 4s+(-2)s} &= w_{8(j+m+1)+1 \rightarrow 8(j+m+1)+7} \otimes w_{8j+3 \rightarrow 8(j+1)}; \\
b_{3s+(j+1)s, 4s+(-2)s} &= -w_{8(j+m+1)+5 \rightarrow 8(j+m+1)+7} \otimes w_{8j+3 \rightarrow 8(j+1)}; \\
b_{4s+(j+1)s, 5s+(-2)s} &= e_{8(j+m+2)} \otimes w_{8j+4 \rightarrow 8(j+1)+1}; \\
b_{s+(j+1)s, 6s+(-2)s} &= -w_{8(j+m+1)+6 \rightarrow 8(j+m+1)+7} \otimes w_{8j+5 \rightarrow 8(j+1)}; \\
b_{2s+(j+1)s, 6s+(-2)s} &= -w_{8(j+m+1)+1 \rightarrow 8(j+m+1)+7} \otimes w_{8j+5 \rightarrow 8(j+1)}; \\
b_{2s+(j+1)s, 6s+(-1)s} &= -w_{8(j+m+1)+1 \rightarrow 8(j+m+1)+7} \otimes w_{8j+5 \rightarrow 8(j+1)}; \\
b_{4s+(j+1)s, 8s+(-2)s} &= w_{8(j+m+2) \rightarrow 8(j+m+2)+1} \otimes w_{8j+7 \rightarrow 8(j+1)+1}.
\end{aligned}$$

(21) If  $r_0 = 20$ , then  $\Omega^{20}(Z_t^{(14)})$  is described with  $(16s \times 11s)$  matrix with the following nonzero entries:

$$\begin{aligned}
b_{(j+1)s, (-2)s} &= e_{8(j+m)+7} \otimes w_{8j \rightarrow 8(j+1)}; \\
b_{(j+1)s, (-1)s} &= e_{8(j+m)+7} \otimes w_{8j \rightarrow 8(j+1)}; \\
b_{j+3s, (-1)s} &= w_{8(j+m)+6 \rightarrow 8(j+m)+7} \otimes w_{8j \rightarrow 8j+1}; \\
b_{j+10s, (-1)s} &= -w_{8(j+m)+1 \rightarrow 8(j+m)+7} \otimes w_{8j \rightarrow 8j+5}; \\
b_{(j+1)s, s+(-2)s} &= w_{8(j+m)+7 \rightarrow 8(j+m+1)} \otimes w_{8j \rightarrow 8(j+1)}; \\
b_{s+(j+1)s, s+(-2)s} &= -e_{8(j+m+1)} \otimes w_{8j \rightarrow 8(j+1)}; \\
b_{(j+1)s, s+(-1)s} &= w_{8(j+m)+7 \rightarrow 8(j+m+1)} \otimes w_{8j \rightarrow 8(j+1)}; \\
b_{s+(j+1)s, s+(-1)s} &= -e_{8(j+m+1)} \otimes w_{8j \rightarrow 8(j+1)}; \\
b_{j+6s, s+(-1)s} &= -w_{8(j+m)+6 \rightarrow 8(j+m+1)} \otimes w_{8j \rightarrow 8j+4}; \\
b_{j+7s, s+(-1)s} &= -w_{8(j+m)+6 \rightarrow 8(j+m+1)} \otimes w_{8j \rightarrow 8j+5}; \\
b_{s+(j+1)s, 2s+(-2)s} &= w_{8(j+m+1) \rightarrow 8(j+m+1)+3} \otimes w_{8j+1 \rightarrow 8(j+1)}; \\
b_{(j+1)s, 2s+(-1)s} &= w_{8(j+m)+7 \rightarrow 8(j+m+1)+3} \otimes w_{8j+1 \rightarrow 8(j+1)}; \\
b_{s+(j+1)s, 3s+(-2)s} &= -w_{8(j+m+1) \rightarrow 8(j+m+1)+4} \otimes w_{8j+2 \rightarrow 8(j+1)}; \\
b_{s+(j+1)s, 4s+(-2)s} &= -w_{8(j+m+1) \rightarrow 8(j+m+1)+5} \otimes w_{8j+3 \rightarrow 8(j+1)}; \\
b_{6s+(j+1)s, 4s+(-2)s} &= -e_{8(j+m+1)+5} \otimes w_{8j+3 \rightarrow 8(j+1)+3}; \\
b_{3s+(j+1)s, 5s+(-2)s} &= -e_{8(j+m+1)+6} \otimes w_{8j+4 \rightarrow 8(j+1)+1}; \\
b_{j+3s, 7s+(-2)s} &= -w_{8(j+m)+1 \rightarrow 8(j+m+1)+1} \otimes e_{8j+5}; \\
b_{j+3s, 7s+(-1)s} &= -w_{8(j+m)+1 \rightarrow 8(j+m+1)+1} \otimes e_{8j+5}.
\end{aligned}$$

(22) If  $r_0 = 21$ , then  $\Omega^{21}(Z_t^{(14)})$  is described with  $(14s \times 11s)$  matrix with the following nonzero entries:

$$\begin{aligned}
b_{j+2s,(-1)_s} &= -w_{8(j+m)+6 \rightarrow 8(j+m+1)+5} \otimes e_{8j}; \\
b_{j+4s,(-1)_s} &= -w_{8(j+m+1) \rightarrow 8(j+m+1)+5} \otimes w_{8j \rightarrow 8j+2}; \\
b_{j+5s,(-1)_s} &= -w_{8(j+m)+7 \rightarrow 8(j+m+1)+5} \otimes w_{8j \rightarrow 8j+3}; \\
b_{j+6s,(-1)_s} &= -w_{8(j+m+1) \rightarrow 8(j+m+1)+5} \otimes w_{8j \rightarrow 8j+4}; \\
b_{j+9s,(-1)_s} &= -w_{8(j+m+1) \rightarrow 8(j+m+1)+5} \otimes w_{8j \rightarrow 8j+6}; \\
b_{(j+1)_s, s+(-2)_s} &= w_{8(j+m+1)+2 \rightarrow 8(j+m+1)+3} \otimes w_{8j \rightarrow 8(j+1)}; \\
b_{j-2s, 2s+(-2)_s} &= w_{8(j+m)+2 \rightarrow 8(j+m+1)+1} \otimes e_{8j}; \\
b_{j+s, 2s+(-2)_s} &= w_{8(j+m)+7 \rightarrow 8(j+m+1)+1} \otimes w_{8j \rightarrow 8j+1}; \\
b_{j+2s, 2s+(-2)_s} &= w_{8(j+m+1) \rightarrow 8(j+m+1)+1} \otimes w_{8j \rightarrow 8j+2}; \\
b_{j+3s, 2s+(-2)_s} &= w_{8(j+m)+7 \rightarrow 8(j+m+1)+1} \otimes w_{8j \rightarrow 8j+3}; \\
b_{j+4s, 2s+(-2)_s} &= w_{8(j+m+1) \rightarrow 8(j+m+1)+1} \otimes w_{8j \rightarrow 8j+4}; \\
b_{j+7s, 2s+(-2)_s} &= w_{8(j+m+1) \rightarrow 8(j+m+1)+1} \otimes w_{8j \rightarrow 8j+6}; \\
b_{j-2s, 2s+(-1)_s} &= w_{8(j+m)+2 \rightarrow 8(j+m+1)+1} \otimes e_{8j}; \\
b_{j+s, 2s+(-1)_s} &= w_{8(j+m)+7 \rightarrow 8(j+m+1)+1} \otimes w_{8j \rightarrow 8j+1}; \\
b_{j+2s, 2s+(-1)_s} &= w_{8(j+m+1) \rightarrow 8(j+m+1)+1} \otimes w_{8j \rightarrow 8j+2}; \\
b_{j+3s, 2s+(-1)_s} &= w_{8(j+m)+7 \rightarrow 8(j+m+1)+1} \otimes w_{8j \rightarrow 8j+3}; \\
b_{j+4s, 2s+(-1)_s} &= w_{8(j+m+1) \rightarrow 8(j+m+1)+1} \otimes w_{8j \rightarrow 8j+4}; \\
b_{j+7s, 2s+(-1)_s} &= w_{8(j+m+1) \rightarrow 8(j+m+1)+1} \otimes w_{8j \rightarrow 8j+6}; \\
b_{(j+1)_s, 3s+(-1)_s} &= -w_{8(j+m+1)+2 \rightarrow 8(j+m+1)+4} \otimes w_{8j+1 \rightarrow 8(j+1)}; \\
b_{s+(j+1)_s, 3s+(-1)_s} &= -e_{8(j+m+1)+4} \otimes w_{8j+1 \rightarrow 8(j+1)}; \\
b_{2s+(j+1)_s, 5s+(-2)_s} &= w_{8(j+m+1)+6 \rightarrow 8(j+m+2)} \otimes w_{8j+3 \rightarrow 8(j+1)}; \\
b_{(j+1)_s, 7s+(-2)_s} &= -w_{8(j+m+1)+2 \rightarrow 8(j+m+2)} \otimes w_{8j+5 \rightarrow 8(j+1)}; \\
b_{2s+(j+1)_s, 7s+(-2)_s} &= -w_{8(j+m+1)+6 \rightarrow 8(j+m+2)} \otimes w_{8j+5 \rightarrow 8(j+1)}.
\end{aligned}$$

(23) If  $r_0 = 22$ , then  $\Omega^{22}(Z_t^{(14)})$  is described with  $(13s \times 13s)$  matrix with the following nonzero entries:

$$\begin{aligned}
b_{j,(-2)_s} &= w_{8(j+m) \rightarrow 8(j+m)+7} \otimes e_{8j}; \\
b_{j+s,(-2)_s} &= -w_{8(j+m-1)+7 \rightarrow 8(j+m)+7} \otimes e_{8j}; \\
b_{j+6s,(-2)_s} &= w_{8(j+m)+1 \rightarrow 8(j+m)+7} \otimes w_{8j \rightarrow 8j+4}; \\
b_{j+7s,(-2)_s} &= w_{8(j+m)+2 \rightarrow 8(j+m)+7} \otimes w_{8j \rightarrow 8j+5}; \\
b_{j+2s,(-1)_s} &= w_{8(j+m)+3 \rightarrow 8(j+m)+7} \otimes w_{8j \rightarrow 8j+1}; \\
b_{j+3s,(-1)_s} &= -w_{8(j+m)+4 \rightarrow 8(j+m)+7} \otimes w_{8j \rightarrow 8j+2}; \\
b_{(j+1)_s, s+(-1)_s} &= e_{8(j+m+1)} \otimes w_{8j \rightarrow 8(j+1)}; \\
b_{(j+1)_s, 2s+(-1)_s} &= w_{8(j+m+1) \rightarrow 8(j+m+1)+4} \otimes w_{8j+1 \rightarrow 8(j+1)}; \\
b_{(j+1)_s, 3s+(-2)_s} &= -w_{8(j+m+1) \rightarrow 8(j+m+1)+5} \otimes w_{8j+2 \rightarrow 8(j+1)}; \\
b_{(j+1)_s, 4s+(-2)_s} &= w_{8(j+m+1) \rightarrow 8(j+m+1)+6} \otimes w_{8j+3 \rightarrow 8(j+1)}; \\
b_{5s+(j+1)_s, 4s+(-2)_s} &= e_{8(j+m+1)+6} \otimes w_{8j+3 \rightarrow 8(j+1)+3}; \\
b_{(j+1)_s, 5s+(-2)_s} &= w_{8(j+m+1) \rightarrow 8(j+m+1)+1} \otimes w_{8j+3 \rightarrow 8(j+1)}; \\
b_{s+(j+1)_s, 5s+(-2)_s} &= -w_{8(j+m)+7 \rightarrow 8(j+m+1)+1} \otimes w_{8j+3 \rightarrow 8(j+1)};
\end{aligned}$$

$$\begin{aligned}
b_{(j+1)s, 5s+(-3)s} &= w_{8(j+m+1) \rightarrow 8(j+m+1)+1} \otimes w_{8j+3 \rightarrow 8(j+1)}; \\
b_{s+(j+1)s, 5s+(-3)s} &= -w_{8(j+m)+7 \rightarrow 8(j+m+1)+1} \otimes w_{8j+3 \rightarrow 8(j+1)}; \\
b_{(j+1)s, 6s+(-2)s} &= w_{8(j+m+1) \rightarrow 8(j+m+1)+2} \otimes w_{8j+4 \rightarrow 8(j+1)}; \\
b_{s+(j+1)s, 6s+(-2)s} &= -w_{8(j+m)+7 \rightarrow 8(j+m+1)+2} \otimes w_{8j+4 \rightarrow 8(j+1)}; \\
b_{6s+(j+1)s, 6s+(-2)s} &= w_{8(j+m+1)+1 \rightarrow 8(j+m+1)+2} \otimes w_{8j+4 \rightarrow 8(j+1)+4}; \\
b_{(j+1)s, 6s+(-3)s} &= w_{8(j+m+1) \rightarrow 8(j+m+1)+2} \otimes w_{8j+4 \rightarrow 8(j+1)}; \\
b_{s+(j+1)s, 6s+(-3)s} &= -w_{8(j+m)+7 \rightarrow 8(j+m+1)+2} \otimes w_{8j+4 \rightarrow 8(j+1)}; \\
b_{6s+(j+1)s, 6s+(-3)s} &= w_{8(j+m+1)+1 \rightarrow 8(j+m+1)+2} \otimes w_{8j+4 \rightarrow 8(j+1)+4}; \\
b_{j, 7s+(-2)s} &= -w_{8(j+m)+2 \rightarrow 8(j+m+1)+2} \otimes e_{8j+5}; \\
b_{(j+1)s, 9s+(-2)s} &= w_{8(j+m+1) \rightarrow 8(j+m+1)+3} \otimes w_{8j+6 \rightarrow 8(j+1)}; \\
b_{s+(j+1)s, 9s+(-2)s} &= -w_{8(j+m)+7 \rightarrow 8(j+m+1)+3} \otimes w_{8j+6 \rightarrow 8(j+1)}; \\
b_{7s+(j+1)s, 9s+(-2)s} &= w_{8(j+m+1)+2 \rightarrow 8(j+m+1)+3} \otimes w_{8j+6 \rightarrow 8(j+1)+5}; \\
b_{(j+1)s, 9s+(-3)s} &= w_{8(j+m+1) \rightarrow 8(j+m+1)+3} \otimes w_{8j+6 \rightarrow 8(j+1)}; \\
b_{s+(j+1)s, 9s+(-3)s} &= -w_{8(j+m)+7 \rightarrow 8(j+m+1)+3} \otimes w_{8j+6 \rightarrow 8(j+1)}; \\
b_{7s+(j+1)s, 9s+(-3)s} &= w_{8(j+m+1)+2 \rightarrow 8(j+m+1)+3} \otimes w_{8j+6 \rightarrow 8(j+1)+5}; \\
b_{(j+1)s, 11s+(-2)s} &= -w_{8(j+m+1) \rightarrow 8(j+m+1)+7} \otimes w_{8j+7 \rightarrow 8(j+1)}; \\
b_{s+(j+1)s, 11s+(-2)s} &= w_{8(j+m)+7 \rightarrow 8(j+m+1)+7} \otimes w_{8j+7 \rightarrow 8(j+1)}; \\
b_{6s+(j+1)s, 11s+(-2)s} &= -w_{8(j+m+1)+1 \rightarrow 8(j+m+1)+7} \otimes w_{8j+7 \rightarrow 8(j+1)+4}; \\
b_{7s+(j+1)s, 11s+(-2)s} &= -w_{8(j+m+1)+2 \rightarrow 8(j+m+1)+7} \otimes w_{8j+7 \rightarrow 8(j+1)+5}; \\
b_{(j+1)s, 11s+(-3)s} &= -w_{8(j+m+1) \rightarrow 8(j+m+1)+7} \otimes w_{8j+7 \rightarrow 8(j+1)}; \\
b_{s+(j+1)s, 11s+(-3)s} &= w_{8(j+m)+7 \rightarrow 8(j+m+1)+7} \otimes w_{8j+7 \rightarrow 8(j+1)}; \\
b_{6s+(j+1)s, 11s+(-3)s} &= -w_{8(j+m+1)+1 \rightarrow 8(j+m+1)+7} \otimes w_{8j+7 \rightarrow 8(j+1)+4}; \\
b_{7s+(j+1)s, 11s+(-3)s} &= -w_{8(j+m+1)+2 \rightarrow 8(j+m+1)+7} \otimes w_{8j+7 \rightarrow 8(j+1)+5}.
\end{aligned}$$

(24) If  $r_0 = 23$ , then  $\Omega^{23}(Z_t^{(14)})$  is described with  $(11s \times 14s)$  matrix with the following nonzero entries:

$$\begin{aligned}
b_{j+2s, (-1)s} &= -w_{8(j+m+1) \rightarrow 8(j+m+1)+2} \otimes w_{8j \rightarrow 8j+1}; \\
b_{s+(j+1)s, 3s+(-2)s} &= e_{8(j+m+1)+5} \otimes w_{8j \rightarrow 8(j+1)}; \\
b_{s+(j+1)s, 3s+(-1)s} &= e_{8(j+m+1)+5} \otimes w_{8j \rightarrow 8(j+1)}; \\
b_{(j+1)s, 4s+(-2)s} &= -w_{8(j+m+1)+3 \rightarrow 8(j+m+1)+7} \otimes w_{8j+1 \rightarrow 8(j+1)}; \\
b_{s+(j+1)s, 4s+(-2)s} &= w_{8(j+m+1)+5 \rightarrow 8(j+m+1)+7} \otimes w_{8j+1 \rightarrow 8(j+1)}; \\
b_{s+(j+1)s, 4s+(-1)s} &= w_{8(j+m+1)+5 \rightarrow 8(j+m+1)+7} \otimes w_{8j+1 \rightarrow 8(j+1)}; \\
b_{2s+(j+1)s, 5s+(-2)s} &= e_{8(j+m+2)} \otimes w_{8j+2 \rightarrow 8(j+1)+1}; \\
b_{(j+1)s, 6s+(-2)s} &= w_{8(j+m+1)+3 \rightarrow 8(j+m+1)+7} \otimes w_{8j+3 \rightarrow 8(j+1)}; \\
b_{s+(j+1)s, 6s+(-2)s} &= -w_{8(j+m+1)+5 \rightarrow 8(j+m+1)+7} \otimes w_{8j+3 \rightarrow 8(j+1)}; \\
b_{3s+(j+1)s, 6s+(-2)s} &= e_{8(j+m+1)+7} \otimes w_{8j+3 \rightarrow 8(j+1)+2}; \\
b_{(j+1)s, 8s+(-2)s} &= w_{8(j+m+1)+3 \rightarrow 8(j+m+1)+7} \otimes w_{8j+5 \rightarrow 8(j+1)}; \\
b_{2s+(j+1)s, 12s+(-2)s} &= w_{8(j+m+2) \rightarrow 8(j+m+2)+3} \otimes w_{8j+7 \rightarrow 8(j+1)+1}.
\end{aligned}$$

(25) If  $r_0 = 24$ , then  $\Omega^{24}(Z_t^{(14)})$  is described with  $(11s \times 16s)$  matrix with the following nonzero entries:

$$b_{j+2s, (-1)s} = -w_{8(j+m)+5 \rightarrow 8(j+m)+7} \otimes w_{8j \rightarrow 8j+1};$$

$$\begin{aligned}
b_{(j+1)s, 2s+(-2)_s} &= -e_{8(j+m+1)} \otimes w_{8j \rightarrow 8(j+1)}; \\
b_{j-s, 3s+(-2)_s} &= -w_{8(j+m)+5 \rightarrow 8(j+m+1)+5} \otimes e_{8j+1}; \\
b_{2s+(j+1)s, 3s+(-2)_s} &= e_{8(j+m+1)+5} \otimes w_{8j+1 \rightarrow 8(j+1)+1}; \\
b_{j-s, 3s+(-1)_s} &= -w_{8(j+m)+5 \rightarrow 8(j+m+1)+5} \otimes e_{8j+1}; \\
b_{2s+(j+1)s, 4s+(-2)_s} &= -w_{8(j+m+1)+5 \rightarrow 8(j+m+1)+6} \otimes w_{8j+2 \rightarrow 8(j+1)+1}; \\
b_{(j+1)s, 5s+(-2)_s} &= -w_{8(j+m+1) \rightarrow 8(j+m+1)+1} \otimes w_{8j+2 \rightarrow 8(j+1)}; \\
b_{(j+1)s, 6s+(-2)_s} &= -w_{8(j+m+1) \rightarrow 8(j+m+1)+2} \otimes w_{8j+3 \rightarrow 8(j+1)}; \\
b_{4s+(j+1)s, 6s+(-2)_s} &= w_{8(j+m+1)+1 \rightarrow 8(j+m+1)+2} \otimes w_{8j+3 \rightarrow 8(j+1)+3}; \\
b_{j-3s, 9s+(-2)_s} &= w_{8(j+m)+3 \rightarrow 8(j+m+1)+3} \otimes e_{8j+5}.
\end{aligned}$$

(26) If  $r_0 = 25$ , then  $\Omega^{25}(Z_t^{(14)})$  is described with  $(10s \times 16s)$  matrix with the following nonzero entries:

$$\begin{aligned}
b_{j+2s, (-2)_s} &= w_{8(j+m)+7 \rightarrow 8(j+m+1)+5} \otimes w_{8j \rightarrow 8j+1}; \\
b_{j+3s, (-2)_s} &= w_{8(j+m+1) \rightarrow 8(j+m+1)+5} \otimes w_{8j \rightarrow 8j+2}; \\
b_{j+7s, (-2)_s} &= w_{8(j+m+1) \rightarrow 8(j+m+1)+5} \otimes w_{8j \rightarrow 8j+6}; \\
b_{j-s, s+(-2)_s} &= -w_{8(j+m)+4 \rightarrow 8(j+m+1)+3} \otimes e_{8j}; \\
b_{j+s, s+(-2)_s} &= -w_{8(j+m)+7 \rightarrow 8(j+m+1)+3} \otimes w_{8j \rightarrow 8j+1}; \\
b_{j+2s, s+(-2)_s} &= -w_{8(j+m+1) \rightarrow 8(j+m+1)+3} \otimes w_{8j \rightarrow 8j+2}; \\
b_{j+6s, s+(-2)_s} &= -w_{8(j+m+1) \rightarrow 8(j+m+1)+3} \otimes w_{8j \rightarrow 8j+6}; \\
b_{s+(j+1)s, 6s+(-2)_s} &= w_{8(j+m+1)+6 \rightarrow 8(j+m+2)} \otimes w_{8j+3 \rightarrow 8(j+1)}; \\
b_{3s+(j+1)s, 6s+(-2)_s} &= e_{8(j+m+2)} \otimes w_{8j+3 \rightarrow 8(j+1)+2}; \\
b_{2s+(j+1)s, 15s+(-2)_s} &= -w_{8(j+m+1)+7 \rightarrow 8(j+m+2)+5} \otimes w_{8j+7 \rightarrow 8(j+1)+1}; \\
b_{3s+(j+1)s, 15s+(-2)_s} &= -w_{8(j+m+2) \rightarrow 8(j+m+2)+5} \otimes w_{8j+7 \rightarrow 8(j+1)+2}; \\
b_{7s+(j+1)s, 15s+(-2)_s} &= -w_{8(j+m+2) \rightarrow 8(j+m+2)+5} \otimes w_{8j+7 \rightarrow 8(j+1)+6}; \\
b_{2s+(j+1)s, 15s+(-3)_s} &= -w_{8(j+m+1)+7 \rightarrow 8(j+m+2)+5} \otimes w_{8j+7 \rightarrow 8(j+1)+1}; \\
b_{3s+(j+1)s, 15s+(-3)_s} &= -w_{8(j+m+2) \rightarrow 8(j+m+2)+5} \otimes w_{8j+7 \rightarrow 8(j+1)+2}; \\
b_{7s+(j+1)s, 15s+(-3)_s} &= -w_{8(j+m+2) \rightarrow 8(j+m+2)+5} \otimes w_{8j+7 \rightarrow 8(j+1)+6}.
\end{aligned}$$

(27) If  $r_0 = 26$ , then  $\Omega^{26}(Z_t^{(14)})$  is described with  $(8s \times 19s)$  matrix with the following nonzero entries:

$$\begin{aligned}
b_{(j+1)s, s+(-2)_s} &= w_{8(j+m)+7 \rightarrow 8(j+m+1)} \otimes w_{8j \rightarrow 8(j+1)}; \\
b_{j+j_1s, s+(-2)_s} &= (-1 + 2f(j_1, 2))w_{8(j+m)+j_1 \rightarrow 8(j+m+1)} \otimes w_{8j \rightarrow 8j+j_1+1}, \quad 1 \leq j_1 \leq 4; \\
b_{s+(j+1)s, 3s+(-3)_s} &= e_{8(j+m+1)+6} \otimes w_{8j+1 \rightarrow 8(j+1)+1}; \\
b_{2s+(j+1)s, 5s+(-2)_s} &= w_{8(j+m+1)+1 \rightarrow 8(j+m+1)+2} \otimes w_{8j+2 \rightarrow 8(j+1)+2}; \\
b_{2s+(j+1)s, 6s+(-2)_s} &= -w_{8(j+m+1)+1 \rightarrow 8(j+m+1)+3} \otimes w_{8j+3 \rightarrow 8(j+1)+2}; \\
b_{3s+(j+1)s, 6s+(-2)_s} &= w_{8(j+m+1)+2 \rightarrow 8(j+m+1)+3} \otimes w_{8j+3 \rightarrow 8(j+1)+3}; \\
b_{(j+1)s, 6s+(-3)_s} &= -w_{8(j+m)+7 \rightarrow 8(j+m+1)+3} \otimes w_{8j+3 \rightarrow 8(j+1)}; \\
b_{2s+(j+1)s, 6s+(-3)_s} &= -w_{8(j+m+1)+1 \rightarrow 8(j+m+1)+3} \otimes w_{8j+3 \rightarrow 8(j+1)+2}; \\
b_{3s+(j+1)s, 6s+(-3)_s} &= w_{8(j+m+1)+2 \rightarrow 8(j+m+1)+3} \otimes w_{8j+3 \rightarrow 8(j+1)+3}; \\
b_{(j+1)s, 7s+(-2)_s} &= -w_{8(j+m)+7 \rightarrow 8(j+m+1)+5} \otimes w_{8j+3 \rightarrow 8(j+1)}; \\
b_{(j+1)s, 8s+(-3)_s} &= w_{8(j+m)+7 \rightarrow 8(j+m+1)+4} \otimes w_{8j+4 \rightarrow 8(j+1)}; \\
b_{(j_1+1)s+(j+1)s, 8s+(-3)_s} &= (-1)^{j_1+1}w_{8(j+m+1)+j_1 \rightarrow 8(j+m+1)+4} \otimes w_{8j+4 \rightarrow 8(j+1)+j_1+1}, \quad 1 \leq j_1 \leq 3;
\end{aligned}$$

$$\begin{aligned}
b_{6s+(j+1)s,15s+(-2)s} &= -e_{8(j+m+1)+5} \otimes w_{8j+6 \rightarrow 8(j+1)+6}; \\
b_{6s+(j+1)s,15s+(-3)s} &= -e_{8(j+m+1)+5} \otimes w_{8j+6 \rightarrow 8(j+1)+6}; \\
b_{(j+1)s,16s+(-2)s} &= w_{8(j+m)+7 \rightarrow 8(j+m+1)+7} \otimes w_{8j+7 \rightarrow 8(j+1)}; \\
b_{(j_1+1)s+(j+1)s,16s+(-2)s} &= (1-2f(j_1, 2))w_{8(j+m+1)+j_1 \rightarrow 8(j+m+1)+7} \otimes w_{8j+7 \rightarrow 8(j+1)+j_1+1}, \quad 1 \leq j_1 \leq 4; \\
b_{(j+1)s,16s+(-3)s} &= w_{8(j+m)+7 \rightarrow 8(j+m+1)+7} \otimes w_{8j+7 \rightarrow 8(j+1)}; \\
b_{(j_1+1)s+(j+1)s,16s+(-3)s} &= (1-2f(j_1, 2))w_{8(j+m+1)+j_1 \rightarrow 8(j+m+1)+7} \otimes w_{8j+7 \rightarrow 8(j+1)+j_1+1}, \quad 1 \leq j_1 \leq 4; \\
b_{(j+1)s,17s+(-2)s} &= w_{8(j+m)+7 \rightarrow 8(j+m+1)+7} \otimes w_{8j+7 \rightarrow 8(j+1)}; \\
b_{(j_1+1)s+(j+1)s,17s+(-2)s} &= (1-2f(j_1, 2))w_{8(j+m+1)+j_1 \rightarrow 8(j+m+1)+7} \otimes w_{8j+7 \rightarrow 8(j+1)+j_1+1}, \quad 1 \leq j_1 \leq 4.
\end{aligned}$$

(28) If  $r_0 = 27$ , then  $\Omega^{27}(Z_t^{(14)})$  is described with  $(9s \times 18s)$  matrix with the following nonzero entries:

$$\begin{aligned}
b_{j+s,(-2)s} &= w_{8(j+m+1) \rightarrow 8(j+m+1)+2} \otimes w_{8j \rightarrow 8j+1}; \\
b_{j+5s,(-2)s} &= -w_{8(j+m+1) \rightarrow 8(j+m+1)+2} \otimes w_{8j \rightarrow 8j+5}; \\
b_{j-s,2s+(-2)s} &= w_{8(j+m+1) \rightarrow 8(j+m+1)+4} \otimes w_{8j \rightarrow 8j+1}; \\
b_{j+3s,2s+(-2)s} &= -w_{8(j+m+1) \rightarrow 8(j+m+1)+4} \otimes w_{8j \rightarrow 8j+5}; \\
b_{(j+1)s,5s+(-3)s} &= e_{8(j+m+1)+7} \otimes w_{8j+1 \rightarrow 8(j+1)}; \\
b_{(j+1)s,10s+(-2)s} &= e_{8(j+m+1)+7} \otimes w_{8j+5 \rightarrow 8(j+1)}; \\
b_{(j+1)s,11s+(-2)s} &= w_{8(j+m+1)+7 \rightarrow 8(j+m+2)} \otimes w_{8j+5 \rightarrow 8(j+1)}; \\
b_{(j+1)s,11s+(-3)s} &= w_{8(j+m+1)+7 \rightarrow 8(j+m+2)} \otimes w_{8j+5 \rightarrow 8(j+1)}; \\
b_{(j+1)s,12s+(-2)s} &= -e_{8(j+m+1)+7} \otimes w_{8j+6 \rightarrow 8(j+1)}; \\
b_{(j+1)s,12s+(-3)s} &= -e_{8(j+m+1)+7} \otimes w_{8j+6 \rightarrow 8(j+1)}; \\
b_{(j+1)s,15s+(-2)s} &= w_{8(j+m+1)+7 \rightarrow 8(j+m+2)+3} \otimes w_{8j+7 \rightarrow 8(j+1)}; \\
b_{(j+1)s,15s+(-3)s} &= w_{8(j+m+1)+7 \rightarrow 8(j+m+2)+3} \otimes w_{8j+7 \rightarrow 8(j+1)}.
\end{aligned}$$

(29) If  $r_0 = 28$ , then  $\Omega^{28}(Z_t^{(14)})$  is described with  $(8s \times 19s)$  matrix with the following nonzero entries:

$$\begin{aligned}
b_{j+j_1s,(-2)s} &= (-1+2(f(j_1, 1)+f(j_1, 3)+f(j_1, 6)))w_{8(j+m)+j_1 \rightarrow 8(j+m)+7} \otimes w_{8j \rightarrow 8j+j_1}, \quad 1 \leq j_1 \leq 7; \\
b_{j+(j_1-2)s,2s+(-2)s} &= (-1+2(f(j_1, 1)+f(j_1, 3)+f(j_1, 6)))w_{8(j+m)+j_1 \rightarrow 8(j+m)+7} \otimes w_{8j \rightarrow 8j+j_1}, \quad 1 \leq j_1 \leq 7; \\
b_{(j+1)s,3s+(-3)s} &= -w_{8(j+m+1) \rightarrow 8(j+m+1)+2} \otimes w_{8j+1 \rightarrow 8(j+1)}; \\
b_{j-s,4s+(-2)s} &= -w_{8(j+m)+3 \rightarrow 8(j+m+1)+3} \otimes w_{8j+2 \rightarrow 8j+3}; \\
b_{j,4s+(-2)s} &= w_{8(j+m)+4 \rightarrow 8(j+m+1)+3} \otimes w_{8j+2 \rightarrow 8j+4}; \\
b_{j+3s,4s+(-2)s} &= w_{8(j+m)+7 \rightarrow 8(j+m+1)+3} \otimes w_{8j+2 \rightarrow 8j+7}; \\
b_{s+(j+1)s,4s+(-3)s} &= w_{8(j+m+1)+1 \rightarrow 8(j+m+1)+3} \otimes w_{8j+2 \rightarrow 8(j+1)+1}; \\
b_{2s+(j+1)s,4s+(-3)s} &= -w_{8(j+m+1)+2 \rightarrow 8(j+m+1)+3} \otimes w_{8j+2 \rightarrow 8(j+1)+2}; \\
b_{j-s,4s+(-3)s} &= -w_{8(j+m)+3 \rightarrow 8(j+m+1)+3} \otimes w_{8j+2 \rightarrow 8j+3}; \\
b_{j,4s+(-3)s} &= w_{8(j+m)+4 \rightarrow 8(j+m+1)+3} \otimes w_{8j+2 \rightarrow 8j+4}; \\
b_{j+3s,4s+(-3)s} &= w_{8(j+m)+7 \rightarrow 8(j+m+1)+3} \otimes w_{8j+2 \rightarrow 8j+7}; \\
b_{j-2s,6s+(-2)s} &= -w_{8(j+m)+4 \rightarrow 8(j+m+1)+4} \otimes w_{8j+3 \rightarrow 8j+4}; \\
b_{j+s,6s+(-2)s} &= -w_{8(j+m)+7 \rightarrow 8(j+m+1)+4} \otimes w_{8j+3 \rightarrow 8j+7}; \\
b_{j-2s,6s+(-3)s} &= -w_{8(j+m)+4 \rightarrow 8(j+m+1)+4} \otimes w_{8j+3 \rightarrow 8j+4}; \\
b_{j+s,6s+(-3)s} &= -w_{8(j+m)+7 \rightarrow 8(j+m+1)+4} \otimes w_{8j+3 \rightarrow 8j+7};
\end{aligned}$$



$$\begin{aligned}
b_{(j+1)s, 10s+(-3)s} &= w_{8(j+m+1) \rightarrow 8(j+m+1)+2} \otimes w_{8j+5 \rightarrow 8(j+1)}; \\
b_{j-5s, 11s+(-3)s} &= w_{8(j+m)+6 \rightarrow 8(j+m+1)+6} \otimes w_{8j+5 \rightarrow 8j+6}; \\
b_{j-4s, 11s+(-3)s} &= -w_{8(j+m)+7 \rightarrow 8(j+m+1)+6} \otimes w_{8j+5 \rightarrow 8j+7}; \\
b_{j-7s, 13s+(-2)s} &= w_{8(j+m)+6 \rightarrow 8(j+m+1)+6} \otimes e_{8j+6}; \\
b_{j-6s, 13s+(-2)s} &= -w_{8(j+m)+7 \rightarrow 8(j+m+1)+6} \otimes w_{8j+6 \rightarrow 8j+7}; \\
b_{j-7s, 13s+(-3)s} &= w_{8(j+m)+6 \rightarrow 8(j+m+1)+6} \otimes e_{8j+6}; \\
b_{j-6s, 13s+(-3)s} &= -w_{8(j+m)+7 \rightarrow 8(j+m+1)+6} \otimes w_{8j+6 \rightarrow 8j+7}; \\
b_{j-9s, 16s+(-2)s} &= w_{8(j+m)+7 \rightarrow 8(j+m+1)+7} \otimes e_{8j+7}; \\
b_{j-9s, 16s+(-3)s} &= w_{8(j+m)+7 \rightarrow 8(j+m+1)+7} \otimes e_{8j+7};
\end{aligned}$$

$$b_{j_1s+(j+1)s, 18s+(-3)s} = (-1+2(f(j_1, 1)+f(j_1, 3)+f(j_1, 6)))w_{8(j+m+1)+j_1 \rightarrow 8(j+m+2)} \otimes w_{8j+7 \rightarrow 8(j+1)+j_1}, \quad 1 \leq j_1 \leq 7.$$

(II) Represent an arbitrary  $t_0 \in \mathbb{N}$  in the form  $t_0 = 29\ell_0 + r_0$ , where  $0 \leq r_0 \leq 28$ . Then  $\Omega^{t_0}(Z_t^{(14)})$  is a  $\Omega^{r_0}(Z_t^{(14)})$ , whose left components twisted by  $\sigma^{\ell_0}$ , and coefficients multiplied by  $(-1)^{\ell_0}$ .

**Proposition 12** (Translates for the case 16). (I) Let  $r_0 \in \mathbb{N}$ ,  $r_0 < 29$ .  $r_0$ -translates of the elements  $Z_t^{(16)}$  are described by the following way.

(1) If  $r_0 = 0$ , then  $\Omega^0(Z_t^{(16)})$  is described with  $(8s \times 19s)$  matrix with unique nonzero entry:

$$b_{j-s, s+(1)s} = w_{8(j+m) \rightarrow 8(j+m+1)} \otimes e_{8j}.$$

(2) If  $r_0 = 1$ , then  $\Omega^1(Z_t^{(16)})$  is described with  $(9s \times 18s)$  matrix with the following nonzero entries:

$$\begin{aligned}
b_{s+(j+1)s, 5s} &= -w_{8(j+m+1)+5 \rightarrow 8(j+m+2)} \otimes w_{8j+1 \rightarrow 8(j+1)}; \\
b_{s+(j+1)s, 6s} &= -w_{8(j+m+1)+5 \rightarrow 8(j+m+2)} \otimes w_{8j+2 \rightarrow 8(j+1)}; \\
b_{(j+1)s, 9s} &= -w_{8(j+m+1)+1 \rightarrow 8(j+m+2)} \otimes w_{8j+5 \rightarrow 8(j+1)}.
\end{aligned}$$

(3) If  $r_0 = 2$ , then  $\Omega^2(Z_t^{(16)})$  is described with  $(8s \times 19s)$  matrix with two nonzero entries:

$$\begin{aligned}
b_{(j+1)s, s} &= w_{8(j+m)+7 \rightarrow 8(j+m+1)} \otimes w_{8j \rightarrow 8(j+1)}; \\
b_{(j+1)s, 3s} &= w_{8(j+m)+7 \rightarrow 8(j+m+1)+5} \otimes w_{8j+1 \rightarrow 8(j+1)}.
\end{aligned}$$

(4) If  $r_0 = 3$ , then  $\Omega^3(Z_t^{(16)})$  is described with  $(10s \times 16s)$  matrix with two nonzero entries:

$$\begin{aligned}
b_{(j+1)s, 0} &= -w_{8(j+m+1)+2 \rightarrow 8(j+m+1)+3} \otimes w_{8j \rightarrow 8(j+1)}; \\
b_{s+(j+1)s, s} &= -e_{8(j+m+1)+6} \otimes w_{8j \rightarrow 8(j+1)}.
\end{aligned}$$

(5) If  $r_0 = 4$ , then  $\Omega^4(Z_t^{(16)})$  is described with  $(11s \times 16s)$  matrix with the following nonzero entries:

$$\begin{aligned}
b_{(j+1)s, 0} &= e_{8(j+m)+7} \otimes w_{8j \rightarrow 8(j+1)}; \\
b_{(j+1)s, s} &= -w_{8(j+m)+7 \rightarrow 8(j+m+1)} \otimes w_{8j \rightarrow 8(j+1)}; \\
b_{s+(j+1)s, s} &= -e_{8(j+m+1)} \otimes w_{8j \rightarrow 8(j+1)}.
\end{aligned}$$

(6) If  $r_0 = 5$ , then  $\Omega^5(Z_t^{(16)})$  is described with  $(11s \times 14s)$  matrix with the following nonzero entries:

$$\begin{aligned}
b_{2s+(j+1)s, 0} &= w_{8(j+m+1)+1 \rightarrow 8(j+m+1)+2} \otimes w_{8j \rightarrow 8(j+1)}; \\
b_{s+(j+1)s, s} &= -w_{8(j+m+1)+3 \rightarrow 8(j+m+1)+4} \otimes w_{8j \rightarrow 8(j+1)}; \\
b_{2s+(j+1)s, s} &= -w_{8(j+m+1)+1 \rightarrow 8(j+m+1)+4} \otimes w_{8j \rightarrow 8(j+1)};
\end{aligned}$$

$$b_{(j+1)s,2s} = w_{8(j+m+1)+5 \rightarrow 8(j+m+1)+6} \otimes w_{8j \rightarrow 8(j+1)}.$$

(7) If  $r_0 = 6$ , then  $\Omega^6(Z_t^{(16)})$  is described with  $(13s \times 13s)$  matrix with two nonzero entries:

$$b_{s+(j+1)s,0} = e_{8(j+m+1)} \otimes w_{8j \rightarrow 8(j+1)};$$

$$b_{(j+1)s,s} = e_{8(j+m)+7} \otimes w_{8j \rightarrow 8(j+1)}.$$

(8) If  $r_0 = 7$ , then  $\Omega^7(Z_t^{(16)})$  is described with  $(14s \times 11s)$  matrix with two nonzero entries:

$$b_{(j+1)s,0} = -w_{8(j+m+1)+2 \rightarrow 8(j+m+1)+3} \otimes w_{8j \rightarrow 8(j+1)};$$

$$b_{3s+(j+1)s,s} = e_{8(j+m+1)+5} \otimes w_{8j \rightarrow 8(j+1)}.$$

(9) If  $r_0 = 8$ , then  $\Omega^8(Z_t^{(16)})$  is described with  $(16s \times 11s)$  matrix with two nonzero entries:

$$b_{(j+1)s,0} = -w_{8(j+m)+7 \rightarrow 8(j+m+1)} \otimes w_{8j \rightarrow 8(j+1)};$$

$$b_{2s+(j+1)s,0} = -e_{8(j+m+1)} \otimes w_{8j \rightarrow 8(j+1)}.$$

(10) If  $r_0 = 9$ , then  $\Omega^9(Z_t^{(16)})$  is described with  $(16s \times 10s)$  matrix with the following nonzero entries:

$$b_{s+(j+1)s,0} = -w_{8(j+m+1)+3 \rightarrow 8(j+m+1)+4} \otimes w_{8j \rightarrow 8(j+1)};$$

$$b_{3s+(j+1)s,0} = -w_{8(j+m+1)+1 \rightarrow 8(j+m+1)+4} \otimes w_{8j \rightarrow 8(j+1)};$$

$$b_{(j+1)s,s} = w_{8(j+m+1)+5 \rightarrow 8(j+m+1)+6} \otimes w_{8j \rightarrow 8(j+1)};$$

$$b_{2s+(j+1)s,s} = e_{8(j+m+1)+6} \otimes w_{8j \rightarrow 8(j+1)}.$$

(11) If  $r_0 = 10$ , then  $\Omega^{10}(Z_t^{(16)})$  is described with  $(19s \times 8s)$  matrix with unique nonzero entry:

$$b_{(j+1)s,0} = e_{8(j+m)+7} \otimes w_{8j \rightarrow 8(j+1)}.$$

(12) If  $r_0 = 11$ , then  $\Omega^{11}(Z_t^{(16)})$  is described with  $(18s \times 9s)$  matrix with two nonzero entries:

$$b_{(j+1)s,0} = -w_{8(j+m+1)+2 \rightarrow 8(j+m+1)+7} \otimes w_{8j \rightarrow 8(j+1)};$$

$$b_{2s+(j+1)s,0} = w_{8(j+m+1)+4 \rightarrow 8(j+m+1)+7} \otimes w_{8j \rightarrow 8(j+1)}.$$

(13) If  $r_0 = 12$ , then  $\Omega^{12}(Z_t^{(16)})$  is described with  $(19s \times 8s)$  matrix with unique nonzero entry:

$$b_{s+(j+1)s,0} = e_{8(j+m+1)} \otimes w_{8j \rightarrow 8(j+1)}.$$

(14) If  $r_0 = 13$ , then  $\Omega^{13}(Z_t^{(16)})$  is described with  $(18s \times 8s)$  matrix with unique nonzero entry:

$$b_{(j+1)s,0} = w_{8(j+m+1)+2 \rightarrow 8(j+m+2)} \otimes w_{8j \rightarrow 8(j+1)}.$$

(15) If  $r_0 = 14$ , then  $\Omega^{14}(Z_t^{(16)})$  is described with  $(20s \times 9s)$  matrix with two nonzero entries:

$$b_{(j+1)s,0} = w_{8(j+m)+7 \rightarrow 8(j+m+1)+1} \otimes w_{8j \rightarrow 8(j+1)};$$

$$b_{s+(j+1)s,0} = w_{8(j+m+1) \rightarrow 8(j+m+1)+1} \otimes w_{8j \rightarrow 8(j+1)}.$$

(16) If  $r_0 = 15$ , then  $\Omega^{15}(Z_t^{(16)})$  is described with  $(18s \times 8s)$  matrix with unique nonzero entry:

$$b_{(j+1)s,0} = w_{8(j+m+1)+3 \rightarrow 8(j+m+1)+7} \otimes w_{8j \rightarrow 8(j+1)}.$$

(17) If  $r_0 = 16$ , then  $\Omega^{16}(Z_t^{(16)})$  is described with  $(19s \times 10s)$  matrix with unique nonzero entry:

$$b_{(j+1)s,0} = w_{8(j+m)+7 \rightarrow 8(j+m+1)+2} \otimes w_{8j \rightarrow 8(j+1)}.$$

(18) If  $r_0 = 17$ , then  $\Omega^{17}(Z_t^{(16)})$  is described with  $(18s \times 11s)$  matrix with unique nonzero entry:

$$b_{s+(j+1)s,0} = w_{8(j+m+1)+4 \rightarrow 8(j+m+1)+7} \otimes w_{8j \rightarrow 8(j+1)}.$$

(19) If  $r_0 = 18$ , then  $\Omega^{18}(Z_t^{(16)})$  is described with  $(19s \times 11s)$  matrix with unique nonzero entry:

$$b_{(j+1)s,s} = -w_{8(j+m)+7 \rightarrow 8(j+m+1)+3} \otimes w_{8j \rightarrow 8(j+1)}.$$

(20) If  $r_0 = 19$ , then  $\Omega^{19}(Z_t^{(16)})$  is described with  $(16s \times 13s)$  matrix with two nonzero entries:

$$b_{s+(j+1)s,0} = w_{8(j+m+1)+6 \rightarrow 8(j+m+1)+7} \otimes w_{8j \rightarrow 8(j+1)};$$

$$b_{2s+(j+1)s,0} = w_{8(j+m+1)+1 \rightarrow 8(j+m+1)+7} \otimes w_{8j \rightarrow 8(j+1)}.$$

(21) If  $r_0 = 20$ , then  $\Omega^{20}(Z_t^{(16)})$  is described with  $(16s \times 14s)$  matrix with unique nonzero entry:

$$b_{(j+1)s,2s} = -w_{8(j+m)+7 \rightarrow 8(j+m+1)+6} \otimes w_{8j \rightarrow 8(j+1)}.$$

(22) If  $r_0 = 21$ , then  $\Omega^{21}(Z_t^{(16)})$  is described with  $(14s \times 16s)$  matrix with two nonzero entries:

$$b_{(j+1)s,0} = w_{8(j+m+1)+2 \rightarrow 8(j+m+1)+7} \otimes w_{8j \rightarrow 8(j+1)};$$

$$b_{s+(j+1)s,0} = w_{8(j+m+1)+4 \rightarrow 8(j+m+1)+7} \otimes w_{8j \rightarrow 8(j+1)}.$$

(23) If  $r_0 = 22$ , then  $\Omega^{22}(Z_t^{(16)})$  is described with  $(13s \times 16s)$  matrix with unique nonzero entry:

$$b_{(j+1)s,s} = w_{8(j+m+1) \rightarrow 8(j+m+1)+3} \otimes w_{8j \rightarrow 8(j+1)}.$$

(24) If  $r_0 = 23$ , then  $\Omega^{23}(Z_t^{(16)})$  is described with  $(11s \times 19s)$  matrix with two nonzero entries:

$$b_{s+(j+1)s,0} = -w_{8(j+m+1)+5 \rightarrow 8(j+m+1)+7} \otimes w_{8j \rightarrow 8(j+1)};$$

$$b_{(j+1)s,s} = w_{8(j+m+1)+3 \rightarrow 8(j+m+2)} \otimes w_{8j \rightarrow 8(j+1)}.$$

(25) If  $r_0 = 24$ , then  $\Omega^{24}(Z_t^{(16)})$  is described with  $(11s \times 18s)$  matrix with unique nonzero entry:

$$b_{(j+1)s,0} = w_{8(j+m+1) \rightarrow 8(j+m+1)+2} \otimes w_{8j \rightarrow 8(j+1)}.$$

(26) If  $r_0 = 25$ , then  $\Omega^{25}(Z_t^{(16)})$  is described with  $(10s \times 19s)$  matrix with two nonzero entries:

$$b_{(j+1)s,0} = w_{8(j+m+1)+4 \rightarrow 8(j+m+1)+7} \otimes w_{8j \rightarrow 8(j+1)};$$

$$b_{(j+1)s,s} = w_{8(j+m+1)+4 \rightarrow 8(j+m+2)} \otimes w_{8j \rightarrow 8(j+1)}.$$

(27) If  $r_0 = 26$ , then  $\Omega^{26}(Z_t^{(16)})$  is described with  $(8s \times 18s)$  matrix with unique nonzero entry:

$$b_{(j+1)s,s} = w_{8(j+m)+7 \rightarrow 8(j+m+1)+3} \otimes w_{8j \rightarrow 8(j+1)}.$$

(28) If  $r_0 = 27$ , then  $\Omega^{27}(Z_t^{(16)})$  is described with  $(9s \times 20s)$  matrix with unique nonzero entry:

$$b_{(j+1)s,0} = -e_{8(j+m+1)+7} \otimes w_{8j \rightarrow 8(j+1)}.$$

(29) If  $r_0 = 28$ , then  $\Omega^{28}(Z_t^{(16)})$  is described with  $(8s \times 18s)$  matrix with two nonzero entries:

$$b_{(j+1)s,0} = -w_{8(j+m+1) \rightarrow 8(j+m+1)+3} \otimes w_{8j \rightarrow 8(j+1)};$$

$$b_{(j+1)s,s} = -w_{8(j+m+1) \rightarrow 8(j+m+1)+6} \otimes w_{8j \rightarrow 8(j+1)}.$$

(II) Represent an arbitrary  $t_0 \in \mathbb{N}$  in the form  $t_0 = 29\ell_0 + r_0$ , where  $0 \leq r_0 \leq 28$ . Then  $\Omega^{t_0}(Z_t^{(16)})$  is a  $\Omega^{r_0}(Z_t^{(16)})$ , whose left components twisted by  $\sigma^{\ell_0}$ , and coefficients multiplied by  $(-1)^{\ell_0}$ .

**Proposition 13** (Translates for the case 17). (I) Let  $r_0 \in \mathbb{N}$ ,  $r_0 < 29$ .  $r_0$ -translates of the elements  $Z_t^{(17)}$  are described by the following way.

(1) If  $r_0 = 0$ , then  $\Omega^0(Z_t^{(17)})$  is described with  $(8s \times 18s)$  matrix, whose entries  $b_{ij}$  have the following form:

If  $3s \leq j < 4s$ , then

$$b_{ij} = \begin{cases} w_{8(j+m) \rightarrow 8(j+m)+5} \otimes e_{8j}, & i = j - 3s; \\ 0, & \text{otherwise.} \end{cases}$$

If  $4s \leq j < 5s$ , then

$$b_{ij} = \begin{cases} -w_{8(j+m)+1 \rightarrow 8(j+m)+7} \otimes e_{8j+1}, & i = j - 3s; \\ 0, & \text{otherwise.} \end{cases}$$

If  $5s \leq j < 7s$ , then  $b_{ij} = 0$ .

If  $7s \leq j < 8s$ , then

$$b_{ij} = \begin{cases} -w_{8(j+m)+3 \rightarrow 8(j+m)+7} \otimes e_{8j+3}, & i = j - 4s; \\ 0, & \text{otherwise.} \end{cases}$$

If  $8s \leq j < 9s$ , then  $b_{ij} = 0$ .

If  $9s \leq j < 10s$ , then

$$b_{ij} = \begin{cases} -w_{8(j+m)+5 \rightarrow 8(j+m)+7} \otimes e_{8j+5}, & i = j - 4s; \\ 0, & \text{otherwise.} \end{cases}$$

If  $10s \leq j < 13s$ , then  $b_{ij} = 0$ .

If  $13s \leq j < 14s$ , then

$$b_{ij} = \begin{cases} w_{8(j+m)+7 \rightarrow 8(j+m)+3} \otimes e_{8j+7}, & i = j - 6s; \\ 0, & \text{otherwise.} \end{cases}$$

If  $14s \leq j < 18s$ , then  $b_{ij} = 0$ .

(2) If  $r_0 = 1$ , then  $\Omega^1(Z_t^{(17)})$  is described with  $(9s \times 19s)$  matrix, whose entries  $b_{ij}$  have the following form:

If  $0 \leq j < s$ , then

$$b_{ij} = \begin{cases} w_{8(j+m)+1 \rightarrow 8(j+m)+7} \otimes e_{8j}, & i = j; \\ -w_{8(j+m)+2 \rightarrow 8(j+m)+7} \otimes w_{8j \rightarrow 8j+1}, & i = j + 2s; \\ -w_{8(j+m)+3 \rightarrow 8(j+m)+7} \otimes w_{8j \rightarrow 8j+2}, & i = j + 3s; \\ 0, & \text{otherwise.} \end{cases}$$

If  $s \leq j < 2s$ , then

$$b_{ij} = \begin{cases} w_{8(j+m)+1 \rightarrow 8(j+m)+1} \otimes e_{8j}, & i = j - s; \\ -w_{8(j+m)+5 \rightarrow 8(j+m)+1} \otimes e_{8j}, & i = j; \\ 0, & \text{otherwise.} \end{cases}$$

If  $2s \leq j < 3s$ , then  $b_{ij} = 0$ .

If  $3s \leq j < 4s$ , then

$$b_{ij} = \begin{cases} e_{8(j+m+1)+5} \otimes w_{8j+1 \rightarrow 8(j+1)}, & i = s + (j+1)_s; \\ 0, & \text{otherwise.} \end{cases}$$

If  $4s \leq j < 6s$ , then  $b_{ij} = 0$ .

If  $6s \leq j < 7s$ , then

$$b_{ij} = \begin{cases} w_{8(j+m+1)+5 \rightarrow 8(j+m+1)+6} \otimes w_{8j+2 \rightarrow 8(j+1)}, & i = s + (j+1)_s; \\ 0, & \text{otherwise.} \end{cases}$$

If  $7s \leq j < 8s$ , then

$$b_{ij} = \begin{cases} -w_{8(j+m)+4 \rightarrow 8(j+m+1)+3} \otimes e_{8j+3}, & i = j - 3s; \\ -w_{8(j+m)+7 \rightarrow 8(j+m+1)+3} \otimes w_{8j+3 \rightarrow 8j+4}, & i = j - 2s; \\ 0, & \text{otherwise.} \end{cases}$$

If  $8s \leq j < 10s$ , then  $b_{ij} = 0$ .

If  $10s \leq j < 11s$ , then

$$b_{ij} = \begin{cases} w_{8(j+m)+7 \rightarrow 8(j+m+1)+3} \otimes w_{8j+5 \rightarrow 8j+6}, & i = j - 3s; \\ 0, & \text{otherwise.} \end{cases}$$

If  $11s \leq j < 12s$ , then  $b_{ij} = 0$ .

If  $12s \leq j < 13s$ , then

$$b_{ij} = \begin{cases} -w_{8(j+m)+6 \rightarrow 8(j+m+1)+5} \otimes e_{8j+5}, & i = j - 6s; \\ -w_{8(j+m)+7 \rightarrow 8(j+m+1)+5} \otimes w_{8j+5 \rightarrow 8j+6}, & i = j - 5s; \\ -w_{8(j+m+1) \rightarrow 8(j+m+1)+5} \otimes w_{8j+5 \rightarrow 8j+7}, & i = j - 4s; \\ 0, & \text{otherwise.} \end{cases}$$

If  $13s \leq j < 14s$ , then  $b_{ij} = 0$ .

If  $14s \leq j < 15s$ , then

$$b_{ij} = \begin{cases} w_{8(j+m)+7 \rightarrow 8(j+m+1)+4} \otimes e_{8j+6}, & i = j - 7s; \\ 0, & \text{otherwise.} \end{cases}$$

If  $15s \leq j < 16s$ , then  $b_{ij} = 0$ .

If  $16s \leq j < 17s$ , then

$$b_{ij} = \begin{cases} w_{8(j+m+1)+1 \rightarrow 8(j+m+1)+7} \otimes w_{8j+7 \rightarrow 8(j+1)}, & i = (j+1)_s; \\ w_{8(j+m+1) \rightarrow 8(j+m+1)+7} \otimes e_{8j+7}, & i = j - 8s; \\ 0, & \text{otherwise.} \end{cases}$$

If  $17s \leq j < 18s$ , then

$$b_{ij} = \begin{cases} w_{8(j+m+1)+1 \rightarrow 8(j+m+2)} \otimes w_{8j+7 \rightarrow 8(j+1)}, & i = (j+1)_s; \\ w_{8(j+m+1) \rightarrow 8(j+m+2)} \otimes e_{8j+7}, & i = j - 9s; \\ 0, & \text{otherwise.} \end{cases}$$

If  $18s \leq j < 19s$ , then  $b_{ij} = 0$ .

(3) If  $r_0 = 2$ , then  $\Omega^2(Z_t^{(17)})$  is described with  $(8s \times 16s)$  matrix, whose entries  $b_{ij}$  have the following form:

If  $0 \leq j < s$ , then

$$b_{ij} = \begin{cases} -w_{8(j+m-1)+7 \rightarrow 8(j+m)+3} \otimes e_{8j}, & i = j; \\ 0, & \text{otherwise.} \end{cases}$$

If  $s \leq j < 3s$ , then  $b_{ij} = 0$ .

If  $3s \leq j < 4s$ , then

$$b_{ij} = \begin{cases} w_{8(j+m-1)+7 \rightarrow 8(j+m)+5} \otimes e_{8j}, & i = j - 3s; \\ -e_{8(j+m)+5} \otimes w_{8j \rightarrow 8j+4}, & i = j + s; \\ 0, & \text{otherwise.} \end{cases}$$

If  $4s \leq j < 5s$ , then

$$b_{ij} = \begin{cases} w_{8(j+m)+7 \rightarrow 8(j+m+1)} \otimes w_{8j+1 \rightarrow 8(j+1)}, & i = (j+1)_s; \\ 0, & \text{otherwise.} \end{cases}$$

If  $5s \leq j < 6s$ , then

$$b_{ij} = \begin{cases} e_{8(j+m)+7} \otimes w_{8j+2 \rightarrow 8(j+1)}, & i = (j+1)_s; \\ w_{8(j+m)+3 \rightarrow 8(j+m)+7} \otimes e_{8j+2}, & i = j - 3s; \\ 0, & \text{otherwise.} \end{cases}$$

If  $6s \leq j < 7s$ , then

$$b_{ij} = \begin{cases} w_{8(j+m)+7 \rightarrow 8(j+m+1)} \otimes w_{8j+3 \rightarrow 8(j+1)}, & i = (j+1)_s; \\ -w_{8(j+m)+4 \rightarrow 8(j+m+1)} \otimes e_{8j+3}, & i = j - 3s; \\ 0, & \text{otherwise.} \end{cases}$$

If  $7s \leq j < 8s$ , then  $b_{ij} = 0$ .

If  $8s \leq j < 9s$ , then

$$b_{ij} = \begin{cases} -e_{8(j+m)+7} \otimes w_{8j+5 \rightarrow 8(j+1)}, & i = (j+1)_s; \\ -w_{8(j+m)+6 \rightarrow 8(j+m)+7} \otimes e_{8j+5}, & i = j - 3s; \\ 0, & \text{otherwise.} \end{cases}$$

If  $9s \leq j < 10s$ , then  $b_{ij} = 0$ .

If  $10s \leq j < 11s$ , then

$$b_{ij} = \begin{cases} -w_{8(j+m)+1 \rightarrow 8(j+m)+7} \otimes e_{8j+6}, & i = j - 4s; \\ 0, & \text{otherwise.} \end{cases}$$

If  $11s \leq j < 12s$ , then

$$b_{ij} = \begin{cases} w_{8(j+m)+1 \rightarrow 8(j+m+1)} \otimes e_{8j+6}, & i = j - 5s; \\ 0, & \text{otherwise.} \end{cases}$$

If  $12s \leq j < 13s$ , then  $b_{ij} = 0$ .

If  $13s \leq j < 14s$ , then

$$b_{ij} = \begin{cases} -w_{8(j+m)+7 \rightarrow 8(j+m+1)+4} \otimes w_{8j+7 \rightarrow 8(j+1)}, & i = (j+1)_s; \\ 0, & \text{otherwise.} \end{cases}$$

If  $14s \leq j < 16s$ , then  $b_{ij} = 0$ .

(4) If  $r_0 = 3$ , then  $\Omega^3(Z_t^{(17)})$  is described with  $(10s \times 16s)$  matrix, whose entries  $b_{ij}$  have the following form:

If  $0 \leq j < s$ , then

$$b_{ij} = \begin{cases} w_{8(j+m)+6 \rightarrow 8(j+m)+7} \otimes e_{8j}, & i = j + s; \\ w_{8(j+m)+4 \rightarrow 8(j+m)+7} \otimes w_{8j \rightarrow 8j+2}, & i = j + 3s; \\ e_{8(j+m)+7} \otimes w_{8j \rightarrow 8j+3}, & i = j + 4s; \\ 0, & \text{otherwise.} \end{cases}$$

If  $s \leq j < 2s$ , then

$$b_{ij} = \begin{cases} w_{8(j+m)+6 \rightarrow 8(j+m+1)} \otimes e_{8j}, & i = j; \\ w_{8(j+m)+7 \rightarrow 8(j+m+1)} \otimes w_{8j \rightarrow 8j+3}, & i = j + 3s; \\ 0, & \text{otherwise.} \end{cases}$$

If  $2s \leq j < 3s$ , then

$$b_{ij} = \begin{cases} w_{8(j+m)+4 \rightarrow 8(j+m+1)+2} \otimes w_{8j+1 \rightarrow 8j+2}, & i = j + s; \\ 0, & \text{otherwise.} \end{cases}$$

If  $3s \leq j < 4s$ , then

$$b_{ij} = \begin{cases} -e_{8(j+m+1)+6} \otimes w_{8j+1 \rightarrow 8(j+1)}, & i = s + (j+1)_s; \\ 0, & \text{otherwise.} \end{cases}$$

If  $4s \leq j < 5s$ , then

$$b_{ij} = \begin{cases} w_{8(j+m)+4 \rightarrow 8(j+m+1)+3} \otimes e_{8j+2}, & i = j - s; \\ 0, & \text{otherwise.} \end{cases}$$

If  $5s \leq j < 6s$ , then

$$b_{ij} = \begin{cases} -w_{8(j+m)+7 \rightarrow 8(j+m+1)+4} \otimes e_{8j+3}, & i = j - s; \\ 0, & \text{otherwise.} \end{cases}$$

If  $6s \leq j < 8s$ , then  $b_{ij} = 0$ .

If  $8s \leq j < 9s$ , then

$$b_{ij} = \begin{cases} -w_{8(j+m)+7 \rightarrow 8(j+m+1)+6} \otimes e_{8j+5}, & i = j - 2s; \\ 0, & \text{otherwise.} \end{cases}$$

If  $9s \leq j < 13s$ , then  $b_{ij} = 0$ .

If  $13s \leq j < 14s$ , then

$$b_{ij} = \begin{cases} w_{8(j+m+1)+2 \rightarrow 8(j+m+1)+7} \otimes w_{8j+7 \rightarrow 8(j+1)}, & i = (j+1)_s; \\ w_{8(j+m+1)+3 \rightarrow 8(j+m+1)+7} \otimes w_{8j+7 \rightarrow 8(j+1)+1}, & i = 2s + (j+1)_s; \\ 0, & \text{otherwise.} \end{cases}$$

If  $14s \leq j < 15s$ , then

$$b_{ij} = \begin{cases} -w_{8(j+m+1)+2 \rightarrow 8(j+m+2)} \otimes w_{8j+7 \rightarrow 8(j+1)}, & i = (j+1)_s; \\ -w_{8(j+m+1)+3 \rightarrow 8(j+m+2)} \otimes w_{8j+7 \rightarrow 8(j+1)+1}, & i = 2s + (j+1)_s; \\ 0, & \text{otherwise.} \end{cases}$$

If  $15s \leq j < 16s$ , then  $b_{ij} = 0$ .

(5) If  $r_0 = 4$ , then  $\Omega^4(Z_t^{(17)})$  is described with  $(11s \times 14s)$  matrix, whose entries  $b_{ij}$  have the following form:

If  $2s \leq j < 3s$ , then

$$b_{ij} = \begin{cases} -w_{8(j+m-1)+7 \rightarrow 8(j+m)+6} \otimes e_{8j}, & i = j - 2s; \\ -w_{8(j+m)+5 \rightarrow 8(j+m)+6} \otimes w_{8j \rightarrow 8j+3}, & i = j + 2s; \\ e_{8(j+m)+6} \otimes w_{8j \rightarrow 8j+4}, & i = j + 3s; \\ 0, & \text{otherwise.} \end{cases}$$

If  $3s \leq j < 4s$ , then  $b_{ij} = 0$ .

If  $4s \leq j < 5s$ , then

$$b_{ij} = \begin{cases} -w_{8(j+m)+7 \rightarrow 8(j+m+1)} \otimes w_{8j+2 \rightarrow 8(j+1)}, & i = (j+1)_s; \\ -e_{8(j+m+1)} \otimes w_{8j+2 \rightarrow 8(j+1)}, & i = s + (j+1)_s; \\ 0, & \text{otherwise.} \end{cases}$$

If  $5s \leq j < 6s$ , then

$$b_{ij} = \begin{cases} e_{8(j+m)+7} \otimes w_{8j+3 \rightarrow 8(j+1)}, & i = (j+1)_s; \\ -w_{8(j+m)+5 \rightarrow 8(j+m)+7} \otimes e_{8j+3}, & i = j - s; \\ w_{8(j+m)+6 \rightarrow 8(j+m)+7} \otimes w_{8j+3 \rightarrow 8j+4}, & i = j; \\ 0, & \text{otherwise.} \end{cases}$$

If  $6s \leq j < 7s$ , then  $b_{ij} = 0$ .

If  $7s \leq j < 8s$ , then

$$b_{ij} = \begin{cases} -w_{8(j+m)+1 \rightarrow 8(j+m)+7} \otimes e_{8j+5}, & i = j; \\ w_{8(j+m)+2 \rightarrow 8(j+m)+7} \otimes w_{8j+5 \rightarrow 8j+6}, & i = j + s; \\ 0, & \text{otherwise.} \end{cases}$$

If  $8s \leq j < 9s$ , then

$$b_{ij} = \begin{cases} -w_{8(j+m)+7 \rightarrow 8(j+m+1)} \otimes w_{8j+5 \rightarrow 8(j+1)}, & i = (j+1)_s; \\ -e_{8(j+m+1)} \otimes w_{8j+5 \rightarrow 8(j+1)}, & i = s + (j+1)_s; \\ 0, & \text{otherwise.} \end{cases}$$

If  $9s \leq j < 11s$ , then  $b_{ij} = 0$ .



If  $11s \leq j < 12s$ , then

$$b_{ij} = \begin{cases} -w_{8(j+m)+7 \rightarrow 8(j+m+1)+6} \otimes w_{8j+7 \rightarrow 8(j+1)}, & i = (j+1)_s; \\ -w_{8(j+m+1)+5 \rightarrow 8(j+m+1)+6} \otimes w_{8j+7 \rightarrow 8(j+1)+3}, & i = 4s + (j+1)_s; \\ e_{8(j+m+1)+6} \otimes w_{8j+7 \rightarrow 8(j+1)+4}, & i = 5s + (j+1)_s; \\ 0, & \text{otherwise.} \end{cases}$$

If  $12s \leq j < 14s$ , then  $b_{ij} = 0$ .

(6) If  $r_0 = 5$ , then  $\Omega^5(Z_t^{(17)})$  is described with  $(11s \times 13s)$  matrix, whose entries  $b_{ij}$  have the following form:

If  $s \leq j < 2s$ , then

$$b_{ij} = \begin{cases} w_{8(j+m)+3 \rightarrow 8(j+m)+7} \otimes e_{8j}, & i = j; \\ w_{8(j+m)+4 \rightarrow 8(j+m)+7} \otimes w_{8j \rightarrow 8j+1}, & i = j + 2s; \\ e_{8(j+m)+7} \otimes w_{8j \rightarrow 8j+2}, & i = j + 3s; \\ 0, & \text{otherwise.} \end{cases}$$

If  $2s \leq j < 3s$ , then

$$b_{ij} = \begin{cases} -w_{8(j+m+1)+1 \rightarrow 8(j+m+1)+3} \otimes w_{8j+1 \rightarrow 8(j+1)}, & i = 2s + (j+1)_s; \\ 0, & \text{otherwise.} \end{cases}$$

If  $3s \leq j < 4s$ , then

$$b_{ij} = \begin{cases} -w_{8(j+m+1)+1 \rightarrow 8(j+m+1)+4} \otimes w_{8j+2 \rightarrow 8(j+1)}, & i = 2s + (j+1)_s; \\ 0, & \text{otherwise.} \end{cases}$$

If  $4s \leq j < 5s$ , then

$$b_{ij} = \begin{cases} -e_{8(j+m+1)+5} \otimes w_{8j+2 \rightarrow 8(j+1)}, & i = (j+1)_s; \\ 0, & \text{otherwise.} \end{cases}$$

If  $5s \leq j < 6s$ , then

$$b_{ij} = \begin{cases} -w_{8(j+m+1)+5 \rightarrow 8(j+m+1)+6} \otimes w_{8j+3 \rightarrow 8(j+1)}, & i = (j+1)_s; \\ -w_{8(j+m+1) \rightarrow 8(j+m+1)+6} \otimes e_{8j+3}, & i = j; \\ 0, & \text{otherwise.} \end{cases}$$

If  $6s \leq j < 7s$ , then  $b_{ij} = 0$ .

If  $7s \leq j < 8s$ , then

$$b_{ij} = \begin{cases} -w_{8(j+m+1) \rightarrow 8(j+m+1)+2} \otimes e_{8j+5}, & i = j; \\ 0, & \text{otherwise.} \end{cases}$$

If  $8s \leq j < 9s$ , then

$$b_{ij} = \begin{cases} -e_{8(j+m+1)+5} \otimes w_{8j+5 \rightarrow 8(j+1)}, & i = (j+1)_s; \\ 0, & \text{otherwise.} \end{cases}$$

If  $9s \leq j < 12s$ , then  $b_{ij} = 0$ .

If  $12s \leq j < 13s$ , then

$$b_{ij} = \begin{cases} e_{8(j+m+2)} \otimes w_{8j+7 \rightarrow 8(j+1)+3}, & i = 5s + (j+1)_s; \\ 0, & \text{otherwise.} \end{cases}$$

(7) If  $r_0 = 6$ , then  $\Omega^6(Z_t^{(17)})$  is described with  $(13s \times 11s)$  matrix, whose entries  $b_{ij}$  have the following form:

If  $0 \leq j < s$ , then

$$b_{ij} = \begin{cases} -w_{8(j+m) \rightarrow 8(j+m)+3} \otimes e_{8j}, & i = j + s; \\ w_{8(j+m)+1 \rightarrow 8(j+m)+3} \otimes w_{8j \rightarrow 8j+3}, & i = j + 5s; \\ 0, & \text{otherwise.} \end{cases}$$

If  $s \leq j < 3s$ , then  $b_{ij} = 0$ .

If  $3s \leq j < 4s$ , then

$$b_{ij} = \begin{cases} -e_{8(j+m)+7} \otimes w_{8j+2 \rightarrow 8(j+1)}, & i = (j+1)_s; \\ w_{8(j+m)+1 \rightarrow 8(j+m)+7} \otimes w_{8j+2 \rightarrow 8j+3}, & i = j + 2s; \\ 0, & \text{otherwise.} \end{cases}$$

If  $4s \leq j < 5s$ , then

$$b_{ij} = \begin{cases} -w_{8(j+m)+7 \rightarrow 8(j+m)+1} \otimes w_{8j+3 \rightarrow 8(j+1)}, & i = (j+1)_s; \\ e_{8(j+m)+1} \otimes w_{8j+3 \rightarrow 8(j+1)}, & i = s + (j+1)_s; \\ -w_{8(j+m)+1 \rightarrow 8(j+m)+1} \otimes e_{8j+3}, & i = j + s; \\ 0, & \text{otherwise.} \end{cases}$$

If  $5s \leq j < 6s$ , then

$$b_{ij} = \begin{cases} w_{8(j+m+1) \rightarrow 8(j+m+1)+1} \otimes w_{8j+4 \rightarrow 8(j+1)}, & i = s + (j+1)_s; \\ e_{8(j+m+1)+1} \otimes w_{8j+4 \rightarrow 8(j+1)+3}, & i = 5s + (j+1)_s; \\ 0, & \text{otherwise.} \end{cases}$$

If  $6s \leq j < 7s$ , then

$$b_{ij} = \begin{cases} -w_{8(j+m)+5 \rightarrow 8(j+m)+1} \otimes e_{8j+5}, & i = j + 2s; \\ 0, & \text{otherwise.} \end{cases}$$

If  $7s \leq j < 8s$ , then  $b_{ij} = 0$ .

If  $8s \leq j < 9s$ , then

$$b_{ij} = \begin{cases} w_{8(j+m+1) \rightarrow 8(j+m+1)+2} \otimes w_{8j+7 \rightarrow 8(j+1)}, & i = s + (j+1)_s; \\ w_{8(j+m+1)+1 \rightarrow 8(j+m+1)+2} \otimes w_{8j+7 \rightarrow 8(j+1)+3}, & i = 5s + (j+1)_s; \\ 0, & \text{otherwise.} \end{cases}$$

If  $9s \leq j < 10s$ , then

$$b_{ij} = \begin{cases} -w_{8(j+m+1) \rightarrow 8(j+m+1)+4} \otimes w_{8j+7 \rightarrow 8(j+1)}, & i = s + (j+1)_s; \\ -w_{8(j+m+1)+1 \rightarrow 8(j+m+1)+4} \otimes w_{8j+7 \rightarrow 8(j+1)+3}, & i = 5s + (j+1)_s; \\ 0, & \text{otherwise.} \end{cases}$$

If  $10s \leq j < 11s$ , then  $b_{ij} = 0$ .

(8) If  $r_0 = 7$ , then  $\Omega^7(Z_t^{(17)})$  is described with  $(14s \times 11s)$  matrix, whose entries  $b_{ij}$  have the following form:

If  $0 \leq j < s$ , then

$$b_{ij} = \begin{cases} -w_{8(j+m)+5 \rightarrow 8(j+m+1)} \otimes e_{8j}, & i = j + 3s; \\ -e_{8(j+m+1)} \otimes w_{8j \rightarrow 8j+2}, & i = j + 5s; \\ 0, & \text{otherwise.} \end{cases}$$

If  $s \leq j < 2s$ , then

$$b_{ij} = \begin{cases} w_{8(j+m+1)+2 \rightarrow 8(j+m+1)+4} \otimes w_{8j+1 \rightarrow 8(j+1)}, & i = (j+1)_s; \\ 0, & \text{otherwise.} \end{cases}$$

If  $2s \leq j < 3s$ , then  $b_{ij} = 0$ .

If  $3s \leq j < 4s$ , then

$$b_{ij} = \begin{cases} e_{8(j+m+1)+6} \otimes w_{8j+2 \rightarrow 8(j+1)}, & i = 2s + (j+1)_s; \\ w_{8(j+m+1)+5 \rightarrow 8(j+m+1)+6} \otimes w_{8j+2 \rightarrow 8(j+1)}, & i = 3s + (j+1)_s; \\ 0, & \text{otherwise.} \end{cases}$$

If  $4s \leq j < 5s$ , then

$$b_{ij} = \begin{cases} w_{8(j+m)+7 \rightarrow 8(j+m+1)+1} \otimes e_{8j+3}, & i = j + 2s; \\ w_{8(j+m+1) \rightarrow 8(j+m+1)+1} \otimes w_{8j+3 \rightarrow 8j+4}, & i = j + 3s; \\ -e_{8(j+m+1)+1} \otimes w_{8j+3 \rightarrow 8j+7}, & i = j + 9s; \\ 0, & \text{otherwise.} \end{cases}$$

If  $5s \leq j < 11s$ , then  $b_{ij} = 0$ .

(9) If  $r_0 = 8$ , then  $\Omega^8(Z_t^{(17)})$  is described with  $(16s \times 10s)$  matrix, whose entries  $b_{ij}$  have the following form:

If  $0 \leq j < s$ , then

$$b_{ij} = \begin{cases} -w_{8(j+m)+1 \rightarrow 8(j+m)+4} \otimes w_{8j \rightarrow 8j+2}, & i = j + 5s; \\ -w_{8(j+m)+2 \rightarrow 8(j+m)+4} \otimes w_{8j \rightarrow 8j+3}, & i = j + 6s; \\ 0, & \text{otherwise.} \end{cases}$$

If  $s \leq j < 2s$ , then

$$b_{ij} = \begin{cases} -e_{8(j+m)+6} \otimes w_{8j \rightarrow 8j+2}, & i = j + 3s; \\ 0, & \text{otherwise.} \end{cases}$$

If  $2s \leq j < 3s$ , then

$$b_{ij} = \begin{cases} e_{8(j+m)+7} \otimes w_{8j+1 \rightarrow 8(j+1)}, & i = (j+1)_s; \\ 0, & \text{otherwise.} \end{cases}$$

If  $3s \leq j < 4s$ , then

$$b_{ij} = \begin{cases} -e_{8(j+m+1)} \otimes w_{8j+2 \rightarrow 8(j+1)}, & i = 2s + (j+1)_s; \\ -w_{8(j+m)+6 \rightarrow 8(j+m+1)} \otimes e_{8j+2}, & i = j + s; \\ w_{8(j+m)+1 \rightarrow 8(j+m+1)} \otimes e_{8j+2}, & i = j + 2s; \\ 0, & \text{otherwise.} \end{cases}$$

If  $4s \leq j < 5s$ , then

$$b_{ij} = \begin{cases} -w_{8(j+m)+7 \rightarrow 8(j+m+1)+1} \otimes w_{8j+3 \rightarrow 8(j+1)}, & i = (j+1)_s; \\ w_{8(j+m+1) \rightarrow 8(j+m+1)+1} \otimes w_{8j+3 \rightarrow 8(j+1)}, & i = 2s + (j+1)_s; \\ w_{8(j+m)+2 \rightarrow 8(j+m+1)+1} \otimes e_{8j+3}, & i = j + 2s; \\ 0, & \text{otherwise.} \end{cases}$$

If  $5s \leq j < 6s$ , then

$$b_{ij} = \begin{cases} -w_{8(j+m+1) \rightarrow 8(j+m+1)+2} \otimes w_{8j+4 \rightarrow 8(j+1)}, & i = 2s + (j+1)_s; \\ -e_{8(j+m+1)+2} \otimes w_{8j+4 \rightarrow 8(j+1)+3}, & i = 6s + (j+1)_s; \\ 0, & \text{otherwise.} \end{cases}$$

If  $6s \leq j < 8s$ , then  $b_{ij} = 0$ .

If  $8s \leq j < 9s$ , then

$$b_{ij} = \begin{cases} w_{8(j+m+1)+1 \rightarrow 8(j+m+1)+3} \otimes w_{8j+7 \rightarrow 8(j+1)+2}, & i = 5s + (j+1)_s; \\ -w_{8(j+m+1)+2 \rightarrow 8(j+m+1)+3} \otimes w_{8j+7 \rightarrow 8(j+1)+3}, & i = 6s + (j+1)_s; \\ 0, & \text{otherwise.} \end{cases}$$

If  $9s \leq j < 10s$ , then  $b_{ij} = 0$ .

(10) If  $r_0 = 9$ , then  $\Omega^9(Z_t^{(17)})$  is described with  $(16s \times 8s)$  matrix, whose entries  $b_{ij}$  have the following form:

If  $0 \leq j < s$ , then

$$b_{ij} = \begin{cases} e_{8(j+m)+7} \otimes w_{8j \rightarrow 8j+2}, & i = j + 5s; \\ 0, & \text{otherwise.} \end{cases}$$

If  $s \leq j < 2s$ , then

$$b_{ij} = \begin{cases} w_{8(j+m+1)+5 \rightarrow 8(j+m+1)+6} \otimes w_{8j+1 \rightarrow 8(j+1)}, & i = (j+1)_s; \\ e_{8(j+m+1)+6} \otimes w_{8j+1 \rightarrow 8(j+1)}, & i = 2s + (j+1)_s; \\ w_{8(j+m+1) \rightarrow 8(j+m+1)+6} \otimes e_{8j+1}, & i = j + 3s; \\ 0, & \text{otherwise.} \end{cases}$$

If  $2s \leq j < 3s$ , then

$$b_{ij} = \begin{cases} -w_{8(j+m)+7 \rightarrow 8(j+m+1)+1} \otimes e_{8j+2}, & i = j + 3s; \\ 0, & \text{otherwise.} \end{cases}$$

If  $3s \leq j < 4s$ , then

$$b_{ij} = \begin{cases} w_{8(j+m+1)+1 \rightarrow 8(j+m+1)+2} \otimes w_{8j+3 \rightarrow 8(j+1)}, & i = 3s + (j+1)_s; \\ w_{8(j+m+1) \rightarrow 8(j+m+1)+2} \otimes e_{8j+3}, & i = j + 3s; \\ w_{8(j+m)+7 \rightarrow 8(j+m+1)+2} \otimes w_{8j+3 \rightarrow 8j+4}, & i = j + 4s; \\ e_{8(j+m+1)+2} \otimes w_{8j+3 \rightarrow 8j+7}, & i = j + 9s; \\ 0, & \text{otherwise.} \end{cases}$$

If  $4s \leq j < 5s$ , then

$$b_{ij} = \begin{cases} -w_{8(j+m+1)+1 \rightarrow 8(j+m+1)+3} \otimes w_{8j+4 \rightarrow 8(j+1)}, & i = 3s + (j+1)_s; \\ 0, & \text{otherwise.} \end{cases}$$

If  $5s \leq j < 7s$ , then  $b_{ij} = 0$ .

If  $7s \leq j < 8s$ , then

$$b_{ij} = \begin{cases} -w_{8(j+m+1)+7 \rightarrow 8(j+m+2)} \otimes w_{8j+7 \rightarrow 8(j+1)+2}, & i = 5s + (j+1)_s; \\ 0, & \text{otherwise.} \end{cases}$$

(11) If  $r_0 = 10$ , then  $\Omega^{10}(Z_t^{(17)})$  is described with  $(19s \times 9s)$  matrix, whose entries  $b_{ij}$  have the following form:

If  $0 \leq j < s$ , then

$$b_{ij} = \begin{cases} w_{8(j+m)+6 \rightarrow 8(j+m)+7} \otimes w_{8j \rightarrow 8j+1}, & i = j + 3s; \\ w_{8(j+m)+1 \rightarrow 8(j+m)+7} \otimes w_{8j \rightarrow 8j+1}, & i = j + 4s; \\ -w_{8(j+m)+2 \rightarrow 8(j+m)+7} \otimes w_{8j \rightarrow 8j+2}, & i = j + 5s; \\ 0, & \text{otherwise.} \end{cases}$$

If  $s \leq j < 2s$ , then

$$b_{ij} = \begin{cases} -w_{8(j+m)+7 \rightarrow 8(j+m+1)} \otimes w_{8j+1 \rightarrow 8(j+1)}, & i = (j+1)_s; \\ -e_{8(j+m+1)} \otimes w_{8j+1 \rightarrow 8(j+1)}, & i = s + (j+1)_s; \\ w_{8(j+m)+6 \rightarrow 8(j+m+1)} \otimes e_{8j+1}, & i = j + 2s; \\ w_{8(j+m)+2 \rightarrow 8(j+m+1)} \otimes w_{8j+1 \rightarrow 8j+2}, & i = j + 4s; \\ 0, & \text{otherwise.} \end{cases}$$

If  $2s \leq j < 3s$ , then

$$b_{ij} = \begin{cases} w_{8(j+m)+7 \rightarrow 8(j+m+1)+1} \otimes w_{8j+2 \rightarrow 8(j+1)}, & i = (j+1)_s; \\ w_{8(j+m+1) \rightarrow 8(j+m+1)+1} \otimes w_{8j+2 \rightarrow 8(j+1)}, & i = s + (j+1)_s; \\ -w_{8(j+m)+2 \rightarrow 8(j+m+1)+1} \otimes e_{8j+2}, & i = j + 3s; \\ 0, & \text{otherwise.} \end{cases}$$

If  $3s \leq j < 4s$ , then

$$b_{ij} = \begin{cases} -w_{8(j+m)+7 \rightarrow 8(j+m+1)+2} \otimes w_{8j+3 \rightarrow 8(j+1)}, & i = (j+1)_s; \\ w_{8(j+m+1) \rightarrow 8(j+m+1)+2} \otimes w_{8j+3 \rightarrow 8(j+1)}, & i = s + (j+1)_s; \\ w_{8(j+m)+3 \rightarrow 8(j+m+1)+2} \otimes e_{8j+3}, & i = j + 3s; \\ 0, & \text{otherwise.} \end{cases}$$

If  $4s \leq j < 5s$ , then

$$b_{ij} = \begin{cases} w_{8(j+m)+7 \rightarrow 8(j+m+1)+3} \otimes w_{8j+4 \rightarrow 8(j+1)}, & i = (j+1)_s; \\ w_{8(j+m+1) \rightarrow 8(j+m+1)+3} \otimes w_{8j+4 \rightarrow 8(j+1)}, & i = s + (j+1)_s; \\ -e_{8(j+m+1)+3} \otimes w_{8j+4 \rightarrow 8(j+1)+3}, & i = 6s + (j+1)_s; \\ 0, & \text{otherwise.} \end{cases}$$

If  $5s \leq j < 7s$ , then  $b_{ij} = 0$ .

If  $7s \leq j < 8s$ , then

$$b_{ij} = \begin{cases} -w_{8(j+m+1)+2 \rightarrow 8(j+m+1)+4} \otimes w_{8j+7 \rightarrow 8(j+1)+2}, & i = 5s + (j+1)_s; \\ -w_{8(j+m+1)+3 \rightarrow 8(j+m+1)+4} \otimes w_{8j+7 \rightarrow 8(j+1)+3}, & i = 6s + (j+1)_s; \\ 0, & \text{otherwise.} \end{cases}$$

If  $8s \leq j < 9s$ , then

$$b_{ij} = \begin{cases} -e_{8(j+m+1)+6} \otimes w_{8j+7 \rightarrow 8(j+1)+1}, & i = 3s + (j+1)_s; \\ 0, & \text{otherwise.} \end{cases}$$

(12) If  $r_0 = 11$ , then  $\Omega^{11}(Z_t^{(17)})$  is described with  $(18s \times 8s)$  matrix, whose entries  $b_{ij}$  have the following form:

If  $0 \leq j < s$ , then

$$b_{ij} = \begin{cases} -w_{8(j+m)+7 \rightarrow 8(j+m+1)} \otimes w_{8j \rightarrow 8j+1}, & i = j + 5s; \\ -e_{8(j+m+1)} \otimes w_{8j \rightarrow 8j+2}, & i = j + 6s; \\ 0, & \text{otherwise.} \end{cases}$$

If  $s \leq j < 2s$ , then  $b_{ij} = 0$ .

If  $2s \leq j < 3s$ , then

$$b_{ij} = \begin{cases} -w_{8(j+m+1) \rightarrow 8(j+m+1)+2} \otimes e_{8j+2}, & i = j + 4s; \\ 0, & \text{otherwise.} \end{cases}$$

If  $3s \leq j < 4s$ , then

$$b_{ij} = \begin{cases} -w_{8(j+m+1)+2 \rightarrow 8(j+m+1)+3} \otimes w_{8j+3 \rightarrow 8(j+1)}, & i = (j+1)_s; \\ w_{8(j+m)+7 \rightarrow 8(j+m+1)+3} \otimes e_{8j+3}, & i = j + 4s; \\ e_{8(j+m+1)+3} \otimes w_{8j+3 \rightarrow 8j+7}, & i = j + 12s; \\ 0, & \text{otherwise.} \end{cases}$$

If  $4s \leq j < 5s$ , then

$$b_{ij} = \begin{cases} w_{8(j+m+1)+2 \rightarrow 8(j+m+1)+4} \otimes w_{8j+4 \rightarrow 8(j+1)}, & i = (j+1)_s; \\ 0, & \text{otherwise.} \end{cases}$$

If  $5s \leq j < 7s$ , then  $b_{ij} = 0$ .

If  $7s \leq j < 8s$ , then

$$b_{ij} = \begin{cases} -e_{8(j+m+1)+7} \otimes w_{8j+7 \rightarrow 8(j+1)+1}, & i = 5s + (j+1)_s; \\ 0, & \text{otherwise.} \end{cases}$$

(13) If  $r_0 = 12$ , then  $\Omega^{12}(Z_t^{(17)})$  is described with  $(19s \times 8s)$  matrix, whose entries  $b_{ij}$  have the following form:

If  $0 \leq j < s$ , then

$$b_{ij} = \begin{cases} -w_{8(j+m)+2 \rightarrow 8(j+m+1)} \otimes w_{8j \rightarrow 8j+1}, & i = j + 3s; \\ -w_{8(j+m)+3 \rightarrow 8(j+m+1)} \otimes w_{8j \rightarrow 8j+2}, & i = j + 4s; \\ 0, & \text{otherwise.} \end{cases}$$

If  $s \leq j < 2s$ , then

$$b_{ij} = \begin{cases} -w_{8(j+m+1) \rightarrow 8(j+m+1)+1} \otimes w_{8j+1 \rightarrow 8(j+1)}, & i = s + (j + 1)_s; \\ -w_{8(j+m)+7 \rightarrow 8(j+m+1)+1} \otimes w_{8j+1 \rightarrow 8(j+1)}, & i = 2s + (j + 1)_s; \\ w_{8(j+m)+3 \rightarrow 8(j+m+1)+1} \otimes w_{8j+1 \rightarrow 8j+2}, & i = j + 3s; \\ 0, & \text{otherwise.} \end{cases}$$

If  $2s \leq j < 3s$ , then

$$b_{ij} = \begin{cases} w_{8(j+m+1) \rightarrow 8(j+m+1)+2} \otimes w_{8j+2 \rightarrow 8(j+1)}, & i = s + (j + 1)_s; \\ w_{8(j+m)+7 \rightarrow 8(j+m+1)+2} \otimes w_{8j+2 \rightarrow 8(j+1)}, & i = 2s + (j + 1)_s; \\ -w_{8(j+m)+3 \rightarrow 8(j+m+1)+2} \otimes e_{8j+2}, & i = j + 2s; \\ 0, & \text{otherwise.} \end{cases}$$

If  $3s \leq j < 4s$ , then

$$b_{ij} = \begin{cases} -w_{8(j+m+1) \rightarrow 8(j+m+1)+3} \otimes w_{8j+3 \rightarrow 8(j+1)}, & i = s + (j + 1)_s; \\ w_{8(j+m)+7 \rightarrow 8(j+m+1)+3} \otimes w_{8j+3 \rightarrow 8(j+1)}, & i = 2s + (j + 1)_s; \\ w_{8(j+m)+4 \rightarrow 8(j+m+1)+3} \otimes e_{8j+3}, & i = j + 3s; \\ 0, & \text{otherwise.} \end{cases}$$

If  $4s \leq j < 5s$ , then

$$b_{ij} = \begin{cases} w_{8(j+m)+7 \rightarrow 8(j+m+1)+4} \otimes w_{8j+4 \rightarrow 8(j+1)}, & i = (j + 1)_s; \\ -w_{8(j+m+1)+2 \rightarrow 8(j+m+1)+4} \otimes w_{8j+4 \rightarrow 8(j+1)+1}, & i = 3s + (j + 1)_s; \\ -e_{8(j+m+1)+4} \otimes w_{8j+4 \rightarrow 8(j+1)+3}, & i = 6s + (j + 1)_s; \\ 0, & \text{otherwise.} \end{cases}$$

If  $5s \leq j < 7s$ , then  $b_{ij} = 0$ .

If  $7s \leq j < 8s$ , then

$$b_{ij} = \begin{cases} w_{8(j+m+1)+3 \rightarrow 8(j+m+1)+7} \otimes w_{8j+7 \rightarrow 8(j+1)+2}, & i = 4s + (j + 1)_s; \\ w_{8(j+m+1)+5 \rightarrow 8(j+m+1)+7} \otimes w_{8j+7 \rightarrow 8(j+1)+2}, & i = 5s + (j + 1)_s; \\ 0, & \text{otherwise.} \end{cases}$$

(14) If  $r_0 = 13$ , then  $\Omega^{13}(Z_t^{(17)})$  is described with  $(18s \times 9s)$  matrix, whose entries  $b_{ij}$  have the following form:

If  $0 \leq j < s$ , then

$$b_{ij} = \begin{cases} w_{8(j+m+1) \rightarrow 8(j+m+1)+1} \otimes w_{8j \rightarrow 8j+1}, & i = j + 4s; \\ 0, & \text{otherwise.} \end{cases}$$

If  $s \leq j < 3s$ , then  $b_{ij} = 0$ .

If  $3s \leq j < 4s$ , then

$$b_{ij} = \begin{cases} w_{8(j+m)+7 \rightarrow 8(j+m+1)+3} \otimes e_{8j+2}, & i = j + 2s; \\ 0, & \text{otherwise.} \end{cases}$$

If  $4s \leq j < 5s$ , then

$$b_{ij} = \begin{cases} w_{8(j+m+1)+2 \rightarrow 8(j+m+1)+4} \otimes w_{8j+3 \rightarrow 8(j+1)}, & i = (j+1)_s; \\ w_{8(j+m+1)+3 \rightarrow 8(j+m+1)+4} \otimes w_{8j+3 \rightarrow 8(j+1)}, & i = s + (j+1)_s; \\ -w_{8(j+m)+7 \rightarrow 8(j+m+1)+4} \otimes e_{8j+3}, & i = j + 2s; \\ -w_{8(j+m+1) \rightarrow 8(j+m+1)+4} \otimes e_{8j+3}, & i = j + 3s; \\ -e_{8(j+m+1)+4} \otimes w_{8j+3 \rightarrow 8j+7}, & i = j + 11s; \\ 0, & \text{otherwise.} \end{cases}$$

If  $5s \leq j < 6s$ , then

$$b_{ij} = \begin{cases} w_{8(j+m+1)+3 \rightarrow 8(j+m+1)+7} \otimes w_{8j+4 \rightarrow 8(j+1)}, & i = s + (j+1)_s; \\ e_{8(j+m+1)+7} \otimes w_{8j+4 \rightarrow 8(j+1)+2}, & i = 5s + (j+1)_s; \\ 0, & \text{otherwise.} \end{cases}$$

If  $6s \leq j < 8s$ , then  $b_{ij} = 0$ .

If  $8s \leq j < 9s$ , then

$$b_{ij} = \begin{cases} e_{8(j+m+2)} \otimes w_{8j+7 \rightarrow 8(j+1)+1}, & i = 4s + (j+1)_s; \\ 0, & \text{otherwise.} \end{cases}$$

(15) If  $r_0 = 14$ , then  $\Omega^{14}(Z_t^{(17)})$  is described with  $(20s \times 8s)$  matrix, whose entries  $b_{ij}$  have the following form:

If  $0 \leq j < s$ , then

$$b_{ij} = \begin{cases} -w_{8(j+m)+3 \rightarrow 8(j+m)+7} \otimes w_{8j \rightarrow 8j+1}, & i = j + 3s; \\ -w_{8(j+m)+4 \rightarrow 8(j+m)+7} \otimes w_{8j \rightarrow 8j+2}, & i = j + 5s; \\ 0, & \text{otherwise.} \end{cases}$$

If  $s \leq j < 2s$ , then

$$b_{ij} = \begin{cases} w_{8(j+m)+7 \rightarrow 8(j+m+1)+2} \otimes w_{8j+1 \rightarrow 8(j+1)}, & i = (j+1)_s; \\ w_{8(j+m)+4 \rightarrow 8(j+m+1)+2} \otimes w_{8j+1 \rightarrow 8j+2}, & i = j + 4s; \\ 0, & \text{otherwise.} \end{cases}$$

If  $2s \leq j < 3s$ , then

$$b_{ij} = \begin{cases} -w_{8(j+m)+7 \rightarrow 8(j+m+1)+3} \otimes w_{8j+2 \rightarrow 8(j+1)}, & i = (j+1)_s; \\ -w_{8(j+m)+4 \rightarrow 8(j+m+1)+3} \otimes e_{8j+2}, & i = j + 3s; \\ 0, & \text{otherwise.} \end{cases}$$



If  $3s \leq j < 4s$ , then

$$b_{ij} = \begin{cases} w_{8(j+m)+7 \rightarrow 8(j+m+1)+4} \otimes w_{8j+3 \rightarrow 8(j+1)}, & i = (j+1)_s; \\ -w_{8(j+m+1) \rightarrow 8(j+m+1)+4} \otimes w_{8j+3 \rightarrow 8(j+1)}, & i = s + (j+1)_s; \\ -w_{8(j+m+1) \rightarrow 8(j+m+1)+4} \otimes w_{8j+3 \rightarrow 8(j+1)}, & i = 2s + (j+1)_s; \\ -w_{8(j+m+1) \rightarrow 8(j+m+1)+4} \otimes w_{8j+3 \rightarrow 8j+7}, & i = j + 15s; \\ 0, & \text{otherwise.} \end{cases}$$

If  $4s \leq j < 5s$ , then

$$b_{ij} = \begin{cases} e_{8(j+m+1)+5} \otimes w_{8j+4 \rightarrow 8(j+1)+1}, & i = 4s + (j+1)_s; \\ 0, & \text{otherwise.} \end{cases}$$

If  $5s \leq j < 7s$ , then  $b_{ij} = 0$ .

If  $7s \leq j < 8s$ , then

$$b_{ij} = \begin{cases} w_{8(j+m+1)+4 \rightarrow 8(j+m+2)} \otimes w_{8j+7 \rightarrow 8(j+1)+2}, & i = 5s + (j+1)_s; \\ 0, & \text{otherwise.} \end{cases}$$

(16) If  $r_0 = 15$ , then  $\Omega^{15}(Z_t^{(17)})$  is described with  $(18s \times 10s)$  matrix, whose entries  $b_{ij}$  have the following form:

If  $0 \leq j < s$ , then

$$b_{ij} = \begin{cases} w_{8(j+m)+7 \rightarrow 8(j+m+1)+2} \otimes w_{8j \rightarrow 8j+1}, & i = j + 5s; \\ 0, & \text{otherwise.} \end{cases}$$

If  $s \leq j < 3s$ , then  $b_{ij} = 0$ .

If  $3s \leq j < 4s$ , then

$$b_{ij} = \begin{cases} -w_{8(j+m+1)+1 \rightarrow 8(j+m+1)+4} \otimes w_{8j+2 \rightarrow 8(j+1)}, & i = 3s + (j+1)_s; \\ w_{8(j+m)+7 \rightarrow 8(j+m+1)+4} \otimes e_{8j+2}, & i = j + 3s; \\ w_{8(j+m+1) \rightarrow 8(j+m+1)+4} \otimes w_{8j+2 \rightarrow 8j+3}, & i = j + 5s; \\ 0, & \text{otherwise.} \end{cases}$$

If  $4s \leq j < 5s$ , then

$$b_{ij} = \begin{cases} w_{8(j+m+1)+3 \rightarrow 8(j+m+1)+7} \otimes w_{8j+3 \rightarrow 8(j+1)}, & i = (j+1)_s; \\ w_{8(j+m+1)+6 \rightarrow 8(j+m+1)+7} \otimes w_{8j+3 \rightarrow 8(j+1)}, & i = s + (j+1)_s; \\ w_{8(j+m+1)+4 \rightarrow 8(j+m+1)+7} \otimes w_{8j+3 \rightarrow 8(j+1)}, & i = 2s + (j+1)_s; \\ -w_{8(j+m+1)+1 \rightarrow 8(j+m+1)+7} \otimes w_{8j+3 \rightarrow 8(j+1)}, & i = 3s + (j+1)_s; \\ w_{8(j+m+1)+5 \rightarrow 8(j+m+1)+7} \otimes w_{8j+3 \rightarrow 8(j+1)}, & i = 4s + (j+1)_s; \\ -w_{8(j+m+1) \rightarrow 8(j+m+1)+7} \otimes e_{8j+3}, & i = j + 4s; \\ w_{8(j+m+1)+6 \rightarrow 8(j+m+1)+7} \otimes w_{8j+3 \rightarrow 8j+7}, & i = j + 12s; \\ 0, & \text{otherwise.} \end{cases}$$

If  $5s \leq j < 6s$ , then

$$b_{ij} = \begin{cases} w_{8(j+m+1)+7 \rightarrow 8(j+m+2)} \otimes w_{8j+4 \rightarrow 8(j+1)+1}, & i = 5s + (j+1)_s; \\ e_{8(j+m+2)} \otimes w_{8j+4 \rightarrow 8(j+1)+2}, & i = 7s + (j+1)_s; \\ 0, & \text{otherwise.} \end{cases}$$

If  $6s \leq j < 8s$ , then  $b_{ij} = 0$ .

If  $8s \leq j < 9s$ , then

$$b_{ij} = \begin{cases} w_{8(j+m+1)+7 \rightarrow 8(j+m+2)+1} \otimes w_{8j+7 \rightarrow 8(j+1)+1}, & i = 5s + (j+1)_s; \\ 0, & \text{otherwise.} \end{cases}$$

If  $9s \leq j < 10s$ , then  $b_{ij} = 0$ .

(17) If  $r_0 = 16$ , then  $\Omega^{16}(Z_t^{(17)})$  is described with  $(19s \times 11s)$  matrix, whose entries  $b_{ij}$  have the following form:

If  $0 \leq j < s$ , then

$$b_{ij} = \begin{cases} -e_{8(j+m)+7} \otimes w_{8j \rightarrow 8(j+1)}, & i = (j+1)_s; \\ -w_{8(j+m)+4 \rightarrow 8(j+m)+7} \otimes w_{8j \rightarrow 8j+1}, & i = j + 3s; \\ -w_{8(j+m)+6 \rightarrow 8(j+m)+7} \otimes w_{8j \rightarrow 8j+1}, & i = j + 4s; \\ w_{8(j+m)+5 \rightarrow 8(j+m)+7} \otimes w_{8j \rightarrow 8j+2}, & i = j + 5s; \\ -w_{8(j+m)+6 \rightarrow 8(j+m)+7} \otimes w_{8j \rightarrow 8j+3}, & i = j + 8s; \\ 0, & \text{otherwise.} \end{cases}$$

If  $s \leq j < 2s$ , then  $b_{ij} = 0$ .

If  $2s \leq j < 3s$ , then

$$b_{ij} = \begin{cases} -w_{8(j+m)+7 \rightarrow 8(j+m+1)+3} \otimes w_{8j+1 \rightarrow 8(j+1)}, & i = (j+1)_s; \\ -w_{8(j+m+1) \rightarrow 8(j+m+1)+3} \otimes w_{8j+1 \rightarrow 8(j+1)}, & i = s + (j+1)_s; \\ 0, & \text{otherwise.} \end{cases}$$

If  $3s \leq j < 4s$ , then

$$b_{ij} = \begin{cases} -w_{8(j+m)+7 \rightarrow 8(j+m+1)+4} \otimes w_{8j+2 \rightarrow 8(j+1)}, & i = (j+1)_s; \\ -w_{8(j+m)+7 \rightarrow 8(j+m+1)+4} \otimes w_{8j+2 \rightarrow 8(j+1)}, & i = 2s + (j+1)_s; \\ 0, & \text{otherwise.} \end{cases}$$

If  $4s \leq j < 5s$ , then

$$b_{ij} = \begin{cases} w_{8(j+m)+7 \rightarrow 8(j+m+1)+5} \otimes w_{8j+3 \rightarrow 8(j+1)}, & i = (j+1)_s; \\ -w_{8(j+m+1) \rightarrow 8(j+m+1)+5} \otimes w_{8j+3 \rightarrow 8j+7}, & i = j + 14s; \\ 0, & \text{otherwise.} \end{cases}$$

If  $5s \leq j < 6s$ , then

$$b_{ij} = \begin{cases} -e_{8(j+m+1)+6} \otimes w_{8j+4 \rightarrow 8(j+1)+1}, & i = 4s + (j+1)_s; \\ 0, & \text{otherwise.} \end{cases}$$

If  $6s \leq j < 7s$ , then

$$b_{ij} = \begin{cases} -e_{8(j+m+1)+1} \otimes w_{8j+4 \rightarrow 8(j+1)+2}, & i = 6s + (j+1)_s; \\ 0, & \text{otherwise.} \end{cases}$$

If  $7s \leq j < 10s$ , then  $b_{ij} = 0$ .

If  $10s \leq j < 11s$ , then

$$b_{ij} = \begin{cases} w_{8(j+m+1)+4 \rightarrow 8(j+m+1)+7} \otimes w_{8j+7 \rightarrow 8(j+1)+1}, & i = 3s + (j+1)_s; \\ -w_{8(j+m+1)+6 \rightarrow 8(j+m+1)+7} \otimes w_{8j+7 \rightarrow 8(j+1)+1}, & i = 4s + (j+1)_s; \\ w_{8(j+m+1)+5 \rightarrow 8(j+m+1)+7} \otimes w_{8j+7 \rightarrow 8(j+1)+2}, & i = 5s + (j+1)_s; \\ -w_{8(j+m+1)+6 \rightarrow 8(j+m+1)+7} \otimes w_{8j+7 \rightarrow 8(j+1)+3}, & i = 8s + (j+1)_s; \\ 0, & \text{otherwise.} \end{cases}$$

(18) If  $r_0 = 17$ , then  $\Omega^{17}(Z_t^{(17)})$  is described with  $(18s \times 11s)$  matrix, whose entries  $b_{ij}$  have the following form:

If  $0 \leq j < s$ , then

$$b_{ij} = \begin{cases} -e_{8(j+m+1)+5} \otimes w_{8j \rightarrow 8(j+1)}, & i = 3s + (j+1)_s; \\ -w_{8(j+m)+7 \rightarrow 8(j+m+1)+5} \otimes w_{8j \rightarrow 8j+1}, & i = j + 4s; \\ -w_{8(j+m+1) \rightarrow 8(j+m+1)+5} \otimes w_{8j \rightarrow 8j+2}, & i = j + 6s; \\ 0, & \text{otherwise.} \end{cases}$$

If  $s \leq j < 2s$ , then

$$b_{ij} = \begin{cases} -w_{8(j+m+1)+2 \rightarrow 8(j+m+1)+3} \otimes w_{8j \rightarrow 8(j+1)}, & i = (j+1)_s; \\ -w_{8(j+m)+7 \rightarrow 8(j+m+1)+3} \otimes w_{8j \rightarrow 8j+1}, & i = j + 3s; \\ 0, & \text{otherwise.} \end{cases}$$

If  $2s \leq j < 3s$ , then  $b_{ij} = 0$ .

If  $3s \leq j < 4s$ , then

$$b_{ij} = \begin{cases} -w_{8(j+m+1)+2 \rightarrow 8(j+m+1)+4} \otimes w_{8j+1 \rightarrow 8(j+1)}, & i = (j+1)_s; \\ 0, & \text{otherwise.} \end{cases}$$

If  $4s \leq j < 5s$ , then

$$b_{ij} = \begin{cases} -w_{8(j+m+1)+4 \rightarrow 8(j+m+1)+7} \otimes w_{8j+2 \rightarrow 8(j+1)}, & i = s + (j+1)_s; \\ w_{8(j+m+1)+6 \rightarrow 8(j+m+1)+7} \otimes w_{8j+2 \rightarrow 8(j+1)}, & i = 2s + (j+1)_s; \\ -w_{8(j+m+1)+5 \rightarrow 8(j+m+1)+7} \otimes w_{8j+2 \rightarrow 8(j+1)}, & i = 3s + (j+1)_s; \\ -w_{8(j+m+1) \rightarrow 8(j+m+1)+7} \otimes e_{8j+2}, & i = j + 2s; \\ 0, & \text{otherwise.} \end{cases}$$

If  $5s \leq j < 6s$ , then

$$b_{ij} = \begin{cases} -w_{8(j+m+1)+6 \rightarrow 8(j+m+2)} \otimes w_{8j+3 \rightarrow 8j+7}, & i = j + 9s; \\ 0, & \text{otherwise.} \end{cases}$$

If  $6s \leq j < 7s$ , then

$$b_{ij} = \begin{cases} -e_{8(j+m+1)+7} \otimes w_{8j+4 \rightarrow 8(j+1)+1}, & i = 4s + (j+1)_s; \\ 0, & \text{otherwise.} \end{cases}$$

If  $7s \leq j < 9s$ , then  $b_{ij} = 0$ .

If  $9s \leq j < 10s$ , then

$$b_{ij} = \begin{cases} w_{8(j+m+1)+7 \rightarrow 8(j+m+2)+2} \otimes w_{8j+7 \rightarrow 8(j+1)+1}, & i = 4s + (j+1)_s; \\ 0, & \text{otherwise.} \end{cases}$$

If  $10s \leq j < 11s$ , then

$$b_{ij} = \begin{cases} w_{8(j+m+1)+7 \rightarrow 8(j+m+2)+6} \otimes w_{8j+7 \rightarrow 8(j+1)+1}, & i = 4s + (j+1)_s; \\ w_{8(j+m+2) \rightarrow 8(j+m+2)+6} \otimes w_{8j+7 \rightarrow 8(j+1)+2}, & i = 6s + (j+1)_s; \\ 0, & \text{otherwise.} \end{cases}$$

(19) If  $r_0 = 18$ , then  $\Omega^{18}(Z_t^{(17)})$  is described with  $(19s \times 13s)$  matrix, whose entries  $b_{ij}$  have the following form:

If  $0 \leq j < s$ , then

$$b_{ij} = \begin{cases} -e_{8(j+m)+7} \otimes w_{8j \rightarrow 8(j+1)}, & i = (j+1)_s; \\ w_{8(j+m)+5 \rightarrow 8(j+m)+7} \otimes w_{8j \rightarrow 8j+1}, & i = j+3s; \\ -w_{8(j+m)+1 \rightarrow 8(j+m)+7} \otimes w_{8j \rightarrow 8j+1}, & i = j+4s; \\ -w_{8(j+m)+2 \rightarrow 8(j+m)+7} \otimes w_{8j \rightarrow 8j+2}, & i = j+5s; \\ 0, & \text{otherwise.} \end{cases}$$

If  $s \leq j < 2s$ , then

$$b_{ij} = \begin{cases} e_{8(j+m+1)} \otimes w_{8j \rightarrow 8(j+1)}, & i = s + (j+1)_s; \\ e_{8(j+m+1)} \otimes w_{8j \rightarrow 8(j+1)}, & i = 2s + (j+1)_s; \\ w_{8(j+m)+6 \rightarrow 8(j+m+1)} \otimes w_{8j \rightarrow 8j+2}, & i = j+5s; \\ 0, & \text{otherwise.} \end{cases}$$

If  $2s \leq j < 3s$ , then

$$b_{ij} = \begin{cases} -w_{8(j+m)+7 \rightarrow 8(j+m+1)+4} \otimes w_{8j+1 \rightarrow 8(j+1)}, & i = (j+1)_s; \\ 0, & \text{otherwise.} \end{cases}$$

If  $3s \leq j < 4s$ , then

$$b_{ij} = \begin{cases} -w_{8(j+m+1) \rightarrow 8(j+m+1)+5} \otimes w_{8j+2 \rightarrow 8(j+1)}, & i = s + (j+1)_s; \\ w_{8(j+m+1) \rightarrow 8(j+m+1)+5} \otimes w_{8j+2 \rightarrow 8(j+1)}, & i = 2s + (j+1)_s; \\ w_{8(j+m)+6 \rightarrow 8(j+m+1)+5} \otimes e_{8j+2}, & i = j+3s; \\ 0, & \text{otherwise.} \end{cases}$$

If  $4s \leq j < 5s$ , then

$$b_{ij} = \begin{cases} -w_{8(j+m)+7 \rightarrow 8(j+m+1)+6} \otimes w_{8j+3 \rightarrow 8j+7}, & i = j+12s; \\ 0, & \text{otherwise.} \end{cases}$$

If  $5s \leq j < 12s$ , then  $b_{ij} = 0$ .

If  $12s \leq j < 13s$ , then

$$b_{ij} = \begin{cases} w_{8(j+m+1)+6 \rightarrow 8(j+m+2)} \otimes w_{8j+7 \rightarrow 8(j+1)+2}, & i = 6s + (j+1)_s; \\ 0, & \text{otherwise.} \end{cases}$$

(20) If  $r_0 = 19$ , then  $\Omega^{19}(Z_t^{(17)})$  is described with  $(16s \times 14s)$  matrix, whose entries  $b_{ij}$  have the following form:

If  $0 \leq j < s$ , then

$$b_{ij} = \begin{cases} -w_{8(j+m+1)+1 \rightarrow 8(j+m+1)+2} \otimes w_{8j \rightarrow 8(j+1)}, & i = 2s + (j+1)_s; \\ -w_{8(j+m+1) \rightarrow 8(j+m+1)+2} \otimes w_{8j \rightarrow 8j+1}, & i = j + 4s; \\ 0, & \text{otherwise.} \end{cases}$$

If  $s \leq j < 2s$ , then

$$b_{ij} = \begin{cases} w_{8(j+m+1)+3 \rightarrow 8(j+m+1)+4} \otimes w_{8j \rightarrow 8(j+1)}, & i = (j+1)_s; \\ w_{8(j+m+1)+1 \rightarrow 8(j+m+1)+4} \otimes w_{8j \rightarrow 8(j+1)}, & i = 2s + (j+1)_s; \\ 0, & \text{otherwise.} \end{cases}$$

If  $2s \leq j < 3s$ , then

$$b_{ij} = \begin{cases} e_{8(j+m+1)+6} \otimes w_{8j \rightarrow 8(j+1)}, & i = s + (j+1)_s; \\ w_{8(j+m+1)+5 \rightarrow 8(j+m+1)+6} \otimes w_{8j \rightarrow 8(j+1)}, & i = 3s + (j+1)_s; \\ w_{8(j+m)+7 \rightarrow 8(j+m+1)+6} \otimes w_{8j \rightarrow 8j+2}, & i = j + 3s; \\ 0, & \text{otherwise.} \end{cases}$$

If  $3s \leq j < 4s$ , then

$$b_{ij} = \begin{cases} -e_{8(j+m+1)+5} \otimes w_{8j \rightarrow 8(j+1)}, & i = 3s + (j+1)_s; \\ 0, & \text{otherwise.} \end{cases}$$

If  $4s \leq j < 5s$ , then

$$b_{ij} = \begin{cases} w_{8(j+m+1)+3 \rightarrow 8(j+m+1)+7} \otimes w_{8j+1 \rightarrow 8(j+1)}, & i = (j+1)_s; \\ w_{8(j+m+1)+6 \rightarrow 8(j+m+1)+7} \otimes w_{8j+1 \rightarrow 8(j+1)}, & i = s + (j+1)_s; \\ 0, & \text{otherwise.} \end{cases}$$

If  $5s \leq j < 6s$ , then

$$b_{ij} = \begin{cases} w_{8(j+m+1)+3 \rightarrow 8(j+m+2)} \otimes w_{8j+2 \rightarrow 8(j+1)}, & i = (j+1)_s; \\ w_{8(j+m+1)+6 \rightarrow 8(j+m+2)} \otimes w_{8j+2 \rightarrow 8(j+1)}, & i = s + (j+1)_s; \\ 0, & \text{otherwise.} \end{cases}$$

If  $6s \leq j < 7s$ , then

$$b_{ij} = \begin{cases} w_{8(j+m+1)+5 \rightarrow 8(j+m+1)+7} \otimes w_{8j+3 \rightarrow 8(j+1)}, & i = 3s + (j+1)_s; \\ -w_{8(j+m+1) \rightarrow 8(j+m+1)+7} \otimes e_{8j+3}, & i = j; \\ -w_{8(j+m)+7 \rightarrow 8(j+m+1)+7} \otimes w_{8j+3 \rightarrow 8j+4}, & i = j + s; \\ w_{8(j+m+1)+2 \rightarrow 8(j+m+1)+7} \otimes w_{8j+3 \rightarrow 8j+7}, & i = j + 6s; \\ 0, & \text{otherwise.} \end{cases}$$

If  $7s \leq j < 14s$ , then  $b_{ij} = 0$ .

(21) If  $r_0 = 20$ , then  $\Omega^{20}(Z_t^{(17)})$  is described with  $(16s \times 16s)$  matrix, whose entries  $b_{ij}$  have the following form:

If  $0 \leq j < s$ , then

$$b_{ij} = \begin{cases} w_{8(j+m)+2 \rightarrow 8(j+m)+7} \otimes w_{8j \rightarrow 8j+1}, & i = j + 2s; \\ w_{8(j+m)+6 \rightarrow 8(j+m)+7} \otimes w_{8j \rightarrow 8j+1}, & i = j + 3s; \\ 0, & \text{otherwise.} \end{cases}$$

If  $s \leq j < 2s$ , then

$$b_{ij} = \begin{cases} -e_{8(j+m)+7} \otimes w_{8j \rightarrow 8(j+1)}, & i = (j + 1)_s; \\ 0, & \text{otherwise.} \end{cases}$$

If  $2s \leq j < 3s$ , then

$$b_{ij} = \begin{cases} -w_{8(j+m)+7 \rightarrow 8(j+m+1)} \otimes w_{8j \rightarrow 8(j+1)}, & i = (j + 1)_s; \\ w_{8(j+m)+2 \rightarrow 8(j+m+1)} \otimes w_{8j \rightarrow 8j+1}, & i = j; \\ -w_{8(j+m)+6 \rightarrow 8(j+m+1)} \otimes w_{8j \rightarrow 8j+1}, & i = j + s; \\ 0, & \text{otherwise.} \end{cases}$$

If  $3s \leq j < 4s$ , then  $b_{ij} = 0$ .

If  $4s \leq j < 5s$ , then

$$b_{ij} = \begin{cases} w_{8(j+m)+7 \rightarrow 8(j+m+1)+6} \otimes w_{8j+2 \rightarrow 8(j+1)}, & i = (j + 1)_s; \\ 0, & \text{otherwise.} \end{cases}$$

If  $5s \leq j < 6s$ , then

$$b_{ij} = \begin{cases} w_{8(j+m)+3 \rightarrow 8(j+m+1)+1} \otimes e_{8j+2}, & i = j - s; \\ 0, & \text{otherwise.} \end{cases}$$

If  $6s \leq j < 7s$ , then

$$b_{ij} = \begin{cases} w_{8(j+m)+7 \rightarrow 8(j+m+1)+2} \otimes w_{8j+3 \rightarrow 8(j+1)}, & i = (j + 1)_s; \\ w_{8(j+m)+4 \rightarrow 8(j+m+1)+2} \otimes e_{8j+3}, & i = j - s; \\ -w_{8(j+m+1) \rightarrow 8(j+m+1)+2} \otimes w_{8j+3 \rightarrow 8j+7}, & i = j + 8s; \\ 0, & \text{otherwise.} \end{cases}$$

If  $7s \leq j < 8s$ , then

$$b_{ij} = \begin{cases} w_{8(j+m)+7 \rightarrow 8(j+m+1)+3} \otimes w_{8j+4 \rightarrow 8(j+1)}, & i = (j + 1)_s; \\ -w_{8(j+m+1) \rightarrow 8(j+m+1)+3} \otimes w_{8j+4 \rightarrow 8(j+1)}, & i = s + (j + 1)_s; \\ -e_{8(j+m+1)+3} \otimes w_{8j+4 \rightarrow 8(j+1)+2}, & i = 4s + (j + 1)_s; \\ 0, & \text{otherwise.} \end{cases}$$

If  $8s \leq j < 14s$ , then  $b_{ij} = 0$ .

If  $14s \leq j < 15s$ , then

$$b_{ij} = \begin{cases} -w_{8(j+m+1)+6 \rightarrow 8(j+m+1)+7} \otimes w_{8j+7 \rightarrow 8(j+1)+1}, & i = 3s + (j + 1)_s; \\ 0, & \text{otherwise.} \end{cases}$$

If  $15s \leq j < 16s$ , then

$$b_{ij} = \begin{cases} -w_{8(j+m+1)+6 \rightarrow 8(j+m+2)} \otimes w_{8j+7 \rightarrow 8(j+1)+1}, & i = 3s + (j+1)_s; \\ 0, & \text{otherwise.} \end{cases}$$

(22) If  $r_0 = 21$ , then  $\Omega^{21}(Z_t^{(17)})$  is described with  $(14s \times 16s)$  matrix, whose entries  $b_{ij}$  have the following form:

If  $0 \leq j < s$ , then

$$b_{ij} = \begin{cases} -w_{8(j+m)+7 \rightarrow 8(j+m+1)+5} \otimes w_{8j \rightarrow 8j+1}, & i = j + 3s; \\ 0, & \text{otherwise.} \end{cases}$$

If  $s \leq j < 2s$ , then

$$b_{ij} = \begin{cases} w_{8(j+m)+7 \rightarrow 8(j+m+1)+3} \otimes w_{8j \rightarrow 8j+1}, & i = j + 2s; \\ w_{8(j+m+1) \rightarrow 8(j+m+1)+3} \otimes w_{8j \rightarrow 8j+2}, & i = j + 3s; \\ 0, & \text{otherwise.} \end{cases}$$

If  $2s \leq j < 3s$ , then  $b_{ij} = 0$ .

If  $3s \leq j < 4s$ , then

$$b_{ij} = \begin{cases} -w_{8(j+m)+7 \rightarrow 8(j+m+1)+1} \otimes w_{8j \rightarrow 8j+1}, & i = j; \\ 0, & \text{otherwise.} \end{cases}$$

If  $4s \leq j < 5s$ , then

$$b_{ij} = \begin{cases} -w_{8(j+m+1)+2 \rightarrow 8(j+m+2)} \otimes w_{8j+1 \rightarrow 8(j+1)}, & i = (j+1)_s; \\ -w_{8(j+m+1)+6 \rightarrow 8(j+m+2)} \otimes w_{8j+1 \rightarrow 8(j+1)}, & i = 2s + (j+1)_s; \\ 0, & \text{otherwise.} \end{cases}$$

If  $5s \leq j < 6s$ , then

$$b_{ij} = \begin{cases} -w_{8(j+m+1)+2 \rightarrow 8(j+m+1)+7} \otimes w_{8j+2 \rightarrow 8(j+1)}, & i = (j+1)_s; \\ w_{8(j+m+1)+6 \rightarrow 8(j+m+1)+7} \otimes w_{8j+2 \rightarrow 8(j+1)}, & i = 2s + (j+1)_s; \\ w_{8(j+m+1) \rightarrow 8(j+m+1)+7} \otimes e_{8j+2}, & i = j - s; \\ 0, & \text{otherwise.} \end{cases}$$

If  $6s \leq j < 7s$ , then

$$b_{ij} = \begin{cases} -w_{8(j+m+1)+2 \rightarrow 8(j+m+2)} \otimes w_{8j+3 \rightarrow 8(j+1)}, & i = (j+1)_s; \\ w_{8(j+m+1)+3 \rightarrow 8(j+m+2)} \otimes w_{8j+3 \rightarrow 8j+7}, & i = j + 4s; \\ 0, & \text{otherwise.} \end{cases}$$

If  $7s \leq j < 8s$ , then

$$b_{ij} = \begin{cases} -w_{8(j+m+1)+2 \rightarrow 8(j+m+1)+7} \otimes w_{8j+4 \rightarrow 8(j+1)}, & i = (j+1)_s; \\ -e_{8(j+m+1)+7} \otimes w_{8j+4 \rightarrow 8(j+1)+1}, & i = 3s + (j+1)_s; \\ 0, & \text{otherwise.} \end{cases}$$

If  $8s \leq j < 12s$ , then  $b_{ij} = 0$ .

If  $12s \leq j < 13s$ , then

$$b_{ij} = \begin{cases} w_{8(j+m+2) \rightarrow 8(j+m+2)+2} \otimes w_{8j+7 \rightarrow 8(j+1)+2}, & i = 4s + (j+1)_s; \\ 0, & \text{otherwise.} \end{cases}$$

If  $13s \leq j < 14s$ , then  $b_{ij} = 0$ .

If  $14s \leq j < 15s$ , then

$$b_{ij} = \begin{cases} w_{8(j+m+1)+7 \rightarrow 8(j+m+2)+6} \otimes w_{8j+7 \rightarrow 8(j+1)+1}, & i = 3s + (j+1)_s; \\ 0, & \text{otherwise.} \end{cases}$$

If  $15s \leq j < 16s$ , then

$$b_{ij} = \begin{cases} w_{8(j+m+1)+7 \rightarrow 8(j+m+2)+5} \otimes w_{8j+7 \rightarrow 8(j+1)+1}, & i = 3s + (j+1)_s; \\ 0, & \text{otherwise.} \end{cases}$$

(23) If  $r_0 = 22$ , then  $\Omega^{22}(Z_t^{(17)})$  is described with  $(13s \times 19s)$  matrix, whose entries  $b_{ij}$  have the following form:

If  $0 \leq j < s$ , then

$$b_{ij} = \begin{cases} e_{8(j+m)+7} \otimes w_{8j \rightarrow 8(j+1)}, & i = s + (j+1)_s; \\ -w_{8(j+m)+3 \rightarrow 8(j+m)+7} \otimes w_{8j \rightarrow 8j+1}, & i = j + 2s; \\ w_{8(j+m)+4 \rightarrow 8(j+m)+7} \otimes w_{8j \rightarrow 8j+2}, & i = j + 3s; \\ 0, & \text{otherwise.} \end{cases}$$

If  $s \leq j < 2s$ , then

$$b_{ij} = \begin{cases} w_{8(j+m)+3 \rightarrow 8(j+m+1)} \otimes w_{8j \rightarrow 8j+1}, & i = j + s; \\ 0, & \text{otherwise.} \end{cases}$$

If  $2s \leq j < 3s$ , then

$$b_{ij} = \begin{cases} -e_{8(j+m+1)} \otimes w_{8j \rightarrow 8(j+1)}, & i = (j+1)_s; \\ w_{8(j+m)+7 \rightarrow 8(j+m+1)} \otimes w_{8j \rightarrow 8(j+1)}, & i = s + (j+1)_s; \\ 0, & \text{otherwise.} \end{cases}$$

If  $3s \leq j < 4s$ , then

$$b_{ij} = \begin{cases} w_{8(j+m)+7 \rightarrow 8(j+m+1)+6} \otimes w_{8j+1 \rightarrow 8(j+1)}, & i = s + (j+1)_s; \\ 0, & \text{otherwise.} \end{cases}$$

If  $4s \leq j < 5s$ , then

$$b_{ij} = \begin{cases} w_{8(j+m+1) \rightarrow 8(j+m+1)+1} \otimes w_{8j+1 \rightarrow 8(j+1)}, & i = (j+1)_s; \\ -w_{8(j+m)+7 \rightarrow 8(j+m+1)+1} \otimes w_{8j+1 \rightarrow 8(j+1)}, & i = s + (j+1)_s; \\ 0, & \text{otherwise.} \end{cases}$$



If  $5s \leq j < 6s$ , then

$$b_{ij} = \begin{cases} w_{8(j+m+1) \rightarrow 8(j+m+1)+2} \otimes w_{8j+2 \rightarrow 8(j+1)}, & i = (j+1)_s; \\ w_{8(j+m)+7 \rightarrow 8(j+m+1)+2} \otimes w_{8j+2 \rightarrow 8(j+1)}, & i = s + (j+1)_s; \\ -w_{8(j+m)+4 \rightarrow 8(j+m+1)+2} \otimes e_{8j+2}, & i = j - 2s; \\ 0, & \text{otherwise.} \end{cases}$$

If  $6s \leq j < 7s$ , then

$$b_{ij} = \begin{cases} -w_{8(j+m)+7 \rightarrow 8(j+m+1)+3} \otimes w_{8j+3 \rightarrow 8j+7}, & i = j + 5s; \\ 0, & \text{otherwise.} \end{cases}$$

If  $7s \leq j < 19s$ , then  $b_{ij} = 0$ .

(24) If  $r_0 = 23$ , then  $\Omega^{23}(Z_t^{(17)})$  is described with  $(11s \times 18s)$  matrix, whose entries  $b_{ij}$  have the following form:

If  $0 \leq j < s$ , then

$$b_{ij} = \begin{cases} -w_{8(j+m+1) \rightarrow 8(j+m+1)+2} \otimes w_{8j \rightarrow 8j+1}, & i = j + 2s; \\ 0, & \text{otherwise.} \end{cases}$$

If  $s \leq j < 2s$ , then

$$b_{ij} = \begin{cases} -w_{8(j+m+1)+5 \rightarrow 8(j+m+1)+6} \otimes w_{8j \rightarrow 8(j+1)}, & i = s + (j+1)_s; \\ 0, & \text{otherwise.} \end{cases}$$

If  $2s \leq j < 3s$ , then

$$b_{ij} = \begin{cases} w_{8(j+m+1)+3 \rightarrow 8(j+m+1)+4} \otimes w_{8j \rightarrow 8(j+1)}, & i = (j+1)_s; \\ w_{8(j+m+1) \rightarrow 8(j+m+1)+4} \otimes w_{8j \rightarrow 8j+1}, & i = j; \\ w_{8(j+m)+7 \rightarrow 8(j+m+1)+4} \otimes w_{8j \rightarrow 8j+2}, & i = j + s; \\ 0, & \text{otherwise.} \end{cases}$$

If  $3s \leq j < 5s$ , then  $b_{ij} = 0$ .

If  $5s \leq j < 6s$ , then

$$b_{ij} = \begin{cases} w_{8(j+m+1)+3 \rightarrow 8(j+m+1)+7} \otimes w_{8j+1 \rightarrow 8(j+1)}, & i = (j+1)_s; \\ -w_{8(j+m+1)+5 \rightarrow 8(j+m+1)+7} \otimes w_{8j+1 \rightarrow 8(j+1)}, & i = s + (j+1)_s; \\ w_{8(j+m)+7 \rightarrow 8(j+m+1)+7} \otimes w_{8j+1 \rightarrow 8j+2}, & i = j - 2s; \\ 0, & \text{otherwise.} \end{cases}$$

If  $6s \leq j < 7s$ , then

$$b_{ij} = \begin{cases} -w_{8(j+m+1)+3 \rightarrow 8(j+m+2)} \otimes w_{8j+2 \rightarrow 8(j+1)}, & i = (j+1)_s; \\ 0, & \text{otherwise.} \end{cases}$$

If  $7s \leq j < 8s$ , then

$$b_{ij} = \begin{cases} -w_{8(j+m+1) \rightarrow 8(j+m+1)+7} \otimes e_{8j+3}, & i = j - 3s; \\ w_{8(j+m+1)+4 \rightarrow 8(j+m+1)+7} \otimes w_{8j+3 \rightarrow 8j+7}, & i = j + 2s; \\ 0, & \text{otherwise.} \end{cases}$$

If  $8s \leq j < 15s$ , then  $b_{ij} = 0$ .

If  $15s \leq j < 16s$ , then

$$b_{ij} = \begin{cases} w_{8(j+m+1)+7 \rightarrow 8(j+m+2)+3} \otimes w_{8j+7 \rightarrow 8(j+1)+2}, & i = 3s + (j+1)_s; \\ 0, & \text{otherwise.} \end{cases}$$

If  $16s \leq j < 18s$ , then  $b_{ij} = 0$ .

(25) If  $r_0 = 24$ , then  $\Omega^{24}(Z_t^{(17)})$  is described with  $(11s \times 19s)$  matrix, whose entries  $b_{ij}$  have the following form:

If  $0 \leq j < s$ , then

$$b_{ij} = \begin{cases} w_{8(j+m)+4 \rightarrow 8(j+m)+7} \otimes w_{8j \rightarrow 8j+1}, & i = j + s; \\ w_{8(j+m)+5 \rightarrow 8(j+m)+7} \otimes w_{8j \rightarrow 8j+1}, & i = j + 2s; \\ 0, & \text{otherwise.} \end{cases}$$

If  $s \leq j < 2s$ , then

$$b_{ij} = \begin{cases} -e_{8(j+m+1)} \otimes w_{8j \rightarrow 8(j+1)}, & i = (j+1)_s; \\ -w_{8(j+m)+5 \rightarrow 8(j+m+1)} \otimes w_{8j \rightarrow 8j+1}, & i = j + s; \\ 0, & \text{otherwise.} \end{cases}$$

If  $2s \leq j < 3s$ , then

$$b_{ij} = \begin{cases} w_{8(j+m)+4 \rightarrow 8(j+m)+7} \otimes w_{8j \rightarrow 8j+1}, & i = j - s; \\ 0, & \text{otherwise.} \end{cases}$$

If  $3s \leq j < 4s$ , then

$$b_{ij} = \begin{cases} w_{8(j+m+1) \rightarrow 8(j+m+1)+2} \otimes w_{8j+1 \rightarrow 8(j+1)}, & i = (j+1)_s; \\ 0, & \text{otherwise.} \end{cases}$$

If  $4s \leq j < 5s$ , then

$$b_{ij} = \begin{cases} w_{8(j+m+1) \rightarrow 8(j+m+1)+3} \otimes w_{8j+2 \rightarrow 8(j+1)}, & i = (j+1)_s; \\ w_{8(j+m+1) \rightarrow 8(j+m+1)+3} \otimes w_{8j+2 \rightarrow 8j+7}, & i = j + 5s; \\ 0, & \text{otherwise.} \end{cases}$$

If  $5s \leq j < 6s$ , then  $b_{ij} = 0$ .

If  $6s \leq j < 7s$ , then

$$b_{ij} = \begin{cases} -w_{8(j+m+1) \rightarrow 8(j+m+1)+4} \otimes w_{8j+3 \rightarrow 8j+7}, & i = j + 3s; \\ 0, & \text{otherwise.} \end{cases}$$

If  $7s \leq j < 18s$ , then  $b_{ij} = 0$ .

If  $18s \leq j < 19s$ , then

$$b_{ij} = \begin{cases} w_{8(j+m+1)+4 \rightarrow 8(j+m+2)} \otimes w_{8j+7 \rightarrow 8(j+1)+1}, & i = s + (j+1)_s; \\ 0, & \text{otherwise.} \end{cases}$$

(26) If  $r_0 = 25$ , then  $\Omega^{25}(Z_t^{(17)})$  is described with  $(10s \times 18s)$  matrix, whose entries  $b_{ij}$  have the following form:

If  $s \leq j < 2s$ , then

$$b_{ij} = \begin{cases} w_{8(j+m)+7 \rightarrow 8(j+m+1)+3} \otimes w_{8j \rightarrow 8j+1}, & i = j + s; \\ w_{8(j+m+1) \rightarrow 8(j+m+1)+3} \otimes w_{8j \rightarrow 8j+2}, & i = j + 2s; \\ 0, & \text{otherwise.} \end{cases}$$

If  $2s \leq j < 3s$ , then  $b_{ij} = 0$ .

If  $3s \leq j < 4s$ , then

$$b_{ij} = \begin{cases} w_{8(j+m)+7 \rightarrow 8(j+m+1)+5} \otimes w_{8j \rightarrow 8j+1}, & i = j - s; \\ w_{8(j+m+1) \rightarrow 8(j+m+1)+5} \otimes w_{8j \rightarrow 8j+2}, & i = j; \\ w_{8(j+m+1) \rightarrow 8(j+m+1)+5} \otimes w_{8j \rightarrow 8j+6}, & i = j + 4s; \\ 0, & \text{otherwise.} \end{cases}$$

If  $4s \leq j < 5s$ , then

$$b_{ij} = \begin{cases} w_{8(j+m+1)+4 \rightarrow 8(j+m+2)} \otimes w_{8j+1 \rightarrow 8(j+1)}, & i = (j+1)_s; \\ w_{8(j+m+1)+6 \rightarrow 8(j+m+2)} \otimes w_{8j+1 \rightarrow 8(j+1)}, & i = s + (j+1)_s; \\ 0, & \text{otherwise.} \end{cases}$$

If  $5s \leq j < 6s$ , then

$$b_{ij} = \begin{cases} -w_{8(j+m+1)+4 \rightarrow 8(j+m+1)+7} \otimes w_{8j+2 \rightarrow 8(j+1)}, & i = (j+1)_s; \\ 0, & \text{otherwise.} \end{cases}$$

If  $6s \leq j < 7s$ , then

$$b_{ij} = \begin{cases} -w_{8(j+m+1)+5 \rightarrow 8(j+m+1)+7} \otimes w_{8j+3 \rightarrow 8j+7}, & i = j + 3s; \\ 0, & \text{otherwise.} \end{cases}$$

If  $7s \leq j < 18s$ , then  $b_{ij} = 0$ .

(27) If  $r_0 = 26$ , then  $\Omega^{26}(Z_t^{(17)})$  is described with  $(8s \times 20s)$  matrix, whose entries  $b_{ij}$  have the following form:

If  $0 \leq j < s$ , then

$$b_{ij} = \begin{cases} w_{8(j+m-1)+7 \rightarrow 8(j+m)+7} \otimes e_{8j}, & i = j; \\ e_{8(j+m)+7} \otimes w_{8j \rightarrow 8(j+1)}, & i = (j+1)_s; \\ w_{8(j+m)+6 \rightarrow 8(j+m)+7} \otimes w_{8j \rightarrow 8j+1}, & i = j + s; \\ w_{8(j+m)+1 \rightarrow 8(j+m)+7} \otimes w_{8j \rightarrow 8j+2}, & i = j + 2s; \\ -w_{8(j+m)+2 \rightarrow 8(j+m)+7} \otimes w_{8j \rightarrow 8j+3}, & i = j + 3s; \\ w_{8(j+m)+3 \rightarrow 8(j+m)+7} \otimes w_{8j \rightarrow 8j+4}, & i = j + 4s; \\ w_{8(j+m)+4 \rightarrow 8(j+m)+7} \otimes w_{8j \rightarrow 8j+5}, & i = j + 5s; \\ 0, & \text{otherwise.} \end{cases}$$

If  $s \leq j < 2s$ , then

$$b_{ij} = \begin{cases} w_{8(j+m)+6 \rightarrow 8(j+m+1)} \otimes w_{8j \rightarrow 8j+1}, & i = j; \\ 0, & \text{otherwise.} \end{cases}$$

If  $2s \leq j < 3s$ , then  $b_{ij} = 0$ .

If  $3s \leq j < 4s$ , then

$$b_{ij} = \begin{cases} -w_{8(j+m)+7 \rightarrow 8(j+m+1)+3} \otimes w_{8j+1 \rightarrow 8(j+1)}, & i = (j+1)_s; \\ 0, & \text{otherwise.} \end{cases}$$

If  $4s \leq j < 5s$ , then

$$b_{ij} = \begin{cases} -w_{8(j+m)+7 \rightarrow 8(j+m+1)+5} \otimes w_{8j+1 \rightarrow 8(j+1)}, & i = (j+1)_s; \\ 0, & \text{otherwise.} \end{cases}$$

If  $5s \leq j < 6s$ , then

$$b_{ij} = \begin{cases} w_{8(j+m)+7 \rightarrow 8(j+m+1)+4} \otimes w_{8j+2 \rightarrow 8(j+1)}, & i = (j+1)_s; \\ w_{8(j+m+1)+1 \rightarrow 8(j+m+1)+4} \otimes w_{8j+2 \rightarrow 8(j+1)+2}, & i = 2s + (j+1)_s; \\ 0, & \text{otherwise.} \end{cases}$$

If  $6s \leq j < 7s$ , then  $b_{ij} = 0$ .

If  $7s \leq j < 8s$ , then

$$b_{ij} = \begin{cases} -w_{8(j+m+1) \rightarrow 8(j+m+1)+5} \otimes w_{8j+3 \rightarrow 8j+7}, & i = j; \\ 0, & \text{otherwise.} \end{cases}$$

If  $8s \leq j < 10s$ , then  $b_{ij} = 0$ .

If  $10s \leq j < 11s$ , then

$$b_{ij} = \begin{cases} e_{8(j+m+1)+6} \otimes w_{8j+4 \rightarrow 8(j+1)+1}, & i = s + (j+1)_s; \\ 0, & \text{otherwise.} \end{cases}$$

If  $11s \leq j < 17s$ , then  $b_{ij} = 0$ .

If  $17s \leq j < 18s$ , then

$$b_{ij} = \begin{cases} w_{8(j+m)+7 \rightarrow 8(j+m+1)+7} \otimes w_{8j+7 \rightarrow 8(j+1)}, & i = (j+1)_s; \\ w_{8(j+m+1)+1 \rightarrow 8(j+m+1)+7} \otimes w_{8j+7 \rightarrow 8(j+1)+2}, & i = 2s + (j+1)_s; \\ -w_{8(j+m+1)+2 \rightarrow 8(j+m+1)+7} \otimes w_{8j+7 \rightarrow 8(j+1)+3}, & i = 3s + (j+1)_s; \\ w_{8(j+m+1)+3 \rightarrow 8(j+m+1)+7} \otimes w_{8j+7 \rightarrow 8(j+1)+4}, & i = 4s + (j+1)_s; \\ w_{8(j+m+1)+4 \rightarrow 8(j+m+1)+7} \otimes w_{8j+7 \rightarrow 8(j+1)+5}, & i = 5s + (j+1)_s; \\ 0, & \text{otherwise.} \end{cases}$$

If  $18s \leq j < 20s$ , then  $b_{ij} = 0$ .

(28) If  $r_0 = 27$ , then  $\Omega^{27}(Z_t^{(17)})$  is described with  $(9s \times 18s)$  matrix, whose entries  $b_{ij}$  have the following form:

If  $0 \leq j < s$ , then

$$b_{ij} = \begin{cases} -w_{8(j+m+1)+2 \rightarrow 8(j+m+1)+3} \otimes w_{8j \rightarrow 8j+3}, & i = j + 3s; \\ w_{8(j+m+1) \rightarrow 8(j+m+1)+3} \otimes w_{8j \rightarrow 8j+5}, & i = j + 5s; \\ 0, & \text{otherwise.} \end{cases}$$

If  $s \leq j < 2s$ , then

$$b_{ij} = \begin{cases} w_{8(j+m+1) \rightarrow 8(j+m+1)+6} \otimes w_{8j \rightarrow 8j+1}, & i = j; \\ 0, & \text{otherwise.} \end{cases}$$

If  $2s \leq j < 4s$ , then  $b_{ij} = 0$ .

If  $4s \leq j < 5s$ , then

$$b_{ij} = \begin{cases} w_{8(j+m+1) \rightarrow 8(j+m+1)+5} \otimes w_{8j \rightarrow 8j+1}, & i = j - 3s; \\ 0, & \text{otherwise.} \end{cases}$$

If  $5s \leq j < 6s$ , then

$$b_{ij} = \begin{cases} e_{8(j+m+1)+7} \otimes w_{8j+1 \rightarrow 8(j+1)}, & i = (j+1)_s; \\ 0, & \text{otherwise.} \end{cases}$$

If  $6s \leq j < 7s$ , then

$$b_{ij} = \begin{cases} e_{8(j+m+1)+7} \otimes w_{8j+2 \rightarrow 8(j+1)}, & i = (j+1)_s; \\ w_{8(j+m+1)+1 \rightarrow 8(j+m+1)+7} \otimes e_{8j+2}, & i = j - 4s; \\ 0, & \text{otherwise.} \end{cases}$$

If  $7s \leq j < 8s$ , then  $b_{ij} = 0$ .

If  $8s \leq j < 9s$ , then

$$b_{ij} = \begin{cases} -w_{8(j+m+1)+2 \rightarrow 8(j+m+2)} \otimes e_{8j+3}, & i = j - 5s; \\ 0, & \text{otherwise.} \end{cases}$$

If  $9s \leq j < 10s$ , then

$$b_{ij} = \begin{cases} -e_{8(j+m+1)+7} \otimes w_{8j+4 \rightarrow 8(j+1)}, & i = (j+1)_s; \\ 0, & \text{otherwise.} \end{cases}$$

If  $10s \leq j < 15s$ , then  $b_{ij} = 0$ .

If  $15s \leq j < 16s$ , then

$$b_{ij} = \begin{cases} w_{8(j+m+1)+7 \rightarrow 8(j+m+2)+3} \otimes w_{8j+7 \rightarrow 8(j+1)}, & i = (j+1)_s; \\ 0, & \text{otherwise.} \end{cases}$$

If  $16s \leq j < 18s$ , then  $b_{ij} = 0$ .

(29) If  $r_0 = 28$ , then  $\Omega^{28}(Z_t^{(17)})$  is described with  $(8s \times 19s)$  matrix, whose entries  $b_{ij}$  have the following form:

If  $0 \leq j < s$ , then

$$b_{ij} = \begin{cases} w_{8(j+m)+3 \rightarrow 8(j+m)+7} \otimes w_{8j \rightarrow 8j+3}, & i = j + 3s; \\ -w_{8(j+m)+4 \rightarrow 8(j+m)+7} \otimes w_{8j \rightarrow 8j+4}, & i = j + 4s; \\ -w_{8(j+m)+5 \rightarrow 8(j+m)+7} \otimes w_{8j \rightarrow 8j+5}, & i = j + 5s; \\ w_{8(j+m)+6 \rightarrow 8(j+m)+7} \otimes w_{8j \rightarrow 8j+6}, & i = j + 6s; \\ -e_{8(j+m)+7} \otimes w_{8j \rightarrow 8j+7}, & i = j + 7s; \\ 0, & \text{otherwise.} \end{cases}$$

If  $s \leq j < 2s$ , then

$$b_{ij} = \begin{cases} w_{8(j+m) \rightarrow 8(j+m+1)} \otimes e_{8j}, & i = j - s; \\ -w_{8(j+m)+1 \rightarrow 8(j+m+1)} \otimes w_{8j \rightarrow 8j+1}, & i = j; \\ w_{8(j+m)+3 \rightarrow 8(j+m+1)} \otimes w_{8j \rightarrow 8j+3}, & i = j + 2s; \\ -w_{8(j+m)+4 \rightarrow 8(j+m+1)} \otimes w_{8j \rightarrow 8j+4}, & i = j + 3s; \\ -w_{8(j+m)+5 \rightarrow 8(j+m+1)} \otimes w_{8j \rightarrow 8j+5}, & i = j + 4s; \\ w_{8(j+m)+6 \rightarrow 8(j+m+1)} \otimes w_{8j \rightarrow 8j+6}, & i = j + 5s; \\ -w_{8(j+m)+7 \rightarrow 8(j+m+1)} \otimes w_{8j \rightarrow 8j+7}, & i = j + 6s; \\ 0, & \text{otherwise.} \end{cases}$$

If  $2s \leq j < 3s$ , then

$$b_{ij} = \begin{cases} -w_{8(j+m)+1 \rightarrow 8(j+m)+7} \otimes w_{8j \rightarrow 8j+1}, & i = j - s; \\ 0, & \text{otherwise.} \end{cases}$$

If  $3s \leq j < 4s$ , then

$$b_{ij} = \begin{cases} -w_{8(j+m+1) \rightarrow 8(j+m+1)+4} \otimes w_{8j+1 \rightarrow 8(j+1)}, & i = (j+1)_s; \\ w_{8(j+m+1)+1 \rightarrow 8(j+m+1)+4} \otimes w_{8j+1 \rightarrow 8(j+1)+1}, & i = s + (j+1)_s; \\ 0, & \text{otherwise.} \end{cases}$$

If  $4s \leq j < 5s$ , then

$$b_{ij} = \begin{cases} w_{8(j+m+1) \rightarrow 8(j+m+1)+6} \otimes w_{8j+1 \rightarrow 8(j+1)}, & i = (j+1)_s; \\ 0, & \text{otherwise.} \end{cases}$$

If  $5s \leq j < 6s$ , then

$$b_{ij} = \begin{cases} -w_{8(j+m+1) \rightarrow 8(j+m+1)+5} \otimes w_{8j+2 \rightarrow 8(j+1)}, & i = (j+1)_s; \\ 0, & \text{otherwise.} \end{cases}$$

If  $6s \leq j < 7s$ , then  $b_{ij} = 0$ .

If  $7s \leq j < 8s$ , then

$$b_{ij} = \begin{cases} -w_{8(j+m)+3 \rightarrow 8(j+m+1)+2} \otimes e_{8j+3}, & i = j - 4s; \\ w_{8(j+m)+4 \rightarrow 8(j+m+1)+2} \otimes w_{8j+3 \rightarrow 8j+4}, & i = j - 3s; \\ w_{8(j+m)+7 \rightarrow 8(j+m+1)+2} \otimes w_{8j+3 \rightarrow 8j+7}, & i = j; \\ 0, & \text{otherwise.} \end{cases}$$

If  $8s \leq j < 13s$ , then  $b_{ij} = 0$ .

If  $13s \leq j < 14s$ , then

$$b_{ij} = \begin{cases} w_{8(j+m+1) \rightarrow 8(j+m+1)+3} \otimes w_{8j+6 \rightarrow 8(j+1)}, & i = (j+1)_s; \\ 0, & \text{otherwise.} \end{cases}$$

If  $14s \leq j < 16s$ , then  $b_{ij} = 0$ .

If  $16s \leq j < 17s$ , then

$$b_{ij} = \begin{cases} w_{8(j+m+1) \rightarrow 8(j+m+1)+7} \otimes w_{8j+7 \rightarrow 8(j+1)}, & i = (j+1)_s; \\ -w_{8(j+m+1)+1 \rightarrow 8(j+m+1)+7} \otimes w_{8j+7 \rightarrow 8(j+1)+1}, & i = s + (j+1)_s; \\ w_{8(j+m+1)+2 \rightarrow 8(j+m+1)+7} \otimes w_{8j+7 \rightarrow 8(j+1)+2}, & i = 2s + (j+1)_s; \\ 0, & \text{otherwise.} \end{cases}$$

If  $17s \leq j < 19s$ , then  $b_{ij} = 0$ .

(II) Represent an arbitrary  $t_0 \in \mathbb{N}$  in the form  $t_0 = 29\ell_0 + r_0$ , where  $0 \leq r_0 \leq 28$ . Then  $\Omega^{t_0}(Z_t^{(17)})$  is a  $\Omega^{r_0}(Z_t^{(17)})$ , whose left components twisted by  $\sigma^{\ell_0}$ , and coefficients multiplied by  $(-1)^{\ell_0}$ .

**Proposition 14** (Translates for the case 19). (I) Let  $r_0 \in \mathbb{N}$ ,  $r_0 < 29$ .  $r_0$ -translates of the elements  $Z_t^{(19)}$  are described by the following way.

(1) If  $r_0 = 0$ , then  $\Omega^0(Z_t^{(19)})$  is described with  $(8s \times 19s)$  matrix with unique nonzero entry:

$$b_{j,(1)_s} = -w_{8(j+m) \rightarrow 8(j+m)+7} \otimes e_{8j}.$$

(2) If  $r_0 = 1$ , then  $\Omega^1(Z_t^{(19)})$  is described with  $(9s \times 16s)$  matrix with the following nonzero entries:

$$\begin{aligned} b_{s+(j+1)_s, 4s} &= w_{8(j+m+1)+5 \rightarrow 8(j+m+2)} \otimes w_{8j+1 \rightarrow 8(j+1)}; \\ b_{s+(j+1)_s, 5s} &= -w_{8(j+m+1)+5 \rightarrow 8(j+m+1)+7} \otimes w_{8j+2 \rightarrow 8(j+1)}; \\ b_{(j+1)_s, 8s} &= -w_{8(j+m+1)+1 \rightarrow 8(j+m+1)+7} \otimes w_{8j+5 \rightarrow 8(j+1)}. \end{aligned}$$

(3) If  $r_0 = 2$ , then  $\Omega^2(Z_t^{(19)})$  is described with  $(8s \times 16s)$  matrix with two nonzero entries:

$$\begin{aligned} b_{(j+1)_s, 0} &= e_{8(j+m)+7} \otimes w_{8j \rightarrow 8(j+1)}; \\ b_{(j+1)_s, s} &= w_{8(j+m)+7 \rightarrow 8(j+m+1)} \otimes w_{8j \rightarrow 8(j+1)}. \end{aligned}$$

(4) If  $r_0 = 3$ , then  $\Omega^3(Z_t^{(19)})$  is described with  $(10s \times 14s)$  matrix with two nonzero entries:

$$\begin{aligned} b_{(j+1)_s, s} &= w_{8(j+m+1)+2 \rightarrow 8(j+m+1)+4} \otimes w_{8j \rightarrow 8(j+1)}; \\ b_{s+(j+1)_s, 2s} &= e_{8(j+m+1)+6} \otimes w_{8j \rightarrow 8(j+1)}. \end{aligned}$$

(5) If  $r_0 = 4$ , then  $\Omega^4(Z_t^{(19)})$  is described with  $(11s \times 13s)$  matrix with the following nonzero entries:

$$\begin{aligned} b_{(j+1)_s, 0} &= w_{8(j+m)+7 \rightarrow 8(j+m+1)} \otimes w_{8j \rightarrow 8(j+1)}; \\ b_{s+(j+1)_s, 0} &= e_{8(j+m+1)} \otimes w_{8j \rightarrow 8(j+1)}; \\ b_{(j+1)_s, s} &= e_{8(j+m)+7} \otimes w_{8j \rightarrow 8(j+1)}. \end{aligned}$$

(6) If  $r_0 = 5$ , then  $\Omega^5(Z_t^{(19)})$  is described with  $(11s \times 11s)$  matrix with two nonzero entries:

$$\begin{aligned} b_{2s+(j+1)_s, 0} &= w_{8(j+m+1)+1 \rightarrow 8(j+m+1)+3} \otimes w_{8j \rightarrow 8(j+1)}; \\ b_{(j+1)_s, s} &= e_{8(j+m+1)+5} \otimes w_{8j \rightarrow 8(j+1)}. \end{aligned}$$

(7) If  $r_0 = 6$ , then  $\Omega^6(Z_t^{(19)})$  is described with  $(13s \times 11s)$  matrix with two nonzero entries:

$$\begin{aligned} b_{(j+1)_s, 0} &= -w_{8(j+m)+7 \rightarrow 8(j+m+1)} \otimes w_{8j \rightarrow 8(j+1)}; \\ b_{s+(j+1)_s, 0} &= -e_{8(j+m+1)} \otimes w_{8j \rightarrow 8(j+1)}. \end{aligned}$$

(8) If  $r_0 = 7$ , then  $\Omega^7(Z_t^{(19)})$  is described with  $(14s \times 10s)$  matrix with the following nonzero entries:

$$\begin{aligned} b_{(j+1)s,0} &= -w_{8(j+m+1)+2 \rightarrow 8(j+m+1)+4} \otimes w_{8j \rightarrow 8(j+1)}; \\ b_{2s+(j+1)s,s} &= -e_{8(j+m+1)+6} \otimes w_{8j \rightarrow 8(j+1)}; \\ b_{3s+(j+1)s,s} &= -w_{8(j+m+1)+5 \rightarrow 8(j+m+1)+6} \otimes w_{8j \rightarrow 8(j+1)}. \end{aligned}$$

(9) If  $r_0 = 8$ , then  $\Omega^8(Z_t^{(19)})$  is described with  $(16s \times 8s)$  matrix with unique nonzero entry:

$$b_{(j+1)s,0} = -e_{8(j+m)+7} \otimes w_{8j \rightarrow 8(j+1)}.$$

(10) If  $r_0 = 9$ , then  $\Omega^9(Z_t^{(19)})$  is described with  $(16s \times 9s)$  matrix with unique nonzero entry:

$$b_{s+(j+1)s,0} = -w_{8(j+m+1)+3 \rightarrow 8(j+m+1)+7} \otimes w_{8j \rightarrow 8(j+1)}.$$

(11) If  $r_0 = 10$ , then  $\Omega^{10}(Z_t^{(19)})$  is described with  $(19s \times 8s)$  matrix with unique nonzero entry:

$$b_{s+(j+1)s,0} = -e_{8(j+m+1)} \otimes w_{8j \rightarrow 8(j+1)}.$$

(12) If  $r_0 = 11$ , then  $\Omega^{11}(Z_t^{(19)})$  is described with  $(18s \times 8s)$  matrix with unique nonzero entry:

$$b_{(j+1)s,0} = -w_{8(j+m+1)+2 \rightarrow 8(j+m+2)} \otimes w_{8j \rightarrow 8(j+1)}.$$

(13) If  $r_0 = 12$ , then  $\Omega^{12}(Z_t^{(19)})$  is described with  $(19s \times 9s)$  matrix with two nonzero entries:

$$\begin{aligned} b_{s+(j+1)s,0} &= w_{8(j+m+1) \rightarrow 8(j+m+1)+1} \otimes w_{8j \rightarrow 8(j+1)}; \\ b_{2s+(j+1)s,0} &= w_{8(j+m)+7 \rightarrow 8(j+m+1)+1} \otimes w_{8j \rightarrow 8(j+1)}. \end{aligned}$$

(14) If  $r_0 = 13$ , then  $\Omega^{13}(Z_t^{(19)})$  is described with  $(18s \times 8s)$  matrix with two nonzero entries:

$$\begin{aligned} b_{(j+1)s,0} &= w_{8(j+m+1)+2 \rightarrow 8(j+m+1)+7} \otimes w_{8j \rightarrow 8(j+1)}; \\ b_{s+(j+1)s,0} &= -w_{8(j+m+1)+3 \rightarrow 8(j+m+1)+7} \otimes w_{8j \rightarrow 8(j+1)}. \end{aligned}$$

(15) If  $r_0 = 14$ , then  $\Omega^{14}(Z_t^{(19)})$  is described with  $(20s \times 10s)$  matrix with unique nonzero entry:

$$b_{(j+1)s,0} = -w_{8(j+m)+7 \rightarrow 8(j+m+1)+2} \otimes w_{8j \rightarrow 8(j+1)}.$$

(16) If  $r_0 = 15$ , then  $\Omega^{15}(Z_t^{(19)})$  is described with  $(18s \times 11s)$  matrix with two nonzero entries:

$$\begin{aligned} b_{(j+1)s,0} &= -w_{8(j+m+1)+3 \rightarrow 8(j+m+1)+7} \otimes w_{8j \rightarrow 8(j+1)}; \\ b_{2s+(j+1)s,0} &= w_{8(j+m+1)+4 \rightarrow 8(j+m+1)+7} \otimes w_{8j \rightarrow 8(j+1)}. \end{aligned}$$

(17) If  $r_0 = 16$ , then  $\Omega^{16}(Z_t^{(19)})$  is described with  $(19s \times 11s)$  matrix with unique nonzero entry:

$$b_{s+(j+1)s,s} = -w_{8(j+m+1) \rightarrow 8(j+m+1)+3} \otimes w_{8j \rightarrow 8(j+1)}.$$

(18) If  $r_0 = 17$ , then  $\Omega^{17}(Z_t^{(19)})$  is described with  $(18s \times 13s)$  matrix with the following nonzero entries:

$$\begin{aligned} b_{(j+1)s,0} &= w_{8(j+m+1)+2 \rightarrow 8(j+m+1)+7} \otimes w_{8j \rightarrow 8(j+1)}; \\ b_{s+(j+1)s,0} &= -w_{8(j+m+1)+4 \rightarrow 8(j+m+1)+7} \otimes w_{8j \rightarrow 8(j+1)}; \\ b_{2s+(j+1)s,0} &= w_{8(j+m+1)+6 \rightarrow 8(j+m+1)+7} \otimes w_{8j \rightarrow 8(j+1)}; \\ b_{(j+1)s,s} &= w_{8(j+m+1)+2 \rightarrow 8(j+m+2)} \otimes w_{8j \rightarrow 8(j+1)}. \end{aligned}$$

(19) If  $r_0 = 18$ , then  $\Omega^{18}(Z_t^{(19)})$  is described with  $(19s \times 14s)$  matrix with two nonzero entries:

$$\begin{aligned} b_{s+(j+1)s,0} &= w_{8(j+m+1) \rightarrow 8(j+m+1)+2} \otimes w_{8j \rightarrow 8(j+1)}; \\ b_{(j+1)s,2s} &= w_{8(j+m)+7 \rightarrow 8(j+m+1)+6} \otimes w_{8j \rightarrow 8(j+1)}. \end{aligned}$$



(20) If  $r_0 = 19$ , then  $\Omega^{19}(Z_t^{(19)})$  is described with  $(16s \times 16s)$  matrix with unique nonzero entry:

$$b_{(j+1)s,0} = w_{8(j+m+1)+3 \rightarrow 8(j+m+1)+7} \otimes w_{8j \rightarrow 8(j+1)}.$$

(21) If  $r_0 = 20$ , then  $\Omega^{20}(Z_t^{(19)})$  is described with  $(16s \times 16s)$  matrix with unique nonzero entry:

$$b_{(j+1)s,s} = w_{8(j+m)+7 \rightarrow 8(j+m+1)+3} \otimes w_{8j \rightarrow 8(j+1)}.$$

(22) If  $r_0 = 21$ , then  $\Omega^{21}(Z_t^{(19)})$  is described with  $(14s \times 19s)$  matrix with two nonzero entries:

$$b_{(j+1)s,0} = w_{8(j+m+1)+2 \rightarrow 8(j+m+1)+7} \otimes w_{8j \rightarrow 8(j+1)};$$

$$b_{s+(j+1)s,0} = w_{8(j+m+1)+4 \rightarrow 8(j+m+1)+7} \otimes w_{8j \rightarrow 8(j+1)}.$$

(23) If  $r_0 = 22$ , then  $\Omega^{22}(Z_t^{(19)})$  is described with  $(13s \times 18s)$  matrix with unique nonzero entry:

$$b_{(j+1)s,0} = -w_{8(j+m+1) \rightarrow 8(j+m+1)+2} \otimes w_{8j \rightarrow 8(j+1)}.$$

(24) If  $r_0 = 23$ , then  $\Omega^{23}(Z_t^{(19)})$  is described with  $(11s \times 19s)$  matrix with two nonzero entries:

$$b_{s+(j+1)s,0} = -w_{8(j+m+1)+5 \rightarrow 8(j+m+1)+7} \otimes w_{8j \rightarrow 8(j+1)};$$

$$b_{(j+1)s,s} = w_{8(j+m+1)+3 \rightarrow 8(j+m+2)} \otimes w_{8j \rightarrow 8(j+1)}.$$

(25) If  $r_0 = 24$ , then  $\Omega^{24}(Z_t^{(19)})$  is described with  $(11s \times 18s)$  matrix with unique nonzero entry:

$$b_{(j+1)s,0} = -w_{8(j+m+1) \rightarrow 8(j+m+1)+2} \otimes w_{8j \rightarrow 8(j+1)}.$$

(26) If  $r_0 = 25$ , then  $\Omega^{25}(Z_t^{(19)})$  is described with  $(10s \times 20s)$  matrix with unique nonzero entry:

$$b_{(j+1)s,0} = -w_{8(j+m+1)+4 \rightarrow 8(j+m+1)+7} \otimes w_{8j \rightarrow 8(j+1)}.$$

(27) If  $r_0 = 26$ , then  $\Omega^{26}(Z_t^{(19)})$  is described with  $(8s \times 18s)$  matrix with unique nonzero entry:

$$b_{(j+1)s,0} = -w_{8(j+m)+7 \rightarrow 8(j+m+1)+3} \otimes w_{8j \rightarrow 8(j+1)}.$$

(28) If  $r_0 = 27$ , then  $\Omega^{27}(Z_t^{(19)})$  is described with  $(9s \times 19s)$  matrix with unique nonzero entry:

$$b_{(j+1)s,0} = e_{8(j+m+1)+7} \otimes w_{8j \rightarrow 8(j+1)}.$$

(29) If  $r_0 = 28$ , then  $\Omega^{28}(Z_t^{(19)})$  is described with  $(8s \times 18s)$  matrix with two nonzero entries:

$$b_{(j+1)s,0} = -w_{8(j+m+1) \rightarrow 8(j+m+1)+2} \otimes w_{8j \rightarrow 8(j+1)};$$

$$b_{(j+1)s,s} = -w_{8(j+m+1) \rightarrow 8(j+m+1)+4} \otimes w_{8j \rightarrow 8(j+1)}.$$

(II) Represent an arbitrary  $t_0 \in \mathbb{N}$  in the form  $t_0 = 29\ell_0 + r_0$ , where  $0 \leq r_0 \leq 28$ . Then  $\Omega^{t_0}(Z_t^{(19)})$  is a  $\Omega^{r_0}(Z_t^{(19)})$ , whose left components twisted by  $\sigma^{\ell_0}$ .

**Proposition 15** (Translates for the case 20). (I) Let  $r_0 \in \mathbb{N}$ ,  $r_0 < 29$ .  $r_0$ -translates of the elements  $Z_t^{(20)}$  are described by the following way.

(1) If  $r_0 = 0$ , then  $\Omega^0(Z_t^{(20)})$  is described with  $(8s \times 16s)$  matrix with two nonzero entries:

$$b_{j,0} = w_{8(j+m) \rightarrow 8(j+m)+3} \otimes e_{8j};$$

$$b_{j-3s,3s} = -w_{8(j+m) \rightarrow 8(j+m)+5} \otimes e_{8j}.$$

(2) If  $r_0 = 1$ , then  $\Omega^1(Z_t^{(20)})$  is described with  $(9s \times 16s)$  matrix with the following nonzero entries:

$$b_{s+(j+1)s,3s+(-1)s} = w_{8(j+m+1)+5 \rightarrow 8(j+m+1)+6} \otimes w_{8j+1 \rightarrow 8(j+1)};$$

$$b_{(j+1)s,4s+(-1)s} = -w_{8(j+m+1)+1 \rightarrow 8(j+m+1)+3} \otimes w_{8j+2 \rightarrow 8(j+1)};$$

$$\begin{aligned}
b_{2s+(j+1)s,4s+(-1)s} &= -w_{8(j+m+1)+2 \rightarrow 8(j+m+1)+3} \otimes w_{8j+2 \rightarrow 8(j+1)+1}; \\
b_{3s+(j+1)s,4s+(-1)s} &= -e_{8(j+m+1)+3} \otimes w_{8j+2 \rightarrow 8(j+1)+2}; \\
b_{(j+1)s,5s+(-1)s} &= w_{8(j+m+1)+1 \rightarrow 8(j+m+1)+4} \otimes w_{8j+3 \rightarrow 8(j+1)}; \\
b_{2s+(j+1)s,5s+(-1)s} &= w_{8(j+m+1)+2 \rightarrow 8(j+m+1)+4} \otimes w_{8j+3 \rightarrow 8(j+1)+1}; \\
b_{3s+(j+1)s,5s+(-1)s} &= w_{8(j+m+1)+3 \rightarrow 8(j+m+1)+4} \otimes w_{8j+3 \rightarrow 8(j+1)+2}; \\
b_{4s+(j+1)s,5s+(-1)s} &= e_{8(j+m+1)+4} \otimes w_{8j+3 \rightarrow 8(j+1)+3}; \\
b_{s+(j+1)s,6s+(-1)s} &= e_{8(j+m+1)+5} \otimes w_{8j+3 \rightarrow 8(j+1)}.
\end{aligned}$$

(3) If  $r_0 = 2$ , then  $\Omega^2(Z_t^{(20)})$  is described with  $(8s \times 14s)$  matrix with two nonzero entries:

$$\begin{aligned}
b_{(j+1)s,3s+(-1)s} &= -e_{8(j+m)+7} \otimes w_{8j+1 \rightarrow 8(j+1)}; \\
b_{(j+1)s,5s+(-1)s} &= e_{8(j+m)+7} \otimes w_{8j+3 \rightarrow 8(j+1)}.
\end{aligned}$$

(4) If  $r_0 = 3$ , then  $\Omega^3(Z_t^{(20)})$  is described with  $(10s \times 13s)$  matrix with the following nonzero entries:

$$\begin{aligned}
b_{(j+1)s,3s+(-1)s} &= -w_{8(j+m+1)+2 \rightarrow 8(j+m+1)+4} \otimes w_{8j+2 \rightarrow 8(j+1)}; \\
b_{2s+(j+1)s,3s+(-1)s} &= -w_{8(j+m+1)+3 \rightarrow 8(j+m+1)+4} \otimes w_{8j+2 \rightarrow 8(j+1)+1}; \\
b_{3s+(j+1)s,3s+(-1)s} &= -e_{8(j+m+1)+4} \otimes w_{8j+2 \rightarrow 8(j+1)+2}; \\
b_{s+(j+1)s,5s+(-1)s} &= e_{8(j+m+1)+6} \otimes w_{8j+3 \rightarrow 8(j+1)}.
\end{aligned}$$

(5) If  $r_0 = 4$ , then  $\Omega^4(Z_t^{(20)})$  is described with  $(11s \times 11s)$  matrix with the following nonzero entries:

$$\begin{aligned}
b_{(j+1)s,2s+(-1)s} &= -w_{8(j+m)+7 \rightarrow 8(j+m+1)} \otimes w_{8j+1 \rightarrow 8(j+1)}; \\
b_{s+(j+1)s,2s+(-1)s} &= -e_{8(j+m+1)} \otimes w_{8j+1 \rightarrow 8(j+1)}; \\
b_{(j+1)s,3s+(-1)s} &= -e_{8(j+m)+7} \otimes w_{8j+2 \rightarrow 8(j+1)}; \\
b_{s+(j+1)s,4s+(-1)s} &= e_{8(j+m+1)} \otimes w_{8j+3 \rightarrow 8(j+1)}.
\end{aligned}$$

(6) If  $r_0 = 5$ , then  $\Omega^5(Z_t^{(20)})$  is described with  $(11s \times 11s)$  matrix with the following nonzero entries:

$$\begin{aligned}
b_{(j+1)s,2s+(-1)s} &= -e_{8(j+m+1)+5} \otimes w_{8j+1 \rightarrow 8(j+1)}; \\
b_{(j+1)s,3s+(-1)s} &= -w_{8(j+m+1)+5 \rightarrow 8(j+m+1)+6} \otimes w_{8j+2 \rightarrow 8(j+1)}; \\
b_{2s+(j+1)s,4s+(-1)s} &= -e_{8(j+m+1)+1} \otimes w_{8j+3 \rightarrow 8(j+1)}.
\end{aligned}$$

(7) If  $r_0 = 6$ , then  $\Omega^6(Z_t^{(20)})$  is described with  $(13s \times 10s)$  matrix with the following nonzero entries:

$$\begin{aligned}
b_{(j+1)s,3s+(-1)s} &= -w_{8(j+m)+7 \rightarrow 8(j+m+1)} \otimes w_{8j+2 \rightarrow 8(j+1)}; \\
b_{s+(j+1)s,3s+(-1)s} &= -e_{8(j+m+1)} \otimes w_{8j+2 \rightarrow 8(j+1)}; \\
b_{j+s,4s+(-1)s} &= w_{8(j+m)+1 \rightarrow 8(j+m+1)+1} \otimes e_{8j+3}.
\end{aligned}$$

(8) If  $r_0 = 7$ , then  $\Omega^7(Z_t^{(20)})$  is described with  $(14s \times 8s)$  matrix with the following nonzero entries:

$$\begin{aligned}
b_{2s+(j+1)s,s+(-1)s} &= e_{8(j+m+1)+6} \otimes w_{8j+1 \rightarrow 8(j+1)}; \\
b_{3s+(j+1)s,s+(-1)s} &= w_{8(j+m+1)+5 \rightarrow 8(j+m+1)+6} \otimes w_{8j+1 \rightarrow 8(j+1)}; \\
b_{j+3s,2s+(-1)s} &= -w_{8(j+m+1) \rightarrow 8(j+m+1)+1} \otimes e_{8j+2}.
\end{aligned}$$

(9) If  $r_0 = 8$ , then  $\Omega^8(Z_t^{(20)})$  is described with  $(16s \times 9s)$  matrix with the following nonzero entries:

$$b_{j+4s,(-1)s} = w_{8(j+m)+6 \rightarrow 8(j+m)+7} \otimes w_{8j \rightarrow 8j+2};$$

$$\begin{aligned}
b_{2s+(j+1)_s, s+(-1)_s} &= e_{8(j+m+1)} \otimes w_{8j+1 \rightarrow 8(j+1)}; \\
b_{j+2s, s+(-1)_s} &= w_{8(j+m)+5 \rightarrow 8(j+m+1)} \otimes e_{8j+1}; \\
b_{2s+(j+1)_s, 2s+(-2)_s} &= -w_{8(j+m+1) \rightarrow 8(j+m+1)+1} \otimes w_{8j+2 \rightarrow 8(j+1)}; \\
b_{2s+(j+1)_s, 3s+(-2)_s} &= -w_{8(j+m+1) \rightarrow 8(j+m+1)+2} \otimes w_{8j+3 \rightarrow 8(j+1)}; \\
b_{6s+(j+1)_s, 3s+(-2)_s} &= e_{8(j+m+1)+2} \otimes w_{8j+3 \rightarrow 8(j+1)+3}; \\
b_{2s+(j+1)_s, 4s+(-2)_s} &= -w_{8(j+m+1) \rightarrow 8(j+m+1)+3} \otimes w_{8j+4 \rightarrow 8(j+1)}; \\
b_{6s+(j+1)_s, 4s+(-2)_s} &= w_{8(j+m+1)+2 \rightarrow 8(j+m+1)+3} \otimes w_{8j+4 \rightarrow 8(j+1)+3}; \\
b_{5s+(j+1)_s, 7s+(-2)_s} &= -w_{8(j+m+1)+1 \rightarrow 8(j+m+1)+4} \otimes w_{8j+7 \rightarrow 8(j+1)+2}; \\
b_{6s+(j+1)_s, 7s+(-2)_s} &= -w_{8(j+m+1)+2 \rightarrow 8(j+m+1)+4} \otimes w_{8j+7 \rightarrow 8(j+1)+3}.
\end{aligned}$$

(10) If  $r_0 = 9$ , then  $\Omega^9(Z_t^{(20)})$  is described with  $(16s \times 8s)$  matrix with the following nonzero entries:

$$\begin{aligned}
b_{j+4s, (-1)_s} &= e_{8(j+m+1)} \otimes w_{8j \rightarrow 8j+1}; \\
b_{3s+(j+1)_s, s+(-2)_s} &= -e_{8(j+m+1)+1} \otimes w_{8j+1 \rightarrow 8(j+1)}; \\
b_{3s+(j+1)_s, s+(-1)_s} &= -e_{8(j+m+1)+1} \otimes w_{8j+1 \rightarrow 8(j+1)}; \\
b_{3s+(j+1)_s, 4s+(-2)_s} &= w_{8(j+m+1)+1 \rightarrow 8(j+m+1)+4} \otimes w_{8j+4 \rightarrow 8(j+1)}; \\
b_{5s+(j+1)_s, 7s+(-2)_s} &= e_{8(j+m+1)+7} \otimes w_{8j+7 \rightarrow 8(j+1)+2}.
\end{aligned}$$

(11) If  $r_0 = 10$ , then  $\Omega^{10}(Z_t^{(20)})$  is described with  $(19s \times 8s)$  matrix with the following nonzero entries:

$$\begin{aligned}
b_{(j+1)_s, (-1)_s} &= -w_{8(j+m)+7 \rightarrow 8(j+m+1)} \otimes w_{8j \rightarrow 8(j+1)}; \\
b_{s+(j+1)_s, (-1)_s} &= -e_{8(j+m+1)} \otimes w_{8j \rightarrow 8(j+1)}; \\
b_{j+3s, (-1)_s} &= -w_{8(j+m)+6 \rightarrow 8(j+m+1)} \otimes w_{8j \rightarrow 8j+1}; \\
b_{2s+(j+1)_s, s+(-2)_s} &= -w_{8(j+m+1) \rightarrow 8(j+m+1)+1} \otimes w_{8j+1 \rightarrow 8(j+1)}; \\
b_{(j+1)_s, s+(-1)_s} &= -w_{8(j+m)+7 \rightarrow 8(j+m+1)+1} \otimes w_{8j+1 \rightarrow 8(j+1)}; \\
b_{s+(j+1)_s, s+(-1)_s} &= -w_{8(j+m+1) \rightarrow 8(j+m+1)+1} \otimes w_{8j+1 \rightarrow 8(j+1)}; \\
b_{(j+1)_s, 2s+(-2)_s} &= w_{8(j+m)+7 \rightarrow 8(j+m+1)+2} \otimes w_{8j+2 \rightarrow 8(j+1)}; \\
b_{s+(j+1)_s, 2s+(-2)_s} &= w_{8(j+m+1) \rightarrow 8(j+m+1)+2} \otimes w_{8j+2 \rightarrow 8(j+1)}; \\
b_{2s+(j+1)_s, 2s+(-2)_s} &= -w_{8(j+m+1) \rightarrow 8(j+m+1)+2} \otimes w_{8j+2 \rightarrow 8(j+1)}; \\
b_{(j+1)_s, 3s+(-2)_s} &= w_{8(j+m)+7 \rightarrow 8(j+m+1)+3} \otimes w_{8j+3 \rightarrow 8(j+1)}; \\
b_{2s+(j+1)_s, 3s+(-2)_s} &= -w_{8(j+m+1) \rightarrow 8(j+m+1)+3} \otimes w_{8j+3 \rightarrow 8(j+1)}; \\
b_{j+3s, 3s+(-2)_s} &= w_{8(j+m)+3 \rightarrow 8(j+m+1)+3} \otimes e_{8j+3}; \\
b_{(j+1)_s, 4s+(-2)_s} &= w_{8(j+m)+7 \rightarrow 8(j+m+1)+4} \otimes w_{8j+4 \rightarrow 8(j+1)}; \\
b_{s+(j+1)_s, 4s+(-2)_s} &= w_{8(j+m+1) \rightarrow 8(j+m+1)+4} \otimes w_{8j+4 \rightarrow 8(j+1)}; \\
b_{2s+(j+1)_s, 4s+(-2)_s} &= -w_{8(j+m+1) \rightarrow 8(j+m+1)+4} \otimes w_{8j+4 \rightarrow 8(j+1)}; \\
b_{6s+(j+1)_s, 4s+(-2)_s} &= w_{8(j+m+1)+3 \rightarrow 8(j+m+1)+4} \otimes w_{8j+4 \rightarrow 8(j+1)+3}; \\
b_{3s+(j+1)_s, 7s+(-2)_s} &= -w_{8(j+m+1)+6 \rightarrow 8(j+m+1)+7} \otimes w_{8j+7 \rightarrow 8(j+1)+1}.
\end{aligned}$$

(12) If  $r_0 = 11$ , then  $\Omega^{11}(Z_t^{(20)})$  is described with  $(18s \times 9s)$  matrix with the following nonzero entries:

$$\begin{aligned}
b_{3s+(j+1)_s, (-2)_s} &= e_{8(j+m+1)+1} \otimes w_{8j \rightarrow 8(j+1)}; \\
b_{4s+(j+1)_s, s+(-1)_s} &= -e_{8(j+m+1)+5} \otimes w_{8j \rightarrow 8(j+1)}; \\
b_{j+4s, s+(-1)_s} &= -w_{8(j+m)+7 \rightarrow 8(j+m+1)+5} \otimes w_{8j \rightarrow 8j+1};
\end{aligned}$$

$$\begin{aligned}
b_{(j+1)s, 2s+(-2)_s} &= -e_{8(j+m+1)+2} \otimes w_{8j+1 \rightarrow 8(j+1)}; \\
b_{(j+1)s, 2s+(-1)_s} &= -e_{8(j+m+1)+2} \otimes w_{8j+1 \rightarrow 8(j+1)}; \\
b_{j+3s, 3s+(-2)_s} &= w_{8(j+m+1) \rightarrow 8(j+m+1)+3} \otimes e_{8j+2}; \\
b_{2s+(j+1)s, 4s+(-2)_s} &= -e_{8(j+m+1)+4} \otimes w_{8j+3 \rightarrow 8(j+1)}; \\
b_{(j+1)s, 5s+(-2)_s} &= w_{8(j+m+1)+2 \rightarrow 8(j+m+1)+7} \otimes w_{8j+4 \rightarrow 8(j+1)}; \\
b_{3s+(j+1)s, 5s+(-2)_s} &= -w_{8(j+m+1)+1 \rightarrow 8(j+m+1)+7} \otimes w_{8j+4 \rightarrow 8(j+1)}; \\
b_{5s+(j+1)s, 5s+(-2)_s} &= e_{8(j+m+1)+7} \otimes w_{8j+4 \rightarrow 8(j+1)+1}.
\end{aligned}$$

(13) If  $r_0 = 12$ , then  $\Omega^{12}(Z_t^{(20)})$  is described with  $(19s \times 8s)$  matrix with the following nonzero entries:

$$\begin{aligned}
b_{2s+(j+1)s, (-2)_s} &= -e_{8(j+m)+7} \otimes w_{8j \rightarrow 8(j+1)}; \\
b_{j+5s, (-2)_s} &= w_{8(j+m)+5 \rightarrow 8(j+m)+7} \otimes w_{8j \rightarrow 8j+2}; \\
b_{j+3s, (-1)_s} &= w_{8(j+m)+2 \rightarrow 8(j+m)+7} \otimes w_{8j \rightarrow 8j+1}; \\
b_{j+5s, (-1)_s} &= -w_{8(j+m)+5 \rightarrow 8(j+m)+7} \otimes w_{8j \rightarrow 8j+2}; \\
b_{(j+1)s, s+(-2)_s} &= w_{8(j+m)+7 \rightarrow 8(j+m+1)+2} \otimes w_{8j+1 \rightarrow 8(j+1)}; \\
b_{s+(j+1)s, s+(-2)_s} &= -w_{8(j+m+1) \rightarrow 8(j+m+1)+2} \otimes w_{8j+1 \rightarrow 8(j+1)}; \\
b_{2s+(j+1)s, s+(-2)_s} &= -2w_{8(j+m)+7 \rightarrow 8(j+m+1)+2} \otimes w_{8j+1 \rightarrow 8(j+1)}; \\
b_{s+(j+1)s, s+(-1)_s} &= -w_{8(j+m+1) \rightarrow 8(j+m+1)+2} \otimes w_{8j+1 \rightarrow 8(j+1)}; \\
b_{2s+(j+1)s, s+(-1)_s} &= -w_{8(j+m)+7 \rightarrow 8(j+m+1)+2} \otimes w_{8j+1 \rightarrow 8(j+1)}; \\
b_{(j+1)s, 2s+(-2)_s} &= w_{8(j+m)+7 \rightarrow 8(j+m+1)+3} \otimes w_{8j+2 \rightarrow 8(j+1)}; \\
b_{2s+(j+1)s, 2s+(-2)_s} &= -w_{8(j+m)+7 \rightarrow 8(j+m+1)+3} \otimes w_{8j+2 \rightarrow 8(j+1)}; \\
b_{s+(j+1)s, 2s+(-3)_s} &= -w_{8(j+m+1) \rightarrow 8(j+m+1)+3} \otimes w_{8j+2 \rightarrow 8(j+1)}; \\
b_{2s+(j+1)s, 2s+(-3)_s} &= -w_{8(j+m)+7 \rightarrow 8(j+m+1)+3} \otimes w_{8j+2 \rightarrow 8(j+1)}; \\
b_{(j+1)s, 3s+(-2)_s} &= w_{8(j+m)+7 \rightarrow 8(j+m+1)+4} \otimes w_{8j+3 \rightarrow 8(j+1)}; \\
b_{j+3s, 3s+(-2)_s} &= -w_{8(j+m)+4 \rightarrow 8(j+m+1)+4} \otimes e_{8j+3}; \\
b_{6s+(j+1)s, 3s+(-2)_s} &= e_{8(j+m+1)+4} \otimes w_{8j+3 \rightarrow 8(j+1)+3}; \\
b_{s+(j+1)s, 3s+(-3)_s} &= -w_{8(j+m+1) \rightarrow 8(j+m+1)+4} \otimes w_{8j+3 \rightarrow 8(j+1)}; \\
b_{j+3s, 3s+(-3)_s} &= -w_{8(j+m)+4 \rightarrow 8(j+m+1)+4} \otimes e_{8j+3}; \\
b_{3s+(j+1)s, 7s+(-3)_s} &= w_{8(j+m+1)+2 \rightarrow 8(j+m+2)} \otimes w_{8j+7 \rightarrow 8(j+1)+1}.
\end{aligned}$$

(14) If  $r_0 = 13$ , then  $\Omega^{13}(Z_t^{(20)})$  is described with  $(18s \times 10s)$  matrix with the following nonzero entries:

$$\begin{aligned}
b_{(j+1)s, (-2)_s} &= -e_{8(j+m+1)+2} \otimes w_{8j \rightarrow 8(j+1)}; \\
b_{j+4s, (-1)_s} &= w_{8(j+m+1) \rightarrow 8(j+m+1)+2} \otimes w_{8j \rightarrow 8j+1}; \\
b_{2s+(j+1)s, s+(-2)_s} &= -e_{8(j+m+1)+6} \otimes w_{8j \rightarrow 8(j+1)}; \\
b_{(j+1)s, 2s+(-3)_s} &= -w_{8(j+m+1)+2 \rightarrow 8(j+m+1)+3} \otimes w_{8j+1 \rightarrow 8(j+1)}; \\
b_{s+(j+1)s, 2s+(-3)_s} &= e_{8(j+m+1)+3} \otimes w_{8j+1 \rightarrow 8(j+1)}; \\
b_{(j+1)s, 2s+(-2)_s} &= w_{8(j+m+1)+2 \rightarrow 8(j+m+1)+3} \otimes w_{8j+1 \rightarrow 8(j+1)}; \\
b_{s+(j+1)s, 2s+(-2)_s} &= -e_{8(j+m+1)+3} \otimes w_{8j+1 \rightarrow 8(j+1)}; \\
b_{(j+1)s, 2s+(-1)_s} &= w_{8(j+m+1)+2 \rightarrow 8(j+m+1)+3} \otimes w_{8j+1 \rightarrow 8(j+1)}; \\
b_{s+(j+1)s, 2s+(-1)_s} &= -e_{8(j+m+1)+3} \otimes w_{8j+1 \rightarrow 8(j+1)}; \\
b_{j+2s, 3s+(-3)_s} &= -w_{8(j+m)+7 \rightarrow 8(j+m+1)+4} \otimes e_{8j+2};
\end{aligned}$$

$$\begin{aligned}
b_{j+2s,3s+(-2)_s} &= -w_{8(j+m)+7 \rightarrow 8(j+m+1)+4} \otimes e_{8j+2}; \\
b_{3s+(j+1)_s,4s+(-3)_s} &= -w_{8(j+m+1)+5 \rightarrow 8(j+m+1)+7} \otimes w_{8j+3 \rightarrow 8(j+1)}; \\
b_{s+(j+1)_s,4s+(-2)_s} &= w_{8(j+m+1)+3 \rightarrow 8(j+m+1)+7} \otimes w_{8j+3 \rightarrow 8(j+1)}; \\
b_{5s+(j+1)_s,4s+(-2)_s} &= -e_{8(j+m+1)+7} \otimes w_{8j+3 \rightarrow 8(j+1)+2}; \\
b_{4s+(j+1)_s,5s+(-3)_s} &= -e_{8(j+m+2)} \otimes w_{8j+4 \rightarrow 8(j+1)+1}; \\
b_{4s+(j+1)_s,5s+(-2)_s} &= e_{8(j+m+2)} \otimes w_{8j+4 \rightarrow 8(j+1)+1}; \\
b_{4s+(j+1)_s,8s+(-3)_s} &= w_{8(j+m+2) \rightarrow 8(j+m+2)+1} \otimes w_{8j+7 \rightarrow 8(j+1)+1}; \\
b_{4s+(j+1)_s,8s+(-2)_s} &= -w_{8(j+m+2) \rightarrow 8(j+m+2)+1} \otimes w_{8j+7 \rightarrow 8(j+1)+1}.
\end{aligned}$$

(15) If  $r_0 = 14$ , then  $\Omega^{14}(Z_t^{(20)})$  is described with  $(20s \times 11s)$  matrix with the following nonzero entries:

$$\begin{aligned}
b_{j+3s,(-3)_s} &= -w_{8(j+m)+3 \rightarrow 8(j+m)+7} \otimes w_{8j \rightarrow 8j+1}; \\
b_{j+4s,(-3)_s} &= w_{8(j+m)+5 \rightarrow 8(j+m)+7} \otimes w_{8j \rightarrow 8j+1}; \\
b_{(j+1)_s,(-2)_s} &= e_{8(j+m)+7} \otimes w_{8j \rightarrow 8(j+1)}; \\
b_{j+3s,(-2)_s} &= -w_{8(j+m)+3 \rightarrow 8(j+m)+7} \otimes w_{8j \rightarrow 8j+1}; \\
b_{j+4s,(-2)_s} &= w_{8(j+m)+5 \rightarrow 8(j+m)+7} \otimes w_{8j \rightarrow 8j+1}; \\
b_{j+3s,(-1)_s} &= w_{8(j+m)+3 \rightarrow 8(j+m)+7} \otimes w_{8j \rightarrow 8j+1}; \\
b_{2s+(j+1)_s,s+(-2)_s} &= -e_{8(j+m+1)} \otimes w_{8j \rightarrow 8(j+1)}; \\
b_{(j+1)_s,2s+(-3)_s} &= -w_{8(j+m)+7 \rightarrow 8(j+m+1)+3} \otimes w_{8j+1 \rightarrow 8(j+1)}; \\
b_{(j+1)_s,2s+(-2)_s} &= w_{8(j+m)+7 \rightarrow 8(j+m+1)+3} \otimes w_{8j+1 \rightarrow 8(j+1)}; \\
b_{s+(j+1)_s,2s+(-2)_s} &= w_{8(j+m+1) \rightarrow 8(j+m+1)+3} \otimes w_{8j+1 \rightarrow 8(j+1)}; \\
b_{(j+1)_s,2s+(-1)_s} &= w_{8(j+m)+7 \rightarrow 8(j+m+1)+3} \otimes w_{8j+1 \rightarrow 8(j+1)}; \\
b_{(j+1)_s,3s+(-3)_s} &= -w_{8(j+m)+7 \rightarrow 8(j+m+1)+4} \otimes w_{8j+2 \rightarrow 8(j+1)}; \\
b_{s+(j+1)_s,3s+(-2)_s} &= w_{8(j+m+1) \rightarrow 8(j+m+1)+4} \otimes w_{8j+2 \rightarrow 8(j+1)}; \\
b_{(j+1)_s,3s+(-4)_s} &= -w_{8(j+m)+7 \rightarrow 8(j+m+1)+4} \otimes w_{8j+2 \rightarrow 8(j+1)}; \\
b_{(j+1)_s,4s+(-3)_s} &= -w_{8(j+m)+7 \rightarrow 8(j+m+1)+5} \otimes w_{8j+3 \rightarrow 8(j+1)}; \\
b_{s+(j+1)_s,4s+(-3)_s} &= -w_{8(j+m+1) \rightarrow 8(j+m+1)+5} \otimes w_{8j+3 \rightarrow 8(j+1)}; \\
b_{2s+(j+1)_s,4s+(-3)_s} &= w_{8(j+m+1) \rightarrow 8(j+m+1)+5} \otimes w_{8j+3 \rightarrow 8(j+1)}; \\
b_{4s+(j+1)_s,4s+(-2)_s} &= e_{8(j+m+1)+5} \otimes w_{8j+3 \rightarrow 8(j+1)+1}; \\
b_{4s+(j+1)_s,5s+(-3)_s} &= -w_{8(j+m+1)+5 \rightarrow 8(j+m+1)+6} \otimes w_{8j+4 \rightarrow 8(j+1)+1}; \\
b_{6s+(j+1)_s,5s+(-3)_s} &= -e_{8(j+m+1)+6} \otimes w_{8j+4 \rightarrow 8(j+1)+2}; \\
b_{4s+(j+1)_s,5s+(-2)_s} &= w_{8(j+m+1)+5 \rightarrow 8(j+m+1)+6} \otimes w_{8j+4 \rightarrow 8(j+1)+1}; \\
b_{6s+(j+1)_s,5s+(-2)_s} &= e_{8(j+m+1)+6} \otimes w_{8j+4 \rightarrow 8(j+1)+2}; \\
b_{4s+(j+1)_s,10s+(-3)_s} &= w_{8(j+m+1)+5 \rightarrow 8(j+m+1)+7} \otimes w_{8j+7 \rightarrow 8(j+1)+1}; \\
b_{3s+(j+1)_s,10s+(-4)_s} &= -w_{8(j+m+1)+3 \rightarrow 8(j+m+1)+7} \otimes w_{8j+7 \rightarrow 8(j+1)+1}; \\
b_{4s+(j+1)_s,10s+(-4)_s} &= w_{8(j+m+1)+5 \rightarrow 8(j+m+1)+7} \otimes w_{8j+7 \rightarrow 8(j+1)+1}.
\end{aligned}$$

(16) If  $r_0 = 15$ , then  $\Omega^{15}(Z_t^{(20)})$  is described with  $(18s \times 11s)$  matrix with the following nonzero entries:

$$\begin{aligned}
b_{4s+(j+1)_s,(-3)_s} &= e_{8(j+m+1)+5} \otimes w_{8j \rightarrow 8(j+1)}; \\
b_{j+5s,(-3)_s} &= -w_{8(j+m)+7 \rightarrow 8(j+m+1)+5} \otimes w_{8j \rightarrow 8j+1}; \\
b_{j+7s,(-3)_s} &= -w_{8(j+m+1) \rightarrow 8(j+m+1)+5} \otimes w_{8j \rightarrow 8j+2};
\end{aligned}$$

$$\begin{aligned}
b_{j+5s,(-2)_s} &= -w_{8(j+m)+7 \rightarrow 8(j+m+1)+5} \otimes w_{8j \rightarrow 8j+1}; \\
b_{j+7s,(-2)_s} &= -w_{8(j+m+1) \rightarrow 8(j+m+1)+5} \otimes w_{8j \rightarrow 8j+2}; \\
b_{j+4s,s+(-3)_s} &= -w_{8(j+m)+7 \rightarrow 8(j+m+1)+3} \otimes w_{8j \rightarrow 8j+1}; \\
b_{(j+1)_s,s+(-2)_s} &= -e_{8(j+m+1)+3} \otimes w_{8j \rightarrow 8(j+1)}; \\
b_{j+4s,s+(-2)_s} &= -w_{8(j+m)+7 \rightarrow 8(j+m+1)+3} \otimes w_{8j \rightarrow 8j+1}; \\
b_{j+4s,s+(-1)_s} &= w_{8(j+m)+7 \rightarrow 8(j+m+1)+3} \otimes w_{8j \rightarrow 8j+1}; \\
b_{3s+(j+1)_s,2s+(-2)_s} &= -e_{8(j+m+1)+1} \otimes w_{8j \rightarrow 8(j+1)}; \\
b_{(j+1)_s,3s+(-4)_s} &= w_{8(j+m+1)+3 \rightarrow 8(j+m+1)+4} \otimes w_{8j+1 \rightarrow 8(j+1)}; \\
b_{2s+(j+1)_s,3s+(-4)_s} &= -e_{8(j+m+1)+4} \otimes w_{8j+1 \rightarrow 8(j+1)}; \\
b_{(j+1)_s,3s+(-2)_s} &= w_{8(j+m+1)+3 \rightarrow 8(j+m+1)+4} \otimes w_{8j+1 \rightarrow 8(j+1)}; \\
b_{2s+(j+1)_s,3s+(-2)_s} &= -e_{8(j+m+1)+4} \otimes w_{8j+1 \rightarrow 8(j+1)}; \\
b_{(j+1)_s,3s+(-1)_s} &= w_{8(j+m+1)+3 \rightarrow 8(j+m+1)+4} \otimes w_{8j+1 \rightarrow 8(j+1)}; \\
b_{2s+(j+1)_s,3s+(-1)_s} &= -e_{8(j+m+1)+4} \otimes w_{8j+1 \rightarrow 8(j+1)}; \\
b_{(j+1)_s,4s+(-4)_s} &= -w_{8(j+m+1)+3 \rightarrow 8(j+m+1)+7} \otimes w_{8j+2 \rightarrow 8(j+1)}; \\
b_{4s+(j+1)_s,4s+(-4)_s} &= w_{8(j+m+1)+5 \rightarrow 8(j+m+1)+7} \otimes w_{8j+2 \rightarrow 8(j+1)}; \\
b_{(j+1)_s,4s+(-3)_s} &= -w_{8(j+m+1)+3 \rightarrow 8(j+m+1)+7} \otimes w_{8j+2 \rightarrow 8(j+1)}; \\
b_{s+(j+1)_s,4s+(-3)_s} &= w_{8(j+m+1)+6 \rightarrow 8(j+m+1)+7} \otimes w_{8j+2 \rightarrow 8(j+1)}; \\
b_{4s+(j+1)_s,4s+(-3)_s} &= 2w_{8(j+m+1)+5 \rightarrow 8(j+m+1)+7} \otimes w_{8j+2 \rightarrow 8(j+1)}; \\
b_{(j+1)_s,4s+(-2)_s} &= w_{8(j+m+1)+3 \rightarrow 8(j+m+1)+7} \otimes w_{8j+2 \rightarrow 8(j+1)}; \\
b_{s+(j+1)_s,4s+(-2)_s} &= -w_{8(j+m+1)+6 \rightarrow 8(j+m+1)+7} \otimes w_{8j+2 \rightarrow 8(j+1)}; \\
b_{3s+(j+1)_s,4s+(-2)_s} &= -w_{8(j+m+1)+1 \rightarrow 8(j+m+1)+7} \otimes w_{8j+2 \rightarrow 8(j+1)}; \\
b_{s+(j+1)_s,5s+(-3)_s} &= -w_{8(j+m+1)+6 \rightarrow 8(j+m+2)} \otimes w_{8j+3 \rightarrow 8(j+1)}; \\
b_{4s+(j+1)_s,5s+(-3)_s} &= -w_{8(j+m+1)+5 \rightarrow 8(j+m+2)} \otimes w_{8j+3 \rightarrow 8(j+1)}; \\
b_{7s+(j+1)_s,5s+(-2)_s} &= -e_{8(j+m+2)} \otimes w_{8j+3 \rightarrow 8(j+1)+2}; \\
b_{5s+(j+1)_s,6s+(-3)_s} &= e_{8(j+m+1)+7} \otimes w_{8j+4 \rightarrow 8(j+1)+1}; \\
b_{5s+(j+1)_s,6s+(-2)_s} &= -e_{8(j+m+1)+7} \otimes w_{8j+4 \rightarrow 8(j+1)+1}; \\
b_{5s+(j+1)_s,9s+(-3)_s} &= w_{8(j+m+1)+7 \rightarrow 8(j+m+2)+2} \otimes w_{8j+7 \rightarrow 8(j+1)+1}; \\
b_{5s+(j+1)_s,9s+(-2)_s} &= -w_{8(j+m+1)+7 \rightarrow 8(j+m+2)+2} \otimes w_{8j+7 \rightarrow 8(j+1)+1}.
\end{aligned}$$

(17) If  $r_0 = 16$ , then  $\Omega^{16}(Z_t^{(20)})$  is described with  $(19s \times 13s)$  matrix with the following nonzero entries:

$$\begin{aligned}
b_{2s+(j+1)_s,(-4)_s} &= e_{8(j+m)+7} \otimes w_{8j \rightarrow 8(j+1)}; \\
b_{(j+1)_s,(-3)_s} &= e_{8(j+m)+7} \otimes w_{8j \rightarrow 8(j+1)}; \\
b_{j+6s,(-3)_s} &= -w_{8(j+m)+1 \rightarrow 8(j+m)+7} \otimes w_{8j \rightarrow 8j+2}; \\
b_{(j+1)_s,(-2)_s} &= -e_{8(j+m)+7} \otimes w_{8j \rightarrow 8(j+1)}; \\
b_{2s+(j+1)_s,(-2)_s} &= e_{8(j+m)+7} \otimes w_{8j \rightarrow 8(j+1)}; \\
b_{j+6s,(-2)_s} &= -w_{8(j+m)+1 \rightarrow 8(j+m)+7} \otimes w_{8j \rightarrow 8j+2}; \\
b_{(j+1)_s,(-1)_s} &= -e_{8(j+m)+7} \otimes w_{8j \rightarrow 8(j+1)}; \\
b_{2s+(j+1)_s,(-1)_s} &= e_{8(j+m)+7} \otimes w_{8j \rightarrow 8(j+1)}; \\
b_{j+4s,(-1)_s} &= -w_{8(j+m)+6 \rightarrow 8(j+m)+7} \otimes w_{8j \rightarrow 8j+1}; \\
b_{j+6s,(-1)_s} &= w_{8(j+m)+1 \rightarrow 8(j+m)+7} \otimes w_{8j \rightarrow 8j+2};
\end{aligned}$$

$$\begin{aligned}
b_{2s+(j+1)s,s+(-4)s} &= -w_{8(j+m)+7 \rightarrow 8(j+m+1)} \otimes w_{8j \rightarrow 8(j+1)}; \\
b_{s+(j+1)s,s+(-3)s} &= -e_{8(j+m+1)} \otimes w_{8j \rightarrow 8(j+1)}; \\
b_{2s+(j+1)s,s+(-3)s} &= -w_{8(j+m)+7 \rightarrow 8(j+m+1)} \otimes w_{8j \rightarrow 8(j+1)}; \\
b_{(j+1)s,s+(-2)s} &= w_{8(j+m)+7 \rightarrow 8(j+m+1)} \otimes w_{8j \rightarrow 8(j+1)}; \\
b_{2s+(j+1)s,s+(-2)s} &= -w_{8(j+m)+7 \rightarrow 8(j+m+1)} \otimes w_{8j \rightarrow 8(j+1)}; \\
b_{s+(j+1)s,s+(-1)s} &= e_{8(j+m+1)} \otimes w_{8j \rightarrow 8(j+1)}; \\
b_{(j+1)s,2s+(-4)s} &= -w_{8(j+m)+7 \rightarrow 8(j+m+1)+4} \otimes w_{8j+1 \rightarrow 8(j+1)}; \\
b_{s+(j+1)s,2s+(-4)s} &= w_{8(j+m+1) \rightarrow 8(j+m+1)+4} \otimes w_{8j+1 \rightarrow 8(j+1)}; \\
b_{(j+1)s,2s+(-3)s} &= -w_{8(j+m)+7 \rightarrow 8(j+m+1)+4} \otimes w_{8j+1 \rightarrow 8(j+1)}; \\
b_{(j+1)s,2s+(-2)s} &= w_{8(j+m)+7 \rightarrow 8(j+m+1)+4} \otimes w_{8j+1 \rightarrow 8(j+1)}; \\
b_{s+(j+1)s,2s+(-2)s} &= w_{8(j+m+1) \rightarrow 8(j+m+1)+4} \otimes w_{8j+1 \rightarrow 8(j+1)}; \\
b_{s+(j+1)s,2s+(-1)s} &= w_{8(j+m+1) \rightarrow 8(j+m+1)+4} \otimes w_{8j+1 \rightarrow 8(j+1)}; \\
b_{s+(j+1)s,3s+(-4)s} &= -w_{8(j+m+1) \rightarrow 8(j+m+1)+5} \otimes w_{8j+2 \rightarrow 8(j+1)}; \\
b_{2s+(j+1)s,3s+(-4)s} &= -w_{8(j+m)+7 \rightarrow 8(j+m+1)+5} \otimes w_{8j+2 \rightarrow 8(j+1)}; \\
b_{s+(j+1)s,3s+(-3)s} &= -w_{8(j+m+1) \rightarrow 8(j+m+1)+5} \otimes w_{8j+2 \rightarrow 8(j+1)}; \\
b_{2s+(j+1)s,3s+(-3)s} &= -w_{8(j+m)+7 \rightarrow 8(j+m+1)+5} \otimes w_{8j+2 \rightarrow 8(j+1)}; \\
b_{(j+1)s,3s+(-2)s} &= w_{8(j+m)+7 \rightarrow 8(j+m+1)+5} \otimes w_{8j+2 \rightarrow 8(j+1)}; \\
b_{s+(j+1)s,3s+(-2)s} &= -w_{8(j+m+1) \rightarrow 8(j+m+1)+5} \otimes w_{8j+2 \rightarrow 8(j+1)}; \\
b_{2s+(j+1)s,3s+(-2)s} &= -w_{8(j+m)+7 \rightarrow 8(j+m+1)+5} \otimes w_{8j+2 \rightarrow 8(j+1)}; \\
b_{4s+(j+1)s,4s+(-4)s} &= -e_{8(j+m+1)+6} \otimes w_{8j+3 \rightarrow 8(j+1)+1}; \\
b_{(j+1)s,4s+(-3)s} &= w_{8(j+m)+7 \rightarrow 8(j+m+1)+6} \otimes w_{8j+3 \rightarrow 8(j+1)}; \\
b_{4s+(j+1)s,4s+(-3)s} &= -e_{8(j+m+1)+6} \otimes w_{8j+3 \rightarrow 8(j+1)+1}; \\
b_{4s+(j+1)s,4s+(-2)s} &= -e_{8(j+m+1)+6} \otimes w_{8j+3 \rightarrow 8(j+1)+1}; \\
b_{6s+(j+1)s,5s+(-2)s} &= -e_{8(j+m+1)+1} \otimes w_{8j+3 \rightarrow 8(j+1)+2}; \\
b_{3s+(j+1)s,11s+(-4)s} &= -w_{8(j+m+1)+4 \rightarrow 8(j+m+1)+7} \otimes w_{8j+7 \rightarrow 8(j+1)+1}.
\end{aligned}$$

(18) If  $r_0 = 17$ , then  $\Omega^{17}(Z_t^{(20)})$  is described with  $(18s \times 14s)$  matrix with the following nonzero entries:

$$\begin{aligned}
b_{(j+1)s,(-3)s} &= e_{8(j+m+1)+2} \otimes w_{8j \rightarrow 8(j+1)}; \\
b_{(j+1)s,(-1)s} &= -e_{8(j+m+1)+2} \otimes w_{8j \rightarrow 8(j+1)}; \\
b_{(j+1)s,s+(-4)s} &= w_{8(j+m+1)+2 \rightarrow 8(j+m+1)+4} \otimes w_{8j \rightarrow 8(j+1)}; \\
b_{(j+1)s,s+(-3)s} &= w_{8(j+m+1)+2 \rightarrow 8(j+m+1)+4} \otimes w_{8j \rightarrow 8(j+1)}; \\
b_{(j+1)s,s+(-2)s} &= w_{8(j+m+1)+2 \rightarrow 8(j+m+1)+4} \otimes w_{8j \rightarrow 8(j+1)}; \\
b_{s+(j+1)s,s+(-2)s} &= -e_{8(j+m+1)+4} \otimes w_{8j \rightarrow 8(j+1)}; \\
b_{3s+(j+1)s,2s+(-4)s} &= -w_{8(j+m+1)+5 \rightarrow 8(j+m+1)+6} \otimes w_{8j \rightarrow 8(j+1)}; \\
b_{2s+(j+1)s,2s+(-3)s} &= -e_{8(j+m+1)+6} \otimes w_{8j \rightarrow 8(j+1)}; \\
b_{3s+(j+1)s,2s+(-3)s} &= -w_{8(j+m+1)+5 \rightarrow 8(j+m+1)+6} \otimes w_{8j \rightarrow 8(j+1)}; \\
b_{3s+(j+1)s,2s+(-2)s} &= -w_{8(j+m+1)+5 \rightarrow 8(j+m+1)+6} \otimes w_{8j \rightarrow 8(j+1)}; \\
b_{j+2s,2s+(-1)s} &= w_{8(j+m)+7 \rightarrow 8(j+m+1)+6} \otimes w_{8j \rightarrow 8(j+1)}; \\
b_{3s+(j+1)s,3s+(-4)s} &= e_{8(j+m+1)+5} \otimes w_{8j \rightarrow 8(j+1)}; \\
b_{3s+(j+1)s,3s+(-2)s} &= e_{8(j+m+1)+5} \otimes w_{8j \rightarrow 8(j+1)};
\end{aligned}$$

$$\begin{aligned}
b_{3s+(j+1)s,3s+(-1)s} &= e_{8(j+m+1)+5} \otimes w_{8j \rightarrow 8(j+1)}; \\
b_{(j+1)s,4s+(-4)s} &= -w_{8(j+m+1)+2 \rightarrow 8(j+m+1)+7} \otimes w_{8j+1 \rightarrow 8(j+1)}; \\
b_{3s+(j+1)s,4s+(-4)s} &= w_{8(j+m+1)+5 \rightarrow 8(j+m+1)+7} \otimes w_{8j+1 \rightarrow 8(j+1)}; \\
b_{(j+1)s,4s+(-3)s} &= -w_{8(j+m+1)+2 \rightarrow 8(j+m+1)+7} \otimes w_{8j+1 \rightarrow 8(j+1)}; \\
b_{2s+(j+1)s,4s+(-2)s} &= w_{8(j+m+1)+6 \rightarrow 8(j+m+1)+7} \otimes w_{8j+1 \rightarrow 8(j+1)}; \\
b_{3s+(j+1)s,4s+(-2)s} &= 2w_{8(j+m+1)+5 \rightarrow 8(j+m+1)+7} \otimes w_{8j+1 \rightarrow 8(j+1)}; \\
b_{3s+(j+1)s,4s+(-1)s} &= w_{8(j+m+1)+5 \rightarrow 8(j+m+1)+7} \otimes w_{8j+1 \rightarrow 8(j+1)}; \\
b_{(j+1)s,5s+(-4)s} &= w_{8(j+m+1)+2 \rightarrow 8(j+m+2)} \otimes w_{8j+2 \rightarrow 8(j+1)}; \\
b_{(j+1)s,5s+(-3)s} &= w_{8(j+m+1)+2 \rightarrow 8(j+m+2)} \otimes w_{8j+2 \rightarrow 8(j+1)}; \\
b_{2s+(j+1)s,5s+(-2)s} &= -w_{8(j+m+1)+6 \rightarrow 8(j+m+2)} \otimes w_{8j+2 \rightarrow 8(j+1)}; \\
b_{3s+(j+1)s,5s+(-2)s} &= -w_{8(j+m+1)+5 \rightarrow 8(j+m+2)} \otimes w_{8j+2 \rightarrow 8(j+1)}; \\
b_{4s+(j+1)s,6s+(-4)s} &= e_{8(j+m+1)+7} \otimes w_{8j+3 \rightarrow 8(j+1)+1}; \\
b_{s+(j+1)s,6s+(-3)s} &= w_{8(j+m+1)+4 \rightarrow 8(j+m+1)+7} \otimes w_{8j+3 \rightarrow 8(j+1)}; \\
b_{4s+(j+1)s,6s+(-3)s} &= e_{8(j+m+1)+7} \otimes w_{8j+3 \rightarrow 8(j+1)+1}; \\
b_{4s+(j+1)s,7s+(-4)s} &= -w_{8(j+m+1)+7 \rightarrow 8(j+m+2)} \otimes w_{8j+4 \rightarrow 8(j+1)+1}; \\
b_{5s+(j+1)s,7s+(-4)s} &= -e_{8(j+m+2)} \otimes w_{8j+4 \rightarrow 8(j+1)+1}; \\
b_{4s+(j+1)s,12s+(-4)s} &= -w_{8(j+m+1)+7 \rightarrow 8(j+m+2)+3} \otimes w_{8j+7 \rightarrow 8(j+1)+1}.
\end{aligned}$$

(19) If  $r_0 = 18$ , then  $\Omega^{18}(Z_t^{(20)})$  is described with  $(19s \times 16s)$  matrix with the following nonzero entries:

$$\begin{aligned}
b_{(j+1)s,(-3)s} &= e_{8(j+m)+7} \otimes w_{8j \rightarrow 8(j+1)}; \\
b_{j+3s,(-1)s} &= -w_{8(j+m)+5 \rightarrow 8(j+m)+7} \otimes w_{8j \rightarrow 8j+1}; \\
b_{j+4s,(-1)s} &= w_{8(j+m)+1 \rightarrow 8(j+m)+7} \otimes w_{8j \rightarrow 8j+1}; \\
b_{j+5s,(-1)s} &= w_{8(j+m)+2 \rightarrow 8(j+m)+7} \otimes w_{8j \rightarrow 8j+2}; \\
b_{(j+1)s,s+(-2)s} &= e_{8(j+m)+7} \otimes w_{8j \rightarrow 8(j+1)}; \\
b_{(j+1)s,2s+(-4)s} &= -w_{8(j+m)+7 \rightarrow 8(j+m+1)} \otimes w_{8j \rightarrow 8(j+1)}; \\
b_{s+(j+1)s,2s+(-4)s} &= -e_{8(j+m+1)} \otimes w_{8j \rightarrow 8(j+1)}; \\
b_{2s+(j+1)s,2s+(-4)s} &= e_{8(j+m+1)} \otimes w_{8j \rightarrow 8(j+1)}; \\
b_{(j+1)s,2s+(-3)s} &= -w_{8(j+m)+7 \rightarrow 8(j+m+1)} \otimes w_{8j \rightarrow 8(j+1)}; \\
b_{2s+(j+1)s,2s+(-2)s} &= e_{8(j+m+1)} \otimes w_{8j \rightarrow 8(j+1)}; \\
b_{(j+1)s,3s+(-4)s} &= w_{8(j+m)+7 \rightarrow 8(j+m+1)+5} \otimes w_{8j+1 \rightarrow 8(j+1)}; \\
b_{s+(j+1)s,3s+(-4)s} &= w_{8(j+m+1) \rightarrow 8(j+m+1)+5} \otimes w_{8j+1 \rightarrow 8(j+1)}; \\
b_{2s+(j+1)s,3s+(-4)s} &= -w_{8(j+m+1) \rightarrow 8(j+m+1)+5} \otimes w_{8j+1 \rightarrow 8(j+1)}; \\
b_{(j+1)s,3s+(-2)s} &= w_{8(j+m)+7 \rightarrow 8(j+m+1)+5} \otimes w_{8j+1 \rightarrow 8(j+1)}; \\
b_{s+(j+1)s,3s+(-2)s} &= w_{8(j+m+1) \rightarrow 8(j+m+1)+5} \otimes w_{8j+1 \rightarrow 8(j+1)}; \\
b_{2s+(j+1)s,3s+(-2)s} &= -w_{8(j+m+1) \rightarrow 8(j+m+1)+5} \otimes w_{8j+1 \rightarrow 8(j+1)}; \\
b_{(j+1)s,3s+(-1)s} &= w_{8(j+m)+7 \rightarrow 8(j+m+1)+5} \otimes w_{8j+1 \rightarrow 8(j+1)}; \\
b_{s+(j+1)s,3s+(-1)s} &= w_{8(j+m+1) \rightarrow 8(j+m+1)+5} \otimes w_{8j+1 \rightarrow 8(j+1)}; \\
b_{2s+(j+1)s,3s+(-1)s} &= -w_{8(j+m+1) \rightarrow 8(j+m+1)+5} \otimes w_{8j+1 \rightarrow 8(j+1)}; \\
b_{(j+1)s,4s+(-2)s} &= -w_{8(j+m)+7 \rightarrow 8(j+m+1)+6} \otimes w_{8j+2 \rightarrow 8(j+1)}; \\
b_{(j+1)s,5s+(-4)s} &= w_{8(j+m)+7 \rightarrow 8(j+m+1)+1} \otimes w_{8j+2 \rightarrow 8(j+1)};
\end{aligned}$$



$$\begin{aligned}
b_{s+(j+1)_s, 5s+(-4)_s} &= w_{8(j+m+1) \rightarrow 8(j+m+1)+1} \otimes w_{8j+2 \rightarrow 8(j+1)}; \\
b_{(j+1)_s, 5s+(-3)_s} &= w_{8(j+m)+7 \rightarrow 8(j+m+1)+1} \otimes w_{8j+2 \rightarrow 8(j+1)}; \\
b_{2s+(j+1)_s, 6s+(-4)_s} &= -w_{8(j+m+1) \rightarrow 8(j+m+1)+2} \otimes w_{8j+3 \rightarrow 8(j+1)}; \\
b_{5s+(j+1)_s, 6s+(-4)_s} &= -e_{8(j+m+1)+2} \otimes w_{8j+3 \rightarrow 8(j+1)+2}; \\
b_{s+(j+1)_s, 6s+(-3)_s} &= w_{8(j+m+1) \rightarrow 8(j+m+1)+2} \otimes w_{8j+3 \rightarrow 8(j+1)}; \\
b_{2s+(j+1)_s, 6s+(-3)_s} &= -w_{8(j+m+1) \rightarrow 8(j+m+1)+2} \otimes w_{8j+3 \rightarrow 8(j+1)}; \\
b_{5s+(j+1)_s, 6s+(-3)_s} &= -e_{8(j+m+1)+2} \otimes w_{8j+3 \rightarrow 8(j+1)+2}; \\
b_{2s+(j+1)_s, 7s+(-4)_s} &= -w_{8(j+m+1) \rightarrow 8(j+m+1)+3} \otimes w_{8j+4 \rightarrow 8(j+1)}; \\
b_{5s+(j+1)_s, 7s+(-4)_s} &= -w_{8(j+m+1)+2 \rightarrow 8(j+m+1)+3} \otimes w_{8j+4 \rightarrow 8(j+1)+2}; \\
b_{3s+(j+1)_s, 8s+(-4)_s} &= -e_{8(j+m+1)+5} \otimes w_{8j+4 \rightarrow 8(j+1)+1}; \\
b_{3s+(j+1)_s, 14s+(-4)_s} &= w_{8(j+m+1)+5 \rightarrow 8(j+m+1)+7} \otimes w_{8j+7 \rightarrow 8(j+1)+1}; \\
b_{4s+(j+1)_s, 14s+(-4)_s} &= -w_{8(j+m+1)+1 \rightarrow 8(j+m+1)+7} \otimes w_{8j+7 \rightarrow 8(j+1)+1}; \\
b_{5s+(j+1)_s, 14s+(-4)_s} &= -w_{8(j+m+1)+2 \rightarrow 8(j+m+1)+7} \otimes w_{8j+7 \rightarrow 8(j+1)+2}.
\end{aligned}$$

(20) If  $r_0 = 19$ , then  $\Omega^{19}(Z_t^{(20)})$  is described with  $(16s \times 16s)$  matrix with the following nonzero entries:

$$\begin{aligned}
b_{3s+(j+1)_s, (-2)_s} &= e_{8(j+m+1)+5} \otimes w_{8j \rightarrow 8(j+1)}; \\
b_{j+4s, (-1)_s} &= -w_{8(j+m+1) \rightarrow 8(j+m+1)+5} \otimes w_{8j \rightarrow 8j+1}; \\
b_{(j+1)_s, s+(-3)_s} &= e_{8(j+m+1)+3} \otimes w_{8j \rightarrow 8(j+1)}; \\
b_{2s+(j+1)_s, s+(-3)_s} &= -w_{8(j+m+1)+1 \rightarrow 8(j+m+1)+3} \otimes w_{8j \rightarrow 8(j+1)}; \\
b_{s+(j+1)_s, 2s+(-4)_s} &= -e_{8(j+m+1)+6} \otimes w_{8j \rightarrow 8(j+1)}; \\
b_{3s+(j+1)_s, 2s+(-4)_s} &= -w_{8(j+m+1)+5 \rightarrow 8(j+m+1)+6} \otimes w_{8j \rightarrow 8(j+1)}; \\
b_{s+(j+1)_s, 2s+(-2)_s} &= -e_{8(j+m+1)+6} \otimes w_{8j \rightarrow 8(j+1)}; \\
b_{3s+(j+1)_s, 2s+(-2)_s} &= -w_{8(j+m+1)+5 \rightarrow 8(j+m+1)+6} \otimes w_{8j \rightarrow 8(j+1)}; \\
b_{s+(j+1)_s, 2s+(-1)_s} &= -e_{8(j+m+1)+6} \otimes w_{8j \rightarrow 8(j+1)}; \\
b_{3s+(j+1)_s, 2s+(-1)_s} &= -w_{8(j+m+1)+5 \rightarrow 8(j+m+1)+6} \otimes w_{8j \rightarrow 8(j+1)}; \\
b_{2s+(j+1)_s, 3s+(-4)_s} &= e_{8(j+m+1)+1} \otimes w_{8j \rightarrow 8(j+1)}; \\
b_{2s+(j+1)_s, 3s+(-2)_s} &= e_{8(j+m+1)+1} \otimes w_{8j \rightarrow 8(j+1)}; \\
b_{(j+1)_s, 4s+(-4)_s} &= w_{8(j+m+1)+3 \rightarrow 8(j+m+2)} \otimes w_{8j+1 \rightarrow 8(j+1)}; \\
b_{2s+(j+1)_s, 4s+(-4)_s} &= -w_{8(j+m+1)+1 \rightarrow 8(j+m+2)} \otimes w_{8j+1 \rightarrow 8(j+1)}; \\
b_{(j+1)_s, 4s+(-2)_s} &= w_{8(j+m+1)+3 \rightarrow 8(j+m+2)} \otimes w_{8j+1 \rightarrow 8(j+1)}; \\
b_{2s+(j+1)_s, 4s+(-2)_s} &= -w_{8(j+m+1)+1 \rightarrow 8(j+m+2)} \otimes w_{8j+1 \rightarrow 8(j+1)}; \\
b_{(j+1)_s, 4s+(-1)_s} &= w_{8(j+m+1)+3 \rightarrow 8(j+m+2)} \otimes w_{8j+1 \rightarrow 8(j+1)}; \\
b_{2s+(j+1)_s, 4s+(-1)_s} &= -w_{8(j+m+1)+1 \rightarrow 8(j+m+2)} \otimes w_{8j+1 \rightarrow 8(j+1)}; \\
b_{(j+1)_s, 5s+(-4)_s} &= -w_{8(j+m+1)+3 \rightarrow 8(j+m+1)+7} \otimes w_{8j+2 \rightarrow 8(j+1)}; \\
b_{2s+(j+1)_s, 5s+(-4)_s} &= w_{8(j+m+1)+1 \rightarrow 8(j+m+1)+7} \otimes w_{8j+2 \rightarrow 8(j+1)}; \\
b_{(j+1)_s, 5s+(-3)_s} &= -w_{8(j+m+1)+3 \rightarrow 8(j+m+1)+7} \otimes w_{8j+2 \rightarrow 8(j+1)}; \\
b_{2s+(j+1)_s, 5s+(-3)_s} &= w_{8(j+m+1)+1 \rightarrow 8(j+m+1)+7} \otimes w_{8j+2 \rightarrow 8(j+1)}; \\
b_{(j+1)_s, 5s+(-2)_s} &= -w_{8(j+m+1)+3 \rightarrow 8(j+m+1)+7} \otimes w_{8j+2 \rightarrow 8(j+1)}; \\
b_{3s+(j+1)_s, 5s+(-2)_s} &= w_{8(j+m+1)+5 \rightarrow 8(j+m+1)+7} \otimes w_{8j+2 \rightarrow 8(j+1)}; \\
b_{2s+(j+1)_s, 6s+(-3)_s} &= -w_{8(j+m+1)+1 \rightarrow 8(j+m+2)} \otimes w_{8j+3 \rightarrow 8(j+1)};
\end{aligned}$$

$$\begin{aligned}
b_{3s+(j+1)s,6s+(-3)s} &= w_{8(j+m+1)+5 \rightarrow 8(j+m+2)} \otimes w_{8j+3 \rightarrow 8(j+1)}; \\
b_{4s+(j+1)s,6s+(-3)s} &= e_{8(j+m+2)} \otimes w_{8j+3 \rightarrow 8(j+1)+1}; \\
b_{4s+(j+1)s,6s+(-2)s} &= e_{8(j+m+2)} \otimes w_{8j+3 \rightarrow 8(j+1)+1}; \\
b_{2s+(j+1)s,7s+(-4)s} &= -w_{8(j+m+1)+1 \rightarrow 8(j+m+1)+7} \otimes w_{8j+4 \rightarrow 8(j+1)}; \\
b_{4s+(j+1)s,12s+(-4)s} &= w_{8(j+m+2) \rightarrow 8(j+m+2)+2} \otimes w_{8j+7 \rightarrow 8(j+1)+1}.
\end{aligned}$$

(21) If  $r_0 = 20$ , then  $\Omega^{20}(Z_t^{(20)})$  is described with  $(16s \times 19s)$  matrix with the following nonzero entries:

$$\begin{aligned}
b_{(j+1)s,(-4)s} &= e_{8(j+m)+7} \otimes w_{8j \rightarrow 8(j+1)}; \\
b_{(j+1)s,(-2)s} &= e_{8(j+m)+7} \otimes w_{8j \rightarrow 8(j+1)}; \\
b_{j+3s,(-1)s} &= -w_{8(j+m)+6 \rightarrow 8(j+m)+7} \otimes w_{8j \rightarrow 8j+1}; \\
b_{s+(j+1)s,s+(-3)s} &= e_{8(j+m+1)} \otimes w_{8j \rightarrow 8(j+1)}; \\
b_{(j+1)s,2s+(-4)s} &= w_{8(j+m)+7 \rightarrow 8(j+m+1)} \otimes w_{8j \rightarrow 8(j+1)}; \\
b_{(j+1)s,2s+(-2)s} &= w_{8(j+m)+7 \rightarrow 8(j+m+1)} \otimes w_{8j \rightarrow 8(j+1)}; \\
b_{(j+1)s,2s+(-1)s} &= w_{8(j+m)+7 \rightarrow 8(j+m+1)} \otimes w_{8j \rightarrow 8(j+1)}; \\
b_{s+(j+1)s,3s+(-2)s} &= -w_{8(j+m+1) \rightarrow 8(j+m+1)+6} \otimes w_{8j+1 \rightarrow 8(j+1)}; \\
b_{(j+1)s,4s+(-4)s} &= w_{8(j+m)+7 \rightarrow 8(j+m+1)+1} \otimes w_{8j+1 \rightarrow 8(j+1)}; \\
b_{(j+1)s,4s+(-2)s} &= w_{8(j+m)+7 \rightarrow 8(j+m+1)+1} \otimes w_{8j+1 \rightarrow 8(j+1)}; \\
b_{(j+1)s,4s+(-1)s} &= w_{8(j+m)+7 \rightarrow 8(j+m+1)+1} \otimes w_{8j+1 \rightarrow 8(j+1)}; \\
b_{s+(j+1)s,5s+(-4)s} &= -w_{8(j+m+1) \rightarrow 8(j+m+1)+2} \otimes w_{8j+2 \rightarrow 8(j+1)}; \\
b_{s+(j+1)s,5s+(-3)s} &= -w_{8(j+m+1) \rightarrow 8(j+m+1)+2} \otimes w_{8j+2 \rightarrow 8(j+1)}; \\
b_{s+(j+1)s,5s+(-2)s} &= -w_{8(j+m+1) \rightarrow 8(j+m+1)+2} \otimes w_{8j+2 \rightarrow 8(j+1)}; \\
b_{(j+1)s,6s+(-4)s} &= w_{8(j+m)+7 \rightarrow 8(j+m+1)+3} \otimes w_{8j+3 \rightarrow 8(j+1)}; \\
b_{s+(j+1)s,6s+(-4)s} &= -w_{8(j+m+1) \rightarrow 8(j+m+1)+3} \otimes w_{8j+3 \rightarrow 8(j+1)}; \\
b_{4s+(j+1)s,6s+(-4)s} &= -e_{8(j+m+1)+3} \otimes w_{8j+3 \rightarrow 8(j+1)+2}; \\
b_{(j+1)s,6s+(-3)s} &= w_{8(j+m)+7 \rightarrow 8(j+m+1)+3} \otimes w_{8j+3 \rightarrow 8(j+1)}; \\
b_{s+(j+1)s,6s+(-3)s} &= -w_{8(j+m+1) \rightarrow 8(j+m+1)+3} \otimes w_{8j+3 \rightarrow 8(j+1)}; \\
b_{4s+(j+1)s,6s+(-3)s} &= -e_{8(j+m+1)+3} \otimes w_{8j+3 \rightarrow 8(j+1)+2}; \\
b_{(j+1)s,6s+(-2)s} &= w_{8(j+m)+7 \rightarrow 8(j+m+1)+3} \otimes w_{8j+3 \rightarrow 8(j+1)}; \\
b_{s+(j+1)s,6s+(-2)s} &= -w_{8(j+m+1) \rightarrow 8(j+m+1)+3} \otimes w_{8j+3 \rightarrow 8(j+1)}; \\
b_{4s+(j+1)s,6s+(-2)s} &= -e_{8(j+m+1)+3} \otimes w_{8j+3 \rightarrow 8(j+1)+2}; \\
b_{s+(j+1)s,7s+(-3)s} &= -w_{8(j+m+1) \rightarrow 8(j+m+1)+5} \otimes w_{8j+3 \rightarrow 8(j+1)}; \\
b_{6s+(j+1)s,7s+(-3)s} &= -e_{8(j+m+1)+5} \otimes w_{8j+3 \rightarrow 8(j+1)+3}; \\
b_{(j+1)s,8s+(-4)s} &= w_{8(j+m)+7 \rightarrow 8(j+m+1)+4} \otimes w_{8j+4 \rightarrow 8(j+1)}; \\
b_{s+(j+1)s,8s+(-4)s} &= -w_{8(j+m+1) \rightarrow 8(j+m+1)+4} \otimes w_{8j+4 \rightarrow 8(j+1)}; \\
b_{4s+(j+1)s,8s+(-4)s} &= -w_{8(j+m+1)+3 \rightarrow 8(j+m+1)+4} \otimes w_{8j+4 \rightarrow 8(j+1)+2}; \\
b_{3s+(j+1)s,16s+(-4)s} &= w_{8(j+m+1)+6 \rightarrow 8(j+m+1)+7} \otimes w_{8j+7 \rightarrow 8(j+1)+1}.
\end{aligned}$$

(22) If  $r_0 = 21$ , then  $\Omega^{21}(Z_t^{(20)})$  is described with  $(14s \times 18s)$  matrix with the following nonzero entries:

$$\begin{aligned}
b_{(j+1)s,(-4)s} &= e_{8(j+m+1)+2} \otimes w_{8j \rightarrow 8(j+1)}; \\
b_{(j+1)s,(-2)s} &= e_{8(j+m+1)+2} \otimes w_{8j \rightarrow 8(j+1)};
\end{aligned}$$

$$\begin{aligned}
b_{2s+(j+1)_s, s+(-2)_s} &= -e_{8(j+m+1)+6} \otimes w_{8j \rightarrow 8(j+1)}; \\
b_{j+2s, s+(-1)_s} &= w_{8(j+m)+7 \rightarrow 8(j+m+1)+6} \otimes w_{8j \rightarrow 8j+1}; \\
b_{(j+1)_s, 2s+(-3)_s} &= w_{8(j+m+1)+2 \rightarrow 8(j+m+1)+4} \otimes w_{8j \rightarrow 8(j+1)}; \\
b_{s+(j+1)_s, 2s+(-3)_s} &= e_{8(j+m+1)+4} \otimes w_{8j \rightarrow 8(j+1)}; \\
b_{(j+1)_s, 2s+(-2)_s} &= w_{8(j+m+1)+2 \rightarrow 8(j+m+1)+4} \otimes w_{8j \rightarrow 8(j+1)}; \\
b_{(j+1)_s, 5s+(-3)_s} &= w_{8(j+m+1)+2 \rightarrow 8(j+m+1)+7} \otimes w_{8j+1 \rightarrow 8(j+1)}; \\
b_{s+(j+1)_s, 5s+(-3)_s} &= w_{8(j+m+1)+4 \rightarrow 8(j+m+1)+7} \otimes w_{8j+1 \rightarrow 8(j+1)}; \\
b_{2s+(j+1)_s, 5s+(-2)_s} &= -w_{8(j+m+1)+6 \rightarrow 8(j+m+1)+7} \otimes w_{8j+1 \rightarrow 8(j+1)}; \\
b_{(j+1)_s, 5s+(-1)_s} &= -w_{8(j+m+1)+2 \rightarrow 8(j+m+1)+7} \otimes w_{8j+1 \rightarrow 8(j+1)}; \\
b_{s+(j+1)_s, 5s+(-1)_s} &= -w_{8(j+m+1)+4 \rightarrow 8(j+m+1)+7} \otimes w_{8j+1 \rightarrow 8(j+1)}; \\
b_{(j+1)_s, 6s+(-4)_s} &= -w_{8(j+m+1)+2 \rightarrow 8(j+m+2)} \otimes w_{8j+2 \rightarrow 8(j+1)}; \\
b_{s+(j+1)_s, 6s+(-4)_s} &= -w_{8(j+m+1)+4 \rightarrow 8(j+m+2)} \otimes w_{8j+2 \rightarrow 8(j+1)}; \\
b_{(j+1)_s, 6s+(-3)_s} &= -w_{8(j+m+1)+2 \rightarrow 8(j+m+2)} \otimes w_{8j+2 \rightarrow 8(j+1)}; \\
b_{s+(j+1)_s, 6s+(-3)_s} &= -w_{8(j+m+1)+4 \rightarrow 8(j+m+2)} \otimes w_{8j+2 \rightarrow 8(j+1)}; \\
b_{(j+1)_s, 6s+(-2)_s} &= -w_{8(j+m+1)+2 \rightarrow 8(j+m+2)} \otimes w_{8j+2 \rightarrow 8(j+1)}; \\
b_{s+(j+1)_s, 6s+(-2)_s} &= -w_{8(j+m+1)+4 \rightarrow 8(j+m+2)} \otimes w_{8j+2 \rightarrow 8(j+1)}; \\
b_{(j+1)_s, 7s+(-4)_s} &= w_{8(j+m+1)+2 \rightarrow 8(j+m+1)+7} \otimes w_{8j+3 \rightarrow 8(j+1)}; \\
b_{3s+(j+1)_s, 7s+(-4)_s} &= e_{8(j+m+1)+7} \otimes w_{8j+3 \rightarrow 8(j+1)+1}; \\
b_{(j+1)_s, 7s+(-3)_s} &= w_{8(j+m+1)+2 \rightarrow 8(j+m+1)+7} \otimes w_{8j+3 \rightarrow 8(j+1)}; \\
b_{2s+(j+1)_s, 7s+(-3)_s} &= w_{8(j+m+1)+6 \rightarrow 8(j+m+1)+7} \otimes w_{8j+3 \rightarrow 8(j+1)}; \\
b_{3s+(j+1)_s, 7s+(-3)_s} &= e_{8(j+m+1)+7} \otimes w_{8j+3 \rightarrow 8(j+1)+1}; \\
b_{(j+1)_s, 7s+(-2)_s} &= w_{8(j+m+1)+2 \rightarrow 8(j+m+1)+7} \otimes w_{8j+3 \rightarrow 8(j+1)}; \\
b_{3s+(j+1)_s, 7s+(-2)_s} &= e_{8(j+m+1)+7} \otimes w_{8j+3 \rightarrow 8(j+1)+1}; \\
b_{(j+1)_s, 8s+(-4)_s} &= w_{8(j+m+1)+2 \rightarrow 8(j+m+1)+7} \otimes w_{8j+4 \rightarrow 8(j+1)}; \\
b_{3s+(j+1)_s, 8s+(-4)_s} &= e_{8(j+m+1)+7} \otimes w_{8j+4 \rightarrow 8(j+1)+1}; \\
b_{3s+(j+1)_s, 14s+(-4)_s} &= -w_{8(j+m+1)+7 \rightarrow 8(j+m+2)+5} \otimes w_{8j+7 \rightarrow 8(j+1)+1}.
\end{aligned}$$

(23) If  $r_0 = 22$ , then  $\Omega^{22}(Z_t^{(20)})$  is described with  $(13s \times 19s)$  matrix with the following nonzero entries:

$$\begin{aligned}
b_{s+(j+1)_s, (-3)_s} &= e_{8(j+m)+7} \otimes w_{8j \rightarrow 8(j+1)}; \\
b_{j+2s, (-1)_s} &= -w_{8(j+m)+3 \rightarrow 8(j+m)+7} \otimes w_{8j \rightarrow 8j+1}; \\
b_{j+3s, (-1)_s} &= w_{8(j+m)+4 \rightarrow 8(j+m)+7} \otimes w_{8j \rightarrow 8j+2}; \\
b_{(j+1)_s, s+(-4)_s} &= e_{8(j+m+1)} \otimes w_{8j \rightarrow 8(j+1)}; \\
b_{(j+1)_s, s+(-2)_s} &= e_{8(j+m+1)} \otimes w_{8j \rightarrow 8(j+1)}; \\
b_{s+(j+1)_s, 2s+(-3)_s} &= e_{8(j+m)+7} \otimes w_{8j \rightarrow 8(j+1)}; \\
b_{(j+1)_s, 3s+(-4)_s} &= -w_{8(j+m+1) \rightarrow 8(j+m+1)+2} \otimes w_{8j+1 \rightarrow 8(j+1)}; \\
b_{(j+1)_s, 3s+(-2)_s} &= -w_{8(j+m+1) \rightarrow 8(j+m+1)+2} \otimes w_{8j+1 \rightarrow 8(j+1)}; \\
b_{(j+1)_s, 3s+(-1)_s} &= -w_{8(j+m+1) \rightarrow 8(j+m+1)+2} \otimes w_{8j+1 \rightarrow 8(j+1)}; \\
b_{s+(j+1)_s, 4s+(-4)_s} &= -w_{8(j+m)+7 \rightarrow 8(j+m+1)+3} \otimes w_{8j+2 \rightarrow 8(j+1)}; \\
b_{s+(j+1)_s, 4s+(-3)_s} &= -w_{8(j+m)+7 \rightarrow 8(j+m+1)+3} \otimes w_{8j+2 \rightarrow 8(j+1)}; \\
b_{s+(j+1)_s, 4s+(-2)_s} &= -w_{8(j+m)+7 \rightarrow 8(j+m+1)+3} \otimes w_{8j+2 \rightarrow 8(j+1)};
\end{aligned}$$

$$\begin{aligned}
b_{(j+1)s, 6s+(-4)s} &= w_{8(j+m+1) \rightarrow 8(j+m+1)+4} \otimes w_{8j+3 \rightarrow 8(j+1)}; \\
b_{s+(j+1)s, 6s+(-4)s} &= -w_{8(j+m)+7 \rightarrow 8(j+m+1)+4} \otimes w_{8j+3 \rightarrow 8(j+1)}; \\
b_{3s+(j+1)s, 6s+(-4)s} &= -e_{8(j+m+1)+4} \otimes w_{8j+3 \rightarrow 8(j+1)+2}; \\
b_{(j+1)s, 6s+(-3)s} &= w_{8(j+m+1) \rightarrow 8(j+m+1)+4} \otimes w_{8j+3 \rightarrow 8(j+1)}; \\
b_{s+(j+1)s, 6s+(-3)s} &= -w_{8(j+m)+7 \rightarrow 8(j+m+1)+4} \otimes w_{8j+3 \rightarrow 8(j+1)}; \\
b_{3s+(j+1)s, 6s+(-3)s} &= -e_{8(j+m+1)+4} \otimes w_{8j+3 \rightarrow 8(j+1)+2}; \\
b_{(j+1)s, 6s+(-2)s} &= w_{8(j+m+1) \rightarrow 8(j+m+1)+4} \otimes w_{8j+3 \rightarrow 8(j+1)}; \\
b_{s+(j+1)s, 6s+(-2)s} &= -w_{8(j+m)+7 \rightarrow 8(j+m+1)+4} \otimes w_{8j+3 \rightarrow 8(j+1)}; \\
b_{3s+(j+1)s, 6s+(-2)s} &= -e_{8(j+m+1)+4} \otimes w_{8j+3 \rightarrow 8(j+1)+2}; \\
b_{s+(j+1)s, 7s+(-3)s} &= -w_{8(j+m)+7 \rightarrow 8(j+m+1)+6} \otimes w_{8j+3 \rightarrow 8(j+1)}; \\
b_{5s+(j+1)s, 7s+(-3)s} &= -e_{8(j+m+1)+6} \otimes w_{8j+3 \rightarrow 8(j+1)+3}; \\
b_{2s+(j+1)s, 16s+(-4)s} &= -w_{8(j+m+1)+3 \rightarrow 8(j+m+1)+7} \otimes w_{8j+7 \rightarrow 8(j+1)+1}; \\
b_{3s+(j+1)s, 16s+(-4)s} &= w_{8(j+m+1)+4 \rightarrow 8(j+m+1)+7} \otimes w_{8j+7 \rightarrow 8(j+1)+2}.
\end{aligned}$$

(24) If  $r_0 = 23$ , then  $\Omega^{23}(Z_t^{(20)})$  is described with  $(11s \times 18s)$  matrix with the following nonzero entries:

$$\begin{aligned}
b_{j+2s, (-1)s} &= -w_{8(j+m+1) \rightarrow 8(j+m+1)+2} \otimes w_{8j \rightarrow 8j+1}; \\
b_{(j+1)s, s+(-4)s} &= e_{8(j+m+1)+3} \otimes w_{8j \rightarrow 8(j+1)}; \\
b_{(j+1)s, s+(-2)s} &= e_{8(j+m+1)+3} \otimes w_{8j \rightarrow 8(j+1)}; \\
b_{j+s, s+(-1)s} &= -w_{8(j+m+1) \rightarrow 8(j+m+1)+3} \otimes w_{8j \rightarrow 8j+1}; \\
b_{s+(j+1)s, 3s+(-4)s} &= e_{8(j+m+1)+5} \otimes w_{8j \rightarrow 8(j+1)}; \\
b_{s+(j+1)s, 3s+(-2)s} &= e_{8(j+m+1)+5} \otimes w_{8j \rightarrow 8(j+1)}; \\
b_{s+(j+1)s, 4s+(-4)s} &= -w_{8(j+m+1)+5 \rightarrow 8(j+m+2)} \otimes w_{8j+1 \rightarrow 8(j+1)}; \\
b_{s+(j+1)s, 4s+(-2)s} &= -w_{8(j+m+1)+5 \rightarrow 8(j+m+2)} \otimes w_{8j+1 \rightarrow 8(j+1)}; \\
b_{s+(j+1)s, 4s+(-1)s} &= -w_{8(j+m+1)+5 \rightarrow 8(j+m+2)} \otimes w_{8j+1 \rightarrow 8(j+1)}; \\
b_{s+(j+1)s, 5s+(-4)s} &= -w_{8(j+m+1)+5 \rightarrow 8(j+m+1)+7} \otimes w_{8j+2 \rightarrow 8(j+1)}; \\
b_{3s+(j+1)s, 5s+(-4)s} &= e_{8(j+m+1)+7} \otimes w_{8j+2 \rightarrow 8(j+1)+2}; \\
b_{s+(j+1)s, 5s+(-3)s} &= -w_{8(j+m+1)+5 \rightarrow 8(j+m+1)+7} \otimes w_{8j+2 \rightarrow 8(j+1)}; \\
b_{3s+(j+1)s, 5s+(-3)s} &= e_{8(j+m+1)+7} \otimes w_{8j+2 \rightarrow 8(j+1)+2}; \\
b_{s+(j+1)s, 5s+(-2)s} &= -w_{8(j+m+1)+5 \rightarrow 8(j+m+1)+7} \otimes w_{8j+2 \rightarrow 8(j+1)}; \\
b_{3s+(j+1)s, 5s+(-2)s} &= e_{8(j+m+1)+7} \otimes w_{8j+2 \rightarrow 8(j+1)+2}; \\
b_{(j+1)s, 6s+(-4)s} &= w_{8(j+m+1)+3 \rightarrow 8(j+m+1)+7} \otimes w_{8j+3 \rightarrow 8(j+1)}; \\
b_{s+(j+1)s, 6s+(-3)s} &= w_{8(j+m+1)+5 \rightarrow 8(j+m+1)+7} \otimes w_{8j+3 \rightarrow 8(j+1)}; \\
b_{3s+(j+1)s, 6s+(-3)s} &= -e_{8(j+m+1)+7} \otimes w_{8j+3 \rightarrow 8(j+1)+2}; \\
b_{(j+1)s, 6s+(-2)s} &= w_{8(j+m+1)+3 \rightarrow 8(j+m+1)+7} \otimes w_{8j+3 \rightarrow 8(j+1)}; \\
b_{2s+(j+1)s, 7s+(-4)s} &= e_{8(j+m+2)} \otimes w_{8j+3 \rightarrow 8(j+1)+1}; \\
b_{(j+1)s, 7s+(-3)s} &= w_{8(j+m+1)+3 \rightarrow 8(j+m+2)} \otimes w_{8j+3 \rightarrow 8(j+1)}; \\
b_{s+(j+1)s, 7s+(-3)s} &= -w_{8(j+m+1)+5 \rightarrow 8(j+m+2)} \otimes w_{8j+3 \rightarrow 8(j+1)}; \\
b_{2s+(j+1)s, 7s+(-3)s} &= e_{8(j+m+2)} \otimes w_{8j+3 \rightarrow 8(j+1)+1}; \\
b_{3s+(j+1)s, 7s+(-3)s} &= w_{8(j+m+1)+7 \rightarrow 8(j+m+2)} \otimes w_{8j+3 \rightarrow 8(j+1)+2}; \\
b_{2s+(j+1)s, 7s+(-2)s} &= e_{8(j+m+2)} \otimes w_{8j+3 \rightarrow 8(j+1)+1};
\end{aligned}$$

$$\begin{aligned}
b_{2s+(j+1)s,8s+(-4)s} &= e_{8(j+m+2)} \otimes w_{8j+4 \rightarrow 8(j+1)+1}; \\
b_{2s+(j+1)s,13s+(-4)s} &= -w_{8(j+m+2) \rightarrow 8(j+m+2)+2} \otimes w_{8j+7 \rightarrow 8(j+1)+1}; \\
b_{2s+(j+1)s,16s+(-2)s} &= -w_{8(j+m+2) \rightarrow 8(j+m+2)+1} \otimes w_{8j+7 \rightarrow 8(j+1)+1}.
\end{aligned}$$

(25) If  $r_0 = 24$ , then  $\Omega^{24}(Z_t^{(20)})$  is described with  $(11s \times 20s)$  matrix with the following nonzero entries:

$$\begin{aligned}
b_{(j+1)s,s+(-3)s} &= -e_{8(j+m+1)} \otimes w_{8j \rightarrow 8(j+1)}; \\
b_{j+s,s+(-1)s} &= -w_{8(j+m)+5 \rightarrow 8(j+m+1)} \otimes w_{8j \rightarrow 8j+1}; \\
b_{(j+1)s,2s+(-3)s} &= -e_{8(j+m+1)} \otimes w_{8j \rightarrow 8(j+1)}; \\
b_{j-2s,4s+(-3)s} &= w_{8(j+m)+5 \rightarrow 8(j+m+1)+5} \otimes e_{8j+1}; \\
b_{j-2s,4s+(-1)s} &= -w_{8(j+m)+5 \rightarrow 8(j+m+1)+5} \otimes e_{8j+1}; \\
b_{(j+1)s,5s+(-4)s} &= w_{8(j+m+1) \rightarrow 8(j+m+1)+4} \otimes w_{8j+2 \rightarrow 8(j+1)}; \\
b_{(j+1)s,5s+(-3)s} &= w_{8(j+m+1) \rightarrow 8(j+m+1)+4} \otimes w_{8j+2 \rightarrow 8(j+1)}; \\
b_{(j+1)s,5s+(-2)s} &= w_{8(j+m+1) \rightarrow 8(j+m+1)+4} \otimes w_{8j+2 \rightarrow 8(j+1)}; \\
b_{(j+1)s,6s+(-4)s} &= w_{8(j+m+1) \rightarrow 8(j+m+1)+6} \otimes w_{8j+2 \rightarrow 8(j+1)}; \\
b_{2s+(j+1)s,6s+(-4)s} &= -w_{8(j+m+1)+5 \rightarrow 8(j+m+1)+6} \otimes w_{8j+2 \rightarrow 8(j+1)+1}; \\
b_{(j+1)s,6s+(-3)s} &= w_{8(j+m+1) \rightarrow 8(j+m+1)+6} \otimes w_{8j+2 \rightarrow 8(j+1)}; \\
b_{2s+(j+1)s,6s+(-3)s} &= -w_{8(j+m+1)+5 \rightarrow 8(j+m+1)+6} \otimes w_{8j+2 \rightarrow 8(j+1)+1}; \\
b_{(j+1)s,6s+(-2)s} &= w_{8(j+m+1) \rightarrow 8(j+m+1)+6} \otimes w_{8j+2 \rightarrow 8(j+1)}; \\
b_{2s+(j+1)s,6s+(-2)s} &= -w_{8(j+m+1)+5 \rightarrow 8(j+m+1)+6} \otimes w_{8j+2 \rightarrow 8(j+1)+1}; \\
b_{2s+(j+1)s,7s+(-4)s} &= e_{8(j+m+1)+5} \otimes w_{8j+3 \rightarrow 8(j+1)+1}; \\
b_{2s+(j+1)s,7s+(-3)s} &= e_{8(j+m+1)+5} \otimes w_{8j+3 \rightarrow 8(j+1)+1}; \\
b_{2s+(j+1)s,7s+(-2)s} &= e_{8(j+m+1)+5} \otimes w_{8j+3 \rightarrow 8(j+1)+1}; \\
b_{(j+1)s,8s+(-3)s} &= w_{8(j+m+1) \rightarrow 8(j+m+1)+1} \otimes w_{8j+3 \rightarrow 8(j+1)}; \\
b_{4s+(j+1)s,8s+(-3)s} &= -e_{8(j+m+1)+1} \otimes w_{8j+3 \rightarrow 8(j+1)+3}; \\
b_{2s+(j+1)s,10s+(-4)s} &= w_{8(j+m+1)+5 \rightarrow 8(j+m+1)+6} \otimes w_{8j+4 \rightarrow 8(j+1)+1}; \\
b_{2s+(j+1)s,17s+(-4)s} &= -w_{8(j+m+1)+5 \rightarrow 8(j+m+1)+7} \otimes w_{8j+7 \rightarrow 8(j+1)+1}; \\
b_{2s+(j+1)s,18s+(-4)s} &= -w_{8(j+m+1)+5 \rightarrow 8(j+m+2)} \otimes w_{8j+7 \rightarrow 8(j+1)+1}.
\end{aligned}$$

(26) If  $r_0 = 25$ , then  $\Omega^{25}(Z_t^{(20)})$  is described with  $(10s \times 18s)$  matrix with the following nonzero entries:

$$\begin{aligned}
b_{s+(j+1)s,s+(-4)s} &= -e_{8(j+m+1)+6} \otimes w_{8j \rightarrow 8(j+1)}; \\
b_{s+(j+1)s,s+(-2)s} &= -e_{8(j+m+1)+6} \otimes w_{8j \rightarrow 8(j+1)}; \\
b_{(j+1)s,2s+(-4)s} &= e_{8(j+m+1)+4} \otimes w_{8j \rightarrow 8(j+1)}; \\
b_{(j+1)s,2s+(-2)s} &= e_{8(j+m+1)+4} \otimes w_{8j \rightarrow 8(j+1)}; \\
b_{j-2s,4s+(-3)s} &= w_{8(j+m)+7 \rightarrow 8(j+m+1)+5} \otimes w_{8j \rightarrow 8j+1}; \\
b_{j-s,4s+(-3)s} &= w_{8(j+m+1) \rightarrow 8(j+m+1)+5} \otimes w_{8j \rightarrow 8j+2}; \\
b_{j+3s,4s+(-3)s} &= w_{8(j+m+1) \rightarrow 8(j+m+1)+5} \otimes w_{8j \rightarrow 8j+6}; \\
b_{s+(j+1)s,5s+(-4)s} &= -w_{8(j+m+1)+6 \rightarrow 8(j+m+1)+7} \otimes w_{8j+1 \rightarrow 8(j+1)}; \\
b_{s+(j+1)s,5s+(-3)s} &= -w_{8(j+m+1)+6 \rightarrow 8(j+m+1)+7} \otimes w_{8j+1 \rightarrow 8(j+1)}; \\
b_{s+(j+1)s,5s+(-2)s} &= -w_{8(j+m+1)+6 \rightarrow 8(j+m+1)+7} \otimes w_{8j+1 \rightarrow 8(j+1)}; \\
b_{s+(j+1)s,7s+(-4)s} &= w_{8(j+m+1)+6 \rightarrow 8(j+m+2)} \otimes w_{8j+2 \rightarrow 8(j+1)};
\end{aligned}$$

$$\begin{aligned}
b_{3s+(j+1)s,7s+(-4)s} &= e_{8(j+m+2)} \otimes w_{8j+2 \rightarrow 8(j+1)+2}; \\
b_{s+(j+1)s,7s+(-3)s} &= w_{8(j+m+1)+6 \rightarrow 8(j+m+2)} \otimes w_{8j+2 \rightarrow 8(j+1)}; \\
b_{3s+(j+1)s,7s+(-3)s} &= e_{8(j+m+2)} \otimes w_{8j+2 \rightarrow 8(j+1)+2}; \\
b_{s+(j+1)s,7s+(-2)s} &= w_{8(j+m+1)+6 \rightarrow 8(j+m+2)} \otimes w_{8j+2 \rightarrow 8(j+1)}; \\
b_{3s+(j+1)s,7s+(-2)s} &= e_{8(j+m+2)} \otimes w_{8j+2 \rightarrow 8(j+1)+2}; \\
b_{s+(j+1)s,8s+(-3)s} &= -w_{8(j+m+1)+6 \rightarrow 8(j+m+2)} \otimes w_{8j+3 \rightarrow 8(j+1)}; \\
b_{3s+(j+1)s,8s+(-3)s} &= -e_{8(j+m+2)} \otimes w_{8j+3 \rightarrow 8(j+1)+2}; \\
b_{2s+(j+1)s,17s+(-2)s} &= w_{8(j+m+1)+7 \rightarrow 8(j+m+2)+5} \otimes w_{8j+7 \rightarrow 8(j+1)+1}; \\
b_{3s+(j+1)s,17s+(-2)s} &= w_{8(j+m+2) \rightarrow 8(j+m+2)+5} \otimes w_{8j+7 \rightarrow 8(j+1)+2}; \\
b_{7s+(j+1)s,17s+(-2)s} &= w_{8(j+m+2) \rightarrow 8(j+m+2)+5} \otimes w_{8j+7 \rightarrow 8(j+1)+6}.
\end{aligned}$$

(27) If  $r_0 = 26$ , then  $\Omega^{26}(Z_t^{(20)})$  is described with  $(8s \times 19s)$  matrix with the following nonzero entries:

$$\begin{aligned}
b_{j,(-3)s} &= -w_{8(j+m-1)+7 \rightarrow 8(j+m)+7} \otimes e_{8j}; \\
b_{(j+1)s,(-3)s} &= e_{8(j+m)+7} \otimes w_{8j \rightarrow 8(j+1)}; \\
b_{j+2s,(-3)s} &= -w_{8(j+m)+1 \rightarrow 8(j+m)+7} \otimes w_{8j \rightarrow 8j+2}; \\
b_{j+3s,(-3)s} &= w_{8(j+m)+2 \rightarrow 8(j+m)+7} \otimes w_{8j \rightarrow 8j+3}; \\
b_{j+4s,(-3)s} &= -w_{8(j+m)+3 \rightarrow 8(j+m)+7} \otimes w_{8j \rightarrow 8j+4}; \\
b_{j+5s,(-3)s} &= -w_{8(j+m)+4 \rightarrow 8(j+m)+7} \otimes w_{8j \rightarrow 8j+5}; \\
b_{(j+1)s,s+(-4)s} &= -w_{8(j+m)+7 \rightarrow 8(j+m+1)} \otimes w_{8j \rightarrow 8(j+1)}; \\
b_{(j+1)s,s+(-2)s} &= -w_{8(j+m)+7 \rightarrow 8(j+m+1)} \otimes w_{8j \rightarrow 8(j+1)}; \\
b_{(j+1)s,2s+(-4)s} &= e_{8(j+m)+7} \otimes w_{8j \rightarrow 8(j+1)}; \\
b_{j-2s,2s+(-3)s} &= -w_{8(j+m-1)+7 \rightarrow 8(j+m)+7} \otimes e_{8j}; \\
b_{(j+1)s,2s+(-3)s} &= e_{8(j+m)+7} \otimes w_{8j \rightarrow 8(j+1)}; \\
b_{j,2s+(-3)s} &= -w_{8(j+m)+1 \rightarrow 8(j+m)+7} \otimes w_{8j \rightarrow 8j+2}; \\
b_{j+s,2s+(-3)s} &= w_{8(j+m)+2 \rightarrow 8(j+m)+7} \otimes w_{8j \rightarrow 8j+3}; \\
b_{j+2s,2s+(-3)s} &= -w_{8(j+m)+3 \rightarrow 8(j+m)+7} \otimes w_{8j \rightarrow 8j+4}; \\
b_{j+3s,2s+(-3)s} &= -w_{8(j+m)+4 \rightarrow 8(j+m)+7} \otimes w_{8j \rightarrow 8j+5}; \\
b_{(j+1)s,2s+(-2)s} &= e_{8(j+m)+7} \otimes w_{8j \rightarrow 8(j+1)}; \\
b_{(j+1)s,5s+(-4)s} &= -w_{8(j+m)+7 \rightarrow 8(j+m+1)+5} \otimes w_{8j+2 \rightarrow 8(j+1)}; \\
b_{(j+1)s,5s+(-2)s} &= -w_{8(j+m)+7 \rightarrow 8(j+m+1)+5} \otimes w_{8j+2 \rightarrow 8(j+1)}; \\
b_{2s+(j+1)s,6s+(-4)s} &= e_{8(j+m+1)+1} \otimes w_{8j+2 \rightarrow 8(j+1)+2}; \\
b_{2s+(j+1)s,6s+(-3)s} &= e_{8(j+m+1)+1} \otimes w_{8j+2 \rightarrow 8(j+1)+2}; \\
b_{2s+(j+1)s,6s+(-2)s} &= e_{8(j+m+1)+1} \otimes w_{8j+2 \rightarrow 8(j+1)+2}; \\
b_{2s+(j+1)s,7s+(-3)s} &= -w_{8(j+m+1)+1 \rightarrow 8(j+m+1)+2} \otimes w_{8j+3 \rightarrow 8(j+1)+2}; \\
b_{3s+(j+1)s,7s+(-3)s} &= e_{8(j+m+1)+2} \otimes w_{8j+3 \rightarrow 8(j+1)+3}; \\
b_{s+(j+1)s,8s+(-4)s} &= -e_{8(j+m+1)+6} \otimes w_{8j+3 \rightarrow 8(j+1)+1}; \\
b_{(j+1)s,8s+(-3)s} &= w_{8(j+m)+7 \rightarrow 8(j+m+1)+6} \otimes w_{8j+3 \rightarrow 8(j+1)}; \\
b_{s+(j+1)s,8s+(-3)s} &= -e_{8(j+m+1)+6} \otimes w_{8j+3 \rightarrow 8(j+1)+1}; \\
b_{s+(j+1)s,8s+(-2)s} &= -e_{8(j+m+1)+6} \otimes w_{8j+3 \rightarrow 8(j+1)+1}; \\
b_{6s+(j+1)s,15s+(-2)s} &= e_{8(j+m+1)+5} \otimes w_{8j+6 \rightarrow 8(j+1)+6};
\end{aligned}$$

$$\begin{aligned}
b_{(j+1)s, 16s+(-2)_s} &= w_{8(j+m)+7 \rightarrow 8(j+m+1)+7} \otimes w_{8j+7 \rightarrow 8(j+1)}; \\
b_{2s+(j+1)s, 16s+(-2)_s} &= w_{8(j+m+1)+1 \rightarrow 8(j+m+1)+7} \otimes w_{8j+7 \rightarrow 8(j+1)+2}; \\
b_{3s+(j+1)s, 16s+(-2)_s} &= -w_{8(j+m+1)+2 \rightarrow 8(j+m+1)+7} \otimes w_{8j+7 \rightarrow 8(j+1)+3}; \\
b_{4s+(j+1)s, 16s+(-2)_s} &= w_{8(j+m+1)+3 \rightarrow 8(j+m+1)+7} \otimes w_{8j+7 \rightarrow 8(j+1)+4}; \\
b_{5s+(j+1)s, 16s+(-2)_s} &= w_{8(j+m+1)+4 \rightarrow 8(j+m+1)+7} \otimes w_{8j+7 \rightarrow 8(j+1)+5}.
\end{aligned}$$

(28) If  $r_0 = 27$ , then  $\Omega^{27}(Z_t^{(20)})$  is described with  $(9s \times 18s)$  matrix with the following nonzero entries:

$$\begin{aligned}
b_{j,s+(-3)_s} &= w_{8(j+m+1) \rightarrow 8(j+m+1)+4} \otimes w_{8j \rightarrow 8j+1}; \\
b_{j+4s,s+(-3)_s} &= -w_{8(j+m+1) \rightarrow 8(j+m+1)+4} \otimes w_{8j \rightarrow 8j+5}; \\
b_{(j+1)s, 6s+(-4)_s} &= -w_{8(j+m+1)+7 \rightarrow 8(j+m+2)} \otimes w_{8j+2 \rightarrow 8(j+1)}; \\
b_{(j+1)s, 6s+(-3)_s} &= -w_{8(j+m+1)+7 \rightarrow 8(j+m+2)} \otimes w_{8j+2 \rightarrow 8(j+1)}; \\
b_{(j+1)s, 6s+(-2)_s} &= -w_{8(j+m+1)+7 \rightarrow 8(j+m+2)} \otimes w_{8j+2 \rightarrow 8(j+1)}; \\
b_{(j+1)s, 7s+(-4)_s} &= -e_{8(j+m+1)+7} \otimes w_{8j+3 \rightarrow 8(j+1)}; \\
b_{(j+1)s, 7s+(-3)_s} &= -e_{8(j+m+1)+7} \otimes w_{8j+3 \rightarrow 8(j+1)}; \\
b_{(j+1)s, 7s+(-2)_s} &= -e_{8(j+m+1)+7} \otimes w_{8j+3 \rightarrow 8(j+1)}; \\
b_{(j+1)s, 10s+(-4)_s} &= e_{8(j+m+1)+7} \otimes w_{8j+5 \rightarrow 8(j+1)}; \\
b_{(j+1)s, 11s+(-2)_s} &= e_{8(j+m+1)+7} \otimes w_{8j+6 \rightarrow 8(j+1)}; \\
b_{(j+1)s, 13s+(-4)_s} &= w_{8(j+m+1)+7 \rightarrow 8(j+m+2)+3} \otimes w_{8j+7 \rightarrow 8(j+1)}; \\
b_{(j+1)s, 13s+(-2)_s} &= w_{8(j+m+1)+7 \rightarrow 8(j+m+2)+3} \otimes w_{8j+7 \rightarrow 8(j+1)}.
\end{aligned}$$

(29) If  $r_0 = 28$ , then  $\Omega^{28}(Z_t^{(20)})$  is described with  $(8s \times 19s)$  matrix with the following nonzero entries:

$$\begin{aligned}
b_{j+s,(-3)_s} &= -w_{8(j+m)+1 \rightarrow 8(j+m)+7} \otimes w_{8j \rightarrow 8j+1}; \\
b_{j+2s,(-3)_s} &= w_{8(j+m)+2 \rightarrow 8(j+m)+7} \otimes w_{8j \rightarrow 8j+2}; \\
b_{j+3s,(-3)_s} &= -w_{8(j+m)+3 \rightarrow 8(j+m)+7} \otimes w_{8j \rightarrow 8j+3}; \\
b_{j+4s,(-3)_s} &= w_{8(j+m)+4 \rightarrow 8(j+m)+7} \otimes w_{8j \rightarrow 8j+4}; \\
b_{j+5s,(-3)_s} &= w_{8(j+m)+5 \rightarrow 8(j+m)+7} \otimes w_{8j \rightarrow 8j+5}; \\
b_{j+6s,(-3)_s} &= -w_{8(j+m)+6 \rightarrow 8(j+m)+7} \otimes w_{8j \rightarrow 8j+6}; \\
b_{j+7s,(-3)_s} &= e_{8(j+m)+7} \otimes w_{8j \rightarrow 8j+7}; \\
b_{j-s,s+(-3)_s} &= w_{8(j+m) \rightarrow 8(j+m+1)} \otimes e_{8j}; \\
b_{(j+1)s, 2s+(-4)_s} &= e_{8(j+m+1)} \otimes w_{8j \rightarrow 8(j+1)}; \\
b_{(j+1)s, 2s+(-3)_s} &= e_{8(j+m+1)} \otimes w_{8j \rightarrow 8(j+1)}; \\
b_{(j+1)s, 2s+(-2)_s} &= e_{8(j+m+1)} \otimes w_{8j \rightarrow 8(j+1)}; \\
b_{(j+1)s, 4s+(-4)_s} &= w_{8(j+m+1) \rightarrow 8(j+m+1)+1} \otimes w_{8j+1 \rightarrow 8(j+1)}; \\
b_{s+(j+1)s, 4s+(-4)_s} &= -e_{8(j+m+1)+1} \otimes w_{8j+1 \rightarrow 8(j+1)+1}; \\
b_{(j+1)s, 4s+(-3)_s} &= w_{8(j+m+1) \rightarrow 8(j+m+1)+1} \otimes w_{8j+1 \rightarrow 8(j+1)}; \\
b_{s+(j+1)s, 4s+(-3)_s} &= -e_{8(j+m+1)+1} \otimes w_{8j+1 \rightarrow 8(j+1)+1}; \\
b_{(j+1)s, 4s+(-2)_s} &= w_{8(j+m+1) \rightarrow 8(j+m+1)+1} \otimes w_{8j+1 \rightarrow 8(j+1)}; \\
b_{s+(j+1)s, 4s+(-2)_s} &= -e_{8(j+m+1)+1} \otimes w_{8j+1 \rightarrow 8(j+1)+1}; \\
b_{(j+1)s, 5s+(-4)_s} &= -w_{8(j+m+1) \rightarrow 8(j+m+1)+2} \otimes w_{8j+2 \rightarrow 8(j+1)}; \\
b_{s+(j+1)s, 5s+(-4)_s} &= w_{8(j+m+1)+1 \rightarrow 8(j+m+1)+2} \otimes w_{8j+2 \rightarrow 8(j+1)+1};
\end{aligned}$$

$$\begin{aligned}
b_{2s+(j+1)s, 5s+(-4)s} &= -e_{8(j+m+1)+2} \otimes w_{8j+2 \rightarrow 8(j+1)+2}; \\
b_{(j+1)s, 5s+(-3)s} &= -w_{8(j+m+1) \rightarrow 8(j+m+1)+2} \otimes w_{8j+2 \rightarrow 8(j+1)}; \\
b_{s+(j+1)s, 5s+(-3)s} &= w_{8(j+m+1)+1 \rightarrow 8(j+m+1)+2} \otimes w_{8j+2 \rightarrow 8(j+1)+1}; \\
b_{2s+(j+1)s, 5s+(-3)s} &= -e_{8(j+m+1)+2} \otimes w_{8j+2 \rightarrow 8(j+1)+2}; \\
b_{(j+1)s, 5s+(-2)s} &= -w_{8(j+m+1) \rightarrow 8(j+m+1)+2} \otimes w_{8j+2 \rightarrow 8(j+1)}; \\
b_{s+(j+1)s, 5s+(-2)s} &= w_{8(j+m+1)+1 \rightarrow 8(j+m+1)+2} \otimes w_{8j+2 \rightarrow 8(j+1)+1}; \\
b_{2s+(j+1)s, 5s+(-2)s} &= -e_{8(j+m+1)+2} \otimes w_{8j+2 \rightarrow 8(j+1)+2}; \\
b_{j-4s, 7s+(-3)s} &= w_{8(j+m)+3 \rightarrow 8(j+m+1)+3} \otimes e_{8j+3}; \\
b_{j-3s, 7s+(-3)s} &= -w_{8(j+m)+4 \rightarrow 8(j+m+1)+3} \otimes w_{8j+3 \rightarrow 8j+4}; \\
b_{j, 7s+(-3)s} &= -w_{8(j+m)+7 \rightarrow 8(j+m+1)+3} \otimes w_{8j+3 \rightarrow 8j+7}; \\
b_{(j+1)s, 11s+(-4)s} &= w_{8(j+m+1) \rightarrow 8(j+m+1)+6} \otimes w_{8j+5 \rightarrow 8(j+1)}; \\
b_{5s+(j+1)s, 11s+(-4)s} &= w_{8(j+m+1)+5 \rightarrow 8(j+m+1)+6} \otimes w_{8j+5 \rightarrow 8(j+1)+5}; \\
b_{j-7s, 13s+(-2)s} &= -w_{8(j+m)+6 \rightarrow 8(j+m+1)+6} \otimes e_{8j+6}; \\
b_{j-6s, 13s+(-2)s} &= w_{8(j+m)+7 \rightarrow 8(j+m+1)+6} \otimes w_{8j+6 \rightarrow 8j+7}; \\
b_{(j+1)s, 14s+(-4)s} &= -w_{8(j+m+1) \rightarrow 8(j+m+1)+4} \otimes w_{8j+6 \rightarrow 8(j+1)}; \\
b_{(j+1)s, 16s+(-4)s} &= w_{8(j+m+1) \rightarrow 8(j+m+1)+7} \otimes w_{8j+7 \rightarrow 8(j+1)}; \\
b_{j-9s, 16s+(-2)s} &= w_{8(j+m)+7 \rightarrow 8(j+m+1)+7} \otimes e_{8j+7}; \\
b_{(j+1)s, 17s+(-4)s} &= w_{8(j+m+1) \rightarrow 8(j+m+2)} \otimes w_{8j+7 \rightarrow 8(j+1)}.
\end{aligned}$$

(II) Represent an arbitrary  $t_0 \in \mathbb{N}$  in the form  $t_0 = 29\ell_0 + r_0$ , where  $0 \leq r_0 \leq 28$ . Then  $\Omega^{t_0}(Z_t^{(20)})$  is a  $\Omega^{r_0}(Z_t^{(20)})$ , whose left components twisted by  $\sigma^{\ell_0}$ .

**Proposition 16** (Translates for the case 21). (I) Let  $r_0 \in \mathbb{N}$ ,  $r_0 < 29$ .  $r_0$ -translates of the elements  $Z_t^{(21)}$  are described by the following way.

(1) If  $r_0 = 0$ , then  $\Omega^0(Z_t^{(21)})$  is described with  $(8s \times 16s)$  matrix, whose entries  $b_{ij}$  have the following form:

If  $s \leq j < 2s$ , then

$$b_{ij} = \begin{cases} e_{8(j+m)} \otimes e_{8j}, & i = j - s; \\ 0, & \text{otherwise.} \end{cases}$$

If  $2s \leq j < 3s$ , then

$$b_{ij} = \begin{cases} -w_{8(j+m)+1 \rightarrow 8(j+m)+2} \otimes e_{8j+1}, & i = j - s; \\ 0, & \text{otherwise.} \end{cases}$$

If  $3s \leq j < 4s$ , then  $b_{ij} = 0$ .

If  $4s \leq j < 5s$ , then

$$b_{ij} = \begin{cases} -w_{8(j+m)+2 \rightarrow 8(j+m)+3} \otimes e_{8j+2}, & i = j - 2s; \\ 0, & \text{otherwise.} \end{cases}$$

If  $5s \leq j < 6s$ , then

$$b_{ij} = \begin{cases} -w_{8(j+m)+3 \rightarrow 8(j+m)+4} \otimes e_{8j+3}, & i = j - 2s; \\ 0, & \text{otherwise.} \end{cases}$$

If  $6s \leq j < 8s$ , then  $b_{ij} = 0$ .



If  $8s \leq j < 9s$ , then

$$b_{ij} = \begin{cases} -w_{8(j+m)+5 \rightarrow 8(j+m)+6} \otimes e_{8j+5}, & i = j - 3s; \\ 0, & \text{otherwise.} \end{cases}$$

If  $9s \leq j < 13s$ , then  $b_{ij} = 0$ .

If  $13s \leq j < 14s$ , then

$$b_{ij} = \begin{cases} e_{8(j+m)+7} \otimes e_{8j+7}, & i = j - 6s; \\ 0, & \text{otherwise.} \end{cases}$$

If  $14s \leq j < 15s$ , then

$$b_{ij} = \begin{cases} -w_{8(j+m)+7 \rightarrow 8(j+m)+8} \otimes e_{8j+7}, & i = j - 7s; \\ 0, & \text{otherwise.} \end{cases}$$

If  $15s \leq j < 16s$ , then  $b_{ij} = 0$ .

(2) If  $r_0 = 1$ , then  $\Omega^1(Z_t^{(21)})$  is described with  $(9s \times 14s)$  matrix, whose entries  $b_{ij}$  have the following form:

If  $0 \leq j < s$ , then

$$b_{ij} = \begin{cases} -w_{8(j+m)+1 \rightarrow 8(j+m)+2} \otimes e_{8j}, & i = j; \\ 0, & \text{otherwise.} \end{cases}$$

If  $s \leq j < 2s$ , then

$$b_{ij} = \begin{cases} w_{8(j+m)+1 \rightarrow 8(j+m)+4} \otimes e_{8j}, & i = j - s; \\ w_{8(j+m)+3 \rightarrow 8(j+m)+4} \otimes w_{8j \rightarrow 8j+2}, & i = j + 2s; \\ 0, & \text{otherwise.} \end{cases}$$

If  $2s \leq j < 3s$ , then

$$b_{ij} = \begin{cases} w_{8(j+m)+5 \rightarrow 8(j+m)+6} \otimes e_{8j}, & i = j - s; \\ 0, & \text{otherwise.} \end{cases}$$

If  $3s \leq j < 4s$ , then

$$b_{ij} = \begin{cases} -w_{8(j+m)+2 \rightarrow 8(j+m)+7} \otimes e_{8j+1}, & i = j - s; \\ 0, & \text{otherwise.} \end{cases}$$

If  $4s \leq j < 5s$ , then

$$b_{ij} = \begin{cases} -w_{8(j+m)+3 \rightarrow 8(j+m)+1} \otimes e_{8j+2}, & i = j - s; \\ -e_{8(j+m)+1} \otimes w_{8j+2 \rightarrow 8j+7}, & i = j + 4s; \\ 0, & \text{otherwise.} \end{cases}$$

If  $5s \leq j < 6s$ , then

$$b_{ij} = \begin{cases} -w_{8(j+m)+4 \rightarrow 8(j+m)+7} \otimes e_{8j+3}, & i = j - s; \\ -e_{8(j+m)+7} \otimes w_{8j+3 \rightarrow 8j+4}, & i = j; \\ 0, & \text{otherwise.} \end{cases}$$

If  $6s \leq j < 7s$ , then  $b_{ij} = 0$ .

If  $7s \leq j < 8s$ , then

$$b_{ij} = \begin{cases} -w_{8(j+m)+6 \rightarrow 8(j+m)+7} \otimes e_{8j+5}, & i = j - s; \\ -e_{8(j+m)+7} \otimes w_{8j+5 \rightarrow 8j+6}, & i = j; \\ 0, & \text{otherwise.} \end{cases}$$

If  $8s \leq j < 9s$ , then

$$b_{ij} = \begin{cases} -e_{8(j+m+1)} \otimes w_{8j+5 \rightarrow 8j+7}, & i = j; \\ 0, & \text{otherwise.} \end{cases}$$

If  $9s \leq j < 10s$ , then  $b_{ij} = 0$ .

If  $10s \leq j < 11s$ , then

$$b_{ij} = \begin{cases} w_{8(j+m+1)+2 \rightarrow 8(j+m+1)+3} \otimes w_{8j+7 \rightarrow 8(j+1)+1}, & i = 2s + (j+1)_s; \\ 0, & \text{otherwise.} \end{cases}$$

If  $11s \leq j < 12s$ , then

$$b_{ij} = \begin{cases} w_{8(j+m+1)+5 \rightarrow 8(j+m+1)+6} \otimes w_{8j+7 \rightarrow 8(j+1)}, & i = s + (j+1)_s; \\ w_{8(j+m+1) \rightarrow 8(j+m+1)+6} \otimes e_{8j+7}, & i = j - 3s; \\ 0, & \text{otherwise.} \end{cases}$$

If  $12s \leq j < 13s$ , then  $b_{ij} = 0$ .

If  $13s \leq j < 14s$ , then

$$b_{ij} = \begin{cases} -w_{8(j+m+1) \rightarrow 8(j+m+1)+5} \otimes e_{8j+7}, & i = j - 5s; \\ 0, & \text{otherwise.} \end{cases}$$

(3) If  $r_0 = 2$ , then  $\Omega^2(Z_t^{(21)})$  is described with  $(8s \times 13s)$  matrix, whose entries  $b_{ij}$  have the following form:

If  $s \leq j < 2s$ , then

$$b_{ij} = \begin{cases} e_{8(j+m-1)+7} \otimes e_{8j}, & i = j - s; \\ 0, & \text{otherwise.} \end{cases}$$

If  $2s \leq j < 3s$ , then

$$b_{ij} = \begin{cases} -w_{8(j+m)+2 \rightarrow 8(j+m)+3} \otimes e_{8j+1}, & i = j - s; \\ 0, & \text{otherwise.} \end{cases}$$

If  $3s \leq j < 4s$ , then

$$b_{ij} = \begin{cases} -w_{8(j+m)+3 \rightarrow 8(j+m)+4} \otimes e_{8j+2}, & i = j - s; \\ 0, & \text{otherwise.} \end{cases}$$

If  $4s \leq j < 5s$ , then  $b_{ij} = 0$ .

If  $5s \leq j < 6s$ , then

$$b_{ij} = \begin{cases} -w_{8(j+m)+5 \rightarrow 8(j+m)+6} \otimes w_{8j+3 \rightarrow 8j+4}, & i = j - s; \\ 0, & \text{otherwise.} \end{cases}$$

If  $6s \leq j < 7s$ , then  $b_{ij} = 0$ .

If  $7s \leq j < 8s$ , then

$$b_{ij} = \begin{cases} -w_{8(j+m)+1 \rightarrow 8(j+m)+2} \otimes w_{8j+5 \rightarrow 8j+6}, & i = j - s; \\ 0, & \text{otherwise.} \end{cases}$$

If  $8s \leq j < 12s$ , then  $b_{ij} = 0$ .

If  $12s \leq j < 13s$ , then

$$b_{ij} = \begin{cases} e_{8(j+m+1)} \otimes e_{8j+7}, & i = j - 5s; \\ 0, & \text{otherwise.} \end{cases}$$

(4) If  $r_0 = 3$ , then  $\Omega^3(Z_t^{(21)})$  is described with  $(10s \times 11s)$  matrix, whose entries  $b_{ij}$  have the following form:

If  $0 \leq j < s$ , then

$$b_{ij} = \begin{cases} -w_{8(j+m)+2 \rightarrow 8(j+m)+3} \otimes e_{8j}, & i = j; \\ 0, & \text{otherwise.} \end{cases}$$

If  $s \leq j < 2s$ , then  $b_{ij} = 0$ .

If  $2s \leq j < 3s$ , then

$$b_{ij} = \begin{cases} -w_{8(j+m)+3 \rightarrow 8(j+m)+4} \otimes e_{8j+1}, & i = j; \\ 0, & \text{otherwise.} \end{cases}$$

If  $3s \leq j < 4s$ , then

$$b_{ij} = \begin{cases} -w_{8(j+m)+4 \rightarrow 8(j+m)+7} \otimes e_{8j+2}, & i = j; \\ -e_{8(j+m)+7} \otimes w_{8j+2 \rightarrow 8j+3}, & i = j + s; \\ 0, & \text{otherwise.} \end{cases}$$

If  $4s \leq j < 5s$ , then

$$b_{ij} = \begin{cases} -e_{8(j+m+1)} \otimes w_{8j+3 \rightarrow 8j+4}, & i = j + s; \\ 0, & \text{otherwise.} \end{cases}$$

If  $5s \leq j < 6s$ , then

$$b_{ij} = \begin{cases} w_{8(j+m+1) \rightarrow 8(j+m+1)+1} \otimes e_{8j+4}, & i = j; \\ 0, & \text{otherwise.} \end{cases}$$

If  $6s \leq j < 7s$ , then

$$b_{ij} = \begin{cases} -e_{8(j+m+1)} \otimes w_{8j+5 \rightarrow 8j+6}, & i = j + s; \\ 0, & \text{otherwise.} \end{cases}$$

If  $7s \leq j < 8s$ , then  $b_{ij} = 0$ .

If  $8s \leq j < 9s$ , then

$$b_{ij} = \begin{cases} -w_{8(j+m+1)+1 \rightarrow 8(j+m+1)+2} \otimes e_{8j+7}, & i = j; \\ 0, & \text{otherwise.} \end{cases}$$

If  $9s \leq j < 10s$ , then

$$b_{ij} = \begin{cases} w_{8(j+m+1)+3 \rightarrow 8(j+m+1)+4} \otimes w_{8j+7 \rightarrow 8(j+1)+1}, & i = 2s + (j+1)_s; \\ w_{8(j+m+1)+1 \rightarrow 8(j+m+1)+4} \otimes e_{8j+7}, & i = j - s; \\ 0, & \text{otherwise.} \end{cases}$$

If  $10s \leq j < 11s$ , then

$$b_{ij} = \begin{cases} w_{8(j+m+1)+5 \rightarrow 8(j+m+1)+6} \otimes e_{8j+7}, & i = j - s; \\ 0, & \text{otherwise.} \end{cases}$$

(5) If  $r_0 = 4$ , then  $\Omega^4(Z_t^{(21)})$  is described with  $(11s \times 11s)$  matrix, whose entries  $b_{ij}$  have the following form:

If  $0 \leq j < s$ , then

$$b_{ij} = \begin{cases} -w_{8(j+m-1)+7 \rightarrow 8(j+m)} \otimes e_{8j}, & i = j; \\ -e_{8(j+m)} \otimes e_{8j}, & i = j + s; \\ 0, & \text{otherwise.} \end{cases}$$

If  $s \leq j < 2s$ , then

$$b_{ij} = \begin{cases} -w_{8(j+m)+3 \rightarrow 8(j+m)+4} \otimes e_{8j+1}, & i = j + s; \\ -w_{8(j+m)+1 \rightarrow 8(j+m)+4} \otimes w_{8j+1 \rightarrow 8j+4}, & i = j + 5s; \\ 0, & \text{otherwise.} \end{cases}$$

If  $2s \leq j < 3s$ , then  $b_{ij} = 0$ .

If  $3s \leq j < 4s$ , then

$$b_{ij} = \begin{cases} -w_{8(j+m)+5 \rightarrow 8(j+m)+6} \otimes w_{8j+2 \rightarrow 8j+3}, & i = j + s; \\ 0, & \text{otherwise.} \end{cases}$$

If  $4s \leq j < 5s$ , then  $b_{ij} = 0$ .

If  $5s \leq j < 6s$ , then

$$b_{ij} = \begin{cases} w_{8(j+m)+1 \rightarrow 8(j+m)+2} \otimes e_{8j+4}, & i = j + s; \\ 0, & \text{otherwise.} \end{cases}$$

If  $6s \leq j < 7s$ , then

$$b_{ij} = \begin{cases} -w_{8(j+m)+2 \rightarrow 8(j+m)+3} \otimes w_{8j+5 \rightarrow 8j+6}, & i = j + 2s; \\ 0, & \text{otherwise.} \end{cases}$$

If  $7s \leq j < 8s$ , then

$$b_{ij} = \begin{cases} -w_{8(j+m)+5 \rightarrow 8(j+m)+6} \otimes w_{8j+5 \rightarrow 8j+6}, & i = j + 2s; \\ 0, & \text{otherwise.} \end{cases}$$

If  $8s \leq j < 10s$ , then  $b_{ij} = 0$ .

If  $10s \leq j < 11s$ , then

$$b_{ij} = \begin{cases} e_{8(j+m)+7} \otimes e_{8j+7}, & i = j; \\ 0, & \text{otherwise.} \end{cases}$$

(6) If  $r_0 = 5$ , then  $\Omega^5(Z_t^{(21)})$  is described with  $(11s \times 10s)$  matrix, whose entries  $b_{ij}$  have the following form:

If  $0 \leq j < s$ , then

$$b_{ij} = \begin{cases} -w_{8(j+m)+3 \rightarrow 8(j+m)+4} \otimes e_{8j}, & i = j + s; \\ -w_{8(j+m)+1 \rightarrow 8(j+m)+4} \otimes e_{8j}, & i = j + 2s; \\ 0, & \text{otherwise.} \end{cases}$$

If  $s \leq j < 2s$ , then

$$b_{ij} = \begin{cases} -w_{8(j+m)+5 \rightarrow 8(j+m)+6} \otimes e_{8j}, & i = j - s; \\ 0, & \text{otherwise.} \end{cases}$$

If  $2s \leq j < 3s$ , then

$$b_{ij} = \begin{cases} -w_{8(j+m)+4 \rightarrow 8(j+m)+7} \otimes e_{8j+1}, & i = j + s; \\ -e_{8(j+m)+7} \otimes w_{8j+1 \rightarrow 8j+2}, & i = j + 2s; \\ e_{8(j+m)+7} \otimes w_{8j+1 \rightarrow 8j+4}, & i = j + 4s; \\ 0, & \text{otherwise.} \end{cases}$$

If  $3s \leq j < 4s$ , then

$$b_{ij} = \begin{cases} -e_{8(j+m)+1} \otimes w_{8j+2 \rightarrow 8j+3}, & i = j + 2s; \\ -w_{8(j+m)+7 \rightarrow 8(j+m)+1} \otimes w_{8j+2 \rightarrow 8j+4}, & i = j + 3s; \\ 0, & \text{otherwise.} \end{cases}$$

If  $4s \leq j < 5s$ , then

$$b_{ij} = \begin{cases} -e_{8(j+m)+1+1} \otimes w_{8j+3 \rightarrow 8(j+1)}, & i = 2s + (j+1)_s; \\ w_{8(j+m)+7 \rightarrow 8(j+m)+1+1} \otimes w_{8j+3 \rightarrow 8j+4}, & i = j + 2s; \\ 0, & \text{otherwise.} \end{cases}$$

If  $5s \leq j < 6s$ , then

$$b_{ij} = \begin{cases} w_{8(j+m)+1 \rightarrow 8(j+m)+2} \otimes w_{8j+4 \rightarrow 8(j+1)}, & i = 2s + (j+1)_s; \\ -w_{8(j+m)+7 \rightarrow 8(j+m)+2} \otimes e_{8j+4}, & i = j + s; \\ 0, & \text{otherwise.} \end{cases}$$

If  $6s \leq j < 7s$ , then

$$b_{ij} = \begin{cases} -e_{8(j+m)+7} \otimes w_{8j+5 \rightarrow 8j+6}, & i = j + 2s; \\ 0, & \text{otherwise.} \end{cases}$$

If  $7s \leq j < 8s$ , then  $b_{ij} = 0$ .

If  $8s \leq j < 9s$ , then

$$b_{ij} = \begin{cases} -w_{8(j+m)+2 \rightarrow 8(j+m)+3} \otimes e_{8j+7}, & i = j + s; \\ 0, & \text{otherwise.} \end{cases}$$

If  $9s \leq j < 10s$ , then  $b_{ij} = 0$ .

(7) If  $r_0 = 6$ , then  $\Omega^6(Z_t^{(21)})$  is described with  $(13s \times 8s)$  matrix, whose entries  $b_{ij}$  have the following form:

If  $0 \leq j < s$ , then

$$b_{ij} = \begin{cases} e_{8(j+m-1)+7} \otimes e_{8j}, & i = j; \\ 0, & \text{otherwise.} \end{cases}$$

If  $s \leq j < 2s$ , then

$$b_{ij} = \begin{cases} -w_{8(j+m)+5 \rightarrow 8(j+m)+6} \otimes w_{8j+1 \rightarrow 8j+2}, & i = j + 2s; \\ 0, & \text{otherwise.} \end{cases}$$

If  $2s \leq j < 3s$ , then

$$b_{ij} = \begin{cases} -e_{8(j+m)+1} \otimes w_{8j+2 \rightarrow 8j+3}, & i = j + 3s; \\ 0, & \text{otherwise.} \end{cases}$$

If  $3s \leq j < 4s$ , then  $b_{ij} = 0$ .

If  $4s \leq j < 5s$ , then

$$b_{ij} = \begin{cases} -w_{8(j+m)+2 \rightarrow 8(j+m)+3} \otimes e_{8j+4}, & i = j + 2s; \\ 0, & \text{otherwise.} \end{cases}$$

If  $5s \leq j < 6s$ , then

$$b_{ij} = \begin{cases} -w_{8(j+m)+3 \rightarrow 8(j+m)+4} \otimes w_{8j+5 \rightarrow 8j+6}, & i = j + 4s; \\ 0, & \text{otherwise.} \end{cases}$$

If  $6s \leq j < 7s$ , then  $b_{ij} = 0$ .

If  $7s \leq j < 8s$ , then

$$b_{ij} = \begin{cases} -w_{8(j+m)+7 \rightarrow 8(j+m)+1} \otimes e_{8j+7}, & i = j + 4s; \\ -e_{8(j+m)+1} \otimes e_{8j+7}, & i = j + 5s; \\ 0, & \text{otherwise.} \end{cases}$$

(8) If  $r_0 = 7$ , then  $\Omega^7(Z_t^{(21)})$  is described with  $(14s \times 9s)$  matrix, whose entries  $b_{ij}$  have the following form:

If  $0 \leq j < s$ , then

$$b_{ij} = \begin{cases} w_{8(j+m)+2 \rightarrow 8(j+m)+7} \otimes e_{8j}, & i = j; \\ -w_{8(j+m)+4 \rightarrow 8(j+m)+7} \otimes e_{8j}, & i = j + s; \\ -e_{8(j+m)+7} \otimes w_{8j \rightarrow 8j+1}, & i = j + 4s; \\ 0, & \text{otherwise.} \end{cases}$$

If  $s \leq j < 2s$ , then

$$b_{ij} = \begin{cases} -e_{8(j+m)+1} \otimes w_{8j+1 \rightarrow 8j+2}, & i = j + 4s; \\ e_{8(j+m)+1} \otimes w_{8j+1 \rightarrow 8j+4}, & i = j + 6s; \\ 0, & \text{otherwise.} \end{cases}$$

If  $2s \leq j < 3s$ , then

$$b_{ij} = \begin{cases} w_{8(j+m+1) \rightarrow 8(j+m+1)+1} \otimes e_{8j+2}, & i = j + 3s; \\ -w_{8(j+m+1) \rightarrow 8(j+m+1)+1} \otimes w_{8j+2 \rightarrow 8j+4}, & i = j + 5s; \\ 0, & \text{otherwise.} \end{cases}$$

If  $3s \leq j < 4s$ , then

$$b_{ij} = \begin{cases} e_{8(j+m+1)+2} \otimes w_{8j+3 \rightarrow 8(j+1)}, & i = (j+1)_s; \\ w_{8(j+m+1) \rightarrow 8(j+m+1)+2} \otimes w_{8j+3 \rightarrow 8j+4}, & i = j+4s; \\ 0, & \text{otherwise.} \end{cases}$$

If  $4s \leq j < 5s$ , then

$$b_{ij} = \begin{cases} -w_{8(j+m+1)+2 \rightarrow 8(j+m+1)+3} \otimes w_{8j+4 \rightarrow 8(j+1)}, & i = (j+1)_s; \\ -w_{8(j+m+1) \rightarrow 8(j+m+1)+3} \otimes e_{8j+4}, & i = j+3s; \\ 0, & \text{otherwise.} \end{cases}$$

If  $5s \leq j < 6s$ , then

$$b_{ij} = \begin{cases} -w_{8(j+m)+7 \rightarrow 8(j+m+1)} \otimes w_{8j+5 \rightarrow 8j+6}, & i = j+4s; \\ -e_{8(j+m+1)} \otimes w_{8j+5 \rightarrow 8j+6}, & i = j+5s; \\ 0, & \text{otherwise.} \end{cases}$$

If  $6s \leq j < 7s$ , then

$$b_{ij} = \begin{cases} w_{8(j+m)+7 \rightarrow 8(j+m+1)+5} \otimes e_{8j+6}, & i = j+3s; \\ w_{8(j+m+1) \rightarrow 8(j+m+1)+5} \otimes e_{8j+6}, & i = j+4s; \\ 0, & \text{otherwise.} \end{cases}$$

If  $7s \leq j < 8s$ , then

$$b_{ij} = \begin{cases} -w_{8(j+m+1)+3 \rightarrow 8(j+m+1)+4} \otimes e_{8j+7}, & i = j+5s; \\ -w_{8(j+m+1)+1 \rightarrow 8(j+m+1)+4} \otimes e_{8j+7}, & i = j+6s; \\ 0, & \text{otherwise.} \end{cases}$$

If  $8s \leq j < 9s$ , then

$$b_{ij} = \begin{cases} -w_{8(j+m+1)+5 \rightarrow 8(j+m+1)+6} \otimes e_{8j+7}, & i = j+3s; \\ 0, & \text{otherwise.} \end{cases}$$

(9) If  $r_0 = 8$ , then  $\Omega^8(Z_t^{(21)})$  is described with  $(16s \times 8s)$  matrix, whose entries  $b_{ij}$  have the following form:

If  $0 \leq j < s$ , then

$$b_{ij} = \begin{cases} w_{8(j+m-1)+7 \rightarrow 8(j+m)} \otimes e_{8j}, & i = j; \\ -w_{8(j+m-1)+7 \rightarrow 8(j+m)} \otimes e_{8j}, & i = j+s; \\ e_{8(j+m)} \otimes e_{8j}, & i = j+2s; \\ 0, & \text{otherwise.} \end{cases}$$

If  $s \leq j < 2s$ , then  $b_{ij} = 0$ .

If  $2s \leq j < 3s$ , then

$$b_{ij} = \begin{cases} w_{8(j+m)+1 \rightarrow 8(j+m)+2} \otimes e_{8j+2}, & i = j+3s; \\ e_{8(j+m)+2} \otimes w_{8j+2 \rightarrow 8j+3}, & i = j+4s; \\ 0, & \text{otherwise.} \end{cases}$$

If  $3s \leq j < 4s$ , then  $b_{ij} = 0$ .

If  $4s \leq j < 5s$ , then

$$b_{ij} = \begin{cases} -w_{8(j+m)+3 \rightarrow 8(j+m)+4} \otimes e_{8j+4}, & i = j + 3s; \\ 0, & \text{otherwise.} \end{cases}$$

If  $5s \leq j < 6s$ , then  $b_{ij} = 0$ .

If  $6s \leq j < 7s$ , then

$$b_{ij} = \begin{cases} w_{8(j+m)+5 \rightarrow 8(j+m)+6} \otimes e_{8j+6}, & i = j + 5s; \\ 0, & \text{otherwise.} \end{cases}$$

If  $7s \leq j < 8s$ , then

$$b_{ij} = \begin{cases} e_{8(j+m)+7} \otimes e_{8j+7}, & i = j + 7s; \\ 0, & \text{otherwise.} \end{cases}$$

(10) If  $r_0 = 9$ , then  $\Omega^9(Z_t^{(21)})$  is described with  $(16s \times 8s)$  matrix, whose entries  $b_{ij}$  have the following form:

If  $0 \leq j < s$ , then

$$b_{ij} = \begin{cases} w_{8(j+m)+5 \rightarrow 8(j+m+1)} \otimes e_{8j}, & i = j; \\ -e_{8(j+m+1)} \otimes w_{8j \rightarrow 8j+1}, & i = j + 4s; \\ -w_{8(j+m)+7 \rightarrow 8(j+m+1)} \otimes w_{8j \rightarrow 8j+2}, & i = j + 5s; \\ -w_{8(j+m)+7 \rightarrow 8(j+m+1)} \otimes w_{8j \rightarrow 8j+4}, & i = j + 7s; \\ 0, & \text{otherwise.} \end{cases}$$

If  $s \leq j < 2s$ , then

$$b_{ij} = \begin{cases} e_{8(j+m+1)+1} \otimes w_{8j+1 \rightarrow 8(j+1)}, & i = 3s + (j+1)_s; \\ w_{8(j+m)+7 \rightarrow 8(j+m+1)+1} \otimes w_{8j+1 \rightarrow 8j+2}, & i = j + 4s; \\ w_{8(j+m)+7 \rightarrow 8(j+m+1)+1} \otimes w_{8j+1 \rightarrow 8j+4}, & i = j + 6s; \\ 0, & \text{otherwise.} \end{cases}$$

If  $2s \leq j < 3s$ , then

$$b_{ij} = \begin{cases} -w_{8(j+m+1)+1 \rightarrow 8(j+m+1)+2} \otimes w_{8j+2 \rightarrow 8(j+1)}, & i = 3s + (j+1)_s; \\ -w_{8(j+m)+7 \rightarrow 8(j+m+1)+2} \otimes e_{8j+2}, & i = j + 3s; \\ -w_{8(j+m)+7 \rightarrow 8(j+m+1)+2} \otimes w_{8j+2 \rightarrow 8j+4}, & i = j + 5s; \\ 0, & \text{otherwise.} \end{cases}$$

If  $3s \leq j < 4s$ , then

$$b_{ij} = \begin{cases} e_{8(j+m+1)+3} \otimes w_{8j+3 \rightarrow 8(j+1)}, & i = s + (j+1)_s; \\ w_{8(j+m+1)+1 \rightarrow 8(j+m+1)+3} \otimes w_{8j+3 \rightarrow 8(j+1)}, & i = 3s + (j+1)_s; \\ w_{8(j+m)+7 \rightarrow 8(j+m+1)+3} \otimes w_{8j+3 \rightarrow 8j+4}, & i = j + 4s; \\ 0, & \text{otherwise.} \end{cases}$$



If  $4s \leq j < 5s$ , then

$$b_{ij} = \begin{cases} -w_{8(j+m+1)+3 \rightarrow 8(j+m+1)+4} \otimes w_{8j+4 \rightarrow 8(j+1)}, & i = s + (j+1)_s; \\ -w_{8(j+m+1)+1 \rightarrow 8(j+m+1)+4} \otimes w_{8j+4 \rightarrow 8(j+1)}, & i = 3s + (j+1)_s; \\ -w_{8(j+m)+7 \rightarrow 8(j+m+1)+4} \otimes e_{8j+4}, & i = j + 3s; \\ 0, & \text{otherwise.} \end{cases}$$

If  $5s \leq j < 6s$ , then

$$b_{ij} = \begin{cases} -e_{8(j+m+1)+5} \otimes w_{8j+5 \rightarrow 8(j+1)}, & i = (j+1)_s; \\ -w_{8(j+m)+7 \rightarrow 8(j+m+1)+5} \otimes w_{8j+5 \rightarrow 8j+6}, & i = j + 5s; \\ 0, & \text{otherwise.} \end{cases}$$

If  $6s \leq j < 7s$ , then

$$b_{ij} = \begin{cases} w_{8(j+m+1)+5 \rightarrow 8(j+m+1)+6} \otimes w_{8j+6 \rightarrow 8(j+1)}, & i = (j+1)_s; \\ w_{8(j+m)+7 \rightarrow 8(j+m+1)+6} \otimes e_{8j+6}, & i = j + 4s; \\ 0, & \text{otherwise.} \end{cases}$$

If  $7s \leq j < 8s$ , then

$$b_{ij} = \begin{cases} -w_{8(j+m+1)+1 \rightarrow 8(j+m+1)+7} \otimes w_{8j+7 \rightarrow 8(j+1)}, & i = 3s + (j+1)_s; \\ e_{8(j+m+1)+7} \otimes w_{8j+7 \rightarrow 8(j+1)+6}, & i = 10s + (j+1)_s; \\ w_{8(j+m+1)+2 \rightarrow 8(j+m+1)+7} \otimes e_{8j+7}, & i = j + 5s; \\ -w_{8(j+m+1)+4 \rightarrow 8(j+m+1)+7} \otimes e_{8j+7}, & i = j + 6s; \\ 0, & \text{otherwise.} \end{cases}$$

(11) If  $r_0 = 10$ , then  $\Omega^{10}(Z_t^{(21)})$  is described with  $(19s \times 9s)$  matrix, whose entries  $b_{ij}$  have the following form:

If  $0 \leq j < s$ , then

$$b_{ij} = \begin{cases} e_{8(j+m)+1} \otimes w_{8j \rightarrow 8j+1}, & i = j + 4s; \\ 0, & \text{otherwise.} \end{cases}$$

If  $s \leq j < 2s$ , then

$$b_{ij} = \begin{cases} w_{8(j+m-1)+7 \rightarrow 8(j+m)+5} \otimes e_{8j}, & i = j - s; \\ -w_{8(j+m) \rightarrow 8(j+m)+5} \otimes e_{8j}, & i = j + s; \\ e_{8(j+m)+5} \otimes w_{8j \rightarrow 8j+5}, & i = j + 9s; \\ 0, & \text{otherwise.} \end{cases}$$

If  $2s \leq j < 3s$ , then  $b_{ij} = 0$ .

If  $3s \leq j < 4s$ , then

$$b_{ij} = \begin{cases} w_{8(j+m)+2 \rightarrow 8(j+m)+3} \otimes e_{8j+2}, & i = j + 2s; \\ -e_{8(j+m)+3} \otimes w_{8j+2 \rightarrow 8j+3}, & i = j + 3s; \\ 0, & \text{otherwise.} \end{cases}$$

If  $4s \leq j < 5s$ , then  $b_{ij} = 0$ .

If  $5s \leq j < 6s$ , then

$$b_{ij} = \begin{cases} -w_{8(j+m)+4 \rightarrow 8(j+m)+7} \otimes e_{8j+4}, & i = j + 3s; \\ 0, & \text{otherwise.} \end{cases}$$

If  $6s \leq j < 7s$ , then  $b_{ij} = 0$ .

If  $7s \leq j < 8s$ , then

$$b_{ij} = \begin{cases} -e_{8(j+m)+7} \otimes w_{8j+6 \rightarrow 8(j+1)}, & i = (j+1)_s; \\ -w_{8(j+m)+2 \rightarrow 8(j+m)+7} \otimes e_{8j+6}, & i = j + 6s; \\ w_{8(j+m)+5 \rightarrow 8(j+m)+7} \otimes e_{8j+6}, & i = j + 8s; \\ e_{8(j+m)+7} \otimes w_{8j+6 \rightarrow 8j+7}, & i = j + 10s; \\ 0, & \text{otherwise.} \end{cases}$$

If  $8s \leq j < 9s$ , then

$$b_{ij} = \begin{cases} -w_{8(j+m)+7 \rightarrow 8(j+m+1)} \otimes w_{8j+7 \rightarrow 8(j+1)}, & i = (j+1)_s; \\ -w_{8(j+m)+7 \rightarrow 8(j+m+1)} \otimes e_{8j+7}, & i = j + 8s; \\ w_{8(j+m)+7 \rightarrow 8(j+m+1)} \otimes e_{8j+7}, & i = j + 9s; \\ -e_{8(j+m+1)} \otimes e_{8j+7}, & i = j + 10s; \\ 0, & \text{otherwise.} \end{cases}$$

(12) If  $r_0 = 11$ , then  $\Omega^{11}(Z_t^{(21)})$  is described with  $(18s \times 8s)$  matrix, whose entries  $b_{ij}$  have the following form:

If  $0 \leq j < s$ , then

$$b_{ij} = \begin{cases} -w_{8(j+m)+2 \rightarrow 8(j+m)+7} \otimes e_{8j}, & i = j; \\ w_{8(j+m)+1 \rightarrow 8(j+m)+7} \otimes e_{8j}, & i = j + 3s; \\ w_{8(j+m)+5 \rightarrow 8(j+m)+7} \otimes e_{8j}, & i = j + 4s; \\ e_{8(j+m)+7} \otimes w_{8j \rightarrow 8j+3}, & i = j + 7s; \\ -e_{8(j+m)+7} \otimes w_{8j \rightarrow 8j+4}, & i = j + 8s; \\ 0, & \text{otherwise.} \end{cases}$$

If  $s \leq j < 2s$ , then

$$b_{ij} = \begin{cases} w_{8(j+m+1)+1 \rightarrow 8(j+m+1)+2} \otimes w_{8j+1 \rightarrow 8(j+1)}, & i = 3s + (j+1)_s; \\ -w_{8(j+m)+7 \rightarrow 8(j+m+1)+2} \otimes e_{8j+1}, & i = j + 4s; \\ w_{8(j+m)+7 \rightarrow 8(j+m+1)+2} \otimes w_{8j+1 \rightarrow 8j+4}, & i = j + 7s; \\ w_{8(j+m+1) \rightarrow 8(j+m+1)+2} \otimes w_{8j+1 \rightarrow 8j+4}, & i = j + 8s; \\ 0, & \text{otherwise.} \end{cases}$$

If  $2s \leq j < 3s$ , then

$$b_{ij} = \begin{cases} w_{8(j+m+1)+2 \rightarrow 8(j+m+1)+3} \otimes w_{8j+2 \rightarrow 8(j+1)}, & i = (j+1)_s; \\ -w_{8(j+m+1)+1 \rightarrow 8(j+m+1)+3} \otimes w_{8j+2 \rightarrow 8(j+1)}, & i = 3s + (j+1)_s; \\ -w_{8(j+m+1) \rightarrow 8(j+m+1)+3} \otimes e_{8j+2}, & i = j + 4s; \\ -w_{8(j+m)+7 \rightarrow 8(j+m+1)+3} \otimes w_{8j+2 \rightarrow 8j+4}, & i = j + 6s; \\ -w_{8(j+m+1) \rightarrow 8(j+m+1)+3} \otimes w_{8j+2 \rightarrow 8j+4}, & i = j + 7s; \\ 0, & \text{otherwise.} \end{cases}$$

If  $3s \leq j < 4s$ , then

$$b_{ij} = \begin{cases} -w_{8(j+m+1)+2 \rightarrow 8(j+m+1)+4} \otimes w_{8j+3 \rightarrow 8(j+1)}, & i = (j+1)_s; \\ e_{8(j+m+1)+4} \otimes w_{8j+3 \rightarrow 8(j+1)}, & i = 2s + (j+1)_s; \\ w_{8(j+m+1)+1 \rightarrow 8(j+m+1)+4} \otimes w_{8j+3 \rightarrow 8(j+1)}, & i = 3s + (j+1)_s; \\ w_{8(j+m)+7 \rightarrow 8(j+m+1)+4} \otimes w_{8j+3 \rightarrow 8j+4}, & i = j + 5s; \\ w_{8(j+m+1) \rightarrow 8(j+m+1)+4} \otimes w_{8j+3 \rightarrow 8j+4}, & i = j + 6s; \\ 0, & \text{otherwise.} \end{cases}$$

If  $4s \leq j < 5s$ , then

$$b_{ij} = \begin{cases} w_{8(j+m)+7 \rightarrow 8(j+m+1)+5} \otimes e_{8j+4}, & i = j + 4s; \\ w_{8(j+m+1) \rightarrow 8(j+m+1)+5} \otimes e_{8j+4}, & i = j + 5s; \\ 0, & \text{otherwise.} \end{cases}$$

If  $5s \leq j < 6s$ , then

$$b_{ij} = \begin{cases} -e_{8(j+m+1)+6} \otimes w_{8j+5 \rightarrow 8(j+1)}, & i = s + (j+1)_s; \\ -w_{8(j+m)+7 \rightarrow 8(j+m+1)+6} \otimes w_{8j+5 \rightarrow 8j+6}, & i = j + 7s; \\ -w_{8(j+m+1) \rightarrow 8(j+m+1)+6} \otimes w_{8j+5 \rightarrow 8j+6}, & i = j + 8s; \\ 0, & \text{otherwise.} \end{cases}$$

If  $6s \leq j < 7s$ , then

$$b_{ij} = \begin{cases} -w_{8(j+m)+7 \rightarrow 8(j+m+1)+1} \otimes e_{8j+6}, & i = j + 6s; \\ -w_{8(j+m+1) \rightarrow 8(j+m+1)+1} \otimes e_{8j+6}, & i = j + 7s; \\ 0, & \text{otherwise.} \end{cases}$$

If  $7s \leq j < 8s$ , then

$$b_{ij} = \begin{cases} -w_{8(j+m+1)+1 \rightarrow 8(j+m+2)} \otimes w_{8j+7 \rightarrow 8(j+1)}, & i = 3s + (j+1)_s; \\ e_{8(j+m+2)} \otimes w_{8j+7 \rightarrow 8(j+1)+2}, & i = 6s + (j+1)_s; \\ w_{8(j+m+1)+7 \rightarrow 8(j+m+2)} \otimes w_{8j+7 \rightarrow 8(j+1)+4}, & i = 8s + (j+1)_s; \\ e_{8(j+m+2)} \otimes w_{8j+7 \rightarrow 8(j+1)+4}, & i = 9s + (j+1)_s; \\ w_{8(j+m+1)+7 \rightarrow 8(j+m+2)} \otimes w_{8j+7 \rightarrow 8(j+1)+5}, & i = 10s + (j+1)_s; \\ e_{8(j+m+2)} \otimes w_{8j+7 \rightarrow 8(j+1)+5}, & i = 11s + (j+1)_s; \\ w_{8(j+m+1)+5 \rightarrow 8(j+m+2)} \otimes e_{8j+7}, & i = j + 7s; \\ 0, & \text{otherwise.} \end{cases}$$

(13) If  $r_0 = 12$ , then  $\Omega^{12}(Z_t^{(21)})$  is described with  $(19s \times 10s)$  matrix, whose entries  $b_{ij}$  have the following form:

If  $0 \leq j < s$ , then

$$b_{ij} = \begin{cases} w_{8(j+m) \rightarrow 8(j+m)+2} \otimes e_{8j}, & i = j + s; \\ w_{8(j+m-1)+7 \rightarrow 8(j+m)+2} \otimes e_{8j}, & i = j + 2s; \\ e_{8(j+m)+2} \otimes w_{8j \rightarrow 8j+1}, & i = j + 3s; \\ e_{8(j+m)+2} \otimes w_{8j \rightarrow 8j+5}, & i = j + 10s; \\ 0, & \text{otherwise.} \end{cases}$$

If  $s \leq j < 2s$ , then

$$b_{ij} = \begin{cases} -w_{8(j+m-1)+7 \rightarrow 8(j+m)+6} \otimes e_{8j}, & i = j + s; \\ w_{8(j+m)+5 \rightarrow 8(j+m)+6} \otimes w_{8j \rightarrow 8j+4}, & i = j + 7s; \\ -e_{8(j+m)+6} \otimes w_{8j \rightarrow 8j+5}, & i = j + 10s; \\ 0, & \text{otherwise.} \end{cases}$$

If  $2s \leq j < 3s$ , then

$$b_{ij} = \begin{cases} w_{8(j+m)+2 \rightarrow 8(j+m)+3} \otimes e_{8j+1}, & i = j + s; \\ 0, & \text{otherwise.} \end{cases}$$

If  $3s \leq j < 4s$ , then

$$b_{ij} = \begin{cases} w_{8(j+m)+3 \rightarrow 8(j+m)+4} \otimes e_{8j+2}, & i = j + s; \\ -e_{8(j+m)+4} \otimes w_{8j+2 \rightarrow 8j+3}, & i = j + 3s; \\ 0, & \text{otherwise.} \end{cases}$$

If  $4s \leq j < 5s$ , then

$$b_{ij} = \begin{cases} e_{8(j+m)+7} \otimes w_{8j+3 \rightarrow 8(j+1)}, & i = 2s + (j+1)_s; \\ 0, & \text{otherwise.} \end{cases}$$

If  $5s \leq j < 6s$ , then

$$b_{ij} = \begin{cases} e_{8(j+m+1)} \otimes w_{8j+4 \rightarrow 8(j+1)}, & i = s + (j+1)_s; \\ w_{8(j+m)+7 \rightarrow 8(j+m+1)} \otimes w_{8j+4 \rightarrow 8(j+1)}, & i = 2s + (j+1)_s; \\ -w_{8(j+m)+5 \rightarrow 8(j+m+1)} \otimes e_{8j+4}, & i = j + 3s; \\ 0, & \text{otherwise.} \end{cases}$$

If  $6s \leq j < 7s$ , then

$$b_{ij} = \begin{cases} -e_{8(j+m)+7} \otimes w_{8j+5 \rightarrow 8(j+1)}, & i = (j+1)_s; \\ 0, & \text{otherwise.} \end{cases}$$

If  $7s \leq j < 8s$ , then

$$b_{ij} = \begin{cases} w_{8(j+m)+7 \rightarrow 8(j+m+1)} \otimes w_{8j+6 \rightarrow 8(j+1)}, & i = 2s + (j+1)_s; \\ -w_{8(j+m)+6 \rightarrow 8(j+m+1)} \otimes e_{8j+6}, & i = j + 6s; \\ e_{8(j+m+1)} \otimes w_{8j+6 \rightarrow 8j+7}, & i = j + 11s; \\ 0, & \text{otherwise.} \end{cases}$$

If  $8s \leq j < 9s$ , then

$$b_{ij} = \begin{cases} w_{8(j+m+1) \rightarrow 8(j+m+1)+1} \otimes w_{8j+7 \rightarrow 8(j+1)}, & i = s + (j+1)_s; \\ w_{8(j+m)+7 \rightarrow 8(j+m+1)+1} \otimes w_{8j+7 \rightarrow 8(j+1)}, & i = 2s + (j+1)_s; \\ 0, & \text{otherwise.} \end{cases}$$

If  $9s \leq j < 10s$ , then

$$b_{ij} = \begin{cases} -w_{8(j+m)+7 \rightarrow 8(j+m+1)+5} \otimes w_{8j+7 \rightarrow 8(j+1)}, & i = 2s + (j+1)_s; \\ w_{8(j+m)+7 \rightarrow 8(j+m+1)+5} \otimes e_{8j+7}, & i = j + 7s; \\ -w_{8(j+m+1) \rightarrow 8(j+m+1)+5} \otimes e_{8j+7}, & i = j + 9s; \\ 0, & \text{otherwise.} \end{cases}$$

(14) If  $r_0 = 13$ , then  $\Omega^{13}(Z_t^{(21)})$  is described with  $(18s \times 11s)$  matrix, whose entries  $b_{ij}$  have the following form:

If  $0 \leq j < s$ , then

$$b_{ij} = \begin{cases} w_{8(j+m)+5 \rightarrow 8(j+m)+7} \otimes e_{8j}, & i = j + 3s; \\ e_{8(j+m)+7} \otimes w_{8j \rightarrow 8j+2}, & i = j + 5s; \\ e_{8(j+m)+7} \otimes w_{8j \rightarrow 8j+5}, & i = j + 9s; \\ 0, & \text{otherwise.} \end{cases}$$

If  $s \leq j < 2s$ , then

$$b_{ij} = \begin{cases} -w_{8(j+m)+6 \rightarrow 8(j+m+1)} \otimes e_{8j}, & i = j + s; \\ e_{8(j+m+1)} \otimes w_{8j \rightarrow 8j+3}, & i = j + 6s; \\ -e_{8(j+m+1)} \otimes w_{8j \rightarrow 8j+4}, & i = j + 7s; \\ 0, & \text{otherwise.} \end{cases}$$

If  $2s \leq j < 3s$ , then

$$b_{ij} = \begin{cases} w_{8(j+m+1)+2 \rightarrow 8(j+m+1)+3} \otimes w_{8j+1 \rightarrow 8(j+1)}, & i = (j+1)_s; \\ -e_{8(j+m+1)+3} \otimes w_{8j+1 \rightarrow 8(j+1)}, & i = s + (j+1)_s; \\ w_{8(j+m)+7 \rightarrow 8(j+m+1)+3} \otimes w_{8j+1 \rightarrow 8j+2}, & i = j + 3s; \\ 0, & \text{otherwise.} \end{cases}$$

If  $3s \leq j < 4s$ , then

$$b_{ij} = \begin{cases} -w_{8(j+m+1)+2 \rightarrow 8(j+m+1)+4} \otimes w_{8j+2 \rightarrow 8(j+1)}, & i = (j+1)_s; \\ w_{8(j+m+1)+3 \rightarrow 8(j+m+1)+4} \otimes w_{8j+2 \rightarrow 8(j+1)}, & i = s + (j+1)_s; \\ -w_{8(j+m)+7 \rightarrow 8(j+m+1)+4} \otimes e_{8j+2}, & i = j + 2s; \\ 0, & \text{otherwise.} \end{cases}$$

If  $4s \leq j < 5s$ , then

$$b_{ij} = \begin{cases} w_{8(j+m)+7 \rightarrow 8(j+m+1)+5} \otimes e_{8j+3}, & i = j + 2s; \\ w_{8(j+m+1) \rightarrow 8(j+m+1)+5} \otimes e_{8j+3}, & i = j + 3s; \\ -w_{8(j+m+1) \rightarrow 8(j+m+1)+5} \otimes w_{8j+3 \rightarrow 8j+4}, & i = j + 4s; \\ 0, & \text{otherwise.} \end{cases}$$

If  $5s \leq j < 6s$ , then

$$b_{ij} = \begin{cases} -e_{8(j+m+1)+6} \otimes w_{8j+4 \rightarrow 8j+7}, & i = j + 9s; \\ 0, & \text{otherwise.} \end{cases}$$

If  $6s \leq j < 7s$ , then  $b_{ij} = 0$ .

If  $7s \leq j < 8s$ , then

$$b_{ij} = \begin{cases} -w_{8(j+m+1) \rightarrow 8(j+m+1)+1} \otimes e_{8j+5}, & i = j + 3s; \\ 0, & \text{otherwise.} \end{cases}$$

If  $8s \leq j < 9s$ , then

$$b_{ij} = \begin{cases} -e_{8(j+m+1)+2} \otimes w_{8j+6 \rightarrow 8(j+1)}, & i = (j+1)_s; \\ w_{8(j+m+1)+1 \rightarrow 8(j+m+1)+2} \otimes w_{8j+6 \rightarrow 8j+7}, & i = j + 8s; \\ 0, & \text{otherwise.} \end{cases}$$

If  $9s \leq j < 10s$ , then

$$b_{ij} = \begin{cases} -w_{8(j+m)+7 \rightarrow 8(j+m+1)+5} \otimes e_{8j+6}, & i = j + 2s; \\ 0, & \text{otherwise.} \end{cases}$$

If  $10s \leq j < 11s$ , then

$$b_{ij} = \begin{cases} w_{8(j+m+1)+5 \rightarrow 8(j+m+1)+7} \otimes w_{8j+7 \rightarrow 8(j+1)}, & i = 3s + (j+1)_s; \\ e_{8(j+m+1)+7} \otimes w_{8j+7 \rightarrow 8(j+1)+2}, & i = 5s + (j+1)_s; \\ e_{8(j+m+1)+7} \otimes w_{8j+7 \rightarrow 8(j+1)+5}, & i = 9s + (j+1)_s; \\ -w_{8(j+m+1)+6 \rightarrow 8(j+m+1)+7} \otimes e_{8j+7}, & i = j + 4s; \\ 0, & \text{otherwise.} \end{cases}$$

(15) If  $r_0 = 14$ , then  $\Omega^{14}(Z_t^{(21)})$  is described with  $(20s \times 11s)$  matrix, whose entries  $b_{ij}$  have the following form:

If  $0 \leq j < s$ , then

$$b_{ij} = \begin{cases} -w_{8(j+m-1)+7 \rightarrow 8(j+m)+5} \otimes e_{8j}, & i = j; \\ 0, & \text{otherwise.} \end{cases}$$

If  $s \leq j < 2s$ , then

$$b_{ij} = \begin{cases} -w_{8(j+m) \rightarrow 8(j+m)+3} \otimes e_{8j}, & i = j + s; \\ -w_{8(j+m)+1 \rightarrow 8(j+m)+3} \otimes w_{8j \rightarrow 8j+3}, & i = j + 7s; \\ e_{8(j+m)+3} \otimes w_{8j \rightarrow 8j+5}, & i = j + 11s; \\ 0, & \text{otherwise.} \end{cases}$$

If  $2s \leq j < 3s$ , then

$$b_{ij} = \begin{cases} w_{8(j+m) \rightarrow 8(j+m)+1} \otimes e_{8j}, & i = j; \\ 0, & \text{otherwise.} \end{cases}$$

If  $3s \leq j < 4s$ , then  $b_{ij} = 0$ .

If  $4s \leq j < 5s$ , then

$$b_{ij} = \begin{cases} -e_{8(j+m)+7} \otimes w_{8j+2 \rightarrow 8(j+1)}, & i = (j+1)_s; \\ -w_{8(j+m)+6 \rightarrow 8(j+m)+7} \otimes e_{8j+2}, & i = j+2s; \\ -w_{8(j+m)+5 \rightarrow 8(j+m)+7} \otimes w_{8j+2 \rightarrow 8j+3}, & i = j+3s; \\ w_{8(j+m)+6 \rightarrow 8(j+m)+7} \otimes w_{8j+2 \rightarrow 8j+4}, & i = j+6s; \\ 0, & \text{otherwise.} \end{cases}$$

If  $5s \leq j < 6s$ , then

$$b_{ij} = \begin{cases} e_{8(j+m+1)} \otimes w_{8j+3 \rightarrow 8(j+1)}, & i = 2s + (j+1)_s; \\ -w_{8(j+m)+5 \rightarrow 8(j+m)+1} \otimes e_{8j+3}, & i = j+2s; \\ w_{8(j+m)+6 \rightarrow 8(j+m)+1} \otimes w_{8j+3 \rightarrow 8j+4}, & i = j+5s; \\ 0, & \text{otherwise.} \end{cases}$$

If  $6s \leq j < 7s$ , then  $b_{ij} = 0$ .

If  $7s \leq j < 8s$ , then

$$b_{ij} = \begin{cases} -w_{8(j+m)+7 \rightarrow 8(j+m)+1} \otimes w_{8j+5 \rightarrow 8(j+1)}, & i = (j+1)_s; \\ -e_{8(j+m+1)} \otimes w_{8j+5 \rightarrow 8(j+1)}, & i = s + (j+1)_s; \\ -w_{8(j+m)+1 \rightarrow 8(j+m)+1} \otimes e_{8j+5}, & i = j+6s; \\ 0, & \text{otherwise.} \end{cases}$$

If  $8s \leq j < 9s$ , then

$$b_{ij} = \begin{cases} w_{8(j+m)+2 \rightarrow 8(j+m)+7} \otimes e_{8j+6}, & i = j+6s; \\ -w_{8(j+m)+5 \rightarrow 8(j+m)+7} \otimes e_{8j+6}, & i = j+8s; \\ -e_{8(j+m)+7} \otimes w_{8j+6 \rightarrow 8j+7}, & i = j+9s; \\ 0, & \text{otherwise.} \end{cases}$$

If  $9s \leq j < 10s$ , then

$$b_{ij} = \begin{cases} -w_{8(j+m+1)+1 \rightarrow 8(j+m+1)+2} \otimes w_{8j+7 \rightarrow 8(j+1)+3}, & i = 8s + (j+1)_s; \\ 0, & \text{otherwise.} \end{cases}$$

If  $10s \leq j < 11s$ , then

$$b_{ij} = \begin{cases} e_{8(j+m+1)+6} \otimes w_{8j+7 \rightarrow 8(j+1)+2}, & i = 6s + (j+1)_s; \\ w_{8(j+m+1)+5 \rightarrow 8(j+m+1)+6} \otimes w_{8j+7 \rightarrow 8(j+1)+3}, & i = 7s + (j+1)_s; \\ -e_{8(j+m+1)+6} \otimes w_{8j+7 \rightarrow 8(j+1)+4}, & i = 10s + (j+1)_s; \\ w_{8(j+m)+7 \rightarrow 8(j+m+1)+6} \otimes e_{8j+7}, & i = j+7s; \\ 0, & \text{otherwise.} \end{cases}$$

(16) If  $r_0 = 15$ , then  $\Omega^{15}(Z_t^{(21)})$  is described with  $(18s \times 13s)$  matrix, whose entries  $b_{ij}$  have the following form:

If  $0 \leq j < s$ , then

$$b_{ij} = \begin{cases} -w_{8(j+m)+3 \rightarrow 8(j+m)+7} \otimes e_{8j}, & i = j; \\ w_{8(j+m)+5 \rightarrow 8(j+m)+7} \otimes e_{8j}, & i = j + 4s; \\ -e_{8(j+m)+7} \otimes w_{8j \rightarrow 8j+1}, & i = j + 5s; \\ e_{8(j+m)+7} \otimes w_{8j \rightarrow 8j+4}, & i = j + 9s; \\ 0, & \text{otherwise.} \end{cases}$$

If  $s \leq j < 2s$ , then

$$b_{ij} = \begin{cases} -w_{8(j+m)+1 \rightarrow 8(j+m+1)} \otimes e_{8j}, & i = j + 2s; \\ e_{8(j+m+1)} \otimes w_{8j \rightarrow 8j+2}, & i = j + 6s; \\ e_{8(j+m+1)} \otimes w_{8j \rightarrow 8j+5}, & i = j + 10s; \\ 0, & \text{otherwise.} \end{cases}$$

If  $2s \leq j < 3s$ , then

$$b_{ij} = \begin{cases} w_{8(j+m+1)+3 \rightarrow 8(j+m+1)+4} \otimes w_{8j+1 \rightarrow 8(j+1)}, & i = (j+1)_s; \\ -e_{8(j+m+1)+4} \otimes w_{8j+1 \rightarrow 8(j+1)}, & i = 2s + (j+1)_s; \\ w_{8(j+m+1)+1 \rightarrow 8(j+m+1)+4} \otimes w_{8j+1 \rightarrow 8(j+1)}, & i = 3s + (j+1)_s; \\ 0, & \text{otherwise.} \end{cases}$$

If  $3s \leq j < 4s$ , then

$$b_{ij} = \begin{cases} w_{8(j+m+1) \rightarrow 8(j+m+1)+5} \otimes e_{8j+2}, & i = j + 4s; \\ 0, & \text{otherwise.} \end{cases}$$

If  $4s \leq j < 5s$ , then

$$b_{ij} = \begin{cases} e_{8(j+m+1)+6} \otimes w_{8j+3 \rightarrow 8(j+1)}, & i = s + (j+1)_s; \\ w_{8(j+m)+7 \rightarrow 8(j+m+1)+6} \otimes w_{8j+3 \rightarrow 8j+4}, & i = j + 5s; \\ 0, & \text{otherwise.} \end{cases}$$

If  $5s \leq j < 6s$ , then  $b_{ij} = 0$ .

If  $6s \leq j < 7s$ , then

$$b_{ij} = \begin{cases} w_{8(j+m+1)+1 \rightarrow 8(j+m+1)+2} \otimes w_{8j+4 \rightarrow 8(j+1)}, & i = 3s + (j+1)_s; \\ 0, & \text{otherwise.} \end{cases}$$

If  $7s \leq j < 8s$ , then

$$b_{ij} = \begin{cases} w_{8(j+m)+7 \rightarrow 8(j+m+1)+2} \otimes e_{8j+5}, & i = j + 3s; \\ w_{8(j+m+1) \rightarrow 8(j+m+1)+2} \otimes e_{8j+5}, & i = j + 4s; \\ 0, & \text{otherwise.} \end{cases}$$

If  $8s \leq j < 9s$ , then

$$b_{ij} = \begin{cases} -e_{8(j+m+1)+5} \otimes w_{8j+5 \rightarrow 8(j+1)}, & i = 4s + (j+1)_s; \\ 0, & \text{otherwise.} \end{cases}$$



If  $9s \leq j < 10s$ , then

$$b_{ij} = \begin{cases} -e_{8(j+m+1)+3} \otimes w_{8j+6 \rightarrow 8(j+1)}, & i = (j+1)_s; \\ w_{8(j+m+1) \rightarrow 8(j+m+1)+3} \otimes e_{8j+6}, & i = j+3s; \\ w_{8(j+m)+7 \rightarrow 8(j+m+1)+3} \otimes e_{8j+6}, & i = j+4s; \\ -w_{8(j+m+1)+2 \rightarrow 8(j+m+1)+3} \otimes w_{8j+6 \rightarrow 8j+7}, & i = j+5s; \\ 0, & \text{otherwise.} \end{cases}$$

If  $10s \leq j < 11s$ , then  $b_{ij} = 0$ .

If  $11s \leq j < 12s$ , then

$$b_{ij} = \begin{cases} w_{8(j+m+1)+3 \rightarrow 8(j+m+1)+7} \otimes e_{8j+7}, & i = j+4s; \\ 0, & \text{otherwise.} \end{cases}$$

If  $12s \leq j < 13s$ , then

$$b_{ij} = \begin{cases} e_{8(j+m+2)} \otimes w_{8j+7 \rightarrow 8(j+1)+2}, & i = 7s + (j+1)_s; \\ 0, & \text{otherwise.} \end{cases}$$

(17) If  $r_0 = 16$ , then  $\Omega^{16}(Z_t^{(21)})$  is described with  $(19s \times 14s)$  matrix, whose entries  $b_{ij}$  have the following form:

If  $0 \leq j < s$ , then

$$b_{ij} = \begin{cases} w_{8(j+m-1)+7 \rightarrow 8(j+m)+2} \otimes e_{8j}, & i = j; \\ w_{8(j+m)+1 \rightarrow 8(j+m)+2} \otimes w_{8j \rightarrow 8j+2}, & i = j+6s; \\ 0, & \text{otherwise.} \end{cases}$$

If  $s \leq j < 2s$ , then

$$b_{ij} = \begin{cases} w_{8(j+m-1)+7 \rightarrow 8(j+m)+4} \otimes e_{8j}, & i = j-s; \\ -w_{8(j+m) \rightarrow 8(j+m)+4} \otimes e_{8j}, & i = j; \\ -w_{8(j+m-1)+7 \rightarrow 8(j+m)+4} \otimes e_{8j}, & i = j+s; \\ 2w_{8(j+m)+1 \rightarrow 8(j+m)+4} \otimes w_{8j \rightarrow 8j+2}, & i = j+5s; \\ w_{8(j+m)+2 \rightarrow 8(j+m)+4} \otimes w_{8j \rightarrow 8j+3}, & i = j+6s; \\ e_{8(j+m)+4} \otimes w_{8j \rightarrow 8j+5}, & i = j+10s; \\ 0, & \text{otherwise.} \end{cases}$$

If  $2s \leq j < 3s$ , then

$$b_{ij} = \begin{cases} -e_{8(j+m)+6} \otimes w_{8j \rightarrow 8j+1}, & i = j+2s; \\ 0, & \text{otherwise.} \end{cases}$$

If  $3s \leq j < 4s$ , then

$$b_{ij} = \begin{cases} e_{8(j+m)+5} \otimes w_{8j \rightarrow 8j+5}, & i = j+9s; \\ 0, & \text{otherwise.} \end{cases}$$

If  $4s \leq j < 5s$ , then

$$b_{ij} = \begin{cases} -e_{8(j+m)+7} \otimes w_{8j+1 \rightarrow 8(j+1)}, & i = (j+1)_s; \\ w_{8(j+m)+4 \rightarrow 8(j+m)+7} \otimes e_{8j+1}, & i = j-s; \\ -w_{8(j+m)+6 \rightarrow 8(j+m)+7} \otimes e_{8j+1}, & i = j; \\ 0, & \text{otherwise.} \end{cases}$$

If  $5s \leq j < 6s$ , then

$$b_{ij} = \begin{cases} -e_{8(j+m+1)} \otimes w_{8j+2 \rightarrow 8(j+1)}, & i = s + (j+1)_s; \\ -w_{8(j+m)+7 \rightarrow 8(j+m+1)} \otimes w_{8j+2 \rightarrow 8(j+1)}, & i = 2s + (j+1)_s; \\ -w_{8(j+m)+1 \rightarrow 8(j+m+1)} \otimes e_{8j+2}, & i = j+s; \\ 0, & \text{otherwise.} \end{cases}$$

If  $6s \leq j < 7s$ , then

$$b_{ij} = \begin{cases} e_{8(j+m)+7} \otimes w_{8j+3 \rightarrow 8(j+1)}, & i = (j+1)_s; \\ -w_{8(j+m)+3 \rightarrow 8(j+m)+7} \otimes w_{8j+3 \rightarrow 8j+4}, & i = j+3s; \\ 0, & \text{otherwise.} \end{cases}$$

If  $7s \leq j < 8s$ , then

$$b_{ij} = \begin{cases} -w_{8(j+m)+3 \rightarrow 8(j+m+1)} \otimes e_{8j+4}, & i = j+2s; \\ 0, & \text{otherwise.} \end{cases}$$

If  $8s \leq j < 9s$ , then

$$b_{ij} = \begin{cases} w_{8(j+m)+2 \rightarrow 8(j+m)+7} \otimes e_{8j+5}, & i = j+2s; \\ 0, & \text{otherwise.} \end{cases}$$

If  $9s \leq j < 10s$ , then

$$b_{ij} = \begin{cases} -w_{8(j+m)+3 \rightarrow 8(j+m)+7} \otimes e_{8j+6}, & i = j+4s; \\ 0, & \text{otherwise.} \end{cases}$$

If  $10s \leq j < 12s$ , then  $b_{ij} = 0$ .

If  $12s \leq j < 13s$ , then

$$b_{ij} = \begin{cases} e_{8(j+m+1)+3} \otimes w_{8j+7 \rightarrow 8(j+1)+4}, & i = 9s + (j+1)_s; \\ -e_{8(j+m+1)+3} \otimes w_{8j+7 \rightarrow 8(j+1)+6}, & i = 13s + (j+1)_s; \\ -w_{8(j+m)+7 \rightarrow 8(j+m+1)+3} \otimes e_{8j+7}, & i = j+4s; \\ 0, & \text{otherwise.} \end{cases}$$

If  $13s \leq j < 14s$ , then

$$b_{ij} = \begin{cases} -e_{8(j+m+1)+1} \otimes w_{8j+7 \rightarrow 8(j+1)+2}, & i = 6s + (j+1)_s; \\ 0, & \text{otherwise.} \end{cases}$$

(18) If  $r_0 = 17$ , then  $\Omega^{17}(Z_t^{(21)})$  is described with  $(18s \times 16s)$  matrix, whose entries  $b_{ij}$  have the following form:

If  $0 \leq j < s$ , then

$$b_{ij} = \begin{cases} w_{8(j+m)+4 \rightarrow 8(j+m)+7} \otimes e_{8j}, & i = j + s; \\ e_{8(j+m)+7} \otimes w_{8j \rightarrow 8j+1}, & i = j + 4s; \\ e_{8(j+m)+7} \otimes w_{8j \rightarrow 8j+5}, & i = j + 10s; \\ 0, & \text{otherwise.} \end{cases}$$

If  $s \leq j < 2s$ , then

$$b_{ij} = \begin{cases} w_{8(j+m)+2 \rightarrow 8(j+m)+7} \otimes e_{8j}, & i = j - s; \\ e_{8(j+m)+7} \otimes w_{8j \rightarrow 8j+1}, & i = j + 3s; \\ e_{8(j+m)+7} \otimes w_{8j \rightarrow 8j+5}, & i = j + 9s; \\ 0, & \text{otherwise.} \end{cases}$$

If  $2s \leq j < 3s$ , then

$$b_{ij} = \begin{cases} -e_{8(j+m+1)} \otimes w_{8j \rightarrow 8j+1}, & i = j + 3s; \\ 0, & \text{otherwise.} \end{cases}$$

If  $3s \leq j < 4s$ , then

$$b_{ij} = \begin{cases} -e_{8(j+m+1)+5} \otimes w_{8j+1 \rightarrow 8(j+1)}, & i = 3s + (j + 1)_s; \\ -w_{8(j+m)+7 \rightarrow 8(j+m+1)+5} \otimes e_{8j+1}, & i = j + s; \\ 0, & \text{otherwise.} \end{cases}$$

If  $4s \leq j < 5s$ , then

$$b_{ij} = \begin{cases} e_{8(j+m+1)+6} \otimes w_{8j+2 \rightarrow 8(j+1)}, & i = 2s + (j + 1)_s; \\ w_{8(j+m+1)+5 \rightarrow 8(j+m+1)+6} \otimes w_{8j+2 \rightarrow 8(j+1)}, & i = 3s + (j + 1)_s; \\ 0, & \text{otherwise.} \end{cases}$$

If  $5s \leq j < 6s$ , then

$$b_{ij} = \begin{cases} -w_{8(j+m+1) \rightarrow 8(j+m+1)+1} \otimes e_{8j+2}, & i = j + s; \\ -e_{8(j+m+1)+1} \otimes w_{8j+2 \rightarrow 8j+7}, & i = j + 11s; \\ 0, & \text{otherwise.} \end{cases}$$

If  $6s \leq j < 7s$ , then  $b_{ij} = 0$ .

If  $7s \leq j < 8s$ , then

$$b_{ij} = \begin{cases} -w_{8(j+m+1)+2 \rightarrow 8(j+m+1)+3} \otimes w_{8j+4 \rightarrow 8(j+1)}, & i = (j + 1)_s; \\ w_{8(j+m+1) \rightarrow 8(j+m+1)+3} \otimes e_{8j+4}, & i = j + s; \\ e_{8(j+m+1)+3} \otimes w_{8j+4 \rightarrow 8j+7}, & i = j + 6s; \\ 0, & \text{otherwise.} \end{cases}$$

If  $8s \leq j < 9s$ , then  $b_{ij} = 0$ .

If  $9s \leq j < 10s$ , then

$$b_{ij} = \begin{cases} -w_{8(j+m)+7 \rightarrow 8(j+m+1)+3} \otimes w_{8j+5 \rightarrow 8j+6}, & i = j + 2s; \\ 0, & \text{otherwise.} \end{cases}$$

If  $10s \leq j < 12s$ , then  $b_{ij} = 0$ .

If  $12s \leq j < 13s$ , then

$$b_{ij} = \begin{cases} w_{8(j+m+1)+2 \rightarrow 8(j+m+1)+4} \otimes w_{8j+6 \rightarrow 8(j+1)}, & i = (j+1)_s; \\ -e_{8(j+m+1)+4} \otimes w_{8j+6 \rightarrow 8(j+1)}, & i = s + (j+1)_s; \\ w_{8(j+m)+7 \rightarrow 8(j+m+1)+4} \otimes e_{8j+6}, & i = j - s; \\ 0, & \text{otherwise.} \end{cases}$$

If  $13s \leq j < 14s$ , then  $b_{ij} = 0$ .

If  $14s \leq j < 15s$ , then

$$b_{ij} = \begin{cases} -e_{8(j+m+1)+7} \otimes w_{8j+7 \rightarrow 8(j+1)+1}, & i = 4s + (j+1)_s; \\ -w_{8(j+m+1)+3 \rightarrow 8(j+m+1)+7} \otimes e_{8j+7}, & i = j - s; \\ w_{8(j+m+1)+4 \rightarrow 8(j+m+1)+7} \otimes e_{8j+7}, & i = j + s; \\ 0, & \text{otherwise.} \end{cases}$$

If  $15s \leq j < 16s$ , then

$$b_{ij} = \begin{cases} -w_{8(j+m+1)+2 \rightarrow 8(j+m+2)} \otimes w_{8j+7 \rightarrow 8(j+1)}, & i = (j+1)_s; \\ w_{8(j+m+1)+4 \rightarrow 8(j+m+2)} \otimes w_{8j+7 \rightarrow 8(j+1)}, & i = s + (j+1)_s; \\ e_{8(j+m+2)} \otimes w_{8j+7 \rightarrow 8(j+1)+1}, & i = 5s + (j+1)_s; \\ 0, & \text{otherwise.} \end{cases}$$

(19) If  $r_0 = 18$ , then  $\Omega^{18}(Z_t^{(21)})$  is described with  $(19s \times 16s)$  matrix, whose entries  $b_{ij}$  have the following form:

If  $0 \leq j < s$ , then

$$b_{ij} = \begin{cases} -e_{8(j+m)+5} \otimes w_{8j \rightarrow 8j+1}, & i = j + 3s; \\ 0, & \text{otherwise.} \end{cases}$$

If  $s \leq j < 2s$ , then

$$b_{ij} = \begin{cases} -w_{8(j+m-1)+7 \rightarrow 8(j+m)+3} \otimes e_{8j}, & i = j - s; \\ -e_{8(j+m)+3} \otimes w_{8j \rightarrow 8j+3}, & i = j + 6s; \\ 0, & \text{otherwise.} \end{cases}$$

If  $2s \leq j < 3s$ , then

$$b_{ij} = \begin{cases} e_{8(j+m)+6} \otimes w_{8j \rightarrow 8j+5}, & i = j + 9s; \\ 0, & \text{otherwise.} \end{cases}$$

If  $3s \leq j < 4s$ , then

$$b_{ij} = \begin{cases} e_{8(j+m)+1} \otimes w_{8j \rightarrow 8j+1}, & i = j + s; \\ 0, & \text{otherwise.} \end{cases}$$

If  $4s \leq j < 5s$ , then

$$b_{ij} = \begin{cases} -e_{8(j+m+1)} \otimes w_{8j+1 \rightarrow 8(j+1)}, & i = 2s + (j+1)_s; \\ 0, & \text{otherwise.} \end{cases}$$

If  $5s \leq j < 6s$ , then

$$b_{ij} = \begin{cases} -e_{8(j+m)+7} \otimes w_{8j+2 \rightarrow 8(j+1)}, & i = (j+1)_s; \\ -w_{8(j+m)+2 \rightarrow 8(j+m)+7} \otimes e_{8j+2}, & i = j; \\ 0, & \text{otherwise.} \end{cases}$$

If  $6s \leq j < 7s$ , then

$$b_{ij} = \begin{cases} -w_{8(j+m)+3 \rightarrow 8(j+m)+1} \otimes e_{8j+3}, & i = j+s; \\ 0, & \text{otherwise.} \end{cases}$$

If  $7s \leq j < 8s$ , then

$$b_{ij} = \begin{cases} -w_{8(j+m)+4 \rightarrow 8(j+m)+7} \otimes e_{8j+4}, & i = j+s; \\ 0, & \text{otherwise.} \end{cases}$$

If  $8s \leq j < 10s$ , then  $b_{ij} = 0$ .

If  $10s \leq j < 11s$ , then

$$b_{ij} = \begin{cases} -w_{8(j+m)+4 \rightarrow 8(j+m)+7} \otimes e_{8j+6}, & i = j+4s; \\ 0, & \text{otherwise.} \end{cases}$$

If  $11s \leq j < 12s$ , then  $b_{ij} = 0$ .

If  $12s \leq j < 13s$ , then

$$b_{ij} = \begin{cases} -e_{8(j+m+1)+2} \otimes w_{8j+7 \rightarrow 8(j+1)+2}, & i = 5s + (j+1)_s; \\ w_{8(j+m+1) \rightarrow 8(j+m+1)+2} \otimes e_{8j+7}, & i = j+5s; \\ 0, & \text{otherwise.} \end{cases}$$

If  $13s \leq j < 14s$ , then

$$b_{ij} = \begin{cases} w_{8(j+m+1)+1 \rightarrow 8(j+m+1)+4} \otimes w_{8j+7 \rightarrow 8(j+1)+1}, & i = 4s + (j+1)_s; \\ e_{8(j+m+1)+4} \otimes w_{8j+7 \rightarrow 8(j+1)+4}, & i = 8s + (j+1)_s; \\ -e_{8(j+m+1)+4} \otimes w_{8j+7 \rightarrow 8(j+1)+6}, & i = 14s + (j+1)_s; \\ 0, & \text{otherwise.} \end{cases}$$

If  $14s \leq j < 15s$ , then  $b_{ij} = 0$ .

If  $15s \leq j < 16s$ , then

$$b_{ij} = \begin{cases} e_{8(j+m+1)+5} \otimes w_{8j+7 \rightarrow 8(j+1)+1}, & i = 3s + (j+1)_s; \\ 0, & \text{otherwise.} \end{cases}$$

(20) If  $r_0 = 19$ , then  $\Omega^{19}(Z_t^{(21)})$  is described with  $(16s \times 19s)$  matrix, whose entries  $b_{ij}$  have the following form:

If  $0 \leq j < s$ , then

$$b_{ij} = \begin{cases} -w_{8(j+m)+6 \rightarrow 8(j+m)+7} \otimes e_{8j}, & i = j + s; \\ -w_{8(j+m)+1 \rightarrow 8(j+m)+7} \otimes e_{8j}, & i = j + 2s; \\ e_{8(j+m)+7} \otimes w_{8j \rightarrow 8j+2}, & i = j + 5s; \\ e_{8(j+m)+7} \otimes w_{8j \rightarrow 8j+4}, & i = j + 7s; \\ e_{8(j+m)+7} \otimes w_{8j \rightarrow 8j+6}, & i = j + 10s; \\ 0, & \text{otherwise.} \end{cases}$$

If  $s \leq j < 2s$ , then  $b_{ij} = 0$ .

If  $2s \leq j < 3s$ , then

$$b_{ij} = \begin{cases} e_{8(j+m+1)} \otimes w_{8j \rightarrow 8j+5}, & i = j + 7s; \\ 0, & \text{otherwise.} \end{cases}$$

If  $3s \leq j < 4s$ , then

$$b_{ij} = \begin{cases} -e_{8(j+m+1)+6} \otimes w_{8j+1 \rightarrow 8(j+1)}, & i = s + (j + 1)_s; \\ 0, & \text{otherwise.} \end{cases}$$

If  $4s \leq j < 5s$ , then

$$b_{ij} = \begin{cases} e_{8(j+m+1)+1} \otimes w_{8j+1 \rightarrow 8(j+1)}, & i = 2s + (j + 1)_s; \\ 0, & \text{otherwise.} \end{cases}$$

If  $5s \leq j < 6s$ , then

$$b_{ij} = \begin{cases} w_{8(j+m)+7 \rightarrow 8(j+m+1)+2} \otimes e_{8j+2}, & i = j; \\ w_{8(j+m)+7 \rightarrow 8(j+m+1)+2} \otimes w_{8j+2 \rightarrow 8j+4}, & i = j + 2s; \\ -e_{8(j+m+1)+2} \otimes w_{8j+2 \rightarrow 8j+7}, & i = j + 7s; \\ 0, & \text{otherwise.} \end{cases}$$

If  $6s \leq j < 7s$ , then

$$b_{ij} = \begin{cases} -e_{8(j+m+1)+3} \otimes w_{8j+3 \rightarrow 8(j+1)}, & i = (j + 1)_s; \\ w_{8(j+m+1) \rightarrow 8(j+m+1)+3} \otimes e_{8j+3}, & i = j; \\ 0, & \text{otherwise.} \end{cases}$$

If  $7s \leq j < 8s$ , then  $b_{ij} = 0$ .

If  $8s \leq j < 9s$ , then

$$b_{ij} = \begin{cases} w_{8(j+m)+7 \rightarrow 8(j+m+1)+4} \otimes e_{8j+4}, & i = j - s; \\ -w_{8(j+m+1)+2 \rightarrow 8(j+m+1)+4} \otimes w_{8j+4 \rightarrow 8j+7}, & i = j + 4s; \\ e_{8(j+m+1)+4} \otimes w_{8j+4 \rightarrow 8j+7}, & i = j + 5s; \\ 0, & \text{otherwise.} \end{cases}$$

If  $9s \leq j < 13s$ , then  $b_{ij} = 0$ .

If  $13s \leq j < 14s$ , then

$$b_{ij} = \begin{cases} w_{8(j+m+1) \rightarrow 8(j+m+1)+2} \otimes e_{8j+6}, & i = j - 2s; \\ 0, & \text{otherwise.} \end{cases}$$

If  $14s \leq j < 16s$ , then  $b_{ij} = 0$ .

If  $16s \leq j < 17s$ , then

$$b_{ij} = \begin{cases} w_{8(j+m+1)+5 \rightarrow 8(j+m+1)+7} \otimes e_{8j+7}, & i = j - s; \\ 0, & \text{otherwise.} \end{cases}$$

If  $17s \leq j < 18s$ , then

$$b_{ij} = \begin{cases} -w_{8(j+m+1)+6 \rightarrow 8(j+m+1)+7} \otimes w_{8j+7 \rightarrow 8(j+1)}, & i = s + (j+1)_s; \\ -w_{8(j+m+1)+1 \rightarrow 8(j+m+1)+7} \otimes w_{8j+7 \rightarrow 8(j+1)}, & i = 2s + (j+1)_s; \\ e_{8(j+m+1)+7} \otimes w_{8j+7 \rightarrow 8(j+1)+2}, & i = 5s + (j+1)_s; \\ e_{8(j+m+1)+7} \otimes w_{8j+7 \rightarrow 8(j+1)+4}, & i = 7s + (j+1)_s; \\ e_{8(j+m+1)+7} \otimes w_{8j+7 \rightarrow 8(j+1)+6}, & i = 10s + (j+1)_s; \\ 0, & \text{otherwise.} \end{cases}$$

If  $18s \leq j < 19s$ , then  $b_{ij} = 0$ .

(21) If  $r_0 = 20$ , then  $\Omega^{20}(Z_t^{(21)})$  is described with  $(16s \times 18s)$  matrix, whose entries  $b_{ij}$  have the following form:

If  $0 \leq j < s$ , then

$$b_{ij} = \begin{cases} -w_{8(j+m-1)+7 \rightarrow 8(j+m)+2} \otimes e_{8j}, & i = j; \\ w_{8(j+m) \rightarrow 8(j+m)+2} \otimes e_{8j}, & i = j + s; \\ e_{8(j+m)+2} \otimes w_{8j \rightarrow 8j+1}, & i = j + 2s; \\ w_{8(j+m)+1 \rightarrow 8(j+m)+2} \otimes w_{8j \rightarrow 8j+5}, & i = j + 10s; \\ 0, & \text{otherwise.} \end{cases}$$

If  $s \leq j < 2s$ , then

$$b_{ij} = \begin{cases} w_{8(j+m-1)+7 \rightarrow 8(j+m)+6} \otimes e_{8j}, & i = j - s; \\ e_{8(j+m)+6} \otimes w_{8j \rightarrow 8j+4}, & i = j + 6s; \\ e_{8(j+m)+6} \otimes w_{8j \rightarrow 8j+5}, & i = j + 7s; \\ 0, & \text{otherwise.} \end{cases}$$

If  $2s \leq j < 3s$ , then

$$b_{ij} = \begin{cases} -e_{8(j+m)+4} \otimes w_{8j \rightarrow 8j+3}, & i = j + 3s; \\ 0, & \text{otherwise.} \end{cases}$$

If  $3s \leq j < 4s$ , then

$$b_{ij} = \begin{cases} -e_{8(j+m)+1} \otimes w_{8j \rightarrow 8j+5}, & i = j + 7s; \\ 0, & \text{otherwise.} \end{cases}$$

If  $4s \leq j < 5s$ , then  $b_{ij} = 0$ .

If  $5s \leq j < 6s$ , then

$$b_{ij} = \begin{cases} e_{8(j+m)+7} \otimes w_{8j+1 \rightarrow 8(j+1)}, & i = (j+1)_s; \\ -w_{8(j+m)+2 \rightarrow 8(j+m)+7} \otimes e_{8j+1}, & i = j - 3s; \\ w_{8(j+m)+6 \rightarrow 8(j+m)+7} \otimes e_{8j+1}, & i = j - 2s; \\ 0, & \text{otherwise.} \end{cases}$$

If  $6s \leq j < 7s$ , then

$$b_{ij} = \begin{cases} -w_{8(j+m)+3 \rightarrow 8(j+m+1)} \otimes e_{8j+2}, & i = j - 2s; \\ 0, & \text{otherwise.} \end{cases}$$

If  $7s \leq j < 8s$ , then

$$b_{ij} = \begin{cases} e_{8(j+m)+7} \otimes w_{8j+3 \rightarrow 8(j+1)}, & i = (j+1)_s; \\ -w_{8(j+m)+5 \rightarrow 8(j+m)+7} \otimes e_{8j+3}, & i = j - s; \\ 0, & \text{otherwise.} \end{cases}$$

If  $8s \leq j < 9s$ , then

$$b_{ij} = \begin{cases} w_{8(j+m)+6 \rightarrow 8(j+m)+7} \otimes e_{8j+4}, & i = j - s; \\ -e_{8(j+m)+7} \otimes w_{8j+4 \rightarrow 8j+7}, & i = j + 5s; \\ 0, & \text{otherwise.} \end{cases}$$

If  $9s \leq j < 11s$ , then  $b_{ij} = 0$ .

If  $11s \leq j < 12s$ , then

$$b_{ij} = \begin{cases} w_{8(j+m)+7 \rightarrow 8(j+m+1)} \otimes w_{8j+5 \rightarrow 8(j+1)}, & i = (j+1)_s; \\ -e_{8(j+m+1)} \otimes w_{8j+5 \rightarrow 8(j+1)}, & i = s + (j+1)_s; \\ 0, & \text{otherwise.} \end{cases}$$

If  $12s \leq j < 13s$ , then

$$b_{ij} = \begin{cases} w_{8(j+m)+5 \rightarrow 8(j+m)+7} \otimes e_{8j+6}, & i = j; \\ 0, & \text{otherwise.} \end{cases}$$

If  $13s \leq j < 14s$ , then  $b_{ij} = 0$ .

If  $14s \leq j < 15s$ , then

$$b_{ij} = \begin{cases} -w_{8(j+m)+7 \rightarrow 8(j+m+1)+5} \otimes e_{8j+7}, & i = j - s; \\ w_{8(j+m+1) \rightarrow 8(j+m+1)+5} \otimes e_{8j+7}, & i = j + s; \\ 0, & \text{otherwise.} \end{cases}$$

If  $15s \leq j < 16s$ , then

$$b_{ij} = \begin{cases} -e_{8(j+m+1)+3} \otimes w_{8j+7 \rightarrow 8(j+1)+2}, & i = 4s + (j+1)_s; \\ 0, & \text{otherwise.} \end{cases}$$

If  $16s \leq j < 17s$ , then

$$b_{ij} = \begin{cases} w_{8(j+m)+7 \rightarrow 8(j+m+1)+6} \otimes w_{8j+7 \rightarrow 8(j+1)}, & i = (j+1)_s; \\ e_{8(j+m+1)+6} \otimes w_{8j+7 \rightarrow 8(j+1)+4}, & i = 7s + (j+1)_s; \\ e_{8(j+m+1)+6} \otimes w_{8j+7 \rightarrow 8(j+1)+5}, & i = 8s + (j+1)_s; \\ 0, & \text{otherwise.} \end{cases}$$

If  $17s \leq j < 18s$ , then  $b_{ij} = 0$ .

(22) If  $r_0 = 21$ , then  $\Omega^{21}(Z_t^{(21)})$  is described with  $(14s \times 19s)$  matrix, whose entries  $b_{ij}$  have the following form:



If  $0 \leq j < s$ , then

$$b_{ij} = \begin{cases} w_{8(j+m)+6 \rightarrow 8(j+m)+7} \otimes e_{8j}, & i = j + 2s; \\ 0, & \text{otherwise.} \end{cases}$$

If  $s \leq j < 2s$ , then

$$b_{ij} = \begin{cases} w_{8(j+m)+2 \rightarrow 8(j+m+1)} \otimes e_{8j}, & i = j - s; \\ e_{8(j+m+1)} \otimes w_{8j \rightarrow 8j+2}, & i = j + 3s; \\ e_{8(j+m+1)} \otimes w_{8j \rightarrow 8j+4}, & i = j + 5s; \\ e_{8(j+m+1)} \otimes w_{8j \rightarrow 8j+6}, & i = j + 8s; \\ 0, & \text{otherwise.} \end{cases}$$

If  $2s \leq j < 3s$ , then

$$b_{ij} = \begin{cases} -e_{8(j+m)+7} \otimes w_{8j \rightarrow 8j+3}, & i = j + 3s; \\ 0, & \text{otherwise.} \end{cases}$$

If  $3s \leq j < 4s$ , then

$$b_{ij} = \begin{cases} e_{8(j+m+1)+2} \otimes w_{8j+1 \rightarrow 8(j+1)}, & i = (j+1)_s; \\ w_{8(j+m)+7 \rightarrow 8(j+m+1)+2} \otimes e_{8j+1}, & i = j; \\ 0, & \text{otherwise.} \end{cases}$$

If  $4s \leq j < 5s$ , then

$$b_{ij} = \begin{cases} w_{8(j+m+1) \rightarrow 8(j+m+1)+3} \otimes e_{8j+2}, & i = j; \\ w_{8(j+m)+7 \rightarrow 8(j+m+1)+3} \otimes w_{8j+2 \rightarrow 8j+3}, & i = j + s; \\ -e_{8(j+m+1)+3} \otimes w_{8j+2 \rightarrow 8j+7}, & i = j + 6s; \\ 0, & \text{otherwise.} \end{cases}$$

If  $5s \leq j < 6s$ , then  $b_{ij} = 0$ .

If  $6s \leq j < 7s$ , then

$$b_{ij} = \begin{cases} -e_{8(j+m+1)+4} \otimes w_{8j+3 \rightarrow 8(j+1)}, & i = s + (j+1)_s; \\ 0, & \text{otherwise.} \end{cases}$$

If  $7s \leq j < 8s$ , then

$$b_{ij} = \begin{cases} w_{8(j+m)+7 \rightarrow 8(j+m+1)+6} \otimes e_{8j+3}, & i = j - 2s; \\ 0, & \text{otherwise.} \end{cases}$$

If  $8s \leq j < 9s$ , then

$$b_{ij} = \begin{cases} -w_{8(j+m+1) \rightarrow 8(j+m+1)+5} \otimes e_{8j+4}, & i = j - 2s; \\ 0, & \text{otherwise.} \end{cases}$$

If  $9s \leq j < 11s$ , then  $b_{ij} = 0$ .

If  $11s \leq j < 12s$ , then

$$b_{ij} = \begin{cases} e_{8(j+m+1)+6} \otimes w_{8j+5 \rightarrow 8(j+1)}, & i = 2s + (j+1)_s; \\ -w_{8(j+m+1) \rightarrow 8(j+m+1)+6} \otimes e_{8j+5}, & i = j - 3s; \\ -w_{8(j+m+1) \rightarrow 8(j+m+1)+6} \otimes w_{8j+5 \rightarrow 8j+6}, & i = j - 2s; \\ 0, & \text{otherwise.} \end{cases}$$

If  $12s \leq j < 13s$ , then

$$b_{ij} = \begin{cases} -w_{8(j+m+1) \rightarrow 8(j+m+1)+5} \otimes e_{8j+5}, & i = j - 4s; \\ -w_{8(j+m+1) \rightarrow 8(j+m+1)+5} \otimes w_{8j+5 \rightarrow 8j+6}, & i = j - 3s; \\ 0, & \text{otherwise.} \end{cases}$$

If  $13s \leq j < 14s$ , then

$$b_{ij} = \begin{cases} e_{8(j+m+1)+6} \otimes w_{8j+6 \rightarrow 8j+7}, & i = j - 2s; \\ 0, & \text{otherwise.} \end{cases}$$

If  $14s \leq j < 16s$ , then  $b_{ij} = 0$ .

If  $16s \leq j < 17s$ , then

$$b_{ij} = \begin{cases} e_{8(j+m+1)+7} \otimes w_{8j+7 \rightarrow 8(j+1)+1}, & i = 3s + (j+1)_s; \\ -w_{8(j+m+1)+6 \rightarrow 8(j+m+1)+7} \otimes e_{8j+7}, & i = j - 5s; \\ 0, & \text{otherwise.} \end{cases}$$

If  $17s \leq j < 18s$ , then  $b_{ij} = 0$ .

If  $18s \leq j < 19s$ , then

$$b_{ij} = \begin{cases} w_{8(j+m+1)+2 \rightarrow 8(j+m+2)} \otimes w_{8j+7 \rightarrow 8(j+1)}, & i = (j+1)_s; \\ w_{8(j+m+1)+6 \rightarrow 8(j+m+2)} \otimes w_{8j+7 \rightarrow 8(j+1)}, & i = 2s + (j+1)_s; \\ e_{8(j+m+2)} \otimes w_{8j+7 \rightarrow 8(j+1)+2}, & i = 4s + (j+1)_s; \\ e_{8(j+m+2)} \otimes w_{8j+7 \rightarrow 8(j+1)+4}, & i = 6s + (j+1)_s; \\ e_{8(j+m+2)} \otimes w_{8j+7 \rightarrow 8(j+1)+6}, & i = 8s + (j+1)_s; \\ 0, & \text{otherwise.} \end{cases}$$

(23) If  $r_0 = 22$ , then  $\Omega^{22}(Z_t^{(21)})$  is described with  $(13s \times 18s)$  matrix, whose entries  $b_{ij}$  have the following form:

If  $0 \leq j < s$ , then

$$b_{ij} = \begin{cases} -w_{8(j+m) \rightarrow 8(j+m)+2} \otimes e_{8j}, & i = j; \\ w_{8(j+m-1)+7 \rightarrow 8(j+m)+2} \otimes e_{8j}, & i = j + s; \\ -w_{8(j+m)+1 \rightarrow 8(j+m)+2} \otimes w_{8j \rightarrow 8j+4}, & i = j + 6s; \\ -e_{8(j+m)+2} \otimes w_{8j \rightarrow 8j+5}, & i = j + 7s; \\ 0, & \text{otherwise.} \end{cases}$$

If  $s \leq j < 2s$ , then

$$b_{ij} = \begin{cases} e_{8(j+m)+3} \otimes w_{8j \rightarrow 8j+1}, & i = j + s; \\ 0, & \text{otherwise.} \end{cases}$$

If  $2s \leq j < 3s$ , then

$$b_{ij} = \begin{cases} w_{8(j+m) \rightarrow 8(j+m)+6} \otimes e_{8j}, & i = j - 2s; \\ -w_{8(j+m)+5 \rightarrow 8(j+m)+6} \otimes w_{8j \rightarrow 8j+2}, & i = j + 2s; \\ -e_{8(j+m)+6} \otimes w_{8j \rightarrow 8j+6}, & i = j + 8s; \\ 0, & \text{otherwise.} \end{cases}$$

If  $3s \leq j < 4s$ , then

$$b_{ij} = \begin{cases} w_{8(j+m) \rightarrow 8(j+m)+5} \otimes e_{8j}, & i = j - 3s; \\ 0, & \text{otherwise.} \end{cases}$$

If  $4s \leq j < 5s$ , then  $b_{ij} = 0$ .

If  $5s \leq j < 6s$ , then

$$b_{ij} = \begin{cases} -w_{8(j+m)+4 \rightarrow 8(j+m)+7} \otimes e_{8j+2}, & i = j - 2s; \\ 0, & \text{otherwise.} \end{cases}$$

If  $6s \leq j < 7s$ , then

$$b_{ij} = \begin{cases} -e_{8(j+m)+7} \otimes w_{8j+3 \rightarrow 8(j+1)}, & i = s + (j+1)_s; \\ w_{8(j+m)+6 \rightarrow 8(j+m)+7} \otimes e_{8j+3}, & i = j - s; \\ 0, & \text{otherwise.} \end{cases}$$

If  $7s \leq j < 8s$ , then

$$b_{ij} = \begin{cases} e_{8(j+m)+1} \otimes w_{8j+3 \rightarrow 8(j+1)}, & i = (j+1)_s; \\ -w_{8(j+m)+7 \rightarrow 8(j+m)+1} \otimes w_{8j+3 \rightarrow 8(j+1)}, & i = s + (j+1)_s; \\ w_{8(j+m)+6 \rightarrow 8(j+m)+1} \otimes e_{8j+3}, & i = j - 2s; \\ 0, & \text{otherwise.} \end{cases}$$

If  $8s \leq j < 9s$ , then

$$b_{ij} = \begin{cases} w_{8(j+m)+1 \rightarrow 8(j+m)+1} \otimes e_{8j+4}, & i = j - 2s; \\ w_{8(j+m)+7 \rightarrow 8(j+m)+1} \otimes w_{8j+4 \rightarrow 8j+7}, & i = j + 3s; \\ -e_{8(j+m)+1} \otimes w_{8j+4 \rightarrow 8j+7}, & i = j + 4s; \\ 0, & \text{otherwise.} \end{cases}$$

If  $9s \leq j < 10s$ , then  $b_{ij} = 0$ .

If  $10s \leq j < 11s$ , then

$$b_{ij} = \begin{cases} -w_{8(j+m)+5 \rightarrow 8(j+m)+1} \otimes e_{8j+5}, & i = j - 2s; \\ -w_{8(j+m)+6 \rightarrow 8(j+m)+1} \otimes w_{8j+5 \rightarrow 8j+6}, & i = j; \\ 0, & \text{otherwise.} \end{cases}$$

If  $11s \leq j < 14s$ , then  $b_{ij} = 0$ .

If  $14s \leq j < 15s$ , then

$$b_{ij} = \begin{cases} -w_{8(j+m+1) \rightarrow 8(j+m+1)+6} \otimes w_{8j+7 \rightarrow 8(j+1)}, & i = (j+1)_s; \\ w_{8(j+m+1)+5 \rightarrow 8(j+m+1)+6} \otimes w_{8j+7 \rightarrow 8(j+1)+2}, & i = 4s + (j+1)_s; \\ e_{8(j+m+1)+6} \otimes w_{8j+7 \rightarrow 8(j+1)+3}, & i = 5s + (j+1)_s; \\ e_{8(j+m+1)+6} \otimes w_{8j+7 \rightarrow 8(j+1)+6}, & i = 10s + (j+1)_s; \\ w_{8(j+m)+7 \rightarrow 8(j+m+1)+6} \otimes e_{8j+7}, & i = j - 3s; \\ 0, & \text{otherwise.} \end{cases}$$

If  $15s \leq j < 16s$ , then

$$b_{ij} = \begin{cases} -e_{8(j+m+1)+4} \otimes w_{8j+7 \rightarrow 8(j+1)+2}, & i = 3s + (j+1)_s; \\ 0, & \text{otherwise.} \end{cases}$$

If  $16s \leq j < 18s$ , then  $b_{ij} = 0$ .

(24) If  $r_0 = 23$ , then  $\Omega^{23}(Z_t^{(21)})$  is described with  $(11s \times 20s)$  matrix, whose entries  $b_{ij}$  have the following form:

If  $0 \leq j < s$ , then

$$b_{ij} = \begin{cases} -w_{8(j+m)+3 \rightarrow 8(j+m)+7} \otimes e_{8j}, & i = j; \\ -e_{8(j+m)+7} \otimes w_{8j \rightarrow 8j+2}, & i = j + 3s; \\ -e_{8(j+m)+7} \otimes w_{8j \rightarrow 8j+6}, & i = j + 7s; \\ 0, & \text{otherwise.} \end{cases}$$

If  $s \leq j < 2s$ , then

$$b_{ij} = \begin{cases} e_{8(j+m+1)} \otimes w_{8j \rightarrow 8j+1}, & i = j + s; \\ 0, & \text{otherwise.} \end{cases}$$

If  $2s \leq j < 3s$ , then

$$b_{ij} = \begin{cases} w_{8(j+m)+5 \rightarrow 8(j+m+1)} \otimes e_{8j}, & i = j - s; \\ -e_{8(j+m+1)} \otimes w_{8j \rightarrow 8j+3}, & i = j + 2s; \\ 0, & \text{otherwise.} \end{cases}$$

If  $3s \leq j < 4s$ , then

$$b_{ij} = \begin{cases} e_{8(j+m+1)+3} \otimes w_{8j+1 \rightarrow 8(j+1)}, & i = (j+1)_s; \\ 0, & \text{otherwise.} \end{cases}$$

If  $4s \leq j < 5s$ , then

$$b_{ij} = \begin{cases} -e_{8(j+m+1)+5} \otimes w_{8j+1 \rightarrow 8(j+1)}, & i = s + (j+1)_s; \\ 0, & \text{otherwise.} \end{cases}$$

If  $5s \leq j < 6s$ , then

$$b_{ij} = \begin{cases} w_{8(j+m)+7 \rightarrow 8(j+m+1)+4} \otimes e_{8j+2}, & i = j - 2s; \\ w_{8(j+m+1) \rightarrow 8(j+m+1)+4} \otimes w_{8j+2 \rightarrow 8j+3}, & i = j - s; \\ -e_{8(j+m+1)+4} \otimes w_{8j+2 \rightarrow 8j+7}, & i = j + 4s; \\ 0, & \text{otherwise.} \end{cases}$$

If  $6s \leq j < 7s$ , then

$$b_{ij} = \begin{cases} -w_{8(j+m+1)+5 \rightarrow 8(j+m+1)+6} \otimes w_{8j+2 \rightarrow 8(j+1)}, & i = s + (j+1)_s; \\ 0, & \text{otherwise.} \end{cases}$$

If  $7s \leq j < 8s$ , then  $b_{ij} = 0$ .

If  $8s \leq j < 9s$ , then

$$b_{ij} = \begin{cases} -w_{8(j+m+1) \rightarrow 8(j+m+1)+1} \otimes e_{8j+3}, & i = j - 4s; \\ 0, & \text{otherwise.} \end{cases}$$

If  $9s \leq j < 10s$ , then

$$b_{ij} = \begin{cases} w_{8(j+m+1)+1 \rightarrow 8(j+m+1)+2} \otimes e_{8j+4}, & i = j - 4s; \\ 0, & \text{otherwise.} \end{cases}$$

If  $10s \leq j < 11s$ , then

$$b_{ij} = \begin{cases} e_{8(j+m+1)+6} \otimes w_{8j+4 \rightarrow 8j+7}, & i = j; \\ 0, & \text{otherwise.} \end{cases}$$

If  $11s \leq j < 12s$ , then

$$b_{ij} = \begin{cases} -w_{8(j+m)+7 \rightarrow 8(j+m+1)+6} \otimes w_{8j+5 \rightarrow 8j+6}, & i = j - 4s; \\ 0, & \text{otherwise.} \end{cases}$$

If  $12s \leq j < 17s$ , then  $b_{ij} = 0$ .

If  $17s \leq j < 18s$ , then

$$b_{ij} = \begin{cases} -w_{8(j+m+1)+3 \rightarrow 8(j+m+1)+7} \otimes w_{8j+7 \rightarrow 8(j+1)}, & i = (j+1)_s; \\ -e_{8(j+m+1)+7} \otimes w_{8j+7 \rightarrow 8(j+1)+2}, & i = 3s + (j+1)_s; \\ -e_{8(j+m+1)+7} \otimes w_{8j+7 \rightarrow 8(j+1)+6}, & i = 7s + (j+1)_s; \\ w_{8(j+m+1)+2 \rightarrow 8(j+m+1)+7} \otimes e_{8j+7}, & i = j - 9s; \\ w_{8(j+m+1)+4 \rightarrow 8(j+m+1)+7} \otimes e_{8j+7}, & i = j - 8s; \\ 0, & \text{otherwise.} \end{cases}$$

If  $18s \leq j < 20s$ , then  $b_{ij} = 0$ .

(25) If  $r_0 = 24$ , then  $\Omega^{24}(Z_t^{(21)})$  is described with  $(11s \times 18s)$  matrix, whose entries  $b_{ij}$  have the following form:

If  $0 \leq j < s$ , then

$$b_{ij} = \begin{cases} -w_{8(j+m) \rightarrow 8(j+m)+3} \otimes e_{8j}, & i = j; \\ -w_{8(j+m)+2 \rightarrow 8(j+m)+3} \otimes w_{8j \rightarrow 8j+4}, & i = j + 5s; \\ -e_{8(j+m)+3} \otimes w_{8j \rightarrow 8j+5}, & i = j + 6s; \\ 0, & \text{otherwise.} \end{cases}$$

If  $s \leq j < 2s$ , then

$$b_{ij} = \begin{cases} -e_{8(j+m)+6} \otimes w_{8j \rightarrow 8j+2}, & i = j + 2s; \\ 0, & \text{otherwise.} \end{cases}$$

If  $2s \leq j < 3s$ , then

$$b_{ij} = \begin{cases} e_{8(j+m)+4} \otimes w_{8j \rightarrow 8j+1}, & i = j - s; \\ 0, & \text{otherwise.} \end{cases}$$

If  $3s \leq j < 4s$ , then  $b_{ij} = 0$ .

If  $4s \leq j < 5s$ , then

$$b_{ij} = \begin{cases} e_{8(j+m)+5} \otimes w_{8j \rightarrow 8j+1}, & i = j - 2s; \\ 0, & \text{otherwise.} \end{cases}$$

If  $5s \leq j < 6s$ , then  $b_{ij} = 0$ .

If  $6s \leq j < 7s$ , then

$$b_{ij} = \begin{cases} w_{8(j+m)+6 \rightarrow 8(j+m)+7} \otimes e_{8j+2}, & i = j - 3s; \\ -e_{8(j+m)+7} \otimes w_{8j+2 \rightarrow 8j+7}, & i = j + 4s; \\ 0, & \text{otherwise.} \end{cases}$$

If  $7s \leq j < 8s$ , then  $b_{ij} = 0$ .

If  $8s \leq j < 9s$ , then

$$b_{ij} = \begin{cases} e_{8(j+m+1)} \otimes w_{8j+3 \rightarrow 8(j+1)}, & i = (j+1)_s; \\ w_{8(j+m)+1 \rightarrow 8(j+m+1)} \otimes e_{8j+3}, & i = j - 4s; \\ 0, & \text{otherwise.} \end{cases}$$

If  $9s \leq j < 10s$ , then

$$b_{ij} = \begin{cases} w_{8(j+m)+2 \rightarrow 8(j+m)+7} \otimes e_{8j+4}, & i = j - 4s; \\ -e_{8(j+m)+7} \otimes w_{8j+4 \rightarrow 8j+7}, & i = j + s; \\ 0, & \text{otherwise.} \end{cases}$$

If  $10s \leq j < 11s$ , then

$$b_{ij} = \begin{cases} w_{8(j+m)+4 \rightarrow 8(j+m)+7} \otimes w_{8j+5 \rightarrow 8j+6}, & i = j - 2s; \\ 0, & \text{otherwise.} \end{cases}$$

If  $11s \leq j < 14s$ , then  $b_{ij} = 0$ .

If  $14s \leq j < 15s$ , then

$$b_{ij} = \begin{cases} -w_{8(j+m+1)+1 \rightarrow 8(j+m+1)+2} \otimes w_{8j+7 \rightarrow 8(j+1)+3}, & i = 4s + (j+1)_s; \\ -w_{8(j+m+1) \rightarrow 8(j+m+1)+2} \otimes e_{8j+7}, & i = j - 5s; \\ 0, & \text{otherwise.} \end{cases}$$

If  $15s \leq j < 16s$ , then

$$b_{ij} = \begin{cases} -w_{8(j+m+1) \rightarrow 8(j+m+1)+3} \otimes w_{8j+7 \rightarrow 8(j+1)}, & i = (j+1)_s; \\ w_{8(j+m+1)+1 \rightarrow 8(j+m+1)+3} \otimes w_{8j+7 \rightarrow 8(j+1)+3}, & i = 4s + (j+1)_s; \\ -w_{8(j+m+1)+2 \rightarrow 8(j+m+1)+3} \otimes w_{8j+7 \rightarrow 8(j+1)+4}, & i = 5s + (j+1)_s; \\ -e_{8(j+m+1)+3} \otimes w_{8j+7 \rightarrow 8(j+1)+5}, & i = 6s + (j+1)_s; \\ w_{8(j+m+1) \rightarrow 8(j+m+1)+3} \otimes e_{8j+7}, & i = j - 6s; \\ 0, & \text{otherwise.} \end{cases}$$

If  $16s \leq j < 18s$ , then  $b_{ij} = 0$ .

(26) If  $r_0 = 25$ , then  $\Omega^{25}(Z_t^{(21)})$  is described with  $(10s \times 19s)$  matrix, whose entries  $b_{ij}$  have the following form:

If  $0 \leq j < s$ , then

$$b_{ij} = \begin{cases} w_{8(j+m)+4 \rightarrow 8(j+m)+7} \otimes e_{8j}, & i = j; \\ e_{8(j+m)+7} \otimes w_{8j \rightarrow 8j+1}, & i = j + 2s; \\ 0, & \text{otherwise.} \end{cases}$$

If  $s \leq j < 2s$ , then

$$b_{ij} = \begin{cases} -w_{8(j+m)+4 \rightarrow 8(j+m+1)} \otimes e_{8j}, & i = j - s; \\ -e_{8(j+m+1)} \otimes w_{8j \rightarrow 8j+2}, & i = j + 2s; \\ -e_{8(j+m+1)} \otimes w_{8j \rightarrow 8j+6}, & i = j + 6s; \\ 0, & \text{otherwise.} \end{cases}$$

If  $2s \leq j < 3s$ , then

$$b_{ij} = \begin{cases} e_{8(j+m)+7} \otimes w_{8j \rightarrow 8j+1}, & i = j; \\ 0, & \text{otherwise.} \end{cases}$$

If  $3s \leq j < 4s$ , then

$$b_{ij} = \begin{cases} e_{8(j+m+1)+4} \otimes w_{8j+1 \rightarrow 8(j+1)}, & i = (j+1)_s; \\ 0, & \text{otherwise.} \end{cases}$$

If  $4s \leq j < 5s$ , then  $b_{ij} = 0$ .

If  $5s \leq j < 6s$ , then

$$b_{ij} = \begin{cases} -w_{8(j+m+1) \rightarrow 8(j+m+1)+5} \otimes e_{8j+2}, & i = j - 2s; \\ e_{8(j+m+1)+5} \otimes w_{8j+2 \rightarrow 8j+7}, & i = j + 4s; \\ 0, & \text{otherwise.} \end{cases}$$

If  $6s \leq j < 7s$ , then  $b_{ij} = 0$ .

If  $7s \leq j < 8s$ , then

$$b_{ij} = \begin{cases} w_{8(j+m+1)+1 \rightarrow 8(j+m+1)+2} \otimes e_{8j+3}, & i = j - 3s; \\ 0, & \text{otherwise.} \end{cases}$$

If  $8s \leq j < 9s$ , then

$$b_{ij} = \begin{cases} -e_{8(j+m+1)+6} \otimes w_{8j+3 \rightarrow 8(j+1)}, & i = s + (j+1)_s; \\ 0, & \text{otherwise.} \end{cases}$$

If  $9s \leq j < 10s$ , then

$$b_{ij} = \begin{cases} w_{8(j+m+1)+2 \rightarrow 8(j+m+1)+3} \otimes e_{8j+4}, & i = j - 4s; \\ 0, & \text{otherwise.} \end{cases}$$

If  $10s \leq j < 11s$ , then

$$b_{ij} = \begin{cases} -w_{8(j+m+1) \rightarrow 8(j+m+1)+2} \otimes w_{8j+5 \rightarrow 8j+6}, & i = j - 3s; \\ 0, & \text{otherwise.} \end{cases}$$

If  $11s \leq j < 17s$ , then  $b_{ij} = 0$ .

If  $17s \leq j < 18s$ , then

$$b_{ij} = \begin{cases} w_{8(j+m+1)+3 \rightarrow 8(j+m+2)} \otimes e_{8j+7}, & i = j - 9s; \\ 0, & \text{otherwise.} \end{cases}$$

If  $18s \leq j < 19s$ , then  $b_{ij} = 0$ .

(27) If  $r_0 = 26$ , then  $\Omega^{26}(Z_t^{(21)})$  is described with  $(8s \times 18s)$  matrix, whose entries  $b_{ij}$  have the following form:

If  $0 \leq j < s$ , then

$$b_{ij} = \begin{cases} w_{8(j+m)+1 \rightarrow 8(j+m)+2} \otimes w_{8j \rightarrow 8j+2}, & i = j + 2s; \\ 0, & \text{otherwise.} \end{cases}$$

If  $s \leq j < 2s$ , then

$$b_{ij} = \begin{cases} -w_{8(j+m-1)+7 \rightarrow 8(j+m)+4} \otimes e_{8j}, & i = j - s; \\ -w_{8(j+m)+3 \rightarrow 8(j+m)+4} \otimes w_{8j \rightarrow 8j+4}, & i = j + 3s; \\ -e_{8(j+m)+4} \otimes w_{8j \rightarrow 8j+5}, & i = j + 4s; \\ 0, & \text{otherwise.} \end{cases}$$

If  $2s \leq j < 3s$ , then

$$b_{ij} = \begin{cases} e_{8(j+m)+6} \otimes w_{8j \rightarrow 8j+1}, & i = j - s; \\ 0, & \text{otherwise.} \end{cases}$$

If  $3s \leq j < 4s$ , then

$$b_{ij} = \begin{cases} -e_{8(j+m)+5} \otimes w_{8j \rightarrow 8j+6}, & i = j + 3s; \\ 0, & \text{otherwise.} \end{cases}$$

If  $4s \leq j < 6s$ , then  $b_{ij} = 0$ .

If  $6s \leq j < 7s$ , then

$$b_{ij} = \begin{cases} -w_{8(j+m)+7 \rightarrow 8(j+m+1)} \otimes w_{8j+2 \rightarrow 8(j+1)}, & i = (j+1)s; \\ w_{8(j+m)+1 \rightarrow 8(j+m+1)} \otimes e_{8j+2}, & i = j - 4s; \\ -w_{8(j+m)+2 \rightarrow 8(j+m+1)} \otimes w_{8j+2 \rightarrow 8j+3}, & i = j - 3s; \\ w_{8(j+m)+3 \rightarrow 8(j+m+1)} \otimes w_{8j+2 \rightarrow 8j+4}, & i = j - 2s; \\ e_{8(j+m+1)} \otimes w_{8j+2 \rightarrow 8j+7}, & i = j + s; \\ 0, & \text{otherwise.} \end{cases}$$

If  $7s \leq j < 8s$ , then

$$b_{ij} = \begin{cases} e_{8(j+m)+7} \otimes w_{8j+3 \rightarrow 8(j+1)}, & i = (j+1)s; \\ w_{8(j+m)+2 \rightarrow 8(j+m)+7} \otimes e_{8j+3}, & i = j - 4s; \\ 0, & \text{otherwise.} \end{cases}$$

If  $8s \leq j < 9s$ , then

$$b_{ij} = \begin{cases} w_{8(j+m)+3 \rightarrow 8(j+m+1)} \otimes e_{8j+4}, & i = j - 4s; \\ 0, & \text{otherwise.} \end{cases}$$



If  $9s \leq j < 10s$ , then

$$b_{ij} = \begin{cases} w_{8(j+m)+4 \rightarrow 8(j+m+1)} \otimes e_{8j+5}, & i = j - 4s; \\ 0, & \text{otherwise.} \end{cases}$$

If  $10s \leq j < 13s$ , then  $b_{ij} = 0$ .

If  $13s \leq j < 14s$ , then

$$b_{ij} = \begin{cases} -w_{8(j+m+1)+2 \rightarrow 8(j+m+1)+3} \otimes w_{8j+7 \rightarrow 8(j+1)+3}, & i = 3s + (j+1)s; \\ -w_{8(j+m+1) \rightarrow 8(j+m+1)+3} \otimes e_{8j+7}, & i = j - 6s; \\ 0, & \text{otherwise.} \end{cases}$$

If  $14s \leq j < 18s$ , then  $b_{ij} = 0$ .

(28) If  $r_0 = 27$ , then  $\Omega^{27}(Z_t^{(21)})$  is described with  $(9s \times 19s)$  matrix, whose entries  $b_{ij}$  have the following form:

If  $0 \leq j < s$ , then

$$b_{ij} = \begin{cases} e_{8(j+m)+7} \otimes e_{8j}, & i = j; \\ 0, & \text{otherwise.} \end{cases}$$

If  $s \leq j < 2s$ , then  $b_{ij} = 0$ .

If  $2s \leq j < 3s$ , then

$$b_{ij} = \begin{cases} e_{8(j+m+1)} \otimes w_{8j \rightarrow 8j+1}, & i = j - s; \\ 0, & \text{otherwise.} \end{cases}$$

If  $3s \leq j < 4s$ , then  $b_{ij} = 0$ .

If  $4s \leq j < 5s$ , then

$$b_{ij} = \begin{cases} -w_{8(j+m+1) \rightarrow 8(j+m+1)+1} \otimes e_{8j+1}, & i = j - 3s; \\ 0, & \text{otherwise.} \end{cases}$$

If  $5s \leq j < 6s$ , then

$$b_{ij} = \begin{cases} w_{8(j+m+1)+1 \rightarrow 8(j+m+1)+2} \otimes e_{8j+2}, & i = j - 3s; \\ 0, & \text{otherwise.} \end{cases}$$

If  $6s \leq j < 7s$ , then

$$b_{ij} = \begin{cases} -e_{8(j+m+1)+6} \otimes w_{8j+2 \rightarrow 8j+7}, & i = j + 2s; \\ 0, & \text{otherwise.} \end{cases}$$

If  $7s \leq j < 8s$ , then

$$b_{ij} = \begin{cases} w_{8(j+m+1)+2 \rightarrow 8(j+m+1)+3} \otimes e_{8j+3}, & i = j - 4s; \\ 0, & \text{otherwise.} \end{cases}$$

If  $8s \leq j < 10s$ , then  $b_{ij} = 0$ .

If  $10s \leq j < 11s$ , then

$$b_{ij} = \begin{cases} -w_{8(j+m+1) \rightarrow 8(j+m+1)+3} \otimes e_{8j+5}, & i = j - 5s; \\ 0, & \text{otherwise.} \end{cases}$$

If  $11s \leq j < 14s$ , then  $b_{ij} = 0$ .

If  $14s \leq j < 15s$ , then

$$b_{ij} = \begin{cases} -e_{8(j+m+1)+4} \otimes w_{8j+6 \rightarrow 8j+7}, & i = j - 7s; \\ 0, & \text{otherwise.} \end{cases}$$

If  $15s \leq j < 16s$ , then  $b_{ij} = 0$ .

If  $16s \leq j < 17s$ , then

$$b_{ij} = \begin{cases} w_{8(j+m+1)+4 \rightarrow 8(j+m+1)+7} \otimes e_{8j+7}, & i = j - 9s; \\ 0, & \text{otherwise.} \end{cases}$$

If  $17s \leq j < 18s$ , then

$$b_{ij} = \begin{cases} -w_{8(j+m+1)+4 \rightarrow 8(j+m+2)} \otimes e_{8j+7}, & i = j - 10s; \\ 0, & \text{otherwise.} \end{cases}$$

If  $18s \leq j < 19s$ , then  $b_{ij} = 0$ .

(29) If  $r_0 = 28$ , then  $\Omega^{28}(Z_t^{(21)})$  is described with  $(8s \times 16s)$  matrix, whose entries  $b_{ij}$  have the following form:

If  $0 \leq j < s$ , then

$$b_{ij} = \begin{cases} w_{8(j+m) \rightarrow 8(j+m)+3} \otimes e_{8j}, & i = j; \\ w_{8(j+m)+2 \rightarrow 8(j+m)+3} \otimes w_{8j \rightarrow 8j+2}, & i = j + 2s; \\ 0, & \text{otherwise.} \end{cases}$$

If  $s \leq j < 2s$ , then

$$b_{ij} = \begin{cases} w_{8(j+m) \rightarrow 8(j+m)+6} \otimes e_{8j}, & i = j - s; \\ w_{8(j+m)+5 \rightarrow 8(j+m)+6} \otimes w_{8j \rightarrow 8j+5}, & i = j + 4s; \\ -e_{8(j+m)+6} \otimes w_{8j \rightarrow 8j+6}, & i = j + 5s; \\ 0, & \text{otherwise.} \end{cases}$$

If  $2s \leq j < 4s$ , then  $b_{ij} = 0$ .

If  $4s \leq j < 5s$ , then

$$b_{ij} = \begin{cases} e_{8(j+m+1)} \otimes w_{8j+1 \rightarrow 8(j+1)}, & i = (j+1)s; \\ w_{8(j+m)+1 \rightarrow 8(j+m+1)} \otimes e_{8j+1}, & i = j - 3s; \\ 0, & \text{otherwise.} \end{cases}$$

If  $5s \leq j < 6s$ , then

$$b_{ij} = \begin{cases} w_{8(j+m)+2 \rightarrow 8(j+m)+7} \otimes e_{8j+2}, & i = j - 3s; \\ e_{8(j+m)+7} \otimes w_{8j+2 \rightarrow 8j+7}, & i = j + 2s; \\ 0, & \text{otherwise.} \end{cases}$$

If  $6s \leq j < 7s$ , then

$$b_{ij} = \begin{cases} w_{8(j+m)+3 \rightarrow 8(j+m+1)} \otimes e_{8j+3}, & i = j - 3s; \\ -w_{8(j+m)+4 \rightarrow 8(j+m+1)} \otimes w_{8j+3 \rightarrow 8j+4}, & i = j - 2s; \\ 0, & \text{otherwise.} \end{cases}$$

If  $7s \leq j < 8s$ , then  $b_{ij} = 0$ .

If  $8s \leq j < 9s$ , then

$$b_{ij} = \begin{cases} w_{8(j+m)+5 \rightarrow 8(j+m)+7} \otimes e_{8j+5}, & i = j - 3s; \\ -w_{8(j+m)+6 \rightarrow 8(j+m)+7} \otimes w_{8j+5 \rightarrow 8j+6}, & i = j - 2s; \\ e_{8(j+m)+7} \otimes w_{8j+5 \rightarrow 8j+7}, & i = j - s; \\ 0, & \text{otherwise.} \end{cases}$$

If  $9s \leq j < 12s$ , then  $b_{ij} = 0$ .

If  $12s \leq j < 13s$ , then

$$b_{ij} = \begin{cases} w_{8(j+m+1)+1 \rightarrow 8(j+m+1)+2} \otimes w_{8j+7 \rightarrow 8(j+1)+1}, & i = s + (j+1)_s; \\ 0, & \text{otherwise.} \end{cases}$$

If  $13s \leq j < 14s$ , then

$$b_{ij} = \begin{cases} -w_{8(j+m+1)+3 \rightarrow 8(j+m+1)+4} \otimes w_{8j+7 \rightarrow 8(j+1)+3}, & i = 3s + (j+1)_s; \\ e_{8(j+m+1)+4} \otimes w_{8j+7 \rightarrow 8(j+1)+4}, & i = 4s + (j+1)_s; \\ -w_{8(j+m)+7 \rightarrow 8(j+m+1)+4} \otimes e_{8j+7}, & i = j - 6s; \\ 0, & \text{otherwise.} \end{cases}$$

If  $14s \leq j < 16s$ , then  $b_{ij} = 0$ .

(II) Represent an arbitrary  $t_0 \in \mathbb{N}$  in the form  $t_0 = 29\ell_0 + r_0$ , where  $0 \leq r_0 \leq 28$ . Then  $\Omega^{t_0}(Z_t^{(21)})$  is a  $\Omega^{r_0}(Z_t^{(21)})$ , whose left components twisted by  $\sigma^{\ell_0}$ .

**Proposition 17** (Translates for the case 22). (I) Let  $r_0 \in \mathbb{N}$ ,  $r_0 < 29$ .  $r_0$ -translates of the elements  $Z_t^{(22)}$  are described by the following way.

(1) If  $r_0 = 0$ , then  $\Omega^0(Z_t^{(22)})$  is described with  $(8s \times 14s)$  matrix with the following nonzero entries:

$$\begin{aligned} b_{j,0} &= -w_{8(j+m) \rightarrow 8(j+m)+2} \otimes e_{8j}; \\ b_{j-s,s} &= w_{8(j+m) \rightarrow 8(j+m)+4} \otimes e_{8j}; \\ b_{j-2s,7s} &= -w_{8(j+m)+5 \rightarrow 8(j+m)+7} \otimes e_{8j+5}. \end{aligned}$$

(2) If  $r_0 = 1$ , then  $\Omega^1(Z_t^{(22)})$  is described with  $(9s \times 13s)$  matrix with the following nonzero entries:

$$\begin{aligned} b_{j,s} &= w_{8(j+m)+5 \rightarrow 8(j+m)+7} \otimes e_{8j}; \\ b_{(j+1)_s, 2s+(-1)_s} &= -w_{8(j+m+1)+1 \rightarrow 8(j+m+1)+3} \otimes w_{8j+1 \rightarrow 8(j+1)}; \\ b_{2s+(j+1)_s, 2s+(-1)_s} &= -w_{8(j+m+1)+2 \rightarrow 8(j+m+1)+3} \otimes w_{8j+1 \rightarrow 8(j+1)+1}; \\ b_{(j+1)_s, 3s+(-1)_s} &= -w_{8(j+m+1)+1 \rightarrow 8(j+m+1)+4} \otimes w_{8j+2 \rightarrow 8(j+1)}; \\ b_{2s+(j+1)_s, 3s+(-1)_s} &= -w_{8(j+m+1)+2 \rightarrow 8(j+m+1)+4} \otimes w_{8j+2 \rightarrow 8(j+1)+1}; \\ b_{3s+(j+1)_s, 3s+(-1)_s} &= -w_{8(j+m+1)+3 \rightarrow 8(j+m+1)+4} \otimes w_{8j+2 \rightarrow 8(j+1)+2}; \\ b_{(j+1)_s, 7s+(-1)_s} &= -w_{8(j+m+1)+1 \rightarrow 8(j+m+1)+2} \otimes w_{8j+5 \rightarrow 8(j+1)}; \\ b_{j-4s, 12s+(-1)_s} &= -w_{8(j+m+1) \rightarrow 8(j+m+2)} \otimes e_{8j+7}. \end{aligned}$$

(3) If  $r_0 = 2$ , then  $\Omega^2(Z_t^{(22)})$  is described with  $(8s \times 11s)$  matrix with the following nonzero entries:

$$\begin{aligned} b_{(j+1)_s, 3s+(-1)_s} &= -e_{8(j+m)+7} \otimes w_{8j+2 \rightarrow 8(j+1)}; \\ b_{(j+1)_s, 4s+(-1)_s} &= w_{8(j+m)+7 \rightarrow 8(j+m+1)} \otimes w_{8j+3 \rightarrow 8(j+1)}; \end{aligned}$$

$$\begin{aligned}
b_{j-s,4s+(-1)_s} &= -w_{8(j+m)+4 \rightarrow 8(j+m+1)} \otimes e_{8j+3}; \\
b_{(j+1)_s,6s+(-1)_s} &= -w_{8(j+m)+7 \rightarrow 8(j+m+1)} \otimes w_{8j+5 \rightarrow 8(j+1)}; \\
b_{j-s,6s+(-1)_s} &= -w_{8(j+m)+6 \rightarrow 8(j+m+1)} \otimes e_{8j+5}.
\end{aligned}$$

(4) If  $r_0 = 3$ , then  $\Omega^3(Z_t^{(22)})$  is described with  $(10s \times 11s)$  matrix with the following nonzero entries:

$$\begin{aligned}
b_{j+s,(-1)_s} &= w_{8(j+m)+6 \rightarrow 8(j+m+1)} \otimes e_{8j}; \\
b_{j+4s,(-1)_s} &= -w_{8(j+m)+7 \rightarrow 8(j+m+1)} \otimes w_{8j \rightarrow 8j+3}; \\
b_{j+2s,s+(-1)_s} &= w_{8(j+m)+4 \rightarrow 8(j+m+1)+4} \otimes w_{8j+1 \rightarrow 8j+2}; \\
b_{j,4s+(-1)_s} &= -w_{8(j+m)+7 \rightarrow 8(j+m+1)+1} \otimes e_{8j+3}; \\
b_{(j+1)_s,6s+(-1)_s} &= -w_{8(j+m+1)+2 \rightarrow 8(j+m+1)+3} \otimes w_{8j+5 \rightarrow 8(j+1)}; \\
b_{j-s,7s+(-1)_s} &= -w_{8(j+m)+7 \rightarrow 8(j+m+1)+6} \otimes e_{8j+5}.
\end{aligned}$$

(5) If  $r_0 = 4$ , then  $\Omega^4(Z_t^{(22)})$  is described with  $(11s \times 10s)$  matrix with the following nonzero entries:

$$\begin{aligned}
b_{j+2s,(-1)_s} &= -w_{8(j+m)+3 \rightarrow 8(j+m)+4} \otimes w_{8j \rightarrow 8j+1}; \\
b_{j-s,s+(-1)_s} &= -w_{8(j+m-1)+7 \rightarrow 8(j+m)+6} \otimes e_{8j}; \\
b_{s+(j+1)_s,3s+(-2)_s} &= -e_{8(j+m+1)} \otimes w_{8j+2 \rightarrow 8(j+1)}; \\
b_{j+s,6s+(-1)_s} &= w_{8(j+m)+1 \rightarrow 8(j+m)+7} \otimes e_{8j+5}; \\
b_{j+2s,6s+(-1)_s} &= -w_{8(j+m)+2 \rightarrow 8(j+m)+7} \otimes w_{8j+5 \rightarrow 8j+6}.
\end{aligned}$$

(6) If  $r_0 = 5$ , then  $\Omega^5(Z_t^{(22)})$  is described with  $(11s \times 8s)$  matrix with the following nonzero entries:

$$\begin{aligned}
b_{j+s,(-1)_s} &= w_{8(j+m)+3 \rightarrow 8(j+m)+7} \otimes e_{8j}; \\
b_{(j+1)_s,s+(-2)_s} &= -w_{8(j+m+1)+5 \rightarrow 8(j+m+1)+6} \otimes w_{8j+1 \rightarrow 8(j+1)}; \\
b_{2s+(j+1)_s,2s+(-2)_s} &= -e_{8(j+m+1)+1} \otimes w_{8j+2 \rightarrow 8(j+1)}; \\
b_{3s+(j+1)_s,7s+(-2)_s} &= -w_{8(j+m+1)+4 \rightarrow 8(j+m+2)} \otimes w_{8j+7 \rightarrow 8(j+1)+1}; \\
b_{4s+(j+1)_s,7s+(-2)_s} &= -w_{8(j+m+1)+7 \rightarrow 8(j+m+2)} \otimes w_{8j+7 \rightarrow 8(j+1)+2}; \\
b_{5s+(j+1)_s,7s+(-2)_s} &= -e_{8(j+m+2)} \otimes w_{8j+7 \rightarrow 8(j+1)+3}.
\end{aligned}$$

(7) If  $r_0 = 6$ , then  $\Omega^6(Z_t^{(22)})$  is described with  $(13s \times 9s)$  matrix with the following nonzero entries:

$$\begin{aligned}
b_{(j+1)_s,(-2)_s} &= e_{8(j+m)+7} \otimes w_{8j \rightarrow 8(j+1)}; \\
b_{(j+1)_s,s+(-2)_s} &= -w_{8(j+m)+7 \rightarrow 8(j+m+1)} \otimes w_{8j+1 \rightarrow 8(j+1)}; \\
b_{(j+1)_s,2s+(-2)_s} &= w_{8(j+m)+7 \rightarrow 8(j+m+1)+1} \otimes w_{8j+2 \rightarrow 8(j+1)}; \\
b_{s+(j+1)_s,3s+(-2)_s} &= w_{8(j+m+1) \rightarrow 8(j+m+1)+2} \otimes w_{8j+3 \rightarrow 8(j+1)}; \\
b_{s+(j+1)_s,4s+(-2)_s} &= -w_{8(j+m+1) \rightarrow 8(j+m+1)+3} \otimes w_{8j+4 \rightarrow 8(j+1)}; \\
b_{2s+(j+1)_s,7s+(-2)_s} &= -e_{8(j+m+1)+4} \otimes w_{8j+7 \rightarrow 8(j+1)+1}; \\
b_{5s+(j+1)_s,7s+(-2)_s} &= -w_{8(j+m+1)+1 \rightarrow 8(j+m+1)+4} \otimes w_{8j+7 \rightarrow 8(j+1)+3}; \\
b_{3s+(j+1)_s,8s+(-2)_s} &= -w_{8(j+m+1)+5 \rightarrow 8(j+m+1)+6} \otimes w_{8j+7 \rightarrow 8(j+1)+2}.
\end{aligned}$$

(8) If  $r_0 = 7$ , then  $\Omega^7(Z_t^{(22)})$  is described with  $(14s \times 8s)$  matrix with the following nonzero entries:

$$\begin{aligned}
b_{(j+1)_s,2s+(-2)_s} &= e_{8(j+m+1)+2} \otimes w_{8j+2 \rightarrow 8(j+1)}; \\
b_{s+(j+1)_s,4s+(-2)_s} &= -e_{8(j+m+1)+4} \otimes w_{8j+4 \rightarrow 8(j+1)};
\end{aligned}$$

$$b_{4s+(j+1)s,7s+(-2)s} = -e_{8(j+m+1)+7} \otimes w_{8j+7 \rightarrow 8(j+1)+1}.$$

(9) If  $r_0 = 8$ , then  $\Omega^8(Z_t^{(22)})$  is described with  $(16s \times 8s)$  matrix with the following nonzero entries:

$$\begin{aligned} b_{(j+1)s,(-2)s} &= w_{8(j+m)+7 \rightarrow 8(j+m+1)} \otimes w_{8j \rightarrow 8(j+1)}; \\ b_{s+(j+1)s,(-2)s} &= -w_{8(j+m)+7 \rightarrow 8(j+m+1)} \otimes w_{8j \rightarrow 8(j+1)}; \\ b_{2s+(j+1)s,(-2)s} &= e_{8(j+m+1)} \otimes w_{8j \rightarrow 8(j+1)}; \\ b_{(j+1)s,s+(-2)s} &= -w_{8(j+m)+7 \rightarrow 8(j+m+1)+1} \otimes w_{8j+1 \rightarrow 8(j+1)}; \\ b_{s+(j+1)s,s+(-2)s} &= w_{8(j+m)+7 \rightarrow 8(j+m+1)+1} \otimes w_{8j+1 \rightarrow 8(j+1)}; \\ b_{(j+1)s,2s+(-2)s} &= w_{8(j+m)+7 \rightarrow 8(j+m+1)+2} \otimes w_{8j+2 \rightarrow 8(j+1)}; \\ b_{s+(j+1)s,2s+(-2)s} &= -w_{8(j+m)+7 \rightarrow 8(j+m+1)+2} \otimes w_{8j+2 \rightarrow 8(j+1)}; \\ b_{s+(j+1)s,3s+(-2)s} &= w_{8(j+m)+7 \rightarrow 8(j+m+1)+3} \otimes w_{8j+3 \rightarrow 8(j+1)}; \\ b_{s+(j+1)s,4s+(-2)s} &= -w_{8(j+m)+7 \rightarrow 8(j+m+1)+4} \otimes w_{8j+4 \rightarrow 8(j+1)}; \\ b_{3s+(j+1)s,7s+(-2)s} &= -w_{8(j+m+1)+5 \rightarrow 8(j+m+1)+7} \otimes w_{8j+7 \rightarrow 8(j+1)+1}; \\ b_{4s+(j+1)s,7s+(-2)s} &= w_{8(j+m+1)+6 \rightarrow 8(j+m+1)+7} \otimes w_{8j+7 \rightarrow 8(j+1)+2}. \end{aligned}$$

(10) If  $r_0 = 9$ , then  $\Omega^9(Z_t^{(22)})$  is described with  $(16s \times 9s)$  matrix with the following nonzero entries:

$$\begin{aligned} b_{3s+(j+1)s,(-2)s} &= -e_{8(j+m+1)+1} \otimes w_{8j \rightarrow 8(j+1)}; \\ b_{(j+1)s,s+(-2)s} &= e_{8(j+m+1)+5} \otimes w_{8j \rightarrow 8(j+1)}; \\ b_{s+(j+1)s,3s+(-2)s} &= -e_{8(j+m+1)+3} \otimes w_{8j+2 \rightarrow 8(j+1)}; \\ b_{2s+(j+1)s,5s+(-2)s} &= -w_{8(j+m+1)+6 \rightarrow 8(j+m+1)+7} \otimes w_{8j+4 \rightarrow 8(j+1)}; \\ b_{4s+(j+1)s,8s+(-2)s} &= e_{8(j+m+2)} \otimes w_{8j+7 \rightarrow 8(j+1)+1}. \end{aligned}$$

(11) If  $r_0 = 10$ , then  $\Omega^{10}(Z_t^{(22)})$  is described with  $(19s \times 8s)$  matrix with the following nonzero entries:

$$\begin{aligned} b_{(j+1)s,(-2)s} &= -e_{8(j+m)+7} \otimes w_{8j \rightarrow 8(j+1)}; \\ b_{(j+1)s,s+(-2)s} &= w_{8(j+m)+7 \rightarrow 8(j+m+1)+2} \otimes w_{8j+1 \rightarrow 8(j+1)}; \\ b_{2s+(j+1)s,s+(-2)s} &= w_{8(j+m+1) \rightarrow 8(j+m+1)+2} \otimes w_{8j+1 \rightarrow 8(j+1)}; \\ b_{s+(j+1)s,2s+(-2)s} &= w_{8(j+m+1) \rightarrow 8(j+m+1)+3} \otimes w_{8j+2 \rightarrow 8(j+1)}; \\ b_{2s+(j+1)s,2s+(-2)s} &= -w_{8(j+m+1) \rightarrow 8(j+m+1)+3} \otimes w_{8j+2 \rightarrow 8(j+1)}; \\ b_{2s+(j+1)s,3s+(-2)s} &= w_{8(j+m+1) \rightarrow 8(j+m+1)+4} \otimes w_{8j+3 \rightarrow 8(j+1)}; \\ b_{2s+(j+1)s,4s+(-2)s} &= w_{8(j+m+1) \rightarrow 8(j+m+1)+5} \otimes w_{8j+4 \rightarrow 8(j+1)}; \\ b_{3s+(j+1)s,7s+(-2)s} &= -w_{8(j+m+1)+6 \rightarrow 8(j+m+2)} \otimes w_{8j+7 \rightarrow 8(j+1)+1}. \end{aligned}$$

(12) If  $r_0 = 11$ , then  $\Omega^{11}(Z_t^{(22)})$  is described with  $(18s \times 10s)$  matrix with the following nonzero entries:

$$\begin{aligned} b_{3s+(j+1)s,(-2)s} &= -w_{8(j+m+1)+1 \rightarrow 8(j+m+1)+2} \otimes w_{8j \rightarrow 8(j+1)}; \\ b_{s+(j+1)s,s+(-2)s} &= -e_{8(j+m+1)+6} \otimes w_{8j \rightarrow 8(j+1)}; \\ b_{(j+1)s,2s+(-2)s} &= -w_{8(j+m+1)+2 \rightarrow 8(j+m+1)+3} \otimes w_{8j+1 \rightarrow 8(j+1)}; \\ b_{2s+(j+1)s,3s+(-2)s} &= -e_{8(j+m+1)+4} \otimes w_{8j+2 \rightarrow 8(j+1)}; \\ b_{3s+(j+1)s,5s+(-2)s} &= -w_{8(j+m+1)+1 \rightarrow 8(j+m+2)} \otimes w_{8j+4 \rightarrow 8(j+1)}; \\ b_{5s+(j+1)s,5s+(-2)s} &= w_{8(j+m+1)+7 \rightarrow 8(j+m+2)} \otimes w_{8j+4 \rightarrow 8(j+1)+1}; \\ b_{6s+(j+1)s,5s+(-2)s} &= e_{8(j+m+2)} \otimes w_{8j+4 \rightarrow 8(j+1)+2}; \end{aligned}$$

$$b_{5s+(j+1)s,9s+(-2)s} = -w_{8(j+m+1)+7 \rightarrow 8(j+m+2)+5} \otimes w_{8j+7 \rightarrow 8(j+1)+1}.$$

(13) If  $r_0 = 12$ , then  $\Omega^{12}(Z_t^{(22)})$  is described with  $(19s \times 11s)$  matrix with the following nonzero entries:

$$\begin{aligned} b_{(j+1)s,(-2)s} &= e_{8(j+m)+7} \otimes w_{8j \rightarrow 8(j+1)}; \\ b_{2s+(j+1)s,(-2)s} &= -e_{8(j+m)+7} \otimes w_{8j \rightarrow 8(j+1)}; \\ b_{(j+1)s,s+(-2)s} &= w_{8(j+m)+7 \rightarrow 8(j+m+1)} \otimes w_{8j \rightarrow 8(j+1)}; \\ b_{s+(j+1)s,s+(-2)s} &= -e_{8(j+m+1)} \otimes w_{8j \rightarrow 8(j+1)}; \\ b_{2s+(j+1)s,s+(-2)s} &= -w_{8(j+m)+7 \rightarrow 8(j+m+1)} \otimes w_{8j \rightarrow 8(j+1)}; \\ b_{s+(j+1)s,2s+(-2)s} &= w_{8(j+m+1) \rightarrow 8(j+m+1)+3} \otimes w_{8j+1 \rightarrow 8(j+1)}; \\ b_{2s+(j+1)s,3s+(-2)s} &= w_{8(j+m)+7 \rightarrow 8(j+m+1)+4} \otimes w_{8j+2 \rightarrow 8(j+1)}; \\ b_{s+(j+1)s,4s+(-2)s} &= -w_{8(j+m+1) \rightarrow 8(j+m+1)+5} \otimes w_{8j+3 \rightarrow 8(j+1)}; \\ b_{5s+(j+1)s,5s+(-2)s} &= -w_{8(j+m+1)+5 \rightarrow 8(j+m+1)+6} \otimes w_{8j+4 \rightarrow 8(j+1)+2}; \\ b_{(j+1)s,6s+(-2)s} &= -w_{8(j+m)+7 \rightarrow 8(j+m+1)+1} \otimes w_{8j+4 \rightarrow 8(j+1)}; \\ b_{s+(j+1)s,6s+(-2)s} &= w_{8(j+m+1) \rightarrow 8(j+m+1)+1} \otimes w_{8j+4 \rightarrow 8(j+1)}; \\ b_{2s+(j+1)s,6s+(-2)s} &= w_{8(j+m)+7 \rightarrow 8(j+m+1)+1} \otimes w_{8j+4 \rightarrow 8(j+1)}; \\ b_{9s+(j+1)s,6s+(-2)s} &= e_{8(j+m+1)+1} \otimes w_{8j+4 \rightarrow 8(j+1)+4}; \\ b_{3s+(j+1)s,10s+(-2)s} &= w_{8(j+m+1)+2 \rightarrow 8(j+m+1)+7} \otimes w_{8j+7 \rightarrow 8(j+1)+1}; \\ b_{5s+(j+1)s,10s+(-2)s} &= -w_{8(j+m+1)+5 \rightarrow 8(j+m+1)+7} \otimes w_{8j+7 \rightarrow 8(j+1)+2}. \end{aligned}$$

(14) If  $r_0 = 13$ , then  $\Omega^{13}(Z_t^{(22)})$  is described with  $(18s \times 11s)$  matrix with the following nonzero entries:

$$\begin{aligned} b_{(j+1)s,s+(-2)s} &= w_{8(j+m+1)+2 \rightarrow 8(j+m+1)+3} \otimes w_{8j \rightarrow 8(j+1)}; \\ b_{(j+1)s,3s+(-2)s} &= w_{8(j+m+1)+2 \rightarrow 8(j+m+1)+4} \otimes w_{8j+1 \rightarrow 8(j+1)}; \\ b_{s+(j+1)s,3s+(-2)s} &= -w_{8(j+m+1)+3 \rightarrow 8(j+m+1)+4} \otimes w_{8j+1 \rightarrow 8(j+1)}; \\ b_{2s+(j+1)s,4s+(-2)s} &= w_{8(j+m+1)+6 \rightarrow 8(j+m+1)+7} \otimes w_{8j+2 \rightarrow 8(j+1)}; \\ b_{3s+(j+1)s,4s+(-2)s} &= w_{8(j+m+1)+5 \rightarrow 8(j+m+1)+7} \otimes w_{8j+2 \rightarrow 8(j+1)}; \\ b_{3s+(j+1)s,5s+(-2)s} &= w_{8(j+m+1)+5 \rightarrow 8(j+m+2)} \otimes w_{8j+3 \rightarrow 8(j+1)}; \\ b_{(j+1)s,6s+(-2)s} &= -w_{8(j+m+1)+2 \rightarrow 8(j+m+1)+7} \otimes w_{8j+4 \rightarrow 8(j+1)}; \\ b_{4s+(j+1)s,9s+(-2)s} &= -w_{8(j+m+2) \rightarrow 8(j+m+2)+2} \otimes w_{8j+7 \rightarrow 8(j+1)+1}. \end{aligned}$$

(15) If  $r_0 = 14$ , then  $\Omega^{14}(Z_t^{(22)})$  is described with  $(20s \times 13s)$  matrix with the following nonzero entries:

$$\begin{aligned} b_{(j+1)s,(-2)s} &= -e_{8(j+m)+7} \otimes w_{8j \rightarrow 8(j+1)}; \\ b_{s+(j+1)s,s+(-2)s} &= e_{8(j+m+1)} \otimes w_{8j \rightarrow 8(j+1)}; \\ b_{2s+(j+1)s,s+(-2)s} &= -e_{8(j+m+1)} \otimes w_{8j \rightarrow 8(j+1)}; \\ b_{2s+(j+1)s,3s+(-2)s} &= -w_{8(j+m+1) \rightarrow 8(j+m+1)+5} \otimes w_{8j+2 \rightarrow 8(j+1)}; \\ b_{(j+1)s,6s+(-2)s} &= w_{8(j+m)+7 \rightarrow 8(j+m+1)+2} \otimes w_{8j+4 \rightarrow 8(j+1)}; \\ b_{s+(j+1)s,6s+(-2)s} &= w_{8(j+m+1) \rightarrow 8(j+m+1)+2} \otimes w_{8j+4 \rightarrow 8(j+1)}; \\ b_{2s+(j+1)s,6s+(-2)s} &= -w_{8(j+m+1) \rightarrow 8(j+m+1)+2} \otimes w_{8j+4 \rightarrow 8(j+1)}; \\ b_{9s+(j+1)s,6s+(-2)s} &= e_{8(j+m+1)+2} \otimes w_{8j+4 \rightarrow 8(j+1)+4}; \\ b_{3s+(j+1)s,11s+(-2)s} &= -w_{8(j+m+1)+3 \rightarrow 8(j+m+1)+7} \otimes w_{8j+7 \rightarrow 8(j+1)+1}. \end{aligned}$$

(16) If  $r_0 = 15$ , then  $\Omega^{15}(Z_t^{(22)})$  is described with  $(18s \times 14s)$  matrix with the following nonzero entries:

$$\begin{aligned}
b_{2s+(j+1)s, s+(-2)s} &= e_{8(j+m+1)+4} \otimes w_{8j \rightarrow 8(j+1)}; \\
b_{3s+(j+1)s, s+(-2)s} &= -w_{8(j+m+1)+1 \rightarrow 8(j+m+1)+4} \otimes w_{8j \rightarrow 8(j+1)}; \\
b_{s+(j+1)s, 2s+(-2)s} &= -e_{8(j+m+1)+6} \otimes w_{8j \rightarrow 8(j+1)}; \\
b_{4s+(j+1)s, 3s+(-2)s} &= e_{8(j+m+1)+5} \otimes w_{8j \rightarrow 8(j+1)}; \\
b_{(j+1)s, 4s+(-2)s} &= w_{8(j+m+1)+3 \rightarrow 8(j+m+1)+7} \otimes w_{8j+1 \rightarrow 8(j+1)}; \\
b_{s+(j+1)s, 4s+(-2)s} &= -w_{8(j+m+1)+6 \rightarrow 8(j+m+1)+7} \otimes w_{8j+1 \rightarrow 8(j+1)}; \\
b_{2s+(j+1)s, 4s+(-2)s} &= -w_{8(j+m+1)+4 \rightarrow 8(j+m+1)+7} \otimes w_{8j+1 \rightarrow 8(j+1)}; \\
b_{3s+(j+1)s, 5s+(-2)s} &= w_{8(j+m+1)+1 \rightarrow 8(j+m+2)} \otimes w_{8j+2 \rightarrow 8(j+1)}; \\
b_{(j+1)s, 6s+(-2)s} &= -w_{8(j+m+1)+3 \rightarrow 8(j+m+1)+7} \otimes w_{8j+3 \rightarrow 8(j+1)}; \\
b_{3s+(j+1)s, 6s+(-2)s} &= w_{8(j+m+1)+1 \rightarrow 8(j+m+1)+7} \otimes w_{8j+3 \rightarrow 8(j+1)}; \\
b_{(j+1)s, 7s+(-2)s} &= -w_{8(j+m+1)+3 \rightarrow 8(j+m+2)} \otimes w_{8j+4 \rightarrow 8(j+1)}; \\
b_{3s+(j+1)s, 7s+(-2)s} &= w_{8(j+m+1)+1 \rightarrow 8(j+m+2)} \otimes w_{8j+4 \rightarrow 8(j+1)}; \\
b_{5s+(j+1)s, 12s+(-2)s} &= -w_{8(j+m+1)+7 \rightarrow 8(j+m+2)+3} \otimes w_{8j+7 \rightarrow 8(j+1)+1}.
\end{aligned}$$

(17) If  $r_0 = 16$ , then  $\Omega^{16}(Z_t^{(22)})$  is described with  $(19s \times 16s)$  matrix with the following nonzero entries:

$$\begin{aligned}
b_{(j+1)s, (-2)s} &= e_{8(j+m)+7} \otimes w_{8j \rightarrow 8(j+1)}; \\
b_{(j+1)s, s+(-2)s} &= e_{8(j+m)+7} \otimes w_{8j \rightarrow 8(j+1)}; \\
b_{(j+1)s, 2s+(-2)s} &= w_{8(j+m)+7 \rightarrow 8(j+m+1)} \otimes w_{8j \rightarrow 8(j+1)}; \\
b_{s+(j+1)s, 2s+(-2)s} &= -e_{8(j+m+1)} \otimes w_{8j \rightarrow 8(j+1)}; \\
b_{2s+(j+1)s, 2s+(-2)s} &= -w_{8(j+m)+7 \rightarrow 8(j+m+1)} \otimes w_{8j \rightarrow 8(j+1)}; \\
b_{(j+1)s, 3s+(-2)s} &= -w_{8(j+m)+7 \rightarrow 8(j+m+1)+5} \otimes w_{8j+1 \rightarrow 8(j+1)}; \\
b_{2s+(j+1)s, 3s+(-2)s} &= w_{8(j+m)+7 \rightarrow 8(j+m+1)+5} \otimes w_{8j+1 \rightarrow 8(j+1)}; \\
b_{j+s, 5s+(-2)s} &= w_{8(j+m)+1 \rightarrow 8(j+m+1)+1} \otimes e_{8j+2}; \\
b_{(j+1)s, 7s+(-2)s} &= w_{8(j+m)+7 \rightarrow 8(j+m+1)+3} \otimes w_{8j+4 \rightarrow 8(j+1)}; \\
b_{9s+(j+1)s, 7s+(-2)s} &= e_{8(j+m+1)+3} \otimes w_{8j+4 \rightarrow 8(j+1)+4}; \\
b_{3s+(j+1)s, 14s+(-2)s} &= -w_{8(j+m+1)+4 \rightarrow 8(j+m+1)+7} \otimes w_{8j+7 \rightarrow 8(j+1)+1}.
\end{aligned}$$

(18) If  $r_0 = 17$ , then  $\Omega^{17}(Z_t^{(22)})$  is described with  $(18s \times 16s)$  matrix with the following nonzero entries:

$$\begin{aligned}
b_{3s+(j+1)s, (-2)s} &= -e_{8(j+m+1)+5} \otimes w_{8j \rightarrow 8(j+1)}; \\
b_{2s+(j+1)s, 2s+(-2)s} &= e_{8(j+m+1)+6} \otimes w_{8j \rightarrow 8(j+1)}; \\
b_{j+2s, 3s+(-2)s} &= -w_{8(j+m+1) \rightarrow 8(j+m+1)+1} \otimes w_{8j \rightarrow 8j+1}; \\
b_{s+(j+1)s, 7s+(-2)s} &= -w_{8(j+m+1)+4 \rightarrow 8(j+m+1)+7} \otimes w_{8j+4 \rightarrow 8(j+1)}; \\
b_{4s+(j+1)s, 12s+(-2)s} &= w_{8(j+m+1)+7 \rightarrow 8(j+m+2)+2} \otimes w_{8j+7 \rightarrow 8(j+1)+1}.
\end{aligned}$$

(19) If  $r_0 = 18$ , then  $\Omega^{18}(Z_t^{(22)})$  is described with  $(19s \times 19s)$  matrix with the following nonzero entries:

$$\begin{aligned}
b_{(j+1)s, (-2)s} &= -e_{8(j+m)+7} \otimes w_{8j \rightarrow 8(j+1)}; \\
b_{j+4s, (-2)s} &= -w_{8(j+m)+1 \rightarrow 8(j+m)+7} \otimes w_{8j \rightarrow 8j+1}; \\
b_{j+5s, (-2)s} &= -w_{8(j+m)+2 \rightarrow 8(j+m)+7} \otimes w_{8j \rightarrow 8j+2};
\end{aligned}$$

$$\begin{aligned}
b_{2s+(j+1)s,2s+(-2)s} &= e_{8(j+m+1)} \otimes w_{8j \rightarrow 8(j+1)}; \\
b_{2s+(j+1)s,4s+(-3)s} &= w_{8(j+m+1) \rightarrow 8(j+m+1)+1} \otimes w_{8j+1 \rightarrow 8(j+1)}; \\
b_{(j+1)s,5s+(-2)s} &= -w_{8(j+m)+7 \rightarrow 8(j+m+1)+2} \otimes w_{8j+2 \rightarrow 8(j+1)}; \\
b_{j,5s+(-2)s} &= -w_{8(j+m)+2 \rightarrow 8(j+m+1)+2} \otimes e_{8j+2}; \\
b_{(j+1)s,5s+(-3)s} &= w_{8(j+m)+7 \rightarrow 8(j+m+1)+2} \otimes w_{8j+2 \rightarrow 8(j+1)}; \\
b_{s+(j+1)s,5s+(-3)s} &= w_{8(j+m+1) \rightarrow 8(j+m+1)+2} \otimes w_{8j+2 \rightarrow 8(j+1)}; \\
b_{j,5s+(-3)s} &= w_{8(j+m)+2 \rightarrow 8(j+m+1)+2} \otimes e_{8j+2}; \\
b_{s+(j+1)s,6s+(-2)s} &= -w_{8(j+m+1) \rightarrow 8(j+m+1)+3} \otimes w_{8j+3 \rightarrow 8(j+1)}; \\
b_{2s+(j+1)s,6s+(-2)s} &= w_{8(j+m+1) \rightarrow 8(j+m+1)+3} \otimes w_{8j+3 \rightarrow 8(j+1)}; \\
b_{5s+(j+1)s,6s+(-2)s} &= w_{8(j+m+1)+2 \rightarrow 8(j+m+1)+3} \otimes w_{8j+3 \rightarrow 8(j+1)+2}; \\
b_{2s+(j+1)s,6s+(-3)s} &= -w_{8(j+m+1) \rightarrow 8(j+m+1)+3} \otimes w_{8j+3 \rightarrow 8(j+1)}; \\
b_{5s+(j+1)s,6s+(-3)s} &= -w_{8(j+m+1)+2 \rightarrow 8(j+m+1)+3} \otimes w_{8j+3 \rightarrow 8(j+1)+2}; \\
b_{s+(j+1)s,8s+(-2)s} &= w_{8(j+m+1) \rightarrow 8(j+m+1)+4} \otimes w_{8j+4 \rightarrow 8(j+1)}; \\
b_{2s+(j+1)s,8s+(-2)s} &= -w_{8(j+m+1) \rightarrow 8(j+m+1)+4} \otimes w_{8j+4 \rightarrow 8(j+1)}; \\
b_{5s+(j+1)s,8s+(-2)s} &= -w_{8(j+m+1)+2 \rightarrow 8(j+m+1)+4} \otimes w_{8j+4 \rightarrow 8(j+1)+2}; \\
b_{8s+(j+1)s,8s+(-2)s} &= e_{8(j+m+1)+4} \otimes w_{8j+4 \rightarrow 8(j+1)+4}; \\
b_{3s+(j+1)s,16s+(-2)s} &= w_{8(j+m+1)+5 \rightarrow 8(j+m+1)+7} \otimes w_{8j+7 \rightarrow 8(j+1)+1}; \\
b_{4s+(j+1)s,16s+(-2)s} &= -w_{8(j+m+1)+1 \rightarrow 8(j+m+1)+7} \otimes w_{8j+7 \rightarrow 8(j+1)+1}; \\
b_{5s+(j+1)s,16s+(-2)s} &= -w_{8(j+m+1)+2 \rightarrow 8(j+m+1)+7} \otimes w_{8j+7 \rightarrow 8(j+1)+2}.
\end{aligned}$$

(20) If  $r_0 = 19$ , then  $\Omega^9(Z_t^{(22)})$  is described with  $(16s \times 18s)$  matrix with the following nonzero entries:

$$\begin{aligned}
b_{2s+(j+1)s,(-3)s} &= w_{8(j+m+1)+1 \rightarrow 8(j+m+1)+2} \otimes w_{8j \rightarrow 8(j+1)}; \\
b_{j+4s,(-3)s} &= -w_{8(j+m+1) \rightarrow 8(j+m+1)+2} \otimes w_{8j \rightarrow 8j+1}; \\
b_{s+(j+1)s,s+(-2)s} &= -e_{8(j+m+1)+6} \otimes w_{8j \rightarrow 8(j+1)}; \\
b_{2s+(j+1)s,2s+(-3)s} &= w_{8(j+m+1)+1 \rightarrow 8(j+m+1)+4} \otimes w_{8j \rightarrow 8(j+1)}; \\
b_{2s+(j+1)s,3s+(-2)s} &= -e_{8(j+m+1)+1} \otimes w_{8j \rightarrow 8(j+1)}; \\
b_{2s+(j+1)s,3s+(-3)s} &= -e_{8(j+m+1)+1} \otimes w_{8j \rightarrow 8(j+1)}; \\
b_{(j+1)s,5s+(-2)s} &= w_{8(j+m+1)+3 \rightarrow 8(j+m+1)+7} \otimes w_{8j+1 \rightarrow 8(j+1)}; \\
b_{2s+(j+1)s,5s+(-2)s} &= -w_{8(j+m+1)+1 \rightarrow 8(j+m+1)+7} \otimes w_{8j+1 \rightarrow 8(j+1)}; \\
b_{(j+1)s,5s+(-3)s} &= -w_{8(j+m+1)+3 \rightarrow 8(j+m+1)+7} \otimes w_{8j+1 \rightarrow 8(j+1)}; \\
b_{2s+(j+1)s,5s+(-3)s} &= 2w_{8(j+m+1)+1 \rightarrow 8(j+m+1)+7} \otimes w_{8j+1 \rightarrow 8(j+1)}; \\
b_{(j+1)s,6s+(-2)s} &= w_{8(j+m+1)+3 \rightarrow 8(j+m+2)} \otimes w_{8j+2 \rightarrow 8(j+1)}; \\
b_{2s+(j+1)s,6s+(-2)s} &= -w_{8(j+m+1)+1 \rightarrow 8(j+m+2)} \otimes w_{8j+2 \rightarrow 8(j+1)}; \\
b_{(j+1)s,6s+(-3)s} &= -w_{8(j+m+1)+3 \rightarrow 8(j+m+2)} \otimes w_{8j+2 \rightarrow 8(j+1)}; \\
b_{2s+(j+1)s,6s+(-3)s} &= w_{8(j+m+1)+1 \rightarrow 8(j+m+2)} \otimes w_{8j+2 \rightarrow 8(j+1)}; \\
b_{2s+(j+1)s,7s+(-2)s} &= -w_{8(j+m+1)+1 \rightarrow 8(j+m+1)+7} \otimes w_{8j+3 \rightarrow 8(j+1)}; \\
b_{3s+(j+1)s,7s+(-2)s} &= w_{8(j+m+1)+5 \rightarrow 8(j+m+1)+7} \otimes w_{8j+3 \rightarrow 8(j+1)}; \\
b_{2s+(j+1)s,7s+(-3)s} &= w_{8(j+m+1)+1 \rightarrow 8(j+m+1)+7} \otimes w_{8j+3 \rightarrow 8(j+1)}; \\
b_{2s+(j+1)s,8s+(-2)s} &= -w_{8(j+m+1)+1 \rightarrow 8(j+m+1)+7} \otimes w_{8j+4 \rightarrow 8(j+1)}; \\
b_{3s+(j+1)s,8s+(-2)s} &= w_{8(j+m+1)+5 \rightarrow 8(j+m+1)+7} \otimes w_{8j+4 \rightarrow 8(j+1)};
\end{aligned}$$



$$b_{7s+(j+1)s,8s+(-2)s} = e_{8(j+m+1)+7} \otimes w_{8j+4 \rightarrow 8(j+1)+4};$$

$$b_{4s+(j+1)s,14s+(-2)s} = -w_{8(j+m+2) \rightarrow 8(j+m+2)+5} \otimes w_{8j+7 \rightarrow 8(j+1)+1}.$$

(21) If  $r_0 = 20$ , then  $\Omega^{20}(Z_t^{(22)})$  is described with  $(16s \times 19s)$  matrix with the following nonzero entries:

$$b_{(j+1)s,(-2)s} = e_{8(j+m)+7} \otimes w_{8j \rightarrow 8(j+1)};$$

$$b_{(j+1)s,(-3)s} = -e_{8(j+m)+7} \otimes w_{8j \rightarrow 8(j+1)};$$

$$b_{j+3s,(-3)s} = -w_{8(j+m)+6 \rightarrow 8(j+m)+7} \otimes w_{8j \rightarrow 8j+1};$$

$$b_{s+(j+1)s,s+(-2)s} = -e_{8(j+m+1)} \otimes w_{8j \rightarrow 8(j+1)};$$

$$b_{(j+1)s,s+(-3)s} = w_{8(j+m)+7 \rightarrow 8(j+m+1)} \otimes w_{8j \rightarrow 8(j+1)};$$

$$b_{j+2s,s+(-3)s} = w_{8(j+m)+6 \rightarrow 8(j+m+1)} \otimes w_{8j \rightarrow 8j+1};$$

$$b_{(j+1)s,3s+(-4)s} = w_{8(j+m)+7 \rightarrow 8(j+m+1)+2} \otimes w_{8j+1 \rightarrow 8(j+1)};$$

$$b_{s+(j+1)s,3s+(-4)s} = -w_{8(j+m+1) \rightarrow 8(j+m+1)+2} \otimes w_{8j+1 \rightarrow 8(j+1)};$$

$$b_{s+(j+1)s,4s+(-4)s} = w_{8(j+m+1) \rightarrow 8(j+m+1)+3} \otimes w_{8j+2 \rightarrow 8(j+1)};$$

$$b_{j,4s+(-4)s} = w_{8(j+m)+3 \rightarrow 8(j+m+1)+3} \otimes e_{8j+2};$$

$$b_{j,4s+(-2)s} = w_{8(j+m)+3 \rightarrow 8(j+m+1)+3} \otimes e_{8j+2};$$

$$b_{j,4s+(-3)s} = -w_{8(j+m)+3 \rightarrow 8(j+m+1)+3} \otimes e_{8j+2};$$

$$b_{(j+1)s,6s+(-4)s} = w_{8(j+m)+7 \rightarrow 8(j+m+1)+4} \otimes w_{8j+3 \rightarrow 8(j+1)};$$

$$b_{s+(j+1)s,6s+(-4)s} = -w_{8(j+m+1) \rightarrow 8(j+m+1)+4} \otimes w_{8j+3 \rightarrow 8(j+1)};$$

$$b_{4s+(j+1)s,6s+(-4)s} = -w_{8(j+m+1)+3 \rightarrow 8(j+m+1)+4} \otimes w_{8j+3 \rightarrow 8(j+1)+2};$$

$$b_{s+(j+1)s,8s+(-2)s} = w_{8(j+m+1) \rightarrow 8(j+m+1)+5} \otimes w_{8j+4 \rightarrow 8(j+1)};$$

$$b_{6s+(j+1)s,8s+(-2)s} = e_{8(j+m+1)+5} \otimes w_{8j+4 \rightarrow 8(j+1)+3};$$

$$b_{3s+(j+1)s,16s+(-2)s} = -w_{8(j+m+1)+6 \rightarrow 8(j+m+1)+7} \otimes w_{8j+7 \rightarrow 8(j+1)+1}.$$

(22) If  $r_0 = 21$ , then  $\Omega^{21}(Z_t^{(22)})$  is described with  $(14s \times 18s)$  matrix with the following nonzero entries:

$$b_{(j+1)s,(-4)s} = -e_{8(j+m+1)+2} \otimes w_{8j \rightarrow 8(j+1)};$$

$$b_{(j+1)s,(-2)s} = -e_{8(j+m+1)+2} \otimes w_{8j \rightarrow 8(j+1)};$$

$$b_{j+2s,s+(-4)s} = -w_{8(j+m)+7 \rightarrow 8(j+m+1)+3} \otimes w_{8j \rightarrow 8j+1};$$

$$b_{j+2s,s+(-3)s} = w_{8(j+m)+7 \rightarrow 8(j+m+1)+3} \otimes w_{8j \rightarrow 8j+1};$$

$$b_{j+2s,s+(-2)s} = -w_{8(j+m)+7 \rightarrow 8(j+m+1)+3} \otimes w_{8j \rightarrow 8j+1};$$

$$b_{j,3s+(-3)s} = -w_{8(j+m)+7 \rightarrow 8(j+m+1)+5} \otimes w_{8j \rightarrow 8j+1};$$

$$b_{2s+(j+1)s,4s+(-4)s} = w_{8(j+m+1)+6 \rightarrow 8(j+m+2)} \otimes w_{8j+1 \rightarrow 8(j+1)};$$

$$b_{(j+1)s,5s+(-4)s} = -w_{8(j+m+1)+2 \rightarrow 8(j+m+1)+7} \otimes w_{8j+2 \rightarrow 8(j+1)};$$

$$b_{s+(j+1)s,5s+(-4)s} = -w_{8(j+m+1)+4 \rightarrow 8(j+m+1)+7} \otimes w_{8j+2 \rightarrow 8(j+1)};$$

$$b_{(j+1)s,6s+(-4)s} = w_{8(j+m+1)+2 \rightarrow 8(j+m+1)+7} \otimes w_{8j+3 \rightarrow 8(j+1)};$$

$$b_{3s+(j+1)s,6s+(-4)s} = e_{8(j+m+1)+7} \otimes w_{8j+3 \rightarrow 8(j+1)+1};$$

$$b_{2s+(j+1)s,6s+(-2)s} = -w_{8(j+m+1)+6 \rightarrow 8(j+m+1)+7} \otimes w_{8j+3 \rightarrow 8(j+1)};$$

$$b_{2s+(j+1)s,7s+(-2)s} = -w_{8(j+m+1)+6 \rightarrow 8(j+m+2)} \otimes w_{8j+3 \rightarrow 8(j+1)};$$

$$b_{2s+(j+1)s,8s+(-2)s} = -w_{8(j+m+1)+6 \rightarrow 8(j+m+2)} \otimes w_{8j+4 \rightarrow 8(j+1)};$$

$$b_{6s+(j+1)s,8s+(-2)s} = e_{8(j+m+2)} \otimes w_{8j+4 \rightarrow 8(j+1)+4};$$

$$b_{3s+(j+1)s,14s+(-4)s} = w_{8(j+m+1)+7 \rightarrow 8(j+m+2)+6} \otimes w_{8j+7 \rightarrow 8(j+1)+1};$$

$$b_{3s+(j+1)s,14s+(-2)s} = w_{8(j+m+1)+7 \rightarrow 8(j+m+2)+6} \otimes w_{8j+7 \rightarrow 8(j+1)+1}.$$

(23) If  $r_0 = 22$ , then  $\Omega^{22}(Z_t^{(22)})$  is described with  $(13s \times 20s)$  matrix with the following nonzero entries:

$$\begin{aligned} b_{j+2s,(-4)s} &= -w_{8(j+m)+3 \rightarrow 8(j+m)+7} \otimes w_{8j \rightarrow 8j+1}; \\ b_{j+3s,(-4)s} &= w_{8(j+m)+4 \rightarrow 8(j+m)+7} \otimes w_{8j \rightarrow 8j+2}; \\ b_{s+(j+1)s,(-2)s} &= e_{8(j+m)+7} \otimes w_{8j \rightarrow 8(j+1)}; \\ b_{j+2s,(-2)s} &= -w_{8(j+m)+3 \rightarrow 8(j+m)+7} \otimes w_{8j \rightarrow 8j+1}; \\ b_{j+3s,(-2)s} &= w_{8(j+m)+4 \rightarrow 8(j+m)+7} \otimes w_{8j \rightarrow 8j+2}; \\ b_{s+(j+1)s,s+(-4)s} &= -w_{8(j+m)+7 \rightarrow 8(j+m+1)} \otimes w_{8j \rightarrow 8(j+1)}; \\ b_{(j+1)s,3s+(-4)s} &= -w_{8(j+m+1) \rightarrow 8(j+m+1)+3} \otimes w_{8j+1 \rightarrow 8(j+1)}; \\ b_{s+(j+1)s,3s+(-4)s} &= w_{8(j+m)+7 \rightarrow 8(j+m+1)+3} \otimes w_{8j+1 \rightarrow 8(j+1)}; \\ b_{(j+1)s,3s+(-3)s} &= w_{8(j+m+1) \rightarrow 8(j+m+1)+3} \otimes w_{8j+1 \rightarrow 8(j+1)}; \\ b_{s+(j+1)s,3s+(-3)s} &= -w_{8(j+m)+7 \rightarrow 8(j+m+1)+3} \otimes w_{8j+1 \rightarrow 8(j+1)}; \\ b_{(j+1)s,3s+(-5)s} &= w_{8(j+m+1) \rightarrow 8(j+m+1)+3} \otimes w_{8j+1 \rightarrow 8(j+1)}; \\ b_{s+(j+1)s,3s+(-5)s} &= -w_{8(j+m)+7 \rightarrow 8(j+m+1)+3} \otimes w_{8j+1 \rightarrow 8(j+1)}; \\ b_{s+(j+1)s,4s+(-4)s} &= -w_{8(j+m)+7 \rightarrow 8(j+m+1)+5} \otimes w_{8j+1 \rightarrow 8(j+1)}; \\ b_{j-2s,5s+(-4)s} &= -w_{8(j+m)+4 \rightarrow 8(j+m+1)+4} \otimes e_{8j+2}; \\ b_{s+(j+1)s,5s+(-3)s} &= w_{8(j+m)+7 \rightarrow 8(j+m+1)+4} \otimes w_{8j+2 \rightarrow 8(j+1)}; \\ b_{j-2s,5s+(-3)s} &= w_{8(j+m)+4 \rightarrow 8(j+m+1)+4} \otimes e_{8j+2}; \\ b_{s+(j+1)s,5s+(-5)s} &= w_{8(j+m)+7 \rightarrow 8(j+m+1)+4} \otimes w_{8j+2 \rightarrow 8(j+1)}; \\ b_{j-2s,5s+(-5)s} &= w_{8(j+m)+4 \rightarrow 8(j+m+1)+4} \otimes e_{8j+2}; \\ b_{6s+(j+1)s,9s+(-2)s} &= w_{8(j+m+1)+1 \rightarrow 8(j+m+1)+2} \otimes w_{8j+4 \rightarrow 8(j+1)+4}; \\ b_{s+(j+1)s,10s+(-2)s} &= -w_{8(j+m)+7 \rightarrow 8(j+m+1)+6} \otimes w_{8j+4 \rightarrow 8(j+1)}; \\ b_{5s+(j+1)s,10s+(-2)s} &= -e_{8(j+m+1)+6} \otimes w_{8j+4 \rightarrow 8(j+1)+3}; \\ b_{2s+(j+1)s,17s+(-2)s} &= w_{8(j+m+1)+3 \rightarrow 8(j+m+1)+7} \otimes w_{8j+7 \rightarrow 8(j+1)+1}; \\ b_{3s+(j+1)s,17s+(-2)s} &= -w_{8(j+m+1)+4 \rightarrow 8(j+m+1)+7} \otimes w_{8j+7 \rightarrow 8(j+1)+2}. \end{aligned}$$

(24) If  $r_0 = 23$ , then  $\Omega^{23}(Z_t^{(22)})$  is described with  $(11s \times 18s)$  matrix with the following nonzero entries:

$$\begin{aligned} b_{j+2s,(-4)s} &= -w_{8(j+m+1) \rightarrow 8(j+m+1)+3} \otimes w_{8j \rightarrow 8j+1}; \\ b_{(j+1)s,(-3)s} &= -e_{8(j+m+1)+3} \otimes w_{8j \rightarrow 8(j+1)}; \\ b_{(j+1)s,(-2)s} &= -e_{8(j+m+1)+3} \otimes w_{8j \rightarrow 8(j+1)}; \\ b_{j+2s,(-2)s} &= -w_{8(j+m+1) \rightarrow 8(j+m+1)+3} \otimes w_{8j \rightarrow 8j+1}; \\ b_{(j+1)s,(-5)s} &= -e_{8(j+m+1)+3} \otimes w_{8j \rightarrow 8(j+1)}; \\ b_{j,2s+(-4)s} &= w_{8(j+m+1) \rightarrow 8(j+m+1)+4} \otimes w_{8j \rightarrow 8j+1}; \\ b_{j,2s+(-3)s} &= -w_{8(j+m+1) \rightarrow 8(j+m+1)+4} \otimes w_{8j \rightarrow 8j+1}; \\ b_{j,2s+(-5)s} &= -w_{8(j+m+1) \rightarrow 8(j+m+1)+4} \otimes w_{8j \rightarrow 8j+1}; \\ b_{s+(j+1)s,5s+(-4)s} &= w_{8(j+m+1)+5 \rightarrow 8(j+m+1)+7} \otimes w_{8j+1 \rightarrow 8(j+1)}; \\ b_{(j+1)s,5s+(-3)s} &= -w_{8(j+m+1)+3 \rightarrow 8(j+m+1)+7} \otimes w_{8j+1 \rightarrow 8(j+1)}; \\ b_{(j+1)s,5s+(-5)s} &= -w_{8(j+m+1)+3 \rightarrow 8(j+m+1)+7} \otimes w_{8j+1 \rightarrow 8(j+1)}; \\ b_{(j+1)s,6s+(-3)s} &= -w_{8(j+m+1)+3 \rightarrow 8(j+m+1)+7} \otimes w_{8j+2 \rightarrow 8(j+1)}; \end{aligned}$$

$$\begin{aligned}
b_{s+(j+1)s,6s+(-3)s} &= w_{8(j+m+1)+5 \rightarrow 8(j+m+1)+7} \otimes w_{8j+2 \rightarrow 8(j+1)}; \\
b_{3s+(j+1)s,6s+(-3)s} &= -e_{8(j+m+1)+7} \otimes w_{8j+2 \rightarrow 8(j+1)+2}; \\
b_{(j+1)s,6s+(-5)s} &= -w_{8(j+m+1)+3 \rightarrow 8(j+m+1)+7} \otimes w_{8j+2 \rightarrow 8(j+1)}; \\
b_{s+(j+1)s,6s+(-5)s} &= w_{8(j+m+1)+5 \rightarrow 8(j+m+1)+7} \otimes w_{8j+2 \rightarrow 8(j+1)}; \\
b_{3s+(j+1)s,6s+(-5)s} &= -e_{8(j+m+1)+7} \otimes w_{8j+2 \rightarrow 8(j+1)+2}; \\
b_{2s+(j+1)s,8s+(-3)s} &= e_{8(j+m+2)} \otimes w_{8j+3 \rightarrow 8(j+1)+1}; \\
b_{2s+(j+1)s,8s+(-5)s} &= e_{8(j+m+2)} \otimes w_{8j+3 \rightarrow 8(j+1)+1}; \\
b_{(j+1)s,9s+(-2)s} &= w_{8(j+m+1)+3 \rightarrow 8(j+m+1)+7} \otimes w_{8j+4 \rightarrow 8(j+1)}; \\
b_{s+(j+1)s,9s+(-2)s} &= -w_{8(j+m+1)+5 \rightarrow 8(j+m+1)+7} \otimes w_{8j+4 \rightarrow 8(j+1)}; \\
b_{3s+(j+1)s,9s+(-2)s} &= e_{8(j+m+1)+7} \otimes w_{8j+4 \rightarrow 8(j+1)+2}; \\
b_{2s+(j+1)s,14s+(-3)s} &= -w_{8(j+m+2) \rightarrow 8(j+m+2)+2} \otimes w_{8j+7 \rightarrow 8(j+1)+1}; \\
b_{2s+(j+1)s,14s+(-2)s} &= -w_{8(j+m+2) \rightarrow 8(j+m+2)+2} \otimes w_{8j+7 \rightarrow 8(j+1)+1}; \\
b_{2s+(j+1)s,14s+(-5)s} &= -w_{8(j+m+2) \rightarrow 8(j+m+2)+2} \otimes w_{8j+7 \rightarrow 8(j+1)+1}; \\
b_{2s+(j+1)s,15s+(-2)s} &= w_{8(j+m+2) \rightarrow 8(j+m+2)+3} \otimes w_{8j+7 \rightarrow 8(j+1)+1}.
\end{aligned}$$

(25) If  $r_0 = 24$ , then  $\Omega^{24}(Z_t^{(22)})$  is described with  $(11s \times 19s)$  matrix with the following nonzero entries:

$$\begin{aligned}
b_{j+2s,(-4)s} &= w_{8(j+m)+5 \rightarrow 8(j+m)+7} \otimes w_{8j \rightarrow 8j+1}; \\
b_{j+2s,(-2)s} &= w_{8(j+m)+5 \rightarrow 8(j+m)+7} \otimes w_{8j \rightarrow 8j+1}; \\
b_{j+s,s+(-3)s} &= -w_{8(j+m)+5 \rightarrow 8(j+m+1)} \otimes w_{8j \rightarrow 8j+1}; \\
b_{(j+1)s,s+(-2)s} &= -e_{8(j+m+1)} \otimes w_{8j \rightarrow 8(j+1)}; \\
b_{j+s,s+(-2)s} &= -w_{8(j+m)+5 \rightarrow 8(j+m+1)} \otimes w_{8j \rightarrow 8j+1}; \\
b_{j+s,s+(-5)s} &= -w_{8(j+m)+5 \rightarrow 8(j+m+1)} \otimes w_{8j \rightarrow 8j+1}; \\
b_{j,2s+(-4)s} &= w_{8(j+m)+5 \rightarrow 8(j+m)+7} \otimes w_{8j \rightarrow 8j+1}; \\
b_{j,2s+(-3)s} &= -w_{8(j+m)+5 \rightarrow 8(j+m)+7} \otimes w_{8j \rightarrow 8j+1}; \\
b_{j,2s+(-5)s} &= -w_{8(j+m)+5 \rightarrow 8(j+m)+7} \otimes w_{8j \rightarrow 8j+1}; \\
b_{(j+1)s,3s+(-4)s} &= w_{8(j+m+1) \rightarrow 8(j+m+1)+4} \otimes w_{8j+1 \rightarrow 8(j+1)}; \\
b_{(j+1)s,3s+(-3)s} &= w_{8(j+m+1) \rightarrow 8(j+m+1)+4} \otimes w_{8j+1 \rightarrow 8(j+1)}; \\
b_{(j+1)s,3s+(-6)s} &= w_{8(j+m+1) \rightarrow 8(j+m+1)+4} \otimes w_{8j+1 \rightarrow 8(j+1)}; \\
b_{(j+1)s,5s+(-3)s} &= w_{8(j+m+1) \rightarrow 8(j+m+1)+5} \otimes w_{8j+2 \rightarrow 8(j+1)}; \\
b_{(j+1)s,5s+(-5)s} &= w_{8(j+m+1) \rightarrow 8(j+m+1)+5} \otimes w_{8j+2 \rightarrow 8(j+1)}; \\
b_{(j+1)s,7s+(-2)s} &= -w_{8(j+m+1) \rightarrow 8(j+m+1)+2} \otimes w_{8j+3 \rightarrow 8(j+1)}; \\
b_{4s+(j+1)s,7s+(-2)s} &= w_{8(j+m+1)+1 \rightarrow 8(j+m+1)+2} \otimes w_{8j+3 \rightarrow 8(j+1)+3}; \\
b_{2s+(j+1)s,8s+(-3)s} &= -w_{8(j+m+1)+5 \rightarrow 8(j+m+1)+6} \otimes w_{8j+3 \rightarrow 8(j+1)+1}; \\
b_{2s+(j+1)s,8s+(-5)s} &= -w_{8(j+m+1)+5 \rightarrow 8(j+m+1)+6} \otimes w_{8j+3 \rightarrow 8(j+1)+1}; \\
b_{(j+1)s,9s+(-2)s} &= w_{8(j+m+1) \rightarrow 8(j+m+1)+3} \otimes w_{8j+4 \rightarrow 8(j+1)}; \\
b_{4s+(j+1)s,9s+(-2)s} &= -w_{8(j+m+1)+1 \rightarrow 8(j+m+1)+3} \otimes w_{8j+4 \rightarrow 8(j+1)+3}; \\
b_{5s+(j+1)s,9s+(-2)s} &= w_{8(j+m+1)+2 \rightarrow 8(j+m+1)+3} \otimes w_{8j+4 \rightarrow 8(j+1)+4}; \\
b_{2s+(j+1)s,17s+(-2)s} &= w_{8(j+m+1)+5 \rightarrow 8(j+m+2)} \otimes w_{8j+7 \rightarrow 8(j+1)+1}.
\end{aligned}$$

(26) If  $r_0 = 25$ , then  $\Omega^{25}(Z_t^{(22)})$  is described with  $(10s \times 18s)$  matrix with the following nonzero entries:

$$\begin{aligned}
b_{(j+1)_s, s+(-4)_s} &= -e_{8(j+m+1)+4} \otimes w_{8j \rightarrow 8(j+1)}; \\
b_{(j+1)_s, s+(-3)_s} &= -e_{8(j+m+1)+4} \otimes w_{8j \rightarrow 8(j+1)}; \\
b_{(j+1)_s, s+(-2)_s} &= -e_{8(j+m+1)+4} \otimes w_{8j \rightarrow 8(j+1)}; \\
b_{(j+1)_s, s+(-6)_s} &= -e_{8(j+m+1)+4} \otimes w_{8j \rightarrow 8(j+1)}; \\
b_{s+(j+1)_s, 2s+(-3)_s} &= -e_{8(j+m+1)+6} \otimes w_{8j \rightarrow 8(j+1)}; \\
b_{s+(j+1)_s, 2s+(-5)_s} &= -e_{8(j+m+1)+6} \otimes w_{8j \rightarrow 8(j+1)}; \\
b_{j-s, 3s+(-3)_s} &= w_{8(j+m)+7 \rightarrow 8(j+m+1)+5} \otimes w_{8j \rightarrow 8j+1}; \\
b_{j, 3s+(-3)_s} &= w_{8(j+m+1) \rightarrow 8(j+m+1)+5} \otimes w_{8j \rightarrow 8j+2}; \\
b_{j+4s, 3s+(-3)_s} &= w_{8(j+m+1) \rightarrow 8(j+m+1)+5} \otimes w_{8j \rightarrow 8j+6}; \\
b_{j-s, 3s+(-2)_s} &= w_{8(j+m)+7 \rightarrow 8(j+m+1)+5} \otimes w_{8j \rightarrow 8j+1}; \\
b_{j, 3s+(-2)_s} &= w_{8(j+m+1) \rightarrow 8(j+m+1)+5} \otimes w_{8j \rightarrow 8j+2}; \\
b_{j+4s, 3s+(-2)_s} &= w_{8(j+m+1) \rightarrow 8(j+m+1)+5} \otimes w_{8j \rightarrow 8j+6}; \\
b_{j-s, 3s+(-5)_s} &= w_{8(j+m)+7 \rightarrow 8(j+m+1)+5} \otimes w_{8j \rightarrow 8j+1}; \\
b_{j, 3s+(-5)_s} &= w_{8(j+m+1) \rightarrow 8(j+m+1)+5} \otimes w_{8j \rightarrow 8j+2}; \\
b_{j+4s, 3s+(-5)_s} &= w_{8(j+m+1) \rightarrow 8(j+m+1)+5} \otimes w_{8j \rightarrow 8j+6}; \\
b_{s+(j+1)_s, 4s+(-4)_s} &= w_{8(j+m+1)+6 \rightarrow 8(j+m+1)+7} \otimes w_{8j+1 \rightarrow 8(j+1)}; \\
b_{s+(j+1)_s, 4s+(-3)_s} &= w_{8(j+m+1)+6 \rightarrow 8(j+m+1)+7} \otimes w_{8j+1 \rightarrow 8(j+1)}; \\
b_{s+(j+1)_s, 4s+(-6)_s} &= w_{8(j+m+1)+6 \rightarrow 8(j+m+1)+7} \otimes w_{8j+1 \rightarrow 8(j+1)}; \\
b_{s+(j+1)_s, 6s+(-3)_s} &= -w_{8(j+m+1)+6 \rightarrow 8(j+m+2)} \otimes w_{8j+2 \rightarrow 8(j+1)}; \\
b_{3s+(j+1)_s, 6s+(-3)_s} &= -e_{8(j+m+2)} \otimes w_{8j+2 \rightarrow 8(j+1)+2}; \\
b_{s+(j+1)_s, 6s+(-5)_s} &= -w_{8(j+m+1)+6 \rightarrow 8(j+m+2)} \otimes w_{8j+2 \rightarrow 8(j+1)}; \\
b_{3s+(j+1)_s, 6s+(-5)_s} &= -e_{8(j+m+2)} \otimes w_{8j+2 \rightarrow 8(j+1)+2}; \\
b_{s+(j+1)_s, 8s+(-2)_s} &= w_{8(j+m+1)+6 \rightarrow 8(j+m+2)} \otimes w_{8j+4 \rightarrow 8(j+1)}; \\
b_{3s+(j+1)_s, 8s+(-2)_s} &= e_{8(j+m+2)} \otimes w_{8j+4 \rightarrow 8(j+1)+2}; \\
b_{2s+(j+1)_s, 17s+(-2)_s} &= -w_{8(j+m+1)+7 \rightarrow 8(j+m+2)+5} \otimes w_{8j+7 \rightarrow 8(j+1)+1}; \\
b_{3s+(j+1)_s, 17s+(-2)_s} &= -w_{8(j+m+2) \rightarrow 8(j+m+2)+5} \otimes w_{8j+7 \rightarrow 8(j+1)+2}; \\
b_{7s+(j+1)_s, 17s+(-2)_s} &= -w_{8(j+m+2) \rightarrow 8(j+m+2)+5} \otimes w_{8j+7 \rightarrow 8(j+1)+6}.
\end{aligned}$$

(27) If  $r_0 = 26$ , then  $\Omega^{26}(Z_t^{(22)})$  is described with  $(8s \times 19s)$  matrix with the following nonzero entries:

$$\begin{aligned}
b_{j, (-5)_s} &= w_{8(j+m-1)+7 \rightarrow 8(j+m)+7} \otimes e_{8j}; \\
b_{(j+1)_s, (-5)_s} &= -e_{8(j+m)+7} \otimes w_{8j \rightarrow 8(j+1)}; \\
b_{j+2s, (-5)_s} &= w_{8(j+m)+1 \rightarrow 8(j+m)+7} \otimes w_{8j \rightarrow 8j+2}; \\
b_{j+3s, (-5)_s} &= -w_{8(j+m)+2 \rightarrow 8(j+m)+7} \otimes w_{8j \rightarrow 8j+3}; \\
b_{j+4s, (-5)_s} &= w_{8(j+m)+3 \rightarrow 8(j+m)+7} \otimes w_{8j \rightarrow 8j+4}; \\
b_{j+5s, (-5)_s} &= w_{8(j+m)+4 \rightarrow 8(j+m)+7} \otimes w_{8j \rightarrow 8j+5}; \\
b_{(j+1)_s, (-4)_s} &= e_{8(j+m)+7} \otimes w_{8j \rightarrow 8(j+1)}; \\
b_{j, (-3)_s} &= w_{8(j+m-1)+7 \rightarrow 8(j+m)+7} \otimes e_{8j}; \\
b_{j+2s, (-3)_s} &= w_{8(j+m)+1 \rightarrow 8(j+m)+7} \otimes w_{8j \rightarrow 8j+2};
\end{aligned}$$

$$\begin{aligned}
b_{j+3s,(-3)_s} &= -w_{8(j+m)+2 \rightarrow 8(j+m)+7} \otimes w_{8j \rightarrow 8j+3}; \\
b_{j+4s,(-3)_s} &= w_{8(j+m)+3 \rightarrow 8(j+m)+7} \otimes w_{8j \rightarrow 8j+4}; \\
b_{j+5s,(-3)_s} &= w_{8(j+m)+4 \rightarrow 8(j+m)+7} \otimes w_{8j \rightarrow 8j+5}; \\
b_{j,(-2)_s} &= w_{8(j+m-1)+7 \rightarrow 8(j+m)+7} \otimes e_{8j}; \\
b_{j+2s,(-2)_s} &= w_{8(j+m)+1 \rightarrow 8(j+m)+7} \otimes w_{8j \rightarrow 8j+2}; \\
b_{j+3s,(-2)_s} &= -w_{8(j+m)+2 \rightarrow 8(j+m)+7} \otimes w_{8j \rightarrow 8j+3}; \\
b_{j+4s,(-2)_s} &= w_{8(j+m)+3 \rightarrow 8(j+m)+7} \otimes w_{8j \rightarrow 8j+4}; \\
b_{j+5s,(-2)_s} &= w_{8(j+m)+4 \rightarrow 8(j+m)+7} \otimes w_{8j \rightarrow 8j+5}; \\
b_{(j+1)_s,(-6)_s} &= e_{8(j+m)+7} \otimes w_{8j \rightarrow 8(j+1)}; \\
b_{(j+1)_s,s+(-4)_s} &= w_{8(j+m)+7 \rightarrow 8(j+m+1)} \otimes w_{8j \rightarrow 8(j+1)}; \\
b_{(j+1)_s,s+(-3)_s} &= w_{8(j+m)+7 \rightarrow 8(j+m+1)} \otimes w_{8j \rightarrow 8(j+1)}; \\
b_{(j+1)_s,s+(-2)_s} &= w_{8(j+m)+7 \rightarrow 8(j+m+1)} \otimes w_{8j \rightarrow 8(j+1)}; \\
b_{(j+1)_s,s+(-6)_s} &= w_{8(j+m)+7 \rightarrow 8(j+m+1)} \otimes w_{8j \rightarrow 8(j+1)}; \\
b_{(j+1)_s,3s+(-4)_s} &= w_{8(j+m)+7 \rightarrow 8(j+m+1)+5} \otimes w_{8j+1 \rightarrow 8(j+1)}; \\
b_{(j+1)_s,3s+(-3)_s} &= w_{8(j+m)+7 \rightarrow 8(j+m+1)+5} \otimes w_{8j+1 \rightarrow 8(j+1)}; \\
b_{(j+1)_s,3s+(-6)_s} &= w_{8(j+m)+7 \rightarrow 8(j+m+1)+5} \otimes w_{8j+1 \rightarrow 8(j+1)}; \\
b_{2s+(j+1)_s,5s+(-5)_s} &= -w_{8(j+m+1)+1 \rightarrow 8(j+m+1)+2} \otimes w_{8j+2 \rightarrow 8(j+1)+2}; \\
b_{2s+(j+1)_s,5s+(-3)_s} &= -w_{8(j+m+1)+1 \rightarrow 8(j+m+1)+2} \otimes w_{8j+2 \rightarrow 8(j+1)+2}; \\
b_{(j+1)_s,6s+(-5)_s} &= -w_{8(j+m)+7 \rightarrow 8(j+m+1)+6} \otimes w_{8j+2 \rightarrow 8(j+1)}; \\
b_{s+(j+1)_s,6s+(-5)_s} &= e_{8(j+m+1)+6} \otimes w_{8j+2 \rightarrow 8(j+1)+1}; \\
b_{s+(j+1)_s,6s+(-4)_s} &= -e_{8(j+m+1)+6} \otimes w_{8j+2 \rightarrow 8(j+1)+1}; \\
b_{(j+1)_s,6s+(-3)_s} &= -w_{8(j+m)+7 \rightarrow 8(j+m+1)+6} \otimes w_{8j+2 \rightarrow 8(j+1)}; \\
b_{s+(j+1)_s,6s+(-6)_s} &= -e_{8(j+m+1)+6} \otimes w_{8j+2 \rightarrow 8(j+1)+1}; \\
b_{2s+(j+1)_s,7s+(-2)_s} &= -w_{8(j+m+1)+1 \rightarrow 8(j+m+1)+3} \otimes w_{8j+3 \rightarrow 8(j+1)+2}; \\
b_{3s+(j+1)_s,7s+(-2)_s} &= w_{8(j+m+1)+2 \rightarrow 8(j+m+1)+3} \otimes w_{8j+3 \rightarrow 8(j+1)+3}; \\
b_{2s+(j+1)_s,8s+(-2)_s} &= w_{8(j+m+1)+1 \rightarrow 8(j+m+1)+4} \otimes w_{8j+4 \rightarrow 8(j+1)+2}; \\
b_{3s+(j+1)_s,8s+(-2)_s} &= -w_{8(j+m+1)+2 \rightarrow 8(j+m+1)+4} \otimes w_{8j+4 \rightarrow 8(j+1)+3}; \\
b_{4s+(j+1)_s,8s+(-2)_s} &= w_{8(j+m+1)+3 \rightarrow 8(j+m+1)+4} \otimes w_{8j+4 \rightarrow 8(j+1)+4}; \\
b_{(j+1)_s,9s+(-2)_s} &= -w_{8(j+m)+7 \rightarrow 8(j+m+1)+5} \otimes w_{8j+4 \rightarrow 8(j+1)}; \\
b_{(j+1)_s,16s+(-2)_s} &= w_{8(j+m)+7 \rightarrow 8(j+m+1)+7} \otimes w_{8j+7 \rightarrow 8(j+1)}; \\
b_{2s+(j+1)_s,16s+(-2)_s} &= w_{8(j+m+1)+1 \rightarrow 8(j+m+1)+7} \otimes w_{8j+7 \rightarrow 8(j+1)+2}; \\
b_{3s+(j+1)_s,16s+(-2)_s} &= -w_{8(j+m+1)+2 \rightarrow 8(j+m+1)+7} \otimes w_{8j+7 \rightarrow 8(j+1)+3}; \\
b_{4s+(j+1)_s,16s+(-2)_s} &= w_{8(j+m+1)+3 \rightarrow 8(j+m+1)+7} \otimes w_{8j+7 \rightarrow 8(j+1)+4}; \\
b_{5s+(j+1)_s,16s+(-2)_s} &= w_{8(j+m+1)+4 \rightarrow 8(j+m+1)+7} \otimes w_{8j+7 \rightarrow 8(j+1)+5}; \\
b_{(j+1)_s,18s+(-2)_s} &= w_{8(j+m)+7 \rightarrow 8(j+m+1)+7} \otimes w_{8j+7 \rightarrow 8(j+1)}; \\
b_{2s+(j+1)_s,18s+(-2)_s} &= w_{8(j+m+1)+1 \rightarrow 8(j+m+1)+7} \otimes w_{8j+7 \rightarrow 8(j+1)+2}; \\
b_{3s+(j+1)_s,18s+(-2)_s} &= -w_{8(j+m+1)+2 \rightarrow 8(j+m+1)+7} \otimes w_{8j+7 \rightarrow 8(j+1)+3}; \\
b_{4s+(j+1)_s,18s+(-2)_s} &= w_{8(j+m+1)+3 \rightarrow 8(j+m+1)+7} \otimes w_{8j+7 \rightarrow 8(j+1)+4}; \\
b_{5s+(j+1)_s,18s+(-2)_s} &= w_{8(j+m+1)+4 \rightarrow 8(j+m+1)+7} \otimes w_{8j+7 \rightarrow 8(j+1)+5}.
\end{aligned}$$

(28) If  $r_0 = 27$ , then  $\Omega^{27}(Z_t^{(22)})$  is described with  $(9s \times 16s)$  matrix with the following nonzero entries:

$$\begin{aligned}
b_{j+s,(-5)_s} &= -w_{8(j+m+1) \rightarrow 8(j+m+1)+3} \otimes w_{8j \rightarrow 8j+1}; \\
b_{j+5s,(-5)_s} &= w_{8(j+m+1) \rightarrow 8(j+m+1)+3} \otimes w_{8j \rightarrow 8j+5}; \\
b_{j+s,(-3)_s} &= -w_{8(j+m+1) \rightarrow 8(j+m+1)+3} \otimes w_{8j \rightarrow 8j+1}; \\
b_{j+5s,(-3)_s} &= w_{8(j+m+1) \rightarrow 8(j+m+1)+3} \otimes w_{8j \rightarrow 8j+5}; \\
b_{j+s,(-2)_s} &= -w_{8(j+m+1) \rightarrow 8(j+m+1)+3} \otimes w_{8j \rightarrow 8j+1}; \\
b_{j+5s,(-2)_s} &= w_{8(j+m+1) \rightarrow 8(j+m+1)+3} \otimes w_{8j \rightarrow 8j+5}; \\
b_{j-3s,5s+(-5)_s} &= w_{8(j+m+1)+1 \rightarrow 8(j+m+1)+7} \otimes e_{8j+2}; \\
b_{j+3s,5s+(-5)_s} &= -w_{8(j+m+1)+6 \rightarrow 8(j+m+1)+7} \otimes w_{8j+2 \rightarrow 8j+7}; \\
b_{j-3s,5s+(-4)_s} &= -w_{8(j+m+1)+1 \rightarrow 8(j+m+1)+7} \otimes e_{8j+2}; \\
b_{j+3s,5s+(-4)_s} &= w_{8(j+m+1)+6 \rightarrow 8(j+m+1)+7} \otimes w_{8j+2 \rightarrow 8j+7}; \\
b_{j-3s,5s+(-6)_s} &= -w_{8(j+m+1)+1 \rightarrow 8(j+m+1)+7} \otimes e_{8j+2}; \\
b_{j+3s,5s+(-6)_s} &= w_{8(j+m+1)+6 \rightarrow 8(j+m+1)+7} \otimes w_{8j+2 \rightarrow 8j+7}; \\
b_{j-3s,8s+(-4)_s} &= -w_{8(j+m+1) \rightarrow 8(j+m+1)+7} \otimes e_{8j+5}; \\
b_{j-s,8s+(-4)_s} &= -w_{8(j+m+1)+4 \rightarrow 8(j+m+1)+7} \otimes w_{8j+5 \rightarrow 8j+7}; \\
b_{j-3s,8s+(-3)_s} &= -w_{8(j+m+1) \rightarrow 8(j+m+1)+7} \otimes e_{8j+5}; \\
b_{j-s,8s+(-3)_s} &= -w_{8(j+m+1)+4 \rightarrow 8(j+m+1)+7} \otimes w_{8j+5 \rightarrow 8j+7}; \\
b_{j-3s,8s+(-2)_s} &= -w_{8(j+m+1) \rightarrow 8(j+m+1)+7} \otimes e_{8j+5}; \\
b_{j-s,8s+(-2)_s} &= -w_{8(j+m+1)+4 \rightarrow 8(j+m+1)+7} \otimes w_{8j+5 \rightarrow 8j+7}; \\
b_{j-3s,8s+(-6)_s} &= -w_{8(j+m+1) \rightarrow 8(j+m+1)+7} \otimes e_{8j+5}; \\
b_{j-s,8s+(-6)_s} &= -w_{8(j+m+1)+4 \rightarrow 8(j+m+1)+7} \otimes w_{8j+5 \rightarrow 8j+7}; \\
b_{(j+1)_s,13s+(-4)_s} &= -w_{8(j+m+1)+7 \rightarrow 8(j+m+2)+4} \otimes w_{8j+7 \rightarrow 8(j+1)}; \\
b_{(j+1)_s,13s+(-3)_s} &= -w_{8(j+m+1)+7 \rightarrow 8(j+m+2)+4} \otimes w_{8j+7 \rightarrow 8(j+1)}; \\
b_{(j+1)_s,13s+(-2)_s} &= -w_{8(j+m+1)+7 \rightarrow 8(j+m+2)+4} \otimes w_{8j+7 \rightarrow 8(j+1)}; \\
b_{(j+1)_s,13s+(-6)_s} &= -w_{8(j+m+1)+7 \rightarrow 8(j+m+2)+4} \otimes w_{8j+7 \rightarrow 8(j+1)}.
\end{aligned}$$

(29) If  $r_0 = 28$ , then  $\Omega^{28}(Z_t^{(22)})$  is described with  $(8s \times 16s)$  matrix with the following nonzero entries:

$$\begin{aligned}
b_{j+2s,(-6)_s} &= -w_{8(j+m)+2 \rightarrow 8(j+m)+7} \otimes w_{8j \rightarrow 8j+2}; \\
b_{j+3s,(-6)_s} &= w_{8(j+m)+3 \rightarrow 8(j+m)+7} \otimes w_{8j \rightarrow 8j+3}; \\
b_{j+4s,(-6)_s} &= -w_{8(j+m)+4 \rightarrow 8(j+m)+7} \otimes w_{8j \rightarrow 8j+4}; \\
b_{j+5s,(-6)_s} &= w_{8(j+m)+5 \rightarrow 8(j+m)+7} \otimes w_{8j \rightarrow 8j+5}; \\
b_{j+6s,(-6)_s} &= -w_{8(j+m)+6 \rightarrow 8(j+m)+7} \otimes w_{8j \rightarrow 8j+6}; \\
b_{j+s,(-5)_s} &= w_{8(j+m)+1 \rightarrow 8(j+m)+7} \otimes w_{8j \rightarrow 8j+1}; \\
b_{j+5s,(-5)_s} &= -w_{8(j+m)+5 \rightarrow 8(j+m)+7} \otimes w_{8j \rightarrow 8j+5}; \\
b_{j+6s,(-5)_s} &= w_{8(j+m)+6 \rightarrow 8(j+m)+7} \otimes w_{8j \rightarrow 8j+6}; \\
b_{j+2s,(-4)_s} &= -w_{8(j+m)+2 \rightarrow 8(j+m)+7} \otimes w_{8j \rightarrow 8j+2}; \\
b_{j+3s,(-4)_s} &= w_{8(j+m)+3 \rightarrow 8(j+m)+7} \otimes w_{8j \rightarrow 8j+3}; \\
b_{j+4s,(-4)_s} &= -w_{8(j+m)+4 \rightarrow 8(j+m)+7} \otimes w_{8j \rightarrow 8j+4}; \\
b_{j+5s,(-4)_s} &= w_{8(j+m)+5 \rightarrow 8(j+m)+7} \otimes w_{8j \rightarrow 8j+5};
\end{aligned}$$

$$\begin{aligned}
b_{j+6s,(-4)_s} &= -w_{8(j+m)+6 \rightarrow 8(j+m)+7} \otimes w_{8j \rightarrow 8j+6}; \\
b_{j+s,(-3)_s} &= w_{8(j+m)+1 \rightarrow 8(j+m)+7} \otimes w_{8j \rightarrow 8j+1}; \\
b_{j+2s,(-3)_s} &= -w_{8(j+m)+2 \rightarrow 8(j+m)+7} \otimes w_{8j \rightarrow 8j+2}; \\
b_{j+3s,(-3)_s} &= w_{8(j+m)+3 \rightarrow 8(j+m)+7} \otimes w_{8j \rightarrow 8j+3}; \\
b_{j+4s,(-3)_s} &= -w_{8(j+m)+4 \rightarrow 8(j+m)+7} \otimes w_{8j \rightarrow 8j+4}; \\
b_{j+s,(-2)_s} &= w_{8(j+m)+1 \rightarrow 8(j+m)+7} \otimes w_{8j \rightarrow 8j+1}; \\
b_{j+2s,(-2)_s} &= -w_{8(j+m)+2 \rightarrow 8(j+m)+7} \otimes w_{8j \rightarrow 8j+2}; \\
b_{j+3s,(-2)_s} &= w_{8(j+m)+3 \rightarrow 8(j+m)+7} \otimes w_{8j \rightarrow 8j+3}; \\
b_{j+4s,(-2)_s} &= -w_{8(j+m)+4 \rightarrow 8(j+m)+7} \otimes w_{8j \rightarrow 8j+4}; \\
b_{j-s,s+(-6)_s} &= w_{8(j+m) \rightarrow 8(j+m+1)} \otimes e_{8j}; \\
b_{j,s+(-6)_s} &= -w_{8(j+m)+1 \rightarrow 8(j+m+1)} \otimes w_{8j \rightarrow 8j+1}; \\
b_{j+s,s+(-6)_s} &= w_{8(j+m)+2 \rightarrow 8(j+m+1)} \otimes w_{8j \rightarrow 8j+2}; \\
b_{j+2s,s+(-6)_s} &= -w_{8(j+m)+3 \rightarrow 8(j+m+1)} \otimes w_{8j \rightarrow 8j+3}; \\
b_{j+3s,s+(-6)_s} &= w_{8(j+m)+4 \rightarrow 8(j+m+1)} \otimes w_{8j \rightarrow 8j+4}; \\
b_{j-s,s+(-5)_s} &= -w_{8(j+m) \rightarrow 8(j+m+1)} \otimes e_{8j}; \\
b_{j-s,s+(-4)_s} &= w_{8(j+m) \rightarrow 8(j+m+1)} \otimes e_{8j}; \\
b_{j,s+(-4)_s} &= -w_{8(j+m)+1 \rightarrow 8(j+m+1)} \otimes w_{8j \rightarrow 8j+1}; \\
b_{j+s,s+(-4)_s} &= w_{8(j+m)+2 \rightarrow 8(j+m+1)} \otimes w_{8j \rightarrow 8j+2}; \\
b_{j+2s,s+(-4)_s} &= -w_{8(j+m)+3 \rightarrow 8(j+m+1)} \otimes w_{8j \rightarrow 8j+3}; \\
b_{j+3s,s+(-4)_s} &= w_{8(j+m)+4 \rightarrow 8(j+m+1)} \otimes w_{8j \rightarrow 8j+4}; \\
b_{j,s+(-3)_s} &= -w_{8(j+m)+1 \rightarrow 8(j+m+1)} \otimes w_{8j \rightarrow 8j+1}; \\
b_{j+s,s+(-3)_s} &= w_{8(j+m)+2 \rightarrow 8(j+m+1)} \otimes w_{8j \rightarrow 8j+2}; \\
b_{j+2s,s+(-3)_s} &= -w_{8(j+m)+3 \rightarrow 8(j+m+1)} \otimes w_{8j \rightarrow 8j+3}; \\
b_{j+3s,s+(-3)_s} &= w_{8(j+m)+4 \rightarrow 8(j+m+1)} \otimes w_{8j \rightarrow 8j+4}; \\
b_{j,s+(-2)_s} &= -w_{8(j+m)+1 \rightarrow 8(j+m+1)} \otimes w_{8j \rightarrow 8j+1}; \\
b_{j+s,s+(-2)_s} &= w_{8(j+m)+2 \rightarrow 8(j+m+1)} \otimes w_{8j \rightarrow 8j+2}; \\
b_{j+2s,s+(-2)_s} &= -w_{8(j+m)+3 \rightarrow 8(j+m+1)} \otimes w_{8j \rightarrow 8j+3}; \\
b_{j+3s,s+(-2)_s} &= w_{8(j+m)+4 \rightarrow 8(j+m+1)} \otimes w_{8j \rightarrow 8j+4}; \\
b_{s+(j+1)_s,4s+(-6)_s} &= w_{8(j+m+1)+1 \rightarrow 8(j+m+1)+3} \otimes w_{8j+2 \rightarrow 8(j+1)+1}; \\
b_{2s+(j+1)_s,4s+(-6)_s} &= -w_{8(j+m+1)+2 \rightarrow 8(j+m+1)+3} \otimes w_{8j+2 \rightarrow 8(j+1)+2}; \\
b_{s+(j+1)_s,4s+(-4)_s} &= w_{8(j+m+1)+1 \rightarrow 8(j+m+1)+3} \otimes w_{8j+2 \rightarrow 8(j+1)+1}; \\
b_{2s+(j+1)_s,4s+(-4)_s} &= -w_{8(j+m+1)+2 \rightarrow 8(j+m+1)+3} \otimes w_{8j+2 \rightarrow 8(j+1)+2}; \\
b_{s+(j+1)_s,4s+(-3)_s} &= w_{8(j+m+1)+1 \rightarrow 8(j+m+1)+3} \otimes w_{8j+2 \rightarrow 8(j+1)+1}; \\
b_{2s+(j+1)_s,4s+(-3)_s} &= -w_{8(j+m+1)+2 \rightarrow 8(j+m+1)+3} \otimes w_{8j+2 \rightarrow 8(j+1)+2}; \\
b_{s+(j+1)_s,5s+(-6)_s} &= -w_{8(j+m+1)+1 \rightarrow 8(j+m+1)+4} \otimes w_{8j+3 \rightarrow 8(j+1)+1}; \\
b_{2s+(j+1)_s,5s+(-6)_s} &= w_{8(j+m+1)+2 \rightarrow 8(j+m+1)+4} \otimes w_{8j+3 \rightarrow 8(j+1)+2}; \\
b_{3s+(j+1)_s,5s+(-6)_s} &= -w_{8(j+m+1)+3 \rightarrow 8(j+m+1)+4} \otimes w_{8j+3 \rightarrow 8(j+1)+3}; \\
b_{j-s,5s+(-6)_s} &= -w_{8(j+m)+4 \rightarrow 8(j+m+1)+4} \otimes w_{8j+3 \rightarrow 8j+4}; \\
b_{j+2s,5s+(-6)_s} &= -w_{8(j+m)+7 \rightarrow 8(j+m+1)+4} \otimes w_{8j+3 \rightarrow 8j+7};
\end{aligned}$$





$$\begin{aligned}
b_{5s+(j+1)s, 14s+(-6)s} &= w_{8(j+m+1)+5 \rightarrow 8(j+m+2)} \otimes w_{8j+7 \rightarrow 8(j+1)+5}; \\
b_{6s+(j+1)s, 14s+(-6)s} &= -w_{8(j+m+1)+6 \rightarrow 8(j+m+2)} \otimes w_{8j+7 \rightarrow 8(j+1)+6}; \\
b_{(j+1)s, 14s+(-5)s} &= -w_{8(j+m+1) \rightarrow 8(j+m+2)} \otimes w_{8j+7 \rightarrow 8(j+1)}; \\
b_{s+(j+1)s, 14s+(-5)s} &= w_{8(j+m+1)+1 \rightarrow 8(j+m+2)} \otimes w_{8j+7 \rightarrow 8(j+1)+1}; \\
b_{5s+(j+1)s, 14s+(-5)s} &= -w_{8(j+m+1)+5 \rightarrow 8(j+m+2)} \otimes w_{8j+7 \rightarrow 8(j+1)+5}; \\
b_{6s+(j+1)s, 14s+(-5)s} &= w_{8(j+m+1)+6 \rightarrow 8(j+m+2)} \otimes w_{8j+7 \rightarrow 8(j+1)+6}.
\end{aligned}$$

(II) Represent an arbitrary  $t_0 \in \mathbb{N}$  in the form  $t_0 = 29\ell_0 + r_0$ , where  $0 \leq r_0 \leq 28$ . Then  $\Omega^{t_0}(Z_t^{(22)})$  is a  $\Omega^{r_0}(Z_t^{(22)})$ , whose left components twisted by  $\sigma^{\ell_0}$ , and coefficients multiplied by  $(-1)^{\ell_0}$ .

**Proposition 18** (Translates for the case 23). (I) Let  $r_0 \in \mathbb{N}$ ,  $r_0 < 29$ .  $r_0$ -translates of the elements  $Z_t^{(23)}$  are described by the following way.

(1) If  $r_0 = 0$ , then  $\Omega^0(Z_t^{(23)})$  is described with  $(8s \times 13s)$  matrix, whose entries  $b_{ij}$  have the following form:

If  $0 \leq j < s$ , then

$$b_{ij} = \begin{cases} e_{8(j+m)} \otimes e_{8j}, & i = j; \\ 0, & \text{otherwise.} \end{cases}$$

If  $s \leq j < 2s$ , then  $b_{ij} = 0$ .

If  $2s \leq j < 4s$ , then

$$b_{ij} = \begin{cases} -w_{8(j+m)+j_2-1 \rightarrow 8(j+m)+j_2+1} \otimes e_{8j+j_2-1}, & i = j - s; \\ 0, & \text{otherwise.} \end{cases}$$

If  $4s \leq j < 8s$ , then  $b_{ij} = 0$ .

If  $8s \leq j < 9s$ , then

$$b_{ij} = \begin{cases} -e_{8(j+m)+5} \otimes e_{8j+5}, & i = j - 3s; \\ 0, & \text{otherwise.} \end{cases}$$

If  $9s \leq j < 10s$ , then  $b_{ij} = 0$ .

If  $10s \leq j < 12s$ , then

$$b_{ij} = \begin{cases} e_{8(j+m)+j_2-4} \otimes e_{8j+j_2-4}, & i = j - 4s; \\ 0, & \text{otherwise.} \end{cases}$$

If  $12s \leq j < 13s$ , then

$$b_{ij} = \begin{cases} w_{8(j+m)+7 \rightarrow 8(j+m+1)} \otimes e_{8j+7}, & i = j - 5s; \\ 0, & \text{otherwise.} \end{cases}$$

(2) If  $r_0 = 1$ , then  $\Omega^1(Z_t^{(23)})$  is described with  $(9s \times 11s)$  matrix, whose entries  $b_{ij}$  have the following form:

If  $0 \leq j < s$ , then

$$b_{ij} = \begin{cases} -w_{8(j+m)+1 \rightarrow 8(j+m)+3} \otimes e_{8j}, & i = j; \\ 0, & \text{otherwise.} \end{cases}$$

If  $s \leq j < 2s$ , then

$$b_{ij} = \begin{cases} e_{8(j+m)+5} \otimes e_{8j}, & i = j; \\ 0, & \text{otherwise.} \end{cases}$$

If  $2s \leq j < 3s$ , then

$$b_{ij} = \begin{cases} -w_{8(j+m)+2 \rightarrow 8(j+m+1)} \otimes e_{8j+1}, & i = j; \\ w_{8(j+m)+3 \rightarrow 8(j+m+1)} \otimes w_{8j+1 \rightarrow 8j+2}, & i = j + s; \\ w_{8(j+m)+4 \rightarrow 8(j+m+1)} \otimes w_{8j+1 \rightarrow 8j+3}, & i = j + 2s; \\ w_{8(j+m)+7 \rightarrow 8(j+m+1)} \otimes w_{8j+1 \rightarrow 8j+4}, & i = j + 3s; \\ e_{8(j+m+1)} \otimes w_{8j+1 \rightarrow 8j+7}, & i = j + 6s; \\ 0, & \text{otherwise.} \end{cases}$$

If  $3s \leq j < 4s$ , then

$$b_{ij} = \begin{cases} -w_{8(j+m)+3 \rightarrow 8(j+m)+7} \otimes e_{8j+2}, & i = j; \\ -w_{8(j+m)+4 \rightarrow 8(j+m)+7} \otimes w_{8j+2 \rightarrow 8j+3}, & i = j + s; \\ -e_{8(j+m)+7} \otimes w_{8j+2 \rightarrow 8j+4}, & i = j + 2s; \\ 0, & \text{otherwise.} \end{cases}$$

If  $4s \leq j < 5s$ , then

$$b_{ij} = \begin{cases} -e_{8(j+m+1)} \otimes w_{8j+3 \rightarrow 8j+7}, & i = j + 4s; \\ 0, & \text{otherwise.} \end{cases}$$

If  $5s \leq j < 6s$ , then

$$b_{ij} = \begin{cases} -w_{8(j+m+1) \rightarrow 8(j+m+1)+1} \otimes w_{8j+4 \rightarrow 8j+7}, & i = j + 3s; \\ 0, & \text{otherwise.} \end{cases}$$

If  $6s \leq j < 7s$ , then

$$b_{ij} = \begin{cases} -w_{8(j+m)+6 \rightarrow 8(j+m+1)} \otimes e_{8j+5}, & i = j; \\ -w_{8(j+m)+7 \rightarrow 8(j+m+1)} \otimes w_{8j+5 \rightarrow 8j+6}, & i = j + s; \\ 0, & \text{otherwise.} \end{cases}$$

If  $7s \leq j < 8s$ , then

$$b_{ij} = \begin{cases} e_{8(j+m)+7} \otimes e_{8j+6}, & i = j; \\ 0, & \text{otherwise.} \end{cases}$$

If  $8s \leq j < 9s$ , then

$$b_{ij} = \begin{cases} w_{8(j+m+1) \rightarrow 8(j+m+1)+2} \otimes e_{8j+7}, & i = j; \\ 0, & \text{otherwise.} \end{cases}$$

If  $9s \leq j < 10s$ , then

$$b_{ij} = \begin{cases} -w_{8(j+m+1)+1 \rightarrow 8(j+m+1)+4} \otimes w_{8j+7 \rightarrow 8(j+1)}, & i = (j+1)_s; \\ w_{8(j+m+1)+2 \rightarrow 8(j+m+1)+4} \otimes w_{8j+7 \rightarrow 8(j+1)+1}, & i = 2s + (j+1)_s; \\ w_{8(j+m+1) \rightarrow 8(j+m+1)+4} \otimes e_{8j+7}, & i = j - s; \\ 0, & \text{otherwise.} \end{cases}$$

If  $10s \leq j < 11s$ , then

$$b_{ij} = \begin{cases} -w_{8(j+m+1)+5 \rightarrow 8(j+m+1)+6} \otimes w_{8j+7 \rightarrow 8(j+1)}, & i = s + (j+1)_s; \\ -e_{8(j+m+1)+6} \otimes w_{8j+7 \rightarrow 8(j+1)+5}, & i = 6s + (j+1)_s; \\ -w_{8(j+m+1) \rightarrow 8(j+m+1)+6} \otimes e_{8j+7}, & i = j - 2s; \\ 0, & \text{otherwise.} \end{cases}$$

(3) If  $r_0 = 2$ , then  $\Omega^2(Z_t^{(23)})$  is described with  $(8s \times 11s)$  matrix, whose entries  $b_{ij}$  have the following form:

If  $0 \leq j < s$ , then

$$b_{ij} = \begin{cases} -w_{8(j+m-1)+7 \rightarrow 8(j+m)} \otimes e_{8j}, & i = j; \\ 0, & \text{otherwise.} \end{cases}$$

If  $s \leq j < 2s$ , then

$$b_{ij} = \begin{cases} -w_{8(j+m)+2 \rightarrow 8(j+m)+4} \otimes e_{8j+1}, & i = j; \\ 0, & \text{otherwise.} \end{cases}$$

If  $2s \leq j < 3s$ , then

$$b_{ij} = \begin{cases} e_{8(j+m)+5} \otimes w_{8j+1 \rightarrow 8j+4}, & i = j + 2s; \\ 0, & \text{otherwise.} \end{cases}$$

If  $3s \leq j < 4s$ , then

$$b_{ij} = \begin{cases} -w_{8(j+m)+5 \rightarrow 8(j+m)+6} \otimes w_{8j+2 \rightarrow 8j+4}, & i = j + s; \\ 0, & \text{otherwise.} \end{cases}$$

If  $4s \leq j < 6s$ , then  $b_{ij} = 0$ .

If  $6s \leq j < 7s$ , then

$$b_{ij} = \begin{cases} -w_{8(j+m)+1 \rightarrow 8(j+m)+3} \otimes w_{8j+5 \rightarrow 8j+6}, & i = j; \\ 0, & \text{otherwise.} \end{cases}$$

If  $7s \leq j < 8s$ , then

$$b_{ij} = \begin{cases} e_{8(j+m)+6} \otimes e_{8j+5}, & i = j - 2s; \\ 0, & \text{otherwise.} \end{cases}$$

If  $8s \leq j < 9s$ , then

$$b_{ij} = \begin{cases} -w_{8(j+m)+1 \rightarrow 8(j+m)+4} \otimes e_{8j+6}, & i = j - 2s; \\ 0, & \text{otherwise.} \end{cases}$$

If  $9s \leq j < 10s$ , then

$$b_{ij} = \begin{cases} e_{8(j+m+1)} \otimes e_{8j+7}, & i = j - 2s; \\ 0, & \text{otherwise.} \end{cases}$$

If  $10s \leq j < 11s$ , then

$$b_{ij} = \begin{cases} e_{8(j+m)+7} \otimes w_{8j+7 \rightarrow 8(j+1)}, & i = (j+1)_s; \\ 0, & \text{otherwise.} \end{cases}$$

(4) If  $r_0 = 3$ , then  $\Omega^3(Z_t^{(23)})$  is described with  $(10s \times 10s)$  matrix, whose entries  $b_{ij}$  have the following form:

If  $0 \leq j < s$ , then

$$b_{ij} = \begin{cases} -w_{8(j+m)+2 \rightarrow 8(j+m)+4} \otimes e_{8j}, & i = j; \\ 0, & \text{otherwise.} \end{cases}$$

If  $s \leq j < 2s$ , then

$$b_{ij} = \begin{cases} e_{8(j+m)+6} \otimes e_{8j}, & i = j; \\ 0, & \text{otherwise.} \end{cases}$$

If  $2s \leq j < 3s$ , then

$$b_{ij} = \begin{cases} -w_{8(j+m)+3 \rightarrow 8(j+m)+7} \otimes e_{8j+1}, & i = j; \\ -w_{8(j+m)+4 \rightarrow 8(j+m)+7} \otimes w_{8j+1 \rightarrow 8j+2}, & i = j + s; \\ -e_{8(j+m)+7} \otimes w_{8j+1 \rightarrow 8j+3}, & i = j + 2s; \\ 0, & \text{otherwise.} \end{cases}$$

If  $3s \leq j < 4s$ , then

$$b_{ij} = \begin{cases} -e_{8(j+m+1)} \otimes w_{8j+2 \rightarrow 8j+4}, & i = j + 2s; \\ 0, & \text{otherwise.} \end{cases}$$

If  $4s \leq j < 5s$ , then

$$b_{ij} = \begin{cases} -w_{8(j+m+1) \rightarrow 8(j+m+1)+1} \otimes w_{8j+3 \rightarrow 8j+4}, & i = j + s; \\ 0, & \text{otherwise.} \end{cases}$$

If  $5s \leq j < 6s$ , then

$$b_{ij} = \begin{cases} -w_{8(j+m+1) \rightarrow 8(j+m+1)+2} \otimes e_{8j+4}, & i = j; \\ 0, & \text{otherwise.} \end{cases}$$

If  $6s \leq j < 7s$ , then

$$b_{ij} = \begin{cases} e_{8(j+m)+7} \otimes e_{8j+5}, & i = j; \\ 0, & \text{otherwise.} \end{cases}$$

If  $7s \leq j < 8s$ , then

$$b_{ij} = \begin{cases} e_{8(j+m+1)} \otimes e_{8j+6}, & i = j; \\ 0, & \text{otherwise.} \end{cases}$$

If  $8s \leq j < 9s$ , then

$$b_{ij} = \begin{cases} -w_{8(j+m+1)+1 \rightarrow 8(j+m+1)+3} \otimes e_{8j+7}, & i = j; \\ 0, & \text{otherwise.} \end{cases}$$

If  $9s \leq j < 10s$ , then

$$b_{ij} = \begin{cases} e_{8(j+m+1)+5} \otimes e_{8j+7}, & i = j; \\ 0, & \text{otherwise.} \end{cases}$$

(5) If  $r_0 = 4$ , then  $\Omega^4(Z_t^{(23)})$  is described with  $(11s \times 8s)$  matrix, whose entries  $b_{ij}$  have the following form:

If  $0 \leq j < s$ , then

$$b_{ij} = \begin{cases} -e_{8(j+m-1)+7} \otimes e_{8j}, & i = j; \\ 0, & \text{otherwise.} \end{cases}$$

If  $s \leq j < 2s$ , then

$$b_{ij} = \begin{cases} -w_{8(j+m)+5 \rightarrow 8(j+m)+6} \otimes w_{8j+1 \rightarrow 8j+3}, & i = j + 3s; \\ -e_{8(j+m)+6} \otimes w_{8j+1 \rightarrow 8j+4}, & i = j + 4s; \\ 0, & \text{otherwise.} \end{cases}$$

If  $2s \leq j < 4s$ , then  $b_{ij} = 0$ .

If  $4s \leq j < 5s$ , then

$$b_{ij} = \begin{cases} w_{8(j+m)+1 \rightarrow 8(j+m)+3} \otimes e_{8j+4}, & i = j + 2s; \\ 0, & \text{otherwise.} \end{cases}$$

If  $5s \leq j < 6s$ , then

$$b_{ij} = \begin{cases} -w_{8(j+m)+1 \rightarrow 8(j+m)+4} \otimes e_{8j+5}, & i = j + 2s; \\ -w_{8(j+m)+2 \rightarrow 8(j+m)+4} \otimes w_{8j+5 \rightarrow 8j+6}, & i = j + 3s; \\ 0, & \text{otherwise.} \end{cases}$$

If  $6s \leq j < 7s$ , then

$$b_{ij} = \begin{cases} e_{8(j+m)+5} \otimes e_{8j+6}, & i = j + 3s; \\ 0, & \text{otherwise.} \end{cases}$$

If  $7s \leq j < 8s$ , then

$$b_{ij} = \begin{cases} -w_{8(j+m)+7 \rightarrow 8(j+m)+1} \otimes w_{8j+7 \rightarrow 8(j+1)}, & i = (j+1)s; \\ -e_{8(j+m)+1} \otimes w_{8j+7 \rightarrow 8(j+1)}, & i = s + (j+1)s; \\ -w_{8(j+m)+7 \rightarrow 8(j+m)+1} \otimes e_{8j+7}, & i = j + 3s; \\ 0, & \text{otherwise.} \end{cases}$$

(6) If  $r_0 = 5$ , then  $\Omega^5(Z_t^{(23)})$  is described with  $(11s \times 9s)$  matrix, whose entries  $b_{ij}$  have the following form:

If  $0 \leq j < s$ , then

$$b_{ij} = \begin{cases} -w_{8(j+m)+5 \rightarrow 8(j+m)+7} \otimes e_{8j}, & i = j; \\ -w_{8(j+m)+3 \rightarrow 8(j+m)+7} \otimes e_{8j}, & i = j + s; \\ w_{8(j+m)+1 \rightarrow 8(j+m)+7} \otimes e_{8j}, & i = j + 2s; \\ -w_{8(j+m)+4 \rightarrow 8(j+m)+7} \otimes w_{8j \rightarrow 8j+1}, & i = j + 3s; \\ -e_{8(j+m)+7} \otimes w_{8j \rightarrow 8j+2}, & i = j + 4s; \\ 0, & \text{otherwise.} \end{cases}$$

If  $s \leq j < 2s$ , then

$$b_{ij} = \begin{cases} -e_{8(j+m)+1} \otimes w_{8j+1 \rightarrow 8j+3}, & i = j + 4s; \\ w_{8(j+m)+7 \rightarrow 8(j+m)+1} \otimes w_{8j+1 \rightarrow 8j+4}, & i = j + 5s; \\ 0, & \text{otherwise.} \end{cases}$$

If  $2s \leq j < 3s$ , then

$$b_{ij} = \begin{cases} e_{8(j+m+1)+1} \otimes w_{8j+2 \rightarrow 8(j+1)}, & i = 2s + (j+1)_s; \\ w_{8(j+m)+7 \rightarrow 8(j+m+1)+1} \otimes w_{8j+2 \rightarrow 8j+4}, & i = j + 4s; \\ 0, & \text{otherwise.} \end{cases}$$

If  $3s \leq j < 4s$ , then

$$b_{ij} = \begin{cases} w_{8(j+m+1)+1 \rightarrow 8(j+m+1)+2} \otimes w_{8j+3 \rightarrow 8(j+1)}, & i = 2s + (j+1)_s; \\ w_{8(j+m)+7 \rightarrow 8(j+m+1)+2} \otimes w_{8j+3 \rightarrow 8j+4}, & i = j + 3s; \\ 0, & \text{otherwise.} \end{cases}$$

If  $4s \leq j < 5s$ , then

$$b_{ij} = \begin{cases} w_{8(j+m+1)+1 \rightarrow 8(j+m+1)+3} \otimes w_{8j+4 \rightarrow 8(j+1)}, & i = 2s + (j+1)_s; \\ w_{8(j+m)+7 \rightarrow 8(j+m+1)+3} \otimes e_{8j+4}, & i = j + 2s; \\ 0, & \text{otherwise.} \end{cases}$$

If  $5s \leq j < 6s$ , then

$$b_{ij} = \begin{cases} e_{8(j+m+1)} \otimes e_{8j+5}, & i = j + 2s; \\ -w_{8(j+m)+7 \rightarrow 8(j+m+1)} \otimes w_{8j+5 \rightarrow 8j+6}, & i = j + 3s; \\ 0, & \text{otherwise.} \end{cases}$$

If  $6s \leq j < 7s$ , then

$$b_{ij} = \begin{cases} -e_{8(j+m+1)+5} \otimes w_{8j+6 \rightarrow 8(j+1)}, & i = (j+1)_s; \\ w_{8(j+m)+7 \rightarrow 8(j+m+1)+5} \otimes e_{8j+6}, & i = j + 2s; \\ 0, & \text{otherwise.} \end{cases}$$

If  $7s \leq j < 8s$ , then

$$b_{ij} = \begin{cases} w_{8(j+m+1)+1 \rightarrow 8(j+m+1)+4} \otimes w_{8j+7 \rightarrow 8(j+1)}, & i = 2s + (j+1)_s; \\ -w_{8(j+m+1)+2 \rightarrow 8(j+m+1)+4} \otimes e_{8j+7}, & i = j + 2s; \\ 0, & \text{otherwise.} \end{cases}$$

If  $8s \leq j < 9s$ , then

$$b_{ij} = \begin{cases} w_{8(j+m+1)+5 \rightarrow 8(j+m+1)+6} \otimes w_{8j+7 \rightarrow 8(j+1)}, & i = (j+1)_s; \\ e_{8(j+m+1)+6} \otimes e_{8j+7}, & i = j + 2s; \\ 0, & \text{otherwise.} \end{cases}$$

(7) If  $r_0 = 6$ , then  $\Omega^6(Z_t^{(23)})$  is described with  $(13s \times 8s)$  matrix, whose entries  $b_{ij}$  have the following form:

If  $0 \leq j < s$ , then

$$b_{ij} = \begin{cases} w_{8(j+m-1)+7 \rightarrow 8(j+m)} \otimes e_{8j}, & i = j; \\ -e_{8(j+m)} \otimes e_{8j}, & i = j + s; \\ 0, & \text{otherwise.} \end{cases}$$

If  $s \leq j < 2s$ , then

$$b_{ij} = \begin{cases} e_{8(j+m)+1} \otimes w_{8j+1 \rightarrow 8j+3}, & i = j + 4s; \\ 0, & \text{otherwise.} \end{cases}$$

If  $2s \leq j < 4s$ , then  $b_{ij} = 0$ .

If  $4s \leq j < 5s$ , then

$$b_{ij} = \begin{cases} -w_{8(j+m)+2 \rightarrow 8(j+m)+4} \otimes e_{8j+4}, & i = j + 2s; \\ 0, & \text{otherwise.} \end{cases}$$

If  $5s \leq j < 6s$ , then

$$b_{ij} = \begin{cases} e_{8(j+m)+5} \otimes e_{8j+5}, & i = j + 3s; \\ 0, & \text{otherwise.} \end{cases}$$

If  $6s \leq j < 7s$ , then

$$b_{ij} = \begin{cases} -e_{8(j+m)+6} \otimes e_{8j+6}, & i = j + 4s; \\ 0, & \text{otherwise.} \end{cases}$$

If  $7s \leq j < 8s$ , then

$$b_{ij} = \begin{cases} -e_{8(j+m)+7} \otimes e_{8j+7}, & i = j + 4s; \\ 0, & \text{otherwise.} \end{cases}$$

(8) If  $r_0 = 7$ , then  $\Omega^7(Z_t^{(23)})$  is described with  $(14s \times 8s)$  matrix, whose entries  $b_{ij}$  have the following form:

If  $0 \leq j < s$ , then

$$b_{ij} = \begin{cases} -w_{8(j+m)+6 \rightarrow 8(j+m)+1} \otimes e_{8j}, & i = j + 2s; \\ w_{8(j+m)+5 \rightarrow 8(j+m)+1} \otimes e_{8j}, & i = j + 3s; \\ -e_{8(j+m)+1} \otimes w_{8j \rightarrow 8j+2}, & i = j + 5s; \\ -w_{8(j+m)+7 \rightarrow 8(j+m)+1} \otimes w_{8j \rightarrow 8j+3}, & i = j + 6s; \\ 0, & \text{otherwise.} \end{cases}$$

If  $s \leq j < 2s$ , then

$$b_{ij} = \begin{cases} -w_{8(j+m)+1 \rightarrow 8(j+m)+1} \otimes w_{8j+1 \rightarrow 8j+2}, & i = j + 4s; \\ -w_{8(j+m)+7 \rightarrow 8(j+m)+1} \otimes w_{8j+1 \rightarrow 8j+3}, & i = j + 5s; \\ 0, & \text{otherwise.} \end{cases}$$

If  $2s \leq j < 3s$ , then

$$b_{ij} = \begin{cases} e_{8(j+m)+2} \otimes w_{8j+2 \rightarrow 8(j+1)}, & i = (j+1)_s; \\ -w_{8(j+m)+7 \rightarrow 8(j+m)+2} \otimes w_{8j+2 \rightarrow 8j+3}, & i = j + 4s; \\ 0, & \text{otherwise.} \end{cases}$$

If  $3s \leq j < 4s$ , then

$$b_{ij} = \begin{cases} w_{8(j+m)+2 \rightarrow 8(j+m)+3} \otimes w_{8j+3 \rightarrow 8(j+1)}, & i = (j+1)_s; \\ -w_{8(j+m)+7 \rightarrow 8(j+m)+3} \otimes e_{8j+3}, & i = j + 3s; \\ 0, & \text{otherwise.} \end{cases}$$

If  $4s \leq j < 5s$ , then

$$b_{ij} = \begin{cases} w_{8(j+m+1)+2 \rightarrow 8(j+m+1)+4} \otimes w_{8j+4 \rightarrow 8(j+1)}, & i = (j+1)_s; \\ w_{8(j+m+1)+3 \rightarrow 8(j+m+1)+4} \otimes w_{8j+4 \rightarrow 8j+7}, & i = j+8s; \\ 0, & \text{otherwise.} \end{cases}$$

If  $5s \leq j < 6s$ , then

$$b_{ij} = \begin{cases} e_{8(j+m+1)+5} \otimes w_{8j+5 \rightarrow 8(j+1)}, & i = 3s + (j+1)_s; \\ w_{8(j+m)+7 \rightarrow 8(j+m+1)+5} \otimes e_{8j+5}, & i = j+3s; \\ -w_{8(j+m)+7 \rightarrow 8(j+m+1)+5} \otimes w_{8j+5 \rightarrow 8j+6}, & i = j+4s; \\ 0, & \text{otherwise.} \end{cases}$$

If  $6s \leq j < 7s$ , then

$$b_{ij} = \begin{cases} -e_{8(j+m+1)+6} \otimes w_{8j+6 \rightarrow 8(j+1)}, & i = 2s + (j+1)_s; \\ w_{8(j+m+1)+5 \rightarrow 8(j+m+1)+6} \otimes w_{8j+6 \rightarrow 8(j+1)}, & i = 3s + (j+1)_s; \\ -w_{8(j+m)+7 \rightarrow 8(j+m+1)+6} \otimes e_{8j+6}, & i = j+3s; \\ 0, & \text{otherwise.} \end{cases}$$

If  $7s \leq j < 8s$ , then

$$b_{ij} = \begin{cases} -w_{8(j+m+1)+2 \rightarrow 8(j+m+1)+7} \otimes w_{8j+7 \rightarrow 8(j+1)}, & i = (j+1)_s; \\ w_{8(j+m+1)+4 \rightarrow 8(j+m+1)+7} \otimes w_{8j+7 \rightarrow 8(j+1)}, & i = s + (j+1)_s; \\ -w_{8(j+m+1)+6 \rightarrow 8(j+m+1)+7} \otimes w_{8j+7 \rightarrow 8(j+1)}, & i = 2s + (j+1)_s; \\ w_{8(j+m+1)+5 \rightarrow 8(j+m+1)+7} \otimes w_{8j+7 \rightarrow 8(j+1)}, & i = 3s + (j+1)_s; \\ e_{8(j+m+1)+7} \otimes w_{8j+7 \rightarrow 8(j+1)+1}, & i = 4s + (j+1)_s; \\ -e_{8(j+m+1)+7} \otimes w_{8j+7 \rightarrow 8(j+1)+3}, & i = 6s + (j+1)_s; \\ w_{8(j+m+1)+3 \rightarrow 8(j+m+1)+7} \otimes e_{8j+7}, & i = j+5s; \\ 0, & \text{otherwise.} \end{cases}$$

(9) If  $r_0 = 8$ , then  $\Omega^8(Z_t^{(23)})$  is described with  $(16s \times 9s)$  matrix, whose entries  $b_{ij}$  have the following form:

If  $s \leq j < 2s$ , then

$$b_{ij} = \begin{cases} w_{8(j+m-1)+7 \rightarrow 8(j+m)+5} \otimes e_{8j}, & i = j-s; \\ w_{8(j+m-1)+7 \rightarrow 8(j+m)+5} \otimes e_{8j}, & i = j; \\ -e_{8(j+m)+5} \otimes w_{8j \rightarrow 8j+1}, & i = j+2s; \\ 0, & \text{otherwise.} \end{cases}$$

If  $2s \leq j < 3s$ , then

$$b_{ij} = \begin{cases} -w_{8(j+m)+1 \rightarrow 8(j+m)+2} \otimes w_{8j+1 \rightarrow 8j+2}, & i = j+3s; \\ -e_{8(j+m)+2} \otimes w_{8j+1 \rightarrow 8j+3}, & i = j+4s; \\ 0, & \text{otherwise.} \end{cases}$$

If  $3s \leq j < 4s$ , then  $b_{ij} = 0$ .



If  $4s \leq j < 5s$ , then

$$b_{ij} = \begin{cases} -w_{8(j+m)+2 \rightarrow 8(j+m)+4} \otimes e_{8j+3}, & i = j + 2s; \\ w_{8(j+m)+3 \rightarrow 8(j+m)+4} \otimes w_{8j+3 \rightarrow 8j+4}, & i = j + 3s; \\ 0, & \text{otherwise.} \end{cases}$$

If  $5s \leq j < 6s$ , then

$$b_{ij} = \begin{cases} -e_{8(j+m)+7} \otimes w_{8j+4 \rightarrow 8(j+1)}, & i = (j+1)_s; \\ -e_{8(j+m)+7} \otimes w_{8j+4 \rightarrow 8(j+1)}, & i = s + (j+1)_s; \\ 0, & \text{otherwise.} \end{cases}$$

If  $6s \leq j < 7s$ , then

$$b_{ij} = \begin{cases} e_{8(j+m)+6} \otimes e_{8j+5}, & i = j + 4s; \\ 0, & \text{otherwise.} \end{cases}$$

If  $7s \leq j < 8s$ , then

$$b_{ij} = \begin{cases} -w_{8(j+m)+4 \rightarrow 8(j+m)+7} \otimes e_{8j+6}, & i = j + 5s; \\ 0, & \text{otherwise.} \end{cases}$$

If  $8s \leq j < 9s$ , then

$$b_{ij} = \begin{cases} e_{8(j+m+1)} \otimes e_{8j+7}, & i = j + 7s; \\ 0, & \text{otherwise.} \end{cases}$$

(10) If  $r_0 = 9$ , then  $\Omega^9(Z_t^{(23)})$  is described with  $(16s \times 8s)$  matrix, whose entries  $b_{ij}$  have the following form:

If  $0 \leq j < s$ , then

$$b_{ij} = \begin{cases} -w_{8(j+m)+3 \rightarrow 8(j+m)+7} \otimes e_{8j}, & i = j + s; \\ -w_{8(j+m)+6 \rightarrow 8(j+m)+7} \otimes e_{8j}, & i = j + 2s; \\ e_{8(j+m)+7} \otimes w_{8j \rightarrow 8j+2}, & i = j + 5s; \\ -e_{8(j+m)+7} \otimes w_{8j \rightarrow 8j+5}, & i = j + 8s; \\ 0, & \text{otherwise.} \end{cases}$$

If  $s \leq j < 2s$ , then

$$b_{ij} = \begin{cases} -w_{8(j+m+1)+1 \rightarrow 8(j+m+1)+2} \otimes w_{8j+1 \rightarrow 8(j+1)}, & i = 3s + (j+1)_s; \\ w_{8(j+m)+7 \rightarrow 8(j+m+1)+2} \otimes w_{8j+1 \rightarrow 8j+2}, & i = j + 4s; \\ -w_{8(j+m+1) \rightarrow 8(j+m+1)+2} \otimes w_{8j+1 \rightarrow 8j+3}, & i = j + 5s; \\ 0, & \text{otherwise.} \end{cases}$$

If  $2s \leq j < 3s$ , then

$$b_{ij} = \begin{cases} e_{8(j+m+1)+3} \otimes w_{8j+2 \rightarrow 8(j+1)}, & i = s + (j+1)_s; \\ -w_{8(j+m+1)+1 \rightarrow 8(j+m+1)+3} \otimes w_{8j+2 \rightarrow 8(j+1)}, & i = 3s + (j+1)_s; \\ -w_{8(j+m+1) \rightarrow 8(j+m+1)+3} \otimes w_{8j+2 \rightarrow 8j+3}, & i = j + 4s; \\ 0, & \text{otherwise.} \end{cases}$$

If  $3s \leq j < 4s$ , then

$$b_{ij} = \begin{cases} w_{8(j+m+1)+3 \rightarrow 8(j+m+1)+4} \otimes w_{8j+3 \rightarrow 8(j+1)}, & i = s + (j+1)_s; \\ -w_{8(j+m+1)+1 \rightarrow 8(j+m+1)+4} \otimes w_{8j+3 \rightarrow 8(j+1)}, & i = 3s + (j+1)_s; \\ -w_{8(j+m+1) \rightarrow 8(j+m+1)+4} \otimes e_{8j+3}, & i = j + 3s; \\ 0, & \text{otherwise.} \end{cases}$$

If  $4s \leq j < 5s$ , then

$$b_{ij} = \begin{cases} e_{8(j+m+1)+5} \otimes w_{8j+4 \rightarrow 8j+7}, & i = j + 11s; \\ 0, & \text{otherwise.} \end{cases}$$

If  $5s \leq j < 6s$ , then

$$b_{ij} = \begin{cases} -e_{8(j+m+1)+6} \otimes w_{8j+5 \rightarrow 8(j+1)}, & i = 2s + (j+1)_s; \\ -w_{8(j+m)+7 \rightarrow 8(j+m+1)+6} \otimes e_{8j+5}, & i = j + 3s; \\ -w_{8(j+m+1) \rightarrow 8(j+m+1)+6} \otimes w_{8j+5 \rightarrow 8j+6}, & i = j + 6s; \\ 0, & \text{otherwise.} \end{cases}$$

If  $6s \leq j < 7s$ , then

$$b_{ij} = \begin{cases} -w_{8(j+m+1) \rightarrow 8(j+m+1)+1} \otimes e_{8j+6}, & i = j + 5s; \\ 0, & \text{otherwise.} \end{cases}$$

If  $7s \leq j < 8s$ , then

$$b_{ij} = \begin{cases} -e_{8(j+m+2)} \otimes w_{8j+7 \rightarrow 8(j+1)+3}, & i = 6s + (j+1)_s; \\ w_{8(j+m+1)+2 \rightarrow 8(j+m+2)} \otimes e_{8j+7}, & i = j + 5s; \\ 0, & \text{otherwise.} \end{cases}$$

(11) If  $r_0 = 10$ , then  $\Omega^{10}(Z_t^{(23)})$  is described with  $(19s \times 10s)$  matrix, whose entries  $b_{ij}$  have the following form:

If  $0 \leq j < s$ , then

$$b_{ij} = \begin{cases} -w_{8(j+m) \rightarrow 8(j+m)+2} \otimes e_{8j}, & i = j + s; \\ w_{8(j+m) \rightarrow 8(j+m)+2} \otimes e_{8j}, & i = j + 2s; \\ -w_{8(j+m)+1 \rightarrow 8(j+m)+2} \otimes w_{8j \rightarrow 8j+1}, & i = j + 4s; \\ 0, & \text{otherwise.} \end{cases}$$

If  $s \leq j < 2s$ , then

$$b_{ij} = \begin{cases} -w_{8(j+m) \rightarrow 8(j+m)+6} \otimes e_{8j}, & i = j; \\ -w_{8(j+m) \rightarrow 8(j+m)+6} \otimes e_{8j}, & i = j + s; \\ e_{8(j+m)+6} \otimes w_{8j \rightarrow 8j+1}, & i = j + 2s; \\ -w_{8(j+m)+5 \rightarrow 8(j+m)+6} \otimes w_{8j \rightarrow 8j+3}, & i = j + 6s; \\ -w_{8(j+m)+5 \rightarrow 8(j+m)+6} \otimes w_{8j \rightarrow 8j+5}, & i = j + 9s; \\ 0, & \text{otherwise.} \end{cases}$$

If  $2s \leq j < 3s$ , then

$$b_{ij} = \begin{cases} w_{8(j+m)+2 \rightarrow 8(j+m)+3} \otimes w_{8j+1 \rightarrow 8j+2}, & i = j + 3s; \\ -e_{8(j+m)+3} \otimes w_{8j+1 \rightarrow 8j+3}, & i = j + 4s; \\ 0, & \text{otherwise.} \end{cases}$$

If  $3s \leq j < 4s$ , then  $b_{ij} = 0$ .

If  $4s \leq j < 5s$ , then

$$b_{ij} = \begin{cases} e_{8(j+m)+7} \otimes w_{8j+3 \rightarrow 8(j+1)}, & i = (j+1)_s; \\ -w_{8(j+m)+5 \rightarrow 8(j+m)+7} \otimes e_{8j+3}, & i = j + 3s; \\ 0, & \text{otherwise.} \end{cases}$$

If  $5s \leq j < 6s$ , then

$$b_{ij} = \begin{cases} -e_{8(j+m)+1} \otimes w_{8j+4 \rightarrow 8(j+1)}, & i = s + (j+1)_s; \\ -w_{8(j+m)+6 \rightarrow 8(j+m)+1} \otimes e_{8j+4}, & i = j + 4s; \\ -w_{8(j+m)+7 \rightarrow 8(j+m)+1} \otimes w_{8j+4 \rightarrow 8j+7}, & i = j + 11s; \\ 0, & \text{otherwise.} \end{cases}$$

If  $6s \leq j < 7s$ , then

$$b_{ij} = \begin{cases} e_{8(j+m)+7} \otimes w_{8j+5 \rightarrow 8(j+1)}, & i = (j+1)_s; \\ -w_{8(j+m)+5 \rightarrow 8(j+m)+7} \otimes e_{8j+5}, & i = j + 4s; \\ w_{8(j+m)+1 \rightarrow 8(j+m)+7} \otimes e_{8j+5}, & i = j + 6s; \\ 0, & \text{otherwise.} \end{cases}$$

If  $7s \leq j < 8s$ , then

$$b_{ij} = \begin{cases} -w_{8(j+m)+2 \rightarrow 8(j+m)+1} \otimes e_{8j+6}, & i = j + 6s; \\ 0, & \text{otherwise.} \end{cases}$$

If  $8s \leq j < 9s$ , then

$$b_{ij} = \begin{cases} w_{8(j+m)+1 \rightarrow 8(j+m)+1} \otimes w_{8j+7 \rightarrow 8(j+1)}, & i = s + (j+1)_s; \\ -w_{8(j+m)+1 \rightarrow 8(j+m)+1} \otimes w_{8j+7 \rightarrow 8(j+1)}, & i = 2s + (j+1)_s; \\ e_{8(j+m)+1} \otimes w_{8j+7 \rightarrow 8(j+1)+1}, & i = 4s + (j+1)_s; \\ w_{8(j+m)+7 \rightarrow 8(j+m)+1} \otimes e_{8j+7}, & i = j + 8s; \\ 0, & \text{otherwise.} \end{cases}$$

If  $9s \leq j < 10s$ , then

$$b_{ij} = \begin{cases} -e_{8(j+m)+5} \otimes w_{8j+7 \rightarrow 8(j+1)+3}, & i = 7s + (j+1)_s; \\ 0, & \text{otherwise.} \end{cases}$$

(12) If  $r_0 = 11$ , then  $\Omega^{11}(Z_t^{(23)})$  is described with  $(18s \times 11s)$  matrix, whose entries  $b_{ij}$  have the following form:

If  $0 \leq j < s$ , then

$$b_{ij} = \begin{cases} -w_{8(j+m)+1 \rightarrow 8(j+m)+7} \otimes e_{8j}, & i = j + 3s; \\ -e_{8(j+m)+7} \otimes w_{8j \rightarrow 8j+1}, & i = j + 5s; \\ 0, & \text{otherwise.} \end{cases}$$

If  $s \leq j < 2s$ , then

$$b_{ij} = \begin{cases} -w_{8(j+m)+2 \rightarrow 8(j+m+1)} \otimes e_{8j}, & i = j - s; \\ -w_{8(j+m)+1 \rightarrow 8(j+m+1)} \otimes e_{8j}, & i = j + 2s; \\ w_{8(j+m)+7 \rightarrow 8(j+m+1)} \otimes w_{8j \rightarrow 8j+1}, & i = j + 4s; \\ -e_{8(j+m+1)} \otimes w_{8j \rightarrow 8j+2}, & i = j + 5s; \\ w_{8(j+m)+7 \rightarrow 8(j+m+1)} \otimes w_{8j \rightarrow 8j+3}, & i = j + 6s; \\ 0, & \text{otherwise.} \end{cases}$$

If  $2s \leq j < 3s$ , then

$$b_{ij} = \begin{cases} -w_{8(j+m+1)+2 \rightarrow 8(j+m+1)+3} \otimes w_{8j+1 \rightarrow 8(j+1)}, & i = (j+1)_s; \\ w_{8(j+m+1)+1 \rightarrow 8(j+m+1)+3} \otimes w_{8j+1 \rightarrow 8(j+1)}, & i = 3s + (j+1)_s; \\ -w_{8(j+m)+7 \rightarrow 8(j+m+1)+3} \otimes e_{8j+1}, & i = j + 3s; \\ 0, & \text{otherwise.} \end{cases}$$

If  $3s \leq j < 4s$ , then

$$b_{ij} = \begin{cases} w_{8(j+m+1)+2 \rightarrow 8(j+m+1)+4} \otimes w_{8j+2 \rightarrow 8(j+1)}, & i = (j+1)_s; \\ e_{8(j+m+1)+4} \otimes w_{8j+2 \rightarrow 8(j+1)}, & i = 2s + (j+1)_s; \\ w_{8(j+m+1)+1 \rightarrow 8(j+m+1)+4} \otimes w_{8j+2 \rightarrow 8(j+1)}, & i = 3s + (j+1)_s; \\ 0, & \text{otherwise.} \end{cases}$$

If  $4s \leq j < 5s$ , then

$$b_{ij} = \begin{cases} -e_{8(j+m+1)+5} \otimes w_{8j+3 \rightarrow 8(j+1)}, & i = 4s + (j+1)_s; \\ w_{8(j+m)+7 \rightarrow 8(j+m+1)+5} \otimes e_{8j+3}, & i = j + 3s; \\ 0, & \text{otherwise.} \end{cases}$$

If  $5s \leq j < 6s$ , then

$$b_{ij} = \begin{cases} w_{8(j+m)+7 \rightarrow 8(j+m+1)+6} \otimes e_{8j+4}, & i = j + 3s; \\ -e_{8(j+m+1)+6} \otimes w_{8j+4 \rightarrow 8j+7}, & i = j + 11s; \\ 0, & \text{otherwise.} \end{cases}$$

If  $6s \leq j < 7s$ , then

$$b_{ij} = \begin{cases} -e_{8(j+m+1)+1} \otimes w_{8j+4 \rightarrow 8(j+1)}, & i = 3s + (j+1)_s; \\ 0, & \text{otherwise.} \end{cases}$$

If  $7s \leq j < 8s$ , then

$$b_{ij} = \begin{cases} -w_{8(j+m)+7 \rightarrow 8(j+m+1)+1} \otimes e_{8j+5}, & i = j + 3s; \\ -w_{8(j+m+1) \rightarrow 8(j+m+1)+1} \otimes e_{8j+5}, & i = j + 4s; \\ -w_{8(j+m)+7 \rightarrow 8(j+m+1)+1} \otimes w_{8j+5 \rightarrow 8j+6}, & i = j + 5s; \\ 0, & \text{otherwise.} \end{cases}$$

If  $8s \leq j < 9s$ , then

$$b_{ij} = \begin{cases} -w_{8(j+m)+7 \rightarrow 8(j+m+1)+2} \otimes e_{8j+6}, & i = j + 4s; \\ 0, & \text{otherwise.} \end{cases}$$

If  $9s \leq j < 10s$ , then  $b_{ij} = 0$ .

If  $10s \leq j < 11s$ , then

$$b_{ij} = \begin{cases} w_{8(j+m+1)+3 \rightarrow 8(j+m+1)+7} \otimes e_{8j+7}, & i = j + 5s; \\ 0, & \text{otherwise.} \end{cases}$$

(13) If  $r_0 = 12$ , then  $\Omega^{12}(Z_t^{(23)})$  is described with  $(19s \times 11s)$  matrix, whose entries  $b_{ij}$  have the following form:

If  $0 \leq j < s$ , then

$$b_{ij} = \begin{cases} -e_{8(j+m)+5} \otimes w_{8j \rightarrow 8j+2}, & i = j + 5s; \\ 0, & \text{otherwise.} \end{cases}$$

If  $s \leq j < 2s$ , then

$$b_{ij} = \begin{cases} w_{8(j+m)+2 \rightarrow 8(j+m)+3} \otimes w_{8j \rightarrow 8j+5}, & i = j + 9s; \\ 0, & \text{otherwise.} \end{cases}$$

If  $2s \leq j < 3s$ , then

$$b_{ij} = \begin{cases} w_{8(j+m-1)+7 \rightarrow 8(j+m)+1} \otimes e_{8j}, & i = j - 2s; \\ w_{8(j+m) \rightarrow 8(j+m)+1} \otimes e_{8j}, & i = j - s; \\ w_{8(j+m-1)+7 \rightarrow 8(j+m)+1} \otimes e_{8j}, & i = j; \\ e_{8(j+m)+1} \otimes w_{8j \rightarrow 8j+4}, & i = j + 7s; \\ -e_{8(j+m)+1} \otimes w_{8j \rightarrow 8j+6}, & i = j + 13s; \\ 0, & \text{otherwise.} \end{cases}$$

If  $3s \leq j < 4s$ , then

$$b_{ij} = \begin{cases} -w_{8(j+m)+2 \rightarrow 8(j+m)+4} \otimes e_{8j+1}, & i = j; \\ w_{8(j+m)+3 \rightarrow 8(j+m)+4} \otimes w_{8j+1 \rightarrow 8j+2}, & i = j + s; \\ -e_{8(j+m)+4} \otimes w_{8j+1 \rightarrow 8j+3}, & i = j + 3s; \\ 0, & \text{otherwise.} \end{cases}$$

If  $4s \leq j < 5s$ , then

$$b_{ij} = \begin{cases} e_{8(j+m)+7} \otimes w_{8j+2 \rightarrow 8(j+1)}, & i = (j+1)_s; \\ e_{8(j+m)+7} \otimes w_{8j+2 \rightarrow 8(j+1)}, & i = 2s + (j+1)_s; \\ -w_{8(j+m)+6 \rightarrow 8(j+m)+7} \otimes w_{8j+2 \rightarrow 8j+3}, & i = j+3s; \\ 0, & \text{otherwise.} \end{cases}$$

If  $5s \leq j < 6s$ , then

$$b_{ij} = \begin{cases} -w_{8(j+m)+7 \rightarrow 8(j+m)+1} \otimes w_{8j+3 \rightarrow 8(j+1)}, & i = (j+1)_s; \\ -e_{8(j+m)+1} \otimes w_{8j+3 \rightarrow 8(j+1)}, & i = s + (j+1)_s; \\ -w_{8(j+m)+7 \rightarrow 8(j+m)+1} \otimes w_{8j+3 \rightarrow 8(j+1)}, & i = 2s + (j+1)_s; \\ w_{8(j+m)+6 \rightarrow 8(j+m)+1} \otimes e_{8j+3}, & i = j+2s; \\ 0, & \text{otherwise.} \end{cases}$$

If  $6s \leq j < 7s$ , then

$$b_{ij} = \begin{cases} w_{8(j+m)+5 \rightarrow 8(j+m)+7} \otimes e_{8j+4}, & i = j+2s; \\ -w_{8(j+m)+1 \rightarrow 8(j+m)+7} \otimes e_{8j+4}, & i = j+3s; \\ -e_{8(j+m)+7} \otimes w_{8j+4 \rightarrow 8j+7}, & i = j+10s; \\ 0, & \text{otherwise.} \end{cases}$$

If  $7s \leq j < 8s$ , then

$$b_{ij} = \begin{cases} -w_{8(j+m)+2 \rightarrow 8(j+m)+1} \otimes e_{8j+5}, & i = j+3s; \\ 0, & \text{otherwise.} \end{cases}$$

If  $8s \leq j < 9s$ , then

$$b_{ij} = \begin{cases} -w_{8(j+m)+3 \rightarrow 8(j+m)+7} \otimes e_{8j+6}, & i = j+6s; \\ 0, & \text{otherwise.} \end{cases}$$

If  $9s \leq j < 10s$ , then

$$b_{ij} = \begin{cases} w_{8(j+m)+7 \rightarrow 8(j+m)+2} \otimes w_{8j+7 \rightarrow 8(j+1)}, & i = (j+1)_s; \\ e_{8(j+m)+2} \otimes w_{8j+7 \rightarrow 8(j+1)+1}, & i = 3s + (j+1)_s; \\ -w_{8(j+m)+7 \rightarrow 8(j+m)+2} \otimes e_{8j+7}, & i = j+7s; \\ 0, & \text{otherwise.} \end{cases}$$

If  $10s \leq j < 11s$ , then

$$b_{ij} = \begin{cases} -e_{8(j+m)+6} \otimes w_{8j+7 \rightarrow 8(j+1)+3}, & i = 7s + (j+1)_s; \\ 0, & \text{otherwise.} \end{cases}$$

(14) If  $r_0 = 13$ , then  $\Omega^{13}(Z_t^{(23)})$  is described with  $(18s \times 13s)$  matrix, whose entries  $b_{ij}$  have the following form:

If  $0 \leq j < s$ , then

$$b_{ij} = \begin{cases} w_{8(j+m)+2 \rightarrow 8(j+m)+7} \otimes e_{8j}, & i = j; \\ w_{8(j+m)+3 \rightarrow 8(j+m)+7} \otimes e_{8j}, & i = j + s; \\ e_{8(j+m)+7} \otimes w_{8j \rightarrow 8j+2}, & i = j + 5s; \\ -e_{8(j+m)+7} \otimes w_{8j \rightarrow 8j+3}, & i = j + 6s; \\ 0, & \text{otherwise.} \end{cases}$$

If  $s \leq j < 2s$ , then

$$b_{ij} = \begin{cases} -e_{8(j+m+1)} \otimes w_{8j \rightarrow 8j+1}, & i = j + 3s; \\ w_{8(j+m)+7 \rightarrow 8(j+m+1)} \otimes w_{8j \rightarrow 8j+2}, & i = j + 4s; \\ 0, & \text{otherwise.} \end{cases}$$

If  $2s \leq j < 3s$ , then

$$b_{ij} = \begin{cases} w_{8(j+m+1)+3 \rightarrow 8(j+m+1)+4} \otimes w_{8j+1 \rightarrow 8(j+1)}, & i = s + (j + 1)_s; \\ w_{8(j+m)+7 \rightarrow 8(j+m+1)+4} \otimes w_{8j+1 \rightarrow 8j+2}, & i = j + 3s; \\ 0, & \text{otherwise.} \end{cases}$$

If  $3s \leq j < 4s$ , then

$$b_{ij} = \begin{cases} -e_{8(j+m+1)+5} \otimes w_{8j+2 \rightarrow 8(j+1)}, & i = 3s + (j + 1)_s; \\ 0, & \text{otherwise.} \end{cases}$$

If  $4s \leq j < 5s$ , then

$$b_{ij} = \begin{cases} e_{8(j+m+1)+6} \otimes w_{8j+3 \rightarrow 8(j+1)}, & i = 2s + (j + 1)_s; \\ -w_{8(j+m+1)+5 \rightarrow 8(j+m+1)+6} \otimes w_{8j+3 \rightarrow 8(j+1)}, & i = 3s + (j + 1)_s; \\ -w_{8(j+m)+7 \rightarrow 8(j+m+1)+6} \otimes e_{8j+3}, & i = j + 2s; \\ 0, & \text{otherwise.} \end{cases}$$

If  $5s \leq j < 6s$ , then  $b_{ij} = 0$ .

If  $6s \leq j < 7s$ , then

$$b_{ij} = \begin{cases} e_{8(j+m+1)+2} \otimes w_{8j+4 \rightarrow 8(j+1)}, & i = (j + 1)_s; \\ 0, & \text{otherwise.} \end{cases}$$

If  $7s \leq j < 8s$ , then

$$b_{ij} = \begin{cases} -w_{8(j+m)+7 \rightarrow 8(j+m+1)+2} \otimes e_{8j+5}, & i = j + 2s; \\ w_{8(j+m)+7 \rightarrow 8(j+m+1)+2} \otimes w_{8j+5 \rightarrow 8j+6}, & i = j + 4s; \\ 0, & \text{otherwise.} \end{cases}$$

If  $8s \leq j < 9s$ , then  $b_{ij} = 0$ .

If  $9s \leq j < 10s$ , then

$$b_{ij} = \begin{cases} -w_{8(j+m+1)+2 \rightarrow 8(j+m+1)+3} \otimes w_{8j+6 \rightarrow 8(j+1)}, & i = (j + 1)_s; \\ w_{8(j+m)+7 \rightarrow 8(j+m+1)+3} \otimes e_{8j+6}, & i = j + 2s; \\ 0, & \text{otherwise.} \end{cases}$$

If  $10s \leq j < 11s$ , then  $b_{ij} = 0$ .

If  $11s \leq j < 12s$ , then

$$b_{ij} = \begin{cases} -w_{8(j+m+1)+2 \rightarrow 8(j+m+1)+7} \otimes w_{8j+7 \rightarrow 8(j+1)}, & i = (j+1)_s; \\ -w_{8(j+m+1)+2 \rightarrow 8(j+m+1)+7} \otimes e_{8j+7}, & i = j + 2s; \\ w_{8(j+m+1)+4 \rightarrow 8(j+m+1)+7} \otimes e_{8j+7}, & i = j + 4s; \\ 0, & \text{otherwise.} \end{cases}$$

If  $12s \leq j < 13s$ , then  $b_{ij} = 0$ .

(15) If  $r_0 = 14$ , then  $\Omega^{14}(Z_t^{(23)})$  is described with  $(20s \times 14s)$  matrix, whose entries  $b_{ij}$  have the following form:

If  $0 \leq j < s$ , then

$$b_{ij} = \begin{cases} w_{8(j+m-1)+7 \rightarrow 8(j+m)+2} \otimes e_{8j}, & i = j; \\ -w_{8(j+m) \rightarrow 8(j+m)+2} \otimes e_{8j}, & i = j + s; \\ -w_{8(j+m)+1 \rightarrow 8(j+m)+2} \otimes w_{8j \rightarrow 8j+3}, & i = j + 8s; \\ -e_{8(j+m)+2} \otimes w_{8j \rightarrow 8j+4}, & i = j + 9s; \\ e_{8(j+m)+2} \otimes w_{8j \rightarrow 8j+6}, & i = j + 14s; \\ 0, & \text{otherwise.} \end{cases}$$

If  $s \leq j < 2s$ , then

$$b_{ij} = \begin{cases} -w_{8(j+m)+3 \rightarrow 8(j+m)+4} \otimes w_{8j \rightarrow 8j+1}, & i = j + 2s; \\ w_{8(j+m)+3 \rightarrow 8(j+m)+4} \otimes w_{8j \rightarrow 8j+5}, & i = j + 11s; \\ 0, & \text{otherwise.} \end{cases}$$

If  $2s \leq j < 3s$ , then

$$b_{ij} = \begin{cases} e_{8(j+m)+6} \otimes w_{8j \rightarrow 8j+2}, & i = j + 4s; \\ 0, & \text{otherwise.} \end{cases}$$

If  $3s \leq j < 4s$ , then

$$b_{ij} = \begin{cases} -e_{8(j+m)+5} \otimes w_{8j \rightarrow 8j+1}, & i = j + s; \\ 0, & \text{otherwise.} \end{cases}$$

If  $4s \leq j < 5s$ , then

$$b_{ij} = \begin{cases} w_{8(j+m)+3 \rightarrow 8(j+m)+7} \otimes e_{8j+1}, & i = j - s; \\ -w_{8(j+m)+5 \rightarrow 8(j+m)+7} \otimes e_{8j+1}, & i = j; \\ 0, & \text{otherwise.} \end{cases}$$

If  $5s \leq j < 6s$ , then

$$b_{ij} = \begin{cases} -w_{8(j+m)+7 \rightarrow 8(j+m+1)} \otimes w_{8j+2 \rightarrow 8(j+1)}, & i = (j+1)_s; \\ e_{8(j+m+1)} \otimes w_{8j+2 \rightarrow 8(j+1)}, & i = s + (j+1)_s; \\ e_{8(j+m+1)} \otimes w_{8j+2 \rightarrow 8(j+1)}, & i = 2s + (j+1)_s; \\ 0, & \text{otherwise.} \end{cases}$$



If  $6s \leq j < 7s$ , then

$$b_{ij} = \begin{cases} e_{8(j+m)+7} \otimes w_{8j+3 \rightarrow 8(j+1)}, & i = (j+1)_s; \\ -w_{8(j+m)+5 \rightarrow 8(j+m)+7} \otimes e_{8j+3}, & i = j+s; \\ w_{8(j+m)+1 \rightarrow 8(j+m)+7} \otimes e_{8j+3}, & i = j+2s; \\ w_{8(j+m)+2 \rightarrow 8(j+m)+7} \otimes w_{8j+3 \rightarrow 8j+4}, & i = j+3s; \\ -e_{8(j+m)+7} \otimes w_{8j+3 \rightarrow 8j+7}, & i = j+13s; \\ 0, & \text{otherwise.} \end{cases}$$

If  $7s \leq j < 8s$ , then

$$b_{ij} = \begin{cases} -e_{8(j+m+1)} \otimes w_{8j+4 \rightarrow 8j+7}, & i = j+11s; \\ 0, & \text{otherwise.} \end{cases}$$

If  $8s \leq j < 9s$ , then

$$b_{ij} = \begin{cases} -w_{8(j+m)+3 \rightarrow 8(j+m)+7} \otimes e_{8j+5}, & i = j+4s; \\ 0, & \text{otherwise.} \end{cases}$$

If  $9s \leq j < 10s$ , then

$$b_{ij} = \begin{cases} w_{8(j+m)+2 \rightarrow 8(j+m)+7} \otimes e_{8j+6}, & i = j+5s; \\ -w_{8(j+m)+4 \rightarrow 8(j+m)+7} \otimes e_{8j+6}, & i = j+6s; \\ 0, & \text{otherwise.} \end{cases}$$

If  $10s \leq j < 12s$ , then  $b_{ij} = 0$ .

If  $12s \leq j < 13s$ , then

$$b_{ij} = \begin{cases} -w_{8(j+m)+7 \rightarrow 8(j+m+1)+3} \otimes w_{8j+7 \rightarrow 8(j+1)}, & i = (j+1)_s; \\ -e_{8(j+m+1)+3} \otimes w_{8j+7 \rightarrow 8(j+1)+1}, & i = 3s + (j+1)_s; \\ e_{8(j+m+1)+3} \otimes w_{8j+7 \rightarrow 8(j+1)+5}, & i = 12s + (j+1)_s; \\ -w_{8(j+m+1) \rightarrow 8(j+m+1)+3} \otimes e_{8j+7}, & i = j+6s; \\ 0, & \text{otherwise.} \end{cases}$$

If  $13s \leq j < 14s$ , then  $b_{ij} = 0$ .

(16) If  $r_0 = 15$ , then  $\Omega^{15}(Z_t^{(23)})$  is described with  $(18s \times 16s)$  matrix, whose entries  $b_{ij}$  have the following form:

If  $0 \leq j < s$ , then

$$b_{ij} = \begin{cases} w_{8(j+m)+3 \rightarrow 8(j+m)+7} \otimes e_{8j}, & i = j; \\ w_{8(j+m)+4 \rightarrow 8(j+m)+7} \otimes e_{8j}, & i = j+2s; \\ -e_{8(j+m)+7} \otimes w_{8j \rightarrow 8j+1}, & i = j+5s; \\ -e_{8(j+m)+7} \otimes w_{8j \rightarrow 8j+2}, & i = j+6s; \\ 0, & \text{otherwise.} \end{cases}$$

If  $s \leq j < 2s$ , then  $b_{ij} = 0$ .

If  $2s \leq j < 3s$ , then

$$b_{ij} = \begin{cases} e_{8(j+m+1)} \otimes w_{8j \rightarrow 8j+2}, & i = j + 5s; \\ -e_{8(j+m+1)} \otimes w_{8j \rightarrow 8j+3}, & i = j + 6s; \\ 0, & \text{otherwise.} \end{cases}$$

If  $3s \leq j < 4s$ , then

$$b_{ij} = \begin{cases} e_{8(j+m+1)+5} \otimes w_{8j+1 \rightarrow 8(j+1)}, & i = 4s + (j+1)_s; \\ w_{8(j+m)+7 \rightarrow 8(j+m+1)+5} \otimes e_{8j+1}, & i = j + 2s; \\ w_{8(j+m+1) \rightarrow 8(j+m+1)+5} \otimes w_{8j+1 \rightarrow 8j+2}, & i = j + 4s; \\ 0, & \text{otherwise.} \end{cases}$$

If  $4s \leq j < 5s$ , then

$$b_{ij} = \begin{cases} -e_{8(j+m+1)+6} \otimes w_{8j+2 \rightarrow 8(j+1)}, & i = s + (j+1)_s; \\ w_{8(j+m+1)+5 \rightarrow 8(j+m+1)+6} \otimes w_{8j+2 \rightarrow 8(j+1)}, & i = 4s + (j+1)_s; \\ 0, & \text{otherwise.} \end{cases}$$

If  $5s \leq j < 6s$ , then

$$b_{ij} = \begin{cases} -e_{8(j+m+1)+1} \otimes w_{8j+2 \rightarrow 8(j+1)}, & i = 3s + (j+1)_s; \\ w_{8(j+m+1) \rightarrow 8(j+m+1)+1} \otimes w_{8j+2 \rightarrow 8j+3}, & i = j + 3s; \\ 0, & \text{otherwise.} \end{cases}$$

If  $6s \leq j < 7s$ , then

$$b_{ij} = \begin{cases} -w_{8(j+m+1)+1 \rightarrow 8(j+m+1)+2} \otimes w_{8j+3 \rightarrow 8(j+1)}, & i = 3s + (j+1)_s; \\ -w_{8(j+m+1) \rightarrow 8(j+m+1)+2} \otimes e_{8j+3}, & i = j + 2s; \\ 0, & \text{otherwise.} \end{cases}$$

If  $7s \leq j < 8s$ , then

$$b_{ij} = \begin{cases} -e_{8(j+m+1)+3} \otimes w_{8j+4 \rightarrow 8(j+1)}, & i = (j+1)_s; \\ 0, & \text{otherwise.} \end{cases}$$

If  $8s \leq j < 9s$ , then

$$b_{ij} = \begin{cases} -e_{8(j+m+1)+5} \otimes w_{8j+4 \rightarrow 8j+7}, & i = j + 9s; \\ 0, & \text{otherwise.} \end{cases}$$

If  $9s \leq j < 10s$ , then

$$b_{ij} = \begin{cases} -e_{8(j+m+1)+3} \otimes w_{8j+5 \rightarrow 8(j+1)}, & i = (j+1)_s; \\ -w_{8(j+m+1) \rightarrow 8(j+m+1)+3} \otimes e_{8j+5}, & i = j + 2s; \\ w_{8(j+m+1) \rightarrow 8(j+m+1)+3} \otimes w_{8j+5 \rightarrow 8j+6}, & i = j + 3s; \\ 0, & \text{otherwise.} \end{cases}$$

If  $10s \leq j < 12s$ , then  $b_{ij} = 0$ .

If  $12s \leq j < 13s$ , then

$$b_{ij} = \begin{cases} w_{8(j+m+1)+3 \rightarrow 8(j+m+1)+4} \otimes w_{8j+6 \rightarrow 8(j+1)}, & i = (j+1)_s; \\ w_{8(j+m+1) \rightarrow 8(j+m+1)+4} \otimes e_{8j+6}, & i = j; \\ 0, & \text{otherwise.} \end{cases}$$

If  $13s \leq j < 14s$ , then  $b_{ij} = 0$ .

If  $14s \leq j < 15s$ , then

$$b_{ij} = \begin{cases} w_{8(j+m+1)+3 \rightarrow 8(j+m+1)+7} \otimes w_{8j+7 \rightarrow 8(j+1)}, & i = (j+1)_s; \\ -e_{8(j+m+1)+7} \otimes w_{8j+7 \rightarrow 8(j+1)+1}, & i = 5s + (j+1)_s; \\ -w_{8(j+m+1)+2 \rightarrow 8(j+m+1)+7} \otimes e_{8j+7}, & i = j; \\ w_{8(j+m+1)+3 \rightarrow 8(j+m+1)+7} \otimes e_{8j+7}, & i = j+s; \\ -w_{8(j+m+1)+6 \rightarrow 8(j+m+1)+7} \otimes e_{8j+7}, & i = j+2s; \\ 0, & \text{otherwise.} \end{cases}$$

If  $15s \leq j < 16s$ , then

$$b_{ij} = \begin{cases} -w_{8(j+m+1)+3 \rightarrow 8(j+m+2)} \otimes w_{8j+7 \rightarrow 8(j+1)}, & i = (j+1)_s; \\ w_{8(j+m+1)+7 \rightarrow 8(j+m+2)} \otimes w_{8j+7 \rightarrow 8(j+1)+1}, & i = 5s + (j+1)_s; \\ e_{8(j+m+2)} \otimes w_{8j+7 \rightarrow 8(j+1)+2}, & i = 7s + (j+1)_s; \\ e_{8(j+m+2)} \otimes w_{8j+7 \rightarrow 8(j+1)+5}, & i = 11s + (j+1)_s; \\ w_{8(j+m+1)+2 \rightarrow 8(j+m+2)} \otimes e_{8j+7}, & i = j-s; \\ 0, & \text{otherwise.} \end{cases}$$

(17) If  $r_0 = 16$ , then  $\Omega^{16}(Z_t^{(23)})$  is described with  $(19s \times 16s)$  matrix, whose entries  $b_{ij}$  have the following form:

If  $0 \leq j < s$ , then

$$b_{ij} = \begin{cases} -e_{8(j+m)+5} \otimes w_{8j \rightarrow 8j+2}, & i = j+5s; \\ 0, & \text{otherwise.} \end{cases}$$

If  $s \leq j < 2s$ , then

$$b_{ij} = \begin{cases} w_{8(j+m) \rightarrow 8(j+m)+3} \otimes e_{8j}, & i = j; \\ -w_{8(j+m-1)+7 \rightarrow 8(j+m)+3} \otimes e_{8j}, & i = j+s; \\ -w_{8(j+m)+1 \rightarrow 8(j+m)+3} \otimes w_{8j \rightarrow 8j+2}, & i = j+5s; \\ w_{8(j+m)+2 \rightarrow 8(j+m)+3} \otimes w_{8j \rightarrow 8j+3}, & i = j+6s; \\ -e_{8(j+m)+3} \otimes w_{8j \rightarrow 8j+4}, & i = j+8s; \\ e_{8(j+m)+3} \otimes w_{8j \rightarrow 8j+6}, & i = j+12s; \\ 0, & \text{otherwise.} \end{cases}$$

If  $2s \leq j < 3s$ , then

$$b_{ij} = \begin{cases} -e_{8(j+m)+6} \otimes w_{8j \rightarrow 8j+1}, & i = j+2s; \\ 0, & \text{otherwise.} \end{cases}$$

If  $3s \leq j < 4s$ , then

$$b_{ij} = \begin{cases} e_{8(j+m)+1} \otimes w_{8j \rightarrow 8j+2}, & i = j + 3s; \\ 0, & \text{otherwise.} \end{cases}$$

If  $4s \leq j < 5s$ , then

$$b_{ij} = \begin{cases} w_{8(j+m)+6 \rightarrow 8(j+m+1)} \otimes e_{8j+1}, & i = j; \\ 0, & \text{otherwise.} \end{cases}$$

If  $5s \leq j < 6s$ , then

$$b_{ij} = \begin{cases} e_{8(j+m)+7} \otimes w_{8j+2 \rightarrow 8(j+1)}, & i = (j+1)_s; \\ e_{8(j+m)+7} \otimes w_{8j+2 \rightarrow 8(j+1)}, & i = 2s + (j+1)_s; \\ 0, & \text{otherwise.} \end{cases}$$

If  $6s \leq j < 7s$ , then

$$b_{ij} = \begin{cases} e_{8(j+m+1)} \otimes w_{8j+3 \rightarrow 8(j+1)}, & i = s + (j+1)_s; \\ -w_{8(j+m)+2 \rightarrow 8(j+m+1)} \otimes e_{8j+3}, & i = j + s; \\ 0, & \text{otherwise.} \end{cases}$$

If  $7s \leq j < 8s$ , then

$$b_{ij} = \begin{cases} e_{8(j+m)+7} \otimes w_{8j+4 \rightarrow 8j+7}, & i = j + 9s; \\ 0, & \text{otherwise.} \end{cases}$$

If  $8s \leq j < 9s$ , then

$$b_{ij} = \begin{cases} -w_{8(j+m)+4 \rightarrow 8(j+m)+7} \otimes e_{8j+5}, & i = j + 3s; \\ 0, & \text{otherwise.} \end{cases}$$

If  $9s \leq j < 10s$ , then  $b_{ij} = 0$ .

If  $10s \leq j < 11s$ , then

$$b_{ij} = \begin{cases} -w_{8(j+m)+3 \rightarrow 8(j+m)+7} \otimes e_{8j+6}, & i = j + 3s; \\ w_{8(j+m)+6 \rightarrow 8(j+m)+7} \otimes e_{8j+6}, & i = j + 4s; \\ 0, & \text{otherwise.} \end{cases}$$

If  $11s \leq j < 12s$ , then

$$b_{ij} = \begin{cases} w_{8(j+m)+3 \rightarrow 8(j+m+1)} \otimes e_{8j+6}, & i = j + 2s; \\ -e_{8(j+m+1)} \otimes w_{8j+6 \rightarrow 8j+7}, & i = j + 6s; \\ 0, & \text{otherwise.} \end{cases}$$

If  $12s \leq j < 13s$ , then

$$b_{ij} = \begin{cases} w_{8(j+m+1)+1 \rightarrow 8(j+m+1)+2} \otimes w_{8j+7 \rightarrow 8(j+1)+2}, & i = 6s + (j+1)_s; \\ w_{8(j+m+1) \rightarrow 8(j+m+1)+2} \otimes e_{8j+7}, & i = j + 5s; \\ 0, & \text{otherwise.} \end{cases}$$

If  $13s \leq j < 14s$ , then

$$b_{ij} = \begin{cases} -w_{8(j+m+1) \rightarrow 8(j+m+1)+4} \otimes w_{8j+7 \rightarrow 8(j+1)}, & i = s + (j+1)_s; \\ -w_{8(j+m+1)+1 \rightarrow 8(j+m+1)+4} \otimes w_{8j+7 \rightarrow 8(j+1)+2}, & i = 6s + (j+1)_s; \\ -e_{8(j+m+1)+4} \otimes w_{8j+7 \rightarrow 8(j+1)+5}, & i = 11s + (j+1)_s; \\ 0, & \text{otherwise.} \end{cases}$$

If  $14s \leq j < 15s$ , then

$$b_{ij} = \begin{cases} e_{8(j+m+1)+6} \otimes w_{8j+7 \rightarrow 8(j+1)+1}, & i = 4s + (j+1)_s; \\ -w_{8(j+m)+7 \rightarrow 8(j+m+1)+6} \otimes e_{8j+7}, & i = j + 2s; \\ 0, & \text{otherwise.} \end{cases}$$

If  $15s \leq j < 16s$ , then

$$b_{ij} = \begin{cases} e_{8(j+m+1)+5} \otimes w_{8j+7 \rightarrow 8(j+1)+5}, & i = 12s + (j+1)_s; \\ 0, & \text{otherwise.} \end{cases}$$

(18) If  $r_0 = 17$ , then  $\Omega^{17}(Z_t^{(23)})$  is described with  $(18s \times 19s)$  matrix, whose entries  $b_{ij}$  have the following form:

If  $0 \leq j < s$ , then

$$b_{ij} = \begin{cases} w_{8(j+m)+2 \rightarrow 8(j+m)+7} \otimes e_{8j}, & i = j; \\ -w_{8(j+m)+4 \rightarrow 8(j+m)+7} \otimes e_{8j}, & i = j + s; \\ -w_{8(j+m)+6 \rightarrow 8(j+m)+7} \otimes e_{8j}, & i = j + 2s; \\ -e_{8(j+m)+7} \otimes w_{8j \rightarrow 8j+1}, & i = j + 4s; \\ e_{8(j+m)+7} \otimes w_{8j \rightarrow 8j+3}, & i = j + 7s; \\ 0, & \text{otherwise.} \end{cases}$$

If  $s \leq j < 2s$ , then

$$b_{ij} = \begin{cases} -w_{8(j+m)+2 \rightarrow 8(j+m+1)} \otimes e_{8j}, & i = j - s; \\ w_{8(j+m)+4 \rightarrow 8(j+m+1)} \otimes e_{8j}, & i = j; \\ w_{8(j+m)+7 \rightarrow 8(j+m+1)} \otimes w_{8j \rightarrow 8j+1}, & i = j + 3s; \\ e_{8(j+m+1)} \otimes w_{8j \rightarrow 8j+1}, & i = j + 4s; \\ e_{8(j+m+1)} \otimes w_{8j \rightarrow 8j+4}, & i = j + 7s; \\ 0, & \text{otherwise.} \end{cases}$$

If  $2s \leq j < 3s$ , then  $b_{ij} = 0$ .

If  $3s \leq j < 4s$ , then

$$b_{ij} = \begin{cases} -e_{8(j+m+1)+6} \otimes w_{8j+1 \rightarrow 8(j+1)}, & i = 2s + (j+1)_s; \\ -w_{8(j+m)+7 \rightarrow 8(j+m+1)+6} \otimes e_{8j+1}, & i = j + s; \\ 0, & \text{otherwise.} \end{cases}$$

If  $4s \leq j < 5s$ , then  $b_{ij} = 0$ .

If  $5s \leq j < 6s$ , then

$$b_{ij} = \begin{cases} -e_{8(j+m+1)+2} \otimes w_{8j+2 \rightarrow 8(j+1)}, & i = (j+1)_s; \\ -w_{8(j+m)+7 \rightarrow 8(j+m+1)+2} \otimes w_{8j+2 \rightarrow 8j+3}, & i = j+2s; \\ -w_{8(j+m+1) \rightarrow 8(j+m+1)+2} \otimes w_{8j+2 \rightarrow 8j+4}, & i = j+3s; \\ 0, & \text{otherwise.} \end{cases}$$

If  $6s \leq j < 7s$ , then

$$b_{ij} = \begin{cases} w_{8(j+m+1)+2 \rightarrow 8(j+m+1)+3} \otimes w_{8j+3 \rightarrow 8(j+1)}, & i = (j+1)_s; \\ -w_{8(j+m)+7 \rightarrow 8(j+m+1)+3} \otimes e_{8j+3}, & i = j+s; \\ -w_{8(j+m+1) \rightarrow 8(j+m+1)+3} \otimes w_{8j+3 \rightarrow 8j+4}, & i = j+2s; \\ 0, & \text{otherwise.} \end{cases}$$

If  $7s \leq j < 8s$ , then

$$b_{ij} = \begin{cases} e_{8(j+m+1)+5} \otimes w_{8j+3 \rightarrow 8(j+1)}, & i = 3s + (j+1)_s; \\ 0, & \text{otherwise.} \end{cases}$$

If  $8s \leq j < 9s$ , then

$$b_{ij} = \begin{cases} w_{8(j+m+1)+3 \rightarrow 8(j+m+1)+4} \otimes w_{8j+4 \rightarrow 8j+7}, & i = j+5s; \\ 0, & \text{otherwise.} \end{cases}$$

If  $9s \leq j < 11s$ , then  $b_{ij} = 0$ .

If  $11s \leq j < 12s$ , then

$$b_{ij} = \begin{cases} -w_{8(j+m+1)+2 \rightarrow 8(j+m+1)+4} \otimes w_{8j+5 \rightarrow 8(j+1)}, & i = (j+1)_s; \\ e_{8(j+m+1)+4} \otimes w_{8j+5 \rightarrow 8(j+1)}, & i = s + (j+1)_s; \\ -w_{8(j+m+1) \rightarrow 8(j+m+1)+4} \otimes e_{8j+5}, & i = j-2s; \\ w_{8(j+m)+7 \rightarrow 8(j+m+1)+4} \otimes e_{8j+5}, & i = j-s; \\ 0, & \text{otherwise.} \end{cases}$$

If  $12s \leq j < 14s$ , then  $b_{ij} = 0$ .

If  $14s \leq j < 15s$ , then

$$b_{ij} = \begin{cases} -w_{8(j+m)+7 \rightarrow 8(j+m+1)+6} \otimes e_{8j+6}, & i = j-3s; \\ 0, & \text{otherwise.} \end{cases}$$

If  $15s \leq j < 16s$ , then

$$b_{ij} = \begin{cases} -e_{8(j+m+1)+5} \otimes w_{8j+6 \rightarrow 8j+7}, & i = j+2s; \\ 0, & \text{otherwise.} \end{cases}$$

If  $16s \leq j < 17s$ , then

$$b_{ij} = \begin{cases} -w_{8(j+m+1)+2 \rightarrow 8(j+m+1)+7} \otimes w_{8j+7 \rightarrow 8(j+1)}, & i = (j+1)_s; \\ w_{8(j+m+1)+4 \rightarrow 8(j+m+1)+7} \otimes w_{8j+7 \rightarrow 8(j+1)}, & i = s + (j+1)_s; \\ e_{8(j+m+1)+7} \otimes w_{8j+7 \rightarrow 8(j+1)+1}, & i = 4s + (j+1)_s; \\ e_{8(j+m+1)+7} \otimes w_{8j+7 \rightarrow 8(j+1)+5}, & i = 10s + (j+1)_s; \\ w_{8(j+m+1)+3 \rightarrow 8(j+m+1)+7} \otimes e_{8j+7}, & i = j - 3s; \\ 0, & \text{otherwise.} \end{cases}$$

If  $17s \leq j < 18s$ , then

$$b_{ij} = \begin{cases} -w_{8(j+m+1)+2 \rightarrow 8(j+m+1)+7} \otimes w_{8j+7 \rightarrow 8(j+1)}, & i = (j+1)_s; \\ w_{8(j+m+1)+4 \rightarrow 8(j+m+1)+7} \otimes w_{8j+7 \rightarrow 8(j+1)}, & i = s + (j+1)_s; \\ e_{8(j+m+1)+7} \otimes w_{8j+7 \rightarrow 8(j+1)+1}, & i = 4s + (j+1)_s; \\ e_{8(j+m+1)+7} \otimes w_{8j+7 \rightarrow 8(j+1)+5}, & i = 10s + (j+1)_s; \\ 0, & \text{otherwise.} \end{cases}$$

If  $18s \leq j < 19s$ , then  $b_{ij} = 0$ .

(19) If  $r_0 = 18$ , then  $\Omega^{18}(Z_t^{(23)})$  is described with  $(19s \times 18s)$  matrix, whose entries  $b_{ij}$  have the following form:

If  $0 \leq j < s$ , then

$$b_{ij} = \begin{cases} w_{8(j+m)+1 \rightarrow 8(j+m)+2} \otimes w_{8j \rightarrow 8j+1}, & i = j + 4s; \\ e_{8(j+m)+2} \otimes w_{8j \rightarrow 8j+2}, & i = j + 5s; \\ 0, & \text{otherwise.} \end{cases}$$

If  $s \leq j < 2s$ , then

$$b_{ij} = \begin{cases} -w_{8(j+m-1)+7 \rightarrow 8(j+m)+6} \otimes e_{8j}, & i = j - s; \\ -e_{8(j+m)+6} \otimes w_{8j \rightarrow 8j+5}, & i = j + 10s; \\ 0, & \text{otherwise.} \end{cases}$$

If  $2s \leq j < 3s$ , then

$$b_{ij} = \begin{cases} w_{8(j+m-1)+7 \rightarrow 8(j+m)+4} \otimes e_{8j}, & i = j - 2s; \\ -w_{8(j+m) \rightarrow 8(j+m)+4} \otimes e_{8j}, & i = j - s; \\ -w_{8(j+m)+1 \rightarrow 8(j+m)+4} \otimes w_{8j \rightarrow 8j+1}, & i = j + 2s; \\ -w_{8(j+m)+2 \rightarrow 8(j+m)+4} \otimes w_{8j \rightarrow 8j+2}, & i = j + 3s; \\ -e_{8(j+m)+4} \otimes w_{8j \rightarrow 8j+4}, & i = j + 6s; \\ e_{8(j+m)+4} \otimes w_{8j \rightarrow 8j+6}, & i = j + 12s; \\ 0, & \text{otherwise.} \end{cases}$$

If  $3s \leq j < 4s$ , then  $b_{ij} = 0$ .

If  $4s \leq j < 5s$ , then

$$b_{ij} = \begin{cases} e_{8(j+m)+5} \otimes w_{8j \rightarrow 8j+1}, & i = j - s; \\ e_{8(j+m)+5} \otimes w_{8j \rightarrow 8j+4}, & i = j + 5s; \\ 0, & \text{otherwise.} \end{cases}$$

If  $5s \leq j < 6s$ , then

$$b_{ij} = \begin{cases} e_{8(j+m)+7} \otimes w_{8j+1 \rightarrow 8(j+1)}, & i = (j+1)_s; \\ -w_{8(j+m)+5 \rightarrow 8(j+m)+7} \otimes e_{8j+1}, & i = j - 2s; \\ w_{8(j+m)+1 \rightarrow 8(j+m)+7} \otimes e_{8j+1}, & i = j - s; \\ w_{8(j+m)+2 \rightarrow 8(j+m)+7} \otimes w_{8j+1 \rightarrow 8j+2}, & i = j; \\ 0, & \text{otherwise.} \end{cases}$$

If  $6s \leq j < 7s$ , then

$$b_{ij} = \begin{cases} e_{8(j+m+1)} \otimes w_{8j+2 \rightarrow 8(j+1)}, & i = s + (j+1)_s; \\ 0, & \text{otherwise.} \end{cases}$$

If  $7s \leq j < 8s$ , then

$$b_{ij} = \begin{cases} -e_{8(j+m)+7} \otimes w_{8j+3 \rightarrow 8(j+1)}, & i = (j+1)_s; \\ -w_{8(j+m)+3 \rightarrow 8(j+m)+7} \otimes e_{8j+3}, & i = j; \\ 0, & \text{otherwise.} \end{cases}$$

If  $8s \leq j < 10s$ , then  $b_{ij} = 0$ .

If  $10s \leq j < 11s$ , then

$$b_{ij} = \begin{cases} -e_{8(j+m)+7} \otimes w_{8j+5 \rightarrow 8(j+1)}, & i = (j+1)_s; \\ -w_{8(j+m)+6 \rightarrow 8(j+m)+7} \otimes e_{8j+5}, & i = j + s; \\ w_{8(j+m)+5 \rightarrow 8(j+m)+7} \otimes e_{8j+5}, & i = j + 2s; \\ 0, & \text{otherwise.} \end{cases}$$

If  $11s \leq j < 12s$ , then

$$b_{ij} = \begin{cases} w_{8(j+m)+7 \rightarrow 8(j+m+1)} \otimes w_{8j+5 \rightarrow 8(j+1)}, & i = (j+1)_s; \\ -e_{8(j+m+1)} \otimes w_{8j+5 \rightarrow 8(j+1)}, & i = 2s + (j+1)_s; \\ -w_{8(j+m)+5 \rightarrow 8(j+m+1)} \otimes e_{8j+5}, & i = j + s; \\ 0, & \text{otherwise.} \end{cases}$$

If  $12s \leq j < 13s$ , then

$$b_{ij} = \begin{cases} w_{8(j+m)+6 \rightarrow 8(j+m)+7} \otimes e_{8j+6}, & i = j + s; \\ -w_{8(j+m)+1 \rightarrow 8(j+m)+7} \otimes e_{8j+6}, & i = j + 3s; \\ -e_{8(j+m)+7} \otimes w_{8j+6 \rightarrow 8j+7}, & i = j + 4s; \\ 0, & \text{otherwise.} \end{cases}$$

If  $13s \leq j < 15s$ , then  $b_{ij} = 0$ .

If  $15s \leq j < 16s$ , then

$$b_{ij} = \begin{cases} w_{8(j+m)+7 \rightarrow 8(j+m+1)+3} \otimes e_{8j+7}, & i = j + s; \\ 0, & \text{otherwise.} \end{cases}$$

If  $16s \leq j < 17s$ , then

$$b_{ij} = \begin{cases} e_{8(j+m+1)+6} \otimes w_{8j+7 \rightarrow 8(j+1)+5}, & i = 11s + (j+1)_s; \\ 0, & \text{otherwise.} \end{cases}$$



If  $17s \leq j < 18s$ , then  $b_{ij} = 0$ .

(20) If  $r_0 = 19$ , then  $\Omega^{19}(Z_t^{(23)})$  is described with  $(16s \times 19s)$  matrix, whose entries  $b_{ij}$  have the following form:

If  $0 \leq j < s$ , then

$$b_{ij} = \begin{cases} w_{8(j+m)+6 \rightarrow 8(j+m)+7} \otimes e_{8j}, & i = j + s; \\ w_{8(j+m)+1 \rightarrow 8(j+m)+7} \otimes e_{8j}, & i = j + 2s; \\ -e_{8(j+m)+7} \otimes w_{8j \rightarrow 8j+2}, & i = j + 5s; \\ 0, & \text{otherwise.} \end{cases}$$

If  $s \leq j < 2s$ , then

$$b_{ij} = \begin{cases} w_{8(j+m)+5 \rightarrow 8(j+m+1)} \otimes e_{8j}, & i = j + 2s; \\ e_{8(j+m+1)} \otimes w_{8j \rightarrow 8j+1}, & i = j + 3s; \\ w_{8(j+m)+7 \rightarrow 8(j+m+1)} \otimes w_{8j \rightarrow 8j+4}, & i = j + 6s; \\ w_{8(j+m)+7 \rightarrow 8(j+m+1)} \otimes w_{8j \rightarrow 8j+6}, & i = j + 9s; \\ 0, & \text{otherwise.} \end{cases}$$

If  $2s \leq j < 3s$ , then

$$b_{ij} = \begin{cases} w_{8(j+m)+6 \rightarrow 8(j+m)+7} \otimes e_{8j}, & i = j - s; \\ w_{8(j+m)+1 \rightarrow 8(j+m)+7} \otimes e_{8j}, & i = j; \\ -w_{8(j+m)+5 \rightarrow 8(j+m)+7} \otimes e_{8j}, & i = j + s; \\ -e_{8(j+m)+7} \otimes w_{8j \rightarrow 8j+2}, & i = j + 3s; \\ -e_{8(j+m)+7} \otimes w_{8j \rightarrow 8j+4}, & i = j + 5s; \\ -e_{8(j+m)+7} \otimes w_{8j \rightarrow 8j+6}, & i = j + 8s; \\ 0, & \text{otherwise.} \end{cases}$$

If  $3s \leq j < 4s$ , then

$$b_{ij} = \begin{cases} w_{8(j+m+1)+1 \rightarrow 8(j+m+1)+2} \otimes w_{8j+1 \rightarrow 8(j+1)}, & i = 2s + (j+1)_s; \\ -w_{8(j+m+1) \rightarrow 8(j+m+1)+2} \otimes e_{8j+1}, & i = j + s; \\ 0, & \text{otherwise.} \end{cases}$$

If  $4s \leq j < 5s$ , then

$$b_{ij} = \begin{cases} e_{8(j+m+1)+3} \otimes w_{8j+2 \rightarrow 8(j+1)}, & i = (j+1)_s; \\ w_{8(j+m)+7 \rightarrow 8(j+m+1)+3} \otimes e_{8j+2}, & i = j + s; \\ 0, & \text{otherwise.} \end{cases}$$

If  $5s \leq j < 6s$ , then

$$b_{ij} = \begin{cases} e_{8(j+m+1)+5} \otimes w_{8j+2 \rightarrow 8(j+1)}, & i = 3s + (j+1)_s; \\ 0, & \text{otherwise.} \end{cases}$$

If  $6s \leq j < 7s$ , then

$$b_{ij} = \begin{cases} -w_{8(j+m+1) \rightarrow 8(j+m+1)+4} \otimes e_{8j+3}, & i = j; \\ -w_{8(j+m)+7 \rightarrow 8(j+m+1)+4} \otimes w_{8j+3 \rightarrow 8j+4}, & i = j + s; \\ w_{8(j+m+1)+2 \rightarrow 8(j+m+1)+4} \otimes w_{8j+3 \rightarrow 8j+7}, & i = j + 6s; \\ 0, & \text{otherwise.} \end{cases}$$

If  $7s \leq j < 10s$ , then  $b_{ij} = 0$ .

If  $10s \leq j < 11s$ , then

$$b_{ij} = \begin{cases} -w_{8(j+m+1)+1 \rightarrow 8(j+m+1)+2} \otimes w_{8j+5 \rightarrow 8(j+1)}, & i = 2s + (j + 1)_s; \\ 0, & \text{otherwise.} \end{cases}$$

If  $11s \leq j < 12s$ , then

$$b_{ij} = \begin{cases} -e_{8(j+m+1)+6} \otimes w_{8j+5 \rightarrow 8(j+1)}, & i = s + (j + 1)_s; \\ -w_{8(j+m)+7 \rightarrow 8(j+m+1)+6} \otimes e_{8j+5}, & i = j - 3s; \\ w_{8(j+m+1) \rightarrow 8(j+m+1)+6} \otimes e_{8j+5}, & i = j - 2s; \\ 0, & \text{otherwise.} \end{cases}$$

If  $12s \leq j < 13s$ , then

$$b_{ij} = \begin{cases} w_{8(j+m)+7 \rightarrow 8(j+m+1)+5} \otimes e_{8j+5}, & i = j - 4s; \\ w_{8(j+m+1) \rightarrow 8(j+m+1)+5} \otimes e_{8j+5}, & i = j - 3s; \\ 0, & \text{otherwise.} \end{cases}$$

If  $13s \leq j < 14s$ , then

$$b_{ij} = \begin{cases} w_{8(j+m)+7 \rightarrow 8(j+m+1)+6} \otimes e_{8j+6}, & i = j - 3s; \\ -e_{8(j+m+1)+6} \otimes w_{8j+6 \rightarrow 8j+7}, & i = j + s; \\ 0, & \text{otherwise.} \end{cases}$$

If  $14s \leq j < 16s$ , then  $b_{ij} = 0$ .

If  $16s \leq j < 17s$ , then

$$b_{ij} = \begin{cases} w_{8(j+m+1)+6 \rightarrow 8(j+m+1)+7} \otimes w_{8j+7 \rightarrow 8(j+1)}, & i = s + (j + 1)_s; \\ w_{8(j+m+1)+1 \rightarrow 8(j+m+1)+7} \otimes w_{8j+7 \rightarrow 8(j+1)}, & i = 2s + (j + 1)_s; \\ -e_{8(j+m+1)+7} \otimes w_{8j+7 \rightarrow 8(j+1)+2}, & i = 5s + (j + 1)_s; \\ -e_{8(j+m+1)+7} \otimes w_{8j+7 \rightarrow 8(j+1)+4}, & i = 7s + (j + 1)_s; \\ -e_{8(j+m+1)+7} \otimes w_{8j+7 \rightarrow 8(j+1)+6}, & i = 10s + (j + 1)_s; \\ -w_{8(j+m+1)+4 \rightarrow 8(j+m+1)+7} \otimes e_{8j+7}, & i = j - 3s; \\ 0, & \text{otherwise.} \end{cases}$$

If  $17s \leq j < 18s$ , then  $b_{ij} = 0$ .

If  $18s \leq j < 19s$ , then

$$b_{ij} = \begin{cases} -w_{8(j+m+1)+3 \rightarrow 8(j+m+2)} \otimes w_{8j+7 \rightarrow 8(j+1)}, & i = (j+1)_s; \\ -w_{8(j+m+1)+5 \rightarrow 8(j+m+2)} \otimes w_{8j+7 \rightarrow 8(j+1)}, & i = 3s + (j+1)_s; \\ e_{8(j+m+2)} \otimes w_{8j+7 \rightarrow 8(j+1)+1}, & i = 4s + (j+1)_s; \\ w_{8(j+m+1)+7 \rightarrow 8(j+m+2)} \otimes w_{8j+7 \rightarrow 8(j+1)+4}, & i = 7s + (j+1)_s; \\ w_{8(j+m+1)+7 \rightarrow 8(j+m+2)} \otimes w_{8j+7 \rightarrow 8(j+1)+5}, & i = 8s + (j+1)_s; \\ -e_{8(j+m+2)} \otimes w_{8j+7 \rightarrow 8(j+1)+5}, & i = 9s + (j+1)_s; \\ w_{8(j+m+1)+7 \rightarrow 8(j+m+2)} \otimes w_{8j+7 \rightarrow 8(j+1)+6}, & i = 10s + (j+1)_s; \\ 0, & \text{otherwise.} \end{cases}$$

(21) If  $r_0 = 20$ , then  $\Omega^{20}(Z_t^{(23)})$  is described with  $(16s \times 18s)$  matrix, whose entries  $b_{ij}$  have the following form:

If  $s \leq j < 2s$ , then

$$b_{ij} = \begin{cases} w_{8(j+m)+2 \rightarrow 8(j+m)+3} \otimes w_{8j \rightarrow 8j+1}, & i = j + s; \\ -e_{8(j+m)+3} \otimes w_{8j \rightarrow 8j+2}, & i = j + 3s; \\ 0, & \text{otherwise.} \end{cases}$$

If  $2s \leq j < 3s$ , then

$$b_{ij} = \begin{cases} -w_{8(j+m-1)+7 \rightarrow 8(j+m)+6} \otimes e_{8j}, & i = j - 2s; \\ -e_{8(j+m)+6} \otimes w_{8j \rightarrow 8j+4}, & i = j + 5s; \\ e_{8(j+m)+6} \otimes w_{8j \rightarrow 8j+5}, & i = j + 6s; \\ 0, & \text{otherwise.} \end{cases}$$

If  $3s \leq j < 4s$ , then

$$b_{ij} = \begin{cases} -w_{8(j+m) \rightarrow 8(j+m)+5} \otimes e_{8j}, & i = j - 2s; \\ -e_{8(j+m)+5} \otimes w_{8j \rightarrow 8j+3}, & i = j + 3s; \\ -e_{8(j+m)+5} \otimes w_{8j \rightarrow 8j+6}, & i = j + 9s; \\ 0, & \text{otherwise.} \end{cases}$$

If  $4s \leq j < 5s$ , then

$$b_{ij} = \begin{cases} w_{8(j+m)+7 \rightarrow 8(j+m+1)} \otimes w_{8j+1 \rightarrow 8(j+1)}, & i = (j+1)_s; \\ -e_{8(j+m+1)} \otimes w_{8j+1 \rightarrow 8(j+1)}, & i = s + (j+1)_s; \\ -w_{8(j+m)+6 \rightarrow 8(j+m+1)} \otimes e_{8j+1}, & i = j - s; \\ 0, & \text{otherwise.} \end{cases}$$

If  $5s \leq j < 6s$ , then

$$b_{ij} = \begin{cases} -e_{8(j+m)+7} \otimes w_{8j+2 \rightarrow 8(j+1)}, & i = (j+1)_s; \\ w_{8(j+m)+3 \rightarrow 8(j+m)+7} \otimes e_{8j+2}, & i = j - s; \\ 0, & \text{otherwise.} \end{cases}$$

If  $6s \leq j < 7s$ , then

$$b_{ij} = \begin{cases} -e_{8(j+m)+7} \otimes w_{8j+3 \rightarrow 8(j+1)}, & i = (j+1)_s; \\ -w_{8(j+m)+4 \rightarrow 8(j+m)+7} \otimes e_{8j+3}, & i = j-s; \\ 0, & \text{otherwise.} \end{cases}$$

If  $7s \leq j < 8s$ , then

$$b_{ij} = \begin{cases} e_{8(j+m+1)} \otimes w_{8j+3 \rightarrow 8j+7}, & i = j+7s; \\ 0, & \text{otherwise.} \end{cases}$$

If  $8s \leq j < 9s$ , then

$$b_{ij} = \begin{cases} -w_{8(j+m)+7 \rightarrow 8(j+m+1)} \otimes w_{8j+4 \rightarrow 8(j+1)}, & i = (j+1)_s; \\ e_{8(j+m+1)} \otimes w_{8j+4 \rightarrow 8j+7}, & i = j+6s; \\ 0, & \text{otherwise.} \end{cases}$$

If  $9s \leq j < 10s$ , then

$$b_{ij} = \begin{cases} w_{8(j+m)+1 \rightarrow 8(j+m)+7} \otimes e_{8j+5}, & i = j+s; \\ 0, & \text{otherwise.} \end{cases}$$

If  $10s \leq j < 11s$ , then

$$b_{ij} = \begin{cases} w_{8(j+m)+7 \rightarrow 8(j+m+1)} \otimes w_{8j+5 \rightarrow 8(j+1)}, & i = (j+1)_s; \\ e_{8(j+m+1)} \otimes w_{8j+5 \rightarrow 8(j+1)}, & i = s + (j+1)_s; \\ -w_{8(j+m)+6 \rightarrow 8(j+m+1)} \otimes e_{8j+5}, & i = j-2s; \\ -w_{8(j+m)+1 \rightarrow 8(j+m+1)} \otimes e_{8j+5}, & i = j; \\ 0, & \text{otherwise.} \end{cases}$$

If  $11s \leq j < 12s$ , then

$$b_{ij} = \begin{cases} w_{8(j+m)+2 \rightarrow 8(j+m)+7} \otimes e_{8j+6}, & i = j; \\ -w_{8(j+m)+5 \rightarrow 8(j+m)+7} \otimes e_{8j+6}, & i = j+s; \\ -e_{8(j+m)+7} \otimes w_{8j+6 \rightarrow 8j+7}, & i = j+2s; \\ 0, & \text{otherwise.} \end{cases}$$

If  $12s \leq j < 13s$ , then  $b_{ij} = 0$ .

If  $13s \leq j < 14s$ , then

$$b_{ij} = \begin{cases} w_{8(j+m+1)+1 \rightarrow 8(j+m+1)+2} \otimes w_{8j+7 \rightarrow 8(j+1)+5}, & i = 10s + (j+1)_s; \\ -w_{8(j+m+1) \rightarrow 8(j+m+1)+2} \otimes e_{8j+7}, & i = j+s; \\ 0, & \text{otherwise.} \end{cases}$$

If  $14s \leq j < 15s$ , then  $b_{ij} = 0$ .

If  $15s \leq j < 16s$ , then

$$b_{ij} = \begin{cases} w_{8(j+m+1)+3 \rightarrow 8(j+m+1)+4} \otimes w_{8j+7 \rightarrow 8(j+1)+2}, & i = 4s + (j+1)_s; \\ 0, & \text{otherwise.} \end{cases}$$

If  $16s \leq j < 17s$ , then

$$b_{ij} = \begin{cases} -w_{8(j+m)+7 \rightarrow 8(j+m+1)+1} \otimes w_{8j+7 \rightarrow 8(j+1)}, & i = (j+1)_s; \\ -e_{8(j+m+1)+1} \otimes w_{8j+7 \rightarrow 8(j+1)+5}, & i = 10s + (j+1)_s; \\ 0, & \text{otherwise.} \end{cases}$$

If  $17s \leq j < 18s$ , then  $b_{ij} = 0$ .

(22) If  $r_0 = 21$ , then  $\Omega^{21}(Z_t^{(23)})$  is described with  $(14s \times 20s)$  matrix, whose entries  $b_{ij}$  have the following form:

If  $0 \leq j < s$ , then

$$b_{ij} = \begin{cases} -w_{8(j+m)+2 \rightarrow 8(j+m)+7} \otimes e_{8j}, & i = j; \\ w_{8(j+m)+6 \rightarrow 8(j+m)+7} \otimes e_{8j}, & i = j + 2s; \\ e_{8(j+m)+7} \otimes w_{8j \rightarrow 8j+1}, & i = j + 3s; \\ -e_{8(j+m)+7} \otimes w_{8j \rightarrow 8j+3}, & i = j + 5s; \\ 0, & \text{otherwise.} \end{cases}$$

If  $s \leq j < 2s$ , then

$$b_{ij} = \begin{cases} w_{8(j+m)+7 \rightarrow 8(j+m+1)} \otimes w_{8j \rightarrow 8j+1}, & i = j + 2s; \\ -e_{8(j+m+1)} \otimes w_{8j \rightarrow 8j+2}, & i = j + 3s; \\ 0, & \text{otherwise.} \end{cases}$$

If  $2s \leq j < 3s$ , then

$$b_{ij} = \begin{cases} -w_{8(j+m)+2 \rightarrow 8(j+m+1)} \otimes e_{8j}, & i = j - 2s; \\ -w_{8(j+m)+6 \rightarrow 8(j+m+1)} \otimes e_{8j}, & i = j; \\ -w_{8(j+m)+7 \rightarrow 8(j+m+1)} \otimes w_{8j \rightarrow 8j+1}, & i = j + s; \\ -e_{8(j+m+1)} \otimes w_{8j \rightarrow 8j+2}, & i = j + 2s; \\ -w_{8(j+m)+7 \rightarrow 8(j+m+1)} \otimes w_{8j \rightarrow 8j+3}, & i = j + 3s; \\ -e_{8(j+m+1)} \otimes w_{8j \rightarrow 8j+4}, & i = j + 4s; \\ -e_{8(j+m+1)} \otimes w_{8j \rightarrow 8j+6}, & i = j + 7s; \\ 0, & \text{otherwise.} \end{cases}$$

If  $3s \leq j < 4s$ , then

$$b_{ij} = \begin{cases} w_{8(j+m+1)+2 \rightarrow 8(j+m+1)+3} \otimes w_{8j+1 \rightarrow 8(j+1)}, & i = (j+1)_s; \\ 0, & \text{otherwise.} \end{cases}$$

If  $4s \leq j < 5s$ , then

$$b_{ij} = \begin{cases} w_{8(j+m)+7 \rightarrow 8(j+m+1)+5} \otimes e_{8j+1}, & i = j - s; \\ 0, & \text{otherwise.} \end{cases}$$

If  $5s \leq j < 6s$ , then

$$b_{ij} = \begin{cases} -w_{8(j+m+1)+2 \rightarrow 8(j+m+1)+4} \otimes w_{8j+2 \rightarrow 8(j+1)}, & i = (j+1)_s; \\ e_{8(j+m+1)+4} \otimes w_{8j+2 \rightarrow 8(j+1)}, & i = s + (j+1)_s; \\ w_{8(j+m+1) \rightarrow 8(j+m+1)+4} \otimes e_{8j+2}, & i = j - s; \\ 0, & \text{otherwise.} \end{cases}$$

If  $6s \leq j < 7s$ , then  $b_{ij} = 0$ .

If  $7s \leq j < 8s$ , then

$$b_{ij} = \begin{cases} e_{8(j+m+1)+5} \otimes w_{8j+3 \rightarrow 8j+7}, & i = j + 6s; \\ 0, & \text{otherwise.} \end{cases}$$

If  $8s \leq j < 10s$ , then  $b_{ij} = 0$ .

If  $10s \leq j < 11s$ , then

$$b_{ij} = \begin{cases} w_{8(j+m+1)+5 \rightarrow 8(j+m+1)+6} \otimes w_{8j+4 \rightarrow 8j+7}, & i = j + 3s; \\ 0, & \text{otherwise.} \end{cases}$$

If  $11s \leq j < 12s$ , then

$$b_{ij} = \begin{cases} e_{8(j+m+1)+6} \otimes w_{8j+5 \rightarrow 8(j+1)}, & i = 2s + (j+1)_s; \\ -w_{8(j+m)+7 \rightarrow 8(j+m+1)+6} \otimes e_{8j+5}, & i = j - 4s; \\ 0, & \text{otherwise.} \end{cases}$$

If  $12s \leq j < 13s$ , then  $b_{ij} = 0$ .

If  $13s \leq j < 14s$ , then

$$b_{ij} = \begin{cases} w_{8(j+m)+7 \rightarrow 8(j+m+1)+1} \otimes e_{8j+5}, & i = j - 6s; \\ w_{8(j+m+1) \rightarrow 8(j+m+1)+1} \otimes e_{8j+5}, & i = j - 5s; \\ w_{8(j+m+1) \rightarrow 8(j+m+1)+1} \otimes w_{8j+5 \rightarrow 8j+6}, & i = j - 4s; \\ -e_{8(j+m+1)+1} \otimes w_{8j+5 \rightarrow 8j+7}, & i = j - s; \\ 0, & \text{otherwise.} \end{cases}$$

If  $14s \leq j < 15s$ , then

$$b_{ij} = \begin{cases} w_{8(j+m+1) \rightarrow 8(j+m+1)+2} \otimes e_{8j+6}, & i = j - 5s; \\ -w_{8(j+m+1)+1 \rightarrow 8(j+m+1)+2} \otimes w_{8j+6 \rightarrow 8j+7}, & i = j - 2s; \\ 0, & \text{otherwise.} \end{cases}$$

If  $15s \leq j < 17s$ , then  $b_{ij} = 0$ .

If  $17s \leq j < 18s$ , then

$$b_{ij} = \begin{cases} -w_{8(j+m+1)+6 \rightarrow 8(j+m+1)+7} \otimes w_{8j+7 \rightarrow 8(j+1)}, & i = 2s + (j+1)_s; \\ -e_{8(j+m+1)+7} \otimes w_{8j+7 \rightarrow 8(j+1)+1}, & i = 3s + (j+1)_s; \\ -w_{8(j+m+1)+3 \rightarrow 8(j+m+1)+7} \otimes e_{8j+7}, & i = j - 7s; \\ w_{8(j+m+1)+6 \rightarrow 8(j+m+1)+7} \otimes e_{8j+7}, & i = j - 6s; \\ w_{8(j+m+1)+1 \rightarrow 8(j+m+1)+7} \otimes e_{8j+7}, & i = j - 5s; \\ 0, & \text{otherwise.} \end{cases}$$

If  $18s \leq j < 19s$ , then

$$b_{ij} = \begin{cases} -w_{8(j+m+1)+7 \rightarrow 8(j+m+2)} \otimes w_{8j+7 \rightarrow 8(j+1)+1}, & i = 3s + (j+1)_s; \\ -w_{8(j+m+1)+3 \rightarrow 8(j+m+2)} \otimes e_{8j+7}, & i = j - 8s; \\ 0, & \text{otherwise.} \end{cases}$$

If  $19s \leq j < 20s$ , then  $b_{ij} = 0$ .

(23) If  $r_0 = 22$ , then  $\Omega^{22}(Z_t^{(23)})$  is described with  $(13s \times 18s)$  matrix, whose entries  $b_{ij}$  have the following form:

If  $0 \leq j < s$ , then

$$b_{ij} = \begin{cases} -w_{8(j+m) \rightarrow 8(j+m)+3} \otimes e_{8j}, & i = j; \\ w_{8(j+m-1)+7 \rightarrow 8(j+m)+3} \otimes e_{8j}, & i = j + s; \\ -w_{8(j+m)+2 \rightarrow 8(j+m)+3} \otimes w_{8j \rightarrow 8j+5}, & i = j + 7s; \\ 0, & \text{otherwise.} \end{cases}$$

If  $s \leq j < 2s$ , then

$$b_{ij} = \begin{cases} w_{8(j+m-1)+7 \rightarrow 8(j+m)+6} \otimes e_{8j}, & i = j; \\ w_{8(j+m)+5 \rightarrow 8(j+m)+6} \otimes w_{8j \rightarrow 8j+2}, & i = j + 3s; \\ e_{8(j+m)+6} \otimes w_{8j \rightarrow 8j+3}, & i = j + 4s; \\ e_{8(j+m)+6} \otimes w_{8j \rightarrow 8j+6}, & i = j + 9s; \\ 0, & \text{otherwise.} \end{cases}$$

If  $2s \leq j < 3s$ , then

$$b_{ij} = \begin{cases} w_{8(j+m)+3 \rightarrow 8(j+m)+4} \otimes w_{8j \rightarrow 8j+1}, & i = j; \\ -e_{8(j+m)+4} \otimes w_{8j \rightarrow 8j+2}, & i = j + s; \\ 0, & \text{otherwise.} \end{cases}$$

If  $3s \leq j < 4s$ , then

$$b_{ij} = \begin{cases} -w_{8(j+m) \rightarrow 8(j+m)+1} \otimes e_{8j}, & i = j - 3s; \\ w_{8(j+m-1)+7 \rightarrow 8(j+m)+1} \otimes e_{8j}, & i = j - 2s; \\ -e_{8(j+m)+1} \otimes w_{8j \rightarrow 8j+4}, & i = j + 3s; \\ 0, & \text{otherwise.} \end{cases}$$

If  $4s \leq j < 5s$ , then

$$b_{ij} = \begin{cases} -e_{8(j+m)+5} \otimes w_{8j \rightarrow 8j+2}, & i = j; \\ 0, & \text{otherwise.} \end{cases}$$

If  $5s \leq j < 6s$ , then

$$b_{ij} = \begin{cases} e_{8(j+m)+7} \otimes w_{8j+1 \rightarrow 8(j+1)}, & i = s + (j+1)_s; \\ -w_{8(j+m)+3 \rightarrow 8(j+m)+7} \otimes e_{8j+1}, & i = j - 3s; \\ w_{8(j+m)+4 \rightarrow 8(j+m)+7} \otimes w_{8j+1 \rightarrow 8j+2}, & i = j - 2s; \\ 0, & \text{otherwise.} \end{cases}$$

If  $6s \leq j < 7s$ , then

$$b_{ij} = \begin{cases} e_{8(j+m)+7} \otimes w_{8j+2 \rightarrow 8(j+1)}, & i = s + (j+1)_s; \\ w_{8(j+m)+5 \rightarrow 8(j+m)+7} \otimes e_{8j+2}, & i = j - 2s; \\ 0, & \text{otherwise.} \end{cases}$$

If  $7s \leq j < 8s$ , then

$$b_{ij} = \begin{cases} -e_{8(j+m+1)} \otimes w_{8j+2 \rightarrow 8(j+1)}, & i = (j+1)_s; \\ w_{8(j+m)+7 \rightarrow 8(j+m)+1} \otimes w_{8j+2 \rightarrow 8(j+1)}, & i = s + (j+1)_s; \\ 0, & \text{otherwise.} \end{cases}$$

If  $8s \leq j < 9s$ , then

$$b_{ij} = \begin{cases} w_{8(j+m)+6 \rightarrow 8(j+m)+1} \otimes e_{8j+3}, & i = j - 3s; \\ -w_{8(j+m)+1 \rightarrow 8(j+m)+1} \otimes w_{8j+3 \rightarrow 8j+4}, & i = j - 2s; \\ -w_{8(j+m)+7 \rightarrow 8(j+m)+1} \otimes w_{8j+3 \rightarrow 8j+7}, & i = j + 3s; \\ 0, & \text{otherwise.} \end{cases}$$

If  $9s \leq j < 10s$ , then

$$b_{ij} = \begin{cases} e_{8(j+m)+7} \otimes w_{8j+4 \rightarrow 8j+7}, & i = j + 2s; \\ 0, & \text{otherwise.} \end{cases}$$

If  $10s \leq j < 11s$ , then

$$b_{ij} = \begin{cases} w_{8(j+m)+2 \rightarrow 8(j+m)+7} \otimes e_{8j+5}, & i = j - 3s; \\ w_{8(j+m)+5 \rightarrow 8(j+m)+7} \otimes e_{8j+5}, & i = j - 2s; \\ -w_{8(j+m)+3 \rightarrow 8(j+m)+7} \otimes w_{8j+5 \rightarrow 8j+6}, & i = j - s; \\ w_{8(j+m)+6 \rightarrow 8(j+m)+7} \otimes w_{8j+5 \rightarrow 8j+6}, & i = j; \\ 0, & \text{otherwise.} \end{cases}$$

If  $11s \leq j < 12s$ , then  $b_{ij} = 0$ .

If  $12s \leq j < 13s$ , then

$$b_{ij} = \begin{cases} w_{8(j+m)+3 \rightarrow 8(j+m)+1} \otimes e_{8j+6}, & i = j - 3s; \\ 0, & \text{otherwise.} \end{cases}$$

If  $13s \leq j < 14s$ , then  $b_{ij} = 0$ .

If  $14s \leq j < 15s$ , then

$$b_{ij} = \begin{cases} w_{8(j+m+1) \rightarrow 8(j+m+1)+2} \otimes w_{8j+7 \rightarrow 8(j+1)}, & i = (j+1)_s; \\ -w_{8(j+m)+7 \rightarrow 8(j+m)+1+2} \otimes w_{8j+7 \rightarrow 8(j+1)}, & i = s + (j+1)_s; \\ e_{8(j+m+1)+2} \otimes w_{8j+7 \rightarrow 8(j+1)+5}, & i = 7s + (j+1)_s; \\ 0, & \text{otherwise.} \end{cases}$$

If  $15s \leq j < 16s$ , then

$$b_{ij} = \begin{cases} -w_{8(j+m)+7 \rightarrow 8(j+m)+1+3} \otimes e_{8j+7}, & i = j - 4s; \\ 0, & \text{otherwise.} \end{cases}$$

If  $16s \leq j < 18s$ , then  $b_{ij} = 0$ .



(24) If  $r_0 = 23$ , then  $\Omega^{23}(Z_t^{(23)})$  is described with  $(11s \times 19s)$  matrix, whose entries  $b_{ij}$  have the following form:

If  $0 \leq j < s$ , then

$$b_{ij} = \begin{cases} w_{8(j+m)+3 \rightarrow 8(j+m)+7} \otimes e_{8j}, & i = j; \\ -w_{8(j+m)+5 \rightarrow 8(j+m)+7} \otimes e_{8j}, & i = j + s; \\ e_{8(j+m)+7} \otimes w_{8j \rightarrow 8j+2}, & i = j + 3s; \\ -e_{8(j+m)+7} \otimes w_{8j \rightarrow 8j+6}, & i = j + 7s; \\ 0, & \text{otherwise.} \end{cases}$$

If  $s \leq j < 2s$ , then

$$b_{ij} = \begin{cases} -w_{8(j+m)+3 \rightarrow 8(j+m+1)} \otimes e_{8j}, & i = j - s; \\ e_{8(j+m+1)} \otimes w_{8j \rightarrow 8j+1}, & i = j + s; \\ -w_{8(j+m)+7 \rightarrow 8(j+m+1)} \otimes w_{8j \rightarrow 8j+2}, & i = j + 2s; \\ 0, & \text{otherwise.} \end{cases}$$

If  $2s \leq j < 3s$ , then  $b_{ij} = 0$ .

If  $3s \leq j < 4s$ , then

$$b_{ij} = \begin{cases} w_{8(j+m+1)+3 \rightarrow 8(j+m+1)+4} \otimes w_{8j+1 \rightarrow 8(j+1)}, & i = (j+1)_s; \\ -w_{8(j+m+1) \rightarrow 8(j+m+1)+4} \otimes e_{8j+1}, & i = j - s; \\ 0, & \text{otherwise.} \end{cases}$$

If  $4s \leq j < 5s$ , then

$$b_{ij} = \begin{cases} -w_{8(j+m+1)+5 \rightarrow 8(j+m+1)+6} \otimes w_{8j+1 \rightarrow 8(j+1)}, & i = s + (j+1)_s; \\ 0, & \text{otherwise.} \end{cases}$$

If  $5s \leq j < 6s$ , then

$$b_{ij} = \begin{cases} -e_{8(j+m+1)+5} \otimes w_{8j+2 \rightarrow 8(j+1)}, & i = s + (j+1)_s; \\ -w_{8(j+m)+7 \rightarrow 8(j+m+1)+5} \otimes e_{8j+2}, & i = j - 2s; \\ 0, & \text{otherwise.} \end{cases}$$

If  $6s \leq j < 8s$ , then  $b_{ij} = 0$ .

If  $8s \leq j < 9s$ , then

$$b_{ij} = \begin{cases} -w_{8(j+m+1)+5 \rightarrow 8(j+m+1)+6} \otimes w_{8j+3 \rightarrow 8(j+1)}, & i = s + (j+1)_s; \\ w_{8(j+m+1) \rightarrow 8(j+m+1)+6} \otimes e_{8j+3}, & i = j - 4s; \\ -e_{8(j+m+1)+6} \otimes w_{8j+3 \rightarrow 8j+7}, & i = j + 2s; \\ 0, & \text{otherwise.} \end{cases}$$

If  $9s \leq j < 10s$ , then  $b_{ij} = 0$ .

If  $10s \leq j < 11s$ , then

$$b_{ij} = \begin{cases} w_{8(j+m+1) \rightarrow 8(j+m+1)+2} \otimes e_{8j+5}, & i = j - 4s; \\ w_{8(j+m)+7 \rightarrow 8(j+m+1)+2} \otimes w_{8j+5 \rightarrow 8j+6}, & i = j - 3s; \\ e_{8(j+m+1)+2} \otimes w_{8j+5 \rightarrow 8j+7}, & i = j - 2s; \\ 0, & \text{otherwise.} \end{cases}$$

If  $11s \leq j < 13s$ , then  $b_{ij} = 0$ .

If  $13s \leq j < 14s$ , then

$$b_{ij} = \begin{cases} w_{8(j+m)+7 \rightarrow 8(j+m+1)+3} \otimes e_{8j+6}, & i = j - 6s; \\ 0, & \text{otherwise.} \end{cases}$$

If  $14s \leq j < 16s$ , then  $b_{ij} = 0$ .

If  $16s \leq j < 17s$ , then

$$b_{ij} = \begin{cases} w_{8(j+m+1)+2 \rightarrow 8(j+m+1)+7} \otimes e_{8j+7}, & i = j - 8s; \\ w_{8(j+m+1)+4 \rightarrow 8(j+m+1)+7} \otimes e_{8j+7}, & i = j - 7s; \\ 0, & \text{otherwise.} \end{cases}$$

If  $17s \leq j < 19s$ , then  $b_{ij} = 0$ .

(25) If  $r_0 = 24$ , then  $\Omega^{24}(Z_t^{(23)})$  is described with  $(11s \times 18s)$  matrix, whose entries  $b_{ij}$  have the following form:

If  $0 \leq j < s$ , then

$$b_{ij} = \begin{cases} -w_{8(j+m) \rightarrow 8(j+m)+2} \otimes e_{8j}, & i = j; \\ w_{8(j+m)+1 \rightarrow 8(j+m)+2} \otimes w_{8j \rightarrow 8j+3}, & i = j + 4s; \\ -e_{8(j+m)+2} \otimes w_{8j \rightarrow 8j+4}, & i = j + 5s; \\ 0, & \text{otherwise.} \end{cases}$$

If  $s \leq j < 2s$ , then

$$b_{ij} = \begin{cases} w_{8(j+m) \rightarrow 8(j+m)+4} \otimes e_{8j}, & i = j - s; \\ -w_{8(j+m)+1 \rightarrow 8(j+m)+4} \otimes w_{8j \rightarrow 8j+3}, & i = j + 3s; \\ w_{8(j+m)+2 \rightarrow 8(j+m)+4} \otimes w_{8j \rightarrow 8j+4}, & i = j + 4s; \\ -w_{8(j+m)+3 \rightarrow 8(j+m)+4} \otimes w_{8j \rightarrow 8j+5}, & i = j + 5s; \\ 0, & \text{otherwise.} \end{cases}$$

If  $2s \leq j < 3s$ , then

$$b_{ij} = \begin{cases} -e_{8(j+m)+6} \otimes w_{8j \rightarrow 8j+2}, & i = j + s; \\ 0, & \text{otherwise.} \end{cases}$$

If  $3s \leq j < 4s$ , then

$$b_{ij} = \begin{cases} e_{8(j+m)+5} \otimes w_{8j \rightarrow 8j+1}, & i = j - s; \\ 0, & \text{otherwise.} \end{cases}$$

If  $4s \leq j < 5s$ , then

$$b_{ij} = \begin{cases} -w_{8(j+m)+5 \rightarrow 8(j+m)+7} \otimes e_{8j+1}, & i = j - 2s; \\ 0, & \text{otherwise.} \end{cases}$$

If  $5s \leq j < 6s$ , then

$$b_{ij} = \begin{cases} -e_{8(j+m+1)} \otimes w_{8j+1 \rightarrow 8(j+1)}, & i = (j+1)_s; \\ 0, & \text{otherwise.} \end{cases}$$

If  $6s \leq j < 7s$ , then

$$b_{ij} = \begin{cases} -e_{8(j+m+1)} \otimes w_{8j+2 \rightarrow 8(j+1)}, & i = (j+1)_s; \\ -w_{8(j+m)+6 \rightarrow 8(j+m+1)} \otimes e_{8j+2}, & i = j - 3s; \\ 0, & \text{otherwise.} \end{cases}$$

If  $7s \leq j < 8s$ , then

$$b_{ij} = \begin{cases} -w_{8(j+m)+1 \rightarrow 8(j+m)+7} \otimes e_{8j+3}, & i = j - 3s; \\ w_{8(j+m)+2 \rightarrow 8(j+m)+7} \otimes w_{8j+3 \rightarrow 8j+4}, & i = j - 2s; \\ -e_{8(j+m)+7} \otimes w_{8j+3 \rightarrow 8j+7}, & i = j + 3s; \\ 0, & \text{otherwise.} \end{cases}$$

If  $8s \leq j < 9s$ , then  $b_{ij} = 0$ .

If  $9s \leq j < 10s$ , then

$$b_{ij} = \begin{cases} w_{8(j+m)+3 \rightarrow 8(j+m+1)} \otimes e_{8j+5}, & i = j - 3s; \\ 0, & \text{otherwise.} \end{cases}$$

If  $10s \leq j < 11s$ , then  $b_{ij} = 0$ .

If  $11s \leq j < 12s$ , then

$$b_{ij} = \begin{cases} w_{8(j+m)+4 \rightarrow 8(j+m)+7} \otimes e_{8j+6}, & i = j - 3s; \\ 0, & \text{otherwise.} \end{cases}$$

If  $12s \leq j < 13s$ , then  $b_{ij} = 0$ .

If  $13s \leq j < 14s$ , then

$$b_{ij} = \begin{cases} w_{8(j+m+1) \rightarrow 8(j+m+1)+3} \otimes w_{8j+7 \rightarrow 8(j+1)}, & i = (j+1)_s; \\ -w_{8(j+m+1)+1 \rightarrow 8(j+m+1)+3} \otimes w_{8j+7 \rightarrow 8(j+1)+3}, & i = 4s + (j+1)_s; \\ w_{8(j+m+1)+2 \rightarrow 8(j+m+1)+3} \otimes w_{8j+7 \rightarrow 8(j+1)+4}, & i = 5s + (j+1)_s; \\ e_{8(j+m+1)+3} \otimes w_{8j+7 \rightarrow 8(j+1)+5}, & i = 6s + (j+1)_s; \\ w_{8(j+m+1) \rightarrow 8(j+m+1)+3} \otimes e_{8j+7}, & i = j - 4s; \\ 0, & \text{otherwise.} \end{cases}$$

If  $14s \leq j < 18s$ , then  $b_{ij} = 0$ .

(26) If  $r_0 = 25$ , then  $\Omega^{25}(Z_t^{(23)})$  is described with  $(10s \times 19s)$  matrix, whose entries  $b_{ij}$  have the following form:

If  $0 \leq j < s$ , then

$$b_{ij} = \begin{cases} w_{8(j+m)+4 \rightarrow 8(j+m)+7} \otimes e_{8j}, & i = j; \\ e_{8(j+m)+7} \otimes w_{8j \rightarrow 8j+1}, & i = j + 2s; \\ 0, & \text{otherwise.} \end{cases}$$

If  $s \leq j < 2s$ , then

$$b_{ij} = \begin{cases} w_{8(j+m)+4 \rightarrow 8(j+m+1)} \otimes e_{8j}, & i = j - s; \\ w_{8(j+m)+7 \rightarrow 8(j+m+1)} \otimes w_{8j \rightarrow 8j+1}, & i = j + s; \\ e_{8(j+m+1)} \otimes w_{8j \rightarrow 8j+2}, & i = j + 2s; \\ e_{8(j+m+1)} \otimes w_{8j \rightarrow 8j+6}, & i = j + 6s; \\ 0, & \text{otherwise.} \end{cases}$$

If  $2s \leq j < 3s$ , then  $b_{ij} = 0$ .

If  $3s \leq j < 4s$ , then

$$b_{ij} = \begin{cases} w_{8(j+m)+7 \rightarrow 8(j+m+1)+5} \otimes e_{8j+1}, & i = j - s; \\ w_{8(j+m+1) \rightarrow 8(j+m+1)+5} \otimes w_{8j+1 \rightarrow 8j+2}, & i = j; \\ -e_{8(j+m+1)+5} \otimes w_{8j+1 \rightarrow 8j+7}, & i = j + 6s; \\ 0, & \text{otherwise.} \end{cases}$$

If  $4s \leq j < 6s$ , then  $b_{ij} = 0$ .

If  $6s \leq j < 7s$ , then

$$b_{ij} = \begin{cases} e_{8(j+m+1)+6} \otimes w_{8j+2 \rightarrow 8(j+1)}, & i = s + (j+1)_s; \\ -w_{8(j+m+1) \rightarrow 8(j+m+1)+6} \otimes e_{8j+2}, & i = j - 3s; \\ w_{8(j+m+1)+5 \rightarrow 8(j+m+1)+6} \otimes w_{8j+2 \rightarrow 8j+7}, & i = j + 3s; \\ 0, & \text{otherwise.} \end{cases}$$

If  $7s \leq j < 8s$ , then

$$b_{ij} = \begin{cases} -w_{8(j+m+1)+1 \rightarrow 8(j+m+1)+3} \otimes e_{8j+3}, & i = j - 3s; \\ 0, & \text{otherwise.} \end{cases}$$

If  $8s \leq j < 10s$ , then  $b_{ij} = 0$ .

If  $10s \leq j < 11s$ , then

$$b_{ij} = \begin{cases} w_{8(j+m)+7 \rightarrow 8(j+m+1)+3} \otimes e_{8j+5}, & i = j - 4s; \\ -w_{8(j+m+1) \rightarrow 8(j+m+1)+3} \otimes w_{8j+5 \rightarrow 8j+6}, & i = j - 3s; \\ e_{8(j+m+1)+3} \otimes w_{8j+5 \rightarrow 8j+7}, & i = j - 2s; \\ 0, & \text{otherwise.} \end{cases}$$

If  $11s \leq j < 14s$ , then  $b_{ij} = 0$ .

If  $14s \leq j < 15s$ , then

$$b_{ij} = \begin{cases} w_{8(j+m+1) \rightarrow 8(j+m+1)+4} \otimes e_{8j+6}, & i = j - 7s; \\ 0, & \text{otherwise.} \end{cases}$$

If  $15s \leq j < 16s$ , then  $b_{ij} = 0$ .

If  $16s \leq j < 17s$ , then

$$b_{ij} = \begin{cases} w_{8(j+m+1)+5 \rightarrow 8(j+m+1)+7} \otimes e_{8j+7}, & i = j - 7s; \\ 0, & \text{otherwise.} \end{cases}$$

If  $17s \leq j < 18s$ , then

$$b_{ij} = \begin{cases} w_{8(j+m+1)+4 \rightarrow 8(j+m+2)} \otimes w_{8j+7 \rightarrow 8(j+1)}, & i = (j+1)_s; \\ w_{8(j+m+1)+7 \rightarrow 8(j+m+2)} \otimes w_{8j+7 \rightarrow 8(j+1)+1}, & i = 2s + (j+1)_s; \\ e_{8(j+m+2)} \otimes w_{8j+7 \rightarrow 8(j+1)+2}, & i = 3s + (j+1)_s; \\ e_{8(j+m+2)} \otimes w_{8j+7 \rightarrow 8(j+1)+6}, & i = 7s + (j+1)_s; \\ w_{8(j+m+1)+3 \rightarrow 8(j+m+2)} \otimes e_{8j+7}, & i = j - 9s; \\ 0, & \text{otherwise.} \end{cases}$$

If  $18s \leq j < 19s$ , then  $b_{ij} = 0$ .

(27) If  $r_0 = 26$ , then  $\Omega^{26}(Z_t^{(23)})$  is described with  $(8s \times 16s)$  matrix, whose entries  $b_{ij}$  have the following form:

If  $0 \leq j < s$ , then

$$b_{ij} = \begin{cases} -w_{8(j+m-1)+7 \rightarrow 8(j+m)+3} \otimes e_{8j}, & i = j; \\ w_{8(j+m)+1 \rightarrow 8(j+m)+3} \otimes w_{8j \rightarrow 8j+2}, & i = j + 2s; \\ w_{8(j+m)+2 \rightarrow 8(j+m)+3} \otimes w_{8j \rightarrow 8j+3}, & i = j + 3s; \\ -e_{8(j+m)+3} \otimes w_{8j \rightarrow 8j+4}, & i = j + 4s; \\ 0, & \text{otherwise.} \end{cases}$$

If  $s \leq j < 2s$ , then

$$b_{ij} = \begin{cases} -e_{8(j+m)+6} \otimes w_{8j \rightarrow 8j+1}, & i = j; \\ 0, & \text{otherwise.} \end{cases}$$

If  $2s \leq j < 3s$ , then  $b_{ij} = 0$ .

If  $3s \leq j < 4s$ , then

$$b_{ij} = \begin{cases} e_{8(j+m)+5} \otimes w_{8j \rightarrow 8j+6}, & i = j + 3s; \\ 0, & \text{otherwise.} \end{cases}$$

If  $4s \leq j < 5s$ , then

$$b_{ij} = \begin{cases} w_{8(j+m)+7 \rightarrow 8(j+m+1)} \otimes w_{8j+1 \rightarrow 8(j+1)}, & i = (j+1)_s; \\ w_{8(j+m)+6 \rightarrow 8(j+m+1)} \otimes e_{8j+1}, & i = j - 3s; \\ 0, & \text{otherwise.} \end{cases}$$

If  $5s \leq j < 6s$ , then

$$b_{ij} = \begin{cases} e_{8(j+m)+7} \otimes w_{8j+2 \rightarrow 8(j+1)}, & i = (j+1)_s; \\ w_{8(j+m)+1 \rightarrow 8(j+m)+7} \otimes e_{8j+2}, & i = j - 3s; \\ 0, & \text{otherwise.} \end{cases}$$

If  $6s \leq j < 7s$ , then

$$b_{ij} = \begin{cases} -w_{8(j+m)+2 \rightarrow 8(j+m+1)} \otimes e_{8j+3}, & i = j - 3s; \\ w_{8(j+m)+3 \rightarrow 8(j+m+1)} \otimes w_{8j+3 \rightarrow 8j+4}, & i = j - 2s; \\ 0, & \text{otherwise.} \end{cases}$$

If  $7s \leq j < 8s$ , then  $b_{ij} = 0$ .

If  $8s \leq j < 9s$ , then

$$b_{ij} = \begin{cases} w_{8(j+m)+4 \rightarrow 8(j+m)+7} \otimes e_{8j+5}, & i = j - 3s; \\ w_{8(j+m)+5 \rightarrow 8(j+m)+7} \otimes w_{8j+5 \rightarrow 8j+6}, & i = j - 2s; \\ 0, & \text{otherwise.} \end{cases}$$

If  $9s \leq j < 10s$ , then  $b_{ij} = 0$ .

If  $10s \leq j < 11s$ , then

$$b_{ij} = \begin{cases} -w_{8(j+m)+5 \rightarrow 8(j+m)+7} \otimes e_{8j+6}, & i = j - 4s; \\ 0, & \text{otherwise.} \end{cases}$$

If  $11s \leq j < 12s$ , then

$$b_{ij} = \begin{cases} w_{8(j+m)+5 \rightarrow 8(j+m+1)} \otimes e_{8j+6}, & i = j - 5s; \\ e_{8(j+m+1)} \otimes w_{8j+6 \rightarrow 8j+7}, & i = j - 4s; \\ 0, & \text{otherwise.} \end{cases}$$

If  $12s \leq j < 13s$ , then

$$b_{ij} = \begin{cases} -w_{8(j+m+1) \rightarrow 8(j+m+1)+2} \otimes e_{8j+7}, & i = j - 5s; \\ 0, & \text{otherwise.} \end{cases}$$

If  $13s \leq j < 14s$ , then

$$b_{ij} = \begin{cases} w_{8(j+m)+7 \rightarrow 8(j+m+1)+4} \otimes w_{8j+7 \rightarrow 8(j+1)}, & i = (j+1)_s; \\ -w_{8(j+m+1)+2 \rightarrow 8(j+m+1)+4} \otimes w_{8j+7 \rightarrow 8(j+1)+3}, & i = 3s + (j+1)_s; \\ w_{8(j+m+1)+3 \rightarrow 8(j+m+1)+4} \otimes w_{8j+7 \rightarrow 8(j+1)+4}, & i = 4s + (j+1)_s; \\ e_{8(j+m+1)+4} \otimes w_{8j+7 \rightarrow 8(j+1)+5}, & i = 5s + (j+1)_s; \\ 0, & \text{otherwise.} \end{cases}$$

If  $14s \leq j < 15s$ , then  $b_{ij} = 0$ .

If  $15s \leq j < 16s$ , then

$$b_{ij} = \begin{cases} e_{8(j+m+1)+5} \otimes w_{8j+7 \rightarrow 8(j+1)+6}, & i = 6s + (j+1)_s; \\ 0, & \text{otherwise.} \end{cases}$$

(28) If  $r_0 = 27$ , then  $\Omega^{27}(Z_t^{(23)})$  is described with  $(9s \times 16s)$  matrix, whose entries  $b_{ij}$  have the following form:

If  $0 \leq j < s$ , then

$$b_{ij} = \begin{cases} -e_{8(j+m)+7} \otimes e_{8j}, & i = j; \\ 0, & \text{otherwise.} \end{cases}$$

If  $s \leq j < 2s$ , then

$$b_{ij} = \begin{cases} -w_{8(j+m)+7 \rightarrow 8(j+m+1)} \otimes e_{8j}, & i = j - s; \\ e_{8(j+m+1)} \otimes w_{8j \rightarrow 8j+1}, & i = j; \\ 0, & \text{otherwise.} \end{cases}$$

If  $2s \leq j < 3s$ , then

$$b_{ij} = \begin{cases} -w_{8(j+m+1) \rightarrow 8(j+m+1)+2} \otimes e_{8j+1}, & i = j - s; \\ 0, & \text{otherwise.} \end{cases}$$

If  $3s \leq j < 4s$ , then

$$b_{ij} = \begin{cases} w_{8(j+m+1) \rightarrow 8(j+m+1)+6} \otimes e_{8j+1}, & i = j - 2s; \\ e_{8(j+m+1)+6} \otimes w_{8j+1 \rightarrow 8j+7}, & i = j + 5s; \\ 0, & \text{otherwise.} \end{cases}$$

If  $4s \leq j < 5s$ , then

$$b_{ij} = \begin{cases} w_{8(j+m+1)+1 \rightarrow 8(j+m+1)+3} \otimes e_{8j+2}, & i = j - 2s; \\ 0, & \text{otherwise.} \end{cases}$$

If  $5s \leq j < 6s$ , then

$$b_{ij} = \begin{cases} -w_{8(j+m+1)+2 \rightarrow 8(j+m+1)+4} \otimes e_{8j+3}, & i = j - 2s; \\ 0, & \text{otherwise.} \end{cases}$$

If  $6s \leq j < 9s$ , then  $b_{ij} = 0$ .

If  $9s \leq j < 10s$ , then

$$b_{ij} = \begin{cases} w_{8(j+m+1) \rightarrow 8(j+m+1)+4} \otimes e_{8j+5}, & i = j - 4s; \\ e_{8(j+m+1)+4} \otimes w_{8j+5 \rightarrow 8j+7}, & i = j - 2s; \\ 0, & \text{otherwise.} \end{cases}$$

If  $10s \leq j < 12s$ , then  $b_{ij} = 0$ .

If  $12s \leq j < 13s$ , then

$$b_{ij} = \begin{cases} e_{8(j+m+1)+5} \otimes e_{8j+6}, & i = j - 6s; \\ 0, & \text{otherwise.} \end{cases}$$

If  $13s \leq j < 14s$ , then

$$b_{ij} = \begin{cases} e_{8(j+m+1)+7} \otimes w_{8j+7 \rightarrow 8(j+1)}, & i = (j+1)_s; \\ -w_{8(j+m+1)+4 \rightarrow 8(j+m+1)+7} \otimes e_{8j+7}, & i = j - 6s; \\ 0, & \text{otherwise.} \end{cases}$$

If  $14s \leq j < 15s$ , then

$$b_{ij} = \begin{cases} w_{8(j+m+1)+7 \rightarrow 8(j+m+2)} \otimes w_{8j+7 \rightarrow 8(j+1)}, & i = (j+1)_s; \\ 0, & \text{otherwise.} \end{cases}$$

If  $15s \leq j < 16s$ , then  $b_{ij} = 0$ .

(29) If  $r_0 = 28$ , then  $\Omega^{28}(Z_t^{(23)})$  is described with  $(8s \times 14s)$  matrix, whose entries  $b_{ij}$  have the following form:

If  $s \leq j < 2s$ , then

$$b_{ij} = \begin{cases} -w_{8(j+m) \rightarrow 8(j+m)+4} \otimes e_{8j}, & i = j - s; \\ w_{8(j+m)+1 \rightarrow 8(j+m)+4} \otimes w_{8j \rightarrow 8j+1}, & i = j; \\ w_{8(j+m)+2 \rightarrow 8(j+m)+4} \otimes w_{8j \rightarrow 8j+2}, & i = j + s; \\ w_{8(j+m)+3 \rightarrow 8(j+m)+4} \otimes w_{8j \rightarrow 8j+3}, & i = j + 2s; \\ -e_{8(j+m)+4} \otimes w_{8j \rightarrow 8j+4}, & i = j + 3s; \\ 0, & \text{otherwise.} \end{cases}$$

If  $2s \leq j < 3s$ , then

$$b_{ij} = \begin{cases} -w_{8(j+m) \rightarrow 8(j+m)+6} \otimes e_{8j}, & i = j - 2s; \\ -w_{8(j+m)+5 \rightarrow 8(j+m)+6} \otimes w_{8j \rightarrow 8j+5}, & i = j + 3s; \\ -e_{8(j+m)+6} \otimes w_{8j \rightarrow 8j+6}, & i = j + 4s; \\ 0, & \text{otherwise.} \end{cases}$$

If  $3s \leq j < 4s$ , then

$$b_{ij} = \begin{cases} w_{8(j+m)+1 \rightarrow 8(j+m)+7} \otimes e_{8j+1}, & i = j - 2s; \\ w_{8(j+m)+2 \rightarrow 8(j+m)+7} \otimes w_{8j+1 \rightarrow 8j+2}, & i = j - s; \\ -w_{8(j+m)+3 \rightarrow 8(j+m)+7} \otimes w_{8j+1 \rightarrow 8j+3}, & i = j; \\ w_{8(j+m)+4 \rightarrow 8(j+m)+7} \otimes w_{8j+1 \rightarrow 8j+4}, & i = j + s; \\ e_{8(j+m)+7} \otimes w_{8j+1 \rightarrow 8j+7}, & i = j + 4s; \\ 0, & \text{otherwise.} \end{cases}$$

If  $4s \leq j < 5s$ , then

$$b_{ij} = \begin{cases} e_{8(j+m)+1} \otimes w_{8j+2 \rightarrow 8(j+1)}, & i = (j+1)_s; \\ w_{8(j+m)+2 \rightarrow 8(j+m)+1} \otimes e_{8j+2}, & i = j - 2s; \\ 0, & \text{otherwise.} \end{cases}$$

If  $5s \leq j < 6s$ , then

$$b_{ij} = \begin{cases} -w_{8(j+m)+3 \rightarrow 8(j+m)+7} \otimes e_{8j+3}, & i = j - 2s; \\ w_{8(j+m)+4 \rightarrow 8(j+m)+7} \otimes w_{8j+3 \rightarrow 8j+4}, & i = j - s; \\ 0, & \text{otherwise.} \end{cases}$$

If  $6s \leq j < 7s$ , then  $b_{ij} = 0$ .

If  $7s \leq j < 8s$ , then

$$b_{ij} = \begin{cases} -w_{8(j+m)+5 \rightarrow 8(j+m)+7} \otimes e_{8j+5}, & i = j - 2s; \\ -w_{8(j+m)+6 \rightarrow 8(j+m)+7} \otimes w_{8j+5 \rightarrow 8j+6}, & i = j - s; \\ e_{8(j+m)+7} \otimes w_{8j+5 \rightarrow 8j+7}, & i = j; \\ 0, & \text{otherwise.} \end{cases}$$



If  $8s \leq j < 9s$ , then

$$b_{ij} = \begin{cases} w_{8(j+m)+5 \rightarrow 8(j+m+1)} \otimes e_{8j+5}, & i = j - 3s; \\ -w_{8(j+m)+6 \rightarrow 8(j+m+1)} \otimes w_{8j+5 \rightarrow 8j+6}, & i = j - 2s; \\ w_{8(j+m)+7 \rightarrow 8(j+m+1)} \otimes w_{8j+5 \rightarrow 8j+7}, & i = j - s; \\ 0, & \text{otherwise.} \end{cases}$$

If  $9s \leq j < 10s$ , then

$$b_{ij} = \begin{cases} -w_{8(j+m)+6 \rightarrow 8(j+m+1)} \otimes e_{8j+6}, & i = j - 3s; \\ w_{8(j+m)+7 \rightarrow 8(j+m+1)} \otimes w_{8j+6 \rightarrow 8j+7}, & i = j - 2s; \\ 0, & \text{otherwise.} \end{cases}$$

If  $10s \leq j < 11s$ , then

$$b_{ij} = \begin{cases} w_{8(j+m+1)+1 \rightarrow 8(j+m+1)+3} \otimes w_{8j+7 \rightarrow 8(j+1)+1}, & i = s + (j+1)_s; \\ -w_{8(j+m)+7 \rightarrow 8(j+m+1)+3} \otimes e_{8j+7}, & i = j - 3s; \\ 0, & \text{otherwise.} \end{cases}$$

If  $11s \leq j < 13s$ , then  $b_{ij} = 0$ .

If  $13s \leq j < 14s$ , then

$$b_{ij} = \begin{cases} w_{8(j+m+1) \rightarrow 8(j+m+1)+5} \otimes w_{8j+7 \rightarrow 8(j+1)}, & i = (j+1)_s; \\ e_{8(j+m+1)+5} \otimes w_{8j+7 \rightarrow 8(j+1)+5}, & i = 5s + (j+1)_s; \\ 0, & \text{otherwise.} \end{cases}$$

(II) Represent an arbitrary  $t_0 \in \mathbb{N}$  in the form  $t_0 = 29\ell_0 + r_0$ , where  $0 \leq r_0 \leq 28$ . Then  $\Omega^{t_0}(Z_t^{(23)})$  is a  $\Omega^{r_0}(Z_t^{(23)})$ , whose left components twisted by  $\sigma^{\ell_0}$ , and coefficients multiplied by  $(-1)^{\ell_0}$ .

**Proposition 19** (Translates for the case 24). (I) Let  $r_0 \in \mathbb{N}$ ,  $r_0 < 29$ .  $r_0$ -translates of the elements  $Z_t^{(24)}$  are described by the following way.

(1) If  $r_0 = 0$ , then  $\Omega^0(Z_t^{(24)})$  is described with  $(8s \times 11s)$  matrix with two nonzero entries:

$$b_{j-s,s} = w_{8(j+m) \rightarrow 8(j+m)+5} \otimes e_{8j};$$

$$b_{j-s,2s} = -w_{8(j+m)+1 \rightarrow 8(j+m+1)} \otimes e_{8j+1}.$$

(2) If  $r_0 = 1$ , then  $\Omega^1(Z_t^{(24)})$  is described with  $(9s \times 11s)$  matrix with the following nonzero entries:

$$b_{j,0} = w_{8(j+m)+1 \rightarrow 8(j+m+1)} \otimes e_{8j};$$

$$b_{s+(j+1)_s, 2s+(-1)_s} = e_{8(j+m+1)+5} \otimes w_{8j+1 \rightarrow 8(j+1)};$$

$$b_{s+(j+1)_s, 3s+(-1)_s} = w_{8(j+m+1)+5 \rightarrow 8(j+m+1)+6} \otimes w_{8j+2 \rightarrow 8(j+1)};$$

$$b_{(j+1)_s, 9s+(-1)_s} = w_{8(j+m+1)+1 \rightarrow 8(j+m+2)} \otimes w_{8j+7 \rightarrow 8(j+1)};$$

$$b_{j-s, 9s+(-1)_s} = w_{8(j+m+1) \rightarrow 8(j+m+2)} \otimes e_{8j+7}.$$

(3) If  $r_0 = 2$ , then  $\Omega^2(Z_t^{(24)})$  is described with  $(8s \times 10s)$  matrix with the following nonzero entries:

$$b_{(j+1)_s, 3s+(-1)_s} = -w_{8(j+m)+7 \rightarrow 8(j+m+1)} \otimes w_{8j+2 \rightarrow 8(j+1)};$$

$$b_{j-s, 3s+(-1)_s} = w_{8(j+m)+3 \rightarrow 8(j+m+1)} \otimes e_{8j+2};$$

$$b_{j-s,7s+(-1)_s} = -w_{8(j+m)+1 \rightarrow 8(j+m+1)} \otimes e_{8j+6}.$$

(4) If  $r_0 = 3$ , then  $\Omega^3(Z_t^{(24)})$  is described with  $(10s \times 8s)$  matrix with the following nonzero entries:

$$\begin{aligned} b_{s+(j+1)_s,s+(-1)_s} &= e_{8(j+m+1)+6} \otimes w_{8j+1 \rightarrow 8(j+1)}; \\ b_{j+s,2s+(-1)_s} &= -w_{8(j+m)+4 \rightarrow 8(j+m+1)+1} \otimes e_{8j+2}; \\ b_{j+2s,2s+(-1)_s} &= -w_{8(j+m)+7 \rightarrow 8(j+m+1)+1} \otimes w_{8j+2 \rightarrow 8j+3}; \\ b_{(j+1)_s,7s+(-2)_s} &= -w_{8(j+m+1)+2 \rightarrow 8(j+m+2)} \otimes w_{8j+7 \rightarrow 8(j+1)}; \\ b_{2s+(j+1)_s,7s+(-2)_s} &= -w_{8(j+m+1)+3 \rightarrow 8(j+m+2)} \otimes w_{8j+7 \rightarrow 8(j+1)+1}. \end{aligned}$$

(5) If  $r_0 = 4$ , then  $\Omega^4(Z_t^{(24)})$  is described with  $(11s \times 9s)$  matrix with the following nonzero entries:

$$\begin{aligned} b_{(j+1)_s,(-1)_s} &= -e_{8(j+m)+7} \otimes w_{8j \rightarrow 8(j+1)}; \\ b_{j+2s,(-1)_s} &= w_{8(j+m)+3 \rightarrow 8(j+m)+7} \otimes w_{8j \rightarrow 8j+1}; \\ b_{(j+1)_s,s+(-2)_s} &= w_{8(j+m)+7 \rightarrow 8(j+m+1)} \otimes w_{8j+1 \rightarrow 8(j+1)}; \\ b_{s+(j+1)_s,s+(-2)_s} &= e_{8(j+m+1)} \otimes w_{8j+1 \rightarrow 8(j+1)}; \\ b_{s+(j+1)_s,s+(-1)_s} &= e_{8(j+m+1)} \otimes w_{8j+1 \rightarrow 8(j+1)}; \\ b_{(j+1)_s,2s+(-2)_s} &= w_{8(j+m)+7 \rightarrow 8(j+m+1)+1} \otimes w_{8j+2 \rightarrow 8(j+1)}; \\ b_{(j+1)_s,3s+(-2)_s} &= w_{8(j+m)+7 \rightarrow 8(j+m+1)+2} \otimes w_{8j+3 \rightarrow 8(j+1)}; \\ b_{(j+1)_s,4s+(-2)_s} &= w_{8(j+m)+7 \rightarrow 8(j+m+1)+3} \otimes w_{8j+4 \rightarrow 8(j+1)}; \\ b_{(j+1)_s,5s+(-2)_s} &= w_{8(j+m)+7 \rightarrow 8(j+m+1)} \otimes w_{8j+5 \rightarrow 8(j+1)}; \\ b_{s+(j+1)_s,5s+(-2)_s} &= e_{8(j+m+1)} \otimes w_{8j+5 \rightarrow 8(j+1)}; \\ b_{2s+(j+1)_s,7s+(-2)_s} &= -w_{8(j+m+1)+3 \rightarrow 8(j+m+1)+4} \otimes w_{8j+7 \rightarrow 8(j+1)+1}. \end{aligned}$$

(6) If  $r_0 = 5$ , then  $\Omega^5(Z_t^{(24)})$  is described with  $(11s \times 8s)$  matrix with the following nonzero entries:

$$\begin{aligned} b_{j+3s,(-1)_s} &= -w_{8(j+m)+4 \rightarrow 8(j+m+1)} \otimes w_{8j \rightarrow 8j+1}; \\ b_{j+4s,(-1)_s} &= -w_{8(j+m)+7 \rightarrow 8(j+m+1)} \otimes w_{8j \rightarrow 8j+2}; \\ b_{j+5s,(-1)_s} &= -e_{8(j+m+1)} \otimes w_{8j \rightarrow 8j+3}; \\ b_{2s+(j+1)_s,s+(-2)_s} &= -e_{8(j+m+1)+1} \otimes w_{8j+1 \rightarrow 8(j+1)}; \\ b_{2s+(j+1)_s,s+(-1)_s} &= -e_{8(j+m+1)+1} \otimes w_{8j+1 \rightarrow 8(j+1)}; \\ b_{s+(j+1)_s,4s+(-2)_s} &= -w_{8(j+m+1)+3 \rightarrow 8(j+m+1)+4} \otimes w_{8j+4 \rightarrow 8(j+1)}; \\ b_{(j+1)_s,5s+(-2)_s} &= e_{8(j+m+1)+5} \otimes w_{8j+5 \rightarrow 8(j+1)}. \end{aligned}$$

(7) If  $r_0 = 6$ , then  $\Omega^6(Z_t^{(24)})$  is described with  $(13s \times 8s)$  matrix with the following nonzero entries:

$$\begin{aligned} b_{(j+1)_s,(-2)_s} &= -w_{8(j+m)+7 \rightarrow 8(j+m+1)} \otimes w_{8j \rightarrow 8(j+1)}; \\ b_{(j+1)_s,(-1)_s} &= -w_{8(j+m)+7 \rightarrow 8(j+m+1)} \otimes w_{8j \rightarrow 8(j+1)}; \\ b_{s+(j+1)_s,(-1)_s} &= -e_{8(j+m+1)} \otimes w_{8j \rightarrow 8(j+1)}; \\ b_{j+3s,(-1)_s} &= w_{8(j+m)+5 \rightarrow 8(j+m+1)} \otimes w_{8j \rightarrow 8j+2}; \\ b_{(j+1)_s,s+(-2)_s} &= -w_{8(j+m)+7 \rightarrow 8(j+m+1)+1} \otimes w_{8j+1 \rightarrow 8(j+1)}; \\ b_{(j+1)_s,s+(-1)_s} &= -w_{8(j+m)+7 \rightarrow 8(j+m+1)+1} \otimes w_{8j+1 \rightarrow 8(j+1)}; \\ b_{s+(j+1)_s,s+(-1)_s} &= -w_{8(j+m+1) \rightarrow 8(j+m+1)+1} \otimes w_{8j+1 \rightarrow 8(j+1)}; \\ b_{(j+1)_s,2s+(-2)_s} &= -w_{8(j+m)+7 \rightarrow 8(j+m+1)+2} \otimes w_{8j+2 \rightarrow 8(j+1)}; \end{aligned}$$

$$\begin{aligned}
b_{s+(j+1)_s, 3s+(-2)_s} &= w_{8(j+m+1) \rightarrow 8(j+m+1)+3} \otimes w_{8j+3 \rightarrow 8(j+1)}; \\
b_{s+(j+1)_s, 4s+(-2)_s} &= w_{8(j+m+1) \rightarrow 8(j+m+1)+4} \otimes w_{8j+4 \rightarrow 8(j+1)}; \\
b_{(j+1)_s, 5s+(-2)_s} &= -w_{8(j+m)+7 \rightarrow 8(j+m+1)+5} \otimes w_{8j+5 \rightarrow 8(j+1)}; \\
b_{3s+(j+1)_s, 7s+(-2)_s} &= w_{8(j+m+1)+5 \rightarrow 8(j+m+1)+7} \otimes w_{8j+7 \rightarrow 8(j+1)+2}.
\end{aligned}$$

(8) If  $r_0 = 7$ , then  $\Omega^7(Z_t^{(24)})$  is described with  $(14s \times 9s)$  matrix with the following nonzero entries:

$$\begin{aligned}
b_{3s+(j+1)_s, s+(-1)_s} &= -e_{8(j+m+1)+5} \otimes w_{8j \rightarrow 8(j+1)}; \\
b_{j+3s, s+(-1)_s} &= -w_{8(j+m)+7 \rightarrow 8(j+m+1)+5} \otimes w_{8j \rightarrow 8j+1}; \\
b_{(j+1)_s, 2s+(-1)_s} &= -e_{8(j+m+1)+2} \otimes w_{8j+1 \rightarrow 8(j+1)}; \\
b_{(j+1)_s, 3s+(-2)_s} &= -w_{8(j+m+1)+2 \rightarrow 8(j+m+1)+3} \otimes w_{8j+2 \rightarrow 8(j+1)}; \\
b_{3s+(j+1)_s, 5s+(-2)_s} &= w_{8(j+m+1)+5 \rightarrow 8(j+m+1)+7} \otimes w_{8j+4 \rightarrow 8(j+1)}; \\
b_{2s+(j+1)_s, 6s+(-2)_s} &= -e_{8(j+m+1)+6} \otimes w_{8j+5 \rightarrow 8(j+1)}.
\end{aligned}$$

(9) If  $r_0 = 8$ , then  $\Omega^8(Z_t^{(24)})$  is described with  $(16s \times 8s)$  matrix with the following nonzero entries:

$$\begin{aligned}
b_{(j+1)_s, (-2)_s} &= -e_{8(j+m)+7} \otimes w_{8j \rightarrow 8(j+1)}; \\
b_{(j+1)_s, (-1)_s} &= -e_{8(j+m)+7} \otimes w_{8j \rightarrow 8(j+1)}; \\
b_{j+3s, (-1)_s} &= w_{8(j+m)+5 \rightarrow 8(j+m)+7} \otimes w_{8j \rightarrow 8j+1}; \\
b_{j+4s, (-1)_s} &= -w_{8(j+m)+6 \rightarrow 8(j+m)+7} \otimes w_{8j \rightarrow 8j+2}; \\
b_{(j+1)_s, s+(-2)_s} &= -w_{8(j+m)+7 \rightarrow 8(j+m+1)+2} \otimes w_{8j+1 \rightarrow 8(j+1)}; \\
b_{(j+1)_s, s+(-1)_s} &= -w_{8(j+m)+7 \rightarrow 8(j+m+1)+2} \otimes w_{8j+1 \rightarrow 8(j+1)}; \\
b_{s+(j+1)_s, 4s+(-2)_s} &= -w_{8(j+m)+7 \rightarrow 8(j+m+1)+5} \otimes w_{8j+4 \rightarrow 8(j+1)}; \\
b_{(j+1)_s, 5s+(-2)_s} &= w_{8(j+m)+7 \rightarrow 8(j+m+1)+6} \otimes w_{8j+5 \rightarrow 8(j+1)}; \\
b_{s+(j+1)_s, 5s+(-2)_s} &= -w_{8(j+m)+7 \rightarrow 8(j+m+1)+6} \otimes w_{8j+5 \rightarrow 8(j+1)}.
\end{aligned}$$

(10) If  $r_0 = 9$ , then  $\Omega^9(Z_t^{(24)})$  is described with  $(16s \times 10s)$  matrix with the following nonzero entries:

$$\begin{aligned}
b_{(j+1)_s, s+(-1)_s} &= -w_{8(j+m+1)+5 \rightarrow 8(j+m+1)+6} \otimes w_{8j \rightarrow 8(j+1)}; \\
b_{2s+(j+1)_s, s+(-1)_s} &= -e_{8(j+m+1)+6} \otimes w_{8j \rightarrow 8(j+1)}; \\
b_{j+3s, s+(-1)_s} &= w_{8(j+m+1) \rightarrow 8(j+m+1)+6} \otimes w_{8j \rightarrow 8j+1}; \\
b_{s+(j+1)_s, 2s+(-2)_s} &= -e_{8(j+m+1)+3} \otimes w_{8j+1 \rightarrow 8(j+1)}; \\
b_{s+(j+1)_s, 2s+(-1)_s} &= -e_{8(j+m+1)+3} \otimes w_{8j+1 \rightarrow 8(j+1)}; \\
b_{2s+(j+1)_s, 4s+(-2)_s} &= w_{8(j+m+1)+6 \rightarrow 8(j+m+1)+7} \otimes w_{8j+3 \rightarrow 8(j+1)}; \\
b_{2s+(j+1)_s, 5s+(-2)_s} &= -w_{8(j+m+1)+6 \rightarrow 8(j+m+2)} \otimes w_{8j+4 \rightarrow 8(j+1)}; \\
b_{(j+1)_s, 6s+(-2)_s} &= w_{8(j+m+1)+5 \rightarrow 8(j+m+1)+7} \otimes w_{8j+5 \rightarrow 8(j+1)}; \\
b_{3s+(j+1)_s, 6s+(-2)_s} &= -w_{8(j+m+1)+1 \rightarrow 8(j+m+1)+7} \otimes w_{8j+5 \rightarrow 8(j+1)}.
\end{aligned}$$

(11) If  $r_0 = 10$ , then  $\Omega^{10}(Z_t^{(24)})$  is described with  $(19s \times 11s)$  matrix with the following nonzero entries:

$$\begin{aligned}
b_{(j+1)_s, (-2)_s} &= e_{8(j+m)+7} \otimes w_{8j \rightarrow 8(j+1)}; \\
b_{(j+1)_s, (-1)_s} &= e_{8(j+m)+7} \otimes w_{8j \rightarrow 8(j+1)}; \\
b_{j+4s, (-1)_s} &= -w_{8(j+m)+1 \rightarrow 8(j+m)+7} \otimes w_{8j \rightarrow 8j+1}; \\
b_{(j+1)_s, s+(-2)_s} &= -w_{8(j+m)+7 \rightarrow 8(j+m+1)} \otimes w_{8j \rightarrow 8(j+1)};
\end{aligned}$$

$$\begin{aligned}
b_{s+(j+1)_s, s+(-2)_s} &= -e_{8(j+m+1)} \otimes w_{8j \rightarrow 8(j+1)}; \\
b_{j+2s, s+(-1)_s} &= w_{8(j+m)+6 \rightarrow 8(j+m+1)} \otimes w_{8j \rightarrow 8j+1}; \\
b_{(j+1)_s, 2s+(-2)_s} &= w_{8(j+m)+7 \rightarrow 8(j+m+1)+3} \otimes w_{8j+1 \rightarrow 8(j+1)}; \\
b_{(j+1)_s, 2s+(-1)_s} &= w_{8(j+m)+7 \rightarrow 8(j+m+1)+3} \otimes w_{8j+1 \rightarrow 8(j+1)}; \\
b_{2s+(j+1)_s, 5s+(-2)_s} &= -w_{8(j+m+1) \rightarrow 8(j+m+1)+6} \otimes w_{8j+4 \rightarrow 8(j+1)}; \\
b_{(j+1)_s, 7s+(-2)_s} &= w_{8(j+m)+7 \rightarrow 8(j+m+1)+1} \otimes w_{8j+5 \rightarrow 8(j+1)}; \\
b_{s+(j+1)_s, 7s+(-2)_s} &= w_{8(j+m+1) \rightarrow 8(j+m+1)+1} \otimes w_{8j+5 \rightarrow 8(j+1)}; \\
b_{2s+(j+1)_s, 7s+(-2)_s} &= -w_{8(j+m+1) \rightarrow 8(j+m+1)+1} \otimes w_{8j+5 \rightarrow 8(j+1)}.
\end{aligned}$$

(12) If  $r_0 = 11$ , then  $\Omega^{11}(Z_t^{(24)})$  is described with  $(18s \times 11s)$  matrix with the following nonzero entries:

$$\begin{aligned}
b_{4s+(j+1)_s, (-2)_s} &= -e_{8(j+m+1)+5} \otimes w_{8j \rightarrow 8(j+1)}; \\
b_{j+5s, (-1)_s} &= w_{8(j+m)+7 \rightarrow 8(j+m+1)+5} \otimes w_{8j \rightarrow 8j+1}; \\
b_{(j+1)_s, s+(-2)_s} &= -w_{8(j+m+1)+2 \rightarrow 8(j+m+1)+3} \otimes w_{8j \rightarrow 8(j+1)}; \\
b_{3s+(j+1)_s, s+(-2)_s} &= w_{8(j+m+1)+1 \rightarrow 8(j+m+1)+3} \otimes w_{8j \rightarrow 8(j+1)}; \\
b_{3s+(j+1)_s, 2s+(-2)_s} &= -e_{8(j+m+1)+1} \otimes w_{8j \rightarrow 8(j+1)}; \\
b_{(j+1)_s, 3s+(-2)_s} &= w_{8(j+m+1)+2 \rightarrow 8(j+m+1)+4} \otimes w_{8j+1 \rightarrow 8(j+1)}; \\
b_{2s+(j+1)_s, 3s+(-2)_s} &= -e_{8(j+m+1)+4} \otimes w_{8j+1 \rightarrow 8(j+1)}; \\
b_{(j+1)_s, 3s+(-1)_s} &= w_{8(j+m+1)+2 \rightarrow 8(j+m+1)+4} \otimes w_{8j+1 \rightarrow 8(j+1)}; \\
b_{2s+(j+1)_s, 3s+(-1)_s} &= -e_{8(j+m+1)+4} \otimes w_{8j+1 \rightarrow 8(j+1)}; \\
b_{3s+(j+1)_s, 4s+(-2)_s} &= -w_{8(j+m+1)+1 \rightarrow 8(j+m+1)+7} \otimes w_{8j+2 \rightarrow 8(j+1)}; \\
b_{s+(j+1)_s, 5s+(-2)_s} &= -w_{8(j+m+1)+6 \rightarrow 8(j+m+2)} \otimes w_{8j+3 \rightarrow 8(j+1)}; \\
b_{3s+(j+1)_s, 6s+(-2)_s} &= -w_{8(j+m+1)+1 \rightarrow 8(j+m+1)+7} \otimes w_{8j+4 \rightarrow 8(j+1)}; \\
b_{(j+1)_s, 7s+(-2)_s} &= w_{8(j+m+1)+2 \rightarrow 8(j+m+2)} \otimes w_{8j+5 \rightarrow 8(j+1)}; \\
b_{3s+(j+1)_s, 7s+(-2)_s} &= -w_{8(j+m+1)+1 \rightarrow 8(j+m+2)} \otimes w_{8j+5 \rightarrow 8(j+1)}.
\end{aligned}$$

(13) If  $r_0 = 12$ , then  $\Omega^{12}(Z_t^{(24)})$  is described with  $(19s \times 13s)$  matrix with the following nonzero entries:

$$\begin{aligned}
b_{2s+(j+1)_s, (-2)_s} &= e_{8(j+m)+7} \otimes w_{8j \rightarrow 8(j+1)}; \\
b_{2s+(j+1)_s, (-1)_s} &= e_{8(j+m)+7} \otimes w_{8j \rightarrow 8(j+1)}; \\
b_{j+3s, (-1)_s} &= w_{8(j+m)+2 \rightarrow 8(j+m)+7} \otimes w_{8j \rightarrow 8j+1}; \\
b_{j+5s, (-1)_s} &= -w_{8(j+m)+5 \rightarrow 8(j+m)+7} \otimes w_{8j \rightarrow 8j+2}; \\
b_{(j+1)_s, s+(-2)_s} &= w_{8(j+m)+7 \rightarrow 8(j+m+1)} \otimes w_{8j \rightarrow 8(j+1)}; \\
b_{2s+(j+1)_s, s+(-2)_s} &= -w_{8(j+m)+7 \rightarrow 8(j+m+1)} \otimes w_{8j \rightarrow 8(j+1)}; \\
b_{s+(j+1)_s, s+(-1)_s} &= e_{8(j+m+1)} \otimes w_{8j \rightarrow 8(j+1)}; \\
b_{s+(j+1)_s, 2s+(-2)_s} &= w_{8(j+m+1) \rightarrow 8(j+m+1)+4} \otimes w_{8j+1 \rightarrow 8(j+1)}; \\
b_{s+(j+1)_s, 2s+(-1)_s} &= w_{8(j+m+1) \rightarrow 8(j+m+1)+4} \otimes w_{8j+1 \rightarrow 8(j+1)}; \\
b_{(j+1)_s, 3s+(-2)_s} &= w_{8(j+m)+7 \rightarrow 8(j+m+1)+5} \otimes w_{8j+2 \rightarrow 8(j+1)}; \\
b_{2s+(j+1)_s, 3s+(-2)_s} &= -w_{8(j+m)+7 \rightarrow 8(j+m+1)+5} \otimes w_{8j+2 \rightarrow 8(j+1)}; \\
b_{(j+1)_s, 4s+(-2)_s} &= w_{8(j+m)+7 \rightarrow 8(j+m+1)+6} \otimes w_{8j+3 \rightarrow 8(j+1)}; \\
b_{2s+(j+1)_s, 4s+(-2)_s} &= -w_{8(j+m)+7 \rightarrow 8(j+m+1)+6} \otimes w_{8j+3 \rightarrow 8(j+1)}; \\
b_{(j+1)_s, 7s+(-2)_s} &= w_{8(j+m)+7 \rightarrow 8(j+m+1)+2} \otimes w_{8j+5 \rightarrow 8(j+1)}.
\end{aligned}$$

(14) If  $r_0 = 13$ , then  $\Omega^{13}(Z_t^{(24)})$  is described with  $(18s \times 14s)$  matrix with the following nonzero entries:

$$\begin{aligned}
b_{j+4s,(-1)_s} &= w_{8(j+m+1) \rightarrow 8(j+m+1)+2} \otimes w_{8j \rightarrow 8j+1}; \\
b_{(j+1)_s, s+(-2)_s} &= w_{8(j+m+1)+2 \rightarrow 8(j+m+1)+4} \otimes w_{8j \rightarrow 8(j+1)}; \\
b_{s+(j+1)_s, s+(-2)_s} &= -w_{8(j+m+1)+3 \rightarrow 8(j+m+1)+4} \otimes w_{8j \rightarrow 8(j+1)}; \\
b_{2s+(j+1)_s, 2s+(-2)_s} &= e_{8(j+m+1)+6} \otimes w_{8j \rightarrow 8(j+1)}; \\
b_{2s+(j+1)_s, 2s+(-1)_s} &= e_{8(j+m+1)+6} \otimes w_{8j \rightarrow 8(j+1)}; \\
b_{3s+(j+1)_s, 3s+(-1)_s} &= e_{8(j+m+1)+5} \otimes w_{8j \rightarrow 8(j+1)}; \\
b_{(j+1)_s, 4s+(-2)_s} &= -w_{8(j+m+1)+2 \rightarrow 8(j+m+1)+7} \otimes w_{8j+1 \rightarrow 8(j+1)}; \\
b_{(j+1)_s, 4s+(-1)_s} &= -w_{8(j+m+1)+2 \rightarrow 8(j+m+1)+7} \otimes w_{8j+1 \rightarrow 8(j+1)}; \\
b_{s+(j+1)_s, 4s+(-1)_s} &= w_{8(j+m+1)+3 \rightarrow 8(j+m+1)+7} \otimes w_{8j+1 \rightarrow 8(j+1)}; \\
b_{2s+(j+1)_s, 4s+(-1)_s} &= -w_{8(j+m+1)+6 \rightarrow 8(j+m+1)+7} \otimes w_{8j+1 \rightarrow 8(j+1)}; \\
b_{(j+1)_s, 5s+(-2)_s} &= w_{8(j+m+1)+2 \rightarrow 8(j+m+2)} \otimes w_{8j+2 \rightarrow 8(j+1)}; \\
b_{3s+(j+1)_s, 5s+(-2)_s} &= w_{8(j+m+1)+5 \rightarrow 8(j+m+2)} \otimes w_{8j+2 \rightarrow 8(j+1)}; \\
b_{(j+1)_s, 6s+(-2)_s} &= w_{8(j+m+1)+2 \rightarrow 8(j+m+1)+7} \otimes w_{8j+3 \rightarrow 8(j+1)}; \\
b_{3s+(j+1)_s, 6s+(-2)_s} &= w_{8(j+m+1)+5 \rightarrow 8(j+m+1)+7} \otimes w_{8j+3 \rightarrow 8(j+1)}; \\
b_{s+(j+1)_s, 8s+(-2)_s} &= w_{8(j+m+1)+3 \rightarrow 8(j+m+1)+7} \otimes w_{8j+5 \rightarrow 8(j+1)}.
\end{aligned}$$

(15) If  $r_0 = 14$ , then  $\Omega^{14}(Z_t^{(24)})$  is described with  $(20s \times 16s)$  matrix with the following nonzero entries:

$$\begin{aligned}
b_{(j+1)_s, (-2)_s} &= -e_{8(j+m)+7} \otimes w_{8j \rightarrow 8(j+1)}; \\
b_{(j+1)_s, (-1)_s} &= -e_{8(j+m)+7} \otimes w_{8j \rightarrow 8(j+1)}; \\
b_{j+3s, (-1)_s} &= w_{8(j+m)+3 \rightarrow 8(j+m)+7} \otimes w_{8j \rightarrow 8j+1}; \\
b_{(j+1)_s, s+(-1)_s} &= -e_{8(j+m)+7} \otimes w_{8j \rightarrow 8(j+1)}; \\
b_{2s+(j+1)_s, 2s+(-2)_s} &= e_{8(j+m+1)} \otimes w_{8j \rightarrow 8(j+1)}; \\
b_{2s+(j+1)_s, 2s+(-1)_s} &= e_{8(j+m+1)} \otimes w_{8j \rightarrow 8(j+1)}; \\
b_{(j+1)_s, 3s+(-2)_s} &= w_{8(j+m)+7 \rightarrow 8(j+m+1)+5} \otimes w_{8j+1 \rightarrow 8(j+1)}; \\
b_{2s+(j+1)_s, 3s+(-2)_s} &= -w_{8(j+m+1) \rightarrow 8(j+m+1)+5} \otimes w_{8j+1 \rightarrow 8(j+1)}; \\
b_{2s+(j+1)_s, 3s+(-1)_s} &= -w_{8(j+m+1) \rightarrow 8(j+m+1)+5} \otimes w_{8j+1 \rightarrow 8(j+1)}; \\
b_{(j+1)_s, 6s+(-2)_s} &= w_{8(j+m)+7 \rightarrow 8(j+m+1)+2} \otimes w_{8j+3 \rightarrow 8(j+1)}; \\
b_{s+(j+1)_s, 6s+(-2)_s} &= w_{8(j+m+1) \rightarrow 8(j+m+1)+2} \otimes w_{8j+3 \rightarrow 8(j+1)}; \\
b_{2s+(j+1)_s, 6s+(-2)_s} &= -w_{8(j+m+1) \rightarrow 8(j+m+1)+2} \otimes w_{8j+3 \rightarrow 8(j+1)}; \\
b_{3s+(j+1)_s, 7s+(-2)_s} &= e_{8(j+m+1)+3} \otimes w_{8j+4 \rightarrow 8(j+1)+1}; \\
b_{s+(j+1)_s, 9s+(-2)_s} &= w_{8(j+m+1) \rightarrow 8(j+m+1)+3} \otimes w_{8j+5 \rightarrow 8(j+1)}; \\
b_{3s+(j+1)_s, 14s+(-2)_s} &= w_{8(j+m+1)+3 \rightarrow 8(j+m+1)+7} \otimes w_{8j+7 \rightarrow 8(j+1)+1}; \\
b_{3s+(j+1)_s, 15s+(-2)_s} &= -w_{8(j+m+1)+3 \rightarrow 8(j+m+2)} \otimes w_{8j+7 \rightarrow 8(j+1)+1}.
\end{aligned}$$

(16) If  $r_0 = 15$ , then  $\Omega^{15}(Z_t^{(24)})$  is described with  $(18s \times 16s)$  matrix with the following nonzero entries:

$$\begin{aligned}
b_{3s+(j+1)_s, s+(-2)_s} &= -w_{8(j+m+1)+1 \rightarrow 8(j+m+1)+3} \otimes w_{8j \rightarrow 8(j+1)}; \\
b_{j+4s, s+(-1)_s} &= w_{8(j+m)+7 \rightarrow 8(j+m+1)+3} \otimes w_{8j \rightarrow 8j+1}; \\
b_{s+(j+1)_s, 2s+(-2)_s} &= -e_{8(j+m+1)+6} \otimes w_{8j \rightarrow 8(j+1)};
\end{aligned}$$

$$\begin{aligned}
b_{s+(j+1)s, 2s+(-1)s} &= -e_{8(j+m+1)+6} \otimes w_{8j \rightarrow 8(j+1)}; \\
b_{3s+(j+1)s, 3s+(-2)s} &= e_{8(j+m+1)+1} \otimes w_{8j \rightarrow 8(j+1)}; \\
b_{3s+(j+1)s, 3s+(-1)s} &= e_{8(j+m+1)+1} \otimes w_{8j \rightarrow 8(j+1)}; \\
b_{s+(j+1)s, 4s+(-2)s} &= w_{8(j+m+1)+6 \rightarrow 8(j+m+2)} \otimes w_{8j+1 \rightarrow 8(j+1)}; \\
b_{s+(j+1)s, 4s+(-1)s} &= w_{8(j+m+1)+6 \rightarrow 8(j+m+2)} \otimes w_{8j+1 \rightarrow 8(j+1)}; \\
b_{(j+1)s, 5s+(-2)s} &= -w_{8(j+m+1)+3 \rightarrow 8(j+m+1)+7} \otimes w_{8j+2 \rightarrow 8(j+1)}; \\
b_{3s+(j+1)s, 5s+(-2)s} &= w_{8(j+m+1)+1 \rightarrow 8(j+m+1)+7} \otimes w_{8j+2 \rightarrow 8(j+1)}; \\
b_{(j+1)s, 6s+(-2)s} &= w_{8(j+m+1)+3 \rightarrow 8(j+m+2)} \otimes w_{8j+3 \rightarrow 8(j+1)}; \\
b_{3s+(j+1)s, 6s+(-2)s} &= -w_{8(j+m+1)+1 \rightarrow 8(j+m+2)} \otimes w_{8j+3 \rightarrow 8(j+1)}; \\
b_{2s+(j+1)s, 8s+(-2)s} &= w_{8(j+m+1)+4 \rightarrow 8(j+m+1)+7} \otimes w_{8j+5 \rightarrow 8(j+1)}.
\end{aligned}$$

(17) If  $r_0 = 16$ , then  $\Omega^{16}(Z_t^{(24)})$  is described with  $(19s \times 19s)$  matrix with the following nonzero entries:

$$\begin{aligned}
b_{(j+1)s, (-2)s} &= e_{8(j+m)+7} \otimes w_{8j \rightarrow 8(j+1)}; \\
b_{2s+(j+1)s, (-2)s} &= -e_{8(j+m)+7} \otimes w_{8j \rightarrow 8(j+1)}; \\
b_{(j+1)s, (-1)s} &= e_{8(j+m)+7} \otimes w_{8j \rightarrow 8(j+1)}; \\
b_{2s+(j+1)s, (-1)s} &= -e_{8(j+m)+7} \otimes w_{8j \rightarrow 8(j+1)}; \\
b_{j+3s, (-1)s} &= -w_{8(j+m)+4 \rightarrow 8(j+m)+7} \otimes w_{8j \rightarrow 8j+1}; \\
b_{s+(j+1)s, s+(-2)s} &= -e_{8(j+m+1)} \otimes w_{8j \rightarrow 8(j+1)}; \\
b_{(j+1)s, 3s+(-2)s} &= -w_{8(j+m)+7 \rightarrow 8(j+m+1)+6} \otimes w_{8j+1 \rightarrow 8(j+1)}; \\
b_{2s+(j+1)s, 3s+(-2)s} &= w_{8(j+m)+7 \rightarrow 8(j+m+1)+6} \otimes w_{8j+1 \rightarrow 8(j+1)}; \\
b_{(j+1)s, 3s+(-1)s} &= -w_{8(j+m)+7 \rightarrow 8(j+m+1)+6} \otimes w_{8j+1 \rightarrow 8(j+1)}; \\
b_{2s+(j+1)s, 3s+(-1)s} &= w_{8(j+m)+7 \rightarrow 8(j+m+1)+6} \otimes w_{8j+1 \rightarrow 8(j+1)}; \\
b_{(j+1)s, 6s+(-2)s} &= w_{8(j+m)+7 \rightarrow 8(j+m+1)+3} \otimes w_{8j+3 \rightarrow 8(j+1)}; \\
b_{3s+(j+1)s, 8s+(-2)s} &= e_{8(j+m+1)+4} \otimes w_{8j+4 \rightarrow 8(j+1)+1}; \\
b_{2s+(j+1)s, 11s+(-2)s} &= w_{8(j+m)+7 \rightarrow 8(j+m+1)+4} \otimes w_{8j+5 \rightarrow 8(j+1)}; \\
b_{3s+(j+1)s, 17s+(-2)s} &= -w_{8(j+m+1)+4 \rightarrow 8(j+m+1)+7} \otimes w_{8j+7 \rightarrow 8(j+1)+1}.
\end{aligned}$$

(18) If  $r_0 = 17$ , then  $\Omega^{17}(Z_t^{(24)})$  is described with  $(18s \times 18s)$  matrix with the following nonzero entries:

$$\begin{aligned}
b_{(j+1)s, (-2)s} &= e_{8(j+m+1)+2} \otimes w_{8j \rightarrow 8(j+1)}; \\
b_{j+4s, (-1)s} &= -w_{8(j+m)+7 \rightarrow 8(j+m+1)+2} \otimes w_{8j \rightarrow 8j+1}; \\
b_{(j+1)s, 2s+(-2)s} &= w_{8(j+m+1)+2 \rightarrow 8(j+m+1)+4} \otimes w_{8j \rightarrow 8(j+1)}; \\
b_{3s+(j+1)s, 4s+(-2)s} &= -e_{8(j+m+1)+5} \otimes w_{8j \rightarrow 8(j+1)}; \\
b_{(j+1)s, 5s+(-2)s} &= -w_{8(j+m+1)+2 \rightarrow 8(j+m+1)+7} \otimes w_{8j+1 \rightarrow 8(j+1)}; \\
b_{s+(j+1)s, 5s+(-2)s} &= w_{8(j+m+1)+4 \rightarrow 8(j+m+1)+7} \otimes w_{8j+1 \rightarrow 8(j+1)}; \\
b_{3s+(j+1)s, 5s+(-2)s} &= -w_{8(j+m+1)+5 \rightarrow 8(j+m+1)+7} \otimes w_{8j+1 \rightarrow 8(j+1)}; \\
b_{(j+1)s, 5s+(-1)s} &= -w_{8(j+m+1)+2 \rightarrow 8(j+m+1)+7} \otimes w_{8j+1 \rightarrow 8(j+1)}; \\
b_{3s+(j+1)s, 5s+(-1)s} &= -w_{8(j+m+1)+5 \rightarrow 8(j+m+1)+7} \otimes w_{8j+1 \rightarrow 8(j+1)}; \\
b_{s+(j+1)s, 7s+(-2)s} &= w_{8(j+m+1)+4 \rightarrow 8(j+m+1)+7} \otimes w_{8j+3 \rightarrow 8(j+1)}; \\
b_{2s+(j+1)s, 10s+(-2)s} &= -w_{8(j+m+1)+6 \rightarrow 8(j+m+1)+7} \otimes w_{8j+5 \rightarrow 8(j+1)}.
\end{aligned}$$

(19) If  $r_0 = 18$ , then  $\Omega^{18}(Z_t^{(24)})$  is described with  $(19s \times 19s)$  matrix with the following nonzero entries:

$$\begin{aligned}
b_{j+3s,(-1)_s} &= -w_{8(j+m)+5 \rightarrow 8(j+m)+7} \otimes w_{8j \rightarrow 8j+1}; \\
b_{j+4s,(-1)_s} &= w_{8(j+m)+1 \rightarrow 8(j+m)+7} \otimes w_{8j \rightarrow 8j+1}; \\
b_{j+5s,(-1)_s} &= w_{8(j+m)+2 \rightarrow 8(j+m)+7} \otimes w_{8j \rightarrow 8j+2}; \\
b_{(j+1)_s, 2s+(-2)_s} &= e_{8(j+m)+7} \otimes w_{8j \rightarrow 8(j+1)}; \\
b_{(j+1)_s, 3s+(-2)_s} &= -w_{8(j+m)+7 \rightarrow 8(j+m+1)+2} \otimes w_{8j+1 \rightarrow 8(j+1)}; \\
b_{(j+1)_s, 3s+(-1)_s} &= -w_{8(j+m)+7 \rightarrow 8(j+m+1)+2} \otimes w_{8j+1 \rightarrow 8(j+1)}; \\
b_{s+(j+1)_s, 3s+(-1)_s} &= -w_{8(j+m+1) \rightarrow 8(j+m+1)+2} \otimes w_{8j+1 \rightarrow 8(j+1)}; \\
b_{2s+(j+1)_s, 3s+(-1)_s} &= w_{8(j+m+1) \rightarrow 8(j+m+1)+2} \otimes w_{8j+1 \rightarrow 8(j+1)}; \\
b_{(j+1)_s, 4s+(-2)_s} &= -w_{8(j+m)+7 \rightarrow 8(j+m+1)+3} \otimes w_{8j+2 \rightarrow 8(j+1)}; \\
b_{s+(j+1)_s, 6s+(-2)_s} &= w_{8(j+m+1) \rightarrow 8(j+m+1)+4} \otimes w_{8j+3 \rightarrow 8(j+1)}; \\
b_{2s+(j+1)_s, 6s+(-2)_s} &= -w_{8(j+m+1) \rightarrow 8(j+m+1)+4} \otimes w_{8j+3 \rightarrow 8(j+1)}; \\
b_{5s+(j+1)_s, 6s+(-2)_s} &= -w_{8(j+m+1)+2 \rightarrow 8(j+m+1)+4} \otimes w_{8j+3 \rightarrow 8(j+1)+2}; \\
b_{2s+(j+1)_s, 11s+(-2)_s} &= -w_{8(j+m+1) \rightarrow 8(j+m+1)+6} \otimes w_{8j+5 \rightarrow 8(j+1)}.
\end{aligned}$$

(20) If  $r_0 = 19$ , then  $\Omega^{19}(Z_t^{(24)})$  is described with  $(16s \times 18s)$  matrix with the following nonzero entries:

$$\begin{aligned}
b_{j+4s,(-1)_s} &= -w_{8(j+m+1) \rightarrow 8(j+m+1)+2} \otimes w_{8j \rightarrow 8j+1}; \\
b_{(j+1)_s, s+(-1)_s} &= e_{8(j+m+1)+3} \otimes w_{8j \rightarrow 8(j+1)}; \\
b_{2s+(j+1)_s, s+(-1)_s} &= -w_{8(j+m+1)+1 \rightarrow 8(j+m+1)+3} \otimes w_{8j \rightarrow 8(j+1)}; \\
b_{s+(j+1)_s, 2s+(-2)_s} &= e_{8(j+m+1)+6} \otimes w_{8j \rightarrow 8(j+1)}; \\
b_{(j+1)_s, 4s+(-1)_s} &= -w_{8(j+m+1)+3 \rightarrow 8(j+m+2)} \otimes w_{8j+1 \rightarrow 8(j+1)}; \\
b_{2s+(j+1)_s, 4s+(-1)_s} &= w_{8(j+m+1)+1 \rightarrow 8(j+m+2)} \otimes w_{8j+1 \rightarrow 8(j+1)}; \\
b_{(j+1)_s, 5s+(-2)_s} &= -w_{8(j+m+1)+3 \rightarrow 8(j+m+1)+7} \otimes w_{8j+2 \rightarrow 8(j+1)}; \\
b_{2s+(j+1)_s, 5s+(-2)_s} &= w_{8(j+m+1)+1 \rightarrow 8(j+m+1)+7} \otimes w_{8j+2 \rightarrow 8(j+1)}; \\
b_{2s+(j+1)_s, 6s+(-2)_s} &= -w_{8(j+m+1)+1 \rightarrow 8(j+m+1)+7} \otimes w_{8j+3 \rightarrow 8(j+1)}; \\
b_{3s+(j+1)_s, 6s+(-2)_s} &= w_{8(j+m+1)+5 \rightarrow 8(j+m+1)+7} \otimes w_{8j+3 \rightarrow 8(j+1)}; \\
b_{4s+(j+1)_s, 7s+(-2)_s} &= e_{8(j+m+2)} \otimes w_{8j+3 \rightarrow 8(j+1)+1}; \\
b_{2s+(j+1)_s, 9s+(-2)_s} &= w_{8(j+m+1)+1 \rightarrow 8(j+m+1)+7} \otimes w_{8j+5 \rightarrow 8(j+1)}; \\
b_{2s+(j+1)_s, 10s+(-2)_s} &= -w_{8(j+m+1)+1 \rightarrow 8(j+m+2)} \otimes w_{8j+5 \rightarrow 8(j+1)}; \\
b_{4s+(j+1)_s, 16s+(-2)_s} &= -w_{8(j+m+2) \rightarrow 8(j+m+2)+1} \otimes w_{8j+7 \rightarrow 8(j+1)+1}.
\end{aligned}$$

(21) If  $r_0 = 20$ , then  $\Omega^{20}(Z_t^{(24)})$  is described with  $(16s \times 20s)$  matrix with the following nonzero entries:

$$\begin{aligned}
b_{(j+1)_s, (-2)_s} &= -e_{8(j+m)+7} \otimes w_{8j \rightarrow 8(j+1)}; \\
b_{(j+1)_s, (-1)_s} &= -e_{8(j+m)+7} \otimes w_{8j \rightarrow 8(j+1)}; \\
b_{j+3s,(-1)_s} &= -w_{8(j+m)+6 \rightarrow 8(j+m)+7} \otimes w_{8j \rightarrow 8j+1}; \\
b_{s+(j+1)_s, s+(-2)_s} &= e_{8(j+m+1)} \otimes w_{8j \rightarrow 8(j+1)}; \\
b_{(j+1)_s, 2s+(-2)_s} &= -w_{8(j+m)+7 \rightarrow 8(j+m+1)} \otimes w_{8j \rightarrow 8(j+1)}; \\
b_{s+(j+1)_s, 2s+(-2)_s} &= e_{8(j+m+1)} \otimes w_{8j \rightarrow 8(j+1)}; \\
b_{(j+1)_s, 3s+(-2)_s} &= -w_{8(j+m)+7 \rightarrow 8(j+m+1)+3} \otimes w_{8j+1 \rightarrow 8(j+1)};
\end{aligned}$$

$$\begin{aligned}
b_{s+(j+1)s,3s+(-2)s} &= w_{8(j+m+1) \rightarrow 8(j+m+1)+3} \otimes w_{8j+1 \rightarrow 8(j+1)}; \\
b_{(j+1)s,3s+(-1)s} &= -w_{8(j+m)+7 \rightarrow 8(j+m+1)+3} \otimes w_{8j+1 \rightarrow 8(j+1)}; \\
b_{s+(j+1)s,7s+(-2)s} &= -w_{8(j+m+1) \rightarrow 8(j+m+1)+5} \otimes w_{8j+3 \rightarrow 8(j+1)}; \\
b_{6s+(j+1)s,7s+(-2)s} &= -e_{8(j+m+1)+5} \otimes w_{8j+3 \rightarrow 8(j+1)+3}; \\
b_{j-3s,13s+(-2)s} &= -w_{8(j+m)+1 \rightarrow 8(j+m+1)+1} \otimes e_{8j+5}.
\end{aligned}$$

(22) If  $r_0 = 21$ , then  $\Omega^{21}(Z_t^{(24)})$  is described with  $(14s \times 18s)$  matrix with the following nonzero entries:

$$\begin{aligned}
b_{j+2s,s+(-1)s} &= w_{8(j+m)+7 \rightarrow 8(j+m+1)+6} \otimes w_{8j \rightarrow 8j+1}; \\
b_{(j+1)s,2s+(-2)s} &= w_{8(j+m+1)+2 \rightarrow 8(j+m+1)+4} \otimes w_{8j \rightarrow 8(j+1)}; \\
b_{s+(j+1)s,2s+(-2)s} &= e_{8(j+m+1)+4} \otimes w_{8j \rightarrow 8(j+1)}; \\
b_{(j+1)s,2s+(-1)s} &= w_{8(j+m+1)+2 \rightarrow 8(j+m+1)+4} \otimes w_{8j \rightarrow 8(j+1)}; \\
b_{s+(j+1)s,2s+(-1)s} &= e_{8(j+m+1)+4} \otimes w_{8j \rightarrow 8(j+1)}; \\
b_{j-3s,3s+(-2)s} &= w_{8(j+m)+2 \rightarrow 8(j+m+1)+1} \otimes e_{8j}; \\
b_{j,3s+(-2)s} &= w_{8(j+m)+7 \rightarrow 8(j+m+1)+1} \otimes w_{8j \rightarrow 8j+1}; \\
b_{j+s,3s+(-2)s} &= w_{8(j+m+1) \rightarrow 8(j+m+1)+1} \otimes w_{8j \rightarrow 8j+2}; \\
b_{j+2s,3s+(-2)s} &= w_{8(j+m)+7 \rightarrow 8(j+m+1)+1} \otimes w_{8j \rightarrow 8j+3}; \\
b_{j+3s,3s+(-2)s} &= w_{8(j+m+1) \rightarrow 8(j+m+1)+1} \otimes w_{8j \rightarrow 8j+4}; \\
b_{j+6s,3s+(-2)s} &= w_{8(j+m+1) \rightarrow 8(j+m+1)+1} \otimes w_{8j \rightarrow 8j+6}; \\
b_{(j+1)s,5s+(-2)s} &= -w_{8(j+m+1)+2 \rightarrow 8(j+m+1)+7} \otimes w_{8j+1 \rightarrow 8(j+1)}; \\
b_{s+(j+1)s,5s+(-2)s} &= -w_{8(j+m+1)+4 \rightarrow 8(j+m+1)+7} \otimes w_{8j+1 \rightarrow 8(j+1)}; \\
b_{2s+(j+1)s,5s+(-2)s} &= w_{8(j+m+1)+6 \rightarrow 8(j+m+1)+7} \otimes w_{8j+1 \rightarrow 8(j+1)}; \\
b_{(j+1)s,5s+(-1)s} &= -w_{8(j+m+1)+2 \rightarrow 8(j+m+1)+7} \otimes w_{8j+1 \rightarrow 8(j+1)}; \\
b_{s+(j+1)s,5s+(-1)s} &= -w_{8(j+m+1)+4 \rightarrow 8(j+m+1)+7} \otimes w_{8j+1 \rightarrow 8(j+1)}; \\
b_{2s+(j+1)s,6s+(-2)s} &= w_{8(j+m+1)+6 \rightarrow 8(j+m+1)+7} \otimes w_{8j+2 \rightarrow 8(j+1)}; \\
b_{2s+(j+1)s,8s+(-2)s} &= -w_{8(j+m+1)+6 \rightarrow 8(j+m+2)} \otimes w_{8j+3 \rightarrow 8(j+1)}.
\end{aligned}$$

(23) If  $r_0 = 22$ , then  $\Omega^{22}(Z_t^{(24)})$  is described with  $(13s \times 19s)$  matrix with the following nonzero entries:

$$\begin{aligned}
b_{j,(-2)s} &= -w_{8(j+m) \rightarrow 8(j+m)+7} \otimes e_{8j}; \\
b_{j+s,(-2)s} &= w_{8(j+m-1)+7 \rightarrow 8(j+m)+7} \otimes e_{8j}; \\
b_{s+(j+1)s,(-2)s} &= -e_{8(j+m)+7} \otimes w_{8j \rightarrow 8(j+1)}; \\
b_{j+6s,(-2)s} &= -w_{8(j+m)+1 \rightarrow 8(j+m)+7} \otimes w_{8j \rightarrow 8j+4}; \\
b_{j+7s,(-2)s} &= -w_{8(j+m)+2 \rightarrow 8(j+m)+7} \otimes w_{8j \rightarrow 8j+5}; \\
b_{j+2s,(-1)s} &= -w_{8(j+m)+3 \rightarrow 8(j+m)+7} \otimes w_{8j \rightarrow 8j+1}; \\
b_{j+3s,(-1)s} &= w_{8(j+m)+4 \rightarrow 8(j+m)+7} \otimes w_{8j \rightarrow 8j+2}; \\
b_{(j+1)s,s+(-2)s} &= -e_{8(j+m+1)} \otimes w_{8j \rightarrow 8(j+1)}; \\
b_{(j+1)s,s+(-1)s} &= -e_{8(j+m+1)} \otimes w_{8j \rightarrow 8(j+1)}; \\
b_{(j+1)s,3s+(-2)s} &= -w_{8(j+m+1) \rightarrow 8(j+m+1)+4} \otimes w_{8j+1 \rightarrow 8(j+1)}; \\
b_{(j+1)s,3s+(-1)s} &= -w_{8(j+m+1) \rightarrow 8(j+m+1)+4} \otimes w_{8j+1 \rightarrow 8(j+1)}; \\
b_{s+(j+1)s,4s+(-2)s} &= -w_{8(j+m)+7 \rightarrow 8(j+m+1)+6} \otimes w_{8j+1 \rightarrow 8(j+1)}; \\
b_{(j+1)s,6s+(-3)s} &= -w_{8(j+m+1) \rightarrow 8(j+m+1)+1} \otimes w_{8j+2 \rightarrow 8(j+1)};
\end{aligned}$$



$$\begin{aligned}
b_{s+(j+1)_s, 6s+(-3)_s} &= w_{8(j+m)+7 \rightarrow 8(j+m+1)+1} \otimes w_{8j+2 \rightarrow 8(j+1)}; \\
b_{(j+1)_s, 7s+(-3)_s} &= w_{8(j+m+1) \rightarrow 8(j+m+1)+2} \otimes w_{8j+3 \rightarrow 8(j+1)}; \\
b_{s+(j+1)_s, 7s+(-3)_s} &= -w_{8(j+m)+7 \rightarrow 8(j+m+1)+2} \otimes w_{8j+3 \rightarrow 8(j+1)}; \\
b_{s+(j+1)_s, 8s+(-2)_s} &= w_{8(j+m)+7 \rightarrow 8(j+m+1)+6} \otimes w_{8j+3 \rightarrow 8(j+1)}; \\
b_{5s+(j+1)_s, 8s+(-2)_s} &= e_{8(j+m+1)+6} \otimes w_{8j+3 \rightarrow 8(j+1)+3}.
\end{aligned}$$

(24) If  $r_0 = 23$ , then  $\Omega^{23}(Z_t^{(24)})$  is described with  $(11s \times 18s)$  matrix with the following nonzero entries:

$$\begin{aligned}
b_{j,(-2)_s} &= -w_{8(j+m)+3 \rightarrow 8(j+m+1)+2} \otimes e_{8j}; \\
b_{j+2s,(-2)_s} &= -w_{8(j+m+1) \rightarrow 8(j+m+1)+2} \otimes w_{8j \rightarrow 8j+1}; \\
b_{j+3s,(-2)_s} &= -w_{8(j+m)+7 \rightarrow 8(j+m+1)+2} \otimes w_{8j \rightarrow 8j+2}; \\
b_{j+7s,(-2)_s} &= -w_{8(j+m)+7 \rightarrow 8(j+m+1)+2} \otimes w_{8j \rightarrow 8j+6}; \\
b_{j+2s,(-1)_s} &= -w_{8(j+m+1) \rightarrow 8(j+m+1)+2} \otimes w_{8j \rightarrow 8j+1}; \\
b_{(j+1)_s, s+(-2)_s} &= w_{8(j+m+1)+3 \rightarrow 8(j+m+1)+4} \otimes w_{8j \rightarrow 8(j+1)}; \\
b_{j+s, s+(-1)_s} &= -w_{8(j+m+1) \rightarrow 8(j+m+1)+4} \otimes w_{8j \rightarrow 8j+1}; \\
b_{s+(j+1)_s, 3s+(-2)_s} &= -e_{8(j+m+1)+5} \otimes w_{8j \rightarrow 8(j+1)}; \\
b_{s+(j+1)_s, 3s+(-1)_s} &= -e_{8(j+m+1)+5} \otimes w_{8j \rightarrow 8(j+1)}; \\
b_{(j+1)_s, 4s+(-2)_s} &= -w_{8(j+m+1)+3 \rightarrow 8(j+m+1)+7} \otimes w_{8j+1 \rightarrow 8(j+1)}; \\
b_{s+(j+1)_s, 4s+(-1)_s} &= -w_{8(j+m+1)+5 \rightarrow 8(j+m+1)+7} \otimes w_{8j+1 \rightarrow 8(j+1)}; \\
b_{(j+1)_s, 5s+(-2)_s} &= w_{8(j+m+1)+3 \rightarrow 8(j+m+2)} \otimes w_{8j+1 \rightarrow 8(j+1)}; \\
b_{s+(j+1)_s, 5s+(-2)_s} &= -w_{8(j+m+1)+5 \rightarrow 8(j+m+2)} \otimes w_{8j+1 \rightarrow 8(j+1)}; \\
b_{2s+(j+1)_s, 6s+(-2)_s} &= -e_{8(j+m+2)} \otimes w_{8j+2 \rightarrow 8(j+1)+1}; \\
b_{(j+1)_s, 7s+(-2)_s} &= w_{8(j+m+1)+3 \rightarrow 8(j+m+1)+7} \otimes w_{8j+3 \rightarrow 8(j+1)}; \\
b_{s+(j+1)_s, 7s+(-2)_s} &= -w_{8(j+m+1)+5 \rightarrow 8(j+m+1)+7} \otimes w_{8j+3 \rightarrow 8(j+1)}; \\
b_{3s+(j+1)_s, 7s+(-2)_s} &= e_{8(j+m+1)+7} \otimes w_{8j+3 \rightarrow 8(j+1)+2}.
\end{aligned}$$

(25) If  $r_0 = 24$ , then  $\Omega^{24}(Z_t^{(24)})$  is described with  $(11s \times 19s)$  matrix with the following nonzero entries:

$$\begin{aligned}
b_{j,(-2)_s} &= -w_{8(j+m) \rightarrow 8(j+m)+7} \otimes e_{8j}; \\
b_{j+4s,(-2)_s} &= w_{8(j+m)+1 \rightarrow 8(j+m)+7} \otimes w_{8j \rightarrow 8j+3}; \\
b_{j+5s,(-2)_s} &= -w_{8(j+m)+2 \rightarrow 8(j+m)+7} \otimes w_{8j \rightarrow 8j+4}; \\
b_{j+6s,(-2)_s} &= -w_{8(j+m)+3 \rightarrow 8(j+m)+7} \otimes w_{8j \rightarrow 8j+5}; \\
b_{(j+1)_s, s+(-2)_s} &= e_{8(j+m+1)} \otimes w_{8j \rightarrow 8(j+1)}; \\
b_{j+s, s+(-1)_s} &= -w_{8(j+m)+5 \rightarrow 8(j+m+1)} \otimes w_{8j \rightarrow 8j+1}; \\
b_{(j+1)_s, 2s+(-2)_s} &= e_{8(j+m+1)} \otimes w_{8j \rightarrow 8(j+1)}; \\
b_{j-s, 3s+(-2)_s} &= -w_{8(j+m)+5 \rightarrow 8(j+m+1)+5} \otimes e_{8j+1}; \\
b_{j-s, 3s+(-1)_s} &= -w_{8(j+m)+5 \rightarrow 8(j+m+1)+5} \otimes e_{8j+1}; \\
b_{(j+1)_s, 4s+(-2)_s} &= w_{8(j+m+1) \rightarrow 8(j+m+1)+1} \otimes w_{8j+1 \rightarrow 8(j+1)}; \\
b_{(j+1)_s, 5s+(-3)_s} &= w_{8(j+m+1) \rightarrow 8(j+m+1)+2} \otimes w_{8j+2 \rightarrow 8(j+1)}; \\
b_{(j+1)_s, 6s+(-2)_s} &= -w_{8(j+m+1) \rightarrow 8(j+m+1)+6} \otimes w_{8j+2 \rightarrow 8(j+1)}; \\
b_{(j+1)_s, 7s+(-2)_s} &= w_{8(j+m+1) \rightarrow 8(j+m+1)+3} \otimes w_{8j+3 \rightarrow 8(j+1)}; \\
b_{4s+(j+1)_s, 7s+(-2)_s} &= -w_{8(j+m+1)+1 \rightarrow 8(j+m+1)+3} \otimes w_{8j+3 \rightarrow 8(j+1)+3};
\end{aligned}$$

$$\begin{aligned}
b_{(j+1)s, 7s+(-3)s} &= w_{8(j+m+1) \rightarrow 8(j+m+1)+3} \otimes w_{8j+3 \rightarrow 8(j+1)}; \\
b_{4s+(j+1)s, 7s+(-3)s} &= -w_{8(j+m+1)+1 \rightarrow 8(j+m+1)+3} \otimes w_{8j+3 \rightarrow 8(j+1)+3}; \\
b_{(j+1)s, 14s+(-3)s} &= -w_{8(j+m+1) \rightarrow 8(j+m+1)+4} \otimes w_{8j+6 \rightarrow 8(j+1)}; \\
b_{6s+(j+1)s, 14s+(-3)s} &= -w_{8(j+m+1)+3 \rightarrow 8(j+m+1)+4} \otimes w_{8j+6 \rightarrow 8(j+1)+5}; \\
b_{(j+1)s, 16s+(-3)s} &= w_{8(j+m+1) \rightarrow 8(j+m+1)+7} \otimes w_{8j+7 \rightarrow 8(j+1)}; \\
b_{4s+(j+1)s, 16s+(-3)s} &= -w_{8(j+m+1)+1 \rightarrow 8(j+m+1)+7} \otimes w_{8j+7 \rightarrow 8(j+1)+3}; \\
b_{5s+(j+1)s, 16s+(-3)s} &= w_{8(j+m+1)+2 \rightarrow 8(j+m+1)+7} \otimes w_{8j+7 \rightarrow 8(j+1)+4}; \\
b_{6s+(j+1)s, 16s+(-3)s} &= w_{8(j+m+1)+3 \rightarrow 8(j+m+1)+7} \otimes w_{8j+7 \rightarrow 8(j+1)+5}; \\
b_{2s+(j+1)s, 17s+(-3)s} &= w_{8(j+m+1)+5 \rightarrow 8(j+m+2)} \otimes w_{8j+7 \rightarrow 8(j+1)+1}.
\end{aligned}$$

(26) If  $r_0 = 25$ , then  $\Omega^{25}(Z_t^{(24)})$  is described with  $(10s \times 16s)$  matrix with the following nonzero entries:

$$\begin{aligned}
b_{j, (-2)s} &= -w_{8(j+m)+4 \rightarrow 8(j+m+1)+3} \otimes e_{8j}; \\
b_{j+2s, (-2)s} &= -w_{8(j+m)+7 \rightarrow 8(j+m+1)+3} \otimes w_{8j \rightarrow 8j+1}; \\
b_{j+3s, (-2)s} &= -w_{8(j+m+1) \rightarrow 8(j+m+1)+3} \otimes w_{8j \rightarrow 8j+2}; \\
b_{j+7s, (-2)s} &= -w_{8(j+m+1) \rightarrow 8(j+m+1)+3} \otimes w_{8j \rightarrow 8j+6}; \\
b_{j-s, 3s+(-2)s} &= -w_{8(j+m)+7 \rightarrow 8(j+m+1)+5} \otimes w_{8j \rightarrow 8j+1}; \\
b_{j, 3s+(-2)s} &= -w_{8(j+m+1) \rightarrow 8(j+m+1)+5} \otimes w_{8j \rightarrow 8j+2}; \\
b_{j+4s, 3s+(-2)s} &= -w_{8(j+m+1) \rightarrow 8(j+m+1)+5} \otimes w_{8j \rightarrow 8j+6}; \\
b_{s+(j+1)s, 4s+(-2)s} &= -w_{8(j+m+1)+6 \rightarrow 8(j+m+2)} \otimes w_{8j+1 \rightarrow 8(j+1)}; \\
b_{s+(j+1)s, 6s+(-2)s} &= w_{8(j+m+1)+6 \rightarrow 8(j+m+2)} \otimes w_{8j+3 \rightarrow 8(j+1)}; \\
b_{3s+(j+1)s, 6s+(-2)s} &= e_{8(j+m+2)} \otimes w_{8j+3 \rightarrow 8(j+1)+2}; \\
b_{s+(j+1)s, 6s+(-3)s} &= w_{8(j+m+1)+6 \rightarrow 8(j+m+2)} \otimes w_{8j+3 \rightarrow 8(j+1)}; \\
b_{3s+(j+1)s, 6s+(-3)s} &= e_{8(j+m+2)} \otimes w_{8j+3 \rightarrow 8(j+1)+2}; \\
b_{(j+1)s, 11s+(-3)s} &= -w_{8(j+m+1)+4 \rightarrow 8(j+m+2)} \otimes w_{8j+6 \rightarrow 8(j+1)}; \\
b_{7s+(j+1)s, 11s+(-3)s} &= -e_{8(j+m+2)} \otimes w_{8j+6 \rightarrow 8(j+1)+6}; \\
b_{(j+1)s, 12s+(-3)s} &= w_{8(j+m+1)+4 \rightarrow 8(j+m+2)+2} \otimes w_{8j+7 \rightarrow 8(j+1)}; \\
b_{2s+(j+1)s, 12s+(-3)s} &= w_{8(j+m+1)+7 \rightarrow 8(j+m+2)+2} \otimes w_{8j+7 \rightarrow 8(j+1)+1}; \\
b_{3s+(j+1)s, 12s+(-3)s} &= w_{8(j+m+2) \rightarrow 8(j+m+2)+2} \otimes w_{8j+7 \rightarrow 8(j+1)+2}; \\
b_{7s+(j+1)s, 12s+(-3)s} &= w_{8(j+m+2) \rightarrow 8(j+m+2)+2} \otimes w_{8j+7 \rightarrow 8(j+1)+6}; \\
b_{2s+(j+1)s, 15s+(-2)s} &= -w_{8(j+m+1)+7 \rightarrow 8(j+m+2)+5} \otimes w_{8j+7 \rightarrow 8(j+1)+1}; \\
b_{3s+(j+1)s, 15s+(-2)s} &= -w_{8(j+m+2) \rightarrow 8(j+m+2)+5} \otimes w_{8j+7 \rightarrow 8(j+1)+2}; \\
b_{7s+(j+1)s, 15s+(-2)s} &= -w_{8(j+m+2) \rightarrow 8(j+m+2)+5} \otimes w_{8j+7 \rightarrow 8(j+1)+6}; \\
b_{2s+(j+1)s, 15s+(-3)s} &= w_{8(j+m+1)+7 \rightarrow 8(j+m+2)+5} \otimes w_{8j+7 \rightarrow 8(j+1)+1}; \\
b_{3s+(j+1)s, 15s+(-3)s} &= w_{8(j+m+2) \rightarrow 8(j+m+2)+5} \otimes w_{8j+7 \rightarrow 8(j+1)+2}; \\
b_{7s+(j+1)s, 15s+(-3)s} &= w_{8(j+m+2) \rightarrow 8(j+m+2)+5} \otimes w_{8j+7 \rightarrow 8(j+1)+6}.
\end{aligned}$$

(27) If  $r_0 = 26$ , then  $\Omega^{26}(Z_t^{(24)})$  is described with  $(8s \times 16s)$  matrix with the following nonzero entries:

$$\begin{aligned}
b_{(j+1)s, s+(-3)s} &= w_{8(j+m)+7 \rightarrow 8(j+m+1)} \otimes w_{8j \rightarrow 8(j+1)}; \\
b_{(j+1)s, 2s+(-3)s} &= -w_{8(j+m)+7 \rightarrow 8(j+m+1)+2} \otimes w_{8j+1 \rightarrow 8(j+1)}; \\
b_{j-2s, 3s+(-2)s} &= -w_{8(j+m)+6 \rightarrow 8(j+m+1)+6} \otimes e_{8j+1};
\end{aligned}$$

$$\begin{aligned}
b_{s+(j+1)s,3s+(-3)s} &= -e_{8(j+m+1)+6} \otimes w_{8j+1 \rightarrow 8(j+1)+1}; \\
b_{2s+(j+1)s,4s+(-2)s} &= w_{8(j+m+1)+1 \rightarrow 8(j+m+1)+3} \otimes w_{8j+2 \rightarrow 8(j+1)+2}; \\
b_{2s+(j+1)s,4s+(-3)s} &= w_{8(j+m+1)+1 \rightarrow 8(j+m+1)+3} \otimes w_{8j+2 \rightarrow 8(j+1)+2}; \\
b_{2s+(j+1)s,5s+(-2)s} &= w_{8(j+m+1)+1 \rightarrow 8(j+m+1)+4} \otimes w_{8j+3 \rightarrow 8(j+1)+2}; \\
b_{3s+(j+1)s,5s+(-2)s} &= -w_{8(j+m+1)+2 \rightarrow 8(j+m+1)+4} \otimes w_{8j+3 \rightarrow 8(j+1)+3}; \\
b_{2s+(j+1)s,5s+(-3)s} &= w_{8(j+m+1)+1 \rightarrow 8(j+m+1)+4} \otimes w_{8j+3 \rightarrow 8(j+1)+2}; \\
b_{3s+(j+1)s,5s+(-3)s} &= -w_{8(j+m+1)+2 \rightarrow 8(j+m+1)+4} \otimes w_{8j+3 \rightarrow 8(j+1)+3}; \\
b_{(j+1)s,6s+(-2)s} &= -w_{8(j+m)+7 \rightarrow 8(j+m+1)+5} \otimes w_{8j+3 \rightarrow 8(j+1)}; \\
b_{(j+1)s,6s+(-3)s} &= -w_{8(j+m)+7 \rightarrow 8(j+m+1)+5} \otimes w_{8j+3 \rightarrow 8(j+1)}; \\
b_{6s+(j+1)s,12s+(-2)s} &= e_{8(j+m+1)+5} \otimes w_{8j+6 \rightarrow 8(j+1)+6}; \\
b_{6s+(j+1)s,12s+(-3)s} &= e_{8(j+m+1)+5} \otimes w_{8j+6 \rightarrow 8(j+1)+6}; \\
b_{(j+1)s,13s+(-2)s} &= -w_{8(j+m)+7 \rightarrow 8(j+m+1)+7} \otimes w_{8j+7 \rightarrow 8(j+1)}; \\
b_{2s+(j+1)s,13s+(-2)s} &= -w_{8(j+m+1)+1 \rightarrow 8(j+m+1)+7} \otimes w_{8j+7 \rightarrow 8(j+1)+2}; \\
b_{3s+(j+1)s,13s+(-2)s} &= w_{8(j+m+1)+2 \rightarrow 8(j+m+1)+7} \otimes w_{8j+7 \rightarrow 8(j+1)+3}; \\
b_{4s+(j+1)s,13s+(-2)s} &= -w_{8(j+m+1)+3 \rightarrow 8(j+m+1)+7} \otimes w_{8j+7 \rightarrow 8(j+1)+4}; \\
b_{5s+(j+1)s,13s+(-2)s} &= -w_{8(j+m+1)+4 \rightarrow 8(j+m+1)+7} \otimes w_{8j+7 \rightarrow 8(j+1)+5}; \\
b_{(j+1)s,13s+(-3)s} &= -w_{8(j+m)+7 \rightarrow 8(j+m+1)+7} \otimes w_{8j+7 \rightarrow 8(j+1)}; \\
b_{2s+(j+1)s,13s+(-3)s} &= -w_{8(j+m+1)+1 \rightarrow 8(j+m+1)+7} \otimes w_{8j+7 \rightarrow 8(j+1)+2}; \\
b_{3s+(j+1)s,13s+(-3)s} &= w_{8(j+m+1)+2 \rightarrow 8(j+m+1)+7} \otimes w_{8j+7 \rightarrow 8(j+1)+3}; \\
b_{4s+(j+1)s,13s+(-3)s} &= -w_{8(j+m+1)+3 \rightarrow 8(j+m+1)+7} \otimes w_{8j+7 \rightarrow 8(j+1)+4}; \\
b_{5s+(j+1)s,13s+(-3)s} &= -w_{8(j+m+1)+4 \rightarrow 8(j+m+1)+7} \otimes w_{8j+7 \rightarrow 8(j+1)+5}.
\end{aligned}$$

(28) If  $r_0 = 27$ , then  $\Omega^{27}(Z_t^{(24)})$  is described with  $(9s \times 14s)$  matrix with the following nonzero entries:

$$\begin{aligned}
b_{j-s,2s+(-2)s} &= -w_{8(j+m+1) \rightarrow 8(j+m+1)+6} \otimes w_{8j \rightarrow 8j+1}; \\
b_{j+4s,2s+(-2)s} &= -w_{8(j+m+1)+5 \rightarrow 8(j+m+1)+6} \otimes w_{8j \rightarrow 8j+6}; \\
b_{(j+1)s,3s+(-3)s} &= -e_{8(j+m+1)+7} \otimes w_{8j+1 \rightarrow 8(j+1)}; \\
b_{(j+1)s,7s+(-2)s} &= -e_{8(j+m+1)+7} \otimes w_{8j+5 \rightarrow 8(j+1)}; \\
b_{(j+1)s,7s+(-3)s} &= -e_{8(j+m+1)+7} \otimes w_{8j+5 \rightarrow 8(j+1)}; \\
b_{(j+1)s,9s+(-2)s} &= w_{8(j+m+1)+7 \rightarrow 8(j+m+2)} \otimes w_{8j+6 \rightarrow 8(j+1)}; \\
b_{(j+1)s,9s+(-3)s} &= w_{8(j+m+1)+7 \rightarrow 8(j+m+2)} \otimes w_{8j+6 \rightarrow 8(j+1)}; \\
b_{(j+1)s,10s+(-2)s} &= -w_{8(j+m+1)+7 \rightarrow 8(j+m+2)+3} \otimes w_{8j+7 \rightarrow 8(j+1)}; \\
b_{(j+1)s,10s+(-3)s} &= -w_{8(j+m+1)+7 \rightarrow 8(j+m+2)+3} \otimes w_{8j+7 \rightarrow 8(j+1)}.
\end{aligned}$$

(29) If  $r_0 = 28$ , then  $\Omega^{28}(Z_t^{(24)})$  is described with  $(8s \times 13s)$  matrix with the following nonzero entries:

$$\begin{aligned}
b_{j,s+(-2)s} &= w_{8(j+m)+1 \rightarrow 8(j+m)+7} \otimes w_{8j \rightarrow 8j+1}; \\
b_{j+s,s+(-2)s} &= -w_{8(j+m)+2 \rightarrow 8(j+m)+7} \otimes w_{8j \rightarrow 8j+2}; \\
b_{j+2s,s+(-2)s} &= w_{8(j+m)+3 \rightarrow 8(j+m)+7} \otimes w_{8j \rightarrow 8j+3}; \\
b_{j+3s,s+(-2)s} &= -w_{8(j+m)+4 \rightarrow 8(j+m)+7} \otimes w_{8j \rightarrow 8j+4}; \\
b_{j+5s,s+(-2)s} &= w_{8(j+m)+6 \rightarrow 8(j+m)+7} \otimes w_{8j \rightarrow 8j+6}; \\
b_{j+6s,s+(-2)s} &= -e_{8(j+m)+7} \otimes w_{8j \rightarrow 8j+7};
\end{aligned}$$

$$\begin{aligned}
b_{j+s, 2s+(-2)_s} &= -w_{8(j+m)+3 \rightarrow 8(j+m+1)+3} \otimes w_{8j+1 \rightarrow 8j+3}; \\
b_{j+2s, 2s+(-2)_s} &= w_{8(j+m)+4 \rightarrow 8(j+m+1)+3} \otimes w_{8j+1 \rightarrow 8j+4}; \\
b_{j+5s, 2s+(-2)_s} &= w_{8(j+m)+7 \rightarrow 8(j+m+1)+3} \otimes w_{8j+1 \rightarrow 8j+7}; \\
b_{j+s, 3s+(-2)_s} &= w_{8(j+m)+4 \rightarrow 8(j+m+1)+4} \otimes w_{8j+2 \rightarrow 8j+4}; \\
b_{j+4s, 3s+(-2)_s} &= w_{8(j+m)+7 \rightarrow 8(j+m+1)+4} \otimes w_{8j+2 \rightarrow 8j+7}; \\
b_{j+s, 3s+(-3)_s} &= w_{8(j+m)+4 \rightarrow 8(j+m+1)+4} \otimes w_{8j+2 \rightarrow 8j+4}; \\
b_{j+4s, 3s+(-3)_s} &= w_{8(j+m)+7 \rightarrow 8(j+m+1)+4} \otimes w_{8j+2 \rightarrow 8j+7}; \\
b_{(j+1)_s, 10s+(-2)_s} &= w_{8(j+m+1) \rightarrow 8(j+m+1)+6} \otimes w_{8j+6 \rightarrow 8(j+1)}; \\
b_{5s+(j+1)_s, 10s+(-2)_s} &= w_{8(j+m+1)+5 \rightarrow 8(j+m+1)+6} \otimes w_{8j+6 \rightarrow 8(j+1)+5}; \\
b_{6s+(j+1)_s, 10s+(-2)_s} &= -e_{8(j+m+1)+6} \otimes w_{8j+6 \rightarrow 8(j+1)+6}; \\
b_{(j+1)_s, 10s+(-3)_s} &= w_{8(j+m+1) \rightarrow 8(j+m+1)+6} \otimes w_{8j+6 \rightarrow 8(j+1)}; \\
b_{5s+(j+1)_s, 10s+(-3)_s} &= w_{8(j+m+1)+5 \rightarrow 8(j+m+1)+6} \otimes w_{8j+6 \rightarrow 8(j+1)+5}; \\
b_{j-4s, 11s+(-2)_s} &= -w_{8(j+m)+7 \rightarrow 8(j+m+1)+7} \otimes e_{8j+7}; \\
b_{s+(j+1)_s, 11s+(-3)_s} &= -w_{8(j+m+1)+1 \rightarrow 8(j+m+1)+7} \otimes w_{8j+7 \rightarrow 8(j+1)+1}; \\
b_{2s+(j+1)_s, 11s+(-3)_s} &= w_{8(j+m+1)+2 \rightarrow 8(j+m+1)+7} \otimes w_{8j+7 \rightarrow 8(j+1)+2}; \\
b_{3s+(j+1)_s, 11s+(-3)_s} &= -w_{8(j+m+1)+3 \rightarrow 8(j+m+1)+7} \otimes w_{8j+7 \rightarrow 8(j+1)+3}; \\
b_{4s+(j+1)_s, 11s+(-3)_s} &= w_{8(j+m+1)+4 \rightarrow 8(j+m+1)+7} \otimes w_{8j+7 \rightarrow 8(j+1)+4}; \\
b_{6s+(j+1)_s, 11s+(-3)_s} &= -w_{8(j+m+1)+6 \rightarrow 8(j+m+1)+7} \otimes w_{8j+7 \rightarrow 8(j+1)+6}; \\
b_{7s+(j+1)_s, 11s+(-3)_s} &= e_{8(j+m+1)+7} \otimes w_{8j+7 \rightarrow 8(j+1)+7}; \\
b_{j-4s, 11s+(-3)_s} &= -w_{8(j+m)+7 \rightarrow 8(j+m+1)+7} \otimes e_{8j+7}.
\end{aligned}$$

(II) Represent an arbitrary  $t_0 \in \mathbb{N}$  in the form  $t_0 = 29\ell_0 + r_0$ , where  $0 \leq r_0 \leq 28$ . Then  $\Omega^{t_0}(Z_t^{(24)})$  is a  $\Omega^{r_0}(Z_t^{(24)})$ , whose left components twisted by  $\sigma^{\ell_0}$ .

**Proposition 20** (Translates for the case 25). (I) Let  $r_0 \in \mathbb{N}$ ,  $r_0 < 29$ .  $r_0$ -translates of the elements  $Z_t^{(25)}$  are described by the following way.

(1) If  $r_0 = 0$ , then  $\Omega^0(Z_t^{(25)})$  is described with  $(8s \times 11s)$  matrix, whose entries  $b_{ij}$  have the following form:

If  $0 \leq j < s$ , then

$$b_{ij} = \begin{cases} e_{8(j+m)} \otimes e_{8j}, & i = j; \\ 0, & \text{otherwise.} \end{cases}$$

If  $s \leq j < 2s$ , then

$$b_{ij} = \begin{cases} w_{8(j+m)+1 \rightarrow 8(j+m)+4} \otimes e_{8j+1}, & i = j; \\ 0, & \text{otherwise.} \end{cases}$$

If  $2s \leq j < 7s$ , then  $b_{ij} = 0$ .

If  $7s \leq j < 8s$ , then

$$b_{ij} = \begin{cases} -w_{8(j+m)+5 \rightarrow 8(j+m)+6} \otimes e_{8j+5}, & i = j - 2s; \\ 0, & \text{otherwise.} \end{cases}$$

If  $8s \leq j < 10s$ , then  $b_{ij} = 0$ .

If  $10s \leq j < 11s$ , then

$$b_{ij} = \begin{cases} -e_{8(j+m)+7} \otimes e_{8j+7}, & i = j - 3s; \\ 0, & \text{otherwise.} \end{cases}$$

(2) If  $r_0 = 1$ , then  $\Omega^1(Z_t^{(25)})$  is described with  $(9s \times 10s)$  matrix, whose entries  $b_{ij}$  have the following form:

If  $0 \leq j < s$ , then

$$b_{ij} = \begin{cases} w_{8(j+m)+1 \rightarrow 8(j+m)+4} \otimes e_{8j}, & i = j; \\ 0, & \text{otherwise.} \end{cases}$$

If  $s \leq j < 2s$ , then

$$b_{ij} = \begin{cases} w_{8(j+m)+5 \rightarrow 8(j+m)+6} \otimes e_{8j}, & i = j; \\ 0, & \text{otherwise.} \end{cases}$$

If  $2s \leq j < 3s$ , then

$$b_{ij} = \begin{cases} w_{8(j+m)+2 \rightarrow 8(j+m)+7} \otimes e_{8j+1}, & i = j; \\ w_{8(j+m)+3 \rightarrow 8(j+m)+7} \otimes w_{8j+1 \rightarrow 8j+2}, & i = j + s; \\ w_{8(j+m)+4 \rightarrow 8(j+m)+7} \otimes w_{8j+1 \rightarrow 8j+3}, & i = j + 2s; \\ e_{8(j+m)+7} \otimes w_{8j+1 \rightarrow 8j+4}, & i = j + 3s; \\ 0, & \text{otherwise.} \end{cases}$$

If  $3s \leq j < 4s$ , then

$$b_{ij} = \begin{cases} e_{8(j+m)+1} \otimes w_{8j+2 \rightarrow 8j+7}, & i = j + 5s; \\ 0, & \text{otherwise.} \end{cases}$$

If  $4s \leq j < 5s$ , then

$$b_{ij} = \begin{cases} -w_{8(j+m)+1 \rightarrow 8(j+m)+1} \otimes w_{8j+3 \rightarrow 8j+7}, & i = j + 4s; \\ 0, & \text{otherwise.} \end{cases}$$

If  $5s \leq j < 6s$ , then

$$b_{ij} = \begin{cases} w_{8(j+m)+1 \rightarrow 8(j+m)+2} \otimes w_{8j+4 \rightarrow 8j+7}, & i = j + 3s; \\ 0, & \text{otherwise.} \end{cases}$$

If  $6s \leq j < 7s$ , then

$$b_{ij} = \begin{cases} w_{8(j+m)+6 \rightarrow 8(j+m)+7} \otimes e_{8j+5}, & i = j; \\ e_{8(j+m)+7} \otimes w_{8j+5 \rightarrow 8j+6}, & i = j + s; \\ 0, & \text{otherwise.} \end{cases}$$

If  $7s \leq j < 8s$ , then  $b_{ij} = 0$ .

If  $8s \leq j < 9s$ , then

$$b_{ij} = \begin{cases} w_{8(j+m)+1 \rightarrow 8(j+m)+3} \otimes e_{8j+7}, & i = j; \\ 0, & \text{otherwise.} \end{cases}$$

If  $9s \leq j < 10s$ , then  $b_{ij} = 0$ .

(3) If  $r_0 = 2$ , then  $\Omega^2(Z_t^{(25)})$  is described with  $(8s \times 8s)$  matrix, whose entries  $b_{ij}$  have the following form:

If  $0 \leq j < s$ , then

$$b_{ij} = \begin{cases} e_{8(j+m-1)+7} \otimes e_{8j}, & i = j; \\ 0, & \text{otherwise.} \end{cases}$$

If  $s \leq j < 2s$ , then

$$b_{ij} = \begin{cases} w_{8(j+m)+5 \rightarrow 8(j+m)+6} \otimes w_{8j+1 \rightarrow 8j+4}, & i = j + 3s; \\ 0, & \text{otherwise.} \end{cases}$$

If  $2s \leq j < 5s$ , then  $b_{ij} = 0$ .

If  $5s \leq j < 6s$ , then

$$b_{ij} = \begin{cases} w_{8(j+m)+1 \rightarrow 8(j+m)+4} \otimes w_{8j+5 \rightarrow 8j+6}, & i = j + s; \\ 0, & \text{otherwise.} \end{cases}$$

If  $6s \leq j < 7s$ , then  $b_{ij} = 0$ .

If  $7s \leq j < 8s$ , then

$$b_{ij} = \begin{cases} e_{8(j+m+1)} \otimes e_{8j+7}, & i = j; \\ 0, & \text{otherwise.} \end{cases}$$

(4) If  $r_0 = 3$ , then  $\Omega^3(Z_t^{(25)})$  is described with  $(10s \times 9s)$  matrix, whose entries  $b_{ij}$  have the following form:

If  $0 \leq j < s$ , then

$$b_{ij} = \begin{cases} w_{8(j+m)+2 \rightarrow 8(j+m)+7} \otimes e_{8j}, & i = j; \\ w_{8(j+m)+3 \rightarrow 8(j+m)+7} \otimes w_{8j \rightarrow 8j+1}, & i = j + 2s; \\ w_{8(j+m)+4 \rightarrow 8(j+m)+7} \otimes w_{8j \rightarrow 8j+2}, & i = j + 3s; \\ e_{8(j+m)+7} \otimes w_{8j \rightarrow 8j+3}, & i = j + 4s; \\ 0, & \text{otherwise.} \end{cases}$$

If  $s \leq j < 2s$ , then

$$b_{ij} = \begin{cases} e_{8(j+m+1)} \otimes w_{8j+1 \rightarrow 8j+4}, & i = j + 4s; \\ 0, & \text{otherwise.} \end{cases}$$

If  $2s \leq j < 3s$ , then

$$b_{ij} = \begin{cases} -w_{8(j+m+1) \rightarrow 8(j+m+1)+1} \otimes w_{8j+2 \rightarrow 8j+4}, & i = j + 3s; \\ 0, & \text{otherwise.} \end{cases}$$

If  $3s \leq j < 4s$ , then

$$b_{ij} = \begin{cases} w_{8(j+m+1) \rightarrow 8(j+m+1)+2} \otimes w_{8j+3 \rightarrow 8j+4}, & i = j + 2s; \\ 0, & \text{otherwise.} \end{cases}$$

If  $4s \leq j < 5s$ , then

$$b_{ij} = \begin{cases} -w_{8(j+m+1) \rightarrow 8(j+m+1)+3} \otimes e_{8j+4}, & i = j + s; \\ 0, & \text{otherwise.} \end{cases}$$

If  $5s \leq j < 6s$ , then

$$b_{ij} = \begin{cases} e_{8(j+m+1)} \otimes w_{8j+5 \rightarrow 8j+6}, & i = j + 2s; \\ 0, & \text{otherwise.} \end{cases}$$

If  $6s \leq j < 7s$ , then

$$b_{ij} = \begin{cases} -w_{8(j+m+1) \rightarrow 8(j+m+1)+5} \otimes e_{8j+6}, & i = j + s; \\ 0, & \text{otherwise.} \end{cases}$$

If  $7s \leq j < 8s$ , then

$$b_{ij} = \begin{cases} w_{8(j+m+1)+1 \rightarrow 8(j+m+1)+4} \otimes e_{8j+7}, & i = j + s; \\ 0, & \text{otherwise.} \end{cases}$$

If  $8s \leq j < 9s$ , then

$$b_{ij} = \begin{cases} w_{8(j+m+1)+5 \rightarrow 8(j+m+1)+6} \otimes e_{8j+7}, & i = j + s; \\ 0, & \text{otherwise.} \end{cases}$$

(5) If  $r_0 = 4$ , then  $\Omega^4(Z_t^{(25)})$  is described with  $(11s \times 8s)$  matrix, whose entries  $b_{ij}$  have the following form:

If  $0 \leq j < s$ , then

$$b_{ij} = \begin{cases} w_{8(j+m-1)+7 \rightarrow 8(j+m)} \otimes e_{8j}, & i = j; \\ e_{8(j+m)} \otimes e_{8j}, & i = j + s; \\ 0, & \text{otherwise.} \end{cases}$$

If  $s \leq j < 4s$ , then  $b_{ij} = 0$ .

If  $4s \leq j < 5s$ , then

$$b_{ij} = \begin{cases} -w_{8(j+m)+1 \rightarrow 8(j+m)+4} \otimes e_{8j+4}, & i = j + 2s; \\ 0, & \text{otherwise.} \end{cases}$$

If  $5s \leq j < 6s$ , then  $b_{ij} = 0$ .

If  $6s \leq j < 7s$ , then

$$b_{ij} = \begin{cases} -w_{8(j+m)+5 \rightarrow 8(j+m)+6} \otimes e_{8j+6}, & i = j + 3s; \\ 0, & \text{otherwise.} \end{cases}$$

If  $7s \leq j < 8s$ , then

$$b_{ij} = \begin{cases} e_{8(j+m)+7} \otimes e_{8j+7}, & i = j + 3s; \\ 0, & \text{otherwise.} \end{cases}$$

(6) If  $r_0 = 5$ , then  $\Omega^5(Z_t^{(25)})$  is described with  $(11s \times 8s)$  matrix, whose entries  $b_{ij}$  have the following form:

If  $0 \leq j < s$ , then

$$b_{ij} = \begin{cases} w_{8(j+m)+5 \rightarrow 8(j+m+1)} \otimes e_{8j}, & i = j; \\ e_{8(j+m+1)} \otimes w_{8j \rightarrow 8j+3}, & i = j + 5s; \\ w_{8(j+m)+7 \rightarrow 8(j+m+1)} \otimes w_{8j \rightarrow 8j+4}, & i = j + 6s; \\ 0, & \text{otherwise.} \end{cases}$$

If  $s \leq j < 2s$ , then

$$b_{ij} = \begin{cases} e_{8(j+m+1)+1} \otimes w_{8j+1 \rightarrow 8(j+1)}, & i = 2s + (j+1)_s; \\ -w_{8(j+m)+7 \rightarrow 8(j+m+1)+1} \otimes w_{8j+1 \rightarrow 8j+4}, & i = j + 5s; \\ 0, & \text{otherwise.} \end{cases}$$

If  $2s \leq j < 3s$ , then

$$b_{ij} = \begin{cases} -w_{8(j+m+1)+1 \rightarrow 8(j+m+1)+2} \otimes w_{8j+2 \rightarrow 8(j+1)}, & i = 2s + (j+1)_s; \\ w_{8(j+m)+7 \rightarrow 8(j+m+1)+2} \otimes w_{8j+2 \rightarrow 8j+4}, & i = j + 4s; \\ 0, & \text{otherwise.} \end{cases}$$

If  $3s \leq j < 4s$ , then

$$b_{ij} = \begin{cases} w_{8(j+m+1)+1 \rightarrow 8(j+m+1)+3} \otimes w_{8j+3 \rightarrow 8(j+1)}, & i = 2s + (j+1)_s; \\ -w_{8(j+m)+7 \rightarrow 8(j+m+1)+3} \otimes w_{8j+3 \rightarrow 8j+4}, & i = j + 3s; \\ 0, & \text{otherwise.} \end{cases}$$

If  $4s \leq j < 5s$ , then

$$b_{ij} = \begin{cases} -w_{8(j+m+1)+1 \rightarrow 8(j+m+1)+4} \otimes w_{8j+4 \rightarrow 8(j+1)}, & i = 2s + (j+1)_s; \\ w_{8(j+m)+7 \rightarrow 8(j+m+1)+4} \otimes e_{8j+4}, & i = j + 2s; \\ 0, & \text{otherwise.} \end{cases}$$

If  $5s \leq j < 6s$ , then

$$b_{ij} = \begin{cases} -e_{8(j+m+1)+5} \otimes w_{8j+5 \rightarrow 8(j+1)}, & i = (j+1)_s; \\ -w_{8(j+m)+7 \rightarrow 8(j+m+1)+5} \otimes w_{8j+5 \rightarrow 8j+6}, & i = j + 3s; \\ 0, & \text{otherwise.} \end{cases}$$

If  $6s \leq j < 7s$ , then

$$b_{ij} = \begin{cases} w_{8(j+m+1)+5 \rightarrow 8(j+m+1)+6} \otimes w_{8j+6 \rightarrow 8(j+1)}, & i = (j+1)_s; \\ w_{8(j+m)+7 \rightarrow 8(j+m+1)+6} \otimes e_{8j+6}, & i = j + 2s; \\ 0, & \text{otherwise.} \end{cases}$$

If  $7s \leq j < 8s$ , then

$$b_{ij} = \begin{cases} -w_{8(j+m+1)+5 \rightarrow 8(j+m+1)+7} \otimes w_{8j+7 \rightarrow 8(j+1)}, & i = (j+1)_s; \\ w_{8(j+m+1)+3 \rightarrow 8(j+m+1)+7} \otimes w_{8j+7 \rightarrow 8(j+1)}, & i = s + (j+1)_s; \\ w_{8(j+m+1)+1 \rightarrow 8(j+m+1)+7} \otimes w_{8j+7 \rightarrow 8(j+1)}, & i = 2s + (j+1)_s; \\ w_{8(j+m+1)+4 \rightarrow 8(j+m+1)+7} \otimes w_{8j+7 \rightarrow 8(j+1)+1}, & i = 3s + (j+1)_s; \\ e_{8(j+m+1)+7} \otimes w_{8j+7 \rightarrow 8(j+1)+2}, & i = 4s + (j+1)_s; \\ -e_{8(j+m+1)+7} \otimes w_{8j+7 \rightarrow 8(j+1)+4}, & i = 6s + (j+1)_s; \\ w_{8(j+m+1)+2 \rightarrow 8(j+m+1)+7} \otimes e_{8j+7}, & i = j + 2s; \\ 0, & \text{otherwise.} \end{cases}$$

(7) If  $r_0 = 6$ , then  $\Omega^6(Z_t^{(25)})$  is described with  $(13s \times 9s)$  matrix, whose entries  $b_{ij}$  have the following form:



If  $0 \leq j < s$ , then

$$b_{ij} = \begin{cases} -e_{8(j+m)+1} \otimes w_{8j \rightarrow 8j+3}, & i = j + 5s; \\ 0, & \text{otherwise.} \end{cases}$$

If  $s \leq j < 2s$ , then

$$b_{ij} = \begin{cases} w_{8(j+m-1)+7 \rightarrow 8(j+m)+5} \otimes e_{8j}, & i = j - s; \\ e_{8(j+m)+5} \otimes w_{8j \rightarrow 8j+2}, & i = j + 2s; \\ 0, & \text{otherwise.} \end{cases}$$

If  $2s \leq j < 5s$ , then  $b_{ij} = 0$ .

If  $5s \leq j < 6s$ , then

$$b_{ij} = \begin{cases} e_{8(j+m)+7} \otimes w_{8j+4 \rightarrow 8(j+1)}, & i = (j + 1)_s; \\ w_{8(j+m)+2 \rightarrow 8(j+m)+7} \otimes e_{8j+4}, & i = j + s; \\ 0, & \text{otherwise.} \end{cases}$$

If  $6s \leq j < 7s$ , then  $b_{ij} = 0$ .

If  $7s \leq j < 8s$ , then

$$b_{ij} = \begin{cases} -w_{8(j+m)+3 \rightarrow 8(j+m)+7} \otimes e_{8j+6}, & i = j + 2s; \\ 0, & \text{otherwise.} \end{cases}$$

If  $8s \leq j < 9s$ , then

$$b_{ij} = \begin{cases} -w_{8(j+m)+7 \rightarrow 8(j+m+1)} \otimes e_{8j+7}, & i = j + 3s; \\ -e_{8(j+m+1)} \otimes e_{8j+7}, & i = j + 4s; \\ 0, & \text{otherwise.} \end{cases}$$

(8) If  $r_0 = 7$ , then  $\Omega^7(Z_t^{(25)})$  is described with  $(14s \times 8s)$  matrix, whose entries  $b_{ij}$  have the following form:

If  $0 \leq j < s$ , then

$$b_{ij} = \begin{cases} -w_{8(j+m)+2 \rightarrow 8(j+m)+7} \otimes e_{8j}, & i = j; \\ w_{8(j+m)+4 \rightarrow 8(j+m)+7} \otimes e_{8j}, & i = j + s; \\ e_{8(j+m)+7} \otimes w_{8j \rightarrow 8j+1}, & i = j + 4s; \\ 0, & \text{otherwise.} \end{cases}$$

If  $s \leq j < 2s$ , then

$$b_{ij} = \begin{cases} -e_{8(j+m+1)+2} \otimes w_{8j+1 \rightarrow 8(j+1)}, & i = (j + 1)_s; \\ -w_{8(j+m+1) \rightarrow 8(j+m+1)+2} \otimes w_{8j+1 \rightarrow 8j+4}, & i = j + 6s; \\ 0, & \text{otherwise.} \end{cases}$$

If  $2s \leq j < 3s$ , then

$$b_{ij} = \begin{cases} w_{8(j+m+1)+2 \rightarrow 8(j+m+1)+3} \otimes w_{8j+2 \rightarrow 8(j+1)}, & i = (j + 1)_s; \\ w_{8(j+m+1) \rightarrow 8(j+m+1)+3} \otimes w_{8j+2 \rightarrow 8j+4}, & i = j + 5s; \\ 0, & \text{otherwise.} \end{cases}$$

If  $3s \leq j < 4s$ , then

$$b_{ij} = \begin{cases} -w_{8(j+m+1)+2 \rightarrow 8(j+m+1)+4} \otimes w_{8j+3 \rightarrow 8(j+1)}, & i = (j+1)s; \\ -w_{8(j+m+1) \rightarrow 8(j+m+1)+4} \otimes w_{8j+3 \rightarrow 8j+4}, & i = j+4s; \\ 0, & \text{otherwise.} \end{cases}$$

If  $4s \leq j < 5s$ , then

$$b_{ij} = \begin{cases} -e_{8(j+m+1)+5} \otimes w_{8j+4 \rightarrow 8(j+1)}, & i = 3s + (j+1)s; \\ -w_{8(j+m+1) \rightarrow 8(j+m+1)+5} \otimes e_{8j+4}, & i = j+3s; \\ 0, & \text{otherwise.} \end{cases}$$

If  $5s \leq j < 6s$ , then

$$b_{ij} = \begin{cases} -e_{8(j+m+1)+6} \otimes w_{8j+5 \rightarrow 8(j+1)}, & i = 2s + (j+1)s; \\ -w_{8(j+m)+7 \rightarrow 8(j+m+1)+6} \otimes w_{8j+5 \rightarrow 8j+6}, & i = j+4s; \\ -w_{8(j+m+1) \rightarrow 8(j+m+1)+6} \otimes w_{8j+5 \rightarrow 8j+6}, & i = j+5s; \\ 0, & \text{otherwise.} \end{cases}$$

If  $6s \leq j < 7s$ , then

$$b_{ij} = \begin{cases} -w_{8(j+m)+7 \rightarrow 8(j+m+1)+1} \otimes e_{8j+6}, & i = j+3s; \\ -w_{8(j+m+1) \rightarrow 8(j+m+1)+1} \otimes e_{8j+6}, & i = j+4s; \\ 0, & \text{otherwise.} \end{cases}$$

If  $7s \leq j < 8s$ , then

$$b_{ij} = \begin{cases} e_{8(j+m+2)} \otimes w_{8j+7 \rightarrow 8(j+1)+2}, & i = 5s + (j+1)s; \\ -e_{8(j+m+2)} \otimes w_{8j+7 \rightarrow 8(j+1)+4}, & i = 7s + (j+1)s; \\ w_{8(j+m+1)+5 \rightarrow 8(j+m+2)} \otimes e_{8j+7}, & i = j+4s; \\ 0, & \text{otherwise.} \end{cases}$$

(9) If  $r_0 = 8$ , then  $\Omega^8(Z_t^{(25)})$  is described with  $(16s \times 10s)$  matrix, whose entries  $b_{ij}$  have the following form:

If  $0 \leq j < s$ , then

$$b_{ij} = \begin{cases} w_{8(j+m-1)+7 \rightarrow 8(j+m)+2} \otimes e_{8j}, & i = j; \\ -w_{8(j+m-1)+7 \rightarrow 8(j+m)+2} \otimes e_{8j}, & i = j+s; \\ w_{8(j+m) \rightarrow 8(j+m)+2} \otimes e_{8j}, & i = j+2s; \\ w_{8(j+m)+1 \rightarrow 8(j+m)+2} \otimes w_{8j \rightarrow 8j+2}, & i = j+5s; \\ e_{8(j+m)+2} \otimes w_{8j \rightarrow 8j+3}, & i = j+6s; \\ 0, & \text{otherwise.} \end{cases}$$

If  $s \leq j < 2s$ , then

$$b_{ij} = \begin{cases} -w_{8(j+m-1)+7 \rightarrow 8(j+m)+6} \otimes e_{8j}, & i = j - s; \\ w_{8(j+m-1)+7 \rightarrow 8(j+m)+6} \otimes e_{8j}, & i = j; \\ -w_{8(j+m) \rightarrow 8(j+m)+6} \otimes e_{8j}, & i = j + s; \\ -e_{8(j+m)+6} \otimes w_{8j \rightarrow 8j+2}, & i = j + 3s; \\ 0, & \text{otherwise.} \end{cases}$$

If  $2s \leq j < 4s$ , then  $b_{ij} = 0$ .

If  $4s \leq j < 5s$ , then

$$b_{ij} = \begin{cases} -e_{8(j+m)+7} \otimes w_{8j+3 \rightarrow 8(j+1)}, & i = s + (j+1)_s; \\ 0, & \text{otherwise.} \end{cases}$$

If  $5s \leq j < 6s$ , then

$$b_{ij} = \begin{cases} w_{8(j+m)+7 \rightarrow 8(j+m+1)} \otimes w_{8j+4 \rightarrow 8(j+1)}, & i = (j+1)_s; \\ -w_{8(j+m)+7 \rightarrow 8(j+m+1)} \otimes w_{8j+4 \rightarrow 8(j+1)}, & i = s + (j+1)_s; \\ e_{8(j+m+1)} \otimes w_{8j+4 \rightarrow 8(j+1)}, & i = 2s + (j+1)_s; \\ w_{8(j+m)+5 \rightarrow 8(j+m+1)} \otimes e_{8j+4}, & i = j + 3s; \\ 0, & \text{otherwise.} \end{cases}$$

If  $6s \leq j < 7s$ , then

$$b_{ij} = \begin{cases} -e_{8(j+m)+7} \otimes w_{8j+5 \rightarrow 8(j+1)}, & i = (j+1)_s; \\ e_{8(j+m)+7} \otimes w_{8j+5 \rightarrow 8(j+1)}, & i = s + (j+1)_s; \\ 0, & \text{otherwise.} \end{cases}$$

If  $7s \leq j < 8s$ , then

$$b_{ij} = \begin{cases} -w_{8(j+m)+5 \rightarrow 8(j+m+1)} \otimes e_{8j+6}, & i = j + 4s; \\ 0, & \text{otherwise.} \end{cases}$$

If  $8s \leq j < 9s$ , then

$$b_{ij} = \begin{cases} w_{8(j+m)+7 \rightarrow 8(j+m+1)+1} \otimes w_{8j+7 \rightarrow 8(j+1)}, & i = (j+1)_s; \\ -w_{8(j+m)+7 \rightarrow 8(j+m+1)+1} \otimes w_{8j+7 \rightarrow 8(j+1)}, & i = s + (j+1)_s; \\ w_{8(j+m+1) \rightarrow 8(j+m+1)+1} \otimes w_{8j+7 \rightarrow 8(j+1)}, & i = 2s + (j+1)_s; \\ 0, & \text{otherwise.} \end{cases}$$

If  $9s \leq j < 10s$ , then

$$b_{ij} = \begin{cases} e_{8(j+m+1)+5} \otimes w_{8j+7 \rightarrow 8(j+1)+1}, & i = 3s + (j+1)_s; \\ w_{8(j+m)+7 \rightarrow 8(j+m+1)+5} \otimes e_{8j+7}, & i = j + 5s; \\ 0, & \text{otherwise.} \end{cases}$$

(10) If  $r_0 = 9$ , then  $\Omega^9(Z_t^{(25)})$  is described with  $(16s \times 11s)$  matrix, whose entries  $b_{ij}$  have the following form:

If  $0 \leq j < s$ , then

$$b_{ij} = \begin{cases} -e_{8(j+m)+7} \otimes w_{8j \rightarrow 8j+2}, & i = j + 5s; \\ 0, & \text{otherwise.} \end{cases}$$

If  $s \leq j < 2s$ , then

$$b_{ij} = \begin{cases} -w_{8(j+m)+5 \rightarrow 8(j+m+1)} \otimes e_{8j}, & i = j - s; \\ e_{8(j+m+1)} \otimes w_{8j \rightarrow 8j+1}, & i = j + 3s; \\ 0, & \text{otherwise.} \end{cases}$$

If  $2s \leq j < 3s$ , then

$$b_{ij} = \begin{cases} -e_{8(j+m+1)+3} \otimes w_{8j+1 \rightarrow 8(j+1)}, & i = s + (j + 1)_s; \\ -w_{8(j+m+1)+1 \rightarrow 8(j+m+1)+3} \otimes w_{8j+1 \rightarrow 8(j+1)}, & i = 3s + (j + 1)_s; \\ 0, & \text{otherwise.} \end{cases}$$

If  $3s \leq j < 4s$ , then

$$b_{ij} = \begin{cases} w_{8(j+m+1)+3 \rightarrow 8(j+m+1)+4} \otimes w_{8j+2 \rightarrow 8(j+1)}, & i = s + (j + 1)_s; \\ w_{8(j+m+1)+1 \rightarrow 8(j+m+1)+4} \otimes w_{8j+2 \rightarrow 8(j+1)}, & i = 3s + (j + 1)_s; \\ 0, & \text{otherwise.} \end{cases}$$

If  $4s \leq j < 5s$ , then

$$b_{ij} = \begin{cases} e_{8(j+m+1)+5} \otimes w_{8j+3 \rightarrow 8(j+1)}, & i = (j + 1)_s; \\ -w_{8(j+m)+7 \rightarrow 8(j+m+1)+5} \otimes w_{8j+3 \rightarrow 8j+4}, & i = j + 3s; \\ 0, & \text{otherwise.} \end{cases}$$

If  $5s \leq j < 6s$ , then

$$b_{ij} = \begin{cases} e_{8(j+m+1)+6} \otimes w_{8j+4 \rightarrow 8(j+1)}, & i = 2s + (j + 1)_s; \\ w_{8(j+m)+7 \rightarrow 8(j+m+1)+6} \otimes e_{8j+4}, & i = j + 2s; \\ 0, & \text{otherwise.} \end{cases}$$

If  $6s \leq j < 7s$ , then  $b_{ij} = 0$ .

If  $7s \leq j < 8s$ , then

$$b_{ij} = \begin{cases} e_{8(j+m+1)+1} \otimes w_{8j+5 \rightarrow 8(j+1)}, & i = 3s + (j + 1)_s; \\ 0, & \text{otherwise.} \end{cases}$$

If  $8s \leq j < 9s$ , then  $b_{ij} = 0$ .

If  $9s \leq j < 10s$ , then

$$b_{ij} = \begin{cases} -w_{8(j+m)+7 \rightarrow 8(j+m+1)+5} \otimes e_{8j+6}, & i = j + s; \\ 0, & \text{otherwise.} \end{cases}$$

If  $10s \leq j < 11s$ , then

$$b_{ij} = \begin{cases} -w_{8(j+m+1)+3 \rightarrow 8(j+m+1)+7} \otimes w_{8j+7 \rightarrow 8(j+1)}, & i = s + (j+1)_s; \\ w_{8(j+m+1)+6 \rightarrow 8(j+m+1)+7} \otimes w_{8j+7 \rightarrow 8(j+1)}, & i = 2s + (j+1)_s; \\ -e_{8(j+m+1)+7} \otimes w_{8j+7 \rightarrow 8(j+1)+2}, & i = 5s + (j+1)_s; \\ -e_{8(j+m+1)+7} \otimes w_{8j+7 \rightarrow 8(j+1)+5}, & i = 8s + (j+1)_s; \\ -w_{8(j+m+1)+2 \rightarrow 8(j+m+1)+7} \otimes e_{8j+7}, & i = j + 2s; \\ w_{8(j+m+1)+4 \rightarrow 8(j+m+1)+7} \otimes e_{8j+7}, & i = j + 3s; \\ 0, & \text{otherwise.} \end{cases}$$

(11) If  $r_0 = 10$ , then  $\Omega^{10}(Z_t^{(25)})$  is described with  $(19s \times 11s)$  matrix, whose entries  $b_{ij}$  have the following form:

If  $0 \leq j < s$ , then

$$b_{ij} = \begin{cases} -w_{8(j+m-1)+7 \rightarrow 8(j+m)+5} \otimes e_{8j}, & i = j; \\ w_{8(j+m) \rightarrow 8(j+m)+5} \otimes e_{8j}, & i = j + 2s; \\ -e_{8(j+m)+5} \otimes w_{8j \rightarrow 8j+5}, & i = j + 10s; \\ 0, & \text{otherwise.} \end{cases}$$

If  $s \leq j < 2s$ , then

$$b_{ij} = \begin{cases} -w_{8(j+m)+2 \rightarrow 8(j+m)+3} \otimes w_{8j \rightarrow 8j+2}, & i = j + 4s; \\ e_{8(j+m)+3} \otimes w_{8j \rightarrow 8j+3}, & i = j + 5s; \\ 0, & \text{otherwise.} \end{cases}$$

If  $2s \leq j < 3s$ , then

$$b_{ij} = \begin{cases} -e_{8(j+m)+1} \otimes w_{8j \rightarrow 8j+1}, & i = j + 2s; \\ 0, & \text{otherwise.} \end{cases}$$

If  $3s \leq j < 4s$ , then  $b_{ij} = 0$ .

If  $4s \leq j < 5s$ , then

$$b_{ij} = \begin{cases} -e_{8(j+m)+7} \otimes w_{8j+2 \rightarrow 8(j+1)}, & i = (j+1)_s; \\ 0, & \text{otherwise.} \end{cases}$$

If  $5s \leq j < 6s$ , then

$$b_{ij} = \begin{cases} -e_{8(j+m+1)} \otimes w_{8j+3 \rightarrow 8(j+1)}, & i = 2s + (j+1)_s; \\ 0, & \text{otherwise.} \end{cases}$$

If  $6s \leq j < 7s$ , then

$$b_{ij} = \begin{cases} -w_{8(j+m)+4 \rightarrow 8(j+m)+7} \otimes e_{8j+4}, & i = j + 2s; \\ 0, & \text{otherwise.} \end{cases}$$

If  $7s \leq j < 8s$ , then

$$b_{ij} = \begin{cases} -w_{8(j+m)+7 \rightarrow 8(j+m+1)} \otimes w_{8j+5 \rightarrow 8(j+1)}, & i = (j+1)_s; \\ -e_{8(j+m+1)} \otimes w_{8j+5 \rightarrow 8(j+1)}, & i = s + (j+1)_s; \\ e_{8(j+m+1)} \otimes w_{8j+5 \rightarrow 8(j+1)}, & i = 2s + (j+1)_s; \\ 0, & \text{otherwise.} \end{cases}$$

If  $8s \leq j < 9s$ , then

$$b_{ij} = \begin{cases} w_{8(j+m)+2 \rightarrow 8(j+m)+7} \otimes e_{8j+6}, & i = j + 5s; \\ -w_{8(j+m)+5 \rightarrow 8(j+m)+7} \otimes e_{8j+6}, & i = j + 7s; \\ -e_{8(j+m)+7} \otimes w_{8j+6 \rightarrow 8j+7}, & i = j + 9s; \\ 0, & \text{otherwise.} \end{cases}$$

If  $9s \leq j < 10s$ , then

$$b_{ij} = \begin{cases} -w_{8(j+m+1)+1 \rightarrow 8(j+m+1)+2} \otimes w_{8j+7 \rightarrow 8(j+1)+1}, & i = 4s + (j+1)_s; \\ w_{8(j+m)+7 \rightarrow 8(j+m+1)+2} \otimes e_{8j+7}, & i = j + 7s; \\ -w_{8(j+m)+7 \rightarrow 8(j+m+1)+2} \otimes e_{8j+7}, & i = j + 8s; \\ 0, & \text{otherwise.} \end{cases}$$

If  $10s \leq j < 11s$ , then

$$b_{ij} = \begin{cases} w_{8(j+m+1) \rightarrow 8(j+m+1)+6} \otimes w_{8j+7 \rightarrow 8(j+1)}, & i = 2s + (j+1)_s; \\ -e_{8(j+m+1)+6} \otimes w_{8j+7 \rightarrow 8(j+1)+1}, & i = 3s + (j+1)_s; \\ -w_{8(j+m+1)+5 \rightarrow 8(j+m+1)+6} \otimes w_{8j+7 \rightarrow 8(j+1)+5}, & i = 10s + (j+1)_s; \\ 0, & \text{otherwise.} \end{cases}$$

(12) If  $r_0 = 11$ , then  $\Omega^{11}(Z_t^{(25)})$  is described with  $(18s \times 13s)$  matrix, whose entries  $b_{ij}$  have the following form:

If  $0 \leq j < s$ , then

$$b_{ij} = \begin{cases} -w_{8(j+m)+2 \rightarrow 8(j+m)+7} \otimes e_{8j}, & i = j; \\ w_{8(j+m)+1 \rightarrow 8(j+m)+7} \otimes e_{8j}, & i = j + 3s; \\ w_{8(j+m)+5 \rightarrow 8(j+m)+7} \otimes e_{8j}, & i = j + 4s; \\ e_{8(j+m)+7} \otimes w_{8j \rightarrow 8j+3}, & i = j + 7s; \\ -e_{8(j+m)+7} \otimes w_{8j \rightarrow 8j+4}, & i = j + 8s; \\ 0, & \text{otherwise.} \end{cases}$$

If  $s \leq j < 2s$ , then

$$b_{ij} = \begin{cases} -e_{8(j+m+1)} \otimes w_{8j \rightarrow 8j+2}, & i = j + 5s; \\ 0, & \text{otherwise.} \end{cases}$$

If  $2s \leq j < 3s$ , then

$$b_{ij} = \begin{cases} w_{8(j+m+1)+2 \rightarrow 8(j+m+1)+4} \otimes w_{8j+1 \rightarrow 8(j+1)}, & i = (j+1)_s; \\ -e_{8(j+m+1)+4} \otimes w_{8j+1 \rightarrow 8(j+1)}, & i = 2s + (j+1)_s; \\ 0, & \text{otherwise.} \end{cases}$$

If  $3s \leq j < 4s$ , then  $b_{ij} = 0$ .

If  $4s \leq j < 5s$ , then

$$b_{ij} = \begin{cases} e_{8(j+m+1)+6} \otimes w_{8j+3 \rightarrow 8(j+1)}, & i = s + (j+1)_s; \\ 0, & \text{otherwise.} \end{cases}$$

If  $5s \leq j < 6s$ , then

$$b_{ij} = \begin{cases} e_{8(j+m+1)+1} \otimes w_{8j+3 \rightarrow 8(j+1)}, & i = 3s + (j+1)_s; \\ 0, & \text{otherwise.} \end{cases}$$

If  $6s \leq j < 7s$ , then

$$b_{ij} = \begin{cases} w_{8(j+m)+7 \rightarrow 8(j+m+1)+2} \otimes e_{8j+4}, & i = j + 2s; \\ 0, & \text{otherwise.} \end{cases}$$

If  $7s \leq j < 8s$ , then

$$b_{ij} = \begin{cases} -e_{8(j+m+1)+2} \otimes w_{8j+5 \rightarrow 8(j+1)}, & i = (j+1)_s; \\ w_{8(j+m+1)+1 \rightarrow 8(j+m+1)+2} \otimes w_{8j+5 \rightarrow 8(j+1)}, & i = 3s + (j+1)_s; \\ -w_{8(j+m)+7 \rightarrow 8(j+m+1)+2} \otimes w_{8j+5 \rightarrow 8j+6}, & i = j + 5s; \\ 0, & \text{otherwise.} \end{cases}$$

If  $8s \leq j < 9s$ , then

$$b_{ij} = \begin{cases} -e_{8(j+m+1)+5} \otimes w_{8j+5 \rightarrow 8(j+1)}, & i = 4s + (j+1)_s; \\ 0, & \text{otherwise.} \end{cases}$$

If  $9s \leq j < 10s$ , then

$$b_{ij} = \begin{cases} w_{8(j+m)+7 \rightarrow 8(j+m+1)+3} \otimes e_{8j+6}, & i = j + 3s; \\ 0, & \text{otherwise.} \end{cases}$$

If  $10s \leq j < 11s$ , then

$$b_{ij} = \begin{cases} w_{8(j+m)+7 \rightarrow 8(j+m+1)+6} \otimes e_{8j+6}, & i = j + 2s; \\ w_{8(j+m+1) \rightarrow 8(j+m+1)+6} \otimes e_{8j+6}, & i = j + 3s; \\ w_{8(j+m+1)+5 \rightarrow 8(j+m+1)+6} \otimes w_{8j+6 \rightarrow 8j+7}, & i = j + 4s; \\ 0, & \text{otherwise.} \end{cases}$$

If  $11s \leq j < 12s$ , then

$$b_{ij} = \begin{cases} w_{8(j+m+1)+3 \rightarrow 8(j+m+1)+7} \otimes e_{8j+7}, & i = j + 4s; \\ -w_{8(j+m+1)+6 \rightarrow 8(j+m+1)+7} \otimes e_{8j+7}, & i = j + 5s; \\ 0, & \text{otherwise.} \end{cases}$$

If  $12s \leq j < 13s$ , then

$$b_{ij} = \begin{cases} w_{8(j+m+1)+1 \rightarrow 8(j+m+2)} \otimes w_{8j+7 \rightarrow 8(j+1)}, & i = 3s + (j+1)_s; \\ -w_{8(j+m+1)+7 \rightarrow 8(j+m+2)} \otimes w_{8j+7 \rightarrow 8(j+1)+1}, & i = 5s + (j+1)_s; \\ -e_{8(j+m+2)} \otimes w_{8j+7 \rightarrow 8(j+1)+2}, & i = 6s + (j+1)_s; \\ -w_{8(j+m+1)+7 \rightarrow 8(j+m+2)} \otimes w_{8j+7 \rightarrow 8(j+1)+5}, & i = 10s + (j+1)_s; \\ -e_{8(j+m+2)} \otimes w_{8j+7 \rightarrow 8(j+1)+5}, & i = 11s + (j+1)_s; \\ 0, & \text{otherwise.} \end{cases}$$

(13) If  $r_0 = 12$ , then  $\Omega^{12}(Z_t^{(25)})$  is described with  $(19s \times 14s)$  matrix, whose entries  $b_{ij}$  have the following form:

If  $0 \leq j < s$ , then

$$b_{ij} = \begin{cases} w_{8(j+m-1)+7 \rightarrow 8(j+m)+2} \otimes e_{8j}, & i = j; \\ -e_{8(j+m)+2} \otimes w_{8j \rightarrow 8j+1}, & i = j + 3s; \\ 0, & \text{otherwise.} \end{cases}$$

If  $s \leq j < 2s$ , then

$$b_{ij} = \begin{cases} -w_{8(j+m)+3 \rightarrow 8(j+m)+4} \otimes w_{8j \rightarrow 8j+2}, & i = j + 3s; \\ e_{8(j+m)+4} \otimes w_{8j \rightarrow 8j+3}, & i = j + 5s; \\ 0, & \text{otherwise.} \end{cases}$$

If  $2s \leq j < 3s$ , then

$$b_{ij} = \begin{cases} -w_{8(j+m-1)+7 \rightarrow 8(j+m)+6} \otimes e_{8j}, & i = j; \\ -e_{8(j+m)+6} \otimes w_{8j \rightarrow 8j+5}, & i = j + 9s; \\ 0, & \text{otherwise.} \end{cases}$$

If  $3s \leq j < 4s$ , then

$$b_{ij} = \begin{cases} -e_{8(j+m)+5} \otimes w_{8j \rightarrow 8j+2}, & i = j + 2s; \\ 0, & \text{otherwise.} \end{cases}$$

If  $4s \leq j < 5s$ , then

$$b_{ij} = \begin{cases} -e_{8(j+m)+7} \otimes w_{8j+1 \rightarrow 8(j+1)}, & i = 2s + (j+1)_s; \\ 0, & \text{otherwise.} \end{cases}$$

If  $5s \leq j < 6s$ , then

$$b_{ij} = \begin{cases} -e_{8(j+m+1)} \otimes w_{8j+2 \rightarrow 8(j+1)}, & i = s + (j+1)_s; \\ -w_{8(j+m)+7 \rightarrow 8(j+m+1)} \otimes w_{8j+2 \rightarrow 8(j+1)}, & i = 2s + (j+1)_s; \\ 0, & \text{otherwise.} \end{cases}$$

If  $6s \leq j < 7s$ , then

$$b_{ij} = \begin{cases} e_{8(j+m)+7} \otimes w_{8j+3 \rightarrow 8(j+1)}, & i = 2s + (j+1)_s; \\ -w_{8(j+m)+4 \rightarrow 8(j+m)+7} \otimes e_{8j+3}, & i = j; \\ w_{8(j+m)+6 \rightarrow 8(j+m)+7} \otimes e_{8j+3}, & i = j + s; \\ 0, & \text{otherwise.} \end{cases}$$



If  $7s \leq j < 8s$ , then

$$b_{ij} = \begin{cases} -w_{8(j+m)+5 \rightarrow 8(j+m+1)} \otimes e_{8j+4}, & i = j + s; \\ w_{8(j+m)+1 \rightarrow 8(j+m+1)} \otimes e_{8j+4}, & i = j + 2s; \\ w_{8(j+m)+7 \rightarrow 8(j+m+1)} \otimes w_{8j+4 \rightarrow 8j+7}, & i = j + 9s; \\ 0, & \text{otherwise.} \end{cases}$$

If  $8s \leq j < 9s$ , then  $b_{ij} = 0$ .

If  $9s \leq j < 10s$ , then

$$b_{ij} = \begin{cases} w_{8(j+m)+6 \rightarrow 8(j+m)+7} \otimes e_{8j+6}, & i = j + 4s; \\ -w_{8(j+m)+3 \rightarrow 8(j+m)+7} \otimes e_{8j+6}, & i = j + 5s; \\ 0, & \text{otherwise.} \end{cases}$$

If  $10s \leq j < 11s$ , then

$$b_{ij} = \begin{cases} -w_{8(j+m)+7 \rightarrow 8(j+m+1)} \otimes w_{8j+6 \rightarrow 8(j+1)}, & i = 2s + (j + 1)_s; \\ w_{8(j+m)+6 \rightarrow 8(j+m+1)} \otimes e_{8j+6}, & i = j + 3s; \\ -e_{8(j+m+1)} \otimes w_{8j+6 \rightarrow 8j+7}, & i = j + 8s; \\ 0, & \text{otherwise.} \end{cases}$$

If  $11s \leq j < 12s$ , then

$$b_{ij} = \begin{cases} w_{8(j+m)+7 \rightarrow 8(j+m+1)+5} \otimes w_{8j+7 \rightarrow 8(j+1)}, & i = 2s + (j + 1)_s; \\ w_{8(j+m+1) \rightarrow 8(j+m+1)+5} \otimes e_{8j+7}, & i = j + 7s; \\ 0, & \text{otherwise.} \end{cases}$$

If  $12s \leq j < 13s$ , then

$$b_{ij} = \begin{cases} -w_{8(j+m)+7 \rightarrow 8(j+m+1)+3} \otimes w_{8j+7 \rightarrow 8(j+1)}, & i = (j + 1)_s; \\ -w_{8(j+m)+7 \rightarrow 8(j+m+1)+3} \otimes e_{8j+7}, & i = j + 4s; \\ 0, & \text{otherwise.} \end{cases}$$

If  $13s \leq j < 14s$ , then

$$b_{ij} = \begin{cases} w_{8(j+m)+7 \rightarrow 8(j+m+1)+1} \otimes w_{8j+7 \rightarrow 8(j+1)}, & i = (j + 1)_s; \\ -w_{8(j+m+1) \rightarrow 8(j+m+1)+1} \otimes w_{8j+7 \rightarrow 8(j+1)}, & i = s + (j + 1)_s; \\ -w_{8(j+m)+7 \rightarrow 8(j+m+1)+1} \otimes w_{8j+7 \rightarrow 8(j+1)}, & i = 2s + (j + 1)_s; \\ -e_{8(j+m+1)+1} \otimes w_{8j+7 \rightarrow 8(j+1)+4}, & i = 9s + (j + 1)_s; \\ e_{8(j+m+1)+1} \otimes w_{8j+7 \rightarrow 8(j+1)+6}, & i = 15s + (j + 1)_s; \\ 0, & \text{otherwise.} \end{cases}$$

(14) If  $r_0 = 13$ , then  $\Omega^{13}(Z_t^{(25)})$  is described with  $(18s \times 16s)$  matrix, whose entries  $b_{ij}$  have the following form:

If  $0 \leq j < s$ , then

$$b_{ij} = \begin{cases} w_{8(j+m)+3 \rightarrow 8(j+m)+7} \otimes e_{8j}, & i = j + s; \\ -w_{8(j+m)+6 \rightarrow 8(j+m)+7} \otimes e_{8j}, & i = j + 2s; \\ -e_{8(j+m)+7} \otimes w_{8j \rightarrow 8j+2}, & i = j + 5s; \\ 0, & \text{otherwise.} \end{cases}$$

If  $s \leq j < 2s$ , then

$$b_{ij} = \begin{cases} -e_{8(j+m)+7} \otimes w_{8j \rightarrow 8j+2}, & i = j + 4s; \\ 0, & \text{otherwise.} \end{cases}$$

If  $2s \leq j < 3s$ , then

$$b_{ij} = \begin{cases} -w_{8(j+m)+6 \rightarrow 8(j+m+1)} \otimes e_{8j}, & i = j; \\ w_{8(j+m)+7 \rightarrow 8(j+m+1)} \otimes w_{8j \rightarrow 8j+3}, & i = j + 4s; \\ e_{8(j+m+1)} \otimes w_{8j \rightarrow 8j+3}, & i = j + 5s; \\ -e_{8(j+m+1)} \otimes w_{8j \rightarrow 8j+4}, & i = j + 6s; \\ 0, & \text{otherwise.} \end{cases}$$

If  $3s \leq j < 4s$ , then

$$b_{ij} = \begin{cases} -e_{8(j+m+1)+5} \otimes w_{8j+1 \rightarrow 8(j+1)}, & i = 3s + (j+1)_s; \\ 0, & \text{otherwise.} \end{cases}$$

If  $4s \leq j < 5s$ , then

$$b_{ij} = \begin{cases} w_{8(j+m+1)+5 \rightarrow 8(j+m+1)+6} \otimes w_{8j+2 \rightarrow 8(j+1)}, & i = 3s + (j+1)_s; \\ 0, & \text{otherwise.} \end{cases}$$

If  $5s \leq j < 6s$ , then

$$b_{ij} = \begin{cases} w_{8(j+m)+7 \rightarrow 8(j+m+1)+1} \otimes w_{8j+2 \rightarrow 8j+3}, & i = j + s; \\ 0, & \text{otherwise.} \end{cases}$$

If  $6s \leq j < 7s$ , then

$$b_{ij} = \begin{cases} e_{8(j+m+1)+2} \otimes w_{8j+3 \rightarrow 8(j+1)}, & i = (j+1)_s; \\ w_{8(j+m)+7 \rightarrow 8(j+m+1)+2} \otimes e_{8j+3}, & i = j; \\ 0, & \text{otherwise.} \end{cases}$$

If  $7s \leq j < 8s$ , then

$$b_{ij} = \begin{cases} -w_{8(j+m+1)+2 \rightarrow 8(j+m+1)+3} \otimes w_{8j+4 \rightarrow 8(j+1)}, & i = (j+1)_s; \\ 0, & \text{otherwise.} \end{cases}$$

If  $8s \leq j < 9s$ , then

$$b_{ij} = \begin{cases} -w_{8(j+m+1) \rightarrow 8(j+m+1)+5} \otimes e_{8j+4}, & i = j; \\ -e_{8(j+m+1)+5} \otimes w_{8j+4 \rightarrow 8j+7}, & i = j + 9s; \\ 0, & \text{otherwise.} \end{cases}$$

If  $9s \leq j < 10s$ , then

$$b_{ij} = \begin{cases} -e_{8(j+m+1)+3} \otimes w_{8j+5 \rightarrow 8(j+1)}, & i = s + (j+1)_s; \\ w_{8(j+m)+7 \rightarrow 8(j+m+1)+3} \otimes w_{8j+5 \rightarrow 8j+6}, & i = j + 2s; \\ 0, & \text{otherwise.} \end{cases}$$

If  $10s \leq j < 11s$ , then

$$b_{ij} = \begin{cases} -e_{8(j+m+1)+6} \otimes w_{8j+5 \rightarrow 8(j+1)}, & i = 2s + (j+1)_s; \\ 0, & \text{otherwise.} \end{cases}$$

If  $11s \leq j < 12s$ , then  $b_{ij} = 0$ .

If  $12s \leq j < 13s$ , then

$$b_{ij} = \begin{cases} -w_{8(j+m)+7 \rightarrow 8(j+m+1)+4} \otimes e_{8j+6}, & i = j - s; \\ 0, & \text{otherwise.} \end{cases}$$

If  $13s \leq j < 14s$ , then

$$b_{ij} = \begin{cases} e_{8(j+m+1)+1} \otimes w_{8j+6 \rightarrow 8j+7}, & i = j + 3s; \\ 0, & \text{otherwise.} \end{cases}$$

If  $14s \leq j < 15s$ , then

$$b_{ij} = \begin{cases} w_{8(j+m+1)+2 \rightarrow 8(j+m+1)+7} \otimes w_{8j+7 \rightarrow 8(j+1)}, & i = (j+1)_s; \\ w_{8(j+m+1)+5 \rightarrow 8(j+m+1)+7} \otimes w_{8j+7 \rightarrow 8(j+1)}, & i = 3s + (j+1)_s; \\ e_{8(j+m+1)+7} \otimes w_{8j+7 \rightarrow 8(j+1)+2}, & i = 5s + (j+1)_s; \\ e_{8(j+m+1)+7} \otimes w_{8j+7 \rightarrow 8(j+1)+5}, & i = 9s + (j+1)_s; \\ -w_{8(j+m+1)+6 \rightarrow 8(j+m+1)+7} \otimes e_{8j+7}, & i = j; \\ 0, & \text{otherwise.} \end{cases}$$

If  $15s \leq j < 16s$ , then

$$b_{ij} = \begin{cases} -e_{8(j+m+2)} \otimes w_{8j+7 \rightarrow 8(j+1)+1}, & i = 4s + (j+1)_s; \\ w_{8(j+m+1)+7 \rightarrow 8(j+m+2)} \otimes w_{8j+7 \rightarrow 8(j+1)+2}, & i = 5s + (j+1)_s; \\ 0, & \text{otherwise.} \end{cases}$$

(15) If  $r_0 = 14$ , then  $\Omega^{14}(Z_t^{(25)})$  is described with  $(20s \times 16s)$  matrix, whose entries  $b_{ij}$  have the following form:

If  $0 \leq j < s$ , then

$$b_{ij} = \begin{cases} e_{8(j+m)+5} \otimes w_{8j \rightarrow 8j+3}, & i = j + 7s; \\ 0, & \text{otherwise.} \end{cases}$$

If  $s \leq j < 2s$ , then

$$b_{ij} = \begin{cases} -w_{8(j+m-1)+7 \rightarrow 8(j+m)+3} \otimes e_{8j}, & i = j - s; \\ e_{8(j+m)+3} \otimes w_{8j \rightarrow 8j+5}, & i = j + 11s; \\ 0, & \text{otherwise.} \end{cases}$$

If  $2s \leq j < 3s$ , then

$$b_{ij} = \begin{cases} -e_{8(j+m)+6} \otimes w_{8j \rightarrow 8j+2}, & i = j + 4s; \\ 0, & \text{otherwise.} \end{cases}$$

If  $3s \leq j < 4s$ , then

$$b_{ij} = \begin{cases} -e_{8(j+m)+1} \otimes w_{8j \rightarrow 8j+3}, & i = j + 5s; \\ 0, & \text{otherwise.} \end{cases}$$

If  $4s \leq j < 5s$ , then

$$b_{ij} = \begin{cases} -e_{8(j+m+1)} \otimes w_{8j+1 \rightarrow 8(j+1)}, & i = 2s + (j+1)_s; \\ 0, & \text{otherwise.} \end{cases}$$

If  $5s \leq j < 6s$ , then

$$b_{ij} = \begin{cases} -e_{8(j+m)+7} \otimes w_{8j+2 \rightarrow 8(j+1)}, & i = (j+1)_s; \\ 0, & \text{otherwise.} \end{cases}$$

If  $6s \leq j < 7s$ , then

$$b_{ij} = \begin{cases} e_{8(j+m+1)} \otimes w_{8j+3 \rightarrow 8(j+1)}, & i = s + (j+1)_s; \\ 0, & \text{otherwise.} \end{cases}$$

If  $7s \leq j < 8s$ , then

$$b_{ij} = \begin{cases} w_{8(j+m)+6 \rightarrow 8(j+m)+7} \otimes e_{8j+4}, & i = j + 3s; \\ 0, & \text{otherwise.} \end{cases}$$

If  $8s \leq j < 10s$ , then  $b_{ij} = 0$ .

If  $10s \leq j < 11s$ , then

$$b_{ij} = \begin{cases} w_{8(j+m)+2 \rightarrow 8(j+m)+7} \otimes e_{8j+6}, & i = j + 4s; \\ -w_{8(j+m)+5 \rightarrow 8(j+m)+7} \otimes e_{8j+6}, & i = j + 6s; \\ -e_{8(j+m)+7} \otimes w_{8j+6 \rightarrow 8j+7}, & i = j + 7s; \\ 0, & \text{otherwise.} \end{cases}$$

If  $11s \leq j < 12s$ , then  $b_{ij} = 0$ .

If  $12s \leq j < 13s$ , then

$$b_{ij} = \begin{cases} -w_{8(j+m)+7 \rightarrow 8(j+m+1)+2} \otimes w_{8j+7 \rightarrow 8(j+1)}, & i = (j+1)_s; \\ -w_{8(j+m+1) \rightarrow 8(j+m+1)+2} \otimes w_{8j+7 \rightarrow 8(j+1)}, & i = s + (j+1)_s; \\ -w_{8(j+m+1)+1 \rightarrow 8(j+m+1)+2} \otimes w_{8j+7 \rightarrow 8(j+1)+3}, & i = 8s + (j+1)_s; \\ -e_{8(j+m+1)+2} \otimes w_{8j+7 \rightarrow 8(j+1)+4}, & i = 9s + (j+1)_s; \\ e_{8(j+m+1)+2} \otimes w_{8j+7 \rightarrow 8(j+1)+6}, & i = 14s + (j+1)_s; \\ 0, & \text{otherwise.} \end{cases}$$

If  $13s \leq j < 14s$ , then

$$b_{ij} = \begin{cases} w_{8(j+m)+7 \rightarrow 8(j+m+1)+4} \otimes w_{8j+7 \rightarrow 8(j+1)}, & i = (j+1)_s; \\ -w_{8(j+m+1)+3 \rightarrow 8(j+m+1)+4} \otimes w_{8j+7 \rightarrow 8(j+1)+1}, & i = 3s + (j+1)_s; \\ -w_{8(j+m+1)+3 \rightarrow 8(j+m+1)+4} \otimes w_{8j+7 \rightarrow 8(j+1)+5}, & i = 12s + (j+1)_s; \\ 0, & \text{otherwise.} \end{cases}$$

If  $14s \leq j < 15s$ , then

$$b_{ij} = \begin{cases} e_{8(j+m+1)+6} \otimes w_{8j+7 \rightarrow 8(j+1)+2}, & i = 6s + (j+1)_s; \\ w_{8(j+m)+7 \rightarrow 8(j+m+1)+6} \otimes e_{8j+7}, & i = j + 3s; \\ 0, & \text{otherwise.} \end{cases}$$

If  $15s \leq j < 16s$ , then

$$b_{ij} = \begin{cases} -e_{8(j+m+1)+5} \otimes w_{8j+7 \rightarrow 8(j+1)+1}, & i = 4s + (j+1)_s; \\ 0, & \text{otherwise.} \end{cases}$$

(16) If  $r_0 = 15$ , then  $\Omega^{15}(Z_t^{(25)})$  is described with  $(18s \times 19s)$  matrix, whose entries  $b_{ij}$  have the following form:

If  $0 \leq j < s$ , then

$$b_{ij} = \begin{cases} -w_{8(j+m)+3 \rightarrow 8(j+m)+7} \otimes e_{8j}, & i = j; \\ w_{8(j+m)+5 \rightarrow 8(j+m)+7} \otimes e_{8j}, & i = j + 4s; \\ -e_{8(j+m)+7} \otimes w_{8j \rightarrow 8j+1}, & i = j + 5s; \\ e_{8(j+m)+7} \otimes w_{8j \rightarrow 8j+4}, & i = j + 9s; \\ 0, & \text{otherwise.} \end{cases}$$

If  $s \leq j < 2s$ , then

$$b_{ij} = \begin{cases} e_{8(j+m+1)} \otimes w_{8j \rightarrow 8j+5}, & i = j + 10s; \\ 0, & \text{otherwise.} \end{cases}$$

If  $2s \leq j < 3s$ , then

$$b_{ij} = \begin{cases} -e_{8(j+m+1)} \otimes w_{8j \rightarrow 8j+2}, & i = j + 5s; \\ 0, & \text{otherwise.} \end{cases}$$

If  $3s \leq j < 4s$ , then

$$b_{ij} = \begin{cases} -e_{8(j+m+1)+6} \otimes w_{8j+1 \rightarrow 8(j+1)}, & i = s + (j+1)_s; \\ 0, & \text{otherwise.} \end{cases}$$

If  $4s \leq j < 5s$ , then

$$b_{ij} = \begin{cases} e_{8(j+m+1)+1} \otimes w_{8j+1 \rightarrow 8(j+1)}, & i = 3s + (j+1)_s; \\ 0, & \text{otherwise.} \end{cases}$$

If  $5s \leq j < 7s$ , then  $b_{ij} = 0$ .

If  $7s \leq j < 8s$ , then

$$b_{ij} = \begin{cases} e_{8(j+m+1)+5} \otimes w_{8j+3 \rightarrow 8(j+1)}, & i = 4s + (j+1)_s; \\ 0, & \text{otherwise.} \end{cases}$$

If  $8s \leq j < 9s$ , then

$$b_{ij} = \begin{cases} -w_{8(j+m+1)+3 \rightarrow 8(j+m+1)+4} \otimes w_{8j+4 \rightarrow 8(j+1)}, & i = (j+1)_s; \\ 0, & \text{otherwise.} \end{cases}$$

If  $9s \leq j < 10s$ , then

$$b_{ij} = \begin{cases} -w_{8(j+m)+7 \rightarrow 8(j+m+1)+6} \otimes e_{8j+4}, & i = j; \\ 0, & \text{otherwise.} \end{cases}$$

If  $10s \leq j < 11s$ , then  $b_{ij} = 0$ .

If  $11s \leq j < 12s$ , then

$$b_{ij} = \begin{cases} w_{8(j+m+1)+3 \rightarrow 8(j+m+1)+4} \otimes w_{8j+5 \rightarrow 8(j+1)}, & i = (j+1)_s; \\ -e_{8(j+m+1)+4} \otimes w_{8j+5 \rightarrow 8(j+1)}, & i = 2s + (j+1)_s; \\ 0, & \text{otherwise.} \end{cases}$$

If  $12s \leq j < 13s$ , then  $b_{ij} = 0$ .

If  $13s \leq j < 14s$ , then

$$b_{ij} = \begin{cases} -w_{8(j+m+1) \rightarrow 8(j+m+1)+2} \otimes e_{8j+6}, & i = j - s; \\ -w_{8(j+m)+7 \rightarrow 8(j+m+1)+2} \otimes e_{8j+6}, & i = j; \\ e_{8(j+m+1)+2} \otimes w_{8j+6 \rightarrow 8j+7}, & i = j + s; \\ 0, & \text{otherwise.} \end{cases}$$

If  $14s \leq j < 16s$ , then  $b_{ij} = 0$ .

If  $16s \leq j < 17s$ , then

$$b_{ij} = \begin{cases} -w_{8(j+m+1)+3 \rightarrow 8(j+m+1)+7} \otimes w_{8j+7 \rightarrow 8(j+1)}, & i = (j+1)_s; \\ -e_{8(j+m+1)+7} \otimes w_{8j+7 \rightarrow 8(j+1)+1}, & i = 5s + (j+1)_s; \\ w_{8(j+m+1)+3 \rightarrow 8(j+m+1)+7} \otimes e_{8j+7}, & i = j - s; \\ 0, & \text{otherwise.} \end{cases}$$

If  $17s \leq j < 18s$ , then

$$b_{ij} = \begin{cases} -e_{8(j+m+1)+7} \otimes w_{8j+7 \rightarrow 8(j+1)+1}, & i = 5s + (j+1)_s; \\ 0, & \text{otherwise.} \end{cases}$$

If  $18s \leq j < 19s$ , then

$$b_{ij} = \begin{cases} e_{8(j+m+2)} \otimes w_{8j+7 \rightarrow 8(j+1)+2}, & i = 7s + (j+1)_s; \\ 0, & \text{otherwise.} \end{cases}$$

(17) If  $r_0 = 16$ , then  $\Omega^{16}(Z_t^{(25)})$  is described with  $(19s \times 18s)$  matrix, whose entries  $b_{ij}$  have the following form:

If  $0 \leq j < s$ , then

$$b_{ij} = \begin{cases} w_{8(j+m) \rightarrow 8(j+m)+2} \otimes e_{8j}, & i = j + s; \\ w_{8(j+m-1)+7 \rightarrow 8(j+m)+2} \otimes e_{8j}, & i = j + 2s; \\ -w_{8(j+m)+1 \rightarrow 8(j+m)+2} \otimes w_{8j \rightarrow 8j+2}, & i = j + 6s; \\ -e_{8(j+m)+2} \otimes w_{8j \rightarrow 8j+3}, & i = j + 7s; \\ 0, & \text{otherwise.} \end{cases}$$

If  $s \leq j < 2s$ , then

$$b_{ij} = \begin{cases} -e_{8(j+m)+6} \otimes w_{8j \rightarrow 8j+1}, & i = j + 3s; \\ 0, & \text{otherwise.} \end{cases}$$

If  $2s \leq j < 3s$ , then

$$b_{ij} = \begin{cases} e_{8(j+m)+4} \otimes w_{8j \rightarrow 8j+5}, & i = j + 9s; \\ 0, & \text{otherwise.} \end{cases}$$

If  $3s \leq j < 4s$ , then

$$b_{ij} = \begin{cases} e_{8(j+m)+1} \otimes w_{8j \rightarrow 8j+2}, & i = j + 3s; \\ 0, & \text{otherwise.} \end{cases}$$

If  $4s \leq j < 5s$ , then

$$b_{ij} = \begin{cases} e_{8(j+m)+5} \otimes w_{8j \rightarrow 8j+5}, & i = j + 8s; \\ 0, & \text{otherwise.} \end{cases}$$

If  $5s \leq j < 6s$ , then

$$b_{ij} = \begin{cases} -e_{8(j+m)+7} \otimes w_{8j+1 \rightarrow 8(j+1)}, & i = (j+1)_s; \\ 0, & \text{otherwise.} \end{cases}$$

If  $6s \leq j < 7s$ , then  $b_{ij} = 0$ .

If  $7s \leq j < 8s$ , then

$$b_{ij} = \begin{cases} -w_{8(j+m)+3 \rightarrow 8(j+m)+7} \otimes w_{8j+3 \rightarrow 8j+4}, & i = j + 2s; \\ 0, & \text{otherwise.} \end{cases}$$

If  $8s \leq j < 9s$ , then

$$b_{ij} = \begin{cases} -w_{8(j+m)+3 \rightarrow 8(j+m)+7} \otimes e_{8j+4}, & i = j + s; \\ 0, & \text{otherwise.} \end{cases}$$

If  $9s \leq j < 10s$ , then  $b_{ij} = 0$ .

If  $10s \leq j < 11s$ , then

$$b_{ij} = \begin{cases} e_{8(j+m)+7} \otimes w_{8j+5 \rightarrow 8(j+1)}, & i = 2s + (j+1)_s; \\ 0, & \text{otherwise.} \end{cases}$$

If  $11s \leq j < 12s$ , then

$$b_{ij} = \begin{cases} -e_{8(j+m)+1} \otimes w_{8j+5 \rightarrow 8(j+1)}, & i = s + (j+1)_s; \\ 0, & \text{otherwise.} \end{cases}$$

If  $12s \leq j < 13s$ , then

$$b_{ij} = \begin{cases} -w_{8(j+m)+3 \rightarrow 8(j+m)+7} \otimes e_{8j+6}, & i = j + s; \\ 0, & \text{otherwise.} \end{cases}$$

If  $13s \leq j < 15s$ , then  $b_{ij} = 0$ .

If  $15s \leq j < 16s$ , then

$$b_{ij} = \begin{cases} -w_{8(j+m)+7 \rightarrow 8(j+m+1)+3} \otimes e_{8j+7}, & i = j + s; \\ 0, & \text{otherwise.} \end{cases}$$

If  $16s \leq j < 17s$ , then

$$b_{ij} = \begin{cases} -e_{8(j+m+1)+6} \otimes w_{8j+7 \rightarrow 8(j+1)+1}, & i = 4s + (j+1)_s; \\ 0, & \text{otherwise.} \end{cases}$$

If  $17s \leq j < 18s$ , then

$$b_{ij} = \begin{cases} -e_{8(j+m+1)+1} \otimes w_{8j+7 \rightarrow 8(j+1)+2}, & i = 6s + (j+1)_s; \\ 0, & \text{otherwise.} \end{cases}$$

(18) If  $r_0 = 17$ , then  $\Omega^{17}(Z_t^{(25)})$  is described with  $(18s \times 19s)$  matrix, whose entries  $b_{ij}$  have the following form:

If  $0 \leq j < s$ , then

$$b_{ij} = \begin{cases} -w_{8(j+m)+2 \rightarrow 8(j+m)+7} \otimes e_{8j}, & i = j; \\ w_{8(j+m)+4 \rightarrow 8(j+m)+7} \otimes e_{8j}, & i = j + s; \\ e_{8(j+m)+7} \otimes w_{8j \rightarrow 8j+1}, & i = j + 4s; \\ e_{8(j+m)+7} \otimes w_{8j \rightarrow 8j+5}, & i = j + 10s; \\ 0, & \text{otherwise.} \end{cases}$$

If  $s \leq j < 2s$ , then

$$b_{ij} = \begin{cases} w_{8(j+m)+2 \rightarrow 8(j+m+1)} \otimes e_{8j}, & i = j - s; \\ -w_{8(j+m)+4 \rightarrow 8(j+m+1)} \otimes e_{8j}, & i = j; \\ -w_{8(j+m)+7 \rightarrow 8(j+m+1)} \otimes w_{8j \rightarrow 8j+1}, & i = j + 3s; \\ -e_{8(j+m+1)} \otimes w_{8j \rightarrow 8j+1}, & i = j + 4s; \\ 0, & \text{otherwise.} \end{cases}$$

If  $2s \leq j < 3s$ , then

$$b_{ij} = \begin{cases} e_{8(j+m)+7} \otimes w_{8j \rightarrow 8j+5}, & i = j + 8s; \\ 0, & \text{otherwise.} \end{cases}$$

If  $3s \leq j < 4s$ , then

$$b_{ij} = \begin{cases} e_{8(j+m+1)+2} \otimes w_{8j+1 \rightarrow 8(j+1)}, & i = (j+1)_s; \\ 0, & \text{otherwise.} \end{cases}$$

If  $4s \leq j < 5s$ , then

$$b_{ij} = \begin{cases} -w_{8(j+m+1)+2 \rightarrow 8(j+m+1)+3} \otimes w_{8j+2 \rightarrow 8(j+1)}, & i = (j+1)_s; \\ w_{8(j+m)+7 \rightarrow 8(j+m+1)+3} \otimes w_{8j+2 \rightarrow 8j+3}, & i = j + 3s; \\ 0, & \text{otherwise.} \end{cases}$$

If  $5s \leq j < 6s$ , then  $b_{ij} = 0$ .

If  $6s \leq j < 7s$ , then

$$b_{ij} = \begin{cases} w_{8(j+m+1)+2 \rightarrow 8(j+m+1)+4} \otimes w_{8j+3 \rightarrow 8(j+1)}, & i = (j+1)_s; \\ -w_{8(j+m)+7 \rightarrow 8(j+m+1)+4} \otimes e_{8j+3}, & i = j + s; \\ 0, & \text{otherwise.} \end{cases}$$

If  $7s \leq j < 11s$ , then  $b_{ij} = 0$ .

If  $11s \leq j < 12s$ , then

$$b_{ij} = \begin{cases} e_{8(j+m+1)+6} \otimes w_{8j+5 \rightarrow 8(j+1)}, & i = 2s + (j+1)_s; \\ 0, & \text{otherwise.} \end{cases}$$



If  $12s \leq j < 13s$ , then

$$b_{ij} = \begin{cases} -e_{8(j+m+1)+5} \otimes w_{8j+5 \rightarrow 8(j+1)}, & i = 3s + (j+1)_s; \\ 0, & \text{otherwise.} \end{cases}$$

If  $13s \leq j < 14s$ , then  $b_{ij} = 0$ .

If  $14s \leq j < 15s$ , then

$$b_{ij} = \begin{cases} -w_{8(j+m)+7 \rightarrow 8(j+m+1)+3} \otimes e_{8j+6}, & i = j - 3s; \\ 0, & \text{otherwise.} \end{cases}$$

If  $15s \leq j < 16s$ , then  $b_{ij} = 0$ .

If  $16s \leq j < 17s$ , then

$$b_{ij} = \begin{cases} w_{8(j+m+1)+2 \rightarrow 8(j+m+1)+7} \otimes w_{8j+7 \rightarrow 8(j+1)}, & i = (j+1)_s; \\ -w_{8(j+m+1)+4 \rightarrow 8(j+m+1)+7} \otimes w_{8j+7 \rightarrow 8(j+1)}, & i = s + (j+1)_s; \\ -e_{8(j+m+1)+7} \otimes w_{8j+7 \rightarrow 8(j+1)+1}, & i = 4s + (j+1)_s; \\ -w_{8(j+m+1)+3 \rightarrow 8(j+m+1)+7} \otimes e_{8j+7}, & i = j - 3s; \\ w_{8(j+m+1)+4 \rightarrow 8(j+m+1)+7} \otimes e_{8j+7}, & i = j - s; \\ 0, & \text{otherwise.} \end{cases}$$

If  $17s \leq j < 18s$ , then  $b_{ij} = 0$ .

If  $18s \leq j < 19s$ , then

$$b_{ij} = \begin{cases} -e_{8(j+m+2)} \otimes w_{8j+7 \rightarrow 8(j+1)+1}, & i = 5s + (j+1)_s; \\ w_{8(j+m+1)+7 \rightarrow 8(j+m+2)} \otimes w_{8j+7 \rightarrow 8(j+1)+5}, & i = 10s + (j+1)_s; \\ 0, & \text{otherwise.} \end{cases}$$

(19) If  $r_0 = 18$ , then  $\Omega^{18}(Z_t^{(25)})$  is described with  $(19s \times 18s)$  matrix, whose entries  $b_{ij}$  have the following form:

If  $0 \leq j < s$ , then

$$b_{ij} = \begin{cases} w_{8(j+m)+1 \rightarrow 8(j+m)+2} \otimes w_{8j \rightarrow 8j+1}, & i = j + 4s; \\ e_{8(j+m)+2} \otimes w_{8j \rightarrow 8j+2}, & i = j + 5s; \\ 0, & \text{otherwise.} \end{cases}$$

If  $s \leq j < 2s$ , then

$$b_{ij} = \begin{cases} -w_{8(j+m-1)+7 \rightarrow 8(j+m)+3} \otimes e_{8j}, & i = j - s; \\ 0, & \text{otherwise.} \end{cases}$$

If  $2s \leq j < 3s$ , then

$$b_{ij} = \begin{cases} e_{8(j+m)+6} \otimes w_{8j \rightarrow 8j+5}, & i = j + 9s; \\ 0, & \text{otherwise.} \end{cases}$$

If  $3s \leq j < 4s$ , then

$$b_{ij} = \begin{cases} -e_{8(j+m)+5} \otimes w_{8j \rightarrow 8j+1}, & i = j; \\ 0, & \text{otherwise.} \end{cases}$$

If  $4s \leq j < 5s$ , then

$$b_{ij} = \begin{cases} -e_{8(j+m+1)} \otimes w_{8j+1 \rightarrow 8(j+1)}, & i = s + (j+1)_s; \\ 0, & \text{otherwise.} \end{cases}$$

If  $5s \leq j < 6s$ , then  $b_{ij} = 0$ .

If  $6s \leq j < 7s$ , then

$$b_{ij} = \begin{cases} -w_{8(j+m)+3 \rightarrow 8(j+m)+7} \otimes e_{8j+3}, & i = j + s; \\ w_{8(j+m)+4 \rightarrow 8(j+m)+7} \otimes w_{8j+3 \rightarrow 8j+4}, & i = j + 2s; \\ 0, & \text{otherwise.} \end{cases}$$

If  $7s \leq j < 8s$ , then

$$b_{ij} = \begin{cases} -e_{8(j+m+1)} \otimes w_{8j+3 \rightarrow 8(j+1)}, & i = s + (j+1)_s; \\ -w_{8(j+m)+3 \rightarrow 8(j+m+1)} \otimes e_{8j+3}, & i = j; \\ w_{8(j+m)+4 \rightarrow 8(j+m+1)} \otimes w_{8j+3 \rightarrow 8j+4}, & i = j + s; \\ 0, & \text{otherwise.} \end{cases}$$

If  $8s \leq j < 9s$ , then

$$b_{ij} = \begin{cases} -e_{8(j+m+1)} \otimes w_{8j+4 \rightarrow 8j+7}, & i = j + 9s; \\ 0, & \text{otherwise.} \end{cases}$$

If  $9s \leq j < 10s$ , then

$$b_{ij} = \begin{cases} e_{8(j+m)+7} \otimes w_{8j+5 \rightarrow 8(j+1)}, & i = (j+1)_s; \\ 0, & \text{otherwise.} \end{cases}$$

If  $10s \leq j < 11s$ , then

$$b_{ij} = \begin{cases} e_{8(j+m+1)} \otimes w_{8j+5 \rightarrow 8(j+1)}, & i = 2s + (j+1)_s; \\ 0, & \text{otherwise.} \end{cases}$$

If  $11s \leq j < 12s$ , then

$$b_{ij} = \begin{cases} -w_{8(j+m)+4 \rightarrow 8(j+m)+7} \otimes e_{8j+6}, & i = j + 3s; \\ 0, & \text{otherwise.} \end{cases}$$

If  $12s \leq j < 13s$ , then  $b_{ij} = 0$ .

If  $13s \leq j < 14s$ , then

$$b_{ij} = \begin{cases} -w_{8(j+m+1)+1 \rightarrow 8(j+m+1)+2} \otimes w_{8j+7 \rightarrow 8(j+1)+1}, & i = 4s + (j+1)_s; \\ -e_{8(j+m+1)+2} \otimes w_{8j+7 \rightarrow 8(j+1)+2}, & i = 5s + (j+1)_s; \\ w_{8(j+m+1) \rightarrow 8(j+m+1)+2} \otimes e_{8j+7}, & i = j + 4s; \\ 0, & \text{otherwise.} \end{cases}$$

If  $14s \leq j < 18s$ , then  $b_{ij} = 0$ .

(20) If  $r_0 = 19$ , then  $\Omega^{19}(Z_t^{(25)})$  is described with  $(16s \times 20s)$  matrix, whose entries  $b_{ij}$  have the following form:

If  $0 \leq j < s$ , then

$$b_{ij} = \begin{cases} -w_{8(j+m)+6 \rightarrow 8(j+m)+7} \otimes e_{8j}, & i = j + s; \\ -w_{8(j+m)+1 \rightarrow 8(j+m)+7} \otimes e_{8j}, & i = j + 2s; \\ e_{8(j+m)+7} \otimes w_{8j \rightarrow 8j+2}, & i = j + 5s; \\ e_{8(j+m)+7} \otimes w_{8j \rightarrow 8j+4}, & i = j + 7s; \\ e_{8(j+m)+7} \otimes w_{8j \rightarrow 8j+6}, & i = j + 10s; \\ 0, & \text{otherwise.} \end{cases}$$

If  $s \leq j < 2s$ , then  $b_{ij} = 0$ .

If  $2s \leq j < 3s$ , then

$$b_{ij} = \begin{cases} e_{8(j+m+1)} \otimes w_{8j \rightarrow 8j+3}, & i = j + 4s; \\ e_{8(j+m+1)} \otimes w_{8j \rightarrow 8j+5}, & i = j + 7s; \\ 0, & \text{otherwise.} \end{cases}$$

If  $3s \leq j < 4s$ , then

$$b_{ij} = \begin{cases} e_{8(j+m+1)+3} \otimes w_{8j+1 \rightarrow 8(j+1)}, & i = (j+1)_s; \\ 0, & \text{otherwise.} \end{cases}$$

If  $4s \leq j < 5s$ , then

$$b_{ij} = \begin{cases} -e_{8(j+m+1)+5} \otimes w_{8j+1 \rightarrow 8(j+1)}, & i = 3s + (j+1)_s; \\ 0, & \text{otherwise.} \end{cases}$$

If  $5s \leq j < 6s$ , then

$$b_{ij} = \begin{cases} -w_{8(j+m+1)+3 \rightarrow 8(j+m+1)+4} \otimes w_{8j+2 \rightarrow 8(j+1)}, & i = (j+1)_s; \\ 0, & \text{otherwise.} \end{cases}$$

If  $6s \leq j < 7s$ , then  $b_{ij} = 0$ .

If  $7s \leq j < 8s$ , then

$$b_{ij} = \begin{cases} -e_{8(j+m+1)+5} \otimes w_{8j+3 \rightarrow 8(j+1)}, & i = 3s + (j+1)_s; \\ 0, & \text{otherwise.} \end{cases}$$

If  $8s \leq j < 9s$ , then

$$b_{ij} = \begin{cases} w_{8(j+m+1) \rightarrow 8(j+m+1)+1} \otimes e_{8j+3}, & i = j - 2s; \\ 0, & \text{otherwise.} \end{cases}$$

If  $9s \leq j < 10s$ , then  $b_{ij} = 0$ .

If  $10s \leq j < 11s$ , then

$$b_{ij} = \begin{cases} w_{8(j+m+1)+5 \rightarrow 8(j+m+1)+6} \otimes w_{8j+4 \rightarrow 8j+7}, & i = j + 5s; \\ 0, & \text{otherwise.} \end{cases}$$

If  $11s \leq j < 12s$ , then

$$b_{ij} = \begin{cases} e_{8(j+m+1)+6} \otimes w_{8j+5 \rightarrow 8(j+1)}, & i = s + (j+1)_s; \\ 0, & \text{otherwise.} \end{cases}$$

If  $12s \leq j < 13s$ , then  $b_{ij} = 0$ .

If  $13s \leq j < 14s$ , then

$$b_{ij} = \begin{cases} -e_{8(j+m+1)+1} \otimes w_{8j+5 \rightarrow 8(j+1)}, & i = 2s + (j+1)s; \\ 0, & \text{otherwise.} \end{cases}$$

If  $14s \leq j < 15s$ , then

$$b_{ij} = \begin{cases} w_{8(j+m+1) \rightarrow 8(j+m+1)+2} \otimes e_{8j+6}, & i = j - 3s; \\ 0, & \text{otherwise.} \end{cases}$$

If  $15s \leq j < 17s$ , then  $b_{ij} = 0$ .

If  $17s \leq j < 18s$ , then

$$b_{ij} = \begin{cases} w_{8(j+m+1)+5 \rightarrow 8(j+m+1)+7} \otimes e_{8j+7}, & i = j - 2s; \\ 0, & \text{otherwise.} \end{cases}$$

If  $18s \leq j < 19s$ , then

$$b_{ij} = \begin{cases} w_{8(j+m+1)+2 \rightarrow 8(j+m+2)} \otimes e_{8j+7}, & i = j - 6s; \\ 0, & \text{otherwise.} \end{cases}$$

If  $19s \leq j < 20s$ , then  $b_{ij} = 0$ .

(21) If  $r_0 = 20$ , then  $\Omega^{20}(Z_t^{(25)})$  is described with  $(16s \times 18s)$  matrix, whose entries  $b_{ij}$  have the following form:

If  $0 \leq j < s$ , then

$$b_{ij} = \begin{cases} w_{8(j+m-1)+7 \rightarrow 8(j+m)+3} \otimes e_{8j}, & i = j; \\ -w_{8(j+m) \rightarrow 8(j+m)+3} \otimes e_{8j}, & i = j + s; \\ -w_{8(j+m)+2 \rightarrow 8(j+m)+3} \otimes w_{8j \rightarrow 8j+1}, & i = j + 2s; \\ e_{8(j+m)+3} \otimes w_{8j \rightarrow 8j+2}, & i = j + 4s; \\ -w_{8(j+m)+1 \rightarrow 8(j+m)+3} \otimes w_{8j \rightarrow 8j+5}, & i = j + 10s; \\ 0, & \text{otherwise.} \end{cases}$$

If  $s \leq j < 2s$ , then

$$b_{ij} = \begin{cases} w_{8(j+m-1)+7 \rightarrow 8(j+m)+6} \otimes e_{8j}, & i = j - s; \\ w_{8(j+m)+5 \rightarrow 8(j+m)+6} \otimes w_{8j \rightarrow 8j+3}, & i = j + 5s; \\ e_{8(j+m)+6} \otimes w_{8j \rightarrow 8j+4}, & i = j + 6s; \\ e_{8(j+m)+6} \otimes w_{8j \rightarrow 8j+5}, & i = j + 7s; \\ 0, & \text{otherwise.} \end{cases}$$

If  $2s \leq j < 3s$ , then  $b_{ij} = 0$ .

If  $3s \leq j < 4s$ , then

$$b_{ij} = \begin{cases} -e_{8(j+m)+1} \otimes w_{8j \rightarrow 8j+5}, & i = j + 7s; \\ 0, & \text{otherwise.} \end{cases}$$

If  $4s \leq j < 5s$ , then  $b_{ij} = 0$ .

If  $5s \leq j < 6s$ , then

$$b_{ij} = \begin{cases} -e_{8(j+m)+7} \otimes w_{8j+1 \rightarrow 8(j+1)}, & i = (j+1)_s; \\ 0, & \text{otherwise.} \end{cases}$$

If  $6s \leq j < 7s$ , then

$$b_{ij} = \begin{cases} -e_{8(j+m)+7} \otimes w_{8j+2 \rightarrow 8(j+1)}, & i = (j+1)_s; \\ 0, & \text{otherwise.} \end{cases}$$

If  $7s \leq j < 8s$ , then  $b_{ij} = 0$ .

If  $8s \leq j < 9s$ , then

$$b_{ij} = \begin{cases} -2w_{8(j+m)+7 \rightarrow 8(j+m+1)} \otimes w_{8j+3 \rightarrow 8(j+1)}, & i = (j+1)_s; \\ e_{8(j+m+1)} \otimes w_{8j+3 \rightarrow 8(j+1)}, & i = s + (j+1)_s; \\ -w_{8(j+m)+4 \rightarrow 8(j+m+1)} \otimes e_{8j+3}, & i = j - 3s; \\ e_{8(j+m+1)} \otimes w_{8j+3 \rightarrow 8j+7}, & i = j + 6s; \\ 0, & \text{otherwise.} \end{cases}$$

If  $9s \leq j < 10s$ , then  $b_{ij} = 0$ .

If  $10s \leq j < 11s$ , then

$$b_{ij} = \begin{cases} -w_{8(j+m)+5 \rightarrow 8(j+m)+7} \otimes w_{8j+5 \rightarrow 8j+6}, & i = j + 2s; \\ 0, & \text{otherwise.} \end{cases}$$

If  $11s \leq j < 12s$ , then  $b_{ij} = 0$ .

If  $12s \leq j < 13s$ , then

$$b_{ij} = \begin{cases} -w_{8(j+m)+2 \rightarrow 8(j+m+1)} \otimes e_{8j+6}, & i = j - s; \\ 0, & \text{otherwise.} \end{cases}$$

If  $13s \leq j < 14s$ , then  $b_{ij} = 0$ .

If  $14s \leq j < 15s$ , then

$$b_{ij} = \begin{cases} w_{8(j+m)+7 \rightarrow 8(j+m+1)+2} \otimes w_{8j+7 \rightarrow 8(j+1)}, & i = (j+1)_s; \\ -w_{8(j+m+1) \rightarrow 8(j+m+1)+2} \otimes w_{8j+7 \rightarrow 8(j+1)}, & i = s + (j+1)_s; \\ -w_{8(j+m)+7 \rightarrow 8(j+m+1)+2} \otimes e_{8j+7}, & i = j - s; \\ -w_{8(j+m+1) \rightarrow 8(j+m+1)+2} \otimes e_{8j+7}, & i = j; \\ 0, & \text{otherwise.} \end{cases}$$

If  $15s \leq j < 18s$ , then  $b_{ij} = 0$ .

(22) If  $r_0 = 21$ , then  $\Omega^{21}(Z_t^{(25)})$  is described with  $(14s \times 19s)$  matrix, whose entries  $b_{ij}$  have the following form:

If  $0 \leq j < s$ , then

$$b_{ij} = \begin{cases} w_{8(j+m)+6 \rightarrow 8(j+m)+7} \otimes e_{8j}, & i = j + 2s; \\ e_{8(j+m)+7} \otimes w_{8j \rightarrow 8j+1}, & i = j + 3s; \\ 0, & \text{otherwise.} \end{cases}$$

If  $s \leq j < 2s$ , then

$$b_{ij} = \begin{cases} w_{8(j+m)+2 \rightarrow 8(j+m+1)} \otimes e_{8j}, & i = j - s; \\ e_{8(j+m+1)} \otimes w_{8j \rightarrow 8j+2}, & i = j + 3s; \\ 0, & \text{otherwise.} \end{cases}$$

If  $2s \leq j < 3s$ , then  $b_{ij} = 0$ .

If  $3s \leq j < 4s$ , then

$$b_{ij} = \begin{cases} e_{8(j+m+1)+4} \otimes w_{8j+1 \rightarrow 8(j+1)}, & i = s + (j+1)s; \\ 0, & \text{otherwise.} \end{cases}$$

If  $4s \leq j < 5s$ , then  $b_{ij} = 0$ .

If  $5s \leq j < 6s$ , then

$$b_{ij} = \begin{cases} w_{8(j+m+1) \rightarrow 8(j+m+1)+5} \otimes e_{8j+2}, & i = j - s; \\ 0, & \text{otherwise.} \end{cases}$$

If  $6s \leq j < 7s$ , then  $b_{ij} = 0$ .

If  $7s \leq j < 8s$ , then

$$b_{ij} = \begin{cases} -w_{8(j+m)+7 \rightarrow 8(j+m+1)+2} \otimes e_{8j+3}, & i = j - 2s; \\ 0, & \text{otherwise.} \end{cases}$$

If  $8s \leq j < 9s$ , then

$$b_{ij} = \begin{cases} -w_{8(j+m+1)+5 \rightarrow 8(j+m+1)+6} \otimes w_{8j+3 \rightarrow 8j+7}, & i = j + 5s; \\ 0, & \text{otherwise.} \end{cases}$$

If  $9s \leq j < 10s$ , then  $b_{ij} = 0$ .

If  $10s \leq j < 11s$ , then

$$b_{ij} = \begin{cases} w_{8(j+m)+7 \rightarrow 8(j+m+1)+2} \otimes e_{8j+5}, & i = j - 3s; \\ w_{8(j+m+1) \rightarrow 8(j+m+1)+2} \otimes e_{8j+5}, & i = j - 2s; \\ 0, & \text{otherwise.} \end{cases}$$

If  $11s \leq j < 13s$ , then  $b_{ij} = 0$ .

If  $13s \leq j < 14s$ , then

$$b_{ij} = \begin{cases} -e_{8(j+m+1)+3} \otimes w_{8j+6 \rightarrow 8j+7}, & i = j - 3s; \\ 0, & \text{otherwise.} \end{cases}$$

If  $14s \leq j < 16s$ , then  $b_{ij} = 0$ .

If  $16s \leq j < 17s$ , then

$$b_{ij} = \begin{cases} -w_{8(j+m+1)+3 \rightarrow 8(j+m+1)+7} \otimes e_{8j+7}, & i = j - 6s; \\ 0, & \text{otherwise.} \end{cases}$$

If  $17s \leq j < 19s$ , then  $b_{ij} = 0$ .

(23) If  $r_0 = 22$ , then  $\Omega^{22}(Z_t^{(25)})$  is described with  $(13s \times 18s)$  matrix, whose entries  $b_{ij}$  have the following form:

If  $0 \leq j < s$ , then

$$b_{ij} = \begin{cases} -w_{8(j+m) \rightarrow 8(j+m)+2} \otimes e_{8j}, & i = j; \\ w_{8(j+m-1)+7 \rightarrow 8(j+m)+2} \otimes e_{8j}, & i = j + s; \\ 0, & \text{otherwise.} \end{cases}$$

If  $s \leq j < 2s$ , then

$$b_{ij} = \begin{cases} -w_{8(j+m) \rightarrow 8(j+m)+4} \otimes e_{8j}, & i = j - s; \\ w_{8(j+m-1)+7 \rightarrow 8(j+m)+4} \otimes e_{8j}, & i = j; \\ e_{8(j+m)+4} \otimes w_{8j \rightarrow 8j+2}, & i = j + 2s; \\ 0, & \text{otherwise.} \end{cases}$$

If  $2s \leq j < 3s$ , then

$$b_{ij} = \begin{cases} -w_{8(j+m)+5 \rightarrow 8(j+m)+6} \otimes w_{8j \rightarrow 8j+2}, & i = j + 2s; \\ 0, & \text{otherwise.} \end{cases}$$

If  $3s \leq j < 4s$ , then  $b_{ij} = 0$ .

If  $4s \leq j < 5s$ , then

$$b_{ij} = \begin{cases} e_{8(j+m)+7} \otimes w_{8j+1 \rightarrow 8(j+1)}, & i = s + (j + 1)_s; \\ 0, & \text{otherwise.} \end{cases}$$

If  $5s \leq j < 6s$ , then

$$b_{ij} = \begin{cases} -e_{8(j+m+1)} \otimes w_{8j+1 \rightarrow 8(j+1)}, & i = (j + 1)_s; \\ w_{8(j+m)+7 \rightarrow 8(j+m+1)} \otimes w_{8j+1 \rightarrow 8(j+1)}, & i = s + (j + 1)_s; \\ 0, & \text{otherwise.} \end{cases}$$

If  $6s \leq j < 7s$ , then

$$b_{ij} = \begin{cases} -e_{8(j+m+1)} \otimes w_{8j+2 \rightarrow 8(j+1)}, & i = (j + 1)_s; \\ w_{8(j+m)+7 \rightarrow 8(j+m+1)} \otimes w_{8j+2 \rightarrow 8(j+1)}, & i = s + (j + 1)_s; \\ -w_{8(j+m)+5 \rightarrow 8(j+m+1)} \otimes e_{8j+2}, & i = j - 2s; \\ 0, & \text{otherwise.} \end{cases}$$

If  $7s \leq j < 8s$ , then

$$b_{ij} = \begin{cases} -w_{8(j+m)+6 \rightarrow 8(j+m)+7} \otimes e_{8j+3}, & i = j - 2s; \\ w_{8(j+m)+1 \rightarrow 8(j+m)+7} \otimes w_{8j+3 \rightarrow 8j+4}, & i = j - s; \\ e_{8(j+m)+7} \otimes w_{8j+3 \rightarrow 8j+7}, & i = j + 4s; \\ 0, & \text{otherwise.} \end{cases}$$

If  $8s \leq j < 9s$ , then  $b_{ij} = 0$ .

If  $9s \leq j < 10s$ , then

$$b_{ij} = \begin{cases} -w_{8(j+m)+2 \rightarrow 8(j+m+1)} \otimes e_{8j+5}, & i = j - 2s; \\ w_{8(j+m)+3 \rightarrow 8(j+m+1)} \otimes w_{8j+5 \rightarrow 8j+6}, & i = j; \\ 0, & \text{otherwise.} \end{cases}$$

If  $10s \leq j < 13s$ , then  $b_{ij} = 0$ .

If  $13s \leq j < 14s$ , then

$$b_{ij} = \begin{cases} e_{8(j+m+1)+3} \otimes w_{8j+7 \rightarrow 8(j+1)+1}, & i = 2s + (j+1)_s; \\ -w_{8(j+m)+7 \rightarrow 8(j+m+1)+3} \otimes e_{8j+7}, & i = j - 2s; \\ 0, & \text{otherwise.} \end{cases}$$

If  $14s \leq j < 18s$ , then  $b_{ij} = 0$ .

(24) If  $r_0 = 23$ , then  $\Omega^{23}(Z_t^{(25)})$  is described with  $(11s \times 19s)$  matrix, whose entries  $b_{ij}$  have the following form:

If  $0 \leq j < s$ , then

$$b_{ij} = \begin{cases} -e_{8(j+m)+7} \otimes w_{8j \rightarrow 8j+2}, & i = j + 3s; \\ 0, & \text{otherwise.} \end{cases}$$

If  $s \leq j < 2s$ , then

$$b_{ij} = \begin{cases} w_{8(j+m)+3 \rightarrow 8(j+m+1)} \otimes e_{8j}, & i = j - s; \\ e_{8(j+m+1)} \otimes w_{8j \rightarrow 8j+1}, & i = j + s; \\ 0, & \text{otherwise.} \end{cases}$$

If  $2s \leq j < 3s$ , then  $b_{ij} = 0$ .

If  $3s \leq j < 4s$ , then

$$b_{ij} = \begin{cases} -e_{8(j+m+1)+5} \otimes w_{8j+1 \rightarrow 8(j+1)}, & i = s + (j+1)_s; \\ 0, & \text{otherwise.} \end{cases}$$

If  $4s \leq j < 6s$ , then  $b_{ij} = 0$ .

If  $6s \leq j < 7s$ , then

$$b_{ij} = \begin{cases} w_{8(j+m+1)+5 \rightarrow 8(j+m+1)+6} \otimes w_{8j+2 \rightarrow 8(j+1)}, & i = s + (j+1)_s; \\ -w_{8(j+m)+7 \rightarrow 8(j+m+1)+6} \otimes e_{8j+2}, & i = j - 3s; \\ 0, & \text{otherwise.} \end{cases}$$

If  $7s \leq j < 8s$ , then

$$b_{ij} = \begin{cases} -e_{8(j+m+1)+3} \otimes w_{8j+3 \rightarrow 8(j+1)}, & i = (j+1)_s; \\ 0, & \text{otherwise.} \end{cases}$$

If  $8s \leq j < 10s$ , then  $b_{ij} = 0$ .

If  $10s \leq j < 11s$ , then

$$b_{ij} = \begin{cases} -w_{8(j+m)+7 \rightarrow 8(j+m+1)+3} \otimes w_{8j+5 \rightarrow 8j+6}, & i = j - 3s; \\ 0, & \text{otherwise.} \end{cases}$$

If  $11s \leq j < 14s$ , then  $b_{ij} = 0$ .

If  $14s \leq j < 15s$ , then

$$b_{ij} = \begin{cases} w_{8(j+m)+7 \rightarrow 8(j+m+1)+4} \otimes e_{8j+6}, & i = j - 7s; \\ 0, & \text{otherwise.} \end{cases}$$

If  $15s \leq j < 16s$ , then  $b_{ij} = 0$ .



If  $16s \leq j < 17s$ , then

$$b_{ij} = \begin{cases} w_{8(j+m+1)+2 \rightarrow 8(j+m+1)+7} \otimes e_{8j+7}, & i = j - 8s; \\ w_{8(j+m+1)+4 \rightarrow 8(j+m+1)+7} \otimes e_{8j+7}, & i = j - 7s; \\ 0, & \text{otherwise.} \end{cases}$$

If  $17s \leq j < 18s$ , then

$$b_{ij} = \begin{cases} e_{8(j+m+2)} \otimes w_{8j+7 \rightarrow 8(j+1)+1}, & i = 2s + (j+1)_s; \\ 0, & \text{otherwise.} \end{cases}$$

If  $18s \leq j < 19s$ , then  $b_{ij} = 0$ .

(25) If  $r_0 = 24$ , then  $\Omega^{24}(Z_t^{(25)})$  is described with  $(11s \times 16s)$  matrix, whose entries  $b_{ij}$  have the following form:

If  $0 \leq j < s$ , then

$$b_{ij} = \begin{cases} -w_{8(j+m) \rightarrow 8(j+m)+3} \otimes e_{8j}, & i = j; \\ w_{8(j+m)+1 \rightarrow 8(j+m)+3} \otimes w_{8j \rightarrow 8j+3}, & i = j + 4s; \\ -w_{8(j+m)+2 \rightarrow 8(j+m)+3} \otimes w_{8j \rightarrow 8j+4}, & i = j + 5s; \\ -e_{8(j+m)+3} \otimes w_{8j \rightarrow 8j+5}, & i = j + 6s; \\ 0, & \text{otherwise.} \end{cases}$$

If  $s \leq j < 3s$ , then  $b_{ij} = 0$ .

If  $3s \leq j < 4s$ , then

$$b_{ij} = \begin{cases} e_{8(j+m)+5} \otimes w_{8j \rightarrow 8j+1}, & i = j - s; \\ 0, & \text{otherwise.} \end{cases}$$

If  $4s \leq j < 5s$ , then

$$b_{ij} = \begin{cases} -e_{8(j+m+1)} \otimes w_{8j+1 \rightarrow 8(j+1)}, & i = (j+1)_s; \\ 0, & \text{otherwise.} \end{cases}$$

If  $5s \leq j < 6s$ , then

$$b_{ij} = \begin{cases} -w_{8(j+m)+6 \rightarrow 8(j+m)+7} \otimes e_{8j+2}, & i = j - 2s; \\ w_{8(j+m)+1 \rightarrow 8(j+m)+7} \otimes w_{8j+2 \rightarrow 8j+3}, & i = j - s; \\ -w_{8(j+m)+2 \rightarrow 8(j+m)+7} \otimes w_{8j+2 \rightarrow 8j+4}, & i = j; \\ e_{8(j+m)+7} \otimes w_{8j+2 \rightarrow 8j+7}, & i = j + 5s; \\ 0, & \text{otherwise.} \end{cases}$$

If  $6s \leq j < 8s$ , then  $b_{ij} = 0$ .

If  $8s \leq j < 9s$ , then

$$b_{ij} = \begin{cases} w_{8(j+m)+4 \rightarrow 8(j+m)+7} \otimes w_{8j+5 \rightarrow 8j+6}, & i = j; \\ 0, & \text{otherwise.} \end{cases}$$

If  $9s \leq j < 10s$ , then  $b_{ij} = 0$ .

If  $10s \leq j < 11s$ , then

$$b_{ij} = \begin{cases} -w_{8(j+m)+4 \rightarrow 8(j+m)+7} \otimes e_{8j+6}, & i = j - 2s; \\ 0, & \text{otherwise.} \end{cases}$$

If  $11s \leq j < 12s$ , then  $b_{ij} = 0$ .

If  $12s \leq j < 13s$ , then

$$b_{ij} = \begin{cases} -w_{8(j+m+1) \rightarrow 8(j+m+1)+2} \otimes e_{8j+7}, & i = j - 3s; \\ 0, & \text{otherwise.} \end{cases}$$

If  $13s \leq j < 14s$ , then

$$b_{ij} = \begin{cases} w_{8(j+m+1) \rightarrow 8(j+m+1)+4} \otimes w_{8j+7 \rightarrow 8(j+1)}, & i = (j+1)_s; \\ -w_{8(j+m+1)+1 \rightarrow 8(j+m+1)+4} \otimes w_{8j+7 \rightarrow 8(j+1)+3}, & i = 4s + (j+1)_s; \\ w_{8(j+m+1)+2 \rightarrow 8(j+m+1)+4} \otimes w_{8j+7 \rightarrow 8(j+1)+4}, & i = 5s + (j+1)_s; \\ w_{8(j+m+1)+3 \rightarrow 8(j+m+1)+4} \otimes w_{8j+7 \rightarrow 8(j+1)+5}, & i = 6s + (j+1)_s; \\ -w_{8(j+m+1) \rightarrow 8(j+m+1)+4} \otimes e_{8j+7}, & i = j - 4s; \\ 0, & \text{otherwise.} \end{cases}$$

If  $14s \leq j < 15s$ , then  $b_{ij} = 0$ .

If  $15s \leq j < 16s$ , then

$$b_{ij} = \begin{cases} e_{8(j+m+1)+5} \otimes w_{8j+7 \rightarrow 8(j+1)+1}, & i = 2s + (j+1)_s; \\ 0, & \text{otherwise.} \end{cases}$$

(26) If  $r_0 = 25$ , then  $\Omega^{25}(Z_t^{(25)})$  is described with  $(10s \times 16s)$  matrix, whose entries  $b_{ij}$  have the following form:

If  $0 \leq j < s$ , then

$$b_{ij} = \begin{cases} w_{8(j+m)+4 \rightarrow 8(j+m)+7} \otimes e_{8j}, & i = j; \\ e_{8(j+m)+7} \otimes w_{8j \rightarrow 8j+1}, & i = j + 2s; \\ 0, & \text{otherwise.} \end{cases}$$

If  $s \leq j < 2s$ , then

$$b_{ij} = \begin{cases} -w_{8(j+m)+4 \rightarrow 8(j+m+1)} \otimes e_{8j}, & i = j - s; \\ -w_{8(j+m)+7 \rightarrow 8(j+m+1)} \otimes w_{8j \rightarrow 8j+1}, & i = j + s; \\ -e_{8(j+m+1)} \otimes w_{8j \rightarrow 8j+2}, & i = j + 2s; \\ -e_{8(j+m+1)} \otimes w_{8j \rightarrow 8j+6}, & i = j + 6s; \\ 0, & \text{otherwise.} \end{cases}$$

If  $2s \leq j < 3s$ , then

$$b_{ij} = \begin{cases} w_{8(j+m+1) \rightarrow 8(j+m+1)+2} \otimes w_{8j+1 \rightarrow 8j+2}, & i = j + s; \\ 0, & \text{otherwise.} \end{cases}$$

If  $3s \leq j < 4s$ , then

$$b_{ij} = \begin{cases} e_{8(j+m+1)+6} \otimes w_{8j+1 \rightarrow 8(j+1)}, & i = s + (j+1)_s; \\ 0, & \text{otherwise.} \end{cases}$$

If  $4s \leq j < 5s$ , then

$$b_{ij} = \begin{cases} -w_{8(j+m+1) \rightarrow 8(j+m+1)+3} \otimes e_{8j+2}, & i = j - s; \\ 0, & \text{otherwise.} \end{cases}$$

If  $5s \leq j < 9s$ , then  $b_{ij} = 0$ .

If  $9s \leq j < 10s$ , then

$$b_{ij} = \begin{cases} -e_{8(j+m+1)+4} \otimes w_{8j+5 \rightarrow 8(j+1)}, & i = (j+1)_s; \\ -w_{8(j+m+1) \rightarrow 8(j+m+1)+4} \otimes w_{8j+5 \rightarrow 8j+6}, & i = j - 2s; \\ 0, & \text{otherwise.} \end{cases}$$

If  $10s \leq j < 11s$ , then  $b_{ij} = 0$ .

If  $11s \leq j < 12s$ , then

$$b_{ij} = \begin{cases} w_{8(j+m+1) \rightarrow 8(j+m+1)+2} \otimes e_{8j+6}, & i = j - 4s; \\ 0, & \text{otherwise.} \end{cases}$$

If  $12s \leq j < 13s$ , then  $b_{ij} = 0$ .

If  $13s \leq j < 14s$ , then

$$b_{ij} = \begin{cases} -w_{8(j+m+1)+4 \rightarrow 8(j+m+1)+7} \otimes w_{8j+7 \rightarrow 8(j+1)}, & i = (j+1)_s; \\ -e_{8(j+m+1)+7} \otimes w_{8j+7 \rightarrow 8(j+1)+1}, & i = 2s + (j+1)_s; \\ 0, & \text{otherwise.} \end{cases}$$

If  $14s \leq j < 15s$ , then

$$b_{ij} = \begin{cases} e_{8(j+m+2)} \otimes w_{8j+7 \rightarrow 8(j+1)+2}, & i = 3s + (j+1)_s; \\ e_{8(j+m+2)} \otimes w_{8j+7 \rightarrow 8(j+1)+6}, & i = 7s + (j+1)_s; \\ w_{8(j+m+1)+3 \rightarrow 8(j+m+2)} \otimes e_{8j+7}, & i = j - 6s; \\ 0, & \text{otherwise.} \end{cases}$$

If  $15s \leq j < 16s$ , then  $b_{ij} = 0$ .

(27) If  $r_0 = 26$ , then  $\Omega^{26}(Z_t^{(25)})$  is described with  $(8s \times 14s)$  matrix, whose entries  $b_{ij}$  have the following form:

If  $s \leq j < 2s$ , then

$$b_{ij} = \begin{cases} -w_{8(j+m-1)+7 \rightarrow 8(j+m)+4} \otimes e_{8j}, & i = j - s; \\ -w_{8(j+m)+1 \rightarrow 8(j+m)+4} \otimes w_{8j \rightarrow 8j+2}, & i = j + s; \\ w_{8(j+m)+2 \rightarrow 8(j+m)+4} \otimes w_{8j \rightarrow 8j+3}, & i = j + 2s; \\ -w_{8(j+m)+3 \rightarrow 8(j+m)+4} \otimes w_{8j \rightarrow 8j+4}, & i = j + 3s; \\ -e_{8(j+m)+4} \otimes w_{8j \rightarrow 8j+5}, & i = j + 4s; \\ 0, & \text{otherwise.} \end{cases}$$

If  $2s \leq j < 3s$ , then

$$b_{ij} = \begin{cases} e_{8(j+m)+6} \otimes w_{8j \rightarrow 8j+1}, & i = j - s; \\ w_{8(j+m)+5 \rightarrow 8(j+m)+6} \otimes w_{8j \rightarrow 8j+6}, & i = j + 4s; \\ 0, & \text{otherwise.} \end{cases}$$

If  $3s \leq j < 4s$ , then

$$b_{ij} = \begin{cases} -e_{8(j+m)+7} \otimes w_{8j+1 \rightarrow 8(j+1)}, & i = (j+1)_s; \\ 0, & \text{otherwise.} \end{cases}$$

If  $4s \leq j < 5s$ , then

$$b_{ij} = \begin{cases} -w_{8(j+m)+1 \rightarrow 8(j+m+1)} \otimes e_{8j+2}, & i = j - 2s; \\ w_{8(j+m)+2 \rightarrow 8(j+m+1)} \otimes w_{8j+2 \rightarrow 8j+3}, & i = j - s; \\ -w_{8(j+m)+3 \rightarrow 8(j+m+1)} \otimes w_{8j+2 \rightarrow 8j+4}, & i = j; \\ 0, & \text{otherwise.} \end{cases}$$

If  $5s \leq j < 8s$ , then  $b_{ij} = 0$ .

If  $8s \leq j < 9s$ , then

$$b_{ij} = \begin{cases} w_{8(j+m)+4 \rightarrow 8(j+m+1)} \otimes e_{8j+5}, & i = j - 3s; \\ 0, & \text{otherwise.} \end{cases}$$

If  $9s \leq j < 10s$ , then

$$b_{ij} = \begin{cases} -w_{8(j+m)+5 \rightarrow 8(j+m+1)} \otimes e_{8j+6}, & i = j - 3s; \\ -e_{8(j+m+1)} \otimes w_{8j+6 \rightarrow 8j+7}, & i = j - 2s; \\ 0, & \text{otherwise.} \end{cases}$$

If  $10s \leq j < 11s$ , then

$$b_{ij} = \begin{cases} -w_{8(j+m+1) \rightarrow 8(j+m+1)+3} \otimes e_{8j+7}, & i = j - 3s; \\ 0, & \text{otherwise.} \end{cases}$$

If  $11s \leq j < 14s$ , then  $b_{ij} = 0$ .

(28) If  $r_0 = 27$ , then  $\Omega^{27}(Z_t^{(25)})$  is described with  $(9s \times 13s)$  matrix, whose entries  $b_{ij}$  have the following form:

If  $s \leq j < 2s$ , then

$$b_{ij} = \begin{cases} -e_{8(j+m)+7} \otimes e_{8j}, & i = j - s; \\ 0, & \text{otherwise.} \end{cases}$$

If  $2s \leq j < 3s$ , then

$$b_{ij} = \begin{cases} -w_{8(j+m+1) \rightarrow 8(j+m+1)+3} \otimes e_{8j+1}, & i = j - s; \\ 0, & \text{otherwise.} \end{cases}$$

If  $3s \leq j < 4s$ , then

$$b_{ij} = \begin{cases} -w_{8(j+m+1)+1 \rightarrow 8(j+m+1)+4} \otimes e_{8j+2}, & i = j - s; \\ 0, & \text{otherwise.} \end{cases}$$

If  $4s \leq j < 7s$ , then  $b_{ij} = 0$ .

If  $7s \leq j < 8s$ , then

$$b_{ij} = \begin{cases} w_{8(j+m+1) \rightarrow 8(j+m+1)+2} \otimes e_{8j+5}, & i = j - 2s; \\ 0, & \text{otherwise.} \end{cases}$$

If  $8s \leq j < 10s$ , then  $b_{ij} = 0$ .

If  $10s \leq j < 11s$ , then

$$b_{ij} = \begin{cases} w_{8(j+m+1)+5 \rightarrow 8(j+m+1)+6} \otimes e_{8j+6}, & i = j - 4s; \\ 0, & \text{otherwise.} \end{cases}$$

If  $11s \leq j < 12s$ , then

$$b_{ij} = \begin{cases} e_{8(j+m+1)+7} \otimes w_{8j+7 \rightarrow 8(j+1)}, & i = (j+1)_s; \\ w_{8(j+m+1)+4 \rightarrow 8(j+m+1)+7} \otimes e_{8j+7}, & i = j - 4s; \\ 0, & \text{otherwise.} \end{cases}$$

If  $12s \leq j < 13s$ , then

$$b_{ij} = \begin{cases} -w_{8(j+m+1)+7 \rightarrow 8(j+m+2)} \otimes w_{8j+7 \rightarrow 8(j+1)}, & i = (j+1)_s; \\ -e_{8(j+m+2)} \otimes w_{8j+7 \rightarrow 8(j+1)+1}, & i = s + (j+1)_s; \\ -w_{8(j+m+1)+4 \rightarrow 8(j+m+2)} \otimes e_{8j+7}, & i = j - 5s; \\ 0, & \text{otherwise.} \end{cases}$$

(29) If  $r_0 = 28$ , then  $\Omega^{28}(Z_t^{(25)})$  is described with  $(8s \times 11s)$  matrix, whose entries  $b_{ij}$  have the following form:

If  $0 \leq j < s$ , then

$$b_{ij} = \begin{cases} w_{8(j+m) \rightarrow 8(j+m)+3} \otimes e_{8j}, & i = j; \\ 0, & \text{otherwise.} \end{cases}$$

If  $s \leq j < 2s$ , then  $b_{ij} = 0$ .

If  $2s \leq j < 3s$ , then

$$b_{ij} = \begin{cases} -w_{8(j+m)+1 \rightarrow 8(j+m+1)} \otimes e_{8j+1}, & i = j - s; \\ 0, & \text{otherwise.} \end{cases}$$

If  $3s \leq j < 4s$ , then

$$b_{ij} = \begin{cases} -w_{8(j+m)+2 \rightarrow 8(j+m)+7} \otimes e_{8j+2}, & i = j - s; \\ w_{8(j+m)+3 \rightarrow 8(j+m)+7} \otimes w_{8j+2 \rightarrow 8j+3}, & i = j; \\ -w_{8(j+m)+4 \rightarrow 8(j+m)+7} \otimes w_{8j+2 \rightarrow 8j+4}, & i = j + s; \\ 0, & \text{otherwise.} \end{cases}$$

If  $4s \leq j < 5s$ , then

$$b_{ij} = \begin{cases} -e_{8(j+m+1)} \otimes w_{8j+3 \rightarrow 8(j+1)}, & i = (j+1)_s; \\ 0, & \text{otherwise.} \end{cases}$$

If  $5s \leq j < 6s$ , then

$$b_{ij} = \begin{cases} -w_{8(j+m+1) \rightarrow 8(j+m+1)+1} \otimes w_{8j+4 \rightarrow 8(j+1)}, & i = (j+1)_s; \\ 0, & \text{otherwise.} \end{cases}$$

If  $6s \leq j < 7s$ , then

$$b_{ij} = \begin{cases} -w_{8(j+m)+5 \rightarrow 8(j+m+1)} \otimes e_{8j+5}, & i = j - s; \\ w_{8(j+m)+6 \rightarrow 8(j+m+1)} \otimes w_{8j+5 \rightarrow 8j+6}, & i = j; \\ -w_{8(j+m)+7 \rightarrow 8(j+m+1)} \otimes w_{8j+5 \rightarrow 8j+7}, & i = j + s; \\ 0, & \text{otherwise.} \end{cases}$$

If  $7s \leq j < 8s$ , then

$$b_{ij} = \begin{cases} w_{8(j+m)+6 \rightarrow 8(j+m)+7} \otimes e_{8j+6}, & i = j - s; \\ -e_{8(j+m)+7} \otimes w_{8j+6 \rightarrow 8j+7}, & i = j; \\ 0, & \text{otherwise.} \end{cases}$$

If  $8s \leq j < 9s$ , then

$$b_{ij} = \begin{cases} w_{8(j+m+1) \rightarrow 8(j+m+1)+2} \otimes w_{8j+7 \rightarrow 8(j+1)}, & i = (j+1)_s; \\ 0, & \text{otherwise.} \end{cases}$$

If  $9s \leq j < 10s$ , then

$$b_{ij} = \begin{cases} -w_{8(j+m+1) \rightarrow 8(j+m+1)+4} \otimes w_{8j+7 \rightarrow 8(j+1)}, & i = (j+1)_s; \\ -w_{8(j+m+1)+1 \rightarrow 8(j+m+1)+4} \otimes w_{8j+7 \rightarrow 8(j+1)+1}, & i = s + (j+1)_s; \\ -w_{8(j+m)+7 \rightarrow 8(j+m+1)+4} \otimes e_{8j+7}, & i = j - 2s; \\ 0, & \text{otherwise.} \end{cases}$$

If  $10s \leq j < 11s$ , then

$$b_{ij} = \begin{cases} w_{8(j+m+1) \rightarrow 8(j+m+1)+6} \otimes w_{8j+7 \rightarrow 8(j+1)}, & i = (j+1)_s; \\ w_{8(j+m+1)+5 \rightarrow 8(j+m+1)+6} \otimes w_{8j+7 \rightarrow 8(j+1)+5}, & i = 5s + (j+1)_s; \\ 0, & \text{otherwise.} \end{cases}$$

(II) Represent an arbitrary  $t_0 \in \mathbb{N}$  in the form  $t_0 = 29\ell_0 + r_0$ , where  $0 \leq r_0 \leq 28$ . Then  $\Omega^{t_0}(Z_t^{(25)})$  is a  $\Omega^{r_0}(Z_t^{(25)})$ , whose left components twisted by  $\sigma^{\ell_0}$ .

**Proposition 21** (Translates for the case 26). (I) Let  $r_0 \in \mathbb{N}$ ,  $r_0 < 29$ .  $r_0$ -translates of the elements  $Z_t^{(26)}$  are described by the following way.

(1) If  $r_0 = 0$ , then  $\Omega^0(Z_t^{(26)})$  is described with  $(8s \times 10s)$  matrix with two nonzero entries:

$$b_{j,(2)_s} = w_{8(j+m) \rightarrow 8(j+m)+4} \otimes e_{8j};$$

$$b_{j-s,s+(2)_s} = w_{8(j+m) \rightarrow 8(j+m)+6} \otimes e_{8j}.$$

(2) If  $r_0 = 1$ , then  $\Omega^1(Z_t^{(26)})$  is described with  $(9s \times 8s)$  matrix with the following nonzero entries:

$$b_{s+(j+1)_s,s+(1)_s} = w_{8(j+m+1)+5 \rightarrow 8(j+m+1)+6} \otimes w_{8j+1 \rightarrow 8(j+1)};$$

$$b_{(j+1)_s,5s+(1)_s} = w_{8(j+m+1)+1 \rightarrow 8(j+m+1)+4} \otimes w_{8j+5 \rightarrow 8(j+1)};$$

$$b_{j+s,7s+(1)_s} = -w_{8(j+m+1) \rightarrow 8(j+m+2)} \otimes e_{8j+7}.$$

(3) If  $r_0 = 2$ , then  $\Omega^2(Z_t^{(26)})$  is described with  $(8s \times 9s)$  matrix with the following nonzero entries:

$$b_{(j+1)_s,(1)_s} = e_{8(j+m)+7} \otimes w_{8j \rightarrow 8(j+1)};$$

$$b_{(j+1)_s,s+(1)_s} = -w_{8(j+m)+7 \rightarrow 8(j+m+1)} \otimes w_{8j+1 \rightarrow 8(j+1)};$$

$$\begin{aligned}
b_{j,s+(1)_s} &= w_{8(j+m)+2 \rightarrow 8(j+m+1)} \otimes e_{8j+1}; \\
b_{(j+1)_s, 5s+(1)_s} &= w_{8(j+m)+7 \rightarrow 8(j+m+1)} \otimes w_{8j+5 \rightarrow 8(j+1)}; \\
b_{j, 5s+(1)_s} &= w_{8(j+m)+6 \rightarrow 8(j+m+1)} \otimes e_{8j+5}.
\end{aligned}$$

(4) If  $r_0 = 3$ , then  $\Omega^3(Z_t^{(26)})$  is described with  $(10s \times 8s)$  matrix with the following nonzero entries:

$$\begin{aligned}
b_{j+s, (1)_s} &= -w_{8(j+m)+6 \rightarrow 8(j+m+1)} \otimes e_{8j}; \\
b_{j+2s, (1)_s} &= w_{8(j+m)+3 \rightarrow 8(j+m+1)} \otimes w_{8j \rightarrow 8j+1}; \\
b_{j+3s, (1)_s} &= w_{8(j+m)+4 \rightarrow 8(j+m+1)} \otimes w_{8j \rightarrow 8j+2}; \\
b_{j+4s, (1)_s} &= w_{8(j+m)+7 \rightarrow 8(j+m+1)} \otimes w_{8j \rightarrow 8j+3}; \\
b_{j+s, s+(1)_s} &= w_{8(j+m)+3 \rightarrow 8(j+m+1)+1} \otimes e_{8j+1}; \\
b_{j+2s, s+(1)_s} &= w_{8(j+m)+4 \rightarrow 8(j+m+1)+1} \otimes w_{8j+1 \rightarrow 8j+2}; \\
b_{j+3s, s+(1)_s} &= w_{8(j+m)+7 \rightarrow 8(j+m+1)+1} \otimes w_{8j+1 \rightarrow 8j+3}; \\
b_{j+s, 5s+(1)_s} &= w_{8(j+m)+7 \rightarrow 8(j+m+1)+5} \otimes e_{8j+5}.
\end{aligned}$$

(5) If  $r_0 = 4$ , then  $\Omega^4(Z_t^{(26)})$  is described with  $(11s \times 8s)$  matrix with the following nonzero entries:

$$\begin{aligned}
b_{s+(j+1)_s, 0} &= e_{8(j+m+1)} \otimes w_{8j \rightarrow 8(j+1)}; \\
b_{(j+1)_s, 5s} &= -w_{8(j+m)+7 \rightarrow 8(j+m+1)+5} \otimes w_{8j+5 \rightarrow 8(j+1)}; \\
b_{(j+1)_s, 6s} &= w_{8(j+m)+7 \rightarrow 8(j+m+1)+6} \otimes w_{8j+6 \rightarrow 8(j+1)}; \\
b_{(j+1)_s, 7s} &= -w_{8(j+m)+7 \rightarrow 8(j+m+1)+7} \otimes w_{8j+7 \rightarrow 8(j+1)}; \\
b_{2s+(j+1)_s, 7s} &= w_{8(j+m+1)+3 \rightarrow 8(j+m+1)+7} \otimes w_{8j+7 \rightarrow 8(j+1)+1}.
\end{aligned}$$

(6) If  $r_0 = 5$ , then  $\Omega^5(Z_t^{(26)})$  is described with  $(11s \times 9s)$  matrix with the following nonzero entries:

$$\begin{aligned}
b_{2s+(j+1)_s, 0} &= -e_{8(j+m+1)+1} \otimes w_{8j \rightarrow 8(j+1)}; \\
b_{(j+1)_s, s} &= e_{8(j+m+1)+5} \otimes w_{8j \rightarrow 8(j+1)}; \\
b_{s+(j+1)_s, 5s} &= w_{8(j+m+1)+3 \rightarrow 8(j+m+1)+7} \otimes w_{8j+4 \rightarrow 8(j+1)}; \\
b_{3s+(j+1)_s, 8s} &= -w_{8(j+m+1)+4 \rightarrow 8(j+m+2)} \otimes w_{8j+7 \rightarrow 8(j+1)+1}; \\
b_{4s+(j+1)_s, 8s} &= -w_{8(j+m+1)+7 \rightarrow 8(j+m+2)} \otimes w_{8j+7 \rightarrow 8(j+1)+2}; \\
b_{5s+(j+1)_s, 8s} &= -e_{8(j+m+2)} \otimes w_{8j+7 \rightarrow 8(j+1)+3}.
\end{aligned}$$

(7) If  $r_0 = 6$ , then  $\Omega^6(Z_t^{(26)})$  is described with  $(13s \times 8s)$  matrix with the following nonzero entries:

$$\begin{aligned}
b_{(j+1)_s, 0} &= -e_{8(j+m)+7} \otimes w_{8j \rightarrow 8(j+1)}; \\
b_{(j+1)_s, s} &= w_{8(j+m)+7 \rightarrow 8(j+m+1)+2} \otimes w_{8j+1 \rightarrow 8(j+1)}; \\
b_{(j+1)_s, 2s} &= -w_{8(j+m)+7 \rightarrow 8(j+m+1)+3} \otimes w_{8j+2 \rightarrow 8(j+1)}; \\
b_{s+(j+1)_s, 3s} &= -w_{8(j+m+1) \rightarrow 8(j+m+1)+4} \otimes w_{8j+3 \rightarrow 8(j+1)}; \\
b_{s+(j+1)_s, 4s} &= -w_{8(j+m+1) \rightarrow 8(j+m+1)+5} \otimes w_{8j+4 \rightarrow 8(j+1)}; \\
b_{3s+(j+1)_s, 7s} &= w_{8(j+m+1)+5 \rightarrow 8(j+m+2)} \otimes w_{8j+7 \rightarrow 8(j+1)+2}.
\end{aligned}$$

(8) If  $r_0 = 7$ , then  $\Omega^7(Z_t^{(26)})$  is described with  $(14s \times 10s)$  matrix with the following nonzero entries:

$$\begin{aligned}
b_{2s+(j+1)_s, s} &= -e_{8(j+m+1)+6} \otimes w_{8j \rightarrow 8(j+1)}; \\
b_{3s+(j+1)_s, s} &= -w_{8(j+m+1)+5 \rightarrow 8(j+m+1)+6} \otimes w_{8j \rightarrow 8(j+1)};
\end{aligned}$$

$$\begin{aligned}
b_{(j+1)s,3s} &= w_{8(j+m+1)+2 \rightarrow 8(j+m+1)+4} \otimes w_{8j+2 \rightarrow 8(j+1)}; \\
b_{3s+(j+1)s,5s} &= w_{8(j+m+1)+5 \rightarrow 8(j+m+2)} \otimes w_{8j+4 \rightarrow 8(j+1)}; \\
b_{4s+(j+1)s,9s} &= -w_{8(j+m+1)+7 \rightarrow 8(j+m+2)+5} \otimes w_{8j+7 \rightarrow 8(j+1)+1}.
\end{aligned}$$

(9) If  $r_0 = 8$ , then  $\Omega^8(Z_t^{(26)})$  is described with  $(16s \times 11s)$  matrix with the following nonzero entries:

$$\begin{aligned}
b_{(j+1)s,0} &= e_{8(j+m)+7} \otimes w_{8j \rightarrow 8(j+1)}; \\
b_{2s+(j+1)s,s} &= -e_{8(j+m+1)} \otimes w_{8j \rightarrow 8(j+1)}; \\
b_{s+(j+1)s,4s} &= -w_{8(j+m)+7 \rightarrow 8(j+m+1)+5} \otimes w_{8j+3 \rightarrow 8(j+1)}; \\
b_{s+(j+1)s,5s} &= w_{8(j+m)+7 \rightarrow 8(j+m+1)+6} \otimes w_{8j+4 \rightarrow 8(j+1)}; \\
b_{3s+(j+1)s,10s} &= w_{8(j+m+1)+5 \rightarrow 8(j+m+1)+7} \otimes w_{8j+7 \rightarrow 8(j+1)+1}; \\
b_{4s+(j+1)s,10s} &= -w_{8(j+m+1)+6 \rightarrow 8(j+m+1)+7} \otimes w_{8j+7 \rightarrow 8(j+1)+2}.
\end{aligned}$$

(10) If  $r_0 = 9$ , then  $\Omega^9(Z_t^{(26)})$  is described with  $(16s \times 11s)$  matrix with the following nonzero entries:

$$\begin{aligned}
b_{(j+1)s,0} &= -e_{8(j+m+1)+5} \otimes w_{8j \rightarrow 8(j+1)}; \\
b_{s+(j+1)s,s} &= e_{8(j+m+1)+3} \otimes w_{8j \rightarrow 8(j+1)}; \\
b_{3s+(j+1)s,2s} &= e_{8(j+m+1)+1} \otimes w_{8j \rightarrow 8(j+1)}; \\
b_{2s+(j+1)s,6s} &= -w_{8(j+m+1)+6 \rightarrow 8(j+m+1)+7} \otimes w_{8j+4 \rightarrow 8(j+1)}; \\
b_{4s+(j+1)s,10s} &= w_{8(j+m+2) \rightarrow 8(j+m+2)+6} \otimes w_{8j+7 \rightarrow 8(j+1)+1}.
\end{aligned}$$

(11) If  $r_0 = 10$ , then  $\Omega^{10}(Z_t^{(26)})$  is described with  $(19s \times 13s)$  matrix with the following nonzero entries:

$$\begin{aligned}
b_{(j+1)s,0} &= -e_{8(j+m)+7} \otimes w_{8j \rightarrow 8(j+1)}; \\
b_{s+(j+1)s,s} &= e_{8(j+m+1)} \otimes w_{8j \rightarrow 8(j+1)}; \\
b_{2s+(j+1)s,4s} &= -w_{8(j+m+1) \rightarrow 8(j+m+1)+6} \otimes w_{8j+3 \rightarrow 8(j+1)}; \\
b_{4s+(j+1)s,11s} &= w_{8(j+m+1)+1 \rightarrow 8(j+m+1)+7} \otimes w_{8j+7 \rightarrow 8(j+1)+1}; \\
b_{3s+(j+1)s,12s} &= w_{8(j+m+1)+6 \rightarrow 8(j+m+2)} \otimes w_{8j+7 \rightarrow 8(j+1)+1}.
\end{aligned}$$

(12) If  $r_0 = 11$ , then  $\Omega^{11}(Z_t^{(26)})$  is described with  $(18s \times 14s)$  matrix with the following nonzero entries:

$$\begin{aligned}
b_{(j+1)s,0} &= e_{8(j+m+1)+2} \otimes w_{8j \rightarrow 8(j+1)}; \\
b_{2s+(j+1)s,s} &= e_{8(j+m+1)+4} \otimes w_{8j \rightarrow 8(j+1)}; \\
b_{s+(j+1)s,2s} &= -e_{8(j+m+1)+6} \otimes w_{8j \rightarrow 8(j+1)}; \\
b_{4s+(j+1)s,3s} &= e_{8(j+m+1)+5} \otimes w_{8j \rightarrow 8(j+1)}; \\
b_{3s+(j+1)s,6s} &= w_{8(j+m+1)+1 \rightarrow 8(j+m+1)+7} \otimes w_{8j+3 \rightarrow 8(j+1)}; \\
b_{5s+(j+1)s,7s} &= w_{8(j+m+1)+7 \rightarrow 8(j+m+2)} \otimes w_{8j+4 \rightarrow 8(j+1)+1}; \\
b_{6s+(j+1)s,7s} &= e_{8(j+m+2)} \otimes w_{8j+4 \rightarrow 8(j+1)+2}; \\
b_{5s+(j+1)s,11s} &= w_{8(j+m+1)+7 \rightarrow 8(j+m+2)+5} \otimes w_{8j+7 \rightarrow 8(j+1)+1}.
\end{aligned}$$

(13) If  $r_0 = 12$ , then  $\Omega^{12}(Z_t^{(26)})$  is described with  $(19s \times 16s)$  matrix with the following nonzero entries:

$$\begin{aligned}
b_{(j+1)s,0} &= e_{8(j+m)+7} \otimes w_{8j \rightarrow 8(j+1)}; \\
b_{2s+(j+1)s,s} &= e_{8(j+m)+7} \otimes w_{8j \rightarrow 8(j+1)}; \\
b_{(j+1)s,2s} &= w_{8(j+m)+7 \rightarrow 8(j+m+1)} \otimes w_{8j \rightarrow 8(j+1)};
\end{aligned}$$



$$\begin{aligned}
b_{s+(j+1)s,2s} &= -e_{8(j+m+1)} \otimes w_{8j \rightarrow 8(j+1)}; \\
b_{2s+(j+1)s,2s} &= -w_{8(j+m)+7 \rightarrow 8(j+m+1)} \otimes w_{8j \rightarrow 8(j+1)}; \\
b_{(j+1)s,5s} &= w_{8(j+m)+7 \rightarrow 8(j+m+1)+1} \otimes w_{8j+2 \rightarrow 8(j+1)}; \\
b_{s+(j+1)s,5s} &= -w_{8(j+m+1) \rightarrow 8(j+m+1)+1} \otimes w_{8j+2 \rightarrow 8(j+1)}; \\
b_{2s+(j+1)s,5s} &= -w_{8(j+m)+7 \rightarrow 8(j+m+1)+1} \otimes w_{8j+2 \rightarrow 8(j+1)}; \\
b_{(j+1)s,6s} &= w_{8(j+m)+7 \rightarrow 8(j+m+1)+2} \otimes w_{8j+3 \rightarrow 8(j+1)}; \\
b_{s+(j+1)s,6s} &= -w_{8(j+m+1) \rightarrow 8(j+m+1)+2} \otimes w_{8j+3 \rightarrow 8(j+1)}; \\
b_{2s+(j+1)s,6s} &= -w_{8(j+m)+7 \rightarrow 8(j+m+1)+2} \otimes w_{8j+3 \rightarrow 8(j+1)}; \\
b_{3s+(j+1)s,7s} &= -w_{8(j+m+1)+2 \rightarrow 8(j+m+1)+3} \otimes w_{8j+4 \rightarrow 8(j+1)+1}; \\
b_{5s+(j+1)s,8s} &= e_{8(j+m+1)+5} \otimes w_{8j+4 \rightarrow 8(j+1)+2}; \\
b_{3s+(j+1)s,14s} &= w_{8(j+m+1)+2 \rightarrow 8(j+m+1)+7} \otimes w_{8j+7 \rightarrow 8(j+1)+1}; \\
b_{5s+(j+1)s,14s} &= -w_{8(j+m+1)+5 \rightarrow 8(j+m+1)+7} \otimes w_{8j+7 \rightarrow 8(j+1)+2}.
\end{aligned}$$

(14) If  $r_0 = 13$ , then  $\Omega^{13}(Z_t^{(26)})$  is described with  $(18s \times 16s)$  matrix with the following nonzero entries:

$$\begin{aligned}
b_{3s+(j+1)s,0} &= -e_{8(j+m+1)+5} \otimes w_{8j \rightarrow 8(j+1)}; \\
b_{(j+1)s,s} &= -w_{8(j+m+1)+2 \rightarrow 8(j+m+1)+3} \otimes w_{8j \rightarrow 8(j+1)}; \\
b_{s+(j+1)s,s} &= e_{8(j+m+1)+3} \otimes w_{8j \rightarrow 8(j+1)}; \\
b_{2s+(j+1)s,2s} &= e_{8(j+m+1)+6} \otimes w_{8j \rightarrow 8(j+1)}; \\
b_{(j+1)s,6s} &= -w_{8(j+m+1)+2 \rightarrow 8(j+m+2)} \otimes w_{8j+3 \rightarrow 8(j+1)}; \\
b_{4s+(j+1)s,12s} &= -w_{8(j+m+2) \rightarrow 8(j+m+2)+2} \otimes w_{8j+7 \rightarrow 8(j+1)+1}.
\end{aligned}$$

(15) If  $r_0 = 14$ , then  $\Omega^{14}(Z_t^{(26)})$  is described with  $(20s \times 19s)$  matrix with the following nonzero entries:

$$\begin{aligned}
b_{(j+1)s,0} &= -e_{8(j+m)+7} \otimes w_{8j \rightarrow 8(j+1)}; \\
b_{s+(j+1)s,s} &= e_{8(j+m+1)} \otimes w_{8j \rightarrow 8(j+1)}; \\
b_{2s+(j+1)s,2s} &= e_{8(j+m+1)} \otimes w_{8j \rightarrow 8(j+1)}; \\
b_{(j+1)s,5s} &= -w_{8(j+m)+7 \rightarrow 8(j+m+1)+2} \otimes w_{8j+2 \rightarrow 8(j+1)}; \\
b_{s+(j+1)s,5s} &= -w_{8(j+m+1) \rightarrow 8(j+m+1)+2} \otimes w_{8j+2 \rightarrow 8(j+1)}; \\
b_{(j+1)s,6s} &= w_{8(j+m)+7 \rightarrow 8(j+m+1)+3} \otimes w_{8j+3 \rightarrow 8(j+1)}; \\
b_{s+(j+1)s,6s} &= w_{8(j+m+1) \rightarrow 8(j+m+1)+3} \otimes w_{8j+3 \rightarrow 8(j+1)}; \\
b_{2s+(j+1)s,6s} &= -w_{8(j+m+1) \rightarrow 8(j+m+1)+3} \otimes w_{8j+3 \rightarrow 8(j+1)}; \\
b_{3s+(j+1)s,8s} &= -w_{8(j+m+1)+3 \rightarrow 8(j+m+1)+4} \otimes w_{8j+4 \rightarrow 8(j+1)+1}; \\
b_{3s+(j+1)s,16s} &= -w_{8(j+m+1)+3 \rightarrow 8(j+m+1)+7} \otimes w_{8j+7 \rightarrow 8(j+1)+1}.
\end{aligned}$$

(16) If  $r_0 = 15$ , then  $\Omega^{15}(Z_t^{(26)})$  is described with  $(18s \times 18s)$  matrix with the following nonzero entries:

$$\begin{aligned}
b_{s+(j+1)s,s} &= -e_{8(j+m+1)+6} \otimes w_{8j \rightarrow 8(j+1)}; \\
b_{(j+1)s,2s} &= -w_{8(j+m+1)+3 \rightarrow 8(j+m+1)+4} \otimes w_{8j \rightarrow 8(j+1)}; \\
b_{2s+(j+1)s,2s} &= e_{8(j+m+1)+4} \otimes w_{8j \rightarrow 8(j+1)}; \\
b_{3s+(j+1)s,2s} &= w_{8(j+m+1)+1 \rightarrow 8(j+m+1)+4} \otimes w_{8j \rightarrow 8(j+1)}; \\
b_{3s+(j+1)s,3s} &= -e_{8(j+m+1)+1} \otimes w_{8j \rightarrow 8(j+1)}; \\
b_{4s+(j+1)s,4s} &= e_{8(j+m+1)+5} \otimes w_{8j \rightarrow 8(j+1)};
\end{aligned}$$

$$\begin{aligned}
b_{(j+1)s,5s} &= w_{8(j+m+1)+3 \rightarrow 8(j+m+1)+7} \otimes w_{8j+1 \rightarrow 8(j+1)}; \\
b_{s+(j+1)s,5s} &= -w_{8(j+m+1)+6 \rightarrow 8(j+m+1)+7} \otimes w_{8j+1 \rightarrow 8(j+1)}; \\
b_{2s+(j+1)s,5s} &= -w_{8(j+m+1)+4 \rightarrow 8(j+m+1)+7} \otimes w_{8j+1 \rightarrow 8(j+1)}; \\
b_{3s+(j+1)s,6s} &= w_{8(j+m+1)+1 \rightarrow 8(j+m+2)} \otimes w_{8j+2 \rightarrow 8(j+1)}; \\
b_{(j+1)s,7s} &= -w_{8(j+m+1)+3 \rightarrow 8(j+m+1)+7} \otimes w_{8j+3 \rightarrow 8(j+1)}; \\
b_{3s+(j+1)s,7s} &= w_{8(j+m+1)+1 \rightarrow 8(j+m+1)+7} \otimes w_{8j+3 \rightarrow 8(j+1)}; \\
b_{5s+(j+1)s,15s} &= -w_{8(j+m+1)+7 \rightarrow 8(j+m+2)+3} \otimes w_{8j+7 \rightarrow 8(j+1)+1}.
\end{aligned}$$

(17) If  $r_0 = 16$ , then  $\Omega^{16}(Z_t^{(26)})$  is described with  $(19s \times 19s)$  matrix with the following nonzero entries:

$$\begin{aligned}
b_{(j+1)s,0} &= 2e_{8(j+m)+7} \otimes w_{8j \rightarrow 8(j+1)}; \\
b_{2s+(j+1)s,0} &= -e_{8(j+m)+7} \otimes w_{8j \rightarrow 8(j+1)}; \\
b_{s+(j+1)s,s} &= -e_{8(j+m+1)} \otimes w_{8j \rightarrow 8(j+1)}; \\
b_{2s+(j+1)s,2s} &= e_{8(j+m)+7} \otimes w_{8j \rightarrow 8(j+1)}; \\
b_{s+(j+1)s,3s} &= -w_{8(j+m+1) \rightarrow 8(j+m+1)+2} \otimes w_{8j+1 \rightarrow 8(j+1)}; \\
b_{(j+1)s,4s} &= -w_{8(j+m)+7 \rightarrow 8(j+m+1)+3} \otimes w_{8j+2 \rightarrow 8(j+1)}; \\
b_{(j+1)s,6s} &= w_{8(j+m)+7 \rightarrow 8(j+m+1)+4} \otimes w_{8j+3 \rightarrow 8(j+1)}; \\
b_{3s+(j+1)s,16s} &= -w_{8(j+m+1)+4 \rightarrow 8(j+m+1)+7} \otimes w_{8j+7 \rightarrow 8(j+1)+1}.
\end{aligned}$$

(18) If  $r_0 = 17$ , then  $\Omega^{17}(Z_t^{(26)})$  is described with  $(18s \times 18s)$  matrix with the following nonzero entries:

$$\begin{aligned}
b_{(j+1)s,0} &= -2e_{8(j+m+1)+2} \otimes w_{8j \rightarrow 8(j+1)}; \\
b_{(j+1)s,s} &= w_{8(j+m+1)+2 \rightarrow 8(j+m+1)+3} \otimes w_{8j \rightarrow 8(j+1)}; \\
b_{2s+(j+1)s,2s} &= e_{8(j+m+1)+6} \otimes w_{8j \rightarrow 8(j+1)}; \\
b_{3s+(j+1)s,3s} &= -e_{8(j+m+1)+5} \otimes w_{8j \rightarrow 8(j+1)}; \\
b_{(j+1)s,4s} &= -w_{8(j+m+1)+2 \rightarrow 8(j+m+2)} \otimes w_{8j+1 \rightarrow 8(j+1)}; \\
b_{s+(j+1)s,6s} &= w_{8(j+m+1)+4 \rightarrow 8(j+m+1)+7} \otimes w_{8j+3 \rightarrow 8(j+1)}; \\
b_{s+(j+1)s,7s} &= w_{8(j+m+1)+4 \rightarrow 8(j+m+2)} \otimes w_{8j+3 \rightarrow 8(j+1)}; \\
b_{4s+(j+1)s,8s} &= -w_{8(j+m+1)+7 \rightarrow 8(j+m+2)} \otimes w_{8j+4 \rightarrow 8(j+1)+1}; \\
b_{5s+(j+1)s,8s} &= -e_{8(j+m+2)} \otimes w_{8j+4 \rightarrow 8(j+1)+1}; \\
b_{4s+(j+1)s,13s} &= w_{8(j+m+1)+7 \rightarrow 8(j+m+2)+2} \otimes w_{8j+7 \rightarrow 8(j+1)+1}.
\end{aligned}$$

(19) If  $r_0 = 18$ , then  $\Omega^{18}(Z_t^{(26)})$  is described with  $(19s \times 20s)$  matrix with the following nonzero entries:

$$\begin{aligned}
b_{(j+1)s,0} &= -e_{8(j+m)+7} \otimes w_{8j \rightarrow 8(j+1)}; \\
b_{s+(j+1)s,2s} &= -e_{8(j+m+1)} \otimes w_{8j \rightarrow 8(j+1)}; \\
b_{2s+(j+1)s,2s} &= e_{8(j+m+1)} \otimes w_{8j \rightarrow 8(j+1)}; \\
b_{s+(j+1)s,8s} &= -w_{8(j+m+1) \rightarrow 8(j+m+1)+1} \otimes w_{8j+3 \rightarrow 8(j+1)}; \\
b_{2s+(j+1)s,9s} &= -w_{8(j+m+1) \rightarrow 8(j+m+1)+2} \otimes w_{8j+4 \rightarrow 8(j+1)}; \\
b_{5s+(j+1)s,9s} &= -e_{8(j+m+1)+2} \otimes w_{8j+4 \rightarrow 8(j+1)+2}; \\
b_{3s+(j+1)s,10s} &= w_{8(j+m+1)+5 \rightarrow 8(j+m+1)+6} \otimes w_{8j+4 \rightarrow 8(j+1)+1}; \\
b_{3s+(j+1)s,17s} &= w_{8(j+m+1)+5 \rightarrow 8(j+m+1)+7} \otimes w_{8j+7 \rightarrow 8(j+1)+1}; \\
b_{4s+(j+1)s,17s} &= -w_{8(j+m+1)+1 \rightarrow 8(j+m+1)+7} \otimes w_{8j+7 \rightarrow 8(j+1)+1};
\end{aligned}$$

$$b_{5s+(j+1)s,17s} = -w_{8(j+m+1)+2 \rightarrow 8(j+m+1)+7} \otimes w_{8j+7 \rightarrow 8(j+1)+2}.$$

(20) If  $r_0 = 19$ , then  $\Omega^{19}(Z_t^{(26)})$  is described with  $(16s \times 18s)$  matrix with the following nonzero entries:

$$\begin{aligned} b_{(j+1)s,0} &= -e_{8(j+m+1)+3} \otimes w_{8j \rightarrow 8(j+1)}; \\ b_{2s+(j+1)s,0} &= w_{8(j+m+1)+1 \rightarrow 8(j+m+1)+3} \otimes w_{8j \rightarrow 8(j+1)}; \\ b_{s+(j+1)s,s} &= -e_{8(j+m+1)+6} \otimes w_{8j \rightarrow 8(j+1)}; \\ b_{3s+(j+1)s,s} &= -w_{8(j+m+1)+5 \rightarrow 8(j+m+1)+6} \otimes w_{8j \rightarrow 8(j+1)}; \\ b_{2s+(j+1)s,3s} &= -e_{8(j+m+1)+1} \otimes w_{8j \rightarrow 8(j+1)}; \\ b_{2s+(j+1)s,8s} &= -w_{8(j+m+1)+1 \rightarrow 8(j+m+2)} \otimes w_{8j+3 \rightarrow 8(j+1)}; \\ b_{3s+(j+1)s,8s} &= w_{8(j+m+1)+5 \rightarrow 8(j+m+2)} \otimes w_{8j+3 \rightarrow 8(j+1)}; \\ b_{4s+(j+1)s,8s} &= e_{8(j+m+2)} \otimes w_{8j+3 \rightarrow 8(j+1)+1}; \\ b_{2s+(j+1)s,9s} &= -w_{8(j+m+1)+1 \rightarrow 8(j+m+1)+7} \otimes w_{8j+4 \rightarrow 8(j+1)}; \\ b_{4s+(j+1)s,14s} &= -w_{8(j+m+2) \rightarrow 8(j+m+2)+2} \otimes w_{8j+7 \rightarrow 8(j+1)+1}. \end{aligned}$$

(21) If  $r_0 = 20$ , then  $\Omega^{20}(Z_t^{(26)})$  is described with  $(16s \times 19s)$  matrix with the following nonzero entries:

$$\begin{aligned} b_{(j+1)s,0} &= e_{8(j+m)+7} \otimes w_{8j \rightarrow 8(j+1)}; \\ b_{s+(j+1)s,s} &= -e_{8(j+m+1)} \otimes w_{8j \rightarrow 8(j+1)}; \\ b_{s+(j+1)s,5s} &= -w_{8(j+m+1) \rightarrow 8(j+m+1)+5} \otimes w_{8j+2 \rightarrow 8(j+1)}; \\ b_{3s+(j+1)s,8s} &= -e_{8(j+m+1)+6} \otimes w_{8j+3 \rightarrow 8(j+1)+1}; \\ b_{3s+(j+1)s,16s} &= -w_{8(j+m+1)+6 \rightarrow 8(j+m+1)+7} \otimes w_{8j+7 \rightarrow 8(j+1)+1}. \end{aligned}$$

(22) If  $r_0 = 21$ , then  $\Omega^{21}(Z_t^{(26)})$  is described with  $(14s \times 18s)$  matrix with the following nonzero entries:

$$\begin{aligned} b_{(j+1)s,0} &= -e_{8(j+m+1)+2} \otimes w_{8j \rightarrow 8(j+1)}; \\ b_{(j+1)s,s} &= -w_{8(j+m+1)+2 \rightarrow 8(j+m+1)+4} \otimes w_{8j \rightarrow 8(j+1)}; \\ b_{s+(j+1)s,s} &= -e_{8(j+m+1)+4} \otimes w_{8j \rightarrow 8(j+1)}; \\ b_{2s+(j+1)s,2s} &= e_{8(j+m+1)+6} \otimes w_{8j \rightarrow 8(j+1)}; \\ b_{2s+(j+1)s,6s} &= w_{8(j+m+1)+6 \rightarrow 8(j+m+2)} \otimes w_{8j+2 \rightarrow 8(j+1)}; \\ b_{3s+(j+1)s,14s} &= w_{8(j+m+1)+7 \rightarrow 8(j+m+2)+6} \otimes w_{8j+7 \rightarrow 8(j+1)+1}. \end{aligned}$$

(23) If  $r_0 = 22$ , then  $\Omega^{22}(Z_t^{(26)})$  is described with  $(13s \times 19s)$  matrix with the following nonzero entries:

$$\begin{aligned} b_{s+(j+1)s,0} &= e_{8(j+m)+7} \otimes w_{8j \rightarrow 8(j+1)}; \\ b_{(j+1)s,s} &= e_{8(j+m+1)} \otimes w_{8j \rightarrow 8(j+1)}; \\ b_{s+(j+1)s,6s} &= w_{8(j+m)+7 \rightarrow 8(j+m+1)+6} \otimes w_{8j+2 \rightarrow 8(j+1)}; \\ b_{2s+(j+1)s,16s} &= w_{8(j+m+1)+3 \rightarrow 8(j+m+1)+7} \otimes w_{8j+7 \rightarrow 8(j+1)+1}; \\ b_{3s+(j+1)s,16s} &= -w_{8(j+m+1)+4 \rightarrow 8(j+m+1)+7} \otimes w_{8j+7 \rightarrow 8(j+1)+2}. \end{aligned}$$

(24) If  $r_0 = 23$ , then  $\Omega^{23}(Z_t^{(26)})$  is described with  $(11s \times 16s)$  matrix with the following nonzero entries:

$$\begin{aligned} b_{(j+1)s,0} &= -e_{8(j+m+1)+3} \otimes w_{8j \rightarrow 8(j+1)}; \\ b_{s+(j+1)s,3s} &= e_{8(j+m+1)+5} \otimes w_{8j \rightarrow 8(j+1)}; \\ b_{(j+1)s,5s} &= -w_{8(j+m+1)+3 \rightarrow 8(j+m+1)+7} \otimes w_{8j+2 \rightarrow 8(j+1)}; \end{aligned}$$

$$\begin{aligned}
b_{s+(j+1)s,5s} &= w_{8(j+m+1)+5 \rightarrow 8(j+m+1)+7} \otimes w_{8j+2 \rightarrow 8(j+1)}; \\
b_{3s+(j+1)s,5s} &= -e_{8(j+m+1)+7} \otimes w_{8j+2 \rightarrow 8(j+1)+2}; \\
b_{2s+(j+1)s,12s} &= -w_{8(j+m+2) \rightarrow 8(j+m+2)+2} \otimes w_{8j+7 \rightarrow 8(j+1)+1}; \\
b_{2s+(j+1)s,13s} &= -w_{8(j+m+2) \rightarrow 8(j+m+2)+4} \otimes w_{8j+7 \rightarrow 8(j+1)+1}.
\end{aligned}$$

(25) If  $r_0 = 24$ , then  $\Omega^{24}(Z_t^{(26)})$  is described with  $(11s \times 16s)$  matrix with the following nonzero entries:

$$\begin{aligned}
b_{(j+1)s,s} &= -e_{8(j+m+1)} \otimes w_{8j \rightarrow 8(j+1)}; \\
b_{(j+1)s,2s} &= w_{8(j+m+1) \rightarrow 8(j+m+1)+2} \otimes w_{8j+1 \rightarrow 8(j+1)}; \\
b_{(j+1)s,4s} &= -w_{8(j+m+1) \rightarrow 8(j+m+1)+3} \otimes w_{8j+2 \rightarrow 8(j+1)}; \\
b_{2s+(j+1)s,14s} &= w_{8(j+m+1)+5 \rightarrow 8(j+m+2)} \otimes w_{8j+7 \rightarrow 8(j+1)+1}.
\end{aligned}$$

(26) If  $r_0 = 25$ , then  $\Omega^{25}(Z_t^{(26)})$  is described with  $(10s \times 14s)$  matrix with the following nonzero entries:

$$\begin{aligned}
b_{(j+1)s,s} &= -e_{8(j+m+1)+4} \otimes w_{8j \rightarrow 8(j+1)}; \\
b_{s+(j+1)s,2s} &= e_{8(j+m+1)+6} \otimes w_{8j \rightarrow 8(j+1)}; \\
b_{s+(j+1)s,4s} &= -w_{8(j+m+1)+6 \rightarrow 8(j+m+2)} \otimes w_{8j+2 \rightarrow 8(j+1)}; \\
b_{3s+(j+1)s,4s} &= -e_{8(j+m+2)} \otimes w_{8j+2 \rightarrow 8(j+1)+2}; \\
b_{2s+(j+1)s,13s} &= -w_{8(j+m+1)+7 \rightarrow 8(j+m+2)+5} \otimes w_{8j+7 \rightarrow 8(j+1)+1}; \\
b_{3s+(j+1)s,13s} &= -w_{8(j+m+2) \rightarrow 8(j+m+2)+5} \otimes w_{8j+7 \rightarrow 8(j+1)+2}; \\
b_{7s+(j+1)s,13s} &= -w_{8(j+m+2) \rightarrow 8(j+m+2)+5} \otimes w_{8j+7 \rightarrow 8(j+1)+6}.
\end{aligned}$$

(27) If  $r_0 = 26$ , then  $\Omega^{26}(Z_t^{(26)})$  is described with  $(8s \times 13s)$  matrix with the following nonzero entries:

$$\begin{aligned}
b_{(j+1)s,0} &= w_{8(j+m)+7 \rightarrow 8(j+m+1)} \otimes w_{8j \rightarrow 8(j+1)}; \\
b_{(j+1)s,s} &= -e_{8(j+m)+7} \otimes w_{8j \rightarrow 8(j+1)}; \\
b_{2s+(j+1)s,3s} &= -w_{8(j+m+1)+1 \rightarrow 8(j+m+1)+4} \otimes w_{8j+2 \rightarrow 8(j+1)+2}; \\
b_{(j+1)s,4s} &= w_{8(j+m)+7 \rightarrow 8(j+m+1)+5} \otimes w_{8j+2 \rightarrow 8(j+1)}; \\
b_{6s+(j+1)s,10s} &= w_{8(j+m+1)+5 \rightarrow 8(j+m+1)+6} \otimes w_{8j+6 \rightarrow 8(j+1)+6}; \\
b_{(j+1)s,11s} &= w_{8(j+m)+7 \rightarrow 8(j+m+1)+7} \otimes w_{8j+7 \rightarrow 8(j+1)}; \\
b_{2s+(j+1)s,11s} &= w_{8(j+m+1)+1 \rightarrow 8(j+m+1)+7} \otimes w_{8j+7 \rightarrow 8(j+1)+2}; \\
b_{3s+(j+1)s,11s} &= -w_{8(j+m+1)+2 \rightarrow 8(j+m+1)+7} \otimes w_{8j+7 \rightarrow 8(j+1)+3}; \\
b_{4s+(j+1)s,11s} &= w_{8(j+m+1)+3 \rightarrow 8(j+m+1)+7} \otimes w_{8j+7 \rightarrow 8(j+1)+4}; \\
b_{5s+(j+1)s,11s} &= w_{8(j+m+1)+4 \rightarrow 8(j+m+1)+7} \otimes w_{8j+7 \rightarrow 8(j+1)+5}; \\
b_{2s+(j+1)s,12s} &= -w_{8(j+m+1)+1 \rightarrow 8(j+m+2)} \otimes w_{8j+7 \rightarrow 8(j+1)+2}; \\
b_{3s+(j+1)s,12s} &= w_{8(j+m+1)+2 \rightarrow 8(j+m+2)} \otimes w_{8j+7 \rightarrow 8(j+1)+3}; \\
b_{4s+(j+1)s,12s} &= -w_{8(j+m+1)+3 \rightarrow 8(j+m+2)} \otimes w_{8j+7 \rightarrow 8(j+1)+4}; \\
b_{5s+(j+1)s,12s} &= -w_{8(j+m+1)+4 \rightarrow 8(j+m+2)} \otimes w_{8j+7 \rightarrow 8(j+1)+5}.
\end{aligned}$$

(28) If  $r_0 = 27$ , then  $\Omega^{27}(Z_t^{(26)})$  is described with  $(9s \times 11s)$  matrix with the following nonzero entries:

$$\begin{aligned}
b_{(j+1)s,6s} &= -w_{8(j+m+1)+7 \rightarrow 8(j+m+2)} \otimes w_{8j+5 \rightarrow 8(j+1)}; \\
b_{(j+1)s,7s} &= -e_{8(j+m+1)+7} \otimes w_{8j+6 \rightarrow 8(j+1)}; \\
b_{(j+1)s,9s} &= -w_{8(j+m+1)+7 \rightarrow 8(j+m+2)+4} \otimes w_{8j+7 \rightarrow 8(j+1)}.
\end{aligned}$$

(29) If  $r_0 = 28$ , then  $\Omega^{28}(Z_t^{(26)})$  is described with  $(8s \times 11s)$  matrix with the following nonzero entries:

$$\begin{aligned} b_{(j+1)s,0} &= e_{8(j+m+1)} \otimes w_{8j \rightarrow 8(j+1)}; \\ b_{j+3s,s} &= w_{8(j+m)+4 \rightarrow 8(j+m+1)+4} \otimes w_{8j+1 \rightarrow 8j+4}; \\ b_{j+6s,s} &= w_{8(j+m)+7 \rightarrow 8(j+m+1)+4} \otimes w_{8j+1 \rightarrow 8j+7}; \\ b_{j-s,7s} &= -w_{8(j+m)+6 \rightarrow 8(j+m+1)+6} \otimes w_{8j+5 \rightarrow 8j+6}; \\ b_{j,7s} &= w_{8(j+m)+7 \rightarrow 8(j+m+1)+6} \otimes w_{8j+5 \rightarrow 8j+7}; \\ b_{j-3s,10s} &= -w_{8(j+m)+7 \rightarrow 8(j+m+1)+7} \otimes e_{8j+7}. \end{aligned}$$

(II) Represent an arbitrary  $t_0 \in \mathbb{N}$  in the form  $t_0 = 29\ell_0 + r_0$ , where  $0 \leq r_0 \leq 28$ . Then  $\Omega^{t_0}(Z_t^{(26)})$  is a  $\Omega^{r_0}(Z_t^{(26)})$ , whose left components twisted by  $\sigma^{\ell_0}$ , and coefficients multiplied by  $(-1)^{\ell_0}$ .

**Proposition 22** (Translates for the case 27). (I) Let  $r_0 \in \mathbb{N}$ ,  $r_0 < 29$ .  $r_0$ -translates of the elements  $Z_t^{(27)}$  are described by the following way.

(1) If  $r_0 = 0$ , then  $\Omega^0(Z_t^{(27)})$  is described with  $(8s \times 9s)$  matrix, whose entries  $b_{ij}$  have the following form:

If  $0 \leq j < 5s$ , then

$$b_{ij} = \begin{cases} w_{8(j+m)+j_2 \rightarrow 8(j+m)+7+j_2} \otimes e_{8j+j_2}, & i = j; \\ 0, & \text{otherwise.} \end{cases}$$

If  $5s \leq j < 7s$ , then  $b_{ij} = 0$ .

If  $7s \leq j < 8s$ , then

$$b_{ij} = \begin{cases} -w_{8(j+m)+7 \rightarrow 8(j+m+1)+4} \otimes e_{8j+7}, & i = j; \\ 0, & \text{otherwise.} \end{cases}$$

If  $8s \leq j < 9s$ , then  $b_{ij} = 0$ .

(2) If  $r_0 = 1$ , then  $\Omega^1(Z_t^{(27)})$  is described with  $(9s \times 8s)$  matrix, whose entries  $b_{ij}$  have the following form:

If  $0 \leq j < s$ , then

$$b_{ij} = \begin{cases} -w_{8(j+m)+1 \rightarrow 8(j+m+1)} \otimes e_{8j}, & i = j; \\ 0, & \text{otherwise.} \end{cases}$$

If  $s \leq j < 5s$ , then

$$b_{ij} = \begin{cases} -w_{8(j+m)+1+j_2+2f(j_2,4) \rightarrow 8(j+m+1)+j_2} \otimes e_{8j+j_2}, & i = j + s; \\ 0, & \text{otherwise.} \end{cases}$$

If  $5s \leq j < 7s$ , then  $b_{ij} = 0$ .

If  $7s \leq j < 8s$ , then

$$b_{ij} = \begin{cases} -w_{8(j+m+1) \rightarrow 8(j+m+1)+7} \otimes e_{8j+7}, & i = j + s; \\ 0, & \text{otherwise.} \end{cases}$$

(3) If  $r_0 = 2$ , then  $\Omega^2(Z_t^{(27)})$  is described with  $(8s \times 8s)$  matrix, whose entries  $b_{ij}$  have the following form:

If  $0 \leq j < s$ , then

$$b_{ij} = \begin{cases} w_{8(j+m)+2 \rightarrow 8(j+m+1)} \otimes w_{8j \rightarrow 8j+1}, & i = j + s; \\ 0, & \text{otherwise.} \end{cases}$$

If  $s \leq j < 5s$ , then

$$b_{ij} = \begin{cases} w_{8(j+m)+7 \rightarrow 8(j+m+1)+j_2} \otimes w_{8j+j_2 \rightarrow 8(j+1)}, & i = (j+1)_s; \\ 0, & \text{otherwise.} \end{cases}$$

If  $5s \leq j < 7s$ , then  $b_{ij} = 0$ .

If  $7s \leq j < 8s$ , then

$$b_{ij} = \begin{cases} w_{8(j+m+1)+2 \rightarrow 8(j+m+1)+7} \otimes w_{8j+7 \rightarrow 8(j+1)+1}, & i = s + (j+1)_s; \\ 0, & \text{otherwise.} \end{cases}$$

(4) If  $r_0 = 3$ , then  $\Omega^3(Z_t^{(27)})$  is described with  $(10s \times 9s)$  matrix, whose entries  $b_{ij}$  have the following form:

If  $0 \leq j < s$ , then

$$b_{ij} = \begin{cases} w_{8(j+m)+3 \rightarrow 8(j+m+1)+1} \otimes w_{8j \rightarrow 8j+1}, & i = j + 2s; \\ w_{8(j+m)+4 \rightarrow 8(j+m+1)+1} \otimes w_{8j \rightarrow 8j+2}, & i = j + 3s; \\ w_{8(j+m)+7 \rightarrow 8(j+m+1)+1} \otimes w_{8j \rightarrow 8j+3}, & i = j + 4s; \\ 0, & \text{otherwise.} \end{cases}$$

If  $s \leq j < 5s$ , then  $b_{ij} = 0$ .

If  $5s \leq j < 6s$ , then

$$b_{ij} = \begin{cases} w_{8(j+m+1)+2 \rightarrow 8(j+m+1)+7} \otimes w_{8j+4 \rightarrow 8(j+1)}, & i = (j+1)_s; \\ 0, & \text{otherwise.} \end{cases}$$

If  $6s \leq j < 9s$ , then  $b_{ij} = 0$ .

(5) If  $r_0 = 4$ , then  $\Omega^4(Z_t^{(27)})$  is described with  $(11s \times 8s)$  matrix, whose entries  $b_{ij}$  have the following form:

If  $0 \leq j < s$ , then

$$b_{ij} = \begin{cases} w_{8(j+m)+3 \rightarrow 8(j+m)+7} \otimes w_{8j \rightarrow 8j+1}, & i = j + 2s; \\ 0, & \text{otherwise.} \end{cases}$$

If  $s \leq j < 4s$ , then

$$b_{ij} = \begin{cases} w_{8(j+m)+7 \rightarrow 8(j+m+1)+1+j_2} \otimes w_{8j+j_2 \rightarrow 8(j+1)}, & i = (j+1)_s; \\ 0, & \text{otherwise.} \end{cases}$$

If  $4s \leq j < 8s$ , then  $b_{ij} = 0$ .

(6) If  $r_0 = 5$ , then  $\Omega^5(Z_t^{(27)})$  is described with  $(11s \times 10s)$  matrix, whose entries  $b_{ij}$  have the following form:

If  $0 \leq j < s$ , then

$$b_{ij} = \begin{cases} w_{8(j+m)+4 \rightarrow 8(j+m+1)+2} \otimes w_{8j \rightarrow 8j+1}, & i = j + 3s; \\ w_{8(j+m)+7 \rightarrow 8(j+m+1)+2} \otimes w_{8j \rightarrow 8j+2}, & i = j + 4s; \\ 0, & \text{otherwise.} \end{cases}$$

If  $s \leq j < 4s$ , then  $b_{ij} = 0$ .

If  $4s \leq j < 5s$ , then

$$b_{ij} = \begin{cases} w_{8(j+m+1)+3 \rightarrow 8(j+m+1)+7} \otimes w_{8j+3 \rightarrow 8(j+1)}, & i = s + (j + 1)_s; \\ 0, & \text{otherwise.} \end{cases}$$

If  $5s \leq j < 6s$ , then

$$b_{ij} = \begin{cases} -w_{8(j+m+1)+3 \rightarrow 8(j+m+2)} \otimes w_{8j+4 \rightarrow 8(j+1)}, & i = s + (j + 1)_s; \\ 0, & \text{otherwise.} \end{cases}$$

If  $6s \leq j < 8s$ , then  $b_{ij} = 0$ .

If  $8s \leq j < 9s$ , then

$$b_{ij} = \begin{cases} -w_{8(j+m+1)+4 \rightarrow 8(j+m+2)+1} \otimes w_{8j+7 \rightarrow 8(j+1)+1}, & i = 3s + (j + 1)_s; \\ -w_{8(j+m+1)+7 \rightarrow 8(j+m+2)+1} \otimes w_{8j+7 \rightarrow 8(j+1)+2}, & i = 4s + (j + 1)_s; \\ 0, & \text{otherwise.} \end{cases}$$

If  $9s \leq j < 10s$ , then  $b_{ij} = 0$ .

(7) If  $r_0 = 6$ , then  $\Omega^6(Z_t^{(27)})$  is described with  $(13s \times 11s)$  matrix, whose entries  $b_{ij}$  have the following form:

If  $0 \leq j < s$ , then

$$b_{ij} = \begin{cases} w_{8(j+m)+4 \rightarrow 8(j+m)+7} \otimes w_{8j \rightarrow 8j+1}, & i = j + 2s; \\ 0, & \text{otherwise.} \end{cases}$$

If  $s \leq j < 2s$ , then

$$b_{ij} = \begin{cases} -e_{8(j+m+1)} \otimes w_{8j \rightarrow 8(j+1)}, & i = s + (j + 1)_s; \\ 0, & \text{otherwise.} \end{cases}$$

If  $2s \leq j < 3s$ , then

$$b_{ij} = \begin{cases} -w_{8(j+m)+7 \rightarrow 8(j+m+1)+3} \otimes w_{8j+1 \rightarrow 8(j+1)}, & i = (j + 1)_s; \\ 0, & \text{otherwise.} \end{cases}$$

If  $3s \leq j < 4s$ , then

$$b_{ij} = \begin{cases} -w_{8(j+m)+7 \rightarrow 8(j+m+1)+4} \otimes w_{8j+2 \rightarrow 8(j+1)}, & i = (j + 1)_s; \\ 0, & \text{otherwise.} \end{cases}$$

If  $4s \leq j < 6s$ , then  $b_{ij} = 0$ .

If  $6s \leq j < 7s$ , then

$$b_{ij} = \begin{cases} -w_{8(j+m+1) \rightarrow 8(j+m+1)+1} \otimes w_{8j+4 \rightarrow 8(j+1)}, & i = s + (j + 1)_s; \\ e_{8(j+m+1)+1} \otimes w_{8j+4 \rightarrow 8(j+1)+3}, & i = 5s + (j + 1)_s; \\ 0, & \text{otherwise.} \end{cases}$$

If  $7s \leq j < 11s$ , then  $b_{ij} = 0$ .

(8) If  $r_0 = 7$ , then  $\Omega^7(Z_t^{(27)})$  is described with  $(14s \times 11s)$  matrix, whose entries  $b_{ij}$  have the following form:

If  $0 \leq j < s$ , then

$$b_{ij} = \begin{cases} -e_{8(j+m+1)+5} \otimes w_{8j \rightarrow 8(j+1)}, & i = 3s + (j+1)_s; \\ 0, & \text{otherwise.} \end{cases}$$

If  $s \leq j < 2s$ , then

$$b_{ij} = \begin{cases} w_{8(j+m)+7 \rightarrow 8(j+m+1)+3} \otimes w_{8j \rightarrow 8j+1}, & i = j + 3s; \\ 0, & \text{otherwise.} \end{cases}$$

If  $2s \leq j < 4s$ , then  $b_{ij} = 0$ .

If  $4s \leq j < 5s$ , then

$$b_{ij} = \begin{cases} -w_{8(j+m+1)+2 \rightarrow 8(j+m+1)+7} \otimes w_{8j+2 \rightarrow 8(j+1)}, & i = (j+1)_s; \\ w_{8(j+m+1)+4 \rightarrow 8(j+m+1)+7} \otimes w_{8j+2 \rightarrow 8(j+1)}, & i = s + (j+1)_s; \\ 0, & \text{otherwise.} \end{cases}$$

If  $5s \leq j < 6s$ , then  $b_{ij} = 0$ .

If  $6s \leq j < 7s$ , then

$$b_{ij} = \begin{cases} w_{8(j+m+1)+4 \rightarrow 8(j+m+1)+7} \otimes w_{8j+4 \rightarrow 8(j+1)}, & i = s + (j+1)_s; \\ 0, & \text{otherwise.} \end{cases}$$

If  $7s \leq j < 9s$ , then  $b_{ij} = 0$ .

If  $9s \leq j < 10s$ , then

$$b_{ij} = \begin{cases} -w_{8(j+m+1)+7 \rightarrow 8(j+m+2)+2} \otimes w_{8j+7 \rightarrow 8(j+1)+1}, & i = 4s + (j+1)_s; \\ 0, & \text{otherwise.} \end{cases}$$

If  $10s \leq j < 11s$ , then  $b_{ij} = 0$ .

(9) If  $r_0 = 8$ , then  $\Omega^8(Z_t^{(27)})$  is described with  $(16s \times 13s)$  matrix, whose entries  $b_{ij}$  have the following form:

If  $0 \leq j < s$ , then

$$b_{ij} = \begin{cases} e_{8(j+m)+7} \otimes w_{8j \rightarrow 8(j+1)}, & i = (j+1)_s; \\ -w_{8(j+m)+5 \rightarrow 8(j+m)+7} \otimes w_{8j \rightarrow 8j+1}, & i = j + 3s; \\ w_{8(j+m)+6 \rightarrow 8(j+m)+7} \otimes w_{8j \rightarrow 8j+2}, & i = j + 4s; \\ 0, & \text{otherwise.} \end{cases}$$

If  $s \leq j < 2s$ , then

$$b_{ij} = \begin{cases} -w_{8(j+m)+7 \rightarrow 8(j+m+1)} \otimes w_{8j \rightarrow 8(j+1)}, & i = (j+1)_s; \\ w_{8(j+m)+7 \rightarrow 8(j+m+1)} \otimes w_{8j \rightarrow 8(j+1)}, & i = s + (j+1)_s; \\ -e_{8(j+m+1)} \otimes w_{8j \rightarrow 8(j+1)}, & i = 2s + (j+1)_s; \\ 0, & \text{otherwise.} \end{cases}$$



If  $2s \leq j < 3s$ , then

$$b_{ij} = \begin{cases} w_{8(j+m)+7 \rightarrow 8(j+m+1)+4} \otimes w_{8j+1 \rightarrow 8(j+1)}, & i = s + (j+1)_s; \\ 0, & \text{otherwise.} \end{cases}$$

If  $3s \leq j < 6s$ , then  $b_{ij} = 0$ .

If  $6s \leq j < 7s$ , then

$$b_{ij} = \begin{cases} w_{8(j+m)+7 \rightarrow 8(j+m+1)+2} \otimes w_{8j+4 \rightarrow 8(j+1)}, & i = s + (j+1)_s; \\ 0, & \text{otherwise.} \end{cases}$$

If  $7s \leq j < 13s$ , then  $b_{ij} = 0$ .

(10) If  $r_0 = 9$ , then  $\Omega^9(Z_t^{(27)})$  is described with  $(16s \times 14s)$  matrix, whose entries  $b_{ij}$  have the following form:

If  $0 \leq j < s$ , then

$$b_{ij} = \begin{cases} -w_{8(j+m+1)+1 \rightarrow 8(j+m+1)+2} \otimes w_{8j \rightarrow 8(j+1)}, & i = 3s + (j+1)_s; \\ 0, & \text{otherwise.} \end{cases}$$

If  $s \leq j < 2s$ , then

$$b_{ij} = \begin{cases} -w_{8(j+m+1)+3 \rightarrow 8(j+m+1)+4} \otimes w_{8j \rightarrow 8(j+1)}, & i = s + (j+1)_s; \\ -w_{8(j+m+1)+1 \rightarrow 8(j+m+1)+4} \otimes w_{8j \rightarrow 8(j+1)}, & i = 3s + (j+1)_s; \\ 0, & \text{otherwise.} \end{cases}$$

If  $2s \leq j < 3s$ , then

$$b_{ij} = \begin{cases} w_{8(j+m+1)+5 \rightarrow 8(j+m+1)+6} \otimes w_{8j \rightarrow 8(j+1)}, & i = (j+1)_s; \\ e_{8(j+m+1)+6} \otimes w_{8j \rightarrow 8(j+1)}, & i = 2s + (j+1)_s; \\ -w_{8(j+m+1) \rightarrow 8(j+m+1)+6} \otimes w_{8j \rightarrow 8j+1}, & i = j + 2s; \\ 0, & \text{otherwise.} \end{cases}$$

If  $3s \leq j < 4s$ , then

$$b_{ij} = \begin{cases} -e_{8(j+m+1)+5} \otimes w_{8j \rightarrow 8(j+1)}, & i = (j+1)_s; \\ 0, & \text{otherwise.} \end{cases}$$

If  $4s \leq j < 5s$ , then

$$b_{ij} = \begin{cases} w_{8(j+m+1)+6 \rightarrow 8(j+m+1)+7} \otimes w_{8j+1 \rightarrow 8(j+1)}, & i = 2s + (j+1)_s; \\ 0, & \text{otherwise.} \end{cases}$$

If  $5s \leq j < 6s$ , then

$$b_{ij} = \begin{cases} -w_{8(j+m+1)+6 \rightarrow 8(j+m+2)} \otimes w_{8j+2 \rightarrow 8(j+1)}, & i = 2s + (j+1)_s; \\ 0, & \text{otherwise.} \end{cases}$$

If  $6s \leq j < 7s$ , then

$$b_{ij} = \begin{cases} -w_{8(j+m+1)+6 \rightarrow 8(j+m+1)+7} \otimes w_{8j+3 \rightarrow 8(j+1)}, & i = 2s + (j+1)_s; \\ 0, & \text{otherwise.} \end{cases}$$

If  $7s \leq j < 14s$ , then  $b_{ij} = 0$ .

(11) If  $r_0 = 10$ , then  $\Omega^{10}(Z_t^{(27)})$  is described with  $(19s \times 16s)$  matrix, whose entries  $b_{ij}$  have the following form:

If  $0 \leq j < s$ , then

$$b_{ij} = \begin{cases} w_{8(j+m)+1 \rightarrow 8(j+m)+7} \otimes w_{8j \rightarrow 8j+1}, & i = j + 4s; \\ 0, & \text{otherwise.} \end{cases}$$

If  $s \leq j < 2s$ , then

$$b_{ij} = \begin{cases} e_{8(j+m)+7} \otimes w_{8j \rightarrow 8(j+1)}, & i = (j + 1)_s; \\ 0, & \text{otherwise.} \end{cases}$$

If  $2s \leq j < 3s$ , then

$$b_{ij} = \begin{cases} -w_{8(j+m)+6 \rightarrow 8(j+m)+1} \otimes w_{8j \rightarrow 8j+1}, & i = j + s; \\ 0, & \text{otherwise.} \end{cases}$$

If  $3s \leq j < 4s$ , then  $b_{ij} = 0$ .

If  $4s \leq j < 5s$ , then

$$b_{ij} = \begin{cases} -w_{8(j+m+1) \rightarrow 8(j+m+1)+6} \otimes w_{8j+2 \rightarrow 8(j+1)}, & i = 2s + (j + 1)_s; \\ 0, & \text{otherwise.} \end{cases}$$

If  $5s \leq j < 16s$ , then  $b_{ij} = 0$ .

(12) If  $r_0 = 11$ , then  $\Omega^{11}(Z_t^{(27)})$  is described with  $(18s \times 16s)$  matrix, whose entries  $b_{ij}$  have the following form:

If  $0 \leq j < s$ , then

$$b_{ij} = \begin{cases} -w_{8(j+m)+7 \rightarrow 8(j+m+1)+5} \otimes w_{8j \rightarrow 8j+1}, & i = j + 5s; \\ 0, & \text{otherwise.} \end{cases}$$

If  $s \leq j < 2s$ , then  $b_{ij} = 0$ .

If  $2s \leq j < 3s$ , then

$$b_{ij} = \begin{cases} e_{8(j+m+1)+6} \otimes w_{8j \rightarrow 8(j+1)}, & i = s + (j + 1)_s; \\ 0, & \text{otherwise.} \end{cases}$$

If  $3s \leq j < 4s$ , then  $b_{ij} = 0$ .

If  $4s \leq j < 5s$ , then

$$b_{ij} = \begin{cases} -w_{8(j+m+1)+6 \rightarrow 8(j+m+2)} \otimes w_{8j+1 \rightarrow 8(j+1)}, & i = s + (j + 1)_s; \\ 0, & \text{otherwise.} \end{cases}$$

If  $5s \leq j < 6s$ , then

$$b_{ij} = \begin{cases} -w_{8(j+m+1)+1 \rightarrow 8(j+m+1)+7} \otimes w_{8j+2 \rightarrow 8(j+1)}, & i = 3s + (j + 1)_s; \\ 0, & \text{otherwise.} \end{cases}$$

If  $6s \leq j < 7s$ , then

$$b_{ij} = \begin{cases} w_{8(j+m+1)+6 \rightarrow 8(j+m+2)} \otimes w_{8j+3 \rightarrow 8(j+1)}, & i = s + (j + 1)_s; \\ w_{8(j+m+1)+1 \rightarrow 8(j+m+2)} \otimes w_{8j+3 \rightarrow 8(j+1)}, & i = 3s + (j + 1)_s; \\ 0, & \text{otherwise.} \end{cases}$$

If  $7s \leq j < 16s$ , then  $b_{ij} = 0$ .

(13) If  $r_0 = 12$ , then  $\Omega^{12}(Z_t^{(27)})$  is described with  $(19s \times 19s)$  matrix, whose entries  $b_{ij}$  have the following form:

If  $0 \leq j < s$ , then

$$b_{ij} = \begin{cases} -e_{8(j+m)+7} \otimes w_{8j \rightarrow 8(j+1)}, & i = (j+1)_s; \\ -w_{8(j+m)+2 \rightarrow 8(j+m)+7} \otimes w_{8j \rightarrow 8j+1}, & i = j+3s; \\ w_{8(j+m)+5 \rightarrow 8(j+m)+7} \otimes w_{8j \rightarrow 8j+2}, & i = j+5s; \\ 0, & \text{otherwise.} \end{cases}$$

If  $s \leq j < 2s$ , then

$$b_{ij} = \begin{cases} w_{8(j+m)+7 \rightarrow 8(j+m+1)} \otimes w_{8j \rightarrow 8(j+1)}, & i = (j+1)_s; \\ -e_{8(j+m+1)} \otimes w_{8j \rightarrow 8(j+1)}, & i = s + (j+1)_s; \\ -w_{8(j+m)+7 \rightarrow 8(j+m+1)} \otimes w_{8j \rightarrow 8(j+1)}, & i = 2s + (j+1)_s; \\ 0, & \text{otherwise.} \end{cases}$$

If  $2s \leq j < 3s$ , then  $b_{ij} = 0$ .

If  $3s \leq j < 4s$ , then

$$b_{ij} = \begin{cases} w_{8(j+m)+7 \rightarrow 8(j+m+1)+6} \otimes w_{8j+1 \rightarrow 8(j+1)}, & i = (j+1)_s; \\ 0, & \text{otherwise.} \end{cases}$$

If  $4s \leq j < 7s$ , then  $b_{ij} = 0$ .

If  $7s \leq j < 8s$ , then

$$b_{ij} = \begin{cases} -w_{8(j+m)+7 \rightarrow 8(j+m+1)+5} \otimes w_{8j+3 \rightarrow 8(j+1)}, & i = (j+1)_s; \\ w_{8(j+m)+7 \rightarrow 8(j+m+1)+5} \otimes w_{8j+3 \rightarrow 8(j+1)}, & i = 2s + (j+1)_s; \\ 0, & \text{otherwise.} \end{cases}$$

If  $8s \leq j < 19s$ , then  $b_{ij} = 0$ .

(14) If  $r_0 = 13$ , then  $\Omega^{13}(Z_t^{(27)})$  is described with  $(18s \times 18s)$  matrix, whose entries  $b_{ij}$  have the following form:

If  $0 \leq j < s$ , then

$$b_{ij} = \begin{cases} -w_{8(j+m+1) \rightarrow 8(j+m+1)+2} \otimes w_{8j \rightarrow 8j+1}, & i = j+4s; \\ 0, & \text{otherwise.} \end{cases}$$

If  $s \leq j < 2s$ , then  $b_{ij} = 0$ .

If  $2s \leq j < 3s$ , then

$$b_{ij} = \begin{cases} w_{8(j+m+1)+2 \rightarrow 8(j+m+1)+4} \otimes w_{8j \rightarrow 8(j+1)}, & i = (j+1)_s; \\ 0, & \text{otherwise.} \end{cases}$$

If  $3s \leq j < 4s$ , then  $b_{ij} = 0$ .

If  $4s \leq j < 5s$ , then

$$b_{ij} = \begin{cases} -e_{8(j+m+1)+5} \otimes w_{8j \rightarrow 8(j+1)}, & i = 3s + (j+1)_s; \\ 0, & \text{otherwise.} \end{cases}$$

If  $5s \leq j < 6s$ , then

$$b_{ij} = \begin{cases} w_{8(j+m+1)+3 \rightarrow 8(j+m+1)+7} \otimes w_{8j+1 \rightarrow 8(j+1)}, & i = s + (j+1)_s; \\ 0, & \text{otherwise.} \end{cases}$$

If  $6s \leq j < 7s$ , then  $b_{ij} = 0$ .

If  $7s \leq j < 8s$ , then

$$b_{ij} = \begin{cases} w_{8(j+m+1)+2 \rightarrow 8(j+m+1)+7} \otimes w_{8j+3 \rightarrow 8(j+1)}, & i = (j+1)_s; \\ w_{8(j+m+1)+5 \rightarrow 8(j+m+1)+7} \otimes w_{8j+3 \rightarrow 8(j+1)}, & i = 3s + (j+1)_s; \\ 0, & \text{otherwise.} \end{cases}$$

If  $8s \leq j < 18s$ , then  $b_{ij} = 0$ .

(15) If  $r_0 = 14$ , then  $\Omega^{14}(Z_t^{(27)})$  is described with  $(20s \times 19s)$  matrix, whose entries  $b_{ij}$  have the following form:

If  $0 \leq j < s$ , then

$$b_{ij} = \begin{cases} -w_{8(j+m)+3 \rightarrow 8(j+m)+7} \otimes w_{8j \rightarrow 8j+1}, & i = j + 3s; \\ 0, & \text{otherwise.} \end{cases}$$

If  $s \leq j < 2s$ , then

$$b_{ij} = \begin{cases} -e_{8(j+m+1)} \otimes w_{8j \rightarrow 8(j+1)}, & i = s + (j+1)_s; \\ -w_{8(j+m)+3 \rightarrow 8(j+m+1)} \otimes w_{8j \rightarrow 8j+1}, & i = j + 2s; \\ 0, & \text{otherwise.} \end{cases}$$

If  $2s \leq j < 3s$ , then  $b_{ij} = 0$ .

If  $3s \leq j < 4s$ , then

$$b_{ij} = \begin{cases} w_{8(j+m+1) \rightarrow 8(j+m+1)+2} \otimes w_{8j+1 \rightarrow 8(j+1)}, & i = s + (j+1)_s; \\ 0, & \text{otherwise.} \end{cases}$$

If  $4s \leq j < 5s$ , then

$$b_{ij} = \begin{cases} w_{8(j+m)+7 \rightarrow 8(j+m+1)+3} \otimes w_{8j+2 \rightarrow 8(j+1)}, & i = (j+1)_s; \\ w_{8(j+m+1) \rightarrow 8(j+m+1)+3} \otimes w_{8j+2 \rightarrow 8(j+1)}, & i = s + (j+1)_s; \\ 0, & \text{otherwise.} \end{cases}$$

If  $5s \leq j < 6s$ , then  $b_{ij} = 0$ .

If  $6s \leq j < 7s$ , then

$$b_{ij} = \begin{cases} w_{8(j+m)+7 \rightarrow 8(j+m+1)+4} \otimes w_{8j+3 \rightarrow 8(j+1)}, & i = (j+1)_s; \\ w_{8(j+m+1) \rightarrow 8(j+m+1)+4} \otimes w_{8j+3 \rightarrow 8(j+1)}, & i = s + (j+1)_s; \\ -w_{8(j+m+1) \rightarrow 8(j+m+1)+4} \otimes w_{8j+3 \rightarrow 8(j+1)}, & i = 2s + (j+1)_s; \\ 0, & \text{otherwise.} \end{cases}$$

If  $7s \leq j < 19s$ , then  $b_{ij} = 0$ .

(16) If  $r_0 = 15$ , then  $\Omega^{15}(Z_t^{(27)})$  is described with  $(18s \times 18s)$  matrix, whose entries  $b_{ij}$  have the following form:

If  $s \leq j < 2s$ , then

$$b_{ij} = \begin{cases} -w_{8(j+m)+7 \rightarrow 8(j+m+1)+3} \otimes w_{8j \rightarrow 8j+1}, & i = j + 4s; \\ 0, & \text{otherwise.} \end{cases}$$

If  $2s \leq j < 3s$ , then  $b_{ij} = 0$ .

If  $3s \leq j < 4s$ , then

$$b_{ij} = \begin{cases} -e_{8(j+m+1)+5} \otimes w_{8j \rightarrow 8(j+1)}, & i = 4s + (j + 1)_s; \\ 0, & \text{otherwise.} \end{cases}$$

If  $4s \leq j < 5s$ , then

$$b_{ij} = \begin{cases} w_{8(j+m+1)+3 \rightarrow 8(j+m+2)} \otimes w_{8j+1 \rightarrow 8(j+1)}, & i = (j + 1)_s; \\ 0, & \text{otherwise.} \end{cases}$$

If  $5s \leq j < 6s$ , then

$$b_{ij} = \begin{cases} w_{8(j+m+1)+1 \rightarrow 8(j+m+1)+7} \otimes w_{8j+2 \rightarrow 8(j+1)}, & i = 3s + (j + 1)_s; \\ 0, & \text{otherwise.} \end{cases}$$

If  $6s \leq j < 7s$ , then

$$b_{ij} = \begin{cases} w_{8(j+m+1)+3 \rightarrow 8(j+m+1)+7} \otimes w_{8j+3 \rightarrow 8(j+1)}, & i = (j + 1)_s; \\ -w_{8(j+m+1)+1 \rightarrow 8(j+m+1)+7} \otimes w_{8j+3 \rightarrow 8(j+1)}, & i = 3s + (j + 1)_s; \\ 0, & \text{otherwise.} \end{cases}$$

If  $7s \leq j < 18s$ , then  $b_{ij} = 0$ .

(17) If  $r_0 = 16$ , then  $\Omega^{16}(Z_t^{(27)})$  is described with  $(19s \times 20s)$  matrix, whose entries  $b_{ij}$  have the following form:

If  $0 \leq j < s$ , then

$$b_{ij} = \begin{cases} e_{8(j+m)+7} \otimes w_{8j \rightarrow 8(j+1)}, & i = 2s + (j + 1)_s; \\ w_{8(j+m)+4 \rightarrow 8(j+m)+7} \otimes w_{8j \rightarrow 8j+1}, & i = j + 3s; \\ 0, & \text{otherwise.} \end{cases}$$

If  $s \leq j < 3s$ , then  $b_{ij} = 0$ .

If  $3s \leq j < 4s$ , then

$$b_{ij} = \begin{cases} w_{8(j+m)+7 \rightarrow 8(j+m+1)+3} \otimes w_{8j+1 \rightarrow 8(j+1)}, & i = (j + 1)_s; \\ 0, & \text{otherwise.} \end{cases}$$

If  $4s \leq j < 5s$ , then  $b_{ij} = 0$ .

If  $5s \leq j < 6s$ , then

$$b_{ij} = \begin{cases} w_{8(j+m)+7 \rightarrow 8(j+m+1)+4} \otimes w_{8j+2 \rightarrow 8(j+1)}, & i = (j + 1)_s; \\ 0, & \text{otherwise.} \end{cases}$$

If  $6s \leq j < 20s$ , then  $b_{ij} = 0$ .

(18) If  $r_0 = 17$ , then  $\Omega^{17}(Z_t^{(27)})$  is described with  $(18s \times 18s)$  matrix, whose entries  $b_{ij}$  have the following form:

If  $0 \leq j < s$ , then

$$b_{ij} = \begin{cases} w_{8(j+m)+7 \rightarrow 8(j+m+1)+3} \otimes w_{8j \rightarrow 8j+1}, & i = j + 4s; \\ 0, & \text{otherwise.} \end{cases}$$

If  $s \leq j < 2s$ , then

$$b_{ij} = \begin{cases} e_{8(j+m+1)+6} \otimes w_{8j \rightarrow 8(j+1)}, & i = 2s + (j + 1)_s; \\ 0, & \text{otherwise.} \end{cases}$$

If  $2s \leq j < 5s$ , then  $b_{ij} = 0$ .

If  $5s \leq j < 6s$ , then

$$b_{ij} = \begin{cases} w_{8(j+m+1)+4 \rightarrow 8(j+m+1)+7} \otimes w_{8j+1 \rightarrow 8(j+1)}, & i = s + (j + 1)_s; \\ 0, & \text{otherwise.} \end{cases}$$

If  $6s \leq j < 7s$ , then

$$b_{ij} = \begin{cases} w_{8(j+m+1)+4 \rightarrow 8(j+m+1)+7} \otimes w_{8j+2 \rightarrow 8(j+1)}, & i = s + (j + 1)_s; \\ 0, & \text{otherwise.} \end{cases}$$

If  $7s \leq j < 8s$ , then  $b_{ij} = 0$ .

If  $8s \leq j < 9s$ , then

$$b_{ij} = \begin{cases} -w_{8(j+m+1)+4 \rightarrow 8(j+m+2)} \otimes w_{8j+3 \rightarrow 8(j+1)}, & i = s + (j + 1)_s; \\ 0, & \text{otherwise.} \end{cases}$$

If  $9s \leq j < 14s$ , then  $b_{ij} = 0$ .

If  $14s \leq j < 15s$ , then

$$b_{ij} = \begin{cases} -w_{8(j+m+1)+7 \rightarrow 8(j+m+2)+2} \otimes w_{8j+7 \rightarrow 8(j+1)+1}, & i = 4s + (j + 1)_s; \\ 0, & \text{otherwise.} \end{cases}$$

If  $15s \leq j < 18s$ , then  $b_{ij} = 0$ .

(19) If  $r_0 = 18$ , then  $\Omega^{18}(Z_t^{(27)})$  is described with  $(19s \times 19s)$  matrix, whose entries  $b_{ij}$  have the following form:

If  $0 \leq j < s$ , then

$$b_{ij} = \begin{cases} -e_{8(j+m)+7} \otimes w_{8j \rightarrow 8(j+1)}, & i = (j + 1)_s; \\ w_{8(j+m)+5 \rightarrow 8(j+m)+7} \otimes w_{8j \rightarrow 8j+1}, & i = j + 3s; \\ -w_{8(j+m)+1 \rightarrow 8(j+m)+7} \otimes w_{8j \rightarrow 8j+1}, & i = j + 4s; \\ -w_{8(j+m)+2 \rightarrow 8(j+m)+7} \otimes w_{8j \rightarrow 8j+2}, & i = j + 5s; \\ 0, & \text{otherwise.} \end{cases}$$

If  $s \leq j < 3s$ , then  $b_{ij} = 0$ .

If  $3s \leq j < 4s$ , then

$$b_{ij} = \begin{cases} -w_{8(j+m)+7 \rightarrow 8(j+m+1)+4} \otimes w_{8j+1 \rightarrow 8(j+1)}, & i = (j + 1)_s; \\ 0, & \text{otherwise.} \end{cases}$$

If  $4s \leq j < 7s$ , then  $b_{ij} = 0$ .

If  $7s \leq j < 8s$ , then

$$b_{ij} = \begin{cases} -w_{8(j+m+1) \rightarrow 8(j+m+1)+2} \otimes w_{8j+3 \rightarrow 8(j+1)}, & i = s + (j+1)_s; \\ w_{8(j+m+1) \rightarrow 8(j+m+1)+2} \otimes w_{8j+3 \rightarrow 8(j+1)}, & i = 2s + (j+1)_s; \\ e_{8(j+m+1)+2} \otimes w_{8j+3 \rightarrow 8(j+1)+2}, & i = 5s + (j+1)_s; \\ 0, & \text{otherwise.} \end{cases}$$

If  $8s \leq j < 19s$ , then  $b_{ij} = 0$ .

(20) If  $r_0 = 19$ , then  $\Omega^{19}(Z_t^{(27)})$  is described with  $(16s \times 18s)$  matrix, whose entries  $b_{ij}$  have the following form:

If  $0 \leq j < s$ , then

$$b_{ij} = \begin{cases} w_{8(j+m+1) \rightarrow 8(j+m+1)+2} \otimes w_{8j \rightarrow 8j+1}, & i = j + 4s; \\ 0, & \text{otherwise.} \end{cases}$$

If  $s \leq j < 4s$ , then  $b_{ij} = 0$ .

If  $4s \leq j < 5s$ , then

$$b_{ij} = \begin{cases} -w_{8(j+m+1)+6 \rightarrow 8(j+m+1)+7} \otimes w_{8j+1 \rightarrow 8(j+1)}, & i = s + (j+1)_s; \\ -w_{8(j+m+1)+1 \rightarrow 8(j+m+1)+7} \otimes w_{8j+1 \rightarrow 8(j+1)}, & i = 2s + (j+1)_s; \\ 0, & \text{otherwise.} \end{cases}$$

If  $5s \leq j < 6s$ , then

$$b_{ij} = \begin{cases} w_{8(j+m+1)+6 \rightarrow 8(j+m+2)} \otimes w_{8j+1 \rightarrow 8(j+1)}, & i = s + (j+1)_s; \\ w_{8(j+m+1)+1 \rightarrow 8(j+m+2)} \otimes w_{8j+1 \rightarrow 8(j+1)}, & i = 2s + (j+1)_s; \\ 0, & \text{otherwise.} \end{cases}$$

If  $6s \leq j < 7s$ , then

$$b_{ij} = \begin{cases} w_{8(j+m+1)+3 \rightarrow 8(j+m+2)} \otimes w_{8j+2 \rightarrow 8(j+1)}, & i = (j+1)_s; \\ -w_{8(j+m+1)+5 \rightarrow 8(j+m+2)} \otimes w_{8j+2 \rightarrow 8(j+1)}, & i = 3s + (j+1)_s; \\ 0, & \text{otherwise.} \end{cases}$$

If  $7s \leq j < 8s$ , then

$$b_{ij} = \begin{cases} w_{8(j+m+1)+1 \rightarrow 8(j+m+1)+7} \otimes w_{8j+3 \rightarrow 8(j+1)}, & i = 2s + (j+1)_s; \\ -w_{8(j+m+1)+5 \rightarrow 8(j+m+1)+7} \otimes w_{8j+3 \rightarrow 8(j+1)}, & i = 3s + (j+1)_s; \\ 0, & \text{otherwise.} \end{cases}$$

If  $8s \leq j < 18s$ , then  $b_{ij} = 0$ .

(21) If  $r_0 = 20$ , then  $\Omega^{20}(Z_t^{(27)})$  is described with  $(16s \times 19s)$  matrix, whose entries  $b_{ij}$  have the following form:

If  $0 \leq j < s$ , then

$$b_{ij} = \begin{cases} w_{8(j+m)+6 \rightarrow 8(j+m)+7} \otimes w_{8j \rightarrow 8j+1}, & i = j + 3s; \\ 0, & \text{otherwise.} \end{cases}$$

If  $s \leq j < 2s$ , then  $b_{ij} = 0$ .

If  $2s \leq j < 3s$ , then

$$b_{ij} = \begin{cases} -w_{8(j+m)+7 \rightarrow 8(j+m+1)} \otimes w_{8j \rightarrow 8(j+1)}, & i = (j+1)_s; \\ 0, & \text{otherwise.} \end{cases}$$

If  $3s \leq j < 4s$ , then  $b_{ij} = 0$ .

If  $4s \leq j < 5s$ , then

$$b_{ij} = \begin{cases} -w_{8(j+m)+7 \rightarrow 8(j+m+1)+1} \otimes w_{8j+1 \rightarrow 8(j+1)}, & i = (j+1)_s; \\ 0, & \text{otherwise.} \end{cases}$$

If  $5s \leq j < 6s$ , then

$$b_{ij} = \begin{cases} w_{8(j+m+1) \rightarrow 8(j+m+1)+2} \otimes w_{8j+2 \rightarrow 8(j+1)}, & i = s + (j+1)_s; \\ 0, & \text{otherwise.} \end{cases}$$

If  $6s \leq j < 7s$ , then  $b_{ij} = 0$ .

If  $7s \leq j < 8s$ , then

$$b_{ij} = \begin{cases} -w_{8(j+m)+7 \rightarrow 8(j+m+1)+3} \otimes w_{8j+3 \rightarrow 8(j+1)}, & i = (j+1)_s; \\ w_{8(j+m+1) \rightarrow 8(j+m+1)+3} \otimes w_{8j+3 \rightarrow 8(j+1)}, & i = s + (j+1)_s; \\ e_{8(j+m+1)+3} \otimes w_{8j+3 \rightarrow 8(j+1)+2}, & i = 4s + (j+1)_s; \\ 0, & \text{otherwise.} \end{cases}$$

If  $8s \leq j < 16s$ , then  $b_{ij} = 0$ .

If  $16s \leq j < 17s$ , then

$$b_{ij} = \begin{cases} -w_{8(j+m+1)+6 \rightarrow 8(j+m+1)+7} \otimes w_{8j+7 \rightarrow 8(j+1)+1}, & i = 3s + (j+1)_s; \\ 0, & \text{otherwise.} \end{cases}$$

If  $17s \leq j < 18s$ , then

$$b_{ij} = \begin{cases} -w_{8(j+m+1)+6 \rightarrow 8(j+m+2)} \otimes w_{8j+7 \rightarrow 8(j+1)+1}, & i = 3s + (j+1)_s; \\ 0, & \text{otherwise.} \end{cases}$$

If  $18s \leq j < 19s$ , then  $b_{ij} = 0$ .

(22) If  $r_0 = 21$ , then  $\Omega^{21}(Z_t^{(27)})$  is described with  $(14s \times 16s)$  matrix, whose entries  $b_{ij}$  have the following form:

If  $s \leq j < 2s$ , then

$$b_{ij} = \begin{cases} -w_{8(j+m)+7 \rightarrow 8(j+m+1)+6} \otimes w_{8j \rightarrow 8j+1}, & i = j + 2s; \\ 0, & \text{otherwise.} \end{cases}$$

If  $2s \leq j < 4s$ , then  $b_{ij} = 0$ .

If  $4s \leq j < 5s$ , then

$$b_{ij} = \begin{cases} -w_{8(j+m+1)+6 \rightarrow 8(j+m+2)} \otimes w_{8j+1 \rightarrow 8(j+1)}, & i = 2s + (j+1)_s; \\ 0, & \text{otherwise.} \end{cases}$$



If  $5s \leq j < 6s$ , then

$$b_{ij} = \begin{cases} w_{8(j+m+1)+2 \rightarrow 8(j+m+1)+7} \otimes w_{8j+2 \rightarrow 8(j+1)}, & i = (j+1)_s; \\ w_{8(j+m+1)+4 \rightarrow 8(j+m+1)+7} \otimes w_{8j+2 \rightarrow 8(j+1)}, & i = s + (j+1)_s; \\ 0, & \text{otherwise.} \end{cases}$$

If  $6s \leq j < 7s$ , then

$$b_{ij} = \begin{cases} -w_{8(j+m+1)+2 \rightarrow 8(j+m+2)} \otimes w_{8j+3 \rightarrow 8(j+1)}, & i = (j+1)_s; \\ -w_{8(j+m+1)+7 \rightarrow 8(j+m+2)} \otimes w_{8j+3 \rightarrow 8(j+1)+1}, & i = 3s + (j+1)_s; \\ 0, & \text{otherwise.} \end{cases}$$

If  $7s \leq j < 15s$ , then  $b_{ij} = 0$ .

If  $15s \leq j < 16s$ , then

$$b_{ij} = \begin{cases} w_{8(j+m+1)+7 \rightarrow 8(j+m+2)+5} \otimes w_{8j+7 \rightarrow 8(j+1)+1}, & i = 3s + (j+1)_s; \\ 0, & \text{otherwise.} \end{cases}$$

(23) If  $r_0 = 22$ , then  $\Omega^{22}(Z_t^{(27)})$  is described with  $(13s \times 16s)$  matrix, whose entries  $b_{ij}$  have the following form:

If  $0 \leq j < s$ , then

$$b_{ij} = \begin{cases} w_{8(j+m)+3 \rightarrow 8(j+m)+7} \otimes w_{8j \rightarrow 8j+1}, & i = j + 2s; \\ -w_{8(j+m)+4 \rightarrow 8(j+m)+7} \otimes w_{8j \rightarrow 8j+2}, & i = j + 3s; \\ 0, & \text{otherwise.} \end{cases}$$

If  $s \leq j < 2s$ , then

$$b_{ij} = \begin{cases} e_{8(j+m+1)} \otimes w_{8j \rightarrow 8(j+1)}, & i = (j+1)_s; \\ -w_{8(j+m)+7 \rightarrow 8(j+m+1)} \otimes w_{8j \rightarrow 8(j+1)}, & i = s + (j+1)_s; \\ 0, & \text{otherwise.} \end{cases}$$

If  $2s \leq j < 3s$ , then

$$b_{ij} = \begin{cases} w_{8(j+m)+7 \rightarrow 8(j+m+1)+2} \otimes w_{8j+1 \rightarrow 8(j+1)}, & i = s + (j+1)_s; \\ 0, & \text{otherwise.} \end{cases}$$

If  $3s \leq j < 4s$ , then

$$b_{ij} = \begin{cases} w_{8(j+m)+7 \rightarrow 8(j+m+1)+6} \otimes w_{8j+1 \rightarrow 8(j+1)}, & i = s + (j+1)_s; \\ 0, & \text{otherwise.} \end{cases}$$

If  $4s \leq j < 5s$ , then

$$b_{ij} = \begin{cases} w_{8(j+m)+7 \rightarrow 8(j+m+1)+3} \otimes w_{8j+2 \rightarrow 8(j+1)}, & i = s + (j+1)_s; \\ 0, & \text{otherwise.} \end{cases}$$

If  $5s \leq j < 6s$ , then

$$b_{ij} = \begin{cases} -w_{8(j+m+1) \rightarrow 8(j+m+1)+4} \otimes w_{8j+3 \rightarrow 8(j+1)}, & i = (j+1)_s; \\ w_{8(j+m)+7 \rightarrow 8(j+m+1)+4} \otimes w_{8j+3 \rightarrow 8(j+1)}, & i = s + (j+1)_s; \\ e_{8(j+m+1)+4} \otimes w_{8j+3 \rightarrow 8(j+1)+2}, & i = 3s + (j+1)_s; \\ 0, & \text{otherwise.} \end{cases}$$

If  $6s \leq j < 16s$ , then  $b_{ij} = 0$ .

(24) If  $r_0 = 23$ , then  $\Omega^{23}(Z_t^{(27)})$  is described with  $(11s \times 14s)$  matrix, whose entries  $b_{ij}$  have the following form:

If  $0 \leq j < s$ , then

$$b_{ij} = \begin{cases} w_{8(j+m+1) \rightarrow 8(j+m+1)+2} \otimes w_{8j \rightarrow 8j+1}, & i = j + 2s; \\ 0, & \text{otherwise.} \end{cases}$$

If  $s \leq j < 2s$ , then  $b_{ij} = 0$ .

If  $2s \leq j < 3s$ , then

$$b_{ij} = \begin{cases} w_{8(j+m+1)+5 \rightarrow 8(j+m+1)+6} \otimes w_{8j \rightarrow 8(j+1)}, & i = s + (j+1)_s; \\ 0, & \text{otherwise.} \end{cases}$$

If  $3s \leq j < 4s$ , then

$$b_{ij} = \begin{cases} w_{8(j+m+1)+3 \rightarrow 8(j+m+1)+7} \otimes w_{8j+1 \rightarrow 8(j+1)}, & i = (j+1)_s; \\ -w_{8(j+m+1)+5 \rightarrow 8(j+m+1)+7} \otimes w_{8j+1 \rightarrow 8(j+1)}, & i = s + (j+1)_s; \\ 0, & \text{otherwise.} \end{cases}$$

If  $4s \leq j < 5s$ , then

$$b_{ij} = \begin{cases} w_{8(j+m+1)+3 \rightarrow 8(j+m+2)} \otimes w_{8j+2 \rightarrow 8(j+1)}, & i = (j+1)_s; \\ 0, & \text{otherwise.} \end{cases}$$

If  $5s \leq j < 6s$ , then

$$b_{ij} = \begin{cases} -w_{8(j+m+1)+3 \rightarrow 8(j+m+1)+7} \otimes w_{8j+3 \rightarrow 8(j+1)}, & i = (j+1)_s; \\ 0, & \text{otherwise.} \end{cases}$$

If  $6s \leq j < 14s$ , then  $b_{ij} = 0$ .

(25) If  $r_0 = 24$ , then  $\Omega^{24}(Z_t^{(27)})$  is described with  $(11s \times 13s)$  matrix, whose entries  $b_{ij}$  have the following form:

If  $0 \leq j < s$ , then

$$b_{ij} = \begin{cases} e_{8(j+m+1)} \otimes w_{8j \rightarrow 8(j+1)}, & i = (j+1)_s; \\ w_{8(j+m)+5 \rightarrow 8(j+m+1)} \otimes w_{8j \rightarrow 8j+1}, & i = j + 2s; \\ 0, & \text{otherwise.} \end{cases}$$

If  $s \leq j < 2s$ , then  $b_{ij} = 0$ .

If  $2s \leq j < 3s$ , then

$$b_{ij} = \begin{cases} w_{8(j+m+1) \rightarrow 8(j+m+1)+3} \otimes w_{8j+1 \rightarrow 8(j+1)}, & i = (j+1)_s; \\ 0, & \text{otherwise.} \end{cases}$$

If  $3s \leq j < 12s$ , then  $b_{ij} = 0$ .

If  $12s \leq j < 13s$ , then

$$b_{ij} = \begin{cases} -w_{8(j+m+1)+5 \rightarrow 8(j+m+2)} \otimes w_{8j+7 \rightarrow 8(j+1)+1}, & i = 2s + (j+1)_s; \\ 0, & \text{otherwise.} \end{cases}$$

(26) If  $r_0 = 25$ , then  $\Omega^{25}(Z_t^{(27)})$  is described with  $(10s \times 11s)$  matrix, whose entries  $b_{ij}$  have the following form:

If  $s \leq j < 2s$ , then

$$b_{ij} = \begin{cases} -w_{8(j+m)+7 \rightarrow 8(j+m+1)+5} \otimes w_{8j \rightarrow 8j+1}, & i = j + s; \\ -w_{8(j+m+1) \rightarrow 8(j+m+1)+5} \otimes w_{8j \rightarrow 8j+2}, & i = j + 2s; \\ -w_{8(j+m+1) \rightarrow 8(j+m+1)+5} \otimes w_{8j \rightarrow 8j+6}, & i = j + 6s; \\ 0, & \text{otherwise.} \end{cases}$$

If  $2s \leq j < 3s$ , then

$$b_{ij} = \begin{cases} w_{8(j+m+1)+6 \rightarrow 8(j+m+2)} \otimes w_{8j+1 \rightarrow 8(j+1)}, & i = s + (j+1)_s; \\ 0, & \text{otherwise.} \end{cases}$$

If  $3s \leq j < 11s$ , then  $b_{ij} = 0$ .

(27) If  $r_0 = 26$ , then  $\Omega^{26}(Z_t^{(27)})$  is described with  $(8s \times 11s)$  matrix, whose entries  $b_{ij}$  have the following form:

If  $0 \leq j < s$ , then

$$b_{ij} = \begin{cases} -w_{8(j+m)+7 \rightarrow 8(j+m+1)} \otimes w_{8j \rightarrow 8(j+1)}, & i = (j+1)_s; \\ (1 - 2f(j_1, 2))w_{8(j+m)+j_1 \rightarrow 8(j+m+1)} \otimes w_{8j \rightarrow 8j+1+j_1}, & i = j + (1+j_1)s, \ 1 \leq j_1 \leq 4; \\ 0, & \text{otherwise.} \end{cases}$$

If  $s \leq j < 2s$ , then  $b_{ij} = 0$ .

If  $2s \leq j < 3s$ , then

$$b_{ij} = \begin{cases} -w_{8(j+m)+7 \rightarrow 8(j+m+1)+5} \otimes w_{8j+1 \rightarrow 8(j+1)}, & i = (j+1)_s; \\ 0, & \text{otherwise.} \end{cases}$$

If  $3s \leq j < 4s$ , then

$$b_{ij} = \begin{cases} e_{8(j+m+1)+6} \otimes w_{8j+2 \rightarrow 8(j+1)+1}, & i = s + (j+1)_s; \\ 0, & \text{otherwise.} \end{cases}$$

If  $4s \leq j < 11s$ , then  $b_{ij} = 0$ .

(28) If  $r_0 = 27$ , then  $\Omega^{27}(Z_t^{(27)})$  is described with  $(9s \times 10s)$  matrix, whose entries  $b_{ij}$  have the following form:

If  $0 \leq j < s$ , then

$$b_{ij} = \begin{cases} -w_{8(j+m+1) \rightarrow 8(j+m+1)+4} \otimes w_{8j \rightarrow 8j+1}, & i = j + s; \\ w_{8(j+m+1) \rightarrow 8(j+m+1)+4} \otimes w_{8j \rightarrow 8j+5}, & i = j + 5s; \\ 0, & \text{otherwise.} \end{cases}$$

If  $s \leq j < 2s$ , then  $b_{ij} = 0$ .

If  $2s \leq j < 6s$ , then

$$b_{ij} = \begin{cases} (-1)^{j_2} w_{8(j+m+1)+7 \rightarrow 8(j+m+1)+5+j_2} \otimes w_{8j+j_2-1 \rightarrow 8(j+1)}, & i = (j+1)_s; \\ 0, & \text{otherwise.} \end{cases}$$

If  $6s \leq j < 8s$ , then  $b_{ij} = 0$ .

If  $8s \leq j < 9s$ , then

$$b_{ij} = \begin{cases} -w_{8(j+m+1)+7 \rightarrow 8(j+m+2)+3} \otimes w_{8j+7 \rightarrow 8(j+1)}, & i = (j+1)_s; \\ 0, & \text{otherwise.} \end{cases}$$

If  $9s \leq j < 10s$ , then  $b_{ij} = 0$ .

(29) If  $r_0 = 28$ , then  $\Omega^{28}(Z_t^{(27)})$  is described with  $(8s \times 8s)$  matrix, whose entries  $b_{ij}$  have the following form:

If  $0 \leq j < s$ , then

$$b_{ij} = \begin{cases} (1 - 2(f(j_1, 1) + f(j_1, 3) + f(j_1, 6))) w_{8(j+m)+j_1 \rightarrow 8(j+m)+7} \otimes w_{8j \rightarrow 8j+j_1}, & i = j + j_1 s, \ 1 \leq j_1 \leq 7; \\ 0, & \text{otherwise.} \end{cases}$$

If  $s \leq j < 5s$ , then  $b_{ij} = 0$ .

If  $5s \leq j < 6s$ , then

$$b_{ij} = \begin{cases} -w_{8(j+m+1) \rightarrow 8(j+m+1)+4} \otimes w_{8j+5 \rightarrow 8(j+1)}, & i = (j+1)_s; \\ 0, & \text{otherwise.} \end{cases}$$

If  $6s \leq j < 7s$ , then  $b_{ij} = 0$ .

If  $7s \leq j < 8s$ , then

$$b_{ij} = \begin{cases} -w_{8(j+m+1) \rightarrow 8(j+m+2)} \otimes w_{8j+7 \rightarrow 8(j+1)}, & i = (j+1)_s; \\ 0, & \text{otherwise.} \end{cases}$$

(II) Represent an arbitrary  $t_0 \in \mathbb{N}$  in the form  $t_0 = 29\ell_0 + r_0$ , where  $0 \leq r_0 \leq 28$ . Then  $\Omega^{t_0}(Z_t^{(27)})$  is a  $\Omega^{r_0}(Z_t^{(27)})$ , whose left components twisted by  $\sigma^{\ell_0}$ .

**Proposition 23** (Translates for the case 28). (I) Let  $r_0 \in \mathbb{N}$ ,  $r_0 < 29$ .  $r_0$ -translates of the elements  $Z_t^{(28)}$  are described by the following way.

(1) If  $r_0 = 0$ , then  $\Omega^0(Z_t^{(28)})$  is described with  $(8s \times 8s)$  matrix with unique nonzero entry:

$$b_{j,(1)_s} = -w_{8(j+m) \rightarrow 8(j+m+1)} \otimes e_{8j}.$$

(2) If  $r_0 = 1$ , then  $\Omega^1(Z_t^{(28)})$  is described with  $(9s \times 8s)$  matrix with unique nonzero entry:

$$b_{(j+1)_s,0} = w_{8(j+m+1)+1 \rightarrow 8(j+m+2)} \otimes w_{8j \rightarrow 8(j+1)}.$$

(3) If  $r_0 = 2$ , then  $\Omega^2(Z_t^{(28)})$  is described with  $(8s \times 9s)$  matrix with unique nonzero entry:

$$b_{(j+1)_s,0} = w_{8(j+m)+7 \rightarrow 8(j+m+1)+1} \otimes w_{8j \rightarrow 8(j+1)}.$$

(4) If  $r_0 = 3$ , then  $\Omega^3(Z_t^{(28)})$  is described with  $(10s \times 8s)$  matrix with unique nonzero entry:

$$b_{(j+1)_s,0} = w_{8(j+m+1)+2 \rightarrow 8(j+m+1)+7} \otimes w_{8j \rightarrow 8(j+1)}.$$

(5) If  $r_0 = 4$ , then  $\Omega^4(Z_t^{(28)})$  is described with  $(11s \times 10s)$  matrix with unique nonzero entry:

$$b_{(j+1)_s,0} = w_{8(j+m)+7 \rightarrow 8(j+m+1)+2} \otimes w_{8j \rightarrow 8(j+1)}.$$

(6) If  $r_0 = 5$ , then  $\Omega^5(Z_t^{(28)})$  is described with  $(11s \times 11s)$  matrix with unique nonzero entry:

$$b_{s+(j+1)s,0} = w_{8(j+m+1)+3 \rightarrow 8(j+m+1)+7} \otimes w_{8j \rightarrow 8(j+1)}.$$

(7) If  $r_0 = 6$ , then  $\Omega^6(Z_t^{(28)})$  is described with  $(13s \times 11s)$  matrix with unique nonzero entry:

$$b_{(j+1)s,s} = -w_{8(j+m)+7 \rightarrow 8(j+m+1)+3} \otimes w_{8j \rightarrow 8(j+1)}.$$

(8) If  $r_0 = 7$ , then  $\Omega^7(Z_t^{(28)})$  is described with  $(14s \times 13s)$  matrix with two nonzero entries:

$$b_{(j+1)s,0} = w_{8(j+m+1)+2 \rightarrow 8(j+m+1)+7} \otimes w_{8j \rightarrow 8(j+1)};$$

$$b_{s+(j+1)s,0} = -w_{8(j+m+1)+4 \rightarrow 8(j+m+1)+7} \otimes w_{8j \rightarrow 8(j+1)}.$$

(9) If  $r_0 = 8$ , then  $\Omega^8(Z_t^{(28)})$  is described with  $(16s \times 14s)$  matrix with two nonzero entries:

$$b_{(j+1)s,0} = w_{8(j+m)+7 \rightarrow 8(j+m+1)+2} \otimes w_{8j \rightarrow 8(j+1)};$$

$$b_{s+(j+1)s,0} = -w_{8(j+m)+7 \rightarrow 8(j+m+1)+2} \otimes w_{8j \rightarrow 8(j+1)}.$$

(10) If  $r_0 = 9$ , then  $\Omega^9(Z_t^{(28)})$  is described with  $(16s \times 16s)$  matrix with two nonzero entries:

$$b_{s+(j+1)s,0} = w_{8(j+m+1)+3 \rightarrow 8(j+m+1)+7} \otimes w_{8j \rightarrow 8(j+1)};$$

$$b_{2s+(j+1)s,0} = -w_{8(j+m+1)+6 \rightarrow 8(j+m+1)+7} \otimes w_{8j \rightarrow 8(j+1)}.$$

(11) If  $r_0 = 10$ , then  $\Omega^{10}(Z_t^{(28)})$  is described with  $(19s \times 16s)$  matrix with two nonzero entries:

$$b_{2s+(j+1)s,0} = -w_{8(j+m+1) \rightarrow 8(j+m+1)+5} \otimes w_{8j \rightarrow 8(j+1)};$$

$$b_{(j+1)s,s} = -w_{8(j+m)+7 \rightarrow 8(j+m+1)+3} \otimes w_{8j \rightarrow 8(j+1)}.$$

(12) If  $r_0 = 11$ , then  $\Omega^{11}(Z_t^{(28)})$  is described with  $(18s \times 19s)$  matrix with unique nonzero entry:

$$b_{s+(j+1)s,0} = w_{8(j+m+1)+6 \rightarrow 8(j+m+1)+7} \otimes w_{8j \rightarrow 8(j+1)}.$$

(13) If  $r_0 = 12$ , then  $\Omega^{12}(Z_t^{(28)})$  is described with  $(19s \times 18s)$  matrix with unique nonzero entry:

$$b_{(j+1)s,s} = -w_{8(j+m)+7 \rightarrow 8(j+m+1)+6} \otimes w_{8j \rightarrow 8(j+1)}.$$

(14) If  $r_0 = 13$ , then  $\Omega^{13}(Z_t^{(28)})$  is described with  $(18s \times 19s)$  matrix with unique nonzero entry:

$$b_{s+(j+1)s,0} = w_{8(j+m+1)+3 \rightarrow 8(j+m+1)+7} \otimes w_{8j \rightarrow 8(j+1)}.$$

(15) If  $r_0 = 14$ , then  $\Omega^{14}(Z_t^{(28)})$  is described with  $(20s \times 18s)$  matrix with two nonzero entries:

$$b_{s+(j+1)s,0} = w_{8(j+m+1) \rightarrow 8(j+m+1)+2} \otimes w_{8j \rightarrow 8(j+1)};$$

$$b_{(j+1)s,s} = -w_{8(j+m)+7 \rightarrow 8(j+m+1)+3} \otimes w_{8j \rightarrow 8(j+1)}.$$

(16) If  $r_0 = 15$ , then  $\Omega^{15}(Z_t^{(28)})$  is described with  $(18s \times 20s)$  matrix with unique nonzero entry:

$$b_{(j+1)s,0} = w_{8(j+m+1)+3 \rightarrow 8(j+m+1)+7} \otimes w_{8j \rightarrow 8(j+1)}.$$

(17) If  $r_0 = 16$ , then  $\Omega^{16}(Z_t^{(28)})$  is described with  $(19s \times 18s)$  matrix with unique nonzero entry:

$$b_{(j+1)s,0} = w_{8(j+m)+7 \rightarrow 8(j+m+1)+3} \otimes w_{8j \rightarrow 8(j+1)}.$$

(18) If  $r_0 = 17$ , then  $\Omega^{17}(Z_t^{(28)})$  is described with  $(18s \times 19s)$  matrix with unique nonzero entry:

$$b_{s+(j+1)s,0} = w_{8(j+m+1)+4 \rightarrow 8(j+m+1)+7} \otimes w_{8j \rightarrow 8(j+1)}.$$

(19) If  $r_0 = 18$ , then  $\Omega^{18}(Z_t^{(28)})$  is described with  $(19s \times 18s)$  matrix with two nonzero entries:

$$b_{s+(j+1)s,0} = w_{8(j+m+1) \rightarrow 8(j+m+1)+2} \otimes w_{8j \rightarrow 8(j+1)};$$

$$b_{(j+1)s,s} = -w_{8(j+m)+7 \rightarrow 8(j+m+1)+4} \otimes w_{8j \rightarrow 8(j+1)}.$$

(20) If  $r_0 = 19$ , then  $\Omega^{19}(Z_t^{(28)})$  is described with  $(16s \times 19s)$  matrix with unique nonzero entry:

$$b_{(j+1)s,0} = w_{8(j+m+1)+3 \rightarrow 8(j+m+1)+7} \otimes w_{8j \rightarrow 8(j+1)}.$$

(21) If  $r_0 = 20$ , then  $\Omega^{20}(Z_t^{(28)})$  is described with  $(16s \times 16s)$  matrix with unique nonzero entry:

$$b_{(j+1)s,0} = w_{8(j+m)+7 \rightarrow 8(j+m+1)+3} \otimes w_{8j \rightarrow 8(j+1)}.$$

(22) If  $r_0 = 21$ , then  $\Omega^{21}(Z_t^{(28)})$  is described with  $(14s \times 16s)$  matrix with two nonzero entries:

$$b_{(j+1)s,0} = w_{8(j+m+1)+2 \rightarrow 8(j+m+1)+7} \otimes w_{8j \rightarrow 8(j+1)};$$

$$b_{s+(j+1)s,0} = w_{8(j+m+1)+4 \rightarrow 8(j+m+1)+7} \otimes w_{8j \rightarrow 8(j+1)}.$$

(23) If  $r_0 = 22$ , then  $\Omega^{22}(Z_t^{(28)})$  is described with  $(13s \times 14s)$  matrix with unique nonzero entry:

$$b_{(j+1)s,0} = w_{8(j+m+1) \rightarrow 8(j+m+1)+2} \otimes w_{8j \rightarrow 8(j+1)}.$$

(24) If  $r_0 = 23$ , then  $\Omega^{23}(Z_t^{(28)})$  is described with  $(11s \times 13s)$  matrix with unique nonzero entry:

$$b_{(j+1)s,0} = w_{8(j+m+1)+3 \rightarrow 8(j+m+2)} \otimes w_{8j \rightarrow 8(j+1)}.$$

(25) If  $r_0 = 24$ , then  $\Omega^{24}(Z_t^{(28)})$  is described with  $(11s \times 11s)$  matrix with unique nonzero entry:

$$b_{(j+1)s,0} = w_{8(j+m+1) \rightarrow 8(j+m+1)+3} \otimes w_{8j \rightarrow 8(j+1)}.$$

(26) If  $r_0 = 25$ , then  $\Omega^{25}(Z_t^{(28)})$  is described with  $(10s \times 11s)$  matrix with unique nonzero entry:

$$b_{(j+1)s,0} = w_{8(j+m+1)+4 \rightarrow 8(j+m+2)} \otimes w_{8j \rightarrow 8(j+1)}.$$

(27) If  $r_0 = 26$ , then  $\Omega^{26}(Z_t^{(28)})$  is described with  $(8s \times 10s)$  matrix with unique nonzero entry:

$$b_{(j+1)s,0} = w_{8(j+m)+7 \rightarrow 8(j+m+1)+4} \otimes w_{8j \rightarrow 8(j+1)}.$$

(28) If  $r_0 = 27$ , then  $\Omega^{27}(Z_t^{(28)})$  is described with  $(9s \times 8s)$  matrix with unique nonzero entry:

$$b_{(j+1)s,0} = e_{8(j+m+1)+7} \otimes w_{8j \rightarrow 8(j+1)}.$$

(29) If  $r_0 = 28$ , then  $\Omega^{28}(Z_t^{(28)})$  is described with  $(8s \times 9s)$  matrix with unique nonzero entry:

$$b_{(j+1)s,0} = w_{8(j+m+1) \rightarrow 8(j+m+1)+7} \otimes w_{8j \rightarrow 8(j+1)}.$$

(II) Represent an arbitrary  $t_0 \in \mathbb{N}$  in the form  $t_0 = 29\ell_0 + r_0$ , where  $0 \leq r_0 \leq 28$ . Then  $\Omega^{t_0}(Z_t^{(28)})$  is a  $\Omega^{r_0}(Z_t^{(28)})$ , whose left components twisted by  $\sigma^{\ell_0}$ , and coefficients multiplied by  $(-1)^{\ell_0}$ .

**Proposition 24** (Translates for the case 29). (I) Let  $r_0 \in \mathbb{N}$ ,  $r_0 < 29$ .  $r_0$ -translates of the elements  $Z_t^{(29)}$  are described by the following way.

(1) If  $r_0 = 0$ , then  $\Omega^0(Z_t^{(29)})$  is described with  $(8s \times 8s)$  matrix with unique nonzero entry:

$$b_{j,0} = w_{8(j+m) \rightarrow 8(j+m+1)} \otimes e_{8j}.$$

(2) If  $r_0 = 1$ , then  $\Omega^1(Z_t^{(29)})$  is described with  $(9s \times 9s)$  matrix with unique nonzero entry:

$$b_{j,8s} = w_{8(j+m) \rightarrow 8(j+m+1)} \otimes e_{8j+7}.$$

(3) If  $r_0 = 2$ , then  $\Omega^2(Z_t^{(29)})$  is described with  $(8s \times 8s)$  matrix with unique nonzero entry:

$$b_{j,7s} = w_{8(j+m) \rightarrow 8(j+m+1)} \otimes e_{8j+7}.$$

(4) If  $r_0 = 3$ , then  $\Omega^3(Z_t^{(29)})$  is described with  $(10s \times 10s)$  matrix with two nonzero entries:

$$b_{j,5s} = w_{8(j+m) \rightarrow 8(j+m+1)} \otimes e_{8j+4};$$

$$b_{j,7s} = w_{8(j+m) \rightarrow 8(j+m+1)} \otimes e_{8j+6}.$$

(5) If  $r_0 = 4$ , then  $\Omega^4(Z_t^{(29)})$  is described with  $(11s \times 11s)$  matrix with unique nonzero entry:

$$b_{j,s} = w_{8(j+m) \rightarrow 8(j+m+1)} \otimes e_{8j}.$$

(6) If  $r_0 = 5$ , then  $\Omega^5(Z_t^{(29)})$  is described with  $(11s \times 11s)$  matrix with two nonzero entries:

$$b_{j,5s} = w_{8(j+m) \rightarrow 8(j+m+1)} \otimes e_{8j+3};$$

$$b_{j,7s} = w_{8(j+m) \rightarrow 8(j+m+1)} \otimes e_{8j+5}.$$

(7) If  $r_0 = 6$ , then  $\Omega^6(Z_t^{(29)})$  is described with  $(13s \times 13s)$  matrix with two nonzero entries:

$$b_{j,s} = w_{8(j+m) \rightarrow 8(j+m+1)} \otimes e_{8j};$$

$$b_{j,12s} = w_{8(j+m) \rightarrow 8(j+m+1)} \otimes e_{8j+7}.$$

(8) If  $r_0 = 7$ , then  $\Omega^7(Z_t^{(29)})$  is described with  $(14s \times 14s)$  matrix with the following nonzero entries:

$$b_{j,5s} = w_{8(j+m) \rightarrow 8(j+m+1)} \otimes e_{8j+2};$$

$$b_{j,7s} = w_{8(j+m) \rightarrow 8(j+m+1)} \otimes e_{8j+4};$$

$$b_{j,10s} = w_{8(j+m) \rightarrow 8(j+m+1)} \otimes e_{8j+6}.$$

(9) If  $r_0 = 8$ , then  $\Omega^8(Z_t^{(29)})$  is described with  $(16s \times 16s)$  matrix with two nonzero entries:

$$b_{j,2s} = w_{8(j+m) \rightarrow 8(j+m+1)} \otimes e_{8j};$$

$$b_{j,15s} = w_{8(j+m) \rightarrow 8(j+m+1)} \otimes e_{8j+7}.$$

(10) If  $r_0 = 9$ , then  $\Omega^9(Z_t^{(29)})$  is described with  $(16s \times 16s)$  matrix with the following nonzero entries:

$$b_{j,4s} = w_{8(j+m) \rightarrow 8(j+m+1)} \otimes e_{8j+1};$$

$$b_{j,6s} = w_{8(j+m) \rightarrow 8(j+m+1)} \otimes e_{8j+3};$$

$$b_{j,9s} = w_{8(j+m) \rightarrow 8(j+m+1)} \otimes e_{8j+5};$$

$$b_{j,11s} = w_{8(j+m) \rightarrow 8(j+m+1)} \otimes e_{8j+6}.$$

(11) If  $r_0 = 10$ , then  $\Omega^{10}(Z_t^{(29)})$  is described with  $(19s \times 19s)$  matrix with the following nonzero entries:

$$b_{j,s} = w_{8(j+m) \rightarrow 8(j+m+1)} \otimes e_{8j};$$

$$b_{j,2s} = w_{8(j+m) \rightarrow 8(j+m+1)} \otimes e_{8j};$$

$$b_{j,18s} = w_{8(j+m) \rightarrow 8(j+m+1)} \otimes e_{8j+7}.$$

(12) If  $r_0 = 11$ , then  $\Omega^{11}(Z_t^{(29)})$  is described with  $(18s \times 18s)$  matrix with the following nonzero entries:

$$b_{j,6s} = w_{8(j+m) \rightarrow 8(j+m+1)} \otimes e_{8j+2};$$

$$b_{j,9s} = w_{8(j+m) \rightarrow 8(j+m+1)} \otimes e_{8j+4};$$

$$b_{j,11s} = w_{8(j+m) \rightarrow 8(j+m+1)} \otimes e_{8j+5};$$

$$b_{j,13s} = w_{8(j+m) \rightarrow 8(j+m+1)} \otimes e_{8j+6}.$$

(13) If  $r_0 = 12$ , then  $\Omega^{12}(Z_t^{(29)})$  is described with  $(19s \times 19s)$  matrix with the following nonzero entries:

$$\begin{aligned} b_{j,s} &= w_{8(j+m) \rightarrow 8(j+m+1)} \otimes e_{8j}; \\ b_{j,17s} &= w_{8(j+m) \rightarrow 8(j+m+1)} \otimes e_{8j+7}; \\ b_{j,18s} &= w_{8(j+m) \rightarrow 8(j+m+1)} \otimes e_{8j+7}. \end{aligned}$$

(14) If  $r_0 = 13$ , then  $\Omega^{13}(Z_t^{(29)})$  is described with  $(18s \times 18s)$  matrix with the following nonzero entries:

$$\begin{aligned} b_{j,4s} &= w_{8(j+m) \rightarrow 8(j+m+1)} \otimes e_{8j+1}; \\ b_{j,7s} &= w_{8(j+m) \rightarrow 8(j+m+1)} \otimes e_{8j+3}; \\ b_{j,8s} &= w_{8(j+m) \rightarrow 8(j+m+1)} \otimes e_{8j+4}; \\ b_{j,10s} &= w_{8(j+m) \rightarrow 8(j+m+1)} \otimes e_{8j+5}; \\ b_{j,12s} &= w_{8(j+m) \rightarrow 8(j+m+1)} \otimes e_{8j+6}. \end{aligned}$$

(15) If  $r_0 = 14$ , then  $\Omega^{14}(Z_t^{(29)})$  is described with  $(20s \times 20s)$  matrix with the following nonzero entries:

$$\begin{aligned} b_{j,s} &= w_{8(j+m) \rightarrow 8(j+m+1)} \otimes e_{8j}; \\ b_{j,2s} &= w_{8(j+m) \rightarrow 8(j+m+1)} \otimes e_{8j}; \\ b_{j,18s} &= w_{8(j+m) \rightarrow 8(j+m+1)} \otimes e_{8j+7}. \end{aligned}$$

(16) If  $r_0 = 15$ , then  $\Omega^{15}(Z_t^{(29)})$  is described with  $(18s \times 18s)$  matrix with the following nonzero entries:

$$\begin{aligned} b_{j,7s} &= w_{8(j+m) \rightarrow 8(j+m+1)} \otimes e_{8j+2}; \\ b_{j,8s} &= w_{8(j+m) \rightarrow 8(j+m+1)} \otimes e_{8j+3}; \\ b_{j,11s} &= w_{8(j+m) \rightarrow 8(j+m+1)} \otimes e_{8j+5}; \\ b_{j,12s} &= w_{8(j+m) \rightarrow 8(j+m+1)} \otimes e_{8j+6}. \end{aligned}$$

(17) If  $r_0 = 16$ , then  $\Omega^{16}(Z_t^{(29)})$  is described with  $(19s \times 19s)$  matrix with the following nonzero entries:

$$\begin{aligned} b_{j,s} &= w_{8(j+m) \rightarrow 8(j+m+1)} \otimes e_{8j}; \\ b_{j,17s} &= w_{8(j+m) \rightarrow 8(j+m+1)} \otimes e_{8j+7}; \\ b_{j,18s} &= w_{8(j+m) \rightarrow 8(j+m+1)} \otimes e_{8j+7}. \end{aligned}$$

(18) If  $r_0 = 17$ , then  $\Omega^{17}(Z_t^{(29)})$  is described with  $(18s \times 18s)$  matrix with the following nonzero entries:

$$\begin{aligned} b_{j,5s} &= w_{8(j+m) \rightarrow 8(j+m+1)} \otimes e_{8j+1}; \\ b_{j,6s} &= w_{8(j+m) \rightarrow 8(j+m+1)} \otimes e_{8j+2}; \\ b_{j,8s} &= w_{8(j+m) \rightarrow 8(j+m+1)} \otimes e_{8j+4}; \\ b_{j,9s} &= w_{8(j+m) \rightarrow 8(j+m+1)} \otimes e_{8j+5}; \\ b_{j,12s} &= w_{8(j+m) \rightarrow 8(j+m+1)} \otimes e_{8j+6}. \end{aligned}$$

(19) If  $r_0 = 18$ , then  $\Omega^{18}(Z_t^{(29)})$  is described with  $(19s \times 19s)$  matrix with the following nonzero entries:

$$\begin{aligned} b_{j,s} &= w_{8(j+m) \rightarrow 8(j+m+1)} \otimes e_{8j}; \\ b_{j,2s} &= w_{8(j+m) \rightarrow 8(j+m+1)} \otimes e_{8j}; \\ b_{j,17s} &= w_{8(j+m) \rightarrow 8(j+m+1)} \otimes e_{8j+7}. \end{aligned}$$



(20) If  $r_0 = 19$ , then  $\Omega^{19}(Z_t^{(29)})$  is described with  $(16s \times 16s)$  matrix with the following nonzero entries:

$$\begin{aligned} b_{j,4s} &= w_{8(j+m) \rightarrow 8(j+m+1)} \otimes e_{8j+1}; \\ b_{j,6s} &= w_{8(j+m) \rightarrow 8(j+m+1)} \otimes e_{8j+3}; \\ b_{j,9s} &= w_{8(j+m) \rightarrow 8(j+m+1)} \otimes e_{8j+5}; \\ b_{j,11s} &= w_{8(j+m) \rightarrow 8(j+m+1)} \otimes e_{8j+6}. \end{aligned}$$

(21) If  $r_0 = 20$ , then  $\Omega^{20}(Z_t^{(29)})$  is described with  $(16s \times 16s)$  matrix with the following nonzero entries:

$$\begin{aligned} b_{j,s} &= w_{8(j+m) \rightarrow 8(j+m+1)} \otimes e_{8j}; \\ b_{j,14s} &= w_{8(j+m) \rightarrow 8(j+m+1)} \otimes e_{8j+7}; \\ b_{j,15s} &= w_{8(j+m) \rightarrow 8(j+m+1)} \otimes e_{8j+7}. \end{aligned}$$

(22) If  $r_0 = 21$ , then  $\Omega^{21}(Z_t^{(29)})$  is described with  $(14s \times 14s)$  matrix with the following nonzero entries:

$$\begin{aligned} b_{j,4s} &= w_{8(j+m) \rightarrow 8(j+m+1)} \otimes e_{8j+2}; \\ b_{j,6s} &= w_{8(j+m) \rightarrow 8(j+m+1)} \otimes e_{8j+4}; \\ b_{j,8s} &= w_{8(j+m) \rightarrow 8(j+m+1)} \otimes e_{8j+5}; \\ b_{j,9s} &= w_{8(j+m) \rightarrow 8(j+m+1)} \otimes e_{8j+6}. \end{aligned}$$

(23) If  $r_0 = 22$ , then  $\Omega^{22}(Z_t^{(29)})$  is described with  $(13s \times 13s)$  matrix with two nonzero entries:

$$\begin{aligned} b_{j,0} &= w_{8(j+m) \rightarrow 8(j+m+1)} \otimes e_{8j}; \\ b_{j,12s} &= w_{8(j+m) \rightarrow 8(j+m+1)} \otimes e_{8j+7}. \end{aligned}$$

(24) If  $r_0 = 23$ , then  $\Omega^{23}(Z_t^{(29)})$  is described with  $(11s \times 11s)$  matrix with the following nonzero entries:

$$\begin{aligned} b_{j,2s} &= w_{8(j+m) \rightarrow 8(j+m+1)} \otimes e_{8j+1}; \\ b_{j,4s} &= w_{8(j+m) \rightarrow 8(j+m+1)} \otimes e_{8j+3}; \\ b_{j,6s} &= w_{8(j+m) \rightarrow 8(j+m+1)} \otimes e_{8j+5}. \end{aligned}$$

(25) If  $r_0 = 24$ , then  $\Omega^{24}(Z_t^{(29)})$  is described with  $(11s \times 11s)$  matrix with two nonzero entries:

$$\begin{aligned} b_{j,0} &= w_{8(j+m) \rightarrow 8(j+m+1)} \otimes e_{8j}; \\ b_{j,9s} &= w_{8(j+m) \rightarrow 8(j+m+1)} \otimes e_{8j+7}. \end{aligned}$$

(26) If  $r_0 = 25$ , then  $\Omega^{25}(Z_t^{(29)})$  is described with  $(10s \times 10s)$  matrix with two nonzero entries:

$$\begin{aligned} b_{j,3s} &= w_{8(j+m) \rightarrow 8(j+m+1)} \otimes e_{8j+2}; \\ b_{j,7s} &= w_{8(j+m) \rightarrow 8(j+m+1)} \otimes e_{8j+6}. \end{aligned}$$

(27) If  $r_0 = 26$ , then  $\Omega^{26}(Z_t^{(29)})$  is described with  $(8s \times 8s)$  matrix with unique nonzero entry:

$$b_{j,7s} = w_{8(j+m) \rightarrow 8(j+m+1)} \otimes e_{8j+7}.$$

(28) If  $r_0 = 27$ , then  $\Omega^{27}(Z_t^{(29)})$  is described with  $(9s \times 9s)$  matrix with two nonzero entries:

$$\begin{aligned} b_{j,s} &= w_{8(j+m) \rightarrow 8(j+m+1)} \otimes e_{8j+1}; \\ b_{j,5s} &= w_{8(j+m) \rightarrow 8(j+m+1)} \otimes e_{8j+5}. \end{aligned}$$

(29) If  $r_0 = 28$ , then  $\Omega^{28}(Z_t^{(29)})$  is described with  $(8s \times 8s)$  matrix with unique nonzero entry:

$$b_{j,0} = w_{8(j+m) \rightarrow 8(j+m+1)} \otimes e_{8j}.$$

(II) Represent an arbitrary  $t_0 \in \mathbb{N}$  in the form  $t_0 = 29\ell_0 + r_0$ , where  $0 \leq r_0 \leq 28$ . Then  $\Omega^{t_0}(Z_t^{(29)})$  is a  $\Omega^{r_0}(Z_t^{(29)})$ , whose left components twisted by  $\sigma^{\ell_0}$ , and coefficients multiplied by  $(-1)^{\ell_0}$ .

**Proposition 25** (Translates for the case 30). (I) Let  $r_0 \in \mathbb{N}$ ,  $r_0 < 29$ .  $r_0$ -translates of the elements  $Z_t^{(30)}$  are described by the following way.

(1) If  $r_0 = 0$ , then  $\Omega^0(Z_t^{(30)})$  is described with  $(8s \times 8s)$  matrix with unique nonzero entry:

$$b_{j,s} = w_{8(j+m)+1 \rightarrow 8(j+m+1)+1} \otimes e_{8j+1}.$$

(2) If  $r_0 = 1$ , then  $\Omega^1(Z_t^{(30)})$  is described with  $(9s \times 9s)$  matrix with unique nonzero entry:

$$b_{j,0} = w_{8(j+m)+1 \rightarrow 8(j+m+1)+1} \otimes e_{8j}.$$

(3) If  $r_0 = 2$ , then  $\Omega^2(Z_t^{(30)})$  is described with  $(8s \times 8s)$  matrix with unique nonzero entry:

$$b_{j,6s} = w_{8(j+m)+1 \rightarrow 8(j+m+1)+1} \otimes e_{8j+6}.$$

(4) If  $r_0 = 3$ , then  $\Omega^3(Z_t^{(30)})$  is described with  $(10s \times 10s)$  matrix with unique nonzero entry:

$$b_{j,8s} = w_{8(j+m)+1 \rightarrow 8(j+m+1)+1} \otimes e_{8j+7}.$$

(5) If  $r_0 = 4$ , then  $\Omega^4(Z_t^{(30)})$  is described with  $(11s \times 11s)$  matrix with two nonzero entries:

$$b_{j,6s} = w_{8(j+m)+1 \rightarrow 8(j+m+1)+1} \otimes e_{8j+4};$$

$$b_{j,7s} = w_{8(j+m)+1 \rightarrow 8(j+m+1)+1} \otimes e_{8j+5}.$$

(6) If  $r_0 = 5$ , then  $\Omega^5(Z_t^{(30)})$  is described with  $(11s \times 11s)$  matrix with unique nonzero entry:

$$b_{j,2s} = w_{8(j+m)+1 \rightarrow 8(j+m+1)+1} \otimes e_{8j}.$$

(7) If  $r_0 = 6$ , then  $\Omega^6(Z_t^{(30)})$  is described with  $(13s \times 13s)$  matrix with unique nonzero entry:

$$b_{j,5s} = w_{8(j+m)+1 \rightarrow 8(j+m+1)+1} \otimes e_{8j+3}.$$

(8) If  $r_0 = 7$ , then  $\Omega^7(Z_t^{(30)})$  is described with  $(14s \times 14s)$  matrix with unique nonzero entry:

$$b_{j,13s} = w_{8(j+m)+1 \rightarrow 8(j+m+1)+1} \otimes e_{8j+7}.$$

(9) If  $r_0 = 8$ , then  $\Omega^8(Z_t^{(30)})$  is described with  $(16s \times 16s)$  matrix with two nonzero entries:

$$b_{j,5s} = w_{8(j+m)+1 \rightarrow 8(j+m+1)+1} \otimes e_{8j+2};$$

$$b_{j,13s} = w_{8(j+m)+1 \rightarrow 8(j+m+1)+1} \otimes e_{8j+6}.$$

(10) If  $r_0 = 9$ , then  $\Omega^9(Z_t^{(30)})$  is described with  $(16s \times 16s)$  matrix with unique nonzero entry:

$$b_{j,3s} = w_{8(j+m)+1 \rightarrow 8(j+m+1)+1} \otimes e_{8j}.$$

(11) If  $r_0 = 10$ , then  $\Omega^{10}(Z_t^{(30)})$  is described with  $(19s \times 19s)$  matrix with two nonzero entries:

$$b_{j,4s} = w_{8(j+m)+1 \rightarrow 8(j+m+1)+1} \otimes e_{8j+1};$$

$$b_{j,12s} = w_{8(j+m)+1 \rightarrow 8(j+m+1)+1} \otimes e_{8j+5}.$$

(12) If  $r_0 = 11$ , then  $\Omega^{11}(Z_t^{(30)})$  is described with  $(18s \times 18s)$  matrix with two nonzero entries:

$$b_{j,3s} = w_{8(j+m)+1 \rightarrow 8(j+m+1)+1} \otimes e_{8j};$$

$$b_{j,17s} = w_{8(j+m)+1 \rightarrow 8(j+m+1)+1} \otimes e_{8j+7}.$$

(13) If  $r_0 = 12$ , then  $\Omega^{12}(Z_t^{(30)})$  is described with  $(19s \times 19s)$  matrix with two nonzero entries:

$$b_{j,9s} = w_{8(j+m)+1 \rightarrow 8(j+m+1)+1} \otimes e_{8j+4};$$

$$b_{j,15s} = w_{8(j+m)+1 \rightarrow 8(j+m+1)+1} \otimes e_{8j+6}.$$

(14) If  $r_0 = 13$ , then  $\Omega^{13}(Z_t^{(30)})$  is described with  $(18s \times 18s)$  matrix with unique nonzero entry:

$$b_{j,16s} = w_{8(j+m)+1 \rightarrow 8(j+m+1)+1} \otimes e_{8j+7}.$$

(15) If  $r_0 = 14$ , then  $\Omega^{14}(Z_t^{(30)})$  is described with  $(20s \times 20s)$  matrix with two nonzero entries:

$$b_{j,8s} = w_{8(j+m)+1 \rightarrow 8(j+m+1)+1} \otimes e_{8j+3};$$

$$b_{j,13s} = w_{8(j+m)+1 \rightarrow 8(j+m+1)+1} \otimes e_{8j+5}.$$

(16) If  $r_0 = 15$ , then  $\Omega^{15}(Z_t^{(30)})$  is described with  $(18s \times 18s)$  matrix with unique nonzero entry:

$$b_{j,3s} = w_{8(j+m)+1 \rightarrow 8(j+m+1)+1} \otimes e_{8j}.$$

(17) If  $r_0 = 16$ , then  $\Omega^{16}(Z_t^{(30)})$  is described with  $(19s \times 19s)$  matrix with unique nonzero entry:

$$b_{j,6s} = w_{8(j+m)+1 \rightarrow 8(j+m+1)+1} \otimes e_{8j+2}.$$

(18) If  $r_0 = 17$ , then  $\Omega^{17}(Z_t^{(30)})$  is described with  $(18s \times 18s)$  matrix with unique nonzero entry:

$$b_{j,16s} = w_{8(j+m)+1 \rightarrow 8(j+m+1)+1} \otimes e_{8j+7}.$$

(19) If  $r_0 = 18$ , then  $\Omega^{18}(Z_t^{(30)})$  is described with  $(19s \times 19s)$  matrix with two nonzero entries:

$$b_{j,4s} = w_{8(j+m)+1 \rightarrow 8(j+m+1)+1} \otimes e_{8j+1};$$

$$b_{j,15s} = w_{8(j+m)+1 \rightarrow 8(j+m+1)+1} \otimes e_{8j+6}.$$

(20) If  $r_0 = 19$ , then  $\Omega^{19}(Z_t^{(30)})$  is described with  $(16s \times 16s)$  matrix with unique nonzero entry:

$$b_{j,2s} = w_{8(j+m)+1 \rightarrow 8(j+m+1)+1} \otimes e_{8j}.$$

(21) If  $r_0 = 20$ , then  $\Omega^{20}(Z_t^{(30)})$  is described with  $(16s \times 16s)$  matrix with unique nonzero entry:

$$b_{j,10s} = w_{8(j+m)+1 \rightarrow 8(j+m+1)+1} \otimes e_{8j+5}.$$

(22) If  $r_0 = 21$ , then  $\Omega^{21}(Z_t^{(30)})$  is described with  $(14s \times 14s)$  matrix with unique nonzero entry:

$$b_{j,12s} = w_{8(j+m)+1 \rightarrow 8(j+m+1)+1} \otimes e_{8j+7}.$$

(23) If  $r_0 = 22$ , then  $\Omega^{22}(Z_t^{(30)})$  is described with  $(13s \times 13s)$  matrix with unique nonzero entry:

$$b_{j,6s} = w_{8(j+m)+1 \rightarrow 8(j+m+1)+1} \otimes e_{8j+4}.$$

(24) If  $r_0 = 23$ , then  $\Omega^{23}(Z_t^{(30)})$  is described with  $(11s \times 11s)$  matrix with unique nonzero entry:

$$b_{j,5s} = w_{8(j+m)+1 \rightarrow 8(j+m+1)+1} \otimes e_{8j+4}.$$

(25) If  $r_0 = 24$ , then  $\Omega^{24}(Z_t^{(30)})$  is described with  $(11s \times 11s)$  matrix with unique nonzero entry:

$$b_{j,4s} = w_{8(j+m)+1 \rightarrow 8(j+m+1)+1} \otimes e_{8j+3}.$$

(26) If  $r_0 = 25$ , then  $\Omega^{25}(Z_t^{(30)})$  is described with  $(10s \times 10s)$  matrix with unique nonzero entry:

$$b_{j,4s} = w_{8(j+m)+1 \rightarrow 8(j+m+1)+1} \otimes e_{8j+3}.$$

(27) If  $r_0 = 26$ , then  $\Omega^{26}(Z_t^{(30)})$  is described with  $(8s \times 8s)$  matrix with unique nonzero entry:

$$b_{j,2s} = w_{8(j+m)+1 \rightarrow 8(j+m+1)+1} \otimes e_{8j+2}.$$

(28) If  $r_0 = 27$ , then  $\Omega^{27}(Z_t^{(30)})$  is described with  $(9s \times 9s)$  matrix with unique nonzero entry:

$$b_{j,2s} = w_{8(j+m)+1 \rightarrow 8(j+m+1)+1} \otimes e_{8j+2}.$$

(29) If  $r_0 = 28$ , then  $\Omega^{28}(Z_t^{(30)})$  is described with  $(8s \times 8s)$  matrix with unique nonzero entry:

$$b_{j,s} = w_{8(j+m)+1 \rightarrow 8(j+m+1)+1} \otimes e_{8j+1}.$$

(II) Represent an arbitrary  $t_0 \in \mathbb{N}$  in the form  $t_0 = 29\ell_0 + r_0$ , where  $0 \leq r_0 \leq 28$ . Then  $\Omega^{t_0}(Z_t^{(30)})$  is a  $\Omega^{r_0}(Z_t^{(30)})$ , whose left components twisted by  $\sigma^{\ell_0}$ , and coefficients multiplied by  $(-1)^{\ell_0}$ .

**Proposition 26** (Translates for the case 31). (I) Let  $r_0 \in \mathbb{N}$ ,  $r_0 < 29$ .  $r_0$ -translates of the elements  $Z_t^{(31)}$  are described by the following way.

(1) If  $r_0 = 0$ , then  $\Omega^0(Z_t^{(31)})$  is described with  $(8s \times 8s)$  matrix with unique nonzero entry:

$$b_{j,2s} = w_{8(j+m)+2 \rightarrow 8(j+m+1)+2} \otimes e_{8j+2}.$$

(2) If  $r_0 = 1$ , then  $\Omega^1(Z_t^{(31)})$  is described with  $(9s \times 9s)$  matrix with unique nonzero entry:

$$b_{j,2s} = w_{8(j+m)+2 \rightarrow 8(j+m+1)+2} \otimes e_{8j+1}.$$

(3) If  $r_0 = 2$ , then  $\Omega^2(Z_t^{(31)})$  is described with  $(8s \times 8s)$  matrix with unique nonzero entry:

$$b_{j,s} = w_{8(j+m)+2 \rightarrow 8(j+m+1)+2} \otimes e_{8j+1}.$$

(4) If  $r_0 = 3$ , then  $\Omega^3(Z_t^{(31)})$  is described with  $(10s \times 10s)$  matrix with unique nonzero entry:

$$b_{j,0} = w_{8(j+m)+2 \rightarrow 8(j+m+1)+2} \otimes e_{8j}.$$

(5) If  $r_0 = 4$ , then  $\Omega^4(Z_t^{(31)})$  is described with  $(11s \times 11s)$  matrix with unique nonzero entry:

$$b_{j,8s} = w_{8(j+m)+2 \rightarrow 8(j+m+1)+2} \otimes e_{8j+6}.$$

(6) If  $r_0 = 5$ , then  $\Omega^5(Z_t^{(31)})$  is described with  $(11s \times 11s)$  matrix with unique nonzero entry:

$$b_{j,9s} = w_{8(j+m)+2 \rightarrow 8(j+m+1)+2} \otimes e_{8j+7}.$$

(7) If  $r_0 = 6$ , then  $\Omega^6(Z_t^{(31)})$  is described with  $(13s \times 13s)$  matrix with two nonzero entries:

$$b_{j,6s} = w_{8(j+m)+2 \rightarrow 8(j+m+1)+2} \otimes e_{8j+4};$$

$$b_{j,7s} = w_{8(j+m)+2 \rightarrow 8(j+m+1)+2} \otimes e_{8j+5}.$$

(8) If  $r_0 = 7$ , then  $\Omega^7(Z_t^{(31)})$  is described with  $(14s \times 14s)$  matrix with unique nonzero entry:

$$b_{j,0} = w_{8(j+m)+2 \rightarrow 8(j+m+1)+2} \otimes e_{8j}.$$

(9) If  $r_0 = 8$ , then  $\Omega^8(Z_t^{(31)})$  is described with  $(16s \times 16s)$  matrix with unique nonzero entry:

$$b_{j,6s} = w_{8(j+m)+2 \rightarrow 8(j+m+1)+2} \otimes e_{8j+3}.$$

(10) If  $r_0 = 9$ , then  $\Omega^9(Z_t^{(31)})$  is described with  $(16s \times 16s)$  matrix with unique nonzero entry:

$$b_{j,12s} = w_{8(j+m)+2 \rightarrow 8(j+m+1)+2} \otimes e_{8j+7}.$$

(11) If  $r_0 = 10$ , then  $\Omega^{10}(Z_t^{(31)})$  is described with  $(19s \times 19s)$  matrix with two nonzero entries:

$$b_{j,5s} = w_{8(j+m)+2 \rightarrow 8(j+m+1)+2} \otimes e_{8j+2};$$

$$b_{j,13s} = w_{8(j+m)+2 \rightarrow 8(j+m+1)+2} \otimes e_{8j+6}.$$

(12) If  $r_0 = 11$ , then  $\Omega^{11}(Z_t^{(31)})$  is described with  $(18s \times 18s)$  matrix with unique nonzero entry:

$$b_{j,0} = w_{8(j+m)+2 \rightarrow 8(j+m+1)+2} \otimes e_{8j}.$$

(13) If  $r_0 = 12$ , then  $\Omega^{12}(Z_t^{(31)})$  is described with  $(19s \times 19s)$  matrix with two nonzero entries:

$$b_{j,3s} = w_{8(j+m)+2 \rightarrow 8(j+m+1)+2} \otimes e_{8j+1};$$

$$b_{j,10s} = w_{8(j+m)+2 \rightarrow 8(j+m+1)+2} \otimes e_{8j+5}.$$

(14) If  $r_0 = 13$ , then  $\Omega^{13}(Z_t^{(31)})$  is described with  $(18s \times 18s)$  matrix with two nonzero entries:

$$b_{j,0} = w_{8(j+m)+2 \rightarrow 8(j+m+1)+2} \otimes e_{8j};$$

$$b_{j,13s} = w_{8(j+m)+2 \rightarrow 8(j+m+1)+2} \otimes e_{8j+7}.$$

(15) If  $r_0 = 14$ , then  $\Omega^{14}(Z_t^{(31)})$  is described with  $(20s \times 20s)$  matrix with two nonzero entries:

$$b_{j,9s} = w_{8(j+m)+2 \rightarrow 8(j+m+1)+2} \otimes e_{8j+4};$$

$$b_{j,14s} = w_{8(j+m)+2 \rightarrow 8(j+m+1)+2} \otimes e_{8j+6}.$$

(16) If  $r_0 = 15$ , then  $\Omega^{15}(Z_t^{(31)})$  is described with  $(18s \times 18s)$  matrix with unique nonzero entry:

$$b_{j,14s} = w_{8(j+m)+2 \rightarrow 8(j+m+1)+2} \otimes e_{8j+7}.$$

(17) If  $r_0 = 16$ , then  $\Omega^{16}(Z_t^{(31)})$  is described with  $(19s \times 19s)$  matrix with two nonzero entries:

$$b_{j,7s} = w_{8(j+m)+2 \rightarrow 8(j+m+1)+2} \otimes e_{8j+3};$$

$$b_{j,10s} = w_{8(j+m)+2 \rightarrow 8(j+m+1)+2} \otimes e_{8j+5}.$$

(18) If  $r_0 = 17$ , then  $\Omega^{17}(Z_t^{(31)})$  is described with  $(18s \times 18s)$  matrix with unique nonzero entry:

$$b_{j,0} = w_{8(j+m)+2 \rightarrow 8(j+m+1)+2} \otimes e_{8j}.$$

(19) If  $r_0 = 18$ , then  $\Omega^{18}(Z_t^{(31)})$  is described with  $(19s \times 19s)$  matrix with unique nonzero entry:

$$b_{j,5s} = w_{8(j+m)+2 \rightarrow 8(j+m+1)+2} \otimes e_{8j+2}.$$

(20) If  $r_0 = 19$ , then  $\Omega^{19}(Z_t^{(31)})$  is described with  $(16s \times 16s)$  matrix with unique nonzero entry:

$$b_{j,12s} = w_{8(j+m)+2 \rightarrow 8(j+m+1)+2} \otimes e_{8j+7}.$$

(21) If  $r_0 = 20$ , then  $\Omega^{20}(Z_t^{(31)})$  is described with  $(16s \times 16s)$  matrix with two nonzero entries:

$$b_{j,2s} = w_{8(j+m)+2 \rightarrow 8(j+m+1)+2} \otimes e_{8j+1};$$

$$b_{j,11s} = w_{8(j+m)+2 \rightarrow 8(j+m+1)+2} \otimes e_{8j+6}.$$

(22) If  $r_0 = 21$ , then  $\Omega^{21}(Z_t^{(31)})$  is described with  $(14s \times 14s)$  matrix with unique nonzero entry:

$$b_{j,0} = w_{8(j+m)+2 \rightarrow 8(j+m+1)+2} \otimes e_{8j}.$$

(23) If  $r_0 = 22$ , then  $\Omega^{22}(Z_t^{(31)})$  is described with  $(13s \times 13s)$  matrix with unique nonzero entry:

$$b_{j,7s} = w_{8(j+m)+2 \rightarrow 8(j+m+1)+2} \otimes e_{8j+5}.$$

(24) If  $r_0 = 23$ , then  $\Omega^{23}(Z_t^{(31)})$  is described with  $(11s \times 11s)$  matrix with unique nonzero entry:

$$b_{j,8s} = w_{8(j+m)+2 \rightarrow 8(j+m+1)+2} \otimes e_{8j+7}.$$

(25) If  $r_0 = 24$ , then  $\Omega^{24}(Z_t^{(31)})$  is described with  $(11s \times 11s)$  matrix with unique nonzero entry:

$$b_{j,5s} = w_{8(j+m)+2 \rightarrow 8(j+m+1)+2} \otimes e_{8j+4}.$$

(26) If  $r_0 = 25$ , then  $\Omega^{25}(Z_t^{(31)})$  is described with  $(10s \times 10s)$  matrix with unique nonzero entry:

$$b_{j,5s} = w_{8(j+m)+2 \rightarrow 8(j+m+1)+2} \otimes e_{8j+4}.$$

(27) If  $r_0 = 26$ , then  $\Omega^{26}(Z_t^{(31)})$  is described with  $(8s \times 8s)$  matrix with unique nonzero entry:

$$b_{j,3s} = w_{8(j+m)+2 \rightarrow 8(j+m+1)+2} \otimes e_{8j+3}.$$

(28) If  $r_0 = 27$ , then  $\Omega^{27}(Z_t^{(31)})$  is described with  $(9s \times 9s)$  matrix with unique nonzero entry:

$$b_{j,3s} = w_{8(j+m)+2 \rightarrow 8(j+m+1)+2} \otimes e_{8j+3}.$$

(29) If  $r_0 = 28$ , then  $\Omega^{28}(Z_t^{(31)})$  is described with  $(8s \times 8s)$  matrix with unique nonzero entry:

$$b_{j,2s} = w_{8(j+m)+2 \rightarrow 8(j+m+1)+2} \otimes e_{8j+2}.$$

(II) Represent an arbitrary  $t_0 \in \mathbb{N}$  in the form  $t_0 = 29\ell_0 + r_0$ , where  $0 \leq r_0 \leq 28$ . Then  $\Omega^{t_0}(Z_t^{(31)})$  is a  $\Omega^{r_0}(Z_t^{(31)})$ , whose left components twisted by  $\sigma^{\ell_0}$ , and coefficients multiplied by  $(-1)^{\ell_0}$ .

**Proposition 27** (Translates for the case 32). (I) Let  $r_0 \in \mathbb{N}$ ,  $r_0 < 29$ .  $r_0$ -translates of the elements  $Z_t^{(32)}$  are described by the following way.

(1) If  $r_0 = 0$ , then  $\Omega^0(Z_t^{(32)})$  is described with  $(8s \times 8s)$  matrix with unique nonzero entry:

$$b_{j,3s} = w_{8(j+m)+3 \rightarrow 8(j+m+1)+3} \otimes e_{8j+3}.$$

(2) If  $r_0 = 1$ , then  $\Omega^1(Z_t^{(32)})$  is described with  $(9s \times 9s)$  matrix with unique nonzero entry:

$$b_{j,3s} = w_{8(j+m)+3 \rightarrow 8(j+m+1)+3} \otimes e_{8j+2}.$$

(3) If  $r_0 = 2$ , then  $\Omega^2(Z_t^{(32)})$  is described with  $(8s \times 8s)$  matrix with unique nonzero entry:

$$b_{j,2s} = w_{8(j+m)+3 \rightarrow 8(j+m+1)+3} \otimes e_{8j+2}.$$

(4) If  $r_0 = 3$ , then  $\Omega^3(Z_t^{(32)})$  is described with  $(10s \times 10s)$  matrix with unique nonzero entry:

$$b_{j,2s} = w_{8(j+m)+3 \rightarrow 8(j+m+1)+3} \otimes e_{8j+1}.$$

(5) If  $r_0 = 4$ , then  $\Omega^4(Z_t^{(32)})$  is described with  $(11s \times 11s)$  matrix with unique nonzero entry:

$$b_{j,2s} = w_{8(j+m)+3 \rightarrow 8(j+m+1)+3} \otimes e_{8j+1}.$$

(6) If  $r_0 = 5$ , then  $\Omega^5(Z_t^{(32)})$  is described with  $(11s \times 11s)$  matrix with unique nonzero entry:

$$b_{j,s} = w_{8(j+m)+3 \rightarrow 8(j+m+1)+3} \otimes e_{8j}.$$

(7) If  $r_0 = 6$ , then  $\Omega^6(Z_t^{(32)})$  is described with  $(13s \times 13s)$  matrix with unique nonzero entry:

$$b_{j,9s} = w_{8(j+m)+3 \rightarrow 8(j+m+1)+3} \otimes e_{8j+6}.$$

(8) If  $r_0 = 7$ , then  $\Omega^7(Z_t^{(32)})$  is described with  $(14s \times 14s)$  matrix with unique nonzero entry:

$$b_{j,12s} = w_{8(j+m)+3 \rightarrow 8(j+m+1)+3} \otimes e_{8j+7}.$$

(9) If  $r_0 = 8$ , then  $\Omega^8(Z_t^{(32)})$  is described with  $(16s \times 16s)$  matrix with two nonzero entries:

$$b_{j,7s} = w_{8(j+m)+3 \rightarrow 8(j+m+1)+3} \otimes e_{8j+4};$$

$$b_{j,9s} = w_{8(j+m)+3 \rightarrow 8(j+m+1)+3} \otimes e_{8j+5}.$$

(10) If  $r_0 = 9$ , then  $\Omega^9(Z_t^{(32)})$  is described with  $(16s \times 16s)$  matrix with unique nonzero entry:

$$b_{j,s} = w_{8(j+m)+3 \rightarrow 8(j+m+1)+3} \otimes e_{8j}.$$

(11) If  $r_0 = 10$ , then  $\Omega^{10}(Z_t^{(32)})$  is described with  $(19s \times 19s)$  matrix with unique nonzero entry:

$$b_{j,6s} = w_{8(j+m)+3 \rightarrow 8(j+m+1)+3} \otimes e_{8j+3}.$$

(12) If  $r_0 = 11$ , then  $\Omega^{11}(Z_t^{(32)})$  is described with  $(18s \times 18s)$  matrix with unique nonzero entry:

$$b_{j,15s} = w_{8(j+m)+3 \rightarrow 8(j+m+1)+3} \otimes e_{8j+7}.$$

(13) If  $r_0 = 12$ , then  $\Omega^{12}(Z_t^{(32)})$  is described with  $(19s \times 19s)$  matrix with two nonzero entries:

$$b_{j,4s} = w_{8(j+m)+3 \rightarrow 8(j+m+1)+3} \otimes e_{8j+2};$$

$$b_{j,14s} = w_{8(j+m)+3 \rightarrow 8(j+m+1)+3} \otimes e_{8j+6}.$$

(14) If  $r_0 = 13$ , then  $\Omega^{13}(Z_t^{(32)})$  is described with  $(18s \times 18s)$  matrix with unique nonzero entry:

$$b_{j,s} = w_{8(j+m)+3 \rightarrow 8(j+m+1)+3} \otimes e_{8j}.$$

(15) If  $r_0 = 14$ , then  $\Omega^{14}(Z_t^{(32)})$  is described with  $(20s \times 20s)$  matrix with two nonzero entries:

$$b_{j,3s} = w_{8(j+m)+3 \rightarrow 8(j+m+1)+3} \otimes e_{8j+1};$$

$$b_{j,12s} = w_{8(j+m)+3 \rightarrow 8(j+m+1)+3} \otimes e_{8j+5}.$$

(16) If  $r_0 = 15$ , then  $\Omega^{15}(Z_t^{(32)})$  is described with  $(18s \times 18s)$  matrix with two nonzero entries:

$$b_{j,0} = w_{8(j+m)+3 \rightarrow 8(j+m+1)+3} \otimes e_{8j};$$

$$b_{j,15s} = w_{8(j+m)+3 \rightarrow 8(j+m+1)+3} \otimes e_{8j+7}.$$

(17) If  $r_0 = 16$ , then  $\Omega^{16}(Z_t^{(32)})$  is described with  $(19s \times 19s)$  matrix with two nonzero entries:

$$b_{j,9s} = w_{8(j+m)+3 \rightarrow 8(j+m+1)+3} \otimes e_{8j+4};$$

$$b_{j,13s} = w_{8(j+m)+3 \rightarrow 8(j+m+1)+3} \otimes e_{8j+6}.$$

(18) If  $r_0 = 17$ , then  $\Omega^{17}(Z_t^{(32)})$  is described with  $(18s \times 18s)$  matrix with unique nonzero entry:

$$b_{j,13s} = w_{8(j+m)+3 \rightarrow 8(j+m+1)+3} \otimes e_{8j+7}.$$

(19) If  $r_0 = 18$ , then  $\Omega^{18}(Z_t^{(32)})$  is described with  $(19s \times 19s)$  matrix with two nonzero entries:

$$b_{j,7s} = w_{8(j+m)+3 \rightarrow 8(j+m+1)+3} \otimes e_{8j+3};$$

$$b_{j,10s} = w_{8(j+m)+3 \rightarrow 8(j+m+1)+3} \otimes e_{8j+5}.$$

(20) If  $r_0 = 19$ , then  $\Omega^{19}(Z_t^{(32)})$  is described with  $(16s \times 16s)$  matrix with unique nonzero entry:

$$b_{j,0} = w_{8(j+m)+3 \rightarrow 8(j+m+1)+3} \otimes e_{8j}.$$

(21) If  $r_0 = 20$ , then  $\Omega^{20}(Z_t^{(32)})$  is described with  $(16s \times 16s)$  matrix with unique nonzero entry:

$$b_{j,4s} = w_{8(j+m)+3 \rightarrow 8(j+m+1)+3} \otimes e_{8j+2}.$$

(22) If  $r_0 = 21$ , then  $\Omega^{21}(Z_t^{(32)})$  is described with  $(14s \times 14s)$  matrix with unique nonzero entry:

$$b_{j,10s} = w_{8(j+m)+3 \rightarrow 8(j+m+1)+3} \otimes e_{8j+7}.$$

(23) If  $r_0 = 22$ , then  $\Omega^{22}(Z_t^{(32)})$  is described with  $(13s \times 13s)$  matrix with two nonzero entries:

$$b_{j,2s} = w_{8(j+m)+3 \rightarrow 8(j+m+1)+3} \otimes e_{8j+1};$$

$$b_{j,9s} = w_{8(j+m)+3 \rightarrow 8(j+m+1)+3} \otimes e_{8j+6}.$$

(24) If  $r_0 = 23$ , then  $\Omega^{23}(Z_t^{(32)})$  is described with  $(11s \times 11s)$  matrix with unique nonzero entry:

$$b_{j,0} = w_{8(j+m)+3 \rightarrow 8(j+m+1)+3} \otimes e_{8j}.$$

(25) If  $r_0 = 24$ , then  $\Omega^{24}(Z_t^{(32)})$  is described with  $(11s \times 11s)$  matrix with unique nonzero entry:

$$b_{j,6s} = w_{8(j+m)+3 \rightarrow 8(j+m+1)+3} \otimes e_{8j+5}.$$

(26) If  $r_0 = 25$ , then  $\Omega^{25}(Z_t^{(32)})$  is described with  $(10s \times 10s)$  matrix with unique nonzero entry:

$$b_{j,8s} = w_{8(j+m)+3 \rightarrow 8(j+m+1)+3} \otimes e_{8j+7}.$$

(27) If  $r_0 = 26$ , then  $\Omega^{26}(Z_t^{(32)})$  is described with  $(8s \times 8s)$  matrix with unique nonzero entry:

$$b_{j,4s} = w_{8(j+m)+3 \rightarrow 8(j+m+1)+3} \otimes e_{8j+4}.$$

(28) If  $r_0 = 27$ , then  $\Omega^{27}(Z_t^{(32)})$  is described with  $(9s \times 9s)$  matrix with unique nonzero entry:

$$b_{j,4s} = w_{8(j+m)+3 \rightarrow 8(j+m+1)+3} \otimes e_{8j+4}.$$

(29) If  $r_0 = 28$ , then  $\Omega^{28}(Z_t^{(32)})$  is described with  $(8s \times 8s)$  matrix with unique nonzero entry:

$$b_{j,3s} = w_{8(j+m)+3 \rightarrow 8(j+m+1)+3} \otimes e_{8j+3}.$$

(II) Represent an arbitrary  $t_0 \in \mathbb{N}$  in the form  $t_0 = 29\ell_0 + r_0$ , where  $0 \leq r_0 \leq 28$ . Then  $\Omega^{t_0}(Z_t^{(32)})$  is a  $\Omega^{r_0}(Z_t^{(32)})$ , whose left components twisted by  $\sigma^{\ell_0}$ , and coefficients multiplied by  $(-1)^{\ell_0}$ .

**Proposition 28** (Translates for the case 33). (I) Let  $r_0 \in \mathbb{N}$ ,  $r_0 < 29$ .  $r_0$ -translates of the elements  $Z_t^{(33)}$  are described by the following way.

(1) If  $r_0 = 0$ , then  $\Omega^0(Z_t^{(33)})$  is described with  $(8s \times 8s)$  matrix with unique nonzero entry:

$$b_{j,4s} = w_{8(j+m)+4 \rightarrow 8(j+m+1)+4} \otimes e_{8j+4}.$$

(2) If  $r_0 = 1$ , then  $\Omega^1(Z_t^{(33)})$  is described with  $(9s \times 9s)$  matrix with unique nonzero entry:

$$b_{j,4s} = w_{8(j+m)+4 \rightarrow 8(j+m+1)+4} \otimes e_{8j+3}.$$

(3) If  $r_0 = 2$ , then  $\Omega^2(Z_t^{(33)})$  is described with  $(8s \times 8s)$  matrix with unique nonzero entry:

$$b_{j,3s} = w_{8(j+m)+4 \rightarrow 8(j+m+1)+4} \otimes e_{8j+3}.$$

(4) If  $r_0 = 3$ , then  $\Omega^3(Z_t^{(33)})$  is described with  $(10s \times 10s)$  matrix with unique nonzero entry:

$$b_{j,3s} = w_{8(j+m)+4 \rightarrow 8(j+m+1)+4} \otimes e_{8j+2}.$$



(5) If  $r_0 = 4$ , then  $\Omega^4(Z_t^{(33)})$  is described with  $(11s \times 11s)$  matrix with unique nonzero entry:

$$b_{j,3s} = w_{8(j+m)+4 \rightarrow 8(j+m+1)+4} \otimes e_{8j+2}.$$

(6) If  $r_0 = 5$ , then  $\Omega^5(Z_t^{(33)})$  is described with  $(11s \times 11s)$  matrix with unique nonzero entry:

$$b_{j,3s} = w_{8(j+m)+4 \rightarrow 8(j+m+1)+4} \otimes e_{8j+1}.$$

(7) If  $r_0 = 6$ , then  $\Omega^6(Z_t^{(33)})$  is described with  $(13s \times 13s)$  matrix with unique nonzero entry:

$$b_{j,2s} = w_{8(j+m)+4 \rightarrow 8(j+m+1)+4} \otimes e_{8j+1}.$$

(8) If  $r_0 = 7$ , then  $\Omega^7(Z_t^{(33)})$  is described with  $(14s \times 14s)$  matrix with unique nonzero entry:

$$b_{j,s} = w_{8(j+m)+4 \rightarrow 8(j+m+1)+4} \otimes e_{8j}.$$

(9) If  $r_0 = 8$ , then  $\Omega^8(Z_t^{(33)})$  is described with  $(16s \times 16s)$  matrix with unique nonzero entry:

$$b_{j,12s} = w_{8(j+m)+4 \rightarrow 8(j+m+1)+4} \otimes e_{8j+6}.$$

(10) If  $r_0 = 9$ , then  $\Omega^9(Z_t^{(33)})$  is described with  $(16s \times 16s)$  matrix with unique nonzero entry:

$$b_{j,13s} = w_{8(j+m)+4 \rightarrow 8(j+m+1)+4} \otimes e_{8j+7}.$$

(11) If  $r_0 = 10$ , then  $\Omega^{10}(Z_t^{(33)})$  is described with  $(19s \times 19s)$  matrix with two nonzero entries:

$$b_{j,8s} = w_{8(j+m)+4 \rightarrow 8(j+m+1)+4} \otimes e_{8j+4};$$

$$b_{j,11s} = w_{8(j+m)+4 \rightarrow 8(j+m+1)+4} \otimes e_{8j+5}.$$

(12) If  $r_0 = 11$ , then  $\Omega^{11}(Z_t^{(33)})$  is described with  $(18s \times 18s)$  matrix with unique nonzero entry:

$$b_{j,2s} = w_{8(j+m)+4 \rightarrow 8(j+m+1)+4} \otimes e_{8j}.$$

(13) If  $r_0 = 12$ , then  $\Omega^{12}(Z_t^{(33)})$  is described with  $(19s \times 19s)$  matrix with unique nonzero entry:

$$b_{j,6s} = w_{8(j+m)+4 \rightarrow 8(j+m+1)+4} \otimes e_{8j+3}.$$

(14) If  $r_0 = 13$ , then  $\Omega^{13}(Z_t^{(33)})$  is described with  $(18s \times 18s)$  matrix with unique nonzero entry:

$$b_{j,15s} = w_{8(j+m)+4 \rightarrow 8(j+m+1)+4} \otimes e_{8j+7}.$$

(15) If  $r_0 = 14$ , then  $\Omega^{14}(Z_t^{(33)})$  is described with  $(20s \times 20s)$  matrix with two nonzero entries:

$$b_{j,5s} = w_{8(j+m)+4 \rightarrow 8(j+m+1)+4} \otimes e_{8j+2};$$

$$b_{j,15s} = w_{8(j+m)+4 \rightarrow 8(j+m+1)+4} \otimes e_{8j+6}.$$

(16) If  $r_0 = 15$ , then  $\Omega^{15}(Z_t^{(33)})$  is described with  $(18s \times 18s)$  matrix with unique nonzero entry:

$$b_{j,2s} = w_{8(j+m)+4 \rightarrow 8(j+m+1)+4} \otimes e_{8j}.$$

(17) If  $r_0 = 16$ , then  $\Omega^{16}(Z_t^{(33)})$  is described with  $(19s \times 19s)$  matrix with two nonzero entries:

$$b_{j,3s} = w_{8(j+m)+4 \rightarrow 8(j+m+1)+4} \otimes e_{8j+1};$$

$$b_{j,11s} = w_{8(j+m)+4 \rightarrow 8(j+m+1)+4} \otimes e_{8j+5}.$$

(18) If  $r_0 = 17$ , then  $\Omega^{17}(Z_t^{(33)})$  is described with  $(18s \times 18s)$  matrix with two nonzero entries:

$$b_{j,s} = w_{8(j+m)+4 \rightarrow 8(j+m+1)+4} \otimes e_{8j};$$

$$b_{j,15s} = w_{8(j+m)+4 \rightarrow 8(j+m+1)+4} \otimes e_{8j+7}.$$

(19) If  $r_0 = 18$ , then  $\Omega^{18}(Z_t^{(33)})$  is described with  $(19s \times 19s)$  matrix with two nonzero entries:

$$b_{j,8s} = w_{8(j+m)+4 \rightarrow 8(j+m+1)+4} \otimes e_{8j+4};$$

$$b_{j,14s} = w_{8(j+m)+4 \rightarrow 8(j+m+1)+4} \otimes e_{8j+6}.$$

(20) If  $r_0 = 19$ , then  $\Omega^{19}(Z_t^{(33)})$  is described with  $(16s \times 16s)$  matrix with unique nonzero entry:

$$b_{j,13s} = w_{8(j+m)+4 \rightarrow 8(j+m+1)+4} \otimes e_{8j+7}.$$

(21) If  $r_0 = 20$ , then  $\Omega^{20}(Z_t^{(33)})$  is described with  $(16s \times 16s)$  matrix with two nonzero entries:

$$b_{j,5s} = w_{8(j+m)+4 \rightarrow 8(j+m+1)+4} \otimes e_{8j+3};$$

$$b_{j,9s} = w_{8(j+m)+4 \rightarrow 8(j+m+1)+4} \otimes e_{8j+5}.$$

(22) If  $r_0 = 21$ , then  $\Omega^{21}(Z_t^{(33)})$  is described with  $(14s \times 14s)$  matrix with unique nonzero entry:

$$b_{j,s} = w_{8(j+m)+4 \rightarrow 8(j+m+1)+4} \otimes e_{8j}.$$

(23) If  $r_0 = 22$ , then  $\Omega^{22}(Z_t^{(33)})$  is described with  $(13s \times 13s)$  matrix with unique nonzero entry:

$$b_{j,3s} = w_{8(j+m)+4 \rightarrow 8(j+m+1)+4} \otimes e_{8j+2}.$$

(24) If  $r_0 = 23$ , then  $\Omega^{23}(Z_t^{(33)})$  is described with  $(11s \times 11s)$  matrix with unique nonzero entry:

$$b_{j,9s} = w_{8(j+m)+4 \rightarrow 8(j+m+1)+4} \otimes e_{8j+7}.$$

(25) If  $r_0 = 24$ , then  $\Omega^{24}(Z_t^{(33)})$  is described with  $(11s \times 11s)$  matrix with two nonzero entries:

$$b_{j,s} = w_{8(j+m)+4 \rightarrow 8(j+m+1)+4} \otimes e_{8j+1};$$

$$b_{j,8s} = w_{8(j+m)+4 \rightarrow 8(j+m+1)+4} \otimes e_{8j+6}.$$

(26) If  $r_0 = 25$ , then  $\Omega^{25}(Z_t^{(33)})$  is described with  $(10s \times 10s)$  matrix with unique nonzero entry:

$$b_{j,0} = w_{8(j+m)+4 \rightarrow 8(j+m+1)+4} \otimes e_{8j}.$$

(27) If  $r_0 = 26$ , then  $\Omega^{26}(Z_t^{(33)})$  is described with  $(8s \times 8s)$  matrix with unique nonzero entry:

$$b_{j,5s} = w_{8(j+m)+4 \rightarrow 8(j+m+1)+4} \otimes e_{8j+5}.$$

(28) If  $r_0 = 27$ , then  $\Omega^{27}(Z_t^{(33)})$  is described with  $(9s \times 9s)$  matrix with unique nonzero entry:

$$b_{j,7s} = w_{8(j+m)+4 \rightarrow 8(j+m+1)+4} \otimes e_{8j+7}.$$

(29) If  $r_0 = 28$ , then  $\Omega^{28}(Z_t^{(33)})$  is described with  $(8s \times 8s)$  matrix with unique nonzero entry:

$$b_{j,4s} = w_{8(j+m)+4 \rightarrow 8(j+m+1)+4} \otimes e_{8j+4}.$$

(II) Represent an arbitrary  $t_0 \in \mathbb{N}$  in the form  $t_0 = 29\ell_0 + r_0$ , where  $0 \leq r_0 \leq 28$ . Then  $\Omega^{t_0}(Z_t^{(33)})$  is a  $\Omega^{r_0}(Z_t^{(33)})$ , whose left components twisted by  $\sigma^{\ell_0}$ , and coefficients multiplied by  $(-1)^{\ell_0}$ .

**Proposition 29** (Translates for the case 34). (I) *Let  $r_0 \in \mathbb{N}$ ,  $r_0 < 29$ .  $r_0$ -translates of the elements  $Z_t^{(34)}$  are described by the following way.*

(1) *If  $r_0 = 0$ , then  $\Omega^0(Z_t^{(34)})$  is described with  $(8s \times 8s)$  matrix with unique nonzero entry:*

$$b_{j,5s} = w_{8(j+m)+5 \rightarrow 8(j+m+1)+5} \otimes e_{8j+5}.$$

(2) *If  $r_0 = 1$ , then  $\Omega^1(Z_t^{(34)})$  is described with  $(9s \times 9s)$  matrix with unique nonzero entry:*

$$b_{j,s} = w_{8(j+m)+5 \rightarrow 8(j+m+1)+5} \otimes e_{8j}.$$

(3) *If  $r_0 = 2$ , then  $\Omega^2(Z_t^{(34)})$  is described with  $(8s \times 8s)$  matrix with unique nonzero entry:*

$$b_{j,4s} = w_{8(j+m)+5 \rightarrow 8(j+m+1)+5} \otimes e_{8j+4}.$$

(4) *If  $r_0 = 3$ , then  $\Omega^3(Z_t^{(34)})$  is described with  $(10s \times 10s)$  matrix with unique nonzero entry:*

$$b_{j,9s} = w_{8(j+m)+5 \rightarrow 8(j+m+1)+5} \otimes e_{8j+7}.$$

(5) *If  $r_0 = 4$ , then  $\Omega^4(Z_t^{(34)})$  is described with  $(11s \times 11s)$  matrix with two nonzero entries:*

$$b_{j,4s} = w_{8(j+m)+5 \rightarrow 8(j+m+1)+5} \otimes e_{8j+3};$$

$$b_{j,9s} = w_{8(j+m)+5 \rightarrow 8(j+m+1)+5} \otimes e_{8j+6}.$$

(6) *If  $r_0 = 5$ , then  $\Omega^5(Z_t^{(34)})$  is described with  $(11s \times 11s)$  matrix with unique nonzero entry:*

$$b_{j,0} = w_{8(j+m)+5 \rightarrow 8(j+m+1)+5} \otimes e_{8j}.$$

(7) *If  $r_0 = 6$ , then  $\Omega^6(Z_t^{(34)})$  is described with  $(13s \times 13s)$  matrix with two nonzero entries:*

$$b_{j,3s} = w_{8(j+m)+5 \rightarrow 8(j+m+1)+5} \otimes e_{8j+2};$$

$$b_{j,8s} = w_{8(j+m)+5 \rightarrow 8(j+m+1)+5} \otimes e_{8j+5}.$$

(8) *If  $r_0 = 7$ , then  $\Omega^7(Z_t^{(34)})$  is described with  $(14s \times 14s)$  matrix with two nonzero entries:*

$$b_{j,3s} = w_{8(j+m)+5 \rightarrow 8(j+m+1)+5} \otimes e_{8j};$$

$$b_{j,11s} = w_{8(j+m)+5 \rightarrow 8(j+m+1)+5} \otimes e_{8j+7}.$$

(9) *If  $r_0 = 8$ , then  $\Omega^8(Z_t^{(34)})$  is described with  $(16s \times 16s)$  matrix with the following nonzero entries:*

$$b_{j,3s} = w_{8(j+m)+5 \rightarrow 8(j+m+1)+5} \otimes e_{8j+1};$$

$$b_{j,8s} = w_{8(j+m)+5 \rightarrow 8(j+m+1)+5} \otimes e_{8j+4};$$

$$b_{j,11s} = w_{8(j+m)+5 \rightarrow 8(j+m+1)+5} \otimes e_{8j+6}.$$

(10) *If  $r_0 = 9$ , then  $\Omega^9(Z_t^{(34)})$  is described with  $(16s \times 16s)$  matrix with two nonzero entries:*

$$b_{j,0} = w_{8(j+m)+5 \rightarrow 8(j+m+1)+5} \otimes e_{8j};$$

$$b_{j,15s} = w_{8(j+m)+5 \rightarrow 8(j+m+1)+5} \otimes e_{8j+7}.$$

(11) *If  $r_0 = 10$ , then  $\Omega^{10}(Z_t^{(34)})$  is described with  $(19s \times 19s)$  matrix with the following nonzero entries:*

$$b_{j,7s} = w_{8(j+m)+5 \rightarrow 8(j+m+1)+5} \otimes e_{8j+3};$$

$$b_{j,10s} = w_{8(j+m)+5 \rightarrow 8(j+m+1)+5} \otimes e_{8j+5};$$

$$b_{j,15s} = w_{8(j+m)+5 \rightarrow 8(j+m+1)+5} \otimes e_{8j+6}.$$

(12) If  $r_0 = 11$ , then  $\Omega^{11}(Z_t^{(34)})$  is described with  $(18s \times 18s)$  matrix with two nonzero entries:

$$b_{j,4s} = w_{8(j+m)+5 \rightarrow 8(j+m+1)+5} \otimes e_{8j};$$

$$b_{j,14s} = w_{8(j+m)+5 \rightarrow 8(j+m+1)+5} \otimes e_{8j+7}.$$

(13) If  $r_0 = 12$ , then  $\Omega^{12}(Z_t^{(34)})$  is described with  $(19s \times 19s)$  matrix with the following nonzero entries:

$$b_{j,5s} = w_{8(j+m)+5 \rightarrow 8(j+m+1)+5} \otimes e_{8j+2};$$

$$b_{j,8s} = w_{8(j+m)+5 \rightarrow 8(j+m+1)+5} \otimes e_{8j+4};$$

$$b_{j,12s} = w_{8(j+m)+5 \rightarrow 8(j+m+1)+5} \otimes e_{8j+5}.$$

(14) If  $r_0 = 13$ , then  $\Omega^{13}(Z_t^{(34)})$  is described with  $(18s \times 18s)$  matrix with two nonzero entries:

$$b_{j,3s} = w_{8(j+m)+5 \rightarrow 8(j+m+1)+5} \otimes e_{8j};$$

$$b_{j,17s} = w_{8(j+m)+5 \rightarrow 8(j+m+1)+5} \otimes e_{8j+7}.$$

(15) If  $r_0 = 14$ , then  $\Omega^{14}(Z_t^{(34)})$  is described with  $(20s \times 20s)$  matrix with the following nonzero entries:

$$b_{j,4s} = w_{8(j+m)+5 \rightarrow 8(j+m+1)+5} \otimes e_{8j+1};$$

$$b_{j,7s} = w_{8(j+m)+5 \rightarrow 8(j+m+1)+5} \otimes e_{8j+3};$$

$$b_{j,16s} = w_{8(j+m)+5 \rightarrow 8(j+m+1)+5} \otimes e_{8j+6}.$$

(16) If  $r_0 = 15$ , then  $\Omega^{15}(Z_t^{(34)})$  is described with  $(18s \times 18s)$  matrix with two nonzero entries:

$$b_{j,4s} = w_{8(j+m)+5 \rightarrow 8(j+m+1)+5} \otimes e_{8j};$$

$$b_{j,17s} = w_{8(j+m)+5 \rightarrow 8(j+m+1)+5} \otimes e_{8j+7}.$$

(17) If  $r_0 = 16$ , then  $\Omega^{16}(Z_t^{(34)})$  is described with  $(19s \times 19s)$  matrix with the following nonzero entries:

$$b_{j,5s} = w_{8(j+m)+5 \rightarrow 8(j+m+1)+5} \otimes e_{8j+2};$$

$$b_{j,12s} = w_{8(j+m)+5 \rightarrow 8(j+m+1)+5} \otimes e_{8j+5};$$

$$b_{j,15s} = w_{8(j+m)+5 \rightarrow 8(j+m+1)+5} \otimes e_{8j+6}.$$

(18) If  $r_0 = 17$ , then  $\Omega^{17}(Z_t^{(34)})$  is described with  $(18s \times 18s)$  matrix with two nonzero entries:

$$b_{j,3s} = w_{8(j+m)+5 \rightarrow 8(j+m+1)+5} \otimes e_{8j};$$

$$b_{j,17s} = w_{8(j+m)+5 \rightarrow 8(j+m+1)+5} \otimes e_{8j+7}.$$

(19) If  $r_0 = 18$ , then  $\Omega^{18}(Z_t^{(34)})$  is described with  $(19s \times 19s)$  matrix with the following nonzero entries:

$$b_{j,3s} = w_{8(j+m)+5 \rightarrow 8(j+m+1)+5} \otimes e_{8j+1};$$

$$b_{j,9s} = w_{8(j+m)+5 \rightarrow 8(j+m+1)+5} \otimes e_{8j+4};$$

$$b_{j,12s} = w_{8(j+m)+5 \rightarrow 8(j+m+1)+5} \otimes e_{8j+5}.$$

(20) If  $r_0 = 19$ , then  $\Omega^{19}(Z_t^{(34)})$  is described with  $(16s \times 16s)$  matrix with two nonzero entries:

$$b_{j,3s} = w_{8(j+m)+5 \rightarrow 8(j+m+1)+5} \otimes e_{8j};$$

$$b_{j,15s} = w_{8(j+m)+5 \rightarrow 8(j+m+1)+5} \otimes e_{8j+7}.$$

(21) If  $r_0 = 20$ , then  $\Omega^{20}(Z_t^{(34)})$  is described with  $(16s \times 16s)$  matrix with two nonzero entries:

$$b_{j,6s} = w_{8(j+m)+5 \rightarrow 8(j+m+1)+5} \otimes e_{8j+3};$$

$$b_{j,12s} = w_{8(j+m)+5 \rightarrow 8(j+m+1)+5} \otimes e_{8j+6}.$$

(22) If  $r_0 = 21$ , then  $\Omega^{21}(Z_t^{(34)})$  is described with  $(14s \times 14s)$  matrix with unique nonzero entry:

$$b_{j,13s} = w_{8(j+m)+5 \rightarrow 8(j+m+1)+5} \otimes e_{8j+7}.$$

(23) If  $r_0 = 22$ , then  $\Omega^{22}(Z_t^{(34)})$  is described with  $(13s \times 13s)$  matrix with two nonzero entries:

$$b_{j,4s} = w_{8(j+m)+5 \rightarrow 8(j+m+1)+5} \otimes e_{8j+2};$$

$$b_{j,8s} = w_{8(j+m)+5 \rightarrow 8(j+m+1)+5} \otimes e_{8j+5}.$$

(24) If  $r_0 = 23$ , then  $\Omega^{23}(Z_t^{(34)})$  is described with  $(11s \times 11s)$  matrix with unique nonzero entry:

$$b_{j,s} = w_{8(j+m)+5 \rightarrow 8(j+m+1)+5} \otimes e_{8j}.$$

(25) If  $r_0 = 24$ , then  $\Omega^{24}(Z_t^{(34)})$  is described with  $(11s \times 11s)$  matrix with unique nonzero entry:

$$b_{j,2s} = w_{8(j+m)+5 \rightarrow 8(j+m+1)+5} \otimes e_{8j+1}.$$

(26) If  $r_0 = 25$ , then  $\Omega^{25}(Z_t^{(34)})$  is described with  $(10s \times 10s)$  matrix with unique nonzero entry:

$$b_{j,9s} = w_{8(j+m)+5 \rightarrow 8(j+m+1)+5} \otimes e_{8j+7}.$$

(27) If  $r_0 = 26$ , then  $\Omega^{26}(Z_t^{(34)})$  is described with  $(8s \times 8s)$  matrix with unique nonzero entry:

$$b_{j,6s} = w_{8(j+m)+5 \rightarrow 8(j+m+1)+5} \otimes e_{8j+6}.$$

(28) If  $r_0 = 27$ , then  $\Omega^{27}(Z_t^{(34)})$  is described with  $(9s \times 9s)$  matrix with unique nonzero entry:

$$b_{j,6s} = w_{8(j+m)+5 \rightarrow 8(j+m+1)+5} \otimes e_{8j+6}.$$

(29) If  $r_0 = 28$ , then  $\Omega^{28}(Z_t^{(34)})$  is described with  $(8s \times 8s)$  matrix with unique nonzero entry:

$$b_{j,5s} = w_{8(j+m)+5 \rightarrow 8(j+m+1)+5} \otimes e_{8j+5}.$$

(II) Represent an arbitrary  $t_0 \in \mathbb{N}$  in the form  $t_0 = 29\ell_0 + r_0$ , where  $0 \leq r_0 \leq 28$ . Then  $\Omega^{t_0}(Z_t^{(34)})$  is a  $\Omega^{r_0}(Z_t^{(34)})$ , whose left components twisted by  $\sigma^{\ell_0}$ , and coefficients multiplied by  $(-1)^{\ell_0}$ .

**Proposition 30** (Translates for the case 35). (I) Let  $r_0 \in \mathbb{N}$ ,  $r_0 < 29$ .  $r_0$ -translates of the elements  $Z_t^{(35)}$  are described by the following way.

(1) If  $r_0 = 0$ , then  $\Omega^0(Z_t^{(35)})$  is described with  $(8s \times 8s)$  matrix with unique nonzero entry:

$$b_{j,6s} = w_{8(j+m)+6 \rightarrow 8(j+m+1)+6} \otimes e_{8j+6}.$$

(2) If  $r_0 = 1$ , then  $\Omega^1(Z_t^{(35)})$  is described with  $(9s \times 9s)$  matrix with unique nonzero entry:

$$b_{j,6s} = w_{8(j+m)+6 \rightarrow 8(j+m+1)+6} \otimes e_{8j+5}.$$

(3) If  $r_0 = 2$ , then  $\Omega^2(Z_t^{(35)})$  is described with  $(8s \times 8s)$  matrix with unique nonzero entry:

$$b_{j,5s} = w_{8(j+m)+6 \rightarrow 8(j+m+1)+6} \otimes e_{8j+5}.$$

(4) If  $r_0 = 3$ , then  $\Omega^3(Z_t^{(35)})$  is described with  $(10s \times 10s)$  matrix with unique nonzero entry:

$$b_{j,s} = w_{8(j+m)+6 \rightarrow 8(j+m+1)+6} \otimes e_{8j}.$$

(5) If  $r_0 = 4$ , then  $\Omega^4(Z_t^{(35)})$  is described with  $(11s \times 11s)$  matrix with unique nonzero entry:

$$b_{j,5s} = w_{8(j+m)+6 \rightarrow 8(j+m+1)+6} \otimes e_{8j+4}.$$

(6) If  $r_0 = 5$ , then  $\Omega^5(Z_t^{(35)})$  is described with  $(11s \times 11s)$  matrix with unique nonzero entry:

$$b_{j,10s} = w_{8(j+m)+6 \rightarrow 8(j+m+1)+6} \otimes e_{8j+7}.$$

(7) If  $r_0 = 6$ , then  $\Omega^6(Z_t^{(35)})$  is described with  $(13s \times 13s)$  matrix with two nonzero entries:

$$b_{j,4s} = w_{8(j+m)+6 \rightarrow 8(j+m+1)+6} \otimes e_{8j+3};$$

$$b_{j,10s} = w_{8(j+m)+6 \rightarrow 8(j+m+1)+6} \otimes e_{8j+6}.$$

(8) If  $r_0 = 7$ , then  $\Omega^7(Z_t^{(35)})$  is described with  $(14s \times 14s)$  matrix with unique nonzero entry:

$$b_{j,2s} = w_{8(j+m)+6 \rightarrow 8(j+m+1)+6} \otimes e_{8j}.$$

(9) If  $r_0 = 8$ , then  $\Omega^8(Z_t^{(35)})$  is described with  $(16s \times 16s)$  matrix with two nonzero entries:

$$b_{j,4s} = w_{8(j+m)+6 \rightarrow 8(j+m+1)+6} \otimes e_{8j+2};$$

$$b_{j,10s} = w_{8(j+m)+6 \rightarrow 8(j+m+1)+6} \otimes e_{8j+5}.$$

(10) If  $r_0 = 9$ , then  $\Omega^9(Z_t^{(35)})$  is described with  $(16s \times 16s)$  matrix with two nonzero entries:

$$b_{j,2s} = w_{8(j+m)+6 \rightarrow 8(j+m+1)+6} \otimes e_{8j};$$

$$b_{j,14s} = w_{8(j+m)+6 \rightarrow 8(j+m+1)+6} \otimes e_{8j+7}.$$

(11) If  $r_0 = 10$ , then  $\Omega^{10}(Z_t^{(35)})$  is described with  $(19s \times 19s)$  matrix with the following nonzero entries:

$$b_{j,3s} = w_{8(j+m)+6 \rightarrow 8(j+m+1)+6} \otimes e_{8j+1};$$

$$b_{j,9s} = w_{8(j+m)+6 \rightarrow 8(j+m+1)+6} \otimes e_{8j+4};$$

$$b_{j,14s} = w_{8(j+m)+6 \rightarrow 8(j+m+1)+6} \otimes e_{8j+6}.$$

(12) If  $r_0 = 11$ , then  $\Omega^{11}(Z_t^{(35)})$  is described with  $(18s \times 18s)$  matrix with two nonzero entries:

$$b_{j,s} = w_{8(j+m)+6 \rightarrow 8(j+m+1)+6} \otimes e_{8j};$$

$$b_{j,16s} = w_{8(j+m)+6 \rightarrow 8(j+m+1)+6} \otimes e_{8j+7}.$$

(13) If  $r_0 = 12$ , then  $\Omega^{12}(Z_t^{(35)})$  is described with  $(19s \times 19s)$  matrix with the following nonzero entries:

$$b_{j,7s} = w_{8(j+m)+6 \rightarrow 8(j+m+1)+6} \otimes e_{8j+3};$$

$$b_{j,11s} = w_{8(j+m)+6 \rightarrow 8(j+m+1)+6} \otimes e_{8j+5};$$

$$b_{j,13s} = w_{8(j+m)+6 \rightarrow 8(j+m+1)+6} \otimes e_{8j+6}.$$

(14) If  $r_0 = 13$ , then  $\Omega^{13}(Z_t^{(35)})$  is described with  $(18s \times 18s)$  matrix with two nonzero entries:

$$b_{j,2s} = w_{8(j+m)+6 \rightarrow 8(j+m+1)+6} \otimes e_{8j};$$

$$b_{j,14s} = w_{8(j+m)+6 \rightarrow 8(j+m+1)+6} \otimes e_{8j+7}.$$

(15) If  $r_0 = 14$ , then  $\Omega^{14}(Z_t^{(35)})$  is described with  $(20s \times 20s)$  matrix with the following nonzero entries:

$$b_{j,6s} = w_{8(j+m)+6 \rightarrow 8(j+m+1)+6} \otimes e_{8j+2};$$

$$b_{j,10s} = w_{8(j+m)+6 \rightarrow 8(j+m+1)+6} \otimes e_{8j+4};$$

$$b_{j,11s} = w_{8(j+m)+6 \rightarrow 8(j+m+1)+6} \otimes e_{8j+5}.$$

(16) If  $r_0 = 15$ , then  $\Omega^{15}(Z_t^{(35)})$  is described with  $(18s \times 18s)$  matrix with two nonzero entries:

$$b_{j,s} = w_{8(j+m)+6 \rightarrow 8(j+m+1)+6} \otimes e_{8j};$$

$$b_{j,16s} = w_{8(j+m)+6 \rightarrow 8(j+m+1)+6} \otimes e_{8j+7}.$$

(17) If  $r_0 = 16$ , then  $\Omega^{16}(Z_t^{(35)})$  is described with  $(19s \times 19s)$  matrix with the following nonzero entries:

$$b_{j,4s} = w_{8(j+m)+6 \rightarrow 8(j+m+1)+6} \otimes e_{8j+1};$$

$$b_{j,8s} = w_{8(j+m)+6 \rightarrow 8(j+m+1)+6} \otimes e_{8j+3};$$

$$b_{j,14s} = w_{8(j+m)+6 \rightarrow 8(j+m+1)+6} \otimes e_{8j+6}.$$

(18) If  $r_0 = 17$ , then  $\Omega^{17}(Z_t^{(35)})$  is described with  $(18s \times 18s)$  matrix with two nonzero entries:

$$b_{j,2s} = w_{8(j+m)+6 \rightarrow 8(j+m+1)+6} \otimes e_{8j};$$

$$b_{j,14s} = w_{8(j+m)+6 \rightarrow 8(j+m+1)+6} \otimes e_{8j+7}.$$

(19) If  $r_0 = 18$ , then  $\Omega^{18}(Z_t^{(35)})$  is described with  $(19s \times 19s)$  matrix with the following nonzero entries:

$$b_{j,6s} = w_{8(j+m)+6 \rightarrow 8(j+m+1)+6} \otimes e_{8j+2};$$

$$b_{j,11s} = w_{8(j+m)+6 \rightarrow 8(j+m+1)+6} \otimes e_{8j+5};$$

$$b_{j,13s} = w_{8(j+m)+6 \rightarrow 8(j+m+1)+6} \otimes e_{8j+6}.$$

(20) If  $r_0 = 19$ , then  $\Omega^{19}(Z_t^{(35)})$  is described with  $(16s \times 16s)$  matrix with two nonzero entries:

$$b_{j,s} = w_{8(j+m)+6 \rightarrow 8(j+m+1)+6} \otimes e_{8j};$$

$$b_{j,14s} = w_{8(j+m)+6 \rightarrow 8(j+m+1)+6} \otimes e_{8j+7}.$$

(21) If  $r_0 = 20$ , then  $\Omega^{20}(Z_t^{(35)})$  is described with  $(16s \times 16s)$  matrix with the following nonzero entries:

$$b_{j,3s} = w_{8(j+m)+6 \rightarrow 8(j+m+1)+6} \otimes e_{8j+1};$$

$$b_{j,7s} = w_{8(j+m)+6 \rightarrow 8(j+m+1)+6} \otimes e_{8j+4};$$

$$b_{j,8s} = w_{8(j+m)+6 \rightarrow 8(j+m+1)+6} \otimes e_{8j+5}.$$

(22) If  $r_0 = 21$ , then  $\Omega^{21}(Z_t^{(35)})$  is described with  $(14s \times 14s)$  matrix with two nonzero entries:

$$b_{j,2s} = w_{8(j+m)+6 \rightarrow 8(j+m+1)+6} \otimes e_{8j};$$

$$b_{j,11s} = w_{8(j+m)+6 \rightarrow 8(j+m+1)+6} \otimes e_{8j+7}.$$

(23) If  $r_0 = 22$ , then  $\Omega^{22}(Z_t^{(35)})$  is described with  $(13s \times 13s)$  matrix with two nonzero entries:

$$b_{j,5s} = w_{8(j+m)+6 \rightarrow 8(j+m+1)+6} \otimes e_{8j+3};$$

$$b_{j,10s} = w_{8(j+m)+6 \rightarrow 8(j+m+1)+6} \otimes e_{8j+6}.$$

(24) If  $r_0 = 23$ , then  $\Omega^{23}(Z_t^{(35)})$  is described with  $(11s \times 11s)$  matrix with unique nonzero entry:

$$b_{j,10s} = w_{8(j+m)+6 \rightarrow 8(j+m+1)+6} \otimes e_{8j+7}.$$

(25) If  $r_0 = 24$ , then  $\Omega^{24}(Z_t^{(35)})$  is described with  $(11s \times 11s)$  matrix with two nonzero entries:

$$b_{j,3s} = w_{8(j+m)+6 \rightarrow 8(j+m+1)+6} \otimes e_{8j+2};$$

$$b_{j,7s} = w_{8(j+m)+6 \rightarrow 8(j+m+1)+6} \otimes e_{8j+5}.$$

(26) If  $r_0 = 25$ , then  $\Omega^{25}(Z_t^{(35)})$  is described with  $(10s \times 10s)$  matrix with unique nonzero entry:

$$b_{j,s} = w_{8(j+m)+6 \rightarrow 8(j+m+1)+6} \otimes e_{8j}.$$

(27) If  $r_0 = 26$ , then  $\Omega^{26}(Z_t^{(35)})$  is described with  $(8s \times 8s)$  matrix with unique nonzero entry:

$$b_{j,s} = w_{8(j+m)+6 \rightarrow 8(j+m+1)+6} \otimes e_{8j+1}.$$

(28) If  $r_0 = 27$ , then  $\Omega^{27}(Z_t^{(35)})$  is described with  $(9s \times 9s)$  matrix with unique nonzero entry:

$$b_{j,8s} = w_{8(j+m)+6 \rightarrow 8(j+m+1)+6} \otimes e_{8j+7}.$$

(29) If  $r_0 = 28$ , then  $\Omega^{28}(Z_t^{(35)})$  is described with  $(8s \times 8s)$  matrix with unique nonzero entry:

$$b_{j,6s} = w_{8(j+m)+6 \rightarrow 8(j+m+1)+6} \otimes e_{8j+6}.$$

(II) Represent an arbitrary  $t_0 \in \mathbb{N}$  in the form  $t_0 = 29\ell_0 + r_0$ , where  $0 \leq r_0 \leq 28$ . Then  $\Omega^{t_0}(Z_t^{(35)})$  is a  $\Omega^{r_0}(Z_t^{(35)})$ , whose left components twisted by  $\sigma^{\ell_0}$ , and coefficients multiplied by  $(-1)^{\ell_0}$ .

**Proposition 31** (Translates for the case 36). (I) Let  $r_0 \in \mathbb{N}$ ,  $r_0 < 29$ .  $r_0$ -translates of the elements  $Z_t^{(36)}$  are described by the following way.

(1) If  $r_0 = 0$ , then  $\Omega^0(Z_t^{(36)})$  is described with  $(8s \times 8s)$  matrix with unique nonzero entry:

$$b_{j,7s} = w_{8(j+m)+7 \rightarrow 8(j+m+1)+7} \otimes e_{8j+7}.$$

(2) If  $r_0 = 1$ , then  $\Omega^1(Z_t^{(36)})$  is described with  $(9s \times 9s)$  matrix with two nonzero entries:

$$b_{j,5s} = w_{8(j+m)+7 \rightarrow 8(j+m+1)+7} \otimes e_{8j+4};$$

$$b_{j,7s} = w_{8(j+m)+7 \rightarrow 8(j+m+1)+7} \otimes e_{8j+6}.$$

(3) If  $r_0 = 2$ , then  $\Omega^2(Z_t^{(36)})$  is described with  $(8s \times 8s)$  matrix with unique nonzero entry:

$$b_{j,0} = w_{8(j+m)+7 \rightarrow 8(j+m+1)+7} \otimes e_{8j}.$$

(4) If  $r_0 = 3$ , then  $\Omega^3(Z_t^{(36)})$  is described with  $(10s \times 10s)$  matrix with two nonzero entries:

$$b_{j,4s} = w_{8(j+m)+7 \rightarrow 8(j+m+1)+7} \otimes e_{8j+3};$$

$$b_{j,6s} = w_{8(j+m)+7 \rightarrow 8(j+m+1)+7} \otimes e_{8j+5}.$$

(5) If  $r_0 = 4$ , then  $\Omega^4(Z_t^{(36)})$  is described with  $(11s \times 11s)$  matrix with two nonzero entries:

$$b_{j,0} = w_{8(j+m)+7 \rightarrow 8(j+m+1)+7} \otimes e_{8j};$$

$$b_{j,10s} = w_{8(j+m)+7 \rightarrow 8(j+m+1)+7} \otimes e_{8j+7}.$$

(6) If  $r_0 = 5$ , then  $\Omega^5(Z_t^{(36)})$  is described with  $(11s \times 11s)$  matrix with the following nonzero entries:

$$b_{j,4s} = w_{8(j+m)+7 \rightarrow 8(j+m+1)+7} \otimes e_{8j+2};$$

$$b_{j,6s} = w_{8(j+m)+7 \rightarrow 8(j+m+1)+7} \otimes e_{8j+4};$$

$$b_{j,8s} = w_{8(j+m)+7 \rightarrow 8(j+m+1)+7} \otimes e_{8j+6}.$$

(7) If  $r_0 = 6$ , then  $\Omega^6(Z_t^{(36)})$  is described with  $(13s \times 13s)$  matrix with two nonzero entries:

$$b_{j,0} = w_{8(j+m)+7 \rightarrow 8(j+m+1)+7} \otimes e_{8j};$$

$$b_{j,11s} = w_{8(j+m)+7 \rightarrow 8(j+m+1)+7} \otimes e_{8j+7}.$$

(8) If  $r_0 = 7$ , then  $\Omega^7(Z_t^{(36)})$  is described with  $(14s \times 14s)$  matrix with the following nonzero entries:

$$b_{j,4s} = w_{8(j+m)+7 \rightarrow 8(j+m+1)+7} \otimes e_{8j+1};$$



$$\begin{aligned}
b_{j,6s} &= w_{8(j+m)+7 \rightarrow 8(j+m+1)+7} \otimes e_{8j+3}; \\
b_{j,8s} &= w_{8(j+m)+7 \rightarrow 8(j+m+1)+7} \otimes e_{8j+5}; \\
b_{j,9s} &= w_{8(j+m)+7 \rightarrow 8(j+m+1)+7} \otimes e_{8j+6}.
\end{aligned}$$

(9) If  $r_0 = 8$ , then  $\Omega^8(Z_t^{(36)})$  is described with  $(16s \times 16s)$  matrix with the following nonzero entries:

$$\begin{aligned}
b_{j,0} &= w_{8(j+m)+7 \rightarrow 8(j+m+1)+7} \otimes e_{8j}; \\
b_{j,s} &= w_{8(j+m)+7 \rightarrow 8(j+m+1)+7} \otimes e_{8j}; \\
b_{j,14s} &= w_{8(j+m)+7 \rightarrow 8(j+m+1)+7} \otimes e_{8j+7}.
\end{aligned}$$

(10) If  $r_0 = 9$ , then  $\Omega^9(Z_t^{(36)})$  is described with  $(16s \times 16s)$  matrix with the following nonzero entries:

$$\begin{aligned}
b_{j,5s} &= w_{8(j+m)+7 \rightarrow 8(j+m+1)+7} \otimes e_{8j+2}; \\
b_{j,7s} &= w_{8(j+m)+7 \rightarrow 8(j+m+1)+7} \otimes e_{8j+4}; \\
b_{j,8s} &= w_{8(j+m)+7 \rightarrow 8(j+m+1)+7} \otimes e_{8j+5}; \\
b_{j,10s} &= w_{8(j+m)+7 \rightarrow 8(j+m+1)+7} \otimes e_{8j+6}.
\end{aligned}$$

(11) If  $r_0 = 10$ , then  $\Omega^{10}(Z_t^{(36)})$  is described with  $(19s \times 19s)$  matrix with the following nonzero entries:

$$\begin{aligned}
b_{j,0} &= w_{8(j+m)+7 \rightarrow 8(j+m+1)+7} \otimes e_{8j}; \\
b_{j,16s} &= w_{8(j+m)+7 \rightarrow 8(j+m+1)+7} \otimes e_{8j+7}; \\
b_{j,17s} &= w_{8(j+m)+7 \rightarrow 8(j+m+1)+7} \otimes e_{8j+7}.
\end{aligned}$$

(12) If  $r_0 = 11$ , then  $\Omega^{11}(Z_t^{(36)})$  is described with  $(18s \times 18s)$  matrix with the following nonzero entries:

$$\begin{aligned}
b_{j,5s} &= w_{8(j+m)+7 \rightarrow 8(j+m+1)+7} \otimes e_{8j+1}; \\
b_{j,7s} &= w_{8(j+m)+7 \rightarrow 8(j+m+1)+7} \otimes e_{8j+3}; \\
b_{j,8s} &= w_{8(j+m)+7 \rightarrow 8(j+m+1)+7} \otimes e_{8j+4}; \\
b_{j,10s} &= w_{8(j+m)+7 \rightarrow 8(j+m+1)+7} \otimes e_{8j+5}; \\
b_{j,12s} &= w_{8(j+m)+7 \rightarrow 8(j+m+1)+7} \otimes e_{8j+6}.
\end{aligned}$$

(13) If  $r_0 = 12$ , then  $\Omega^{12}(Z_t^{(36)})$  is described with  $(19s \times 19s)$  matrix with the following nonzero entries:

$$\begin{aligned}
b_{j,0} &= w_{8(j+m)+7 \rightarrow 8(j+m+1)+7} \otimes e_{8j}; \\
b_{j,2s} &= w_{8(j+m)+7 \rightarrow 8(j+m+1)+7} \otimes e_{8j}; \\
b_{j,16s} &= w_{8(j+m)+7 \rightarrow 8(j+m+1)+7} \otimes e_{8j+7}.
\end{aligned}$$

(14) If  $r_0 = 13$ , then  $\Omega^{13}(Z_t^{(36)})$  is described with  $(18s \times 18s)$  matrix with the following nonzero entries:

$$\begin{aligned}
b_{j,5s} &= w_{8(j+m)+7 \rightarrow 8(j+m+1)+7} \otimes e_{8j+2}; \\
b_{j,6s} &= w_{8(j+m)+7 \rightarrow 8(j+m+1)+7} \otimes e_{8j+3}; \\
b_{j,9s} &= w_{8(j+m)+7 \rightarrow 8(j+m+1)+7} \otimes e_{8j+5}; \\
b_{j,11s} &= w_{8(j+m)+7 \rightarrow 8(j+m+1)+7} \otimes e_{8j+6}.
\end{aligned}$$

(15) If  $r_0 = 14$ , then  $\Omega^{14}(Z_t^{(36)})$  is described with  $(20s \times 20s)$  matrix with the following nonzero entries:

$$b_{j,0} = w_{8(j+m)+7 \rightarrow 8(j+m+1)+7} \otimes e_{8j};$$

$$b_{j,17s} = w_{8(j+m)+7 \rightarrow 8(j+m+1)+7} \otimes e_{8j+7};$$

$$b_{j,19s} = w_{8(j+m)+7 \rightarrow 8(j+m+1)+7} \otimes e_{8j+7}.$$

(16) If  $r_0 = 15$ , then  $\Omega^{15}(Z_t^{(36)})$  is described with  $(18s \times 18s)$  matrix with the following nonzero entries:

$$b_{j,5s} = w_{8(j+m)+7 \rightarrow 8(j+m+1)+7} \otimes e_{8j+1};$$

$$b_{j,6s} = w_{8(j+m)+7 \rightarrow 8(j+m+1)+7} \otimes e_{8j+2};$$

$$b_{j,9s} = w_{8(j+m)+7 \rightarrow 8(j+m+1)+7} \otimes e_{8j+4};$$

$$b_{j,10s} = w_{8(j+m)+7 \rightarrow 8(j+m+1)+7} \otimes e_{8j+5};$$

$$b_{j,13s} = w_{8(j+m)+7 \rightarrow 8(j+m+1)+7} \otimes e_{8j+6}.$$

(17) If  $r_0 = 16$ , then  $\Omega^{16}(Z_t^{(36)})$  is described with  $(19s \times 19s)$  matrix with the following nonzero entries:

$$b_{j,0} = w_{8(j+m)+7 \rightarrow 8(j+m+1)+7} \otimes e_{8j};$$

$$b_{j,2s} = w_{8(j+m)+7 \rightarrow 8(j+m+1)+7} \otimes e_{8j};$$

$$b_{j,16s} = w_{8(j+m)+7 \rightarrow 8(j+m+1)+7} \otimes e_{8j+7}.$$

(18) If  $r_0 = 17$ , then  $\Omega^{17}(Z_t^{(36)})$  is described with  $(18s \times 18s)$  matrix with the following nonzero entries:

$$b_{j,4s} = w_{8(j+m)+7 \rightarrow 8(j+m+1)+7} \otimes e_{8j+1};$$

$$b_{j,7s} = w_{8(j+m)+7 \rightarrow 8(j+m+1)+7} \otimes e_{8j+3};$$

$$b_{j,10s} = w_{8(j+m)+7 \rightarrow 8(j+m+1)+7} \otimes e_{8j+5};$$

$$b_{j,11s} = w_{8(j+m)+7 \rightarrow 8(j+m+1)+7} \otimes e_{8j+6}.$$

(19) If  $r_0 = 18$ , then  $\Omega^{18}(Z_t^{(36)})$  is described with  $(19s \times 19s)$  matrix with the following nonzero entries:

$$b_{j,0} = w_{8(j+m)+7 \rightarrow 8(j+m+1)+7} \otimes e_{8j};$$

$$b_{j,16s} = w_{8(j+m)+7 \rightarrow 8(j+m+1)+7} \otimes e_{8j+7};$$

$$b_{j,18s} = w_{8(j+m)+7 \rightarrow 8(j+m+1)+7} \otimes e_{8j+7}.$$

(20) If  $r_0 = 19$ , then  $\Omega^{19}(Z_t^{(36)})$  is described with  $(16s \times 16s)$  matrix with the following nonzero entries:

$$b_{j,5s} = w_{8(j+m)+7 \rightarrow 8(j+m+1)+7} \otimes e_{8j+2};$$

$$b_{j,7s} = w_{8(j+m)+7 \rightarrow 8(j+m+1)+7} \otimes e_{8j+4};$$

$$b_{j,8s} = w_{8(j+m)+7 \rightarrow 8(j+m+1)+7} \otimes e_{8j+5};$$

$$b_{j,10s} = w_{8(j+m)+7 \rightarrow 8(j+m+1)+7} \otimes e_{8j+6}.$$

(21) If  $r_0 = 20$ , then  $\Omega^{20}(Z_t^{(36)})$  is described with  $(16s \times 16s)$  matrix with two nonzero entries:

$$b_{j,0} = w_{8(j+m)+7 \rightarrow 8(j+m+1)+7} \otimes e_{8j};$$

$$b_{j,13s} = w_{8(j+m)+7 \rightarrow 8(j+m+1)+7} \otimes e_{8j+7}.$$

(22) If  $r_0 = 21$ , then  $\Omega^{21}(Z_t^{(36)})$  is described with  $(14s \times 14s)$  matrix with the following nonzero entries:

$$b_{j,3s} = w_{8(j+m)+7 \rightarrow 8(j+m+1)+7} \otimes e_{8j+1};$$

$$b_{j,5s} = w_{8(j+m)+7 \rightarrow 8(j+m+1)+7} \otimes e_{8j+3};$$

$$b_{j,7s} = w_{8(j+m)+7 \rightarrow 8(j+m+1)+7} \otimes e_{8j+5}.$$

(23) If  $r_0 = 22$ , then  $\Omega^{22}(Z_t^{(36)})$  is described with  $(13s \times 13s)$  matrix with two nonzero entries:

$$b_{j,s} = w_{8(j+m)+7 \rightarrow 8(j+m+1)+7} \otimes e_{8j};$$

$$b_{j,11s} = w_{8(j+m)+7 \rightarrow 8(j+m+1)+7} \otimes e_{8j+7}.$$

(24) If  $r_0 = 23$ , then  $\Omega^{23}(Z_t^{(36)})$  is described with  $(11s \times 11s)$  matrix with two nonzero entries:

$$b_{j,3s} = w_{8(j+m)+7 \rightarrow 8(j+m+1)+7} \otimes e_{8j+2};$$

$$b_{j,7s} = w_{8(j+m)+7 \rightarrow 8(j+m+1)+7} \otimes e_{8j+6}.$$

(25) If  $r_0 = 24$ , then  $\Omega^{24}(Z_t^{(36)})$  is described with  $(11s \times 11s)$  matrix with unique nonzero entry:

$$b_{j,10s} = w_{8(j+m)+7 \rightarrow 8(j+m+1)+7} \otimes e_{8j+7}.$$

(26) If  $r_0 = 25$ , then  $\Omega^{25}(Z_t^{(36)})$  is described with  $(10s \times 10s)$  matrix with two nonzero entries:

$$b_{j,2s} = w_{8(j+m)+7 \rightarrow 8(j+m+1)+7} \otimes e_{8j+1};$$

$$b_{j,6s} = w_{8(j+m)+7 \rightarrow 8(j+m+1)+7} \otimes e_{8j+5}.$$

(27) If  $r_0 = 26$ , then  $\Omega^{26}(Z_t^{(36)})$  is described with  $(8s \times 8s)$  matrix with unique nonzero entry:

$$b_{j,0} = w_{8(j+m)+7 \rightarrow 8(j+m+1)+7} \otimes e_{8j}.$$

(28) If  $r_0 = 27$ , then  $\Omega^{27}(Z_t^{(36)})$  is described with  $(9s \times 9s)$  matrix with unique nonzero entry:

$$b_{j,0} = w_{8(j+m)+7 \rightarrow 8(j+m+1)+7} \otimes e_{8j}.$$

(29) If  $r_0 = 28$ , then  $\Omega^{28}(Z_t^{(36)})$  is described with  $(8s \times 8s)$  matrix with unique nonzero entry:

$$b_{j,7s} = w_{8(j+m)+7 \rightarrow 8(j+m+1)+7} \otimes e_{8j+7}.$$

(II) Represent an arbitrary  $t_0 \in \mathbb{N}$  in the form  $t_0 = 29\ell_0 + r_0$ , where  $0 \leq r_0 \leq 28$ . Then  $\Omega^{t_0}(Z_t^{(36)})$  is a  $\Omega^{r_0}(Z_t^{(36)})$ , whose left components twisted by  $\sigma^{\ell_0}$ , and coefficients multiplied by  $(-1)^{\ell_0}$ .
